# Supplementary material for: Natural Swarms in $\bf 3.99$ Dimensions
Source: arXiv:2107.04432 source file (2022-12-19)

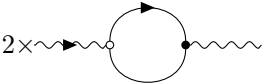

$1 \times$

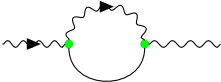

Supplement: Supplementary file 1 [file Pi.pdf]
