# Supplementary material for: Natural Swarms in $\bf 3.99$ Dimensions
Source: arXiv:2107.04432 source file (2022-12-19)

3x

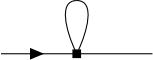

$1 \times$

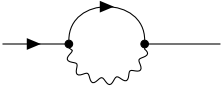

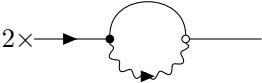

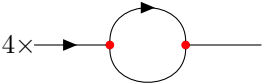

Supplement: Supplementary file 2 [file Sigma.pdf]
