# Supplementary material for: Natural Swarms in $\bf 3.99$ Dimensions
Source: arXiv:2107.04432 source file (2022-12-19)

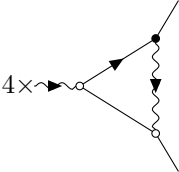

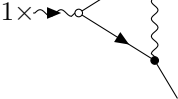

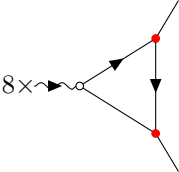

4x

~

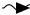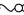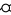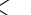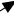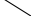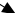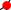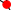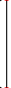

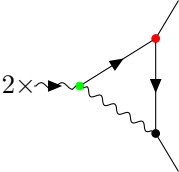

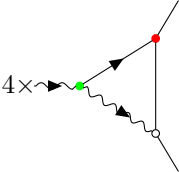

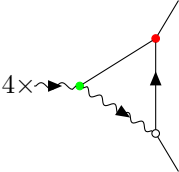

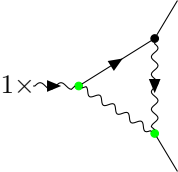



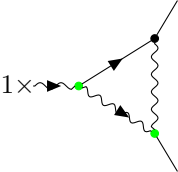

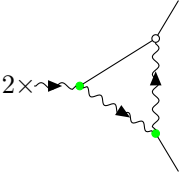

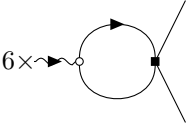

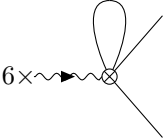

Supplement: Supplementary file 4 [file Vsvv.pdf]
