# Supplementary material for: Natural Swarms in $\bf 3.99$ Dimensions
Source: arXiv:2107.04432 source file (2022-12-19)

36

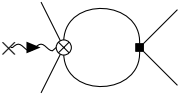

$12 \times$

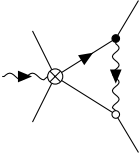

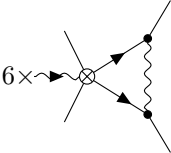

Supplement: Supplementary file 5 [file Vsvvvv.pdf]
