# Supplementary material for: Natural Swarms in $\bf 3.99$ Dimensions
Source: arXiv:2107.04432 source file (2022-12-19)

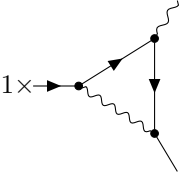

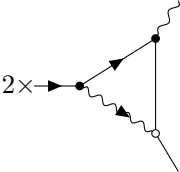

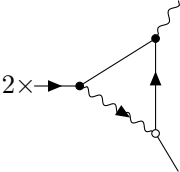

Supplement: Supplementary file 6 [file Vvvs.pdf]
