# Supplementary material for: Natural Swarms in $\bf 3.99$ Dimensions
Source: arXiv:2107.04432 source file (2022-12-19)

8x

$\times$

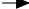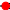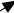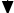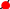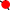

4x

$\times$

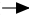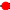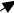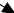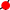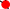

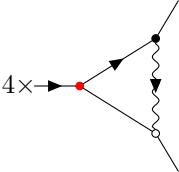

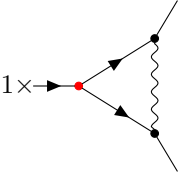

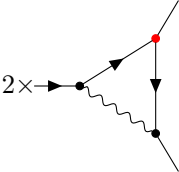

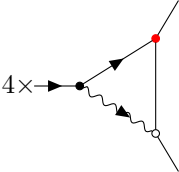

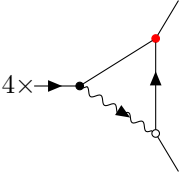

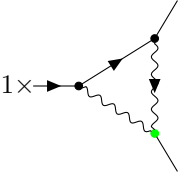



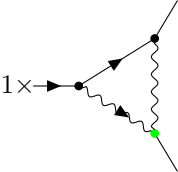

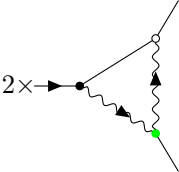

$12 \times$

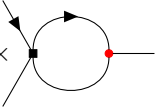

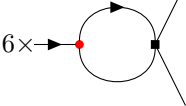

Supplement: Supplementary file 7 [file Vvvv.pdf]
