# Supplementary material for: Natural Swarms in $\bf 3.99$ Dimensions
Source: arXiv:2107.04432 source file (2022-12-19)

$18\times$

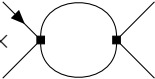

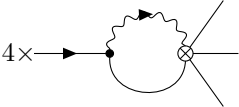

$3\times$

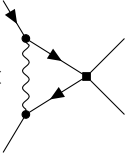

$6\times$

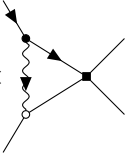

$6\times$

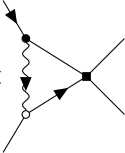

12x

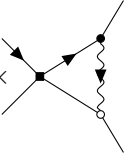

$3\times$

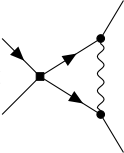

$2\times$

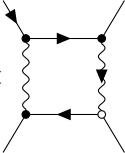



4x

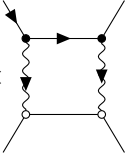

$2\times$

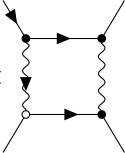

4x

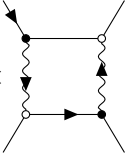

$8 \times$

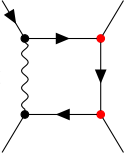

$16\times$

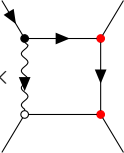

$16\times$

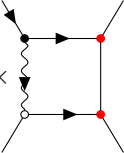

$16\times$

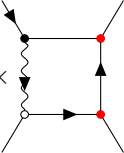

1x

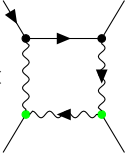



1x

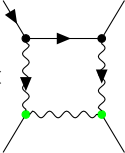

1x

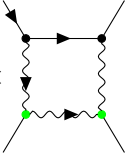

$2\times$

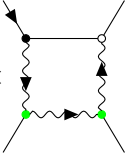

$2\times$

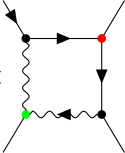

$2\times$

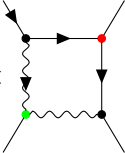

4x

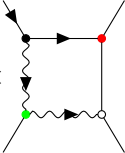

$4\times$

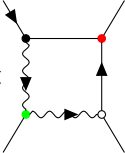

Supplement: Supplementary file 8 [file Vvvvv.pdf]
