# Supplementary material for: Natural Swarms in $\bf 3.99$ Dimensions
Source: arXiv:2107.04432 source file (2022-12-19)

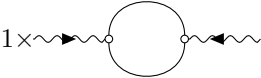

$$\frac{1}{2} \times$$

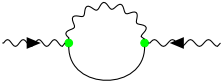

Supplement: Supplementary file 9 [file tPi.pdf]
