# Supplementary material for: Natural Swarms in $\bf 3.99$ Dimensions
Source: arXiv:2107.04432 source file (2022-12-19)

$$\frac{1}{2} \times$$

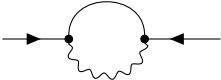

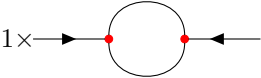

Supplement: Supplementary file 10 [file tSigma.pdf]
