# Supplementary material for: Natural Swarms in $\bf 3.99$ Dimensions
Source: arXiv:2107.04432 ancillary file (2022-12-19)
Supplement: Supplementary file 11 [file beta_functions.pdf]

# Perturbative corrections and beta functions of “Natural swarms in 3.99 dimensions”

Effective parameters and couplings are given by

Parameter (symbol in this notebook)

$w$  (  $w$  )

$x$  (  $x$  )

$\theta^\perp$  (  $\theta p$  )

$\theta''$  (  $\theta l$  )

$\Phi_1$  (  $\Phi 1$  )

$\Phi_2$  (  $\Phi 2$  )

$\mu_1$  (  $\mu 1$  )

$\mu_2$  (  $\mu 2$  )

$c_v$  (  $c v$  )

$c_s$  (  $c \sigma$  )

$f$  (  $f$  )

$\tilde{u}$  (  $u$  )

$\tilde{r}$  (  $r$  )

$\tilde{u}_K$  (  $u_K$  )

$\hat{\eta}$  (  $\eta$  )

$\check{\eta}$  (  $\eta t$  )

## Beta functions for the effective parameters and coupling constants

The following notation has been used in the following definitions

–  $\beta_P$  is the beta function of the parameter / coupling  $P$

$$\begin{aligned} \beta_w = - & \left( w \left( -8 \times (-1 + w (-1 + \eta)) \right) (x (-1 + \eta) - \eta)^3 (-w - x + (-1 + w + x) \eta) \right. \\ & (-1 + \eta t) \theta p \left( -3 c v^2 (1 + w - w \eta)^2 (w + x + \eta - (w + x) \eta)^2 + \right. \\ & c \sigma^2 (-1 + \eta) \left( x^2 (-1 + \eta)^2 (-4 + \mu_1 (2 + \eta + (-3 + \eta) \mu_1)) - x (-1 + \eta) \times \right. \\ & \left. \left. (-5 + 2 \eta^2 \mu_1 (1 + \mu_1) + \eta (-8 + 4 \mu_1 - 6 \mu_1^2) + \mu_1 (-4 + \mu_1 - 8 \mu_2) - 2 \mu_2) + \right. \right. \\ & \left. \left. \eta (-5 + \eta^2 \mu_1 (1 + \mu_1) + \eta (-4 + (2 - 3 \mu_1) \mu_1) + \mu_1 (-4 + \mu_1 - 13 \mu_2) - \mu_2) + \right. \right. \\ & \left. \left. 9 w^3 (-1 + \eta)^3 (1 + 2 \mu_1 \mu_2) + w^2 (-1 + \eta)^2 (-14 - \mu_1 (6 + \mu_1 + 36 \mu_2) - \eta (13 - \right. \right. \end{aligned}$$

$$\begin{aligned}
& 5 \mu_1 + \mu_2 + 13 \mu_1 \mu_2) + x (-1 + \eta) \times (13 + 2 \mu_2 + \mu_1 (-4 + \mu_1 + 8 \mu_2)) + \\
& w (-1 + \eta) \times (5 + x^2 (-1 + \eta)^2 (-2 + \mu_1)^2 - \eta^2 (-4 + \mu_1 (6 + \mu_1)) + \\
& \mu_1 (4 - \mu_1 + 18 \mu_2) + 2 x (-1 + \eta) \times (-9 + \eta (-4 + 5 \mu_1) - 2 \mu_2 - \\
& 2 \mu_1 (1 + \mu_1 + 4 \mu_2)) + 2 \eta (9 + \mu_2 + \mu_1 (2 + 2 \mu_1 + 13 \mu_2))) + \\
& f (2 w^5 (-1 + \eta)^5 (-3 x^2 (-1 + \eta)^2 (20 \eta^5 \theta p + 15 \eta t \theta p + 2 \eta^3 (16 + 9 \eta t) \\
& \theta p - 2 \eta^4 (9 + 10 \eta t) \theta p + \\
& \eta (56 \theta p - 52 \eta t \theta p - (-1 + \eta t) \theta l (37 + 12 \theta p (-4 + \mathfrak{z}2))) + \\
& \eta^2 (-90 \theta p + 39 \eta t \theta p - (-1 + \eta t) \theta l (-37 + 24 \theta p (-4 + \mathfrak{z}2))) + \\
& x (-1 + \eta) \eta (60 \eta^5 \theta p + 91 \eta t \theta p + 6 \eta^3 (16 + 9 \eta t) \theta p - 6 \eta^4 (9 + 10 \eta t) \theta p + \\
& \eta (8 \times (21 - 31 \eta t) \theta p - (-1 + \eta t) \theta l (65 + 36 \theta p (-4 + \mathfrak{z}2))) + \\
& \eta^2 ((-270 + 163 \eta t) \theta p - (-1 + \eta t) \theta l (-65 + 48 \theta p (-4 + \mathfrak{z}2)))) - \\
& 2 \eta^2 \theta p (26 \eta t + \eta (28 + 10 \eta^4 + \eta^2 (16 + 9 \eta t) - \eta^3 (9 + 10 \eta t) - \\
& 3 \eta t (21 + 2 \theta l (-4 + \mathfrak{z}2)) + \eta (-45 + \eta t (38 - 6 \theta l (-4 + \mathfrak{z}2)) + \\
& 6 \theta l (-4 + \mathfrak{z}2)) + 6 \theta l (-4 + \mathfrak{z}2))) + \\
& 2 x^3 (-1 + \eta)^3 ((-1 + \eta)^2 (28 + \eta (11 + 10 \eta - 10 \eta t) - 11 \eta t) \theta p - \\
& 2 \times (-1 + \eta t) \theta l (13 + \eta (-13 + 12 \theta p (-4 + \mathfrak{z}2)) + 3 \theta p (-4 + \mathfrak{z}2))) + \\
& 12 x^4 (-1 + \eta)^4 (-1 + \eta t) \theta l \theta p (-4 + \mathfrak{z}2)) - \\
& 8 w^6 (-1 + \eta)^6 (x + \eta - x \eta)^3 (-1 + \eta t) \theta l \theta p (-4 + \mathfrak{z}2) + \\
& (x + \eta - x \eta)^2 (4 x^4 (-1 + \eta)^4 \theta p (-12 + 30 \eta^4 + 9 \eta t - \\
& 2 \eta^3 (39 - 5 \theta l + 5 \eta t (2 + \theta l)) + 10 \theta l (4 + \mathfrak{z}2) - 10 \eta t \theta l (4 + \mathfrak{z}2) + \\
& \eta (6 - 38 \eta t - 39 \theta l + 39 \eta t \theta l + 10 \times (-1 + \eta t) \theta l \mathfrak{z}2) + \\
& \eta^2 (54 - 19 \theta l + 2 \theta l \mathfrak{z}2 + \eta t (49 + 19 \theta l - 2 \theta l \mathfrak{z}2))) - \\
& 4 x (-1 + \eta) \eta (120 \eta^6 \theta p + 14 \eta t \theta p - 8 \eta^5 (39 - 5 \theta l + 5 \eta t (2 + \theta l)) \theta p + \\
& \eta^2 (-48 \theta p + 50 \eta t \theta p + (-1 + \eta t) \theta l (14 + \theta p (-134 + 33 \mathfrak{z}1 - 27 \mathfrak{z}2))) + \\
& 4 \eta^3 \theta p (6 - 38 \eta t - 39 \theta l + 39 \eta t \theta l + 10 \times (-1 + \eta t) \theta l \mathfrak{z}2) + \\
& 4 \eta^4 \theta p (54 + \eta t (49 + \theta l (19 - 2 \mathfrak{z}2)) + \theta l (-19 + 2 \mathfrak{z}2)) + \eta (-28 \eta t \theta p - \\
& (-1 + \eta t) \theta l (14 + 33 \theta p \mathfrak{z}1 + 13 \theta p (2 + \mathfrak{z}2))) + x^2 (-1 + \eta)^2 \\
& (720 \eta^6 \theta p + 50 \eta t \theta p - 48 \eta^5 (39 - 5 \theta l + 5 \eta t (2 + \theta l)) \theta p + \eta^2 (-288 \\
& \theta p + 266 \eta t \theta p + (-1 + \eta t) \theta l (60 + \theta p (-854 + 141 \mathfrak{z}1 - 187 \mathfrak{z}2))) - \\
& 24 \eta^4 \theta p (-54 - 49 \eta t + 19 \theta l - 19 \eta t \theta l + 2 \times (-1 + \eta t) \theta l \mathfrak{z}2) + \\
& 24 \eta^3 \theta p (6 - 38 \eta t - 39 \theta l + 39 \eta t \theta l + 10 \times (-1 + \eta t) \theta l \mathfrak{z}2) + \\
& \eta (-100 \eta t \theta p - (-1 + \eta t) \theta l (60 + 141 \theta p \mathfrak{z}1 + 53 \theta p (2 + \mathfrak{z}2)))) + \\
& \eta^2 \theta p (42 \eta t + \eta (120 \eta^5 - 8 \eta^4 (39 - 5 \theta l + 5 \eta t (2 + \theta l)) + \eta (-48 + 26 \eta t (3 - \\
& 5 \theta l) + 130 \theta l + 39 \times (-1 + \eta t) \theta l \mathfrak{z}1 - 25 \times (-1 + \eta t) \theta l \mathfrak{z}2) + \\
& 4 \eta^2 (6 - 38 \eta t - 39 \theta l + 39 \eta t \theta l + 10 \times (-1 + \eta t) \theta l \mathfrak{z}2) + \\
& 3 \theta l (13 \mathfrak{z}1 + 5 \times (2 + \mathfrak{z}2)) - 3 \eta t (28 + 13 \theta l \mathfrak{z}1 + 5 \theta l (2 + \mathfrak{z}2)) + \\
& 4 \eta^3 (54 + \eta t (49 + \theta l (19 - 2 \mathfrak{z}2)) + \theta l (-19 + 2 \mathfrak{z}2))) - \\
& 8 x^3 (-1 + \eta)^3 (2 (-1 + \eta)^2 \eta (-12 + 2 \eta (-9 + 15 \eta - 10 \eta t) + 9 \eta t) \theta p - \\
& (-1 + \eta t) \theta l (5 + 20 \eta^4 \theta p + 2 \theta p (2 + 3 \mathfrak{z}1 + \mathfrak{z}2) + 2 \eta^3 \theta p (-19 + 2 \mathfrak{z}2) - \\
& 2 \eta^2 \theta p (39 + 10 \mathfrak{z}2) + \eta (-5 + 2 \theta p (38 - 3 \mathfrak{z}1 + 9 \mathfrak{z}2)))) + \\
& 3 w^4 (-1 + \eta)^4 (8 x^5 (-1 + \eta)^5 (-1 + \eta t) \theta l \theta p (-4 + \mathfrak{z}2) + 4 x^4 (-1 + \eta)^4 \\
& ((-1 + \eta)^2 (28 + \eta (11 + 10 \eta - 10 \eta t) - 11 \eta t) \theta p + 2 \times (-1 + \eta t) \theta l \\
& (-4 + \eta (4 + \theta p (26 + 3 \mathfrak{z}1 - 2 \mathfrak{z}2)) - 3 \theta p (-2 + \mathfrak{z}1 + 2 \mathfrak{z}2))) + \\
& x^2 (-1 + \eta)^2 (240 \eta^6 \theta p + 90 \eta t \theta p - 48 \eta^5 (2 + 5 \eta t) \theta p +
\end{aligned}$$

$$\begin{aligned}
& 12 \eta^4 (23 + 8 \eta t) \theta p - 2 \eta (48 + 47 \eta t) \theta p - 6 \eta (-1 + \eta t) \theta l \\
& (37 + 4 \theta p (8 + \eta^2)) + \eta^2 (996 \theta p - 466 \eta t \theta p - (-1 + \eta t) \theta l \\
& (-86 + 9 \theta p (-82 + 13 \eta^2 + 29 \eta^2)) + \eta^3 (2 \times (-660 + 307 \eta t) \theta p + \\
& (-1 + \eta t) \theta l (136 + \theta p (446 + 117 \eta^2 + 37 \eta^2))) - x (-1 + \eta) \eta \\
& (160 \eta^6 \theta p + 182 \eta t \theta p + 4 \eta^4 (37 + 6 \eta t) \theta p - 24 \eta (4 + 11 \eta t) \theta p - \\
& 8 \eta^5 (3 + 20 \eta t) \theta p - 2 \eta (-1 + \eta t) \theta l (65 + 12 \theta p (8 + \eta^2)) + \\
& \eta^3 (-960 \theta p + 532 \eta t \theta p + (-1 + \eta t) \theta l (58 + \theta p (190 + 69 \eta^2 + 29 \eta^2))) + \\
& \eta^2 (772 \theta p - 314 \eta t \theta p - 3 \times (-1 + \eta t) \theta l \\
& (-24 + \theta p (-214 + 23 \eta^2 + 55 \eta^2))) - x^3 (-1 + \eta)^3 \\
& (4 (-1 + \eta)^2 (-8 + \eta (123 + 2 \eta (27 + 20 \eta - 20 \eta t) - 54 \eta t) + 7 \eta t) \\
& \theta p + (-1 + \eta t) \theta l (-8 \times (13 + \theta p (8 + \eta^2)) + \eta^2 (110 + \\
& \theta p (458 + 87 \eta^2 + 7 \eta^2)) - 3 \eta (2 + \theta p (-114 + 29 \eta^2 + 61 \eta^2))) + \\
& \eta^2 \theta p (104 \eta t + \eta (-32 + 40 \eta^5 + \eta^4 (4 - 40 \eta t) - 4 \eta^3 (-7 + \eta t) + \\
& 8 \theta l (8 + \eta^2) - 2 \eta t (83 + 4 \theta l (8 + \eta^2)) + \eta^2 (-260 - \theta l (26 + 15 \eta^2 + \\
& 7 \eta^2) + \eta t (170 + \theta l (26 + 15 \eta^2 + 7 \eta^2))) + \eta (220 + 3 \theta l \\
& (-66 + 5 \eta^2 + 13 \eta^2) - \eta t (64 + 3 \theta l (-66 + 5 \eta^2 + 13 \eta^2)))) - \\
& w (x (-1 + \eta) - \eta) (-1 + \eta) \times (4 x^4 (-1 + \eta)^4 (-(-1 + \eta)^2 \\
& (3 \eta (-58 + 85 \eta + 50 \eta^2) - 10 \eta (7 + 15 \eta) \eta t + 9 \times (-4 + 3 \eta t)) \theta p + \\
& (-1 + \eta t) \theta l (30 - 30 \eta + 5 \eta^3 \theta p (37 + 2 \eta^2) + 6 \theta p (24 + 6 \eta^2 + 7 \eta^2) - \\
& 4 \eta^2 \theta p (173 + 16 \eta^2) + 3 \eta \theta p (73 - 12 \eta^2 + 16 \eta^2))) + 4 x^5 (-1 + \eta)^5 \\
& \theta p (30 \eta^4 - 3 \eta^3 (9 + 10 \eta t) + \eta (81 - 26 \eta t - 127 \theta l + 127 \eta t \theta l + 14 \times \\
& (-1 + \eta t) \theta l \eta^2) - 2 \times (12 + \eta t - 9 \theta l (4 + \eta^2) + 9 \eta t \theta l (4 + \eta^2)) + \\
& \eta^2 (-60 + 31 \theta l + 2 \theta l \eta^2 + \eta t (58 - 31 \theta l - 2 \theta l \eta^2))) + \\
& x^3 (-1 + \eta)^3 (2 (-1 + \eta)^2 (12 \eta (-24 + \eta (-76 + 5 \eta (23 + 10 \eta))) + 75 \eta t - \\
& 8 \eta (-27 + 65 \eta + 75 \eta^2) \eta t) \theta p - (-1 + \eta t) \theta l (40 \eta^4 \theta p (43 + 2 \eta^2) - \\
& 8 \eta^3 \theta p (749 + 58 \eta^2) + \eta^2 (-300 - 567 \theta p \eta^2 + 33 \theta p (18 + \eta^2)) + 24 \times \\
& (4 + \theta p (2 + 3 \eta^2 + \eta^2)) + 3 \eta (68 + \theta p (762 + 165 \eta^2 + 221 \eta^2))) - \\
& x^2 (-1 + \eta)^2 (1200 \eta^7 \theta p + 120 \eta^6 (9 - 10 \eta t) \theta p + 92 \eta t \theta p + \\
& 8 \eta^4 \theta p (891 + 311 \eta t - 806 \theta l + 806 \eta t \theta l + 52 \times (-1 + \eta t) \theta l \eta^2) + \\
& \eta (134 \eta t \theta p - (-1 + \eta t) \theta l (234 + 189 \theta p \eta^2 + 53 \theta p (2 + \eta^2))) - \\
& 8 \eta^5 \theta p (1002 - 5 \theta l (49 + 2 \eta^2) + 5 \eta t (-22 + \theta l (49 + 2 \eta^2))) + \\
& \eta^3 (-2 \times (264 + 1249 \eta t) \theta p + 3 \times (-1 + \eta t) \theta l \\
& (116 + 3 \theta p (62 + 91 \eta^2 + 35 \eta^2))) - 2 \eta^2 ((432 - 52 \eta t) \theta p + \\
& (-1 + \eta t) \theta l (57 + \theta p (1702 + 315 \eta^2 + 491 \eta^2))) + \\
& x (-1 + \eta) \eta (600 \eta^7 \theta p + 300 \eta^6 (3 - 2 \eta t) \theta p + 190 \eta t \theta p + \\
& 4 \eta^4 \theta p (1053 + 458 \eta t - 863 \theta l + 863 \eta t \theta l + 46 \times (-1 + \eta t) \theta l \eta^2) - \\
& 2 \eta (43 \eta t \theta p + (-1 + \eta t) \theta l (87 + 81 \theta p \eta^2 + 17 \theta p (2 + \eta^2))) - \\
& 4 \eta^5 \theta p (1236 - 5 \theta l (55 + 2 \eta^2) + 5 \eta t (-10 + \theta l (55 + 2 \eta^2))) + \\
& \eta^3 (-2 \times (96 + 785 \eta t) \theta p + 3 \times (-1 + \eta t) \theta l \\
& (56 + \theta p (278 + 171 \eta^2 + 107 \eta^2))) + \eta^2 (-576 \theta p + 34 \eta t \theta p - \\
& (-1 + \eta t) \theta l (-6 + \theta p (2254 + 351 \eta^2 + 647 \eta^2))) + \\
& \eta^2 \theta p (-134 \eta t + \eta (-120 \eta^6 + 12 \eta^5 (-21 + 10 \eta t) - 5 \theta l (2 + 9 \eta^2 + \eta^2) + \\
& 4 \eta^4 (294 + 2 \eta t - 61 \theta l + 61 \eta t \theta l + 2 \times (-1 + \eta t) \theta l \eta^2) + \\
& \eta t (142 + 5 \theta l (2 + 9 \eta^2 + \eta^2)) + \eta^2 (24 + 338 \eta t + \\
& 3 \theta l (90 + 39 \eta^2 + 31 \eta^2) - 3 \eta t \theta l (90 + 39 \eta^2 + 31 \eta^2)) -
\end{aligned}$$

$$\begin{aligned}
& 4 \eta^3 (243 - 8 \theta l (23 + \mathfrak{z}2) + \eta t (121 + 8 \theta l (23 + \mathfrak{z}2))) + 2 \eta (72 - \\
& 4 \theta l (70 + 9 \mathfrak{z}1 + 20 \mathfrak{z}2) + \eta t (5 + 4 \theta l (70 + 9 \mathfrak{z}1 + 20 \mathfrak{z}2))) \Big) \Big) + \\
& w^2 (-1 + \eta)^2 \Big( 4 x^6 (-1 + \eta)^6 \theta p (28 + 10 \eta^4 - 11 \eta t + \eta^2 (16 + 9 \eta t) - \\
& \eta^3 (9 + 10 \eta t) - 16 \theta l + 16 \eta t \theta l - 10 \times (-1 + \eta) \theta l \mathfrak{z}2 + \\
& \eta (-45 - 4 \theta l (2 + \mathfrak{z}2) + 4 \eta t (3 + \theta l (2 + \mathfrak{z}2))) \Big) - 12 x^5 (-1 + \eta)^5 \\
& \Big( (-1 + \eta)^2 (\eta (89 + 4 \eta (13 + 5 \eta - 5 \eta t) - 52 \eta t) - 2 \times (12 + \eta t)) \theta p + \\
& (-1 + \eta t) \theta l (\eta (10 + \theta p (167 + 12 \mathfrak{z}1 - 2 \mathfrak{z}2)) + 3 \eta^2 \theta p (-5 + 2 \mathfrak{z}2) - \\
& 2 \times (5 + \theta p (40 + 6 \mathfrak{z}1 + 11 \mathfrak{z}2))) \Big) - x (-1 + \eta) \eta \\
& (240 \eta^8 \theta p + 12 \eta^6 (17 - 132 \eta t) \theta p + 48 \eta^7 (33 - 5 \eta t) \theta p + 182 \eta t \theta p - \\
& 12 \eta^5 \theta p (702 - 234 \eta t - 179 \theta l + 179 \eta t \theta l + 2 \times (-1 + \eta t) \theta l \mathfrak{z}2) + \\
& 2 \eta (304 \eta t \theta p + (-1 + \eta t) \theta l (-65 + 24 \theta p (2 + \mathfrak{z}2))) + \\
& 6 \eta^4 (2 \times (677 + 79 \eta t) \theta p + (-1 + \eta t) \theta l \\
& (28 + \theta p (1568 + 105 \mathfrak{z}1 + 125 \mathfrak{z}2))) - \eta^2 (576 \theta p + 910 \eta t \theta p + \\
& (-1 + \eta t) \theta l (392 + 3 \theta p (750 + 207 \mathfrak{z}1 + 215 \mathfrak{z}2))) - 3 \eta^3 (4 \times (96 + \\
& 151 \eta t) \theta p + (-1 + \eta t) \theta l (-118 + \theta p (902 + 3 \mathfrak{z}1 + 243 \mathfrak{z}2))) \Big) + \\
& 3 x^4 (-1 + \eta)^4 \Big( 2 (-1 + \eta)^2 (-24 + 43 \eta t + 2 \eta (5 \eta (67 + \eta (41 + \\
& 10 \eta - 10 \eta t) - 41 \eta t) - 6 \times (23 + 5 \eta t))) \theta p + (-1 + \eta t) \\
& \theta l (20 \eta^3 \theta p (-25 + 2 \mathfrak{z}2) - 8 \times (12 + \theta p (26 + 9 \mathfrak{z}1 + 8 \mathfrak{z}2)) + \\
& \eta^2 (140 + \theta p (3106 + 237 \mathfrak{z}1 + 157 \mathfrak{z}2)) - \\
& \eta (44 + \theta p (1406 + 165 \mathfrak{z}1 + 381 \mathfrak{z}2))) \Big) + \\
& 3 x^2 (-1 + \eta)^2 \Big( 200 \eta^8 \theta p + 20 \eta^7 (51 - 10 \eta t) \theta p + 30 \eta t \theta p - \\
& 20 \eta^6 (2 + 51 \eta t) \theta p + 4 \eta^5 (-1293 + 520 \eta t - 330 \times (-1 + \eta t) \theta l) \theta p + \\
& 2 \eta (111 \eta t \theta p + (-1 + \eta t) \theta l (-37 + 8 \theta p (2 + \mathfrak{z}2))) + \\
& 4 \eta^4 (2 \times (637 + 15 \eta t) \theta p + (-1 + \eta t) \theta l \\
& (43 + \theta p (1550 + 111 \mathfrak{z}1 + 121 \mathfrak{z}2))) - \eta^2 (6 \times (48 + 19 \eta t) \theta p + \\
& (-1 + \eta t) \theta l (334 + \theta p (1166 + 351 \mathfrak{z}1 + 343 \mathfrak{z}2))) - \\
& \eta^3 (2 \times (408 + 559 \eta t) \theta p + (-1 + \eta t) \theta l (-236 + \\
& \theta p (2114 + 93 \mathfrak{z}1 + 565 \mathfrak{z}2))) \Big) - x^3 (-1 + \eta)^3 \\
& \Big( 4 (-1 + \eta)^2 (2 \eta (-72 + \eta (-468 + 5 \eta (191 + 4 \eta (28 + 5 \eta)))) + \\
& (69 - 5 \eta (-45 + 4 \eta (15 + 2 \eta (28 + 5 \eta)))) \eta t) \theta p + \\
& (-1 + \eta t) \theta l (40 \eta^4 \theta p (-89 + 2 \mathfrak{z}2) + 8 \times (-13 + 2 \theta p (2 + \mathfrak{z}2)) + \\
& 2 \eta^3 (324 + \theta p (9238 + 693 \mathfrak{z}1 + 653 \mathfrak{z}2)) - 3 \eta^2 (-114 + \theta p (2450 + \\
& 201 \mathfrak{z}1 + 657 \mathfrak{z}2)) - \eta (886 + \theta p (2414 + 783 \mathfrak{z}1 + 727 \mathfrak{z}2))) \Big) + \\
& \eta^2 \theta p (104 \eta t + \eta (40 \eta^7 + 4 \eta^5 (25 - 81 \eta t) + \eta^6 (324 - 40 \eta t) + 6 \eta^2 \\
& (-36 + \eta t (-55 + \theta l (-76 + 3 \mathfrak{z}1 - 21 \mathfrak{z}2)) + \theta l (76 - 3 \mathfrak{z}1 + 21 \mathfrak{z}2))) + \\
& \eta^4 (-1836 + 460 \theta l + 8 \theta l \mathfrak{z}2 + \eta t (504 - 460 \theta l - 8 \theta l \mathfrak{z}2)) + \\
& 2 \times (-8 \theta l (2 + \mathfrak{z}2) + \eta t (97 + 8 \theta l (2 + \mathfrak{z}2))) + \\
& \eta^3 (1732 - \theta l (1906 + 117 \mathfrak{z}1 + 149 \mathfrak{z}2) + \eta t \\
& (358 + \theta l (1906 + 117 \mathfrak{z}1 + 149 \mathfrak{z}2))) + \eta (-144 + \theta l (542 + 135 \\
& \mathfrak{z}1 + 151 \mathfrak{z}2) - \eta t (466 + \theta l (542 + 135 \mathfrak{z}1 + 151 \mathfrak{z}2))) \Big) \Big) + \\
& w^3 (-1 + \eta)^3 \Big( 8 x^6 (-1 + \eta)^6 (-1 + \eta t) \theta l \theta p (-4 + \mathfrak{z}2) + 4 x^5 (-1 + \eta)^5 \\
& \Big( 3 (-1 + \eta)^2 (28 + \eta (11 + 10 \eta - 10 \eta t) - 11 \eta t) \theta p + 2 \times (-1 + \eta t) \\
& \theta l (-5 + \theta p (20 - 6 \mathfrak{z}1 - 17 \mathfrak{z}2) + \eta (5 + 2 \theta p (20 + 3 \mathfrak{z}1 + \mathfrak{z}2))) \Big) - \\
& x^4 (-1 + \eta)^4 \Big( 2 (-1 + \eta)^2 (-144 + 6 \eta (173 + 5 \eta (17 + 10 \eta - 10 \eta t) - 85 \eta t) +
\end{aligned}$$

$$\begin{aligned}
& 13 \eta t) \theta p + (-1 + \eta t) \theta l \left( \eta (148 + \theta p (2458 - 21 \eta 1 - 445 \eta 2)) - \right. \\
& 72 \times (4 + \theta p (14 + 3 \eta 1 + 4 \eta 2)) + \\
& \left. \eta^2 (140 + \theta p (758 + 237 \eta 1 + 181 \eta 2)) \right) + x (-1 + \eta) \eta \\
& (600 \eta^7 \theta p + 12 \eta^5 (2 - 75 \eta t) \theta p + 300 \eta^6 (3 - 2 \eta t) \theta p + 546 \eta t \theta p + \\
& 6 \eta (-2 \times (12 + \eta t) \theta p + (-1 + \eta t) \theta l (-65 + 4 \theta p (-8 + \eta 2))) + \eta^3 (6216 \\
& \theta p - 628 \eta t \theta p + (-1 + \eta t) \theta l (466 + \theta p (7354 + 411 \eta 1 + 83 \eta 2))) + \\
& 2 \eta^4 (2 \times (-1629 + 851 \eta t) \theta p + (-1 + \eta t) \theta l (28 + \theta p \\
& (-386 + 105 \eta 1 + 89 \eta 2))) + \eta^2 (-10 \times (108 + 181 \eta t) \theta p - \\
& 3 \times (-1 + \eta t) \theta l (44 + \theta p (1170 + 207 \eta 1 + 335 \eta 2))) - \\
& x^2 (-1 + \eta)^2 (1200 \eta^7 \theta p + 24 \eta^5 (14 - 45 \eta t) \theta p + 120 \eta^6 (9 - 10 \eta t) \\
& \theta p + 270 \eta t \theta p + \eta^3 (6 \times (1640 - 361 \eta t) \theta p + \\
& (-1 + \eta t) \theta l (1052 + \theta p (11470 + 609 \eta 1 - 127 \eta 2))) + \\
& 6 \eta (3 \times (-8 + 23 \eta t) \theta p + (-1 + \eta t) \theta l (-111 + 4 \theta p (-8 + \eta 2))) + \\
& 4 \eta^4 (9 \times (-296 + 155 \eta t) \theta p + (-1 + \eta t) \theta l \\
& (43 + \theta p (-142 + 111 \eta 1 + 97 \eta 2))) - 3 \eta^2 (6 \times (92 + 101 \eta t) \theta p + \\
& (-1 + \eta t) \theta l (186 + \theta p (1842 + 351 \eta 1 + 527 \eta 2))) + \\
& x^3 (-1 + \eta)^3 (4 (-1 + \eta)^2 (-12 + 6 \eta (-51 + \eta (211 + 5 \eta (23 + 10 \eta))) + \\
& 78 \eta t - 5 \eta (1 + 6 \eta (23 + 10 \eta)) \eta t) \theta p + \\
& (-1 + \eta t) \theta l (\eta^2 (774 + \theta p (8206 + 321 \eta 1 - 479 \eta 2)) + \\
& 8 \times (-39 + \theta p (-8 + \eta 2)) + \eta^3 (216 + \theta p (420 + 462 \eta 1 + 398 \eta 2)) - \\
& \eta (678 + \theta p (3858 + 783 \eta 1 + 1103 \eta 2))) + \\
& \eta^2 \theta p (-312 \eta t + \eta (48 - 120 \eta^6 + 186 \eta t + 12 \eta^5 (-21 + 10 \eta t) + \\
& 12 \eta^4 (1 + 21 \eta t) + 8 \theta l (-8 + \eta 2) - 8 \eta t \theta l (-8 + \eta 2) - 2 \eta^2 (762 - \\
& 4 \theta l (224 + 12 \eta 1 + 5 \eta 2) + \eta t (35 + 4 \theta l (224 + 12 \eta 1 + 5 \eta 2))) + \\
& \eta^3 (1572 + \theta l (-254 + 39 \eta 1 + 31 \eta 2) - \eta t (802 + \theta l (-254 + \\
& 39 \eta 1 + 31 \eta 2))) + \eta (264 - \theta l (834 + 135 \eta 1 + 239 \eta 2) + \\
& \eta t (626 + \theta l (834 + 135 \eta 1 + 239 \eta 2)))))) / \\
& (96 (-1 + w (-1 + \eta))^3 (x (-1 + \eta) - \eta)^3 (w + x + \eta - (w + x) \eta)^3 \\
& (-1 + \\
& \eta t) \theta p))
\end{aligned}$$

$$\beta x = \frac{1}{12} \left( -\frac{1}{(-1+w(-1+\eta))^2 (w+x+\eta-(w+x)\eta)^2} \right. \\
\begin{aligned}
& c\sigma^2 (-1+\eta) (x^3 (-1+\eta)^2 (-4+\mu_1 (2+\eta+(-3+\eta)\mu_1)) + \\
& \eta ((1+\mu_1) \times (4+5\eta+(4+\eta(3+\eta))\mu_1) + (11+6\eta+(11+6\eta(2+\eta))\mu_1)\mu_2 + \\
& 9\mu_2^2) + 9w^3 (-1+\eta)^3 (-1+x-2\mu_2+2\times\mu_1\mu_2-\mu_2^2-\mu_1(2+\mu_1+4\mu_2)) + \\
& x(4(1+\mu_1)^2+10\times(1+\mu_1)\mu_2+9\mu_2^2-\eta^3\mu_1(1+\mu_1+12\mu_2)- \\
& \eta^2(14+12\mu_1+7\mu_1^2+12\times(1+\mu_1)\mu_2) + \\
& \eta(1+3\mu_1^2+\mu_2-9\mu_2^2+\mu_1(4+\mu_2))) - x^2(-1+\eta)(\eta^2\mu_1(1+\mu_1-6\mu_2) + \\
& 4\times(1+\mu_1)(\mu_1+\mu_2)-\eta(13+6\mu_2+\mu_1(3+8\mu_1+6\mu_2))) + \\
& w^2(-1+\eta)^2((1+\mu_1)\times(13+11\mu_1+\eta(14+15\mu_1)) + \\
& (30+23\eta+36\mu_1+65\eta\mu_1)\mu_2+9\times(2+\eta)\mu_2^2 + \\
& x^2(-1+\eta)\times(13+2\mu_2+\mu_1(-4+\mu_1+8\mu_2)) + x((\mu_1+\mu_2)(22+13\mu_1+9\mu_2) - \\
& \eta(27+\mu_1(23+14\mu_1)+23\mu_2+71\mu_1\mu_2+9\mu_2^2))) + w(-1+\eta) \\
& (x^3(-1+\eta)^2(-2+\mu_1)^2-(1+\mu_1)\times(4\times(1+\mu_1)+\eta(18+5\eta+7\times(2+\eta)\mu_1)) - \\
& 2\times(6\times(1+\mu_1)+\eta(17+23\mu_1+3\eta(1+6\mu_1)))\mu_2-9\times(1+2\eta)\mu_2^2 - \\
& x^2(-1+\eta)\times(13-2\mu_2-\mu_1(6+\mu_1+8\mu_2)+\eta(13+5\mu_1^2+6\mu_2+24\mu_1\mu_2)) + \\
& x(-13-15\mu_1^2-2\mu_2(16+9\mu_2)-2\mu_1(14+13\mu_2)+2 \\
& \eta(13+3\mu_1^2+\mu_1(7+5\mu_2)+\mu_2(11+9\mu_2))+\eta^2 \\
& (2\times(7+6\mu_2)+\mu_1(16+11\mu_1+60\mu_2)))) + f\theta l(2+x(-4+\mathfrak{z}2)+\mathfrak{z}2) \Big)
\end{aligned}$$

$$\beta\theta p = \\
\begin{aligned}
& - \left( \left( -cv\,c\sigma\,x(w(-1+\eta)+x(-1+\eta)-\eta)(-1+\eta)(x^2(-1+\eta)^2+\eta(1+\eta)+x(1+\eta-2\eta^2)) \right)^2 \right. \\
& \left( (x+\eta-x\eta)^2(-1+\eta t)\theta l\,\theta p(1+\mu_1)\times(14x(-1+\eta)-14\eta-5\times(2+\mathfrak{z}1+\mathfrak{z}2))+ \right. \\
& w(-1+\eta)\times(-4x^3(-1+\eta)^3\theta p \\
& (1-8\theta l+7\mu_1-14\theta l\mu_1+3\eta^2(1+\mu_1)-\eta\eta t(1+2\theta l)\times(1+\mu_1)+2\eta \\
& (-2+\theta l-5\mu_1+\theta l\mu_1)+\eta t(1+8\theta l+\mu_1+14\theta l\mu_1))+x^2(-1+\eta)^2\theta p \\
& (36\eta^3(1+\mu_1)-12\eta^2(\eta t(1+2\theta l)\times(1+\mu_1)-2\times(-2+\theta l-5\mu_1+\theta l\mu_1))+ \\
& 12\eta(1+7\mu_1-2\theta l(4+7\mu_1)+\eta t(1+\mu_1+2\theta l(4+7\mu_1))) + \\
& (-1+\eta t)\theta l(1+\mu_1)\times(58+15\mathfrak{z}1+15\mathfrak{z}2))-x(-1+\eta)\times \\
& (12\times(-1+\eta)\eta^2\theta p(-1-7\mu_1+3\eta(1+\mu_1)-\eta t(1+\mu_1))-(-1+\eta t)\theta l \\
& (20\times(1+\mu_1)+\theta p(24\eta^3(1+\mu_1)-24\eta^2(4+7\mu_1)+5\times(-6-3\mathfrak{z}1+\mathfrak{z}2)- \\
& 2\eta(1+\mu_1)\times(58+15\mathfrak{z}1+15\mathfrak{z}2)-\mu_1(30+15\mathfrak{z}1+19\mathfrak{z}2)))) + \\
& \theta p(12\eta^5(1+\mu_1)+20\eta t(1+\mu_1)-4\eta^4(\eta t(1+2\theta l)\times(1+\mu_1)-2\times \\
& (-2+\theta l-5\mu_1+\theta l\mu_1))+4\eta^3(1+7\mu_1-2\theta l(4+7\mu_1)+\eta t(1+\mu_1+ \\
& 2\theta l(4+7\mu_1)))+\eta^2(-1+\eta t)\theta l(1+\mu_1)\times(58+15\mathfrak{z}1+15\mathfrak{z}2)+ \\
& \eta(-20\eta t(1+\mu_1)-5\theta l(6+3\mathfrak{z}1-\mathfrak{z}2)-\theta l\mu_1(30+15\mathfrak{z}1+19\mathfrak{z}2)+ \\
& \eta t\theta l(5\times(6+3\mathfrak{z}1-\mathfrak{z}2)+\mu_1(30+15\mathfrak{z}1+19\mathfrak{z}2)))) + w^4(-1+\eta)^4 \\
& (x(-1+\eta)\times(4\times(-1+\eta)\theta p(1-5\mu_1+\eta(1+\mu_1)-\eta t(1+\mu_1))+(-1+\eta t) \\
& \theta l(-20\times(1+\mu_1)+5\theta p(8+3\mathfrak{z}1-\mathfrak{z}2)+\theta p\mu_1(64+15\mathfrak{z}1+19\mathfrak{z}2))) + \\
& \theta p(-4\eta^3(1+\mu_1)-20\eta t(1+\mu_1)+4\eta^2(\eta t+6\mu_1+\eta t\mu_1)+\eta(4-20\mu_1+ \\
& 16\eta t(1+\mu_1)+\theta l(40+64\mu_1+15\mathfrak{z}1+15\mu_1\mathfrak{z}1-5\mathfrak{z}2+19\mu_1\mathfrak{z}2)- \\
& \eta t\theta l(5\times(8+3\mathfrak{z}1-\mathfrak{z}2)+\mu_1(64+15\mathfrak{z}1+19\mathfrak{z}2)))) +
\end{aligned}$$

$$\begin{aligned}
& w^2 (-1 + \eta)^2 (2 x^3 (-1 + \eta)^3 \operatorname{ep} (-2 - 5 \operatorname{el} + 10 \mu 1 - 17 \operatorname{el} \mu 1 + 2 \eta^2 \\
& \quad (1 + \mu 1) - 2 \eta (\eta t + 6 \mu 1 + \eta t \mu 1) + \eta t (2 + 5 \operatorname{el} + 2 \mu 1 + 17 \operatorname{el} \mu 1)) - \\
& \quad x^2 (-1 + \eta)^2 \operatorname{ep} (8 - 94 \operatorname{el} + 56 \mu 1 - 142 \operatorname{el} \mu 1 + 12 \eta^3 (1 + \mu 1) + 8 \eta t (1 + \mu 1) - \\
& \quad 12 \eta^2 (-2 + \eta t + 4 \mu 1 + \eta t \mu 1) + 2 \eta (-22 - 7 \operatorname{el} - 10 \mu 1 - 43 \operatorname{el} \mu 1 + \\
& \quad \eta t (2 + 7 \operatorname{el} + 2 \mu 1 + 43 \operatorname{el} \mu 1)) - 15 \operatorname{el} \boxplus 1 - 15 \operatorname{el} \mu 1 \boxplus 1 - 15 \operatorname{el} \boxplus 2 - 15 \\
& \quad \operatorname{el} \mu 1 \boxplus 2 + \eta t \operatorname{el} (94 + 15 \boxplus 1 + 15 \boxplus 2 + \mu 1 (142 + 15 \boxplus 1 + 15 \boxplus 2))) + \\
& \quad \times (-1 + \eta) \times (4 \times (-1 + \eta) \eta \operatorname{ep} (3 \eta^2 (1 + \mu 1) - 3 \eta (-5 + \eta t + \mu 1 + \eta t \mu 1) - \\
& \quad 4 \times (1 + \eta t + 7 \mu 1 + \eta t \mu 1)) + (-1 + \eta t) \operatorname{el} (-60 \times (1 + \mu 1) + \\
& \quad \operatorname{ep} (104 + \eta^2 (-2 + 70 \mu 1) + 45 \boxplus 1 - 15 \boxplus 2 + \mu 1 (104 + 45 \boxplus 1 + 57 \boxplus 2) + \\
& \quad 2 \eta (94 + 15 \boxplus 1 + 15 \boxplus 2 + \mu 1 (142 + 15 \boxplus 1 + 15 \boxplus 2)))) + \\
& \quad \operatorname{ep} (-4 \eta^5 (1 + \mu 1) - 60 \eta t (1 + \mu 1) + 4 \eta^4 (-6 + \eta t + \eta t \mu 1) + \eta^3 \\
& \quad (36 + 60 \mu 1 + 6 \operatorname{el} (-1 + 3 \mu 1) + \eta t (4 + 6 \operatorname{el} + 4 \mu 1 - 18 \operatorname{el} \mu 1)) + \eta \\
& \quad (60 \eta t (1 + \mu 1) + \operatorname{el} (104 + 45 \boxplus 1 - 15 \boxplus 2 + \mu 1 (104 + 45 \boxplus 1 + 57 \boxplus 2)) - \\
& \quad \eta t \operatorname{el} (104 + 45 \boxplus 1 - 15 \boxplus 2 + \mu 1 (104 + 45 \boxplus 1 + 57 \boxplus 2))) - \eta^2 \\
& \quad (8 + 56 \mu 1 - \operatorname{el} (94 + 15 \boxplus 1 + 15 \boxplus 2 + \mu 1 (142 + 15 \boxplus 1 + 15 \boxplus 2)) + \eta t \\
& \quad (8 \times (1 + \mu 1) + \operatorname{el} (94 + 15 \boxplus 1 + 15 \boxplus 2 + \mu 1 (142 + 15 \boxplus 1 + 15 \boxplus 2)))))) + \\
& w^3 (-1 + \eta)^3 (x^2 (-1 + \eta)^2 \operatorname{ep} (-8 - 30 \operatorname{el} + 40 \mu 1 - 78 \operatorname{el} \mu 1 + 8 \eta^2 (1 + \mu 1) - \\
& \quad 8 \eta (\eta t + 6 \mu 1 + \eta t \mu 1) - 5 \operatorname{el} \boxplus 1 - 5 \operatorname{el} \mu 1 \boxplus 1 - 5 \operatorname{el} \boxplus 2 - 5 \operatorname{el} \mu 1 \boxplus 2 + \eta t \\
& \quad (8 \times (1 + \mu 1) + 5 \operatorname{el} (6 + \boxplus 1 + \boxplus 2) + \operatorname{el} \mu 1 (78 + 5 \boxplus 1 + 5 \boxplus 2))) - \\
& \quad \times (-1 + \eta) \times (4 \times (-1 + \eta) \operatorname{ep} (-1 - 7 \mu 1 + 4 \eta^2 (1 + \mu 1) - \eta t (1 + \mu 1) - \\
& \quad \eta (-7 + 17 \mu 1 + 4 \eta t (1 + \mu 1))) + (-1 + \eta t) \operatorname{el} \\
& \quad (-60 \times (1 + \mu 1) + \operatorname{ep} (122 + 45 \boxplus 1 - 15 \boxplus 2 + \mu 1 (146 + 45 \boxplus 1 + 57 \boxplus 2) + \\
& \quad 2 \eta (26 + 5 \boxplus 1 + 5 \boxplus 2 + \mu 1 (74 + 5 \boxplus 1 + 5 \boxplus 2)))) + \\
& \quad \operatorname{ep} (8 \eta^4 (1 + \mu 1) + 60 \eta t (1 + \mu 1) - 4 \eta^3 (-3 + 9 \mu 1 + 2 \eta t (1 + \mu 1)) + \\
& \quad \eta^2 (-24 - \operatorname{el} (22 + 5 \boxplus 1 + 5 \boxplus 2 + 5 \mu 1 (14 + \boxplus 1 + \boxplus 2)) + \\
& \quad \eta t (4 \times (1 + \mu 1) + \operatorname{el} (22 + 5 \boxplus 1 + 5 \boxplus 2 + 5 \mu 1 (14 + \boxplus 1 + \boxplus 2)))) + \eta (4 + 28 \\
& \quad \mu 1 - \operatorname{el} (122 + 45 \boxplus 1 - 15 \boxplus 2 + \mu 1 (146 + 45 \boxplus 1 + 57 \boxplus 2)) + \eta t (-56 \times (1 + \\
& \quad \mu 1) + \operatorname{el} (122 + 45 \boxplus 1 - 15 \boxplus 2 + \mu 1 (146 + 45 \boxplus 1 + 57 \boxplus 2)))))) - \\
& (1 + x + \eta - x \eta)^2 \operatorname{el} (24 c v^2 x (-1 + w (-1 + \eta))^3 (x + \eta - x \eta)^3 \\
& \quad (w + x + \eta - w \eta - x \eta)^3 (-1 + \eta t) \operatorname{ep} + \\
& f (-4 w^6 (-1 + \eta)^6 (x + \eta - x \eta)^3 (-1 + \eta t) \operatorname{el} \operatorname{ep} (2 + \boxplus 2) \times \\
& \quad (-2 + \operatorname{ep} (2 + \boxplus 2)) + 2 w^5 (-1 + \eta)^5 \\
& \quad (6 \eta^3 (1 + \eta) \times (-1 + \eta t) \operatorname{el} \operatorname{ep} (2 + \boxplus 2) \times (-2 + \operatorname{ep} (2 + \boxplus 2)) + 2 x^4 (-1 + \eta)^4 \\
& \quad ((-1 + \eta) \operatorname{ep} (-54 + 10 \eta^2 + \eta t (-15 + \boxplus 2) - 5 \boxplus 2 - \eta (-15 + 10 \eta t + \boxplus 2)) + \\
& \quad (-1 + \eta t) \operatorname{el} (-12 + 5 \boxplus 2 + 3 \operatorname{ep}^2 (2 + \boxplus 2)^2 + 3 \operatorname{ep} (18 + 3 \boxplus 1 + \boxplus 2))) - x^3 \\
& \quad (-1 + \eta)^3 (60 \eta^4 \operatorname{ep} + 6 \eta^2 \operatorname{ep} (-69 + \eta t (-5 + \boxplus 2) - 4 \boxplus 2) - 6 \eta^3 \operatorname{ep} \\
& \quad (-5 + 10 \eta t + \boxplus 2) + \eta (\operatorname{ep} (324 + 59 \eta t + 30 \boxplus 2 + 4 \eta t \boxplus 2) + (-1 + \eta t) \\
& \quad \operatorname{el} (-41 + 20 \boxplus 2 + 24 \operatorname{ep}^2 (2 + \boxplus 2)^2 + 6 \operatorname{ep} (50 + 9 \boxplus 1 + \boxplus 2))) + \\
& \quad \operatorname{ep} (-6 \operatorname{el} (2 + \boxplus 2) \times (-2 + \operatorname{ep} (2 + \boxplus 2)) + \eta t (31 - 10 \boxplus 2 + \\
& \quad 6 \operatorname{el} (2 + \boxplus 2) \times (-2 + \operatorname{ep} (2 + \boxplus 2)))) + x^2 (-1 + \eta)^2 \\
& \quad \eta (60 \eta^4 \operatorname{ep} + 6 \eta^2 \operatorname{ep} (-69 + \eta t (-5 + \boxplus 2) - 4 \boxplus 2) - 6 \eta^3 \operatorname{ep} \\
& \quad (-5 + 10 \eta t + \boxplus 2) + \eta (\operatorname{ep} (324 + 29 \eta t + 30 \boxplus 2 + 14 \eta t \boxplus 2) + (-1 + \eta t) \\
& \quad \operatorname{el} (-11 + 18 \operatorname{ep} (14 + 3 \boxplus 1 - \boxplus 2) + 10 \boxplus 2 + 36 \operatorname{ep}^2 (2 + \boxplus 2)^2)) + \\
& \quad \operatorname{ep} (-18 \operatorname{el} (2 + \boxplus 2) \times (-2 + \operatorname{ep} (2 + \boxplus 2)) + \eta t (61 - 20 \boxplus 2 +
\end{aligned}$$

$$\begin{aligned}
& 18 \, \theta l \, (2 + \mathfrak{z}2) \times (-2 + \theta p \, (2 + \mathfrak{z}2))) - 2 \\
& \times (-1 + \eta) \, \eta^2 \, \theta p \, (10 \, \eta^4 + \eta^2 \, (-69 + \eta t \, (-5 + \mathfrak{z}2) - 4 \, \mathfrak{z}2) - \\
& \quad \eta^3 \, (-5 + 10 \, \eta t + \mathfrak{z}2) - 9 \, \theta l \, (2 + \mathfrak{z}2) \times (-2 + \theta p \, (2 + \mathfrak{z}2)) + \\
& \quad \eta t \, (12 - 5 \, \mathfrak{z}2 + 9 \, \theta l \, (2 + \mathfrak{z}2) \times (-2 + \theta p \, (2 + \mathfrak{z}2))) + \\
& \quad \eta \, (54 + 5 \, \mathfrak{z}2 - 3 \, \theta l \, (6 + 3 \, \mathfrak{z}1 - 5 \, \mathfrak{z}2 + 4 \, \theta p \, (2 + \mathfrak{z}2)^2) + \\
& \quad \quad \eta t \, (3 + 4 \, \mathfrak{z}2 + 3 \, \theta l \, (6 + 3 \, \mathfrak{z}1 - 5 \, \mathfrak{z}2 + 4 \, \theta p \, (2 + \mathfrak{z}2)^2)))) - \\
& (x + \eta - x \, \eta)^2 \, (4 \, \eta^4 \, (-1 + \eta t) \, \theta l \, \theta p \, (2 + \mathfrak{z}2) \times (-2 + \theta p \, (2 + \mathfrak{z}2)) - 2 \\
& \quad x^5 \, (-1 + \eta)^5 \, \theta p \, (108 + 60 \, \eta^3 - 108 \, \theta l + 6 \, \mathfrak{z}2 - 20 \, \theta l \, \mathfrak{z}2 - \\
& \quad 5 \, \theta l \, \mathfrak{z}2^2 - 2 \, \eta t \, (5 + \mathfrak{z}2) - 4 \, \eta^2 \, (20 - 5 \, \theta l + 5 \, \eta t \, (2 + \theta l) + \mathfrak{z}2) - \\
& \quad 2 \, \eta \, (44 + 5 \, \theta l + \eta t \, (-25 + \theta l \, (-5 + \mathfrak{z}2) - \mathfrak{z}2) + \mathfrak{z}2 - \theta l \, \mathfrak{z}2) + \\
& \quad \eta t \, \theta l \, (108 + 20 \, \mathfrak{z}2 + 5 \, \mathfrak{z}2^2)) + 2 \, x^2 \, (-1 + \eta)^2 \, \eta \\
& (240 \, \eta^5 \, \theta p + 4 \, \eta t \, \theta p \, (13 - 5 \, \mathfrak{z}2) - 16 \, \eta^4 \, \theta p \, (20 - 5 \, \theta l + 5 \, \eta t \, (2 + \theta l) + \mathfrak{z}2) - \\
& \quad 8 \, \eta^3 \, \theta p \, (44 + \eta t \, (-25 + \theta l \, (-5 + \mathfrak{z}2) - \mathfrak{z}2) - \theta l \, (-5 + \mathfrak{z}2) + \mathfrak{z}2) + \\
& \quad 4 \, \eta^2 \, \theta p \, (-2 \, \eta t \, (5 + \mathfrak{z}2) + 6 \times (18 + \mathfrak{z}2) - \theta l \, (108 + 20 \, \mathfrak{z}2 + 5 \, \mathfrak{z}2^2) + \\
& \quad \quad \eta t \, \theta l \, (108 + 20 \, \mathfrak{z}2 + 5 \, \mathfrak{z}2^2)) + \eta \, (4 \, \eta t \, \theta p \, (-13 + 5 \, \mathfrak{z}2) + \\
& \quad \quad (-1 + \eta t) \, \theta l \, (12 \, \theta p^2 \, (2 + \mathfrak{z}2)^2 + 2 \times (-6 + 5 \, \mathfrak{z}2) + \\
& \quad \quad \quad \theta p \, (16 + 66 \, \mathfrak{z}1 - 22 \, \mathfrak{z}2 - 15 \, \mathfrak{z}2^2)))) - x^3 \, (-1 + \eta)^3 \, (720 \, \eta^5 \, \theta p + \\
& \quad 10 \, \eta t \, \theta p \, (3 - 2 \, \mathfrak{z}2) - 48 \, \eta^4 \, \theta p \, (20 - 5 \, \theta l + 5 \, \eta t \, (2 + \theta l) + \mathfrak{z}2) - \\
& \quad 24 \, \eta^3 \, \theta p \, (44 + \eta t \, (-25 + \theta l \, (-5 + \mathfrak{z}2) - \mathfrak{z}2) - \theta l \, (-5 + \mathfrak{z}2) + \mathfrak{z}2) + \\
& \quad 12 \, \eta^2 \, \theta p \, (-2 \, \eta t \, (5 + \mathfrak{z}2) + 6 \times (18 + \mathfrak{z}2) - \\
& \quad \quad \theta l \, (108 + 20 \, \mathfrak{z}2 + 5 \, \mathfrak{z}2^2) + \eta t \, \theta l \, (108 + 20 \, \mathfrak{z}2 + 5 \, \mathfrak{z}2^2)) + \\
& \quad \eta \, (10 \, \eta t \, \theta p \, (-3 + 2 \, \mathfrak{z}2) + (-1 + \eta t) \, \theta l \, (16 \, \theta p^2 \, (2 + \mathfrak{z}2)^2 + \\
& \quad \quad 20 \times (-5 + 2 \, \mathfrak{z}2) + 3 \, \theta p \, (22 + 47 \, \mathfrak{z}1 - 9 \, \mathfrak{z}2 - 10 \, \mathfrak{z}2^2)))) - 2 \, x^4 \\
& (-1 + \eta)^4 \, (-8 \times (-1 + \eta) \, \eta \, \theta p \, (30 \, \eta^2 + \eta t \, (5 + \mathfrak{z}2) - 3 \times (18 + \mathfrak{z}2) - \\
& \quad 2 \, \eta \, (5 + 10 \, \eta t + \mathfrak{z}2)) - (-1 + \eta t) \, \theta l \, (10 \times (-2 + \mathfrak{z}2) + \\
& \quad 2 \, \theta p^2 \, (2 + \mathfrak{z}2)^2 + \theta p \, (12 - 80 \, \eta^3 + 24 \, \mathfrak{z}1 - 8 \, \eta^2 \, (-5 + \mathfrak{z}2) - 4 \, \mathfrak{z}2 - \\
& \quad \quad 5 \, \mathfrak{z}2^2 + 4 \, \eta \, (108 + 20 \, \mathfrak{z}2 + 5 \, \mathfrak{z}2^2)))) - x \, (-1 + \eta) \, \eta^2 \, \theta p \\
& (120 \, \eta^5 + 38 \, \eta t - 20 \, \eta t \, \mathfrak{z}2 - 8 \, \eta^4 \, (20 - 5 \, \theta l + 5 \, \eta t \, (2 + \theta l) + \mathfrak{z}2) - \\
& \quad 4 \, \eta^3 \, (44 + \eta t \, (-25 + \theta l \, (-5 + \mathfrak{z}2) - \mathfrak{z}2) - \theta l \, (-5 + \mathfrak{z}2) + \mathfrak{z}2) + \\
& \quad 2 \, \eta^2 \, (-2 \, \eta t \, (5 + \mathfrak{z}2) + 6 \times (18 + \mathfrak{z}2) - \\
& \quad \quad \theta l \, (108 + 20 \, \mathfrak{z}2 + 5 \, \mathfrak{z}2^2) + \eta t \, \theta l \, (108 + 20 \, \mathfrak{z}2 + 5 \, \mathfrak{z}2^2)) + \\
& \quad \eta \, (\theta l \, (26 - 39 \, \mathfrak{z}1 + 33 \, \mathfrak{z}2 + 10 \, \mathfrak{z}2^2 - 16 \, \theta p \, (2 + \mathfrak{z}2)^2) + \eta t \, (-38 + \\
& \quad \quad 20 \, \mathfrak{z}2 + \theta l \, (-26 + 39 \, \mathfrak{z}1 - 33 \, \mathfrak{z}2 - 10 \, \mathfrak{z}2^2 + 16 \, \theta p \, (2 + \mathfrak{z}2)^2)))) + \\
& w^2 \, (-1 + \eta)^2 \, (-12 \, \eta^4 \, (1 + 3 \, \eta + \eta^2) \times (-1 + \eta t) \, \theta l \, \theta p \, (2 + \mathfrak{z}2) \times \\
& \quad (-2 + \theta p \, (2 + \mathfrak{z}2)) + 2 \, x^7 \, (-1 + \eta)^7 \, \theta p \, (108 + 20 \, \eta^3 - 108 \, \theta l + \\
& \quad 2 \, \eta \, (-69 + \eta t \, (-5 + \mathfrak{z}2) - 4 \, \mathfrak{z}2) + 10 \, \mathfrak{z}2 - 16 \, \theta l \, \mathfrak{z}2 - 5 \, \theta l \, \mathfrak{z}2^2 - \\
& \quad 2 \, \eta^2 \, (-5 + 10 \, \eta t + \mathfrak{z}2) + \eta t \, (30 - 2 \, \mathfrak{z}2 + \theta l \, (108 + 16 \, \mathfrak{z}2 + 5 \, \mathfrak{z}2^2)))) - 6 \, x^6 \\
& (-1 + \eta)^6 \, (2 \times (-1 + \eta) \, \theta p \, (20 \, \eta^3 + \eta \, (-63 + 2 \, \eta t \, (-30 + \mathfrak{z}2) - 13 \, \mathfrak{z}2) + \\
& \quad 2 \times (-74 + \eta t \, (-5 + \mathfrak{z}2) - 4 \, \mathfrak{z}2) - 2 \, \eta^2 \, (-30 + 10 \, \eta t + \mathfrak{z}2)) + \\
& \quad (-1 + \eta t) \, \theta l \, (10 \times (-2 + \mathfrak{z}2) + 2 \, \theta p^2 \, (2 + \mathfrak{z}2)^2 + \theta p \\
& \quad \quad (308 + 24 \, \mathfrak{z}1 + 32 \, \mathfrak{z}2 + 5 \, \mathfrak{z}2^2 + 2 \, \eta \, (73 + 15 \, \mathfrak{z}2 + 5 \, \mathfrak{z}2^2)))) - x^2 \\
& (-1 + \eta)^2 \, \eta \, (240 \, \eta^7 \, \theta p + 12 \, \eta^5 \, \theta p \, (57 + 2 \, \eta t \, (-80 + \mathfrak{z}2) - 23 \, \mathfrak{z}2) + \\
& \quad 2 \, \eta t \, \theta p \, (61 - 20 \, \mathfrak{z}2) - 24 \, \eta^6 \, \theta p \, (-80 + 10 \, \eta t + \mathfrak{z}2) +
\end{aligned}$$



$$\begin{aligned}
& 3 \eta^2 \left( 8 \theta p \left( 6 \times (18 + \mathfrak{z}2) + \eta t \left( -34 + 3 \mathfrak{z}2 \right) \right) + (-1 + \eta t) \theta l \left( -58 + 40 \mathfrak{z}2 + \right. \right. \\
& \quad \left. \left. 120 \theta p^2 \left( 2 + \mathfrak{z}2 \right)^2 + \theta p \left( 814 + 351 \mathfrak{z}1 - 25 \mathfrak{z}2 - 40 \mathfrak{z}2^2 \right) \right) \right) + \\
& 2 \eta \left( \eta t \theta p \left( 497 - 160 \mathfrak{z}2 \right) + (-1 + \eta t) \theta l \left( -11 + 10 \mathfrak{z}2 + \right. \right. \\
& \quad \left. \left. 36 \theta p^2 \left( 2 + \mathfrak{z}2 \right)^2 + 3 \theta p \left( -24 + 18 \mathfrak{z}1 - 22 \mathfrak{z}2 - 5 \mathfrak{z}2^2 \right) \right) \right) + \\
& 12 \eta^4 \theta p \left( -1017 - 23 \mathfrak{z}2 + \theta l \left( 107 - 11 \mathfrak{z}2 - 5 \mathfrak{z}2^2 \right) + \right. \\
& \quad \left. \eta t \left( 50 + 8 \mathfrak{z}2 + \theta l \left( -107 + 11 \mathfrak{z}2 + 5 \mathfrak{z}2^2 \right) \right) \right) + 6 \eta^3 \left( 2 \theta p \right. \\
& \quad \left. (564 + 36 \mathfrak{z}2 + 7 \eta t \left( 15 + 2 \mathfrak{z}2 \right)) + (-1 + \eta t) \theta l \left( 30 \theta p^2 \left( 2 + \mathfrak{z}2 \right)^2 + \right. \right. \\
& \quad \left. \left. 2 \times (-6 + 5 \mathfrak{z}2) + \theta p \left( 1502 + 105 \mathfrak{z}1 + 113 \mathfrak{z}2 + 25 \mathfrak{z}2^2 \right) \right) \right) + \\
& x^3 (-1 + \eta)^3 \left( 600 \eta^7 \theta p + 2 \eta t \theta p \left( 31 - 10 \mathfrak{z}2 \right) + 60 \eta^5 \theta p \right. \\
& \quad \left. (-3 + \eta t \left( -65 + \mathfrak{z}2 \right) - 10 \mathfrak{z}2) - 60 \eta^6 \theta p \left( -65 + 10 \eta t + \mathfrak{z}2 \right) + \right. \\
& \quad \left. 9 \eta^2 \left( \theta p \left( 24 \times (18 + \mathfrak{z}2) - 2 \eta t \left( 43 + 4 \mathfrak{z}2 \right) \right) + (-1 + \eta t) \theta l \left( -96 + \right. \right. \right. \\
& \quad \left. \left. 40 \mathfrak{z}2 + 40 \theta p^2 \left( 2 + \mathfrak{z}2 \right)^2 + \theta p \left( 506 + 189 \mathfrak{z}1 + 37 \mathfrak{z}2 - 20 \mathfrak{z}2^2 \right) \right) \right) + \\
& 2 \eta \left( 10 \eta t \theta p \left( 59 - 17 \mathfrak{z}2 \right) + (-1 + \eta t) \theta l \left( -41 + 20 \mathfrak{z}2 + \right. \right. \\
& \quad \left. \left. 24 \theta p^2 \left( 2 + \mathfrak{z}2 \right)^2 + 3 \theta p \left( -8 + 18 \mathfrak{z}1 - 14 \mathfrak{z}2 - 5 \mathfrak{z}2^2 \right) \right) \right) + \\
& 6 \eta^4 \theta p \left( -3800 - 74 \mathfrak{z}2 - 5 \theta l \left( -56 + 12 \mathfrak{z}2 + 5 \mathfrak{z}2^2 \right) + \right. \\
& \quad \left. 5 \eta t \left( 62 + 6 \mathfrak{z}2 + \theta l \left( -56 + 12 \mathfrak{z}2 + 5 \mathfrak{z}2^2 \right) \right) \right) + 12 \eta^3 \\
& \quad \left( \theta p \left( 1216 + 74 \mathfrak{z}2 + \eta t \left( 181 + 16 \mathfrak{z}2 \right) \right) + (-1 + \eta t) \theta l \left( -37 + 20 \mathfrak{z}2 + \right. \right. \\
& \quad \left. \left. 20 \theta p^2 \left( 2 + \mathfrak{z}2 \right)^2 + \theta p \left( 1536 + 111 \mathfrak{z}1 + 137 \mathfrak{z}2 + 25 \mathfrak{z}2^2 \right) \right) \right) - x^4 \\
& (-1 + \eta)^4 \left( 4 \times (-1 + \eta) \theta p \left( 200 \eta^5 + 12 \eta^2 \left( -380 + 5 \eta t \left( -9 + \mathfrak{z}2 \right) - 22 \mathfrak{z}2 \right) + \right. \right. \\
& \quad \left. \left. 10 \eta^3 \left( 63 + 2 \eta t \left( -60 + \mathfrak{z}2 \right) - 19 \mathfrak{z}2 \right) - 20 \eta^4 \left( -60 + 10 \eta t + \mathfrak{z}2 \right) + \right. \right. \\
& \quad \left. \left. 15 \eta t \left( -7 + 2 \mathfrak{z}2 \right) + 9 \eta \left( -4 \times (18 + \mathfrak{z}2) + \eta t \left( -7 + 8 \mathfrak{z}2 \right) \right) \right) + \right. \\
& \quad \left. (-1 + \eta t) \theta l \left( 40 \eta^3 \theta p \left( -9 + 13 \mathfrak{z}2 + 5 \mathfrak{z}2^2 \right) + 2 \times \right. \right. \\
& \quad \left. \left. (-24 + 18 \theta p \mathfrak{z}1 + 10 \mathfrak{z}2 - 5 \theta p \mathfrak{z}2 \left( 2 + \mathfrak{z}2 \right) + 6 \theta p^2 \left( 2 + \mathfrak{z}2 \right)^2 \right) + \right. \\
& \quad \left. 3 \eta \left( 60 \theta p^2 \left( 2 + \mathfrak{z}2 \right)^2 + 6 \times (-61 + 20 \mathfrak{z}2) + \theta p \left( 1130 + 405 \mathfrak{z}1 + \right. \right. \right. \\
& \quad \left. \left. 133 \mathfrak{z}2 - 40 \mathfrak{z}2^2 \right) \right) + 6 \eta^2 \left( -132 + 60 \mathfrak{z}2 + 30 \theta p^2 \left( 2 + \mathfrak{z}2 \right)^2 + \right. \\
& \quad \left. \theta p \left( 3094 + 231 \mathfrak{z}1 + 299 \mathfrak{z}2 + 50 \mathfrak{z}2^2 \right) \right) \right) + 3 x^5 (-1 + \eta)^5 \\
& \left( 2 \times (-1 + \eta) \theta p \left( 100 \eta^4 + 10 \eta^2 \left( -3 + \eta t \left( -45 + \mathfrak{z}2 \right) - 8 \mathfrak{z}2 \right) - \right. \right. \\
& \quad \left. \left. 6 \times (18 + \mathfrak{z}2) - 10 \eta^3 \left( -45 + 10 \eta t + \mathfrak{z}2 \right) + \eta t \left( -5 + 12 \mathfrak{z}2 \right) + \right. \right. \\
& \quad \left. \left. 4 \eta \left( 5 \eta t \left( -7 + \mathfrak{z}2 \right) - 3 \times (125 + 7 \mathfrak{z}2) \right) \right) + (-1 + \eta t) \theta l \right. \\
& \quad \left( 10 \eta^2 \theta p \left( 34 + 14 \mathfrak{z}2 + 5 \mathfrak{z}2^2 \right) + 2 \times \left( -68 + 20 \mathfrak{z}2 + 6 \theta p^2 \left( 2 + \mathfrak{z}2 \right)^2 + \right. \right. \\
& \quad \left. \left. \theta p \left( 152 + 54 \mathfrak{z}1 + 22 \mathfrak{z}2 - 5 \mathfrak{z}2^2 \right) \right) + \eta \left( 24 \theta p^2 \left( 2 + \mathfrak{z}2 \right)^2 + \right. \right. \\
& \quad \left. \left. 20 \times (-9 + 4 \mathfrak{z}2) + \theta p \left( 3094 + 237 \mathfrak{z}1 + 313 \mathfrak{z}2 + 50 \mathfrak{z}2^2 \right) \right) \right) \right) + x \\
& (-1 + \eta) \eta^2 \theta p \left( 40 \eta^7 + 4 \eta^5 \left( 66 + \eta t \left( -95 + \mathfrak{z}2 \right) - 13 \mathfrak{z}2 \right) + \right. \\
& \quad \left. 4 \eta t \left( 12 - 5 \mathfrak{z}2 \right) - 4 \eta^6 \left( -95 + 10 \eta t + \mathfrak{z}2 \right) + 2 \eta^4 \left( -1290 + 162 \theta l - 32 \mathfrak{z}2 - \right. \right. \\
& \quad \left. \left. 10 \theta l \mathfrak{z}2 - 5 \theta l \mathfrak{z}2^2 + 10 \eta t \left( 3 + \mathfrak{z}2 \right) + \eta t \theta l \left( -162 + 10 \mathfrak{z}2 + 5 \mathfrak{z}2^2 \right) \right) \right) + \\
& 3 \eta^3 \left( 416 + 28 \mathfrak{z}2 + 2 \eta t \left( 51 + 8 \mathfrak{z}2 \right) - \theta l \left( 554 + 39 \mathfrak{z}1 + 19 \mathfrak{z}2 + \right. \right. \\
& \quad \left. \left. 10 \mathfrak{z}2^2 + 24 \theta p \left( 2 + \mathfrak{z}2 \right)^2 \right) + \eta t \theta l \left( 554 + 39 \mathfrak{z}1 + 19 \mathfrak{z}2 + 10 \mathfrak{z}2^2 + \right. \right. \\
& \quad \left. \left. 24 \theta p \left( 2 + \mathfrak{z}2 \right)^2 \right) \right) + 3 \eta^2 \left( 16 \eta t \left( -5 + \mathfrak{z}2 \right) + 12 \times (18 + \mathfrak{z}2) - \right. \\
& \quad \left. \theta l \left( 74 + 81 \mathfrak{z}1 - 71 \mathfrak{z}2 - 10 \mathfrak{z}2^2 + 60 \theta p \left( 2 + \mathfrak{z}2 \right)^2 \right) + \right. \\
& \quad \left. \eta t \theta l \left( 74 + 81 \mathfrak{z}1 - 71 \mathfrak{z}2 - 10 \mathfrak{z}2^2 + 60 \theta p \left( 2 + \mathfrak{z}2 \right)^2 \right) \right) + \\
& 2 \eta \left( \theta l \left( 72 - 18 \mathfrak{z}1 + 46 \mathfrak{z}2 + 5 \mathfrak{z}2^2 - 24 \theta p \left( 2 + \mathfrak{z}2 \right)^2 \right) + \eta t \left( 123 - \right. \right. \\
& \quad \left. \left. 50 \mathfrak{z}2 + \theta l \left( -72 + 18 \mathfrak{z}1 - 46 \mathfrak{z}2 - 5 \mathfrak{z}2^2 + 24 \theta p \left( 2 + \mathfrak{z}2 \right)^2 \right) \right) \right) \right) + \\
& w \left( x \left( -1 + \eta \right) - \eta \right) \left( -1 + \eta \right) \times \left( -12 \eta^4 \left( 1 + \eta \right) \times \left( -1 + \eta t \right) \theta l \theta p \right.
\end{aligned}$$

$$\begin{aligned}
& (2 + \mathfrak{z}) \times (-2 + \mathfrak{p} (2 + \mathfrak{z})) - 4 x^6 (-1 + \eta)^6 \mathfrak{p} \\
& (148 + 30 \eta^3 - 148 \mathfrak{p} + 8 \mathfrak{z} - 18 \mathfrak{p} \mathfrak{z} - 5 \mathfrak{p} \mathfrak{z}^2 - 3 \eta^2 (-5 + 10 \eta \mathfrak{t} + \mathfrak{z}) + \\
& \quad \eta (-193 - 5 \mathfrak{z} + 2 \eta \mathfrak{t} (10 + \mathfrak{z}) + \mathfrak{p} (35 + \mathfrak{z}) - \eta \mathfrak{t} \mathfrak{p} (35 + \mathfrak{z})) + \\
& \quad \eta \mathfrak{t} (-2 \times (-5 + \mathfrak{z}) + \mathfrak{p} (148 + 18 \mathfrak{z} + 5 \mathfrak{z}^2))) - x^2 (-1 + \eta)^2 \eta \\
& (600 \eta^6 \mathfrak{p} + 2 \eta \mathfrak{t} \mathfrak{p} (137 - 40 \mathfrak{z}) - 60 \eta^5 \mathfrak{p} (-29 + 10 \eta \mathfrak{t} + \mathfrak{z}) + \\
& \quad 4 \eta^3 \mathfrak{p} (2 \eta \mathfrak{t} (175 + \mathfrak{z}) + 4 \times (53 + 7 \mathfrak{z}) - \mathfrak{p} (800 + 78 \mathfrak{z} + 25 \mathfrak{z}^2) + \\
& \quad \eta \mathfrak{t} \mathfrak{p} (800 + 78 \mathfrak{z} + 25 \mathfrak{z}^2))) - 4 \eta^4 \mathfrak{p} \\
& \quad (1445 + 49 \mathfrak{z} - 5 \mathfrak{p} (59 + \mathfrak{z}) + 5 \eta \mathfrak{t} (28 - 2 \mathfrak{z} + \mathfrak{p} (59 + \mathfrak{z}))) + \\
& \quad 3 \eta^2 (2 \mathfrak{p} (24 \times (18 + \mathfrak{z}) + \eta \mathfrak{t} (-111 + 22 \mathfrak{z})) + (-1 + \eta \mathfrak{t}) \mathfrak{p} \\
& \quad (40 \mathfrak{p}^2 (2 + \mathfrak{z})^2 + 4 \times (-6 + 5 \mathfrak{z}) + \mathfrak{p} (870 + 171 \mathfrak{z} + 83 \mathfrak{z}^2))) + \\
& \quad 2 \eta (2 \eta \mathfrak{t} \mathfrak{p} (38 - 25 \mathfrak{z}) + (-1 + \eta \mathfrak{t}) \mathfrak{p} (-29 + 20 \mathfrak{z} + 36 \mathfrak{p}^2 \\
& \quad (2 + \mathfrak{z})^2 + \mathfrak{p} (22 + 135 \mathfrak{z} - 49 \mathfrak{z} - 30 \mathfrak{z}^2)))) - x^4 (-1 + \eta)^4 \\
& (2 \times (-1 + \eta) \mathfrak{p} (600 \eta^4 + 8 \eta^2 (-400 + 5 \eta \mathfrak{t} (-17 + \mathfrak{z}) - 26 \mathfrak{z}) - \\
& \quad 60 \eta^3 (-27 + 10 \eta \mathfrak{t} + \mathfrak{z}) + 15 \eta \mathfrak{t} (-3 + 2 \mathfrak{z}) + \\
& \quad 24 \eta (\eta \mathfrak{t} (5 + \mathfrak{z}) - 3 \times (18 + \mathfrak{z}))) - (-1 + \eta \mathfrak{t}) \mathfrak{p} \\
& \quad (40 \eta^3 \mathfrak{p} (47 + \mathfrak{z}) - 8 \eta^2 \mathfrak{p} (770 + 84 \mathfrak{z} + 25 \mathfrak{z}^2) - 3 \eta \\
& \quad (20 \mathfrak{p}^2 (2 + \mathfrak{z})^2 + 20 \times (-7 + 3 \mathfrak{z}) + \mathfrak{p} (954 + 189 \mathfrak{z} + 125 \mathfrak{z}^2)) - \\
& \quad 4 \times (-34 + 10 \mathfrak{z} + 3 \mathfrak{p}^2 (2 + \mathfrak{z})^2 + \mathfrak{p} (22 + 27 \mathfrak{z} + \mathfrak{z} - 5 \mathfrak{z}^2)))) + \\
& x^3 (-1 + \eta)^3 (1200 \eta^6 \mathfrak{p} + 20 \eta \mathfrak{t} \mathfrak{p} (7 - 2 \mathfrak{z}) - 120 \eta^5 \mathfrak{p} \\
& \quad (-23 + 10 \eta \mathfrak{t} + \mathfrak{z}) - 8 \eta^4 \mathfrak{p} (1325 + 43 \mathfrak{z} - \\
& \quad 5 \mathfrak{p} (53 + \mathfrak{z}) + 5 \eta \mathfrak{t} (-2 \times (-8 + \mathfrak{z}) + \mathfrak{p} (53 + \mathfrak{z}))) + \\
& \quad 3 \eta^2 (2 \mathfrak{p} (36 \times (18 + \mathfrak{z}) + \eta \mathfrak{t} (-127 + 18 \mathfrak{z})) + (-1 + \eta \mathfrak{t}) \mathfrak{p} \\
& \quad (-124 + 60 \mathfrak{z} + 40 \mathfrak{p}^2 (2 + \mathfrak{z})^2 + \mathfrak{p} (1394 + 273 \mathfrak{z} + 169 \mathfrak{z}^2))) + \\
& \quad \eta (2 \eta \mathfrak{t} \mathfrak{p} (131 - 70 \mathfrak{z}) + (-1 + \eta \mathfrak{t}) \mathfrak{p} (-230 + 80 \mathfrak{z} + \\
& \quad 48 \mathfrak{p}^2 (2 + \mathfrak{z})^2 + \mathfrak{p} (178 + 297 \mathfrak{z} - 31 \mathfrak{z} - 60 \mathfrak{z}^2)))) + \\
& \quad 8 \eta^3 \mathfrak{p} (344 + 31 \mathfrak{z} - \mathfrak{p} (785 + 81 \mathfrak{z} + 25 \mathfrak{z}^2) + \eta \mathfrak{t} \\
& \quad (275 - \mathfrak{z} + \mathfrak{p} (785 + 81 \mathfrak{z} + 25 \mathfrak{z}^2)))) + 4 x^5 (-1 + \eta)^5 \\
& ((-1 + \eta) \mathfrak{p} (150 \eta^3 + 2 \eta (-385 + 5 \eta \mathfrak{t} (-11 + \mathfrak{z}) - 23 \mathfrak{z}) + \\
& \quad 3 \eta \mathfrak{t} (5 + \mathfrak{z}) - 9 \times (18 + \mathfrak{z}) - 15 \eta^2 (-21 + 10 \eta \mathfrak{t} + \mathfrak{z})) + \\
& \quad (-1 + \eta \mathfrak{t}) \mathfrak{p} (15 \times (-2 + \mathfrak{z}) + 3 \mathfrak{p}^2 (2 + \mathfrak{z})^2 + \mathfrak{p} (-5 \eta^2 (41 + \mathfrak{z}) + \\
& \quad 12 \times (15 + 3 \mathfrak{z} + 2 \mathfrak{z}) + \eta (755 + 87 \mathfrak{z} + 25 \mathfrak{z}^2)))) + x (-1 + \eta) \\
& \eta^2 \mathfrak{p} (120 \eta^6 + 98 \eta \mathfrak{t} - 40 \eta \mathfrak{t} \mathfrak{z} - 12 \eta^5 (-35 + 10 \eta \mathfrak{t} + \mathfrak{z}) - \\
& \quad 4 \eta^4 (313 + 11 \mathfrak{z} - \mathfrak{p} (65 + \mathfrak{z}) + \eta \mathfrak{t} (40 - 2 \mathfrak{z} + \mathfrak{p} (65 + \mathfrak{z}))) + \\
& \quad 4 \eta^3 (16 + 5 \mathfrak{z} - \mathfrak{p} (163 + 15 \mathfrak{z} + 5 \mathfrak{z}^2) + \\
& \quad \eta \mathfrak{t} (85 + \mathfrak{z} + \mathfrak{p} (163 + 15 \mathfrak{z} + 5 \mathfrak{z}^2))) + \\
& \quad 3 \eta^2 (12 \times (18 + \mathfrak{z}) - \mathfrak{p} (174 + 39 \mathfrak{z} - \mathfrak{z} + 20 \mathfrak{p} (2 + \mathfrak{z})^2) + \\
& \quad \eta \mathfrak{t} (-58 + 16 \mathfrak{z} + \mathfrak{p} (174 + 39 \mathfrak{z} - \mathfrak{z} + 20 \mathfrak{p} (2 + \mathfrak{z})^2))) + \\
& \quad \eta (\mathfrak{p} (94 - 81 \mathfrak{z} + 87 \mathfrak{z} + 20 \mathfrak{z}^2 - 48 \mathfrak{p} (2 + \mathfrak{z})^2) + \eta \mathfrak{t} (16 - \\
& \quad 20 \mathfrak{z} + \mathfrak{p} (-94 + 81 \mathfrak{z} - 87 \mathfrak{z} - 20 \mathfrak{z}^2 + 48 \mathfrak{p} (2 + \mathfrak{z})^2)))) + \\
& w^4 (-1 + \eta)^4 (-12 \eta^3 (1 + 3 \eta + \eta^2) \times (-1 + \eta \mathfrak{t}) \mathfrak{p} (2 + \mathfrak{z}) \times \\
& \quad (-2 + \mathfrak{p} (2 + \mathfrak{z})) + 2 x^5 (-1 + \eta)^5 (6 \times (-1 + \eta) \mathfrak{p} \\
& \quad (-54 + 10 \eta^2 + \eta \mathfrak{t} (-15 + \mathfrak{z}) - 5 \mathfrak{z} - \eta (-15 + 10 \eta \mathfrak{t} + \mathfrak{z})) + (-1 + \eta \mathfrak{t}) \\
& \quad \mathfrak{p} (-68 + 20 \mathfrak{z} + 6 \mathfrak{p}^2 (2 + \mathfrak{z})^2 + \mathfrak{p} (368 + 54 \mathfrak{z} + 50 \mathfrak{z} + 5 \mathfrak{z}^2)))) -
\end{aligned}$$

$$\begin{aligned}
& x^4 (-1 + \eta)^4 \left( 4 \times (-1 + \eta) \, \text{op} \left( -148 + 120 \eta^3 - 45 \eta t - 8 \, \mathfrak{z}2 + 12 \eta t \, \mathfrak{z}2 + \right. \right. \\
& \quad \left. \left. 6 \eta \eta t \left( -35 + 2 \, \mathfrak{z}2 \right) - 6 \eta^2 \left( -35 + 20 \eta t + 2 \, \mathfrak{z}2 \right) - 9 \eta \left( 67 + 7 \, \mathfrak{z}2 \right) \right) + \right. \\
& \quad \left( -1 + \eta t \right) \, \text{ol} \left( -144 + 60 \, \mathfrak{z}2 + 36 \, \text{op}^2 \left( 2 + \, \mathfrak{z}2 \right)^2 + 60 \eta \, \text{op}^2 \left( 2 + \, \mathfrak{z}2 \right)^2 + \right. \\
& \quad \left. 6 \eta \left( -61 + 20 \, \mathfrak{z}2 \right) + 2 \, \text{op} \left( 296 + 54 \, \mathfrak{z}1 + 6 \, \mathfrak{z}2 - 5 \, \mathfrak{z}2^2 \right) + \right. \\
& \quad \left. \left. \eta \, \text{op} \left( 2718 + 405 \, \mathfrak{z}1 + 353 \, \mathfrak{z}2 + 40 \, \mathfrak{z}2^2 \right) \right) \right) + 3 x^3 (-1 + \eta)^3 \\
& \quad \left( 240 \eta^5 \, \text{op} + 12 \eta^3 \, \text{op} \left( -133 + 2 \eta t \left( -10 + \, \mathfrak{z}2 \right) - 9 \, \mathfrak{z}2 \right) - 24 \eta^4 \, \text{op} \left( -10 + \right. \right. \\
& \quad \left. \left. 10 \eta t + \, \mathfrak{z}2 \right) + 2 \eta \left( 2 \, \text{op} \left( 148 + \eta t \left( 29 - 7 \, \mathfrak{z}2 \right) + 8 \, \mathfrak{z}2 \right) + \left( -1 + \eta t \right) \, \text{ol} \right. \right. \\
& \quad \left. \left. \left( -41 + 20 \, \mathfrak{z}2 + 24 \, \text{op}^2 \left( 2 + \, \mathfrak{z}2 \right)^2 + \, \text{op} \left( 272 + 54 \, \mathfrak{z}1 - 6 \, \mathfrak{z}2 - 5 \, \mathfrak{z}2^2 \right) \right) \right) \right) + \\
& \quad \eta^2 \left( 2 \, \text{op} \left( 262 + 50 \, \mathfrak{z}2 + \eta t \left( 151 + 12 \, \mathfrak{z}2 \right) \right) + \left( -1 + \eta t \right) \, \text{ol} \left( -96 + 189 \right. \right. \\
& \quad \left. \left. \, \text{op} \, \mathfrak{z}1 + 40 \, \mathfrak{z}2 + 40 \, \text{op}^2 \left( 2 + \, \mathfrak{z}2 \right)^2 + 5 \, \text{op} \left( 246 + 29 \, \mathfrak{z}2 + 4 \, \mathfrak{z}2^2 \right) \right) \right) + \\
& \quad 2 \, \text{op} \left( -2 \, \text{ol} \left( 2 + \, \mathfrak{z}2 \right) \times \left( -2 + \, \text{op} \left( 2 + \, \mathfrak{z}2 \right) \right) + \eta t \left( 31 - 10 \, \mathfrak{z}2 + \right. \right. \\
& \quad \left. \left. 2 \, \text{ol} \left( 2 + \, \mathfrak{z}2 \right) \times \left( -2 + \, \text{op} \left( 2 + \, \mathfrak{z}2 \right) \right) \right) \right) - x^2 \\
& \quad \left( -1 + \eta \right)^2 \eta \left( 480 \eta^5 \, \text{op} - 24 \eta^4 \, \text{op} \left( -25 + 20 \eta t + 2 \, \mathfrak{z}2 \right) + \right. \\
& \quad \left. 12 \eta^3 \, \text{op} \left( -261 - 19 \, \mathfrak{z}2 + \eta t \left( -50 + 4 \, \mathfrak{z}2 \right) \right) + \right. \\
& \quad \left. 6 \eta \left( \, \text{op} \left( 296 + 21 \eta t + 16 \, \mathfrak{z}2 - 4 \eta t \, \mathfrak{z}2 \right) + \left( -1 + \eta t \right) \, \text{ol} \left( -11 + 10 \, \mathfrak{z}2 + \right. \right. \right. \\
& \quad \left. \left. \left. 36 \, \text{op}^2 \left( 2 + \, \mathfrak{z}2 \right)^2 + \, \text{op} \left( 224 + 54 \, \mathfrak{z}1 - 30 \, \mathfrak{z}2 - 5 \, \mathfrak{z}2^2 \right) \right) \right) \right) + \\
& \quad \eta^2 \left( 12 \, \text{op} \left( 23 + 15 \, \mathfrak{z}2 + \eta t \left( 49 + 8 \, \mathfrak{z}2 \right) \right) + \left( -1 + \eta t \right) \, \text{ol} \left( -58 + 40 \, \mathfrak{z}2 + \right. \right. \\
& \quad \left. \left. 120 \, \text{op}^2 \left( 2 + \, \mathfrak{z}2 \right)^2 + \, \text{op} \left( 2122 + 351 \, \mathfrak{z}1 + 187 \, \mathfrak{z}2 + 40 \, \mathfrak{z}2^2 \right) \right) \right) + \\
& \quad 6 \, \text{op} \left( -6 \, \text{ol} \left( 2 + \, \mathfrak{z}2 \right) \times \left( -2 + \, \text{op} \left( 2 + \, \mathfrak{z}2 \right) \right) + \eta t \left( 61 - 20 \, \mathfrak{z}2 + \right. \right. \\
& \quad \left. \left. 6 \, \text{ol} \left( 2 + \, \mathfrak{z}2 \right) \times \left( -2 + \, \text{op} \left( 2 + \, \mathfrak{z}2 \right) \right) \right) \right) + x \\
& \quad \left( -1 + \eta \right) \eta^2 \, \text{op} \left( 120 \eta^5 + 12 \eta^3 \left( -64 + \eta t \left( -15 + \, \mathfrak{z}2 \right) - 5 \, \mathfrak{z}2 \right) - \right. \\
& \quad \left. 12 \eta^4 \left( -15 + 10 \eta t + \, \mathfrak{z}2 \right) + \eta^2 \left( -124 + 40 \, \mathfrak{z}2 + 18 \eta t \left( 9 + 2 \, \mathfrak{z}2 \right) - \right. \right. \\
& \quad \left. \left. \, \text{ol} \left( 366 + 81 \, \mathfrak{z}1 - 19 \, \mathfrak{z}2 + 10 \, \mathfrak{z}2^2 + 60 \, \text{op} \left( 2 + \, \mathfrak{z}2 \right)^2 \right) + \right. \right. \\
& \quad \left. \left. \eta t \, \text{ol} \left( 366 + 81 \, \mathfrak{z}1 - 19 \, \mathfrak{z}2 + 10 \, \mathfrak{z}2^2 + 60 \, \text{op} \left( 2 + \, \mathfrak{z}2 \right)^2 \right) \right) \right) + \\
& \quad 12 \times \left( -3 \, \text{ol} \left( 2 + \, \mathfrak{z}2 \right) \times \left( -2 + \, \text{op} \left( 2 + \, \mathfrak{z}2 \right) \right) + \eta t \left( 12 - 5 \, \mathfrak{z}2 + \right. \right. \\
& \quad \left. \left. 3 \, \text{ol} \left( 2 + \, \mathfrak{z}2 \right) \times \left( -2 + \, \text{op} \left( 2 + \, \mathfrak{z}2 \right) \right) \right) \right) + 2 \eta \left( 8 \times \left( 37 + 2 \, \mathfrak{z}2 \right) - \right. \\
& \quad \left. \, \text{ol} \left( 80 + 54 \, \mathfrak{z}1 - 102 \, \mathfrak{z}2 - 5 \, \mathfrak{z}2^2 + 72 \, \text{op} \left( 2 + \, \mathfrak{z}2 \right)^2 \right) + \eta t \right. \\
& \quad \left. \left( -3 + 6 \, \mathfrak{z}2 + \, \text{ol} \left( 80 + 54 \, \mathfrak{z}1 - 102 \, \mathfrak{z}2 - 5 \, \mathfrak{z}2^2 + 72 \, \text{op} \left( 2 + \, \mathfrak{z}2 \right)^2 \right) \right) \right) \right) + \\
& w^3 (-1 + \eta)^3 \left( 4 \eta^3 \left( 1 + 9 \eta + 9 \eta^2 + \eta^3 \right) \times \left( -1 + \eta t \right) \, \text{ol} \, \text{op} \left( 2 + \, \mathfrak{z}2 \right) \times \right. \\
& \quad \left. \left( -2 + \, \text{op} \left( 2 + \, \mathfrak{z}2 \right) \right) + 4 x^6 (-1 + \eta)^6 \left( 3 \times (-1 + \eta) \, \text{op} \right. \right. \\
& \quad \left. \left( -54 + 10 \eta^2 + \eta t \left( -15 + \, \mathfrak{z}2 \right) - 5 \, \mathfrak{z}2 - \eta \left( -15 + 10 \eta t + \, \mathfrak{z}2 \right) \right) + \left( -1 + \eta t \right) \right. \\
& \quad \left. \, \text{ol} \left( 5 \times \left( -2 + \, \mathfrak{z}2 \right) + \, \text{op}^2 \left( 2 + \, \mathfrak{z}2 \right)^2 + \, \text{op} \left( 168 + 12 \, \mathfrak{z}1 + 22 \, \mathfrak{z}2 + 5 \, \mathfrak{z}2^2 \right) \right) \right) \right) + \\
& x^4 (-1 + \eta)^4 \left( 4 \times (-1 + \eta) \, \text{op} \left( 300 \eta^4 + 6 \eta^2 \left( -175 + 5 \eta t \left( -27 + \, \mathfrak{z}2 \right) - \right. \right. \right. \\
& \quad \left. \left. \left. 31 \, \mathfrak{z}2 \right) - 3 \times \left( 18 + \, \mathfrak{z}2 \right) - 30 \eta^3 \left( -27 + 10 \eta t + \, \mathfrak{z}2 \right) + \right. \right. \\
& \quad \left. \left. \eta t \left( -100 + 31 \, \mathfrak{z}2 \right) + \eta \left( -1786 - 181 \eta t - 98 \, \mathfrak{z}2 + 44 \eta t \, \mathfrak{z}2 \right) \right) \right) + \\
& \quad \left( -1 + \eta t \right) \, \text{ol} \left( \eta \left( 180 \, \text{op}^2 \left( 2 + \, \mathfrak{z}2 \right)^2 + 18 \times \left( -61 + 20 \, \mathfrak{z}2 \right) + \right. \right. \\
& \quad \left. \left. \, \text{op} \left( 7922 + 1215 \, \mathfrak{z}1 + 779 \, \mathfrak{z}2 \right) \right) + 4 \times \left( -36 + 15 \, \mathfrak{z}2 + 9 \, \text{op}^2 \right. \right. \\
& \quad \left. \left. \left( 2 + \, \mathfrak{z}2 \right)^2 + \, \text{op} \left( 54 + 27 \, \mathfrak{z}1 - 5 \, \mathfrak{z}2 - 5 \, \mathfrak{z}2^2 \right) \right) + 2 \eta^2 \left( -132 + 60 \, \mathfrak{z}2 + \right. \right. \\
& \quad \left. \left. 30 \, \text{op}^2 \left( 2 + \, \mathfrak{z}2 \right)^2 + \, \text{op} \left( 2474 + 231 \, \mathfrak{z}1 + 403 \, \mathfrak{z}2 + 100 \, \mathfrak{z}2^2 \right) \right) \right) \right) - \\
& x^5 (-1 + \eta)^5 \left( 2 \times (-1 + \eta) \, \text{op} \left( -888 + 300 \eta^3 - 75 \eta t + 6 \eta \right. \right. \\
& \quad \left. \left( -225 + 5 \eta t \left( -21 + \, \mathfrak{z}2 \right) - 28 \, \mathfrak{z}2 \right) - 48 \, \mathfrak{z}2 + 22 \eta t \, \mathfrak{z}2 - \right. \\
& \quad \left. 30 \eta^2 \left( -21 + 10 \eta t + \, \mathfrak{z}2 \right) \right) + \left( -1 + \eta t \right) \, \text{ol} \left( 12 \times \left( -34 + 10 \, \mathfrak{z}2 + \right. \right. \\
& \quad \left. \left. 3 \, \text{op}^2 \left( 2 + \, \mathfrak{z}2 \right)^2 + \, \text{op} \left( 170 + 27 \, \mathfrak{z}1 + 19 \, \mathfrak{z}2 \right) \right) + \eta \left( 24 \, \text{op}^2 \left( 2 + \, \mathfrak{z}2 \right)^2 + \right. \right.
\end{aligned}$$

$$\begin{aligned}
& 20 \times (-9 + 4 \mathfrak{z}2) + \mathfrak{e}p \left( 2934 + 237 \mathfrak{z}1 + 425 \mathfrak{z}2 + 100 \mathfrak{z}2^2 \right) \Big) \Big) - x^3 \\
& (-1 + \eta)^3 \left( 1200 \eta^6 \mathfrak{e}p + 24 \eta^4 \mathfrak{e}p (-285 + 5 \eta \mathfrak{t} (-23 + \mathfrak{z}2) - 29 \mathfrak{z}2) - \right. \\
& 120 \eta^5 \mathfrak{e}p (-23 + 10 \eta \mathfrak{t} + \mathfrak{z}2) + \\
& 3 \eta^2 \left( 2 \mathfrak{e}p (1688 + 94 \mathfrak{z}2 + 9 \eta \mathfrak{t} (1 + 2 \mathfrak{z}2)) + (-1 + \eta \mathfrak{t}) \mathfrak{e}l \left( 120 \mathfrak{e}p^2 \right. \right. \\
& \quad \left. \left. (2 + \mathfrak{z}2)^2 + 24 \times (-12 + 5 \mathfrak{z}2) + \mathfrak{e}p (3794 + 567 \mathfrak{z}1 + 299 \mathfrak{z}2) \right) \right) \Big) + \\
& 6 \eta \left( 2 \mathfrak{e}p (54 + 83 \eta \mathfrak{t} + 3 \mathfrak{z}2 - 26 \eta \mathfrak{t} \mathfrak{z}2) + (-1 + \eta \mathfrak{t}) \mathfrak{e}l \left( -41 + \right. \right. \\
& \quad \left. \left. 20 \mathfrak{z}2 + 24 \mathfrak{e}p^2 (2 + \mathfrak{z}2)^2 + 2 \mathfrak{e}p (42 + 27 \mathfrak{z}1 - 11 \mathfrak{z}2 - 5 \mathfrak{z}2^2) \right) \right) \Big) + \\
& 4 \eta^3 \left( 3 \mathfrak{e}p (-658 + 18 \mathfrak{z}2 + \eta \mathfrak{t} (227 + 12 \mathfrak{z}2)) + (-1 + \eta \mathfrak{t}) \mathfrak{e}l \left( -37 + \right. \right. \\
& \quad \left. \left. 20 \mathfrak{z}2 + 20 \mathfrak{e}p^2 (2 + \mathfrak{z}2)^2 + \mathfrak{e}p (986 + 111 \mathfrak{z}1 + 185 \mathfrak{z}2 + 50 \mathfrak{z}2^2) \right) \right) \Big) + \\
& 2 \mathfrak{e}p (-2 \mathfrak{e}l (2 + \mathfrak{z}2) \times (-2 + \mathfrak{e}p (2 + \mathfrak{z}2)) + \eta \mathfrak{t} (93 - 30 \mathfrak{z}2 + \\
& \quad 2 \mathfrak{e}l (2 + \mathfrak{z}2) \times (-2 + \mathfrak{e}p (2 + \mathfrak{z}2)))) \Big) + x^2 (-1 + \eta)^2 \\
& \eta \left( 600 \eta^6 \mathfrak{e}p + 12 \eta^4 \mathfrak{e}p (-255 + 5 \eta \mathfrak{t} (-29 + \mathfrak{z}2) - 32 \mathfrak{z}2) - \right. \\
& 60 \eta^5 \mathfrak{e}p (-29 + 10 \eta \mathfrak{t} + \mathfrak{z}2) + \\
& \eta^2 \left( 4 \mathfrak{e}p (1644 + 93 \mathfrak{z}2 + \eta \mathfrak{t} (-39 + 49 \mathfrak{z}2)) + 3 \times (-1 + \eta \mathfrak{t}) \mathfrak{e}l \right. \\
& \quad \left. (-58 + 40 \mathfrak{z}2 + 120 \mathfrak{e}p^2 (2 + \mathfrak{z}2)^2 + \mathfrak{e}p (2338 + 351 \mathfrak{z}1 + 99 \mathfrak{z}2)) \right) \Big) + \\
& 6 \eta \left( \mathfrak{e}p (\eta \mathfrak{t} (115 - 42 \mathfrak{z}2) + 6 \times (18 + \mathfrak{z}2)) + (-1 + \eta \mathfrak{t}) \mathfrak{e}l \left( -11 + \right. \right. \\
& \quad \left. \left. 10 \mathfrak{z}2 + 36 \mathfrak{e}p^2 (2 + \mathfrak{z}2)^2 + 2 \mathfrak{e}p (18 + 27 \mathfrak{z}1 - 23 \mathfrak{z}2 - 5 \mathfrak{z}2^2) \right) \right) \Big) + \\
& 2 \eta^3 \left( 2 \mathfrak{e}p (-1626 + 9 \mathfrak{z}2 + \eta \mathfrak{t} (360 + 29 \mathfrak{z}2)) + (-1 + \eta \mathfrak{t}) \mathfrak{e}l \right. \\
& \quad \left. (30 \mathfrak{e}p^2 (2 + \mathfrak{z}2)^2 + 2 \times (-6 + 5 \mathfrak{z}2) + \mathfrak{e}p (702 + 105 \mathfrak{z}1 + 157 \mathfrak{z}2 + \right. \\
& \quad \left. 50 \mathfrak{z}2^2)) \right) \Big) + 6 \mathfrak{e}p (-2 \mathfrak{e}l (2 + \mathfrak{z}2) \times (-2 + \mathfrak{e}p (2 + \mathfrak{z}2)) + \\
& \quad \eta \mathfrak{t} (61 - 20 \mathfrak{z}2 + 2 \mathfrak{e}l (2 + \mathfrak{z}2) \times (-2 + \mathfrak{e}p (2 + \mathfrak{z}2)))) \Big) - x \\
& (-1 + \eta) \eta^2 \mathfrak{e}p \left( 120 \eta^6 + 12 \eta^4 (-44 + \eta \mathfrak{t} (-35 + \mathfrak{z}2) - 7 \mathfrak{z}2) - \right. \\
& 12 \eta^5 (-35 + 10 \eta \mathfrak{t} + \mathfrak{z}2) + 12 (-\mathfrak{e}l (2 + \mathfrak{z}2) \times (-2 + \mathfrak{e}p (2 + \mathfrak{z}2)) + \\
& \quad \eta \mathfrak{t} (12 - 5 \mathfrak{z}2 + \mathfrak{e}l (2 + \mathfrak{z}2) \times (-2 + \mathfrak{e}p (2 + \mathfrak{z}2)))) \Big) + \\
& \eta^3 \left( -4 \times (457 + 2 \mathfrak{z}2) - \mathfrak{e}l (130 + 39 \mathfrak{z}1 + 35 \mathfrak{z}2 + 20 \mathfrak{z}2^2 + \right. \\
& \quad 24 \mathfrak{e}p (2 + \mathfrak{z}2)^2) + \eta \mathfrak{t} (302 + 32 \mathfrak{z}2 + \\
& \quad \mathfrak{e}l (130 + 39 \mathfrak{z}1 + 35 \mathfrak{z}2 + 20 \mathfrak{z}2^2 + 24 \mathfrak{e}p (2 + \mathfrak{z}2)^2)) \Big) \Big) + \\
& 2 \eta \left( 6 \times (18 + \mathfrak{z}2) + 2 \mathfrak{e}l (54 - 27 \mathfrak{z}1 + 59 \mathfrak{z}2 + 5 \mathfrak{z}2^2 - 36 \mathfrak{e}p (2 + \mathfrak{z}2)^2) + \right. \\
& \quad \eta \mathfrak{t} (65 - 32 \mathfrak{z}2 + 2 \mathfrak{e}l (-54 + 27 \mathfrak{z}1 - 59 \mathfrak{z}2 - 5 \mathfrak{z}2^2 + \\
& \quad 36 \mathfrak{e}p (2 + \mathfrak{z}2)^2)) \Big) \Big) + \eta^2 \left( 1600 + 92 \mathfrak{z}2 - \right. \\
& \quad \mathfrak{e}l (1370 + 243 \mathfrak{z}1 - 121 \mathfrak{z}2 + 180 \mathfrak{e}p (2 + \mathfrak{z}2)^2) + \eta \mathfrak{t} (-36 + \\
& \quad 80 \mathfrak{z}2 + \mathfrak{e}l (1370 + 243 \mathfrak{z}1 - 121 \mathfrak{z}2 + 180 \mathfrak{e}p (2 + \mathfrak{z}2)^2)) \Big) \Big) \Big) \Big) - \\
& 2 \mathfrak{c}\sigma^2 (x (-1 + \eta) - \eta) (w (-1 + \eta) + x (-1 + \eta) - \eta) \\
& (-1 + \\
& \eta) \times (2 \\
& x^7 \\
& (-1 + \eta)^7 \\
& \mathfrak{e}p \\
& (2 - 2 \mathfrak{e}l - 9 \mu 1 - 15 w \mu 1 - 4 w^2 \mu 1 + 5 \mathfrak{e}l \mu 1 + \\
& 7 w \mathfrak{e}l \mu 1 - 5 \mu 1^2 - 9 w \mu 1^2 - 4 w^2 \mu 1^2 + \\
& \mathfrak{e}l \mu 1^2 + w \mathfrak{e}l \mu 1^2 + w^2 \eta^4 (1 + \mu 1) - \\
& w \eta^3 (3 + w (3 + \eta \mathfrak{t} - 4 \mu 1)) \times (1 + \mu 1) + \\
& \eta^2 (2 \times (1 + \mu 1) + 3 w^2 (1 + \eta \mathfrak{t} - 4 \mu 1) \times \\
& \quad (1 + \mu 1) + 3 w (2 + \eta \mathfrak{t} - 3 \mu 1 + \eta \mathfrak{t} \mu 1 - 3 \mu 1^2)) \Big) +
\end{aligned}$$

$$\begin{aligned}
& \eta t \left( 2 \times (1 + \mu_1) + w^2 (1 + \mu_1) - \theta l (-2 + 5 \mu_1 + \mu_1^2) + w \right. \\
& \quad \left. (3 + (3 - 7 \theta l) \mu_1 - \theta l \mu_1^2) \right) - \\
& \eta \left( 4 + 2 \eta t - 7 \mu_1 + 2 \eta t \mu_1 - 5 \mu_1^2 + w^2 (1 + 3 \eta t - 12 \mu_1) \times (1 + \mu_1) + w \right. \\
& \quad \left. (3 + (-27 + 7 \theta l) \mu_1 + (-18 + \theta l) \mu_1^2 + \eta t (6 + (6 - 7 \theta l) \mu_1 - \theta l \mu_1^2)) \right) + \\
& 4 \times (-1 + w (-1 + \eta)) \eta (1 + \eta)^2 \theta p \left( \eta \left( \eta t \theta p (4 + 4 \mu_1^2 + 6 \mu_2 + 9 \mu_2^2 + \right. \right. \\
& \quad \left. \mu_1 (8 + 6 \mu_2)) - \eta^3 (-((-1 + \eta t) \theta l \mu_1 (1 + \mu_1 + 6 \mu_2)) + \right. \\
& \quad \left. \theta p (5 + 5 \mu_1^2 + 12 \mu_2 + 18 \mu_2^2 + 2 \mu_1 (5 + 6 \mu_2)) \right) + \eta^2 \\
& \quad \left( (-1 + \eta t) \theta l (5 + 3 \mu_1^2 + 6 \mu_2 + 4 \mu_1 (2 + 3 \mu_2)) + \right. \\
& \quad \left. \theta p (5 + 5 \mu_1^2 + 12 \mu_2 + 18 \mu_2^2 + 2 \mu_1 (5 + 6 \mu_2)) \right) + \eta \\
& \quad \left. (-\eta t \theta p (4 + 4 \mu_1^2 + 6 \mu_2 + 9 \mu_2^2 + \mu_1 (8 + 6 \mu_2)) + \right. \\
& \quad \left. (-1 + \eta t) \theta l (4 + 4 \mu_1^2 + 11 \mu_2 + 9 \mu_2^2 + \mu_1 (8 + 11 \mu_2)) \right) + \\
& w (-1 + \eta) \left( \eta^4 \theta p (5 + 5 \mu_1^2 + 12 \mu_2 + 18 \mu_2^2 + 2 \mu_1 (5 + 6 \mu_2)) - \eta t \right. \\
& \quad \left. \theta p (4 + 4 \mu_1^2 + 6 \mu_2 + 9 \mu_2^2 + \mu_1 (8 + 6 \mu_2)) + \eta^3 \right. \\
& \quad \left. (-((-1 + \eta t) \theta l (5 + 7 \mu_1^2 + 6 \mu_2 + 12 \mu_1 (1 + 3 \mu_2)) + \right. \\
& \quad \left. \theta p (5 + 5 \mu_1^2 + 12 \mu_2 + 18 \mu_2^2 + 2 \mu_1 (5 + 6 \mu_2)) \right) - \eta \left( (-1 + \eta t) \theta l \right. \\
& \quad \left. (2 + 2 \mu_1 + 3 \mu_2)^2 + \eta t \theta p (4 + 4 \mu_1^2 + 6 \mu_2 + 9 \mu_2^2 + \mu_1 (8 + 6 \mu_2)) \right) - 2 \\
& \quad \eta^2 \left( (-1 + \eta t) \theta l (9 + 7 \mu_1^2 + 17 \mu_2 + 9 \mu_2^2 + \mu_1 (16 + 23 \mu_2)) + \right. \\
& \quad \left. \theta p (5 + 5 \mu_1^2 + 12 \mu_2 + 18 \mu_2^2 + 2 \mu_1 (5 + 6 \mu_2) - \right. \\
& \quad \left. \eta t (4 + 4 \mu_1^2 + 6 \mu_2 + 9 \mu_2^2 + \mu_1 (8 + 6 \mu_2)) \right) + \\
& w^3 (-1 + \eta)^3 \left( \eta^2 \theta p (5 + 5 \mu_1^2 + 12 \mu_2 + 18 \mu_2^2 + 2 \mu_1 (5 + 6 \mu_2)) - \eta t \right. \\
& \quad \left. \theta p (4 + 4 \mu_1^2 + 6 \mu_2 + 9 \mu_2^2 + \mu_1 (8 + 6 \mu_2)) + \eta \right. \\
& \quad \left. (-9 \times (-1 + \eta t) \theta l (\mu_1^2 + (1 + \mu_2)^2 + \mu_1 (2 + 4 \mu_2)) + \right. \\
& \quad \left. \theta p (-5 - 5 \mu_1^2 - 12 \mu_2 - 18 \mu_2^2 - 2 \mu_1 (5 + 6 \mu_2) + \right. \\
& \quad \left. \eta t (4 + 4 \mu_1^2 + 6 \mu_2 + 9 \mu_2^2 + \mu_1 (8 + 6 \mu_2)) \right) - \\
& w^2 (-1 + \eta)^2 \left( 2 \eta^3 \theta p (5 + 5 \mu_1^2 + 12 \mu_2 + 18 \mu_2^2 + 2 \mu_1 (5 + 6 \mu_2)) - 2 \right. \\
& \quad \left. \eta t \theta p (4 + 4 \mu_1^2 + 6 \mu_2 + 9 \mu_2^2 + \mu_1 (8 + 6 \mu_2)) + \eta \right. \\
& \quad \left. (-((-1 + \eta t) \theta l (13 + 11 \mu_1^2 + 30 \mu_2 + 18 \mu_2^2 + 12 \mu_1 (2 + 3 \mu_2)) + \right. \\
& \quad \left. \theta p (-5 - 5 \mu_1^2 - 12 \mu_2 - 18 \mu_2^2 - 2 \mu_1 (5 + 6 \mu_2) + \right. \\
& \quad \left. \eta t (4 + 4 \mu_1^2 + 6 \mu_2 + 9 \mu_2^2 + \mu_1 (8 + 6 \mu_2)) \right) + \eta^2 \\
& \quad \left. (-((-1 + \eta t) \theta l (14 + 15 \mu_1^2 + 23 \mu_2 + 9 \mu_2^2 + \mu_1 (29 + 65 \mu_2)) + \right. \\
& \quad \left. \theta p (-5 - 5 \mu_1^2 - 12 \mu_2 - 18 \mu_2^2 - 2 \mu_1 (5 + 6 \mu_2) + \right. \\
& \quad \left. \eta t (4 + 4 \mu_1^2 + 6 \mu_2 + 9 \mu_2^2 + \mu_1 (8 + 6 \mu_2)) \right) + \\
& x^5 (-1 + \eta)^5 \left( 2 \times (-1 + \eta) \theta p (13 + 7 \eta - 10 \eta^2 + 30 \eta^3 - 2 \eta t - 20 \eta \eta t - 30 \right. \\
& \quad \eta^2 \eta t - 20 \theta p - 60 \eta \theta p + 21 \mu_1 + 112 \eta \mu_1 + 155 \eta^2 \mu_1 + 30 \eta^3 \\
& \quad \mu_1 - 10 \eta t \mu_1 - 18 \eta \eta t \mu_1 - 30 \eta^2 \eta t \mu_1 - 40 \theta p \mu_1 - 120 \eta \theta p \\
& \quad \mu_1 + 2 \mu_1^2 + 45 \eta \mu_1^2 + 75 \eta^2 \mu_1^2 + 4 \eta t \mu_1^2 + 2 \eta \eta t \mu_1^2 - 20 \theta p \\
& \quad \mu_1^2 - 60 \eta \theta p \mu_1^2 + w^4 (-1 + \eta)^4 (1 + \mu_1) (\eta - \eta t + 4 \mu_1) + 19 \\
& \quad \mu_2 + 47 \eta \mu_2 - 2 \eta t \mu_2 - 48 \theta p \mu_2 - 144 \eta \theta p \mu_2 + \mu_1 \mu_2 - 7 \\
& \quad \eta \mu_1 \mu_2 - 60 \eta^2 \mu_1 \mu_2 + 16 \eta t \mu_1 \mu_2 + 30 \eta \eta t \mu_1 \mu_2 - 48 \\
& \quad \theta p \mu_1 \mu_2 - 144 \eta \theta p \mu_1 \mu_2 - 72 \theta p \mu_2^2 - 216 \eta \theta p \mu_2^2 - w^3 \\
& \quad (-1 + \eta)^3 (10 - 20 \theta p + 39 \mu_1 - 40 \theta p \mu_1 + 23 \mu_1^2 - 20 \theta p \mu_1^2 + \\
& \quad 10 \eta^2 (1 + \mu_1) + 22 \mu_2 - 48 \theta p \mu_2 - 14 \mu_1 \mu_2 - 48 \theta p \mu_1 \mu_2 - \\
& \quad \left. 72 \theta p \mu_2^2 + \eta (7 + 47 \mu_1 + 40 \mu_1^2 - 10 \eta t (1 + \mu_1) - 12 \mu_1 \mu_2) + \right.
\end{aligned}$$

$$\begin{aligned}
& \eta t (-7 - 7 \mu_1 + 12 \mu_1 \mu_2) - w (-1 + \eta) \times (32 - 11 \eta t - 60 \theta p + \\
& 83 \mu_1 - 27 \eta t \mu_1 - 120 \theta p \mu_1 + 21 \mu_1^2 + 8 \eta t \mu_1^2 - 60 \theta p \mu_1^2 + \\
& 45 \eta^3 (1 + \mu_1) + 5 \eta^2 (10 + 27 \mu_1^2 - 9 \eta t (1 + \mu_1) + \mu_1 (55 - 18 \mu_2)) + \\
& 62 \mu_2 - 4 \eta t \mu_2 - 144 \theta p \mu_2 - 22 \mu_1 \mu_2 + 44 \eta t \mu_1 \mu_2 - \\
& 144 \theta p \mu_1 \mu_2 - 216 \theta p \mu_2^2 + \eta (41 + 291 \mu_1 + 130 \mu_1^2 + \\
& 102 \mu_2 - 72 \mu_1 \mu_2 + 2 \eta t (-25 + \mu_1^2 + 6 \mu_1 (-4 + 5 \mu_2)) - \\
& 24 \theta p (5 + 5 \mu_1^2 + 12 \mu_2 + 18 \mu_2^2 + 2 \mu_1 (5 + 6 \mu_2))) + w^2 \\
& (-1 + \eta)^2 (33 - 15 \eta t - 60 \theta p + 101 \mu_1 - 23 \eta t \mu_1 - 120 \theta p \mu_1 + \\
& 38 \mu_1^2 + 4 \eta t \mu_1^2 - 60 \theta p \mu_1^2 + 15 \eta^3 (1 + \mu_1) - \\
& 5 \eta^2 (3 \eta t (1 + \mu_1) - 2 \times (4 + 6 \mu_1^2 + \mu_1 (10 - 3 \mu_2))) + 65 \mu_2 - 2 \eta t \mu_2 - \\
& 144 \theta p \mu_2 - 37 \mu_1 \mu_2 + 40 \eta t \mu_1 \mu_2 - 144 \theta p \mu_1 \mu_2 - 216 \theta p \mu_2^2 - \\
& \eta (-40 - 225 \mu_1 - 125 \mu_1^2 + \eta t (40 + \mu_1 (40 - 30 \mu_2)) - 55 \mu_2 + \\
& 77 \mu_1 \mu_2 + 12 \theta p (5 + 5 \mu_1^2 + 12 \mu_2 + 18 \mu_2^2 + 2 \mu_1 (5 + 6 \mu_2))) - \\
& (-1 + \eta t) \theta l (20 - 34 \theta p - 110 \eta \theta p - 60 \eta^2 \theta p + 52 \mu_1 + 80 \eta \mu_1 - 16 \\
& \eta^2 \mu_1 - 66 \theta p \mu_1 - 108 \eta \theta p \mu_1 + 136 \eta^2 \theta p \mu_1 - 28 \mu_1^2 - 16 \eta \\
& \mu_1^2 - 16 \eta^2 \mu_1^2 - 20 \theta p \mu_1^2 - 58 \eta \theta p \mu_1^2 + 16 \eta^2 \theta p \mu_1^2 + 5 \\
& \mu_2 - 62 \theta p \mu_2 - 112 \eta \theta p \mu_2 + 10 \eta^2 \theta p \mu_2 - 19 \mu_1 \mu_2 - 86 \theta p \\
& \mu_1 \mu_2 - 316 \eta \theta p \mu_1 \mu_2 - 194 \eta^2 \theta p \mu_1 \mu_2 + 5 \theta p \mathfrak{x}1 + 22 \theta p \mu_1 \\
& \mathfrak{x}1 + 46 \eta \theta p \mu_1 \mathfrak{x}1 + 5 \eta^2 \theta p \mu_1 \mathfrak{x}1 + 5 \theta p \mu_1^2 \mathfrak{x}1 + 16 \eta \theta p \mu_1^2 \\
& \mathfrak{x}1 + 5 \eta^2 \theta p \mu_1^2 \mathfrak{x}1 + 5 \theta p \mu_2 \mathfrak{x}1 + 5 \theta p \mu_1 \mu_2 \mathfrak{x}1 - 5 \theta p \mathfrak{x}2 - 14 \theta p \\
& \mu_1 \mathfrak{x}2 - 24 \eta \theta p \mu_1 \mathfrak{x}2 + 5 \eta^2 \theta p \mu_1 \mathfrak{x}2 + 3 \theta p \mu_1^2 \mathfrak{x}2 + 6 \eta \theta p \mu_1^2 \\
& \mathfrak{x}2 + 5 \eta^2 \theta p \mu_1^2 \mathfrak{x}2 - 5 \theta p \mu_2 \mathfrak{x}2 - 17 \theta p \mu_1 \mu_2 \mathfrak{x}2 - 60 \eta \theta p \mu_1 \\
& \mu_2 \mathfrak{x}2 + w^3 (-1 + \eta)^3 (28 \mu_1^2 - 5 \times (4 + \mu_2) + \mu_1 (-52 + 19 \mu_2) + \\
& \theta p (40 \mu_1^2 + 5 \times (8 - \mathfrak{x}1 + \mathfrak{x}2) + \mu_2 (64 - 5 \mathfrak{x}1 + 5 \mathfrak{x}2) + \\
& \mu_1 (80 - 11 \mathfrak{x}1 + 11 \mathfrak{x}2 + \mu_2 (208 - 5 \mathfrak{x}1 + 5 \mathfrak{x}2))) + w^2 (-1 + \eta)^2 \\
& (60 + 156 \mu_1 + 80 \eta \mu_1 - 84 \mu_1^2 - 16 \eta \mu_1^2 + 15 \mu_2 - 57 \mu_1 \mu_2 + \\
& \theta p (\mu_1 (-198 + 44 \mathfrak{x}1 + 3 \mu_2 (-174 + 5 \mathfrak{x}1 - 9 \mathfrak{x}2) - 36 \mathfrak{x}2) + \\
& 3 \times (-38 + 5 \mathfrak{x}1 + \mu_2 (-62 + 5 \mathfrak{x}1 - 5 \mathfrak{x}2) - 5 \mathfrak{x}2) + \\
& \mu_1^2 (-96 + 5 \mathfrak{x}1 + 3 \mathfrak{x}2) + \eta (-70 - 94 \mu_2 + \mu_1^2 (-108 + 15 \mathfrak{x}1 + 5 \mathfrak{x}2) - \\
& \mu_1 (118 + 694 \mu_2 - 45 \mathfrak{x}1 + 25 \mathfrak{x}2 + 60 \mu_2 \mathfrak{x}2))) - w (-1 + \eta) \times \\
& (-4 \times (21 + 8 \eta + 4 \eta^2) \mu_1^2 + \mu_1 (156 + 160 \eta - 16 \eta^2 - 57 \mu_2) + \\
& 15 \times (4 + \mu_2) + \theta p (-116 - 184 \mu_2 + 15 \mathfrak{x}1 + 15 \mu_2 \mathfrak{x}1 + \\
& \mu_1 (-192 + 55 \mathfrak{x}1 + \mu_2 (-400 + 15 \mathfrak{x}1 - 39 \mathfrak{x}2) - 39 \mathfrak{x}2) - \\
& 15 \mathfrak{x}2 - 15 \mu_2 \mathfrak{x}2 + 2 \mu_1^2 (-38 + 5 \mathfrak{x}1 + 3 \mathfrak{x}2) + \\
& \eta^2 (10 \mu_2 + \mu_1^2 (16 + 5 \mathfrak{x}1 + 5 \mathfrak{x}2) + \mu_1 (196 - 194 \mu_2 + 5 \mathfrak{x}1 + 5 \mathfrak{x}2)) + \\
& \eta (-2 \times (90 + 103 \mu_2) + \mu_1^2 (-166 + 31 \mathfrak{x}1 + 11 \mathfrak{x}2) - \\
& \mu_1 (226 + 1010 \mu_2 - 91 \mathfrak{x}1 + 49 \mathfrak{x}2 + 120 \mu_2 \mathfrak{x}2))) + \\
& x^6 (-1 + \eta)^6 (-4 \times (-1 + w (-1 + \eta)) \times (-1 + \eta t) \theta l \mu_1 (5 + w (-1 + \eta) \times \\
& (-5 + \mu_1) - \mu_1 - \eta (1 + \mu_1)) + 4 \times (-1 + \eta) \\
& (1 + w - w \eta)^2 \theta p^2 (5 + 5 \mu_1^2 + 12 \mu_2 + 18 \mu_2^2 + 2 \mu_1 (5 + 6 \mu_2)) + \\
& \theta p (2 - 18 \eta + 40 \eta^2 - 24 \eta^3 - 8 \eta t - 16 \eta \eta t + 24 \eta^2 \eta t + 18 \theta l + 24 \\
& \eta \theta l - 18 \eta t \theta l - 24 \eta \eta t \theta l + 44 \mu_1 + 72 \eta \mu_1 - 92 \eta^2 \mu_1 - 24 \\
& \eta^3 \mu_1 - 8 \eta t \mu_1 - 16 \eta \eta t \mu_1 + 24 \eta^2 \eta t \mu_1 + 14 \theta l \mu_1 - 58 \eta \\
& \theta l \mu_1 - 14 \eta t \theta l \mu_1 + 58 \eta \eta t \theta l \mu_1 + 18 \mu_1^2 + 42 \eta \mu_1^2 - 60
\end{aligned}$$

$$\begin{aligned}
& \eta^2 \mu_1^2 + 8 \theta \mu_1^2 - 10 \eta \theta \mu_1^2 - 8 \eta t \theta \mu_1^2 + 10 \eta \eta t \theta \mu_1^2 + 4 w^3 (-1 + \eta)^4 (1 + \mu_1) (\eta - \eta t + 4 \mu_1) + 18 \mu_2 - 18 \\
& \eta \mu_2 + 18 \theta \mu_2 - 2 \eta \theta \mu_2 - 18 \eta t \theta \mu_2 + 2 \eta \eta t \theta \mu_2 + 6 \\
& \mu_1 \mu_2 - 30 \eta \mu_1 \mu_2 + 24 \eta^2 \mu_1 \mu_2 + 12 \eta t \mu_1 \mu_2 - 12 \eta \eta t \mu_1 \\
& \mu_2 + 42 \theta \mu_1 \mu_2 + 34 \eta \theta \mu_1 \mu_2 - 42 \eta t \theta \mu_1 \mu_2 - 34 \eta \eta t \\
& \theta \mu_1 \mu_2 - 9 \theta \mu_1 \mu_1 - \eta \theta \mu_1 \mu_1 + 9 \eta t \theta \mu_1 \mu_1 + \eta \eta t \\
& \theta \mu_1 \mu_1 - 3 \theta \mu_1^2 \mu_1 - \eta \theta \mu_1^2 \mu_1 + 3 \eta t \theta \mu_1^2 \mu_1 + \eta \eta t \\
& \theta \mu_1^2 \mu_1 + 5 \theta \mu_1 \mu_2 - \eta \theta \mu_1 \mu_2 - 5 \eta t \theta \mu_1 \mu_2 + \eta \eta t \\
& \theta \mu_1 \mu_2 - \theta \mu_1^2 \mu_2 - \eta \theta \mu_1^2 \mu_2 + \eta t \theta \mu_1^2 \mu_2 + \eta \eta t \theta \\
& \mu_1^2 \mu_2 + 12 \theta \mu_1 \mu_2 \mu_2 - 12 \eta t \theta \mu_1 \mu_2 \mu_2 - w^2 (-1 + \eta)^2 \\
& (-10 - 10 \theta - 84 \mu_1 - 14 \theta \mu_1 - 50 \mu_1^2 - 16 \theta \mu_1^2 + \\
& 12 \eta^3 (1 + \mu_1) - 22 \mu_2 - 14 \theta \mu_2 + 14 \mu_1 \mu_2 - 110 \theta \mu_1 \mu_2 + \\
& 4 \eta^2 (1 + 13 \mu_1 + 12 \mu_1^2 - 3 \eta t (1 + \mu_1) - 3 \mu_1 \mu_2) + \\
& 2 \eta (-3 + 10 \mu_1 + \mu_1^2 + 11 \mu_2 - \mu_1 \mu_2 + \eta t (-2 - 2 \mu_1 + 6 \mu_1 \mu_2)) + \\
& 9 \theta \mu_1 \mu_1 + 3 \theta \mu_1^2 \mu_1 - 5 \theta \mu_1 \mu_2 + \theta \mu_1^2 \mu_2 - 12 \theta \mu_1 \mu_2 \mu_2 + \\
& \eta t (16 + 4 \mu_1 (4 - 3 \mu_2) + 2 \theta (5 + 7 \mu_2) - \theta \mu_1^2 (-16 + 3 \mu_1 + \mu_2) + \\
& \theta \mu_1 (14 - 9 \mu_1 + 5 \mu_2 + 2 \mu_2 (55 + 6 \mu_2))) + w (-1 + \eta) \times \\
& (36 \eta^3 (1 + \mu_1) - 4 \eta^2 (4 - 27 \mu_1^2 + 9 \eta t (1 + \mu_1) + \mu_1 (-41 + 9 \mu_2)) + \\
& \eta (-8 + 40 \mu_2 + 2 \theta \mu_2 + \mu_1^2 (-56 + \theta (10 + \mu_1 + \mu_2)) + \\
& \mu_1 (-88 + 28 \mu_2 + \theta (82 - 34 \mu_2 + \mu_1 + \mu_2)) - \\
& \eta t (-8 \mu_1 (2 + 3 \mu_2) + 2 \times (-8 + \theta \mu_2) + \\
& \theta \mu_1^2 (10 + \mu_1 + \mu_2) + \theta \mu_1 (82 - 34 \mu_2 + \mu_1 + \mu_2))) - \\
& 2 \times (6 + 56 \mu_1 + 26 \mu_1^2 + 20 \mu_2 - 4 \mu_1 \mu_2 + \theta (2 \times (7 + 8 \mu_2) - \\
& \mu_1^2 (-12 + 3 \mu_1 + \mu_2) + \mu_1 (14 + 76 \mu_2 - 9 \mu_1 + 5 \mu_2 + 12 \mu_2 \mu_2)) + \\
& \eta t (-10 + 2 \mu_1 (-5 + 6 \mu_2) - 2 \theta (7 + 8 \mu_2) + \theta \mu_1^2 (-12 + 3 \mu_1 + \\
& \mu_2) - \theta \mu_1 (14 - 9 \mu_1 + 5 \mu_2 + 4 \mu_2 (19 + 3 \mu_2)))) + \\
& \times (-1 + \eta) \theta p (w^4 (-1 + \eta)^4 (2 \eta^6 (1 + \mu_1) - 2 \eta^5 (-1 + \eta t - 5 \mu_1 + \eta t \mu_1 - \\
& 4 \mu_1^2 + 6 \mu_1 \mu_2) - 2 \eta^4 (-4 - 7 \mu_1 - 3 \mu_1^2 - 11 \mu_2 + 7 \mu_1 \mu_2 + \eta t \\
& (1 + \mu_1 - 6 \mu_1 \mu_2) + 8 \theta p (5 + 5 \mu_1^2 + 12 \mu_2 + 18 \mu_2^2 + 2 \mu_1 (5 + 6 \mu_2))) + \\
& \eta t (-5 \times (1 + \mu_1) \mu_2 + 4 \theta p (4 + 4 \mu_1^2 + 6 \mu_2 + 9 \mu_2^2 + \mu_1 (8 + 6 \mu_2))) + \\
& \eta^2 (-2 \times (5 + 8 \mu_1 + 3 \mu_1^2 + 11 \mu_2 + 5 \mu_1 \mu_2 - \\
& 8 \theta p (5 + 5 \mu_1^2 + 12 \mu_2 + 18 \mu_2^2 + 2 \mu_1 (5 + 6 \mu_2)) + 4 \theta (23 + 23 \mu_1^2 + \\
& 48 \mu_2 + 18 \mu_2^2 + 2 \mu_1 (23 + 51 \mu_2))) + \eta t (2 + 2 \mu_1 - 24 \mu_1^2 + \\
& 5 \mu_2 - 7 \mu_1 \mu_2 - 4 \theta p (4 + 8 \mu_1 + 4 \mu_1^2 + 6 \mu_2 + 6 \mu_1 \mu_2 + 9 \mu_2^2) + \\
& 8 \theta (23 + 23 \mu_1^2 + 48 \mu_2 + 18 \mu_2^2 + 2 \mu_1 (23 + 51 \mu_2)))) + \eta \\
& (8 \theta p (5 + 5 \mu_1^2 + 12 \mu_2 + 18 \mu_2^2 + 2 \mu_1 (5 + 6 \mu_2)) - 4 \theta \\
& (14 + 14 \mu_1^2 + 30 \mu_2 + 9 \mu_2^2 + \mu_1 (28 + 66 \mu_2)) + \eta t (10 + 20 \mu_1 - 2 \mu_1^2 - \\
& 5 \mu_2 - 5 \mu_1 \mu_2 + 12 \theta p (4 + 8 \mu_1 + 4 \mu_1^2 + 6 \mu_2 + 6 \mu_1 \mu_2 + 9 \mu_2^2) + \\
& 4 \theta (14 + 14 \mu_1^2 + 30 \mu_2 + 9 \mu_2^2 + \mu_1 (28 + 66 \mu_2)))) + \eta^3 \\
& (-2 \times (1 + 5 \mu_1 + 4 \mu_1^2 - 18 \mu_1 \mu_2 + 4 \theta p (5 + 5 \mu_1^2 + 12 \mu_2 + \\
& 18 \mu_2^2 + 2 \mu_1 (5 + 6 \mu_2)) + 2 \theta (32 + 32 \mu_1^2 + 66 \mu_2 + \\
& 27 \mu_2^2 + 2 \mu_1 (32 + 69 \mu_2))) + \eta t (-8 - 18 \mu_1 + 26 \mu_1^2 + 5 \mu_2 + \\
& 5 \mu_1 \mu_2 - 12 \theta p (4 + 8 \mu_1 + 4 \mu_1^2 + 6 \mu_2 + 6 \mu_1 \mu_2 + 9 \mu_2^2) + \\
& 4 \theta (32 + 32 \mu_1^2 + 66 \mu_2 + 27 \mu_2^2 + 2 \mu_1 (32 + 69 \mu_2)))) +
\end{aligned}$$

$$\begin{aligned}
& \eta \left( 4 \eta^7 (1 + \mu_1) - 2 \eta^6 (2 \eta t (1 + \mu_1) + \mu_1 (-11 - 5 \mu_1 + 12 \mu_2)) + \eta t \right. \\
& \quad \left( -2 \mu_1^2 + \mu_1 (8 - 19 \mu_2) + 5 \times (2 + \mu_2) + \right. \\
& \quad \left. 8 \Theta p (4 + 4 \mu_1^2 + 6 \mu_2 + 9 \mu_2^2 + \mu_1 (8 + 6 \mu_2)) \right) - \eta^5 (-2 - 22 \mu_1 - 8 \mu_1^2 - \\
& \quad 22 \mu_2 + 14 \mu_1 \mu_2 + 24 \Theta p (5 + 5 \mu_1^2 + 12 \mu_2 + 18 \mu_2^2 + 2 \mu_1 (5 + 6 \mu_2)) - \\
& \quad \Theta l (2 \times (-2 + \mu_2) + \mu_1^2 (-20 + \mathfrak{E}1 + \mathfrak{E}2) + \mu_1 (-12 - 154 \mu_2 + \mathfrak{E}1 + \mathfrak{E}2)) + \\
& \quad \eta t (-4 \times (-1 + \mu_1^2 + 3 \mu_1 \mu_2) + \Theta l (2 \times (-2 + \mu_2) + \\
& \quad \mu_1^2 (-20 + \mathfrak{E}1 + \mathfrak{E}2) + \mu_1 (-12 - 154 \mu_2 + \mathfrak{E}1 + \mathfrak{E}2))) + \eta \\
& \quad \left( -\Theta l (\mu_1^2 (30 + \mathfrak{E}1 - \mathfrak{E}2) + \mu_1 (72 - 4 \mathfrak{E}1 + \mu_2 (90 - 5 \mathfrak{E}1 - 7 \mathfrak{E}2) + 4 \mathfrak{E}2) + \right. \\
& \quad (1 + \mu_2) \times (42 + 72 \mu_2 - 5 \mathfrak{E}1 + 5 \mathfrak{E}2)) + \eta t (20 + 24 \mu_1 + 4 \mu_1^2 + \\
& \quad 5 \mu_2 - 19 \mu_1 \mu_2 + 16 \Theta p (4 + 8 \mu_1 + 4 \mu_1^2 + 6 \mu_2 + 6 \mu_1 \mu_2 + 9 \mu_2^2) + \\
& \quad \Theta l (\mu_1^2 (30 + \mathfrak{E}1 - \mathfrak{E}2) + \mu_1 (72 - 4 \mathfrak{E}1 + \mu_2 (90 - 5 \mathfrak{E}1 - 7 \mathfrak{E}2) + 4 \mathfrak{E}2) + \\
& \quad (1 + \mu_2) \times (42 + 72 \mu_2 - 5 \mathfrak{E}1 + 5 \mathfrak{E}2))) - \eta^3 \\
& \quad \left( 6 + 26 \mu_1 + 8 \mu_1^2 + 30 \mu_2 - 30 \mu_1 \mu_2 - 24 \Theta p (5 + 5 \mu_1^2 + 12 \mu_2 + \right. \\
& \quad 18 \mu_2^2 + 2 \mu_1 (5 + 6 \mu_2)) + \eta t (16 + 32 \mu_1 - 8 \mu_1^2 + 5 \mu_2 - \\
& \quad 7 \mu_1 \mu_2 + 16 \Theta p (4 + 4 \mu_1^2 + 6 \mu_2 + 9 \mu_2^2 + \mu_1 (8 + 6 \mu_2)) + \\
& \quad \Theta l (-258 - 144 \mu_2^2 + 5 \mathfrak{E}1 + \mu_1 \mu_2 (-732 + 5 \mathfrak{E}1 - 17 \mathfrak{E}2) + \\
& \quad \mu_2 (-432 + 5 \mathfrak{E}1 - 5 \mathfrak{E}2) + 3 \mu_1 (-156 + 7 \mathfrak{E}1 - 5 \mathfrak{E}2) - 5 \mathfrak{E}2 + \\
& \quad 2 \mu_1^2 (-99 + 2 \mathfrak{E}1 + \mathfrak{E}2)) + \Theta l (258 + 144 \mu_2^2 - 5 \mathfrak{E}1 + \\
& \quad 5 \mathfrak{E}2 - 2 \mu_1^2 (-99 + 2 \mathfrak{E}1 + \mathfrak{E}2) + \mu_2 (432 - 5 \mathfrak{E}1 + 5 \mathfrak{E}2) + \\
& \quad \mu_1 (468 - 21 \mathfrak{E}1 + 15 \mathfrak{E}2 + \mu_2 (732 - 5 \mathfrak{E}1 + 17 \mathfrak{E}2))) - 2 \\
& \quad \eta^4 (-10 + 40 \Theta p + 3 \mu_1 + 80 \Theta p \mu_1 + 7 \mu_1^2 + 40 \Theta p \mu_1^2 - 8 \mu_2 + \\
& \quad 96 \Theta p \mu_2 - 20 \mu_1 \mu_2 + 96 \Theta p \mu_1 \mu_2 + 144 \Theta p \mu_2^2 + \Theta l (59 + 68 \mu_2 - \\
& \quad \mu_1^2 (-53 + 2 \mathfrak{E}1 + \mathfrak{E}2) + \mu_1 (106 + 266 \mu_2 - 5 \mathfrak{E}1 + 2 \mathfrak{E}2 + 6 \mu_2 \mathfrak{E}2)) + \\
& \quad \eta t (-2 \times (1 + \mu_1^2 - \mu_2 + \mu_1 (-4 + 5 \mu_2)) + \Theta l (-59 - 68 \mu_2 + \mu_1^2 (-53 + \\
& \quad 2 \mathfrak{E}1 + \mathfrak{E}2) - \mu_1 (106 + 266 \mu_2 - 5 \mathfrak{E}1 + 2 \mathfrak{E}2 + 6 \mu_2 \mathfrak{E}2))) - \eta^2 \\
& \quad \left( -2 \times (2 \times (-5 + \mu_1^2 - 2 \mu_2 - 4 \mu_1 (1 + 2 \mu_2) + 4 \Theta p (5 + 5 \mu_1^2 + \right. \\
& \quad 12 \mu_2 + 18 \mu_2^2 + 2 \mu_1 (5 + 6 \mu_2))) + \Theta l (-93 - 108 \mu_2^2 + \\
& \quad 5 \mathfrak{E}1 + \mu_2 (-204 + 5 \mathfrak{E}1 - 5 \mathfrak{E}2) + \mu_1^2 (-71 + \mathfrak{E}2) - 5 \mathfrak{E}2 + \\
& \quad \mu_1 (-170 + 8 \mathfrak{E}1 - 7 \mathfrak{E}2 + \mu_2 (-222 + 5 \mathfrak{E}1 + \mathfrak{E}2))) + \\
& \quad \eta t (10 - 20 \mu_1 + 18 \mu_1^2 + \mu_2 + \mu_1 \mu_2 + 8 \Theta p (4 + 4 \mu_1^2 + 6 \mu_2 + \\
& \quad 9 \mu_2^2 + \mu_1 (8 + 6 \mu_2)) + 2 \Theta l (-93 - 108 \mu_2^2 + 5 \mathfrak{E}1 + \\
& \quad \mu_2 (-204 + 5 \mathfrak{E}1 - 5 \mathfrak{E}2) + \mu_1^2 (-71 + \mathfrak{E}2) - 5 \mathfrak{E}2 + \\
& \quad \mu_1 (-170 + 8 \mathfrak{E}1 - 7 \mathfrak{E}2 + \mu_2 (-222 + 5 \mathfrak{E}1 + \mathfrak{E}2))) \right) + \\
& \quad w^2 (-1 + \eta)^2 (2 \eta^8 (1 + \mu_1) - 2 \eta^7 (-7 + \eta t - 11 \mu_1 + \eta t \mu_1 - 4 \mu_1^2 + \\
& \quad 6 \mu_1 \mu_2) - 2 \eta^6 (-12 - 45 \mu_1 - 21 \mu_1^2 + \eta t (7 + \mu_1 (7 - 6 \mu_2)) - 11 \mu_2 + \\
& \quad 43 \mu_1 \mu_2 + 12 \Theta p (5 + 5 \mu_1^2 + 12 \mu_2 + 18 \mu_2^2 + 2 \mu_1 (5 + 6 \mu_2))) + 3 \eta t \\
& \quad (-5 \times (1 + \mu_1) \mu_2 + 4 \Theta p (4 + 4 \mu_1^2 + 6 \mu_2 + 9 \mu_2^2 + \mu_1 (8 + 6 \mu_2))) + 4 \\
& \quad \eta (2 \Theta p (5 + 5 \mu_1^2 + 12 \mu_2 + 18 \mu_2^2 + 2 \mu_1 (5 + 6 \mu_2)) - \\
& \quad \Theta l (22 + 18 \mu_1^2 + 66 \mu_2 + 27 \mu_2^2 + \mu_1 (40 + 78 \mu_2)) + \\
& \quad \eta t (\Theta l (22 + 18 \mu_1^2 + 66 \mu_2 + 27 \mu_2^2 + \mu_1 (40 + 78 \mu_2)) + 3 \times (5 + 7 \mu_1 - \\
& \quad \mu_1^2 - 6 \mu_1 \mu_2 + 5 \Theta p (4 + 8 \mu_1 + 4 \mu_1^2 + 6 \mu_2 + 6 \mu_1 \mu_2 + 9 \mu_2^2))) - \\
& \quad \eta^3 (60 + 130 \mu_1 + 34 \mu_1^2 + 116 \mu_2 - 76 \mu_1 \mu_2 - 88 \Theta p (5 + 5 \mu_1^2 + \\
& \quad 12 \mu_2 + 18 \mu_2^2 + 2 \mu_1 (5 + 6 \mu_2)) + \eta t (4 \times (11 + 15 \mu_1 + \mu_1^2 - \mu_2 -
\end{aligned}$$



$$\begin{aligned}
& \mu_1 \mu_2 + 15 \, \text{op} \left( 4 + 8 \mu_1 + 4 \mu_1^2 + 6 \mu_2 + 6 \mu_1 \mu_2 + 9 \mu_2^2 \right) + \\
& \text{ol} \left( -1250 - 972 \mu_2^2 + 30 \, \text{el} + \mu_1^2 (\text{el} + 3 \times (-372 + \text{el})) + \right. \\
& \quad \mu_1 (-2378 + 61 \, \text{el} + 6 \mu_2 (-751 + 5 \, \text{el} - 3 \, \text{el}_2) - 57 \, \text{el}_2) + \\
& \quad \left. 30 \mu_2 (-79 + \text{el} - \text{el}_2) - 30 \, \text{el}_2 \right) + \text{ol} \left( 1250 + 972 \mu_2^2 - \right. \\
& \quad \left. 30 \, \text{el} - \mu_1^2 (\text{el} + 3 \times (-372 + \text{el})) - 30 \mu_2 (-79 + \text{el} - \text{el}_2) + \right. \\
& \quad \left. 30 \, \text{el}_2 + \mu_1 (2378 - 61 \, \text{el} - 6 \mu_2 (-751 + 5 \, \text{el} - 3 \, \text{el}_2) + 57 \, \text{el}_2) \right) - \\
& \eta^4 \left( -20 + 200 \, \text{op} + 34 \mu_1 + 400 \, \text{op} \mu_1 + 42 \mu_1^2 + 200 \, \text{op} \mu_1^2 - \right. \\
& \quad 36 \mu_2 + 480 \, \text{op} \mu_2 - 108 \mu_1 \mu_2 + 480 \, \text{op} \mu_1 \mu_2 + \\
& \quad 720 \, \text{op} \mu_2^2 + \eta \text{t} \left( 50 + 118 \mu_1 - 52 \mu_1^2 + 23 \mu_2 - 97 \mu_1 \mu_2 + \right. \\
& \quad \left. 48 \, \text{op} \left( 4 + 8 \mu_1 + 4 \mu_1^2 + 6 \mu_2 + 6 \mu_1 \mu_2 + 9 \mu_2^2 \right) + \right. \\
& \quad \text{ol} \left( \mu_1 (-1558 + 44 \, \text{el} + 3 \mu_2 (-1150 + 5 \, \text{el} - 9 \, \text{el}_2) - 36 \, \text{el}_2) + \right. \\
& \quad \mu_1^2 (-784 + 5 \, \text{el} + 3 \, \text{el}_2) - 3 \times (262 + 144 \mu_2^2 - 5 \, \text{el} - \\
& \quad \left. 5 \mu_2 (-86 + \text{el} - \text{el}_2) + 5 \, \text{el}_2) \right) + \text{ol} \left( \mu_1^2 (784 - 5 \, \text{el} - 3 \, \text{el}_2) + \right. \\
& \quad \left. 3 \times (262 + 144 \mu_2^2 - 5 \, \text{el} - 5 \mu_2 (-86 + \text{el} - \text{el}_2) + 5 \, \text{el}_2) + \right. \\
& \quad \left. \mu_1 (1558 - 44 \, \text{el} + 36 \, \text{el}_2 + \mu_2 (3450 - 15 \, \text{el} + 27 \, \text{el}_2)) \right) - \eta^5 \\
& \left( -46 - 108 \mu_1 - 26 \mu_1^2 - 108 \mu_2 + 72 \mu_1 \mu_2 + 2 \, \text{ol} (55 + 67 \mu_2) + \right. \\
& \quad 96 \, \text{op} (5 + 5 \mu_1^2 + 12 \mu_2 + 18 \mu_2^2 + 2 \mu_1 (5 + 6 \mu_2)) - \\
& \quad \text{ol} \mu_1^2 (-156 + 3 \, \text{el} + \text{el}_2) + \text{ol} \mu_1 (254 - 9 \, \text{el} + 5 \, \text{el}_2 + 2 \mu_2 (415 + 6 \, \text{el}_2)) + \\
& \quad \eta \text{t} (14 + 30 \mu_1 - 8 \mu_1^2 + 4 \mu_2 - 68 \mu_1 \mu_2 + \\
& \quad \text{ol} (-2 \times (55 + 67 \mu_2) + \mu_1^2 (-156 + 3 \, \text{el} + \text{el}_2) - \\
& \quad \left. \mu_1 (254 + 830 \mu_2 - 9 \, \text{el} + 5 \, \text{el}_2 + 12 \mu_2 \, \text{el}_2)) \right) + \\
& \eta^2 \left( 64 \, \text{op} (5 + 5 \mu_1^2 + 12 \mu_2 + 18 \mu_2^2 + 2 \mu_1 (5 + 6 \mu_2)) - \right. \\
& \quad 2 \times (23 + 25 \mu_2 + \mu_1 (29 + 7 \mu_2)) - \text{ol} (662 + 648 \mu_2^2 - 15 \, \text{el} + \\
& \quad \mu_1^2 (560 + \text{el} - \text{el}_2) + 15 \, \text{el}_2 + \mu_2 (1478 - 15 \, \text{el} + 15 \, \text{el}_2) + \\
& \quad \mu_1 (1234 - 26 \, \text{el} + 26 \, \text{el}_2 + \mu_2 (2198 - 15 \, \text{el} + 3 \, \text{el}_2)) + \\
& \quad \eta \text{t} (64 + 140 \mu_1 - 44 \mu_1^2 + 38 \mu_2 - 94 \mu_1 \mu_2 + 36 \, \text{op} \\
& \quad \left( 4 + 4 \mu_1^2 + 6 \mu_2 + 9 \mu_2^2 + \mu_1 (8 + 6 \mu_2) \right) + \text{ol} (662 + 648 \mu_2^2 - \\
& \quad 15 \, \text{el} + \mu_1^2 (560 + \text{el} - \text{el}_2) + 15 \, \text{el}_2 + \mu_2 (1478 - 15 \, \text{el} + 15 \, \text{el}_2) + \\
& \quad \left. \mu_1 (1234 - 26 \, \text{el} + 26 \, \text{el}_2 + \mu_2 (2198 - 15 \, \text{el} + 3 \, \text{el}_2)) \right) - \\
& w^3 (-1 + \eta)^3 \left( 4 \eta^7 (1 + \mu_1) + 2 \eta^6 (5 + 8 \mu_1^2 - 2 \eta \text{t} (1 + \mu_1) + \mu_1 (13 - 12 \mu_2)) - \right. \\
& \quad 2 \eta^5 (-11 - 32 \mu_1 - 15 \mu_1^2 + \eta \text{t} (5 + \mu_1 (5 - 12 \mu_2)) - 22 \mu_2 + 32 \mu_1 \mu_2 + \\
& \quad 20 \, \text{op} (5 + 5 \mu_1^2 + 12 \mu_2 + 18 \mu_2^2 + 2 \mu_1 (5 + 6 \mu_2)) + 3 \eta \text{t} \\
& \quad \left( -5 \times (1 + \mu_1) \mu_2 + 4 \, \text{op} (4 + 4 \mu_1^2 + 6 \mu_2 + 9 \mu_2^2 + \mu_1 (8 + 6 \mu_2)) \right) + 2 \\
& \quad \eta (8 \, \text{op} (5 + 5 \mu_1^2 + 12 \mu_2 + 18 \mu_2^2 + 2 \mu_1 (5 + 6 \mu_2)) - \\
& \quad 2 \, \text{ol} (32 + 28 \mu_1^2 + 78 \mu_2 + 27 \mu_2^2 + 6 \mu_1 (10 + 21 \mu_2)) + \\
& \quad \eta \text{t} (20 + 34 \mu_1 - 4 \mu_1^2 - 5 \mu_2 - 17 \mu_1 \mu_2 + \\
& \quad 22 \, \text{op} (4 + 8 \mu_1 + 4 \mu_1^2 + 6 \mu_2 + 6 \mu_1 \mu_2 + 9 \mu_2^2) + \\
& \quad \left. 2 \, \text{ol} (32 + 28 \mu_1^2 + 78 \mu_2 + 27 \mu_2^2 + 6 \mu_1 (10 + 21 \mu_2)) \right) + \\
& \eta^4 \left( 30 + 36 \mu_1 - 6 \mu_1^2 + 68 \mu_2 - 4 \mu_1 \mu_2 - 56 \, \text{op} (5 + 5 \mu_1^2 + \right. \\
& \quad \left. 12 \mu_2 + 18 \mu_2^2 + 2 \mu_1 (5 + 6 \mu_2)) - \right. \\
& \quad \text{ol} (264 + 280 \mu_1^2 + 144 \mu_2^2 - 5 \, \text{el} + 5 \, \text{el}_2 + \mu_2 (432 - 5 \, \text{el} + 5 \, \text{el}_2) + \\
& \quad \mu_1 (544 - 11 \, \text{el} + 11 \, \text{el}_2 + \mu_2 (1248 - 5 \, \text{el} + 5 \, \text{el}_2)) + \\
& \quad \left. \eta \text{t} (-22 - 50 \mu_1 + 20 \mu_1^2 - 9 \mu_2 + 63 \mu_1 \mu_2 - 16 \, \text{op} \right.
\end{aligned}$$

$$\begin{aligned}
& (4 + 4 \mu_1^2 + 6 \mu_2 + 9 \mu_2^2 + \mu_1 (8 + 6 \mu_2)) + \\
& \theta_l (264 + 280 \mu_1^2 + 144 \mu_2^2 - 5 \mathfrak{z}_1 + 5 \mathfrak{z}_2 + \mu_2 (432 - 5 \mathfrak{z}_1 + 5 \mathfrak{z}_2) + \\
& \quad \mu_1 (544 - 11 \mathfrak{z}_1 + 11 \mathfrak{z}_2 + \mu_2 (1248 - 5 \mathfrak{z}_1 + 5 \mathfrak{z}_2))) + 2 \eta^3 \\
& (-13 + 60 \theta_p - 34 \mu_1 + 120 \theta_p \mu_1 - 15 \mu_1^2 + 60 \theta_p \mu_1^2 - 26 \mu_2 + \\
& \quad 144 \theta_p \mu_2 + 52 \mu_1 \mu_2 + 144 \theta_p \mu_1 \mu_2 + 216 \theta_p \mu_2^2 - \\
& \quad \theta_l (356 \mu_1^2 + 270 \mu_2^2 + 5 \times (72 - \mathfrak{z}_1 + \mathfrak{z}_2) + \mu_2 (688 - 5 \mathfrak{z}_1 + 5 \mathfrak{z}_2) + \\
& \quad \mu_1 (716 - 11 \mathfrak{z}_1 + 11 \mathfrak{z}_2 + \mu_2 (1528 - 5 \mathfrak{z}_1 + 5 \mathfrak{z}_2))) + \\
& \quad \eta t (-15 - 33 \mu_1 + 24 \mu_1^2 + 5 \mu_2 + 5 \mu_1 \mu_2 - 22 \theta_p \\
& \quad (4 + 4 \mu_1^2 + 6 \mu_2 + 9 \mu_2^2 + \mu_1 (8 + 6 \mu_2)) + \\
& \quad \theta_l (356 \mu_1^2 + 270 \mu_2^2 + 5 \times (72 - \mathfrak{z}_1 + \mathfrak{z}_2) + \mu_2 (688 - 5 \mathfrak{z}_1 + 5 \mathfrak{z}_2) + \\
& \quad \mu_1 (716 - 11 \mathfrak{z}_1 + 11 \mathfrak{z}_2 + \mu_2 (1528 - 5 \mathfrak{z}_1 + 5 \mathfrak{z}_2))) + \eta^2 \\
& (2 \times (-20 - 31 \mu_1 - 5 \mu_1^2 - 30 \mu_2 - 6 \mu_1 \mu_2 + 28 \theta_p (5 + 5 \mu_1^2 + \\
& \quad 12 \mu_2 + 18 \mu_2^2 + 2 \mu_1 (5 + 6 \mu_2))) - \\
& \quad \theta_l (584 + 544 \mu_1^2 + 504 \mu_2^2 - 5 \mathfrak{z}_1 + 5 \mathfrak{z}_2 + \mu_2 (1256 - 5 \mathfrak{z}_1 + 5 \mathfrak{z}_2) + \\
& \quad \mu_1 (1128 - 11 \mathfrak{z}_1 + 11 \mathfrak{z}_2 + \mu_2 (2312 - 5 \mathfrak{z}_1 + 5 \mathfrak{z}_2))) + \\
& \quad \eta t (26 + 62 \mu_1 - 60 \mu_1^2 + 24 \mu_2 - 48 \mu_1 \mu_2 + 4 \theta_p \\
& \quad (4 + 4 \mu_1^2 + 6 \mu_2 + 9 \mu_2^2 + \mu_1 (8 + 6 \mu_2)) + \\
& \quad \theta_l (584 + 544 \mu_1^2 + 504 \mu_2^2 - 5 \mathfrak{z}_1 + 5 \mathfrak{z}_2 + \mu_2 (1256 - 5 \mathfrak{z}_1 + 5 \mathfrak{z}_2) + \\
& \quad \mu_1 (1128 - 11 \mathfrak{z}_1 + 11 \mathfrak{z}_2 + \mu_2 (2312 - 5 \mathfrak{z}_1 + 5 \mathfrak{z}_2))) - \\
& w (-1 + \eta) \times (6 \eta^8 (1 + \mu_1) + 2 \eta^7 (7 + 9 \mu_1^2 - 3 \eta t (1 + \mu_1) + \mu_1 (22 - 18 \mu_2)) + \\
& \quad \eta t (-5 \times (1 + \mu_1) \mu_2 + 4 \theta_p (4 + 4 \mu_1^2 + 6 \mu_2 + 9 \mu_2^2 + \mu_1 (8 + 6 \mu_2))) + 2 \eta \\
& \quad (-2 \theta_l (4 + 4 \mu_1^2 + 18 \mu_2 + 9 \mu_2^2 + 2 \mu_1 (4 + 9 \mu_2)) + \eta t (20 + 22 \mu_1 - 4 \mu_1^2 + \\
& \quad 5 \mu_2 - 31 \mu_1 \mu_2 + 18 \theta_p (4 + 8 \mu_1 + 4 \mu_1^2 + 6 \mu_2 + 6 \mu_1 \mu_2 + 9 \mu_2^2) + \\
& \quad 2 \theta_l (4 + 4 \mu_1^2 + 18 \mu_2 + 9 \mu_2^2 + 2 \mu_1 (4 + 9 \mu_2))) - \eta^6 \\
& (-14 - 84 \mu_1 + 8 \theta_l \mu_1 - 34 \mu_1^2 + 20 \theta_l \mu_1^2 - 44 \mu_2 - 2 \theta_l \mu_2 + 76 \mu_1 \mu_2 + \\
& \quad 154 \theta_l \mu_1 \mu_2 + 48 \theta_p (5 + 5 \mu_1^2 + 12 \mu_2 + 18 \mu_2^2 + 2 \mu_1 (5 + 6 \mu_2)) - \\
& \quad \theta_l \mu_1 \mathfrak{z}_1 - \theta_l \mu_1^2 \mathfrak{z}_1 - \theta_l \mu_1 \mathfrak{z}_2 - \theta_l \mu_1^2 \mathfrak{z}_2 + \\
& \quad \eta t (2 \times (7 + \theta_l \mu_2) + \mu_1^2 (-4 + \theta_l (-20 + \mathfrak{z}_1 + \mathfrak{z}_2)) + \\
& \quad \mu_1 (10 - 24 \mu_2 + \theta_l (-8 - 154 \mu_2 + \mathfrak{z}_1 + \mathfrak{z}_2))) + \eta^2 \\
& (4 \times ((1 + \mu_1) \times (-5 + \mu_1 - 3 \mu_2) + 6 \theta_p (5 + 5 \mu_1^2 + 12 \mu_2 + \\
& \quad 18 \mu_2^2 + 2 \mu_1 (5 + 6 \mu_2))) - \theta_l (2 \mu_1^2 (115 + \mathfrak{z}_1 - \mathfrak{z}_2) + \\
& \quad 15 \times (20 + 24 \mu_2^2 - \mathfrak{z}_1 + \mathfrak{z}_2 + \mu_2 (48 - \mathfrak{z}_1 + \mathfrak{z}_2)) + \\
& \quad \mu_1 (542 - 19 \mathfrak{z}_1 + 19 \mathfrak{z}_2 - 3 \mu_2 (-264 + 5 \mathfrak{z}_1 + 3 \mathfrak{z}_2))) + \\
& \quad \eta t (60 + 104 \mu_1 - 4 \mu_1^2 + 24 \mu_2 - 72 \mu_1 \mu_2 + 44 \theta_p (4 + 4 \mu_1^2 + \\
& \quad 6 \mu_2 + 9 \mu_2^2 + \mu_1 (8 + 6 \mu_2)) + 2 \theta_l \mu_1^2 (115 + \mathfrak{z}_1 - \mathfrak{z}_2) + \\
& \quad 15 \theta_l (20 + 24 \mu_2^2 - \mathfrak{z}_1 + \mathfrak{z}_2 + \mu_2 (48 - \mathfrak{z}_1 + \mathfrak{z}_2)) + \\
& \quad \theta_l \mu_1 (542 - 19 \mathfrak{z}_1 + 19 \mathfrak{z}_2 - 3 \mu_2 (-264 + 5 \mathfrak{z}_1 + 3 \mathfrak{z}_2))) - \eta^4 \\
& (74 \mu_1 + 38 \mu_1^2 + 40 \mu_2 - 128 \mu_1 \mu_2 - 24 \theta_p (5 + 5 \mu_1^2 + 12 \mu_2 + 18 \mu_2^2 + \\
& \quad 2 \mu_1 (5 + 6 \mu_2)) + \eta t (46 + 102 \mu_1 - 40 \mu_1^2 + 19 \mu_2 - 53 \mu_1 \mu_2 + \\
& \quad 48 \theta_p (4 + 4 \mu_1^2 + 6 \mu_2 + 9 \mu_2^2 + \mu_1 (8 + 6 \mu_2)) + \theta_l (-788 - 432 \mu_2^2 + \\
& \quad 15 \mathfrak{z}_1 + \mu_1 (-1490 + 54 \mathfrak{z}_1 + 3 \mu_2 (-978 + 5 \mathfrak{z}_1 - 13 \mathfrak{z}_2) - 40 \mathfrak{z}_2) + \\
& \quad 15 \mu_2 (-86 + \mathfrak{z}_1 - \mathfrak{z}_2) - 15 \mathfrak{z}_2 + \mu_1^2 (-702 + 9 \mathfrak{z}_1 + 5 \mathfrak{z}_2))) + \\
& \quad \theta_l (788 + 432 \mu_2^2 - 15 \mathfrak{z}_1 + \mu_1^2 (702 - 9 \mathfrak{z}_1 - 5 \mathfrak{z}_2) - 15 \mu_2
\end{aligned}$$

$$\begin{aligned}
& (-86 + \mathfrak{x}1 - \mathfrak{x}2) + 15 \mathfrak{x}2 + \mu1 (1490 - 54 \mathfrak{x}1 + 40 \mathfrak{x}2 + \\
& \quad \mu2 (2934 - 15 \mathfrak{x}1 + 39 \mathfrak{x}2)) - \eta^5 (-38 - 40 \mu1 + 10 \mu1^2 - 80 \mu2 - \\
& 20 \mu1 \mu2 + 72 \mathfrak{e}p (5 + 5 \mu1^2 + 12 \mu2 + 18 \mu2^2 + 2 \mu1 (5 + 6 \mu2)) + \\
& \mathfrak{e}l (6 \times (38 + 45 \mu2) + \mu1^2 (262 - 7 \mathfrak{x}1 - 3 \mathfrak{x}2) + \\
& \quad \mu1 (466 - 19 \mathfrak{x}1 + 9 \mathfrak{x}2 + 6 \mu2 (227 + 4 \mathfrak{x}2))) + \eta t (2 + 38 \mu1 - 12 \mu1^2 + \\
& 8 \mu2 - 64 \mu1 \mu2 + \mathfrak{e}l (-6 \times (38 + 45 \mu2) + \mu1^2 (-262 + 7 \mathfrak{x}1 + 3 \mathfrak{x}2) - \\
& \quad \mu1 (466 - 19 \mathfrak{x}1 + 9 \mathfrak{x}2 + 6 \mu2 (227 + 4 \mathfrak{x}2)))) - \eta^3 \\
& (52 + 84 \mu1 + 8 \mu1^2 + 72 \mu2 + 24 \mu1 \mu2 - 72 \mathfrak{e}p (5 + 5 \mu1^2 + 12 \mu2 + \\
& 18 \mu2^2 + 2 \mu1 (5 + 6 \mu2)) + \mathfrak{e}l (844 + 756 \mu2^2 - 30 \mathfrak{x}1 + \\
& 30 \mathfrak{x}2 - \mu1^2 (-674 + \mathfrak{x}1 + 5 \mathfrak{x}2) + \mu2 (1666 - 30 \mathfrak{x}1 + 30 \mathfrak{x}2) + \\
& \mu1 (1542 - 55 \mathfrak{x}1 + 49 \mathfrak{x}2 + \mu2 (2446 - 30 \mathfrak{x}1 + 6 \mathfrak{x}2))) + \\
& \eta t (2 \times (16 + 22 \mu1^2 + \mu1 (-4 + \mu2) + \mu2 + 18 \mathfrak{e}p \\
& \quad (4 + 4 \mu1^2 + 6 \mu2 + 9 \mu2^2 + \mu1 (8 + 6 \mu2))) + \\
& \mathfrak{e}l (\mu1 (-1542 + 55 \mathfrak{x}1 + \mu2 (-2446 + 30 \mathfrak{x}1 - 6 \mathfrak{x}2) - 49 \mathfrak{x}2) + \\
& \quad \mu1^2 (-674 + \mathfrak{x}1 + 5 \mathfrak{x}2) - 2 \times (422 + 378 \mu2^2 - 15 \mathfrak{x}1 + \\
& \quad 15 \mathfrak{x}2 + \mu2 (833 - 15 \mathfrak{x}1 + 15 \mathfrak{x}2)))))) - \\
& x^4 (-1 + \eta)^4 ((-1 + \eta) \mathfrak{e}p (20 + 104 \eta + 36 \eta^2 + 80 \eta^4 - 20 \eta t - 16 \eta \eta t - \\
& 80 \eta^2 \eta t - 80 \eta^3 \eta t - 20 \mathfrak{e}p - 200 \eta \mathfrak{e}p - 300 \eta^2 \mathfrak{e}p - 16 \eta t \\
& \mathfrak{e}p + 16 \mu1 + 168 \eta \mu1 + 456 \eta^2 \mu1 + 440 \eta^3 \mu1 + 80 \eta^4 \mu1 - 48 \\
& \eta t \mu1 - 80 \eta \eta t \mu1 - 64 \eta^2 \eta t \mu1 - 80 \eta^3 \eta t \mu1 - 40 \mathfrak{e}p \\
& \mu1 - 400 \eta \mathfrak{e}p \mu1 - 600 \eta^2 \mathfrak{e}p \mu1 - 32 \eta t \mathfrak{e}p \mu1 - 4 \mu1^2 + 16 \eta \\
& \mu1^2 + 180 \eta^2 \mu1^2 + 200 \eta^3 \mu1^2 + 44 \eta t \mu1^2 + 32 \eta \eta t \mu1^2 + 16 \\
& \eta^2 \eta t \mu1^2 - 20 \mathfrak{e}p \mu1^2 - 200 \eta \mathfrak{e}p \mu1^2 - 300 \eta^2 \mathfrak{e}p \mu1^2 - 16 \\
& \eta t \mathfrak{e}p \mu1^2 + 12 \mu2 + 152 \eta \mu2 + 196 \eta^2 \mu2 - 9 \eta t \mu2 - 16 \eta \\
& \eta t \mu2 - 48 \mathfrak{e}p \mu2 - 480 \eta \mathfrak{e}p \mu2 - 720 \eta^2 \mathfrak{e}p \mu2 - 24 \eta t \mathfrak{e}p \\
& \mu2 + 12 \mu1 \mu2 + 8 \eta \mu1 \mu2 - 116 \eta^2 \mu1 \mu2 - 240 \eta^3 \mu1 \mu2 + 39 \\
& \eta t \mu1 \mu2 + 128 \eta \eta t \mu1 \mu2 + 120 \eta^2 \eta t \mu1 \mu2 - 48 \mathfrak{e}p \mu1 \\
& \mu2 - 480 \eta \mathfrak{e}p \mu1 \mu2 - 720 \eta^2 \mathfrak{e}p \mu1 \mu2 - 24 \eta t \mathfrak{e}p \mu1 \mu2 - 72 \\
& \mathfrak{e}p \mu2^2 - 720 \eta \mathfrak{e}p \mu2^2 - 1080 \eta^2 \mathfrak{e}p \mu2^2 - 36 \eta t \mathfrak{e}p \mu2^2 + 2 w^4 \\
& (-1 + \eta)^4 (5 - 10 \mathfrak{e}p + 12 \mu1 - 20 \mathfrak{e}p \mu1 + 7 \mu1^2 - 10 \mathfrak{e}p \mu1^2 + \\
& 4 \eta^2 (1 + \mu1) + 11 \mu2 - 24 \mathfrak{e}p \mu2 - 7 \mu1 \mu2 - 24 \mathfrak{e}p \mu1 \mu2 - \\
& 36 \mathfrak{e}p \mu2^2 + 2 \eta (1 + 9 \mu1 + 8 \mu1^2 - 2 \eta t (1 + \mu1) - 3 \mu1 \mu2) + \\
& \eta t (-2 - 2 \mu1 + 6 \mu1 \mu2) - w^3 (-1 + \eta)^3 \\
& (40 \eta^3 (1 + \mu1) + 8 \eta^2 (7 + 20 \mu1^2 - 5 \eta t (1 + \mu1) - 3 \mu1 (-9 + 4 \mu2)) + \\
& 4 \times (15 + 10 \mu1^2 + \mu1 (31 - 14 \mu2) + 28 \mu2 - \\
& 6 \mathfrak{e}p (5 + 5 \mu1^2 + 12 \mu2 + 18 \mu2^2 + 2 \mu1 (5 + 6 \mu2))) - \\
& 4 \eta (-24 - 82 \mu1 - 46 \mu1^2 + \eta t (14 + \mu1 (14 - 24 \mu2)) - 44 \mu2 + \\
& 43 \mu1 \mu2 + 10 \mathfrak{e}p (5 + 5 \mu1^2 + 12 \mu2 + 18 \mu2^2 + 2 \mu1 (5 + 6 \mu2))) - \\
& \eta t (-44 \mu1^2 + \mu1 (64 - 87 \mu2) + 9 \times (4 + \mu2) + 4 \mathfrak{e}p \\
& \quad (4 + 4 \mu1^2 + 6 \mu2 + 9 \mu2^2 + \mu1 (8 + 6 \mu2)))) + w^2 (-1 + \eta)^2 \\
& (40 \eta^4 (1 + \mu1) - 40 \eta^3 (-4 + \eta t - 8 \mu1 + \eta t \mu1 - 4 \mu1^2 + 3 \mu1 \mu2) + \\
& 2 \times (51 + 17 \mu1^2 + \mu1 (92 - 19 \mu2) + 83 \mu2 - \\
& 20 \mathfrak{e}p (5 + 5 \mu1^2 + 12 \mu2 + 18 \mu2^2 + 2 \mu1 (5 + 6 \mu2))) - \\
& 4 \eta^2 (-55 - 240 \mu1 - 125 \mu1^2 + \eta t (40 + \mu1 (40 - 30 \mu2)) - 55 \mu2 +
\end{aligned}$$

$$\begin{aligned}
& 119 \mu_1 \mu_2 + 15 \theta p \left( 5 + 5 \mu_1^2 + 12 \mu_2 + 18 \mu_2^2 + 2 \mu_1 (5 + 6 \mu_2) \right) - \\
& 4 \eta \left( -71 - 207 \mu_1 - 76 \mu_1^2 - 130 \mu_2 + 98 \mu_1 \mu_2 + \right. \\
& \quad \left. \eta t \left( 30 - 8 \mu_1^2 + \mu_1 (46 - 80 \mu_2) + 4 \mu_2 \right) + \right. \\
& \quad \left. 30 \theta p \left( 5 + 5 \mu_1^2 + 12 \mu_2 + 18 \mu_2^2 + 2 \mu_1 (5 + 6 \mu_2) \right) \right) - \\
& \eta t \left( 80 - 132 \mu_1^2 + \mu_1 (164 - 177 \mu_2) + 27 \mu_2 + 12 \theta p \right. \\
& \quad \left. \left( 4 + 4 \mu_1^2 + 6 \mu_2 + 9 \mu_2^2 + \mu_1 (8 + 6 \mu_2) \right) \right) - w (-1 + \eta) \times \\
& (120 \eta^4 (1 + \mu_1) + 40 \eta^3 (5 + 9 \mu_1^2 - 3 \eta t (1 + \mu_1) + \mu_1 (20 - 9 \mu_2)) + \\
& 4 \times (18 + \mu_1^2 + 22 \mu_2 + \mu_1 (25 + 4 \mu_2) - \\
& 6 \theta p (5 + 5 \mu_1^2 + 12 \mu_2 + 18 \mu_2^2 + 2 \mu_1 (5 + 6 \mu_2)) - \\
& 8 \eta^2 (-26 - 151 \mu_1 - 65 \mu_1^2 + \eta t (25 - 2 \mu_1^2 + \mu_1 (23 - 30 \mu_2)) - 52 \mu_2 + \\
& 62 \mu_1 \mu_2 + 15 \theta p (5 + 5 \mu_1^2 + 12 \mu_2 + 18 \mu_2^2 + 2 \mu_1 (5 + 6 \mu_2)) - \\
& 8 \eta (-33 - 84 \mu_1 - 21 \mu_1^2 - 62 \mu_2 + 28 \mu_1 \mu_2 + \eta t \\
& (11 - 8 \mu_1^2 + \mu_1 (27 - 44 \mu_2) + 4 \mu_2) + \\
& 15 \theta p (5 + 5 \mu_1^2 + 12 \mu_2 + 18 \mu_2^2 + 2 \mu_1 (5 + 6 \mu_2)) - \\
& \eta t (68 - 132 \mu_1^2 + \mu_1 (152 - 141 \mu_2) + 27 \mu_2 + 12 \theta p \\
& (4 + 4 \mu_1^2 + 6 \mu_2 + 9 \mu_2^2 + \mu_1 (8 + 6 \mu_2)) \right) + \\
& (-1 + \eta t) \theta l (-30 - 60 \eta + 30 \theta p + 192 \eta \theta p + 280 \eta^2 \theta p + 80 \eta^3 \theta p - \\
& 32 \mu_1 - 160 \eta \mu_1 - 120 \eta^2 \mu_1 + 24 \eta^3 \mu_1 + 50 \theta p \mu_1 + 366 \eta \theta p \\
& \mu_1 + 332 \eta^2 \theta p \mu_1 - 160 \eta^3 \theta p \mu_1 + 10 \mu_1^2 + 56 \eta \mu_1^2 + 24 \\
& \eta^2 \mu_1^2 + 24 \eta^3 \mu_1^2 + 8 \theta p \mu_1^2 + 126 \eta \theta p \mu_1^2 + 172 \eta^2 \theta p \\
& \mu_1^2 - 10 \mu_2 - 15 \eta \mu_2 + 70 \theta p \mu_2 + 342 \eta \theta p \mu_2 + 292 \eta^2 \theta p \\
& \mu_2 - 20 \eta^3 \theta p \mu_2 + 38 \mu_1 \mu_2 + 57 \eta \mu_1 \mu_2 + 46 \theta p \mu_1 \mu_2 + 498 \\
& \eta \theta p \mu_1 \mu_2 + 940 \eta^2 \theta p \mu_1 \mu_2 + 460 \eta^3 \theta p \mu_1 \mu_2 + 36 \eta \theta p \\
& \mu_2^2 + w^4 (-1 + \eta)^4 (26 \mu_1^2 + 5 \mu_1 (-4 + \mu_2) + 5 \times (-2 + \mu_2) + \\
& 4 \theta p (5 + 5 \mu_1^2 + 12 \mu_2 + 10 \mu_1 (1 + 3 \mu_2)) - 10 \theta p \\
& \mathfrak{z}1 - 20 \eta \theta p \mathfrak{z}1 - 17 \theta p \mu_1 \mathfrak{z}1 - 87 \eta \theta p \mu_1 \mathfrak{z}1 - 94 \eta^2 \theta p \mu_1 \\
& \mathfrak{z}1 - 10 \eta^3 \theta p \mu_1 \mathfrak{z}1 - \theta p \mu_1^2 \mathfrak{z}1 - 19 \eta \theta p \mu_1^2 \mathfrak{z}1 - 34 \eta^2 \\
& \theta p \mu_1^2 \mathfrak{z}1 - 10 \eta^3 \theta p \mu_1^2 \mathfrak{z}1 - 10 \theta p \mu_2 \mathfrak{z}1 - 20 \eta \theta p \mu_2 \\
& \mathfrak{z}1 - 10 \theta p \mu_1 \mu_2 \mathfrak{z}1 - 20 \eta \theta p \mu_1 \mu_2 \mathfrak{z}1 + 10 \theta p \mathfrak{z}2 + 20 \eta \\
& \theta p \mathfrak{z}2 + 13 \theta p \mu_1 \mathfrak{z}2 + 57 \eta \theta p \mu_1 \mathfrak{z}2 + 46 \eta^2 \theta p \mu_1 \mathfrak{z}2 - 10 \\
& \eta^3 \theta p \mu_1 \mathfrak{z}2 - 3 \theta p \mu_1^2 \mathfrak{z}2 - 11 \eta \theta p \mu_1^2 \mathfrak{z}2 - 14 \eta^2 \theta p \mu_1^2 \\
& \mathfrak{z}2 - 10 \eta^3 \theta p \mu_1^2 \mathfrak{z}2 + 10 \theta p \mu_2 \mathfrak{z}2 + 20 \eta \theta p \mu_2 \mathfrak{z}2 - 2 \\
& \theta p \mu_1 \mu_2 \mathfrak{z}2 + 68 \eta \theta p \mu_1 \mu_2 \mathfrak{z}2 + 120 \eta^2 \theta p \mu_1 \mu_2 \mathfrak{z}2 - w^3 \\
& (-1 + \eta)^3 (-60 - 128 \mu_1 + 76 \mu_1^2 + 5 \mu_2 + 53 \mu_1 \mu_2 + \\
& 2 \theta p (60 + 56 \mu_1^2 - 5 \mathfrak{z}1 + 5 \mathfrak{z}2 + \mu_2 (124 - 5 \mathfrak{z}1 + 5 \mathfrak{z}2) + \\
& \mu_1 (116 - 11 \mathfrak{z}1 + 11 \mathfrak{z}2 + \mu_2 (316 - 5 \mathfrak{z}1 + 5 \mathfrak{z}2)) + \\
& \eta (3 \times (20 \mu_1^2 - 5 \times (4 + \mu_2) + \mu_1 (-52 + 19 \mu_2)) + 4 \theta p \\
& (54 + 55 \mu_1^2 + 9 \mu_2^2 - 5 \mathfrak{z}1 + 5 \mathfrak{z}2 + \mu_2 (87 - 5 \mathfrak{z}1 + 5 \mathfrak{z}2) + \\
& \mu_1 (109 - 11 \mathfrak{z}1 + 11 \mathfrak{z}2 + \mu_2 (273 - 5 \mathfrak{z}1 + 5 \mathfrak{z}2)) \right) - \\
& w^2 (-1 + \eta)^2 (3 \times (-28 \mu_1^2 + \mu_1 (76 - 43 \mu_2) + 5 \times (8 + \mu_2)) + \\
& \theta p (-218 + 30 \mathfrak{z}1 + \mu_1^2 (\mathfrak{z}1 + 3 \times (-52 + \mathfrak{z}2)) + \\
& \mu_1 (-386 + 61 \mathfrak{z}1 + 6 \mu_2 (-139 + 5 \mathfrak{z}1 - 3 \mathfrak{z}2) - 57 \mathfrak{z}2) + \\
& 6 \mu_2 (-71 + 5 \mathfrak{z}1 - 5 \mathfrak{z}2) - 30 \mathfrak{z}2) + \\
& \eta (-9 \times (20 \mu_1^2 - 5 \times (4 + \mu_2) + \mu_1 (-52 + 19 \mu_2)) +
\end{aligned}$$

$$\begin{aligned}
& 4 \, \text{Op} \left( \mu_1 (-283 + 44 \, \mathfrak{t}_1 + 3 \, \mu_2 (-235 + 5 \, \mathfrak{t}_1 - 9 \, \mathfrak{t}_2) - 36 \, \mathfrak{t}_2) + \right. \\
& \quad \mu_1^2 (-139 + 5 \, \mathfrak{t}_1 + 3 \, \mathfrak{t}_2) - \\
& \quad \left. 3 \times (52 + 9 \, \mu_2^2 - 5 \, \mathfrak{t}_1 + 5 \, \mathfrak{t}_2 + \mu_2 (85 - 5 \, \mathfrak{t}_1 + 5 \, \mathfrak{t}_2)) \right) + \\
& 2 \, \eta^2 \left( -12 \times (-5 + \mu_1) \, \mu_1 + 5 \, \text{Op} \left( -20 - 26 \, \mu_2 + \mu_1^2 (-30 + 3 \, \mathfrak{t}_1 + \mathfrak{t}_2) - \right. \right. \\
& \quad \left. \left. \mu_1 (38 - 9 \, \mathfrak{t}_1 + 5 \, \mathfrak{t}_2 + 2 \, \mu_2 (91 + 6 \, \mathfrak{t}_2)) \right) \right) + w \\
& (-1 + \eta) \times \left( 100 + 152 \, \mu_1 - 44 \, \mu_1^2 + 25 \, \mu_2 - 119 \, \mu_1 \, \mu_2 + 2 \, \text{Op} \right. \\
& \quad \left( -74 + 15 \, \mathfrak{t}_1 + \mu_1 (-122 + 28 \, \mathfrak{t}_1 + \mu_2 (-184 + 15 \, \mathfrak{t}_1 - 3 \, \mathfrak{t}_2) - 24 \, \mathfrak{t}_2) + \right. \\
& \quad \left. \mu_2 (-148 + 15 \, \mathfrak{t}_1 - 15 \, \mathfrak{t}_2) - 15 \, \mathfrak{t}_2 + \mu_1^2 (-36 + \mathfrak{t}_1 + 3 \, \mathfrak{t}_2) \right) + \\
& 2 \, \eta^3 \left( 10 \, \text{Op} \, \mu_2 + \mu_1^2 (-12 + 5 \, \text{Op} (\mathfrak{t}_1 + \mathfrak{t}_2)) + \right. \\
& \quad \left. \mu_1 (-12 + 5 \, \text{Op} (24 - 46 \, \mu_2 + \mathfrak{t}_1 + \mathfrak{t}_2)) \right) + \\
& 8 \, \eta^2 \left( -6 \times (-5 + \mu_1) \, \mu_1 + \text{Op} \left( -60 - 69 \, \mu_2 + \mu_1^2 (-59 + 8 \, \mathfrak{t}_1 + 3 \, \mathfrak{t}_2) - \right. \right. \\
& \quad \left. \left. \mu_1 (89 + 345 \, \mu_2 - 23 \, \mathfrak{t}_1 + 12 \, \mathfrak{t}_2 + 30 \, \mu_2 \, \mathfrak{t}_2) \right) \right) + \\
& \eta \left( -176 \, \mu_1^2 + \mu_1 (472 - 171 \, \mu_2) + 45 \times (4 + \mu_2) + \text{Op} \right. \\
& \quad \left( \mu_1 (-1094 + 219 \, \mathfrak{t}_1 + 6 \, \mu_2 (-371 + 10 \, \mathfrak{t}_1 - 26 \, \mathfrak{t}_2) - 157 \, \mathfrak{t}_2) + \right. \\
& \quad \left. \mu_1^2 (-462 + 39 \, \mathfrak{t}_1 + 23 \, \mathfrak{t}_2) - 2 \times (316 + 54 \, \mu_2^2 - \right. \\
& \quad \left. 30 \, \mathfrak{t}_1 + 30 \, \mathfrak{t}_2 + \mu_2 (507 - 30 \, \mathfrak{t}_1 + 30 \, \mathfrak{t}_2)) \right) \left. \right) + \\
& x^3 (-1 + \eta)^3 \left( (-1 + \eta) \, \text{Op} \left( 60 \, \eta + 156 \, \eta^2 + 44 \, \eta^3 + 20 \, \eta^4 + 60 \, \eta^5 - 30 \, \eta \, \mathfrak{t} - \right. \right. \\
& 60 \, \eta \, \eta \, \mathfrak{t} - 24 \, \eta^2 \, \eta \, \mathfrak{t} - 80 \, \eta^3 \, \eta \, \mathfrak{t} - 60 \, \eta^4 \, \eta \, \mathfrak{t} - 80 \, \eta \, \text{Op} - 400 \, \eta^2 \\
& \text{Op} - 400 \, \eta^3 \, \text{Op} - 32 \, \eta \, \mathfrak{t} \, \text{Op} - 64 \, \eta \, \eta \, \mathfrak{t} \, \text{Op} + 48 \, \eta \, \mu_1 + 252 \, \eta^2 \\
& \mu_1 + 464 \, \eta^3 \, \mu_1 + 350 \, \eta^4 \, \mu_1 + 60 \, \eta^5 \, \mu_1 - 32 \, \eta \, \mathfrak{t} \, \mu_1 - 148 \, \eta \, \eta \, \mathfrak{t} \\
& \mu_1 - 120 \, \eta^2 \, \eta \, \mathfrak{t} \, \mu_1 - 56 \, \eta^3 \, \eta \, \mathfrak{t} \, \mu_1 - 60 \, \eta^4 \, \eta \, \mathfrak{t} \, \mu_1 - 160 \, \eta \, \text{Op} \\
& \mu_1 - 800 \, \eta^2 \, \text{Op} \, \mu_1 - 800 \, \eta^3 \, \text{Op} \, \mu_1 - 64 \, \eta \, \mathfrak{t} \, \text{Op} \, \mu_1 - 128 \, \eta \, \eta \, \mathfrak{t} \\
& \text{Op} \, \mu_1 - 12 \, \eta \, \mu_1^2 + 24 \, \eta^2 \, \mu_1^2 + 180 \, \eta^3 \, \mu_1^2 + 150 \, \eta^4 \, \mu_1^2 + 22 \\
& \eta \, \mathfrak{t} \, \mu_1^2 + 104 \, \eta \, \eta \, \mathfrak{t} \, \mu_1^2 + 48 \, \eta^2 \, \eta \, \mathfrak{t} \, \mu_1^2 + 24 \, \eta^3 \, \eta \, \mathfrak{t} \, \mu_1^2 - 80 \, \eta \\
& \text{Op} \, \mu_1^2 - 400 \, \eta^2 \, \text{Op} \, \mu_1^2 - 400 \, \eta^3 \, \text{Op} \, \mu_1^2 - 32 \, \eta \, \mathfrak{t} \, \text{Op} \, \mu_1^2 - 64 \, \eta \\
& \eta \, \mathfrak{t} \, \text{Op} \, \mu_1^2 + 32 \, \eta \, \mu_2 + 228 \, \eta^2 \, \mu_2 + 204 \, \eta^3 \, \mu_2 - 10 \, \eta \, \mathfrak{t} \, \mu_2 - 27 \\
& \eta \, \eta \, \mathfrak{t} \, \mu_2 - 24 \, \eta^2 \, \eta \, \mathfrak{t} \, \mu_2 - 192 \, \eta \, \text{Op} \, \mu_2 - 960 \, \eta^2 \, \text{Op} \, \mu_2 - 960 \\
& \eta^3 \, \text{Op} \, \mu_2 - 48 \, \eta \, \mathfrak{t} \, \text{Op} \, \mu_2 - 96 \, \eta \, \eta \, \mathfrak{t} \, \text{Op} \, \mu_2 + 56 \, \eta \, \mu_1 \, \mu_2 + 12 \, \eta^2 \\
& \mu_1 \, \mu_2 - 204 \, \eta^3 \, \mu_1 \, \mu_2 - 240 \, \eta^4 \, \mu_1 \, \mu_2 + 38 \, \eta \, \mathfrak{t} \, \mu_1 \, \mu_2 + 117 \, \eta \\
& \eta \, \mathfrak{t} \, \mu_1 \, \mu_2 + 192 \, \eta^2 \, \eta \, \mathfrak{t} \, \mu_1 \, \mu_2 + 120 \, \eta^3 \, \eta \, \mathfrak{t} \, \mu_1 \, \mu_2 - 192 \, \eta \, \text{Op} \\
& \mu_1 \, \mu_2 - 960 \, \eta^2 \, \text{Op} \, \mu_1 \, \mu_2 - 960 \, \eta^3 \, \text{Op} \, \mu_1 \, \mu_2 - 48 \, \eta \, \mathfrak{t} \, \text{Op} \, \mu_1 \\
& \mu_2 - 96 \, \eta \, \eta \, \mathfrak{t} \, \text{Op} \, \mu_1 \, \mu_2 - 288 \, \eta \, \text{Op} \, \mu_2^2 - 1440 \, \eta^2 \, \text{Op} \, \mu_2^2 - 1440 \\
& \eta^3 \, \text{Op} \, \mu_2^2 - 72 \, \eta \, \mathfrak{t} \, \text{Op} \, \mu_2^2 - 144 \, \eta \, \eta \, \mathfrak{t} \, \text{Op} \, \mu_2^2 + w^4 (-1 + \eta)^4 \\
& \left. \left( 12 \, \eta^3 (1 + \mu_1) - 12 \, \eta^2 (-1 + \eta \, \mathfrak{t} - 5 \, \mu_1 + \eta \, \mathfrak{t} \, \mu_1 - 4 \, \mu_1^2 + 3 \, \mu_1 \, \mu_2) + \right. \right. \\
& 2 \times (5 + 3 \, \mu_1^2 + 11 \, \mu_2 + \mu_1 (8 + 5 \, \mu_2) - \\
& 4 \, \text{Op} (5 + 5 \, \mu_1^2 + 12 \, \mu_2 + 18 \, \mu_2^2 + 2 \, \mu_1 (5 + 6 \, \mu_2)) - \\
& 2 \, \eta (-16 - 37 \, \mu_1 - 21 \, \mu_1^2 - 33 \, \mu_2 + 27 \, \mu_1 \, \mu_2 + 6 \, \eta \, \mathfrak{t} (1 + \mu_1 - 3 \, \mu_1 \, \mu_2) + \\
& 8 \, \text{Op} (5 + 5 \, \mu_1^2 + 12 \, \mu_2 + 18 \, \mu_2^2 + 2 \, \mu_1 (5 + 6 \, \mu_2)) - \\
& \eta \, \mathfrak{t} (12 - 38 \, \mu_1^2 + \mu_1 (22 - 17 \, \mu_2) - 5 \, \mu_2 + 4 \, \text{Op} (4 + 4 \, \mu_1^2 + \\
& 6 \, \mu_2 + 9 \, \mu_2^2 + \mu_1 (8 + 6 \, \mu_2))) \left. \right) - w (-1 + \eta) \times \\
& (90 \, \eta^5 (1 + \mu_1) + 10 \, \eta^4 (20 + 27 \, \mu_1^2 - 9 \, \eta \, \mathfrak{t} (1 + \mu_1) + \mu_1 (65 - 36 \, \mu_2)) - \\
& 4 \times ((1 + \mu_1) \times (-5 + \mu_1 - 3 \, \mu_2) + 2 \, \text{Op} (5 + 5 \, \mu_1^2 + 12 \, \mu_2 + \\
& 18 \, \mu_2^2 + 2 \, \mu_1 (5 + 6 \, \mu_2))) - 12 \, \eta^2 (-34 - 85 \, \mu_1 - 21 \, \mu_1^2 - \\
& 62 \, \mu_2 + 34 \, \mu_1 \, \mu_2 + \eta \, \mathfrak{t} (11 - 8 \, \mu_1^2 + \mu_1 (27 - 44 \, \mu_2) + 4 \, \mu_2) +
\end{aligned}$$

$$\begin{aligned}
& 20 \, \theta p \left( 5 + 5 \, \mu 1^2 + 12 \, \mu 2 + 18 \, \mu 2^2 + 2 \, \mu 1 \left( 5 + 6 \, \mu 2 \right) \right) - 4 \, \eta^3 \\
& \left( -63 - 313 \, \mu 1 - 130 \, \mu 1^2 + \eta t \left( 50 - 6 \, \mu 1^2 + \mu 1 \left( 44 - 60 \, \mu 2 \right) \right) - 106 \, \mu 2 + \right. \\
& \quad \left. 176 \, \mu 1 \, \mu 2 + 40 \, \theta p \left( 5 + 5 \, \mu 1^2 + 12 \, \mu 2 + 18 \, \mu 2^2 + 2 \, \mu 1 \left( 5 + 6 \, \mu 2 \right) \right) \right) - \\
& \eta t \left( 100 - 96 \, \mu 1^2 + \mu 1 \left( 148 - 139 \, \mu 2 \right) + 29 \, \mu 2 + 28 \, \theta p \right. \\
& \quad \left. \left( 4 + 4 \, \mu 1^2 + 6 \, \mu 2 + 9 \, \mu 2^2 + \mu 1 \left( 8 + 6 \, \mu 2 \right) \right) \right) - \\
& \eta \left( \eta t \left( 204 + 460 \, \mu 1 - 320 \, \mu 1^2 + 81 \, \mu 2 - 423 \, \mu 1 \, \mu 2 + 48 \, \theta p \right. \right. \\
& \quad \left. \left( 4 + 8 \, \mu 1 + 4 \, \mu 1^2 + 6 \, \mu 2 + 6 \, \mu 1 \, \mu 2 + 9 \, \mu 2^2 \right) \right) + \\
& \quad \left. 4 \times \left( -54 - 75 \, \mu 1 - 3 \, \mu 1^2 - 65 \, \mu 2 - 17 \, \mu 1 \, \mu 2 + 24 \, \theta p \right. \right. \\
& \quad \left. \left( 5 + 5 \, \mu 1^2 + 12 \, \mu 2 + 18 \, \mu 2^2 + 2 \, \mu 1 \left( 5 + 6 \, \mu 2 \right) \right) \right) \right) + w^2 \\
& (-1 + \eta)^2 \left( 46 + 58 \, \mu 1 + 30 \, \eta^5 \left( 1 + \mu 1 \right) - 10 \, \eta^4 \left( 3 \, \eta t \left( 1 + \mu 1 \right) - \right. \right. \\
& \quad \left. \left. 4 \times \left( 4 + 3 \, \mu 1^2 + \mu 1 \left( 7 - 3 \, \mu 2 \right) \right) \right) + 50 \, \mu 2 + 14 \, \mu 1 \, \mu 2 - \right. \\
& \quad \left. 24 \, \theta p \left( 5 + 5 \, \mu 1^2 + 12 \, \mu 2 + 18 \, \mu 2^2 + 2 \, \mu 1 \left( 5 + 6 \, \mu 2 \right) \right) - \right. \\
& \quad \left. 4 \, \eta^3 \left( -70 - 255 \, \mu 1 - 125 \, \mu 1^2 + \eta t \left( 40 + \mu 1 \left( 40 - 30 \, \mu 2 \right) \right) - 55 \, \mu 2 + \right. \right. \\
& \quad \left. \left. 161 \, \mu 1 \, \mu 2 + 20 \, \theta p \left( 5 + 5 \, \mu 1^2 + 12 \, \mu 2 + 18 \, \mu 2^2 + 2 \, \mu 1 \left( 5 + 6 \, \mu 2 \right) \right) \right) - \right. \\
& \quad \left. 12 \, \eta^2 \left( -38 - 106 \, \mu 1 - 38 \, \mu 1^2 - 65 \, \mu 2 + 61 \, \mu 1 \, \mu 2 + \right. \right. \\
& \quad \left. \left. \eta t \left( 15 - 4 \, \mu 1^2 + \mu 1 \left( 23 - 40 \, \mu 2 \right) + 2 \, \mu 2 \right) + \right. \right. \\
& \quad \left. \left. 20 \, \theta p \left( 5 + 5 \, \mu 1^2 + 12 \, \mu 2 + 18 \, \mu 2^2 + 2 \, \mu 1 \left( 5 + 6 \, \mu 2 \right) \right) \right) - \right. \\
& \quad \left. \eta t \left( 124 - 164 \, \mu 1^2 + \mu 1 \left( 224 - 181 \, \mu 2 \right) + 23 \, \mu 2 + 36 \, \theta p \right. \right. \\
& \quad \left. \left. \left( 4 + 4 \, \mu 1^2 + 6 \, \mu 2 + 9 \, \mu 2^2 + \mu 1 \left( 8 + 6 \, \mu 2 \right) \right) \right) - \right. \\
& \quad \left. \eta \left( 3 \, \eta t \left( 80 + 164 \, \mu 1 - 108 \, \mu 1^2 + 27 \, \mu 2 - 177 \, \mu 1 \, \mu 2 + 16 \, \theta p \right. \right. \right. \\
& \quad \left. \left. \left( 4 + 8 \, \mu 1 + 4 \, \mu 1^2 + 6 \, \mu 2 + 6 \, \mu 1 \, \mu 2 + 9 \, \mu 2^2 \right) \right) + \right. \\
& \quad \left. \left. 2 \times \left( -155 - 278 \, \mu 1 - 51 \, \mu 1^2 - 249 \, \mu 2 + 69 \, \mu 1 \, \mu 2 + 80 \, \theta p \right. \right. \right. \\
& \quad \left. \left. \left( 5 + 5 \, \mu 1^2 + 12 \, \mu 2 + 18 \, \mu 2^2 + 2 \, \mu 1 \left( 5 + 6 \, \mu 2 \right) \right) \right) \right) \right) - w^3 \\
& (-1 + \eta)^3 \left( 40 + 62 \, \mu 1 + 10 \, \mu 1^2 + 40 \, \eta^4 \left( 1 + \mu 1 \right) + 60 \, \mu 2 + 12 \, \mu 1 \, \mu 2 - \right. \\
& \quad \left. 24 \, \theta p \left( 5 + 5 \, \mu 1^2 + 12 \, \mu 2 + 18 \, \mu 2^2 + 2 \, \mu 1 \left( 5 + 6 \, \mu 2 \right) \right) - \right. \\
& \quad \left. 4 \, \eta^3 \left( -21 - 40 \, \mu 1^2 + 10 \, \eta t \left( 1 + \mu 1 \right) + \mu 1 \left( -61 + 36 \, \mu 2 \right) \right) - \right. \\
& \quad \left. 4 \, \eta^2 \left( \eta t \left( 21 + \mu 1 \left( 21 - 36 \, \mu 2 \right) \right) - 3 \times \left( 14 + 23 \, \mu 1^2 + \mu 1 \left( 43 - 29 \, \mu 2 \right) + \right. \right. \right. \\
& \quad \left. \left. 22 \, \mu 2 \right) + 20 \, \theta p \left( 5 + 5 \, \mu 1^2 + 12 \, \mu 2 + 18 \, \mu 2^2 + 2 \, \mu 1 \left( 5 + 6 \, \mu 2 \right) \right) \right) - \right. \\
& \quad \left. \eta t \left( 66 - 128 \, \mu 1^2 + \mu 1 \left( 130 - 97 \, \mu 2 \right) - \mu 2 + 20 \, \theta p \left( 4 + 4 \, \mu 1^2 + 6 \, \mu 2 + \right. \right. \right. \\
& \quad \left. \left. 9 \, \mu 2^2 + \mu 1 \left( 8 + 6 \, \mu 2 \right) \right) \right) - \eta \left( 6 \times \left( -31 - 63 \, \mu 1 - 20 \, \mu 1^2 - 56 \, \mu 2 + \right. \right. \\
& \quad \left. \left. 34 \, \mu 1 \, \mu 2 + 16 \, \theta p \left( 5 + 5 \, \mu 1^2 + 12 \, \mu 2 + 18 \, \mu 2^2 + 2 \, \mu 1 \left( 5 + 6 \, \mu 2 \right) \right) \right) \right) + \\
& \quad \left. \eta t \left( 16 \, \theta p \left( 4 + 4 \, \mu 1^2 + 6 \, \mu 2 + 9 \, \mu 2^2 + \mu 1 \left( 8 + 6 \, \mu 2 \right) \right) - \right. \right. \\
& \quad \left. \left. 3 \times \left( 36 \, \mu 1^2 - 9 \times \left( 4 + \mu 2 \right) + \mu 1 \left( -64 + 87 \, \mu 2 \right) \right) \right) \right) \right) + \\
& (-1 + \eta t) \, \theta l \left( -10 - 60 \, \eta - 60 \, \eta^2 + 10 \, \theta p + 142 \, \eta \, \theta p + 428 \, \eta^2 \, \theta p + 380 \right. \\
& \quad \eta^3 \, \theta p + 60 \, \eta^4 \, \theta p - 8 \, \mu 1 - 64 \, \eta \, \mu 1 - 164 \, \eta^2 \, \mu 1 - 80 \, \eta^3 \, \mu 1 + 16 \\
& \quad \eta^4 \, \mu 1 + 8 \, \theta p \, \mu 1 + 248 \, \eta \, \theta p \, \mu 1 + 802 \, \eta^2 \, \theta p \, \mu 1 + 528 \, \eta^3 \, \theta p \\
& \quad \mu 1 - 90 \, \eta^4 \, \theta p \, \mu 1 + 2 \, \mu 1^2 - 4 \, \eta \, \mu 1^2 + 28 \, \eta^2 \, \mu 1^2 + 16 \, \eta^3 \, \mu 1^2 + 16 \\
& \quad \eta^4 \, \mu 1^2 - 2 \, \theta p \, \mu 1^2 + 70 \, \eta \, \theta p \, \mu 1^2 + 302 \, \eta^2 \, \theta p \, \mu 1^2 + 268 \, \eta^3 \\
& \quad \theta p \, \mu 1^2 + 30 \, \eta^4 \, \theta p \, \mu 1^2 - 5 \, \mu 2 - 20 \, \eta \, \mu 2 - 15 \, \eta^2 \, \mu 2 + 26 \, \theta p \\
& \quad \mu 2 + 324 \, \eta \, \theta p \, \mu 2 + 746 \, \eta^2 \, \theta p \, \mu 2 + 408 \, \eta^3 \, \theta p \, \mu 2 - 20 \, \eta^4 \, \theta p \\
& \quad \mu 2 + 19 \, \mu 1 \, \mu 2 + 76 \, \eta \, \mu 1 \, \mu 2 + 57 \, \eta^2 \, \mu 1 \, \mu 2 + 2 \, \theta p \, \mu 1 \, \mu 2 + 264 \\
& \quad \eta \, \theta p \, \mu 1 \, \mu 2 + 1142 \, \eta^2 \, \theta p \, \mu 1 \, \mu 2 + 1440 \, \eta^3 \, \theta p \, \mu 1 \, \mu 2 + 580 \\
& \quad \eta^4 \, \theta p \, \mu 1 \, \mu 2 + 72 \, \eta \, \theta p \, \mu 2^2 + 144 \, \eta^2 \, \theta p \, \mu 2^2 + 2 \, w^4 \, (-1 + \eta)^4
\end{aligned}$$

$$\begin{aligned}
& \left( -5 - 10 \mu_1 + \mu_1^2 + 5 \mu_2 + 5 \mu_1 \mu_2 + 5 \eta \left( -2 + 4 \mu_1^2 + \mu_1 (-4 + \mu_2) + \mu_2 \right) + \right. \\
& \quad 4 \operatorname{erf} \left( 5 + 5 \mu_1^2 + 12 \mu_2 + 10 \mu_1 (1 + 3 \mu_2) \right) + \\
& \quad \left. 6 \eta \operatorname{erf} \left( 8 + 8 \mu_1^2 + 18 \mu_2 + 3 \mu_2^2 + 2 \mu_1 (8 + 21 \mu_2) \right) \right) - 5 \\
& \operatorname{erf} \mathfrak{z}_1 - 30 \eta \operatorname{erf} \mathfrak{z}_1 - 30 \eta^2 \operatorname{erf} \mathfrak{z}_1 - 4 \operatorname{erf} \mu_1 \mathfrak{z}_1 - 50 \eta \operatorname{erf} \mu_1 \\
& \mathfrak{z}_1 - 129 \eta^2 \operatorname{erf} \mu_1 \mathfrak{z}_1 - 96 \eta^3 \operatorname{erf} \mu_1 \mathfrak{z}_1 - 10 \eta^4 \operatorname{erf} \mu_1 \mathfrak{z}_1 + \operatorname{erf} \\
& \mu_1^2 \mathfrak{z}_1 - 2 \eta \operatorname{erf} \mu_1^2 \mathfrak{z}_1 - 27 \eta^2 \operatorname{erf} \mu_1^2 \mathfrak{z}_1 - 36 \eta^3 \operatorname{erf} \mu_1^2 \\
& \mathfrak{z}_1 - 10 \eta^4 \operatorname{erf} \mu_1^2 \mathfrak{z}_1 - 5 \operatorname{erf} \mu_2 \mathfrak{z}_1 - 30 \eta \operatorname{erf} \mu_2 \mathfrak{z}_1 - 30 \eta^2 \\
& \operatorname{erf} \mu_2 \mathfrak{z}_1 - 5 \operatorname{erf} \mu_1 \mu_2 \mathfrak{z}_1 - 30 \eta \operatorname{erf} \mu_1 \mu_2 \mathfrak{z}_1 - 30 \eta^2 \operatorname{erf} \\
& \mu_1 \mu_2 \mathfrak{z}_1 + 5 \operatorname{erf} \mathfrak{z}_2 + 30 \eta \operatorname{erf} \mathfrak{z}_2 + 30 \eta^2 \operatorname{erf} \mathfrak{z}_2 + 4 \operatorname{erf} \mu_1 \\
& \mathfrak{z}_2 + 40 \eta \operatorname{erf} \mu_1 \mathfrak{z}_2 + 87 \eta^2 \operatorname{erf} \mu_1 \mathfrak{z}_2 + 44 \eta^3 \operatorname{erf} \mu_1 \mathfrak{z}_2 - 10 \\
& \eta^4 \operatorname{erf} \mu_1 \mathfrak{z}_2 - \operatorname{erf} \mu_1^2 \mathfrak{z}_2 - 8 \eta \operatorname{erf} \mu_1^2 \mathfrak{z}_2 - 15 \eta^2 \operatorname{erf} \mu_1^2 \\
& \mathfrak{z}_2 - 16 \eta^3 \operatorname{erf} \mu_1^2 \mathfrak{z}_2 - 10 \eta^4 \operatorname{erf} \mu_1^2 \mathfrak{z}_2 + 5 \operatorname{erf} \mu_2 \mathfrak{z}_2 + 30 \\
& \eta \operatorname{erf} \mu_2 \mathfrak{z}_2 + 30 \eta^2 \operatorname{erf} \mu_2 \mathfrak{z}_2 - 7 \operatorname{erf} \mu_1 \mu_2 \mathfrak{z}_2 - 6 \eta \operatorname{erf} \mu_1 \\
& \mu_2 \mathfrak{z}_2 + 102 \eta^2 \operatorname{erf} \mu_1 \mu_2 \mathfrak{z}_2 + 120 \eta^3 \operatorname{erf} \mu_1 \mu_2 \mathfrak{z}_2 - w^2 \\
& (-1 + \eta)^2 \left( -3 \times \left( 4 \mu_1^2 + 5 \times (-4 + \mu_2) + \mu_1 (-28 + 29 \mu_2) \right) - \right. \\
& \quad \operatorname{erf} \left( 134 - 15 \mathfrak{z}_1 - 5 \mu_2 (-70 + 3 \mathfrak{z}_1 - 3 \mathfrak{z}_2) - 26 \mu_1 (-9 + \mathfrak{z}_1 - \mathfrak{z}_2) + \right. \\
& \quad \left. \mu_1^2 (88 + \mathfrak{z}_1 - \mathfrak{z}_2) + 15 \mathfrak{z}_2 + \mu_1 \mu_2 (542 - 15 \mathfrak{z}_1 + 3 \mathfrak{z}_2) \right) + \\
& \quad \left. \eta^2 \left( -9 \times \left( 12 \mu_1^2 - 5 \times (4 + \mu_2) + \mu_1 (-52 + 19 \mu_2) \right) + \right. \right. \\
& \quad \left. 2 \operatorname{erf} \left( -678 - 216 \mu_2^2 + 45 \mathfrak{z}_1 + \mu_1 \mu_2 (-3030 + 45 \mathfrak{z}_1 - 81 \mathfrak{z}_2) + \right. \right. \\
& \quad \left. 2 \mu_1 (-637 + 66 \mathfrak{z}_1 - 54 \mathfrak{z}_2) + 15 \mu_2 (-74 + 3 \mathfrak{z}_1 - 3 \mathfrak{z}_2) - \right. \\
& \quad \left. \left. 45 \mathfrak{z}_2 + \mu_1^2 (-632 + 15 \mathfrak{z}_1 + 9 \mathfrak{z}_2) \right) \right) + \eta \left( -60 \mu_1^2 + \right. \\
& \quad \left. 6 \mu_1 (76 - 43 \mu_2) + 30 \times (8 + \mu_2) + \operatorname{erf} \mu_1^2 (-788 + 3 \mathfrak{z}_1 + 9 \mathfrak{z}_2) + \right. \\
& \quad \left. \operatorname{erf} \mu_1 (-1822 + 183 \mathfrak{z}_1 + 90 \mu_2 \mathfrak{z}_1 - 171 \mathfrak{z}_2 - 54 \mu_2 (69 + \mathfrak{z}_2)) - \right. \\
& \quad \left. 2 \operatorname{erf} \left( 499 + 162 \mu_2^2 - 45 \mathfrak{z}_1 + 45 \mathfrak{z}_2 + \mu_2 (963 - 45 \mathfrak{z}_1 + 45 \mathfrak{z}_2) \right) \right) + \\
& \quad \left. 2 \eta^3 \left( -8 \times (-5 + \mu_1) \mu_1 + 5 \operatorname{erf} \left( -30 - 38 \mu_2 + \mu_1^2 (-44 + 3 \mathfrak{z}_1 + \mathfrak{z}_2) - \right. \right. \right. \\
& \quad \left. \left. \mu_1 (62 + 254 \mu_2 - 9 \mathfrak{z}_1 + 5 \mathfrak{z}_2 + 12 \mu_2 \mathfrak{z}_2) \right) \right) \right) - \\
& w^3 (-1 + \eta)^3 \left( -40 - 68 \mu_1 + 8 \mu_1^2 + 25 \mu_2 + 49 \mu_1 \mu_2 + \operatorname{erf} \right. \\
& \left( 104 \mu_1^2 + 5 \times (24 - \mathfrak{z}_1 + \mathfrak{z}_2) + \mu_2 (304 - 5 \mathfrak{z}_1 + 5 \mathfrak{z}_2) + \right. \\
& \quad \left. \mu_1 (224 - 11 \mathfrak{z}_1 + 11 \mathfrak{z}_2 + \mu_2 (640 - 5 \mathfrak{z}_1 + 5 \mathfrak{z}_2)) \right) + \\
& \quad \left. \eta^2 \left( 3 \times \left( 12 \mu_1^2 - 5 \times (4 + \mu_2) + \mu_1 (-52 + 19 \mu_2) \right) + 2 \operatorname{erf} \right. \right. \\
& \quad \left( 232 + 240 \mu_1^2 + 72 \mu_2^2 - 15 \mathfrak{z}_1 + 15 \mathfrak{z}_2 + \mu_2 (376 - 15 \mathfrak{z}_1 + 15 \mathfrak{z}_2) + \right. \\
& \quad \left. \mu_1 (472 - 33 \mathfrak{z}_1 + 33 \mathfrak{z}_2 + \mu_2 (1144 - 15 \mathfrak{z}_1 + 15 \mathfrak{z}_2)) \right) \right) + \\
& \quad \left. 2 \eta \left( -60 - 128 \mu_1 + 46 \mu_1^2 + 5 \mu_2 + 53 \mu_1 \mu_2 + \operatorname{erf} \left( 268 \mu_1^2 + \right. \right. \right. \\
& \quad \left. 5 \times (56 + 18 \mu_2^2 - 3 \mathfrak{z}_1 + 3 \mathfrak{z}_2 + \mu_2 (112 - 3 \mathfrak{z}_1 + 3 \mathfrak{z}_2)) + \right. \\
& \quad \left. \left. \mu_1 (548 - 33 \mathfrak{z}_1 + 33 \mathfrak{z}_2 + \mu_2 (1352 - 15 \mathfrak{z}_1 + 15 \mathfrak{z}_2)) \right) \right) \right) + w \\
& (-1 + \eta) \times \left( 40 + 44 \mu_1 - 8 \mu_1^2 + 5 \mu_2 - 67 \mu_1 \mu_2 + 2 \eta^4 \right. \\
& \quad \left( 10 \operatorname{erf} \mu_2 + \mu_1^2 (-8 + 5 \operatorname{erf} (-3 + \mathfrak{z}_1 + \mathfrak{z}_2)) + \right. \\
& \quad \mu_1 (-8 + 5 \operatorname{erf} (15 - 58 \mu_2 + \mathfrak{z}_1 + \mathfrak{z}_2)) - \operatorname{erf} \left( 2 \mu_1^2 (11 + \mathfrak{z}_1 - \mathfrak{z}_2) + \right. \\
& \quad \left. \mu_1 (94 - 19 \mathfrak{z}_1 + 19 \mathfrak{z}_2 - 3 \mu_2 (-48 + 5 \mathfrak{z}_1 + 3 \mathfrak{z}_2)) + \right. \\
& \quad \left. 3 \times (5 \times (4 - \mathfrak{z}_1 + \mathfrak{z}_2) + \mu_2 (56 - 5 \mathfrak{z}_1 + 5 \mathfrak{z}_2)) \right) + 2 \eta^3 \\
& \quad \left( -16 \times (-5 + \mu_1) \mu_1 + \operatorname{erf} \left( -340 - 394 \mu_2 + \mu_1^2 (-354 + 33 \mathfrak{z}_1 + 13 \mathfrak{z}_2) - \right. \right. \\
& \quad \left. \mu_1 (574 + 1990 \mu_2 - 93 \mathfrak{z}_1 + 47 \mathfrak{z}_2 + 120 \mu_2 \mathfrak{z}_2) \right) \right) + \eta^2 \left( -100 \mu_1^2 + \right. \\
& \quad \mu_1 (476 - 171 \mu_2) + 45 \times (4 + \mu_2) + 3 \operatorname{erf} \left( \mu_1^2 (-362 + 19 \mathfrak{z}_1 + 11 \mathfrak{z}_2) + \right. \\
& \quad \left. \mu_1 (-818 + 109 \mathfrak{z}_1 + 30 \mu_2 \mathfrak{z}_1 - 79 \mathfrak{z}_2 - 78 \mu_2 (21 + \mathfrak{z}_2)) - \right.
\end{aligned}$$

$$\begin{aligned}
& 6 \times (76 + 24 \mu_2^2 - 5 \mathfrak{z}1 + 5 \mathfrak{z}2 + \mu_2 (123 - 5 \mathfrak{z}1 + 5 \mathfrak{z}2)) + \\
& \eta (-4 \mu_1^2 + \mu_1 (304 - 238 \mu_2) + 50 \times (4 + \mu_2) + \mathfrak{op} \\
& (\mu_1 (-1166 + 167 \mathfrak{z}1 + 2 \mu_2 (-895 + 45 \mathfrak{z}1 - 9 \mathfrak{z}2) - 145 \mathfrak{z}2) + \\
& \mu_1^2 (-418 + 5 \mathfrak{z}1 + 17 \mathfrak{z}2) - 2 \times (338 + 126 \mu_2^2 - \\
& 45 \mathfrak{z}1 + 45 \mathfrak{z}2 + \mu_2 (673 - 45 \mathfrak{z}1 + 45 \mathfrak{z}2))) - \\
& x^2 (-1 + \eta)^2 (4 w^2 (3 - 5 w + 2 w^2) \eta^9 \mathfrak{op} (1 + \mu_1) - 4 w \eta^8 \mathfrak{op} (9 \times (1 + \mu_1) + \\
& w^3 (7 - \mu_1 - 8 \mu_1^2 + 2 \eta t (1 + \mu_1) + 9 \mu_1 \mu_2) + w \\
& (-11 - 23 \mu_1 - 12 \mu_1^2 + 3 \eta t (1 + \mu_1) + 15 \mu_1 \mu_2) - w^2 \\
& (6 - 14 \mu_1 - 20 \mu_1^2 + 5 \eta t (1 + \mu_1) + 24 \mu_1 \mu_2)) - \\
& 2 \eta^7 \mathfrak{op} (-12 \times (1 + \mu_1) + 2 w (7 + 27 \mu_1^2 - 9 \eta t (1 + \mu_1) + \mu_1 (52 - 45 \mu_2)) + \\
& 2 w^3 (6 - 16 \mu_1 - 34 \mu_1^2 + 44 \mu_2 + 23 \mu_1 \mu_2 + 6 \eta t (1 + \mu_1 + 4 \mu_1 \mu_2) - \\
& 20 \mathfrak{op} (5 + 5 \mu_1^2 + 12 \mu_2 + 18 \mu_2^2 + 2 \mu_1 (5 + 6 \mu_2))) + w^2 \\
& (17 - 96 \mu_1 - 53 \mu_1^2 + \eta t (22 + \mu_1 (22 - 30 \mu_2)) - 55 \mu_2 + 113 \mu_1 \mu_2 + \\
& 30 \mathfrak{op} (5 + 5 \mu_1^2 + 12 \mu_2 + 18 \mu_2^2 + 2 \mu_1 (5 + 6 \mu_2))) + w^4 \\
& (-27 + 32 \mu_1 + 59 \mu_1^2 - 33 \mu_2 - 57 \mu_1 \mu_2 + 12 \mathfrak{op} (5 + 5 \mu_1^2 + 12 \mu_2 + \\
& 18 \mu_2^2 + 2 \mu_1 (5 + 6 \mu_2)) - 2 \eta t (7 + \mu_1 (7 + 9 \mu_2))) + \\
& (1 + w) (-w (\mathfrak{ol} (5 + 24 \mathfrak{op}) \times (1 + \mu_1) \mu_2 + 2 w (-2 \mathfrak{op}^2 (5 + 5 \mu_1^2 + \\
& 12 \mu_2 + 18 \mu_2^2 + 2 \mu_1 (5 + 6 \mu_2)) + \mathfrak{ol} \\
& (5 \times (1 + \mu_1) \mu_2 + 2 \mathfrak{op} (5 + 8 \mu_1 + 3 \mu_1^2 + 18 \mu_2 + 24 \mu_1 \mu_2))) + \\
& w^2 (-4 \mathfrak{op}^2 (5 + 5 \mu_1^2 + 12 \mu_2 + 18 \mu_2^2 + 2 \mu_1 (5 + 6 \mu_2)) + \\
& \mathfrak{ol} (5 \times (1 + \mu_1) \mu_2 + 4 \mathfrak{op} (5 + 10 \mu_1 + 5 \mu_1^2 + 12 \mu_2 + 30 \mu_1 \mu_2)))) + \\
& \eta t (5 w (1 + w)^2 \mathfrak{ol} (1 + \mu_1) \mu_2 + 4 (1 + w)^2 (1 + 2 w) \mathfrak{op}^2 \\
& (4 + 4 \mu_1^2 + 6 \mu_2 + 9 \mu_2^2 + \mu_1 (8 + 6 \mu_2)) + \mathfrak{op} (10 + 8 \mu_1 - 2 \mu_1^2 + 5 \mu_2 - \\
& 19 \mu_1 \mu_2 - 6 w (-5 + 3 \mu_1^2 - 4 \mathfrak{ol} \mu_2 + \mu_1 (-6 - 4 \times (-2 + \mathfrak{ol}) \mu_2)) + \\
& w^2 (30 + 48 \mu_1 - 30 \mu_1^2 - 15 \mu_2 - 39 \mu_1 \mu_2 + 4 \mathfrak{ol} (5 + 3 \mu_1^2 + 18 \mu_2 + \\
& 8 \mu_1 (1 + 3 \mu_2))) + 2 w^3 (5 - 7 \mu_1^2 - 5 \mu_1 (-2 + \mu_2) - \\
& 5 \mu_2 + 2 \mathfrak{ol} (5 + 5 \mu_1^2 + 12 \mu_2 + 10 \mu_1 (1 + 3 \mu_2)))) - \\
& \eta^2 (\mathfrak{op} (60 - 120 \mathfrak{op} + 48 \mu_1 - 88 \eta t \mu_1 - 240 \mathfrak{op} \mu_1 - 12 \mu_1^2 + 56 \eta t \mu_1^2 - \\
& 120 \mathfrak{op} \mu_1^2 + 28 \mu_2 - 7 \eta t \mu_2 - 288 \mathfrak{op} \mu_2 + 76 \mu_1 \mu_2 + 41 \eta t \mu_1 \mu_2 - \\
& 288 \mathfrak{op} \mu_1 \mu_2 - 432 \mathfrak{op} \mu_2^2 + 2 w (68 + 118 \mu_1 + 14 \mu_1^2 + 104 \mu_2 + \\
& 20 \mu_1 \mu_2 + 3 \eta t (26 + 8 \mu_1^2 + \mu_1 (14 - 11 \mu_2) + 5 \mu_2) - \\
& 48 \mathfrak{op} (5 + 5 \mu_1^2 + 12 \mu_2 + 18 \mu_2^2 + 2 \mu_1 (5 + 6 \mu_2)) + \\
& 38 \eta t \mathfrak{op} (4 + 4 \mu_1^2 + 6 \mu_2 + 9 \mu_2^2 + \mu_1 (8 + 6 \mu_2)) - \\
& 2 w^4 (33 + 42 \mu_1 + 9 \mu_1^2 + 77 \mu_2 + 83 \mu_1 \mu_2 - 28 \mathfrak{op} (5 + 5 \mu_1^2 + \\
& 12 \mu_2 + 18 \mu_2^2 + 2 \mu_1 (5 + 6 \mu_2)) + \eta t (-4 - 4 \mu_1 + 90 \mu_1^2 - 25 \mu_2 + \\
& 17 \mu_1 \mu_2 + 10 \mathfrak{op} (4 + 8 \mu_1 + 4 \mu_1^2 + 6 \mu_2 + 6 \mu_1 \mu_2 + 9 \mu_2^2))) + \\
& 2 w^2 (19 + 106 \mu_1 + 51 \mu_1^2 + 99 \mu_2 - 123 \mu_1 \mu_2 - 18 \mathfrak{op} \\
& (5 + 5 \mu_1^2 + 12 \mu_2 + 18 \mu_2^2 + 2 \mu_1 (5 + 6 \mu_2)) + \\
& 3 \eta t (54 + 100 \mu_1 - 44 \mu_1^2 + 17 \mu_2 - 49 \mu_1 \mu_2 + \\
& 24 \mathfrak{op} (4 + 8 \mu_1 + 4 \mu_1^2 + 6 \mu_2 + 6 \mu_1 \mu_2 + 9 \mu_2^2))) + \\
& w^3 (8 \times (5 \mu_1^2 - 14 \mu_1 (1 + 3 \mu_2) - 2 \times (8 + 9 \mu_2) + 12 \mathfrak{op} \\
& (5 + 5 \mu_1^2 + 12 \mu_2 + 18 \mu_2^2 + 2 \mu_1 (5 + 6 \mu_2))) +
\end{aligned}$$



$$\begin{aligned}
& \eta t \left( 180 + 440 \mu_1 - 436 \mu_1^2 + 115 \mu_2 - 221 \mu_1 \mu_2 + \right. \\
& \quad \left. 48 \theta p \left( 4 + 4 \mu_1^2 + 6 \mu_2 + 9 \mu_2^2 + \mu_1 (8 + 6 \mu_2) \right) \right) + \\
& (-1 + \eta t) \theta l \left( 2 \times \left( 7 \mu_1^2 + \mu_1 (16 - 19 \mu_2) + 5 \times (3 + \mu_2) \right) + \right. \\
& \quad w^4 \left( -54 \mu_1^2 + 5 \mu_1 (-12 + \mu_2) + 5 \times (-6 + \mu_2) + \right. \\
& \quad \left. 4 \theta p \left( 80 + 80 \mu_1^2 + 174 \mu_2 + 45 \mu_2^2 + 10 \mu_1 (16 + 39 \mu_2) \right) \right) + \\
& \quad w^3 \left( -60 - 100 \mu_1^2 + 25 \mu_2 + \mu_1 (-76 + 49 \mu_2) + 12 \theta p \right. \\
& \quad \left. (28 + 21 \mu_1^2 + 85 \mu_2 + 18 \mu_2^2 + \mu_1 (49 + 115 \mu_2)) \right) + \\
& \quad w^2 \left( 6 \times (-4 \mu_1^2 + 5 \mu_2 + 5 \mu_1 (2 + \mu_2)) + \theta p (-642 - 324 \mu_2^2 + \right. \\
& \quad \left. 30 \mathfrak{e}1 + \mu_1 (-1246 + 79 \mathfrak{e}1 + \mu_2 (-2470 + 30 \mathfrak{e}1 - 42 \mathfrak{e}2) - 67 \mathfrak{e}2) + \right. \\
& \quad \left. 10 \mu_2 (-79 + 3 \mathfrak{e}1 - 3 \mathfrak{e}2) - 30 \mathfrak{e}2 + \mu_1^2 (-616 + 7 \mathfrak{e}1 + 5 \mathfrak{e}2)) \right) + \\
& \quad \theta p (-216 \mu_2^2 + 6 \times (-41 + 5 \mathfrak{e}1 - 5 \mathfrak{e}2) + 10 \mu_2 (-55 + 3 \mathfrak{e}1 - 3 \mathfrak{e}2) + \\
& \quad \mu_1^2 (-160 + \mathfrak{e}1 + 7 \mathfrak{e}2) + \mu_1 (-442 + 49 \mathfrak{e}1 - 41 \mathfrak{e}2 + \\
& \quad \mu_2 (-526 + 30 \mathfrak{e}1 + 6 \mathfrak{e}2)) \right) + 4 w \left( 15 + 27 \mu_1 + 9 \mu_1^2 + 5 \mu_2 - \right. \\
& \quad \left. 13 \mu_1 \mu_2 + \theta p (-144 \mu_2^2 + \mu_1^2 (2 \mathfrak{e}1 + 3 \times (-56 + \mathfrak{e}2)) + \right. \\
& \quad \left. \mu_2 (-412 + 15 \mathfrak{e}1 - 15 \mathfrak{e}2) + 15 \times (-15 + \mathfrak{e}1 - \mathfrak{e}2) + \right. \\
& \quad \left. \mu_1 (32 \mathfrak{e}1 + \mu_2 (-640 + 15 \mathfrak{e}1 - 9 \mathfrak{e}2) - 27 \times (15 + \mathfrak{e}2)) \right) \left. \right) + \\
& \eta \left( \theta p \left( \eta t (50 - 18 \mu_1^2 + \mu_1 (56 - 57 \mu_2) + 15 \mu_2 + 20 \theta p (4 + 4 \mu_1^2 + \right. \right. \\
& \quad \left. \left. 6 \mu_2 + 9 \mu_2^2 + \mu_1 (8 + 6 \mu_2)) \right) + \right. \\
& \quad w^2 \left( \eta t (68 - 76 \mu_1^2 + \mu_1 (196 - 101 \mu_2) + 91 \mu_2) + 60 \theta p \right. \\
& \quad \left( 5 + 5 \mu_1^2 + 12 \mu_2 + 18 \mu_2^2 + 2 \mu_1 (5 + 6 \mu_2) \right) - 4 \times \\
& \quad \left. (23 + 25 \mu_2 + \mu_1 (29 + 7 \mu_2)) \right) + \\
& \quad 4 w \left( 2 \times (1 + \mu_1) \times (-5 + \mu_1 - 3 \mu_2) + 6 \theta p (5 + 5 \mu_1^2 + 12 \mu_2 + \right. \\
& \quad \left. 18 \mu_2^2 + 2 \mu_1 (5 + 6 \mu_2)) + \eta t (30 + 52 \mu_1 - 17 \mu_1^2 + 12 \mu_2 - \right. \\
& \quad \left. 36 \mu_1 \mu_2 + 11 \theta p (4 + 8 \mu_1 + 4 \mu_1^2 + 6 \mu_2 + 6 \mu_1 \mu_2 + 9 \mu_2^2)) \right) - \\
& \quad 2 w^3 \left( 40 + 62 \mu_1 + 10 \mu_1^2 + 60 \mu_2 + 12 \mu_1 \mu_2 - 20 \theta p (5 + 5 \mu_1^2 + \right. \\
& \quad \left. 12 \mu_2 + 18 \mu_2^2 + 2 \mu_1 (5 + 6 \mu_2)) + \eta t (14 + 6 \mu_1 + 10 \mu_1^2 - 49 \mu_2 - \right. \\
& \quad \left. \mu_1 \mu_2 + 26 \theta p (4 + 8 \mu_1 + 4 \mu_1^2 + 6 \mu_2 + 6 \mu_1 \mu_2 + 9 \mu_2^2)) \right) - \\
& \quad 2 w^4 \left( \eta t (13 + 28 \mu_1 - 3 \mu_1^2 - 20 \mu_2 - 8 \mu_1 \mu_2 + 14 \theta p (4 + 8 \mu_1 + \right. \\
& \quad \left. 4 \mu_1^2 + 6 \mu_2 + 6 \mu_1 \mu_2 + 9 \mu_2^2)) + 2 \times (5 + 8 \mu_1 + 3 \mu_1^2 + 11 \mu_2 + \right. \\
& \quad \left. 5 \mu_1 \mu_2 - \theta p (5 + 5 \mu_1^2 + 12 \mu_2 + 18 \mu_2^2 + 2 \mu_1 (5 + 6 \mu_2)) \right) \left. \right) + \\
& (-1 + \eta t) \theta l \left( -10 - 8 \mu_1 + 2 \mu_1^2 - 5 \mu_2 + 19 \mu_1 \mu_2 + 2 w^4 (-5 \times \right. \\
& \quad \left. (1 + \mu_1) \times (1 + \mu_1 + \mu_2) + 36 \theta p (\mu_1^2 + (1 + \mu_2)^2 + \mu_1 (2 + 4 \mu_2)) \right) + \\
& \quad 2 \theta p (18 + 18 \mu_2^2 - 5 \mathfrak{e}1 + \mu_1 \mu_2 (24 - 5 \mathfrak{e}1 - 7 \mathfrak{e}2) + \mu_1^2 \\
& \quad (6 + \mathfrak{e}1 - \mathfrak{e}2) + 5 \mathfrak{e}2 + 4 \mu_1 (6 - \mathfrak{e}1 + \mathfrak{e}2) + \mu_2 (48 - 5 \mathfrak{e}1 + 5 \mathfrak{e}2)) + \\
& \quad w^2 \left( -3 \times (8 \mu_1^2 + \mu_1 (28 - 19 \mu_2) + 5 \times (4 + \mu_2)) + 2 \theta p (162 \mu_2^2 + \right. \\
& \quad \mu_1^2 (194 + \mathfrak{e}1 - \mathfrak{e}2) + 3 \times (82 - 5 \mathfrak{e}1 + 5 \mathfrak{e}2) + \mu_2 (536 - 15 \mathfrak{e}1 + 15 \\
& \quad \mathfrak{e}2) + \mu_1 (452 - 26 \mathfrak{e}1 + 26 \mathfrak{e}2 + \mu_2 (836 - 15 \mathfrak{e}1 + 3 \mathfrak{e}2)) \right) + \\
& \quad 2 w \left( -2 \mu_1^2 - 5 \times (4 + \mu_2) + \mu_1 (-22 + 31 \mu_2) + \theta p (2 \mu_1^2 (37 + \mathfrak{e}1 - \right. \\
& \quad \mathfrak{e}2) + \mu_1 (206 - 19 \mathfrak{e}1 + 19 \mathfrak{e}2 - 3 \mu_2 (-98 + 5 \mathfrak{e}1 + 3 \mathfrak{e}2)) + \\
& \quad \left. 3 \times (30 \mu_2^2 + 5 \times (8 - \mathfrak{e}1 + \mathfrak{e}2) + \mu_2 (98 - 5 \mathfrak{e}1 + 5 \mathfrak{e}2)) \right) + \\
& \quad 2 w^3 \left( -2 \times (7 \mu_1^2 - \mu_1 (-17 + \mu_2) + 5 \times (2 + \mu_2)) + \theta p \right. \\
& \quad \left. (176 + 166 \mu_1^2 + 126 \mu_2^2 - 5 \mathfrak{e}1 + 5 \mathfrak{e}2 + \mu_2 (362 - 5 \mathfrak{e}1 + 5 \mathfrak{e}2) + \right. \\
& \quad \left. \mu_1 (342 - 11 \mathfrak{e}1 + 11 \mathfrak{e}2 + \mu_2 (734 - 5 \mathfrak{e}1 + 5 \mathfrak{e}2)) \right) \left. \right) +
\end{aligned}$$

$$\begin{aligned}
& \eta^3 \left( \Theta p \left( -44 - 44 \eta t + 280 \Theta p - 96 \eta t \Theta p - 120 \mu_1 - 72 \eta t \mu_1 + 560 \Theta p \mu_1 - \right. \right. \\
& \quad 192 \eta t \Theta p \mu_1 - 28 \mu_1^2 + 44 \eta t \mu_1^2 + 280 \Theta p \mu_1^2 - 96 \eta t \Theta p \mu_1^2 - \\
& \quad 124 \mu_2 - 11 \eta t \mu_2 + 672 \Theta p \mu_2 - 144 \eta t \Theta p \mu_2 + 68 \mu_1 \mu_2 - 11 \eta t \mu_1 \mu_2 + \\
& \quad 672 \Theta p \mu_1 \mu_2 - 144 \eta t \Theta p \mu_1 \mu_2 + 1008 \Theta p \mu_2^2 - 216 \eta t \Theta p \mu_2^2 + \\
& \quad 2 w^4 \left( -21 + 8 \mu_1 + 29 \mu_1^2 - 55 \mu_2 - 247 \mu_1 \mu_2 + 40 \Theta p \left( 5 + 5 \mu_1^2 + \right. \right. \\
& \quad \quad 12 \mu_2 + 18 \mu_2^2 + 2 \mu_1 (5 + 6 \mu_2) \left. \right) + 2 \eta t \left( 22 + 47 \mu_1 - 125 \mu_1^2 - \right. \\
& \quad \quad 15 \mu_1 \mu_2 + 10 \Theta p \left( 4 + 8 \mu_1 + 4 \mu_1^2 + 6 \mu_2 + 6 \mu_1 \mu_2 + 9 \mu_2^2 \right) \left. \right) \left. \right) + \\
& \quad 2 w^2 \left( 171 + 232 \mu_1 + \mu_1^2 + 337 \mu_2 + 7 \mu_1 \mu_2 - 134 \Theta p \left( 5 + 5 \mu_1^2 + 12 \right. \right. \\
& \quad \quad \mu_2 + 18 \mu_2^2 + 2 \mu_1 (5 + 6 \mu_2) \left. \right) + \eta t \left( 42 - 16 \mu_1 + 56 \mu_1^2 - 37 \mu_2 + \right. \\
& \quad \quad 137 \mu_1 \mu_2 + 36 \Theta p \left( 4 + 8 \mu_1 + 4 \mu_1^2 + 6 \mu_2 + 6 \mu_1 \mu_2 + 9 \mu_2^2 \right) \left. \right) \left. \right) + \\
& \quad 4 w^3 \left( 40 + 108 \mu_1 + 44 \mu_1^2 + 112 \mu_2 - 203 \mu_1 \mu_2 - 24 \Theta p \right. \\
& \quad \quad \left( 5 + 5 \mu_1^2 + 12 \mu_2 + 18 \mu_2^2 + 2 \mu_1 (5 + 6 \mu_2) \right) + \\
& \quad \quad \eta t \left( 64 + 144 \mu_1 - 166 \mu_1^2 - 5 \mu_2 - 5 \mu_1 \mu_2 + \right. \\
& \quad \quad \quad 38 \Theta p \left( 4 + 8 \mu_1 + 4 \mu_1^2 + 6 \mu_2 + 6 \mu_1 \mu_2 + 9 \mu_2^2 \right) \left. \right) \left. \right) - \\
& \quad 4 w \left( \eta t \left( 30 + 104 \mu_1 - 79 \mu_1^2 + 18 \mu_2 - 54 \mu_1 \mu_2 + 15 \Theta p \right. \right. \\
& \quad \quad \left( 4 + 8 \mu_1 + 4 \mu_1^2 + 6 \mu_2 + 6 \mu_1 \mu_2 + 9 \mu_2^2 \right) \left. \right) + \\
& \quad \quad 2 \times \left( -14 + 15 \mu_1 + 17 \mu_1^2 + \mu_2 - 59 \mu_1 \mu_2 + 3 \Theta p \left( 5 + 5 \mu_1^2 + \right. \right. \\
& \quad \quad \quad 12 \mu_2 + 18 \mu_2^2 + 2 \mu_1 (5 + 6 \mu_2) \left. \right) \left. \right) \left. \right) + (-1 + \eta t) \Theta l \\
& \quad \left( -20 - 56 \mu_1 - 5 \mu_2 + 19 \mu_1 \mu_2 + 4 w^4 \left( -29 \mu_1^2 + 5 \mu_1 (-2 + \mu_2) + \right. \right. \\
& \quad \quad 5 \times (-1 + \mu_2) + 8 \Theta p \left( 5 + 5 \mu_1^2 + 12 \mu_2 + 10 \mu_1 (1 + 3 \mu_2) \right) \left. \right) + \\
& \quad \quad \Theta p \left( 472 + 216 \mu_2^2 - 20 \mathfrak{E}1 + \mu_1^2 (350 - 17 \mathfrak{E}1 - 9 \mathfrak{E}2) + \right. \\
& \quad \quad 20 \mathfrak{E}2 + \mu_2 (806 - 20 \mathfrak{E}1 + 20 \mathfrak{E}2) + \\
& \quad \quad \mu_1 (870 - 85 \mathfrak{E}1 + 59 \mathfrak{E}2 + \mu_2 (1298 - 20 \mathfrak{E}1 + 68 \mathfrak{E}2)) \left. \right) - \\
& \quad 2 w^2 \left( -3 \times \left( 6 \mu_1^2 + \mu_1 (36 - 19 \mu_2) + 5 \times (4 + \mu_2) \right) + \Theta p \left( 688 + 486 \mu_2^2 - \right. \right. \\
& \quad \quad 45 \mathfrak{E}1 - 5 \mu_2 (-278 + 9 \mathfrak{E}1 - 9 \mathfrak{E}2) + \mu_1^2 (514 + 6 \mathfrak{E}1 - 2 \mathfrak{E}2) + \\
& \quad \quad 45 \mathfrak{E}2 + \mu_1 (1250 - 69 \mathfrak{E}1 + \mu_2 (1978 - 45 \mathfrak{E}1 - 3 \mathfrak{E}2) + 73 \mathfrak{E}2) \left. \right) \left. \right) - \\
& \quad 4 w^3 \left( 2 \times \left( 16 \mu_1^2 + \mu_1 (-16 + \mu_2) - 5 \times (1 + \mu_2) \right) + \Theta p \right. \\
& \quad \quad \left( 252 + 259 \mu_1^2 + 162 \mu_2^2 - 10 \mathfrak{E}1 + 10 \mathfrak{E}2 + \mu_2 (419 - 10 \mathfrak{E}1 + 10 \mathfrak{E}2) + \right. \\
& \quad \quad \mu_1 (511 - 22 \mathfrak{E}1 + 22 \mathfrak{E}2 + \mu_2 (1109 - 10 \mathfrak{E}1 + 10 \mathfrak{E}2)) \left. \right) \left. \right) + \\
& \quad w \left( 40 - 8 \mu_1 + 48 \mu_1^2 + 10 \mu_2 - 62 \mu_1 \mu_2 + \Theta p \left( 332 - 108 \mu_2^2 + \right. \right. \\
& \quad \quad 30 \mathfrak{E}1 + \mu_1^2 (426 - 33 \mathfrak{E}1 - 5 \mathfrak{E}2) + 6 \mu_2 (23 + 5 \mathfrak{E}1 - 5 \mathfrak{E}2) - 30 \mathfrak{E}2 + \\
& \quad \quad \mu_1 (686 - 51 \mathfrak{E}1 + 13 \mathfrak{E}2 + 6 \mu_2 (369 + 5 \mathfrak{E}1 + 23 \mathfrak{E}2)) \left. \right) \left. \right) \left. \right) + \\
& \eta^4 \left( 78 \Theta p + 24 \eta t \Theta p - 290 \Theta l \Theta p + 290 \eta t \Theta l \Theta p - 100 \Theta p^2 + 20 \Theta l \right. \\
& \quad \mu_1 - 20 \eta t \Theta l \mu_1 - 68 \Theta p \mu_1 - 56 \eta t \Theta p \mu_1 - 462 \Theta l \Theta p \\
& \quad \mu_1 + 462 \eta t \Theta l \Theta p \mu_1 - 200 \Theta p^2 \mu_1 - 4 \Theta l \mu_1^2 + 4 \eta t \Theta l \\
& \quad \mu_1^2 - 74 \Theta p \mu_1^2 + 16 \eta t \Theta p \mu_1^2 - 232 \Theta l \Theta p \mu_1^2 + 232 \\
& \quad \eta t \Theta l \Theta p \mu_1^2 - 100 \Theta p^2 \mu_1^2 + 46 \Theta p \mu_2 - 16 \eta t \Theta p \\
& \quad \mu_2 - 322 \Theta l \Theta p \mu_2 + 322 \eta t \Theta l \Theta p \mu_2 - 240 \Theta p^2 \mu_2 + 154 \\
& \quad \Theta p \mu_1 \mu_2 + 68 \eta t \Theta p \mu_1 \mu_2 - 1210 \Theta l \Theta p \mu_1 \mu_2 + 1210 \\
& \quad \eta t \Theta l \Theta p \mu_1 \mu_2 - 240 \Theta p^2 \mu_1 \mu_2 - 360 \Theta p^2 \mu_2^2 + w^4 \\
& \quad \left( (-1 + \eta t) \Theta l \left( 124 \mu_1^2 - 5 \times (4 + \mu_2) - 5 \mu_1 (8 + \mu_2) + \right. \right. \\
& \quad \quad 12 \Theta p \left( 35 + 35 \mu_1^2 + 72 \mu_2 + 30 \mu_2^2 + 10 \mu_1 (7 + 15 \mu_2) \right) \left. \right) - \\
& \quad \quad 2 \Theta p \left( 5 \eta t \left( 11 + 26 \mu_1 - 57 \mu_1^2 - 5 \mu_2 + 7 \mu_1 \mu_2 + 8 \Theta p \right. \right. \\
& \quad \quad \quad \left. \left. (4 + 8 \mu_1 + 4 \mu_1^2 + 6 \mu_2 + 6 \mu_1 \mu_2 + 9 \mu_2^2) \right) \right) +
\end{aligned}$$

$$\begin{aligned}
& 2 \times (22 + 57 \mu_1 + 35 \mu_1^2 + 55 \mu_2 - 170 \mu_1 \mu_2 - 5 \theta p \\
& \quad (5 + 5 \mu_1^2 + 12 \mu_2 + 18 \mu_2^2 + 2 \mu_1 (5 + 6 \mu_2))) + 49 \\
& \theta l \theta p \mu_1 \mathfrak{x}1 - 49 \eta t \theta l \theta p \mu_1 \mathfrak{x}1 + 19 \theta l \theta p \mu_1^2 \mathfrak{x}1 - 19 \eta t \theta l \theta p \\
& \mu_1^2 \mathfrak{x}1 - 21 \theta l \theta p \mu_1 \mathfrak{x}2 + 21 \eta t \theta l \theta p \mu_1 \mathfrak{x}2 + 9 \theta l \theta p \mu_1^2 \\
& \mathfrak{x}2 - 9 \eta t \theta l \theta p \mu_1^2 \mathfrak{x}2 - 60 \theta l \theta p \mu_1 \mu_2 \mathfrak{x}2 + 60 \eta t \theta l \theta p \mu_1 \\
& \mu_2 \mathfrak{x}2 + w^3 (8 \theta p (-47 + 2 \mu_1^2 - 104 \mu_2 + \mu_1 (-63 + 58 \mu_2) + \\
& \quad 33 \theta p (5 + 5 \mu_1^2 + 12 \mu_2 + 18 \mu_2^2 + 2 \mu_1 (5 + 6 \mu_2))) - \\
& \eta t \theta p (44 - 236 \mu_1^2 - 145 \mu_2 + \mu_1 (24 + 455 \mu_2) + \\
& \quad 68 \theta p (4 + 4 \mu_1^2 + 6 \mu_2 + 9 \mu_2^2 + \mu_1 (8 + 6 \mu_2))) + \\
& (-1 + \eta t) \theta l (-80 - 160 \mu_1 + 64 \mu_1^2 + 5 \mu_2 + 53 \mu_1 \mu_2 + \\
& \quad 4 \theta p (205 \mu_1^2 + 180 \mu_2^2 + 5 \times (46 - \mathfrak{x}1 + \mathfrak{x}2) + \mu_2 (527 - 5 \mathfrak{x}1 + 5 \mathfrak{x}2) + \\
& \quad \mu_1 (435 - 11 \mathfrak{x}1 + 11 \mathfrak{x}2 + \mu_2 (917 - 5 \mathfrak{x}1 + 5 \mathfrak{x}2)))) + w \\
& (\theta p (\eta t (128 + 116 \mu_1 - 132 \mu_1^2 + 17 \mu_2 + 161 \mu_1 \mu_2 + 72 \theta p \\
& \quad (4 + 8 \mu_1 + 4 \mu_1^2 + 6 \mu_2 + 6 \mu_1 \mu_2 + 9 \mu_2^2))) + \\
& \quad 4 \times (49 + 107 \mu_1 + 16 \mu_1^2 + 130 \mu_2 - 68 \mu_1 \mu_2 - 54 \theta p \\
& \quad (5 + 5 \mu_1^2 + 12 \mu_2 + 18 \mu_2^2 + 2 \mu_1 (5 + 6 \mu_2)))) + \\
& (-1 + \eta t) \theta l (\mu_1 (120 - 57 \mu_2) + 15 \times (4 + \mu_2) + \theta p \\
& \quad (\mu_1 (-1706 + 123 \mathfrak{x}1 + \mu_2 (-2186 + 60 \mathfrak{x}1 - 36 \mathfrak{x}2) - 113 \mathfrak{x}2) + \\
& \quad \mu_1^2 (-654 + 3 \mathfrak{x}1 + 7 \mathfrak{x}2) - 2 \times (466 + 324 \mu_2^2 - \\
& \quad 30 \mathfrak{x}1 + 30 \mathfrak{x}2 + \mu_2 (883 - 30 \mathfrak{x}1 + 30 \mathfrak{x}2)))) + w^2 \\
& (-((-1 + \eta t) \theta l (44 \mu_1^2 - 15 \mu_2 - \mu_1 (64 + 15 \mu_2))) + 12 \theta p^2 \\
& \quad (-5 - 5 \mu_1^2 - 12 \mu_2 - 18 \mu_2^2 - 2 \mu_1 (5 + 6 \mu_2) + \\
& \quad 9 \eta t (4 + 4 \mu_1^2 + 6 \mu_2 + 9 \mu_2^2 + \mu_1 (8 + 6 \mu_2))) + \\
& \theta p (-48 + 500 \mu_1 + 356 \mu_1^2 + 56 \mu_2 - 832 \mu_1 \mu_2 + \eta t (192 + 556 \mu_1 - \\
& \quad 440 \mu_1^2 + 149 \mu_2 - 331 \mu_1 \mu_2 + 2 \theta l (-496 - 162 \mu_2^2 + 15 \mathfrak{x}1 + \\
& \quad \mu_1 (-982 + 62 \mathfrak{x}1 + \mu_2 (-2398 + 15 \mathfrak{x}1 - 51 \mathfrak{x}2) - 46 \mathfrak{x}2) + \\
& \quad \mu_2 (-634 + 15 \mathfrak{x}1 - 15 \mathfrak{x}2) - 15 \mathfrak{x}2 + \\
& \quad \mu_1^2 (-522 + 11 \mathfrak{x}1 + 5 \mathfrak{x}2))) + 2 \theta l (496 + 162 \mu_2^2 - 15 \mathfrak{x}1 + \\
& \quad \mu_1^2 (522 - 11 \mathfrak{x}1 - 5 \mathfrak{x}2) + 15 \mathfrak{x}2 + \mu_2 (634 - 15 \mathfrak{x}1 + 15 \mathfrak{x}2) + \\
& \quad \mu_1 (982 - 62 \mathfrak{x}1 + 46 \mathfrak{x}2 + \mu_2 (2398 - 15 \mathfrak{x}1 + 51 \mathfrak{x}2)))) + \\
& \eta^6 (-4 \theta p (2 - 15 \mu_1^2 + 6 \eta t (1 + \mu_1) + \mu_1 (-31 + 30 \mu_2)) + w^4 \\
& \quad ((-1 + \eta t) \theta l (14 \mu_1^2 + 5 \mu_1 (-4 + \mu_2) + 5 \times (-2 + \mu_2) + \\
& \quad 12 \theta p (14 + 14 \mu_1^2 + 30 \mu_2 + 9 \mu_2^2 + \mu_1 (28 + 66 \mu_2))) - \\
& \quad 2 \theta p (55 - 6 \mu_1 - 61 \mu_1^2 + 143 \mu_2 + 5 \mu_1 \mu_2 - 48 \theta p (5 + 5 \mu_1^2 + \\
& \quad 12 \mu_2 + 18 \mu_2^2 + 2 \mu_1 (5 + 6 \mu_2)) + \eta t (22 + 32 \mu_1 - 32 \mu_1^2 - 5 \mu_2 + \\
& \quad 73 \mu_1 \mu_2 + 6 \theta p (4 + 8 \mu_1 + 4 \mu_1^2 + 6 \mu_2 + 6 \mu_1 \mu_2 + 9 \mu_2^2)))) + \\
& w^3 (\theta p (\eta t (4 + 88 \mu_1 - 84 \mu_1^2 + 27 \mu_2 + 123 \mu_1 \mu_2 + 24 \theta p \\
& \quad (4 + 8 \mu_1 + 4 \mu_1^2 + 6 \mu_2 + 6 \mu_1 \mu_2 + 9 \mu_2^2))) - \\
& \quad 8 \times (-8 - 40 \mu_1 - 17 \mu_1^2 - 46 \mu_2 + 44 \mu_1 \mu_2 + 22 \theta p \\
& \quad (5 + 5 \mu_1^2 + 12 \mu_2 + 18 \mu_2^2 + 2 \mu_1 (5 + 6 \mu_2)))) - \\
& (-1 + \eta t) \theta l (4 \mu_1^2 - 5 \times (4 + \mu_2) + \mu_1 (-52 + 19 \mu_2) + \\
& \quad 4 \theta p (124 + 130 \mu_1^2 + 54 \mu_2^2 - 5 \mathfrak{x}1 + 5 \mathfrak{x}2 + \mu_2 (202 - 5 \mathfrak{x}1 + 5 \mathfrak{x}2) + \\
& \quad \mu_1 (254 - 11 \mathfrak{x}1 + 11 \mathfrak{x}2 + \mu_2 (598 - 5 \mathfrak{x}1 + 5 \mathfrak{x}2)))) + w
\end{aligned}$$

$$\begin{aligned}
& \left( -4 \times (-1 + \eta t) \, \theta l \, \mu 1 \, (1 + \mu 1) + 120 \, \theta p^2 \, (5 + 5 \, \mu 1^2 + 12 \, \mu 2 + \right. \\
& \quad 18 \, \mu 2^2 + 2 \, \mu 1 \, (5 + 6 \, \mu 2)) + \theta p \, (16 - 2 \times (108 + 5 \, \theta l) \, \mu 2 + \\
& \quad \mu 1 \, (-124 + 96 \, \mu 2 + \theta l \, (-34 + 410 \, \mu 2 - 5 \, \mathfrak{z} 1 - 5 \, \mathfrak{z} 2)) - \\
& \quad \mu 1^2 \, (44 + \theta l \, (-38 + 5 \, \mathfrak{z} 1 + 5 \, \mathfrak{z} 2)) + \\
& \quad \eta t \, (28 + 10 \, \theta l \, \mu 2 + \mu 1^2 \, (-16 + \theta l \, (-38 + 5 \, \mathfrak{z} 1 + 5 \, \mathfrak{z} 2)) + \\
& \quad \quad \left. \mu 1 \, (12 - 120 \, \mu 2 + \theta l \, (34 - 410 \, \mu 2 + 5 \, \mathfrak{z} 1 + 5 \, \mathfrak{z} 2))) \right) - w^2 \\
& \left( -4 \times (-1 + \eta t) \, \theta l \, (-5 + \mu 1) \, \mu 1 + 60 \, \theta p^2 \, (5 + 5 \, \mu 1^2 + 12 \, \mu 2 + \right. \\
& \quad 18 \, \mu 2^2 + 2 \, \mu 1 \, (5 + 6 \, \mu 2)) + \theta p \, (-42 + 380 \, \mu 1 + 302 \, \mu 1^2 - \\
& \quad 190 \, \mu 2 - 454 \, \mu 1 \, \mu 2 - 5 \, \theta l \, (-50 - 62 \, \mu 2 + \mu 1^2 \, (-72 + 3 \, \mathfrak{z} 1 + \mathfrak{z} 2) - \\
& \quad \quad \mu 1 \, (110 + 398 \, \mu 2 - 9 \, \mathfrak{z} 1 + 5 \, \mathfrak{z} 2 + 12 \, \mu 2 \, \mathfrak{z} 2)) + \\
& \quad \eta t \, (-4 \times (21 + 8 \, \mu 1^2 - 4 \, \mu 2 + 5 \, \mu 1 \, (1 + 7 \, \mu 2)) + \\
& \quad \quad 5 \, \theta l \, (-50 - 62 \, \mu 2 + \mu 1^2 \, (-72 + 3 \, \mathfrak{z} 1 + \mathfrak{z} 2) - \\
& \quad \quad \quad \left. \mu 1 \, (110 + 398 \, \mu 2 - 9 \, \mathfrak{z} 1 + 5 \, \mathfrak{z} 2 + 12 \, \mu 2 \, \mathfrak{z} 2))) \right) - \\
& \eta^5 \left( -10 \, \theta p + 16 \, \eta t \, \theta p + 24 \, \theta l \, \theta p - 24 \, \eta t \, \theta l \, \theta p + 300 \, \theta p^2 + 4 \, \theta l \, \mu 1 - 4 \right. \\
& \quad \eta t \, \theta l \, \mu 1 - 88 \, \theta p \, \mu 1 - 10 \, \theta l \, \theta p \, \mu 1 + 10 \, \eta t \, \theta l \, \theta p \, \mu 1 + 600 \\
& \quad \theta p^2 \, \mu 1 + 4 \, \theta l \, \mu 1^2 - 4 \, \eta t \, \theta l \, \mu 1^2 - 30 \, \theta p \, \mu 1^2 - 16 \, \eta t \, \theta p \\
& \quad \mu 1^2 + 38 \, \theta l \, \theta p \, \mu 1^2 - 38 \, \eta t \, \theta l \, \theta p \, \mu 1^2 + 300 \, \theta p^2 \, \mu 1^2 - 106 \\
& \quad \theta p \, \mu 2 - 10 \, \theta l \, \theta p \, \mu 2 + 10 \, \eta t \, \theta l \, \theta p \, \mu 2 + 720 \, \theta p^2 \, \mu 2 + 26 \\
& \quad \theta p \, \mu 1 \, \mu 2 - 60 \, \eta t \, \theta p \, \mu 1 \, \mu 2 + 410 \, \theta l \, \theta p \, \mu 1 \, \mu 2 - 410 \\
& \quad \eta t \, \theta l \, \theta p \, \mu 1 \, \mu 2 + 720 \, \theta p^2 \, \mu 1 \, \mu 2 + 1080 \, \theta p^2 \, \mu 2^2 + 2 \, w^4 \\
& \quad \left( (-1 + \eta t) \, \theta l \, (33 \, \mu 1^2 + 5 \, \mu 1 \, (-6 + \mu 2) + 5 \times (-3 + \mu 2) + \right. \\
& \quad \quad 4 \, \theta p \, (65 + 65 \, \mu 1^2 + 138 \, \mu 2 + 45 \, \mu 2^2 + 10 \, \mu 1 \, (13 + 30 \, \mu 2))) - \\
& \quad \theta p \, (20 \times (4 + \mu 1^2 + \mu 1 \, (5 - 10 \, \mu 2) + 11 \, \mu 2) - 62 \, \theta p \, (5 + 5 \, \mu 1^2 + 12 \, \mu 2 + \\
& \quad \quad 18 \, \mu 2^2 + 2 \, \mu 1 \, (5 + 6 \, \mu 2)) + \eta t \, (35 - 153 \, \mu 1^2 - 20 \, \mu 2 + 20 \, \mu 1 \\
& \quad \quad \left. (4 + 5 \, \mu 2) + 26 \, \theta p \, (4 + 4 \, \mu 1^2 + 6 \, \mu 2 + 9 \, \mu 2^2 + \mu 1 \, (8 + 6 \, \mu 2))) \right) - \\
& \quad 5 \, \theta l \, \theta p \, \mu 1 \, \mathfrak{z} 1 + 5 \, \eta t \, \theta l \, \theta p \, \mu 1 \, \mathfrak{z} 1 - 5 \, \theta l \, \theta p \, \mu 1^2 \, \mathfrak{z} 1 + 5 \, \eta t \, \theta l \, \theta p \, \mu 1^2 \\
& \quad \mathfrak{z} 1 - 5 \, \theta l \, \theta p \, \mu 1 \, \mathfrak{z} 2 + 5 \, \eta t \, \theta l \, \theta p \, \mu 1 \, \mathfrak{z} 2 - 5 \, \theta l \, \theta p \, \mu 1^2 \, \mathfrak{z} 2 + 5 \, \eta t \, \theta l \\
& \quad \theta p \, \mu 1^2 \, \mathfrak{z} 2 + w^2 \, (3 \, \theta p \, (\eta t \, (36 + 56 \, \mu 1 - 52 \, \mu 1^2 + 11 \, \mu 2 + 83 \, \mu 1 \, \mu 2 + \\
& \quad \quad 24 \, \theta p \, (4 + 8 \, \mu 1 + 4 \, \mu 1^2 + 6 \, \mu 2 + 6 \, \mu 1 \, \mu 2 + 9 \, \mu 2^2)) - \\
& \quad \quad 4 \times (-19 - 46 \, \mu 1 - 9 \, \mu 1^2 - 61 \, \mu 2 + 36 \, \mu 1 \, \mu 2 + 25 \, \theta p \\
& \quad \quad \quad (5 + 5 \, \mu 1^2 + 12 \, \mu 2 + 18 \, \mu 2^2 + 2 \, \mu 1 \, (5 + 6 \, \mu 2))) - (-1 + \eta t) \, \theta l \\
& \quad \quad (4 \, \mu 1^2 - 15 \times (4 + \mu 2) + \mu 1 \, (-116 + 57 \, \mu 2) + 2 \, \theta p \, (482 + 324 \, \mu 2^2 - \\
& \quad \quad 30 \, \mathfrak{z} 1 + \mu 1^2 \, (348 + 5 \, \mathfrak{z} 1 - \mathfrak{z} 2) + 30 \, \mathfrak{z} 2 + \mu 2 \, (890 - 30 \, \mathfrak{z} 1 + 30 \, \mathfrak{z} 2) + \\
& \quad \quad \mu 1 \, (866 - 43 \, \mathfrak{z} 1 + 47 \, \mathfrak{z} 2 - 2 \, \mu 2 \, (-625 + 15 \, \mathfrak{z} 1 + 3 \, \mathfrak{z} 2))) \right) + w \\
& \quad \left( 4 \times (-1 + \eta t) \, \theta l \, (-11 + \mu 1) \, \mu 1 + \theta p \, (84 - 328 \, \mu 1 - 244 \, \mu 1^2 + \right. \\
& \quad \quad 64 \, \mu 2 + 412 \, \mu 1 \, \mu 2 - 6 \, \theta l \, (90 + 107 \, \mu 2) + 4 \, \eta t \, (19 + 8 \, \mu 1^2 - \\
& \quad \quad \quad 8 \, \mu 2 + 7 \, \mu 1 \, (-3 + 4 \, \mu 2)) + \theta l \, \mu 1^2 \, (-554 + 29 \, \mathfrak{z} 1 + 9 \, \mathfrak{z} 2) - \\
& \quad \quad \theta l \, \mu 1 \, (1046 - 89 \, \mathfrak{z} 1 + 51 \, \mathfrak{z} 2 + 30 \, \mu 2 \, (93 + 4 \, \mathfrak{z} 2)) + \\
& \quad \quad \eta t \, \theta l \, (540 + 642 \, \mu 2 + \mu 1^2 \, (554 - 29 \, \mathfrak{z} 1 - 9 \, \mathfrak{z} 2) + \\
& \quad \quad \quad \left. \mu 1 \, (1046 - 89 \, \mathfrak{z} 1 + 51 \, \mathfrak{z} 2 + 30 \, \mu 2 \, (93 + 4 \, \mathfrak{z} 2))) \right) + 2 \\
& \quad w^3 \, (2 \times (-1 + \eta t) \, \theta l \, (\mu 1^2 - \mu 1 \, (-7 + \mu 2) + 5 \, \mu 2) + 6 \, \theta p^2 \\
& \quad \quad (2 \times (5 + 5 \, \mu 1^2 + 12 \, \mu 2 + 18 \, \mu 2^2 + 2 \, \mu 1 \, (5 + 6 \, \mu 2)) + \\
& \quad \quad \quad 3 \, \eta t \, (4 + 4 \, \mu 1^2 + 6 \, \mu 2 + 9 \, \mu 2^2 + \mu 1 \, (8 + 6 \, \mu 2))) +
\end{aligned}$$

$$\begin{aligned}
& \left( \begin{aligned}
& \theta p \left( 2 \times \left( -31 + 81 \mu_1^2 + \mu_1 (56 - 96 \mu_2) - 42 \mu_2 \right) + 3 \theta l \right. \\
& \quad \left( 88 + 104 \mu_1^2 + 18 \mu_2^2 - 5 \theta_1 + 5 \theta_2 + \mu_2 (92 - 5 \theta_1 + 5 \theta_2) + \right. \\
& \quad \left. \mu_1 (192 - 11 \theta_1 + 11 \theta_2 + \mu_2 (476 - 5 \theta_1 + 5 \theta_2)) \right) - \\
& \quad \eta t \left( -22 - 126 \mu_1 + 70 \mu_1^2 - 55 \mu_2 + 137 \mu_1 \mu_2 + 3 \theta l \right. \\
& \quad \left. \left( 88 + 104 \mu_1^2 + 18 \mu_2^2 - 5 \theta_1 + 5 \theta_2 + \mu_2 (92 - 5 \theta_1 + 5 \theta_2) + \right. \right. \\
& \quad \left. \left. \mu_1 (192 - 11 \theta_1 + 11 \theta_2 + \mu_2 (476 - 5 \theta_1 + 5 \theta_2)) \right) \right) \right) \Bigg) / \\
& (96 x (-1 + w (-1 + \eta))^3 (x (-1 + \eta) - \eta)^3 (1 + x + \eta - x \eta)^2 \\
& (w + \\
& \quad x + \\
& \quad \eta - \\
& \quad w \\
& \quad \eta - x \\
& \quad \eta)^3 (-1 + \eta t) \theta l) \Bigg) \\
\beta \theta l = & \\
& - \left( \left( -c v c \sigma (w (-1 + \eta) + x (-1 + \eta) - \eta) (-1 + \eta) (x^2 (-1 + \eta)^2 + \eta (1 + \eta) + x (1 + \eta - 2 \eta^2)) \right)^2 \right. \\
& \quad \left( (x + \eta - x \eta)^2 (-1 + \eta t) \theta l \theta p (1 + \mu_1) \times (14 x (-1 + \eta) - 14 \eta - 5 \times (2 + \theta_1 + \theta_2)) + \right. \\
& \quad w (-1 + \eta) \times (-4 x^3 (-1 + \eta)^3 \theta p \\
& \quad \quad (1 - 8 \theta l + 7 \mu_1 - 14 \theta l \mu_1 + 3 \eta^2 (1 + \mu_1) - \eta \eta t (1 + 2 \theta l) \times (1 + \mu_1) + 2 \eta \\
& \quad \quad \quad (-2 + \theta l - 5 \mu_1 + \theta l \mu_1) + \eta t (1 + 8 \theta l + \mu_1 + 14 \theta l \mu_1)) + x^2 (-1 + \eta)^2 \theta p \\
& \quad \quad (36 \eta^3 (1 + \mu_1) - 12 \eta^2 (\eta t (1 + 2 \theta l) \times (1 + \mu_1) - 2 \times (-2 + \theta l - 5 \mu_1 + \theta l \mu_1)) + \\
& \quad \quad 12 \eta (1 + 7 \mu_1 - 2 \theta l (4 + 7 \mu_1) + \eta t (1 + \mu_1 + 2 \theta l (4 + 7 \mu_1))) + \\
& \quad \quad (-1 + \eta t) \theta l (1 + \mu_1) \times (58 + 15 \theta_1 + 15 \theta_2)) - x (-1 + \eta) \times \\
& \quad \quad (12 \times (-1 + \eta) \eta^2 \theta p (-1 - 7 \mu_1 + 3 \eta (1 + \mu_1) - \eta t (1 + \mu_1)) - (-1 + \eta t) \theta l \\
& \quad \quad (20 \times (1 + \mu_1) + \theta p (24 \eta^3 (1 + \mu_1) - 24 \eta^2 (4 + 7 \mu_1) + 5 \times (-6 - 3 \theta_1 + \theta_2) - \\
& \quad \quad 2 \eta (1 + \mu_1) \times (58 + 15 \theta_1 + 15 \theta_2) - \mu_1 (30 + 15 \theta_1 + 19 \theta_2))) \Bigg) + \\
& \quad \theta p (12 \eta^5 (1 + \mu_1) + 20 \eta t (1 + \mu_1) - 4 \eta^4 (\eta t (1 + 2 \theta l) \times (1 + \mu_1) - 2 \times \\
& \quad \quad (-2 + \theta l - 5 \mu_1 + \theta l \mu_1)) + 4 \eta^3 (1 + 7 \mu_1 - 2 \theta l (4 + 7 \mu_1) + \eta t (1 + \mu_1 + \\
& \quad \quad 2 \theta l (4 + 7 \mu_1))) + \eta^2 (-1 + \eta t) \theta l (1 + \mu_1) \times (58 + 15 \theta_1 + 15 \theta_2) + \\
& \quad \quad \eta (-20 \eta t (1 + \mu_1) - 5 \theta l (6 + 3 \theta_1 - \theta_2) - \theta l \mu_1 (30 + 15 \theta_1 + 19 \theta_2) + \\
& \quad \quad \eta t \theta l (5 \times (6 + 3 \theta_1 - \theta_2) + \mu_1 (30 + 15 \theta_1 + 19 \theta_2))) \Bigg) + w^4 (-1 + \eta)^4 \\
& \quad (x (-1 + \eta) \times (4 \times (-1 + \eta) \theta p (1 - 5 \mu_1 + \eta (1 + \mu_1) - \eta t (1 + \mu_1)) + (-1 + \eta t) \\
& \quad \quad \theta l (-20 \times (1 + \mu_1) + 5 \theta p (8 + 3 \theta_1 - \theta_2) + \theta p \mu_1 (64 + 15 \theta_1 + 19 \theta_2))) + \\
& \quad \quad \theta p (-4 \eta^3 (1 + \mu_1) - 20 \eta t (1 + \mu_1) + 4 \eta^2 (\eta t + 6 \mu_1 + \eta t \mu_1) + \eta (4 - 20 \mu_1 + \\
& \quad \quad 16 \eta t (1 + \mu_1) + \theta l (40 + 64 \mu_1 + 15 \theta_1 + 15 \mu_1 \theta_1 - 5 \theta_2 + 19 \mu_1 \theta_2) - \\
& \quad \quad \eta t \theta l (5 \times (8 + 3 \theta_1 - \theta_2) + \mu_1 (64 + 15 \theta_1 + 19 \theta_2))) \Bigg) + \\
& \quad w^2 (-1 + \eta)^2 (2 x^3 (-1 + \eta)^3 \theta p (-2 - 5 \theta l + 10 \mu_1 - 17 \theta l \mu_1 + 2 \eta^2 \\
& \quad \quad (1 + \mu_1) - 2 \eta (\eta t + 6 \mu_1 + \eta t \mu_1) + \eta t (2 + 5 \theta l + 2 \mu_1 + 17 \theta l \mu_1)) - \\
& \quad \quad x^2 (-1 + \eta)^2 \theta p (8 - 94 \theta l + 56 \mu_1 - 142 \theta l \mu_1 + 12 \eta^3 (1 + \mu_1) + 8 \eta t (1 + \mu_1) - \\
& \quad \quad 12 \eta^2 (-2 + \eta t + 4 \mu_1 + \eta t \mu_1) + 2 \eta (-22 - 7 \theta l - 10 \mu_1 - 43 \theta l \mu_1 + \\
& \quad \quad \eta t (2 + 7 \theta l + 2 \mu_1 + 43 \theta l \mu_1)) - 15 \theta l \theta_1 - 15 \theta l \mu_1 \theta_1 - 15 \theta l \theta_2 - 15 \\
& \quad \quad \theta l \mu_1 \theta_2 + \eta t \theta l (94 + 15 \theta_1 + 15 \theta_2 + \mu_1 (142 + 15 \theta_1 + 15 \theta_2))) \Bigg) + \\
& \quad x (-1 + \eta) \times (4 \times (-1 + \eta) \eta \theta p (3 \eta^2 (1 + \mu_1) - 3 \eta (-5 + \eta t + \mu_1 + \eta t \mu_1) - \\
& \quad \quad 4 \times (1 + \eta t + 7 \mu_1 + \eta t \mu_1)) + (-1 + \eta t) \theta l (-60 \times (1 + \mu_1) +
\end{aligned}$$

$$\begin{aligned}
& \left( \begin{aligned} & \text{ep} \left( 104 + \eta^2 (-2 + 70 \mu_1) + 45 \mathfrak{e}1 - 15 \mathfrak{e}2 + \mu_1 (104 + 45 \mathfrak{e}1 + 57 \mathfrak{e}2) + \right. \\ & \quad \left. 2 \eta (94 + 15 \mathfrak{e}1 + 15 \mathfrak{e}2 + \mu_1 (142 + 15 \mathfrak{e}1 + 15 \mathfrak{e}2)) \right) \Big) + \\ & \text{ep} \left( -4 \eta^5 (1 + \mu_1) - 60 \eta \mathfrak{t} (1 + \mu_1) + 4 \eta^4 (-6 + \eta \mathfrak{t} + \eta \mathfrak{t} \mu_1) + \eta^3 \right. \\ & \quad (36 + 60 \mu_1 + 6 \mathfrak{e}1 (-1 + 3 \mu_1) + \eta \mathfrak{t} (4 + 6 \mathfrak{e}1 + 4 \mu_1 - 18 \mathfrak{e}1 \mu_1)) + \eta \\ & \quad (60 \eta \mathfrak{t} (1 + \mu_1) + \mathfrak{e}1 (104 + 45 \mathfrak{e}1 - 15 \mathfrak{e}2 + \mu_1 (104 + 45 \mathfrak{e}1 + 57 \mathfrak{e}2)) - \\ & \quad \eta \mathfrak{t} \mathfrak{e}1 (104 + 45 \mathfrak{e}1 - 15 \mathfrak{e}2 + \mu_1 (104 + 45 \mathfrak{e}1 + 57 \mathfrak{e}2))) - \eta^2 \\ & \quad (8 + 56 \mu_1 - \mathfrak{e}1 (94 + 15 \mathfrak{e}1 + 15 \mathfrak{e}2 + \mu_1 (142 + 15 \mathfrak{e}1 + 15 \mathfrak{e}2)) + \eta \mathfrak{t} \\ & \quad (8 \times (1 + \mu_1) + \mathfrak{e}1 (94 + 15 \mathfrak{e}1 + 15 \mathfrak{e}2 + \mu_1 (142 + 15 \mathfrak{e}1 + 15 \mathfrak{e}2)))) \Big) + \\ & w^3 (-1 + \eta)^3 \left( x^2 (-1 + \eta)^2 \text{ep} \left( -8 - 30 \mathfrak{e}1 + 40 \mu_1 - 78 \mathfrak{e}1 \mu_1 + 8 \eta^2 (1 + \mu_1) - \right. \right. \\ & \quad 8 \eta (\eta \mathfrak{t} + 6 \mu_1 + \eta \mathfrak{t} \mu_1) - 5 \mathfrak{e}1 \mathfrak{e}1 - 5 \mathfrak{e}1 \mu_1 \mathfrak{e}1 - 5 \mathfrak{e}1 \mathfrak{e}2 - 5 \mathfrak{e}1 \mu_1 \mathfrak{e}2 + \eta \mathfrak{t} \\ & \quad (8 \times (1 + \mu_1) + 5 \mathfrak{e}1 (6 + \mathfrak{e}1 + \mathfrak{e}2) + \mathfrak{e}1 \mu_1 (78 + 5 \mathfrak{e}1 + 5 \mathfrak{e}2))) - \\ & \quad \times (-1 + \eta) \times \left( 4 \times (-1 + \eta) \text{ep} \left( -1 - 7 \mu_1 + 4 \eta^2 (1 + \mu_1) - \eta \mathfrak{t} (1 + \mu_1) - \right. \right. \\ & \quad \eta (-7 + 17 \mu_1 + 4 \eta \mathfrak{t} (1 + \mu_1)) \Big) + (-1 + \eta \mathfrak{t}) \mathfrak{e}1 \\ & \quad (-60 \times (1 + \mu_1) + \text{ep} (122 + 45 \mathfrak{e}1 - 15 \mathfrak{e}2 + \mu_1 (146 + 45 \mathfrak{e}1 + 57 \mathfrak{e}2) + \\ & \quad 2 \eta (26 + 5 \mathfrak{e}1 + 5 \mathfrak{e}2 + \mu_1 (74 + 5 \mathfrak{e}1 + 5 \mathfrak{e}2)))) \Big) + \\ & \text{ep} \left( 8 \eta^4 (1 + \mu_1) + 60 \eta \mathfrak{t} (1 + \mu_1) - 4 \eta^3 (-3 + 9 \mu_1 + 2 \eta \mathfrak{t} (1 + \mu_1)) + \right. \\ & \quad \eta^2 (-24 - \mathfrak{e}1 (22 + 5 \mathfrak{e}1 + 5 \mathfrak{e}2 + 5 \mu_1 (14 + \mathfrak{e}1 + \mathfrak{e}2))) + \\ & \quad \eta \mathfrak{t} (4 \times (1 + \mu_1) + \mathfrak{e}1 (22 + 5 \mathfrak{e}1 + 5 \mathfrak{e}2 + 5 \mu_1 (14 + \mathfrak{e}1 + \mathfrak{e}2))) + \eta (4 + 28 \\ & \quad \mu_1 - \mathfrak{e}1 (122 + 45 \mathfrak{e}1 - 15 \mathfrak{e}2 + \mu_1 (146 + 45 \mathfrak{e}1 + 57 \mathfrak{e}2)) + \eta \mathfrak{t} (-56 \times (1 + \\ & \quad \mu_1) + \mathfrak{e}1 (122 + 45 \mathfrak{e}1 - 15 \mathfrak{e}2 + \mu_1 (146 + 45 \mathfrak{e}1 + 57 \mathfrak{e}2)))) \Big) - \\ & (1 + x + \eta - x \eta)^2 \mathfrak{e}1 \left( 24 \text{cv}^2 (-1 + w (-1 + \eta))^3 (x + \eta - x \eta)^3 (w + x + \eta - w \eta - x \eta)^3 \right. \\ & \quad \left. (-1 + \eta \mathfrak{t}) \text{ep} + \right. \\ & f \left( -4 w^6 (-1 + \eta)^6 (x + \eta - x \eta)^3 (-1 + \eta \mathfrak{t}) \mathfrak{e}1 \text{ep} \right. \\ & \quad \left( 2 \times (-4 + \mathfrak{e}2) + \mathfrak{e}1 (8 - 4 \mathfrak{e}2 + 5 \mathfrak{e}2^2) \right) + 2 w^5 (-1 + \eta)^5 \\ & \quad \left( 6 x^4 (-1 + \eta)^4 (-1 + \eta \mathfrak{t}) \mathfrak{e}1 \text{ep} \left( 2 \times (-4 + \mathfrak{e}2) + \mathfrak{e}1 (8 - 4 \mathfrak{e}2 + 5 \mathfrak{e}2^2) \right) + 2 \right. \\ & \quad x^3 (-1 + \eta)^3 \left( -3 \times (1 + 4 \eta) \times (-1 + \eta \mathfrak{t}) \mathfrak{e}1^2 \text{ep} \left( 8 - 4 \mathfrak{e}2 + 5 \mathfrak{e}2^2 \right) + \right. \\ & \quad (-1 + \eta)^2 \text{ep} \left( -54 + 10 \eta^2 + \eta \mathfrak{t} (-15 + \mathfrak{e}2) - 5 \mathfrak{e}2 - \eta (-15 + 10 \eta \mathfrak{t} + \mathfrak{e}2) \right) + \\ & \quad (-1 + \eta \mathfrak{t}) \mathfrak{e}1 (12 - 5 \mathfrak{e}2 - 3 \text{ep} (14 + 3 \mathfrak{e}1 + 5 \mathfrak{e}2) + \\ & \quad \eta (-12 + 3 \text{ep} (54 + 3 \mathfrak{e}1 - 5 \mathfrak{e}2) + 5 \mathfrak{e}2)) \Big) - x^2 (-1 + \eta)^2 \\ & \quad (60 \eta^5 \text{ep} - 6 \eta^4 \text{ep} (5 + 10 \eta \mathfrak{t} + \mathfrak{e}2) + \eta \mathfrak{t} \text{ep} (-31 + 10 \mathfrak{e}2) + \\ & \quad 6 \eta^3 \text{ep} (-74 - 3 \mathfrak{e}2 + \eta \mathfrak{t} (5 + \mathfrak{e}2)) + \eta^2 \left( (-1 + \eta \mathfrak{t}) \mathfrak{e}1 (-41 + 18 \text{ep} \right. \\ & \quad (38 + 3 \mathfrak{e}1 - \mathfrak{e}2) + 20 \mathfrak{e}2) + \text{ep} (738 + \eta \mathfrak{t} (89 - 2 \mathfrak{e}2) + 54 \mathfrak{e}2) - \\ & \quad 36 \times (-1 + \eta \mathfrak{t}) \mathfrak{e}1^2 \text{ep} \left( 8 - 4 \mathfrak{e}2 + 5 \mathfrak{e}2^2 \right) \Big) - \eta (18 \times (-1 + \eta \mathfrak{t}) \\ & \quad \mathfrak{e}1^2 \text{ep} \left( 8 - 4 \mathfrak{e}2 + 5 \mathfrak{e}2^2 \right) + 2 \text{ep} (7 \eta \mathfrak{t} (2 + \mathfrak{e}2) + 3 \times (54 + 5 \mathfrak{e}2)) + \\ & \quad \left. (-1 + \eta \mathfrak{t}) \mathfrak{e}1 (-41 + 20 \mathfrak{e}2 + 18 \text{ep} (14 + 3 \mathfrak{e}1 + 5 \mathfrak{e}2))) \right) + x (-1 + \eta) \\ & \quad \eta (60 \eta^5 \text{ep} - 6 \eta^4 \text{ep} (5 + 10 \eta \mathfrak{t} + \mathfrak{e}2) + \eta \mathfrak{t} \text{ep} (-61 + 20 \mathfrak{e}2) + \\ & \quad 6 \eta^3 \text{ep} (-74 - 3 \mathfrak{e}2 + \eta \mathfrak{t} (5 + \mathfrak{e}2)) - \eta (2 \text{ep} (162 - 16 \eta \mathfrak{t} + 15 \mathfrak{e}2 + \\ & \quad 17 \eta \mathfrak{t} \mathfrak{e}2) + 18 \times (-1 + \eta \mathfrak{t}) \mathfrak{e}1^2 \text{ep} \left( 8 - 4 \mathfrak{e}2 + 5 \mathfrak{e}2^2 \right) + \\ & \quad (-1 + \eta \mathfrak{t}) \mathfrak{e}1 (-11 + 10 \mathfrak{e}2 + 18 \text{ep} (14 + 3 \mathfrak{e}1 + 5 \mathfrak{e}2))) + \\ & \quad \eta^2 \left( -24 \times (-1 + \eta \mathfrak{t}) \mathfrak{e}1^2 \text{ep} \left( 8 - 4 \mathfrak{e}2 + 5 \mathfrak{e}2^2 \right) + (-1 + \eta \mathfrak{t}) \right. \\ & \quad \mathfrak{e}1 (-11 + 10 \mathfrak{e}2 + 6 \text{ep} (98 + 9 \mathfrak{e}1 + \mathfrak{e}2)) + \\ & \quad \left. \text{ep} (738 + 54 \mathfrak{e}2 + \eta \mathfrak{t} (59 + 8 \mathfrak{e}2)) \right) - 2 \eta^2 \text{ep} \left( 10 \eta^5 - \eta^4 \right. \\ & \quad (5 + 10 \eta \mathfrak{t} + \mathfrak{e}2) + \eta \mathfrak{t} (-12 + 5 \mathfrak{e}2) + \eta^3 (-74 - 3 \mathfrak{e}2 + \eta \mathfrak{t} (5 + \mathfrak{e}2)) + \\ & \quad \left. \eta^2 (\eta \mathfrak{t} (8 + 3 \mathfrak{e}2 + 3 \mathfrak{e}1 (30 + 3 \mathfrak{e}1 + \mathfrak{e}2) - 3 \mathfrak{e}1^2 (8 - 4 \mathfrak{e}2 + 5 \mathfrak{e}2^2)) \right) + \end{aligned}
\end{aligned}$$

$$\begin{aligned}
& 3 \times (41 + 3 \mathfrak{z}2 - \mathfrak{el} (30 + 3 \mathfrak{z}1 + \mathfrak{z}2) + \mathfrak{el}^2 (8 - 4 \mathfrak{z}2 + 5 \mathfrak{z}2^2)) - \\
& \eta (54 + 5 \mathfrak{z}2 - 3 \mathfrak{el} (14 + 3 \mathfrak{z}1 + 5 \mathfrak{z}2) - 3 \mathfrak{el}^2 (8 - 4 \mathfrak{z}2 + 5 \mathfrak{z}2^2) + 3 \eta t \\
& (3 \times (-1 + \mathfrak{z}2) + \mathfrak{el} (14 + 3 \mathfrak{z}1 + 5 \mathfrak{z}2) + \mathfrak{el}^2 (8 - 4 \mathfrak{z}2 + 5 \mathfrak{z}2^2))) - \\
& (x + \eta - x \eta)^2 (-2 x^4 (-1 + \eta)^4 \mathfrak{op} (-108 + 60 \eta^4 + 92 \mathfrak{el} + 16 \mathfrak{el}^2 - \\
& 6 \mathfrak{z}2 + 24 \mathfrak{el} \mathfrak{z}2 - 8 \mathfrak{el}^2 \mathfrak{z}2 + 5 \mathfrak{el} \mathfrak{z}2^2 + 10 \mathfrak{el}^2 \mathfrak{z}2^2 - \\
& 4 \eta^3 (35 - 5 \mathfrak{el} + 5 \eta t (2 + \mathfrak{el}) + \mathfrak{z}2) + 2 \eta^2 (-4 + \mathfrak{el} (-15 + \mathfrak{z}2) + \mathfrak{z}2 + \\
& \eta t (45 - \mathfrak{el} (-15 + \mathfrak{z}2) + \mathfrak{z}2)) + \eta (196 + 8 \mathfrak{z}2 - 4 \eta t (15 + \mathfrak{z}2) - \\
& \mathfrak{el} (98 + 22 \mathfrak{z}2 + 5 \mathfrak{z}2^2) + \eta t \mathfrak{el} (98 + 22 \mathfrak{z}2 + 5 \mathfrak{z}2^2)) - \\
& \eta t (-2 \times (5 + \mathfrak{z}2) + 2 \mathfrak{el}^2 (8 - 4 \mathfrak{z}2 + 5 \mathfrak{z}2^2) + \mathfrak{el} (92 + 24 \mathfrak{z}2 + 5 \mathfrak{z}2^2))) + \\
& 2 x^3 (-1 + \eta)^3 (-8 \eta (-1 + \eta t) \mathfrak{el}^2 \mathfrak{op} (8 - 4 \mathfrak{z}2 + 5 \mathfrak{z}2^2) + 8 (-1 + \eta)^2 \\
& \eta \mathfrak{op} (30 \eta^2 + \eta t (5 + \mathfrak{z}2) - 3 \times (18 + \mathfrak{z}2) - 2 \eta (5 + 10 \eta t + \mathfrak{z}2)) - \\
& (-1 + \eta t) \mathfrak{el} (80 \eta^4 \mathfrak{op} + 8 \eta^3 \mathfrak{op} (-15 + \mathfrak{z}2) + 10 \times (-2 + \mathfrak{z}2) - 10 \eta \\
& (-2 + \mathfrak{z}2) + \mathfrak{op} (20 + 24 \mathfrak{z}1 - 5 \mathfrak{z}2^2) - 4 \eta^2 \mathfrak{op} (98 + 22 \mathfrak{z}2 + 5 \mathfrak{z}2^2) + \\
& \eta \mathfrak{op} (348 - 24 \mathfrak{z}1 + 96 \mathfrak{z}2 + 25 \mathfrak{z}2^2))) - x^2 (-1 + \eta)^2 (720 \eta^6 \mathfrak{op} - \\
& 24 \eta^4 \mathfrak{op} (4 + \eta t (-45 + \mathfrak{el} (-15 + \mathfrak{z}2) - \mathfrak{z}2) - \mathfrak{el} (-15 + \mathfrak{z}2) - \mathfrak{z}2) - \\
& 48 \eta^5 \mathfrak{op} (35 - 5 \mathfrak{el} + 5 \eta t (2 + \mathfrak{el}) + \mathfrak{z}2) + 10 \eta t \mathfrak{op} (-3 + 2 \mathfrak{z}2) + \\
& 12 \eta^3 \mathfrak{op} (196 + 8 \mathfrak{z}2 - 4 \eta t (15 + \mathfrak{z}2) - \mathfrak{el} (98 + 22 \mathfrak{z}2 + 5 \mathfrak{z}2^2) + \\
& \eta t \mathfrak{el} (98 + 22 \mathfrak{z}2 + 5 \mathfrak{z}2^2)) + \eta^2 (-24 \times (-1 + \eta t) \mathfrak{el}^2 \mathfrak{op} (8 - 4 \mathfrak{z}2 + \\
& 5 \mathfrak{z}2^2) + 2 \mathfrak{op} (-36 \times (18 + \mathfrak{z}2) + \eta t (45 + 22 \mathfrak{z}2)) + (-1 + \eta t) \mathfrak{el} \\
& (20 \times (-5 + 2 \mathfrak{z}2) + \mathfrak{op} (-974 + 141 \mathfrak{z}1 - 283 \mathfrak{z}2 - 90 \mathfrak{z}2^2))) + \\
& \eta (20 \eta t \mathfrak{op} (3 - 2 \mathfrak{z}2) - (-1 + \eta t) \mathfrak{el} (141 \mathfrak{op} \mathfrak{z}1 + 20 \times (-5 + 2 \mathfrak{z}2) + \\
& 5 \mathfrak{op} (26 + \mathfrak{z}2 - 6 \mathfrak{z}2^2))) + \eta^2 \mathfrak{op} (-120 \eta^6 + 38 \eta t + \\
& 4 \eta^4 (4 + \eta t (-45 + \mathfrak{el} (-15 + \mathfrak{z}2) - \mathfrak{z}2) - \mathfrak{el} (-15 + \mathfrak{z}2) - \mathfrak{z}2) - \\
& 20 \eta t \mathfrak{z}2 + 8 \eta^5 (35 - 5 \mathfrak{el} + 5 \eta t (2 + \mathfrak{el}) + \mathfrak{z}2) - \\
& 2 \eta^3 (196 + 8 \mathfrak{z}2 - 4 \eta t (15 + \mathfrak{z}2) - \mathfrak{el} (98 + 22 \mathfrak{z}2 + 5 \mathfrak{z}2^2) + \\
& \eta t \mathfrak{el} (98 + 22 \mathfrak{z}2 + 5 \mathfrak{z}2^2)) + \eta (\mathfrak{el} (-38 - 39 \mathfrak{z}1 + \mathfrak{z}2 + 10 \mathfrak{z}2^2) + \\
& \eta t (-76 + 40 \mathfrak{z}2 + \mathfrak{el} (38 + 39 \mathfrak{z}1 - \mathfrak{z}2 - 10 \mathfrak{z}2^2))) + \\
& \eta^2 (12 \times (18 + \mathfrak{z}2) + \mathfrak{el} (-146 + 39 \mathfrak{z}1 - 49 \mathfrak{z}2 - 20 \mathfrak{z}2^2) - \\
& 4 \mathfrak{el}^2 (8 - 4 \mathfrak{z}2 + 5 \mathfrak{z}2^2) + \eta t (18 - 24 \mathfrak{z}2 + 4 \mathfrak{el}^2 (8 - 4 \mathfrak{z}2 + 5 \mathfrak{z}2^2) + \\
& \mathfrak{el} (146 - 39 \mathfrak{z}1 + 49 \mathfrak{z}2 + 20 \mathfrak{z}2^2))) + 2 \times (-1 + \eta) \eta (240 \eta^6 \mathfrak{op} - \\
& 8 \eta^4 \mathfrak{op} (4 + \eta t (-45 + \mathfrak{el} (-15 + \mathfrak{z}2) - \mathfrak{z}2) - \mathfrak{el} (-15 + \mathfrak{z}2) - \mathfrak{z}2) - \\
& 16 \eta^5 \mathfrak{op} (35 - 5 \mathfrak{el} + 5 \eta t (2 + \mathfrak{el}) + \mathfrak{z}2) + 4 \eta t \mathfrak{op} (-13 + 5 \mathfrak{z}2) + \\
& 4 \eta^3 \mathfrak{op} (196 + 8 \mathfrak{z}2 - 4 \eta t (15 + \mathfrak{z}2) - \mathfrak{el} (98 + 22 \mathfrak{z}2 + 5 \mathfrak{z}2^2) + \\
& \eta t \mathfrak{el} (98 + 22 \mathfrak{z}2 + 5 \mathfrak{z}2^2)) + \eta (8 \eta t \mathfrak{op} (13 - 5 \mathfrak{z}2) - \\
& (-1 + \eta t) \mathfrak{el} (2 \times (-6 + 5 \mathfrak{z}2) + \mathfrak{op} (64 + 66 \mathfrak{z}1 + 2 \mathfrak{z}2 - 15 \mathfrak{z}2^2))) - \\
& \eta^2 (8 \times (-1 + \eta t) \mathfrak{el}^2 \mathfrak{op} (8 - 4 \mathfrak{z}2 + 5 \mathfrak{z}2^2) + 4 \mathfrak{op} \\
& (\eta t (3 - 7 \mathfrak{z}2) + 6 \times (18 + \mathfrak{z}2)) + (-1 + \eta t) \mathfrak{el} \\
& (12 - 10 \mathfrak{z}2 + \mathfrak{op} (304 - 66 \mathfrak{z}1 + 94 \mathfrak{z}2 + 35 \mathfrak{z}2^2)))) + \\
& w (x (-1 + \eta) - \eta) (-1 + \eta) \times (-4 x^5 (-1 + \eta)^5 \mathfrak{op} (-148 + 30 \eta^4 + \\
& 124 \mathfrak{el} + 24 \mathfrak{el}^2 - 8 \mathfrak{z}2 + 24 \mathfrak{el} \mathfrak{z}2 - 12 \mathfrak{el}^2 \mathfrak{z}2 + 5 \mathfrak{el} \mathfrak{z}2^2 + 15 \mathfrak{el}^2 \mathfrak{z}2^2 - \\
& 3 \eta^3 (5 + 10 \eta t + \mathfrak{z}2) + \eta^2 (2 \eta t (25 + \mathfrak{z}2) + \mathfrak{el} (35 + \mathfrak{z}2) - \\
& \eta t \mathfrak{el} (35 + \mathfrak{z}2) - 2 \times (104 + \mathfrak{z}2)) + \eta (341 + 13 \mathfrak{z}2 - 2 \eta t (5 + 2 \mathfrak{z}2) - \\
& \mathfrak{el} (183 + 19 \mathfrak{z}2 + 5 \mathfrak{z}2^2) + \eta t \mathfrak{el} (183 + 19 \mathfrak{z}2 + 5 \mathfrak{z}2^2)) - \eta t
\end{aligned}$$

$$\begin{aligned}
& \left( -2 \times (-5 + \mathfrak{z}2) + 3 \, \mathfrak{el}^2 (8 - 4 \, \mathfrak{z}2 + 5 \, \mathfrak{z}2^2) + \mathfrak{el} (124 + 24 \, \mathfrak{z}2 + 5 \, \mathfrak{z}2^2) \right) + \\
& 4 \, x^4 (-1 + \eta)^4 \left( -3 \times (1 + 5 \, \eta) \times (-1 + \eta t) \, \mathfrak{el}^2 \, \mathfrak{op} (8 - 4 \, \mathfrak{z}2 + 5 \, \mathfrak{z}2^2) + \right. \\
& \quad (-1 + \eta)^2 \, \mathfrak{op} (150 \, \eta^3 + 2 \, \eta (-385 + 5 \, \eta t (-11 + \mathfrak{z}2) - 23 \, \mathfrak{z}2) + \\
& \quad \quad 3 \, \eta t (5 + \mathfrak{z}2) - 9 \times (18 + \mathfrak{z}2) - 15 \, \eta^2 (-21 + 10 \, \eta t + \mathfrak{z}2)) - \\
& \quad (-1 + \eta t) \, \mathfrak{el} (15 \times (-2 + \mathfrak{z}2) - 15 \, \eta (-2 + \mathfrak{z}2) + 5 \, \eta^3 \, \mathfrak{op} (41 + \mathfrak{z}2) + \\
& \quad \quad 12 \, \mathfrak{op} (14 + 3 \, \mathfrak{z}1 + 3 \, \mathfrak{z}2) + \eta \, \mathfrak{op} (443 - 36 \, \mathfrak{z}1 + 87 \, \mathfrak{z}2 + 25 \, \mathfrak{z}2^2) - \\
& \quad \quad \eta^2 \, \mathfrak{op} (960 + 92 \, \mathfrak{z}2 + 25 \, \mathfrak{z}2^2)) \left. \right) + x^3 \\
& (-1 + \eta)^3 \left( 24 \, \eta (2 + 5 \, \eta) \times (-1 + \eta t) \, \mathfrak{el}^2 \, \mathfrak{op} (8 - 4 \, \mathfrak{z}2 + 5 \, \mathfrak{z}2^2) + \right. \\
& \quad (-1 + \eta t) \, \mathfrak{el} (-136 + 60 \, \eta^2 (7 - 3 \, \mathfrak{z}2) + 40 \, \mathfrak{z}2 + 40 \, \eta^4 \, \mathfrak{op} (47 + \mathfrak{z}2) + \\
& \quad \quad 4 \, \eta (-71 + 35 \, \mathfrak{z}2) + 4 \, \mathfrak{op} (34 + 27 \, \mathfrak{z}1 + 7 \, \mathfrak{z}2 - 5 \, \mathfrak{z}2^2) + \eta \, \mathfrak{op} (2582 + \\
& \quad \quad 459 \, \mathfrak{z}1 + 563 \, \mathfrak{z}2 + 20 \, \mathfrak{z}2^2) - 8 \, \eta^3 \, \mathfrak{op} (1005 + 89 \, \mathfrak{z}2 + 25 \, \mathfrak{z}2^2) + \\
& \quad \quad \eta^2 \, \mathfrak{op} (2098 - 567 \, \mathfrak{z}1 + 417 \, \mathfrak{z}2 + 200 \, \mathfrak{z}2^2)) - 2 (-1 + \eta)^2 \, \mathfrak{op} \\
& \quad \quad (600 \, \eta^4 + 8 \, \eta^2 (-400 + 5 \, \eta t (-17 + \mathfrak{z}2) - 26 \, \mathfrak{z}2) - 60 \, \eta^3 (-27 + 10 \, \eta t + \\
& \quad \quad \quad \mathfrak{z}2) + 15 \, \eta t (-3 + 2 \, \mathfrak{z}2) + 24 \, \eta (\eta t (5 + \mathfrak{z}2) - 3 \times (18 + \mathfrak{z}2))) \left. \right) + \\
& \eta^2 \, \mathfrak{op} (120 \, \eta^7 - 12 \, \eta^6 (-25 + 10 \, \eta t + \mathfrak{z}2) + 2 \, \eta t (-49 + 20 \, \mathfrak{z}2) - \\
& \quad 4 \, \eta^5 (418 - 2 \, \eta t (-5 + \mathfrak{z}2) + 8 \, \mathfrak{z}2 - \mathfrak{el} (65 + \mathfrak{z}2) + \eta t \, \mathfrak{el} (65 + \mathfrak{z}2)) + \\
& \quad \eta (\mathfrak{el} (98 + 81 \, \mathfrak{z}1 + 9 \, \mathfrak{z}2 - 20 \, \mathfrak{z}2^2) - \\
& \quad \quad \eta t (-82 + 20 \, \mathfrak{z}2 + \mathfrak{el} (98 + 81 \, \mathfrak{z}1 + 9 \, \mathfrak{z}2 - 20 \, \mathfrak{z}2^2))) + \\
& \quad \eta^3 (8 \times (73 + 2 \, \mathfrak{z}2) - \mathfrak{el} (206 + 117 \, \mathfrak{z}1 + 33 \, \mathfrak{z}2 - 20 \, \mathfrak{z}2^2) + \\
& \quad \quad 12 \, \mathfrak{el}^2 (8 - 4 \, \mathfrak{z}2 + 5 \, \mathfrak{z}2^2) + \eta t (-514 + 44 \, \mathfrak{z}2 + \\
& \quad \quad \quad \mathfrak{el} (206 + 117 \, \mathfrak{z}1 + 33 \, \mathfrak{z}2 - 20 \, \mathfrak{z}2^2) - 12 \, \mathfrak{el}^2 (8 - 4 \, \mathfrak{z}2 + 5 \, \mathfrak{z}2^2))) \left. \right) + \\
& 4 \, \eta^4 (329 + 16 \, \mathfrak{z}2 - \mathfrak{el} (228 + 16 \, \mathfrak{z}2 + 5 \, \mathfrak{z}2^2) + \eta t (125 - \mathfrak{z}2 + \\
& \quad \mathfrak{el} (228 + 16 \, \mathfrak{z}2 + 5 \, \mathfrak{z}2^2))) - 2 \, \eta^2 (-2 \times (-9 \times (18 + \mathfrak{z}2) + \\
& \quad \quad 3 \, \mathfrak{el}^2 (8 - 4 \, \mathfrak{z}2 + 5 \, \mathfrak{z}2^2) + \mathfrak{el} (142 + 9 \, \mathfrak{z}1 + 33 \, \mathfrak{z}2 + 5 \, \mathfrak{z}2^2)) + \\
& \quad \eta t (-95 + 34 \, \mathfrak{z}2 + 6 \, \mathfrak{el}^2 (8 - 4 \, \mathfrak{z}2 + 5 \, \mathfrak{z}2^2) + 2 \, \mathfrak{el} \\
& \quad \quad (142 + 9 \, \mathfrak{z}1 + 33 \, \mathfrak{z}2 + 5 \, \mathfrak{z}2^2))) \left. \right) + x^2 (-1 + \eta)^2 (1200 \, \eta^7 \, \mathfrak{op} - \\
& 120 \, \eta^6 \, \mathfrak{op} (-13 + 10 \, \eta t + \mathfrak{z}2) + 20 \, \eta t \, \mathfrak{op} (-7 + 2 \, \mathfrak{z}2) - 8 \, \eta^5 \, \mathfrak{op} \\
& \quad (1670 + 28 \, \mathfrak{z}2 - 5 \, \mathfrak{el} (53 + \mathfrak{z}2) + 5 \, \eta t (-2 \times (7 + \mathfrak{z}2) + \mathfrak{el} (53 + \mathfrak{z}2))) + \\
& \quad \eta^3 (-120 \times (-1 + \eta t) \, \mathfrak{el}^2 \, \mathfrak{op} (8 - 4 \, \mathfrak{z}2 + 5 \, \mathfrak{z}2^2) + \\
& \quad \quad 2 \, \mathfrak{op} (568 - 16 \, \mathfrak{z}2 + \eta t (-1481 + 58 \, \mathfrak{z}2)) + (-1 + \eta t) \, \mathfrak{el} \\
& \quad \quad (-372 + 180 \, \mathfrak{z}2 + \mathfrak{op} (-658 + 819 \, \mathfrak{z}1 - 141 \, \mathfrak{z}2 - 200 \, \mathfrak{z}2^2))) \left. \right) + \\
& \eta (2 \, \eta t \, \mathfrak{op} (-61 + 50 \, \mathfrak{z}2) - (-1 + \eta t) \, \mathfrak{el} (-230 + 80 \, \mathfrak{z}2 + \\
& \quad \mathfrak{op} (370 + 297 \, \mathfrak{z}1 + 65 \, \mathfrak{z}2 - 60 \, \mathfrak{z}2^2))) + \\
& 8 \, \eta^4 \, \mathfrak{op} (1669 + 74 \, \mathfrak{z}2 - \mathfrak{el} (1050 + 86 \, \mathfrak{z}2 + 25 \, \mathfrak{z}2^2) + \\
& \quad \eta t (355 - 11 \, \mathfrak{z}2 + \mathfrak{el} (1050 + 86 \, \mathfrak{z}2 + 25 \, \mathfrak{z}2^2))) - \\
& 2 \, \eta^2 (36 \times (-1 + \eta t) \, \mathfrak{el}^2 \, \mathfrak{op} (8 - 4 \, \mathfrak{z}2 + 5 \, \mathfrak{z}2^2) + 4 \, \mathfrak{op} \\
& \quad (27 \times (18 + \mathfrak{z}2) + \eta t (-128 + 31 \, \mathfrak{z}2)) + (-1 + \eta t) \, \mathfrak{el} \\
& \quad (-71 + 50 \, \mathfrak{z}2 + \mathfrak{op} (1858 + 261 \, \mathfrak{z}1 + 413 \, \mathfrak{z}2 + 30 \, \mathfrak{z}2^2))) \left. \right) - x \\
& (-1 + \eta) \, \eta (600 \, \eta^7 \, \mathfrak{op} - 60 \, \eta^6 \, \mathfrak{op} (-19 + 10 \, \eta t + \mathfrak{z}2) + 2 \, \eta t \, \mathfrak{op} \\
& \quad (-137 + 40 \, \mathfrak{z}2) - 4 \, \eta^5 \, \mathfrak{op} (1880 + 34 \, \mathfrak{z}2 - 5 \, \mathfrak{el} (59 + \mathfrak{z}2) + \\
& \quad \quad 5 \, \eta t (-2 \times (1 + \mathfrak{z}2) + \mathfrak{el} (59 + \mathfrak{z}2))) + \eta^3 (-60 \times (-1 + \eta t) \, \mathfrak{el}^2 \, \mathfrak{op} \\
& \quad \quad (8 - 4 \, \mathfrak{z}2 + 5 \, \mathfrak{z}2^2) + 2 \, \mathfrak{op} (872 + 16 \, \mathfrak{z}2 + \eta t (-1033 + 62 \, \mathfrak{z}2)) + \\
& \quad \quad (-1 + \eta t) \, \mathfrak{el} (-72 + 60 \, \mathfrak{z}2 + \mathfrak{op} (370 + 513 \, \mathfrak{z}1 + 57 \, \mathfrak{z}2 - 100 \, \mathfrak{z}2^2))) \left. \right) +
\end{aligned}$$



$$\begin{aligned}
& \eta \left( 2 \eta t \operatorname{ep} (61 + 10 \mathfrak{z}^2) - 2 \times (-1 + \eta t) \operatorname{el} (-29 + 20 \mathfrak{z}^2 + \right. \\
& \quad \left. \operatorname{ep} (166 + 135 \mathfrak{z}^1 + 23 \mathfrak{z}^2 - 30 \mathfrak{z}^2^2)) \right) + \\
& 4 \eta^4 \operatorname{ep} (1657 + 77 \mathfrak{z}^2 - \operatorname{el} (1095 + 83 \mathfrak{z}^2 + 25 \mathfrak{z}^2^2)) + \\
& \quad \eta t (490 - 8 \mathfrak{z}^2 + \operatorname{el} (1095 + 83 \mathfrak{z}^2 + 25 \mathfrak{z}^2^2)) - \\
& \eta^2 (48 \times (-1 + \eta t) \operatorname{el}^2 \operatorname{ep} (8 - 4 \mathfrak{z}^2 + 5 \mathfrak{z}^2^2) + 2 \operatorname{ep} \\
& \quad (72 \times (18 + \mathfrak{z}^2) + \eta t (-409 + 116 \mathfrak{z}^2)) + (-1 + \eta t) \operatorname{el} \\
& \quad (-14 + 20 \mathfrak{z}^2 + \operatorname{ep} (2374 + 243 \mathfrak{z}^1 + 539 \mathfrak{z}^2 + 60 \mathfrak{z}^2^2))) + \\
& w^4 (-1 + \eta)^4 (12 x^5 (-1 + \eta)^5 (-1 + \eta t) \operatorname{el} \operatorname{ep} (2 \times (-4 + \mathfrak{z}^2) + \\
& \quad \operatorname{el} (8 - 4 \mathfrak{z}^2 + 5 \mathfrak{z}^2^2)) - 2 x^4 (-1 + \eta)^4 \\
& (6 \times (3 + 5 \eta) \times (-1 + \eta t) \operatorname{el}^2 \operatorname{ep} (8 - 4 \mathfrak{z}^2 + 5 \mathfrak{z}^2^2) - 6 (-1 + \eta)^2 \\
& \quad \operatorname{ep} (-54 + 10 \eta^2 + \eta t (-15 + \mathfrak{z}^2) - 5 \mathfrak{z}^2 - \eta (-15 + 10 \eta t + \mathfrak{z}^2)) - \\
& (-1 + \eta t) \operatorname{el} (68 - 20 \mathfrak{z}^2 - \operatorname{ep} (248 + 54 \mathfrak{z}^1 + 98 \mathfrak{z}^2 + 5 \mathfrak{z}^2^2)) + \\
& \quad \eta (-68 + 20 \mathfrak{z}^2 + \operatorname{ep} (632 + 54 \mathfrak{z}^1 + 2 \mathfrak{z}^2 + 5 \mathfrak{z}^2^2))) + 3 x^2 (-1 + \eta)^2 \\
& (240 \eta^6 \operatorname{ep} - 24 \eta^5 \operatorname{ep} (10 \eta t + \mathfrak{z}^2) + 2 \eta t \operatorname{ep} (-31 + 10 \mathfrak{z}^2) + 12 \\
& \quad \eta^4 \operatorname{ep} (-153 + (-7 + 2 \eta t) \mathfrak{z}^2) - 2 \eta (\operatorname{ep} (296 + 27 \eta t + 16 \mathfrak{z}^2 - 4 \eta t \mathfrak{z}^2) + \\
& \quad 6 \times (-1 + \eta t) \operatorname{el}^2 \operatorname{ep} (8 - 4 \mathfrak{z}^2 + 5 \mathfrak{z}^2^2) + (-1 + \eta t) \operatorname{el} \\
& \quad (-41 + 20 \mathfrak{z}^2 + \operatorname{ep} (320 + 54 \mathfrak{z}^1 + 54 \mathfrak{z}^2 - 5 \mathfrak{z}^2^2))) + \\
& \eta^3 (2 \operatorname{ep} (1060 + 271 \eta t + 104 \mathfrak{z}^2) - 40 \times (-1 + \eta t) \operatorname{el}^2 \operatorname{ep} \\
& \quad (8 - 4 \mathfrak{z}^2 + 5 \mathfrak{z}^2^2) + (-1 + \eta t) \operatorname{el} (-96 + 189 \operatorname{ep} \mathfrak{z}^1 + 40 \mathfrak{z}^2 + \\
& \quad 5 \operatorname{ep} (342 + 29 \mathfrak{z}^2 + 4 \mathfrak{z}^2^2))) - \eta^2 (72 \times (-1 + \eta t) \operatorname{el}^2 \operatorname{ep} \\
& \quad (8 - 4 \mathfrak{z}^2 + 5 \mathfrak{z}^2^2) + 2 \operatorname{ep} (34 \times (-1 + \mathfrak{z}^2) + \eta t (93 + 26 \mathfrak{z}^2)) + \\
& (-1 + \eta t) \operatorname{el} (-14 + 3 \operatorname{ep} (26 + 27 \mathfrak{z}^1 + 95 \mathfrak{z}^2 + 10 \mathfrak{z}^2^2))) + \eta^2 \operatorname{ep} \\
& (120 \eta^6 + 12 \eta^4 (-79 + \eta t (-5 + \mathfrak{z}^2) - 4 \mathfrak{z}^2) - 12 \eta^5 (-5 + 10 \eta t + \mathfrak{z}^2) + \\
& \quad 12 \eta t (-12 + 5 \mathfrak{z}^2) - 2 \eta (8 \times (37 + 2 \mathfrak{z}^2) - \operatorname{el} (320 + 54 \mathfrak{z}^1 + \\
& \quad 54 \mathfrak{z}^2 - 5 \mathfrak{z}^2^2) - 6 \operatorname{el}^2 (8 - 4 \mathfrak{z}^2 + 5 \mathfrak{z}^2^2) + \eta t (-75 + 36 \mathfrak{z}^2 + \\
& \quad \operatorname{el} (320 + 54 \mathfrak{z}^1 + 54 \mathfrak{z}^2 - 5 \mathfrak{z}^2^2) + 6 \operatorname{el}^2 (8 - 4 \mathfrak{z}^2 + 5 \mathfrak{z}^2^2))) + \\
& \eta^3 (644 + 100 \mathfrak{z}^2 + 12 \operatorname{el}^2 (8 - 4 \mathfrak{z}^2 + 5 \mathfrak{z}^2^2) - \operatorname{el} (702 + \\
& \quad 81 \mathfrak{z}^1 + 77 \mathfrak{z}^2 + 10 \mathfrak{z}^2^2) + \eta t (6 \times (57 + 4 \mathfrak{z}^2) - \\
& \quad 12 \operatorname{el}^2 (8 - 4 \mathfrak{z}^2 + 5 \mathfrak{z}^2^2) + \operatorname{el} (702 + 81 \mathfrak{z}^1 + 77 \mathfrak{z}^2 + 10 \mathfrak{z}^2^2))) - \\
& \eta^2 (-716 + 8 \mathfrak{z}^2 + \operatorname{el} (418 + 27 \mathfrak{z}^1 - 89 \mathfrak{z}^2 - 20 \mathfrak{z}^2^2) - 36 \operatorname{el}^2 \\
& \quad (8 - 4 \mathfrak{z}^2 + 5 \mathfrak{z}^2^2) + \eta t (24 \times (7 + \mathfrak{z}^2) + 36 \operatorname{el}^2 (8 - 4 \mathfrak{z}^2 + 5 \mathfrak{z}^2^2) + \\
& \quad \operatorname{el} (-418 - 27 \mathfrak{z}^1 + 89 \mathfrak{z}^2 + 20 \mathfrak{z}^2^2))) + x^3 (-1 + \eta)^3 \\
& (12 \times (1 + 12 \eta + 10 \eta^2) \times (-1 + \eta t) \operatorname{el}^2 \operatorname{ep} (8 - 4 \mathfrak{z}^2 + 5 \mathfrak{z}^2^2) - \\
& \quad 4 (-1 + \eta)^2 \operatorname{ep} (-148 + 120 \eta^3 - 45 \eta t - 8 \mathfrak{z}^2 + 12 \eta t \mathfrak{z}^2 + \\
& \quad 6 \eta \eta t (-35 + 2 \mathfrak{z}^2) - 6 \eta^2 (-35 + 20 \eta t + 2 \mathfrak{z}^2) - 9 \eta (67 + 7 \mathfrak{z}^2)) - \\
& (-1 + \eta t) \operatorname{el} (-2 \times (-72 + 30 \mathfrak{z}^2 + \operatorname{ep} (320 + 54 \mathfrak{z}^1 + 54 \mathfrak{z}^2 - 5 \mathfrak{z}^2^2)) + \\
& \quad \eta^2 (6 \times (-61 + 20 \mathfrak{z}^2) + \operatorname{ep} (3918 + 405 \mathfrak{z}^1 + 233 \mathfrak{z}^2 + 40 \mathfrak{z}^2^2)) - \\
& \quad \eta (-222 + 60 \mathfrak{z}^2 + \operatorname{ep} (1070 + 297 \mathfrak{z}^1 + 677 \mathfrak{z}^2 + 50 \mathfrak{z}^2^2))) - x \\
& (-1 + \eta) \eta (480 \eta^6 \operatorname{ep} - 24 \eta^5 \operatorname{ep} (-5 + 20 \eta t + 2 \mathfrak{z}^2) + 6 \eta t \operatorname{ep} \\
& \quad (-61 + 20 \mathfrak{z}^2) + 12 \eta^4 \operatorname{ep} (-311 - 15 \mathfrak{z}^2 + 2 \eta t (-5 + 2 \mathfrak{z}^2)) - \\
& 6 \eta (6 \times (-1 + \eta t) \operatorname{el}^2 \operatorname{ep} (8 - 4 \mathfrak{z}^2 + 5 \mathfrak{z}^2^2) + \\
& \quad 8 \operatorname{ep} (37 + 2 \mathfrak{z}^2 + \eta t (-5 + 2 \mathfrak{z}^2)) + (-1 + \eta t) \operatorname{el} (-11 + 10 \mathfrak{z}^2 +
\end{aligned}$$

$$\begin{aligned}
& \left( \text{op} \left( 320 + 54 \, \mathfrak{z}1 + 54 \, \mathfrak{z}2 - 5 \, \mathfrak{z}2^2 \right) \right) + \eta^3 \left( -60 \times (-1 + \eta t) \, \text{el}^2 \, \text{op} \right. \\
& \left( 8 - 4 \, \mathfrak{z}2 + 5 \, \mathfrak{z}2^2 \right) + 12 \, \text{op} \left( 284 + 34 \, \mathfrak{z}2 + \eta t \left( 99 + 4 \, \mathfrak{z}2 \right) \right) + \\
& \left. (-1 + \eta t) \, \text{el} \left( -58 + 40 \, \mathfrak{z}2 + \text{op} \left( 3082 + 351 \, \mathfrak{z}1 + 307 \, \mathfrak{z}2 + 40 \, \mathfrak{z}2^2 \right) \right) \right) - \\
& \eta^2 \left( 144 \times (-1 + \eta t) \, \text{el}^2 \, \text{op} \left( 8 - 4 \, \mathfrak{z}2 + 5 \, \mathfrak{z}2^2 \right) + 6 \, \text{op} \right. \\
& \left( -250 + 14 \, \mathfrak{z}2 + \eta t \left( 77 + 20 \, \mathfrak{z}2 \right) \right) + (-1 + \eta t) \, \text{el} \\
& \left. \left( 8 - 20 \, \mathfrak{z}2 + \text{op} \left( -758 + 27 \, \mathfrak{z}1 + 463 \, \mathfrak{z}2 + 70 \, \mathfrak{z}2^2 \right) \right) \right) + \\
& w^3 \left( -1 + \eta \right)^3 \left( 4 \, x^6 \left( -1 + \eta \right)^6 \left( -1 + \eta t \right) \, \text{el} \, \text{op} \left( 2 \times (-4 + \mathfrak{z}2) + \right. \right. \\
& \left. \left. \text{el} \left( 8 - 4 \, \mathfrak{z}2 + 5 \, \mathfrak{z}2^2 \right) \right) - 4 \, x^5 \left( -1 + \eta \right)^5 \right. \\
& \left( 3 \times (3 + 2 \, \eta) \times (-1 + \eta t) \, \text{el}^2 \, \text{op} \left( 8 - 4 \, \mathfrak{z}2 + 5 \, \mathfrak{z}2^2 \right) - 3 \left( -1 + \eta \right)^2 \right. \\
& \left. \text{op} \left( -54 + 10 \, \eta^2 + \eta t \left( -15 + \mathfrak{z}2 \right) - 5 \, \mathfrak{z}2 - \eta \left( -15 + 10 \, \eta t + \mathfrak{z}2 \right) \right) - \right. \\
& \left. (-1 + \eta t) \, \text{el} \left( -5 \times (-2 + \mathfrak{z}2) + 5 \, \eta \left( -2 + \mathfrak{z}2 \right) + \eta \, \text{op} \right. \right. \\
& \left. \left. \left( 220 + 12 \, \mathfrak{z}1 + 12 \, \mathfrak{z}2 + 5 \, \mathfrak{z}2^2 \right) - \text{op} \left( 100 + 12 \, \mathfrak{z}1 + 42 \, \mathfrak{z}2 + 5 \, \mathfrak{z}2^2 \right) \right) \right) + \\
& \eta^2 \, \text{op} \left( -120 \, \eta^7 - 12 \, \eta^5 \left( -79 + \eta t \left( -25 + \mathfrak{z}2 \right) - 6 \, \mathfrak{z}2 \right) + 12 \, \eta t \right. \\
& \left. \left( 12 - 5 \, \mathfrak{z}2 \right) + 12 \, \eta^6 \left( -25 + 10 \, \eta t + \mathfrak{z}2 \right) + \right. \\
& 2 \, \eta \left( -2 \times (-3 \times (18 + \mathfrak{z}2) + \text{el} \left( 82 + 27 \, \mathfrak{z}1 + 15 \, \mathfrak{z}2 - 5 \, \mathfrak{z}2^2 \right) + \right. \\
& \left. \text{el}^2 \left( 8 - 4 \, \mathfrak{z}2 + 5 \, \mathfrak{z}2^2 \right) \right) + \eta t \left( -7 - 2 \, \mathfrak{z}2 + 2 \, \text{el} \right. \\
& \left. \left( 82 + 27 \, \mathfrak{z}1 + 15 \, \mathfrak{z}2 - 5 \, \mathfrak{z}2^2 \right) + 2 \, \text{el}^2 \left( 8 - 4 \, \mathfrak{z}2 + 5 \, \mathfrak{z}2^2 \right) \right) \right) + \\
& 2 \, \eta^3 \left( -2 \times (857 + 25 \, \mathfrak{z}2 - \text{el} \left( 538 + 51 \, \mathfrak{z}1 + 21 \, \mathfrak{z}2 - 5 \, \mathfrak{z}2^2 \right) + \right. \\
& 9 \, \text{el}^2 \left( 8 - 4 \, \mathfrak{z}2 + 5 \, \mathfrak{z}2^2 \right) \right) + \eta t \left( 169 - 24 \, \mathfrak{z}2 - \right. \\
& 2 \, \text{el} \left( 538 + 51 \, \mathfrak{z}1 + 21 \, \mathfrak{z}2 - 5 \, \mathfrak{z}2^2 \right) + 18 \, \text{el}^2 \left( 8 - 4 \, \mathfrak{z}2 + 5 \, \mathfrak{z}2^2 \right) \right) \right) + \\
& \eta^4 \left( 1300 - 76 \, \mathfrak{z}2 - 4 \, \text{el}^2 \left( 8 - 4 \, \mathfrak{z}2 + 5 \, \mathfrak{z}2^2 \right) + \text{el} \left( 258 + 39 \, \mathfrak{z}1 + \right. \right. \\
& \left. 75 \, \mathfrak{z}2 + 20 \, \mathfrak{z}2^2 \right) + \eta t \left( -722 - 20 \, \mathfrak{z}2 + 4 \, \text{el}^2 \left( 8 - 4 \, \mathfrak{z}2 + 5 \, \mathfrak{z}2^2 \right) - \right. \\
& \left. \text{el} \left( 258 + 39 \, \mathfrak{z}1 + 75 \, \mathfrak{z}2 + 20 \, \mathfrak{z}2^2 \right) \right) \right) + \eta^2 \left( 1384 + 80 \, \mathfrak{z}2 - \right. \\
& 36 \, \text{el}^2 \left( 8 - 4 \, \mathfrak{z}2 + 5 \, \mathfrak{z}2^2 \right) - \text{el} \left( 1442 + 135 \, \mathfrak{z}1 + 259 \, \mathfrak{z}2 + 20 \, \mathfrak{z}2^2 \right) + \\
& \eta t \left( 2 \times (-83 + 72 \, \mathfrak{z}2) + 36 \, \text{el}^2 \left( 8 - 4 \, \mathfrak{z}2 + 5 \, \mathfrak{z}2^2 \right) + \right. \\
& \left. \text{el} \left( 1442 + 135 \, \mathfrak{z}1 + 259 \, \mathfrak{z}2 + 20 \, \mathfrak{z}2^2 \right) \right) \right) + x \left( -1 + \eta \right) \\
& \eta \left( 600 \, \eta^7 \, \text{op} + 12 \, \eta^5 \, \text{op} \left( -400 + 5 \, \eta t \left( -19 + \mathfrak{z}2 \right) - 27 \, \mathfrak{z}2 \right) - \right. \\
& 60 \, \eta^6 \, \text{op} \left( -19 + 10 \, \eta t + \mathfrak{z}2 \right) + 6 \, \eta t \, \text{op} \left( -61 + 20 \, \mathfrak{z}2 \right) + \\
& \eta^3 \left( -180 \times (-1 + \eta t) \, \text{el}^2 \, \text{op} \left( 8 - 4 \, \mathfrak{z}2 + 5 \, \mathfrak{z}2^2 \right) + \right. \\
& 4 \, \text{op} \left( 3270 + 84 \, \mathfrak{z}2 + \eta t \left( -399 + 20 \, \mathfrak{z}2 \right) \right) + (-1 + \eta t) \, \text{el} \\
& \left. \left( 50 \times (-3 + 2 \, \mathfrak{z}2) + \text{op} \left( 8250 + 843 \, \mathfrak{z}1 + 223 \, \mathfrak{z}2 - 100 \, \mathfrak{z}2^2 \right) \right) \right) - \\
& 6 \, \eta \left( 2 \, \text{op} \left( 54 + 27 \, \eta t + 3 \, \mathfrak{z}2 - 11 \, \eta t \, \mathfrak{z}2 \right) + 2 \times (-1 + \eta t) \right. \\
& \left. \text{el}^2 \, \text{op} \left( 8 - 4 \, \mathfrak{z}2 + 5 \, \mathfrak{z}2^2 \right) + (-1 + \eta t) \, \text{el} \right. \\
& \left. \left( -11 + 10 \, \mathfrak{z}2 + 2 \, \text{op} \left( 82 + 27 \, \mathfrak{z}1 + 15 \, \mathfrak{z}2 - 5 \, \mathfrak{z}2^2 \right) \right) \right) - \\
& \eta^2 \left( 144 \times (-1 + \eta t) \, \text{el}^2 \, \text{op} \left( 8 - 4 \, \mathfrak{z}2 + 5 \, \mathfrak{z}2^2 \right) + 2 \, \text{op} \right. \\
& \left. \left( 2964 + 168 \, \mathfrak{z}2 + \eta t \left( -423 + 224 \, \mathfrak{z}2 \right) \right) + 3 \times (-1 + \eta t) \, \text{el} \right. \\
& \left. \left( 4 \times (-9 + 5 \, \mathfrak{z}2) + \text{op} \left( 2074 + 243 \, \mathfrak{z}1 + 383 \, \mathfrak{z}2 + 20 \, \mathfrak{z}2^2 \right) \right) \right) - \\
& 2 \, \eta^4 \left( -2 \, \text{op} \left( -861 + 795 \, \eta t + 105 \, \mathfrak{z}2 + 14 \, \eta t \, \mathfrak{z}2 \right) + 12 \times \right. \\
& \left. (-1 + \eta t) \, \text{el}^2 \, \text{op} \left( 8 - 4 \, \mathfrak{z}2 + 5 \, \mathfrak{z}2^2 \right) - (-1 + \eta t) \, \text{el} \right. \\
& \left. \left( 2 \times (-6 + 5 \, \mathfrak{z}2) + \text{op} \left( 918 + 105 \, \mathfrak{z}1 + 193 \, \mathfrak{z}2 + 50 \, \mathfrak{z}2^2 \right) \right) \right) \right) - x^2 \\
& (-1 + \eta)^2 \left( 1200 \, \eta^7 \, \text{op} - 120 \, \eta^6 \, \text{op} \left( -13 + 10 \, \eta t + \mathfrak{z}2 \right) + 6 \, \eta t \, \text{op} \right. \\
& \left. \left( -31 + 10 \, \mathfrak{z}2 \right) + 24 \, \eta^5 \, \text{op} \left( 5 \, \eta t \left( -13 + \mathfrak{z}2 \right) - 8 \times (50 + 3 \, \mathfrak{z}2) \right) + \right. \\
& \left. \eta^3 \left( -360 \times (-1 + \eta t) \, \text{el}^2 \, \text{op} \left( 8 - 4 \, \mathfrak{z}2 + 5 \, \mathfrak{z}2^2 \right) - \right. \right.
\end{aligned}$$

$$\begin{aligned}
& 6 \, \text{op} \, (-3004 - 58 \, \mathfrak{z}2 + \eta \mathfrak{t} \, (445 + 6 \, \mathfrak{z}2)) + (-1 + \eta \mathfrak{t}) \, \text{el} \\
& \quad (-716 + 280 \, \mathfrak{z}2 + \text{op} \, (11438 + 1257 \, \mathfrak{z}1 - 3 \, \mathfrak{z}2 - 200 \, \mathfrak{z}2^2)) - \\
& 6 \, \eta \, (3 \, \text{op} \, (36 + 45 \, \eta \mathfrak{t} + 2 \, \mathfrak{z}2 - 14 \, \eta \mathfrak{t} \, \mathfrak{z}2) + 2 \times (-1 + \eta \mathfrak{t}) \\
& \quad \text{el}^2 \, \text{op} \, (8 - 4 \, \mathfrak{z}2 + 5 \, \mathfrak{z}2^2) + (-1 + \eta \mathfrak{t}) \, \text{el} \\
& \quad (-41 + 20 \, \mathfrak{z}2 + 2 \, \text{op} \, (82 + 27 \, \mathfrak{z}1 + 15 \, \mathfrak{z}2 - 5 \, \mathfrak{z}2^2))) - \\
& 3 \, \eta^2 \, (72 \times (-1 + \eta \mathfrak{t}) \, \text{el}^2 \, \text{op} \, (8 - 4 \, \mathfrak{z}2 + 5 \, \mathfrak{z}2^2) + 2 \, \text{op} \\
& \quad (1580 + 88 \, \mathfrak{z}2 + \eta \mathfrak{t} \, (-157 + 70 \, \mathfrak{z}2)) + (-1 + \eta \mathfrak{t}) \, \text{el} \\
& \quad (-206 + 80 \, \mathfrak{z}2 + \text{op} \, (3338 + 459 \, \mathfrak{z}1 + 631 \, \mathfrak{z}2 + 20 \, \mathfrak{z}2^2))) - \\
& 4 \, \eta^4 \, (15 \times (-1 + \eta \mathfrak{t}) \, \text{el}^2 \, \text{op} \, (8 - 4 \, \mathfrak{z}2 + 5 \, \mathfrak{z}2^2) - 3 \, \text{op} \\
& \quad (-88 + 76 \, \mathfrak{z}2 + \eta \mathfrak{t} \, (457 + 2 \, \mathfrak{z}2)) - (-1 + \eta \mathfrak{t}) \, \text{el} \\
& \quad (-37 + 20 \, \mathfrak{z}2 + \text{op} \, (1186 + 111 \, \mathfrak{z}1 + 195 \, \mathfrak{z}2 + 50 \, \mathfrak{z}2^2))) + \mathfrak{x}^4 \\
& (-1 + \eta)^4 \, (12 \times (3 + 15 \, \eta + 5 \, \eta^2) \times (-1 + \eta \mathfrak{t}) \, \text{el}^2 \, \text{op} \, (8 - 4 \, \mathfrak{z}2 + 5 \, \mathfrak{z}2^2) - \\
& \quad 2 \, (-1 + \eta)^2 \, \text{op} \, (-888 + 300 \, \eta^3 - 75 \, \eta \mathfrak{t} + 6 \, \eta \, (-225 + 5 \, \eta \mathfrak{t} \, (-21 + \mathfrak{z}2) - \\
& \quad 28 \, \mathfrak{z}2) - 48 \, \mathfrak{z}2 + 22 \, \eta \mathfrak{t} \, \mathfrak{z}2 - 30 \, \eta^2 \, (-21 + 10 \, \eta \mathfrak{t} + \mathfrak{z}2)) - \\
& \quad (-1 + \eta \mathfrak{t}) \, \text{el} \, (-12 \times (-34 + 10 \, \mathfrak{z}2 + \text{op} \, (158 + 27 \, \mathfrak{z}1 + 31 \, \mathfrak{z}2)) + \\
& \quad \eta \, (-228 + 40 \, \mathfrak{z}2 + \text{op} \, (594 + 87 \, \mathfrak{z}1 - 533 \, \mathfrak{z}2 - 100 \, \mathfrak{z}2^2)) + \\
& \quad \eta^2 \, (20 \times (-9 + 4 \, \mathfrak{z}2) + \text{op} \, (3510 + 237 \, \mathfrak{z}1 + 353 \, \mathfrak{z}2 + 100 \, \mathfrak{z}2^2)))) - \\
& \mathfrak{x}^3 \, (-1 + \eta)^3 \, (4 \times (1 + 36 \, \eta + 90 \, \eta^2 + 20 \, \eta^3) \times (-1 + \eta \mathfrak{t}) \, \text{el}^2 \\
& \quad \text{op} \, (8 - 4 \, \mathfrak{z}2 + 5 \, \mathfrak{z}2^2) - 4 \, (-1 + \eta)^2 \, \text{op} \\
& \quad (300 \, \eta^4 + 6 \, \eta^2 \, (-175 + 5 \, \eta \mathfrak{t} \, (-27 + \mathfrak{z}2) - 31 \, \mathfrak{z}2) - \\
& \quad 3 \times (18 + \mathfrak{z}2) - 30 \, \eta^3 \, (-27 + 10 \, \eta \mathfrak{t} + \mathfrak{z}2) + \eta \mathfrak{t} \, (-100 + 31 \, \mathfrak{z}2) + \\
& \quad \eta \, (-1786 - 181 \, \eta \mathfrak{t} - 98 \, \mathfrak{z}2 + 44 \, \eta \mathfrak{t} \, \mathfrak{z}2)) - (-1 + \eta \mathfrak{t}) \, \text{el} \\
& \quad (\eta^2 \, (-834 + 240 \, \mathfrak{z}2 + \text{op} \, (6334 + 753 \, \mathfrak{z}1 - 507 \, \mathfrak{z}2 - 200 \, \mathfrak{z}2^2)) - \\
& \quad 4 \times (-36 + 15 \, \mathfrak{z}2 + \text{op} \, (82 + 27 \, \mathfrak{z}1 + 15 \, \mathfrak{z}2 - 5 \, \mathfrak{z}2^2)) - \\
& \quad \eta \, (-954 + 300 \, \mathfrak{z}2 + \text{op} \, (7130 + 1107 \, \mathfrak{z}1 + 1375 \, \mathfrak{z}2 + 20 \, \mathfrak{z}2^2)) + \\
& \quad 2 \, \eta^3 \, (-132 + 60 \, \mathfrak{z}2 + \text{op} \, (2914 + 231 \, \mathfrak{z}1 + 383 \, \mathfrak{z}2 + 100 \, \mathfrak{z}2^2)))) - \\
& \mathfrak{w}^2 \, (-1 + \eta)^2 \, (-6 \, \mathfrak{x}^5 \, (-1 + \eta)^5 \, (6 \times (1 + 2 \, \eta) \times (-1 + \eta \mathfrak{t}) \, \text{el}^2 \, \text{op} \, (8 - 4 \, \mathfrak{z}2 + \\
& \quad 5 \, \mathfrak{z}2^2) - 2 \, (-1 + \eta)^2 \, \text{op} \, (20 \, \eta^3 + \eta \, (-63 + 2 \, \eta \mathfrak{t} \, (-30 + \mathfrak{z}2) - 13 \, \mathfrak{z}2) + \\
& \quad 2 \times (-74 + \eta \mathfrak{t} \, (-5 + \mathfrak{z}2) - 4 \, \mathfrak{z}2) - 2 \, \eta^2 \, (-30 + 10 \, \eta \mathfrak{t} + \mathfrak{z}2)) - \\
& \quad (-1 + \eta \mathfrak{t}) \, \text{el} \, (-10 \times (-2 + \mathfrak{z}2) + 10 \, \eta \, (-2 + \mathfrak{z}2) + \eta \, \text{op} \\
& \quad (266 + 24 \, \mathfrak{z}1 - 18 \, \mathfrak{z}2 - 5 \, \mathfrak{z}2^2) + 2 \, \eta^2 \, \text{op} \, (73 + 15 \, \mathfrak{z}2 + 5 \, \mathfrak{z}2^2) - \\
& \quad \text{op} \, (268 + 24 \, \mathfrak{z}1 + 48 \, \mathfrak{z}2 + 5 \, \mathfrak{z}2^2))) - 2 \, \mathfrak{x}^6 \, (-1 + \eta)^6 \, \text{op} \\
& \quad (-108 + 20 \, \eta^4 + 60 \, \text{el} + 48 \, \text{el}^2 - 10 \, \mathfrak{z}2 + 28 \, \text{el} \, \mathfrak{z}2 - 24 \, \text{el}^2 \, \mathfrak{z}2 + 5 \, \text{el} \, \mathfrak{z}2^2 + \\
& \quad 30 \, \text{el}^2 \, \mathfrak{z}2^2 - 2 \, \eta^3 \, (5 + 10 \, \eta \mathfrak{t} + \mathfrak{z}2) + 2 \, \eta^2 \, (-74 - 3 \, \mathfrak{z}2 + \eta \mathfrak{t} \, (5 + \mathfrak{z}2)) - \\
& \quad \eta \mathfrak{t} \, (30 - 2 \, \mathfrak{z}2 + 6 \, \text{el}^2 \, (8 - 4 \, \mathfrak{z}2 + 5 \, \mathfrak{z}2^2) + \text{el} \, (60 + 28 \, \mathfrak{z}2 + 5 \, \mathfrak{z}2^2)) + \\
& \quad \eta \, (6 \times (41 + 3 \, \mathfrak{z}2) - \text{el} \, (108 + 16 \, \mathfrak{z}2 + 5 \, \mathfrak{z}2^2) + \\
& \quad \eta \mathfrak{t} \, (40 - 4 \, \mathfrak{z}2 + \text{el} \, (108 + 16 \, \mathfrak{z}2 + 5 \, \mathfrak{z}2^2)))) + \eta^2 \\
& \text{op} \, (-40 \, \eta^8 + 4 \, \eta \mathfrak{t} \, (12 - 5 \, \mathfrak{z}2) + 4 \, \eta^7 \, (-85 + 10 \, \eta \mathfrak{t} + \mathfrak{z}2) + \\
& \quad \eta^6 \, (116 - 4 \, \eta \mathfrak{t} \, (-85 + \mathfrak{z}2) + 48 \, \mathfrak{z}2) + 2 \, \eta \, (-\text{el} \, (24 + 18 \, \mathfrak{z}1 + 2 \, \mathfrak{z}2 - 5 \, \mathfrak{z}2^2) + \\
& \quad \eta \mathfrak{t} \, (99 - 40 \, \mathfrak{z}2 + \text{el} \, (24 + 18 \, \mathfrak{z}1 + 2 \, \mathfrak{z}2 - 5 \, \mathfrak{z}2^2))) + \\
& \quad \eta^2 \, (36 \times (18 + \mathfrak{z}2) - \text{el} \, (798 + 207 \, \mathfrak{z}1 + 167 \, \mathfrak{z}2 - 20 \, \mathfrak{z}2^2) - \\
& \quad 12 \, \text{el}^2 \, (8 - 4 \, \mathfrak{z}2 + 5 \, \mathfrak{z}2^2) + \eta \mathfrak{t} \, (-486 + 148 \, \mathfrak{z}2 + \text{el} \\
& \quad (798 + 207 \, \mathfrak{z}1 + 167 \, \mathfrak{z}2 - 20 \, \mathfrak{z}2^2) + 12 \, \text{el}^2 \, (8 - 4 \, \mathfrak{z}2 + 5 \, \mathfrak{z}2^2))) -
\end{aligned}$$

$$\begin{aligned}
& 2 \eta^5 \left( -6 \times (237 + \mathfrak{z}2) + \mathfrak{el} (162 - 10 \mathfrak{z}2 - 5 \mathfrak{z}2^2) + \eta \mathfrak{t} \right. \\
& \quad \left. (220 + 8 \mathfrak{z}2 + \mathfrak{el} (-162 + 10 \mathfrak{z}2 + 5 \mathfrak{z}2^2)) \right) + 6 \eta^3 (100 + 8 \mathfrak{z}2 + \\
& \quad \mathfrak{el} (-120 + 21 \mathfrak{z}1 - 21 \mathfrak{z}2 - 10 \mathfrak{z}2^2) - 6 \mathfrak{el}^2 (8 - 4 \mathfrak{z}2 + 5 \mathfrak{z}2^2) + \eta \mathfrak{t} \\
& \quad (91 + 6 \mathfrak{el}^2 (8 - 4 \mathfrak{z}2 + 5 \mathfrak{z}2^2) + \mathfrak{el} (120 - 21 \mathfrak{z}1 + 21 \mathfrak{z}2 + 10 \mathfrak{z}2^2))) + \\
& \eta^4 \left( -4 \times (957 + 37 \mathfrak{z}2) - 12 \mathfrak{el}^2 (8 - 4 \mathfrak{z}2 + 5 \mathfrak{z}2^2) + \mathfrak{el} (2370 + 117 \mathfrak{z}1 + \right. \\
& \quad \left. 157 \mathfrak{z}2 + 20 \mathfrak{z}2^2) + \eta \mathfrak{t} (-246 - 28 \mathfrak{z}2 + 12 \mathfrak{el}^2 (8 - 4 \mathfrak{z}2 + 5 \mathfrak{z}2^2) - \right. \\
& \quad \left. \mathfrak{el} (2370 + 117 \mathfrak{z}1 + 157 \mathfrak{z}2 + 20 \mathfrak{z}2^2))) \right) + 3 x^4 (-1 + \eta)^4 \\
& (4 \times (1 + 15 \eta + 15 \eta^2) \times (-1 + \eta \mathfrak{t}) \mathfrak{el}^2 \mathfrak{op} (8 - 4 \mathfrak{z}2 + 5 \mathfrak{z}2^2) - \\
& 2 (-1 + \eta)^2 \mathfrak{op} (100 \eta^4 + 10 \eta^2 (-3 + \eta \mathfrak{t} (-45 + \mathfrak{z}2) - 8 \mathfrak{z}2) - \\
& 6 \times (18 + \mathfrak{z}2) - 10 \eta^3 (-45 + 10 \eta \mathfrak{t} + \mathfrak{z}2) + \eta \mathfrak{t} (-5 + 12 \mathfrak{z}2) + \\
& 4 \eta (5 \eta \mathfrak{t} (-7 + \mathfrak{z}2) - 3 \times (125 + 7 \mathfrak{z}2))) - \\
& (-1 + \eta \mathfrak{t}) \mathfrak{el} (10 \eta^3 \mathfrak{op} (34 + 14 \mathfrak{z}2 + 5 \mathfrak{z}2^2) + \eta^2 \\
& (20 \times (-9 + 4 \mathfrak{z}2) + \mathfrak{op} (3330 + 237 \mathfrak{z}1 + 101 \mathfrak{z}2)) - \\
& 2 \times (-68 + 20 \mathfrak{z}2 + \mathfrak{op} (160 + 54 \mathfrak{z}1 + 38 \mathfrak{z}2 - 5 \mathfrak{z}2^2)) - \\
& \eta (-44 + 40 \mathfrak{z}2 + \mathfrak{op} (2358 + 129 \mathfrak{z}1 + 413 \mathfrak{z}2 + 60 \mathfrak{z}2^2)))) + x \\
& (-1 + \eta) \eta (240 \eta^8 \mathfrak{op} + 12 \eta^6 \mathfrak{op} (-103 + 2 \eta \mathfrak{t} (-70 + \mathfrak{z}2) - 21 \mathfrak{z}2) - \\
& 24 \eta^7 \mathfrak{op} (-70 + 10 \eta \mathfrak{t} + \mathfrak{z}2) + 2 \eta \mathfrak{t} \mathfrak{op} (-61 + 20 \mathfrak{z}2) + \\
& 12 \eta^5 \mathfrak{op} (-1074 + 6 \eta \mathfrak{t} (35 + \mathfrak{z}2) + \mathfrak{el} (107 - 11 \mathfrak{z}2 - 5 \mathfrak{z}2^2) + \\
& \eta \mathfrak{t} \mathfrak{el} (-107 + 11 \mathfrak{z}2 + 5 \mathfrak{z}2^2)) - \\
& \eta^2 (48 \times (-1 + \eta \mathfrak{t}) \mathfrak{el}^2 \mathfrak{op} (8 - 4 \mathfrak{z}2 + 5 \mathfrak{z}2^2) + 2 \mathfrak{op} \\
& (72 \times (18 + \mathfrak{z}2) + \eta \mathfrak{t} (-905 + 196 \mathfrak{z}2)) + (-1 + \eta \mathfrak{t}) \mathfrak{el} \\
& (4 \times (-38 + 25 \mathfrak{z}2) + \mathfrak{op} (3354 + 945 \mathfrak{z}1 + 729 \mathfrak{z}2 - 90 \mathfrak{z}2^2)))) - \\
& 2 \eta (4 \eta \mathfrak{t} \mathfrak{op} (109 - 35 \mathfrak{z}2) + (-1 + \eta \mathfrak{t}) \mathfrak{el} (-11 + 10 \mathfrak{z}2 + \\
& 3 \mathfrak{op} (24 + 18 \mathfrak{z}1 + 2 \mathfrak{z}2 - 5 \mathfrak{z}2^2))) - 6 \eta^4 (12 \times (-1 + \eta \mathfrak{t}) \mathfrak{el}^2 \mathfrak{op} \\
& (8 - 4 \mathfrak{z}2 + 5 \mathfrak{z}2^2) - 2 \mathfrak{op} (1581 + 59 \mathfrak{z}2 + \eta \mathfrak{t} (55 + 6 \mathfrak{z}2)) - (-1 + \eta \mathfrak{t}) \\
& \mathfrak{el} (2 \times (-6 + 5 \mathfrak{z}2) + \mathfrak{op} (1932 + 105 \mathfrak{z}1 + 127 \mathfrak{z}2 + 15 \mathfrak{z}2^2))) - \\
& 3 \eta^3 (60 \times (-1 + \eta \mathfrak{t}) \mathfrak{el}^2 \mathfrak{op} (8 - 4 \mathfrak{z}2 + 5 \mathfrak{z}2^2) + 4 \mathfrak{op} \\
& (348 + 24 \mathfrak{z}2 + \eta \mathfrak{t} (173 + 8 \mathfrak{z}2)) + (-1 + \eta \mathfrak{t}) \mathfrak{el} (34 - 20 \mathfrak{z}2 + \\
& \mathfrak{op} (1470 - 141 \mathfrak{z}1 + 251 \mathfrak{z}2 + 90 \mathfrak{z}2^2)))) - x^3 (-1 + \eta)^3 \\
& (24 \eta (2 + 15 \eta + 10 \eta^2) \times (-1 + \eta \mathfrak{t}) \mathfrak{el}^2 \mathfrak{op} (8 - 4 \mathfrak{z}2 + 5 \mathfrak{z}2^2) - \\
& 4 (-1 + \eta)^2 \mathfrak{op} (200 \eta^5 + 12 \eta^2 (-380 + 5 \eta \mathfrak{t} (-9 + \mathfrak{z}2) - 22 \mathfrak{z}2) + \\
& 10 \eta^3 (63 + 2 \eta \mathfrak{t} (-60 + \mathfrak{z}2) - 19 \mathfrak{z}2) - 20 \eta^4 (-60 + 10 \eta \mathfrak{t} + \mathfrak{z}2) + \\
& 15 \eta \mathfrak{t} (-7 + 2 \mathfrak{z}2) + 9 \eta (-4 \times (18 + \mathfrak{z}2) + \eta \mathfrak{t} (-7 + 8 \mathfrak{z}2))) - \\
& (-1 + \eta \mathfrak{t}) \mathfrak{el} (48 - 20 \mathfrak{z}2 - 2 \mathfrak{op} (24 + 18 \mathfrak{z}1 + 2 \mathfrak{z}2 - 5 \mathfrak{z}2^2) + \\
& 40 \eta^4 \mathfrak{op} (-9 + 13 \mathfrak{z}2 + 5 \mathfrak{z}2^2) - \\
& \eta (-1050 + 340 \mathfrak{z}2 + \mathfrak{op} (3678 + 1179 \mathfrak{z}1 + 851 \mathfrak{z}2 - 110 \mathfrak{z}2^2)) + \\
& 2 \eta^3 (36 \times (-11 + 5 \mathfrak{z}2) + \mathfrak{op} (10782 + 693 \mathfrak{z}1 + 577 \mathfrak{z}2 + 50 \mathfrak{z}2^2)) - \\
& 3 \eta^2 (102 + \mathfrak{op} (4098 + 57 \mathfrak{z}1 + 705 \mathfrak{z}2 + 140 \mathfrak{z}2^2)))) - x^2 \\
& (-1 + \eta)^2 (600 \eta^8 \mathfrak{op} + 60 \eta^6 \mathfrak{op} (-68 + \eta \mathfrak{t} (-55 + \mathfrak{z}2) - 9 \mathfrak{z}2) - \\
& 60 \eta^7 \mathfrak{op} (-55 + 10 \eta \mathfrak{t} + \mathfrak{z}2) + 2 \eta \mathfrak{t} \mathfrak{op} (-31 + 10 \mathfrak{z}2) - \\
& \eta^2 (72 \times (-1 + \eta \mathfrak{t}) \mathfrak{el}^2 \mathfrak{op} (8 - 4 \mathfrak{z}2 + 5 \mathfrak{z}2^2) + \\
& 2 \mathfrak{op} (108 \times (18 + \mathfrak{z}2) + \eta \mathfrak{t} (-977 + 134 \mathfrak{z}2)) + (-1 + \eta \mathfrak{t}) \mathfrak{el} \\
& (-782 + 320 \mathfrak{z}2 + 3 \mathfrak{op} (1758 + 531 \mathfrak{z}1 + 395 \mathfrak{z}2 - 50 \mathfrak{z}2^2)))) -
\end{aligned}$$

$$\begin{aligned}
& 2 \eta \left( \eta t \, \text{ep} \left( 559 - 160 \, \mathfrak{x}^2 \right) + (-1 + \eta t) \, \text{el} \left( -41 + 20 \, \mathfrak{x}^2 + \right. \right. \\
& \quad \left. \left. 3 \, \text{ep} \left( 24 + 18 \, \mathfrak{x}^1 + 2 \, \mathfrak{x}^2 - 5 \, \mathfrak{x}^2{}^2 \right) \right) \right) + \\
& 6 \eta^5 \, \text{ep} \left( 26 \times (-145 + \mathfrak{x}^2) - 5 \, \text{el} \left( -56 + 12 \, \mathfrak{x}^2 + 5 \, \mathfrak{x}^2{}^2 \right) + \right. \\
& \quad \left. 5 \, \eta t \left( 4 \times (48 + \mathfrak{x}^2) + \text{el} \left( -56 + 12 \, \mathfrak{x}^2 + 5 \, \mathfrak{x}^2{}^2 \right) \right) \right) - \\
& 6 \eta^4 \left( 30 \times (-1 + \eta t) \, \text{el}^2 \, \text{ep} \left( 8 - 4 \, \mathfrak{x}^2 + 5 \, \mathfrak{x}^2{}^2 \right) - 2 \, \text{ep} \right. \\
& \quad \left( 3116 + 111 \, \mathfrak{x}^2 + \eta t \left( 26 + \mathfrak{x}^2 \right) \right) - (-1 + \eta t) \, \text{el} \\
& \quad \left( -74 + 40 \, \mathfrak{x}^2 + \text{ep} \left( 3752 + 222 \, \mathfrak{x}^1 + 234 \, \mathfrak{x}^2 + 25 \, \mathfrak{x}^2{}^2 \right) \right) \right) - \\
& 3 \eta^3 \left( 2 \, \text{ep} \left( 1784 + 491 \, \eta t + 112 \, \mathfrak{x}^2 + 44 \, \eta t \, \mathfrak{x}^2 \right) + 120 \times \right. \\
& \quad \left( -1 + \eta t \right) \, \text{el}^2 \, \text{ep} \left( 8 - 4 \, \mathfrak{x}^2 + 5 \, \mathfrak{x}^2{}^2 \right) + (-1 + \eta t) \, \text{el} \\
& \quad \left( 140 - 40 \, \mathfrak{x}^2 + \text{ep} \left( 3506 - 123 \, \mathfrak{x}^1 + 597 \, \mathfrak{x}^2 + 160 \, \mathfrak{x}^2{}^2 \right) \right) \right) \right) - \\
& 2 \, \text{co}^2 \left( \times (-1 + \eta) - \eta \right) \left( w \left( -1 + \eta \right) + \times (-1 + \eta) - \eta \right) \\
& (-1 + \\
& \eta) \times (2 \\
& \mathfrak{x}^6 \\
& (-1 + \eta)^6 \\
& \text{ep} \\
& (-2 + 2 \, \text{el} + 9 \, \mu^1 + 15 \, w \, \mu^1 + \\
& \quad 4 \, w^2 \, \mu^1 - 13 \, \text{el} \, \mu^1 - 27 \, w \, \text{el} \, \mu^1 - \\
& \quad 12 \, w^2 \, \text{el} \, \mu^1 + 5 \, \mu^1{}^2 + 9 \, w \, \mu^1{}^2 + \\
& \quad 4 \, w^2 \, \mu^1{}^2 - 9 \, \text{el} \, \mu^1{}^2 - 21 \, w \, \text{el} \, \mu^1{}^2 - \\
& \quad 12 \, w^2 \, \text{el} \, \mu^1{}^2 + w^2 \, \eta^5 \left( 1 + \mu^1 \right) - \\
& \quad w \, \eta^4 \left( 3 + w \left( 4 + \eta t - 4 \, \mu^1 \right) \right) \times \left( 1 + \mu^1 \right) - \\
& \quad \eta t \left( 2 + 10 \, \text{el} + 2 \, \mu^1 - 9 \, \text{el} \, \mu^1 + 5 \, \text{el} \, \mu^1{}^2 + 3 \, w \left( 1 + \mu^1 \right) + w^2 \right. \\
& \quad \left. \left( 1 + 2 \, \text{el} \left( -2 + \mu^1 \right)^2 + \mu^1 \right) + w \, \text{el} \left( 16 - 19 \, \mu^1 + 7 \, \mu^1{}^2 \right) \right) + \\
& \quad \eta^3 \left( 2 \times \left( 1 + \mu^1 \right) + 3 \, w \left( 3 + \eta t - 2 \, \mu^1 + \eta t \, \mu^1 - 3 \, \mu^1{}^2 \right) + 2 \, w^2 \right. \\
& \quad \left. \left( 3 - 5 \, \mu^1 - 8 \, \mu^1{}^2 + 2 \, \eta t \left( 1 + \mu^1 \right) + \text{el} \left( 4 + 2 \, \mu^1 + 7 \, \mu^1{}^2 \right) \right) \right) + \\
& \quad \eta \left( 6 + 6 \, \text{el} - 16 \, \mu^1 + 7 \, \text{el} \, \mu^1 - 10 \, \mu^1{}^2 + 13 \, \text{el} \, \mu^1{}^2 + 4 \, \eta t \left( 1 + \mu^1 \right) + \eta t \right. \\
& \quad \left. \text{el} \left( 2 - 3 \, \mu^1 + \mu^1{}^2 \right) + w \left( 3 - 42 \, \mu^1 - 27 \, \mu^1{}^2 + 9 \, \eta t \left( 1 + \mu^1 \right) + \right. \right. \\
& \quad \left. \left. 8 \, \eta t \, \text{el} \left( 2 - 3 \, \mu^1 + \mu^1{}^2 \right) + 8 \, \text{el} \left( 2 + 5 \, \mu^1 + 6 \, \mu^1{}^2 \right) \right) + w^2 \left( 1 - 15 \, \mu^1 - \right. \right. \\
& \quad \left. \left. 16 \, \mu^1{}^2 + 4 \, \eta t \left( 1 + \text{el} \left( -2 + \mu^1 \right)^2 + \mu^1 \right) + \text{el} \left( 8 + 28 \, \mu^1 + 38 \, \mu^1{}^2 \right) \right) \right) - \\
& \quad \eta^2 \left( 6 - 5 \, \mu^1 - 5 \, \mu^1{}^2 + 2 \, \eta t \left( 1 + \mu^1 \right) + 2 \, w^2 \left( 2 + \eta t \, \text{el} \left( -2 + \mu^1 \right)^2 - 10 \, \mu^1 - \right. \right. \\
& \quad \left. \left. 12 \, \mu^1{}^2 + 3 \, \eta t \left( 1 + \mu^1 \right) + 2 \, \text{el} \left( 4 + 5 \, \mu^1 + 10 \, \mu^1{}^2 \right) \right) + w \left( 9 + 16 \, \text{el} - 36 \, \mu^1 + \right. \right. \\
& \quad \left. \left. 13 \, \text{el} \, \mu^1 - 27 \, \mu^1{}^2 + 27 \, \text{el} \, \mu^1{}^2 + \eta t \left( 9 + 9 \, \mu^1 - 5 \, \text{el} \, \mu^1 + \text{el} \, \mu^1{}^2 \right) \right) \right) + \\
& \text{ep} \left( w^4 \left( -1 + \eta \right)^4 \left( 2 \, \eta^7 \left( 1 + \mu^1 \right) - 2 \, \eta \, \eta t \left( 5 + 10 \, \mu^1 - \mu^1{}^2 + 2 \, \text{el} \left( 5 - 2 \, \mu^1 + 11 \, \mu^1{}^2 \right) \right) - \right. \right. \\
& \quad 2 \, \eta^6 \left( \eta t \left( 1 + \mu^1 \right) - 2 \, \mu^1 \left( 2 + 2 \, \mu^1 - 3 \, \mu^2 \right) \right) + 5 \, \eta t \left( 1 + \mu^1 \right) \, \mu^2 + 2 \, \eta^5 \\
& \quad \left( 3 - \mu^1{}^2 + 2 \, \text{el} \left( 4 + 2 \, \mu^1 + 7 \, \mu^1{}^2 \right) + 11 \, \mu^2 + \mu^1 \left( 2 - \mu^2 + 6 \, \eta t \, \mu^2 \right) \right) + 2 \, \eta^3 \\
& \quad \left( -4 - 3 \, \mu^1 + \mu^1{}^2 - 11 \, \mu^2 - 23 \, \mu^1 \, \mu^2 + \text{el} \left( 28 - 4 \, \mu^1 - 14 \, \mu^1{}^2 + 72 \, \mu^1 \, \mu^2 \right) + \right. \\
& \quad \left. \eta t \left( 5 + 10 \, \mu^1 - 25 \, \mu^1{}^2 - 6 \, \mu^1 \, \mu^2 + \text{el} \left( -26 - 4 \, \mu^1 + 22 \, \mu^1{}^2 - 72 \, \mu^1 \, \mu^2 \right) \right) \right) + \\
& \quad 2 \, \eta^2 \left( 5 + 8 \, \mu^1 + 3 \, \mu^1{}^2 - 2 \, \text{el} \left( -5 + 7 \, \mu^1{}^2 + \mu^1 \left( 2 - 18 \, \mu^2 \right) \right) + \right. \\
& \quad \left. 11 \, \mu^2 + 5 \, \mu^1 \, \mu^2 + \eta t \left( 4 + 11 \, \mu^1{}^2 - 5 \, \mu^2 + \mu^1 \left( 9 + \mu^2 \right) - \right. \right. \\
& \quad \left. \left. 2 \, \text{el} \left( 14 + 11 \, \mu^1{}^2 + 2 \, \mu^1 \left( -1 + 9 \, \mu^2 \right) \right) \right) \right) + \eta^4 \\
& \quad \left( 2 \times \left( -5 - 12 \, \mu^1 - 7 \, \mu^1{}^2 - 11 \, \mu^2 + 25 \, \mu^1 \, \mu^2 + 2 \, \text{el} \left( 13 + 2 \, \mu^1 + \right. \right. \right. \\
& \quad \left. \left. 7 \, \mu^1{}^2 + 18 \, \mu^1 \, \mu^2 \right) \right) + \eta t \left( -6 - 16 \, \mu^1 + 26 \, \mu^1{}^2 + \right.
\end{aligned}$$

$$\begin{aligned}
& 5 \mu_2 - 7 \mu_1 \mu_2 + 4 \theta l \left( -4 + 11 \mu_1^2 - 2 \mu_1 (1 + 9 \mu_2) \right) \Big) \Big) - \\
& w^3 (-1 + \eta)^3 \left( 4 \eta^8 (1 + \mu_1) + \eta^7 (6 + 16 \mu_1^2 - 4 \eta t (1 + \mu_1) + \right. \\
& \quad \left. \mu_1 (22 - 24 \mu_2) \right) + 15 \eta t (1 + \mu_1) \mu_2 - \eta \eta t \\
& \quad \left( -8 \mu_1^2 + 12 \theta l (5 - 2 \mu_1 + 11 \mu_1^2) + \mu_1 (68 - 19 \mu_2) + 5 \times (8 + \mu_2) \right) + 2 \\
& \quad \eta^6 (6 + 19 \mu_1 + 7 \mu_1^2 + 4 \theta l (4 + 2 \mu_1 + 7 \mu_1^2) + \\
& \quad 22 \mu_2 - 20 \mu_1 \mu_2 + 3 \eta t (-1 + \mu_1 (-1 + 4 \mu_2)) \Big) + \eta^4 \\
& \quad \left( -4 \times (14 + 6 \mu_1^2 + \mu_1 (26 - 27 \mu_2) + 30 \mu_2) + \right. \\
& \quad \theta l (196 + 4 \mu_1^2 + 5 \mathfrak{E}1 + \mu_1 (-16 + 11 \mathfrak{E}1 + 5 \mu_2 (64 + \mathfrak{E}1 - \mathfrak{E}2) - 11 \mathfrak{E}2) + \\
& \quad \mu_2 (8 + 5 \mathfrak{E}1 - 5 \mathfrak{E}2) - 5 \mathfrak{E}2) + \eta t (-8 - 16 \mu_1 + 28 \mu_1^2 + 19 \mu_2 - \\
& \quad 53 \mu_1 \mu_2 + \theta l (-116 + 172 \mu_1^2 - 5 \mathfrak{E}1 - \mu_1 (16 + 11 \mathfrak{E}1 + 5 \mu_2 \\
& \quad (64 + \mathfrak{E}1 - \mathfrak{E}2) - 11 \mathfrak{E}2) + 5 \mathfrak{E}2 + \mu_2 (-8 - 5 \mathfrak{E}1 + 5 \mathfrak{E}2)) \Big) \Big) + \\
& \quad \eta^3 (2 \times (-7 + 10 \mu_1^2 + \mu_1 (3 - 58 \mu_2) - 4 \mu_2) + \eta t (2 \times (-54 \mu_1^2 + \\
& \quad \mu_1 (64 - 29 \mu_2) + 7 \times (4 + \mu_2)) + \\
& \quad \theta l (-196 + 80 \mu_1^2 + 5 \mathfrak{E}1 + \mu_1 \mu_2 (-484 + 5 \mathfrak{E}1 - 5 \mathfrak{E}2) + \\
& \quad \mu_2 (-4 + 5 \mathfrak{E}1 - 5 \mathfrak{E}2) + 11 \mu_1 (-4 + \mathfrak{E}1 - \mathfrak{E}2) - 5 \mathfrak{E}2) \Big) + \\
& \quad \theta l (172 - 104 \mu_1^2 - 5 \mathfrak{E}1 + 5 \mathfrak{E}2 + \mu_2 (4 - 5 \mathfrak{E}1 + 5 \mathfrak{E}2) + \\
& \quad \mu_1 (-4 - 11 \mathfrak{E}1 + 11 \mathfrak{E}2 + \mu_2 (484 - 5 \mathfrak{E}1 + 5 \mathfrak{E}2)) \Big) \Big) + \eta^5 \\
& \quad (4 \times (2 - 9 \mu_1^2 + 6 \mu_2 + \mu_1 (-7 + 15 \mu_2)) + \theta l (116 + 112 \mu_1^2 + \\
& \quad 5 \mathfrak{E}1 + \mu_1 (12 + 11 \mathfrak{E}1 + \mu_2 (52 + 5 \mathfrak{E}1 - 5 \mathfrak{E}2) - 11 \mathfrak{E}2) + \\
& \quad \mu_2 (4 + 5 \mathfrak{E}1 - 5 \mathfrak{E}2) - 5 \mathfrak{E}2) + \eta t (-12 - 40 \mu_1 + 20 \mu_1^2 - 9 \mu_2 + \\
& \quad 39 \mu_1 \mu_2 + \theta l (-32 + 44 \mu_1^2 - 5 \mathfrak{E}1 + 5 \mathfrak{E}2 + \mu_2 (-4 - 5 \mathfrak{E}1 + 5 \mathfrak{E}2) + \\
& \quad \mu_1 (12 - 11 \mathfrak{E}1 + 11 \mathfrak{E}2 + \mu_2 (-52 - 5 \mathfrak{E}1 + 5 \mathfrak{E}2)) \Big) \Big) \Big) + \\
& \quad \eta^2 (40 + 10 \mu_1^2 - 52 \theta l \mu_1^2 + 60 \mu_2 + 2 \mu_1 (31 + 6 \mu_2) + 5 \theta l \\
& \quad (12 - (1 + \mu_2) \mathfrak{E}1 + \mathfrak{E}2 + \mu_2 \mathfrak{E}2) + \\
& \quad \theta l \mu_1 (8 - 11 \mathfrak{E}1 + 11 \mathfrak{E}2 + \mu_2 (216 - 5 \mathfrak{E}1 + 5 \mathfrak{E}2)) + \\
& \quad \eta t (2 \times (7 + 26 \mu_1^2 - 17 \mu_2 + \mu_1 (3 + 7 \mu_2)) - \\
& \quad \theta l (172 + 180 \mu_1^2 - 5 \times (1 + \mu_2) \mathfrak{E}1 + 5 \mathfrak{E}2 + 5 \mu_2 \mathfrak{E}2 + \\
& \quad \mu_1 (-8 - 11 \mathfrak{E}1 + 11 \mathfrak{E}2 + \mu_2 (216 - 5 \mathfrak{E}1 + 5 \mathfrak{E}2)) \Big) \Big) \Big) + \\
& w^2 (-1 + \eta)^2 (2 \eta^9 (1 + \mu_1) + 15 \eta t (1 + \mu_1) \mu_2 + 2 \eta^7 (5 + 34 \mu_1 + 17 \mu_1^2 + \\
& \quad 2 \theta l (4 + 2 \mu_1 + 7 \mu_1^2) + 6 \eta t (-1 + \mu_1 (-1 + \mu_2)) + 11 \mu_2 - 37 \mu_1 \mu_2) - 2 \\
& \quad \eta^8 (-6 + \eta t - 10 \mu_1 + \eta t \mu_1 - 4 \mu_1^2 + 6 \mu_1 \mu_2) - 3 \eta \eta t \\
& \quad (-4 \mu_1^2 + 4 \theta l (5 - 2 \mu_1 + 11 \mu_1^2) + \mu_1 (28 - 19 \mu_2) + 5 \times (4 + \mu_2)) - \eta^5 \\
& \quad (26 + 68 \mu_1^2 + 2 \mu_1 (71 - 90 \mu_2) + 72 \mu_2 - \\
& \quad \theta l (\mu_1 (-20 + 35 \mathfrak{E}1 + \mu_2 (176 + 15 \mathfrak{E}1 - 15 \mathfrak{E}2) - 31 \mathfrak{E}2) + \mu_2 \\
& \quad (8 + 15 \mathfrak{E}1 - 15 \mathfrak{E}2) + 3 \times (72 + 5 \mathfrak{E}1 - 5 \mathfrak{E}2) + 2 \mu_1^2 (62 + \mathfrak{E}1 + \mathfrak{E}2)) \Big) + \\
& \quad \eta t (36 + 88 \mu_1 - 44 \mu_1^2 + 19 \mu_2 - 29 \mu_1 \mu_2 + \theta l (92 + 15 \mathfrak{E}1 + \\
& \quad \mu_1 (-28 + 35 \mathfrak{E}1 + \mu_2 (176 + 15 \mathfrak{E}1 - 15 \mathfrak{E}2) - 31 \mathfrak{E}2) + \\
& \quad \mu_2 (8 + 15 \mathfrak{E}1 - 15 \mathfrak{E}2) - 15 \mathfrak{E}2 + 2 \mu_1^2 (-60 + \mathfrak{E}1 + \mathfrak{E}2)) \Big) \Big) + \eta^3 \\
& \quad (14 + 72 \mu_1 + 34 \mu_1^2 + 66 \mu_2 - 90 \mu_1 \mu_2 + \eta t (108 + 200 \mu_1 - 40 \mu_1^2 + \\
& \quad 34 \mu_2 - 98 \mu_1 \mu_2 + \theta l (\mu_1 (-76 + 35 \mathfrak{E}1 + \mu_2 (-568 + 15 \mathfrak{E}1 - 15 \mathfrak{E}2) - \\
& \quad 31 \mathfrak{E}2) + \mu_2 (-16 + 15 \mathfrak{E}1 - 15 \mathfrak{E}2) + 5 \times (-56 + 3 \mathfrak{E}1 - 3 \mathfrak{E}2) + \\
& \quad 2 \mu_1^2 (-6 + \mathfrak{E}1 + \mathfrak{E}2)) \Big) + \theta l (-2 \mu_1^2 (64 + \mathfrak{E}1 + \mathfrak{E}2) + \\
& \quad 5 \times (40 - 3 \mathfrak{E}1 + 3 \mathfrak{E}2) + \mu_2 (16 - 15 \mathfrak{E}1 + 15 \mathfrak{E}2) +
\end{aligned}$$

$$\begin{aligned}
& \mu_1 (36 - 35 \mathfrak{e}_1 + 31 \mathfrak{e}_2 + \mu_2 (568 - 15 \mathfrak{e}_1 + 15 \mathfrak{e}_2)) \Big) + \eta^4 \\
& \Big( 8 \times (-10 + \mu_1^2 - 19 \mu_2 - 4 \mu_1 (3 + \mu_2)) + \mathfrak{e}_1 (-4 \mu_1^2 (22 + \mathfrak{e}_1) + \\
& 3 \times (84 + 5 \times (1 + \mu_2) \mathfrak{e}_1 - 5 \times (1 + \mu_2) \mathfrak{e}_2) + \\
& \mu_1 (-76 + 17 \mathfrak{e}_1 + 15 \mu_2 \mathfrak{e}_1 - 21 \mathfrak{e}_2 + 9 \mu_2 (64 + \mathfrak{e}_2)) \Big) + \\
& \eta \mathfrak{t} (6 + 58 \mu_1 - 56 \mu_1^2 + 27 \mu_2 - 93 \mu_1 \mu_2 + \mathfrak{e}_1 (-196 - \\
& 15 \times (1 + \mu_2) \mathfrak{e}_1 + 4 \mu_1^2 (60 + \mathfrak{e}_1) + 15 \mathfrak{e}_2 + 15 \mu_2 \mathfrak{e}_2 - \\
& \mu_1 (4 + 17 \mathfrak{e}_1 + 15 \mu_2 \mathfrak{e}_1 - 21 \mathfrak{e}_2 + 9 \mu_2 (64 + \mathfrak{e}_2)) \Big) \Big) + \\
& \eta^2 (46 + 58 \mu_1 + 50 \mu_2 + 14 \mu_1 \mu_2 + \mathfrak{e}_1 (74 - 15 \mathfrak{e}_1 + \mu_1^2 (-28 + \\
& \mathfrak{e}_1 - \mathfrak{e}_2) + 15 \mathfrak{e}_2 + \mu_2 (14 - 15 \mathfrak{e}_1 + 15 \mathfrak{e}_2) + \\
& \mu_1 (58 - 26 \mathfrak{e}_1 + 26 \mathfrak{e}_2 + \mu_2 (182 - 15 \mathfrak{e}_1 + 3 \mathfrak{e}_2)) \Big) - \\
& \eta \mathfrak{t} (4 + 56 \mu_1 - 32 \mu_1^2 + 38 \mu_2 - 22 \mu_1 \mu_2 + \mathfrak{e}_1 (\mu_1^2 (264 + \mathfrak{e}_1 - \mathfrak{e}_2) + \\
& 15 \times (14 - \mathfrak{e}_1 + \mathfrak{e}_2) + \mu_2 (14 - 15 \mathfrak{e}_1 + 15 \mathfrak{e}_2) + \\
& \mu_1 (18 - 26 \mathfrak{e}_1 + 26 \mathfrak{e}_2 + \mu_2 (182 - 15 \mathfrak{e}_1 + 3 \mathfrak{e}_2)) \Big) \Big) + \\
& \eta^6 (22 + 8 \times (-2 + \eta \mathfrak{t}) \mu_1^2 + 86 \mu_2 - 4 \eta \mathfrak{t} \mu_2 + 2 \mu_1 (9 + 7 \mu_2 + \\
& 4 \eta \mathfrak{t} (-2 + 7 \mu_2)) + \mathfrak{e}_1 (2 \times (53 + 5 \mu_2) + \mu_1^2 (140 + 3 \mathfrak{e}_1 + \mathfrak{e}_2) + \\
& \mu_1 (42 + 9 \mathfrak{e}_1 - 5 \mathfrak{e}_2 - 2 \mu_2 (7 + 6 \mathfrak{e}_2)) - \eta \mathfrak{t} (26 + 10 \mu_2 + \\
& \mu_1^2 (3 \mathfrak{e}_1 + \mathfrak{e}_2) + \mu_1 (2 + 9 \mathfrak{e}_1 - 5 \mathfrak{e}_2 - 2 \mu_2 (7 + 6 \mathfrak{e}_2)) \Big) \Big) \Big) + \\
& \eta (4 \eta^8 (1 + \mu_1) - 2 \eta^7 (2 - 5 \mu_1^2 + 2 \eta \mathfrak{t} (1 + \mu_1) + 3 \mu_1 (-3 + 4 \mu_2)) + \\
& \eta \mathfrak{t} (2 \mu_1^2 - 5 \times (2 + \mu_2) + \mu_1 (-8 + 19 \mu_2)) - \eta \\
& (2 \eta \mathfrak{t} (5 + 8 \mu_1 + 3 \mu_1^2) + 5 \mathfrak{e}_1 (1 + \mu_2) \times (-2 + \mathfrak{e}_1 - \mathfrak{e}_2) + \mathfrak{e}_1 \mu_1^2 \\
& (2 - \mathfrak{e}_1 + \mathfrak{e}_2) + \mathfrak{e}_1 \mu_1 (5 \mu_2 \mathfrak{e}_1 + 4 \times (-2 + \mathfrak{e}_1 - \mathfrak{e}_2) + 7 \mu_2 (2 + \mathfrak{e}_2)) + \\
& \eta \mathfrak{t} \mathfrak{e}_1 (\mu_1^2 (42 + \mathfrak{e}_1 - \mathfrak{e}_2) - \mu_1 (5 \mu_2 \mathfrak{e}_1 + 4 (\mathfrak{e}_1 - \mathfrak{e}_2) + 7 \mu_2 (2 + \mathfrak{e}_2)) + \\
& 5 \times (6 - \mathfrak{e}_1 + \mathfrak{e}_2 + \mu_2 (2 - \mathfrak{e}_1 + \mathfrak{e}_2)) \Big) \Big) + \eta^6 \\
& (2 - 2 \mu_1^2 + 22 \mu_2 + 10 \mu_1 \mu_2 + 4 \eta \mathfrak{t} \mu_1 (1 + \mu_1 + 3 \mu_2) + \\
& \mathfrak{e}_1 (2 \times (6 + \mu_2) + \mu_1^2 (28 + \mathfrak{e}_1 + \mathfrak{e}_2) + \mu_1 (16 - 10 \mu_2 + \mathfrak{e}_1 + \mathfrak{e}_2) - \\
& \eta \mathfrak{t} (2 \times (-2 + \mu_2) + \mu_1^2 (\mathfrak{e}_1 + \mathfrak{e}_2) + \mu_1 (8 - 10 \mu_2 + \mathfrak{e}_1 + \mathfrak{e}_2)) \Big) \Big) + \\
& \eta^5 (18 - 28 \mu_1 - 22 \mu_1^2 - 6 \mu_2 + 54 \mu_1 \mu_2 + \mathfrak{e}_1 (38 + 6 \mu_2 + \\
& \mu_1^2 (34 + 3 \mathfrak{e}_1 + \mathfrak{e}_2) + \mu_1 (6 \mu_2 + 9 \mathfrak{e}_1 - 5 \mathfrak{e}_2 - 12 \mu_2 \mathfrak{e}_2)) - \\
& \eta \mathfrak{t} (4 \times (-2 - 2 \mu_1 (-2 + \mu_2) + \mu_2) + \mathfrak{e}_1 (22 + 6 \mu_2 + \mu_1^2 \\
& (6 + 3 \mathfrak{e}_1 + \mathfrak{e}_2) + \mu_1 (-8 + 6 \mu_2 + 9 \mathfrak{e}_1 - 5 \mathfrak{e}_2 - 12 \mu_2 \mathfrak{e}_2)) \Big) \Big) + \\
& \eta^2 (20 - 4 \mu_1^2 + 8 \mu_2 + 4 \mu_1 (4 + 8 \mu_2) - \mathfrak{e}_1 \mu_1^2 (4 + \mathfrak{e}_1 + \mathfrak{e}_2) + \\
& 5 \mathfrak{e}_1 (4 - \mathfrak{e}_1 + \mathfrak{e}_2 + \mu_2 (2 - \mathfrak{e}_1 + \mathfrak{e}_2)) + \\
& \mathfrak{e}_1 \mu_1 (28 - 12 \mathfrak{e}_1 + 10 \mathfrak{e}_2 + \mu_2 (22 - 5 \mathfrak{e}_1 + 5 \mathfrak{e}_2)) + \\
& \eta \mathfrak{t} (30 + 4 \mu_1 + 22 \mu_1^2 + 6 \mu_2 - 18 \mu_1 \mu_2 + \\
& \mathfrak{e}_1 (5 \times (-8 + \mathfrak{e}_1 + \mu_2 (-2 + \mathfrak{e}_1 - \mathfrak{e}_2) - \mathfrak{e}_2) + \mu_1^2 (-40 + \mathfrak{e}_1 + \mathfrak{e}_2) + \\
& \mu_1 (12 \mathfrak{e}_1 + \mu_2 (-22 + 5 \mathfrak{e}_1 - 5 \mathfrak{e}_2) - 10 \times (2 + \mathfrak{e}_2)) \Big) \Big) + \\
& \eta^4 (-26 - 20 \mu_1 + 6 \mu_1^2 - 46 \mu_2 - 10 \mu_1 \mu_2 + \mathfrak{e}_1 (-16 \mu_1^2 + \\
& \mu_1 (-36 + 11 \mathfrak{e}_1 + \mu_2 (92 + 5 \mathfrak{e}_1 - 5 \mathfrak{e}_2) - 11 \mathfrak{e}_2) + \\
& \mu_2 (-4 + 5 \mathfrak{e}_1 - 5 \mathfrak{e}_2) + 5 \times (8 + \mathfrak{e}_1 - \mathfrak{e}_2)) + \eta \mathfrak{t} (-20 - 16 \mu_1 + 4 \mu_1^2 - \\
& \mu_2 - 13 \mu_1 \mu_2 + \mathfrak{e}_1 (-36 + 32 \mu_1^2 - 5 \mathfrak{e}_1 + 5 \mathfrak{e}_2 + \mu_2 (4 - 5 \mathfrak{e}_1 + 5 \mathfrak{e}_2) + \\
& \mu_1 (20 - 11 \mathfrak{e}_1 + 11 \mathfrak{e}_2 + \mu_2 (-92 - 5 \mathfrak{e}_1 + 5 \mathfrak{e}_2)) \Big) \Big) + \\
& \eta^3 (2 \times (-7 + 6 \mu_1^2 + \mu_1 (5 - 31 \mu_2) + 11 \mu_2) + \mathfrak{e}_1 (24 + 5 \mathfrak{e}_1 - \\
& 4 \mu_1^2 (6 + \mathfrak{e}_1) + \mu_2 (-8 + 5 \mathfrak{e}_1 - 5 \mathfrak{e}_2) - 5 \mathfrak{e}_2 +
\end{aligned}$$

$$\begin{aligned}
& \mu_1 (-5 \mathfrak{e}_1 + \mathfrak{e}_2 + \mu_2 (112 + 5 \mathfrak{e}_1 + 19 \mathfrak{e}_2)) + \eta t (6 + 52 \mu_1 - 26 \mu_1^2 + \\
& 4 \mu_2 - 8 \mu_1 \mu_2 + \theta l (4 \mu_1^2 (10 + \mathfrak{e}_1) - 5 \times (4 + \mathfrak{e}_1 - \mathfrak{e}_2) + \mu_2 (8 - 5 \mathfrak{e}_1 + \\
& 5 \mathfrak{e}_2) - \mu_1 (16 - 5 \mathfrak{e}_1 + \mathfrak{e}_2 + \mu_2 (112 + 5 \mathfrak{e}_1 + 19 \mathfrak{e}_2))) - \\
w (-1 + \eta) \times & (6 \eta^9 (1 + \mu_1) + \eta^8 (8 + 18 \mu_1^2 - 6 \eta t (1 + \mu_1) + \mu_1 \\
& (38 - 36 \mu_2)) + 5 \eta t (1 + \mu_1) \mu_2 - \eta \eta t \\
& (40 + 44 \mu_1 - 8 \mu_1^2 + 4 \theta l (5 - 2 \mu_1 + 11 \mu_1^2) + 15 \mu_2 - 57 \mu_1 \mu_2) - \eta^5 \\
& (2 \times (19 + 14 \mu_1^2 + \mu_1 (57 - 54 \mu_2) + 60 \mu_2) - \theta l (148 + 15 \times (1 + \mu_2) \mathfrak{e}_1 + \\
& \mu_1 (-68 + 35 \mathfrak{e}_1 + 3 \mu_2 (72 + 5 \mathfrak{e}_1 - 5 \mathfrak{e}_2) - 31 \mathfrak{e}_2) - 15 \mathfrak{e}_2 - 15 \mu_2 \mathfrak{e}_2 + \\
& 2 \mu_1^2 (12 + \mathfrak{e}_1 + \mathfrak{e}_2)) + \eta t (44 + 64 \mu_1 - 28 \mu_1^2 + 11 \mu_2 + 11 \mu_1 \mu_2 + \\
& \theta l (88 + 15 \times (1 + \mu_2) \mathfrak{e}_1 + \mu_1 (-44 + 35 \mathfrak{e}_1 + 3 \mu_2 (72 + 5 \mathfrak{e}_1 - 5 \mathfrak{e}_2) - \\
& 31 \mathfrak{e}_2) - 15 \mathfrak{e}_2 - 15 \mu_2 \mathfrak{e}_2 + 2 \mu_1^2 (-54 + \mathfrak{e}_1 + \mathfrak{e}_2))) + \\
\eta^7 & (40 \mu_1 + 16 \mu_1^2 + 44 \mu_2 - 40 \mu_1 \mu_2 + \theta l (2 \times (16 + \mu_2) + \mu_1^2 \\
& (56 + \mathfrak{e}_1 + \mathfrak{e}_2) + \mu_1 (28 - 10 \mu_2 + \mathfrak{e}_1 + \mathfrak{e}_2)) - \eta t (8 + 2 \theta l \mu_2 + \mu_1^2 \\
& (-4 + \theta l (\mathfrak{e}_1 + \mathfrak{e}_2)) + \mu_1 (4 - 24 \mu_2 + \theta l (12 - 10 \mu_2 + \mathfrak{e}_1 + \mathfrak{e}_2))) + \\
\eta^3 & (4 \times (8 + 3 \mu_1^2 + 15 \mu_2 + \mu_1 (17 + 3 \mu_2)) + \theta l (-\mu_1^2 (56 + 3 \mathfrak{e}_1 + 3 \mathfrak{e}_2) + \\
& 3 \times (36 - 5 \mathfrak{e}_1 + 5 \mathfrak{e}_2) + \mu_2 (22 - 15 \mathfrak{e}_1 + 15 \mathfrak{e}_2) + \\
& \mu_1 (64 - 36 \mathfrak{e}_1 - 5 \mu_2 (-50 + 3 \mathfrak{e}_1 - 3 \mathfrak{e}_2) + 30 \mathfrak{e}_2)) + \\
\eta t & (92 + 96 \mu_1 + 40 \mu_1^2 + 26 \mu_2 - 70 \mu_1 \mu_2 + \theta l (\mu_1 (-64 + 36 \mathfrak{e}_1 + \\
& 5 \mu_2 (-50 + 3 \mathfrak{e}_1 - 3 \mathfrak{e}_2) - 30 \mathfrak{e}_2) + \mu_2 (-22 + 15 \mathfrak{e}_1 - 15 \mathfrak{e}_2) + \\
& 15 \times (-12 + \mathfrak{e}_1 - \mathfrak{e}_2) + \mu_1^2 (-88 + 3 \mathfrak{e}_1 + 3 \mathfrak{e}_2))) - \eta^2 \\
& (4 \times (1 + \mu_1) \times (-5 + \mu_1 - 3 \mu_2) + \eta t (20 + 4 \mu_1^2 - 10 \mu_1 (-6 + \mu_2) + \\
& 14 \mu_2 - 3 \theta l (\mu_2 (-8 + 5 \mathfrak{e}_1 - 5 \mathfrak{e}_2) + 5 \times (-8 + \mathfrak{e}_1 - \mathfrak{e}_2)) + \\
& 2 \theta l \mu_1^2 (85 + \mathfrak{e}_1 - \mathfrak{e}_2) + \theta l \mu_1 \\
& (14 - 19 \mathfrak{e}_1 + 19 \mathfrak{e}_2 - 3 \mu_2 (-8 + 5 \mathfrak{e}_1 + 3 \mathfrak{e}_2))) + \theta l \\
& (3 \mu_2 (-8 + 5 \mathfrak{e}_1 - 5 \mathfrak{e}_2) + 5 \times (-8 + 3 \mathfrak{e}_1 - 3 \mathfrak{e}_2) + \mu_1^2 (6 - 2 \mathfrak{e}_1 + 2 \mathfrak{e}_2) + \\
& \mu_1 (-46 + 19 \mathfrak{e}_1 - 19 \mathfrak{e}_2 + 3 \mu_2 (-8 + 5 \mathfrak{e}_1 + 3 \mathfrak{e}_2))) - 2 \\
\eta^6 & (2 \times (-6 + 11 \mu_1^2 + \mu_1 (11 - 24 \mu_2) - 9 \mu_2) - \theta l (54 + 8 \mu_2 + \\
& \mu_1^2 (59 + 3 \mathfrak{e}_1 + \mathfrak{e}_2) + \mu_1 (11 + 9 \mathfrak{e}_1 - 5 \mathfrak{e}_2 - 4 \mu_2 (1 + 3 \mathfrak{e}_2))) + \\
\eta t & (-6 + 14 \mu_1 - 4 \mu_1^2 + 4 \mu_2 - 20 \mu_1 \mu_2 + \theta l (22 + 8 \mu_2 + \\
& \mu_1^2 (3 + 3 \mathfrak{e}_1 + \mathfrak{e}_2) - \mu_1 (5 + 4 \mu_2 - 9 \mathfrak{e}_1 + 5 \mathfrak{e}_2 + 12 \mu_2 \mathfrak{e}_2))) + \\
\eta^4 & (2 \times (-26 - 5 \mu_1 + 15 \mu_1^2 - 16 \mu_2 - 76 \mu_1 \mu_2) + \theta l (-8 \mu_1^2 \\
& (11 + \mathfrak{e}_1) + \mu_2 (-16 + 15 \mathfrak{e}_1 - 15 \mathfrak{e}_2) + 5 \times (28 + 3 \mathfrak{e}_1 - 3 \mathfrak{e}_2) + \\
& \mu_1 (-44 + \mathfrak{e}_1 - 9 \mathfrak{e}_2 + \mu_2 (440 + 15 \mathfrak{e}_1 + 33 \mathfrak{e}_2))) + \\
\eta t & (14 - 84 \mu_1^2 - 55 \mu_1 (-2 + \mu_2) + 17 \mu_2 + \theta l (-124 - 15 \mathfrak{e}_1 + \\
& 8 \mu_1^2 (19 + \mathfrak{e}_1) + 15 \mathfrak{e}_2 + \mu_2 (16 - 15 \mathfrak{e}_1 + 15 \mathfrak{e}_2) - \\
& \mu_1 (20 + \mathfrak{e}_1 - 9 \mathfrak{e}_2 + \mu_2 (440 + 15 \mathfrak{e}_1 + 33 \mathfrak{e}_2)))) + \\
x^5 & (-1 + \eta)^5 (4 (-1 + w (-1 + \eta))^3 (-1 + \eta t) \theta l^2 (5 - 2 \mu_1 + 11 \mu_1^2) + \\
& 2 (-1 + \eta)^2 \theta p (-1 + 8 \eta - 12 \eta^2 + 4 \eta t + 12 \eta \eta t - 22 \mu_1 - 58 \\
& \eta \mu_1 - 12 \eta^2 \mu_1 + 4 \eta t \mu_1 + 12 \eta \eta t \mu_1 - 9 \mu_1^2 - 30 \\
& \eta \mu_1^2 + 2 w^3 (-1 + \eta)^3 (1 + \mu_1) (\eta - \eta t + 4 \mu_1) - 9 \\
& \mu_2 - 3 \mu_1 \mu_2 + 12 \eta \mu_1 \mu_2 - 6 \eta t \mu_1 \mu_2 - w^2 (-1 + \eta)^2 \\
& (5 + 42 \mu_1 + 25 \mu_1^2 + 6 \eta^2 (1 + \mu_1) + 11 \mu_2 - 7 \mu_1 \mu_2 + \\
& \eta (8 + 32 \mu_1 + 24 \mu_1^2 - 6 \eta t (1 + \mu_1) - 6 \mu_1 \mu_2) +
\end{aligned}$$



$$\begin{aligned}
& \eta t (-8 - 8 \mu 1 + 6 \mu 1 \mu 2) + 2 w (-1 + \eta) \times \\
& (3 + 28 \mu 1 + 13 \mu 1^2 + 9 \eta^2 (1 + \mu 1) + 10 \mu 2 - 2 \mu 1 \mu 2 + \eta (5 + 50 \mu 1 + \\
& 27 \mu 1^2 - 9 \eta t (1 + \mu 1) - 9 \mu 1 \mu 2) + \eta t (-5 - 5 \mu 1 + 6 \mu 1 \mu 2)) + \\
& \theta l (-4 \times (-1 + w (-1 + \eta)) \times (-1 + \eta) \times (-1 + \eta t) \mu 1 (5 + w (-1 + \eta) \times \\
& (-5 + \mu 1) - \mu 1 - \eta (1 + \mu 1)) + \theta p \\
& (-18 - 58 \eta - 72 \eta^2 + 50 \eta t + 122 \eta \eta t - 24 \eta^2 \eta t + 34 \mu 1 + 132 \eta \mu 1 - \\
& 86 \eta^2 \mu 1 - 18 \eta t \mu 1 - 100 \eta \eta t \mu 1 + 38 \eta^2 \eta t \mu 1 + 40 \mu 1^2 + 58 \eta \mu 1^2 - \\
& 158 \eta^2 \mu 1^2 + 16 \eta t \mu 1^2 + 54 \eta \eta t \mu 1^2 - 10 \eta^2 \eta t \mu 1^2 - 2 \mu 2 - 4 \eta \mu 2 - \\
& 2 \eta^2 \mu 2 + 2 \eta t \mu 2 + 4 \eta \eta t \mu 2 + 2 \eta^2 \eta t \mu 2 - 26 \mu 1 \mu 2 - 16 \eta \mu 1 \mu 2 + \\
& 10 \eta^2 \mu 1 \mu 2 + 26 \eta t \mu 1 \mu 2 + 16 \eta \eta t \mu 1 \mu 2 - 10 \eta^2 \eta t \mu 1 \mu 2 + \\
& 4 w^3 (-1 + \eta)^3 (5 - 8 \mu 1 - 13 \mu 1^2 + 2 \eta (4 + 2 \mu 1 + 7 \mu 1^2) + 2 \mu 2 + \\
& 8 \mu 1 \mu 2 - \eta t (13 - 4 \mu 1 + \mu 1^2 + 2 \mu 2 + 8 \mu 1 \mu 2) + 9 \mu 1 \mathfrak{e} 1 - \\
& 8 \eta \mu 1 \mathfrak{e} 1 - \eta^2 \mu 1 \mathfrak{e} 1 - 9 \eta t \mu 1 \mathfrak{e} 1 + 8 \eta \eta t \mu 1 \mathfrak{e} 1 + \eta^2 \eta t \mu 1 \mathfrak{e} 1 + \\
& 3 \mu 1^2 \mathfrak{e} 1 - 2 \eta \mu 1^2 \mathfrak{e} 1 - \eta^2 \mu 1^2 \mathfrak{e} 1 - 3 \eta t \mu 1^2 \mathfrak{e} 1 + 2 \eta \eta t \mu 1^2 \mathfrak{e} 1 + \\
& \eta^2 \eta t \mu 1^2 \mathfrak{e} 1 - 5 \mu 1 \mathfrak{e} 2 + 6 \eta \mu 1 \mathfrak{e} 2 - \eta^2 \mu 1 \mathfrak{e} 2 + 5 \eta t \mu 1 \mathfrak{e} 2 - \\
& 6 \eta \eta t \mu 1 \mathfrak{e} 2 + \eta^2 \eta t \mu 1 \mathfrak{e} 2 + \mu 1^2 \mathfrak{e} 2 - \eta^2 \mu 1^2 \mathfrak{e} 2 - \eta t \mu 1^2 \mathfrak{e} 2 + \\
& \eta^2 \eta t \mu 1^2 \mathfrak{e} 2 - 12 \mu 1 \mu 2 \mathfrak{e} 2 + 12 \eta \mu 1 \mu 2 \mathfrak{e} 2 + 12 \eta t \mu 1 \mu 2 \mathfrak{e} 2 - \\
& 12 \eta \eta t \mu 1 \mu 2 \mathfrak{e} 2 - w^2 (-1 + \eta)^2 (50 - 106 \mu 1 - 144 \mu 1^2 + \\
& 24 \eta^2 (4 + 2 \mu 1 + 7 \mu 1^2) + 14 \mu 2 + 110 \mu 1 \mu 2 - 9 \mu 1 \mathfrak{e} 1 - 3 \mu 1^2 \mathfrak{e} 1 + \\
& 5 \mu 1 \mathfrak{e} 2 - \mu 1^2 \mathfrak{e} 2 + 12 \mu 1 \mu 2 \mathfrak{e} 2 - \eta (-1 + \eta t) \times (2 \times (53 + 5 \mu 2) + \\
& \mu 1^2 (20 + 3 \mathfrak{e} 1 + \mathfrak{e} 2) - \mu 1 (78 - 9 \mathfrak{e} 1 + 5 \mathfrak{e} 2 + 2 \mu 2 (7 + 6 \mathfrak{e} 2))) + \\
& \eta t (-2 \times (73 + 7 \mu 2) + \mu 1^2 (-24 + 3 \mathfrak{e} 1 + \mathfrak{e} 2) + \\
& \mu 1 (58 + 9 \mathfrak{e} 1 - 5 \mathfrak{e} 2 - 2 \mu 2 (55 + 6 \mathfrak{e} 2))) - \\
& w (-1 + \eta) (\eta^2 (2 \times (-96 + (-1 + \eta t) \mu 2) - \mu 1 (158 - 10 \mu 2 + \\
& \mathfrak{e} 1 + \eta t (-62 + 10 \mu 2 - \mathfrak{e} 1 - \mathfrak{e} 2) + \mathfrak{e} 2) + \\
& \mu 1^2 (-326 - \mathfrak{e} 1 - \mathfrak{e} 2 + \eta t (-10 + \mathfrak{e} 1 + \mathfrak{e} 2))) + \eta \\
& (-2 \times (54 + 7 \mu 2) - \mu 1^2 (-94 + 5 \mathfrak{e} 1 + \mathfrak{e} 2) + \mu 1 (250 - 2 \mu 2 - 17 \mathfrak{e} 1 + \\
& 11 \mathfrak{e} 2 + 24 \mu 2 \mathfrak{e} 2) + \eta t (204 + 14 \mu 2 + \mu 1^2 (74 + 5 \mathfrak{e} 1 + \mathfrak{e} 2) + \\
& \mu 1 (-202 + 2 \mu 2 + 17 \mathfrak{e} 1 - 11 \mathfrak{e} 2 - 24 \mu 2 \mathfrak{e} 2))) - 2 \times \\
& (4 \times (6 + \mu 2) - \mu 1^2 (66 + 3 \mathfrak{e} 1 + \mathfrak{e} 2) + \mu 1 (-54 + 52 \mu 2 - 9 \mathfrak{e} 1 + 5 \\
& \mathfrak{e} 2 + 12 \mu 2 \mathfrak{e} 2) + \eta t (-4 \times (18 + \mu 2) + \mu 1^2 (-18 + 3 \mathfrak{e} 1 + \mathfrak{e} 2) + \\
& \mu 1 (30 + 9 \mathfrak{e} 1 - 5 \mathfrak{e} 2 - 4 \mu 2 (13 + 3 \mathfrak{e} 2)))) + x^2 (-1 + \eta)^2 \\
& (4 (-1 + w (-1 + \eta))^3 (1 + \eta) \times (-2 \eta (1 + 2 \eta) + w (-1 - 2 \eta + 3 \eta^2)) \times \\
& (-1 + \eta t) \theta l^2 (5 - 2 \mu 1 + 11 \mu 1^2) + \\
& (-1 + \eta)^2 \theta p (60 \eta + 156 \eta^2 + 44 \eta^3 + 20 \eta^4 + 60 \eta^5 - 30 \eta t - 60 \eta \\
& \eta t - 24 \eta^2 \eta t - 80 \eta^3 \eta t - 60 \eta^4 \eta t + 48 \eta \mu 1 + 252 \eta^2 \mu 1 + 464 \\
& \eta^3 \mu 1 + 350 \eta^4 \mu 1 + 60 \eta^5 \mu 1 - 32 \eta t \mu 1 - 148 \eta \eta t \mu 1 - 120 \eta^2 \\
& \eta t \mu 1 - 56 \eta^3 \eta t \mu 1 - 60 \eta^4 \eta t \mu 1 - 12 \eta \mu 1^2 + 24 \eta^2 \mu 1^2 + 180 \\
& \eta^3 \mu 1^2 + 150 \eta^4 \mu 1^2 + 22 \eta t \mu 1^2 + 104 \eta \eta t \mu 1^2 + 48 \eta^2 \eta t \\
& \mu 1^2 + 24 \eta^3 \eta t \mu 1^2 + 32 \eta \mu 2 + 228 \eta^2 \mu 2 + 204 \eta^3 \mu 2 - 10 \\
& \eta t \mu 2 - 27 \eta \eta t \mu 2 - 24 \eta^2 \eta t \mu 2 + 56 \eta \mu 1 \mu 2 + 12 \eta^2 \mu 1 \\
& \mu 2 - 204 \eta^3 \mu 1 \mu 2 - 240 \eta^4 \mu 1 \mu 2 + 38 \eta t \mu 1 \mu 2 + 117 \eta \eta t \\
& \mu 1 \mu 2 + 192 \eta^2 \eta t \mu 1 \mu 2 + 120 \eta^3 \eta t \mu 1 \mu 2 + w^4 (-1 + \eta)^4 \\
& (12 \eta^3 (1 + \mu 1) - 12 \eta^2 (-1 + \eta t - 5 \mu 1 + \eta t \mu 1 - 4 \mu 1^2 + 3 \mu 1 \mu 2) +
\end{aligned}$$

$$\begin{aligned}
& 2 \times (5 + 8 \mu_1 + 3 \mu_1^2 + 11 \mu_2 + 5 \mu_1 \mu_2) + \\
& \eta t (-12 - 22 \mu_1 + 38 \mu_1^2 + 5 \mu_2 + 17 \mu_1 \mu_2) + \\
& 2 \eta (16 + 37 \mu_1 + 21 \mu_1^2 + 33 \mu_2 - 27 \mu_1 \mu_2 + 6 \eta t (-1 - \mu_1 + 3 \mu_1 \mu_2)) - \\
& w^3 (-1 + \eta)^3 (40 \eta^4 (1 + \mu_1) + 2 \times (20 + 31 \mu_1 + 5 \mu_1^2 + 30 \mu_2 + 6 \mu_1 \mu_2) - \\
& 4 \eta^3 (-21 - 61 \mu_1 - 40 \mu_1^2 + 10 \eta t (1 + \mu_1) + 36 \mu_1 \mu_2) + \\
& \eta t (-66 - 130 \mu_1 + 128 \mu_1^2 + \mu_2 + 97 \mu_1 \mu_2) + \\
& 3 \eta (62 + 40 \mu_1^2 + 36 \eta t \mu_1^2 + 2 \mu_1 (63 - 34 \mu_2) + \\
& 112 \mu_2 - 9 \eta t (4 + \mu_2) + \eta t \mu_1 (-64 + 87 \mu_2)) + 12 \eta^2 \\
& (14 + 43 \mu_1 + 23 \mu_1^2 + 22 \mu_2 - 29 \mu_1 \mu_2 + \eta t (-7 - 7 \mu_1 + 12 \mu_1 \mu_2)) + \\
& w^2 (-1 + \eta)^2 (46 + 58 \mu_1 + 30 \eta^5 (1 + \mu_1) + 50 \mu_2 + 14 \mu_1 \mu_2 + \\
& \eta t (-124 - 224 \mu_1 + 164 \mu_1^2 - 23 \mu_2 + 181 \mu_1 \mu_2) - \\
& 10 \eta^4 (3 \eta t (1 + \mu_1) - 4 \times (4 + 7 \mu_1 + 3 \mu_1^2 - 3 \mu_1 \mu_2)) + \\
& 4 \eta^3 (70 + 255 \mu_1 + 125 \mu_1^2 + 55 \mu_2 - 161 \mu_1 \mu_2 + \\
& 10 \eta t (-4 - 4 \mu_1 + 3 \mu_1 \mu_2)) + 12 \eta^2 (38 + 106 \mu_1 + 38 \mu_1^2 + \\
& 65 \mu_2 - 61 \mu_1 \mu_2 + \eta t (-15 - 23 \mu_1 + 4 \mu_1^2 - 2 \mu_2 + 40 \mu_1 \mu_2)) + \\
& \eta (2 \times (155 + 278 \mu_1 + 51 \mu_1^2 + 249 \mu_2 - 69 \mu_1 \mu_2) + \\
& 3 \eta t (-80 - 164 \mu_1 + 108 \mu_1^2 - 27 \mu_2 + 177 \mu_1 \mu_2)) - w \\
& (-1 + \eta) \times (90 \eta^5 (1 + \mu_1) - 4 \times (1 + \mu_1) \times (-5 + \mu_1 - 3 \mu_2) + \\
& 10 \eta^4 (20 + 65 \mu_1 + 27 \mu_1^2 - 9 \eta t (1 + \mu_1) - 36 \mu_1 \mu_2) + \\
& \eta t (-100 - 148 \mu_1 + 96 \mu_1^2 - 29 \mu_2 + 139 \mu_1 \mu_2) + \\
& 12 \eta^2 (34 + 85 \mu_1 + 21 \mu_1^2 + 62 \mu_2 - 34 \mu_1 \mu_2 + \\
& \eta t (-11 - 27 \mu_1 + 8 \mu_1^2 - 4 \mu_2 + 44 \mu_1 \mu_2)) + 4 \eta^3 (63 + 313 \mu_1 + \\
& 130 \mu_1^2 + 106 \mu_2 - 176 \mu_1 \mu_2 + \eta t (-50 - 44 \mu_1 + 6 \mu_1^2 + 60 \mu_1 \mu_2)) + \\
& \eta (4 \times (54 + 75 \mu_1 + 3 \mu_1^2 + 65 \mu_2 + 17 \mu_1 \mu_2) + \eta t \\
& (-204 - 460 \mu_1 + 320 \mu_1^2 - 81 \mu_2 + 423 \mu_1 \mu_2)) + \\
& \text{el} (-10 - 50 \eta + 60 \eta^3 + 10 \eta t + 50 \eta \eta t - 60 \eta^3 \eta t + 10 \text{ep} + 80 \eta \\
& \text{ep} + 174 \eta^2 \text{ep} + 312 \eta^3 \text{ep} + 400 \eta^4 \text{ep} + 180 \eta^5 \text{ep} - 30 \\
& \eta t \text{ep} - 180 \eta \eta t \text{ep} - 270 \eta^2 \eta t \text{ep} - 416 \eta^3 \eta t \text{ep} - 320 \\
& \eta^4 \eta t \text{ep} + 60 \eta^5 \eta t \text{ep} - 8 \mu_1 - 56 \eta \mu_1 - 100 \eta^2 \mu_1 + 84 \\
& \eta^3 \mu_1 + 96 \eta^4 \mu_1 - 16 \eta^5 \mu_1 + 8 \eta t \mu_1 + 56 \eta \eta t \mu_1 + 100 \\
& \eta^2 \eta t \mu_1 - 84 \eta^3 \eta t \mu_1 - 96 \eta^4 \eta t \mu_1 + 16 \eta^5 \eta t \mu_1 + 8 \text{ep} \\
& \mu_1 + 96 \eta \text{ep} \mu_1 + 58 \eta^2 \text{ep} \mu_1 - 346 \eta^3 \text{ep} \mu_1 - 138 \eta^4 \text{ep} \\
& \mu_1 + 230 \eta^5 \text{ep} \mu_1 - 56 \eta \eta t \text{ep} \mu_1 - 106 \eta^2 \eta t \text{ep} \mu_1 + 186 \\
& \eta^3 \eta t \text{ep} \mu_1 + 178 \eta^4 \eta t \text{ep} \mu_1 - 110 \eta^5 \eta t \text{ep} \mu_1 + 2 \mu_1^2 - 6 \\
& \eta \mu_1^2 + 32 \eta^2 \mu_1^2 - 12 \eta^3 \mu_1^2 - 16 \eta^5 \mu_1^2 - 2 \eta t \mu_1^2 + 6 \eta \\
& \eta t \mu_1^2 - 32 \eta^2 \eta t \mu_1^2 + 12 \eta^3 \eta t \mu_1^2 + 16 \eta^5 \eta t \mu_1^2 - 2 \text{ep} \\
& \mu_1^2 - 20 \eta \text{ep} \mu_1^2 - 152 \eta^2 \text{ep} \mu_1^2 - 250 \eta^3 \text{ep} \mu_1^2 + 242 \eta^4 \\
& \text{ep} \mu_1^2 + 410 \eta^5 \text{ep} \mu_1^2 - 42 \eta t \text{ep} \mu_1^2 - 200 \eta \eta t \text{ep} \mu_1^2 - 16 \\
& \eta^2 \eta t \text{ep} \mu_1^2 + 122 \eta^3 \eta t \text{ep} \mu_1^2 - 102 \eta^4 \eta t \text{ep} \mu_1^2 + 10 \\
& \eta^5 \eta t \text{ep} \mu_1^2 - 5 \mu_2 - 15 \eta \mu_2 + 5 \eta^2 \mu_2 + 15 \eta^3 \mu_2 + 5 \eta t \\
& \mu_2 + 15 \eta \eta t \mu_2 - 5 \eta^2 \eta t \mu_2 - 15 \eta^3 \eta t \mu_2 + 10 \text{ep} \mu_2 + 54 \eta \\
& \text{ep} \mu_2 + 22 \eta^2 \text{ep} \mu_2 - 10 \eta^3 \text{ep} \mu_2 + 52 \eta^4 \text{ep} \mu_2 + 20 \eta^5 \text{ep} \\
& \mu_2 - 10 \eta t \text{ep} \mu_2 - 54 \eta \eta t \text{ep} \mu_2 - 22 \eta^2 \eta t \text{ep} \mu_2 + 10 \eta^3 \\
& \eta t \text{ep} \mu_2 - 52 \eta^4 \eta t \text{ep} \mu_2 - 20 \eta^5 \eta t \text{ep} \mu_2 + 19 \mu_1 \mu_2 + 57
\end{aligned}$$

$$\begin{aligned}
& \eta \mu_1 \mu_2 - 19 \eta^2 \mu_1 \mu_2 - 57 \eta^3 \mu_1 \mu_2 - 19 \eta t \mu_1 \mu_2 - 57 \eta \eta t \\
& \mu_1 \mu_2 + 19 \eta^2 \eta t \mu_1 \mu_2 + 57 \eta^3 \eta t \mu_1 \mu_2 - 14 \text{ep} \mu_1 \mu_2 + 18 \\
& \eta \text{ep} \mu_1 \mu_2 + 430 \eta^2 \text{ep} \mu_1 \mu_2 + 626 \eta^3 \text{ep} \mu_1 \mu_2 + 100 \eta^4 \\
& \text{ep} \mu_1 \mu_2 - 100 \eta^5 \text{ep} \mu_1 \mu_2 + 14 \eta t \text{ep} \mu_1 \mu_2 - 18 \eta \eta t \text{ep} \\
& \mu_1 \mu_2 - 430 \eta^2 \eta t \text{ep} \mu_1 \mu_2 - 626 \eta^3 \eta t \text{ep} \mu_1 \mu_2 - 100 \\
& \eta^4 \eta t \text{ep} \mu_1 \mu_2 + 100 \eta^5 \eta t \text{ep} \mu_1 \mu_2 + 2 w^4 (-1 + \eta)^4 \\
& (-5 + 10 \text{ep} - 10 \mu_1 - 4 \text{ep} \mu_1 + \mu_1^2 - 14 \text{ep} \mu_1^2 + 12 \eta^3 \text{ep} (4 + 2 \mu_1 + 7 \mu_1^2) + \\
& 5 \mu_2 + 5 \mu_1 \mu_2 + 36 \text{ep} \mu_1 \mu_2 - \eta t (\mu_1^2 + 5 \mu_1 (-2 + \mu_2) + \\
& 5 \times (-1 + \mu_2) + \text{ep} (38 + 44 \mu_1^2 + 4 \mu_1 (-2 + 9 \mu_2))) - \\
& \eta (5 + 10 \mu_1 - 19 \mu_1^2 + \text{ep} (-68 + 20 \mu_1 + 70 \mu_1^2 - 216 \mu_1 \mu_2) + \\
& \eta t (-5 - 10 \mu_1 + 19 \mu_1^2 + 2 \text{ep} (59 - 2 \mu_1 + 11 \mu_1^2 + 108 \mu_1 \mu_2))) + \\
& \eta^2 (-5 \times (-2 + 4 \mu_1^2 + \mu_1 (-4 + \mu_2) + \mu_2) + 108 \text{ep} (1 + 2 \mu_1 \mu_2) + \\
& \eta t (5 \times (-2 + 4 \mu_1^2 + \mu_1 (-4 + \mu_2) + \mu_2) + \\
& 6 \text{ep} (-13 + 11 \mu_1^2 - 2 \mu_1 (1 + 18 \mu_2)))) - 5 \text{ep} \\
& \mathfrak{E}1 - 25 \eta \text{ep} \mathfrak{E}1 + 30 \eta^3 \text{ep} \mathfrak{E}1 + 5 \eta t \text{ep} \mathfrak{E}1 + 25 \eta \eta t \text{ep} \mathfrak{E}1 - 30 \\
& \eta^3 \eta t \text{ep} \mathfrak{E}1 - 4 \text{ep} \mu_1 \mathfrak{E}1 - 46 \eta \text{ep} \mu_1 \mathfrak{E}1 - 79 \eta^2 \text{ep} \mu_1 \\
& \mathfrak{E}1 + 33 \eta^3 \text{ep} \mu_1 \mathfrak{E}1 + 86 \eta^4 \text{ep} \mu_1 \mathfrak{E}1 + 10 \eta^5 \text{ep} \mu_1 \mathfrak{E}1 + 4 \\
& \eta t \text{ep} \mu_1 \mathfrak{E}1 + 46 \eta \eta t \text{ep} \mu_1 \mathfrak{E}1 + 79 \eta^2 \eta t \text{ep} \mu_1 \mathfrak{E}1 - 33 \eta^3 \\
& \eta t \text{ep} \mu_1 \mathfrak{E}1 - 86 \eta^4 \eta t \text{ep} \mu_1 \mathfrak{E}1 - 10 \eta^5 \eta t \text{ep} \mu_1 \mathfrak{E}1 + \text{ep} \\
& \mu_1^2 \mathfrak{E}1 - 3 \eta \text{ep} \mu_1^2 \mathfrak{E}1 - 25 \eta^2 \text{ep} \mu_1^2 \mathfrak{E}1 - 9 \eta^3 \text{ep} \mu_1^2 \\
& \mathfrak{E}1 + 26 \eta^4 \text{ep} \mu_1^2 \mathfrak{E}1 + 10 \eta^5 \text{ep} \mu_1^2 \mathfrak{E}1 - \eta t \text{ep} \mu_1^2 \mathfrak{E}1 + 3 \\
& \eta \eta t \text{ep} \mu_1^2 \mathfrak{E}1 + 25 \eta^2 \eta t \text{ep} \mu_1^2 \mathfrak{E}1 + 9 \eta^3 \eta t \text{ep} \mu_1^2 \\
& \mathfrak{E}1 - 26 \eta^4 \eta t \text{ep} \mu_1^2 \mathfrak{E}1 - 10 \eta^5 \eta t \text{ep} \mu_1^2 \mathfrak{E}1 - 5 \text{ep} \mu_2 \\
& \mathfrak{E}1 - 25 \eta \text{ep} \mu_2 \mathfrak{E}1 + 30 \eta^3 \text{ep} \mu_2 \mathfrak{E}1 + 5 \eta t \text{ep} \mu_2 \mathfrak{E}1 + 25 \\
& \eta \eta t \text{ep} \mu_2 \mathfrak{E}1 - 30 \eta^3 \eta t \text{ep} \mu_2 \mathfrak{E}1 - 5 \text{ep} \mu_1 \mu_2 \mathfrak{E}1 - 25 \eta \\
& \text{ep} \mu_1 \mu_2 \mathfrak{E}1 + 30 \eta^3 \text{ep} \mu_1 \mu_2 \mathfrak{E}1 + 5 \eta t \text{ep} \mu_1 \mu_2 \mathfrak{E}1 + 25 \eta \\
& \eta t \text{ep} \mu_1 \mu_2 \mathfrak{E}1 - 30 \eta^3 \eta t \text{ep} \mu_1 \mu_2 \mathfrak{E}1 + 5 \text{ep} \mathfrak{E}2 + 25 \eta \text{ep} \\
& \mathfrak{E}2 - 30 \eta^3 \text{ep} \mathfrak{E}2 - 5 \eta t \text{ep} \mathfrak{E}2 - 25 \eta \eta t \text{ep} \mathfrak{E}2 + 30 \eta^3 \eta t \\
& \text{ep} \mathfrak{E}2 + 4 \text{ep} \mu_1 \mathfrak{E}2 + 36 \eta \text{ep} \mu_1 \mathfrak{E}2 + 47 \eta^2 \text{ep} \mu_1 \mathfrak{E}2 - 43 \\
& \eta^3 \text{ep} \mu_1 \mathfrak{E}2 - 54 \eta^4 \text{ep} \mu_1 \mathfrak{E}2 + 10 \eta^5 \text{ep} \mu_1 \mathfrak{E}2 - 4 \eta t \text{ep} \\
& \mu_1 \mathfrak{E}2 - 36 \eta \eta t \text{ep} \mu_1 \mathfrak{E}2 - 47 \eta^2 \eta t \text{ep} \mu_1 \mathfrak{E}2 + 43 \eta^3 \eta t \\
& \text{ep} \mu_1 \mathfrak{E}2 + 54 \eta^4 \eta t \text{ep} \mu_1 \mathfrak{E}2 - 10 \eta^5 \eta t \text{ep} \mu_1 \mathfrak{E}2 - \text{ep} \mu_1^2 \\
& \mathfrak{E}2 - 7 \eta \text{ep} \mu_1^2 \mathfrak{E}2 - 7 \eta^2 \text{ep} \mu_1^2 \mathfrak{E}2 - \eta^3 \text{ep} \mu_1^2 \mathfrak{E}2 + 6 \eta^4 \\
& \text{ep} \mu_1^2 \mathfrak{E}2 + 10 \eta^5 \text{ep} \mu_1^2 \mathfrak{E}2 + \eta t \text{ep} \mu_1^2 \mathfrak{E}2 + 7 \eta \eta t \text{ep} \mu_1^2 \\
& \mathfrak{E}2 + 7 \eta^2 \eta t \text{ep} \mu_1^2 \mathfrak{E}2 + \eta^3 \eta t \text{ep} \mu_1^2 \mathfrak{E}2 - 6 \eta^4 \eta t \text{ep} \mu_1^2 \\
& \mathfrak{E}2 - 10 \eta^5 \eta t \text{ep} \mu_1^2 \mathfrak{E}2 + 5 \text{ep} \mu_2 \mathfrak{E}2 + 25 \eta \text{ep} \mu_2 \mathfrak{E}2 - 30 \\
& \eta^3 \text{ep} \mu_2 \mathfrak{E}2 - 5 \eta t \text{ep} \mu_2 \mathfrak{E}2 - 25 \eta \eta t \text{ep} \mu_2 \mathfrak{E}2 + 30 \eta^3 \eta t \\
& \text{ep} \mu_2 \mathfrak{E}2 - 7 \text{ep} \mu_1 \mu_2 \mathfrak{E}2 + \eta \text{ep} \mu_1 \mu_2 \mathfrak{E}2 + 108 \eta^2 \text{ep} \mu_1 \\
& \mu_2 \mathfrak{E}2 + 18 \eta^3 \text{ep} \mu_1 \mu_2 \mathfrak{E}2 - 120 \eta^4 \text{ep} \mu_1 \mu_2 \mathfrak{E}2 + 7 \eta t \text{ep} \\
& \mu_1 \mu_2 \mathfrak{E}2 - \eta \eta t \text{ep} \mu_1 \mu_2 \mathfrak{E}2 - 108 \eta^2 \eta t \text{ep} \mu_1 \mu_2 \mathfrak{E}2 - 18 \\
& \eta^3 \eta t \text{ep} \mu_1 \mu_2 \mathfrak{E}2 + 120 \eta^4 \eta t \text{ep} \mu_1 \mu_2 \mathfrak{E}2 + w (-1 + \eta) \times \\
& (40 - 40 \eta t - 40 \text{ep} + 140 \eta t \text{ep} + 44 \mu_1 - 44 \eta t \mu_1 - 46 \text{ep} \mu_1 + 6 \eta t \text{ep} \mu_1 - \\
& 8 \mu_1^2 + 8 \eta t \mu_1^2 + 6 \text{ep} \mu_1^2 + 214 \eta t \text{ep} \mu_1^2 + 5 \mu_2 - 5 \eta t \mu_2 - \\
& 24 \text{ep} \mu_2 + 24 \eta t \text{ep} \mu_2 - 67 \mu_1 \mu_2 + 67 \eta t \mu_1 \mu_2 - 24 \text{ep} \mu_1 \mu_2 + \\
& 24 \eta t \text{ep} \mu_1 \mu_2 + 15 \text{ep} \mathfrak{E}1 - 15 \eta t \text{ep} \mathfrak{E}1 + 19 \text{ep} \mu_1 \mathfrak{E}1 - 19 \eta t \text{ep} \mu_1 \mathfrak{E}1 - \\
& 2 \text{ep} \mu_1^2 \mathfrak{E}1 + 2 \eta t \text{ep} \mu_1^2 \mathfrak{E}1 + 15 \text{ep} \mu_2 \mathfrak{E}1 - 15 \eta t \text{ep} \mu_2 \mathfrak{E}1 +
\end{aligned}$$

$$\begin{aligned}
& 15 \operatorname{ep} \mu_1 \mu_2 \mathfrak{x}_1 - 15 \eta t \operatorname{ep} \mu_1 \mu_2 \mathfrak{x}_1 - 15 \operatorname{ep} \mathfrak{x}_2 + 15 \eta t \operatorname{ep} \mathfrak{x}_2 - \\
& 19 \operatorname{ep} \mu_1 \mathfrak{x}_2 + 19 \eta t \operatorname{ep} \mu_1 \mathfrak{x}_2 + 2 \operatorname{ep} \mu_1^2 \mathfrak{x}_2 - 2 \eta t \operatorname{ep} \mu_1^2 \mathfrak{x}_2 - \\
& 15 \operatorname{ep} \mu_2 \mathfrak{x}_2 + 15 \eta t \operatorname{ep} \mu_2 \mathfrak{x}_2 + 9 \operatorname{ep} \mu_1 \mu_2 \mathfrak{x}_2 - 9 \eta t \operatorname{ep} \mu_1 \mu_2 \mathfrak{x}_2 + \\
& 2 \eta^5 \left( -8 \times (-1 + \eta t) \mu_1 (1 + \mu_1) + 5 \operatorname{ep} (-48 + 2 \times (-1 + \eta t) \mu_2 - \right. \\
& \quad \mu_1 (41 - 10 \mu_2 + \mathfrak{x}_1 + \eta t (-17 + 10 \mu_2 - \mathfrak{x}_1 - \mathfrak{x}_2) + \mathfrak{x}_2) + \\
& \quad \left. \mu_1^2 (-83 - \mathfrak{x}_1 - \mathfrak{x}_2 + \eta t (-1 + \mathfrak{x}_1 + \mathfrak{x}_2)) \right) + \\
& \eta \left( 160 + 260 \mu_1 + 4 \mu_1^2 + 45 \mu_2 - 171 \mu_1 \mu_2 + \operatorname{ep} (-364 + 75 \mathfrak{x}_1 + \right. \\
& \quad \mu_2 (-134 + 75 \mathfrak{x}_1 - 75 \mathfrak{x}_2) + 2 \mu_1 (-124 + 74 \mathfrak{x}_1 - 63 \mathfrak{x}_2) + \\
& \quad \left. \mu_1 \mu_2 (-554 + 75 \mathfrak{x}_1 - 27 \mathfrak{x}_2) - 75 \mathfrak{x}_2 + \mu_1^2 (176 + 7 \mathfrak{x}_1 + 15 \mathfrak{x}_2) \right) + \\
& \eta t \left( -160 - 260 \mu_1 - 4 \mu_1^2 - 45 \mu_2 + 171 \mu_1 \mu_2 + \operatorname{ep} (780 - 75 \mathfrak{x}_1 + \mu_1^2 \right. \\
& \quad (696 - 7 \mathfrak{x}_1 - 15 \mathfrak{x}_2) + 75 \mathfrak{x}_2 + \mu_1 \mu_2 (554 - 75 \mathfrak{x}_1 + 27 \mathfrak{x}_2) + \\
& \quad \left. 2 \mu_1 (84 - 74 \mathfrak{x}_1 + 63 \mathfrak{x}_2) + \mu_2 (134 - 75 \mathfrak{x}_1 + 75 \mathfrak{x}_2) \right) + \\
& \eta^2 \left( -20 + 172 \mu_1 - 96 \mu_1^2 - 5 \mu_2 + 67 \mu_1 \mu_2 + 4 \operatorname{ep} (-207 - \right. \\
& \quad 19 \mu_2 + \mu_1^2 (173 + 13 \mathfrak{x}_1 + 4 \mathfrak{x}_2) + \mu_1 (38 - 499 \mu_2 + 40 \mathfrak{x}_1 - \\
& \quad 23 \mathfrak{x}_2 - 54 \mu_2 \mathfrak{x}_2) + \eta t (20 - 172 \mu_1 + 96 \mu_1^2 + 5 \mu_2 - \\
& \quad 67 \mu_1 \mu_2 - 4 \operatorname{ep} (-312 - 19 \mu_2 + \mu_1^2 (-4 + 13 \mathfrak{x}_1 + 4 \mathfrak{x}_2) - \\
& \quad \left. \mu_1 (28 + 499 \mu_2 - 40 \mathfrak{x}_1 + 23 \mathfrak{x}_2 + 54 \mu_2 \mathfrak{x}_2) \right) + \\
& \eta^3 \left( -180 - 316 \mu_1 + 68 \mu_1^2 - 45 \mu_2 + 171 \mu_1 \mu_2 + \operatorname{ep} (834 \mu_1 - \right. \\
& \quad 141 \mu_1 \mathfrak{x}_1 - 2 \mu_2 (19 + 45 \mathfrak{x}_1 - 45 \mathfrak{x}_2) + \mu_1^2 (378 + 9 \mathfrak{x}_1 - 7 \mathfrak{x}_2) - \\
& \quad 90 \times (12 + \mathfrak{x}_1 - \mathfrak{x}_2) + 143 \mu_1 \mathfrak{x}_2 - 2 \mu_1 \mu_2 (841 + 45 \mathfrak{x}_1 + 3 \mathfrak{x}_2) + \\
& \quad \eta t (-68 \mu_1^2 + \mu_1 (316 - 171 \mu_2) + 45 \times (4 + \mu_2) + \operatorname{ep} (1104 + 90 \mathfrak{x}_1 + \\
& \quad \mu_2 (38 + 90 \mathfrak{x}_1 - 90 \mathfrak{x}_2) - 90 \mathfrak{x}_2 + \mu_1^2 (-498 - 9 \mathfrak{x}_1 + 7 \mathfrak{x}_2) + \\
& \quad \left. \mu_1 (-498 + 141 \mathfrak{x}_1 - 143 \mathfrak{x}_2 + 2 \mu_2 (841 + 45 \mathfrak{x}_1 + 3 \mathfrak{x}_2)) \right) + \\
& 2 \eta^4 \left( -8 \times (-1 + \eta t) \times (-11 + \mu_1) \mu_1 + \operatorname{ep} (-540 - 76 \mu_2 - \right. \\
& \quad \mu_1^2 (481 + 28 \mathfrak{x}_1 + 8 \mathfrak{x}_2) + \mu_1 (29 - 88 \mathfrak{x}_1 + 52 \mathfrak{x}_2 + \\
& \quad 20 \mu_2 (1 + 6 \mathfrak{x}_2)) + \eta t (300 + 76 \mu_2 + \mu_1^2 (61 + 28 \mathfrak{x}_1 + 8 \mathfrak{x}_2) - \\
& \quad \left. \mu_1 (149 - 88 \mathfrak{x}_1 + 52 \mathfrak{x}_2 + 20 \mu_2 (1 + 6 \mathfrak{x}_2)) \right) + w^2 \\
& (-1 + \eta)^2 \left( -60 + 60 \eta t + 74 \operatorname{ep} - 270 \eta t \operatorname{ep} - 84 \mu_1 + 84 \eta t \mu_1 + \right. \\
& \quad 58 \operatorname{ep} \mu_1 + 6 \eta t \operatorname{ep} \mu_1 + 12 \mu_1^2 - 12 \eta t \mu_1^2 - 28 \operatorname{ep} \mu_1^2 - \\
& \quad 396 \eta t \operatorname{ep} \mu_1^2 + 60 \eta^5 \operatorname{ep} (4 + 2 \mu_1 + 7 \mu_1^2) + 15 \mu_2 - 15 \eta t \mu_2 + \\
& \quad 14 \operatorname{ep} \mu_2 - 14 \eta t \operatorname{ep} \mu_2 + 87 \mu_1 \mu_2 - 87 \eta t \mu_1 \mu_2 + 182 \operatorname{ep} \mu_1 \mu_2 - \\
& \quad 182 \eta t \operatorname{ep} \mu_1 \mu_2 - 15 \operatorname{ep} \mathfrak{x}_1 + 15 \eta t \operatorname{ep} \mathfrak{x}_1 - 26 \operatorname{ep} \mu_1 \mathfrak{x}_1 + \\
& \quad 26 \eta t \operatorname{ep} \mu_1 \mathfrak{x}_1 + \operatorname{ep} \mu_1^2 \mathfrak{x}_1 - \eta t \operatorname{ep} \mu_1^2 \mathfrak{x}_1 - 15 \operatorname{ep} \mu_2 \mathfrak{x}_1 + \\
& \quad 15 \eta t \operatorname{ep} \mu_2 \mathfrak{x}_1 - 15 \operatorname{ep} \mu_1 \mu_2 \mathfrak{x}_1 + 15 \eta t \operatorname{ep} \mu_1 \mu_2 \mathfrak{x}_1 + 15 \operatorname{ep} \mathfrak{x}_2 - \\
& \quad 15 \eta t \operatorname{ep} \mathfrak{x}_2 + 26 \operatorname{ep} \mu_1 \mathfrak{x}_2 - 26 \eta t \operatorname{ep} \mu_1 \mathfrak{x}_2 - \operatorname{ep} \mu_1^2 \mathfrak{x}_2 + \\
& \quad \eta t \operatorname{ep} \mu_1^2 \mathfrak{x}_2 + 15 \operatorname{ep} \mu_2 \mathfrak{x}_2 - 15 \eta t \operatorname{ep} \mu_2 \mathfrak{x}_2 + 3 \operatorname{ep} \mu_1 \mu_2 \mathfrak{x}_2 - \\
& \quad 3 \eta t \operatorname{ep} \mu_1 \mu_2 \mathfrak{x}_2 + \eta^3 (180 + 388 \mu_1 - 92 \mu_1^2 + 45 \mu_2 - 171 \mu_1 \mu_2 - \\
& \quad \eta t (-92 \mu_1^2 + \mu_1 (388 - 171 \mu_2) + 45 \times (4 + \mu_2) + 2 \operatorname{ep} (568 + 45 \mathfrak{x}_1 + \\
& \quad \mu_1 (-200 + 87 \mathfrak{x}_1 + \mu_2 (748 + 45 \mathfrak{x}_1 - 21 \mathfrak{x}_2) - 83 \mathfrak{x}_2) + \\
& \quad \mu_2 (52 + 45 \mathfrak{x}_1 - 45 \mathfrak{x}_2) + 4 \mu_1^2 (-78 + \mathfrak{x}_2) - 45 \mathfrak{x}_2) + 2 \operatorname{ep} \\
& \quad (748 + 45 \mathfrak{x}_1 + \mu_1 (-272 + 87 \mathfrak{x}_1 + \mu_2 (748 + 45 \mathfrak{x}_1 - 21 \mathfrak{x}_2) - \\
& \quad 83 \mathfrak{x}_2) + \mu_2 (52 + 45 \mathfrak{x}_1 - 45 \mathfrak{x}_2) - 45 \mathfrak{x}_2 + 4 \mu_1^2 (21 + \mathfrak{x}_2)) + \\
& \quad \eta (48 \mu_1^2 - 45 \times (4 + \mu_2) + 3 \mu_1 (-124 + 57 \mu_2) + \eta t (180 + \\
& \quad 372 \mu_1 - 48 \mu_1^2 + 45 \mu_2 - 171 \mu_1 \mu_2 + \operatorname{ep} (-1228 + 75 \mathfrak{x}_1 + \mu_1
\end{aligned}$$

$$\begin{aligned}
& (-144 + 157 \, \mathfrak{e}1 + \mu2 \, (-1516 + 75 \, \mathfrak{e}1 - 51 \, \mathfrak{e}2) - 145 \, \mathfrak{e}2) + 25 \\
& \mu2 \, (-4 + 3 \, \mathfrak{e}1 - 3 \, \mathfrak{e}2) - 75 \, \mathfrak{e}2 + 4 \, \mu1^2 \, (-209 + \mathfrak{e}1 + 2 \, \mathfrak{e}2) \Big) + \\
& \mathfrak{e}p \, (596 - 75 \, \mathfrak{e}1 - 25 \, \mu2 \, (-4 + 3 \, \mathfrak{e}1 - 3 \, \mathfrak{e}2) + 75 \, \mathfrak{e}2 - \\
& 4 \, \mu1^2 \, (\mathfrak{e}1 + 2 \times (54 + \mathfrak{e}2)) + \\
& \mu1 \, (152 - 157 \, \mathfrak{e}1 + 145 \, \mathfrak{e}2 + \mu2 \, (1516 - 75 \, \mathfrak{e}1 + 51 \, \mathfrak{e}2)) \Big) - \\
& 2 \, \eta^4 \, (-8 \times (-1 + \eta t) \times (-5 + \mu1) \, \mu1 + 5 \, \mathfrak{e}p \, (-2 \times (53 + 5 \, \mu2) - \\
& \mu1^2 \, (128 + 3 \, \mathfrak{e}1 + \mathfrak{e}2) + \mu1 \, (-30 - 9 \, \mathfrak{e}1 + 5 \, \mathfrak{e}2 + 2 \, \mu2 \, (7 + 6 \, \mathfrak{e}2)) + \\
& \eta t \, (34 + 10 \, \mu2 + \mu1^2 \, (2 + 3 \, \mathfrak{e}1 + \mathfrak{e}2) - \mu1 \, (6 - 9 \, \mathfrak{e}1 + 5 \, \mathfrak{e}2 + \\
& 2 \, \mu2 \, (7 + 6 \, \mathfrak{e}2))) \Big) + 3 \, \eta^2 \, (20 - 4 \, \mu1 + 16 \, \mu1^2 - 5 \, \mu2 - \\
& 29 \, \mu1 \, \mu2 + \mathfrak{e}p \, (6 \times (71 + 7 \, \mu2) - \mu1^2 \, (332 + 9 \, \mathfrak{e}1 + 3 \, \mathfrak{e}2) + \\
& \mu1 \, (-158 + 978 \, \mu2 - 27 \, \mathfrak{e}1 + 15 \, \mathfrak{e}2 + 36 \, \mu2 \, \mathfrak{e}2)) + \eta t \, (-20 + 4 \, \mu1 - \\
& 16 \, \mu1^2 + 5 \, \mu2 + 29 \, \mu1 \, \mu2 + \mathfrak{e}p \, (-590 - 42 \, \mu2 + 3 \, \mu1^2 \, (24 + 3 \, \mathfrak{e}1 + \\
& \mathfrak{e}2) + \mu1 \, (22 + 27 \, \mathfrak{e}1 - 15 \, \mathfrak{e}2 - 6 \, \mu2 \, (163 + 6 \, \mathfrak{e}2)))) \Big) - \\
& w^3 \, (-1 + \eta)^3 \, (-40 + 40 \, \eta t + 60 \, \mathfrak{e}p - 232 \, \eta t \, \mathfrak{e}p - 68 \, \mu1 + 68 \, \eta t \, \mu1 + \\
& 8 \, \mathfrak{e}p \, \mu1 + 32 \, \eta t \, \mathfrak{e}p \, \mu1 + 8 \, \mu1^2 - 8 \, \eta t \, \mu1^2 - 52 \, \mathfrak{e}p \, \mu1^2 - \\
& 312 \, \eta t \, \mathfrak{e}p \, \mu1^2 + 80 \, \eta^4 \, \mathfrak{e}p \, (4 + 2 \, \mu1 + 7 \, \mu1^2) + 25 \, \mu2 - 25 \, \eta t \, \mu2 + \\
& 49 \, \mu1 \, \mu2 - 49 \, \eta t \, \mu1 \, \mu2 + 216 \, \mathfrak{e}p \, \mu1 \, \mu2 - 216 \, \eta t \, \mathfrak{e}p \, \mu1 \, \mu2 + \\
& \eta^2 \, (60 + 100 \, \mu1 - 56 \, \mu1^2 - 25 \, \mu2 - 49 \, \mu1 \, \mu2 - 24 \, \mathfrak{e}p \\
& (-37 + 9 \, \mu1 + 19 \, \mu1^2 - 3 \, \mu2 - 75 \, \mu1 \, \mu2) + \eta t \, (-60 - 100 \, \mu1 + 56 \, \mu1^2 + \\
& 25 \, \mu2 + 49 \, \mu1 \, \mu2 + 12 \, \mathfrak{e}p \, (-83 + 29 \, \mu1^2 - 6 \, \mu2 - 150 \, \mu1 \, \mu2))) \Big) - \\
& 5 \, \mathfrak{e}p \, \mathfrak{e}1 + 5 \, \eta t \, \mathfrak{e}p \, \mathfrak{e}1 - 11 \, \mathfrak{e}p \, \mu1 \, \mathfrak{e}1 + 11 \, \eta t \, \mathfrak{e}p \, \mu1 \, \mathfrak{e}1 - 5 \, \mathfrak{e}p \, \mu2 \, \mathfrak{e}1 + \\
& 5 \, \eta t \, \mathfrak{e}p \, \mu2 \, \mathfrak{e}1 - 5 \, \mathfrak{e}p \, \mu1 \, \mu2 \, \mathfrak{e}1 + 5 \, \eta t \, \mathfrak{e}p \, \mu1 \, \mu2 \, \mathfrak{e}1 + 5 \, \mathfrak{e}p \, \mathfrak{e}2 - \\
& 5 \, \eta t \, \mathfrak{e}p \, \mathfrak{e}2 + 11 \, \mathfrak{e}p \, \mu1 \, \mathfrak{e}2 - 11 \, \eta t \, \mathfrak{e}p \, \mu1 \, \mathfrak{e}2 + 5 \, \mathfrak{e}p \, \mu2 \, \mathfrak{e}2 - \\
& 5 \, \eta t \, \mathfrak{e}p \, \mu2 \, \mathfrak{e}2 + 5 \, \mathfrak{e}p \, \mu1 \, \mu2 \, \mathfrak{e}2 - 5 \, \eta t \, \mathfrak{e}p \, \mu1 \, \mu2 \, \mathfrak{e}2 + \\
& \eta^3 \, (60 + 156 \, \mu1 - 36 \, \mu1^2 + 15 \, \mu2 - 57 \, \mu1 \, \mu2 + \mathfrak{e}p \, (776 + 464 \, \mu1^2 + \\
& 30 \, \mathfrak{e}1 + \mu1 \, (-56 + 66 \, \mathfrak{e}1 + 10 \, \mu2 \, (44 + 3 \, \mathfrak{e}1 - 3 \, \mathfrak{e}2) - 66 \, \mathfrak{e}2) + \\
& \mu2 \, (56 + 30 \, \mathfrak{e}1 - 30 \, \mathfrak{e}2) - 30 \, \mathfrak{e}2) + \\
& \eta t \, (3 \times (12 \, \mu1^2 - 5 \times (4 + \mu2) + \mu1 \, (-52 + 19 \, \mu2)) + \\
& 2 \, \mathfrak{e}p \, (124 \, \mu1^2 - 5 \times (40 + 3 \, \mathfrak{e}1 - 3 \, \mathfrak{e}2) + \mu2 \, (-28 - 15 \, \mathfrak{e}1 + 15 \, \mathfrak{e}2) + \\
& \mu1 \, (68 - 33 \, \mathfrak{e}1 - 5 \, \mu2 \, (44 + 3 \, \mathfrak{e}1 - 3 \, \mathfrak{e}2) + 33 \, \mathfrak{e}2))) \Big) - \\
& \eta \, (80 + 188 \, \mu1 - 84 \, \mu1^2 + 15 \, \mu2 - 57 \, \mu1 \, \mu2 + \mathfrak{e}p \, (-452 + 416 \, \mu1^2 + \\
& 25 \, \mathfrak{e}1 + \mu1 \, (36 + 55 \, \mathfrak{e}1 + \mu2 \, (-1412 + 25 \, \mathfrak{e}1 - 25 \, \mathfrak{e}2) - 55 \, \mathfrak{e}2) + \\
& 5 \, \mu2 \, (-4 + 5 \, \mathfrak{e}1 - 5 \, \mathfrak{e}2) - 25 \, \mathfrak{e}2) + \\
& \eta t \, (-80 - 188 \, \mu1 + 84 \, \mu1^2 - 15 \, \mu2 + 57 \, \mu1 \, \mu2 + \mathfrak{e}p \\
& (868 + 384 \, \mu1^2 - 25 \, \mathfrak{e}1 - 5 \, \mu2 \, (-4 + 5 \, \mathfrak{e}1 - 5 \, \mathfrak{e}2) + 25 \, \mathfrak{e}2 + \\
& \mu1 \, (28 - 55 \, \mathfrak{e}1 + 55 \, \mathfrak{e}2 + \mu2 \, (1412 - 25 \, \mathfrak{e}1 + 25 \, \mathfrak{e}2)))) \Big) - \\
& \times (-1 + \eta) \times (4 \, w^2 \, (3 - 5 \, w + 2 \, w^2) \, \eta^{10} \, \mathfrak{e}p \, (1 + \mu1) - (1 + w)^3 \, (-5 \, w \, \mathfrak{e}l \\
& (1 + \mu1) \, \mu2 + 5 \, w \, \eta t \, \mathfrak{e}l \, (1 + \mu1) \, \mu2 + \eta t \, \mathfrak{e}p \\
& (10 + 8 \, \mu1 - 2 \, \mu1^2 + 2 \, w \, (5 - 7 \, \mu1^2 + 2 \, \mathfrak{e}l \, (5 - 2 \, \mu1 + 11 \, \mu1^2) - \\
& 5 \, \mu1 \, (-2 + \mu2) - 5 \, \mu2) + 5 \, \mu2 - 19 \, \mu1 \, \mu2)) - \\
& 4 \, w \, \eta^9 \, \mathfrak{e}p \, (9 \times (1 + \mu1) + w^3 \, (9 + \mu1 - 8 \, \mu1^2 + 2 \, \eta t \, (1 + \mu1) + 9 \, \mu1 \, \mu2) + \\
& w \, (-8 - 12 \, \mu1^2 + 3 \, \eta t \, (1 + \mu1) + 5 \, \mu1 \, (-4 + 3 \, \mu2)) - w^2 \\
& (11 - 20 \, \mu1^2 + 5 \, \eta t \, (1 + \mu1) + 3 \, \mu1 \, (-3 + 8 \, \mu2))) \Big) +
\end{aligned}$$

$$\begin{aligned}
& 2 \eta^8 \vartheta p \left( 12 \times (1 + \mu_1) + 2 w \left( 2 - 27 \mu_1^2 + 9 \eta t (1 + \mu_1) + \mu_1 (-43 + 45 \mu_2) \right) + \right. \\
& \quad w^4 \left( 41 - 34 \mu_1 - 75 \mu_1^2 + 8 \vartheta l \left( 4 + 2 \mu_1 + 7 \mu_1^2 \right) + \right. \\
& \quad \quad \left. 33 \mu_2 + 75 \mu_1 \mu_2 + 18 \eta t (1 + \mu_1 + \mu_1 \mu_2) \right) + w^2 \\
& \quad \left( -39 + 50 \mu_1 + 29 \mu_1^2 + 12 \vartheta l \left( 4 + 2 \mu_1 + 7 \mu_1^2 \right) + 55 \mu_2 - \right. \\
& \quad \quad \left. 83 \mu_1 \mu_2 + 2 \eta t (-8 + \mu_1 (-8 + 15 \mu_2)) \right) - 2 \\
& \quad w^3 \left( 12 - 30 \mu_1 - 54 \mu_1^2 + 10 \vartheta l \left( 4 + 2 \mu_1 + 7 \mu_1^2 \right) + 44 \mu_2 + \right. \\
& \quad \quad \left. 47 \mu_1 \mu_2 + \eta t (11 + \mu_1 (11 + 24 \mu_2)) \right) \left. \right) - \\
& \eta^2 \left( 4 (1 + w)^2 (-1 - 2 w + 2 w^2) \times (-1 + \eta t) \vartheta l^2 (5 - 2 \mu_1 + 11 \mu_1^2) + \right. \\
& \quad \vartheta p \left( 2 w^4 (43 + 58 \mu_1 + 15 \mu_1^2 + 99 \mu_2 + 93 \mu_1 \mu_2 + \right. \\
& \quad \quad \left. 3 \eta t (3 + 8 \mu_1 + 29 \mu_1^2 - 15 \mu_2 + 3 \mu_1 \mu_2) \right) + \\
& \quad \left. 2 w (-2 \times (24 + 51 \mu_1 + 9 \mu_1^2 + 46 \mu_2 + 4 \mu_1 \mu_2) + \right. \\
& \quad \quad \left. \eta t (-138 - 146 \mu_1 + 10 \mu_1^2 - 39 \mu_2 + 105 \mu_1 \mu_2) \right) + \\
& \quad w^3 \left( 4 \times (52 + 59 \mu_1 - 5 \mu_1^2 + 66 \mu_2 + 90 \mu_1 \mu_2) + \right. \\
& \quad \quad \left. \eta t (-152 - 428 \mu_1 + 456 \mu_1^2 - 213 \mu_2 + 219 \mu_1 \mu_2) \right) + \\
& \quad w^2 \left( 54 - 96 \mu_1 - 102 \mu_1^2 - 98 \mu_2 + 274 \mu_1 \mu_2 + \eta t (-392 - 796 \mu_1 + \right. \\
& \quad \quad \left. 340 \mu_1^2 - 193 \mu_2 + 395 \mu_1 \mu_2) \right) - 2 \times (30 + 24 \mu_1 - 6 \mu_1^2 + 14 \mu_2 + \\
& \quad \quad \left. 38 \mu_1 \mu_2 + \eta t (25 + 19 \mu_1^2 + 4 \mu_2 - 8 \mu_1 (2 + \mu_2)) \right) \left. \right) + \vartheta l \\
& \left( 20 - 20 \eta t - 70 \vartheta p + 150 \eta t \vartheta p + 24 \mu_1 - 24 \eta t \mu_1 - 90 \vartheta p \mu_1 + \right. \\
& \quad 58 \eta t \vartheta p \mu_1 + 16 \mu_1^2 - 16 \eta t \mu_1^2 + 16 \vartheta p \mu_1^2 + \\
& \quad 160 \eta t \vartheta p \mu_1^2 + 5 \mu_2 - 5 \eta t \mu_2 - 42 \vartheta p \mu_2 + 42 \eta t \vartheta p \mu_2 - \\
& \quad 19 \mu_1 \mu_2 + 19 \eta t \mu_1 \mu_2 - 42 \vartheta p \mu_1 \mu_2 + 42 \eta t \vartheta p \mu_1 \mu_2 - \\
& \quad w^4 \left( 40 + 80 \mu_1 + 64 \mu_1^2 + 8 \vartheta p (-1 + 14 \mu_1^2 + \mu_1 (4 - 18 \mu_2)) + \right. \\
& \quad \quad \left. 5 \mu_2 + 5 \mu_1 \mu_2 + \eta t (-64 \mu_1^2 - 5 \times (8 + \mu_2) - 5 \mu_1 (16 + \mu_2) + \right. \\
& \quad \quad \left. 4 \vartheta p (53 + 77 \mu_1^2 + 2 \mu_1 (-7 + 18 \mu_2)) \right) \left. \right) + 20 \vartheta p \mathfrak{z}1 - \\
& \quad 20 \eta t \vartheta p \mathfrak{z}1 + 41 \vartheta p \mu_1 \mathfrak{z}1 - 41 \eta t \vartheta p \mu_1 \mathfrak{z}1 + 3 \vartheta p \mu_1^2 \mathfrak{z}1 - \\
& \quad 3 \eta t \vartheta p \mu_1^2 \mathfrak{z}1 + 20 \vartheta p \mu_2 \mathfrak{z}1 - 20 \eta t \vartheta p \mu_2 \mathfrak{z}1 + 20 \vartheta p \mu_1 \mu_2 \mathfrak{z}1 - \\
& \quad 20 \eta t \vartheta p \mu_1 \mu_2 \mathfrak{z}1 - 20 \vartheta p \mathfrak{z}2 + 20 \eta t \vartheta p \mathfrak{z}2 - 33 \vartheta p \mu_1 \mathfrak{z}2 + \\
& \quad 33 \eta t \vartheta p \mu_1 \mathfrak{z}2 + 5 \vartheta p \mu_1^2 \mathfrak{z}2 - 5 \eta t \vartheta p \mu_1^2 \mathfrak{z}2 - 20 \vartheta p \mu_2 \mathfrak{z}2 + \\
& \quad 20 \eta t \vartheta p \mu_2 \mathfrak{z}2 - 8 \vartheta p \mu_1 \mu_2 \mathfrak{z}2 + 8 \eta t \vartheta p \mu_1 \mu_2 \mathfrak{z}2 + \\
& \quad w^2 \left( -2 \vartheta p (151 + 9 \mu_2) - 3 \times (20 + 8 \mu_1 + 16 \mu_1^2 - 5 \mu_2 - 29 \mu_1 \mu_2) + \right. \\
& \quad \quad \left. 3 \eta t (20 + 8 \mu_1 + 16 \mu_1^2 - 5 \mu_2 - 29 \mu_1 \mu_2) + \vartheta p \mu_1^2 \right. \\
& \quad \quad \left. (296 + 9 \mathfrak{z}1 + 3 \mathfrak{z}2) - 3 \vartheta p \mu_1 (-34 - 9 \mathfrak{z}1 + 5 \mathfrak{z}2 + 6 \mu_2 (49 + 2 \mathfrak{z}2)) + \right. \\
& \quad \quad \left. \eta t \vartheta p (2 \times (67 + 9 \mu_2) - \mu_1^2 (752 + 9 \mathfrak{z}1 + 3 \mathfrak{z}2) + \right. \\
& \quad \quad \left. 3 \mu_1 (46 - 9 \mathfrak{z}1 + 5 \mathfrak{z}2 + 6 \mu_2 (49 + 2 \mathfrak{z}2)) \right) \left. \right) + \\
& \quad w^3 \left( -100 - 144 \mu_1 - 128 \mu_1^2 + 5 \mu_2 + 53 \mu_1 \mu_2 + 2 \vartheta p \right. \\
& \quad \quad \left( -62 + 26 \mu_1^2 - 5 \mathfrak{z}1 + 5 \mathfrak{z}2 + \mu_2 (-8 - 5 \mathfrak{z}1 + 5 \mathfrak{z}2) + \right. \\
& \quad \quad \left. \mu_1 (36 - 11 \mathfrak{z}1 + 11 \mathfrak{z}2 + \mu_2 (-68 - 5 \mathfrak{z}1 + 5 \mathfrak{z}2)) \right) + \\
& \quad \eta t \left( 100 + 144 \mu_1 + 128 \mu_1^2 - 5 \mu_2 - 53 \mu_1 \mu_2 - 2 \vartheta p (152 + 504 \mu_1^2 - \right. \\
& \quad \quad \left. 5 \mathfrak{z}1 - \mu_1 (64 + 11 \mathfrak{z}1 + \mu_2 (68 + 5 \mathfrak{z}1 - 5 \mathfrak{z}2) - 11 \mathfrak{z}2) + 5 \mathfrak{z}2 + \right. \\
& \quad \quad \left. \mu_2 (-8 - 5 \mathfrak{z}1 + 5 \mathfrak{z}2)) \right) \left. \right) - 2 w (-10 - 32 \mu_1 - 16 \mu_1^2 - \\
& \quad 5 \mu_2 - 5 \mu_1 \mu_2 + \eta t (10 + 32 \mu_1 + 16 \mu_1^2 + 5 \mu_2 + 5 \mu_1 \mu_2 + \\
& \quad \quad \vartheta p (\mu_1 \mu_2 (-302 + 15 \mathfrak{z}1 - 27 \mathfrak{z}2) + \mu_2 (-26 + 15 \mathfrak{z}1 - 15 \mathfrak{z}2) + \\
& \quad \quad 5 \mu_1 (-16 + 9 \mathfrak{z}1 - 7 \mathfrak{z}2) + 5 \times (-40 + 3 \mathfrak{z}1 - 3 \mathfrak{z}2) +
\end{aligned}$$

$$\begin{aligned}
& \mu_1^2 (-48 + 6 \mathfrak{z}_1 + 4 \mathfrak{z}_2)) + \Theta p (-2 \mu_1^2 (40 + 3 \mathfrak{z}_1 + 2 \mathfrak{z}_2) + \\
& 3 \times (44 - 5 \mathfrak{z}_1 + 5 \mathfrak{z}_2) + \mu_2 (26 - 15 \mathfrak{z}_1 + 15 \mathfrak{z}_2) + \\
& \mu_1 (64 - 45 \mathfrak{z}_1 + 35 \mathfrak{z}_2 + \mu_2 (302 - 15 \mathfrak{z}_1 + 27 \mathfrak{z}_2))) + \\
& \eta^7 (-4 \Theta p (8 - 15 \mu_1^2 + 6 \eta t (1 + \mu_1) + 5 \mu_1 (-5 + 6 \mu_2)) + w^4 \\
& (4 \times (-1 + \eta t) \Theta l^2 (5 - 2 \mu_1 + 11 \mu_1^2) + \\
& 2 \Theta p (2 \times (-41 + 60 \mu_1^2 + \mu_1 (19 - 31 \mu_2) - 88 \mu_2) + \\
& \eta t (-36 + 32 \mu_1^2 + 5 \mu_2 - \mu_1 (46 + 91 \mu_2))) + \\
& \Theta l (10 + 20 \mu_1 - 14 \mu_1^2 - 8 \Theta p (10 + 49 \mu_1^2 + \mu_1 (14 - 36 \mu_2)) - \\
& 5 \mu_2 - 5 \mu_1 \mu_2 + \eta t (14 \mu_1^2 + 5 \mu_1 (-4 + \mu_2) + 5 \times (-2 + \mu_2) + \\
& 12 \Theta p (-7 + 11 \mu_1^2 - 2 \mu_1 (1 + 12 \mu_2)))) + w \\
& (-4 \times (-1 + \eta t) \Theta l \mu_1 (1 + \mu_1) + \Theta p (44 + 84 \mu_1 + 64 \mu_1^2 - 216 \mu_2 - \\
& 84 \mu_1 \mu_2 - \Theta l (2 \times (96 + 5 \mu_2) + \mu_1^2 (334 + 5 \mathfrak{z}_1 + 5 \mathfrak{z}_2) + \\
& \mu_1 (166 - 50 \mu_2 + 5 \mathfrak{z}_1 + 5 \mathfrak{z}_2)) + \eta t (-8 + 10 \Theta l \mu_2 + \\
& \mu_1 (-24 \times (1 + 5 \mu_2) + 5 \Theta l (14 - 10 \mu_2 + \mathfrak{z}_1 + \mathfrak{z}_2)) + \\
& \mu_1^2 (-16 + \Theta l (-2 + 5 \mathfrak{z}_1 + 5 \mathfrak{z}_2)))) + w^3 \\
& (-4 \times (-1 + \eta t) \Theta l^2 (5 - 2 \mu_1 + 11 \mu_1^2) + \Theta p (88 + 544 \mu_2 - \\
& 4 \mu_1 (-64 + 65 \mu_2) + \eta t (28 - 84 \mu_1^2 + 27 \mu_2 + \mu_1 (112 + 219 \mu_2))) + \\
& \Theta l (-20 - 52 \mu_1 + 4 \mu_1^2 - 5 \mu_2 + 19 \mu_1 \mu_2 + 4 \Theta p \\
& (-1 + 111 \mu_1^2 - 5 \mathfrak{z}_1 + 5 \mathfrak{z}_2 + \mu_2 (-6 - 5 \mathfrak{z}_1 + 5 \mathfrak{z}_2) + \\
& \mu_1 (56 - 11 \mathfrak{z}_1 - 5 \mu_2 (12 + \mathfrak{z}_1 - \mathfrak{z}_2) + 11 \mathfrak{z}_2)) + \\
& \eta t (20 + 52 \mu_1 - 4 \mu_1^2 + 5 \mu_2 - 19 \mu_1 \mu_2 - 4 \Theta p \\
& (43 \mu_1^2 - 5 \times (9 + \mathfrak{z}_1 - \mathfrak{z}_2) + \mu_2 (-6 - 5 \mathfrak{z}_1 + 5 \mathfrak{z}_2) + \\
& \mu_1 (16 - 11 \mathfrak{z}_1 - 5 \mu_2 (12 + \mathfrak{z}_1 - \mathfrak{z}_2) + 11 \mathfrak{z}_2)))) + \\
& w^2 (4 \times (-1 + \eta t) \Theta l (-5 + \mu_1) \mu_1 + \Theta p (76 - 572 \mu_1 - 408 \mu_1^2 + \\
& 80 \mu_2 + 680 \mu_1 \mu_2 + \Theta l (338 + 50 \mu_2 + 5 \mu_1^2 (68 + 3 \mathfrak{z}_1 + \mathfrak{z}_2) - 5 \mu_1 \\
& (-18 - 9 \mathfrak{z}_1 + 5 \mathfrak{z}_2 + 2 \mu_2 (7 + 6 \mathfrak{z}_2))) + \eta t (16 \times (8 + 2 \mu_1^2 - \mu_2 + \\
& \mu_1 (4 + 5 \mu_2)) - \Theta l (146 + 50 \mu_2 + \mu_1^2 (4 + 15 \mathfrak{z}_1 + 5 \mathfrak{z}_2) - \\
& \mu_1 (6 + 70 \mu_2 - 45 \mathfrak{z}_1 + 25 \mathfrak{z}_2 + 60 \mu_2 \mathfrak{z}_2)))) + \\
& \eta (4 w (1 + w)^3 (-1 + \eta t) \Theta l^2 (5 - 2 \mu_1 + 11 \mu_1^2) + \Theta p (2 w^2 (46 + \\
& 58 \mu_1 + \eta t (-4 + 14 \mu_1^2 + 7 \mu_1 (-8 + \mu_2) - 53 \mu_2) + 50 \mu_2 + 14 \mu_1 \mu_2) + \\
& 2 \eta t (8 \mu_1^2 - 5 \times (4 + \mu_2) + \mu_1 (-24 + 19 \mu_2)) + \\
& w^4 (\eta t (36 + 76 \mu_1 - 20 \mu_1^2 - 50 \mu_2 - 26 \mu_1 \mu_2) + \\
& 4 \times (5 + 8 \mu_1 + 3 \mu_1^2 + 11 \mu_2 + 5 \mu_1 \mu_2)) + \\
& w^3 (\eta t (68 + 80 \mu_1 - 24 \mu_1^2 - 123 \mu_2 - 51 \mu_1 \mu_2) + \\
& 4 \times (20 + 31 \mu_1 + 5 \mu_1^2 + 30 \mu_2 + 6 \mu_1 \mu_2)) + w (-8 \times (1 + \mu_1) \times \\
& (-5 + \mu_1 - 3 \mu_2) + \eta t (-80 - 164 \mu_1 + 48 \mu_1^2 - 43 \mu_2 + 77 \mu_1 \mu_2))) + \\
& \Theta l (-10 + 10 \eta t + 20 \Theta p - 60 \eta t \Theta p - 8 \mu_1 + 8 \eta t \mu_1 + 16 \Theta p \mu_1 + \\
& 2 \mu_1^2 - 2 \eta t \mu_1^2 - 4 \Theta p \mu_1^2 - 84 \eta t \Theta p \mu_1^2 - 5 \mu_2 + 5 \eta t \mu_2 + \\
& 20 \Theta p \mu_2 - 20 \eta t \Theta p \mu_2 + 19 \mu_1 \mu_2 - 19 \eta t \mu_1 \mu_2 - 28 \Theta p \mu_1 \mu_2 + \\
& 28 \eta t \Theta p \mu_1 \mu_2 + w^4 (-8 \Theta p (-5 + 7 \mu_1^2 + \mu_1 (2 - 18 \mu_2)) - \\
& 5 \times (1 + \mu_1) \times (2 + 2 \mu_1 + 3 \mu_2) + 5 \eta t (1 + \mu_1) \times (2 + 2 \mu_1 + 3 \mu_2) + \\
& 4 \eta t \Theta p (-13 + 11 \mu_1^2 - 2 \mu_1 (1 + 18 \mu_2)) - 10 \Theta p \mathfrak{z}_1 + \\
& 10 \eta t \Theta p \mathfrak{z}_1 - 8 \Theta p \mu_1 \mathfrak{z}_1 + 8 \eta t \Theta p \mu_1 \mathfrak{z}_1 + 2 \Theta p \mu_1^2 \mathfrak{z}_1 -
\end{aligned}$$

$$\begin{aligned}
& 2 \eta t \operatorname{ep} \mu_1^2 \mathfrak{e}_1 - 10 \operatorname{ep} \mu_2 \mathfrak{e}_1 + 10 \eta t \operatorname{ep} \mu_2 \mathfrak{e}_1 - 10 \operatorname{ep} \mu_1 \mu_2 \mathfrak{e}_1 + \\
& 10 \eta t \operatorname{ep} \mu_1 \mu_2 \mathfrak{e}_1 + 10 \operatorname{ep} \mathfrak{e}_2 - 10 \eta t \operatorname{ep} \mathfrak{e}_2 + 8 \operatorname{ep} \mu_1 \mathfrak{e}_2 - \\
& 8 \eta t \operatorname{ep} \mu_1 \mathfrak{e}_2 - 2 \operatorname{ep} \mu_1^2 \mathfrak{e}_2 + 2 \eta t \operatorname{ep} \mu_1^2 \mathfrak{e}_2 + 10 \operatorname{ep} \mu_2 \mathfrak{e}_2 - \\
& 10 \eta t \operatorname{ep} \mu_2 \mathfrak{e}_2 - 14 \operatorname{ep} \mu_1 \mu_2 \mathfrak{e}_2 + 14 \eta t \operatorname{ep} \mu_1 \mu_2 \mathfrak{e}_2 - \\
& 2 w^2 \left( 3 \times \left( 4 \mu_1^2 - 7 \mu_1 (-2 + \mu_2) + 5 \times (2 + \mu_2) \right) - \operatorname{ep} \right. \\
& \quad \left( 74 - 15 \mathfrak{e}_1 + \mu_1^2 (-28 + \mathfrak{e}_1 - \mathfrak{e}_2) + 15 \mathfrak{e}_2 + \mu_2 (14 - 15 \mathfrak{e}_1 + 15 \mathfrak{e}_2) + \right. \\
& \quad \left. \mu_1 (58 - 26 \mathfrak{e}_1 + 26 \mathfrak{e}_2 + \mu_2 (182 - 15 \mathfrak{e}_1 + 3 \mathfrak{e}_2)) \right) + \\
& \quad \left. \eta t \left( -3 \times \left( 4 \mu_1^2 - 7 \mu_1 (-2 + \mu_2) + 5 \times (2 + \mu_2) \right) + \operatorname{ep} \left( \mu_1^2 (198 + \right. \right. \right. \\
& \quad \left. \left. \mathfrak{e}_1 - \mathfrak{e}_2) + 15 \times (12 - \mathfrak{e}_1 + \mathfrak{e}_2) + \mu_2 (14 - 15 \mathfrak{e}_1 + 15 \mathfrak{e}_2) + \right. \right. \\
& \quad \left. \left. \mu_1 (30 - 26 \mathfrak{e}_1 + 26 \mathfrak{e}_2 + \mu_2 (182 - 15 \mathfrak{e}_1 + 3 \mathfrak{e}_2)) \right) \right) \right) - \\
& w \left( 40 + 44 \mu_1 + 4 \mu_1^2 + 15 \mu_2 - 57 \mu_1 \mu_2 - 2 \operatorname{ep} \left( -3 \mu_2 (-8 + \right. \right. \\
& \quad \left. \left. 5 \mathfrak{e}_1 - 5 \mathfrak{e}_2) + 2 \mu_1^2 (-3 + \mathfrak{e}_1 - \mathfrak{e}_2) + 5 \times (8 - 3 \mathfrak{e}_1 + 3 \mathfrak{e}_2) + \right. \right. \\
& \quad \left. \left. \mu_1 (46 - 19 \mathfrak{e}_1 + 19 \mathfrak{e}_2 - 3 \mu_2 (-8 + 5 \mathfrak{e}_1 + 3 \mathfrak{e}_2)) \right) + \right. \\
& \quad \left. \eta t \left( -4 \mu_1^2 - 5 \times (8 + 3 \mu_2) + \mu_1 (-44 + 57 \mu_2) + 2 \operatorname{ep} \right. \right. \\
& \quad \left. \left( -3 (\mu_2 (-8 + 5 \mathfrak{e}_1 - 5 \mathfrak{e}_2) + 5 \times (-8 + \mathfrak{e}_1 - \mathfrak{e}_2)) + \right. \right. \\
& \quad \left. \left. 2 \mu_1^2 (85 + \mathfrak{e}_1 - \mathfrak{e}_2) + \mu_1 (14 - 19 \mathfrak{e}_1 + \right. \right. \\
& \quad \left. \left. 19 \mathfrak{e}_2 - 3 \mu_2 (-8 + 5 \mathfrak{e}_1 + 3 \mathfrak{e}_2)) \right) \right) \right) - \\
& w^3 \left( 40 + 68 \mu_1 + 28 \mu_1^2 + 35 \mu_2 + 11 \mu_1 \mu_2 + 2 \operatorname{ep} \left( 52 \mu_1^2 + 5 \times \right. \right. \\
& \quad \left. \left( 1 + \mu_2) \mathfrak{e}_1 + \mu_1 (-8 + 11 \mathfrak{e}_1 + \mu_2 (-216 + 5 \mathfrak{e}_1 - 5 \mathfrak{e}_2) - 11 \mathfrak{e}_2) - \right. \right. \\
& \quad \left. \left. 5 \times (12 + \mathfrak{e}_2 + \mu_2 \mathfrak{e}_2) \right) + \eta t \left( -40 - 68 \mu_1 - 28 \mu_1^2 - 35 \mu_2 - \right. \right. \\
& \quad \left. \left. 11 \mu_1 \mu_2 + 2 \operatorname{ep} \left( 112 + 48 \mu_1^2 - 5 \times (1 + \mu_2) \mathfrak{e}_1 + 5 \mathfrak{e}_2 + 5 \mu_2 \mathfrak{e}_2 + \right. \right. \right. \\
& \quad \left. \left. \mu_1 (16 - 11 \mathfrak{e}_1 + 11 \mathfrak{e}_2 + \mu_2 (216 - 5 \mathfrak{e}_1 + 5 \mathfrak{e}_2)) \right) \right) \right) \right) + \\
& \eta^4 \left( 4 \times \left( 1 - 4 w - 6 w^2 + 4 w^3 + 4 w^4 \right) \times (-1 + \eta t) \operatorname{el}^2 \left( 5 - 2 \mu_1 + 11 \mu_1^2 \right) + \right. \\
& \quad \operatorname{ep} \left( \eta t \left( -68 - 16 \mu_1 + 28 \mu_1^2 + 5 \mu_2 - 79 \mu_1 \mu_2 \right) + \right. \\
& \quad \left. 2 \times \left( -61 - 26 \mu_1 + 23 \mu_1^2 - 85 \mu_2 - 43 \mu_1 \mu_2 \right) + \right. \\
& \quad w^3 \left( 4 \times \left( 134 + 234 \mu_1 + 40 \mu_1^2 + 320 \mu_2 - 319 \mu_1 \mu_2 \right) - \right. \\
& \quad \left. 15 \eta t \left( -20 - 40 \mu_1 + 60 \mu_1^2 + 11 \mu_2 - 29 \mu_1 \mu_2 \right) \right) - \\
& \quad 2 w^4 \left( -23 - 122 \mu_1 - 99 \mu_1^2 - 55 \mu_2 + 587 \mu_1 \mu_2 + \right. \\
& \quad \left. \eta t \left( -99 - 224 \mu_1 + 535 \mu_1^2 + 25 \mu_2 - 5 \mu_1 \mu_2 \right) \right) + \\
& \quad w \left( -4 \times \left( 21 + 137 \mu_1 + 50 \mu_1^2 + 132 \mu_2 - 186 \mu_1 \mu_2 \right) + \right. \\
& \quad \left. \eta t \left( -248 - 532 \mu_1 + 448 \mu_1^2 - 89 \mu_2 + 55 \mu_1 \mu_2 \right) \right) + \\
& \quad w^2 \left( 6 \times \left( 65 - 6 \mu_1 - 59 \mu_1^2 + 103 \mu_2 + 141 \mu_1 \mu_2 \right) + \right. \\
& \quad \left. \eta t \left( -108 - 588 \mu_1 + 552 \mu_1^2 - 223 \mu_2 + 605 \mu_1 \mu_2 \right) \right) \right) + \operatorname{el} \\
& \left( 20 - 20 \eta t + 178 \operatorname{ep} - 194 \eta t \operatorname{ep} + 36 \mu_1 - 36 \eta t \mu_1 - 176 \operatorname{ep} \mu_1 + \right. \\
& \quad 96 \eta t \operatorname{ep} \mu_1 + 4 \mu_1^2 - 4 \eta t \mu_1^2 - 102 \operatorname{ep} \mu_1^2 + 110 \eta t \operatorname{ep} \mu_1^2 + 5 \mu_2 - \\
& \quad 5 \eta t \mu_2 - 12 \operatorname{ep} \mu_2 + 12 \eta t \operatorname{ep} \mu_2 - 19 \mu_1 \mu_2 + 19 \eta t \mu_1 \mu_2 + 384 \operatorname{ep} \mu_1 \mu_2 - \\
& \quad 384 \eta t \operatorname{ep} \mu_1 \mu_2 + w^4 \left( -5 \times (-1 + \eta t) \times \left( 48 \mu_1^2 - 5 \mu_2 - 5 \mu_1 \mu_2 \right) + \right. \\
& \quad \left. 4 \operatorname{ep} \left( 4 \times \left( 7 - 35 \mu_1^2 + 2 \mu_1 (-5 + 27 \mu_2) \right) + \right. \right. \\
& \quad \left. \left. \eta t \left( -83 + 55 \mu_1^2 - 2 \mu_1 (5 + 108 \mu_2) \right) \right) \right) + 20 \operatorname{ep} \mathfrak{e}_1 - \\
& \quad 20 \eta t \operatorname{ep} \mathfrak{e}_1 + 36 \operatorname{ep} \mu_1 \mathfrak{e}_1 - 36 \eta t \operatorname{ep} \mu_1 \mathfrak{e}_1 - 2 \operatorname{ep} \mu_1^2 \mathfrak{e}_1 + \\
& \quad 2 \eta t \operatorname{ep} \mu_1^2 \mathfrak{e}_1 + 20 \operatorname{ep} \mu_2 \mathfrak{e}_1 - 20 \eta t \operatorname{ep} \mu_2 \mathfrak{e}_1 + 20 \operatorname{ep} \mu_1 \mu_2 \mathfrak{e}_1 - \\
& \quad 20 \eta t \operatorname{ep} \mu_1 \mu_2 \mathfrak{e}_1 - 20 \operatorname{ep} \mathfrak{e}_2 + 20 \eta t \operatorname{ep} \mathfrak{e}_2 - 38 \operatorname{ep} \mu_1 \mathfrak{e}_2 + 38 \eta t \operatorname{ep} \mu_1 \mathfrak{e}_2 - \\
& \quad 20 \operatorname{ep} \mu_2 \mathfrak{e}_2 + 20 \eta t \operatorname{ep} \mu_2 \mathfrak{e}_2 - 8 \operatorname{ep} \mu_1 \mu_2 \mathfrak{e}_2 + 8 \eta t \operatorname{ep} \mu_1 \mu_2 \mathfrak{e}_2 + \\
& \quad w \left( 20 + 128 \mu_1 - 48 \mu_1^2 + 5 \mu_2 + 5 \mu_1 \mu_2 + 2 \operatorname{ep} \left( 42 + 8 \mu_2 + 15 \mathfrak{e}_1 + 15 \mu_2 \right. \right.
\end{aligned}$$



$$\begin{aligned}
& \mathfrak{z}1 + \mu1 (-120 + 87 \mathfrak{z}1 + \mu2 (-292 + 15 \mathfrak{z}1 - 87 \mathfrak{z}2) - 63 \mathfrak{z}2) - \\
& 15 \mathfrak{z}2 - 15 \mu2 \mathfrak{z}2 + 6 \mu1^2 (31 + 3 \mathfrak{z}1 + \mathfrak{z}2)) - \eta t (20 + 128 \mu1 - \\
& 48 \mu1^2 + 5 \mu2 + 5 \mu1 \mu2 + 2 \theta p (-84 + 8 \mu2 + 15 \mathfrak{z}1 + 15 \mu2 \mathfrak{z}1 + \\
& \mu1 (-156 + 87 \mathfrak{z}1 + \mu2 (-292 + 15 \mathfrak{z}1 - 87 \mathfrak{z}2) - 63 \mathfrak{z}2) - \\
& 15 \mathfrak{z}2 - 15 \mu2 \mathfrak{z}2 + 6 \mu1^2 (-8 + 3 \mathfrak{z}1 + \mathfrak{z}2))) + \\
& w^2 (-120 - 152 \mu1 - 80 \mu1^2 - 15 \mu2 + 129 \mu1 \mu2 + 2 \theta p \\
& (-6 \times (29 + 5 \mathfrak{z}1 + \mu2 (-3 + 5 \mathfrak{z}1 - 5 \mathfrak{z}2) - 5 \mathfrak{z}2) + \mu1^2 (480 + 17 \mathfrak{z}1 + \\
& 3 \mathfrak{z}2) - \mu1 (-282 + 7 \mathfrak{z}1 - 27 \mathfrak{z}2 + 6 \mu2 (153 + 5 \mathfrak{z}1 + 9 \mathfrak{z}2))) + \\
& \eta t (80 \mu1^2 + \mu1 (152 - 129 \mu2) + 15 \times (8 + \mu2) - 2 \theta p (-208 - 30 \mathfrak{z}1 - \\
& 6 \mu2 (-3 + 5 \mathfrak{z}1 - 5 \mathfrak{z}2) + 30 \mathfrak{z}2 + \mu1^2 (542 + 17 \mathfrak{z}1 + 3 \mathfrak{z}2) - \\
& \mu1 (-22 + 7 \mathfrak{z}1 - 27 \mathfrak{z}2 + 6 \mu2 (153 + 5 \mathfrak{z}1 + 9 \mathfrak{z}2)))) - \\
& w^3 (120 + 288 \mu1 - 192 \mu1^2 + 35 \mu2 - 61 \mu1 \mu2 + 4 \theta p (62 + \\
& 40 \mu1^2 + 15 \mathfrak{z}1 + 3 \mu1 (-20 + 11 \mathfrak{z}1 + \mu2 (-32 + 5 \mathfrak{z}1 - 5 \mathfrak{z}2) - \\
& 11 \mathfrak{z}2) + 3 \mu2 (4 + 5 \mathfrak{z}1 - 5 \mathfrak{z}2) - 15 \mathfrak{z}2) + \\
& \eta t (-120 - 288 \mu1 + 192 \mu1^2 - 35 \mu2 + 61 \mu1 \mu2 + 4 \theta p \\
& (67 + 233 \mu1^2 - 15 \mathfrak{z}1 - 3 \mu2 (4 + 5 \mathfrak{z}1 - 5 \mathfrak{z}2) + 15 \mathfrak{z}2 + \\
& \mu1 (30 - 33 \mathfrak{z}1 + 33 \mathfrak{z}2 + \mu2 (96 - 15 \mathfrak{z}1 + 15 \mathfrak{z}2)))))) + \\
& \eta^5 (w^4 (-4 \times (-1 + \eta t) \theta l^2 (5 - 2 \mu1 + 11 \mu1^2) - 4 \theta p (62 + 45 \mu1^2 + \\
& \mu1 (107 - 270 \mu2) + 165 \mu2) + \\
& 6 \eta t \theta p (146 \mu1^2 + 15 \times (-2 + \mu2) - 5 \mu1 (14 + 9 \mu2)) + \\
& \theta l (-5 \times (-10 + 38 \mu1^2 + \mu1 (-20 + \mu2) + \mu2) + 8 \theta p (29 + 35 \mu1^2 + \\
& 2 \mu1 (5 + 9 \mu2)) + \eta t (5 \times (-10 + 38 \mu1^2 + \mu1 (-20 + \mu2) + \mu2) + \\
& 4 \theta p (37 + 121 \mu1^2 - 2 \mu1 (11 + 18 \mu2)))) + w^3 \\
& (20 \times (-1 + \eta t) \theta l^2 (5 - 2 \mu1 + 11 \mu1^2) + \theta p (-500 + 4 \times (85 + 24 \eta t) \mu1^2 + \\
& 5 \times (-200 + 51 \eta t) \mu2 + \mu1 (-280 + 228 \eta t + 80 \mu2 - 729 \eta t \mu2)) + \\
& \theta l (80 + 132 \mu1 - 68 \mu1^2 - 25 \mu2 - 49 \mu1 \mu2 + \eta t (-80 - 132 \mu1 + \\
& 68 \mu1^2 + 25 \mu2 + 49 \mu1 \mu2 + 2 \theta p (-212 + 468 \mu1^2 + 5 \mathfrak{z}1 + \\
& \mu1 (-104 + 11 \mathfrak{z}1 + \mu2 (-784 + 5 \mathfrak{z}1 - 5 \mathfrak{z}2) - 11 \mathfrak{z}2) + \\
& \mu2 (-16 + 5 \mathfrak{z}1 - 5 \mathfrak{z}2) - 5 \mathfrak{z}2)) - 2 \theta p (-144 + 488 \mu1^2 + \\
& 5 \mathfrak{z}1 + \mu1 (128 + 11 \mathfrak{z}1 + \mu2 (-784 + 5 \mathfrak{z}1 - 5 \mathfrak{z}2) - 11 \mathfrak{z}2) + \\
& \mu2 (-16 + 5 \mathfrak{z}1 - 5 \mathfrak{z}2) - 5 \mathfrak{z}2))) - 2 \times \\
& (12 \times (-1 + \eta t) \theta l \mu1 + \theta p (-34 + 78 \mu1 + 52 \mu1^2 + 30 \mu2 - \\
& 90 \mu1 \mu2 - \theta l (97 + 14 \mu2 + \mu1^2 (75 + 7 \mathfrak{z}1 + 2 \mathfrak{z}2) + \\
& \mu1 (-14 + 20 \mu2 + 22 \mathfrak{z}1 - 13 \mathfrak{z}2 - 30 \mu2 \mathfrak{z}2)) + \eta t \\
& (-4 \times (5 + \mu1 (-7 + \mu2) - 2 \mu2) + \theta l (65 + 14 \mu2 + \mu1^2 (19 + 7 \mathfrak{z}1 + \\
& 2 \mathfrak{z}2) + \mu1 (-30 + 20 \mu2 + 22 \mathfrak{z}1 - 13 \mathfrak{z}2 - 30 \mu2 \mathfrak{z}2)))))) + \\
& 2 w^2 (6 \times (-1 + \eta t) \theta l^2 (5 - 2 \mu1 + 11 \mu1^2) + \theta p (90 + 232 \mu1^2 + \\
& \mu1 (526 - 632 \mu2) + 394 \mu2 + \\
& \eta t (150 - 298 \mu1^2 + \mu1 (362 - 41 \mu2) + 91 \mu2)) + \\
& \theta l (3 \times (8 \mu1^2 - 5 \times (2 + \mu2) + \mu1 (-30 + 7 \mu2)) - \theta p (184 + \\
& 45 \times (1 + \mu2) \mathfrak{z}1 + \mu1 (-124 + 105 \mathfrak{z}1 + 9 \mu2 (-24 + 5 \mathfrak{z}1 - 5 \mathfrak{z}2) - \\
& 93 \mathfrak{z}2) - 45 \mathfrak{z}2 - 45 \mu2 \mathfrak{z}2 + \mu1^2 (268 + 6 \mathfrak{z}1 + 6 \mathfrak{z}2)) + \\
& \eta t (3 \times (-8 \mu1^2 + \mu1 (30 - 7 \mu2) + 5 \times (2 + \mu2)) + \theta p
\end{aligned}$$

$$\begin{aligned}
& \left( \mu_1 (-160 + 105 \mathfrak{z}_1 + 9 \mu_2 (-24 + 5 \mathfrak{z}_1 - 5 \mathfrak{z}_2) - 93 \mathfrak{z}_2) + \right. \\
& \quad 2 \mu_1^2 (-91 + 3 \mathfrak{z}_1 + 3 \mathfrak{z}_2) + \\
& \quad \left. 5 \times (-10 + 9 \times (1 + \mu_2) \mathfrak{z}_1 - 9 \times (1 + \mu_2) \mathfrak{z}_2) \right) + w \\
& \left( -12 \times (-1 + \eta t) \vartheta l^2 (5 - 2 \mu_1 + 11 \mu_1^2) + \vartheta p (4 \times (70 - 45 \right. \\
& \quad \mu_1^2 + 146 \mu_2 + 5 \mu_1 (5 + 7 \mu_2)) + \\
& \quad \eta t (204 - 100 \mu_1^2 - 15 \mu_2 + \mu_1 (32 + 273 \mu_2)) \right) + \vartheta l \\
& \left( -60 - 76 \mu_1 - 4 \mu_1^2 - 15 \mu_2 + 57 \mu_1 \mu_2 + 2 \vartheta p (-10 \times (5 + 3 \mathfrak{z}_1 - 3 \mathfrak{z}_2) + \right. \\
& \quad \mu_1^2 (290 + 13 \mathfrak{z}_1 + \mathfrak{z}_2) + \mu_2 (34 - 30 \mathfrak{z}_1 + 30 \mathfrak{z}_2) - \\
& \quad \mu_1 (-216 + 17 \mathfrak{z}_1 - 31 \mathfrak{z}_2 + \mu_2 (494 + 30 \mathfrak{z}_1 + 42 \mathfrak{z}_2)) \right) + \\
& \quad \eta t (60 + 76 \mu_1 + 4 \mu_1^2 + 15 \mu_2 - 57 \mu_1 \mu_2 - 2 \vartheta p (-122 - 30 \mathfrak{z}_1 + \\
& \quad 30 \mathfrak{z}_2 + \mu_1^2 (218 + 13 \mathfrak{z}_1 + \mathfrak{z}_2) + \mu_2 (34 - 30 \mathfrak{z}_1 + 30 \mathfrak{z}_2) - \\
& \quad \mu_1 (-72 + 17 \mathfrak{z}_1 - 31 \mathfrak{z}_2 + \mu_2 (494 + 30 \mathfrak{z}_1 + 42 \mathfrak{z}_2))) \right) - \\
& \eta^3 (4 \times (-2 - 2w + 6w^2 + 7w^3 + w^4) \times (-1 + \eta t) \vartheta l^2 (5 - 2 \mu_1 + 11 \mu_1^2) + \\
& \quad \vartheta p (-8 \times (-2 + 9 \mu_1 + 5 \mu_1^2 + 12 \mu_2 - 18 \mu_1 \mu_2) + \\
& \quad 2 \eta t (-22 - 80 \mu_1 + 50 \mu_1^2 - 9 \mu_2 + 15 \mu_1 \mu_2) + \\
& \quad w^3 (4 \times (8 + 80 \mu_1 + 54 \mu_1^2 + 76 \mu_2 - 287 \mu_1 \mu_2) + \\
& \quad \eta t (436 + 1016 \mu_1 - 1100 \mu_1^2 + 95 \mu_2 - 241 \mu_1 \mu_2)) - \\
& \quad 4w^2 (-95 - 169 \mu_1 - 26 \mu_1^2 - 218 \mu_2 + 58 \mu_1 \mu_2 + \\
& \quad \eta t (-102 - 142 \mu_1 + 38 \mu_1^2 - 7 \mu_2 + 5 \mu_1 \mu_2)) - \\
& \quad 2w^4 (54 + 34 \mu_1 - 20 \mu_1^2 + 132 \mu_2 + 330 \mu_1 \mu_2 + \\
& \quad \eta t (-48 - 98 \mu_1 + 340 \mu_1^2 - 25 \mu_2 + 47 \mu_1 \mu_2)) + \\
& \quad 2w (124 + 58 \mu_1 - 54 \mu_1^2 + 100 \mu_2 + 256 \mu_1 \mu_2 + \\
& \quad \eta t (18 - 166 \mu_1 + 182 \mu_1^2 - 21 \mu_2 + 75 \mu_1 \mu_2)) \right) + \vartheta l \\
& (-10 + 10 \eta t - 106 \vartheta p + 130 \eta t \vartheta p + 24 \mu_1 - 24 \eta t \mu_1 - 20 \vartheta p \mu_1 + \\
& \quad 68 \eta t \vartheta p \mu_1 - 14 \mu_1^2 + 14 \eta t \mu_1^2 + 98 \vartheta p \mu_1^2 - 74 \eta t \vartheta p \mu_1^2 - 5 \mu_2 + \\
& \quad 5 \eta t \mu_2 + 8 \vartheta p \mu_2 - 8 \eta t \vartheta p \mu_2 + 19 \mu_1 \mu_2 - 19 \eta t \mu_1 \mu_2 - 364 \vartheta p \mu_1 \mu_2 + \\
& \quad 364 \eta t \vartheta p \mu_1 \mu_2 + w^4 (-24 \vartheta p (-8 + 7 \mu_1^2 + \mu_1 (2 - 24 \mu_2)) + \\
& \quad 5 \times (34 \mu_1^2 - 5 \mu_1 (-4 + \mu_2) - 5 \times (-2 + \mu_2)) + \\
& \quad 5 \eta t (-34 \mu_1^2 + 5 \mu_1 (-4 + \mu_2) + 5 \times (-2 + \mu_2)) + \\
& \quad 12 \eta t \vartheta p (1 + 55 \mu_1^2 - 2 \mu_1 (5 + 24 \mu_2))) - 10 \vartheta p \mathfrak{z}_1 + \\
& \quad 10 \eta t \vartheta p \mathfrak{z}_1 + 36 \vartheta p \mu_1 \mathfrak{z}_1 - 36 \eta t \vartheta p \mu_1 \mathfrak{z}_1 + 16 \vartheta p \mu_1^2 \mathfrak{z}_1 - \\
& \quad 16 \eta t \vartheta p \mu_1^2 \mathfrak{z}_1 - 10 \vartheta p \mu_2 \mathfrak{z}_1 + 10 \eta t \vartheta p \mu_2 \mathfrak{z}_1 - 10 \vartheta p \mu_1 \mu_2 \mathfrak{z}_1 + \\
& \quad 10 \eta t \vartheta p \mu_1 \mu_2 \mathfrak{z}_1 + 10 \vartheta p \mathfrak{z}_2 - 10 \eta t \vartheta p \mathfrak{z}_2 - 18 \vartheta p \mu_1 \mathfrak{z}_2 + \\
& \quad 18 \eta t \vartheta p \mu_1 \mathfrak{z}_2 + 2 \vartheta p \mu_1^2 \mathfrak{z}_2 - 2 \eta t \vartheta p \mu_1^2 \mathfrak{z}_2 + 10 \vartheta p \mu_2 \mathfrak{z}_2 - \\
& \quad 10 \eta t \vartheta p \mu_2 \mathfrak{z}_2 - 74 \vartheta p \mu_1 \mu_2 \mathfrak{z}_2 + 74 \eta t \vartheta p \mu_1 \mu_2 \mathfrak{z}_2 + \\
& \quad w^3 (20 - 52 \mu_1 + 228 \mu_1^2 - 65 \mu_2 - 41 \mu_1 \mu_2 + \\
& \quad \eta t (-20 + 52 \mu_1 - 228 \mu_1^2 + 65 \mu_2 + 41 \mu_1 \mu_2 + 4 \vartheta p (-117 + 167 \mu_1^2 + \\
& \quad 10 \mathfrak{z}_1 + 2 \mu_1 (-38 + 11 \mathfrak{z}_1 + 5 \mu_2 (-44 + \mathfrak{z}_1 - \mathfrak{z}_2) - 11 \mathfrak{z}_2) + \\
& \quad 2 \mu_2 (-1 + 5 \mathfrak{z}_1 - 5 \mathfrak{z}_2) - 10 \mathfrak{z}_2)) + \vartheta p (404 - 636 \mu_1^2 - \\
& \quad 40 \mathfrak{z}_1 - 8 \mu_1 (2 + 11 \mathfrak{z}_1 + 5 \mu_2 (-44 + \mathfrak{z}_1 - \mathfrak{z}_2) - 11 \mathfrak{z}_2) + \\
& \quad 40 \mathfrak{z}_2 + \mu_2 (8 - 40 \mathfrak{z}_1 + 40 \mathfrak{z}_2))) - w^2 (12 (\mu_1^2 + \\
& \quad \mu_1 (23 - 7 \mu_2) + 5 \times (2 + \mu_2)) - \vartheta p (\mu_1^2 (5 \mathfrak{z}_1 - 9 \times (28 + \mathfrak{z}_2)) + \\
& \quad \mu_1 (454 - 217 \mathfrak{z}_1 + 213 \mathfrak{z}_2 + \mu_2 (726 - 120 \mathfrak{z}_1 + 36 \mathfrak{z}_2)) + 2 \times \\
& \quad (59 - 60 \mathfrak{z}_1 + 60 \mathfrak{z}_2 + \mu_2 (39 - 60 \mathfrak{z}_1 + 60 \mathfrak{z}_2))) + \eta t (-12 (\mu_1^2 +
\end{aligned}$$

$$\begin{aligned}
& \mu_1 (23 - 7 \mu_2) + 5 \times (2 + \mu_2) + \theta p (\mu_1^2 (764 + 5 \mathfrak{z}_1 - 9 \mathfrak{z}_2) + \\
& 6 \times (101 - 20 \mathfrak{z}_1 + 20 \mathfrak{z}_2 + \mu_2 (13 - 20 \mathfrak{z}_1 + 20 \mathfrak{z}_2)) + \\
& \mu_1 (374 - 217 \mathfrak{z}_1 + 213 \mathfrak{z}_2 + \mu_2 (726 - 120 \mathfrak{z}_1 + 36 \mathfrak{z}_2))) + \\
& w (-2 \times (50 + 42 \mu_1^2 + \mu_1 (50 - 57 \mu_2) + 15 \mu_2) + \theta p (-212 - 90 \mathfrak{z}_1 + \\
& \mu_1^2 (234 + 25 \mathfrak{z}_1 - 7 \mathfrak{z}_2) + 90 \mathfrak{z}_2 + \mu_2 (106 - 90 \mathfrak{z}_1 + 90 \mathfrak{z}_2) - \\
& \mu_1 (-358 + 77 \mathfrak{z}_1 - 95 \mathfrak{z}_2 + 2 \mu_2 (445 + 45 \mathfrak{z}_1 + 51 \mathfrak{z}_2))) + \\
& \eta t (2 \times (50 + 42 \mu_1^2 + \mu_1 (50 - 57 \mu_2) + 15 \mu_2) + \\
& \theta p (4 + 90 \mathfrak{z}_1 + 2 \mu_2 (-53 + 45 \mathfrak{z}_1 - 45 \mathfrak{z}_2) - \\
& 90 \mathfrak{z}_2 + \mu_1^2 (-778 - 25 \mathfrak{z}_1 + 7 \mathfrak{z}_2) + \mu_1 \\
& (-102 + 77 \mathfrak{z}_1 - 95 \mathfrak{z}_2 + 2 \mu_2 (445 + 45 \mathfrak{z}_1 + 51 \mathfrak{z}_2)))) + \\
& \eta^6 (18 \theta p + 8 \eta t \theta p + 72 \theta l \theta p + 24 \eta t \theta l \theta p - 4 \theta l \mu_1 + 4 \eta t \theta l \mu_1 - \\
& 36 \theta p \mu_1 + 24 \eta t \theta p \mu_1 + 94 \theta l \theta p \mu_1 - 46 \eta t \theta l \theta p \\
& \mu_1 - 4 \theta l \mu_1^2 + 4 \eta t \theta l \mu_1^2 - 30 \theta p \mu_1^2 + 16 \eta t \\
& \theta p \mu_1^2 + 166 \theta l \theta p \mu_1^2 + 2 \eta t \theta l \theta p \mu_1^2 + 106 \theta p \\
& \mu_2 + 10 \theta l \theta p \mu_2 - 10 \eta t \theta l \theta p \mu_2 + 94 \theta p \mu_1 \mu_2 + 60 \\
& \eta t \theta p \mu_1 \mu_2 - 50 \theta l \theta p \mu_1 \mu_2 + 50 \eta t \theta l \theta p \mu_1 \\
& \mu_2 + w^4 (-8 \times (-1 + \eta t) \theta l^2 (5 - 2 \mu_1 + 11 \mu_1^2) + \\
& \theta l (24 \theta p (-7 + 14 \mu_1^2 + \mu_1 (4 - 30 \mu_2)) + 5 \times (-8 + 16 \mu_1^2 + 3 \mu_2 + \\
& \mu_1 (-16 + 3 \mu_2)) - 5 \eta t (-8 + 16 \mu_1^2 + 3 \mu_2 + \mu_1 (-16 + 3 \mu_2)) + \\
& \eta t \theta p (140 - 484 \mu_1^2 + 8 \mu_1 (11 + 90 \mu_2))) + 2 \\
& \theta p (135 - 41 \mu_1^2 + \mu_1 (94 - 195 \mu_2) + 363 \mu_2 + \\
& \eta t (57 - 185 \mu_1^2 - 25 \mu_2 + \mu_1 (112 + 173 \mu_2))) + 5 \theta l \\
& \theta p \mu_1 \mathfrak{z}_1 - 5 \eta t \theta l \theta p \mu_1 \mathfrak{z}_1 + 5 \theta l \theta p \mu_1^2 \mathfrak{z}_1 - 5 \eta t \theta l \theta p \mu_1^2 \\
& \mathfrak{z}_1 + 5 \theta l \theta p \mu_1 \mathfrak{z}_2 - 5 \eta t \theta l \theta p \mu_1 \mathfrak{z}_2 + 5 \theta l \theta p \mu_1^2 \mathfrak{z}_2 - 5 \eta t \\
& \theta l \theta p \mu_1^2 \mathfrak{z}_2 + w^3 (-8 \times (-1 + \eta t) \theta l^2 (5 - 2 \mu_1 + 11 \mu_1^2) + \\
& \theta p (60 - 460 \mu_1^2 - 200 \mu_2 + 32 \mu_1 (-17 + 23 \mu_2) + \\
& \eta t (-48 + 224 \mu_1^2 - 137 \mu_2 + \mu_1 (-340 + 151 \mu_2))) + \\
& \theta l (20 + 80 \mu_1 + 25 \mu_2 - 23 \mu_1 \mu_2 + 2 \theta p (142 + 246 \mu_1^2 + 25 \mathfrak{z}_1 + \mu_2 \\
& (16 + 25 \mathfrak{z}_1 - 25 \mathfrak{z}_2) + 5 \mu_1 \mu_2 (-52 + 5 \mathfrak{z}_1 - 5 \mathfrak{z}_2) + 11 \mu_1 (-4 + \\
& 5 \mathfrak{z}_1 - 5 \mathfrak{z}_2) - 25 \mathfrak{z}_2) + \eta t (-20 - 80 \mu_1 - 25 \mu_2 + 23 \mu_1 \mu_2 + \\
& 2 \theta p (12 + 28 \mu_1^2 - 25 \mathfrak{z}_1 + 25 \mathfrak{z}_2 + \mu_2 (-16 - 25 \mathfrak{z}_1 + 25 \mathfrak{z}_2) + \\
& \mu_1 (112 - 55 \mathfrak{z}_1 - 5 \mu_2 (-52 + 5 \mathfrak{z}_1 - 5 \mathfrak{z}_2) + 55 \mathfrak{z}_2)))) + 4 \\
& w (12 \times (-1 + \eta t) \theta l \mu_1 + \theta p (-25 + 113 \mu_1 + 72 \mu_1^2 + 38 \mu_2 - \\
& 127 \mu_1 \mu_2 - \theta l (87 + 17 \mu_2 + \mu_1^2 (53 + 6 \mathfrak{z}_1 + \mathfrak{z}_2) + \\
& \mu_1 (21 \mathfrak{z}_1 + \mu_2 (5 - 30 \mathfrak{z}_2) - 14 \times (2 + \mathfrak{z}_2))) + \eta t (-26 - 4 \mu_1^2 + \\
& 8 \mu_2 + 2 \mu_1 (9 + \mu_2) + \theta l (63 + 17 \mu_2 + \mu_1^2 (11 + 6 \mathfrak{z}_1 + \mathfrak{z}_2) + \\
& \mu_1 (-40 + 5 \mu_2 + 21 \mathfrak{z}_1 - 14 \mathfrak{z}_2 - 30 \mu_2 \mathfrak{z}_2))) + w^2 \\
& (12 \times (-1 + \eta t) \theta l^2 (5 - 2 \mu_1 + 11 \mu_1^2) + \theta p (-270 + 194 \mu_1^2 - \\
& 922 \mu_2 - 2 \mu_1 (86 + 11 \mu_2) + \\
& \eta t (-192 + 124 \mu_1^2 - 17 \mu_2 - \mu_1 (188 + 389 \mu_2))) + \\
& \theta l (60 + 96 \mu_1 + 15 \mu_2 - 57 \mu_1 \mu_2 - \theta p (50 - 60 \mathfrak{z}_1 + 60 \mathfrak{z}_2 + \\
& \mu_1^2 (832 + 25 \mathfrak{z}_1 + 3 \mathfrak{z}_2) + \mu_2 (54 - 60 \mathfrak{z}_1 + 60 \mathfrak{z}_2) - \\
& \mu_1 (-510 + 41 \mathfrak{z}_1 - 69 \mathfrak{z}_2 + \mu_2 (954 + 60 \mathfrak{z}_1 + 72 \mathfrak{z}_2))) + \\
& \eta t (-15 \times (4 + \mu_2) + \mu_1 (-96 + 57 \mu_2) + \theta p (-222 - 60 \mathfrak{z}_1 +
\end{aligned}$$

$$\begin{aligned}
& 60 \mathfrak{z}2 + \mu1^2 (464 + 25 \mathfrak{z}1 + 3 \mathfrak{z}2) + \mu2 (54 - 60 \mathfrak{z}1 + 60 \mathfrak{z}2) - \\
& \mu1 (-158 + 41 \mathfrak{z}1 - 69 \mathfrak{z}2 + \mu2 (954 + 60 \mathfrak{z}1 + 72 \mathfrak{z}2)) \Big) \Big) \Big) \Big) \Big) + \\
& x^4 (-1 + \eta)^4 \Big( 4 (-1 + w (-1 + \eta))^3 (-2 + w (-1 + \eta) - 4 \eta) \times (-1 + \eta t) \\
& \quad \vartheta l^2 (5 - 2 \mu1 + 11 \mu1^2) + \\
& 2 (-1 + \eta)^2 \vartheta p (13 + 7 \eta - 10 \eta^2 + 30 \eta^3 - 2 \eta t - 20 \eta \eta t - 30 \eta^2 \\
& \quad \eta t + 21 \mu1 + 112 \eta \mu1 + 155 \eta^2 \mu1 + 30 \eta^3 \mu1 - 10 \eta t \\
& \quad \mu1 - 18 \eta \eta t \mu1 - 30 \eta^2 \eta t \mu1 + 2 \mu1^2 + 45 \eta \mu1^2 + 75 \\
& \quad \eta^2 \mu1^2 + 4 \eta t \mu1^2 + 2 \eta \eta t \mu1^2 + w^4 (-1 + \eta)^4 (1 + \mu1) \\
& \quad (\eta - \eta t + 4 \mu1) + 19 \mu2 + 47 \eta \mu2 - 2 \eta t \mu2 + \mu1 \mu2 - 7 \eta \mu1 \\
& \quad \mu2 - 60 \eta^2 \mu1 \mu2 + 16 \eta t \mu1 \mu2 + 30 \eta \eta t \mu1 \mu2 - w^3 (-1 + \eta)^3 \\
& \quad (10 + 39 \mu1 + 23 \mu1^2 + 10 \eta^2 (1 + \mu1) + 22 \mu2 - 14 \mu1 \mu2 + \\
& \quad \eta (7 + 47 \mu1 + 40 \mu1^2 - 10 \eta t (1 + \mu1) - 12 \mu1 \mu2) + \\
& \quad \eta t (-7 - 7 \mu1 + 12 \mu1 \mu2) \Big) + w^2 (-1 + \eta)^2 \\
& \quad (33 + 101 \mu1 + 38 \mu1^2 + 15 \eta^3 (1 + \mu1) + 65 \mu2 - 37 \mu1 \mu2 + \\
& \quad \eta t (-15 - 23 \mu1 + 4 \mu1^2 - 2 \mu2 + 40 \mu1 \mu2) - \\
& \quad 5 \eta^2 (3 \eta t (1 + \mu1) - 2 \times (4 + 10 \mu1 + 6 \mu1^2 - 3 \mu1 \mu2) \Big) + \eta (40 + 225 \mu1 + \\
& \quad 125 \mu1^2 + 55 \mu2 - 77 \mu1 \mu2 + 10 \eta t (-4 - 4 \mu1 + 3 \mu1 \mu2) \Big) \Big) - w \\
& \quad (-1 + \eta) \times (32 + 83 \mu1 + 21 \mu1^2 + 45 \eta^3 (1 + \mu1) + 62 \mu2 - 22 \mu1 \mu2 + \\
& \quad 5 \eta^2 (10 + 55 \mu1 + 27 \mu1^2 - 9 \eta t (1 + \mu1) - 18 \mu1 \mu2) + \\
& \quad \eta t (-11 - 27 \mu1 + 8 \mu1^2 - 4 \mu2 + 44 \mu1 \mu2) + \eta (41 + 291 \mu1 + 130 \mu1^2 + \\
& \quad 102 \mu2 - 72 \mu1 \mu2 + 2 \eta t (-25 + \mu1^2 + 6 \mu1 (-4 + 5 \mu2) \Big) \Big) \Big) \Big) + \\
& \vartheta l (-20 + 20 \eta + 20 \eta t - 20 \eta \eta t + 34 \vartheta p + 112 \eta \vartheta p + 230 \eta^2 \vartheta p + 180 \\
& \quad \eta^3 \vartheta p - 70 \eta t \vartheta p - 236 \eta \eta t \vartheta p - 310 \eta^2 \eta t \vartheta p + 60 \eta^3 \\
& \quad \eta t \vartheta p - 52 \mu1 - 28 \eta \mu1 + 96 \eta^2 \mu1 - 16 \eta^3 \mu1 + 52 \eta t \\
& \quad \mu1 + 28 \eta \eta t \mu1 - 96 \eta^2 \eta t \mu1 + 16 \eta^3 \eta t \mu1 + 18 \vartheta p \\
& \quad \mu1 - 170 \eta \vartheta p \mu1 - 268 \eta^2 \vartheta p \mu1 + 220 \eta^3 \vartheta p \mu1 - 18 \\
& \quad \eta t \vartheta p \mu1 + 90 \eta \eta t \vartheta p \mu1 + 228 \eta^2 \eta t \vartheta p \mu1 - 100 \\
& \quad \eta^3 \eta t \vartheta p \mu1 + 28 \mu1^2 - 12 \eta \mu1^2 - 16 \eta^3 \mu1^2 - 28 \eta t \\
& \quad \mu1^2 + 12 \eta \eta t \mu1^2 + 16 \eta^3 \eta t \mu1^2 - 28 \vartheta p \mu1^2 - 174 \\
& \quad \eta \vartheta p \mu1^2 - 18 \eta^2 \vartheta p \mu1^2 + 400 \eta^3 \vartheta p \mu1^2 - 44 \eta t \vartheta p \\
& \quad \mu1^2 - 34 \eta \eta t \vartheta p \mu1^2 - 122 \eta^2 \eta t \vartheta p \mu1^2 + 20 \eta^3 \eta t \vartheta p \\
& \quad \mu1^2 - 5 \mu2 + 5 \eta \mu2 + 5 \eta t \mu2 - 5 \eta \eta t \mu2 + 14 \vartheta p \mu2 + 6 \\
& \quad \eta \vartheta p \mu2 + 22 \eta^2 \vartheta p \mu2 + 10 \eta^3 \vartheta p \mu2 - 14 \eta t \vartheta p \mu2 - 6 \\
& \quad \eta \eta t \vartheta p \mu2 - 22 \eta^2 \eta t \vartheta p \mu2 - 10 \eta^3 \eta t \vartheta p \mu2 + 19 \mu1 \\
& \quad \mu2 - 19 \eta \mu1 \mu2 - 19 \eta t \mu1 \mu2 + 19 \eta \eta t \mu1 \mu2 + 38 \vartheta p \\
& \quad \mu1 \mu2 + 186 \eta \vartheta p \mu1 \mu2 + 70 \eta^2 \vartheta p \mu1 \mu2 - 50 \eta^3 \vartheta p \\
& \quad \mu1 \mu2 - 38 \eta t \vartheta p \mu1 \mu2 - 186 \eta \eta t \vartheta p \mu1 \mu2 - 70 \eta^2 \\
& \quad \eta t \vartheta p \mu1 \mu2 + 50 \eta^3 \eta t \vartheta p \mu1 \mu2 + 4 w^4 (-1 + \eta)^4 \vartheta p \\
& \quad (5 - 2 \mu1 - 7 \mu1^2 + \eta (4 + 2 \mu1 + 7 \mu1^2) + 18 \mu1 \mu2 - 9 \eta t (1 + 2 \mu1 \mu2) \Big) - 5 \\
& \quad \vartheta p \mathfrak{z}1 + 5 \eta \vartheta p \mathfrak{z}1 + 5 \eta t \vartheta p \mathfrak{z}1 - 5 \eta \eta t \vartheta p \mathfrak{z}1 - 22 \vartheta p \mu1 \\
& \quad \mathfrak{z}1 - 24 \eta \vartheta p \mu1 \mathfrak{z}1 + 41 \eta^2 \vartheta p \mu1 \mathfrak{z}1 + 5 \eta^3 \vartheta p \mu1 \mathfrak{z}1 + 22 \\
& \quad \eta t \vartheta p \mu1 \mathfrak{z}1 + 24 \eta \eta t \vartheta p \mu1 \mathfrak{z}1 - 41 \eta^2 \eta t \vartheta p \mu1 \mathfrak{z}1 - 5 \\
& \quad \eta^3 \eta t \vartheta p \mu1 \mathfrak{z}1 - 5 \vartheta p \mu1^2 \mathfrak{z}1 - 11 \eta \vartheta p \mu1^2 \mathfrak{z}1 + 11 \eta^2 \\
& \quad \vartheta p \mu1^2 \mathfrak{z}1 + 5 \eta^3 \vartheta p \mu1^2 \mathfrak{z}1 + 5 \eta t \vartheta p \mu1^2 \mathfrak{z}1 + 11 \eta \eta t \\
& \quad \vartheta p \mu1^2 \mathfrak{z}1 - 11 \eta^2 \eta t \vartheta p \mu1^2 \mathfrak{z}1 - 5 \eta^3 \eta t \vartheta p \mu1^2 \mathfrak{z}1 - 5
\end{aligned}$$

$$\begin{aligned}
& \partial_p \mu_2 \mathfrak{x}1 + 5 \eta \partial_p \mu_2 \mathfrak{x}1 + 5 \eta t \partial_p \mu_2 \mathfrak{x}1 - 5 \eta \eta t \partial_p \mu_2 \\
& \mathfrak{x}1 - 5 \partial_p \mu_1 \mu_2 \mathfrak{x}1 + 5 \eta \partial_p \mu_1 \mu_2 \mathfrak{x}1 + 5 \eta t \partial_p \mu_1 \mu_2 \\
& \mathfrak{x}1 - 5 \eta \eta t \partial_p \mu_1 \mu_2 \mathfrak{x}1 + 5 \partial_p \mathfrak{x}2 - 5 \eta \partial_p \mathfrak{x}2 - 5 \eta t \partial_p \\
& \mathfrak{x}2 + 5 \eta \eta t \partial_p \mathfrak{x}2 + 14 \partial_p \mu_1 \mathfrak{x}2 + 10 \eta \partial_p \mu_1 \mathfrak{x}2 - 29 \eta^2 \\
& \partial_p \mu_1 \mathfrak{x}2 + 5 \eta^3 \partial_p \mu_1 \mathfrak{x}2 - 14 \eta t \partial_p \mu_1 \mathfrak{x}2 - 10 \eta \eta t \partial_p \\
& \mu_1 \mathfrak{x}2 + 29 \eta^2 \eta t \partial_p \mu_1 \mathfrak{x}2 - 5 \eta^3 \eta t \partial_p \mu_1 \mathfrak{x}2 - 3 \partial_p \mu_1^2 \\
& \mathfrak{x}2 - 3 \eta \partial_p \mu_1^2 \mathfrak{x}2 + \eta^2 \partial_p \mu_1^2 \mathfrak{x}2 + 5 \eta^3 \partial_p \mu_1^2 \mathfrak{x}2 + 3 \\
& \eta t \partial_p \mu_1^2 \mathfrak{x}2 + 3 \eta \eta t \partial_p \mu_1^2 \mathfrak{x}2 - \eta^2 \eta t \partial_p \mu_1^2 \mathfrak{x}2 - 5 \\
& \eta^3 \eta t \partial_p \mu_1^2 \mathfrak{x}2 + 5 \partial_p \mu_2 \mathfrak{x}2 - 5 \eta \partial_p \mu_2 \mathfrak{x}2 - 5 \eta t \partial_p \\
& \mu_2 \mathfrak{x}2 + 5 \eta \eta t \partial_p \mu_2 \mathfrak{x}2 + 17 \partial_p \mu_1 \mu_2 \mathfrak{x}2 + 43 \eta \partial_p \mu_1 \\
& \mu_2 \mathfrak{x}2 - 60 \eta^2 \partial_p \mu_1 \mu_2 \mathfrak{x}2 - 17 \eta t \partial_p \mu_1 \mu_2 \mathfrak{x}2 - 43 \eta \\
& \eta t \partial_p \mu_1 \mu_2 \mathfrak{x}2 + 60 \eta^2 \eta t \partial_p \mu_1 \mu_2 \mathfrak{x}2 - w^3 (-1 + \eta)^3 \\
& (-20 + 100 \partial_p - 52 \mu_1 - 56 \partial_p \mu_1 + 28 \mu_1^2 - 156 \partial_p \mu_1^2 + \\
& 40 \eta^2 \partial_p (4 + 2 \mu_1 + 7 \mu_1^2) - 5 \mu_2 + 16 \partial_p \mu_2 + 19 \mu_1 \mu_2 + \\
& 280 \partial_p \mu_1 \mu_2 - 5 \partial_p \mathfrak{x}1 - 11 \partial_p \mu_1 \mathfrak{x}1 - 5 \partial_p \mu_2 \mathfrak{x}1 - \\
& 5 \partial_p \mu_1 \mu_2 \mathfrak{x}1 + 5 \partial_p \mathfrak{x}2 + 11 \partial_p \mu_1 \mathfrak{x}2 + 5 \partial_p \mu_2 \mathfrak{x}2 + \\
& 5 \partial_p \mu_1 \mu_2 \mathfrak{x}2 - \eta t (28 \mu_1^2 - 5 \times (4 + \mu_2) + \mu_1 (-52 + 19 \mu_2) + \\
& \partial_p (216 + 56 \mu_1^2 - 5 \mathfrak{x}1 + 5 \mathfrak{x}2 + \mu_2 (16 - 5 \mathfrak{x}1 + 5 \mathfrak{x}2) + \\
& \mu_1 (-16 - 11 \mathfrak{x}1 - 5 \mu_2 (-56 + \mathfrak{x}1 - \mathfrak{x}2) + 11 \mathfrak{x}2))) + \\
& \eta (20 + 52 \mu_1 - 28 \mu_1^2 + 5 \mu_2 - 19 \mu_1 \mu_2 + \partial_p (196 - 96 \mu_1^2 + 5 \mathfrak{x}1 + \\
& \mu_1 (-116 + 11 \mathfrak{x}1 + 5 \mu_2 (36 + \mathfrak{x}1 - \mathfrak{x}2) - 11 \mathfrak{x}2) + \mu_2 (36 + 5 \mathfrak{x}1 - \\
& 5 \mathfrak{x}2) - 5 \mathfrak{x}2) + \eta t (28 \mu_1^2 - 5 \times (4 + \mu_2) + \mu_1 (-52 + 19 \mu_2) + \\
& \partial_p (28 \mu_1^2 - 5 \times (48 + \mathfrak{x}1 - \mathfrak{x}2) + \mu_2 (-36 - 5 \mathfrak{x}1 + 5 \mathfrak{x}2) + \\
& \mu_1 (76 - 11 \mathfrak{x}1 - 5 \mu_2 (36 + \mathfrak{x}1 - \mathfrak{x}2) + 11 \mathfrak{x}2)))) + w^2 \\
& (-1 + \eta)^2 (-60 + 174 \partial_p - 156 \mu_1 - 82 \partial_p \mu_1 + 84 \mu_1^2 - 244 \partial_p \mu_1^2 + \\
& 60 \eta^3 \partial_p (4 + 2 \mu_1 + 7 \mu_1^2) - 15 \mu_2 + 42 \partial_p \mu_2 + 57 \mu_1 \mu_2 + \\
& 402 \partial_p \mu_1 \mu_2 - 15 \partial_p \mathfrak{x}1 - 44 \partial_p \mu_1 \mathfrak{x}1 - 5 \partial_p \mu_1^2 \mathfrak{x}1 - \\
& 15 \partial_p \mu_2 \mathfrak{x}1 - 15 \partial_p \mu_1 \mu_2 \mathfrak{x}1 + \eta t (60 + 156 \mu_1 - 84 \mu_1^2 + 15 \mu_2 - \\
& 57 \mu_1 \mu_2 + \partial_p (-394 + 15 \mathfrak{x}1 + \mu_1^2 (5 \mathfrak{x}1 + 3 \times (-56 + \mathfrak{x}2)) + \\
& \mu_1 (26 + 44 \mathfrak{x}1 + 3 \mu_2 (-134 + 5 \mathfrak{x}1 - 9 \mathfrak{x}2) - 36 \mathfrak{x}2) + \\
& 3 \mu_2 (-14 + 5 \mathfrak{x}1 - 5 \mathfrak{x}2) - 15 \mathfrak{x}2)) + 15 \partial_p \mathfrak{x}2 + \\
& 36 \partial_p \mu_1 \mathfrak{x}2 - 3 \partial_p \mu_1^2 \mathfrak{x}2 + 15 \partial_p \mu_2 \mathfrak{x}2 + 27 \partial_p \mu_1 \mu_2 \mathfrak{x}2 + \\
& \eta^2 (16 \times (-1 + \eta t) \times (-5 + \mu_1) \mu_1 - 5 \partial_p (-2 \times (53 + 5 \mu_2) - \\
& \mu_1^2 (92 + 3 \mathfrak{x}1 + \mathfrak{x}2) + \mu_1 (6 - 9 \mathfrak{x}1 + 5 \mathfrak{x}2 + 2 \mu_2 (7 + 6 \mathfrak{x}2)) + \\
& \eta t (58 + 10 \mu_2 + \mu_1^2 (8 + 3 \mathfrak{x}1 + \mathfrak{x}2) - \\
& \mu_1 (30 - 9 \mathfrak{x}1 + 5 \mathfrak{x}2 + 2 \mu_2 (7 + 6 \mathfrak{x}2)))) + \\
& \eta (60 + 76 \mu_1 - 68 \mu_1^2 + 15 \mu_2 - 57 \mu_1 \mu_2 - \partial_p (-416 - 15 \mathfrak{x}1 + \\
& 15 \mathfrak{x}2 + 2 \mu_1^2 (226 + 5 \mathfrak{x}1 + \mathfrak{x}2) + \mu_2 (-64 - 15 \mathfrak{x}1 + 15 \mathfrak{x}2) + \\
& \mu_1 (444 + \mathfrak{x}1 + 11 \mathfrak{x}2 - \mu_2 (616 + 15 \mathfrak{x}1 + 33 \mathfrak{x}2))) + \\
& \eta t (68 \mu_1^2 - 15 \times (4 + \mu_2) + 19 \mu_1 (-4 + 3 \mu_2) + \partial_p (-676 - 15 \mathfrak{x}1 + \\
& 15 \mathfrak{x}2 + 2 \mu_1^2 (12 + 5 \mathfrak{x}1 + \mathfrak{x}2) + \mu_2 (-64 - 15 \mathfrak{x}1 + 15 \mathfrak{x}2) + \\
& \mu_1 (260 + \mathfrak{x}1 + 11 \mathfrak{x}2 - \mu_2 (616 + 15 \mathfrak{x}1 + 33 \mathfrak{x}2)))) + w \\
& (-1 + \eta) \times (60 - 136 \partial_p + 156 \mu_1 + 8 \partial_p \mu_1 - 84 \mu_1^2 + 144 \partial_p \mu_1^2 + \\
& 15 \mu_2 - 40 \partial_p \mu_2 - 57 \mu_1 \mu_2 - 232 \partial_p \mu_1 \mu_2 +
\end{aligned}$$

$$\begin{aligned}
& 3 \eta t (28 \mu_1^2 - 5 \times (4 + \mu_2) + \mu_1 (-52 + 19 \mu_2)) + 15 \theta p \mathfrak{z}1 + \\
& 55 \theta p \mu_1 \mathfrak{z}1 + 10 \theta p \mu_1^2 \mathfrak{z}1 + 15 \theta p \mu_2 \mathfrak{z}1 + 15 \theta p \mu_1 \mu_2 \mathfrak{z}1 - \\
& 15 \theta p \mathfrak{z}2 - 39 \theta p \mu_1 \mathfrak{z}2 + 6 \theta p \mu_1^2 \mathfrak{z}2 - 15 \theta p \mu_2 \mathfrak{z}2 - 39 \theta p \mu_1 \mu_2 \mathfrak{z}2 + \\
& \eta t \theta p (292 - 15 \mathfrak{z}1 - 5 \mu_2 (-8 + 3 \mathfrak{z}1 - 3 \mathfrak{z}2) + 15 \mathfrak{z}2 - 2 \mu_1^2 (-78 + 5 \mathfrak{z}1 + \\
& \quad 3 \mathfrak{z}2) + \mu_1 (16 - 55 \mathfrak{z}1 + 39 \mathfrak{z}2 + \mu_2 (232 - 15 \mathfrak{z}1 + 39 \mathfrak{z}2))) + \\
& 2 \eta^2 (-1 + \eta t) \times (-8 \times (-11 + \mu_1) \mu_1 + \theta p (270 + 36 \mu_2 + 43 \mu_1 \mathfrak{z}1 + \\
& \quad \mu_1^2 (81 + 13 \mathfrak{z}1 + 3 \mathfrak{z}2) - 3 \mu_1 (73 + (9 + 20 \mu_2) \mathfrak{z}2))) + \\
& \eta^3 (-16 \times (-1 + \eta t) \mu_1 (1 + \mu_1) + 5 \theta p (-96 + 2 \times (-1 + \eta t) \mu_2 - \\
& \quad \mu_1 (80 - 10 \mu_2 + \mathfrak{z}1 + \eta t (-32 + 10 \mu_2 - \mathfrak{z}1 - \mathfrak{z}2) + \mathfrak{z}2) + \\
& \quad \mu_1^2 (-164 - \mathfrak{z}1 - \mathfrak{z}2 + \eta t (-4 + \mathfrak{z}1 + \mathfrak{z}2))) + \\
& \eta (-60 + 4 \mu_1 + 52 \mu_1^2 - 15 \mu_2 + 57 \mu_1 \mu_2 + \theta p (-5 \times (68 + 3 \mathfrak{z}1 - 3 \mathfrak{z}2) + \\
& \quad \mu_1^2 (502 + 21 \mathfrak{z}1 + 5 \mathfrak{z}2) + \mu_2 (-34 - 15 \mathfrak{z}1 + 15 \mathfrak{z}2) - \\
& \quad \mu_1 (-498 - 36 \mathfrak{z}1 + 10 \mathfrak{z}2 + \mu_2 (622 + 15 \mathfrak{z}1 + 81 \mathfrak{z}2))) + \\
& \eta t (60 - 4 \mu_1 - 52 \mu_1^2 + 15 \mu_2 - 57 \mu_1 \mu_2 + \theta p (664 + 15 \mathfrak{z}1 + \\
& \quad \mu_2 (34 + 15 \mathfrak{z}1 - 15 \mathfrak{z}2) + \mu_1^2 (38 - 21 \mathfrak{z}1 - 5 \mathfrak{z}2) - 15 \mathfrak{z}2 + \\
& \quad \mu_1 (-282 - 36 \mathfrak{z}1 + 10 \mathfrak{z}2 + \mu_2 (622 + 15 \mathfrak{z}1 + 81 \mathfrak{z}2)))))) - \\
& x^3 (-1 + \eta)^3 (4 (-1 + w (-1 + \eta))^3 (-1 - 6 \eta - 6 \eta^2 + w (-2 - \eta + 3 \eta^2)) \times \\
& \quad (-1 + \eta t) \theta l^2 (5 - 2 \mu_1 + 11 \mu_1^2) + \\
& (-1 + \eta)^2 \theta p (20 + 104 \eta + 36 \eta^2 + 80 \eta^4 - 20 \eta t - 16 \eta \eta t - 80 \\
& \quad \eta^2 \eta t - 80 \eta^3 \eta t + 16 \mu_1 + 168 \eta \mu_1 + 456 \eta^2 \mu_1 + 440 \\
& \quad \eta^3 \mu_1 + 80 \eta^4 \mu_1 - 48 \eta t \mu_1 - 80 \eta \eta t \mu_1 - 64 \eta^2 \eta t \\
& \quad \mu_1 - 80 \eta^3 \eta t \mu_1 - 4 \mu_1^2 + 16 \eta \mu_1^2 + 180 \eta^2 \mu_1^2 + 200 \\
& \quad \eta^3 \mu_1^2 + 44 \eta t \mu_1^2 + 32 \eta \eta t \mu_1^2 + 16 \eta^2 \eta t \mu_1^2 + 12 \\
& \quad \mu_2 + 152 \eta \mu_2 + 196 \eta^2 \mu_2 - 9 \eta t \mu_2 - 16 \eta \eta t \mu_2 + 12 \mu_1 \\
& \quad \mu_2 + 8 \eta \mu_1 \mu_2 - 116 \eta^2 \mu_1 \mu_2 - 240 \eta^3 \mu_1 \mu_2 + 39 \eta t \mu_1 \\
& \quad \mu_2 + 128 \eta \eta t \mu_1 \mu_2 + 120 \eta^2 \eta t \mu_1 \mu_2 + 2 w^4 (-1 + \eta)^4 \\
& \quad (5 + 12 \mu_1 + 7 \mu_1^2 + 4 \eta^2 (1 + \mu_1) + 11 \mu_2 - 7 \mu_1 \mu_2 + \\
& \quad 2 \eta (1 + 9 \mu_1 + 8 \mu_1^2 - 2 \eta t (1 + \mu_1) - 3 \mu_1 \mu_2) + \\
& \quad \eta t (-2 - 2 \mu_1 + 6 \mu_1 \mu_2)) - w^3 (-1 + \eta)^3 \\
& (60 + 40 \mu_1^2 + 44 \eta t \mu_1^2 + 40 \eta^3 (1 + \mu_1) + 4 \mu_1 (31 - 14 \mu_2) + \\
& \quad 112 \mu_2 - 9 \eta t (4 + \mu_2) + \eta t \mu_1 (-64 + 87 \mu_2) + \\
& \quad 8 \eta^2 (7 + 27 \mu_1 + 20 \mu_1^2 - 5 \eta t (1 + \mu_1) - 12 \mu_1 \mu_2) + 4 \eta \\
& \quad (24 + 82 \mu_1 + 46 \mu_1^2 + 44 \mu_2 - 43 \mu_1 \mu_2 + 2 \eta t (-7 - 7 \mu_1 + 12 \mu_1 \mu_2))) + \\
& w^2 (-1 + \eta)^2 (40 \eta^4 (1 + \mu_1) + 2 \times (51 + 92 \mu_1 + 17 \mu_1^2 + 83 \mu_2 - 19 \mu_1 \mu_2) - \\
& \quad 40 \eta^3 (-4 + \eta t - 8 \mu_1 + \eta t \mu_1 - 4 \mu_1^2 + 3 \mu_1 \mu_2) + \\
& \quad \eta t (-80 - 164 \mu_1 + 132 \mu_1^2 - 27 \mu_2 + 177 \mu_1 \mu_2) + \\
& \quad 4 \eta^2 (55 + 240 \mu_1 + 125 \mu_1^2 + 55 \mu_2 - 119 \mu_1 \mu_2 + \\
& \quad 10 \eta t (-4 - 4 \mu_1 + 3 \mu_1 \mu_2)) + 4 \eta (71 + 207 \mu_1 + 76 \mu_1^2 + 130 \mu_2 - \\
& \quad 98 \mu_1 \mu_2 + \eta t (-30 - 46 \mu_1 + 8 \mu_1^2 - 4 \mu_2 + 80 \mu_1 \mu_2))) - w (-1 + \eta) \times \\
& (120 \eta^4 (1 + \mu_1) + 40 \eta^3 (5 + 9 \mu_1^2 - 3 \eta t (1 + \mu_1) + \mu_1 (20 - 9 \mu_2)) + \\
& \quad 4 \times (18 + \mu_1^2 + 22 \mu_2 + \mu_1 (25 + 4 \mu_2)) + \\
& \quad \eta t (-68 + 132 \mu_1^2 - 27 \mu_2 + \mu_1 (-152 + 141 \mu_2)) + \\
& \quad 8 \eta^2 (26 + 65 \mu_1^2 + \mu_1 (151 - 62 \mu_2) + 52 \mu_2 + \\
& \quad \eta t (-25 + 2 \mu_1^2 + \mu_1 (-23 + 30 \mu_2))) + 8 \eta (33 + 21 \mu_1^2 - 28 \mu_1
\end{aligned}$$

$$\begin{aligned}
& (-3 + \mu_2) + 62 \mu_2 + \eta t \left( -11 + 8 \mu_1^2 - 4 \mu_2 + \mu_1 (-27 + 44 \mu_2) \right) \Big) \Big) + \\
& \text{el} \left( -30 - 30 \eta + 60 \eta^2 + 30 \eta t + 30 \eta \eta t - 60 \eta^2 \eta t + 30 \text{ep} + 126 \eta \right. \\
& \quad \text{ep} + 268 \eta^2 \text{ep} + 420 \eta^3 \text{ep} + 240 \eta^4 \text{ep} - 70 \eta t \text{ep} - 230 \\
& \quad \eta \eta t \text{ep} - 444 \eta^2 \eta t \text{ep} - 420 \eta^3 \eta t \text{ep} + 80 \eta^4 \eta t \text{ep} - 32 \\
& \quad \mu_1 - 128 \eta \mu_1 + 40 \eta^2 \mu_1 + 144 \eta^3 \mu_1 - 24 \eta^4 \mu_1 + 32 \\
& \quad \eta t \mu_1 + 128 \eta \eta t \mu_1 - 40 \eta^2 \eta t \mu_1 - 144 \eta^3 \eta t \mu_1 + 24 \\
& \quad \eta^4 \eta t \mu_1 + 34 \text{ep} \mu_1 + 56 \eta \text{ep} \mu_1 - 342 \eta^2 \text{ep} \mu_1 - 272 \\
& \quad \eta^3 \text{ep} \mu_1 + 300 \eta^4 \text{ep} \mu_1 - 18 \eta t \text{ep} \mu_1 - 72 \eta \eta t \text{ep} \\
& \quad \mu_1 + 182 \eta^2 \eta t \text{ep} \mu_1 + 272 \eta^3 \eta t \text{ep} \mu_1 - 140 \eta^4 \eta t \\
& \quad \text{ep} \mu_1 + 10 \mu_1^2 + 46 \eta \mu_1^2 - 32 \eta^2 \mu_1^2 - 24 \eta^4 \mu_1^2 - 10 \\
& \quad \eta t \mu_1^2 - 46 \eta \eta t \mu_1^2 + 32 \eta^2 \eta t \mu_1^2 + 24 \eta^4 \eta t \mu_1^2 - 8 \\
& \quad \text{ep} \mu_1^2 - 106 \eta \text{ep} \mu_1^2 - 298 \eta^2 \text{ep} \mu_1^2 + 148 \eta^3 \text{ep} \\
& \quad \mu_1^2 + 540 \eta^4 \text{ep} \mu_1^2 - 80 \eta t \text{ep} \mu_1^2 - 94 \eta \eta t \text{ep} \mu_1^2 + 26 \\
& \quad \eta^2 \eta t \text{ep} \mu_1^2 - 148 \eta^3 \eta t \text{ep} \mu_1^2 + 20 \eta^4 \eta t \text{ep} \mu_1^2 - 10 \\
& \quad \mu_2 - 5 \eta \mu_2 + 15 \eta^2 \mu_2 + 10 \eta t \mu_2 + 5 \eta \eta t \mu_2 - 15 \eta^2 \\
& \quad \eta t \mu_2 + 22 \text{ep} \mu_2 + 36 \eta \text{ep} \mu_2 + 2 \eta^2 \text{ep} \mu_2 + 48 \eta^3 \text{ep} \\
& \quad \mu_2 + 20 \eta^4 \text{ep} \mu_2 - 22 \eta t \text{ep} \mu_2 - 36 \eta \eta t \text{ep} \mu_2 - 2 \eta^2 \\
& \quad \eta t \text{ep} \mu_2 - 48 \eta^3 \eta t \text{ep} \mu_2 - 20 \eta^4 \eta t \text{ep} \mu_2 + 38 \mu_1 \\
& \quad \mu_2 + 19 \eta \mu_1 \mu_2 - 57 \eta^2 \mu_1 \mu_2 - 38 \eta t \mu_1 \mu_2 - 19 \eta \\
& \quad \eta t \mu_1 \mu_2 + 57 \eta^2 \eta t \mu_1 \mu_2 - 2 \text{ep} \mu_1 \mu_2 + 216 \eta \text{ep} \mu_1 \\
& \quad \mu_2 + 494 \eta^2 \text{ep} \mu_1 \mu_2 + 120 \eta^3 \text{ep} \mu_1 \mu_2 - 100 \eta^4 \text{ep} \mu_1 \\
& \quad \mu_2 + 2 \eta t \text{ep} \mu_1 \mu_2 - 216 \eta \eta t \text{ep} \mu_1 \mu_2 - 494 \eta^2 \eta t \text{ep} \\
& \quad \mu_1 \mu_2 - 120 \eta^3 \eta t \text{ep} \mu_1 \mu_2 + 100 \eta^4 \eta t \text{ep} \mu_1 \mu_2 + w^4 \\
& \quad (-1 + \eta)^4 \left( -10 + 40 \text{ep} - 20 \mu_1 - 16 \text{ep} \mu_1 + 26 \mu_1^2 - \right. \\
& \quad \quad 56 \text{ep} \mu_1^2 + 16 \eta^2 \text{ep} \left( 4 + 2 \mu_1 + 7 \mu_1^2 \right) + 5 \mu_2 + \\
& \quad \quad 5 \mu_1 \mu_2 + 144 \text{ep} \mu_1 \mu_2 - \eta t \left( 26 \mu_1^2 + 5 \mu_1 (-4 + \mu_2) + \right. \\
& \quad \quad \quad 5 \times (-2 + \mu_2) + 4 \text{ep} \left( 23 + 11 \mu_1^2 + \mu_1 (-2 + 36 \mu_2) \right) \Big) + \\
& \quad \quad \eta \left( 10 + 20 \mu_1 - 26 \mu_1^2 - 8 \text{ep} \left( -14 + 7 \mu_1^2 + \mu_1 (2 - 36 \mu_2) \right) - \right. \\
& \quad \quad \quad 5 \mu_2 - 5 \mu_1 \mu_2 + \eta t \left( 26 \mu_1^2 + 5 \mu_1 (-4 + \mu_2) + 5 \times (-2 + \mu_2) + \right. \\
& \quad \quad \quad \quad \left. \left. 4 \text{ep} \left( -31 + 11 \mu_1^2 - 2 \mu_1 (1 + 36 \mu_2) \right) \right) \right) \Big) \Big) - 10 \text{ep} \\
& \quad \text{e1} - 10 \eta \text{ep} \text{e1} + 20 \eta^2 \text{ep} \text{e1} + 10 \eta t \text{ep} \text{e1} + 10 \eta \eta t \text{ep} \text{e1} - 20 \\
& \quad \eta^2 \eta t \text{ep} \text{e1} - 17 \text{ep} \mu_1 \text{e1} - 70 \eta \text{ep} \mu_1 \text{e1} - 7 \eta^2 \text{ep} \\
& \quad \mu_1 \text{e1} + 84 \eta^3 \text{ep} \mu_1 \text{e1} + 10 \eta^4 \text{ep} \mu_1 \text{e1} + 17 \eta t \text{ep} \mu_1 \\
& \quad \text{e1} + 70 \eta \eta t \text{ep} \mu_1 \text{e1} + 7 \eta^2 \eta t \text{ep} \mu_1 \text{e1} - 84 \eta^3 \eta t \text{ep} \\
& \quad \mu_1 \text{e1} - 10 \eta^4 \eta t \text{ep} \mu_1 \text{e1} - \text{ep} \mu_1^2 \text{e1} - 18 \eta \text{ep} \mu_1^2 \\
& \quad \text{e1} - 15 \eta^2 \text{ep} \mu_1^2 \text{e1} + 24 \eta^3 \text{ep} \mu_1^2 \text{e1} + 10 \eta^4 \text{ep} \mu_1^2 \\
& \quad \text{e1} + \eta t \text{ep} \mu_1^2 \text{e1} + 18 \eta \eta t \text{ep} \mu_1^2 \text{e1} + 15 \eta^2 \eta t \text{ep} \mu_1^2 \\
& \quad \text{e1} - 24 \eta^3 \eta t \text{ep} \mu_1^2 \text{e1} - 10 \eta^4 \eta t \text{ep} \mu_1^2 \text{e1} - 10 \text{ep} \\
& \quad \mu_2 \text{e1} - 10 \eta \text{ep} \mu_2 \text{e1} + 20 \eta^2 \text{ep} \mu_2 \text{e1} + 10 \eta t \text{ep} \mu_2 \\
& \quad \text{e1} + 10 \eta \eta t \text{ep} \mu_2 \text{e1} - 20 \eta^2 \eta t \text{ep} \mu_2 \text{e1} - 10 \text{ep} \mu_1 \mu_2 \\
& \quad \text{e1} - 10 \eta \text{ep} \mu_1 \mu_2 \text{e1} + 20 \eta^2 \text{ep} \mu_1 \mu_2 \text{e1} + 10 \eta t \text{ep} \mu_1 \\
& \quad \mu_2 \text{e1} + 10 \eta \eta t \text{ep} \mu_1 \mu_2 \text{e1} - 20 \eta^2 \eta t \text{ep} \mu_1 \mu_2 \text{e1} + 10 \\
& \quad \text{ep} \text{e2} + 10 \eta \text{ep} \text{e2} - 20 \eta^2 \text{ep} \text{e2} - 10 \eta t \text{ep} \text{e2} - 10 \eta \eta t \\
& \quad \text{ep} \text{e2} + 20 \eta^2 \eta t \text{ep} \text{e2} + 13 \text{ep} \mu_1 \text{e2} + 44 \eta \text{ep} \mu_1 \text{e2} - 11 \\
& \quad \eta^2 \text{ep} \mu_1 \text{e2} - 56 \eta^3 \text{ep} \mu_1 \text{e2} + 10 \eta^4 \text{ep} \mu_1 \text{e2} - 13 \eta t \\
& \quad \text{ep} \mu_1 \text{e2} - 44 \eta \eta t \text{ep} \mu_1 \text{e2} + 11 \eta^2 \eta t \text{ep} \mu_1 \text{e2} + 56
\end{aligned}$$

$$\begin{aligned}
& \eta^3 \eta t \operatorname{op} \mu_1 \mathfrak{z}2 - 10 \eta^4 \eta t \operatorname{op} \mu_1 \mathfrak{z}2 - 3 \operatorname{op} \mu_1^2 \mathfrak{z}2 - 8 \eta \\
& \operatorname{op} \mu_1^2 \mathfrak{z}2 - 3 \eta^2 \operatorname{op} \mu_1^2 \mathfrak{z}2 + 4 \eta^3 \operatorname{op} \mu_1^2 \mathfrak{z}2 + 10 \eta^4 \operatorname{op} \\
& \mu_1^2 \mathfrak{z}2 + 3 \eta t \operatorname{op} \mu_1^2 \mathfrak{z}2 + 8 \eta \eta t \operatorname{op} \mu_1^2 \mathfrak{z}2 + 3 \eta^2 \eta t \operatorname{op} \\
& \mu_1^2 \mathfrak{z}2 - 4 \eta^3 \eta t \operatorname{op} \mu_1^2 \mathfrak{z}2 - 10 \eta^4 \eta t \operatorname{op} \mu_1^2 \mathfrak{z}2 + 10 \operatorname{op} \\
& \mu_2 \mathfrak{z}2 + 10 \eta \operatorname{op} \mu_2 \mathfrak{z}2 - 20 \eta^2 \operatorname{op} \mu_2 \mathfrak{z}2 - 10 \eta t \operatorname{op} \mu_2 \\
& \mathfrak{z}2 - 10 \eta \eta t \operatorname{op} \mu_2 \mathfrak{z}2 + 20 \eta^2 \eta t \operatorname{op} \mu_2 \mathfrak{z}2 - 2 \operatorname{op} \mu_1 \mu_2 \\
& \mathfrak{z}2 + 70 \eta \operatorname{op} \mu_1 \mu_2 \mathfrak{z}2 + 52 \eta^2 \operatorname{op} \mu_1 \mu_2 \mathfrak{z}2 - 120 \eta^3 \operatorname{op} \mu_1 \\
& \mu_2 \mathfrak{z}2 + 2 \eta t \operatorname{op} \mu_1 \mu_2 \mathfrak{z}2 - 70 \eta \eta t \operatorname{op} \mu_1 \mu_2 \mathfrak{z}2 - 52 \eta^2 \\
& \eta t \operatorname{op} \mu_1 \mu_2 \mathfrak{z}2 + 120 \eta^3 \eta t \operatorname{op} \mu_1 \mu_2 \mathfrak{z}2 - w^3 (-1 + \eta)^3 \\
& (-60 + 140 \operatorname{op} - 128 \mu_1 - 16 \operatorname{op} \mu_1 + 76 \mu_1^2 - 156 \operatorname{op} \mu_1^2 + \\
& 80 \eta^3 \operatorname{op} (4 + 2 \mu_1 + 7 \mu_1^2) + 5 \mu_2 + 8 \operatorname{op} \mu_2 + 53 \mu_1 \mu_2 + \\
& 464 \operatorname{op} \mu_1 \mu_2 - 10 \operatorname{op} \mathfrak{z}1 - 22 \operatorname{op} \mu_1 \mathfrak{z}1 - 10 \operatorname{op} \mu_2 \mathfrak{z}1 - \\
& 10 \operatorname{op} \mu_1 \mu_2 \mathfrak{z}1 + 10 \operatorname{op} \mathfrak{z}2 + 22 \operatorname{op} \mu_1 \mathfrak{z}2 + 10 \operatorname{op} \mu_2 \mathfrak{z}2 + \\
& 10 \operatorname{op} \mu_1 \mu_2 \mathfrak{z}2 - \eta t (-60 - 128 \mu_1 + 76 \mu_1^2 + 5 \mu_2 + 53 \mu_1 \mu_2 + \\
& 2 \operatorname{op} (168 + 116 \mu_1^2 - 5 \mathfrak{z}1 + 5 \mathfrak{z}2 + \mu_2 (4 - 5 \mathfrak{z}1 + 5 \mathfrak{z}2) + \\
& \mu_1 (-4 - 11 \mathfrak{z}1 + 11 \mathfrak{z}2 + \mu_2 (232 - 5 \mathfrak{z}1 + 5 \mathfrak{z}2))) + \\
& 2 \eta (2 \times (-1 + \eta t) \times (4 \mu_1^2 - \mu_1 (-7 + \mu_2) + 5 \mu_2) + \operatorname{op} \\
& (248 - 232 \mu_1^2 + 28 \mu_2 - 5 \mathfrak{z}1 - 5 \mu_2 \mathfrak{z}1 + \eta t (-382 + 2 \mu_1^2 + \\
& 5 \mathfrak{z}1 + \mu_1 (16 + 11 \mathfrak{z}1 + 5 \mu_2 (-116 + \mathfrak{z}1 - \mathfrak{z}2) - 11 \mathfrak{z}2) + \\
& \mu_2 (-28 + 5 \mathfrak{z}1 - 5 \mathfrak{z}2) - 5 \mathfrak{z}2) + 5 \mathfrak{z}2 + 5 \mu_2 \mathfrak{z}2 + \\
& \mu_1 (-92 - 11 \mathfrak{z}1 + 11 \mathfrak{z}2 + \mu_2 (580 - 5 \mathfrak{z}1 + 5 \mathfrak{z}2))) + \\
& \eta^2 (60 + 156 \mu_1 - 60 \mu_1^2 + 15 \mu_2 - 57 \mu_1 \mu_2 + 4 \operatorname{op} (146 + 34 \mu_1^2 + \\
& 5 \mathfrak{z}1 + \mu_1 (-36 + 11 \mathfrak{z}1 + 5 \mu_2 (20 + \mathfrak{z}1 - \mathfrak{z}2) - 11 \mathfrak{z}2) + \\
& \mu_2 (16 + 5 \mathfrak{z}1 - 5 \mathfrak{z}2) - 5 \mathfrak{z}2) + \\
& \eta t (3 \times (20 \mu_1^2 - 5 \times (4 + \mu_2) + \mu_1 (-52 + 19 \mu_2)) + \\
& 4 \operatorname{op} (38 \mu_1^2 - 5 \times (22 + \mathfrak{z}1 - \mathfrak{z}2) + \mu_2 (-16 - 5 \mathfrak{z}1 + 5 \mathfrak{z}2) + \\
& \mu_1 (36 - 11 \mathfrak{z}1 - 5 \mu_2 (20 + \mathfrak{z}1 - \mathfrak{z}2) + 11 \mathfrak{z}2))) + \\
& w^2 (-1 + \eta)^2 (-120 + 120 \eta t + 198 \operatorname{op} - 474 \eta t \operatorname{op} - 228 \mu_1 + \\
& 228 \eta t \mu_1 + 58 \operatorname{op} \mu_1 - 34 \eta t \operatorname{op} \mu_1 + 84 \mu_1^2 - 84 \eta t \mu_1^2 - \\
& 152 \operatorname{op} \mu_1^2 - 412 \eta t \operatorname{op} \mu_1^2 + 80 \eta^4 \operatorname{op} (4 + 2 \mu_1 + 7 \mu_1^2) - \\
& 15 \mu_2 + 15 \eta t \mu_2 + 42 \operatorname{op} \mu_2 - 42 \eta t \operatorname{op} \mu_2 + 129 \mu_1 \mu_2 - \\
& 129 \eta t \mu_1 \mu_2 + 474 \operatorname{op} \mu_1 \mu_2 - 474 \eta t \operatorname{op} \mu_1 \mu_2 - 30 \operatorname{op} \mathfrak{z}1 + \\
& 30 \eta t \operatorname{op} \mathfrak{z}1 - 61 \operatorname{op} \mu_1 \mathfrak{z}1 + 61 \eta t \operatorname{op} \mu_1 \mathfrak{z}1 - \operatorname{op} \mu_1^2 \mathfrak{z}1 + \\
& \eta t \operatorname{op} \mu_1^2 \mathfrak{z}1 - 30 \operatorname{op} \mu_2 \mathfrak{z}1 + 30 \eta t \operatorname{op} \mu_2 \mathfrak{z}1 - 30 \operatorname{op} \mu_1 \mu_2 \mathfrak{z}1 + \\
& 30 \eta t \operatorname{op} \mu_1 \mu_2 \mathfrak{z}1 + 30 \operatorname{op} \mathfrak{z}2 - 30 \eta t \operatorname{op} \mathfrak{z}2 + 57 \operatorname{op} \mu_1 \mathfrak{z}2 - \\
& 57 \eta t \operatorname{op} \mu_1 \mathfrak{z}2 - 3 \operatorname{op} \mu_1^2 \mathfrak{z}2 + 3 \eta t \operatorname{op} \mu_1^2 \mathfrak{z}2 + 30 \operatorname{op} \mu_2 \mathfrak{z}2 - \\
& 30 \eta t \operatorname{op} \mu_2 \mathfrak{z}2 + 18 \operatorname{op} \mu_1 \mu_2 \mathfrak{z}2 - 18 \eta t \operatorname{op} \mu_1 \mu_2 \mathfrak{z}2 + \\
& \eta (96 \mu_1^2 - 30 \times (2 + \mu_2) + 6 \mu_1 (-40 + 7 \mu_2) - \operatorname{op} \mu_1^2 (820 + 19 \mathfrak{z}1 + \\
& 9 \mathfrak{z}2) + 6 \operatorname{op} (129 - 5 \mathfrak{z}1 + 5 \mathfrak{z}2 + \mu_2 (21 - 5 \mathfrak{z}1 + 5 \mathfrak{z}2)) + \\
& \operatorname{op} \mu_1 (-322 - 115 \mathfrak{z}1 + 87 \mathfrak{z}2 + \mu_2 (1782 - 30 \mathfrak{z}1 + 90 \mathfrak{z}2)) + \eta t \\
& (6 \times (-16 \mu_1^2 + \mu_1 (40 - 7 \mu_2) + 5 \times (2 + \mu_2)) + \operatorname{op} (-1378 + 30 \mathfrak{z}1 + \\
& \mu_1 (74 + 115 \mathfrak{z}1 + 6 \mu_2 (-297 + 5 \mathfrak{z}1 - 15 \mathfrak{z}2) - 87 \mathfrak{z}2) + 6 \mu_2 \\
& (-21 + 5 \mathfrak{z}1 - 5 \mathfrak{z}2) - 30 \mathfrak{z}2 + \mu_1^2 (-264 + 19 \mathfrak{z}1 + 9 \mathfrak{z}2))) - \\
& 2 \eta^3 (-12 \times (-1 + \eta t) \times (-5 + \mu_1) \mu_1 + 5 \operatorname{op} (-2 \times (53 + 5 \mu_2) - \\
& \mu_1^2 (116 + 3 \mathfrak{z}1 + \mathfrak{z}2) + \mu_1 (-18 - 9 \mathfrak{z}1 + 5 \mathfrak{z}2 + 2 \mu_2 (7 + 6 \mathfrak{z}2)) +
\end{aligned}$$



$$\begin{aligned}
& \eta t \left( 42 + 10 \mu_2 + \mu_1^2 (4 + 3 \mathfrak{e}_1 + \mathfrak{e}_2) - \right. \\
& \quad \left. \mu_1 (14 - 9 \mathfrak{e}_1 + 5 \mathfrak{e}_2 + 2 \mu_2 (7 + 6 \mathfrak{e}_2)) \right) + \\
& \eta^2 \left( 3 \times (-52 \mu_1^2 + \mu_1 (116 - 57 \mu_2) + 15 \times (4 + \mu_2)) - 2 \theta p \right. \\
& \quad (-6 \times (97 + 5 \mathfrak{e}_1 - 5 \mathfrak{e}_2) + \mu_1^2 (184 + 5 \mathfrak{e}_1 - \mathfrak{e}_2) + \\
& \quad \mu_2 (-58 - 30 \mathfrak{e}_1 + 30 \mathfrak{e}_2) - \mu_1 (-358 + 43 \mathfrak{e}_1 - 47 \mathfrak{e}_2 + \\
& \quad \mu_2 (682 + 30 \mathfrak{e}_1 + 6 \mathfrak{e}_2)) + \eta t \left( 3 \times (52 \mu_1^2 - \right. \\
& \quad 15 \times (4 + \mu_2) + \mu_1 (-116 + 57 \mu_2)) + 2 \theta p (-622 - 30 \mathfrak{e}_1 + \\
& \quad \mu_1^2 (168 + 5 \mathfrak{e}_1 - \mathfrak{e}_2) + 30 \mathfrak{e}_2 + \mu_2 (-58 - 30 \mathfrak{e}_1 + 30 \mathfrak{e}_2) - \\
& \quad \mu_1 (-230 + 43 \mathfrak{e}_1 - 47 \mathfrak{e}_2 + \mu_2 (682 + 30 \mathfrak{e}_1 + 6 \mathfrak{e}_2))) \left. \right) + w \\
& (-1 + \eta) \times (100 - 100 \eta t - 128 \theta p + 300 \eta t \theta p + 152 \mu_1 - 152 \eta t \mu_1 - \\
& \quad 92 \theta p \mu_1 + 52 \eta t \theta p \mu_1 - 44 \mu_1^2 + 44 \eta t \mu_1^2 + 60 \theta p \mu_1^2 + \\
& \quad 304 \eta t \theta p \mu_1^2 + 25 \mu_2 - 25 \eta t \mu_2 - 56 \theta p \mu_2 + 56 \eta t \theta p \mu_2 - \\
& \quad 119 \mu_1 \mu_2 + 119 \eta t \mu_1 \mu_2 - 152 \theta p \mu_1 \mu_2 + 152 \eta t \theta p \mu_1 \mu_2 + \\
& \quad 30 \theta p \mathfrak{e}_1 - 30 \eta t \theta p \mathfrak{e}_1 + 56 \theta p \mu_1 \mathfrak{e}_1 - 56 \eta t \theta p \mu_1 \mathfrak{e}_1 + \\
& \quad 2 \theta p \mu_1^2 \mathfrak{e}_1 - 2 \eta t \theta p \mu_1^2 \mathfrak{e}_1 + 30 \theta p \mu_2 \mathfrak{e}_1 - 30 \eta t \theta p \mu_2 \mathfrak{e}_1 + \\
& \quad 30 \theta p \mu_1 \mu_2 \mathfrak{e}_1 - 30 \eta t \theta p \mu_1 \mu_2 \mathfrak{e}_1 - 30 \theta p \mathfrak{e}_2 + 30 \eta t \theta p \mathfrak{e}_2 - \\
& \quad 48 \theta p \mu_1 \mathfrak{e}_2 + 48 \eta t \theta p \mu_1 \mathfrak{e}_2 + 6 \theta p \mu_1^2 \mathfrak{e}_2 - 6 \eta t \theta p \mu_1^2 \mathfrak{e}_2 - \\
& \quad 30 \theta p \mu_2 \mathfrak{e}_2 + 30 \eta t \theta p \mu_2 \mathfrak{e}_2 - 6 \theta p \mu_1 \mu_2 \mathfrak{e}_2 + 6 \eta t \theta p \mu_1 \mu_2 \mathfrak{e}_2 + \\
& \quad 2 \eta^4 (-12 \times (-1 + \eta t) \mu_1 (1 + \mu_1) + 5 \theta p (-64 + 2 \times (-1 + \eta t) \mu_2 - \\
& \quad \mu_1 (54 - 10 \mu_2 + \mathfrak{e}_1 + \eta t (-22 + 10 \mu_2 - \mathfrak{e}_1 - \mathfrak{e}_2) + \mathfrak{e}_2) + \\
& \quad \mu_1^2 (-110 - \mathfrak{e}_1 - \mathfrak{e}_2 + \eta t (-2 + \mathfrak{e}_1 + \mathfrak{e}_2))) + \\
& \quad 2 \eta^3 (-12 \times (-1 + \eta t) \times (-11 + \mu_1) \mu_1 + \theta p (-540 - 74 \mu_2 - \\
& \quad \mu_1^2 (374 + 27 \mathfrak{e}_1 + 7 \mathfrak{e}_2) + \mu_1 (166 + 10 \mu_2 - 87 \mathfrak{e}_1 + 53 \mathfrak{e}_2 + \\
& \quad 120 \mu_2 \mathfrak{e}_2) + \eta t (380 + 74 \mu_2 + \mu_1^2 (94 + 27 \mathfrak{e}_1 + 7 \mathfrak{e}_2) - \\
& \quad \mu_1 (246 + 10 \mu_2 - 87 \mathfrak{e}_1 + 53 \mathfrak{e}_2 + 120 \mu_2 \mathfrak{e}_2))) + \\
& \eta^2 (-180 - 232 \mu_1 + 128 \mu_1^2 - 45 \mu_2 + 171 \mu_1 \mu_2 + \theta p \\
& \quad (-6 \mu_2 (9 + 10 \mathfrak{e}_1 - 10 \mathfrak{e}_2) - 20 \times (44 + 3 \mathfrak{e}_1 - 3 \mathfrak{e}_2) + \\
& \quad \mu_1^2 (690 + 25 \mathfrak{e}_1 + \mathfrak{e}_2) - \mu_1 (-914 + 35 \mathfrak{e}_1 - 61 \mathfrak{e}_2 + \\
& \quad 6 \mu_2 (243 + 10 \mathfrak{e}_1 + 14 \mathfrak{e}_2))) + \eta t (-128 \mu_1^2 + \\
& \quad \mu_1 (232 - 171 \mu_2) + 45 \times (4 + \mu_2) + \theta p (1216 + 60 \mathfrak{e}_1 + \\
& \quad 6 \mu_2 (9 + 10 \mathfrak{e}_1 - 10 \mathfrak{e}_2) - 60 \mathfrak{e}_2 - \mu_1^2 (210 + 25 \mathfrak{e}_1 + \mathfrak{e}_2) + \\
& \quad \mu_1 (-530 + 35 \mathfrak{e}_1 - 61 \mathfrak{e}_2 + 6 \mu_2 (243 + 10 \mathfrak{e}_1 + 14 \mathfrak{e}_2))) \left. \right) + \\
& \eta (4 \times (-33 \mu_1^2 + \mu_1 (80 - 13 \mu_2) + 5 \times (4 + \mu_2)) + \theta p (-548 + \\
& \quad 30 \mathfrak{e}_1 + \mu_1 (66 + 163 \mathfrak{e}_1 + 2 \mu_2 (-563 + 15 \mathfrak{e}_1 - 75 \mathfrak{e}_2) - 109 \mathfrak{e}_2) + \\
& \quad 2 \mu_2 (-53 + 15 \mathfrak{e}_1 - 15 \mathfrak{e}_2) - 30 \mathfrak{e}_2 + \mu_1^2 (518 + 37 \mathfrak{e}_1 + 17 \mathfrak{e}_2)) + \\
& \eta t (4 \times (33 \mu_1^2 - 5 \times (4 + \mu_2) + \mu_1 (-80 + 13 \mu_2)) + \\
& \quad \theta p (1000 - 30 \mathfrak{e}_1 + \mu_1^2 (318 - 37 \mathfrak{e}_1 - 17 \mathfrak{e}_2) + 30 \mathfrak{e}_2 + \\
& \quad \mu_2 (106 - 30 \mathfrak{e}_1 + 30 \mathfrak{e}_2) + \mu_1 (70 - 163 \mathfrak{e}_1 + 109 \mathfrak{e}_2 + \\
& \quad \mu_2 (1126 - 30 \mathfrak{e}_1 + 150 \mathfrak{e}_2)))))) \left. \right) / \\
& (96 (-1 + w (-1 + \eta))^3 (x (-1 + \eta) - \eta)^3 (1 + x + \eta - x \eta)^2 \\
& (w + \\
& \quad x + \\
& \quad \eta - \\
& \quad w
\end{aligned}$$

$$\eta - x$$

$$\eta)^3 (-1 + \eta t) \theta p) \Big)$$

$$\beta_{\mathfrak{L}1} =$$

$$\begin{aligned} & - \Big( \Big( cv \, c \sigma \, (x \, (-1 + \eta) - \eta) \, (-1 + \eta) \, (1 + x + \eta - x \, \eta)^2 \, \Big( (x + \eta - x \, \eta)^4 \, (-1 + \eta t) \, \theta l \, \theta p \, (2 \times (-1 + \\ & \quad \eta) \times (1 + \mu_1 - 32 \, \mu_2 + 7 \, \mathfrak{L}1 + 7 \, \mu_1 \, \mathfrak{L}1) - 2 \, \eta \, (1 + \mu_1 - 32 \, \mu_2 + 7 \, \mathfrak{L}1 + 7 \, \mu_1 \, \mathfrak{L}1) - \\ & \quad (11 + 8 \, \mu_2 + 5 \, \mathfrak{L}1 + \mu_1 \, (11 + 5 \, \mathfrak{L}1)) \times (2 + \mathfrak{L}1 + \mathfrak{L}2) \Big) - w \, (x \, (-1 + \eta) - \eta) \, (-1 + \eta) \times \\ & \quad (4 \, x^4 \, (-1 + \eta)^4 \, \theta p \, (29 - 30 \, \theta l + 29 \, \mu_1 - 30 \, \theta l \, \mu_1 + 72 \, \mu_2 - 40 \, \theta l \, \mu_2 + \mathfrak{L}1 - 8 \, \theta l \, \mathfrak{L}1 + \\ & \quad 7 \, \mu_1 \, \mathfrak{L}1 - 14 \, \theta l \, \mu_1 \, \mathfrak{L}1 + 4 \, \theta l \, \mu_2 \, \mathfrak{L}1 + 3 \, \eta^2 \, (9 + 28 \, \mu_2 + \mathfrak{L}1 + \mu_1 \, (9 + \mathfrak{L}1)) - \eta \\ & \quad (56 + 56 \, \mu_1 + 156 \, \mu_2 + 4 \, \mathfrak{L}1 + 10 \, \mu_1 \, \mathfrak{L}1 - 2 \, \theta l \, (9 + 28 \, \mu_2 + \mathfrak{L}1 + \mu_1 \, (9 + \mathfrak{L}1)) + \\ & \quad \eta t \, (1 + 2 \, \theta l) \times (9 + 28 \, \mu_2 + \mathfrak{L}1 + \mu_1 \, (9 + \mathfrak{L}1)) + \eta t \, (9 + 28 \, \mu_2 + \mathfrak{L}1 + \\ & \quad \mu_1 \, (9 + \mathfrak{L}1) + 2 \, \theta l \, (15 + 20 \, \mu_2 + 4 \, \mathfrak{L}1 - 2 \, \mu_2 \, \mathfrak{L}1 + \mu_1 \, (15 + 7 \, \mathfrak{L}1))) \Big) - \\ & \quad x^3 \, (-1 + \eta)^3 \, \theta p \, (48 \, \eta^3 \, (9 + 28 \, \mu_2 + \mathfrak{L}1 + \mu_1 \, (9 + \mathfrak{L}1)) - 16 \, \eta^2 \, (56 + 56 \, \mu_1 + 156 \, \mu_2 + \\ & \quad 4 \, \mathfrak{L}1 + 10 \, \mu_1 \, \mathfrak{L}1 - 2 \, \theta l \, (9 + 28 \, \mu_2 + \mathfrak{L}1 + \mu_1 \, (9 + \mathfrak{L}1)) + \eta t \, (1 + 2 \, \theta l) \times \\ & \quad (9 + 28 \, \mu_2 + \mathfrak{L}1 + \mu_1 \, (9 + \mathfrak{L}1))) + 16 \, \eta \, (29 + 29 \, \mu_1 + 72 \, \mu_2 + \mathfrak{L}1 + 7 \, \mu_1 \, \mathfrak{L}1 - \\ & \quad 2 \, \theta l \, (15 - 2 \, \mu_2 \, (-10 + \mathfrak{L}1) + 4 \, \mathfrak{L}1 + \mu_1 \, (15 + 7 \, \mathfrak{L}1)) + \eta t \, (9 + 28 \, \mu_2 + \mathfrak{L}1 + \\ & \quad \mu_1 \, (9 + \mathfrak{L}1) + 2 \, \theta l \, (15 + 20 \, \mu_2 + 4 \, \mathfrak{L}1 - 2 \, \mu_2 \, \mathfrak{L}1 + \mu_1 \, (15 + 7 \, \mathfrak{L}1))) + \\ & \quad 3 \times (-1 + \eta t) \, \theta l \, (24 + 35 \, \mathfrak{L}1 + 5 \, \mathfrak{L}1^2 + 11 \, \mathfrak{L}2 + 5 \, \mathfrak{L}1 \, \mathfrak{L}2 + 8 \, \mu_2 \\ & \quad (-6 + \mathfrak{L}1 + \mathfrak{L}2) + \mu_1 \, (24 + 5 \, \mathfrak{L}1^2 + 11 \, \mathfrak{L}2 + 5 \, \mathfrak{L}1 \, (7 + \mathfrak{L}2))) \Big) \Big) - \\ & \quad x \, (-1 + \eta) \times \Big( 48 \, \eta^5 \, \theta p \, (9 + 28 \, \mu_2 + \mathfrak{L}1 + \mu_1 \, (9 + \mathfrak{L}1)) + 4 \, \eta t \, \theta p \\ & \quad (19 + 40 \, \mu_2 + 5 \, \mathfrak{L}1 + \mu_1 \, (19 + 5 \, \mathfrak{L}1)) - 16 \, \eta^4 \, \theta p \\ & \quad (56 + 56 \, \mu_1 + 156 \, \mu_2 + 4 \, \mathfrak{L}1 + 10 \, \mu_1 \, \mathfrak{L}1 - 2 \, \theta l \, (9 + 28 \, \mu_2 + \mathfrak{L}1 + \mu_1 \, (9 + \mathfrak{L}1)) + \\ & \quad \eta t \, (1 + 2 \, \theta l) \times (9 + 28 \, \mu_2 + \mathfrak{L}1 + \mu_1 \, (9 + \mathfrak{L}1))) + 16 \, \eta^3 \, \theta p \\ & \quad (29 + 29 \, \mu_1 + 72 \, \mu_2 + \mathfrak{L}1 + 7 \, \mu_1 \, \mathfrak{L}1 - 2 \, \theta l \, (15 - 2 \, \mu_2 \, (-10 + \mathfrak{L}1) + \\ & \quad 4 \, \mathfrak{L}1 + \mu_1 \, (15 + 7 \, \mathfrak{L}1)) + \eta t \, (9 + 28 \, \mu_2 + \mathfrak{L}1 + \mu_1 \, (9 + \mathfrak{L}1) + \\ & \quad 2 \, \theta l \, (15 + 20 \, \mu_2 + 4 \, \mathfrak{L}1 - 2 \, \mu_2 \, \mathfrak{L}1 + \mu_1 \, (15 + 7 \, \mathfrak{L}1))) + 9 \\ & \quad \eta^2 \, (-1 + \eta t) \, \theta l \, \theta p \, (24 + 35 \, \mathfrak{L}1 + 5 \, \mathfrak{L}1^2 + 11 \, \mathfrak{L}2 + 5 \, \mathfrak{L}1 \, \mathfrak{L}2 + \\ & \quad 8 \, \mu_2 \, (-6 + \mathfrak{L}1 + \mathfrak{L}2) + \mu_1 \, (24 + 5 \, \mathfrak{L}1^2 + 11 \, \mathfrak{L}2 + 5 \, \mathfrak{L}1 \, (7 + \mathfrak{L}2))) + 4 \\ & \quad \eta \, (-\eta t \, \theta p \, (19 + 40 \, \mu_2 + 5 \, \mathfrak{L}1 + \mu_1 \, (19 + 5 \, \mathfrak{L}1)) + (-1 + \eta t) \, \theta l \\ & \quad (-3 - 3 \, \mu_1 + 8 \, \mu_2 - 5 \, \mathfrak{L}1 - 5 \, \mu_1 \, \mathfrak{L}1 + 2 \, \theta p \, (22 + 21 \, \mathfrak{L}1 + 5 \, \mathfrak{L}1^2 + 6 \, \mathfrak{L}2 + 4 \, \mu_2 \\ & \quad (6 + 3 \, \mathfrak{L}1 + 2 \, \mathfrak{L}2) + \mu_1 \, (22 + 5 \, \mathfrak{L}1^2 + 6 \, \mathfrak{L}2 + 3 \, \mathfrak{L}1 \, (7 + 2 \, \mathfrak{L}2)))) \Big) \Big) + \\ & \quad \eta \, \theta p \, (12 \, \eta^5 \, (9 + 28 \, \mu_2 + \mathfrak{L}1 + \mu_1 \, (9 + \mathfrak{L}1)) + 4 \, \eta t \, (7 + 4 \, \mu_2 + 5 \, \mathfrak{L}1 + \\ & \quad \mu_1 \, (7 + 5 \, \mathfrak{L}1)) - 4 \, \eta^4 \, (56 + 56 \, \mu_1 + 156 \, \mu_2 + 4 \, \mathfrak{L}1 + 10 \, \mu_1 \, \mathfrak{L}1 - \\ & \quad 2 \, \theta l \, (9 + 28 \, \mu_2 + \mathfrak{L}1 + \mu_1 \, (9 + \mathfrak{L}1)) + \eta t \, (1 + 2 \, \theta l) \times \\ & \quad (9 + 28 \, \mu_2 + \mathfrak{L}1 + \mu_1 \, (9 + \mathfrak{L}1))) + 4 \, \eta^3 \, (29 + 29 \, \mu_1 + 72 \, \mu_2 + \mathfrak{L}1 + 7 \, \mu_1 \, \mathfrak{L}1 - \\ & \quad 2 \, \theta l \, (15 - 2 \, \mu_2 \, (-10 + \mathfrak{L}1) + 4 \, \mathfrak{L}1 + \mu_1 \, (15 + 7 \, \mathfrak{L}1)) + \eta t \, (9 + 28 \, \mu_2 + \mathfrak{L}1 + \\ & \quad \mu_1 \, (9 + \mathfrak{L}1) + 2 \, \theta l \, (15 + 20 \, \mu_2 + 4 \, \mathfrak{L}1 - 2 \, \mu_2 \, \mathfrak{L}1 + \mu_1 \, (15 + 7 \, \mathfrak{L}1))) + 3 \\ & \quad \eta^2 \, (-1 + \eta t) \, \theta l \, (24 + 35 \, \mathfrak{L}1 + 5 \, \mathfrak{L}1^2 + 11 \, \mathfrak{L}2 + 5 \, \mathfrak{L}1 \, \mathfrak{L}2 + 8 \, \mu_2 \, (-6 + \mathfrak{L}1 + \mathfrak{L}2) + \\ & \quad \mu_1 \, (24 + 5 \, \mathfrak{L}1^2 + 11 \, \mathfrak{L}2 + 5 \, \mathfrak{L}1 \, (7 + \mathfrak{L}2))) + 4 \, \eta \, (-\theta l \, (18 + 19 \, \mathfrak{L}1 + 5 \, \mathfrak{L}1^2 + \\ & \quad 4 \, \mathfrak{L}2 + 2 \, \mu_2 \, (6 + 3 \, \mathfrak{L}1 + \mathfrak{L}2) + \mu_1 \, (18 + 5 \, \mathfrak{L}1^2 + 4 \, \mathfrak{L}2 + \mathfrak{L}1 \, (19 + 6 \, \mathfrak{L}2))) + \\ & \quad \eta t \, (-7 - 7 \, \mu_1 - 4 \, \mu_2 - 5 \, \mathfrak{L}1 - 5 \, \mu_1 \, \mathfrak{L}1 + \theta l \, (18 + 19 \, \mathfrak{L}1 + 5 \, \mathfrak{L}1^2 + 4 \, \mathfrak{L}2 + 2 \, \mu_2 \\ & \quad (6 + 3 \, \mathfrak{L}1 + \mathfrak{L}2) + \mu_1 \, (18 + 5 \, \mathfrak{L}1^2 + 4 \, \mathfrak{L}2 + \mathfrak{L}1 \, (19 + 6 \, \mathfrak{L}2)))) \Big) \Big) + \\ & \quad x^2 \, (-1 + \eta)^2 \, (24 \times (-1 + \eta) \, \eta^2 \, \theta p \, (-29 - 29 \, \mu_1 - 72 \, \mu_2 - \mathfrak{L}1 - 7 \, \mu_1 \, \mathfrak{L}1 + \\ & \quad 3 \, \eta \, (9 + 28 \, \mu_2 + \mathfrak{L}1 + \mu_1 \, (9 + \mathfrak{L}1)) - \eta t \, (9 + 28 \, \mu_2 + \mathfrak{L}1 + \mu_1 \, (9 + \mathfrak{L}1)) - \\ & \quad (-1 + \eta t) \, \theta l \, (4 \times (28 \, \mu_2 + 5 \times (3 + \mathfrak{L}1) + 5 \, \mu_1 \, (3 + \mathfrak{L}1)) + \end{aligned}$$

$$\begin{aligned}
& \text{op} \left( 48 \eta^3 (9 + 28 \mu_2 + \mathfrak{e}1 + \mu_1 (9 + \mathfrak{e}1)) - 48 \eta^2 (15 - 2 \mu_2 (-10 + \mathfrak{e}1) + \right. \\
& \quad 4 \mathfrak{e}1 + \mu_1 (15 + 7 \mathfrak{e}1)) - 9 \eta (24 + 35 \mathfrak{e}1 + 5 \mathfrak{e}1^2 + 11 \mathfrak{e}2 + 5 \mathfrak{e}1 \mathfrak{e}2 + \\
& \quad 8 \mu_2 (-6 + \mathfrak{e}1 + \mathfrak{e}2) + \mu_1 (24 + 5 \mathfrak{e}1^2 + 11 \mathfrak{e}2 + 5 \mathfrak{e}1 (7 + \mathfrak{e}2))) - \\
& \quad 4 \times (26 + 23 \mathfrak{e}1 + 5 \mathfrak{e}1^2 + 8 \mathfrak{e}2 + 2 \mu_2 (18 + 9 \mathfrak{e}1 + 7 \mathfrak{e}2) + \\
& \quad \left. \mu_1 (26 + 5 \mathfrak{e}1^2 + 8 \mathfrak{e}2 + \mathfrak{e}1 (23 + 6 \mathfrak{e}2))) \right) + \\
& w^5 (-1 + \eta)^5 \left( x^2 (-1 + \eta)^2 \left( 4 \times (-1 + \eta) \text{op} (-7 - 7 \mu_1 + \mathfrak{e}1 - 5 \mu_1 \mathfrak{e}1 + \right. \right. \\
& \quad \eta (9 + 28 \mu_2 + \mathfrak{e}1 + \mu_1 (9 + \mathfrak{e}1)) - \eta t (9 + 28 \mu_2 + \mathfrak{e}1 + \mu_1 (9 + \mathfrak{e}1))) + \\
& \quad (-1 + \eta t) \text{el} (-4 \times (3 - 8 \mu_2 + 5 \mathfrak{e}1 + \mu_1 (3 + 5 \mathfrak{e}1)) + \\
& \quad \text{op} (64 + 57 \mathfrak{e}1 + 15 \mathfrak{e}1^2 - 3 \mathfrak{e}2 - 5 \mathfrak{e}1 \mathfrak{e}2 - 8 \mu_2 (10 + 3 \mathfrak{e}1 + 3 \mathfrak{e}2) + \\
& \quad \left. \mu_1 (64 + 15 \mathfrak{e}1^2 - 3 \mathfrak{e}2 + \mathfrak{e}1 (81 + 19 \mathfrak{e}2))) \right) + \\
& \eta \text{op} (4 \eta^3 (9 + 28 \mu_2 + \mathfrak{e}1 + \mu_1 (9 + \mathfrak{e}1)) + 4 \eta t (3 - 8 \mu_2 + 5 \mathfrak{e}1 + \mu_1 (3 + 5 \mathfrak{e}1)) - \\
& \quad 4 \eta^2 (\eta t (9 + 28 \mu_2 + \mathfrak{e}1 + \mu_1 (9 + \mathfrak{e}1)) + 2 \times (8 + 14 \mu_2 + \mu_1 (8 + 3 \mathfrak{e}1))) + \eta \\
& \quad (4 \times (7 - \mathfrak{e}1 + \mu_1 (7 + 5 \mathfrak{e}1)) + \text{el} (-64 - 57 \mathfrak{e}1 - 15 \mathfrak{e}1^2 + 3 \mathfrak{e}2 + 5 \mathfrak{e}1 \mathfrak{e}2 + \\
& \quad 8 \mu_2 (10 + 3 \mathfrak{e}1 + 3 \mathfrak{e}2) - \mu_1 (64 + 15 \mathfrak{e}1^2 - 3 \mathfrak{e}2 + \mathfrak{e}1 (81 + 19 \mathfrak{e}2))) + \\
& \quad \eta t (8 \times (3 + 18 \mu_2 + \mu_1 (3 - 2 \mathfrak{e}1) - 2 \mathfrak{e}1) + \text{el} (64 + 57 \mathfrak{e}1 + \\
& \quad 15 \mathfrak{e}1^2 - 3 \mathfrak{e}2 - 5 \mathfrak{e}1 \mathfrak{e}2 - 8 \mu_2 (10 + 3 \mathfrak{e}1 + 3 \mathfrak{e}2) + \\
& \quad \left. \mu_1 (64 + 15 \mathfrak{e}1^2 - 3 \mathfrak{e}2 + \mathfrak{e}1 (81 + 19 \mathfrak{e}2))) \right) - \\
& 2 \times (-1 + \eta) \times (4 \eta^3 \text{op} (9 + 28 \mu_2 + \mathfrak{e}1 + \mu_1 (9 + \mathfrak{e}1)) + 2 \eta t \text{op} \\
& \quad (7 + 4 \mu_2 + 5 \mathfrak{e}1 + \mu_1 (7 + 5 \mathfrak{e}1)) - 4 \eta^2 \text{op} (\eta t (9 + 28 \mu_2 + \mathfrak{e}1 + \mu_1 (9 + \mathfrak{e}1)) + \\
& \quad 2 \times (8 + 14 \mu_2 + \mu_1 (8 + 3 \mathfrak{e}1))) + \eta (2 \text{op} \\
& \quad (\eta t (11 + 52 \mu_2 + \mu_1 (11 - 3 \mathfrak{e}1) - 3 \mathfrak{e}1) + 2 \times (7 - \mathfrak{e}1 + \mu_1 (7 + 5 \mathfrak{e}1))) + \\
& \quad (-1 + \eta t) \text{el} (2 \times (1 + \mu_1 + 20 \mu_2 - 5 \mathfrak{e}1 - 5 \mu_1 \mathfrak{e}1) + \\
& \quad \text{op} (64 + 57 \mathfrak{e}1 + 15 \mathfrak{e}1^2 - 3 \mathfrak{e}2 - 5 \mathfrak{e}1 \mathfrak{e}2 - 8 \mu_2 (10 + 3 \mathfrak{e}1 + 3 \mathfrak{e}2) + \\
& \quad \left. \mu_1 (64 + 15 \mathfrak{e}1^2 - 3 \mathfrak{e}2 + \mathfrak{e}1 (81 + 19 \mathfrak{e}2))) \right) + \\
& w^2 (-1 + \eta)^2 \left( 2 x^5 (-1 + \eta)^5 \text{op} (14 - 15 \text{el} + 14 \mu_1 - 15 \text{el} \mu_1 + 32 \text{el} \right. \\
& \quad \mu_2 - 2 \mathfrak{e}1 - 5 \text{el} \mathfrak{e}1 + 10 \mu_1 \mathfrak{e}1 - 17 \text{el} \mu_1 \mathfrak{e}1 + 8 \text{el} \mu_2 \mathfrak{e}1 + 2 \eta^2 \\
& \quad (9 + 28 \mu_2 + \mathfrak{e}1 + \mu_1 (9 + \mathfrak{e}1)) + 2 \eta t (9 + 28 \mu_2 + \mathfrak{e}1 + \mu_1 (9 + \mathfrak{e}1)) + \eta t \\
& \quad \text{el} (5 \times (3 + \mathfrak{e}1) - 8 \mu_2 (4 + \mathfrak{e}1) + \mu_1 (15 + 17 \mathfrak{e}1)) - 2 \eta \\
& \quad \left. (\eta t (9 + 28 \mu_2 + \mathfrak{e}1 + \mu_1 (9 + \mathfrak{e}1)) + 2 \times (8 + 14 \mu_2 + \mu_1 (8 + 3 \mathfrak{e}1))) \right) - \\
& x^4 (-1 + \eta)^4 \text{op} (20 \eta^3 (9 + 28 \mu_2 + \mathfrak{e}1 + \mu_1 (9 + \mathfrak{e}1)) - 4 \eta^2 \\
& \quad (-1 - 112 \mu_2 - 9 \mathfrak{e}1 + \mu_1 (-1 + 21 \mathfrak{e}1) + 5 \eta t (9 + 28 \mu_2 + \mathfrak{e}1 + \mu_1 (9 + \mathfrak{e}1))) + \\
& 2 \eta (4 \eta t (9 + 28 \mu_2 + \mathfrak{e}1 + \mu_1 (9 + \mathfrak{e}1)) + \text{el} (33 + \mu_1 (33 - 73 \mathfrak{e}1) - \\
& \quad 13 \mathfrak{e}1 + 8 \mu_2 (62 + 5 \mathfrak{e}1)) - \eta t \text{el} (33 + \mu_1 (33 - 73 \mathfrak{e}1) - 13 \mathfrak{e}1 + \\
& \quad 8 \mu_2 (62 + 5 \mathfrak{e}1)) - 2 \times (133 + 468 \mu_2 + 17 \mathfrak{e}1 + \mu_1 (133 + 5 \mathfrak{e}1))) + 3 \times \\
& \quad (4 \times (29 + 72 \mu_2 + \mathfrak{e}1 + \mu_1 (29 + 7 \mathfrak{e}1)) - \text{el} (142 + 53 \mathfrak{e}1 + 5 \mathfrak{e}1^2 - \\
& \quad 8 \mu_2 (-22 + \mathfrak{e}1 - \mathfrak{e}2) + 11 \mathfrak{e}2 + 5 \mathfrak{e}1 \mathfrak{e}2 + \mu_1 (142 + 5 \mathfrak{e}1^2 + 11 \mathfrak{e}2 + \\
& \quad \mathfrak{e}1 (77 + 5 \mathfrak{e}2))) + \eta t (4 \times (9 + 28 \mu_2 + \mathfrak{e}1 + \mu_1 (9 + \mathfrak{e}1)) + \\
& \quad \text{el} (142 + 53 \mathfrak{e}1 + 5 \mathfrak{e}1^2 - 8 \mu_2 (-22 + \mathfrak{e}1 - \mathfrak{e}2) + 11 \mathfrak{e}2 + \\
& \quad 5 \mathfrak{e}1 \mathfrak{e}2 + \mu_1 (142 + 5 \mathfrak{e}1^2 + 11 \mathfrak{e}2 + \mathfrak{e}1 (77 + 5 \mathfrak{e}2)))) + \\
& 2 x^3 (-1 + \eta)^3 \left( 4 \times (-1 + \eta) \eta \text{op} (5 \eta^2 (9 + 28 \mu_2 + \mathfrak{e}1 + \mu_1 (9 + \mathfrak{e}1)) - \right. \\
& \quad 6 \times (29 + 29 \mu_1 + 72 \mu_2 + \mathfrak{e}1 + 7 \mu_1 \mathfrak{e}1 + \eta t (9 + 28 \mu_2 + \mathfrak{e}1 + \mu_1 (9 + \mathfrak{e}1))) - \\
& \quad \eta (-127 - 127 \mu_1 - 504 \mu_2 - 23 \mathfrak{e}1 + 7 \mu_1 \mathfrak{e}1 + \\
& \quad \left. 5 \eta t (9 + 28 \mu_2 + \mathfrak{e}1 + \mu_1 (9 + \mathfrak{e}1))) \right) + \\
& (-1 + \eta t) \text{el} (-6 \times (28 \mu_2 + 5 \times (3 + \mathfrak{e}1) + 5 \mu_1 (3 + \mathfrak{e}1)) +
\end{aligned}$$

$$\begin{aligned}
& \theta p \left( 2 \eta^2 (-141 + \mathfrak{d}1 - 8 \mu 2 (104 + 5 \mathfrak{d}1) + \mu 1 (-141 + 61 \mathfrak{d}1)) + \right. \\
& \quad 6 \eta \left( 142 + 53 \mathfrak{d}1 + 5 \mathfrak{d}1^2 - 8 \mu 2 (-22 + \mathfrak{d}1 - \mathfrak{d}2) + 11 \mathfrak{d}2 + \right. \\
& \quad \quad \left. 5 \mathfrak{d}1 \mathfrak{d}2 + \mu 1 (142 + 5 \mathfrak{d}1^2 + 11 \mathfrak{d}2 + \mathfrak{d}1 (77 + 5 \mathfrak{d}2)) \right) + \\
& \quad \left. 3 \times (53 + 53 \mathfrak{d}1 + 10 \mathfrak{d}1^2 + 16 \mathfrak{d}2 + 4 \mu 2 (10 + 9 \mathfrak{d}1 + 7 \mathfrak{d}2) + \right. \\
& \quad \quad \left. \mu 1 (53 + 10 \mathfrak{d}1^2 + 16 \mathfrak{d}2 + \mathfrak{d}1 (53 + 12 \mathfrak{d}2))) \right) - \\
& \eta \theta p \left( 4 \eta^6 (9 + 28 \mu 2 + \mathfrak{d}1 + \mu 1 (9 + \mathfrak{d}1)) + 4 \eta t (3 - 8 \mu 2 + 5 \mathfrak{d}1 + \right. \\
& \quad \mu 1 (3 + 5 \mathfrak{d}1)) - 4 \eta^5 (-65 - 224 \mu 2 - 9 \mathfrak{d}1 - \\
& \quad \mu 1 (65 + 3 \mathfrak{d}1) + \eta t (9 + 28 \mu 2 + \mathfrak{d}1 + \mu 1 (9 + \mathfrak{d}1))) + 2 \eta^4 \\
& \quad (-4 \eta t (9 + 28 \mu 2 + \mathfrak{d}1 + \mu 1 (9 + \mathfrak{d}1)) + \theta l (93 + \mu 1 (93 - 5 \mathfrak{d}1) + 7 \mathfrak{d}1 + \\
& \quad \quad 8 \mu 2 (46 + \mathfrak{d}1)) - \eta t \theta l (93 + \mu 1 (93 - 5 \mathfrak{d}1) + 7 \mathfrak{d}1 + 8 \mu 2 (46 + \mathfrak{d}1)) - \\
& \quad \quad 2 \times (161 + 468 \mu 2 + 13 \mathfrak{d}1 + \mu 1 (161 + 25 \mathfrak{d}1))) + 6 \eta^2 \\
& \quad (-\theta l (37 + 45 \mathfrak{d}1 + 10 \mathfrak{d}1^2 + 8 \mathfrak{d}2 + 4 \mu 2 (-2 + 3 \mathfrak{d}1 + \mathfrak{d}2) + \\
& \quad \quad \mu 1 (37 + 10 \mathfrak{d}1^2 + 8 \mathfrak{d}2 + 3 \mathfrak{d}1 (15 + 4 \mathfrak{d}2))) + \eta t (-2 \times (7 + 4 \mu 2 + \\
& \quad \quad 5 \mathfrak{d}1 + \mu 1 (7 + 5 \mathfrak{d}1)) + \theta l (37 + 45 \mathfrak{d}1 + 10 \mathfrak{d}1^2 + 8 \mathfrak{d}2 + 4 \mu 2 (-2 + \\
& \quad \quad 3 \mathfrak{d}1 + \mathfrak{d}2) + \mu 1 (37 + 10 \mathfrak{d}1^2 + 8 \mathfrak{d}2 + 3 \mathfrak{d}1 (15 + 4 \mathfrak{d}2)))) + \\
& 3 \eta^3 (4 \times (29 + 72 \mu 2 + \mathfrak{d}1 + \mu 1 (29 + 7 \mathfrak{d}1)) - \theta l (142 + 53 \mathfrak{d}1 + \\
& \quad 5 \mathfrak{d}1^2 - 8 \mu 2 (-22 + \mathfrak{d}1 - \mathfrak{d}2) + 11 \mathfrak{d}2 + 5 \mathfrak{d}1 \mathfrak{d}2 + \mu 1 (142 + 5 \mathfrak{d}1^2 + \\
& \quad \quad 11 \mathfrak{d}2 + \mathfrak{d}1 (77 + 5 \mathfrak{d}2))) + \eta t (4 \times (9 + 28 \mu 2 + \mathfrak{d}1 + \mu 1 (9 + \mathfrak{d}1)) + \\
& \quad \theta l (142 + 53 \mathfrak{d}1 + 5 \mathfrak{d}1^2 - 8 \mu 2 (-22 + \mathfrak{d}1 - \mathfrak{d}2) + 11 \mathfrak{d}2 + \\
& \quad \quad 5 \mathfrak{d}1 \mathfrak{d}2 + \mu 1 (142 + 5 \mathfrak{d}1^2 + 11 \mathfrak{d}2 + \mathfrak{d}1 (77 + 5 \mathfrak{d}2)))) + \eta \\
& \quad (\theta l (-34 - 47 \mathfrak{d}1 - 15 \mathfrak{d}1^2 + 3 \mathfrak{d}2 + 5 \mathfrak{d}1 \mathfrak{d}2 + 8 \mu 2 (2 + \mathfrak{d}1 + 3 \mathfrak{d}2) - \\
& \quad \quad \mu 1 (34 + 15 \mathfrak{d}1^2 - 3 \mathfrak{d}2 + \mathfrak{d}1 (47 + 19 \mathfrak{d}2))) + \eta t (8 \times (9 + 10 \mu 2 + 5 \mathfrak{d}1 + \\
& \quad \quad \mu 1 (9 + 5 \mathfrak{d}1)) + \theta l (34 + 47 \mathfrak{d}1 + 15 \mathfrak{d}1^2 - 3 \mathfrak{d}2 - 5 \mathfrak{d}1 \mathfrak{d}2 - 8 \mu 2 \\
& \quad \quad (2 + \mathfrak{d}1 + 3 \mathfrak{d}2) + \mu 1 (34 + 15 \mathfrak{d}1^2 - 3 \mathfrak{d}2 + \mathfrak{d}1 (47 + 19 \mathfrak{d}2)))) + \\
& 2 \times (-1 + \eta) \times (10 \eta^6 \theta p (9 + 28 \mu 2 + \mathfrak{d}1 + \mu 1 (9 + \mathfrak{d}1)) + 2 \eta t \theta p \\
& \quad (7 + 4 \mu 2 + 5 \mathfrak{d}1 + \mu 1 (7 + 5 \mathfrak{d}1)) - 2 \eta^5 \theta p \\
& \quad (-2 \times (122 + 122 \mu 1 + 434 \mu 2 + 18 \mathfrak{d}1 + 3 \mu 1 \mathfrak{d}1) + 5 \eta t (9 + 28 \mu 2 + \mathfrak{d}1 + \\
& \quad \quad \mu 1 (9 + \mathfrak{d}1))) + \eta^4 \theta p (-14 \eta t (9 + 28 \mu 2 + \mathfrak{d}1 + \mu 1 (9 + \mathfrak{d}1)) + \\
& \quad \theta l (357 + \mu 1 (357 - 37 \mathfrak{d}1) + 23 \mathfrak{d}1 + 8 \mu 2 (188 + 5 \mathfrak{d}1)) - \\
& \quad \eta t \theta l (357 + \mu 1 (357 - 37 \mathfrak{d}1) + 23 \mathfrak{d}1 + 8 \mu 2 (188 + 5 \mathfrak{d}1)) - \\
& \quad \quad 2 \times (637 + 1872 \mu 2 + 53 \mathfrak{d}1 + \mu 1 (637 + 95 \mathfrak{d}1))) + 6 \eta^3 \theta p \\
& \quad (4 \times (29 + 72 \mu 2 + \mathfrak{d}1 + \mu 1 (29 + 7 \mathfrak{d}1)) - \theta l (142 + 53 \mathfrak{d}1 + 5 \mathfrak{d}1^2 - \\
& \quad \quad 8 \mu 2 (-22 + \mathfrak{d}1 - \mathfrak{d}2) + 11 \mathfrak{d}2 + 5 \mathfrak{d}1 \mathfrak{d}2 + \mu 1 (142 + 5 \mathfrak{d}1^2 + 11 \mathfrak{d}2 + \\
& \quad \quad \mathfrak{d}1 (77 + 5 \mathfrak{d}2))) + \eta t (4 \times (9 + 28 \mu 2 + \mathfrak{d}1 + \mu 1 (9 + \mathfrak{d}1)) + \\
& \quad \theta l (142 + 53 \mathfrak{d}1 + 5 \mathfrak{d}1^2 - 8 \mu 2 (-22 + \mathfrak{d}1 - \mathfrak{d}2) + 11 \mathfrak{d}2 + \\
& \quad \quad 5 \mathfrak{d}1 \mathfrak{d}2 + \mu 1 (142 + 5 \mathfrak{d}1^2 + 11 \mathfrak{d}2 + \mathfrak{d}1 (77 + 5 \mathfrak{d}2)))) + \eta \\
& \quad (2 \eta t \theta p (71 + 128 \mu 2 + 25 \mathfrak{d}1 + \mu 1 (71 + 25 \mathfrak{d}1)) + (-1 + \eta t) \\
& \quad \theta l (2 \times (1 + \mu 1 + 20 \mu 2 - 5 \mathfrak{d}1 - 5 \mu 1 \mathfrak{d}1) + \\
& \quad \theta p (34 + 47 \mathfrak{d}1 + 15 \mathfrak{d}1^2 - 3 \mathfrak{d}2 - 5 \mathfrak{d}1 \mathfrak{d}2 - 8 \mu 2 (2 + \mathfrak{d}1 + 3 \mathfrak{d}2) + \\
& \quad \quad \mu 1 (34 + 15 \mathfrak{d}1^2 - 3 \mathfrak{d}2 + \mathfrak{d}1 (47 + 19 \mathfrak{d}2)))) + 3 \\
& \eta^2 (-4 \eta t \theta p (13 + 22 \mu 2 + 5 \mathfrak{d}1 + \mu 1 (13 + 5 \mathfrak{d}1)) + (-1 + \eta t) \\
& \quad \theta l (-2 \times (3 - 8 \mu 2 + 5 \mathfrak{d}1 + \mu 1 (3 + 5 \mathfrak{d}1)) + \\
& \quad \theta p (127 + 143 \mathfrak{d}1 + 30 \mathfrak{d}1^2 + 32 \mathfrak{d}2 + 12 \mu 2 (2 + 5 \mathfrak{d}1 + 3 \mathfrak{d}2) +
\end{aligned}$$

$$\begin{aligned}
& \mu_1 (127 + 30 \mu_1^2 + 32 \mu_2 + \mu_1 (143 + 36 \mu_2)) \Big) \Big) \Big) - \\
& x^2 (-1 + \eta)^2 \Big( 4 \times (-1 + \eta) \operatorname{ep} (10 \eta^4 (9 + 28 \mu_2 + \mu_1 + \mu_1 (9 + \mu_1)) - \\
& \quad 3 \eta t (19 + 40 \mu_2 + 5 \mu_1 + \mu_1 (19 + 5 \mu_1)) - 18 \eta^2 \\
& \quad (29 + 29 \mu_1 + 72 \mu_2 + \mu_1 + 7 \mu_1 \mu_1 + \eta t (9 + 28 \mu_2 + \mu_1 + \mu_1 (9 + \mu_1))) - \\
& \quad 2 \eta^3 (5 \eta t (9 + 28 \mu_2 + \mu_1 + \mu_1 (9 + \mu_1)) - \\
& \quad \quad 2 (\mu_1 (104 + \mu_1) + 2 \times (52 + 189 \mu_2 + 8 \mu_1))) \Big) + \\
& (-1 + \eta t) \operatorname{el} (-4 \times (3 - 8 \mu_2 + 5 \mu_1 + \mu_1 (3 + 5 \mu_1)) - 4 \eta^3 \operatorname{ep} \\
& \quad (249 + \mu_1 (249 - 49 \mu_1) + 11 \mu_1 + 8 \mu_2 (146 + 5 \mu_1)) + \\
& \quad 18 \eta^2 \operatorname{ep} (142 + 53 \mu_1 + 5 \mu_1^2 - 8 \mu_2 (-22 + \mu_1 - \mu_2) + 11 \mu_2 + \\
& \quad \quad 5 \mu_1 \mu_2 + \mu_1 (142 + 5 \mu_1^2 + 11 \mu_2 + \mu_1 (77 + 5 \mu_2))) \Big) + \\
& \operatorname{ep} (34 + 47 \mu_1 + 15 \mu_1^2 - 3 \mu_2 - 5 \mu_1 \mu_2 - 8 \mu_2 (2 + \mu_1 + 3 \mu_2) + \\
& \quad \mu_1 (34 + 15 \mu_1^2 - 3 \mu_2 + \mu_1 (47 + 19 \mu_2))) \Big) + \\
& 6 \eta (-4 \times (9 + 10 \mu_2 + 5 \mu_1 + \mu_1 (9 + 5 \mu_1)) + \operatorname{ep} \\
& \quad (143 + 151 \mu_1 + 30 \mu_1^2 + 40 \mu_2 + 12 \mu_2 (6 + 7 \mu_1 + 5 \mu_2) + \\
& \quad \mu_1 (143 + 30 \mu_1^2 + 40 \mu_2 + \mu_1 (151 + 36 \mu_2)) \Big) \Big) \Big) \Big) + \\
& w^3 (-1 + \eta)^3 (x^4 (-1 + \eta)^4 \operatorname{ep} (84 - 112 \operatorname{el} \mu_1 + 84 \mu_1 - 112 \operatorname{el} \mu_1 + 176 \operatorname{el} \\
& \quad \mu_2 - 12 \mu_1 - 51 \operatorname{el} \mu_1 + 60 \mu_1 \mu_1 - 123 \operatorname{el} \mu_1 \mu_1 + 40 \operatorname{el} \mu_2 \mu_1 - 5 \\
& \quad \operatorname{el} \mu_1^2 - 5 \operatorname{el} \mu_1 \mu_1^2 + 12 \eta^2 (9 + 28 \mu_2 + \mu_1 + \mu_1 (9 + \mu_1)) + 12 \\
& \quad \eta t (9 + 28 \mu_2 + \mu_1 + \mu_1 (9 + \mu_1)) - 12 \eta \\
& \quad (\eta t (9 + 28 \mu_2 + \mu_1 + \mu_1 (9 + \mu_1)) + 2 \times (8 + 14 \mu_2 + \mu_1 (8 + 3 \mu_1))) - 11 \\
& \quad \operatorname{el} \mu_2 - 11 \operatorname{el} \mu_1 \mu_2 - 8 \operatorname{el} \mu_2 \mu_2 - 5 \operatorname{el} \mu_1 \mu_2 - 5 \operatorname{el} \mu_1 \mu_1 \\
& \quad \mu_2 + \eta t \operatorname{el} (112 + 51 \mu_1 + 5 \mu_1^2 - 8 \mu_2 (22 + 5 \mu_1 - \mu_2) + 11 \mu_2 + \\
& \quad \quad 5 \mu_1 \mu_2 + \mu_1 (112 + 5 \mu_1^2 + 11 \mu_2 + \mu_1 (123 + 5 \mu_2))) \Big) - \\
& 4 x^3 (-1 + \eta)^3 (3 \times (-1 + \eta) \operatorname{ep} (-29 - 29 \mu_1 - 72 \mu_2 - \mu_1 - 7 \mu_1 \mu_1 + \\
& \quad 4 \eta^2 (9 + 28 \mu_2 + \mu_1 + \mu_1 (9 + \mu_1)) - \eta t (9 + 28 \mu_2 + \mu_1 + \mu_1 (9 + \mu_1)) - \\
& \quad \eta (1 + \mu_1 - 84 \mu_2 - 7 \mu_1 + 17 \mu_1 \mu_1 + 4 \eta t (9 + 28 \mu_2 + \mu_1 + \mu_1 (9 + \mu_1))) \Big) + \\
& (-1 + \eta t) \operatorname{el} (-3 \times (28 \mu_2 + 5 \times (3 + \mu_1) + 5 \mu_1 (3 + \mu_1)) + \\
& \operatorname{ep} (\eta (58 + 45 \mu_1 + 5 \mu_1^2 - 8 \mu_2 (43 + 5 \mu_1 - \mu_2) + 11 \mu_2 + \\
& \quad 5 \mu_1 \mu_2 + \mu_1 (58 + 5 \mu_1^2 + 11 \mu_2 + \mu_1 (117 + 5 \mu_2))) \Big) + \\
& \quad 3 \times (56 + 31 \mu_1 + 5 \mu_1^2 + 8 \mu_2 + 2 \mu_2 (38 + 7 \mu_1 + 7 \mu_2) + \\
& \quad \mu_1 (5 \mu_1^2 + 8 \times (7 + \mu_2) + \mu_1 (37 + 6 \mu_2))) \Big) \Big) \Big) + \\
& x^2 (-1 + \eta)^2 (12 \times (-1 + \eta) \operatorname{ep} (6 \eta^3 (9 + 28 \mu_2 + \mu_1 + \mu_1 (9 + \mu_1)) - \\
& \quad \eta t (19 + 40 \mu_2 + 5 \mu_1 + \mu_1 (19 + 5 \mu_1)) - 3 \eta (29 + 29 \mu_1 + 72 \mu_2 + \mu_1 + \\
& \quad \quad 7 \mu_1 \mu_1 + \eta t (9 + 28 \mu_2 + \mu_1 + \mu_1 (9 + \mu_1))) - 3 \eta^2 (-13 - 13 \mu_1 - \\
& \quad \quad 84 \mu_2 - 5 \mu_1 + 7 \mu_1 \mu_1 + 2 \eta t (9 + 28 \mu_2 + \mu_1 + \mu_1 (9 + \mu_1))) \Big) + \\
& (-1 + \eta t) \operatorname{el} (-12 \times (3 - 8 \mu_2 + 5 \mu_1 + \mu_1 (3 + 5 \mu_1)) + 6 \eta^2 \operatorname{ep} \\
& \quad (4 + 39 \mu_1 + 5 \mu_1^2 - 8 \mu_2 (64 + 5 \mu_1 - \mu_2) + 11 \mu_2 + \\
& \quad \quad 5 \mu_1 \mu_2 + \mu_1 (4 + 5 \mu_1^2 + 11 \mu_2 + \mu_1 (111 + 5 \mu_2))) \Big) + \\
& \operatorname{ep} (104 + 155 \mu_1 + 45 \mu_1^2 - 9 \mu_2 - 15 \mu_1 \mu_2 - 8 \mu_2 (14 + 3 \mu_1 + 9 \mu_2) + \\
& \quad \mu_1 (104 + 45 \mu_1^2 - 9 \mu_2 + \mu_1 (155 + 57 \mu_2))) \Big) + \\
& 12 \eta (-2 \times (9 + 10 \mu_2 + 5 \mu_1 + \mu_1 (9 + 5 \mu_1)) + \operatorname{ep} \\
& \quad (160 + 89 \mu_1 + 15 \mu_1^2 + 20 \mu_2 + 6 \mu_2 (34 + 5 \mu_1 + 5 \mu_2) + \\
& \quad \mu_1 (15 \mu_1^2 + 20 \times (8 + \mu_2) + \mu_1 (107 + 18 \mu_2))) \Big) \Big) \Big) +
\end{aligned}$$

$$\begin{aligned}
& \eta \, \text{op} \left( 12 \, \eta^5 \left( 9 + 28 \, \mu_2 + \mathfrak{e}1 + \mu_1 \left( 9 + \mathfrak{e}1 \right) \right) + 12 \, \eta \mathfrak{t} \left( 3 - 8 \, \mu_2 + 5 \, \mathfrak{e}1 + \right. \right. \\
& \quad \left. \mu_1 \left( 3 + 5 \, \mathfrak{e}1 \right) \right) - 12 \, \eta^4 \left( -11 - 56 \, \mu_2 - 3 \, \mathfrak{e}1 + \right. \\
& \quad \left. \mu_1 \left( -11 + 3 \, \mathfrak{e}1 \right) + \eta \mathfrak{t} \left( 9 + 28 \, \mu_2 + \mathfrak{e}1 + \mu_1 \left( 9 + \mathfrak{e}1 \right) \right) \right) + \eta^3 \\
& \quad \left( -12 \times (49 + 156 \, \mu_2 + 5 \, \mathfrak{e}1 + \mu_1 \left( 49 + 5 \, \mathfrak{e}1 \right)) + (-1 + \eta \mathfrak{t}) \, \text{el} \right. \\
& \quad \left( -104 + 27 \, \mathfrak{e}1 + 5 \, \mathfrak{e}1^2 - 8 \, \mu_2 \left( 106 + 5 \, \mathfrak{e}1 - \mathfrak{e}2 \right) + 11 \, \mathfrak{e}2 + 5 \, \mathfrak{e}1 \, \mathfrak{e}2 + \right. \\
& \quad \left. \mu_1 \left( -104 + 5 \, \mathfrak{e}1^2 + 11 \, \mathfrak{e}2 + \mathfrak{e}1 \left( 99 + 5 \, \mathfrak{e}2 \right) \right) \right) \left. \right) + 12 \, \eta^2 \\
& \quad \left( 29 + 29 \, \mu_1 + 72 \, \mu_2 + \mathfrak{e}1 + 7 \, \mu_1 \, \mathfrak{e}1 - \text{el} \left( 48 + 27 \, \mathfrak{e}1 + 5 \, \mathfrak{e}1^2 + 4 \, \mathfrak{e}2 + \right. \right. \\
& \quad \left. \left. 2 \, \mu_2 \left( 26 + \mathfrak{e}1 + \mathfrak{e}2 \right) + \mu_1 \left( 48 + 33 \, \mathfrak{e}1 + 5 \, \mathfrak{e}1^2 + 4 \, \mathfrak{e}2 + 6 \, \mathfrak{e}1 \, \mathfrak{e}2 \right) \right) \right) + \\
& \quad \eta \mathfrak{t} \left( 2 + 2 \, \mu_1 + 24 \, \mu_2 - 4 \, \mathfrak{e}1 - 4 \, \mu_1 \, \mathfrak{e}1 + \text{el} \left( 48 + 27 \, \mathfrak{e}1 + 5 \, \mathfrak{e}1^2 + 4 \, \mathfrak{e}2 + \right. \right. \\
& \quad \left. \left. 2 \, \mu_2 \left( 26 + \mathfrak{e}1 + \mathfrak{e}2 \right) + \mu_1 \left( 48 + 33 \, \mathfrak{e}1 + 5 \, \mathfrak{e}1^2 + 4 \, \mathfrak{e}2 + 6 \, \mathfrak{e}1 \, \mathfrak{e}2 \right) \right) \right) \left. \right) + \\
& \quad \eta \left( \text{el} \left( -104 - 155 \, \mathfrak{e}1 - 45 \, \mathfrak{e}1^2 + 9 \, \mathfrak{e}2 + 15 \, \mathfrak{e}1 \, \mathfrak{e}2 + 8 \, \mu_2 \left( 14 + 3 \, \mathfrak{e}1 + \right. \right. \right. \\
& \quad \left. \left. 9 \, \mathfrak{e}2 \right) - \mu_1 \left( 104 + 45 \, \mathfrak{e}1^2 - 9 \, \mathfrak{e}2 + \mathfrak{e}1 \left( 155 + 57 \, \mathfrak{e}2 \right) \right) \right) \right) + \\
& \quad \eta \mathfrak{t} \left( 48 \times (1 + \mu_1 + 3 \, \mu_2) + \text{el} \left( 104 + 155 \, \mathfrak{e}1 + 45 \, \mathfrak{e}1^2 - 9 \, \mathfrak{e}2 - \right. \right. \\
& \quad \left. \left. 15 \, \mathfrak{e}1 \, \mathfrak{e}2 - 8 \, \mu_2 \left( 14 + 3 \, \mathfrak{e}1 + 9 \, \mathfrak{e}2 \right) + \right. \right. \\
& \quad \left. \left. \mu_1 \left( 104 + 45 \, \mathfrak{e}1^2 - 9 \, \mathfrak{e}2 + \mathfrak{e}1 \left( 155 + 57 \, \mathfrak{e}2 \right) \right) \right) \right) \left. \right) - \\
& \quad 2 \times (-1 + \eta) \times \left( 24 \, \eta^5 \, \text{op} \left( 9 + 28 \, \mu_2 + \mathfrak{e}1 + \mu_1 \left( 9 + \mathfrak{e}1 \right) \right) + 6 \, \eta \mathfrak{t} \, \text{op} \right. \\
& \quad \left( 7 + 4 \, \mu_2 + 5 \, \mathfrak{e}1 + \mu_1 \left( 7 + 5 \, \mathfrak{e}1 \right) \right) - 6 \, \eta^4 \, \text{op} \left( -17 - 140 \, \mu_2 - 9 \, \mathfrak{e}1 + \right. \\
& \quad \left. \mu_1 \left( -17 + 15 \, \mathfrak{e}1 \right) + 4 \, \eta \mathfrak{t} \left( 9 + 28 \, \mu_2 + \mathfrak{e}1 + \mu_1 \left( 9 + \mathfrak{e}1 \right) \right) \right) + 6 \, \eta^2 \\
& \quad \left( \text{op} \left( \eta \mathfrak{t} \left( 1 + \mu_1 + 40 \, \mu_2 - 7 \, \mathfrak{e}1 - 7 \, \mu_1 \, \mathfrak{e}1 \right) + 3 \times (29 + 72 \, \mu_2 + \mathfrak{e}1 + \right. \right. \\
& \quad \left. \left. \mu_1 \left( 29 + 7 \, \mathfrak{e}1 \right) \right) \right) + (-1 + \eta \mathfrak{t}) \, \text{el} \left( -3 - 3 \, \mu_1 + 8 \, \mu_2 - 5 \, \mathfrak{e}1 - \right. \\
& \quad \left. 5 \, \mu_1 \, \mathfrak{e}1 + \text{op} \left( 152 + 85 \, \mathfrak{e}1 + 15 \, \mathfrak{e}1^2 + 16 \, \mathfrak{e}2 + 18 \, \mu_2 \left( 10 + \mathfrak{e}1 + \mathfrak{e}2 \right) + \right. \right. \\
& \quad \left. \left. \mu_1 \left( 152 + 103 \, \mathfrak{e}1 + 15 \, \mathfrak{e}1^2 + 16 \, \mathfrak{e}2 + 18 \, \mathfrak{e}1 \, \mathfrak{e}2 \right) \right) \right) \left. \right) + 2 \, \eta^3 \, \text{op} \\
& \quad \left( -6 \times (70 + 234 \, \mu_2 + 8 \, \mathfrak{e}1 + 5 \, \mu_1 \left( 14 + \mathfrak{e}1 \right)) - \text{el} \left( -50 + 33 \, \mathfrak{e}1 + \right. \right. \\
& \quad \left. \left. 5 \, \mathfrak{e}1^2 - 8 \, \mu_2 \left( 85 + 5 \, \mathfrak{e}1 - \mathfrak{e}2 \right) + 11 \, \mathfrak{e}2 + 5 \, \mathfrak{e}1 \, \mathfrak{e}2 + \mu_1 \left( -50 + 5 \, \mathfrak{e}1^2 + \right. \right. \right. \\
& \quad \left. \left. 11 \, \mathfrak{e}2 + 5 \, \mathfrak{e}1 \left( 21 + \mathfrak{e}2 \right) \right) \right) + \eta \mathfrak{t} \left( 3 \times (9 + 28 \, \mu_2 + \mathfrak{e}1 + \mu_1 \left( 9 + \mathfrak{e}1 \right)) + \right. \\
& \quad \left. \text{el} \left( -50 + 33 \, \mathfrak{e}1 + 5 \, \mathfrak{e}1^2 - 8 \, \mu_2 \left( 85 + 5 \, \mathfrak{e}1 - \mathfrak{e}2 \right) + 11 \, \mathfrak{e}2 + \right. \right. \\
& \quad \left. \left. 5 \, \mathfrak{e}1 \, \mathfrak{e}2 + \mu_1 \left( -50 + 5 \, \mathfrak{e}1^2 + 11 \, \mathfrak{e}2 + 5 \, \mathfrak{e}1 \left( 21 + \mathfrak{e}2 \right) \right) \right) \right) \left. \right) + \eta \\
& \quad \left( 6 \, \eta \mathfrak{t} \, \text{op} \left( 19 + 40 \, \mu_2 + 5 \, \mathfrak{e}1 + \mu_1 \left( 19 + 5 \, \mathfrak{e}1 \right) \right) + (-1 + \eta \mathfrak{t}) \, \text{el} \right. \\
& \quad \left( 6 \times (1 + \mu_1 + 20 \, \mu_2 - 5 \, \mathfrak{e}1 - 5 \, \mu_1 \, \mathfrak{e}1) + \right. \\
& \quad \left. \text{op} \left( 104 + 155 \, \mathfrak{e}1 + 45 \, \mathfrak{e}1^2 - 9 \, \mathfrak{e}2 - 15 \, \mathfrak{e}1 \, \mathfrak{e}2 - 8 \, \mu_2 \left( 14 + 3 \, \mathfrak{e}1 + 9 \, \mathfrak{e}2 \right) + \right. \right. \\
& \quad \left. \left. \mu_1 \left( 104 + 45 \, \mathfrak{e}1^2 - 9 \, \mathfrak{e}2 + \mathfrak{e}1 \left( 155 + 57 \, \mathfrak{e}2 \right) \right) \right) \right) \left. \right) + \\
& \quad w^4 \, (-1 + \eta)^4 \left( 2 \, x^3 \, (-1 + \eta)^3 \left( 6 \times (-1 + \eta) \, \text{op} \left( -7 - 7 \, \mu_1 + \mathfrak{e}1 - 5 \, \mu_1 \, \mathfrak{e}1 + \right. \right. \right. \\
& \quad \left. \left. \eta \left( 9 + 28 \, \mu_2 + \mathfrak{e}1 + \mu_1 \left( 9 + \mathfrak{e}1 \right) \right) - \eta \mathfrak{t} \left( 9 + 28 \, \mu_2 + \mathfrak{e}1 + \mu_1 \left( 9 + \mathfrak{e}1 \right) \right) \right) + \right. \\
& \quad \left. (-1 + \eta \mathfrak{t}) \, \text{el} \left( -2 \times (28 \, \mu_2 + 5 \times (3 + \mathfrak{e}1) + 5 \, \mu_1 \left( 3 + \mathfrak{e}1 \right)) + \right. \right. \\
& \quad \left. \left. \text{op} \left( 97 + 61 \, \mathfrak{e}1 + 10 \, \mathfrak{e}1^2 + 16 \, \mathfrak{e}2 + 4 \, \mu_2 \left( -6 + 3 \, \mathfrak{e}1 + 7 \, \mathfrak{e}2 \right) + \right. \right. \right. \\
& \quad \left. \left. \mu_1 \left( 97 + 10 \, \mathfrak{e}1^2 + 16 \, \mathfrak{e}2 + \mathfrak{e}1 \left( 97 + 12 \, \mathfrak{e}2 \right) \right) \right) \right) \left. \right) - \\
& \quad x^2 \, (-1 + \eta)^2 \left( 4 \times (-1 + \eta) \, \text{op} \left( -29 - 29 \, \mu_1 - 72 \, \mu_2 - \mathfrak{e}1 - 7 \, \mu_1 \, \mathfrak{e}1 - \right. \right. \\
& \quad \left. \left. 2 \, \eta \mathfrak{t} \left( 14 + 14 \, \mu_1 + 34 \, \mu_2 + 3 \, \mathfrak{e}1 + 3 \, \mu_1 \, \mathfrak{e}1 \right) + \right. \right. \\
& \quad \left. \left. 9 \, \eta^2 \left( 9 + 28 \, \mu_2 + \mathfrak{e}1 + \mu_1 \left( 9 + \mathfrak{e}1 \right) \right) - 3 \, \eta \left( -4 \times (-3 + 7 \, \mu_2 + \mathfrak{e}1) + \right. \right. \right. \\
& \quad \left. \left. 2 \, \mu_1 \left( 6 + 7 \, \mathfrak{e}1 \right) + 3 \, \eta \mathfrak{t} \left( 9 + 28 \, \mu_2 + \mathfrak{e}1 + \mu_1 \left( 9 + \mathfrak{e}1 \right) \right) \right) \right) + \\
& \quad (-1 + \eta \mathfrak{t}) \, \text{el} \left( -12 \times (3 - 8 \, \mu_2 + 5 \, \mathfrak{e}1 + \mu_1 \left( 3 + 5 \, \mathfrak{e}1 \right)) + \right. \\
& \quad \left. \text{op} \left( 222 + 173 \, \mathfrak{e}1 + 45 \, \mathfrak{e}1^2 - 9 \, \mathfrak{e}2 - 15 \, \mathfrak{e}1 \, \mathfrak{e}2 - 8 \, \mu_2 \left( -14 + 5 \, \mathfrak{e}1 + 9 \, \mathfrak{e}2 \right) + \right. \right. \\
& \quad \left. \left. \mu_1 \left( 222 + 45 \, \mathfrak{e}1^2 - 9 \, \mathfrak{e}2 + \mathfrak{e}1 \left( 197 + 57 \, \mathfrak{e}2 \right) \right) \right) \right) +
\end{aligned}$$

$$\begin{aligned}
& 2 \eta \left( -4 \times (9 + 10 \mu_2 + 5 \mathfrak{z}_1 + \mu_1 (9 + 5 \mathfrak{z}_1)) + \theta p \right. \\
& \quad \left( 239 + 171 \mathfrak{z}_1 + 30 \mathfrak{z}_1^2 + 40 \mathfrak{z}_2 + 4 \mu_2 (-58 + 3 \mathfrak{z}_1 + 15 \mathfrak{z}_2) + \right. \\
& \quad \left. \mu_1 (239 + 30 \mathfrak{z}_1^2 + 40 \mathfrak{z}_2 + 9 \mathfrak{z}_1 (31 + 4 \mathfrak{z}_2)) \right) \left. \right) - \\
& \eta \theta p \left( 12 \eta^4 (9 + 28 \mu_2 + \mathfrak{z}_1 + \mu_1 (9 + \mathfrak{z}_1)) + 12 \eta t (3 - 8 \mu_2 + 5 \mathfrak{z}_1 + \right. \\
& \quad \left. \mu_1 (3 + 5 \mathfrak{z}_1)) - 12 \eta^3 \right. \\
& \quad \left( 7 - \mathfrak{z}_1 + \mu_1 (7 + 5 \mathfrak{z}_1) + \eta t (9 + 28 \mu_2 + \mathfrak{z}_1 + \mu_1 (9 + \mathfrak{z}_1)) \right) + 2 \\
& \quad \eta^2 \left( -2 \times (156 \mu_2 - 5 \mu_1 (-7 + \mathfrak{z}_1) + 7 \times (5 + \mathfrak{z}_1)) - \right. \\
& \quad \theta l \left( 45 + 49 \mathfrak{z}_1 + 10 \mathfrak{z}_1^2 - 4 \mu_2 (46 + 3 \mathfrak{z}_1 - \mathfrak{z}_2) + 8 \mathfrak{z}_2 + \right. \\
& \quad \left. \mu_1 (45 + 10 \mathfrak{z}_1^2 + 8 \mathfrak{z}_2 + \mathfrak{z}_1 (85 + 12 \mathfrak{z}_2)) \right) + \eta t \left( 22 + 22 \mu_1 + 104 \mu_2 - \right. \\
& \quad \left. 6 \mathfrak{z}_1 - 6 \mu_1 \mathfrak{z}_1 + \theta l \left( 45 + 49 \mathfrak{z}_1 + 10 \mathfrak{z}_1^2 - 4 \mu_2 (46 + 3 \mathfrak{z}_1 - \mathfrak{z}_2) + \right. \right. \\
& \quad \left. \left. 8 \mathfrak{z}_2 + \mu_1 (45 + 10 \mathfrak{z}_1^2 + 8 \mathfrak{z}_2 + \mathfrak{z}_1 (85 + 12 \mathfrak{z}_2)) \right) \right) \left. \right) + \eta \\
& \quad \left( 4 \times (29 + 72 \mu_2 + \mathfrak{z}_1 + \mu_1 (29 + 7 \mathfrak{z}_1)) - \theta l \left( 222 + 173 \mathfrak{z}_1 + \right. \right. \\
& \quad \left. \left. 45 \mathfrak{z}_1^2 - 9 \mathfrak{z}_2 - 15 \mathfrak{z}_1 \mathfrak{z}_2 - 8 \mu_2 (-14 + 5 \mathfrak{z}_1 + 9 \mathfrak{z}_2) + \right. \right. \\
& \quad \left. \left. \mu_1 (222 + 45 \mathfrak{z}_1^2 - 9 \mathfrak{z}_2 + \mathfrak{z}_1 (197 + 57 \mathfrak{z}_2)) \right) \right) + \\
& \quad \eta t \left( 4 \times (7 + 56 \mu_2 + \mu_1 (7 - 9 \mathfrak{z}_1) - 9 \mathfrak{z}_1) + \theta l \left( 222 + 173 \mathfrak{z}_1 + \right. \right. \\
& \quad \left. \left. 45 \mathfrak{z}_1^2 - 9 \mathfrak{z}_2 - 15 \mathfrak{z}_1 \mathfrak{z}_2 - 8 \mu_2 (-14 + 5 \mathfrak{z}_1 + 9 \mathfrak{z}_2) + \right. \right. \\
& \quad \left. \left. \mu_1 (222 + 45 \mathfrak{z}_1^2 - 9 \mathfrak{z}_2 + \mathfrak{z}_1 (197 + 57 \mathfrak{z}_2)) \right) \right) \left. \right) + \\
& 2 \times (-1 + \eta) \times \left( 18 \eta^4 \theta p (9 + 28 \mu_2 + \mathfrak{z}_1 + \mu_1 (9 + \mathfrak{z}_1)) + 6 \eta t \theta p \right. \\
& \quad \left( 7 + 4 \mu_2 + 5 \mathfrak{z}_1 + \mu_1 (7 + 5 \mathfrak{z}_1)) - 6 \eta^3 \theta p \right. \\
& \quad \left( 30 + 28 \mu_2 - 2 \mathfrak{z}_1 + 2 \mu_1 (15 + 8 \mathfrak{z}_1) + 3 \eta t (9 + 28 \mu_2 + \mathfrak{z}_1 + \mu_1 (9 + \mathfrak{z}_1)) \right) + \\
& \quad \eta^2 \left( -2 \theta p (49 + 312 \mu_2 + \mu_1 (49 - 25 \mathfrak{z}_1) + 17 \mathfrak{z}_1 + \right. \\
& \quad \eta t (-37 - 152 \mu_2 + 3 \mathfrak{z}_1 + \mu_1 (-37 + 3 \mathfrak{z}_1)) + \\
& \quad (-1 + \eta t) \theta l \left( -2 \times (3 - 8 \mu_2 + 5 \mathfrak{z}_1 + \mu_1 (3 + 5 \mathfrak{z}_1)) + \right. \\
& \quad \theta p \left( 187 + 159 \mathfrak{z}_1 + 30 \mathfrak{z}_1^2 - 4 \mu_2 (98 + 3 \mathfrak{z}_1 - 9 \mathfrak{z}_2) + 32 \mathfrak{z}_2 + \right. \\
& \quad \left. \mu_1 (187 + 30 \mathfrak{z}_1^2 + 32 \mathfrak{z}_2 + 3 \mathfrak{z}_1 (89 + 12 \mathfrak{z}_2)) \right) \left. \right) \left. \right) + \eta \\
& \quad \left( 2 \theta p (\eta t (23 + 88 \mu_2 + \mu_1 (23 - 3 \mathfrak{z}_1) - 3 \mathfrak{z}_1) + 2 \times (29 + \right. \\
& \quad \left. 72 \mu_2 + \mathfrak{z}_1 + \mu_1 (29 + 7 \mathfrak{z}_1)) \right) + \\
& \quad (-1 + \eta t) \theta l \left( 6 \times (1 + \mu_1 + 20 \mu_2 - 5 \mathfrak{z}_1 - 5 \mu_1 \mathfrak{z}_1) + \theta p \right. \\
& \quad \left( 222 + 173 \mathfrak{z}_1 + 45 \mathfrak{z}_1^2 - 9 \mathfrak{z}_2 - 15 \mathfrak{z}_1 \mathfrak{z}_2 - 8 \mu_2 (-14 + 5 \mathfrak{z}_1 + 9 \mathfrak{z}_2) + \right. \\
& \quad \left. \mu_1 (222 + 45 \mathfrak{z}_1^2 - 9 \mathfrak{z}_2 + \mathfrak{z}_1 (197 + 57 \mathfrak{z}_2)) \right) \left. \right) \left. \right) \left. \right) + \\
& 2 \times (-1 + w (-1 + \eta)) (w + x + \eta - w \eta - x \eta)^2 \left( x^2 (-1 + \eta)^2 + \eta (1 + \eta) + \right. \\
& \quad \left. x (1 + \eta - 2 \eta^2) \right)^2 \\
& \theta l \left( -8 (x (-1 + \eta) - \eta) (w (-1 + \eta) + x (-1 + \eta) - \eta) \right. \\
& \quad \left. (1 + w - w \eta)^2 \right. \\
& \quad (-1 + \eta t) \\
& \theta p \\
& \quad (-6 u x + u (6 + 7 \mathfrak{z}_1 + 3 \mathfrak{z}_2)) - f \\
& \quad (-1 + \eta) \\
& \left( x^2 (-1 + \eta)^2 \theta p (20 + 4 \eta t - 20 \theta l + 20 \eta t \theta l + 36 \mathfrak{z}_1 + 8 \eta t \mathfrak{z}_1 - 36 \theta l \right. \\
& \quad \mathfrak{z}_1 + 36 \eta t \theta l \mathfrak{z}_1 + 10 \mathfrak{z}_2 + 2 \eta t \mathfrak{z}_2 - 16 \theta l \mathfrak{z}_2 + 16 \eta t \theta l \mathfrak{z}_2 + 6 \mathfrak{z}_1 \\
& \quad \mathfrak{z}_2 - 2 \eta t \mathfrak{z}_1 \mathfrak{z}_2 - 4 \theta l \mathfrak{z}_1 \mathfrak{z}_2 + 4 \eta t \theta l \mathfrak{z}_1 \mathfrak{z}_2 - 3 \theta l \mathfrak{z}_2^2 + 3 \eta t \theta l \\
& \quad \mathfrak{z}_2^2 - 5 \theta l \mathfrak{z}_1 \mathfrak{z}_2^2 + 5 \eta t \theta l \mathfrak{z}_1 \mathfrak{z}_2^2 + 4 \eta^2 (2 - \mathfrak{z}_1 (-4 + \mathfrak{z}_2) + \mathfrak{z}_2) + 2 \\
& \quad \eta (-14 - 26 \mathfrak{z}_1 + \eta t (1 + \theta l) \times (-2 + \mathfrak{z}_1 (-4 + \mathfrak{z}_2) - \mathfrak{z}_2) - \\
& \quad \left. 7 \mathfrak{z}_2 - \mathfrak{z}_1 \mathfrak{z}_2 + \theta l (2 + 4 \mathfrak{z}_1 + \mathfrak{z}_2 - \mathfrak{z}_1 \mathfrak{z}_2)) + w (-1 + \eta) \times \right.
\end{aligned}$$

$$\begin{aligned}
& \left( -12 + 12 \, \theta l - 20 \, \mathfrak{z} 1 + 20 \, \theta l \, \mathfrak{z} 1 + 2 \, \eta^2 \left( -2 + \mathfrak{z} 1 \left( -4 + \mathfrak{z} 2 \right) - \mathfrak{z} 2 \right) - \right. \\
& \quad 6 \, \mathfrak{z} 2 + 12 \, \theta l \, \mathfrak{z} 2 - 10 \, \mathfrak{z} 1 \, \mathfrak{z} 2 + 8 \, \theta l \, \mathfrak{z} 1 \, \mathfrak{z} 2 + 3 \, \theta l \, \mathfrak{z} 2^2 + 5 \, \theta l \, \mathfrak{z} 1 \, \mathfrak{z} 2^2 + \\
& \quad \eta \left( \eta t \left( 4 + 8 \, \mathfrak{z} 1 + 2 \, \mathfrak{z} 2 - 2 \, \mathfrak{z} 1 \, \mathfrak{z} 2 \right) + 4 \times \left( 4 + 7 \, \mathfrak{z} 1 + 2 \, \mathfrak{z} 2 + 2 \, \mathfrak{z} 1 \, \mathfrak{z} 2 \right) \right) - \eta t \left( 4 + \right. \\
& \quad \left. 8 \, \mathfrak{z} 1 + 2 \, \mathfrak{z} 2 - 2 \, \mathfrak{z} 1 \, \mathfrak{z} 2 + 3 \, \theta l \left( 2 + \mathfrak{z} 2 \right)^2 + \theta l \, \mathfrak{z} 1 \left( 20 + 8 \, \mathfrak{z} 2 + 5 \, \mathfrak{z} 2^2 \right) \right) \left. \right) + \\
& \text{op} \left( 20 \, \eta^2 - 28 \, \eta^3 + 8 \, \eta^4 + 12 \, \eta t - 12 \, \eta \, \eta t + 4 \, \eta^2 \, \eta t - 4 \, \eta^3 \, \eta t - 12 \, \eta \right. \\
& \quad \theta l - 20 \, \eta^2 \, \theta l + 4 \, \eta^3 \, \theta l + 12 \, \eta \, \eta t \, \theta l + 20 \, \eta^2 \, \eta t \, \theta l - 4 \, \eta^3 \, \eta t \\
& \quad \theta l + 36 \, \eta^2 \, \mathfrak{z} 1 - 52 \, \eta^3 \, \mathfrak{z} 1 + 16 \, \eta^4 \, \mathfrak{z} 1 + 8 \, \eta t \, \mathfrak{z} 1 - 8 \, \eta \, \eta t \, \mathfrak{z} 1 + 8 \, \eta^2 \\
& \quad \eta t \, \mathfrak{z} 1 - 8 \, \eta^3 \, \eta t \, \mathfrak{z} 1 - 12 \, \eta \, \theta l \, \mathfrak{z} 1 - 36 \, \eta^2 \, \theta l \, \mathfrak{z} 1 + 8 \, \eta^3 \, \theta l \, \mathfrak{z} 1 + 12 \, \eta \\
& \quad \eta t \, \theta l \, \mathfrak{z} 1 + 36 \, \eta^2 \, \eta t \, \theta l \, \mathfrak{z} 1 - 8 \, \eta^3 \, \eta t \, \theta l \, \mathfrak{z} 1 - 2 \, \eta \, \theta l \, \mathfrak{z} 1^2 + 2 \, \eta \, \eta t \\
& \quad \theta l \, \mathfrak{z} 1^2 + 10 \, \eta^2 \, \mathfrak{z} 2 - 14 \, \eta^3 \, \mathfrak{z} 2 + 4 \, \eta^4 \, \mathfrak{z} 2 + 6 \, \eta t \, \mathfrak{z} 2 - 6 \, \eta \, \eta t \, \mathfrak{z} 2 + 2 \, \eta^2 \\
& \quad \eta t \, \mathfrak{z} 2 - 2 \, \eta^3 \, \eta t \, \mathfrak{z} 2 - 12 \, \eta \, \theta l \, \mathfrak{z} 2 - 16 \, \eta^2 \, \theta l \, \mathfrak{z} 2 + 2 \, \eta^3 \, \theta l \, \mathfrak{z} 2 + 12 \, \eta \\
& \quad \eta t \, \theta l \, \mathfrak{z} 2 + 16 \, \eta^2 \, \eta t \, \theta l \, \mathfrak{z} 2 - 2 \, \eta^3 \, \eta t \, \theta l \, \mathfrak{z} 2 + 6 \, \eta^2 \, \mathfrak{z} 1 \, \mathfrak{z} 2 - 2 \, \eta^3 \, \mathfrak{z} 1 \\
& \quad \mathfrak{z} 2 - 4 \, \eta^4 \, \mathfrak{z} 1 \, \mathfrak{z} 2 - 10 \, \eta t \, \mathfrak{z} 1 \, \mathfrak{z} 2 + 10 \, \eta \, \eta t \, \mathfrak{z} 1 \, \mathfrak{z} 2 - 2 \, \eta^2 \, \eta t \, \mathfrak{z} 1 \, \mathfrak{z} 2 + 2 \\
& \quad \eta^3 \, \eta t \, \mathfrak{z} 1 \, \mathfrak{z} 2 + 4 \, \eta \, \theta l \, \mathfrak{z} 1 \, \mathfrak{z} 2 - 4 \, \eta^2 \, \theta l \, \mathfrak{z} 1 \, \mathfrak{z} 2 - 2 \, \eta^3 \, \theta l \, \mathfrak{z} 1 \, \mathfrak{z} 2 - 4 \, \eta \\
& \quad \eta t \, \theta l \, \mathfrak{z} 1 \, \mathfrak{z} 2 + 4 \, \eta^2 \, \eta t \, \theta l \, \mathfrak{z} 1 \, \mathfrak{z} 2 + 2 \, \eta^3 \, \eta t \, \theta l \, \mathfrak{z} 1 \, \mathfrak{z} 2 - 3 \, \eta \, \theta l \, \mathfrak{z} 2^2 - 3 \\
& \quad \eta^2 \, \theta l \, \mathfrak{z} 2^2 + 3 \, \eta \, \eta t \, \theta l \, \mathfrak{z} 2^2 + 3 \, \eta^2 \, \eta t \, \theta l \, \mathfrak{z} 2^2 + 5 \, \eta \, \theta l \, \mathfrak{z} 1 \, \mathfrak{z} 2^2 - 5 \, \eta^2 \\
& \quad \theta l \, \mathfrak{z} 1 \, \mathfrak{z} 2^2 - 5 \, \eta \, \eta t \, \theta l \, \mathfrak{z} 1 \, \mathfrak{z} 2^2 + 5 \, \eta^2 \, \eta t \, \theta l \, \mathfrak{z} 1 \, \mathfrak{z} 2^2 - 2 \, w^2 \left( -1 + \eta \right)^2 \\
& \quad \left( \eta^3 \left( -2 + \mathfrak{z} 1 \left( -4 + \mathfrak{z} 2 \right) - \mathfrak{z} 2 \right) + \eta^2 \left( 8 + 14 \, \mathfrak{z} 1 + 4 \, \mathfrak{z} 2 + 4 \, \mathfrak{z} 1 \, \mathfrak{z} 2 + \right. \right. \\
& \quad \left. \left. \eta t \left( 2 - \mathfrak{z} 1 \left( -4 + \mathfrak{z} 2 \right) + \mathfrak{z} 2 \right) \right) + \eta t \left( -3 \times \left( 2 + \mathfrak{z} 2 \right) + \mathfrak{z} 1 \left( -4 + 5 \, \mathfrak{z} 2 \right) \right) - \right. \\
& \quad \left. \eta \left( \left( 3 + 5 \, \mathfrak{z} 1 \right) \times \left( 2 + \mathfrak{z} 2 \right) - \theta l \left( \mathfrak{z} 1^2 + 3 \left( 2 + \mathfrak{z} 2 \right)^2 + 2 \, \mathfrak{z} 1 \left( 8 + \mathfrak{z} 2 \right) \right) + \right. \right. \\
& \quad \left. \left. \eta t \left( -4 - 2 \, \mathfrak{z} 2 + 4 \, \mathfrak{z} 1 \, \mathfrak{z} 2 + \theta l \left( \mathfrak{z} 1^2 + 3 \left( 2 + \mathfrak{z} 2 \right)^2 + 2 \, \mathfrak{z} 1 \left( 8 + \mathfrak{z} 2 \right) \right) \right) \right) \right) + w \\
& \quad \left( -1 + \eta \right) \times \left( 2 \, \eta^4 \left( -2 + \mathfrak{z} 1 \left( -4 + \mathfrak{z} 2 \right) - \mathfrak{z} 2 \right) + 4 \, \eta t \left( -3 \times \left( 2 + \mathfrak{z} 2 \right) + \right. \right. \\
& \quad \left. \left. \mathfrak{z} 1 \left( -4 + 5 \, \mathfrak{z} 2 \right) \right) + 2 \, \eta^3 \left( \eta t \left( 2 - \mathfrak{z} 1 \left( -4 + \mathfrak{z} 2 \right) + \mathfrak{z} 2 \right) + \right. \right. \\
& \quad \left. \left. 2 \times \left( 2 + \mathfrak{z} 2 + 3 \, \mathfrak{z} 1 \left( 1 + \mathfrak{z} 2 \right) \right) \right) + \eta^2 \left( 8 \times \left( 2 - \mathfrak{z} 1 \left( -4 + \mathfrak{z} 2 \right) + \mathfrak{z} 2 \right) - \right. \right. \\
& \quad \left. \left. \left( -1 + \eta t \right) \theta l \left( 8 + 10 \, \mathfrak{z} 2 + 3 \, \mathfrak{z} 2^2 + \mathfrak{z} 1 \left( 12 + 10 \, \mathfrak{z} 2 + 5 \, \mathfrak{z} 2^2 \right) \right) \right) - \right. \\
& \quad \left. \eta \left( 20 + 36 \, \mathfrak{z} 1 + 10 \, \mathfrak{z} 2 + 6 \, \mathfrak{z} 1 \, \mathfrak{z} 2 - \theta l \left( 44 + 4 \, \mathfrak{z} 1^2 + 40 \, \mathfrak{z} 2 + 9 \, \mathfrak{z} 2^2 + \mathfrak{z} 1 \right. \right. \right. \\
& \quad \left. \left. \left( 60 - 4 \, \mathfrak{z} 2 - 5 \, \mathfrak{z} 2^2 \right) \right) + \eta t \left( 2 \times \left( -5 \times \left( 2 + \mathfrak{z} 2 \right) + \mathfrak{z} 1 \left( -4 + 9 \, \mathfrak{z} 2 \right) \right) + \right. \right. \\
& \quad \left. \left. \theta l \left( 44 + 4 \, \mathfrak{z} 1^2 + 40 \, \mathfrak{z} 2 + 9 \, \mathfrak{z} 2^2 + \mathfrak{z} 1 \left( 60 - 4 \, \mathfrak{z} 2 - 5 \, \mathfrak{z} 2^2 \right) \right) \right) \right) \left. \right) - \\
& \times \left( -1 + \eta \right) \times \left( -2 \left( w \left( -1 + \eta \right) - 2 \, \eta \right) \left( -1 + \eta \right) \text{op} \left( -10 + 4 \, \eta - 2 \, \eta t - \right. \right. \\
& \quad 18 \, \mathfrak{z} 1 + 8 \, \eta \, \mathfrak{z} 1 - 4 \, \eta t \, \mathfrak{z} 1 - 5 \, \mathfrak{z} 2 + 2 \, \eta \, \mathfrak{z} 2 - \eta t \, \mathfrak{z} 2 - 3 \, \mathfrak{z} 1 \, \mathfrak{z} 2 - \\
& \quad 2 \, \eta \, \mathfrak{z} 1 \, \mathfrak{z} 2 + \eta t \, \mathfrak{z} 1 \, \mathfrak{z} 2 + w \left( -1 + \eta \right) \left( \eta \left( -2 + \mathfrak{z} 1 \left( -4 + \mathfrak{z} 2 \right) - \mathfrak{z} 2 \right) + \right. \\
& \quad \left. \left( 3 + 5 \, \mathfrak{z} 1 \right) \times \left( 2 + \mathfrak{z} 2 \right) + \eta t \left( 2 + 4 \, \mathfrak{z} 1 + \mathfrak{z} 2 - \mathfrak{z} 1 \, \mathfrak{z} 2 \right) \right) \right) + \left( -1 + \eta t \right) \theta l \\
& \quad \left( -12 + 12 \, \theta p + 40 \, \eta \, \theta p - 8 \, \eta^2 \, \theta p - 8 \, \mathfrak{z} 1 + 12 \, \theta p \, \mathfrak{z} 1 + 72 \, \eta \, \theta p \, \mathfrak{z} 1 - \right. \\
& \quad 16 \, \eta^2 \, \theta p \, \mathfrak{z} 1 + 2 \, \theta p \, \mathfrak{z} 1^2 - 6 \, \mathfrak{z} 2 + 12 \, \theta p \, \mathfrak{z} 2 + 32 \, \eta \, \theta p \, \mathfrak{z} 2 - 4 \, \eta^2 \, \theta p \, \mathfrak{z} 2 + \\
& \quad 10 \, \mathfrak{z} 1 \, \mathfrak{z} 2 - 4 \, \theta p \, \mathfrak{z} 1 \, \mathfrak{z} 2 + 8 \, \eta \, \theta p \, \mathfrak{z} 1 \, \mathfrak{z} 2 + 4 \, \eta^2 \, \theta p \, \mathfrak{z} 1 \, \mathfrak{z} 2 + 3 \, \theta p \, \mathfrak{z} 2^2 + \\
& \quad 6 \, \eta \, \theta p \, \mathfrak{z} 2^2 - 5 \, \theta p \, \mathfrak{z} 1 \, \mathfrak{z} 2^2 + 10 \, \eta \, \theta p \, \mathfrak{z} 1 \, \mathfrak{z} 2^2 + 2 \, w^2 \left( -1 + \eta \right)^2 \left( -3 \times \left( 2 + \mathfrak{z} 2 \right) + \right. \\
& \quad \left. \mathfrak{z} 1 \left( -4 + 5 \, \mathfrak{z} 2 \right) + \theta p \left( \mathfrak{z} 1^2 + 3 \left( 2 + \mathfrak{z} 2 \right)^2 + 2 \, \mathfrak{z} 1 \left( 8 + \mathfrak{z} 2 \right) \right) \right) - \\
& \quad w \left( -1 + \eta \right) \times \left( 4 \times \left( -3 \times \left( 2 + \mathfrak{z} 2 \right) + \mathfrak{z} 1 \left( -4 + 5 \, \mathfrak{z} 2 \right) \right) + \right. \\
& \quad \left. \theta p \left( 44 + 4 \, \mathfrak{z} 1^2 + 40 \, \mathfrak{z} 2 + 9 \, \mathfrak{z} 2^2 + \mathfrak{z} 1 \left( 60 - 4 \, \mathfrak{z} 2 - 5 \, \mathfrak{z} 2^2 \right) + \right. \right. \\
& \quad \left. \left. 2 \, \eta \left( 10 + 11 \, \mathfrak{z} 2 + 3 \, \mathfrak{z} 2^2 + \mathfrak{z} 1 \left( 16 + 9 \, \mathfrak{z} 2 + 5 \, \mathfrak{z} 2^2 \right) \right) \right) \right) \left. \right) \left. \right) + \\
& 2 \, \text{co}^2 \left( -1 + \eta \right)^2 \left( w^5 \left( -1 + \eta \right)^6 \left( 2 \, x^5 \left( -1 + \eta \right)^5 \text{op} \left( \eta - \eta t + 4 \, \mu 1 \right) \right. \right. \\
& \quad \left. \left( 3 + 4 \, \mu 2 + \mathfrak{z} 1 + \mu 1 \left( 3 + \mathfrak{z} 1 \right) \right) - \right. \\
& \quad \left. x^4 \left( -1 + \eta \right)^3 \left( \left( -1 + \eta t \right) \theta l \left( -18 - 21 \, \mu 2 + 8 \, \mu 2^2 - 10 \, \mathfrak{z} 1 + 5 \, \mu 2 \, \mathfrak{z} 1 - \right. \right. \right. \\
& \quad \left. \left. 20 \, \mu 1 \left( 1 + \mathfrak{z} 1 \right) + \mu 1 \, \mu 2 \left( 43 + 5 \, \mathfrak{z} 1 \right) + \mu 1^2 \left( -2 + 26 \, \mathfrak{z} 1 \right) \right) + 2 \times \right.
\end{aligned}$$



$$\begin{aligned}
& (-1 + \eta) \, \Theta p \left( 9 + 42 \mu_1 + 33 \mu_1^2 + 27 \mu_2 + 59 \mu_1 \mu_2 + 5 \, \Xi_1 + 12 \mu_1 \, \Xi_1 + \right. \\
& \quad 7 \mu_1^2 \, \Xi_1 + 11 \mu_2 \, \Xi_1 - 7 \mu_1 \mu_2 \, \Xi_1 + 5 \eta^2 (3 + 4 \mu_2 + \Xi_1 + \mu_1 (3 + \Xi_1)) + \\
& \quad \eta (-5 \eta t (3 + 4 \mu_2 + \Xi_1 + \mu_1 (3 + \Xi_1)) + 2 \times (3 - \mu_2 - 14 \mu_2^2 + \\
& \quad \quad \mu_1 \mu_2 (35 - 3 \, \Xi_1) + \Xi_1 + 11 \mu_1 (3 + \Xi_1) + 10 \mu_1^2 (3 + \Xi_1)) \Big) + \\
& \quad 2 \eta t (-3 + \mu_2 + 14 \mu_2^2 - \Xi_1 + \mu_1 (-3 - \Xi_1 + \mu_2 (5 + 3 \, \Xi_1))) \Big) - \\
& \eta \, \Theta p \left( 2 \eta^5 (3 + 4 \mu_2 + \Xi_1 + \mu_1 (3 + \Xi_1)) + \eta t \mu_2 (11 + 8 \mu_2 + 5 \, \Xi_1 + \right. \\
& \quad \mu_1 (11 + 5 \, \Xi_1)) + 2 \eta \eta t (-9 + 8 \mu_2^2 + \mu_1^2 (-21 + \Xi_1) + \\
& \quad 5 \mu_2 (-1 + \Xi_1) - 5 \, \Xi_1 + 5 \mu_1 (\mu_2 (-1 + \Xi_1) - 2 \times (3 + \Xi_1))) - 2 \\
& \quad \eta^4 (\eta t (3 + 4 \mu_2 + \Xi_1 + \mu_1 (3 + \Xi_1)) - 2 \times (3 - \mu_2 - 14 \mu_2^2 + \\
& \quad \quad \Xi_1 + 2 \mu_1^2 (3 + \Xi_1) + 3 \mu_1 (3 + \mu_2 + \Xi_1 - \mu_2 \, \Xi_1))) + 2 \\
& \quad \eta^3 (12 + 21 \mu_2 - 52 \mu_2^2 + 6 \, \Xi_1 + 11 \mu_2 \, \Xi_1 + \mu_1^2 (33 + 7 \, \Xi_1) + \\
& \quad \mu_1 (45 + 49 \mu_2 + 13 \, \Xi_1 - 13 \mu_2 \, \Xi_1) + \\
& \quad 2 \eta t (-3 + \mu_2 + 14 \mu_2^2 - \Xi_1 + \mu_1 (-3 + 5 \mu_2 - \Xi_1 + 3 \mu_2 \, \Xi_1))) + \eta^2 \\
& \quad (2 \times (9 + 32 \mu_2^2 + 5 \, \Xi_1 + 3 \mu_1^2 (7 + \Xi_1) + \mu_2 (47 + 11 \, \Xi_1) + \\
& \quad \quad \mu_1 (30 + 8 \, \Xi_1 + \mu_2 (63 + 5 \, \Xi_1))) + \\
& \quad \eta t (64 \mu_2^2 - 12 \times (2 + \Xi_1) + \mu_2 (-9 + 5 \, \Xi_1) + \mu_1^2 (-2 + 26 \, \Xi_1) + \\
& \quad \quad \mu_1 (-26 - 22 \, \Xi_1 + \mu_2 (111 + 17 \, \Xi_1))) \Big) + \\
& x^3 (-1 + \eta)^2 \left( (-1 + \eta t) \, \Theta l \left( 2 \times (-9 + 8 \mu_2^2 + \mu_1^2 (-21 + \Xi_1) + \right. \right. \\
& \quad 5 \mu_2 (-1 + \Xi_1) - 5 \, \Xi_1 + 5 \mu_1 (\mu_2 (-1 + \Xi_1) - 2 \times (3 + \Xi_1))) + \\
& \quad \eta (-58 + 12 \mu_2^2 - 30 \, \Xi_1 + 6 \mu_1^2 (-5 + 11 \, \Xi_1) + \mu_2 (-79 + 15 \, \Xi_1) + \\
& \quad \quad \mu_1 (-88 - 60 \, \Xi_1 + 3 \mu_2 (51 + 5 \, \Xi_1))) \Big) + \\
& (-1 + \eta) \, \Theta p \left( 20 \eta^3 (3 + 4 \mu_2 + \Xi_1 + \mu_1 (3 + \Xi_1)) - 4 \eta^2 \right. \\
& \quad (5 \eta t (3 + 4 \mu_2 + \Xi_1 + \mu_1 (3 + \Xi_1)) - 4 \times (3 - \mu_2 - 14 \mu_2^2 - \\
& \quad \quad 3 \mu_1 \mu_2 (-5 + \Xi_1) + \Xi_1 + 6 \mu_1 (3 + \Xi_1) + 5 \mu_1^2 (3 + \Xi_1))) + \\
& \quad 2 \times (9 + 32 \mu_2^2 + 5 \, \Xi_1 + 3 \mu_1^2 (7 + \Xi_1) + \mu_2 (47 + 11 \, \Xi_1) + \\
& \quad \quad \mu_1 (30 + 8 \, \Xi_1 + \mu_2 (63 + 5 \, \Xi_1))) + \eta t (76 \mu_2^2 - 4 \times (5 + 3 \, \Xi_1) + \\
& \quad \quad \mu_2 (7 + 5 \, \Xi_1) + \mu_1^2 (22 + 38 \, \Xi_1) + \mu_1 (2 - 22 \, \Xi_1 + \mu_2 (87 + 17 \, \Xi_1))) + \\
& \quad 2 \eta (39 + 102 \mu_2 - 52 \mu_2^2 + 21 \, \Xi_1 + 44 \mu_2 \, \Xi_1 + 4 \mu_1^2 (33 + 7 \, \Xi_1) + \\
& \quad \quad \mu_1 (171 + 226 \mu_2 + 49 \, \Xi_1 - 34 \mu_2 \, \Xi_1) + \\
& \quad \quad 8 \eta t (-3 + \mu_2 + 14 \mu_2^2 - \Xi_1 + \mu_1 (-3 + 5 \mu_2 - \Xi_1 + 3 \mu_2 \, \Xi_1))) \Big) - \\
& x^2 (-1 + \eta) \times \left( 20 \eta^5 \, \Theta p (3 + 4 \mu_2 + \Xi_1 + \mu_1 (3 + \Xi_1)) - \Theta l \mu_2 \right. \\
& \quad (11 + 8 \mu_2 + 5 \, \Xi_1 + \mu_1 (11 + 5 \, \Xi_1)) - 4 \eta^4 \, \Theta p \\
& \quad (-3 + 26 \mu_2 + 84 \mu_2^2 - \Xi_1 - 21 \mu_1 (3 + \Xi_1) - 20 \mu_1^2 (3 + \Xi_1) + \\
& \quad \quad 2 \mu_1 \mu_2 (-25 + 9 \, \Xi_1) + 5 \eta t (3 + 4 \mu_2 + \Xi_1 + \mu_1 (3 + \Xi_1))) + \eta t \\
& \quad (-2 \, \Theta p (-5 + 11 \mu_2 + 20 \mu_2^2 + 7 \mu_1^2 (-1 + \Xi_1) - 5 \, \Xi_1 + \\
& \quad \quad 5 \mu_2 \, \Xi_1 + 5 \mu_1 \mu_2 (3 + \Xi_1) - 2 \mu_1 (6 + 5 \, \Xi_1)) + \\
& \quad \quad \Theta l \mu_2 (11 + 8 \mu_2 + 5 \, \Xi_1 + \mu_1 (11 + 5 \, \Xi_1))) + 2 \eta^3 \, \Theta p \\
& \quad (2 \mu_1^2 (39 + \Xi_1) + \mu_1 (105 + 224 \mu_2 + 23 \, \Xi_1 - 24 \mu_2 \, \Xi_1) + \\
& \quad \quad 3 \times (9 + 52 \mu_2 + 4 \mu_2^2 + 7 \, \Xi_1 + 22 \mu_2 \, \Xi_1) + \\
& \quad \quad 2 \eta t (-3 + 26 \mu_2 + 84 \mu_2^2 - \Xi_1 + \mu_1 (-3 - \Xi_1 + 6 \mu_2 (5 + 3 \, \Xi_1))) \Big) + \eta^2 \\
& \quad (-1 + \eta t) \, \Theta l (-62 + 54 \mu_1^2 (-1 + \Xi_1) - 30 \, \Xi_1 + 5 \mu_2 (-19 + 3 \, \Xi_1) + \\
& \quad \quad 3 \mu_1 \mu_2 (59 + 5 \, \Xi_1) - 4 \mu_1 (29 + 15 \, \Xi_1)) + \\
& \quad \Theta p (-6 \times (12 + \mu_2 - 84 \mu_2^2 + 6 \, \Xi_1 + 11 \mu_2 \, \Xi_1 + \mu_1^2 (45 + 11 \, \Xi_1) +
\end{aligned}$$

$$\begin{aligned}
& \mu_1 (57 + 45 \mu_2 + 17 \mathfrak{z}_1 - 25 \mu_2 \mathfrak{z}_1) + \\
& \eta t (8 - 19 \mu_2 - 120 \mu_2^2 - 12 \mathfrak{z}_1 + 15 \mu_2 \mathfrak{z}_1 + 6 \mu_1^2 (7 + 17 \mathfrak{z}_1) + \\
& \mu_1 (50 + 165 \mu_2 - 42 \mathfrak{z}_1 - 21 \mu_2 \mathfrak{z}_1)) - \eta \\
& (4 \times (-1 + \eta t) \mathfrak{el} (11 + 13 \mu_2 - 2 \mu_2^2 + 5 \mathfrak{z}_1 - 5 \mu_2 \mathfrak{z}_1 + 2 \mu_1^2 \\
& (14 + \mathfrak{z}_1) + \mu_1 (39 - 5 \mu_2 (-3 + \mathfrak{z}_1) + 10 \mathfrak{z}_1)) + \\
& \mathfrak{op} (6 \times (9 + 47 \mu_2 + 32 \mu_2^2 + 5 \mathfrak{z}_1 + 11 \mu_2 \mathfrak{z}_1 + 3 \mu_1^2 (7 + \mathfrak{z}_1) + \\
& \mu_1 (30 + 63 \mu_2 + 8 \mathfrak{z}_1 + 5 \mu_2 \mathfrak{z}_1)) + \\
& \eta t (-54 - 17 \mu_2 + 176 \mu_2^2 - 26 \mathfrak{z}_1 + 5 \mu_2 \mathfrak{z}_1 + 8 \mu_1^2 \\
& (7 + 11 \mathfrak{z}_1) + \mu_1 (2 + 255 \mu_2 - 46 \mathfrak{z}_1 + 41 \mu_2 \mathfrak{z}_1))) + \\
& \times (10 \eta^6 \mathfrak{op} (3 + 4 \mu_2 + \mathfrak{z}_1 + \mu_1 (3 + \mathfrak{z}_1)) - 2 \eta^5 \mathfrak{op} (-9 + 28 \mu_2 + \\
& 112 \mu_2^2 - 3 \mathfrak{z}_1 - 23 \mu_1 (3 + \mathfrak{z}_1) - 20 \mu_1^2 (3 + \mathfrak{z}_1) + \\
& 8 \mu_1 \mu_2 (-5 + 3 \mathfrak{z}_1) + 5 \eta t (3 + 4 \mu_2 + \mathfrak{z}_1 + \mu_1 (3 + \mathfrak{z}_1))) + 2 \\
& \eta^4 \mathfrak{op} (21 + 98 \mu_2 - 44 \mu_2^2 + 15 \mathfrak{z}_1 + 44 \mu_2 \mathfrak{z}_1 + 8 \mu_1^2 (9 + \mathfrak{z}_1) + \\
& \mu_1 (93 + 166 \mu_2 + 23 \mathfrak{z}_1 - 22 \mu_2 \mathfrak{z}_1) + \\
& \eta t (-9 + 28 \mu_2 + 112 \mu_2^2 - 3 \mathfrak{z}_1 - 3 \mu_1 (3 + \mathfrak{z}_1) + 8 \mu_1 \mu_2 (5 + 3 \mathfrak{z}_1))) - \eta t \\
& \mathfrak{op} (4 + 4 \mu_1^2 + 20 \mu_2^2 + \mu_2 (27 + 5 \mathfrak{z}_1) + \mu_1 (8 + \mu_2 (27 + 5 \mathfrak{z}_1))) + \eta \\
& (\eta t \mathfrak{op} (32 + 15 \mu_2 - 36 \mu_2^2 + \mu_1^2 (60 - 16 \mathfrak{z}_1) + 20 \mathfrak{z}_1 - 15 \mu_2 \mathfrak{z}_1 + \\
& \mu_1 (92 + 7 \mu_2 + 40 \mathfrak{z}_1 - 15 \mu_2 \mathfrak{z}_1)) - (-1 + \eta t) \mathfrak{el} \\
& (4 + 4 \mu_1^2 + 5 \mu_2 + 4 \mu_2^2 - 5 \mu_2 \mathfrak{z}_1 + \mu_1 (8 + 5 \mu_2 - 5 \mu_2 \mathfrak{z}_1))) - \\
& \eta^2 (2 \times (-1 + \eta t) \mathfrak{el} (13 + 21 \mu_2 + 4 \mu_2^2 + 5 \mathfrak{z}_1 - 5 \mu_2 \mathfrak{z}_1 + \\
& 5 \mu_1^2 (7 + \mathfrak{z}_1) + \mu_1 (48 - 5 \mu_2 (-5 + \mathfrak{z}_1) + 10 \mathfrak{z}_1)) + \\
& \mathfrak{op} (6 \times (9 + 47 \mu_2 + 32 \mu_2^2 + 5 \mathfrak{z}_1 + 11 \mu_2 \mathfrak{z}_1 + 3 \mu_1^2 (7 + \mathfrak{z}_1) + \\
& \mu_1 (30 + 63 \mu_2 + 8 \mathfrak{z}_1 + 5 \mu_2 \mathfrak{z}_1)) + \\
& \eta t (-40 - 23 \mu_2 + 148 \mu_2^2 - 16 \mathfrak{z}_1 - 5 \mu_2 \mathfrak{z}_1 + 74 \mu_1^2 (1 + \mathfrak{z}_1) + \\
& \mu_1 (34 + 289 \mu_2 - 26 \mathfrak{z}_1 + 31 \mu_2 \mathfrak{z}_1))) + \eta^3 \\
& ((-1 + \eta t) \mathfrak{el} (-22 - 37 \mu_2 - 4 \mu_2^2 - 10 \mathfrak{z}_1 + 5 \mu_2 \mathfrak{z}_1 + 2 \mu_1^2 \\
& (-13 + 7 \mathfrak{z}_1) + \mu_1 (-48 + 67 \mu_2 - 20 \mathfrak{z}_1 + 5 \mu_2 \mathfrak{z}_1)) + \\
& \mathfrak{op} (-2 \times (18 - 252 \mu_2^2 + 8 \mathfrak{z}_1 + \mu_2 (-51 + 11 \mathfrak{z}_1) + \mu_1^2 \\
& (69 + 19 \mathfrak{z}_1) + \mu_1 (87 + \mu_2 (17 - 61 \mathfrak{z}_1) + 27 \mathfrak{z}_1)) + \\
& \eta t (-20 \mu_2^2 - 20 \times (1 + \mathfrak{z}_1) + 3 \mu_2 (-9 + 5 \mathfrak{z}_1) + 18 \mu_1^2 \\
& (1 + 5 \mathfrak{z}_1) + \mu_1 (-2 - 50 \mathfrak{z}_1 + \mu_2 (229 + 3 \mathfrak{z}_1)))) + \\
& w^4 (-1 + \eta)^4 (6 x^6 (-1 + \eta)^7 \mathfrak{op} (\eta - \eta t + 4 \mu_1) (3 + 4 \mu_2 + \mathfrak{z}_1 + \mu_1 (3 + \mathfrak{z}_1)) + \\
& x^5 (-1 + \eta)^5 (-2 \times (-1 + \eta) \mathfrak{op} (47 + 185 \mu_1 + 138 \mu_1^2 + 141 \mu_2 + \\
& 237 \mu_1 \mu_2 + 15 \mathfrak{z}_1 + 51 \mu_1 \mathfrak{z}_1 + 30 \mu_1^2 \mathfrak{z}_1 + 33 \mu_2 \mathfrak{z}_1 - \\
& 21 \mu_1 \mu_2 \mathfrak{z}_1 + 18 \eta^2 (3 + 4 \mu_2 + \mathfrak{z}_1 + \mu_1 (3 + \mathfrak{z}_1)) + \\
& \eta (29 + 14 \mu_2 - 84 \mu_2^2 + 9 \mathfrak{z}_1 + 72 \mu_1^2 (3 + \mathfrak{z}_1) + \mu_1 (245 + 258 \mu_2 + \\
& 81 \mathfrak{z}_1 - 18 \mu_2 \mathfrak{z}_1) - 18 \eta t (3 + 4 \mu_2 + \mathfrak{z}_1 + \mu_1 (3 + \mathfrak{z}_1))) + \\
& \eta t (-29 - 14 \mu_2 + 84 \mu_2^2 - 9 \mathfrak{z}_1 + \mu_1 (-29 - 9 \mathfrak{z}_1 + 6 \mu_2 (5 + 3 \mathfrak{z}_1)))) + \\
& (-1 + \eta t) \mathfrak{el} (-2 \times (-11 + 24 \mu_2 + 36 \mu_2^2 - 15 \mathfrak{z}_1 + \mu_1^2 (29 + 27 \mathfrak{z}_1) + \\
& 6 \mu_1 (3 - 6 \mathfrak{z}_1 + 2 \mu_2 (12 + \mathfrak{z}_1))) + \mathfrak{op} (72 + 17 \mathfrak{z}_1 + 5 \mathfrak{z}_1^2 + \\
& 12 \mu_2^2 (6 + 3 \mathfrak{z}_1 - \mathfrak{z}_2) + 7 \mathfrak{z}_2 - 5 \mathfrak{z}_1 \mathfrak{z}_2 + 12 \mu_1^2 (6 + \mathfrak{z}_1 + \mathfrak{z}_2) + \\
& \mu_2 (288 + 59 \mathfrak{z}_1 + 5 \mathfrak{z}_1^2 + 37 \mathfrak{z}_2 - 5 \mathfrak{z}_1 \mathfrak{z}_2) + \mu_1 (144 + 29 \mathfrak{z}_1 + 11 \mathfrak{z}_1^2 + \\
& 19 \mathfrak{z}_2 - 11 \mathfrak{z}_1 \mathfrak{z}_2 + \mu_2 (288 + 5 \mathfrak{z}_1^2 - 5 \mathfrak{z}_1 (-7 + \mathfrak{z}_2) + 61 \mathfrak{z}_2)))) +
\end{aligned}$$

$$\begin{aligned}
& \eta \, \theta p \left( 6 \eta^7 (3 + 4 \mu_2 + \mathfrak{e}1 + \mu_1 (3 + \mathfrak{e}1)) - 3 \eta t \mu_2 (11 + 8 \mu_2 + 5 \mathfrak{e}1 + \right. \\
& \quad \mu_1 (11 + 5 \mathfrak{e}1)) + \eta \eta t (-96 \mu_2^2 - 8 \mu_1^2 (-14 + \mathfrak{e}1) + 40 \times (1 + \mathfrak{e}1) - \\
& \quad 3 \mu_2 (11 + 5 \mathfrak{e}1) + \mu_1 (152 + 68 \mathfrak{e}1 - 3 \mu_2 (11 + 13 \mathfrak{e}1))) - 2 \eta^6 \\
& \quad (3 \eta t (3 + 4 \mu_2 + \mathfrak{e}1 + \mu_1 (3 + \mathfrak{e}1)) - 2 \times (10 + \mu_2 - 42 \mu_2^2 + 3 \mathfrak{e}1 + \\
& \quad 6 \mu_1^2 (3 + \mathfrak{e}1) + \mu_1 (28 + 9 \mu_2 + 9 \mathfrak{e}1 - 9 \mu_2 \mathfrak{e}1))) + 2 \eta^5 \\
& \quad (49 + 119 \mu_2 - 156 \mu_2^2 + 15 \mathfrak{e}1 + 33 \mu_2 \mathfrak{e}1 + 6 \mu_1^2 (17 + 3 \mathfrak{e}1) + \\
& \quad \mu_1 (151 + 159 \mu_2 + 39 \mathfrak{e}1 - 39 \mu_2 \mathfrak{e}1) + \\
& \quad 2 \eta t (-10 - \mu_2 + 42 \mu_2^2 - 3 \mathfrak{e}1 + \mu_1 (-10 + 15 \mu_2 - 3 \mathfrak{e}1 + 9 \mu_2 \mathfrak{e}1))) - \\
& \eta^3 (116 + 320 \mu_1 + 144 \eta t \mu_1 + 204 \mu_1^2 + 144 \eta t \mu_1^2 + 294 \mu_2 - \\
& \quad 37 \eta t \mu_2 + 350 \mu_1 \mu_2 + 139 \eta t \mu_1 \mu_2 - 200 \mu_2^2 + 72 \eta t \mu_2^2 + 36 \mathfrak{e}1 + \\
& \quad 28 \eta t \mathfrak{e}1 + 84 \mu_1 \mathfrak{e}1 + 64 \eta t \mu_1 \mathfrak{e}1 + 36 \mu_1^2 \mathfrak{e}1 - 24 \eta t \mu_1^2 \mathfrak{e}1 + 74 \mu_2 \mathfrak{e}1 - \\
& \quad 15 \eta t \mu_2 \mathfrak{e}1 - 94 \mu_1 \mu_2 \mathfrak{e}1 - 3 \eta t \mu_1 \mu_2 \mathfrak{e}1 + 2 \times (-1 + \eta t) \, \theta l (72 + 17 \mathfrak{e}1 + \\
& \quad 5 \mathfrak{e}1^2 + 12 \mu_2^2 (6 + 3 \mathfrak{e}1 - \mathfrak{e}2) + 7 \mathfrak{e}2 - 5 \mathfrak{e}1 \mathfrak{e}2 + 12 \mu_1^2 (6 + \mathfrak{e}1 + \mathfrak{e}2) + \\
& \quad \mu_2 (288 + 59 \mathfrak{e}1 + 5 \mathfrak{e}1^2 + 37 \mathfrak{e}2 - 5 \mathfrak{e}1 \mathfrak{e}2) + \mu_1 (144 + 29 \mathfrak{e}1 + 11 \mathfrak{e}1^2 + \\
& \quad 19 \mathfrak{e}2 - 11 \mathfrak{e}1 \mathfrak{e}2 + \mu_2 (288 + 5 \mathfrak{e}1^2 - 5 \mathfrak{e}1 (-7 + \mathfrak{e}2) + 61 \mathfrak{e}2))) + \\
& \eta^4 (72 + 150 \mu_1 + 78 \mu_1^2 + 520 \mu_2 + 488 \mu_1 \mu_2 + 520 \mu_2^2 + 28 \mathfrak{e}1 + \\
& \quad 26 \mu_1 \mathfrak{e}1 - 14 \mu_1^2 \mathfrak{e}1 + 68 \mu_2 \mathfrak{e}1 + 32 \mu_1 \mu_2 \mathfrak{e}1 + \\
& \quad 2 \eta t (-13 + 92 \mu_2^2 - 2 \mu_2 (-19 + \mathfrak{e}1) - 15 \mathfrak{e}1 + \mu_1^2 (37 + 23 \mathfrak{e}1) + \\
& \quad \mu_1 (24 - 34 \mathfrak{e}1 + \mu_2 (266 + 34 \mathfrak{e}1))) + \theta l (72 + 17 \mathfrak{e}1 + 5 \mathfrak{e}1^2 + \\
& \quad 12 \mu_2^2 (6 + 3 \mathfrak{e}1 - \mathfrak{e}2) + 7 \mathfrak{e}2 - 5 \mathfrak{e}1 \mathfrak{e}2 + 12 \mu_1^2 (6 + \mathfrak{e}1 + \mathfrak{e}2) + \\
& \quad \mu_2 (288 + 59 \mathfrak{e}1 + 5 \mathfrak{e}1^2 + 37 \mathfrak{e}2 - 5 \mathfrak{e}1 \mathfrak{e}2) + \mu_1 (144 + 29 \mathfrak{e}1 + 11 \mathfrak{e}1^2 + \\
& \quad 19 \mathfrak{e}2 - 11 \mathfrak{e}1 \mathfrak{e}2 + \mu_2 (288 + 5 \mathfrak{e}1^2 - 5 \mathfrak{e}1 (-7 + \mathfrak{e}2) + 61 \mathfrak{e}2))) - \\
& \eta t \, \theta l (72 + 17 \mathfrak{e}1 + 5 \mathfrak{e}1^2 + 12 \mu_2^2 (6 + 3 \mathfrak{e}1 - \mathfrak{e}2) + 7 \mathfrak{e}2 - 5 \mathfrak{e}1 \mathfrak{e}2 + \\
& \quad 12 \mu_1^2 (6 + \mathfrak{e}1 + \mathfrak{e}2) + \mu_2 (288 + 59 \mathfrak{e}1 + 5 \mathfrak{e}1^2 + 37 \mathfrak{e}2 - 5 \mathfrak{e}1 \mathfrak{e}2) + \\
& \quad \mu_1 (144 + 29 \mathfrak{e}1 + 11 \mathfrak{e}1^2 + 19 \mathfrak{e}2 - 11 \mathfrak{e}1 \mathfrak{e}2 + \\
& \quad \mu_2 (288 + 5 \mathfrak{e}1^2 - 5 \mathfrak{e}1 (-7 + \mathfrak{e}2) + 61 \mathfrak{e}2))) - \eta^2 \\
& (2 \times (56 + 120 \mu_2^2 + 20 \mathfrak{e}1 + 5 \mu_1^2 (15 + \mathfrak{e}1) + 6 \mu_2 (41 + 5 \mathfrak{e}1) + \\
& \quad \mu_1 (131 + 31 \mathfrak{e}1 + 6 \mu_2 (41 + \mathfrak{e}1))) - \theta l (72 + 17 \mathfrak{e}1 + 5 \mathfrak{e}1^2 + \\
& \quad 12 \mu_2^2 (6 + 3 \mathfrak{e}1 - \mathfrak{e}2) + 7 \mathfrak{e}2 - 5 \mathfrak{e}1 \mathfrak{e}2 + 12 \mu_1^2 (6 + \mathfrak{e}1 + \mathfrak{e}2) + \\
& \quad \mu_2 (288 + 59 \mathfrak{e}1 + 5 \mathfrak{e}1^2 + 37 \mathfrak{e}2 - 5 \mathfrak{e}1 \mathfrak{e}2) + \mu_1 (144 + 29 \mathfrak{e}1 + 11 \mathfrak{e}1^2 + \\
& \quad 19 \mathfrak{e}2 - 11 \mathfrak{e}1 \mathfrak{e}2 + \mu_2 (288 + 5 \mathfrak{e}1^2 - 5 \mathfrak{e}1 (-7 + \mathfrak{e}2) + 61 \mathfrak{e}2))) + \\
& \eta t (-44 - 2 \mu_1 + 42 \mu_1^2 + 19 \mu_2 + 387 \mu_1 \mu_2 + 160 \mu_2^2 - 36 \mathfrak{e}1 - \\
& \quad 82 \mu_1 \mathfrak{e}1 + 62 \mu_1^2 \mathfrak{e}1 - 19 \mu_2 \mathfrak{e}1 + 53 \mu_1 \mu_2 \mathfrak{e}1 + \\
& \quad \theta l (72 + 17 \mathfrak{e}1 + 5 \mathfrak{e}1^2 + 12 \mu_2^2 (6 + 3 \mathfrak{e}1 - \mathfrak{e}2) + 7 \mathfrak{e}2 - 5 \mathfrak{e}1 \mathfrak{e}2 + \\
& \quad 12 \mu_1^2 (6 + \mathfrak{e}1 + \mathfrak{e}2) + \mu_2 (288 + 59 \mathfrak{e}1 + 5 \mathfrak{e}1^2 + 37 \mathfrak{e}2 - 5 \mathfrak{e}1 \mathfrak{e}2) + \\
& \quad \mu_1 (144 + 29 \mathfrak{e}1 + 11 \mathfrak{e}1^2 + 19 \mathfrak{e}2 - 11 \mathfrak{e}1 \mathfrak{e}2 + \\
& \quad \mu_2 (288 + 5 \mathfrak{e}1^2 - 5 \mathfrak{e}1 (-7 + \mathfrak{e}2) + 61 \mathfrak{e}2)))) + \\
& x^4 (-1 + \eta)^4 (2 \times (-1 + \eta) \, \theta p (103 - 38 \eta t + 280 \mu_1 + 25 \eta t \mu_1 + \\
& \quad 177 \mu_1^2 + 63 \eta t \mu_1^2 + 395 \mu_2 + 40 \eta t \mu_2 + 443 \mu_1 \mu_2 + \\
& \quad 244 \eta t \mu_1 \mu_2 + 168 \mu_2^2 + 188 \eta t \mu_2^2 + 35 \mathfrak{e}1 - 24 \eta t \mathfrak{e}1 + 70 \mu_1 \mathfrak{e}1 - \\
& \quad 43 \eta t \mu_1 \mathfrak{e}1 + 23 \mu_1^2 \mathfrak{e}1 + 41 \eta t \mu_1^2 \mathfrak{e}1 + 67 \mu_2 \mathfrak{e}1 - 2 \eta t \mu_2 \mathfrak{e}1 - \\
& \quad 23 \mu_1 \mu_2 \mathfrak{e}1 + 52 \eta t \mu_1 \mu_2 \mathfrak{e}1 + 45 \eta^3 (3 + 4 \mu_2 + \mathfrak{e}1 + \mu_1 (3 + \mathfrak{e}1)) - \\
& \quad 5 \eta^2 (-29 - 14 \mu_2 + 84 \mu_2^2 - 9 \mathfrak{e}1 - 36 \mu_1^2 (3 + \mathfrak{e}1) + 9 \eta t (3 + 4 \mu_2 +
\end{aligned}$$

$$\begin{aligned}
& \left( \mu_1 + \mu_1 (3 + \mu_1) \right) + \mu_1 (-137 - 45 \mu_1 + 6 \mu_2 (-19 + 3 \mu_1)) \Big) + \\
& \eta \left( 266 + 697 \mu_2 - 240 \mu_2^2 + 84 \mu_1 + 165 \mu_2 \mu_1 + 30 \mu_1^2 (23 + 5 \mu_1) + \right. \\
& \quad \left. \mu_1 (956 + 1125 \mu_2 + 264 \mu_1 - 141 \mu_2 \mu_1) + 5 \eta t \right. \\
& \quad \left. (-29 - 14 \mu_2 + 84 \mu_2^2 - 9 \mu_1 + \mu_1 (-29 - 9 \mu_1 + 6 \mu_2 (5 + 3 \mu_1))) \right) \Big) - \\
& (-1 + \eta t) \, \theta l \left( 62 + 132 \mu_1 + 70 \mu_1^2 - 81 \mu_2 - 225 \mu_1 \mu_2 - 168 \mu_2^2 + \right. \\
& \quad 70 \mu_1 + 148 \mu_1 \mu_1 - 78 \mu_1^2 \mu_1 - 15 \mu_2 \mu_1 - 63 \mu_1 \mu_2 \mu_1 + \\
& \quad 2 \, \theta p \left( 72 + 17 \mu_1 + 5 \mu_1^2 + 12 \mu_2^2 (6 + 3 \mu_1 - \mu_2) + 7 \mu_2 - 5 \mu_1 \mu_2 + \right. \\
& \quad \left. 12 \mu_1^2 (6 + \mu_1 + \mu_2) + \mu_2 (288 + 59 \mu_1 + 5 \mu_1^2 + 37 \mu_2 - 5 \mu_1 \mu_2) + \right. \\
& \quad \left. \mu_1 (144 + 29 \mu_1 + 11 \mu_1^2 + 19 \mu_2 - 11 \mu_1 \mu_2 + \right. \\
& \quad \left. \mu_2 (288 + 5 \mu_1^2 - 5 \mu_1 (-7 + \mu_2) + 61 \mu_2) \right) \Big) + \\
& \eta \left( -4 \times (40 \mu_2 + 66 \mu_2^2 + 45 \mu_1^2 (1 + \mu_1) - 6 \times (4 + 5 \mu_1) + \right. \\
& \quad \left. \mu_1 (21 - 72 \mu_1 + \mu_2 (314 + 24 \mu_1)) \right) + 5 \, \theta p \\
& \quad \left( 72 + 17 \mu_1 + 5 \mu_1^2 + 12 \mu_2^2 (6 + 3 \mu_1 - \mu_2) + 7 \mu_2 - 5 \mu_1 \mu_2 + \right. \\
& \quad \left. 12 \mu_1^2 (6 + \mu_1 + \mu_2) + \mu_2 (288 + 59 \mu_1 + 5 \mu_1^2 + 37 \mu_2 - 5 \mu_1 \mu_2) + \right. \\
& \quad \left. \mu_1 (144 + 29 \mu_1 + 11 \mu_1^2 + 19 \mu_2 - 11 \mu_1 \mu_2 + \right. \\
& \quad \left. \mu_2 (288 + 5 \mu_1^2 - 5 \mu_1 (-7 + \mu_2) + 61 \mu_2) \right) \Big) \Big) + \\
& x^3 (-1 + \eta)^3 \left( - \left( (-1 + \eta) \, \theta p (120 \eta^4 (3 + 4 \mu_2 + \mu_1 + \mu_1 (3 + \mu_1)) - \right. \right. \\
& \quad 20 \eta^3 (-29 - 14 \mu_2 + 84 \mu_2^2 - 9 \mu_1 - 24 \mu_1^2 (3 + \mu_1) + \mu_1 (-101 - \\
& \quad \left. 66 \mu_2 - 33 \mu_1 + 18 \mu_2 \mu_1) + 6 \eta t (3 + 4 \mu_2 + \mu_1 + \mu_1 (3 + \mu_1)) \right) + \\
& \quad 2 \times (56 + 120 \mu_2^2 + 20 \mu_1 + 5 \mu_1^2 (15 + \mu_1) + 6 \mu_2 (41 + 5 \mu_1) + \\
& \quad \left. \mu_1 (131 + 31 \mu_1 + 6 \mu_2 (41 + \mu_1)) \right) + \\
& \quad \eta t (-56 + 364 \mu_2^2 - 76 \mu_1 + \mu_2 (197 + 11 \mu_1) + 2 \mu_1^2 \\
& \quad \left. (39 + 71 \mu_1) + \mu_1 (22 - 150 \mu_1 + \mu_2 (469 + 107 \mu_1)) \right) + \\
& \quad 2 \eta (423 + 1578 \mu_2 + 524 \mu_2^2 + 143 \mu_1 + 268 \mu_2 \mu_1 + \\
& \quad \mu_1^2 (708 + 92 \mu_1) + \mu_1 (1131 + 1750 \mu_2 + 283 \mu_1 - 110 \mu_2 \mu_1) + \\
& \quad 2 \eta t (-78 + 72 \mu_2 + 370 \mu_2^2 - 48 \mu_1 - 4 \mu_2 \mu_1 + \\
& \quad \mu_1^2 (113 + 73 \mu_1) + \mu_1 (35 + 514 \mu_2 - 86 \mu_1 + 104 \mu_2 \mu_1)) \Big) + \\
& \quad 4 \eta^2 (297 + 689 \mu_2 - 480 \mu_2^2 + 93 \mu_1 + 165 \mu_2 \mu_1 + 30 \mu_1^2 \\
& \quad \left. (23 + 5 \mu_1) + 3 \mu_1 (329 + 355 \mu_2 + 91 \mu_1 - 59 \mu_2 \mu_1) + 5 \eta t (-29 - \right. \\
& \quad \left. 14 \mu_2 + 84 \mu_2^2 - 9 \mu_1 + \mu_1 (-29 - 9 \mu_1 + 6 \mu_2 (5 + 3 \mu_1))) \right) \Big) + \\
& (-1 + \eta t) \, \theta l \left( -2 \times (60 \mu_2^2 + 4 \mu_1^2 (-14 + \mu_1) - 20 \times (1 + \mu_1) + \right. \\
& \quad \left. 3 \mu_2 (11 + 5 \mu_1) + \mu_1 (-76 - 34 \mu_1 + 3 \mu_2 (11 + 9 \mu_1)) \right) + \\
& \, \theta p \left( 72 + 17 \mu_1 + 5 \mu_1^2 + 12 \mu_2^2 (6 + 3 \mu_1 - \mu_2) + 7 \mu_2 - 5 \mu_1 \mu_2 + \right. \\
& \quad \left. 12 \mu_1^2 (6 + \mu_1 + \mu_2) + \mu_2 (288 + 59 \mu_1 + 5 \mu_1^2 + 37 \mu_2 - 5 \mu_1 \mu_2) + \right. \\
& \quad \left. \mu_1 (144 + 29 \mu_1 + 11 \mu_1^2 + 19 \mu_2 - 11 \mu_1 \mu_2 + \right. \\
& \quad \left. \mu_2 (288 + 5 \mu_1^2 - 5 \mu_1 (-7 + \mu_2) + 61 \mu_2) \right) \Big) + \\
& \quad 2 \eta^2 \left( -6 \times (-13 + 16 \mu_2 + 30 \mu_2^2 - 15 \mu_1 + 2 \mu_1^2 (8 + 9 \mu_1) + \right. \\
& \quad \left. \mu_1 (3 - 36 \mu_1 + 2 \mu_2 (85 + 6 \mu_1)) \right) + 5 \, \theta p \\
& \quad \left( 72 + 17 \mu_1 + 5 \mu_1^2 + 12 \mu_2^2 (6 + 3 \mu_1 - \mu_2) + 7 \mu_2 - 5 \mu_1 \mu_2 + \right. \\
& \quad \left. 12 \mu_1^2 (6 + \mu_1 + \mu_2) + \mu_2 (288 + 59 \mu_1 + 5 \mu_1^2 + 37 \mu_2 - 5 \mu_1 \mu_2) + \right. \\
& \quad \left. \mu_1 (144 + 29 \mu_1 + 11 \mu_1^2 + 19 \mu_2 - 11 \mu_1 \mu_2 + \right. \\
& \quad \left. \mu_2 (288 + 5 \mu_1^2 - 5 \mu_1 (-7 + \mu_2) + 61 \mu_2) \right) \Big) + \\
& \eta (214 + 572 \mu_1 + 358 \mu_1^2 - 131 \mu_2 - 659 \mu_1 \mu_2 - 420 \mu_2^2 +
\end{aligned}$$

$$\begin{aligned}
& 210 \, \mathfrak{e}1 + 444 \, \mu1 \, \mathfrak{e}1 - 162 \, \mu1^2 \, \mathfrak{e}1 - 45 \, \mu2 \, \mathfrak{e}1 - 189 \, \mu1 \, \mu2 \, \mathfrak{e}1 + \\
& 8 \, \Theta p \left( 72 + 17 \, \mathfrak{e}1 + 5 \, \mathfrak{e}1^2 + 12 \, \mu2^2 \left( 6 + 3 \, \mathfrak{e}1 - \mathfrak{e}2 \right) + 7 \, \mathfrak{e}2 - 5 \, \mathfrak{e}1 \, \mathfrak{e}2 + \right. \\
& \quad 12 \, \mu1^2 \left( 6 + \mathfrak{e}1 + \mathfrak{e}2 \right) + \mu2 \left( 288 + 59 \, \mathfrak{e}1 + 5 \, \mathfrak{e}1^2 + 37 \, \mathfrak{e}2 - 5 \, \mathfrak{e}1 \, \mathfrak{e}2 \right) + \\
& \quad \mu1 \left( 144 + 29 \, \mathfrak{e}1 + 11 \, \mathfrak{e}1^2 + 19 \, \mathfrak{e}2 - 11 \, \mathfrak{e}1 \, \mathfrak{e}2 + \right. \\
& \quad \quad \left. \mu2 \left( 288 + 5 \, \mathfrak{e}1^2 - 5 \, \mathfrak{e}1 \left( -7 + \mathfrak{e}2 \right) + 61 \, \mathfrak{e}2 \right) \right) \left. \right) \left. \right) \left. \right) - \\
& \times (-1 + \eta) \times \left( 36 \, \eta^7 \, \Theta p \left( 3 + 4 \, \mu2 + \mathfrak{e}1 + \mu1 \left( 3 + \mathfrak{e}1 \right) \right) - 2 \, \eta^6 \, \Theta p \right. \\
& \quad \left( -91 + 2 \, \mu2 + 420 \, \mu2^2 - 27 \, \mathfrak{e}1 - 72 \, \mu1^2 \left( 3 + \mathfrak{e}1 \right) + \right. \\
& \quad \mu1 \left( -307 - 138 \, \mu2 - 99 \, \mathfrak{e}1 + 90 \, \mu2 \, \mathfrak{e}1 \right) + \\
& \quad \left. 18 \, \eta t \left( 3 + 4 \, \mu2 + \mathfrak{e}1 + \mu1 \left( 3 + \mathfrak{e}1 \right) \right) \right) - 3 \, \eta t \, \Theta p \\
& \quad \left( 4 + 4 \, \mu1^2 + 20 \, \mu2^2 + \mu2 \left( 27 + 5 \, \mathfrak{e}1 \right) + \mu1 \left( 8 + \mu2 \left( 27 + 5 \, \mathfrak{e}1 \right) \right) \right) + \eta \\
& \quad \left( -3 \times (-1 + \eta t) \, \Theta l \left( 4 + 4 \, \mu1^2 + 4 \, \mu2^2 + \mu1 \left( 8 - 5 \, \mu2 \left( -1 + \mathfrak{e}1 \right) \right) - \right. \right. \\
& \quad \quad \left. 5 \, \mu2 \left( -1 + \mathfrak{e}1 \right) \right) + \eta t \, \Theta p \left( 60 - 276 \, \mu2^2 + \mu1^2 \left( 144 - 52 \, \mathfrak{e}1 \right) + 80 \, \mathfrak{e}1 + \right. \\
& \quad \quad \left. 68 \, \mu1 \left( 3 + 2 \, \mathfrak{e}1 \right) - \mu2 \left( 179 + 45 \, \mathfrak{e}1 \right) - \mu1 \, \mu2 \left( 203 + 93 \, \mathfrak{e}1 \right) \right) \left. \right) + 2 \, \eta^5 \, \Theta p \\
& \quad \left( 214 + 603 \, \mu2 - 540 \, \mu2^2 + 66 \, \mathfrak{e}1 + 165 \, \mu2 \, \mathfrak{e}1 + 6 \, \mu1^2 \left( 79 + 13 \, \mathfrak{e}1 \right) + \right. \\
& \quad \mu1 \left( 688 + 807 \, \mu2 + 174 \, \mathfrak{e}1 - 159 \, \mu2 \, \mathfrak{e}1 \right) + \\
& \quad \left. \eta t \left( -91 + 2 \, \mu2 + 420 \, \mu2^2 - 27 \, \mathfrak{e}1 + \mu1 \left( -91 - 27 \, \mathfrak{e}1 + 30 \, \mu2 \left( 5 + 3 \, \mathfrak{e}1 \right) \right) \right) \right) \left. \right) - \\
& \eta^2 \left( \Theta p \left( \eta t \left( 588 \, \mu2^2 + \mu2 \left( 107 - 27 \, \mathfrak{e}1 \right) + 10 \, \mu1^2 \left( 7 + 23 \, \mathfrak{e}1 \right) - \right. \right. \right. \\
& \quad \left. 4 \times \left( 44 + 37 \, \mathfrak{e}1 \right) + \mu1 \left( -106 + 1091 \, \mu2 - 314 \, \mathfrak{e}1 + 213 \, \mu2 \, \mathfrak{e}1 \right) \right) \left. \right) + \\
& \quad \left. 6 \times \left( 56 + 120 \, \mu2^2 + 20 \, \mathfrak{e}1 + 5 \, \mu1^2 \left( 15 + \mathfrak{e}1 \right) + 6 \, \mu2 \left( 41 + 5 \, \mathfrak{e}1 \right) + \right. \right. \\
& \quad \quad \left. \mu1 \left( 131 + 31 \, \mathfrak{e}1 + 6 \, \mu2 \left( 41 + \mathfrak{e}1 \right) \right) \right) \left. \right) + \\
& \quad \left( -1 + \eta t \right) \, \Theta l \left( 72 + 276 \, \mu1 + 204 \, \mu1^2 + 62 \, \mu2 + 86 \, \mu1 \, \mu2 - \right. \\
& \quad 24 \, \mu2^2 + 40 \, \mathfrak{e}1 + 68 \, \mu1 \, \mathfrak{e}1 + 28 \, \mu1^2 \, \mathfrak{e}1 - 30 \, \mu2 \, \mathfrak{e}1 - 54 \, \mu1 \, \mu2 \, \mathfrak{e}1 + \\
& \quad 3 \, \Theta p \left( 72 + 17 \, \mathfrak{e}1 + 5 \, \mathfrak{e}1^2 + 12 \, \mu2^2 \left( 6 + 3 \, \mathfrak{e}1 - \mathfrak{e}2 \right) + 7 \, \mathfrak{e}2 - 5 \, \mathfrak{e}1 \, \mathfrak{e}2 + \right. \\
& \quad \quad 12 \, \mu1^2 \left( 6 + \mathfrak{e}1 + \mathfrak{e}2 \right) + \mu2 \left( 288 + 59 \, \mathfrak{e}1 + 5 \, \mathfrak{e}1^2 + 37 \, \mathfrak{e}2 - 5 \, \mathfrak{e}1 \, \mathfrak{e}2 \right) + \\
& \quad \quad \mu1 \left( 144 + 29 \, \mathfrak{e}1 + 11 \, \mathfrak{e}1^2 + 19 \, \mathfrak{e}2 - 11 \, \mathfrak{e}1 \, \mathfrak{e}2 + \right. \\
& \quad \quad \quad \left. \mu2 \left( 288 + 5 \, \mathfrak{e}1^2 - 5 \, \mathfrak{e}1 \left( -7 + \mathfrak{e}2 \right) + 61 \, \mathfrak{e}2 \right) \right) \left. \right) \left. \right) \left. \right) + \\
& \eta^4 \left( 2 \, \Theta p \left( 86 + 901 \, \mu2 + 1188 \, \mu2^2 + \mu1^2 \left( 18 - 58 \, \mathfrak{e}1 \right) + 38 \, \mathfrak{e}1 + \right. \right. \\
& \quad 103 \, \mu2 \, \mathfrak{e}1 + \mu1 \left( 104 + 761 \, \mu2 - 2 \, \mathfrak{e}1 + 103 \, \mu2 \, \mathfrak{e}1 \right) + \\
& \quad \left. \eta t \left( -19 + 182 \, \mu2 + 296 \, \mu2^2 - 51 \, \mathfrak{e}1 - 8 \, \mu2 \, \mathfrak{e}1 + 2 \, \mu1^2 \left( 87 + 55 \, \mathfrak{e}1 \right) + \right. \right. \\
& \quad \quad \left. \mu1 \left( 155 + 982 \, \mu2 - 127 \, \mathfrak{e}1 + 118 \, \mu2 \, \mathfrak{e}1 \right) \right) \left. \right) - \\
& \quad \left( -1 + \eta t \right) \, \Theta l \left( -2 \times \left( 8 \, \mu2 + 24 \, \mu2^2 - 15 \times \left( 1 + \mathfrak{e}1 \right) + \mu1^2 \right. \right. \\
& \quad \quad \left. \left( 3 + 9 \, \mathfrak{e}1 \right) + 4 \, \mu1 \left( -3 - 9 \, \mathfrak{e}1 + \mu2 \left( 49 + 3 \, \mathfrak{e}1 \right) \right) \right) \left. \right) + 5 \, \Theta p \\
& \quad \left( 72 + 17 \, \mathfrak{e}1 + 5 \, \mathfrak{e}1^2 + 12 \, \mu2^2 \left( 6 + 3 \, \mathfrak{e}1 - \mathfrak{e}2 \right) + 7 \, \mathfrak{e}2 - 5 \, \mathfrak{e}1 \, \mathfrak{e}2 + \right. \\
& \quad \quad 12 \, \mu1^2 \left( 6 + \mathfrak{e}1 + \mathfrak{e}2 \right) + \mu2 \left( 288 + 59 \, \mathfrak{e}1 + 5 \, \mathfrak{e}1^2 + 37 \, \mathfrak{e}2 - 5 \, \mathfrak{e}1 \, \mathfrak{e}2 \right) + \\
& \quad \quad \mu1 \left( 144 + 29 \, \mathfrak{e}1 + 11 \, \mathfrak{e}1^2 + 19 \, \mathfrak{e}2 - 11 \, \mathfrak{e}1 \, \mathfrak{e}2 + \right. \\
& \quad \quad \quad \left. \mu2 \left( 288 + 5 \, \mathfrak{e}1^2 - 5 \, \mathfrak{e}1 \left( -7 + \mathfrak{e}2 \right) + 61 \, \mathfrak{e}2 \right) \right) \left. \right) \left. \right) \left. \right) - \eta^3 \\
& \left( \Theta p \left( 2 \times \left( 277 + 836 \, \mu2 - 132 \, \mu2^2 + 89 \, \mathfrak{e}1 + 178 \, \mu2 \, \mathfrak{e}1 + 7 \, \mu1^2 \right. \right. \right. \\
& \quad \left. \left( 69 + 11 \, \mathfrak{e}1 \right) + \mu1 \left( 760 + 968 \, \mu2 + 196 \, \mathfrak{e}1 - 164 \, \mu2 \, \mathfrak{e}1 \right) \right) \left. \right) + \\
& \quad \left. \eta t \left( -104 - 143 \, \mu2 + 508 \, \mu2^2 + \mu1^2 \left( 410 - 62 \, \mathfrak{e}1 \right) + 36 \, \mathfrak{e}1 - \right. \right. \\
& \quad \quad \left. 49 \, \mu2 \, \mathfrak{e}1 + \mu1 \left( 306 + 889 \, \mu2 + 106 \, \mathfrak{e}1 + 95 \, \mu2 \, \mathfrak{e}1 \right) \right) \left. \right) + \\
& \quad \left( -1 + \eta t \right) \, \Theta l \left( 90 + 308 \, \mu1 + 218 \, \mu1^2 + 31 \, \mu2 - 209 \, \mu1 \, \mu2 - \right. \\
& \quad 84 \, \mu2^2 + 70 \, \mathfrak{e}1 + 148 \, \mu1 \, \mathfrak{e}1 - 6 \, \mu1^2 \, \mathfrak{e}1 - 15 \, \mu2 \, \mathfrak{e}1 - 63 \, \mu1 \, \mu2 \, \mathfrak{e}1 + \\
& \quad \left. 8 \, \Theta p \left( 72 + 17 \, \mathfrak{e}1 + 5 \, \mathfrak{e}1^2 + 12 \, \mu2^2 \left( 6 + 3 \, \mathfrak{e}1 - \mathfrak{e}2 \right) + 7 \, \mathfrak{e}2 - 5 \, \mathfrak{e}1 \, \mathfrak{e}2 + \right. \right.
\end{aligned}$$

$$\begin{aligned}
& 12 \mu_1^2 (6 + \mathfrak{e}_1 + \mathfrak{e}_2) + \mu_2 (288 + 59 \mathfrak{e}_1 + 5 \mathfrak{e}_1^2 + 37 \mathfrak{e}_2 - 5 \mathfrak{e}_1 \mathfrak{e}_2) + \\
& \mu_1 (144 + 29 \mathfrak{e}_1 + 11 \mathfrak{e}_1^2 + 19 \mathfrak{e}_2 - 11 \mathfrak{e}_1 \mathfrak{e}_2 + \\
& \mu_2 (288 + 5 \mathfrak{e}_1^2 - 5 \mathfrak{e}_1 (-7 + \mathfrak{e}_2) + 61 \mathfrak{e}_2)) \Big) \Big) + \\
& x^2 (-1 + \eta)^2 (8 \eta t \mathfrak{e} p + 28 \eta t \mathfrak{e} p \mu_1 + 20 \eta t \mathfrak{e} p \mu_1^2 - 33 \mathfrak{e} l \mu_2 + 33 \eta t \\
& \mathfrak{e} l \mu_2 - 194 \eta t \mathfrak{e} p \mu_2 - 33 \mathfrak{e} l \mu_1 \mu_2 + 33 \eta t \mathfrak{e} l \mu_1 \mu_2 - 218 \\
& \eta t \mathfrak{e} p \mu_1 \mu_2 - 24 \mathfrak{e} l \mu_2^2 + 24 \eta t \mathfrak{e} l \mu_2^2 - 216 \eta t \mathfrak{e} p \\
& \mu_2^2 + 40 \eta t \mathfrak{e} p \mathfrak{e}_1 + 68 \eta t \mathfrak{e} p \mu_1 \mathfrak{e}_1 - 44 \eta t \mathfrak{e} p \mu_1^2 \mathfrak{e}_1 - 15 \\
& \mathfrak{e} l \mu_2 \mathfrak{e}_1 + 15 \eta t \mathfrak{e} l \mu_2 \mathfrak{e}_1 - 30 \eta t \mathfrak{e} p \mu_2 \mathfrak{e}_1 - 15 \mathfrak{e} l \mu_1 \\
& \mu_2 \mathfrak{e}_1 + 15 \eta t \mathfrak{e} l \mu_1 \mu_2 \mathfrak{e}_1 - 54 \eta t \mathfrak{e} p \mu_1 \mu_2 \mathfrak{e}_1 + 90 \eta^6 \mathfrak{e} p \\
& (3 + 4 \mu_2 + \mathfrak{e}_1 + \mu_1 (3 + \mathfrak{e}_1)) - 10 \eta^5 \mathfrak{e} p (-31 + 8 \mu_2 + 168 \mu_2^2 - \\
& 9 \mathfrak{e}_1 - 36 \mu_1^2 (3 + \mathfrak{e}_1) + \mu_1 (-139 - 84 \mu_2 - 45 \mathfrak{e}_1 + 36 \mu_2 \mathfrak{e}_1) + \\
& 9 \eta t (3 + 4 \mu_2 + \mathfrak{e}_1 + \mu_1 (3 + \mathfrak{e}_1)) + 2 \eta^4 \mathfrak{e} p \\
& (2 \times (183 + 611 \mu_2 - 300 \mu_2^2 + 57 \mathfrak{e}_1 + 165 \mu_2 \mathfrak{e}_1 + 60 \mu_1^2 (7 + \mathfrak{e}_1) + \\
& \mu_1 (603 + 795 \mu_2 + 147 \mathfrak{e}_1 - 123 \mu_2 \mathfrak{e}_1)) + 5 \eta t \\
& (-31 + 8 \mu_2 + 168 \mu_2^2 - 9 \mathfrak{e}_1 + \mu_1 (-31 + 60 \mu_2 - 9 \mathfrak{e}_1 + 36 \mu_2 \mathfrak{e}_1)) \Big) - \\
& \eta (\mathfrak{e} p (6 \times (56 + 120 \mu_2^2 + 20 \mathfrak{e}_1 + 5 \mu_1^2 (15 + \mathfrak{e}_1) + 6 \mu_2 (41 + 5 \mathfrak{e}_1) + \\
& \mu_1 (131 + 31 \mathfrak{e}_1 + 6 \mu_2 (41 + \mathfrak{e}_1)) \Big) + \\
& \eta t (792 \mu_2^2 - 188 \times (1 + \mathfrak{e}_1) + 3 \mu_2 (95 + \mathfrak{e}_1) + 2 \mu_1^2 \\
& (53 + 155 \mathfrak{e}_1) + \mu_1 (-82 - 382 \mathfrak{e}_1 + 3 \mu_2 (391 + 89 \mathfrak{e}_1)) \Big) \Big) + \\
& (-1 + \eta t) \mathfrak{e} l (4 \times (28 - \mu_2 - 36 \mu_2^2 + 20 \mathfrak{e}_1 - 15 \mu_2 \mathfrak{e}_1 + \\
& \mu_1^2 (79 + 5 \mathfrak{e}_1) + \mu_1 (107 + \mu_2 (5 - 27 \mathfrak{e}_1) + 34 \mathfrak{e}_1)) + \\
& 3 \mathfrak{e} p (72 + 17 \mathfrak{e}_1 + 5 \mathfrak{e}_1^2 + 12 \mu_2^2 (6 + 3 \mathfrak{e}_1 - \mathfrak{e}_2) + 7 \mathfrak{e}_2 - 5 \mathfrak{e}_1 \mathfrak{e}_2 + \\
& 12 \mu_1^2 (6 + \mathfrak{e}_1 + \mathfrak{e}_2) + \mu_2 (288 + 59 \mathfrak{e}_1 + 5 \mathfrak{e}_1^2 + 37 \mathfrak{e}_2 - 5 \mathfrak{e}_1 \mathfrak{e}_2) + \\
& \mu_1 (144 + 29 \mathfrak{e}_1 + 11 \mathfrak{e}_1^2 + 19 \mathfrak{e}_2 - 11 \mathfrak{e}_1 \mathfrak{e}_2 + \\
& \mu_2 (288 + 5 \mathfrak{e}_1^2 - 5 \mathfrak{e}_1 (-7 + \mathfrak{e}_2) + 61 \mathfrak{e}_2)) \Big) \Big) - 2 \\
& \eta^3 (-\mathfrak{e} p (-5 + 1002 \mu_2 + 2004 \mu_2^2 + 15 \mathfrak{e}_1 + 72 \mu_2 \mathfrak{e}_1 - 6 \mu_1^2 \\
& (53 + 27 \mathfrak{e}_1) + \mu_1 (-323 - 135 \mathfrak{e}_1 + 6 \mu_2 (97 + 39 \mathfrak{e}_1)) + \\
& 2 \eta t (25 + 166 \mu_2 + 126 \mu_2^2 - 27 \mathfrak{e}_1 - 6 \mu_2 \mathfrak{e}_1 + 6 \mu_1^2 (25 + 16 \mathfrak{e}_1) + \\
& \mu_1 (175 - 84 \mathfrak{e}_1 + 66 \mu_2 (10 + \mathfrak{e}_1)) \Big) + (-1 + \eta t) \\
& \mathfrak{e} l (-2 \times (-28 + 24 \mu_2 + 54 \mu_2^2 - 30 \mathfrak{e}_1 + \mu_1^2 (19 + 27 \mathfrak{e}_1) + \\
& 3 \mu_1 (-3 + 122 \mu_2 - 24 \mathfrak{e}_1 + 8 \mu_2 \mathfrak{e}_1)) + 5 \mathfrak{e} p \\
& (72 + 17 \mathfrak{e}_1 + 5 \mathfrak{e}_1^2 + 12 \mu_2^2 (6 + 3 \mathfrak{e}_1 - \mathfrak{e}_2) + 7 \mathfrak{e}_2 - 5 \mathfrak{e}_1 \mathfrak{e}_2 + \\
& 12 \mu_1^2 (6 + \mathfrak{e}_1 + \mathfrak{e}_2) + \mu_2 (288 + 59 \mathfrak{e}_1 + 5 \mathfrak{e}_1^2 + 37 \mathfrak{e}_2 - 5 \mathfrak{e}_1 \mathfrak{e}_2) + \\
& \mu_1 (144 + 29 \mathfrak{e}_1 + 11 \mathfrak{e}_1^2 + 19 \mathfrak{e}_2 - 11 \mathfrak{e}_1 \mathfrak{e}_2 + \\
& \mu_2 (288 + 5 \mathfrak{e}_1^2 - 5 \mathfrak{e}_1 (-7 + \mathfrak{e}_2) + 61 \mathfrak{e}_2)) \Big) \Big) - \\
& \eta^2 (\mathfrak{e} p (6 \times (161 + 542 \mu_2 + 68 \mu_2^2 + 53 \mathfrak{e}_1 + 104 \mu_2 \mathfrak{e}_1 + \mu_1^2 \\
& (279 + 41 \mathfrak{e}_1) + \mu_1 (440 + 618 \mu_2 + 112 \mathfrak{e}_1 - 70 \mu_2 \mathfrak{e}_1)) + \\
& \eta t (-284 - 95 \mu_2 + 1176 \mu_2^2 - 60 \mathfrak{e}_1 - 57 \mu_2 \mathfrak{e}_1 + \mu_1^2 \\
& (514 + 30 \mathfrak{e}_1) + \mu_1 (230 + 1849 \mu_2 - 66 \mathfrak{e}_1 + 303 \mu_2 \mathfrak{e}_1)) \Big) + \\
& (-1 + \eta t) \mathfrak{e} l (242 + 748 \mu_1 + 506 \mu_1^2 - 19 \mu_2 - 643 \mu_1 \mu_2 - \\
& 336 \mu_2^2 + 210 \mathfrak{e}_1 + 444 \mu_1 \mathfrak{e}_1 - 90 \mu_1^2 \mathfrak{e}_1 - 45 \mu_2 \mathfrak{e}_1 - 189 \mu_1 \mu_2 \mathfrak{e}_1 + \\
& 12 \mathfrak{e} p (72 + 17 \mathfrak{e}_1 + 5 \mathfrak{e}_1^2 + 12 \mu_2^2 (6 + 3 \mathfrak{e}_1 - \mathfrak{e}_2) + 7 \mathfrak{e}_2 - 5 \mathfrak{e}_1 \mathfrak{e}_2 + \\
& 12 \mu_1^2 (6 + \mathfrak{e}_1 + \mathfrak{e}_2) + \mu_2 (288 + 59 \mathfrak{e}_1 + 5 \mathfrak{e}_1^2 + 37 \mathfrak{e}_2 - 5 \mathfrak{e}_1 \mathfrak{e}_2) +
\end{aligned}$$

$$\begin{aligned}
& \mu_1 (144 + 29 \mu_1 + 11 \mu_1^2 + 19 \mu_2 - 11 \mu_1 \mu_2 + \\
& \quad \mu_2 (288 + 5 \mu_1^2 - 5 \mu_1 (-7 + \mu_2) + 61 \mu_2)) + \\
w^3 (-1 + \eta)^3 (6 x^7 (-1 + \eta)^8 \theta p (\eta - \eta t + 4 \mu_1) (3 + 4 \mu_2 + \mu_1 + \mu_1 (3 + \mu_1)) - \\
& \quad x^6 (-1 + \eta)^6 (6 \times (-1 + \eta) \theta p (29 + 101 \mu_1 + 72 \mu_1^2 + 87 \mu_2 + \\
& \quad 119 \mu_1 \mu_2 + 5 \mu_1 + 27 \mu_1 \mu_1 + 16 \mu_1^2 \mu_1 + 11 \mu_2 \mu_1 - \\
& \quad 7 \mu_1 \mu_2 \mu_1 + 7 \eta^2 (3 + 4 \mu_2 + \mu_1 + \mu_1 (3 + \mu_1)) + \\
& \quad \eta (17 + 18 \mu_2 - 28 \mu_2^2 + 5 \mu_1 + 28 \mu_1^2 (3 + \mu_1) + \mu_1 (101 - \\
& \quad 6 \mu_2 (-17 + \mu_1) + 33 \mu_1) - 7 \eta t (3 + 4 \mu_2 + \mu_1 + \mu_1 (3 + \mu_1))) + \\
& \quad \eta t (-17 - 18 \mu_2 + 28 \mu_2^2 - 5 \mu_1 + \mu_1 (-17 - 5 \mu_1 + 2 \mu_2 (5 + 3 \mu_1))) - \\
& \quad (-1 + \eta t) \theta l (28 - 52 \mu_1 - 80 \mu_1^2 + 11 \mu_2 - 325 \mu_1 \mu_2 + 8 \mu_2^2 + \\
& \quad 20 \mu_1 + 72 \mu_1 \mu_1 - 32 \mu_1^2 \mu_1 + 5 \mu_2 \mu_1 - 19 \mu_1 \mu_2 \mu_1 + \\
& \quad \theta p (146 + 15 \mu_1 + 5 \mu_1^2 + \mu_2^2 (48 - 88 \mu_2) + \\
& \quad \mu_2 (510 + 5 \mu_1^2 - 5 \mu_1 (-5 + \mu_2) - 3 \mu_2) - 5 \mu_2 - 5 \mu_1 \mu_2 + \mu_1^2 \\
& \quad (148 + 3 \mu_1^2 + 11 \mu_2 + \mu_1 (5 + \mu_2)) + \mu_1 (20 \mu_1^2 - 16 \mu_1 (-2 + \mu_2) + \\
& \quad 6 \times (49 + \mu_2) + \mu_2 (462 + 5 \mu_1^2 + 45 \mu_2 - \mu_1 (39 + 17 \mu_2))) + \\
x^5 (-1 + \eta)^5 ((-1 + \eta) \theta p (126 \eta^3 (3 + 4 \mu_2 + \mu_1 + \mu_1 (3 + \mu_1)) + \\
& \quad 2 \times (235 + 312 \mu_2^2 + 63 \mu_1 + \mu_1^2 (414 + 58 \mu_1) + \\
& \quad \mu_2 (801 + 121 \mu_1) + \mu_1 (649 + \mu_2 (905 - 65 \mu_1) + 163 \mu_1)) + \\
& \quad \eta t (-190 - 103 \mu_2 + 508 \mu_2^2 - 66 \mu_1 - 13 \mu_2 \mu_1 + 4 \mu_1^2 \\
& \quad (36 + 13 \mu_1) + \mu_1 (-46 + 633 \mu_2 - 110 \mu_1 + 167 \mu_2 \mu_1)) - \\
& \quad 18 \eta^2 (7 \eta t (3 + 4 \mu_2 + \mu_1 + \mu_1 (3 + \mu_1)) - 2 \times (17 + 18 \mu_2 - 28 \mu_2^2 + \\
& \quad 5 \mu_1 + 14 \mu_1^2 (3 + \mu_1) + \mu_1 (59 + 46 \mu_2 + 19 \mu_1 - 6 \mu_2 \mu_1))) + \\
& \quad 2 \eta (609 + 1610 \mu_2 - 408 \mu_2^2 + 113 \mu_1 + 198 \mu_2 \mu_1 + 144 \mu_1^2 \\
& \quad (9 + 2 \mu_1) + \mu_1 (1905 + 2022 \mu_2 + 509 \mu_1 - 198 \mu_2 \mu_1) + 18 \eta t \\
& \quad (-17 - 18 \mu_2 + 28 \mu_2^2 - 5 \mu_1 + \mu_1 (-17 + 10 \mu_2 - 5 \mu_1 + 6 \mu_2 \mu_1))) - \\
& \quad (-1 + \eta t) \theta l (-2 \times (-52 + 100 \mu_2^2 + \mu_2 (53 - 5 \mu_1) - 60 \mu_1 + \\
& \quad 20 \mu_1^2 (1 + 4 \mu_1) + \mu_1 (-32 + 261 \mu_2 - 142 \mu_1 + 55 \mu_2 \mu_1)) + \\
& \quad \theta p (366 + 67 \mu_1 + 25 \mu_1^2 + 4 \mu_2^2 (78 + 27 \mu_1 - 43 \mu_2) + 11 \mu_2 - \\
& \quad 25 \mu_1 \mu_2 + \mu_2 (1402 + 209 \mu_1 + 25 \mu_1^2 + 97 \mu_2 - 25 \mu_1 \mu_2) + \\
& \quad \mu_1^2 (408 + 5 \mu_1^2 + 45 \mu_2 + \mu_1 (43 + 3 \mu_2)) + \\
& \quad \mu_1 (774 + 122 \mu_1 + 66 \mu_1^2 + 56 \mu_2 - 58 \mu_1 \mu_2 + \\
& \quad \mu_2 (1450 + 49 \mu_1 + 25 \mu_1^2 + 217 \mu_2 - 37 \mu_1 \mu_2))) + \\
& \quad \eta (136 - 276 \mu_1 - 412 \mu_1^2 + 39 \mu_2 - 1865 \mu_1 \mu_2 + 28 \mu_2^2 + \\
& \quad 100 \mu_1 + 360 \mu_1 \mu_1 - 136 \mu_1^2 \mu_1 + 25 \mu_2 \mu_1 - 95 \mu_1 \mu_2 \mu_1 + \\
& \quad 2 \theta p (446 + 47 \mu_1 + 15 \mu_1^2 + 2 \mu_2^2 (74 + 3 \mu_1 - 129 \mu_2) - 13 \mu_2 - \\
& \quad 15 \mu_1 \mu_2 + \mu_2 (1566 + 83 \mu_1 + 15 \mu_1^2 - \mu_2 - 15 \mu_1 \mu_2) + \\
& \quad \mu_1^2 (452 + 9 \mu_1^2 + 37 \mu_2 + \mu_1 (19 + 3 \mu_2)) + \\
& \quad \mu_1 (898 + 102 \mu_1 + 60 \mu_1^2 + 24 \mu_2 - 48 \mu_1 \mu_2 + \\
& \quad \mu_2 (1422 - 101 \mu_1 + 15 \mu_1^2 + 151 \mu_2 - 51 \mu_1 \mu_2))) - \\
x^3 (-1 + \eta)^3 (-2 \times (-1 + \eta) \theta p (43 + 115 \mu_1 + 72 \mu_1^2 + 209 \mu_2 + \\
& \quad 265 \mu_1 \mu_2 + 120 \mu_2^2 + 23 \mu_1 + 29 \mu_1 \mu_1 + 25 \mu_2 \mu_1 + \\
& \quad 7 \mu_1 \mu_2 \mu_1 + 105 \eta^5 (3 + 4 \mu_2 + \mu_1 + \mu_1 (3 + \mu_1)) - \\
& \quad 15 \eta^4 (7 \eta t (3 + 4 \mu_2 + \mu_1 + \mu_1 (3 + \mu_1)) - 4 \times (17 + 18 \mu_2 - 28 \mu_2^2 +
\end{aligned}$$

$$\begin{aligned}
& 5 \, \mathfrak{e}1 + 7 \, \mu1^2 (3 + \mathfrak{e}1) + \mu1 (38 - 6 \, \mu2 (-3 + \mathfrak{e}1) + 12 \, \mathfrak{e}1) \Big) \Big) + \\
& \eta t \Big( -20 + 348 \, \mu2^2 - 82 \, \mathfrak{e}1 + \mu2 (297 + \mathfrak{e}1) + 8 \, \mu1^2 (5 + 13 \, \mathfrak{e}1) + \\
& \quad \mu1 (20 - 146 \, \mathfrak{e}1 + \mu2 (373 + 115 \, \mathfrak{e}1)) \Big) + \\
& \eta^2 \Big( \eta t \Big( -942 - 483 \, \mu2 + 2564 \, \mu2^2 - 330 \, \mathfrak{e}1 - 65 \, \mu2 \, \mathfrak{e}1 - 22 \, \mu1 \\
& \quad (9 + 25 \, \mathfrak{e}1) + 4 \, \mu1^2 (186 + 53 \, \mathfrak{e}1) + 5 \, \mu1 \, \mu2 (729 + 167 \, \mathfrak{e}1) \Big) + \\
& \quad 2 \times (1289 + 560 \, \mu2^2 + 341 \, \mathfrak{e}1 + 10 \, \mu1^2 (207 + 29 \, \mathfrak{e}1) + 11 \, \mu2 \\
& \quad (371 + 55 \, \mathfrak{e}1) + \mu1 (3359 + \mu2 (4353 - 457 \, \mathfrak{e}1) + 841 \, \mathfrak{e}1)) \Big) + \\
& 10 \, \eta^3 \Big( 261 + 566 \, \mu2 - 408 \, \mu2^2 + 53 \, \mathfrak{e}1 + 66 \, \mu2 \, \mathfrak{e}1 + 48 \, \mu1^2 \\
& \quad (9 + 2 \, \mathfrak{e}1) + \mu1 (693 + 594 \, \mu2 + 185 \, \mathfrak{e}1 - 114 \, \mu2 \, \mathfrak{e}1) + 6 \, \eta t \\
& \quad (-17 - 18 \, \mu2 + 28 \, \mu2^2 - 5 \, \mathfrak{e}1 + \mu1 (-17 + 10 \, \mu2 - 5 \, \mathfrak{e}1 + 6 \, \mu2 \, \mathfrak{e}1)) \Big) + \\
& 2 \, \eta \Big( 388 + 1596 \, \mu2 + 928 \, \mu2^2 + 143 \, \mathfrak{e}1 + 226 \, \mu2 \, \mathfrak{e}1 + \mu1^2 \\
& \quad (612 + 44 \, \mathfrak{e}1) + \mu1 (1000 + 1804 \, \mu2 + 247 \, \mathfrak{e}1 - 32 \, \mu2 \, \mathfrak{e}1) + \\
& \quad \eta t (\mu1^2 (245 + 227 \, \mathfrak{e}1) + 2 \times (-87 + 95 \, \mu2 + 338 \, \mu2^2 - 73 \, \mathfrak{e}1 - \\
& \quad 13 \, \mu2 \, \mathfrak{e}1) + \mu1 (71 + 1136 \, \mu2 - 294 \, \mathfrak{e}1 + 274 \, \mu2 \, \mathfrak{e}1)) \Big) \Big) + \\
& (-1 + \eta t) \, \mathfrak{e}l \Big( -6 \times (-2 + 43 \, \mu2 + 44 \, \mu2^2 + 2 \, \mu1^2 (-7 + \mathfrak{e}1) - 10 \, \mathfrak{e}1 + \\
& \quad 5 \, \mu2 \, \mathfrak{e}1 - 2 \, \mu1 (8 + 7 \, \mathfrak{e}1) + \mu1 \, \mu2 (43 + 17 \, \mathfrak{e}1)) + \\
& \mathfrak{e}p \Big( 74 + 37 \, \mathfrak{e}1 + 15 \, \mathfrak{e}1^2 + 21 \, \mathfrak{e}2 - 15 \, \mathfrak{e}1 \, \mathfrak{e}2 + 4 \, \mu2^2 (54 + 27 \, \mathfrak{e}1 + \mathfrak{e}2) + \\
& \quad \mu2 (382 + 159 \, \mathfrak{e}1 + 15 \, \mathfrak{e}1^2 + 103 \, \mathfrak{e}2 - 15 \, \mathfrak{e}1 \, \mathfrak{e}2) + \\
& \quad \mu1^2 (112 - \mathfrak{e}1^2 + 23 \, \mathfrak{e}2 + \mathfrak{e}1 (33 + \mathfrak{e}2)) + \mu1 (186 + 58 \, \mathfrak{e}1 + 26 \, \mathfrak{e}1^2 + 44 \\
& \quad \mathfrak{e}2 - 26 \, \mathfrak{e}1 \, \mathfrak{e}2 + \mu2 (526 + 127 \, \mathfrak{e}1 + 15 \, \mathfrak{e}1^2 + 127 \, \mathfrak{e}2 - 3 \, \mathfrak{e}1 \, \mathfrak{e}2)) \Big) \Big) + \\
& 2 \, \eta^2 \Big( -6 \times (-56 + 88 \, \mu2^2 + \mu2 (37 - 5 \, \mathfrak{e}1) - 60 \, \mathfrak{e}1 + \mu1^2 \\
& \quad (-27 + 47 \, \mathfrak{e}1) + \mu1 (-83 - 142 \, \mathfrak{e}1 + \mu2 (343 + 55 \, \mathfrak{e}1)) \Big) + \mathfrak{e}p \\
& \quad (1894 + 351 \, \mathfrak{e}1 + 125 \, \mathfrak{e}1^2 + 4 \, \mu2^2 (398 + 147 \, \mathfrak{e}1 - 203 \, \mathfrak{e}2) + 71 \, \mathfrak{e}2 - \\
& \quad 125 \, \mathfrak{e}1 \, \mathfrak{e}2 + \mu2 (7298 + 1109 \, \mathfrak{e}1 + 125 \, \mathfrak{e}1^2 + 549 \, \mathfrak{e}2 - 125 \, \mathfrak{e}1 \, \mathfrak{e}2) + \\
& \quad \mu1^2 (2104 + 25 \, \mathfrak{e}1^2 + 257 \, \mathfrak{e}2 + \mathfrak{e}1 (247 + 15 \, \mathfrak{e}2)) + \\
& \quad \mu1 (3998 + 658 \, \mathfrak{e}1 + 330 \, \mathfrak{e}1^2 + 328 \, \mathfrak{e}2 - 290 \, \mathfrak{e}1 \, \mathfrak{e}2 + \\
& \quad \mu2 (7538 + 373 \, \mathfrak{e}1 + 125 \, \mathfrak{e}1^2 + 1213 \, \mathfrak{e}2 - 185 \, \mathfrak{e}1 \, \mathfrak{e}2)) \Big) \Big) + \\
& 2 \, \eta \Big( 160 + 614 \, \mu1 + 454 \, \mu1^2 - 401 \, \mu2 - 353 \, \mu1 \, \mu2 - 588 \, \mu2^2 + \\
& \quad 240 \, \mathfrak{e}1 + 444 \, \mu1 \, \mathfrak{e}1 - 66 \, \mu1^2 \, \mathfrak{e}1 - 15 \, \mu2 \, \mathfrak{e}1 - 267 \, \mu1 \, \mu2 \, \mathfrak{e}1 + \\
& 2 \, \mathfrak{e}p \Big( 298 + 90 \, \mathfrak{e}1 + 35 \, \mathfrak{e}1^2 + \mu2^2 (482 + 219 \, \mathfrak{e}1 - 77 \, \mathfrak{e}2) + 38 \, \mathfrak{e}2 - \\
& \quad 35 \, \mathfrak{e}1 \, \mathfrak{e}2 + \mu2 (1292 + 347 \, \mathfrak{e}1 + 35 \, \mathfrak{e}1^2 + 207 \, \mathfrak{e}2 - 35 \, \mathfrak{e}1 \, \mathfrak{e}2) + \\
& \quad \mu1^2 (376 + \mathfrak{e}1^2 + 59 \, \mathfrak{e}2 + \mathfrak{e}1 (73 + 3 \, \mathfrak{e}2)) + \\
& \quad \mu1 (674 + 151 \, \mathfrak{e}1 + 72 \, \mathfrak{e}1^2 + 97 \, \mathfrak{e}2 - 68 \, \mathfrak{e}1 \, \mathfrak{e}2 + \\
& \quad \mu2 (1532 + 223 \, \mathfrak{e}1 + 35 \, \mathfrak{e}1^2 + 307 \, \mathfrak{e}2 - 23 \, \mathfrak{e}1 \, \mathfrak{e}2)) \Big) \Big) + \\
& 2 \, \eta^3 \Big( 128 - 308 \, \mu1 - 436 \, \mu1^2 + 7 \, \mu2 - 2345 \, \mu1 \, \mu2 + 4 \, \mu2^2 + \\
& \quad 100 \, \mathfrak{e}1 + 360 \, \mu1 \, \mathfrak{e}1 - 88 \, \mu1^2 \, \mathfrak{e}1 + 25 \, \mu2 \, \mathfrak{e}1 - 95 \, \mu1 \, \mu2 \, \mathfrak{e}1 + \\
& 10 \, \mathfrak{e}p \Big( 154 + 17 \, \mathfrak{e}1 + 5 \, \mathfrak{e}1^2 + \mu2^2 (52 + 6 \, \mathfrak{e}1 - 82 \, \mathfrak{e}2) - 3 \, \mathfrak{e}2 - \\
& \quad 5 \, \mathfrak{e}1 \, \mathfrak{e}2 + \mu2 (546 + 33 \, \mathfrak{e}1 + 5 \, \mathfrak{e}1^2 + 5 \, \mathfrak{e}2 - 5 \, \mathfrak{e}1 \, \mathfrak{e}2) + \\
& \quad \mu1^2 (3 \, \mathfrak{e}1^2 + \mathfrak{e}1 (9 + \mathfrak{e}2) + 3 \times (52 + 5 \, \mathfrak{e}2)) + \\
& \quad \mu1 (\mu2 (498 - 23 \, \mathfrak{e}1 + 5 \, \mathfrak{e}1^2 + 61 \, \mathfrak{e}2 - 17 \, \mathfrak{e}1 \, \mathfrak{e}2) + \\
& \quad 2 \times (155 + 19 \, \mathfrak{e}1 + 10 \, \mathfrak{e}1^2 + 6 \, \mathfrak{e}2 - 8 \, \mathfrak{e}1 \, \mathfrak{e}2)) \Big) \Big) \Big) + \\
& \times (-1 + \eta) \times \Big( 42 \, \eta^8 \, \mathfrak{e}p (3 + 4 \, \mu2 + \mathfrak{e}1 + \mu1 (3 + \mathfrak{e}1)) - 6 \, \eta^7 \, \mathfrak{e}p \\
& \quad (-81 - 80 \, \mu2 + 168 \, \mu2^2 - 23 \, \mathfrak{e}1 - 28 \, \mu1^2 (3 + \mathfrak{e}1) +
\end{aligned}$$



$$\begin{aligned}
& \mu_1 (-165 - 52 \mu_2 - 51 \mathfrak{e}_1 + 36 \mu_2 \mathfrak{e}_1) + \\
& 7 \eta t (3 + 4 \mu_2 + \mathfrak{e}_1 + \mu_1 (3 + \mathfrak{e}_1)) - 3 \eta t \theta p \\
& (4 + 4 \mu_1^2 + 20 \mu_2^2 + \mu_2 (27 + 5 \mathfrak{e}_1) + \mu_1 (8 + \mu_2 (27 + 5 \mathfrak{e}_1))) - 3 \\
& \eta ((-1 + \eta t) \theta l (4 + 4 \mu_1^2 + 4 \mu_2^2 + \mu_1 (8 - 5 \mu_2 (-1 + \mathfrak{e}_1)) - \\
& 5 \mu_2 (-1 + \mathfrak{e}_1)) + \eta t \theta p (4 + 204 \mu_2^2 - 40 \mathfrak{e}_1 + 4 \mu_1^2 (-6 + 5 \mathfrak{e}_1) + \\
& 7 \mu_1 \mu_2 (31 + 9 \mathfrak{e}_1) - 4 \mu_1 (5 + 14 \mathfrak{e}_1) + \mu_2 (209 + 15 \mathfrak{e}_1))) + 2 \\
& \eta^6 \theta p (651 + 1462 \mu_2 - 1536 \mu_2^2 + 115 \mathfrak{e}_1 + 198 \mu_2 \mathfrak{e}_1 + 12 \mu_1^2 \\
& (87 + 17 \mathfrak{e}_1) + \mu_1 (1695 + 1386 \mu_2 + 427 \mathfrak{e}_1 - 378 \mu_2 \mathfrak{e}_1) + 3 \eta t \\
& (-81 - 80 \mu_2 + 168 \mu_2^2 - 23 \mathfrak{e}_1 + \mu_1 (-81 + 60 \mu_2 - 23 \mathfrak{e}_1 + 36 \mu_2 \mathfrak{e}_1))) - \\
& \eta^4 (\theta p (2 \times (603 + 893 \mu_2 - 2040 \mu_2^2 + 77 \mathfrak{e}_1 + 153 \mu_2 \mathfrak{e}_1 + \\
& \mu_1^2 (846 + 202 \mathfrak{e}_1) + \mu_1 (1449 + 565 \mu_2 + 369 \mathfrak{e}_1 - 501 \mu_2 \mathfrak{e}_1)) - \\
& \eta t (206 + 1083 \mu_2 + 20 \mu_2^2 - 254 \mathfrak{e}_1 - 39 \mu_2 \mathfrak{e}_1 + 4 \mu_1^2 \\
& (-41 + 120 \mathfrak{e}_1) + \mu_1 (42 + 1075 \mu_2 - 626 \mathfrak{e}_1 + 261 \mu_2 \mathfrak{e}_1))) + \\
& (-1 + \eta t) \theta l (-2 \times (76 \mu_2^2 + \mu_2 (21 - 5 \mathfrak{e}_1) - 60 \times (1 + \mathfrak{e}_1) + \\
& 2 \mu_1^2 (-37 + 7 \mathfrak{e}_1) + 5 \mu_1 \mu_2 (85 + 11 \mathfrak{e}_1) - 2 \mu_1 (67 + 71 \mathfrak{e}_1)) + \\
& \theta p (1958 + 367 \mathfrak{e}_1 + 125 \mathfrak{e}_1^2 + 4 \mu_2^2 (406 + 159 \mathfrak{e}_1 - 191 \mathfrak{e}_2) + 87 \mathfrak{e}_2 - \\
& 125 \mathfrak{e}_1 \mathfrak{e}_2 + \mu_2 (7586 + 1173 \mathfrak{e}_1 + 125 \mathfrak{e}_1^2 + 613 \mathfrak{e}_2 - 125 \mathfrak{e}_1 \mathfrak{e}_2) + \\
& \mu_1^2 (2168 + 25 \mathfrak{e}_1^2 + 289 \mathfrak{e}_2 + 3 \mathfrak{e}_1 (93 + 5 \mathfrak{e}_2)) + \\
& \mu_1 (4126 + 706 \mathfrak{e}_1 + 330 \mathfrak{e}_1^2 + 376 \mathfrak{e}_2 - 290 \mathfrak{e}_1 \mathfrak{e}_2 + \\
& \mu_2 (7826 + 501 \mathfrak{e}_1 + 125 \mathfrak{e}_1^2 + 1341 \mathfrak{e}_2 - 185 \mathfrak{e}_1 \mathfrak{e}_2)))) + \\
& \eta^5 (\theta p (892 + 4742 \mu_2 + 3200 \mu_2^2 + 324 \mathfrak{e}_1 + 814 \mu_2 \mathfrak{e}_1 + 4 \mu_1^2 \\
& (387 + \mathfrak{e}_1) + \mu_1 (2440 + 5278 \mu_2 + 532 \mathfrak{e}_1 - 206 \mu_2 \mathfrak{e}_1) + \\
& \eta t (-322 + 197 \mu_2 + 1580 \mu_2^2 - 150 \mathfrak{e}_1 - 65 \mu_2 \mathfrak{e}_1 + \\
& 4 \mu_1^2 (192 + 41 \mathfrak{e}_1) + \mu_1 (446 + 3765 \mu_2 - 370 \mathfrak{e}_1 + 619 \mu_2 \mathfrak{e}_1))) - \\
& (-1 + \eta t) \theta l (24 - 68 \mu_1 - 92 \mu_1^2 - 5 \mu_2 - 565 \mu_1 \mu_2 - 4 \mu_2^2 + \\
& 20 \mathfrak{e}_1 + 72 \mu_1 \mathfrak{e}_1 - 8 \mu_1^2 \mathfrak{e}_1 + 5 \mu_2 \mathfrak{e}_1 - 19 \mu_1 \mu_2 \mathfrak{e}_1 + \\
& 2 \theta p (478 + 55 \mathfrak{e}_1 + 15 \mathfrak{e}_1^2 + 2 \mu_2^2 (82 + 15 \mathfrak{e}_1 - 117 \mathfrak{e}_2) - 5 \mathfrak{e}_2 - \\
& 15 \mathfrak{e}_1 \mathfrak{e}_2 + \mu_2 (1710 + 115 \mathfrak{e}_1 + 15 \mathfrak{e}_1^2 + 31 \mathfrak{e}_2 - 15 \mathfrak{e}_1 \mathfrak{e}_2) + \\
& \mu_1^2 (484 + 9 \mathfrak{e}_1^2 + 53 \mathfrak{e}_2 + \mathfrak{e}_1 (35 + 3 \mathfrak{e}_2)) + \\
& \mu_1 (962 + 126 \mathfrak{e}_1 + 60 \mathfrak{e}_1^2 + 48 \mathfrak{e}_2 - 48 \mathfrak{e}_1 \mathfrak{e}_2 + \\
& \mu_2 (1566 - 37 \mathfrak{e}_1 + 15 \mathfrak{e}_1^2 + 215 \mathfrak{e}_2 - 51 \mathfrak{e}_1 \mathfrak{e}_2)))) - 2 \\
& \eta^3 (\theta p (671 + 2637 \mu_2 + 1240 \mu_2^2 + 221 \mathfrak{e}_1 + 377 \mu_2 \mathfrak{e}_1 + 8 \mu_1^2 \\
& (126 + 11 \mathfrak{e}_1) + \mu_1 (1679 + 2821 \mu_2 + 411 \mathfrak{e}_1 - 109 \mu_2 \mathfrak{e}_1) + \\
& \eta t (-248 - 351 \mu_2 + 428 \mu_2^2 - 46 \mathfrak{e}_1 - 55 \mu_2 \mathfrak{e}_1 + \\
& 2 \mu_1^2 (239 + 77 \mathfrak{e}_1) + \mu_1 (230 + 1657 \mu_2 - 150 \mathfrak{e}_1 + 203 \mu_2 \mathfrak{e}_1))) + \\
& (-1 + \eta t) \theta l (72 + 322 \mu_1 + 250 \mu_1^2 - 59 \mu_2 - 59 \mu_1 \mu_2 - \\
& 140 \mu_2^2 + 80 \mathfrak{e}_1 + 148 \mu_1 \mathfrak{e}_1 + 26 \mu_1^2 \mathfrak{e}_1 - 5 \mu_2 \mathfrak{e}_1 - 89 \mu_1 \mu_2 \mathfrak{e}_1 + \\
& 2 \theta p (306 + 92 \mathfrak{e}_1 + 35 \mathfrak{e}_1^2 + \mu_2^2 (486 + 225 \mathfrak{e}_1 - 71 \mathfrak{e}_2) + 40 \mathfrak{e}_2 - \\
& 35 \mathfrak{e}_1 \mathfrak{e}_2 + \mu_2 (1328 + 355 \mathfrak{e}_1 + 35 \mathfrak{e}_1^2 + 215 \mathfrak{e}_2 - 35 \mathfrak{e}_1 \mathfrak{e}_2) + \\
& \mu_1^2 (384 + \mathfrak{e}_1^2 + 63 \mathfrak{e}_2 + \mathfrak{e}_1 (77 + 3 \mathfrak{e}_2)) + \\
& \mu_1 (690 + 157 \mathfrak{e}_1 + 72 \mathfrak{e}_1^2 + 103 \mathfrak{e}_2 - 68 \mathfrak{e}_1 \mathfrak{e}_2 + \\
& \mu_2 (1568 + 239 \mathfrak{e}_1 + 35 \mathfrak{e}_1^2 + 323 \mathfrak{e}_2 - 23 \mathfrak{e}_1 \mathfrak{e}_2)))) + \eta^2 \\
& (-2 \theta p (3 \times (43 + 72 \mu_1^2 + 209 \mu_2 + 120 \mu_2^2 + 23 \mathfrak{e}_1 + 25 \mu_2 \mathfrak{e}_1 +
\end{aligned}$$

$$\begin{aligned}
& \mu_1 (115 + 265 \mu_2 + 29 \mu_1 + 7 \mu_2 \mu_1) + \\
& \eta t (-128 + 313 \mu_2 + 540 \mu_2^2 - 186 \mu_1 - 27 \mu_2 \mu_1 + 2 \mu_1^2 \\
& \quad (-73 + 69 \mu_1) + \mu_1 (-274 + 577 \mu_2 - 354 \mu_1 + 243 \mu_2 \mu_1)) + \\
& 3 \times (-1 + \eta t) \theta l (40 \mu_2^2 - 20 \times (1 + \mu_1) - 28 \mu_1 (3 + \mu_1) - \\
& \quad 8 \mu_1^2 (8 + \mu_1) + 2 \mu_2 (11 + 5 \mu_1) + 2 \mu_1 \mu_2 (7 + 17 \mu_1) + \\
& \quad \theta p (-74 - 37 \mu_1 - 15 \mu_1^2 - 21 \mu_2 + 15 \mu_1 \mu_2 - 4 \mu_2^2 (54 + 27 \mu_1 + \mu_2) - \\
& \quad \mu_2 (382 + 159 \mu_1 + 15 \mu_1^2 + 103 \mu_2 - 15 \mu_1 \mu_2) + \mu_1^2 (-112 + \mu_1^2 - \\
& \quad 23 \mu_2 - \mu_1 (33 + \mu_2)) - \mu_1 (186 + 58 \mu_1 + 26 \mu_1^2 + 44 \mu_2 - 26 \\
& \quad \mu_1 \mu_2 + \mu_2 (526 + 127 \mu_1 + 15 \mu_1^2 + 127 \mu_2 - 3 \mu_1 \mu_2))) - \\
& x^2 (-1 + \eta)^2 (126 \eta^7 \theta p (3 + 4 \mu_2 + \mu_1 + \mu_1 (3 + \mu_1)) - 18 \eta^6 \theta p \\
& \quad (7 \eta t (3 + 4 \mu_2 + \mu_1 + \mu_1 (3 + \mu_1)) - 2 \times (32 + 31 \mu_2 - 70 \mu_2^2 + 9 \mu_1 + \\
& \quad 14 \mu_1^2 (3 + \mu_1) + \mu_1 (74 + 31 \mu_2 + 23 \mu_1 - 15 \mu_2 \mu_1))) + 2 \eta^5 \theta p \\
& \quad (36 \mu_1^2 (69 + 13 \mu_1) + \mu_1 (3894 + 3597 \mu_2 + 968 \mu_1 - 765 \mu_2 \mu_1) + \\
& \quad 5 \times (282 + 709 \mu_2 - 564 \mu_2^2 + 46 \mu_1 + 99 \mu_2 \mu_1) + \\
& \quad 18 \eta t (-32 - 31 \mu_2 + 70 \mu_2^2 - 9 \mu_1 + \mu_1 (-32 - 9 \mu_1 + 5 \mu_2 (5 + 3 \mu_1))) - \\
& 3 (\theta l \mu_2 (11 + 8 \mu_2 + 5 \mu_1 + \mu_1 (11 + 5 \mu_1)) + \eta t (-\theta l \mu_2 (11 + 8 \mu_2 + \\
& \quad 5 \mu_1 + \mu_1 (11 + 5 \mu_1)) + 2 \theta p (6 + 68 \mu_2^2 - 10 \mu_1 + 5 \mu_2 (15 + \mu_1) + \\
& \quad \mu_1^2 (4 + 8 \mu_1) + \mu_1 (10 - 14 \mu_1 + \mu_2 (79 + 17 \mu_1)))) - 2 \\
& \eta^3 (\theta p (1510 + 3396 \mu_2 - 2472 \mu_2^2 + 276 \mu_1 + 532 \mu_2 \mu_1 + \\
& \quad 64 \mu_1^2 (36 + 7 \mu_1) + \mu_1 (3814 + 3116 \mu_2 + 964 \mu_1 - 932 \mu_2 \mu_1) + \\
& \quad \eta t (-404 - 989 \mu_2 + 584 \mu_2^2 + \mu_1^2 (162 - 394 \mu_1) + 108 \mu_1 + \\
& \quad 13 \mu_2 \mu_1 + \mu_1 (-242 + 231 \mu_2 + 332 \mu_1 + 13 \mu_2 \mu_1))) + \\
& (-1 + \eta t) \theta l (2 (\mu_1^2 (101 - 61 \mu_1) + 2 \times (58 - 82 \mu_2^2 + 60 \mu_1 + \\
& \quad \mu_2 (-29 + 5 \mu_1)) + \mu_1 (217 + 284 \mu_1 - 2 \mu_2 (384 + 55 \mu_1))) + \\
& \quad \theta p (1926 + 359 \mu_1 + 125 \mu_1^2 + 4 \mu_2^2 (402 + 153 \mu_1 - 197 \mu_2) + \\
& \quad 79 \mu_2 - 125 \mu_1 \mu_2 + \mu_2 (7442 + 1141 \mu_1 + 125 \mu_1^2 + 581 \mu_2 - 125 \\
& \quad \mu_1 \mu_2) + \mu_1^2 (2136 + 263 \mu_1 + 25 \mu_1^2 + 273 \mu_2 + 15 \mu_1 \mu_2) + \\
& \quad \mu_1 (4062 + 682 \mu_1 + 330 \mu_1^2 + 352 \mu_2 - 290 \mu_1 \mu_2 + \\
& \quad \mu_2 (7682 + 437 \mu_1 + 125 \mu_1^2 + 1277 \mu_2 - 185 \mu_1 \mu_2)))) + \eta^4 \\
& (2 \theta p (517 + 3883 \mu_2 + 4200 \mu_2^2 + 253 \mu_1 + 715 \mu_2 \mu_1 - 20 \mu_1^2 \\
& \quad (-45 + 7 \mu_1) + \mu_1 (1417 + 4379 \mu_2 + 263 \mu_1 - 11 \mu_2 \mu_1) + \\
& \quad \eta t (-173 + 343 \mu_2 + 1316 \mu_2^2 - 105 \mu_1 - 65 \mu_2 \mu_1 + \\
& \quad 4 \mu_1^2 (189 + 47 \mu_1) + \mu_1 (583 + 3435 \mu_2 - 325 \mu_1 + 565 \mu_2 \mu_1))) - \\
& (-1 + \eta t) \theta l (124 - 324 \mu_1 - 448 \mu_1^2 - 9 \mu_2 - 2585 \mu_1 \mu_2 - \\
& \quad 8 \mu_2^2 + 100 \mu_1 + 360 \mu_1 \mu_1 - 64 \mu_1^2 \mu_1 + 25 \mu_2 \mu_1 - 95 \mu_1 \mu_2 \mu_1 + \\
& 5 \theta p (470 + 53 \mu_1 + 15 \mu_1^2 + 8 \mu_2^2 (20 + 3 \mu_1 - 30 \mu_2) - 7 \mu_2 - \\
& \quad 15 \mu_1 \mu_2 + \mu_2 (1674 + 107 \mu_1 + 15 \mu_1^2 + 23 \mu_2 - 15 \mu_1 \mu_2) + \\
& \quad \mu_1^2 (476 + 31 \mu_1 + 9 \mu_1^2 + 49 \mu_2 + 3 \mu_1 \mu_2) + \\
& \quad \mu_1 (946 + 120 \mu_1 + 60 \mu_1^2 + 42 \mu_2 - 48 \mu_1 \mu_2 + \\
& \quad \mu_2 (1530 - 53 \mu_1 + 15 \mu_1^2 + 199 \mu_2 - 51 \mu_1 \mu_2)))) - 2 \\
& \eta^2 (\theta p (3 \times (351 + 1405 \mu_2 + 744 \mu_2^2 + 121 \mu_1 + 201 \mu_2 \mu_1 + \\
& \quad \mu_1^2 (540 + 44 \mu_1) + \mu_1 (891 + 1541 \mu_2 + 219 \mu_1 - 45 \mu_2 \mu_1)) + \\
& \quad \eta t (-446 - 257 \mu_2 + 1032 \mu_2^2 - 192 \mu_1 - 81 \mu_2 \mu_1 +
\end{aligned}$$

$$\begin{aligned}
& \mu^2 (622 + 342 \, \mathfrak{e}1) + \mu (176 + 2623 \, \mu^2 - 444 \, \mathfrak{e}1 + 477 \, \mu^2 \, \mathfrak{e}1) \Big) + \\
& (-1 + \eta t) \, \mathfrak{e}l \, (188 + 790 \, \mu^2 + 602 \, \mu^2 - 289 \, \mu^2 - 265 \, \mu^2 \, \mu^2 - \\
& 504 \, \mu^2 + 240 \, \mathfrak{e}1 + 444 \, \mu^2 \, \mathfrak{e}1 + 6 \, \mu^2 \, \mathfrak{e}1 - 15 \, \mu^2 \, \mathfrak{e}1 - 267 \, \mu^2 \, \mu^2 \, \mathfrak{e}1 + \\
& 3 \, \mathfrak{e}p \, (302 + 91 \, \mathfrak{e}1 + 35 \, \mathfrak{e}1^2 + \mu^2 (484 + 222 \, \mathfrak{e}1 - 74 \, \mathfrak{e}2) + 39 \, \mathfrak{e}2 - \\
& 35 \, \mathfrak{e}1 \, \mathfrak{e}2 + \mu^2 (1310 + 35 \, \mathfrak{e}1^2 + \mathfrak{e}1 (351 - 35 \, \mathfrak{e}2) + 211 \, \mathfrak{e}2) + \\
& \mu^2 (380 + \mathfrak{e}1^2 + 61 \, \mathfrak{e}2 + 3 \, \mathfrak{e}1 (25 + \mathfrak{e}2)) + \\
& \mu (682 + 72 \, \mathfrak{e}1^2 + 2 \, \mathfrak{e}1 (77 - 34 \, \mathfrak{e}2) + 100 \, \mathfrak{e}2 + \\
& \mu^2 (1550 + 231 \, \mathfrak{e}1 + 35 \, \mathfrak{e}1^2 + 315 \, \mathfrak{e}2 - 23 \, \mathfrak{e}1 \, \mathfrak{e}2) \Big) \Big) + \eta \\
& (-2 \, \mathfrak{e}p \, (3 \times (43 + 72 \, \mu^2 + 209 \, \mu^2 + 120 \, \mu^2 + 23 \, \mathfrak{e}1 + 25 \, \mu^2 \, \mathfrak{e}1 + \\
& \mu^2 (115 + 265 \, \mu^2 + 29 \, \mathfrak{e}1 + 7 \, \mu^2 \, \mathfrak{e}1) \Big) + \\
& 2 \, \eta t \, (-53 + 277 \, \mu^2 + 378 \, \mu^2 - 108 \, \mathfrak{e}1 - 6 \, \mu^2 \, \mathfrak{e}1 + 4 \, \mu^2 \\
& (-5 + 27 \, \mathfrak{e}1) + \mu (-73 + 397 \, \mu^2 - 198 \, \mathfrak{e}1 + 147 \, \mu^2 \, \mathfrak{e}1) \Big) \Big) + \\
& 3 \times (-1 + \eta t) \, \mathfrak{e}l \, (-4 \times (6 - 32 \, \mu^2 + 10 \, \mathfrak{e}1 + \mu^2 (23 + \mathfrak{e}1) - \\
& \mu^2 (27 + 5 \, \mathfrak{e}1) + \mu^2 (29 + 14 \, \mathfrak{e}1 - \mu^2 (25 + 17 \, \mathfrak{e}1)) \Big) + \mathfrak{e}p \\
& (-74 - 37 \, \mathfrak{e}1 - 15 \, \mathfrak{e}1^2 - 21 \, \mathfrak{e}2 + 15 \, \mathfrak{e}1 \, \mathfrak{e}2 - 4 \, \mu^2 (54 + 27 \, \mathfrak{e}1 + \mathfrak{e}2) - \\
& \mu^2 (382 + 159 \, \mathfrak{e}1 + 15 \, \mathfrak{e}1^2 + 103 \, \mathfrak{e}2 - 15 \, \mathfrak{e}1 \, \mathfrak{e}2) + \mu^2 (-112 + \mathfrak{e}1^2 - \\
& 23 \, \mathfrak{e}2 - \mathfrak{e}1 (33 + \mathfrak{e}2)) - \mu (186 + 58 \, \mathfrak{e}1 + 26 \, \mathfrak{e}1^2 + 44 \, \mathfrak{e}2 - 26 \\
& \mathfrak{e}1 \, \mathfrak{e}2 + \mu^2 (526 + 127 \, \mathfrak{e}1 + 15 \, \mathfrak{e}1^2 + 127 \, \mathfrak{e}2 - 3 \, \mathfrak{e}1 \, \mathfrak{e}2) \Big) \Big) \Big) + \\
& \eta \, \mathfrak{e}p \, (-6 \, \eta^8 (3 + 4 \, \mu^2 + \mathfrak{e}1 + \mu^2 (3 + \mathfrak{e}1)) + 3 \, \eta t \, \mu^2 (11 + 8 \, \mu^2 + 5 \, \mathfrak{e}1 + \\
& \mu^2 (11 + 5 \, \mathfrak{e}1)) + 3 \, \eta \, \eta t \, (80 \, \mu^2 + 4 \, \mu^2 (-7 + \mathfrak{e}1) + 5 \, \mu^2 (15 + \mathfrak{e}1) - \\
& 4 \times (1 + 5 \, \mathfrak{e}1) - 4 \, \mu^2 (8 + 7 \, \mathfrak{e}1) + \mu^2 (75 + 29 \, \mathfrak{e}1) \Big) + 6 \, \eta^7 \\
& (\eta t (3 + 4 \, \mu^2 + \mathfrak{e}1 + \mu^2 (3 + \mathfrak{e}1)) - 2 \times (7 + 7 \, \mu^2 - 14 \, \mu^2 + 2 \, \mathfrak{e}1 + \\
& 2 \, \mu^2 (3 + \mathfrak{e}1) + \mu^2 (13 + 3 \, \mu^2 + 4 \, \mathfrak{e}1 - 3 \, \mu^2 \, \mathfrak{e}1) \Big) \Big) - 2 \, \eta^6 \\
& (123 + 251 \, \mu^2 - 324 \, \mu^2 + 23 \, \mathfrak{e}1 + 33 \, \mu^2 \, \mathfrak{e}1 + 36 \, \mu^2 (5 + \mathfrak{e}1) + \\
& \mu^2 (303 + 219 \, \mu^2 + 77 \, \mathfrak{e}1 - 75 \, \mu^2 \, \mathfrak{e}1) + \\
& 6 \, \eta t (-7 - 7 \, \mu^2 + 14 \, \mu^2 - 2 \, \mathfrak{e}1 + \mu^2 (-7 + 5 \, \mu^2 - 2 \, \mathfrak{e}1 + 3 \, \mu^2 \, \mathfrak{e}1) \Big) \Big) + \eta^4 \\
& (178 + 394 \, \mu^2 + 52 \, \eta t \, \mu^2 + 216 \, \mu^2 + 52 \, \eta t \, \mu^2 + 28 \, \mu^2 - 229 \, \eta t \, \mu^2 - \\
& 172 \, \mu^2 \, \mu^2 - 509 \, \eta t \, \mu^2 \, \mu^2 - 1112 \, \mu^2 - 120 \, \eta t \, \mu^2 + 6 \, \mathfrak{e}1 + \\
& 80 \, \eta t \, \mathfrak{e}1 + 102 \, \mu^2 \, \mathfrak{e}1 + 184 \, \eta t \, \mu^2 \, \mathfrak{e}1 + 72 \, \mu^2 \, \mathfrak{e}1 - 100 \, \eta t \, \mu^2 \, \mathfrak{e}1 + \\
& 16 \, \mu^2 \, \mathfrak{e}1 + 13 \, \eta t \, \mu^2 \, \mathfrak{e}1 - 212 \, \mu^2 \, \mu^2 \, \mathfrak{e}1 - 107 \, \eta t \, \mu^2 \, \mu^2 \, \mathfrak{e}1 + \\
& (-1 + \eta t) \, \mathfrak{e}l \, (398 + 75 \, \mathfrak{e}1 + 25 \, \mathfrak{e}1^2 + 4 \, \mu^2 (82 + 33 \, \mathfrak{e}1 - 37 \, \mathfrak{e}2) + \\
& 19 \, \mathfrak{e}2 - 25 \, \mathfrak{e}1 \, \mathfrak{e}2 + \mu^2 (1546 + 241 \, \mathfrak{e}1 + 25 \, \mathfrak{e}1^2 + 129 \, \mathfrak{e}2 - 25 \, \mathfrak{e}1 \, \mathfrak{e}2) + \\
& \mu^2 (440 + 5 \, \mathfrak{e}1^2 + 61 \, \mathfrak{e}2 + \mathfrak{e}1 (59 + 3 \, \mathfrak{e}2)) + \\
& \mu (838 + 146 \, \mathfrak{e}1 + 66 \, \mathfrak{e}1^2 + 80 \, \mathfrak{e}2 - 58 \, \mathfrak{e}1 \, \mathfrak{e}2 + \\
& \mu^2 (1594 + 113 \, \mathfrak{e}1 + 25 \, \mathfrak{e}1^2 + 281 \, \mathfrak{e}2 - 37 \, \mathfrak{e}1 \, \mathfrak{e}2) \Big) \Big) + \eta^3 \\
& (4 \times (80 + 124 \, \mu^2 + 25 \, \mathfrak{e}1 + 44 \, \mu^2 (7 + \mathfrak{e}1) + \mu^2 (117 + 11 \, \mathfrak{e}1) + \\
& \mu^2 (197 - 16 \, \mu^2 (-20 + \mathfrak{e}1) + 48 \, \mathfrak{e}1) \Big) - \\
& \mathfrak{e}l \, (310 + 93 \, \mathfrak{e}1 + 35 \, \mathfrak{e}1^2 + 4 \, \mu^2 (122 + 57 \, \mathfrak{e}1 - 17 \, \mathfrak{e}2) + 41 \, \mathfrak{e}2 - \\
& 35 \, \mathfrak{e}1 \, \mathfrak{e}2 + \mu^2 (1346 + 359 \, \mathfrak{e}1 + 35 \, \mathfrak{e}1^2 + 219 \, \mathfrak{e}2 - 35 \, \mathfrak{e}1 \, \mathfrak{e}2) + \\
& \mu^2 (388 + \mathfrak{e}1^2 + 65 \, \mathfrak{e}2 + \mathfrak{e}1 (79 + 3 \, \mathfrak{e}2)) + \\
& \mu (2 \times (349 + 80 \, \mathfrak{e}1 + 36 \, \mathfrak{e}1^2 + 53 \, \mathfrak{e}2 - 34 \, \mathfrak{e}1 \, \mathfrak{e}2) + \\
& \mu^2 (1586 + 247 \, \mathfrak{e}1 + 35 \, \mathfrak{e}1^2 + 331 \, \mathfrak{e}2 - 23 \, \mathfrak{e}1 \, \mathfrak{e}2) \Big) \Big) + \\
& \eta t \, (2 \times (56 \, \mu^2 + 9 \times (-5 + \mathfrak{e}1) + 32 \, \mu^2 (5 + \mathfrak{e}1) - 2 \, \mu^2
\end{aligned}$$

$$\begin{aligned}
& (57 + 7 \mathfrak{e}1) + \mu1 (115 - \mathfrak{e}1 + \mu2 (406 + 22 \mathfrak{e}1)) \Big) + \\
& \mathfrak{e}l \Big( 310 + 93 \mathfrak{e}1 + 35 \mathfrak{e}1^2 + 4 \mu2^2 (122 + 57 \mathfrak{e}1 - 17 \mathfrak{e}2) + 41 \mathfrak{e}2 - \\
& \quad 35 \mathfrak{e}1 \mathfrak{e}2 + \mu2 (1346 + 359 \mathfrak{e}1 + 35 \mathfrak{e}1^2 + 219 \mathfrak{e}2 - 35 \mathfrak{e}1 \mathfrak{e}2) + \\
& \quad \mu1^2 (388 + \mathfrak{e}1^2 + 65 \mathfrak{e}2 + \mathfrak{e}1 (79 + 3 \mathfrak{e}2)) + \\
& \quad \mu1 (2 \times (349 + 80 \mathfrak{e}1 + 36 \mathfrak{e}1^2 + 53 \mathfrak{e}2 - 34 \mathfrak{e}1 \mathfrak{e}2) + \\
& \quad \mu2 (1586 + 247 \mathfrak{e}1 + 35 \mathfrak{e}1^2 + 331 \mathfrak{e}2 - 23 \mathfrak{e}1 \mathfrak{e}2)) \Big) \Big) \Big) + \\
& \eta^5 \Big( -4 \times (59 + 110 \mu2^2 + 19 \mathfrak{e}1 + \mu1^2 (99 + 5 \mathfrak{e}1) + \mu1 (158 + \\
& \quad \mu2 (291 - 19 \mathfrak{e}1) + 36 \mathfrak{e}1) + \mu2 (267 + 44 \mathfrak{e}1)) - \\
& \mathfrak{e}l \Big( 162 + 19 \mathfrak{e}1 + 5 \mathfrak{e}1^2 + 4 \mu2^2 (14 + 3 \mathfrak{e}1 - 19 \mathfrak{e}2) - \mathfrak{e}2 - \\
& \quad 5 \mathfrak{e}1 \mathfrak{e}2 + \mu2 (582 + 41 \mathfrak{e}1 + 5 \mathfrak{e}1^2 + 13 \mathfrak{e}2 - 5 \mathfrak{e}1 \mathfrak{e}2) + \\
& \quad \mu1^2 (164 + 3 \mathfrak{e}1^2 + 19 \mathfrak{e}2 + \mathfrak{e}1 (13 + \mathfrak{e}2)) + \\
& \quad \mu1 (\mu2 (534 - 7 \mathfrak{e}1 + 5 \mathfrak{e}1^2 + 77 \mathfrak{e}2 - 17 \mathfrak{e}1 \mathfrak{e}2) + \\
& \quad 2 \times (163 + 22 \mathfrak{e}1 + 10 \mathfrak{e}1^2 + 9 \mathfrak{e}2 - 8 \mathfrak{e}1 \mathfrak{e}2)) \Big) \Big) + \\
& \eta t \Big( 84 - 72 \mu1 - 156 \mu1^2 - 21 \mu2 - 813 \mu1 \mu2 - 352 \mu2^2 + \\
& \quad 36 \mathfrak{e}1 + 80 \mu1 \mathfrak{e}1 - 28 \mu1^2 \mathfrak{e}1 + 13 \mu2 \mathfrak{e}1 - 131 \mu1 \mu2 \mathfrak{e}1 + \\
& \mathfrak{e}l \Big( 162 + 19 \mathfrak{e}1 + 5 \mathfrak{e}1^2 + 4 \mu2^2 (14 + 3 \mathfrak{e}1 - 19 \mathfrak{e}2) - \mathfrak{e}2 - \\
& \quad 5 \mathfrak{e}1 \mathfrak{e}2 + \mu2 (582 + 41 \mathfrak{e}1 + 5 \mathfrak{e}1^2 + 13 \mathfrak{e}2 - 5 \mathfrak{e}1 \mathfrak{e}2) + \\
& \quad \mu1^2 (164 + 3 \mathfrak{e}1^2 + 19 \mathfrak{e}2 + \mathfrak{e}1 (13 + \mathfrak{e}2)) + \\
& \quad \mu1 (\mu2 (534 - 7 \mathfrak{e}1 + 5 \mathfrak{e}1^2 + 77 \mathfrak{e}2 - 17 \mathfrak{e}1 \mathfrak{e}2) + \\
& \quad 2 \times (163 + 22 \mathfrak{e}1 + 10 \mathfrak{e}1^2 + 9 \mathfrak{e}2 - 8 \mathfrak{e}1 \mathfrak{e}2)) \Big) \Big) \Big) + \\
& \eta^2 \Big( 2 \times (43 + 72 \mu1^2 + 120 \mu2^2 + 23 \mathfrak{e}1 + \mu2 (209 + 25 \mathfrak{e}1) + \\
& \quad \mu1 (115 + 29 \mathfrak{e}1 + \mu2 (265 + 7 \mathfrak{e}1)) \Big) + \\
& \mathfrak{e}l \Big( -74 - 37 \mathfrak{e}1 - 15 \mathfrak{e}1^2 - 21 \mathfrak{e}2 + 15 \mathfrak{e}1 \mathfrak{e}2 - 4 \mu2^2 (54 + 27 \mathfrak{e}1 + \mathfrak{e}2) - \\
& \quad \mu2 (382 + 159 \mathfrak{e}1 + 15 \mathfrak{e}1^2 + 103 \mathfrak{e}2 - 15 \mathfrak{e}1 \mathfrak{e}2) + \mu1^2 \\
& \quad (-112 + \mathfrak{e}1^2 - 23 \mathfrak{e}2 - \mathfrak{e}1 (33 + \mathfrak{e}2)) - \mu1 (186 + 58 \mathfrak{e}1 + 26 \mathfrak{e}1^2 + 44 \\
& \quad \mathfrak{e}2 - 26 \mathfrak{e}1 \mathfrak{e}2 + \mu2 (526 + 127 \mathfrak{e}1 + 15 \mathfrak{e}1^2 + 127 \mathfrak{e}2 - 3 \mathfrak{e}1 \mathfrak{e}2)) \Big) \Big) + \\
& \eta t \Big( 4 \times (-21 + 66 \mu2^2 - 7 \mu2 (-4 + \mathfrak{e}1) - 26 \mathfrak{e}1 + \mu1^2 (-33 + 13 \mathfrak{e}1) + \\
& \quad \mu1 (-54 - 52 \mathfrak{e}1 + \mu2 (78 + 32 \mathfrak{e}1)) \Big) + \mathfrak{e}l \\
& \quad (74 + 37 \mathfrak{e}1 + 15 \mathfrak{e}1^2 + 21 \mathfrak{e}2 - 15 \mathfrak{e}1 \mathfrak{e}2 + 4 \mu2^2 (54 + 27 \mathfrak{e}1 + \mathfrak{e}2) + \\
& \quad \mu2 (382 + 159 \mathfrak{e}1 + 15 \mathfrak{e}1^2 + 103 \mathfrak{e}2 - 15 \mathfrak{e}1 \mathfrak{e}2) + \mu1^2 (112 - \mathfrak{e}1^2 + \\
& \quad 23 \mathfrak{e}2 + \mathfrak{e}1 (33 + \mathfrak{e}2)) + \mu1 (186 + 58 \mathfrak{e}1 + 26 \mathfrak{e}1^2 + 44 \mathfrak{e}2 - 26 \\
& \quad \mathfrak{e}1 \mathfrak{e}2 + \mu2 (526 + 127 \mathfrak{e}1 + 15 \mathfrak{e}1^2 + 127 \mathfrak{e}2 - 3 \mathfrak{e}1 \mathfrak{e}2)) \Big) \Big) \Big) \Big) + \\
& x^4 (-1 + \eta)^4 \Big( - \Big( (-1 + \eta) \mathfrak{e}p \Big( 210 \eta^4 (3 + 4 \mu2 + \mathfrak{e}1 + \mu1 (3 + \mathfrak{e}1)) - \\
& \quad 30 \eta^3 (-51 - 54 \mu2 + 84 \mu2^2 - 15 \mathfrak{e}1 - 28 \mu1^2 (3 + \mathfrak{e}1) + \mu1 (-135 - \\
& \quad 82 \mu2 - 43 \mathfrak{e}1 + 18 \mu2 \mathfrak{e}1) + 7 \eta t (3 + 4 \mu2 + \mathfrak{e}1 + \mu1 (3 + \mathfrak{e}1)) \Big) \Big) + \\
& \quad 10 \eta^2 (348 + 827 \mu2 - 408 \mu2^2 + 68 \mathfrak{e}1 + 99 \mu2 \mathfrak{e}1 + 72 \mu1^2 \\
& \quad (9 + 2 \mathfrak{e}1) + \mu1 (996 + 951 \mu2 + 266 \mathfrak{e}1 - 135 \mu2 \mathfrak{e}1) + 9 \eta t (-17 - \\
& \quad 18 \mu2 + 28 \mu2^2 - 5 \mathfrak{e}1 + \mu1 (-17 + 10 \mu2 - 5 \mathfrak{e}1 + 6 \mu2 \mathfrak{e}1)) \Big) \Big) + \\
& \quad 2 \times (191 + 789 \mu2 + 496 \mu2^2 + 71 \mathfrak{e}1 + 113 \mu2 \mathfrak{e}1 + \mu1^2 \\
& \quad (306 + 22 \mathfrak{e}1) + \mu1 (497 + 901 \mu2 + 123 \mathfrak{e}1 - 13 \mu2 \mathfrak{e}1) + \\
& \quad \eta t (-85 + 103 \mu2 + 344 \mu2^2 - 73 \mathfrak{e}1 - 13 \mu2 \mathfrak{e}1 + \\
& \quad 2 \mu1^2 (73 + 65 \mathfrak{e}1) + \mu1 (61 + 527 \mu2 - 147 \mathfrak{e}1 + 137 \mu2 \mathfrak{e}1)) \Big) \Big) +
\end{aligned}$$

$$\begin{aligned}
& \eta \left( 2 \times \left( 1232 + 4043 \mu_2 + 1060 \mu_2^2 + 328 \mathfrak{e}_1 + 605 \mu_2 \mathfrak{e}_1 + 10 \mu_1^2 \right. \right. \\
& \quad \left. \left. (207 + 29 \mathfrak{e}_1) + \mu_1 (3302 + 4439 \mu_2 + 828 \mathfrak{e}_1 - 391 \mu_2 \mathfrak{e}_1) \right) + \right. \\
& \quad \left. \eta t \left( -946 - 499 \mu_2 + 2552 \mu_2^2 - 330 \mathfrak{e}_1 - 65 \mu_2 \mathfrak{e}_1 + 4 \mu_1^2 (183 + \right. \right. \\
& \quad \left. \left. 59 \mathfrak{e}_1) + \mu_1 (-214 + 3405 \mu_2 - 550 \mathfrak{e}_1 + 835 \mu_2 \mathfrak{e}_1) \right) \right) + \\
& (-1 + \eta t) \mathfrak{e}l \left( -2 \times \left( -44 + 224 \mu_2^2 - 80 \mathfrak{e}_1 + \mu_2 (171 + 5 \mathfrak{e}_1) + \right. \right. \\
& \quad \left. \left. 2 \mu_1^2 (-51 + 23 \mathfrak{e}_1) - 2 \mu_1 (73 + 74 \mathfrak{e}_1) + \mu_1 \mu_2 (147 + 89 \mathfrak{e}_1) \right) + \right. \\
& \quad \mathfrak{e}p \left( 294 + 89 \mathfrak{e}_1 + 35 \mathfrak{e}_1^2 + 8 \mu_2^2 (60 + 27 \mathfrak{e}_1 - 10 \mathfrak{e}_2) + 37 \mathfrak{e}_2 - \right. \\
& \quad \left. 35 \mathfrak{e}_1 \mathfrak{e}_2 + 7 \mu_2 (182 + 49 \mathfrak{e}_1 + 5 \mathfrak{e}_1^2 + 29 \mathfrak{e}_2 - 5 \mathfrak{e}_1 \mathfrak{e}_2) + \right. \\
& \quad \left. \mu_1^2 (372 + \mathfrak{e}_1^2 + 57 \mathfrak{e}_2 + \mathfrak{e}_1 (71 + 3 \mathfrak{e}_2)) + \right. \\
& \quad \left. \mu_1 (666 + 148 \mathfrak{e}_1 + 72 \mathfrak{e}_1^2 + 94 \mathfrak{e}_2 - 68 \mathfrak{e}_1 \mathfrak{e}_2 + \right. \\
& \quad \left. \mu_2 (1514 + 215 \mathfrak{e}_1 + 35 \mathfrak{e}_1^2 + 299 \mathfrak{e}_2 - 23 \mathfrak{e}_1 \mathfrak{e}_2) \right) \right) + \\
& \eta \left( 4 \left( \mu_1^2 (7 - 127 \mathfrak{e}_1) + 2 \times (54 - 94 \mu_2^2 + 5 \mu_2 (-9 + \mathfrak{e}_1) + 60 \mathfrak{e}_1) + \right. \right. \\
& \quad \left. \mu_1 (115 + 284 \mathfrak{e}_1 - 2 \mu_2 (302 + 55 \mathfrak{e}_1)) \right) + \mathfrak{e}p \\
& \quad \left( 1862 + 343 \mathfrak{e}_1 + 125 \mathfrak{e}_1^2 + 4 \mu_2^2 (394 + 141 \mathfrak{e}_1 - 209 \mathfrak{e}_2) + 63 \mathfrak{e}_2 - \right. \\
& \quad \left. 125 \mathfrak{e}_1 \mathfrak{e}_2 + \mu_2 (7154 + 1077 \mathfrak{e}_1 + 125 \mathfrak{e}_1^2 + 517 \mathfrak{e}_2 - 125 \mathfrak{e}_1 \mathfrak{e}_2) + \right. \\
& \quad \left. \mu_1^2 (2072 + 25 \mathfrak{e}_1^2 + 241 \mathfrak{e}_2 + 3 \mathfrak{e}_1 (77 + 5 \mathfrak{e}_2)) + \right. \\
& \quad \left. \mu_1 (3934 + 634 \mathfrak{e}_1 + 330 \mathfrak{e}_1^2 + 304 \mathfrak{e}_2 - 290 \mathfrak{e}_1 \mathfrak{e}_2 + \right. \\
& \quad \left. \mu_2 (7394 + 309 \mathfrak{e}_1 + 125 \mathfrak{e}_1^2 + 1149 \mathfrak{e}_2 - 185 \mathfrak{e}_1 \mathfrak{e}_2) \right) \right) + \\
& \eta^2 \left( 264 - 584 \mu_1 - 848 \mu_1^2 + 46 \mu_2 - 4210 \mu_1 \mu_2 + 32 \mu_2^2 + \right. \\
& \quad \left. 200 \mathfrak{e}_1 + 720 \mu_1 \mathfrak{e}_1 - 224 \mu_1^2 \mathfrak{e}_1 + 50 \mu_2 \mathfrak{e}_1 - 190 \mu_1 \mu_2 \mathfrak{e}_1 + \right. \\
& \quad \left. 5 \mathfrak{e}p \left( 454 + 49 \mathfrak{e}_1 + 15 \mathfrak{e}_1^2 + 4 \mu_2^2 (38 + 3 \mathfrak{e}_1 - 63 \mathfrak{e}_2) - 11 \mathfrak{e}_2 - \right. \right. \\
& \quad \left. \left. 15 \mathfrak{e}_1 \mathfrak{e}_2 + \mu_2 (1602 + 91 \mathfrak{e}_1 + 15 \mathfrak{e}_1^2 + 7 \mathfrak{e}_2 - 15 \mathfrak{e}_1 \mathfrak{e}_2) + \right. \right. \\
& \quad \left. \left. \mu_1^2 (460 + 9 \mathfrak{e}_1^2 + 41 \mathfrak{e}_2 + \mathfrak{e}_1 (23 + 3 \mathfrak{e}_2)) + \right. \right. \\
& \quad \left. \left. \mu_1 (914 + 108 \mathfrak{e}_1 + 60 \mathfrak{e}_1^2 + 30 \mathfrak{e}_2 - 48 \mathfrak{e}_1 \mathfrak{e}_2 + \right. \right. \\
& \quad \left. \left. \mu_2 (1458 + 15 \mathfrak{e}_1^2 + 167 \mathfrak{e}_2 - 17 \mathfrak{e}_1 (5 + 3 \mathfrak{e}_2)) \right) \right) \right) - \\
& (x + \eta - x \eta)^2 \left( -2 x^6 (-1 + \eta)^6 \mathfrak{e}p \left( 2 - 2 \mathfrak{e}l - 25 \mu_1 + 13 \mathfrak{e}l \mu_1 - 27 \mu_1^2 + \right. \right. \\
& \quad \left. \left. 15 \mathfrak{e}l \mu_1^2 + 12 \mu_2 - 12 \mathfrak{e}l \mu_2 - 44 \mu_1 \mu_2 + 28 \mathfrak{e}l \mu_1 \mu_2 + 2 \right. \right. \\
& \quad \left. \left. \mathfrak{e}_1 - 2 \mathfrak{e}l \mathfrak{e}_1 - 9 \mu_1 \mathfrak{e}_1 + 5 \mathfrak{e}l \mu_1 \mathfrak{e}_1 - 5 \mu_1^2 \mathfrak{e}_1 + \mathfrak{e}l \right. \right. \\
& \quad \left. \left. \mu_1^2 \mathfrak{e}_1 + 2 \eta t (4 + 8 \mu_2 + \mathfrak{e}_1 + \mu_1 (4 + \mathfrak{e}_1)) + 2 \eta^2 \right. \right. \\
& \quad \left. \left. (6 + 16 \mu_2 + \mathfrak{e}_1 + \mu_1 (6 + \mathfrak{e}_1)) - \eta (14 - 13 \mu_1 - 27 \mu_1^2 + 44 \mu_2 - \right. \right. \\
& \quad \left. \left. 44 \mu_1 \mu_2 - 4 \mathfrak{e}l (1 + \mu_1 + 4 \mu_2) + 4 \mathfrak{e}_1 - 7 \mu_1 \mathfrak{e}_1 - 5 \mu_1^2 \mathfrak{e}_1 + \right. \right. \\
& \quad \left. \left. 2 \eta t (4 + 8 \mu_2 + 2 \mathfrak{e}l (1 + \mu_1 + 4 \mu_2) + \mathfrak{e}_1 + \mu_1 (4 + \mathfrak{e}_1)) \right) - \eta t \right. \\
& \quad \left. \mathfrak{e}l \left( -2 - 2 \mathfrak{e}_1 + \mu_1^2 (15 + \mathfrak{e}_1) + \mu_1 (13 + 28 \mu_2 + 5 \mathfrak{e}_1) + \right. \right. \\
& \quad \left. \left. 4 \mu_2 (-3 + \mathfrak{e}_2) \right) + 4 \mathfrak{e}l \mu_2 \mathfrak{e}_2 \right) + \\
& x^5 (-1 + \eta)^5 \left( 4 \times (-1 + \eta t) \mathfrak{e}l \left( 4 \mu_2 + \mu_1^2 (3 + \mathfrak{e}_1 + \eta (9 + \mathfrak{e}_1)) + \right. \right. \\
& \quad \left. \mu_1 (3 + 12 \mu_2 - 5 \mathfrak{e}_1 + \eta (9 + 28 \mu_2 + \mathfrak{e}_1)) \right) + \mathfrak{e}p \\
& \quad \left( -10 + 10 \mathfrak{e}l - 136 \mu_1 + 94 \mathfrak{e}l \mu_1 - 126 \mu_1^2 + 84 \mathfrak{e}l \mu_1^2 - 18 \mu_2 + \right. \\
& \quad \left. 26 \mathfrak{e}l \mu_2 - 242 \mu_1 \mu_2 + 202 \mathfrak{e}l \mu_1 \mu_2 - 80 \mu_2^2 + 64 \mathfrak{e}l \mu_2^2 - 2 \mathfrak{e}_1 + \right. \\
& \quad \left. 2 \mathfrak{e}l \mathfrak{e}_1 - 44 \mu_1 \mathfrak{e}_1 + 11 \mathfrak{e}l \mu_1 \mathfrak{e}_1 - 18 \mu_1^2 \mathfrak{e}_1 - 3 \mathfrak{e}l \mu_1^2 \mathfrak{e}_1 - \right. \\
& \quad \left. 18 \mu_2 \mathfrak{e}_1 + 10 \mathfrak{e}l \mu_2 \mathfrak{e}_1 - 6 \mu_1 \mu_2 \mathfrak{e}_1 - 38 \mathfrak{e}l \mu_1 \mu_2 \mathfrak{e}_1 + \right. \\
& \quad \left. 9 \mathfrak{e}l \mu_1 \mathfrak{e}_1^2 + 3 \mathfrak{e}l \mu_1^2 \mathfrak{e}_1^2 + 24 \eta^3 (6 + 16 \mu_2 + \mathfrak{e}_1 + \mu_1 (6 + \mathfrak{e}_1)) - \right. \\
& \quad \left. 4 \eta^2 (30 - 51 \mu_1 - 81 \mu_1^2 + 110 \mu_2 - 122 \mu_1 \mu_2 + 28 \mu_2^2 - \right. \\
& \quad \left. 12 \mathfrak{e}l (1 + \mu_1 + 4 \mu_2) + 10 \mathfrak{e}_1 - 23 \mu_1 \mathfrak{e}_1 - 15 \mu_1^2 \mathfrak{e}_1 + 6 \mu_1 \mu_2 \mathfrak{e}_1 + \right.
\end{aligned}$$

$$\begin{aligned}
& 6 \eta t (4 + 8 \mu_2 + 2 \theta l (1 + \mu_1 + 4 \mu_2) + \mathfrak{e}1 + \mu_1 (4 + \mathfrak{e}1)) + \\
& 3 \theta l \mu_1 \mathfrak{e}2 + 3 \theta l \mu_1^2 \mathfrak{e}2 + 8 \theta l \mu_2 \mathfrak{e}2 - 40 \theta l \mu_2^2 \mathfrak{e}2 - \\
& 5 \theta l \mu_1 \mathfrak{e}1 \mathfrak{e}2 + \theta l \mu_1^2 \mathfrak{e}1 \mathfrak{e}2 - 12 \theta l \mu_1 \mu_2 \mathfrak{e}1 \mathfrak{e}2 - \\
& \eta t (-32 - 44 \mu_2 + 56 \mu_2^2 - 8 \mathfrak{e}1 + 4 \mu_1 (-2 \times (4 + \mathfrak{e}1) + \mu_2 (5 + 3 \mathfrak{e}1)) + \\
& \theta l \mu_1^2 (3 \mathfrak{e}1^2 + \mathfrak{e}1 (-3 + \mathfrak{e}2) + 3 \times (28 + \mathfrak{e}2)) + \\
& 2 \theta l (5 + \mathfrak{e}1 + \mu_2 (13 + 5 \mathfrak{e}1 + 4 \mathfrak{e}2) - 4 \mu_2^2 (-8 + 5 \mathfrak{e}2)) + \theta l \mu_1 \\
& (94 + 202 \mu_2 + 9 \mathfrak{e}1^2 + \mathfrak{e}1 (11 - 5 \mathfrak{e}2) + 3 \mathfrak{e}2 - 2 \mu_2 \mathfrak{e}1 (19 + 6 \mathfrak{e}2))) + \\
& \eta (4 \eta t (37 \mu_2 + 14 \mu_2^2 + 4 \times (4 + \mathfrak{e}1) + 4 \mu_1 (4 + \mathfrak{e}1) + \mu_1 \mu_2 (5 + 3 \mathfrak{e}1)) - \\
& 2 \times (7 - 96 \mu_2^2 - 9 \mathfrak{e}1 + 3 \mu_1^2 (33 + 7 \mathfrak{e}1) - \mu_2 (37 + 9 \mathfrak{e}1) + \mu_1 \\
& (106 + 36 \mathfrak{e}1 - 3 \mu_2 (-41 + 5 \mathfrak{e}1))) + \theta l (-8 \times (1 + 3 \mathfrak{e}1) + 2 \mu_2 \\
& (-41 + \mathfrak{e}1 + 24 \mathfrak{e}2) + \mu_1^2 (\mathfrak{e}1^2 + 9 \times (22 + \mathfrak{e}2) + \mathfrak{e}1 (23 + \mathfrak{e}2)) + \\
& \mu_1 (190 + \mathfrak{e}1^2 + 9 \mathfrak{e}2 + \mathfrak{e}1 (71 + \mathfrak{e}2) + 2 \mu_2 (195 + 9 \mathfrak{e}1 + 14 \mathfrak{e}2))) - \\
& \eta t \theta l (-8 \times (1 + 3 \mathfrak{e}1) + 2 \mu_2 (-41 + \mathfrak{e}1 + 24 \mathfrak{e}2) + \\
& \mu_1^2 (\mathfrak{e}1^2 + 9 \times (22 + \mathfrak{e}2) + \mathfrak{e}1 (23 + \mathfrak{e}2)) + \mu_1 (190 + \mathfrak{e}1^2 + \\
& 9 \mathfrak{e}2 + \mathfrak{e}1 (71 + \mathfrak{e}2) + 2 \mu_2 (195 + 9 \mathfrak{e}1 + 14 \mathfrak{e}2)))) - \\
& x^2 (-1 + \eta)^2 ((-1 + \eta) \theta p (60 \eta^5 (6 + 16 \mu_2 + \mathfrak{e}1 + \mu_1 (6 + \mathfrak{e}1)) + \\
& 2 \eta t (4 \mu_2^2 - 15 \times (1 + \mathfrak{e}1) - \mu_2 (11 + 5 \mathfrak{e}1) - 2 \mu_1 (9 + 8 \mathfrak{e}1) + \\
& \mu_1^2 (-3 + 11 \mathfrak{e}1) + \mu_1 \mu_2 (-15 + 19 \mathfrak{e}1)) - \\
& 10 \eta^4 (-42 - 52 \mu_2 + 112 \mu_2^2 - 2 \mathfrak{e}1 - 3 \mu_1^2 (27 + 5 \mathfrak{e}1) + \mu_1 (-123 - \\
& 92 \mu_2 - 35 \mathfrak{e}1 + 24 \mu_2 \mathfrak{e}1) + 6 \eta t (4 + 8 \mu_2 + \mathfrak{e}1 + \mu_1 (4 + \mathfrak{e}1))) + \\
& 12 \eta^2 (25 + 103 \mu_2 + 136 \mu_2^2 + 13 \mathfrak{e}1 + 19 \mu_2 \mathfrak{e}1 + 2 \mu_1^2 (27 + \mathfrak{e}1) + \\
& \mu_1 (79 + 21 \mathfrak{e}1 + \mu_2 (159 + \mathfrak{e}1)) + 2 \eta t (-4 + 2 \mu_2 + 14 \mu_2^2 - \mathfrak{e}1 - \\
& \mu_2 \mathfrak{e}1 + 2 \mu_1^2 (6 + \mathfrak{e}1) + \mu_1 (8 + 46 \mu_2 - 5 \mathfrak{e}1 + 8 \mu_2 \mathfrak{e}1))) + \\
& \eta (\eta t (-68 + 24 \mu_2^2 - 60 \mathfrak{e}1 + 8 \mu_1^2 (-1 + 13 \mathfrak{e}1) - \mu_2 (5 + 27 \mathfrak{e}1) + \\
& \mu_1 (-76 - 93 \mu_2 - 148 \mathfrak{e}1 + 117 \mu_2 \mathfrak{e}1)) + \\
& 4 \times (88 \mu_2^2 - 3 \mu_1^2 (-9 + \mathfrak{e}1) + 8 \mu_2 (13 + \mathfrak{e}1) + \\
& 3 \times (9 + 5 \mathfrak{e}1) + 2 \mu_1 (27 + 6 \mathfrak{e}1 + \mu_2 (52 + 7 \mathfrak{e}1))) + \\
& 4 \eta^3 (61 + 75 \mu_2 - 40 \mu_2^2 + 11 \mathfrak{e}1 + 51 \mu_2 \mathfrak{e}1 + 45 \mu_1^2 (7 + \mathfrak{e}1) + \\
& \mu_1 (376 + 539 \mu_2 + 116 \mathfrak{e}1 - 51 \mu_2 \mathfrak{e}1) + \\
& 2 \eta t (-55 \mu_2 + 70 \mu_2^2 - 10 \times (4 + \mathfrak{e}1) + 3 \mu_1^2 (9 + \mathfrak{e}1) + \\
& \mu_1 (-13 - 7 \mathfrak{e}1 + \mu_2 (109 + 15 \mathfrak{e}1)))) - \\
& (-1 + \eta t) \theta l (10 + 20 \mu_1 + 10 \mu_1^2 + 11 \mu_2 + 11 \mu_1 \mu_2 + 8 \mu_2^2 + \\
& 120 \eta^5 \theta p (1 + \mu_1 + 4 \mu_2) + 10 \mathfrak{e}1 + 8 \mu_1 \mathfrak{e}1 - 2 \mu_1^2 \mathfrak{e}1 + 5 \mu_2 \mathfrak{e}1 - \\
& 19 \mu_1 \mu_2 \mathfrak{e}1 - \theta p (\mu_1^2 (-5 + \mathfrak{e}1) \times (-2 + \mathfrak{e}1 - \mathfrak{e}2) - 2 \mu_1 (5 + 2 \mathfrak{e}1) \times \\
& (-2 + \mathfrak{e}1 - \mathfrak{e}2) + 8 \mu_2^2 (2 + \mathfrak{e}2) + 5 \times (2 + \mathfrak{e}1 - \mathfrak{e}1^2 + \mathfrak{e}2 + \mathfrak{e}1 \mathfrak{e}2) + \\
& \mu_1 \mu_2 (-5 \mathfrak{e}1^2 + 11 \times (2 + \mathfrak{e}2) - 7 \mathfrak{e}1 (3 + \mathfrak{e}2)) + \\
& \mu_2 (-5 \mathfrak{e}1^2 + 11 \times (2 + \mathfrak{e}2) + \mathfrak{e}1 (3 + 5 \mathfrak{e}2))) + 2 \eta^4 \\
& (-8 \mu_1 (9 + 28 \mu_2 + \mathfrak{e}1 + \mu_1 (9 + \mathfrak{e}1)) + 5 \theta p (\mu_1^2 (\mathfrak{e}1^2 + 9 \times (7 + \mathfrak{e}2) + \\
& \mathfrak{e}1 (14 + \mathfrak{e}2)) + 2 \times (5 - 3 \mathfrak{e}1 + \mu_2 (13 + \mathfrak{e}1 + 6 \mathfrak{e}2)) + \mu_1 \\
& (73 + \mathfrak{e}1^2 + 9 \mathfrak{e}2 + \mathfrak{e}1 (26 + \mathfrak{e}2) + 2 \mu_2 (69 + 9 \mathfrak{e}1 + 14 \mathfrak{e}2)))) + \\
& 4 \eta^3 (-4 \times (4 \mu_2 + \mu_1 (9 + 36 \mu_2 - 5 \mathfrak{e}1) + \mu_1^2 (9 + \mathfrak{e}1)) + \\
& \theta p (37 + 5 \mathfrak{e}1 + 2 \mu_2 (61 + 14 \mathfrak{e}1 + 10 \mathfrak{e}2) - 4 \mu_2^2 (-34 + 25 \mathfrak{e}2) + \\
& \mu_1^2 (249 + 15 \mathfrak{e}1 + 9 \mathfrak{e}1^2 + 27 \mathfrak{e}2 + 4 \mathfrak{e}1 \mathfrak{e}2)) +
\end{aligned}$$

$$\begin{aligned}
& \mu_1 (286 + 50 \mathfrak{e}_1 + 24 \mathfrak{e}_1^2 + 27 \mathfrak{e}_2 - 11 \mathfrak{e}_1 \mathfrak{e}_2 + \\
& \quad \mu_2 (646 - 44 \mathfrak{e}_1 + 66 \mathfrak{e}_2 - 30 \mathfrak{e}_1 \mathfrak{e}_2)) + \\
& \eta^2 (76 + 49 \mu_2 - 28 \mu_1^2 (-7 + \mathfrak{e}_1) + 60 \mathfrak{e}_1 + 15 \mu_2 \mathfrak{e}_1 + \\
& \quad \mu_1 (272 + 321 \mu_2 + 164 \mathfrak{e}_1 - 57 \mu_2 \mathfrak{e}_1) + 3 \mathfrak{e}_p \\
& \quad (\mu_1^2 (142 + 9 \mathfrak{e}_1^2 + 5 \mathfrak{e}_2 + \mathfrak{e}_1 (-9 + 5 \mathfrak{e}_2)) + \mu_1 (194 - 7 \mathfrak{e}_1 + 43 \mathfrak{e}_1^2 - \\
& \quad \mathfrak{e}_2 - 29 \mathfrak{e}_1 \mathfrak{e}_2 + 2 \mu_2 (243 - 40 \mathfrak{e}_1 + 5 \mathfrak{e}_1^2 - \mathfrak{e}_2 - 17 \mathfrak{e}_1 \mathfrak{e}_2)) + \\
& \quad 2 \times (26 + 13 \mathfrak{e}_1 + 5 \mathfrak{e}_1^2 + 2 \mu_2^2 (54 + 3 \mathfrak{e}_1 - 41 \mathfrak{e}_2) - 3 \mathfrak{e}_2 - \\
& \quad 5 \mathfrak{e}_1 \mathfrak{e}_2 + \mu_2 (127 + 24 \mathfrak{e}_1 + 5 \mathfrak{e}_1^2 - 11 \mathfrak{e}_2 - 5 \mathfrak{e}_1 \mathfrak{e}_2))) + \\
& 2 \eta (2 \times (17 + 2 \mu_2^2 + 15 \mathfrak{e}_1 + \mu_1^2 (25 + \mathfrak{e}_1) + \mu_2 (19 + 5 \mathfrak{e}_1) + \\
& \quad \mu_1 (42 + \mu_2 (31 - 19 \mathfrak{e}_1) + 16 \mathfrak{e}_1)) + \\
& \mathfrak{e}_p (5 + 4 \mathfrak{e}_1 + 15 \mathfrak{e}_1^2 + 4 \mu_2^2 (16 + 3 \mathfrak{e}_1 - 18 \mathfrak{e}_2) - 11 \mathfrak{e}_2 - \\
& \quad 15 \mathfrak{e}_1 \mathfrak{e}_2 + \mu_2 (82 + 21 \mathfrak{e}_1 + 15 \mathfrak{e}_1^2 - 29 \mathfrak{e}_2 - 15 \mathfrak{e}_1 \mathfrak{e}_2) + \mu_1^2 (9 + \\
& \quad \mathfrak{e}_1^2 - 9 \mathfrak{e}_2 + \mathfrak{e}_1 (11 + 4 \mathfrak{e}_2)) + \mu_1 (14 - 3 \mathfrak{e}_1 + 25 \mathfrak{e}_1^2 - 20 \mathfrak{e}_2 - \\
& \quad 20 \mathfrak{e}_1 \mathfrak{e}_2 + \mu_2 (94 + 15 \mathfrak{e}_1^2 - 23 \mathfrak{e}_2 + 3 \mathfrak{e}_1 (7 + \mathfrak{e}_2)))) + \\
& \times (-1 + \eta) \times (24 \eta^7 \mathfrak{e}_p (6 + 16 \mu_2 + \mathfrak{e}_1 + \mu_1 (6 + \mathfrak{e}_1)) - 4 \eta^6 \mathfrak{e}_p \\
& \quad (-18 - 99 \mu_1 - 81 \mu_1^2 + 22 \mu_2 - 82 \mu_1 \mu_2 + 140 \mu_2^2 - \\
& \quad 12 \mathfrak{e}_l (1 + \mu_1 + 4 \mu_2) + 2 \mathfrak{e}_1 - 31 \mu_1 \mathfrak{e}_1 - 15 \mu_1^2 \mathfrak{e}_1 + 30 \mu_1 \mu_2 \mathfrak{e}_1 + \\
& \quad 6 \eta \mathfrak{t} (4 + 8 \mu_2 + 2 \mathfrak{e}_l (1 + \mu_1 + 4 \mu_2) + \mathfrak{e}_1 + \mu_1 (4 + \mathfrak{e}_1))) + \eta \mathfrak{t} \\
& \mathfrak{e}_p (-((2 + \mu_2) \times (-3 + 4 \mu_2 - 5 \mathfrak{e}_1)) - 2 \mu_1^2 (-3 + \mathfrak{e}_1) + \\
& \quad \mu_1 (12 + 8 \mathfrak{e}_1 - \mu_2 (5 + 19 \mathfrak{e}_1))) + \eta^5 \\
& (4 \times (-1 + \eta \mathfrak{t}) \mathfrak{e}_l \mu_1 (9 + 28 \mu_2 + \mathfrak{e}_1 + \mu_1 (9 + \mathfrak{e}_1)) + \\
& \mathfrak{e}_p (2 \times (160 \mu_2^2 + 5 \times (-7 + \mathfrak{e}_1) + 3 \mu_1^2 (51 + 5 \mathfrak{e}_1) + \\
& \quad \mu_1 (118 + \mu_2 (353 - 13 \mathfrak{e}_1) + 44 \mathfrak{e}_1) + \mu_2 (-63 + 53 \mathfrak{e}_1)) + \\
& 4 \eta \mathfrak{t} (-7 \mu_2 + 70 \mu_2^2 - 4 \times (4 + \mathfrak{e}_1) + 4 \mu_1^2 (9 + \mathfrak{e}_1) + \mu_1 (20 + \mu_2 \\
& \quad (137 + 15 \mathfrak{e}_1))) + \mathfrak{e}_l (56 - 24 \mathfrak{e}_1 + 2 \mu_2 (83 + 5 \mathfrak{e}_1 + 24 \mathfrak{e}_2) + \\
& \quad \mu_1^2 (5 \mathfrak{e}_1^2 + 45 \times (6 + \mathfrak{e}_2) + \mathfrak{e}_1 (67 + 5 \mathfrak{e}_2)) + \mu_1 (326 + \\
& \quad 5 \mathfrak{e}_1^2 + 45 \mathfrak{e}_2 + 5 \mathfrak{e}_1 (23 + \mathfrak{e}_2) + 2 \mu_2 (303 + 45 \mathfrak{e}_1 + 70 \mathfrak{e}_2))) - \\
& \eta \mathfrak{t} \mathfrak{e}_l (56 - 24 \mathfrak{e}_1 + 2 \mu_2 (83 + 5 \mathfrak{e}_1 + 24 \mathfrak{e}_2) + \mu_1^2 \\
& \quad (5 \mathfrak{e}_1^2 + 45 \times (6 + \mathfrak{e}_2) + \mathfrak{e}_1 (67 + 5 \mathfrak{e}_2)) + \mu_1 (326 + 5 \mathfrak{e}_1^2 + \\
& \quad 45 \mathfrak{e}_2 + 5 \mathfrak{e}_1 (23 + \mathfrak{e}_2) + 2 \mu_2 (303 + 45 \mathfrak{e}_1 + 70 \mathfrak{e}_2))) - \\
& \eta^3 (\mathfrak{e}_p (92 + 4 \times (176 + 47 \eta \mathfrak{t}) \mu_2^2 + 44 \mathfrak{e}_1 + 44 \eta \mathfrak{t} \mathfrak{e}_1 + 4 \mu_1^2 \\
& \quad (81 + \eta \mathfrak{t} (72 - 11 \mathfrak{e}_1) + 7 \mathfrak{e}_1)) + \\
& \quad \mu_2 (420 + 21 \eta \mathfrak{t} + 124 \mathfrak{e}_1 + 11 \eta \mathfrak{t} \mathfrak{e}_1) + \mu_1 (416 + 868 \mu_2 + \\
& \quad 120 \mathfrak{e}_1 - 68 \mu_2 \mathfrak{e}_1 + 72 \eta \mathfrak{t} (4 + \mathfrak{e}_1) + 11 \eta \mathfrak{t} \mu_2 (87 + \mathfrak{e}_1))) + \\
& (-1 + \eta \mathfrak{t}) \mathfrak{e}_l (24 + 84 \mu_1^2 + 11 \mu_2 - 4 \mu_2^2 + 20 \mathfrak{e}_1 + 5 \mu_2 \mathfrak{e}_1 + \mu_1 \\
& \quad (108 + 107 \mu_2 + 56 \mathfrak{e}_1 - 19 \mu_2 \mathfrak{e}_1) + \mathfrak{e}_p (4 \mu_2^2 (106 + 9 \mathfrak{e}_1 - 79 \mathfrak{e}_2) + \\
& \quad 2 \mu_2 (279 + 10 \mathfrak{e}_1^2 + \mathfrak{e}_1 (55 - 10 \mathfrak{e}_2) - 14 \mathfrak{e}_2) + \\
& \quad 4 \times (28 + 5 \mathfrak{e}_1^2 + \mathfrak{e}_1 (14 - 5 \mathfrak{e}_2) - 2 \mathfrak{e}_2) + \mu_1^2 (290 + 17 \mathfrak{e}_1^2 + \\
& \quad 13 \mathfrak{e}_2 + \mathfrak{e}_1 (-17 + 9 \mathfrak{e}_2)) + \mu_1 (402 - 9 \mathfrak{e}_1 + 85 \mathfrak{e}_1^2 + 5 \mathfrak{e}_2 - \\
& \quad 59 \mathfrak{e}_1 \mathfrak{e}_2 + 2 \mu_2 (515 - 65 \mathfrak{e}_1 + 10 \mathfrak{e}_1^2 + 8 \mathfrak{e}_2 - 34 \mathfrak{e}_1 \mathfrak{e}_2)))) + \\
& \eta (\eta \mathfrak{t} \mathfrak{e}_p (46 - 36 \mu_2^2 + \mu_1^2 (38 - 18 \mathfrak{e}_1) + 50 \mathfrak{e}_1 + \mu_2 (17 + 15 \mathfrak{e}_1) + \\
& \quad \mu_1 (84 + \mu_2 (49 - 57 \mathfrak{e}_1) + 56 \mathfrak{e}_1)) + (-1 + \eta \mathfrak{t}) \mathfrak{e}_l \\
& \quad ((2 + \mu_2) \times (-3 + 4 \mu_2 - 5 \mathfrak{e}_1) + 2 \mu_1^2 (-3 + \mathfrak{e}_1) + \mu_1 (-12 +
\end{aligned}$$

$$\begin{aligned}
& 5 \mu_2 - 8 \mathfrak{e}_1 + 19 \mu_2 \mathfrak{e}_1) + 2 \mathfrak{e}_p (6 + 3 \mathfrak{e}_1 - 5 \mathfrak{e}_1^2 + 3 \mathfrak{e}_2 + 5 \mathfrak{e}_1 \mathfrak{e}_2 + \\
& \mu_2^2 (4 - 6 \mathfrak{e}_1 + 2 \mathfrak{e}_2) + \mu_2 (6 - 5 \mathfrak{e}_1 - 5 \mathfrak{e}_1^2 + 3 \mathfrak{e}_2 + 5 \mathfrak{e}_1 \mathfrak{e}_2) + \\
& \mu_1^2 (\mathfrak{e}_1^2 + 3 \times (2 + \mathfrak{e}_2) - \mathfrak{e}_1 (9 + \mathfrak{e}_2)) + \mu_1 (12 - 6 \mathfrak{e}_1 - 4 \mathfrak{e}_1^2 + \\
& 6 \mathfrak{e}_2 + 4 \mathfrak{e}_1 \mathfrak{e}_2 + \mu_2 (6 - 29 \mathfrak{e}_1 - 5 \mathfrak{e}_1^2 + 3 \mathfrak{e}_2 - 7 \mathfrak{e}_1 \mathfrak{e}_2))))) + \\
& \eta^4 (4 \times (-1 + \eta t) \mathfrak{e}_l (4 \mu_2 + \mu_1 (11 + 44 \mu_2 - 5 \mathfrak{e}_1) + \mu_1^2 (11 + \mathfrak{e}_1)) + \\
& \mathfrak{e}_p (4 \eta t (-14 \mu_2^2 + \mu_2 (63 - 4 \mathfrak{e}_1) + 6 \times (4 + \mathfrak{e}_1) + \\
& 4 \mu_1^2 (5 + \mathfrak{e}_1) + \mu_1 (44 - 14 \mathfrak{e}_1 + \mu_2 (79 + 17 \mathfrak{e}_1))) + \\
& 2 \times (27 + 632 \mu_2^2 + 39 \mathfrak{e}_1 + \mu_2 (343 + 23 \mathfrak{e}_1) - \mu_1^2 (99 + 37 \mathfrak{e}_1) + \\
& \mu_1 (-72 - 34 \mathfrak{e}_1 + \mu_2 (135 + 77 \mathfrak{e}_1))) + \mathfrak{e}_l (82 + 10 \mathfrak{e}_1 - \\
& 8 \mu_2^2 (-32 + 25 \mathfrak{e}_2) + \mu_2 (282 + 58 \mathfrak{e}_1 + 40 \mathfrak{e}_2) + \mu_1^2 (524 + \\
& 19 \mathfrak{e}_1^2 + 67 \mathfrak{e}_2 + 9 \mathfrak{e}_1 (5 + \mathfrak{e}_2)) + \mu_1 (606 + 115 \mathfrak{e}_1 + 49 \mathfrak{e}_1^2 + \\
& 67 \mathfrak{e}_2 - 21 \mathfrak{e}_1 \mathfrak{e}_2 - 2 \mu_2 (-693 + 27 \mathfrak{e}_1 - 88 \mathfrak{e}_2 + 30 \mathfrak{e}_1 \mathfrak{e}_2))) - \\
& \eta t \mathfrak{e}_l (82 + 10 \mathfrak{e}_1 - 8 \mu_2^2 (-32 + 25 \mathfrak{e}_2) + \mu_2 (282 + 58 \mathfrak{e}_1 + \\
& 40 \mathfrak{e}_2) + \mu_1^2 (524 + 19 \mathfrak{e}_1^2 + 67 \mathfrak{e}_2 + 9 \mathfrak{e}_1 (5 + \mathfrak{e}_2)) + \\
& \mu_1 (606 + 115 \mathfrak{e}_1 + 49 \mathfrak{e}_1^2 + 67 \mathfrak{e}_2 - 21 \mathfrak{e}_1 \mathfrak{e}_2 - \\
& 2 \mu_2 (-693 + 27 \mathfrak{e}_1 - 88 \mathfrak{e}_2 + 30 \mathfrak{e}_1 \mathfrak{e}_2))) - \\
& \eta^2 (\mathfrak{e}_p (4 \times (27 + 109 \mu_2 + 80 \mu_2^2 - 3 \mu_1^2 (-9 + \mathfrak{e}_1) + 15 \mathfrak{e}_1 + \\
& 7 \mu_2 \mathfrak{e}_1 + \mu_1 (54 + 109 \mu_2 + 12 \mathfrak{e}_1 + 19 \mu_2 \mathfrak{e}_1)) + \\
& \eta t (-12 + 23 \mu_2 - 4 \mu_2^2 - 7 \mu_2 \mathfrak{e}_1 + 4 \mu_1^2 (-5 + 14 \mathfrak{e}_1) + \\
& \mu_1 (-32 - 49 \mu_2 - 88 \mathfrak{e}_1 + 41 \mu_2 \mathfrak{e}_1))) + \\
& (-1 + \eta t) \mathfrak{e}_l (2 \times (-4 \mu_2^2 + \mu_1 \mu_2 (27 - 19 \mathfrak{e}_1) + 15 \times (1 + \mathfrak{e}_1) + \\
& 16 \mu_1 (3 + \mathfrak{e}_1) + \mu_2 (11 + 5 \mathfrak{e}_1) + \mu_1^2 (33 + 7 \mathfrak{e}_1)) + \\
& \mathfrak{e}_p (\mu_1^2 (24 + \mathfrak{e}_1^2 - 15 \mathfrak{e}_2 + \mathfrak{e}_1 (23 + 7 \mathfrak{e}_2)) + 2 \times \\
& (13 + 8 \mathfrak{e}_1 + 15 \mathfrak{e}_1^2 + 4 \mu_2^2 (20 + 6 \mathfrak{e}_1 - 15 \mathfrak{e}_2) - 7 \mathfrak{e}_2 - \\
& 15 \mathfrak{e}_1 \mathfrak{e}_2 + \mu_2 (119 + 36 \mathfrak{e}_1 + 15 \mathfrak{e}_1^2 - 13 \mathfrak{e}_2 - 15 \mathfrak{e}_1 \mathfrak{e}_2)) + \\
& \mu_1 (50 + 3 \mathfrak{e}_1 + 49 \mathfrak{e}_1^2 - 29 \mathfrak{e}_2 - 41 \mathfrak{e}_1 \mathfrak{e}_2 + \mu_2 \\
& (238 + 30 \mathfrak{e}_1^2 - 26 \mathfrak{e}_2 + 6 \mathfrak{e}_1 (12 + \mathfrak{e}_2)))))) - \\
& \eta \mathfrak{e}_p (4 \eta^7 (6 + 16 \mu_2 + \mathfrak{e}_1 + \mu_1 (6 + \mathfrak{e}_1)) - 2 \eta^6 (-10 - 37 \mu_1 - 27 \mu_1^2 - \\
& 24 \mu_1 \mu_2 + 56 \mu_2^2 - 4 \mathfrak{e}_l (1 + \mu_1 + 4 \mu_2) - 11 \mu_1 \mathfrak{e}_1 - 5 \mu_1^2 \mathfrak{e}_1 + \\
& 12 \mu_1 \mu_2 \mathfrak{e}_1 + 2 \eta t (4 + 8 \mu_2 + 2 \mathfrak{e}_l (1 + \mu_1 + 4 \mu_2) + \mathfrak{e}_1 + \mu_1 (4 + \mathfrak{e}_1))) + \\
& \eta t (2 - 16 \mu_2^2 - 2 \mu_1^2 (-1 + \mathfrak{e}_1) + 10 \mathfrak{e}_1 + \mu_2 (-21 + 5 \mathfrak{e}_1) + \\
& \mu_1 (4 + 8 \mathfrak{e}_1 - \mu_2 (21 + 19 \mathfrak{e}_1))) + \eta^5 \\
& (2 \times (-5 + 16 \mu_2^2 + \mathfrak{e}_1 + 4 \mu_1^2 (9 + \mathfrak{e}_1) + \mu_2 (-13 + 11 \mathfrak{e}_1) + \\
& \mu_1 (31 + \mu_2 (75 - 7 \mathfrak{e}_1) + 11 \mathfrak{e}_1)) + 4 \eta t \\
& (-4 - 3 \mu_2 + 14 \mu_2^2 - \mathfrak{e}_1 + \mu_1^2 (9 + \mathfrak{e}_1) + \mu_1 (5 + 3 \mu_2 (11 + \mathfrak{e}_1))) + \\
& \mathfrak{e}_l (\mu_1^2 (48 + \mathfrak{e}_1^2 + 9 \mathfrak{e}_2 + \mathfrak{e}_1 (13 + \mathfrak{e}_2)) + \\
& 2 \times (6 - 2 \mathfrak{e}_1 + \mu_2 (19 + \mathfrak{e}_1 + 4 \mathfrak{e}_2)) + \\
& \mu_1 (60 + \mathfrak{e}_1^2 + 9 \mathfrak{e}_2 + \mathfrak{e}_1 (21 + \mathfrak{e}_2) + 2 \mu_2 (55 + 9 \mathfrak{e}_1 + 14 \mathfrak{e}_2))) - \\
& \eta t \mathfrak{e}_l (\mu_1^2 (48 + \mathfrak{e}_1^2 + 9 \mathfrak{e}_2 + \mathfrak{e}_1 (13 + \mathfrak{e}_2)) + \\
& 2 \times (6 - 2 \mathfrak{e}_1 + \mu_2 (19 + \mathfrak{e}_1 + 4 \mathfrak{e}_2)) + \\
& \mu_1 (60 + \mathfrak{e}_1^2 + 9 \mathfrak{e}_2 + \mathfrak{e}_1 (21 + \mathfrak{e}_2) + 2 \mu_2 (55 + 9 \mathfrak{e}_1 + 14 \mathfrak{e}_2))) - \\
& \eta^3 (2 \times (7 + 72 \mu_2^2 + 3 \mathfrak{e}_1 + 4 \mu_1^2 (9 + \mathfrak{e}_1) + 5 \mu_2 (7 + 3 \mathfrak{e}_1) + \\
& \mu_1 (43 + \mu_2 (91 - 15 \mathfrak{e}_1) + 13 \mathfrak{e}_1)) -
\end{aligned}$$



$$\begin{aligned}
& \theta l \left( 30 + 15 \, \mathfrak{e}1 + 5 \, \mathfrak{e}1^2 + 4 \, \mu2^2 (26 + 3 \, \mathfrak{e}1 - 19 \, \mathfrak{e}2) - \mathfrak{e}2 - \right. \\
& \quad 5 \, \mathfrak{e}1 \, \mathfrak{e}2 + 2 \, \mu1^2 (37 + 2 \, \mathfrak{e}1^2 + \mathfrak{e}1 (-2 + \mathfrak{e}2) + 2 \, \mathfrak{e}2) + \\
& \quad \mu2 (152 + 31 \, \mathfrak{e}1 + 5 \, \mathfrak{e}1^2 - 3 \, \mathfrak{e}2 - 5 \, \mathfrak{e}1 \, \mathfrak{e}2) + \mu1 (104 - \mathfrak{e}1 + 21 \, \mathfrak{e}1^2 + \\
& \quad \quad 3 \, \mathfrak{e}2 - 15 \, \mathfrak{e}1 \, \mathfrak{e}2 + \mu2 (272 - 25 \, \mathfrak{e}1 + 5 \, \mathfrak{e}1^2 + 9 \, \mathfrak{e}2 - 17 \, \mathfrak{e}1 \, \mathfrak{e}2)) \Big) + \\
& \eta t \left( 4 + 108 \, \mu1 + 104 \, \mu1^2 - \mu2 + 279 \, \mu1 \, \mu2 + 40 \, \mu2^2 + 16 \, \mathfrak{e}1 + \right. \\
& \quad 32 \, \mu1 \, \mathfrak{e}1 - 8 \, \mu1^2 \, \mathfrak{e}1 + 5 \, \mu2 \, \mathfrak{e}1 - 7 \, \mu1 \, \mu2 \, \mathfrak{e}1 + \\
& \quad \theta l \left( 30 + 15 \, \mathfrak{e}1 + 5 \, \mathfrak{e}1^2 + 4 \, \mu2^2 (26 + 3 \, \mathfrak{e}1 - 19 \, \mathfrak{e}2) - \mathfrak{e}2 - 5 \, \mathfrak{e}1 \, \mathfrak{e}2 + \right. \\
& \quad \quad 2 \, \mu1^2 (37 + 2 \, \mathfrak{e}1^2 + \mathfrak{e}1 (-2 + \mathfrak{e}2) + 2 \, \mathfrak{e}2) + \mu2 (152 + 31 \, \mathfrak{e}1 + \\
& \quad \quad 5 \, \mathfrak{e}1^2 - 3 \, \mathfrak{e}2 - 5 \, \mathfrak{e}1 \, \mathfrak{e}2) + \mu1 (104 - \mathfrak{e}1 + 21 \, \mathfrak{e}1^2 + 3 \, \mathfrak{e}2 - \\
& \quad \quad 15 \, \mathfrak{e}1 \, \mathfrak{e}2 + \mu2 (272 - 25 \, \mathfrak{e}1 + 5 \, \mathfrak{e}1^2 + 9 \, \mathfrak{e}2 - 17 \, \mathfrak{e}1 \, \mathfrak{e}2)) \Big) \Big) - \\
& 2 \, \eta^4 \left( -8 + \mu1 + 9 \, \mu1^2 - 92 \, \mu2 - 68 \, \mu1 \, \mu2 - 160 \, \mu2^2 - 10 \, \mathfrak{e}1 + \right. \\
& \quad 3 \, \mu1 \, \mathfrak{e}1 + 7 \, \mu1^2 \, \mathfrak{e}1 - 8 \, \mu2 \, \mathfrak{e}1 - 20 \, \mu1 \, \mu2 \, \mathfrak{e}1 - \\
& \quad \theta l \left( 9 + \mathfrak{e}1 + \mu2 (32 + 6 \, \mathfrak{e}1 + 4 \, \mathfrak{e}2) - 4 \, \mu2^2 (-6 + 5 \, \mathfrak{e}2) + \right. \\
& \quad \quad \mu1^2 (55 + 2 \, \mathfrak{e}1^2 + 8 \, \mathfrak{e}2 + \mathfrak{e}1 (6 + \mathfrak{e}2)) + \mu1 (64 + 13 \, \mathfrak{e}1 + 5 \, \mathfrak{e}1^2 + \\
& \quad \quad 8 \, \mathfrak{e}2 - 2 \, \mathfrak{e}1 \, \mathfrak{e}2 - 2 \, \mu2 (-74 + \mathfrak{e}1 - 11 \, \mathfrak{e}2 + 3 \, \mathfrak{e}1 \, \mathfrak{e}2)) \Big) + \\
& \quad \eta t \left( -2 \times (4 - \mu2 (-13 + \mathfrak{e}1) + \mathfrak{e}1 + \mu1^2 (7 + \mathfrak{e}1) + \mu1 \right. \\
& \quad \quad (11 - 4 \, \mathfrak{e}1 + \mu2 (29 + 5 \, \mathfrak{e}1))) + \\
& \quad \theta l \left( 9 + \mathfrak{e}1 + \mu2 (32 + 6 \, \mathfrak{e}1 + 4 \, \mathfrak{e}2) - 4 \, \mu2^2 (-6 + 5 \, \mathfrak{e}2) + \right. \\
& \quad \quad \mu1^2 (55 + 2 \, \mathfrak{e}1^2 + 8 \, \mathfrak{e}2 + \mathfrak{e}1 (6 + \mathfrak{e}2)) + \mu1 (64 + 13 \, \mathfrak{e}1 + 5 \, \mathfrak{e}1^2 + \\
& \quad \quad 8 \, \mathfrak{e}2 - 2 \, \mathfrak{e}1 \, \mathfrak{e}2 - 2 \, \mu2 (-74 + \mathfrak{e}1 - 11 \, \mathfrak{e}2 + 3 \, \mathfrak{e}1 \, \mathfrak{e}2)) \Big) \Big) + \\
& \eta \left( \theta l \left( -2 - \mathfrak{e}1 + 5 \, \mathfrak{e}1^2 - \mathfrak{e}2 - 5 \, \mathfrak{e}1 \, \mathfrak{e}2 + 4 \, \mu2^2 (2 + 3 \, \mathfrak{e}1 + \mathfrak{e}2) + \right. \right. \\
& \quad \mu2 (10 + 13 \, \mathfrak{e}1 + 5 \, \mathfrak{e}1^2 + 5 \, \mathfrak{e}2 - 5 \, \mathfrak{e}1 \, \mathfrak{e}2) - \\
& \quad \mu1^2 (2 + \mathfrak{e}1^2 + \mathfrak{e}2 - \mathfrak{e}1 (11 + \mathfrak{e}2)) + \mu1 (-4 + 10 \, \mathfrak{e}1 + 4 \, \mathfrak{e}1^2 - \\
& \quad \quad 2 \, \mathfrak{e}2 - 4 \, \mathfrak{e}1 \, \mathfrak{e}2 + \mu2 (10 + 37 \, \mathfrak{e}1 + 5 \, \mathfrak{e}1^2 + 5 \, \mathfrak{e}2 + 7 \, \mathfrak{e}1 \, \mathfrak{e}2)) \Big) + \\
& \quad \eta t \left( 20 + 56 \, \mu1 + 36 \, \mu1^2 + 11 \, \mu2 + 35 \, \mu1 \, \mu2 - 16 \, \mu2^2 + 20 \, \mathfrak{e}1 + \right. \\
& \quad 24 \, \mu1 \, \mathfrak{e}1 + 4 \, \mu1^2 \, \mathfrak{e}1 + 5 \, \mu2 \, \mathfrak{e}1 - 19 \, \mu1 \, \mu2 \, \mathfrak{e}1 + \\
& \quad \theta l \left( 2 + \mathfrak{e}1 - 5 \, \mathfrak{e}1^2 + \mathfrak{e}2 + 5 \, \mathfrak{e}1 \, \mathfrak{e}2 - 4 \, \mu2^2 (2 + 3 \, \mathfrak{e}1 + \mathfrak{e}2) - \right. \\
& \quad \quad \mu2 (10 + 13 \, \mathfrak{e}1 + 5 \, \mathfrak{e}1^2 + 5 \, \mathfrak{e}2 - 5 \, \mathfrak{e}1 \, \mathfrak{e}2) + \\
& \quad \quad \mu1^2 (2 + \mathfrak{e}1^2 + \mathfrak{e}2 - \mathfrak{e}1 (11 + \mathfrak{e}2)) - \mu1 (-4 + 10 \, \mathfrak{e}1 + 4 \, \mathfrak{e}1^2 - 2 \, \mathfrak{e}2 - \\
& \quad \quad 4 \, \mathfrak{e}1 \, \mathfrak{e}2 + \mu2 (10 + 37 \, \mathfrak{e}1 + 5 \, \mathfrak{e}1^2 + 5 \, \mathfrak{e}2 + 7 \, \mathfrak{e}1 \, \mathfrak{e}2)) \Big) \Big) - \eta^2 \\
& \left( -2 \times (2 \times (-9 - 24 \, \mu2^2 + \mu1^2 (-9 + \mathfrak{e}1) - 5 \, \mathfrak{e}1 - 2 \, \mu2 (19 + \mathfrak{e}1) - \right. \\
& \quad \quad 2 \, \mu1 (9 + 2 \, \mathfrak{e}1 + \mu2 (19 + 4 \, \mathfrak{e}1))) + \\
& \quad \theta l \left( 7 + 4 \, \mathfrak{e}1 + 5 \, \mathfrak{e}1^2 + 4 \, \mu2^2 (8 + 3 \, \mathfrak{e}1 - 4 \, \mathfrak{e}2) - \mathfrak{e}2 - \right. \\
& \quad \quad 5 \, \mathfrak{e}1 \, \mathfrak{e}2 + \mu2 (52 + 17 \, \mathfrak{e}1 + 5 \, \mathfrak{e}1^2 + \mathfrak{e}2 - 5 \, \mathfrak{e}1 \, \mathfrak{e}2) + \\
& \quad \quad \mu1^2 (5 - 2 \, \mathfrak{e}2 + \mathfrak{e}1 (4 + \mathfrak{e}2)) + \mu1 (12 + 2 \, \mathfrak{e}1 + 8 \, \mathfrak{e}1^2 - 3 \, \mathfrak{e}2 - \\
& \quad \quad 7 \, \mathfrak{e}1 \, \mathfrak{e}2 + \mu2 (48 + 5 \, \mathfrak{e}1^2 - \mathfrak{e}2 + \mathfrak{e}1 (17 + \mathfrak{e}2))) \Big) + \\
& \quad \eta t \left( 2 - 2 \, \mu1^2 - \mu2 - 17 \, \mu1 \, \mu2 - 16 \, \mu2^2 + 10 \, \mathfrak{e}1 - 20 \, \mu1 \, \mathfrak{e}1 + 18 \, \mu1^2 \, \mathfrak{e}1 + \right. \\
& \quad \mu2 \, \mathfrak{e}1 + \mu1 \, \mu2 \, \mathfrak{e}1 + 2 \, \theta l \left( 7 + 4 \, \mathfrak{e}1 + 5 \, \mathfrak{e}1^2 + 4 \, \mu2^2 (8 + 3 \, \mathfrak{e}1 - 4 \, \mathfrak{e}2) - \right. \\
& \quad \quad \mathfrak{e}2 - 5 \, \mathfrak{e}1 \, \mathfrak{e}2 + \mu2 (52 + 17 \, \mathfrak{e}1 + 5 \, \mathfrak{e}1^2 + \mathfrak{e}2 - 5 \, \mathfrak{e}1 \, \mathfrak{e}2) + \\
& \quad \quad \mu1^2 (5 - 2 \, \mathfrak{e}2 + \mathfrak{e}1 (4 + \mathfrak{e}2)) + \mu1 (12 + 2 \, \mathfrak{e}1 + 8 \, \mathfrak{e}1^2 - 3 \, \mathfrak{e}2 - \\
& \quad \quad 7 \, \mathfrak{e}1 \, \mathfrak{e}2 + \mu2 (48 + 5 \, \mathfrak{e}1^2 - \mathfrak{e}2 + \mathfrak{e}1 (17 + \mathfrak{e}2))) \Big) \Big) + \\
& x^4 (-1 + \eta)^4 \left( -2 \times (-1 + \eta) \, \theta p \left( 25 + 79 \, \mu1 + 54 \, \mu1^2 + 95 \, \mu2 + 151 \, \mu1 \, \mu2 + \right. \right. \\
& \quad 152 \, \mu2^2 + 13 \, \mathfrak{e}1 + 21 \, \mu1 \, \mathfrak{e}1 + 2 \, \mu1^2 \, \mathfrak{e}1 + 19 \, \mu2 \, \mathfrak{e}1 + \mu1 \, \mu2 \, \mathfrak{e}1 +
\end{aligned}$$

$$\begin{aligned}
& 30 \eta^3 (6 + 16 \mu_2 + \mathfrak{e}1 + \mu_1 (6 + \mathfrak{e}1)) - 5 \eta^2 (2 \times (-9 - 4 \mu_2 + 28 \mu_2^2 + \mathfrak{e}1) - \\
& \quad 3 \mu_1^2 (27 + 5 \mathfrak{e}1) + 6 \eta t (4 + 8 \mu_2 + \mathfrak{e}1 + \mu_1 (4 + \mathfrak{e}1)) + \\
& \quad \mu_1 (-99 - 31 \mathfrak{e}1 + 4 \mu_2 (-28 + 3 \mathfrak{e}1))) + 2 \eta t (-4 + 14 \mu_2^2 - \\
& \quad \mu_2 (-2 + \mathfrak{e}1) - \mathfrak{e}1 + 2 \mu_1^2 (4 + \mathfrak{e}1) + \mu_1 (4 - 5 \mathfrak{e}1 + \mu_2 (30 + 8 \mathfrak{e}1))) + \\
& \quad \eta (37 + 55 \mu_2 + 120 \mu_2^2 + 7 \mathfrak{e}1 + 47 \mu_2 \mathfrak{e}1 + 45 \mu_1^2 (7 + \mathfrak{e}1) + \\
& \quad \mu_1 (352 + 583 \mu_2 + 112 \mathfrak{e}1 - 7 \mu_2 \mathfrak{e}1) + 2 \eta t (-55 \mu_2 + 70 \mu_2^2 - 10 \times \\
& \quad (4 + \mathfrak{e}1) + \mu_1^2 (9 + \mathfrak{e}1) + \mu_1 (-31 - 9 \mathfrak{e}1 + \mu_2 (53 + 15 \mathfrak{e}1)))) + \\
& (-1 + \eta t) \mathfrak{e}l (28 + 27 \mu_2 - 64 \eta \mu_2 + 8 \mu_2^2 + 20 \mathfrak{e}1 + 5 \mu_2 \mathfrak{e}1 - \\
& \quad 4 \mu_1^2 (7 \times (-1 + \mathfrak{e}1) + 4 \eta (5 + \mathfrak{e}1) + 4 \eta^2 (9 + \mathfrak{e}1)) - \\
& \quad \mu_1 (-56 + 80 \eta (1 + 4 \mu_2 - \mathfrak{e}1) - 52 \mathfrak{e}1 + \\
& \quad 16 \eta^2 (9 + 28 \mu_2 + \mathfrak{e}1) + \mu_2 (-107 + 19 \mathfrak{e}1)) + \\
& \mathfrak{e}p (22 + 102 \mu_2 + 112 \mu_2^2 + 120 \eta^3 (1 + \mu_1 + 4 \mu_2) + 11 \mathfrak{e}1 + \\
& \quad 17 \mu_2 \mathfrak{e}1 + 5 \mathfrak{e}1^2 + 5 \mu_2 \mathfrak{e}1^2 - 5 \mathfrak{e}2 - 19 \mu_2 \mathfrak{e}2 - 88 \mu_2^2 \mathfrak{e}2 - \\
& \quad 5 \mathfrak{e}1 \mathfrak{e}2 - 5 \mu_2 \mathfrak{e}1 \mathfrak{e}2 + \mu_1^2 (68 + 5 \mathfrak{e}1^2 + \mathfrak{e}2 + \mathfrak{e}1 (-5 + 3 \mathfrak{e}2)) + \\
& \quad 5 \eta^2 (\mu_1^2 (\mathfrak{e}1^2 + 9 \times (12 + \mathfrak{e}2) + \mathfrak{e}1 (17 + \mathfrak{e}2)) + \\
& \quad 2 \times (2 - 6 \mathfrak{e}1 + \mu_2 (-5 + \mathfrak{e}1 + 12 \mathfrak{e}2)) + \\
& \quad \mu_1 (112 + \mathfrak{e}1^2 + 9 \mathfrak{e}2 + \mathfrak{e}1 (41 + \mathfrak{e}2) + 2 \mu_2 (111 + 9 \mathfrak{e}1 + 14 \mathfrak{e}2))) + \\
& \quad \mu_1 (90 + 22 \mathfrak{e}1^2 - 4 \mathfrak{e}2 - 2 \mathfrak{e}1 (3 + 7 \mathfrak{e}2) + \mu_2 \\
& \quad (214 + 5 \mathfrak{e}1^2 - 11 \mathfrak{e}2 - \mathfrak{e}1 (55 + 17 \mathfrak{e}2))) + \\
& \quad 2 \eta (29 + 5 \mathfrak{e}1 + \mu_2 (84 + 26 \mathfrak{e}1 + 20 \mathfrak{e}2) - 4 \mu_2^2 (-38 + 25 \mathfrak{e}2) + \\
& \quad \mu_1^2 (223 + 8 \mathfrak{e}1^2 + 14 \mathfrak{e}2 + 3 \mathfrak{e}1 \mathfrak{e}2) + \mu_1 (252 + 35 \mathfrak{e}1 + 23 \mathfrak{e}1^2 + \\
& \quad 14 \mathfrak{e}2 - 12 \mathfrak{e}1 \mathfrak{e}2 + \mu_2 (552 + 22 \mathfrak{e}2 - 6 \mathfrak{e}1 (13 + 5 \mathfrak{e}2)))))) - \\
& x^3 (-1 + \eta)^3 (-((-1 + \eta) \mathfrak{e}p (80 \eta^4 (6 + 16 \mu_2 + \mathfrak{e}1 + \mu_1 (6 + \mathfrak{e}1)) + \\
& \quad \eta t (4 \mu_2^2 - 4 \times (6 + 5 \mathfrak{e}1) - \mu_2 (7 + 9 \mathfrak{e}1) + \\
& \quad 4 \mu_1^2 (4 + 11 \mathfrak{e}1) + \mu_1 (-8 - 31 \mu_2 - 48 \mathfrak{e}1 + 39 \mu_2 \mathfrak{e}1)) - \\
& \quad 40 \eta^3 (2 \times (-5 - 5 \mu_2 + 14 \mu_2^2) - \mu_1^2 (27 + 5 \mathfrak{e}1) + \mu_1 (-37 - \\
& \quad 34 \mu_2 - 11 \mathfrak{e}1 + 6 \mu_2 \mathfrak{e}1) + 2 \eta t (4 + 8 \mu_2 + \mathfrak{e}1 + \mu_1 (4 + \mathfrak{e}1))) + \\
& \quad 4 \times (9 + 32 \mu_2^2 - \mu_1^2 (-9 + \mathfrak{e}1) + 5 \mathfrak{e}1 + 3 \mu_2 (11 + \mathfrak{e}1) + \\
& \quad \mu_1 (18 + 4 \mathfrak{e}1 + 3 \mu_2 (11 + \mathfrak{e}1))) + \\
& \quad 8 \eta (25 + 99 \mu_2 + 144 \mu_2^2 + 13 \mathfrak{e}1 + 19 \mu_2 \mathfrak{e}1 + 2 \mu_1^2 (27 + \mathfrak{e}1) + \\
& \quad \mu_1 (79 + 21 \mathfrak{e}1 + \mu_2 (155 + \mathfrak{e}1)) + 2 \eta t (-4 + 2 \mu_2 + 14 \mu_2^2 - \mathfrak{e}1 - \\
& \quad \mu_2 \mathfrak{e}1 + 2 \mu_1^2 (5 + \mathfrak{e}1) + \mu_1 (6 + 38 \mu_2 - 5 \mathfrak{e}1 + 8 \mu_2 \mathfrak{e}1))) + \\
& \quad 4 \eta^2 (49 + 65 \mu_2 + 40 \mu_2^2 + 9 \mathfrak{e}1 + 49 \mu_2 \mathfrak{e}1 + 45 \mu_1^2 (7 + \mathfrak{e}1) + \\
& \quad \mu_1 (364 + 561 \mu_2 + 114 \mathfrak{e}1 - 29 \mu_2 \mathfrak{e}1) + \\
& \quad 2 \eta t (-55 \mu_2 + 70 \mu_2^2 - 10 \times (4 + \mathfrak{e}1) + 2 \mu_1^2 (9 + \mathfrak{e}1) + \\
& \quad \mu_1 (-22 - 8 \mathfrak{e}1 + 3 \mu_2 (27 + 5 \mathfrak{e}1)))))) + (-1 + \eta t) \mathfrak{e}l \\
& (160 \eta^4 \mathfrak{e}p (1 + \mu_1 + 4 \mu_2) + 2 \times (19 + 8 \mu_2^2 + \mu_1^2 (17 - 5 \mathfrak{e}1) + \\
& \quad 15 \mathfrak{e}1 + \mu_2 (27 + 5 \mathfrak{e}1) + \mu_1 (36 + 35 \mu_2 + 16 \mathfrak{e}1 - 19 \mu_2 \mathfrak{e}1)) + \\
& \quad \mathfrak{e}p (\mu_1^2 (4 + \mathfrak{e}1^2 - 7 \mathfrak{e}2 + \mathfrak{e}1 (7 + 3 \mathfrak{e}2)) - 2 \times (1 - 5 \mathfrak{e}1^2 + \\
& \quad 5 \mathfrak{e}2 + 5 \mathfrak{e}1 \mathfrak{e}2 + 4 \mu_2^2 (-4 + 7 \mathfrak{e}2) + \\
& \quad \mu_2 (-15 - 2 \mathfrak{e}1 - 5 \mathfrak{e}1^2 + 15 \mathfrak{e}2 + 5 \mathfrak{e}1 \mathfrak{e}2)) + \mu_1 (2 - 5 \mathfrak{e}1 + 17 \mathfrak{e}1^2 - \\
& \quad 17 \mathfrak{e}2 - 13 \mathfrak{e}1 \mathfrak{e}2 + 2 \mu_2 (23 + 5 \mathfrak{e}1^2 - 11 \mathfrak{e}2 + \mathfrak{e}1 (2 + \mathfrak{e}2)))) + \\
& \quad 2 \eta^3 (-12 \mu_1 (9 + 28 \mu_2 + \mathfrak{e}1 + \mu_1 (9 + \mathfrak{e}1)) + 5 \mathfrak{e}p (8 - 8 \mathfrak{e}1 +
\end{aligned}$$

$$\begin{aligned}
& 2 \mu_2 (7 + \mathfrak{e}1 + 8 \mathfrak{e}2) + \mu_1^2 (78 + \mathfrak{e}1^2 + 9 \mathfrak{e}2 + \mathfrak{e}1 (15 + \mathfrak{e}2)) + \\
& \mu_1 (86 + \mathfrak{e}1^2 + 9 \mathfrak{e}2 + \mathfrak{e}1 (31 + \mathfrak{e}2) + 2 \mu_2 (83 + 9 \mathfrak{e}1 + 14 \mathfrak{e}2))) + \\
& 2 \eta^2 (-12 \times (4 \mu_2 + \mu_1 (7 + 28 \mu_2 - 5 \mathfrak{e}1) + \mu_1^2 (7 + \mathfrak{e}1)) + \\
& \mathfrak{e}p (66 + 10 \mathfrak{e}1 - 8 \mu_2^2 (-36 + 25 \mathfrak{e}2) + \mu_2 (206 + 54 \mathfrak{e}1 + 40 \mathfrak{e}2) + \\
& \mu_1^2 (472 + 17 \mathfrak{e}1^2 + 41 \mathfrak{e}2 + \mathfrak{e}1 (15 + 7 \mathfrak{e}2)) + \\
& \mu_1 (538 + 85 \mathfrak{e}1 + 47 \mathfrak{e}1^2 + 41 \mathfrak{e}2 - 23 \mathfrak{e}1 \mathfrak{e}2 - \\
& 2 \mu_2 (-599 + 61 \mathfrak{e}1 - 44 \mathfrak{e}2 + 30 \mathfrak{e}1 \mathfrak{e}2))) + \\
& \eta (80 + 65 \mu_2 + 12 \mu_2^2 + 60 \mathfrak{e}1 + 15 \mu_2 \mathfrak{e}1 - 28 \mu_1^2 (-5 + 2 \mathfrak{e}1) + \\
& \mu_1 (220 + 321 \mu_2 + 160 \mathfrak{e}1 - 57 \mu_2 \mathfrak{e}1) + \\
& \mathfrak{e}p (4 \mu_2^2 (110 + 3 \mathfrak{e}1 - 85 \mathfrak{e}2) + \mu_2 (458 + 20 \mathfrak{e}1^2 + \mathfrak{e}1 (82 - 20 \mathfrak{e}2) - \\
& 60 \mathfrak{e}2) + 4 \times (24 + 12 \mathfrak{e}1 + 5 \mathfrak{e}1^2 - 4 \mathfrak{e}2 - 5 \mathfrak{e}1 \mathfrak{e}2) + \\
& \mu_1^2 (278 + 19 \mathfrak{e}1^2 + 7 \mathfrak{e}2 + \mathfrak{e}1 (-19 + 11 \mathfrak{e}2)) + \\
& \mu_1 (374 + 87 \mathfrak{e}1^2 - 9 \mathfrak{e}2 - 19 \mathfrak{e}1 (1 + 3 \mathfrak{e}2) + \\
& 2 \mu_2 (457 + 10 \mathfrak{e}1^2 - 12 \mathfrak{e}2 - \mathfrak{e}1 (95 + 34 \mathfrak{e}2)))))) - \\
& w (\times (-1 + \eta) - \eta) (-1 + \eta) \times (2 x^7 (-1 + \eta)^7 \mathfrak{e}p (-20 + 11 \eta t + 20 \mathfrak{e}l - \\
& 59 \mu_1 + 11 \eta t \mu_1 + 35 \mathfrak{e}l \mu_1 - 39 \mu_1^2 + 15 \mathfrak{e}l \mu_1^2 - 60 \\
& \mu_2 + 20 \eta t \mu_2 + 60 \mathfrak{e}l \mu_2 - 60 \mu_1 \mu_2 + 28 \mathfrak{e}l \mu_1 \mu_2 + 3 \eta t \\
& \mathfrak{e}1 - 15 \mu_1 \mathfrak{e}1 + 3 \eta t \mu_1 \mathfrak{e}1 + 7 \mathfrak{e}l \mu_1 \mathfrak{e}1 - 9 \mu_1^2 \mathfrak{e}1 + \mathfrak{e}l \\
& \mu_1^2 \mathfrak{e}1 + \eta^2 (11 + 20 \mu_2 + 3 \mathfrak{e}1 + \mu_1 (11 + 3 \mathfrak{e}1)) + \eta \\
& (9 + 40 \mu_2 - 3 \mathfrak{e}1 + 12 \mu_1 (4 + 5 \mu_2 + \mathfrak{e}1) + \mu_1^2 (39 + 9 \mathfrak{e}1) - \\
& \eta t (11 + 20 \mu_2 + 3 \mathfrak{e}1 + \mu_1 (11 + 3 \mathfrak{e}1))) + 4 \mathfrak{e}l \mu_2 \mathfrak{e}2 - \eta t \mathfrak{e}l \\
& (20 + \mu_1^2 (15 + \mathfrak{e}1) + 7 \mu_1 (5 + 4 \mu_2 + \mathfrak{e}1) + 4 \mu_2 (15 + \mathfrak{e}2))) + \\
& x^4 (-1 + \eta)^4 (-((-1 + \eta) \mathfrak{e}p (70 \eta^4 (11 + 20 \mu_2 + 3 \mathfrak{e}1 + \mu_1 (11 + 3 \mathfrak{e}1)) - \\
& 10 \eta^3 (-314 - 738 \mu_2 + 252 \mu_2^2 - 36 \mathfrak{e}1 - 21 \mu_1^2 (13 + 3 \mathfrak{e}1) + \\
& 7 \eta t (11 + 20 \mu_2 + 3 \mathfrak{e}1 + \mu_1 (11 + 3 \mathfrak{e}1)) + \\
& \mu_1 (-587 - 141 \mathfrak{e}1 + 6 \mu_2 (-55 + 9 \mathfrak{e}1))) + \\
& 2 \times (93 + 456 \mu_2^2 + 49 \mathfrak{e}1 + 4 \mu_1^2 (45 + \mathfrak{e}1) + \mu_2 (383 + 63 \mathfrak{e}1) + \\
& \mu_1 (273 + 71 \mathfrak{e}1 + \mu_2 (551 + 9 \mathfrak{e}1))) + \\
& \eta t (180 \mu_2^2 - 24 \times (5 + 3 \mathfrak{e}1) - \mu_2 (37 + 31 \mathfrak{e}1) + 4 \mu_1^2 \\
& (36 + 35 \mathfrak{e}1) + \mu_1 (24 - 172 \mathfrak{e}1 + \mu_2 (323 + 173 \mathfrak{e}1))) + \\
& 10 \eta^2 (239 + 552 \mu_2 - 180 \mu_2^2 + 27 \mathfrak{e}1 + 62 \mu_2 \mathfrak{e}1 + \mu_1^2 \\
& (531 + 93 \mathfrak{e}1) + \mu_1 (770 + 844 \mu_2 + 210 \mathfrak{e}1 - 76 \mu_2 \mathfrak{e}1) + \\
& 2 \eta t (3 \times (-23 - 34 \mu_2 + 28 \mu_2^2 - 6 \mathfrak{e}1) + \mu_1^2 (9 + \mathfrak{e}1) + \\
& \mu_1 (-60 + 58 \mu_2 - 17 \mathfrak{e}1 + 18 \mu_2 \mathfrak{e}1))) + \\
& 2 \eta (481 + 1561 \mu_2 + 1536 \mu_2^2 + 171 \mathfrak{e}1 + 357 \mu_2 \mathfrak{e}1 + \\
& 30 \mu_1^2 (47 + 5 \mathfrak{e}1) + \mu_1 (1891 + 3145 \mu_2 + 531 \mathfrak{e}1 - 141 \mu_2 \mathfrak{e}1) + \\
& \eta t (\mu_1^2 (290 + 42 \mathfrak{e}1) + 5 \times (-59 - 46 \mu_2 + 140 \mu_2^2 - 15 \mathfrak{e}1 - \\
& 4 \mu_2 \mathfrak{e}1) + \mu_1 (-5 + 1254 \mu_2 - 153 \mathfrak{e}1 + 250 \mu_2 \mathfrak{e}1)))) + \\
& (-1 + \eta t) \mathfrak{e}l (2 \times (68 - 12 \mu_2^2 + \mu_1^2 (88 - 36 \mathfrak{e}1) + 60 \mathfrak{e}1 + \mu_2 \\
& (49 + 15 \mathfrak{e}1) + \mu_1 (156 + 161 \mu_2 + 102 \mathfrak{e}1 - 69 \mu_2 \mathfrak{e}1)) + \\
& \mathfrak{e}p (50 + 25 \mathfrak{e}1 + 35 \mathfrak{e}1^2 + 4 \mu_2^2 (66 + 9 \mathfrak{e}1 - 65 \mathfrak{e}2) + \\
& \mu_2 (350 + 35 \mathfrak{e}1^2 + \mathfrak{e}1 (91 - 35 \mathfrak{e}2) - 53 \mathfrak{e}2) - 23 \mathfrak{e}2 - \\
& 35 \mathfrak{e}1 \mathfrak{e}2 + 2 \mu_1 (115 + \mathfrak{e}1 + 39 \mathfrak{e}1^2 - 16 \mathfrak{e}2 - 31 \mathfrak{e}1 \mathfrak{e}2) +
\end{aligned}$$

$$\begin{aligned}
& \mu_1^2 (180 + 13 \mu_1 + 7 \mu_1^2 - 9 \mu_2 + 9 \mu_1 \mu_2) + \\
& \mu_1 \mu_2 (718 + 35 \mu_1^2 - 13 \mu_2 - \mu_1 (37 + 23 \mu_2)) + 5 \eta^3 (-8 \mu_1 \\
& (9 + 28 \mu_2 + \mu_1 + \mu_1 (9 + \mu_1)) + \theta p (352 + 2 \mu_2 (561 + 3 \mu_1 + 28 \mu_2) + \\
& \mu_1^2 (264 + 47 \mu_1 + 3 \mu_1^2 + 27 \mu_2 + 3 \mu_1 \mu_2) + \mu_1 (616 + 131 \mu_1 + \\
& 3 \mu_1^2 + 27 \mu_2 + 3 \mu_1 \mu_2 + \mu_2 (554 + 54 \mu_1 + 84 \mu_2))) + \\
& \eta (4 \times (81 + 15 \mu_2^2 + \mu_1^2 (24 - 69 \mu_1) + 60 \mu_1 + \mu_2 (53 + 15 \mu_1) + \\
& \mu_1 (105 - 71 \mu_2 + 177 \mu_1 - 57 \mu_2 \mu_1)) + \\
& \theta p (518 + 117 \mu_1 + 75 \mu_1^2 + 4 \mu_2^2 (338 + 9 \mu_1 - 321 \mu_2) - 63 \mu_2 - \\
& 75 \mu_1 \mu_2 + \mu_2 (2122 + 343 \mu_1 + 75 \mu_1^2 - 77 \mu_2 - 75 \mu_1 \mu_2) + \\
& \mu_1^2 (1784 + 65 \mu_1^2 + 97 \mu_2 + \mu_1 (27 + 35 \mu_2)) + \\
& \mu_1 (2302 + 204 \mu_1 + 320 \mu_1^2 + 34 \mu_2 - 220 \mu_1 \mu_2 + \\
& \mu_2 (5306 - 617 \mu_1 + 75 \mu_1^2 + 243 \mu_2 - 255 \mu_1 \mu_2))) + \\
& 2 \eta^2 (-16 \times (10 \mu_2 + 2 \mu_1 (15 + 58 \mu_2 - 6 \mu_1) + 3 \mu_1^2 (10 + \mu_1)) + \\
& 5 \theta p (\mu_1^2 (347 + 10 \mu_1^2 + 34 \mu_2 + \mu_1 (21 + 4 \mu_2)) + \\
& 2 \times (6 \times (15 + \mu_1) + \mu_2^2 (76 - 60 \mu_2) + \mu_2 (291 + 19 \mu_1 + 18 \mu_2)) + \\
& \mu_1 (527 + 87 \mu_1 + 28 \mu_1^2 + 34 \mu_2 - 14 \mu_1 \mu_2 + \\
& \mu_2 (886 - 62 \mu_1 + 92 \mu_2 - 36 \mu_1 \mu_2))) - \\
& x^6 (-1 + \eta)^6 (4 \times (-1 + \eta t) \theta l (8 \mu_2 + \mu_1^2 (2 \times (7 + \mu_1) + \eta (9 + \mu_1)) + \\
& \mu_1 (2 \times (7 + 28 \mu_2 - 5 \mu_1) + \eta (9 + 28 \mu_2 + \mu_1)) + \theta p \\
& (14 \eta^3 (11 + 20 \mu_2 + 3 \mu_1 + \mu_1 (11 + 3 \mu_1)) - 2 \eta^2 (-121 - 386 \mu_2 + 84 \mu_2^2 + \\
& 9 \mu_1 - 21 \mu_1^2 (13 + 3 \mu_1) + 2 \mu_1 (-197 - 195 \mu_2 - 48 \mu_1 + 9 \mu_2 \mu_1) + \\
& 7 \eta t (11 + 20 \mu_2 + 3 \mu_1 + \mu_1 (11 + 3 \mu_1))) + \\
& \eta (-4 \times (73 - 62 \mu_2^2 + \mu_2 (191 - 10 \mu_1) + 4 \mu_1 + 16 \mu_1^2 (3 + \mu_1) + \\
& \mu_1 (121 + \mu_2 (39 - 7 \mu_1) + 26 \mu_1)) + 2 \eta t (31 + 72 \mu_2 + 56 \mu_2^2 + \\
& 9 \mu_1 + \mu_1 (31 + 9 \mu_1 + 4 \mu_2 (5 + 3 \mu_1))) + \theta l (304 + 2 \mu_2 \\
& (467 + \mu_1 + 28 \mu_2) + \mu_1^2 (228 + \mu_1^2 + 9 \mu_2 + \mu_1 (25 + \mu_2)) + \mu_1 \\
& (532 + \mu_1^2 + 9 \mu_2 + \mu_1 (109 + \mu_2) + 2 \mu_2 (223 + 9 \mu_1 + 14 \mu_2))) - \\
& \eta t \theta l (304 + 2 \mu_2 (467 + \mu_1 + 28 \mu_2) + \mu_1^2 (228 + \mu_1^2 + \\
& 9 \mu_2 + \mu_1 (25 + \mu_2)) + \mu_1 (532 + \mu_1^2 + 9 \mu_2 + \\
& \mu_1 (109 + \mu_2) + 2 \mu_2 (223 + 9 \mu_1 + 14 \mu_2))) - \\
& 2 \times (52 + 229 \mu_1 + 177 \mu_1^2 + 144 \mu_2 + 312 \mu_1 \mu_2 + 40 \mu_2^2 + \\
& 4 \mu_1 + 65 \mu_1 \mu_1 + 31 \mu_1^2 \mu_1 + 20 \mu_2 \mu_1 - 4 \mu_1 \mu_2 \mu_1 - \\
& \theta l (\mu_1^2 (107 + 3 \mu_1^2 + 7 \mu_2 + \mu_1 (2 + \mu_2)) + 4 \times (13 + \mu_1 + \\
& \mu_2 (40 + 3 \mu_1 + 3 \mu_2) - 2 \mu_2^2 (-7 + 5 \mu_2)) + \mu_1 (159 + 24 \mu_1 + \\
& 9 \mu_1^2 + 7 \mu_2 - 5 \mu_1 \mu_2 - 4 \mu_2 (-66 + 8 \mu_1 - 4 \mu_2 + 3 \mu_1 \mu_2))) + \\
& \eta t (-46 - 68 \mu_2 + 56 \mu_2^2 - 12 \mu_1 + 2 \mu_1 (-23 - 6 \mu_1 + \\
& 2 \mu_2 (5 + 3 \mu_1)) + \theta l \mu_1^2 (107 + 3 \mu_1^2 + 7 \mu_2 + \mu_1 (2 + \mu_2)) + \\
& 4 \theta l (13 + \mu_1 + \mu_2 (40 + 3 \mu_1 + 3 \mu_2) - 2 \mu_2^2 (-7 + 5 \mu_2)) + \\
& \theta l \mu_1 (159 + 24 \mu_1 + 9 \mu_1^2 + 7 \mu_2 - 5 \mu_1 \mu_2 - \\
& 4 \mu_2 (-66 + 8 \mu_1 - 4 \mu_2 + 3 \mu_1 \mu_2))) + \\
& x^5 (-1 + \eta)^5 (2 \times (-1 + \eta) \theta p (89 + 371 \mu_1 + 282 \mu_1^2 + 299 \mu_2 + \\
& 635 \mu_1 \mu_2 + 368 \mu_2^2 + 33 \mu_1 + 105 \mu_1 \mu_1 + 30 \mu_1^2 \mu_1 + 71 \mu_2 \mu_1 - \\
& 19 \mu_1 \mu_2 \mu_1 + 21 \eta^3 (11 + 20 \mu_2 + 3 \mu_1 + \mu_1 (11 + 3 \mu_1)) -
\end{aligned}$$

$$\begin{aligned}
& 3 \eta^2 \left( \mu_1 (-529 + 36 \mu_2 (-10 + \mathfrak{e}_1) - 129 \mathfrak{e}_1) + \right. \\
& \quad 8 \times (-32 - 79 \mu_2 + 21 \mu_2^2 - 3 \mathfrak{e}_1) - 21 \mu_1^2 (13 + 3 \mathfrak{e}_1) + \\
& \quad \left. 7 \eta t (11 + 20 \mu_2 + 3 \mathfrak{e}_1 + \mu_1 (11 + 3 \mathfrak{e}_1)) \right) + \\
& \eta t \left( -59 + 140 \mu_2^2 - 15 \mathfrak{e}_1 + 8 \mu_1^2 (6 + \mathfrak{e}_1) - 2 \mu_2 (23 + 2 \mathfrak{e}_1) + \right. \\
& \quad \left. \mu_1 (-11 - 31 \mathfrak{e}_1 + \mu_2 (214 + 50 \mathfrak{e}_1)) \right) + \\
& \eta \left( 395 + 984 \mu_2 - 60 \mu_2^2 + 39 \mathfrak{e}_1 + 122 \mu_2 \mathfrak{e}_1 + 6 \mu_1^2 (177 + 31 \mathfrak{e}_1) + \right. \\
& \quad \mu_1 (1457 + 1780 \mu_2 + 405 \mathfrak{e}_1 - 88 \mu_2 \mathfrak{e}_1) + \\
& \quad 2 \eta t \left( 6 \times (-23 - 34 \mu_2 + 28 \mu_2^2 - 6 \mathfrak{e}_1) + \mu_1^2 (9 + \mathfrak{e}_1) + \right. \\
& \quad \left. \mu_1 (-129 + 88 \mu_2 - 35 \mathfrak{e}_1 + 36 \mu_2 \mathfrak{e}_1) \right) \Big) - \\
& (-1 + \eta t) \mathfrak{e}_l \left( 84 + 65 \mu_2 - 160 \eta \mu_2 + 24 \mu_2^2 + 60 \mathfrak{e}_1 + 15 \mu_2 \mathfrak{e}_1 - \right. \\
& \quad \mu_1 (-92 - 17 \mu_2 + 4 \eta (95 + 372 \mu_2 - 49 \mathfrak{e}_1) - \\
& \quad \left. 176 \mathfrak{e}_1 + 57 \mu_2 \mathfrak{e}_1 + 20 \eta^2 (9 + 28 \mu_2 + \mathfrak{e}_1)) \right) - \\
& 4 \mu_1^2 (-2 + 22 \mathfrak{e}_1 + 5 \eta^2 (9 + \mathfrak{e}_1) + \eta (95 + 11 \mathfrak{e}_1)) + \\
& \mathfrak{e}_p \left( 94 + 378 \mu_2 + 272 \mu_2^2 + 21 \mathfrak{e}_1 + 59 \mu_2 \mathfrak{e}_1 + 15 \mathfrak{e}_1^2 + \right. \\
& \quad 15 \mu_2 \mathfrak{e}_1^2 - 15 \mathfrak{e}_2 - 25 \mu_2 \mathfrak{e}_2 - 264 \mu_2^2 \mathfrak{e}_2 - 15 \mathfrak{e}_1 \mathfrak{e}_2 - \\
& \quad 15 \mu_2 \mathfrak{e}_1 \mathfrak{e}_2 + \mu_1^2 (344 + 13 \mathfrak{e}_1^2 + 13 \mathfrak{e}_2 + \mathfrak{e}_1 (-1 + 7 \mathfrak{e}_2)) \Big) + \\
& 6 \eta^2 \left( \mu_1^2 (123 + \mathfrak{e}_1^2 + 9 \mathfrak{e}_2 + \mathfrak{e}_1 (18 + \mathfrak{e}_2)) \right) + \\
& \quad 2 \times (82 + \mu_2 (257 + \mathfrak{e}_1 + 14 \mathfrak{e}_2)) + \mu_1 \\
& \quad \left( 287 + \mathfrak{e}_1^2 + 9 \mathfrak{e}_2 + \mathfrak{e}_1 (60 + \mathfrak{e}_2) + 2 \mu_2 (125 + 9 \mathfrak{e}_1 + 14 \mathfrak{e}_2) \right) \Big) + \\
& \mu_1 \left( 438 + 64 \mathfrak{e}_1^2 + \mathfrak{e}_1 (32 - 44 \mathfrak{e}_2) - 2 \mathfrak{e}_2 + \mu_2 \right. \\
& \quad \left. (1002 + 15 \mathfrak{e}_1^2 + 23 \mathfrak{e}_2 - \mathfrak{e}_1 (149 + 51 \mathfrak{e}_2)) \right) \Big) + \\
& 2 \eta \left( 24 \times (14 + \mathfrak{e}_1) - 80 \mu_2^2 (-4 + 3 \mathfrak{e}_2) + 2 \mu_2 (531 + 37 \mathfrak{e}_1 + \right. \\
& \quad \left. 36 \mathfrak{e}_2) + \mu_1^2 (668 + 19 \mathfrak{e}_1^2 + 55 \mathfrak{e}_2 + \mathfrak{e}_1 (27 + 7 \mathfrak{e}_2)) \right) + \\
& \mu_1 \left( 1004 + 159 \mathfrak{e}_1 + 55 \mathfrak{e}_1^2 + 55 \mathfrak{e}_2 - 29 \mathfrak{e}_1 \mathfrak{e}_2 - \right. \\
& \quad \left. 2 \mu_2 (-839 + 79 \mathfrak{e}_1 - 70 \mathfrak{e}_2 + 36 \mathfrak{e}_1 \mathfrak{e}_2) \right) \Big) \Big) + \\
& x^2 (-1 + \eta)^2 \left( - \left( (-1 + \eta) \mathfrak{e}_p \left( 42 \eta^6 (11 + 20 \mu_2 + 3 \mathfrak{e}_1 + \mu_1 (11 + 3 \mathfrak{e}_1)) + \right. \right. \right. \\
& \quad \eta t (-10 + 207 \mu_2 + 204 \mu_2^2 - 70 \mathfrak{e}_1 - 76 \mu_1 \mathfrak{e}_1 - \\
& \quad \left. 15 \mu_2 \mathfrak{e}_1 + 2 \mu_1^2 (5 + 21 \mathfrak{e}_1) + 3 \mu_1 \mu_2 (69 + 35 \mathfrak{e}_1)) \right) - \\
& 6 \eta^5 \left( \mu_1 (-703 + 90 \mu_2 (-3 + \mathfrak{e}_1) - 165 \mathfrak{e}_1) + 10 \times \right. \\
& \quad \left( -43 - 95 \mu_2 + 42 \mu_2^2 - 6 \mathfrak{e}_1) - 21 \mu_1^2 (13 + 3 \mathfrak{e}_1) + \right. \\
& \quad \left. 7 \eta t (11 + 20 \mu_2 + 3 \mathfrak{e}_1 + \mu_1 (11 + 3 \mathfrak{e}_1)) \right) \Big) + \\
& 10 \eta^4 \left( 322 + 672 \mu_2 - 480 \mu_2^2 + 42 \mathfrak{e}_1 + 64 \mu_2 \mathfrak{e}_1 + \right. \\
& \quad \mu_1^2 (531 + 93 \mathfrak{e}_1) + \mu_1 (853 + 752 \mu_2 + 225 \mathfrak{e}_1 - 140 \mu_2 \mathfrak{e}_1) + \\
& \quad 2 \eta t \left( 3 \times (-23 - 34 \mu_2 + 28 \mu_2^2 - 6 \mathfrak{e}_1) + 2 \mu_1^2 (9 + \mathfrak{e}_1) + \right. \\
& \quad \left. \mu_1 (-51 + 86 \mu_2 - 16 \mathfrak{e}_1 + 18 \mu_2 \mathfrak{e}_1) \right) \Big) \Big) + \\
& 6 \eta^2 \left( 2 \times \left( 93 + 404 \mu_2 + 416 \mu_2^2 + 49 \mathfrak{e}_1 + 62 \mu_2 \mathfrak{e}_1 + 4 \mu_1^2 \right. \right. \\
& \quad \left. \left. (45 + \mathfrak{e}_1) + \mu_1 (273 + 572 \mu_2 + 71 \mathfrak{e}_1 + 14 \mu_2 \mathfrak{e}_1) \right) \right) + \\
& \quad \eta t \left( -114 - 13 \mu_2 + 198 \mu_2^2 - 72 \mathfrak{e}_1 - 31 \mu_2 \mathfrak{e}_1 + 2 \mu_1^2 \right. \\
& \quad \left. (56 + 51 \mathfrak{e}_1) + \mu_1 (-2 + 499 \mu_2 - 174 \mathfrak{e}_1 + 173 \mu_2 \mathfrak{e}_1) \right) \Big) \Big) + \\
& 4 \eta^3 \left( 553 + 1693 \mu_2 + 928 \mu_2^2 + 183 \mathfrak{e}_1 + 361 \mu_2 \mathfrak{e}_1 + \right. \\
& \quad 30 \mu_1^2 (47 + 5 \mathfrak{e}_1) + \mu_1 (1963 + 3085 \mu_2 + 543 \mathfrak{e}_1 - 233 \mu_2 \mathfrak{e}_1) + \\
& \quad \eta t \left( \mu_1^2 (390 + 46 \mathfrak{e}_1) + 5 \times (-59 - 46 \mu_2 + 140 \mu_2^2 - 15 \mathfrak{e}_1 - \right. \\
& \quad \left. 4 \mu_2 \mathfrak{e}_1) + \mu_1 (95 + 1622 \mu_2 - 149 \mathfrak{e}_1 + 250 \mu_2 \mathfrak{e}_1) \right) \Big) \Big) +
\end{aligned}$$

$$\begin{aligned}
& 2 \eta \left( 2 \times \left( 54 + 227 \mu_2 + 136 \mu_2^2 - 6 \mu_1^2 (-9 + \mathfrak{z}_1) + 30 \mathfrak{z}_1 + \right. \right. \\
& \quad \left. \left. 17 \mu_2 \mathfrak{z}_1 + \mu_1 (108 + 227 \mu_2 + 24 \mathfrak{z}_1 + 23 \mu_2 \mathfrak{z}_1) \right) + \right. \\
& \quad \left. \eta t \left( -148 + 89 \mu_2 + 204 \mu_2^2 - 180 \mathfrak{z}_1 - 57 \mu_2 \mathfrak{z}_1 + 14 \mu_1^2 \right. \right. \\
& \quad \left. \left. (-7 + 11 \mathfrak{z}_1) + \mu_1 (-246 - 55 \mu_2 - 296 \mathfrak{z}_1 + 267 \mu_2 \mathfrak{z}_1) \right) \right) + \\
& (-1 + \eta t) \mathfrak{e} l \left( -2 \times \left( 7 + 48 \mu_2 + 36 \mu_2^2 - 5 \mathfrak{z}_1 + \mu_1^2 (7 + \mathfrak{z}_1) + \right. \right. \\
& \quad \left. \left. 2 \mu_1 (7 - 2 \mathfrak{z}_1 + 6 \mu_2 (4 + \mathfrak{z}_1)) \right) + \right. \\
& \quad \mathfrak{e} p \left( 14 + 7 \mathfrak{z}_1 + 5 \mathfrak{z}_1^2 + 7 \mathfrak{z}_2 - 5 \mathfrak{z}_1 \mathfrak{z}_2 + 4 \mu_2^2 (9 \mathfrak{z}_1 + 7 \times (2 + \mathfrak{z}_2)) + \right. \\
& \quad \mu_2 (5 \mathfrak{z}_1^2 - 5 \mathfrak{z}_1 (-9 + \mathfrak{z}_2) + 37 \times (2 + \mathfrak{z}_2)) + \\
& \quad \mu_1^2 (-\mathfrak{z}_1^2 + 7 \times (2 + \mathfrak{z}_2) + \mathfrak{z}_1 (19 + \mathfrak{z}_2)) + \mu_1 (28 + 26 \mathfrak{z}_1 + 4 \mathfrak{z}_1^2 + \\
& \quad \left. 14 \mathfrak{z}_2 - 4 \mathfrak{z}_1 \mathfrak{z}_2 + \mu_2 (74 + 69 \mathfrak{z}_1 + 5 \mathfrak{z}_1^2 + 37 \mathfrak{z}_2 + 7 \mathfrak{z}_1 \mathfrak{z}_2) \right) + \\
& \quad \eta^5 \left( -20 \mu_1 (9 + 28 \mu_2 + \mathfrak{z}_1 + \mu_1 (9 + \mathfrak{z}_1)) + 3 \mathfrak{e} p \left( 400 + \right. \right. \\
& \quad \left. \left. 2 \mu_2 (655 + 5 \mathfrak{z}_1 + 28 \mathfrak{z}_2) + \mu_1^2 (300 + 5 \mathfrak{z}_1^2 + 45 \mathfrak{z}_2 + \right. \right. \\
& \quad \left. \left. \mathfrak{z}_1 (69 + 5 \mathfrak{z}_2)) + \mu_1 (700 + 153 \mathfrak{z}_1 + 5 \mathfrak{z}_1^2 + \right. \right. \\
& \quad \left. \left. 45 \mathfrak{z}_2 + 5 \mathfrak{z}_1 \mathfrak{z}_2 + 2 \mu_2 (331 + 45 \mathfrak{z}_1 + 70 \mathfrak{z}_2) \right) \right) + \\
& 2 \eta^3 \left( 2 \times \left( 75 - 3 \mu_2^2 + \mu_1^2 (56 - 31 \mathfrak{z}_1) + 60 \mathfrak{z}_1 + \mu_2 (29 + 15 \mathfrak{z}_1) + \right. \right. \\
& \quad \left. \left. \mu_1 (131 + 179 \mathfrak{z}_1 - 19 \mu_2 (13 + 3 \mathfrak{z}_1)) \right) + \right. \\
& \quad \mathfrak{e} p \left( 614 + 141 \mathfrak{z}_1 + 75 \mathfrak{z}_1^2 + 4 \mu_2^2 (334 + 27 \mathfrak{z}_1 - 303 \mathfrak{z}_2) - 39 \mathfrak{z}_2 - \right. \\
& \quad \left. 75 \mathfrak{z}_1 \mathfrak{z}_2 + \mu_2 (2586 + 439 \mathfrak{z}_1 + 75 \mathfrak{z}_1^2 + 19 \mathfrak{z}_2 - 75 \mathfrak{z}_1 \mathfrak{z}_2) + \right. \\
& \quad \mu_1^2 (1912 + 65 \mathfrak{z}_1^2 + 161 \mathfrak{z}_2 + 7 \mathfrak{z}_1 (13 + 5 \mathfrak{z}_2)) + \\
& \quad \mu_1 (2526 + 292 \mathfrak{z}_1 + 320 \mathfrak{z}_1^2 + 122 \mathfrak{z}_2 - 220 \mathfrak{z}_1 \mathfrak{z}_2 + \\
& \quad \left. \left. \mu_2 (5898 - 361 \mathfrak{z}_1 + 75 \mathfrak{z}_1^2 + 499 \mathfrak{z}_2 - 255 \mathfrak{z}_1 \mathfrak{z}_2) \right) \right) + \\
& 2 \eta^2 \left( 188 + 636 \mu_1 + 448 \mu_1^2 + 83 \mu_2 + 443 \mu_1 \mu_2 - 84 \mu_2^2 + \right. \\
& \quad 180 \mathfrak{z}_1 + 310 \mu_1 \mathfrak{z}_1 + 4 \mu_1^2 \mathfrak{z}_1 + 45 \mu_2 \mathfrak{z}_1 - 207 \mu_1 \mu_2 \mathfrak{z}_1 + \\
& \quad 3 \mathfrak{e} p \left( 74 + 37 \mathfrak{z}_1 + 35 \mathfrak{z}_1^2 + 8 \mu_2^2 (38 + 9 \mathfrak{z}_1 - 28 \mathfrak{z}_2) - 11 \mathfrak{z}_2 - \right. \\
& \quad \left. 35 \mathfrak{z}_1 \mathfrak{z}_2 + \mu_2 (464 + 137 \mathfrak{z}_1 + 35 \mathfrak{z}_1^2 - 5 \mathfrak{z}_2 - 35 \mathfrak{z}_1 \mathfrak{z}_2) + \right. \\
& \quad \left. 2 \mu_1^2 (101 + 3 \mathfrak{z}_1^2 + \mathfrak{z}_2 + \mathfrak{z}_1 (11 + 4 \mathfrak{z}_2)) + \right. \\
& \quad \mu_1 (276 + 23 \mathfrak{z}_1 + 77 \mathfrak{z}_1^2 - 9 \mathfrak{z}_2 - 63 \mathfrak{z}_1 \mathfrak{z}_2 + \\
& \quad \left. \left. \mu_2 (840 + 25 \mathfrak{z}_1 + 35 \mathfrak{z}_1^2 + 39 \mathfrak{z}_2 - 23 \mathfrak{z}_1 \mathfrak{z}_2) \right) \right) + \\
& \eta \left( 2 \times \left( 40 + 90 \mu_1^2 - 114 \mu_2^2 + 70 \mathfrak{z}_1 + 3 \mu_2 (-29 + 5 \mathfrak{z}_1) + \right. \right. \\
& \quad \left. \left. \mu_1 (130 + 76 \mathfrak{z}_1 - \mu_2 (59 + 105 \mathfrak{z}_1)) \right) + \right. \\
& \quad \mathfrak{e} p \left( 126 + 69 \mathfrak{z}_1 + 75 \mathfrak{z}_1^2 + 4 \mu_2^2 (134 + 63 \mathfrak{z}_1 - 27 \mathfrak{z}_2) + \right. \\
& \quad \left. 9 \mathfrak{z}_2 - 75 \mathfrak{z}_1 \mathfrak{z}_2 + \mu_2 (844 + 349 \mathfrak{z}_1 + 75 \mathfrak{z}_1^2 + 123 \mathfrak{z}_2 - 75 \mathfrak{z}_1 \mathfrak{z}_2) + \right. \\
& \quad \left. 2 \mu_1^2 (58 + 55 \mathfrak{z}_1 - 2 \mathfrak{z}_1^2 + 2 \mathfrak{z}_2 + 7 \mathfrak{z}_1 \mathfrak{z}_2) + \right. \\
& \quad \mu_1 (242 + 107 \mathfrak{z}_1 + 107 \mathfrak{z}_1^2 + 13 \mathfrak{z}_2 - 97 \mathfrak{z}_1 \mathfrak{z}_2 + \\
& \quad \left. \left. \mu_2 (868 + 397 \mathfrak{z}_1 + 75 \mathfrak{z}_1^2 + 135 \mathfrak{z}_2 + 33 \mathfrak{z}_1 \mathfrak{z}_2) \right) \right) + \\
& 2 \eta^4 \left( -4 \times \left( 20 \mu_2 + \mu_1 (85 + 324 \mu_2 - 23 \mathfrak{z}_1) + \mu_1^2 (85 + 7 \mathfrak{z}_1) \right) + \right. \\
& \quad 5 \mathfrak{e} p \left( 4 \times \left( 10 \mu_2 \mathfrak{z}_1 + 3 \times (17 + \mathfrak{z}_1) + \mu_2^2 (34 - 30 \mathfrak{z}_2) + 9 \mu_2 \right. \right. \\
& \quad \left. \left. (19 + \mathfrak{z}_2) \right) + \mu_1^2 (373 + 11 \mathfrak{z}_1^2 + 47 \mathfrak{z}_2 + \mathfrak{z}_1 (36 + 5 \mathfrak{z}_2)) + \right. \\
& \quad \mu_1 (577 + 29 \mathfrak{z}_1^2 + \mathfrak{z}_1 (102 - 13 \mathfrak{z}_2) + 47 \mathfrak{z}_2 - \\
& \quad \left. \left. 4 \mu_2 (-245 - 34 \mathfrak{z}_2 + \mathfrak{z}_1 (7 + 9 \mathfrak{z}_2)) \right) \right) + \\
& \eta \mathfrak{e} p \left( -2 \eta^8 (11 + 20 \mu_2 + 3 \mathfrak{z}_1 + \mu_1 (11 + 3 \mathfrak{z}_1)) + 2 \eta t \left( 7 + 48 \mu_2 + \right. \right. \\
& \quad \left. \left. 36 \mu_2^2 - 5 \mathfrak{z}_1 + \mu_1^2 (7 + \mathfrak{z}_1) + 2 \mu_1 (7 - 2 \mathfrak{z}_1 + 6 \mu_2 (4 + \mathfrak{z}_1)) \right) + 2 \right.
\end{aligned}$$

$$\begin{aligned}
& \eta^7 \left( -67 - 146 \mu_2 + 84 \mu_2^2 - 9 \mathfrak{e}1 - 3 \mu_1^2 (13 + 3 \mathfrak{e}1) + \right. \\
& \quad 2 \mu_1 (-53 - 15 \mu_2 - 12 \mathfrak{e}1 + 9 \mu_2 \mathfrak{e}1) + \\
& \quad \left. \eta \mathfrak{t} (11 + 20 \mu_2 + 3 \mathfrak{e}1 + \mu_1 (11 + 3 \mathfrak{e}1)) \right) + \eta^6 \\
& \left( -2 \times (57 - 176 \mu_2^2 + 7 \mathfrak{e}1 + 2 \mu_1^2 (69 + 11 \mathfrak{e}1) + \mu_2 (98 + 22 \mathfrak{e}1) + \right. \\
& \quad \mu_1 (195 + \mu_2 (190 - 50 \mathfrak{e}1) + 53 \mathfrak{e}1)) - \\
& \quad \mathfrak{e}1 (64 + 2 \mu_2 (107 + \mathfrak{e}1 + 4 \mathfrak{e}2) + \mu_1^2 (48 + \mathfrak{e}1^2 + 9 \mathfrak{e}2 + \mathfrak{e}1 (13 + \mathfrak{e}2)) + \\
& \quad \mu_1 (112 + \mathfrak{e}1^2 + 9 \mathfrak{e}2 + \mathfrak{e}1 (25 + \mathfrak{e}2) + 2 \mu_2 (55 + 9 \mathfrak{e}1 + 14 \mathfrak{e}2))) + \\
& \quad \eta \mathfrak{t} (-2 \times (-35 - 48 \mu_2 + 56 \mu_2^2 - 9 \mathfrak{e}1 + 2 \mu_1^2 (9 + \mathfrak{e}1) + \\
& \quad \mu_1 (-17 - 7 \mathfrak{e}1 + 4 \mu_2 (19 + 3 \mathfrak{e}1))) + \mathfrak{e}1 (64 + \\
& \quad 2 \mu_2 (107 + \mathfrak{e}1 + 4 \mathfrak{e}2) + \mu_1^2 (48 + \mathfrak{e}1^2 + 9 \mathfrak{e}2 + \mathfrak{e}1 (13 + \mathfrak{e}2)) + \mu_1 \\
& \quad (112 + \mathfrak{e}1^2 + 9 \mathfrak{e}2 + \mathfrak{e}1 (25 + \mathfrak{e}2) + 2 \mu_2 (55 + 9 \mathfrak{e}1 + 14 \mathfrak{e}2))) \left. \right) + \\
& \eta^3 \left( 2 \times (57 + 296 \mu_2^2 + 29 \mathfrak{e}1 + 8 \mu_1^2 (18 + \mathfrak{e}1) + 3 \mu_2 (89 + 17 \mathfrak{e}1) + \right. \\
& \quad \mu_1 (201 - 3 \mu_2 (-145 + \mathfrak{e}1) + 55 \mathfrak{e}1)) - \\
& \quad \mathfrak{e}1 (98 + 49 \mathfrak{e}1 + 35 \mathfrak{e}1^2 + 4 \mu_2^2 (86 + 27 \mathfrak{e}1 - 47 \mathfrak{e}2) + \mathfrak{e}2 - \\
& \quad 35 \mathfrak{e}1 \mathfrak{e}2 + \mu_2 (578 + 183 \mathfrak{e}1 + 35 \mathfrak{e}1^2 + 43 \mathfrak{e}2 - 35 \mathfrak{e}1 \mathfrak{e}2) + \\
& \quad \mu_1^2 (224 + 5 \mathfrak{e}1^2 + 13 \mathfrak{e}2 + \mathfrak{e}1 (31 + 7 \mathfrak{e}2)) + \\
& \quad \mu_1 (322 + 44 \mathfrak{e}1 + 76 \mathfrak{e}1^2 + 14 \mathfrak{e}2 - 64 \mathfrak{e}1 \mathfrak{e}2 + \\
& \quad \mu_2 (962 + 87 \mathfrak{e}1 + 35 \mathfrak{e}1^2 + 91 \mathfrak{e}2 - 23 \mathfrak{e}1 \mathfrak{e}2)) \left. \right) + \\
& \eta \mathfrak{t} (-20 + 248 \mu_1 + 268 \mu_1^2 - 91 \mu_2 + 685 \mu_1 \mu_2 + 48 \mu_2^2 + \\
& \quad 48 \mathfrak{e}1 + 24 \mu_1 \mathfrak{e}1 + 36 \mu_1^2 \mathfrak{e}1 + 7 \mu_2 \mathfrak{e}1 - 5 \mu_1 \mu_2 \mathfrak{e}1 + \\
& \quad \mathfrak{e}1 (98 + 49 \mathfrak{e}1 + 35 \mathfrak{e}1^2 + 4 \mu_2^2 (86 + 27 \mathfrak{e}1 - 47 \mathfrak{e}2) + \mathfrak{e}2 - 35 \mathfrak{e}1 \mathfrak{e}2 + \\
& \quad \mu_2 (578 + 183 \mathfrak{e}1 + 35 \mathfrak{e}1^2 + 43 \mathfrak{e}2 - 35 \mathfrak{e}1 \mathfrak{e}2) + \mu_1^2 (224 + 5 \mathfrak{e}1^2 + \\
& \quad 13 \mathfrak{e}2 + \mathfrak{e}1 (31 + 7 \mathfrak{e}2)) + \mu_1 (322 + 44 \mathfrak{e}1 + 76 \mathfrak{e}1^2 + 14 \mathfrak{e}2 - \\
& \quad 64 \mathfrak{e}1 \mathfrak{e}2 + \mu_2 (962 + 87 \mathfrak{e}1 + 35 \mathfrak{e}1^2 + 91 \mathfrak{e}2 - 23 \mathfrak{e}1 \mathfrak{e}2))) \left. \right) + \\
& 2 \eta^5 (10 - 95 \mu_1 - 105 \mu_1^2 - 101 \mu_2 - 385 \mu_1 \mu_2 - 324 \mu_2^2 - 20 \mathfrak{e}1 - \\
& \quad 31 \mu_1 \mathfrak{e}1 + \mu_1^2 \mathfrak{e}1 - 51 \mu_2 \mathfrak{e}1 - 3 \mu_1 \mu_2 \mathfrak{e}1 - \\
& \quad \mathfrak{e}1 (4 \times (19 + \mathfrak{e}1) - 40 \mu_2^2 (-1 + \mathfrak{e}2) + 2 \mu_2 (131 + 7 \mathfrak{e}1 + 6 \mathfrak{e}2) + \\
& \quad \mu_1^2 (133 + 4 \mathfrak{e}1^2 + 20 \mathfrak{e}2 + \mathfrak{e}1 (17 + 2 \mathfrak{e}2)) + \mu_1 (209 + 39 \mathfrak{e}1 + \\
& \quad 10 \mathfrak{e}1^2 + 20 \mathfrak{e}2 - 4 \mathfrak{e}1 \mathfrak{e}2 + 2 \mu_2 (179 + \mathfrak{e}1 + 30 \mathfrak{e}2 - 6 \mathfrak{e}1 \mathfrak{e}2)) \left. \right) + \\
& \eta \mathfrak{t} (13 - 22 \mu_2 - 84 \mu_2^2 + 3 \mathfrak{e}1 + 4 \mu_2 \mathfrak{e}1 - 8 \mu_1^2 (10 + \mathfrak{e}1) - \\
& \quad \mu_1 (67 - 19 \mathfrak{e}1 + \mu_2 (322 + 38 \mathfrak{e}1)) + \mathfrak{e}1 (4 \times (19 + \mathfrak{e}1) - \\
& \quad 40 \mu_2^2 (-1 + \mathfrak{e}2) + 2 \mu_2 (131 + 7 \mathfrak{e}1 + 6 \mathfrak{e}2) + \mu_1^2 (133 + \\
& \quad 4 \mathfrak{e}1^2 + 20 \mathfrak{e}2 + \mathfrak{e}1 (17 + 2 \mathfrak{e}2)) + \mu_1 (209 + 39 \mathfrak{e}1 + 10 \mathfrak{e}1^2 + \\
& \quad 20 \mathfrak{e}2 - 4 \mathfrak{e}1 \mathfrak{e}2 + 2 \mu_2 (179 + \mathfrak{e}1 + 30 \mathfrak{e}2 - 6 \mathfrak{e}1 \mathfrak{e}2))) \left. \right) + \eta \\
& (\mathfrak{e}1 (-14 - 7 \mathfrak{e}1 - 5 \mathfrak{e}1^2 - 7 \mathfrak{e}2 + 5 \mathfrak{e}1 \mathfrak{e}2 - 4 \mu_2^2 (9 \mathfrak{e}1 + 7 \times (2 + \mathfrak{e}2)) - \\
& \quad \mu_2 (5 \mathfrak{e}1^2 - 5 \mathfrak{e}1 (-9 + \mathfrak{e}2) + 37 \times (2 + \mathfrak{e}2)) + \\
& \quad \mu_1^2 (\mathfrak{e}1^2 - 7 \times (2 + \mathfrak{e}2) - \mathfrak{e}1 (19 + \mathfrak{e}2)) - \mu_1 (28 + 26 \mathfrak{e}1 + 4 \mathfrak{e}1^2 + \\
& \quad 14 \mathfrak{e}2 - 4 \mathfrak{e}1 \mathfrak{e}2 + \mu_2 (74 + 69 \mathfrak{e}1 + 5 \mathfrak{e}1^2 + 37 \mathfrak{e}2 + 7 \mathfrak{e}1 \mathfrak{e}2))) \left. \right) + \\
& \eta \mathfrak{t} (-28 - 96 \mu_1 - 68 \mu_1^2 + 95 \mu_2 + 71 \mu_1 \mu_2 + 120 \mu_2^2 - 60 \mathfrak{e}1 - \\
& \quad 68 \mu_1 \mathfrak{e}1 + 4 \mu_1^2 \mathfrak{e}1 - 15 \mu_2 \mathfrak{e}1 + 81 \mu_1 \mu_2 \mathfrak{e}1 + \\
& \quad \mathfrak{e}1 (14 + 7 \mathfrak{e}1 + 5 \mathfrak{e}1^2 + 7 \mathfrak{e}2 - 5 \mathfrak{e}1 \mathfrak{e}2 + 4 \mu_2^2 (9 \mathfrak{e}1 + 7 \times (2 + \mathfrak{e}2)) + \\
& \quad \mu_2 (5 \mathfrak{e}1^2 - 5 \mathfrak{e}1 (-9 + \mathfrak{e}2) + 37 \times (2 + \mathfrak{e}2)) + \mu_1^2 (-\mathfrak{e}1^2 + \\
& \quad 7 \times (2 + \mathfrak{e}2) + \mathfrak{e}1 (19 + \mathfrak{e}2)) + \mu_1 (28 + 26 \mathfrak{e}1 + 4 \mathfrak{e}1^2 + 14 \mathfrak{e}2 -
\end{aligned}$$

$$\begin{aligned}
& 4 \, \mathfrak{e}1 \, \mathfrak{e}2 + \mu2 \left( 74 + 69 \, \mathfrak{e}1 + 5 \, \mathfrak{e}1^2 + 37 \, \mathfrak{e}2 + 7 \, \mathfrak{e}1 \, \mathfrak{e}2 \right) \Big) \Big) \Big) \Big) + \\
& \eta^2 \left( 4 \times \left( 18 + 79 \, \mu2 + 40 \, \mu2^2 - 2 \, \mu1^2 \left( -9 + \mathfrak{e}1 \right) + 10 \, \mathfrak{e}1 + 5 \, \mu2 \, \mathfrak{e}1 + \right. \right. \\
& \quad \left. \left. \mu1 \left( 36 + 8 \, \mathfrak{e}1 + \mu2 \left( 79 + 11 \, \mathfrak{e}1 \right) \right) \right) + \right. \\
& \quad \mathfrak{e}1 \left( -58 - 31 \, \mathfrak{e}1 - 25 \, \mathfrak{e}1^2 - 12 \, \mu2^2 \left( 18 + 9 \, \mathfrak{e}1 - \mathfrak{e}2 \right) - 11 \, \mathfrak{e}2 + \right. \\
& \quad \left. 25 \, \mathfrak{e}1 \, \mathfrak{e}2 - \mu2 \left( 352 + 147 \, \mathfrak{e}1 + 25 \, \mathfrak{e}1^2 + 73 \, \mathfrak{e}2 - 25 \, \mathfrak{e}1 \, \mathfrak{e}2 \right) + \right. \\
& \quad \left. 2 \, \mu1^2 \left( \mathfrak{e}1^2 - 3 \times \left( 8 + \mathfrak{e}2 \right) - 2 \, \mathfrak{e}1 \left( 10 + \mathfrak{e}2 \right) \right) - \right. \\
& \quad \left. \mu1 \left( 106 + 47 \, \mathfrak{e}1 + 35 \, \mathfrak{e}1^2 + 17 \, \mathfrak{e}2 - 33 \, \mathfrak{e}1 \, \mathfrak{e}2 + \right. \right. \\
& \quad \left. \left. \mu2 \left( 344 + 163 \, \mathfrak{e}1 + 25 \, \mathfrak{e}1^2 + 69 \, \mathfrak{e}2 + 11 \, \mathfrak{e}1 \, \mathfrak{e}2 \right) \right) \right) + \\
& \quad \eta t \left( -74 - 208 \, \mu1 - 134 \, \mu1^2 - 89 \, \mu2 - 177 \, \mu1 \, \mu2 - 24 \, \mu2^2 - \right. \\
& \quad \left. 50 \, \mathfrak{e}1 - 124 \, \mu1 \, \mathfrak{e}1 + 22 \, \mu1^2 \, \mathfrak{e}1 - 23 \, \mu2 \, \mathfrak{e}1 + 73 \, \mu1 \, \mu2 \, \mathfrak{e}1 + \right. \\
& \quad \mathfrak{e}1 \left( 58 + 31 \, \mathfrak{e}1 + 25 \, \mathfrak{e}1^2 + 12 \, \mu2^2 \left( 18 + 9 \, \mathfrak{e}1 - \mathfrak{e}2 \right) + 11 \, \mathfrak{e}2 - \right. \\
& \quad \left. 25 \, \mathfrak{e}1 \, \mathfrak{e}2 + \mu2 \left( 352 + 147 \, \mathfrak{e}1 + 25 \, \mathfrak{e}1^2 + 73 \, \mathfrak{e}2 - 25 \, \mathfrak{e}1 \, \mathfrak{e}2 \right) + \right. \\
& \quad \left. \mu1^2 \left( -2 \, \mathfrak{e}1^2 + 6 \times \left( 8 + \mathfrak{e}2 \right) + 4 \, \mathfrak{e}1 \left( 10 + \mathfrak{e}2 \right) \right) + \right. \\
& \quad \left. \mu1 \left( 106 + 47 \, \mathfrak{e}1 + 35 \, \mathfrak{e}1^2 + 17 \, \mathfrak{e}2 - 33 \, \mathfrak{e}1 \, \mathfrak{e}2 + \right. \right. \\
& \quad \left. \left. \mu2 \left( 344 + 163 \, \mathfrak{e}1 + 25 \, \mathfrak{e}1^2 + 69 \, \mathfrak{e}2 + 11 \, \mathfrak{e}1 \, \mathfrak{e}2 \right) \right) \right) \Big) \Big) \Big) + \eta^4 \\
& \left( 4 \times \left( 16 - 156 \, \mu2^2 + 6 \, \mu2 \left( -5 + \mathfrak{e}1 \right) - 5 \, \mathfrak{e}1 + \mu1^2 \left( 51 + 13 \, \mathfrak{e}1 \right) + \right. \right. \\
& \quad \left. \left. \mu1 \left( 67 + \mu2 \left( 6 - 42 \, \mathfrak{e}1 \right) + 20 \, \mathfrak{e}1 \right) \right) - \right. \\
& \quad \mathfrak{e}1 \left( 142 + 33 \, \mathfrak{e}1 + 15 \, \mathfrak{e}1^2 + 12 \, \mu2^2 \left( 22 + 3 \, \mathfrak{e}1 - 19 \, \mathfrak{e}2 \right) - 3 \, \mathfrak{e}2 - \right. \\
& \quad \left. 15 \, \mathfrak{e}1 \, \mathfrak{e}2 + \mu2 \left( 610 + 107 \, \mathfrak{e}1 + 15 \, \mathfrak{e}1^2 + 23 \, \mathfrak{e}2 - 15 \, \mathfrak{e}1 \, \mathfrak{e}2 \right) + \right. \\
& \quad \left. \mu1^2 \left( 408 + 13 \, \mathfrak{e}1^2 + 45 \, \mathfrak{e}2 + \mathfrak{e}1 \left( 31 + 7 \, \mathfrak{e}2 \right) \right) + \right. \\
& \quad \left. \mu1 \left( 550 + 76 \, \mathfrak{e}1 + 64 \, \mathfrak{e}1^2 + 42 \, \mathfrak{e}2 - 44 \, \mathfrak{e}1 \, \mathfrak{e}2 + \right. \right. \\
& \quad \left. \left. \mu2 \left( 1298 + 15 \, \mathfrak{e}1^2 + 151 \, \mathfrak{e}2 - 3 \, \mathfrak{e}1 \left( 7 + 17 \, \mathfrak{e}2 \right) \right) \right) \right) + \\
& \quad \eta t \left( -10 + 106 \, \mu1 + 116 \, \mu1^2 - 103 \, \mu2 + 121 \, \mu1 \, \mu2 + 64 \, \mu2^2 + \right. \\
& \quad \left. 42 \, \mathfrak{e}1 + 118 \, \mu1 \, \mathfrak{e}1 - 44 \, \mu1^2 \, \mathfrak{e}1 + 23 \, \mu2 \, \mathfrak{e}1 - 73 \, \mu1 \, \mu2 \, \mathfrak{e}1 + \right. \\
& \quad \mathfrak{e}1 \left( 142 + 33 \, \mathfrak{e}1 + 15 \, \mathfrak{e}1^2 + 12 \, \mu2^2 \left( 22 + 3 \, \mathfrak{e}1 - 19 \, \mathfrak{e}2 \right) - 3 \, \mathfrak{e}2 - \right. \\
& \quad \left. 15 \, \mathfrak{e}1 \, \mathfrak{e}2 + \mu2 \left( 610 + 107 \, \mathfrak{e}1 + 15 \, \mathfrak{e}1^2 + 23 \, \mathfrak{e}2 - 15 \, \mathfrak{e}1 \, \mathfrak{e}2 \right) + \right. \\
& \quad \left. \mu1^2 \left( 408 + 13 \, \mathfrak{e}1^2 + 45 \, \mathfrak{e}2 + \mathfrak{e}1 \left( 31 + 7 \, \mathfrak{e}2 \right) \right) + \right. \\
& \quad \left. \mu1 \left( 550 + 76 \, \mathfrak{e}1 + 64 \, \mathfrak{e}1^2 + 42 \, \mathfrak{e}2 - 44 \, \mathfrak{e}1 \, \mathfrak{e}2 + \right. \right. \\
& \quad \left. \left. \mu2 \left( 1298 + 15 \, \mathfrak{e}1^2 + 151 \, \mathfrak{e}2 - 3 \, \mathfrak{e}1 \left( 7 + 17 \, \mathfrak{e}2 \right) \right) \right) \right) \Big) \Big) \Big) - \\
& x^3 \left( -1 + \eta \right)^3 \left( -2 \times \left( -1 + \eta \right) \, \mathfrak{e}p \left( 35 \, \eta^5 \left( 11 + 20 \, \mu2 + 3 \, \mathfrak{e}1 + \mu1 \left( 11 + 3 \, \mathfrak{e}1 \right) \right) + \right. \right. \\
& \quad \left. \left. 4 \times \left( 9 + 24 \, \mu2^2 - \mu1^2 \left( -9 + \mathfrak{e}1 \right) + 5 \, \mathfrak{e}1 + \right. \right. \right. \\
& \quad \left. \left. \left. \mu2 \left( 37 + 3 \, \mathfrak{e}1 \right) + \mu1 \left( 18 + 4 \, \mathfrak{e}1 + \mu2 \left( 37 + 3 \, \mathfrak{e}1 \right) \right) \right) \right) - \right. \\
& \quad \left. 5 \, \eta^4 \left( 4 \times \left( -93 - 211 \, \mu2 + 84 \, \mu2^2 - 12 \, \mathfrak{e}1 \right) - 21 \, \mu1^2 \left( 13 + 3 \, \mathfrak{e}1 \right) + \right. \right. \\
& \quad \left. \left. 7 \, \eta t \left( 11 + 20 \, \mu2 + 3 \, \mathfrak{e}1 + \mu1 \left( 11 + 3 \, \mathfrak{e}1 \right) \right) + \right. \right. \\
& \quad \left. \left. 3 \, \mu1 \left( -215 - 51 \, \mathfrak{e}1 + 4 \, \mu2 \left( -25 + 6 \, \mathfrak{e}1 \right) \right) \right) + \right. \\
& \quad \left. \eta t \left( -52 + 60 \, \mu2^2 - 19 \, \mu2 \left( -1 + \mathfrak{e}1 \right) - 60 \, \mathfrak{e}1 + \mu1^2 \left( -2 + 70 \, \mathfrak{e}1 \right) + \right. \right. \\
& \quad \left. \left. \mu1 \left( -54 - 98 \, \mathfrak{e}1 + \mu2 \left( -25 + 89 \, \mathfrak{e}1 \right) \right) \right) + \right. \\
& \quad \left. 2 \, \eta \left( 186 + 787 \, \mu2 + 872 \, \mu2^2 + 98 \, \mathfrak{e}1 + 125 \, \mu2 \, \mathfrak{e}1 + 8 \, \mu1^2 \right. \right. \\
& \quad \left. \left. \left( 45 + \mathfrak{e}1 \right) + \mu1 \left( 546 + 1123 \, \mu2 + 142 \, \mathfrak{e}1 + 23 \, \mu2 \, \mathfrak{e}1 \right) + \right. \right. \\
& \quad \left. \left. \eta t \left( -117 - 25 \, \mu2 + 189 \, \mu2^2 - 72 \, \mathfrak{e}1 - 31 \, \mu2 \, \mathfrak{e}1 + \right. \right. \right. \\
& \quad \left. \left. \left. \mu1^2 \left( 128 + 121 \, \mathfrak{e}1 \right) + \mu1 \left( 11 + 411 \, \mu2 - 173 \, \mathfrak{e}1 + 173 \, \mu2 \, \mathfrak{e}1 \right) \right) \right) \right) + \\
& \quad \left. 2 \, \eta^2 \left( 517 + 1627 \, \mu2 + 1232 \, \mu2^2 + 177 \, \mathfrak{e}1 + 359 \, \mu2 \, \mathfrak{e}1 + 30 \, \mu1^2 \right. \right. \\
& \quad \left. \left. \left( 47 + 5 \, \mathfrak{e}1 \right) + \mu1 \left( 1927 + 3115 \, \mu2 + 537 \, \mathfrak{e}1 - 187 \, \mu2 \, \mathfrak{e}1 \right) + \eta t \right. \right.
\end{aligned}$$



$$\begin{aligned}
& \left( 4 \mu_1^2 (85 + 11 \mathfrak{e}_1) + 5 \times (-59 - 46 \mu_2 + 140 \mu_2^2 - 15 \mathfrak{e}_1 - 4 \mu_2 \mathfrak{e}_1) + \right. \\
& \quad \left. \mu_1 (45 + 1438 \mu_2 - 151 \mathfrak{e}_1 + 250 \mu_2 \mathfrak{e}_1) \right) + 10 \eta^3 \\
& (187 + 408 \mu_2 - 220 \mu_2^2 + 23 \mathfrak{e}_1 + 42 \mu_2 \mathfrak{e}_1 + \mu_1^2 (354 + 62 \mathfrak{e}_1) + \\
& \quad \mu_1 (541 + 532 \mu_2 + 145 \mathfrak{e}_1 - 72 \mu_2 \mathfrak{e}_1) + 2 \eta t (-46 - 68 \mu_2 + 56 \mu_2^2 - \\
& \quad 12 \mathfrak{e}_1 + \mu_1^2 (9 + \mathfrak{e}_1) + \mu_1 (-37 - 11 \mathfrak{e}_1 + 12 \mu_2 (4 + \mathfrak{e}_1))) + \\
& (-1 + \eta t) \mathfrak{e}_l (38 + 96 \mu_1 + 58 \mu_1^2 - 95 \mu_2 - 79 \mu_1 \mu_2 - 120 \mu_2^2 + \\
& \quad 70 \mathfrak{e}_1 + 76 \mu_1 \mathfrak{e}_1 - 18 \mu_1^2 \mathfrak{e}_1 + 15 \mu_2 \mathfrak{e}_1 - 105 \mu_1 \mu_2 \mathfrak{e}_1 + \\
& \mathfrak{e}_p (34 + 19 \mathfrak{e}_1 + 25 \mathfrak{e}_1^2 + 8 \mu_2^2 (20 + 9 \mathfrak{e}_1 - 6 \mathfrak{e}_2) - \mathfrak{e}_2 - \\
& \quad 25 \mathfrak{e}_1 \mathfrak{e}_2 + \mu_2 (246 + 101 \mathfrak{e}_1 + 25 \mathfrak{e}_1^2 + 25 \mathfrak{e}_2 - 25 \mathfrak{e}_1 \mathfrak{e}_2) - \\
& \quad \mu_1^2 (-34 + \mathfrak{e}_1^2 + \mathfrak{e}_2 - 5 \mathfrak{e}_1 (7 + \mathfrak{e}_2)) + \mu_1 (68 + 30 \mathfrak{e}_1 + 36 \mathfrak{e}_1^2 - 2 \mathfrak{e}_2 - \\
& \quad 32 \mathfrak{e}_1 \mathfrak{e}_2 + \mu_2 (262 + 117 \mathfrak{e}_1 + 25 \mathfrak{e}_1^2 + 33 \mathfrak{e}_2 + 11 \mathfrak{e}_1 \mathfrak{e}_2))) + \\
& 10 \eta^4 (-4 \mu_1 (9 + 28 \mu_2 + \mathfrak{e}_1 + \mu_1 (9 + \mathfrak{e}_1)) + \mathfrak{e}_p \\
& \quad (\mu_1^2 (141 + 29 \mathfrak{e}_1 + 2 \mathfrak{e}_1^2 + 18 \mathfrak{e}_2 + 2 \mathfrak{e}_1 \mathfrak{e}_2) + \\
& \quad 4 \times (47 + \mu_2 (152 + \mathfrak{e}_1 + 7 \mathfrak{e}_2)) + \mu_1 (329 + 71 \mathfrak{e}_1 + 2 \mathfrak{e}_1^2 + \\
& \quad 18 \mathfrak{e}_2 + 2 \mathfrak{e}_1 \mathfrak{e}_2 + 4 \mu_2 (76 + 9 \mathfrak{e}_1 + 14 \mathfrak{e}_2))) + \\
& 2 \eta (196 + 115 \mu_2 - 60 \mu_2^2 + \mu_1^2 (356 - 52 \mathfrak{e}_1) + 180 \mathfrak{e}_1 + \\
& \quad 45 \mu_2 \mathfrak{e}_1 + \mu_1 (552 + 463 \mu_2 + 308 \mathfrak{e}_1 - 207 \mu_2 \mathfrak{e}_1) + \\
& \mathfrak{e}_p (\mu_1^2 (382 + 13 \mathfrak{e}_1^2 - 7 \mathfrak{e}_2 + \mathfrak{e}_1 (35 + 17 \mathfrak{e}_2)) + \\
& \quad 2 \times (62 + 31 \mathfrak{e}_1 + 35 \mathfrak{e}_1^2 + \mu_2^2 (284 + 54 \mathfrak{e}_1 - 242 \mathfrak{e}_2) - 17 \mathfrak{e}_2 - \\
& \quad 35 \mathfrak{e}_1 \mathfrak{e}_2 + \mu_2 (407 + 114 \mathfrak{e}_1 + 35 \mathfrak{e}_1^2 - 29 \mathfrak{e}_2 - 35 \mathfrak{e}_1 \mathfrak{e}_2)) + \\
& \quad \mu_1 (506 + 25 \mathfrak{e}_1 + 155 \mathfrak{e}_1^2 - 41 \mathfrak{e}_2 - 125 \mathfrak{e}_1 \mathfrak{e}_2 + \\
& \quad 2 \mu_2 (779 - 6 \mathfrak{e}_1 + 35 \mathfrak{e}_1^2 + 13 \mathfrak{e}_2 - 23 \mathfrak{e}_1 \mathfrak{e}_2))) + 4 \eta^3 \\
& (-2 \times (40 \mu_2 + \mu_1 (145 + 556 \mu_2 - 47 \mathfrak{e}_1) + \mu_1^2 (145 + 13 \mathfrak{e}_1)) + 5 \\
& \mathfrak{e}_p (8 \times (16 + \mathfrak{e}_1) + \mu_2^2 (96 - 80 \mathfrak{e}_2) + \mu_2 (422 + 26 \mathfrak{e}_1 + 24 \mathfrak{e}_2) + \mu_1^2 \\
& \quad (240 + 19 \mathfrak{e}_1 + 7 \mathfrak{e}_1^2 + 27 \mathfrak{e}_2 + 3 \mathfrak{e}_1 \mathfrak{e}_2) + \mu_1 (368 + 19 \mathfrak{e}_1^2 - 9 \mathfrak{e}_1 \\
& \quad (-7 + \mathfrak{e}_2) + 27 \mathfrak{e}_2 + \mu_2 (622 + 76 \mathfrak{e}_2 - 6 \mathfrak{e}_1 (5 + 4 \mathfrak{e}_2)))) + \\
& 2 \eta^2 (3 \times (78 + 6 \mu_2^2 + \mu_1^2 (40 - 50 \mathfrak{e}_1) + 60 \mathfrak{e}_1 + \mu_2 (41 + 15 \mathfrak{e}_1) - \\
& \quad 3 \mu_1 \mu_2 (53 + 19 \mathfrak{e}_1) + 2 \mu_1 (59 + 89 \mathfrak{e}_1)) + \\
& \mathfrak{e}_p (566 + 129 \mathfrak{e}_1 + 75 \mathfrak{e}_1^2 + 24 \mu_2^2 (56 + 3 \mathfrak{e}_1 - 52 \mathfrak{e}_2) - 51 \mathfrak{e}_2 - \\
& \quad 75 \mathfrak{e}_1 \mathfrak{e}_2 + \mu_2 (2354 + 391 \mathfrak{e}_1 + 75 \mathfrak{e}_1^2 - 29 \mathfrak{e}_2 - 75 \mathfrak{e}_1 \mathfrak{e}_2) + \\
& \quad \mu_1^2 (1848 + 59 \mathfrak{e}_1 + 65 \mathfrak{e}_1^2 + 129 \mathfrak{e}_2 + 35 \mathfrak{e}_1 \mathfrak{e}_2) + \\
& \quad \mu_1 (2414 + 248 \mathfrak{e}_1 + 320 \mathfrak{e}_1^2 + 78 \mathfrak{e}_2 - 220 \mathfrak{e}_1 \mathfrak{e}_2 + \\
& \quad \mu_2 (5602 + 75 \mathfrak{e}_1^2 + 371 \mathfrak{e}_2 - 3 \mathfrak{e}_1 (163 + 85 \mathfrak{e}_2)))) + \\
& \times (-1 + \eta) \times (14 \eta^8 \mathfrak{e}_p (11 + 20 \mu_2 + 3 \mathfrak{e}_1 + \mu_1 (11 + 3 \mathfrak{e}_1)) - 2 \eta^7 \mathfrak{e}_p \\
& \quad (-411 - 916 \mu_2 + 504 \mu_2^2 - 51 \mathfrak{e}_1 - 21 \mu_1^2 (13 + 3 \mathfrak{e}_1) + \\
& \quad 12 \mu_1 (-57 - 20 \mu_2 - 13 \mathfrak{e}_1 + 9 \mu_2 \mathfrak{e}_1) + \\
& \quad 7 \eta t (11 + 20 \mu_2 + 3 \mathfrak{e}_1 + \mu_1 (11 + 3 \mathfrak{e}_1))) - 2 \\
& \eta t \mathfrak{e}_p (11 + 64 \mu_2 + 48 \mu_2^2 - 5 \mathfrak{e}_1 + \mu_1^2 (11 + \mathfrak{e}_1) + \\
& \quad 2 \mu_1 (11 - 2 \mathfrak{e}_1 + \mu_2 (32 + 6 \mathfrak{e}_1))) - \eta^4 \\
& (2 \mathfrak{e}_p (217 + 101 \mu_2 - 960 \mu_2^2 - 7 \mathfrak{e}_1 + 117 \mu_2 \mathfrak{e}_1 + 2 \mu_1^2 \\
& \quad (345 + 67 \mathfrak{e}_1) + \mu_1 (907 + \mu_2 (725 - 345 \mathfrak{e}_1) + 265 \mathfrak{e}_1) + \\
& \quad \eta t (-73 + 286 \mu_2^2 + \mu_1^2 (248 - 118 \mathfrak{e}_1) + 69 \mathfrak{e}_1 + \\
& \quad 6 \mu_2 (-38 + 7 \mathfrak{e}_1) + \mu_1 (175 + 632 \mu_2 + 203 \mathfrak{e}_1 - 96 \mu_2 \mathfrak{e}_1))) +
\end{aligned}$$

$$\begin{aligned}
& (-1 + \eta t) \, \theta l \, (72 + 144 \mu_1 + 72 \mu_1^2 + 17 \mu_2 - 335 \mu_1 \mu_2 - \\
& \quad 12 \mu_2^2 + 60 \, \mathfrak{e}1 + 180 \mu_1 \, \mathfrak{e}1 - 12 \mu_1^2 \, \mathfrak{e}1 + 15 \mu_2 \, \mathfrak{e}1 - 57 \mu_1 \mu_2 \, \mathfrak{e}1 + \\
& \quad \theta p \, (662 + 153 \, \mathfrak{e}1 + 75 \, \mathfrak{e}1^2 + 8 \mu_2^2 \, (166 + 18 \, \mathfrak{e}1 - 147 \, \mathfrak{e}2) - 27 \, \mathfrak{e}2 - \\
& \quad \quad 75 \, \mathfrak{e}1 \, \mathfrak{e}2 + \mu_2 \, (2818 + 487 \, \mathfrak{e}1 + 75 \, \mathfrak{e}1^2 + 67 \, \mathfrak{e}2 - 75 \, \mathfrak{e}1 \, \mathfrak{e}2) + \\
& \quad \quad \mu_1^2 \, (1976 + 65 \, \mathfrak{e}1^2 + 193 \, \mathfrak{e}2 + \, \mathfrak{e}1 \, (123 + 35 \, \mathfrak{e}2)) + \\
& \quad \quad \mu_1 \, (2638 + 336 \, \mathfrak{e}1 + 320 \, \mathfrak{e}1^2 + 166 \, \mathfrak{e}2 - 220 \, \mathfrak{e}1 \, \mathfrak{e}2 + \\
& \quad \quad \quad \mu_2 \, (6194 - 233 \, \mathfrak{e}1 + 75 \, \mathfrak{e}1^2 + 627 \, \mathfrak{e}2 - 255 \, \mathfrak{e}1 \, \mathfrak{e}2))) - 2 \\
& \eta^3 \, (\theta p \, (2 \times (132 + 597 \mu_2 + 664 \mu_2^2 + 68 \, \mathfrak{e}1 + 107 \mu_2 \, \mathfrak{e}1 + 2 \mu_1^2 \\
& \quad (153 + 7 \, \mathfrak{e}1) + \mu_1 \, (438 + 933 \mu_2 + 118 \, \mathfrak{e}1 + 5 \mu_2 \, \mathfrak{e}1)) + \\
& \quad \eta t \, (-82 - 123 \mu_2 + 186 \mu_2^2 + 36 \, \mathfrak{e}1 - 5 \mu_2 \, \mathfrak{e}1 + \mu_1^2 \\
& \quad \quad (382 + 68 \, \mathfrak{e}1) + \mu_1 \, (300 + 1209 \mu_2 - 52 \, \mathfrak{e}1 + 79 \mu_2 \, \mathfrak{e}1))) + \\
& (-1 + \eta t) \, \theta l \, (60 + 17 \mu_2 - 36 \mu_2^2 + 60 \, \mathfrak{e}1 + 15 \mu_2 \, \mathfrak{e}1 + \\
& \quad 20 \mu_1^2 \, (9 + \, \mathfrak{e}1) + \mu_1 \, (240 + 141 \mu_2 + 104 \, \mathfrak{e}1 - 69 \mu_2 \, \mathfrak{e}1) + \\
& \quad \theta p \, (\mu_1^2 \, (426 + 11 \, \mathfrak{e}1^2 + 15 \, \mathfrak{e}2 + \, \mathfrak{e}1 \, (53 + 15 \, \mathfrak{e}2)) + \\
& \quad \quad 2 \times (86 + 43 \, \mathfrak{e}1 + 35 \, \mathfrak{e}1^2 + \mu_2^2 \, (324 + 90 \, \mathfrak{e}1 - 206 \, \mathfrak{e}2) - 5 \, \mathfrak{e}2 - \\
& \quad \quad \quad 35 \, \mathfrak{e}1 \, \mathfrak{e}2 + \mu_2 \, (521 + 160 \, \mathfrak{e}1 + 35 \, \mathfrak{e}1^2 + 19 \, \mathfrak{e}2 - 35 \, \mathfrak{e}1 \, \mathfrak{e}2)) + \\
& \quad \quad \mu_1 \, (598 + 67 \, \mathfrak{e}1 + 153 \, \mathfrak{e}1^2 + 5 \, \mathfrak{e}2 - 127 \, \mathfrak{e}1 \, \mathfrak{e}2 + \\
& \quad \quad \quad 2 \mu_2 \, (901 + 56 \, \mathfrak{e}1 + 35 \, \mathfrak{e}1^2 + 65 \, \mathfrak{e}2 - 23 \, \mathfrak{e}1 \, \mathfrak{e}2)))) + 2 \\
& \eta \, (\eta t \, \theta p \, (23 - 150 \mu_2^2 + \mu_1^2 \, (33 - 23 \, \mathfrak{e}1) + 15 \mu_2 \, (-9 + \, \mathfrak{e}1) + \\
& \quad 65 \, \mathfrak{e}1 + 8 \mu_1 \, (7 + 9 \, \mathfrak{e}1) - 3 \mu_1 \mu_2 \, (41 + 31 \, \mathfrak{e}1)) + \\
& (-1 + \eta t) \, \theta l \, (3 + 6 \mu_1 + 3 \mu_1^2 + 32 \mu_2 + 32 \mu_1 \mu_2 + 24 \mu_2^2 - \\
& \quad 5 \, \mathfrak{e}1 - 4 \mu_1 \, \mathfrak{e}1 + \mu_1^2 \, \mathfrak{e}1 + 12 \mu_1 \mu_2 \, \mathfrak{e}1 + \\
& \quad \theta p \, (-14 - 7 \, \mathfrak{e}1 - 5 \, \mathfrak{e}1^2 - 7 \, \mathfrak{e}2 + 5 \, \mathfrak{e}1 \, \mathfrak{e}2 - 4 \mu_2^2 \, (9 \, \mathfrak{e}1 + 7 \times (2 + \, \mathfrak{e}2)) - \\
& \quad \quad \mu_2 \, (5 \, \mathfrak{e}1^2 - 5 \, \mathfrak{e}1 \, (-9 + \, \mathfrak{e}2) + 37 \times (2 + \, \mathfrak{e}2)) + \mu_1^2 \, (\mathfrak{e}1^2 - \\
& \quad \quad \quad 7 \times (2 + \, \mathfrak{e}2) - \, \mathfrak{e}1 \, (19 + \, \mathfrak{e}2)) - \mu_1 \, (28 + 26 \, \mathfrak{e}1 + 4 \, \mathfrak{e}1^2 + 14 \, \mathfrak{e}2 - \\
& \quad \quad \quad 4 \, \mathfrak{e}1 \, \mathfrak{e}2 + \mu_2 \, (74 + 69 \, \mathfrak{e}1 + 5 \, \mathfrak{e}1^2 + 37 \, \mathfrak{e}2 + 7 \, \mathfrak{e}1 \, \mathfrak{e}2)))) + \\
& \eta^2 \, (-4 \, \theta p \, (\eta t \, (-64 + 15 \mu_2^2 - 55 \, \mathfrak{e}1 - 37 \mu_1 \, (4 + 3 \, \mathfrak{e}1) - 3 \mu_2 \\
& \quad (13 + 7 \, \mathfrak{e}1) + 3 \mu_1 \mu_2 \, (-37 + 27 \, \mathfrak{e}1) + \mu_1^2 \, (-84 + 37 \, \mathfrak{e}1)) + \\
& \quad 2 \times (27 + 116 \mu_2 + 64 \mu_2^2 - 3 \mu_1^2 \, (-9 + \, \mathfrak{e}1) + 15 \, \mathfrak{e}1 + \\
& \quad \quad 8 \mu_2 \, \mathfrak{e}1 + 2 \mu_1 \, (27 + 6 \, \mathfrak{e}1 + \mu_2 \, (58 + 7 \, \mathfrak{e}1)))) + \\
& (-1 + \eta t) \, \theta l \, (-42 - 164 \mu_1 - 122 \mu_1^2 + 79 \mu_2 + 39 \mu_1 \mu_2 + \\
& \quad 108 \mu_2^2 - 70 \, \mathfrak{e}1 - 76 \mu_1 \, \mathfrak{e}1 - 18 \mu_1^2 \, \mathfrak{e}1 - 15 \mu_2 \, \mathfrak{e}1 + 105 \mu_1 \mu_2 \, \mathfrak{e}1 + \\
& \quad \theta p \, (-8 \mu_2^2 \, (74 + 36 \, \mathfrak{e}1 - 9 \, \mathfrak{e}2) - \mu_2 \, (950 + 395 \, \mathfrak{e}1 + 75 \, \mathfrak{e}1^2 + 171 \, \mathfrak{e}2 - \\
& \quad \quad 75 \, \mathfrak{e}1 \, \mathfrak{e}2) - 3 \times (50 + 27 \, \mathfrak{e}1 + 25 \, \mathfrak{e}1^2 + 7 \, \mathfrak{e}2 - 25 \, \mathfrak{e}1 \, \mathfrak{e}2) + \\
& \quad \quad \mu_1^2 \, (-130 + 5 \, \mathfrak{e}1^2 - 11 \, \mathfrak{e}2 - \, \mathfrak{e}1 \, (115 + 13 \, \mathfrak{e}2)) - \\
& \quad \quad \mu_1 \, (2 \times (140 + 62 \, \mathfrak{e}1 + 53 \, \mathfrak{e}1^2 + 16 \, \mathfrak{e}2 - 49 \, \mathfrak{e}1 \, \mathfrak{e}2) + \\
& \quad \quad \quad \mu_2 \, (950 + 443 \, \mathfrak{e}1 + 75 \, \mathfrak{e}1^2 + 171 \, \mathfrak{e}2 + 33 \, \mathfrak{e}1 \, \mathfrak{e}2)))) - 2 \\
& \eta^6 \, (-2 \times (-1 + \eta t) \, \theta l \, \mu_1 \, (9 + 28 \mu_2 + \, \mathfrak{e}1 + \mu_1 \, (9 + \, \mathfrak{e}1)) + \\
& \quad \theta p \, (-239 - 1028 \mu_1 - 789 \mu_1^2 - 408 \mu_2 - 1172 \mu_1 \mu_2 + \\
& \quad 756 \mu_2^2 - 27 \, \mathfrak{e}1 - 288 \mu_1 \, \mathfrak{e}1 - 123 \mu_1^2 \, \mathfrak{e}1 - 130 \mu_2 \, \mathfrak{e}1 + \\
& \quad 236 \mu_1 \mu_2 \, \mathfrak{e}1 - \theta l \, (212 + \mu_2 \, (702 + 6 \, \mathfrak{e}1 + 28 \, \mathfrak{e}2) + \\
& \quad \quad \mu_1^2 \, (159 + 40 \, \mathfrak{e}1 + 3 \, \mathfrak{e}1^2 + 27 \, \mathfrak{e}2 + 3 \, \mathfrak{e}1 \, \mathfrak{e}2) + \mu_1 \, (371 + 82 \, \mathfrak{e}1 + \\
& \quad \quad \quad 3 \, \mathfrak{e}1^2 + 27 \, \mathfrak{e}2 + 3 \, \mathfrak{e}1 \, \mathfrak{e}2 + \mu_2 \, (358 + 54 \, \mathfrak{e}1 + 84 \, \mathfrak{e}2))) +
\end{aligned}$$

$$\begin{aligned}
& \eta t (199 + 268 \mu_2 - 336 \mu_2^2 + 51 \mathfrak{e}1 - 10 \mu_1^2 (9 + \mathfrak{e}1) + \\
& \quad \mu_1 (109 + 41 \mathfrak{e}1 - 8 \mu_2 (50 + 9 \mathfrak{e}1)) + \\
& \quad \mathfrak{e}l (212 + \mu_2 (702 + 6 \mathfrak{e}1 + 28 \mathfrak{e}2) + \mu_1^2 (159 + 40 \mathfrak{e}1 + 3 \mathfrak{e}1^2 + \\
& \quad \quad 27 \mathfrak{e}2 + 3 \mathfrak{e}1 \mathfrak{e}2) + \mu_1 (371 + 82 \mathfrak{e}1 + 3 \mathfrak{e}1^2 + 27 \mathfrak{e}2 + \\
& \quad \quad 3 \mathfrak{e}1 \mathfrak{e}2 + \mu_2 (358 + 54 \mathfrak{e}1 + 84 \mathfrak{e}2))) - 2 \eta^5 \\
& (-2 \times (-1 + \eta t) \mathfrak{e}l (8 \mu_2 + \mu_1 (39 + 148 \mu_2 - 9 \mathfrak{e}1) + 3 \mu_1^2 (13 + \mathfrak{e}1)) + \\
& \quad \mathfrak{e}p (138 - 210 \mu_1 - 348 \mu_1^2 - 295 \mu_2 - 1643 \mu_1 \mu_2 - 1884 \mu_2^2 - \\
& \quad \quad 90 \mathfrak{e}1 - 84 \mu_1 \mathfrak{e}1 + 36 \mu_1^2 \mathfrak{e}1 - 233 \mu_2 \mathfrak{e}1 - 65 \mu_1 \mu_2 \mathfrak{e}1 - \\
& \quad \quad \mathfrak{e}l (24 \times (18 + \mathfrak{e}1) + \mu_2^2 (256 - 240 \mathfrak{e}2) + 2 \mu_2 (735 + 41 \mathfrak{e}1 + 36 \mathfrak{e}2) + \\
& \quad \quad \mu_1^2 (772 + 23 \mathfrak{e}1^2 + 107 \mathfrak{e}2 + \mathfrak{e}1 (87 + 11 \mathfrak{e}2)) + \\
& \quad \quad \mu_1 (1204 + 219 \mathfrak{e}1 + 59 \mathfrak{e}1^2 + 107 \mathfrak{e}2 - 25 \mathfrak{e}1 \mathfrak{e}2 + \\
& \quad \quad \mu_2 (2054 - 22 \mathfrak{e}1 + 316 \mathfrak{e}2 - 72 \mathfrak{e}1 \mathfrak{e}2))) + \\
& \quad \eta t (19 - 178 \mu_2 - 364 \mu_2^2 + 3 \mathfrak{e}1 + 20 \mu_2 \mathfrak{e}1 - 2 \mu_1^2 \\
& \quad \quad (175 + 19 \mathfrak{e}1) - \mu_1 (331 - 85 \mathfrak{e}1 + 2 \mu_2 (703 + 89 \mathfrak{e}1)) + \\
& \quad \quad \mathfrak{e}l (24 \times (18 + \mathfrak{e}1) + \mu_2^2 (256 - 240 \mathfrak{e}2) + 2 \mu_2 (735 + 41 \mathfrak{e}1 + \\
& \quad \quad \quad 36 \mathfrak{e}2) + \mu_1^2 (772 + 23 \mathfrak{e}1^2 + 107 \mathfrak{e}2 + \mathfrak{e}1 (87 + 11 \mathfrak{e}2)) + \\
& \quad \quad \mu_1 (1204 + 219 \mathfrak{e}1 + 59 \mathfrak{e}1^2 + 107 \mathfrak{e}2 - 25 \mathfrak{e}1 \mathfrak{e}2 + \\
& \quad \quad \mu_2 (2054 - 22 \mathfrak{e}1 + 316 \mathfrak{e}2 - 72 \mathfrak{e}1 \mathfrak{e}2)))) + \\
& w^2 (-1 + \eta)^2 (2 x^8 (-1 + \eta)^9 \mathfrak{e}p (\eta - \eta t + 4 \mu_1) (3 + 4 \mu_2 + \mathfrak{e}1 + \mu_1 (3 + \mathfrak{e}1)) - \\
& \quad x^7 (-1 + \eta)^7 \\
& \quad (4 \times (-1 + \eta t) \mathfrak{e}l (4 \mu_2 + \mu_1 (11 + 44 \mu_2 - 5 \mathfrak{e}1) + \mu_1^2 (11 + \mathfrak{e}1)) + \mathfrak{e}p \\
& \quad (-138 + 138 \mathfrak{e}l - 438 \mu_1 + 268 \mathfrak{e}l \mu_1 - 300 \mu_1^2 + \\
& \quad \quad 130 \mathfrak{e}l \mu_1^2 - 414 \mu_2 + 438 \mathfrak{e}l \mu_2 - 478 \mu_1 \mu_2 + \\
& \quad \quad 326 \mathfrak{e}l \mu_1 \mu_2 + 48 \mathfrak{e}l \mu_2^2 - 10 \mathfrak{e}1 + 10 \mathfrak{e}l \mathfrak{e}1 - 114 \mu_1 \mathfrak{e}1 + \\
& \quad \quad 41 \mathfrak{e}l \mu_1 \mathfrak{e}1 - 68 \mu_1^2 \mathfrak{e}1 + 7 \mathfrak{e}l \mu_1^2 \mathfrak{e}1 - 22 \mu_2 \mathfrak{e}1 + \\
& \quad \quad 14 \mathfrak{e}l \mu_2 \mathfrak{e}1 + 14 \mu_1 \mu_2 \mathfrak{e}1 - 26 \mathfrak{e}l \mu_1 \mu_2 \mathfrak{e}1 + 9 \mathfrak{e}l \mu_1 \mathfrak{e}1^2 + \\
& \quad \quad 3 \mathfrak{e}l \mu_1^2 \mathfrak{e}1^2 + 16 \eta^3 (3 + 4 \mu_2 + \mathfrak{e}1 + \mu_1 (3 + \mathfrak{e}1)) - \\
& \quad \quad 2 \eta^2 (-15 - 26 \mu_2 + 28 \mu_2^2 - 3 \mathfrak{e}1 - 32 \mu_1^2 (3 + \mathfrak{e}1) + \mu_1 (-111 - \\
& \quad \quad \quad 118 \mu_2 - 35 \mathfrak{e}1 + 6 \mu_2 \mathfrak{e}1) + 8 \eta t (3 + 4 \mu_2 + \mathfrak{e}1 + \mu_1 (3 + \mathfrak{e}1))) + \\
& \quad \quad 2 \eta (30 + 149 \mu_2 + 28 \mu_2^2 - 6 \mathfrak{e}1 + 11 \mu_2 \mathfrak{e}1 + 2 \mu_1^2 (27 + \mathfrak{e}1) + \\
& \quad \quad \mu_1 (-\mu_2 (-121 + \mathfrak{e}1) + 14 \times (6 + \mathfrak{e}1)) + \eta t (-26 \mu_2 + 28 \mu_2^2 - \\
& \quad \quad \quad 3 \times (5 + \mathfrak{e}1) - 3 \mu_1 (5 + \mathfrak{e}1) + 2 \mu_1 \mu_2 (5 + 3 \mathfrak{e}1))) + \\
& \quad \quad 11 \mathfrak{e}l \mu_1 \mathfrak{e}2 + 11 \mathfrak{e}l \mu_1^2 \mathfrak{e}2 + 16 \mathfrak{e}l \mu_2 \mathfrak{e}2 + 32 \mathfrak{e}l \mu_1 \mu_2 \mathfrak{e}2 - \\
& \quad \quad 40 \mathfrak{e}l \mu_2^2 \mathfrak{e}2 - 5 \mathfrak{e}l \mu_1 \mathfrak{e}1 \mathfrak{e}2 + \mathfrak{e}l \mu_1^2 \mathfrak{e}1 \mathfrak{e}2 - 12 \mathfrak{e}l \mu_1 \mu_2 \mathfrak{e}1 \mathfrak{e}2 - \\
& \quad \quad \eta t (-78 - 116 \mu_2 + 56 \mu_2^2 - 22 \mathfrak{e}1 + 2 \mu_1 (-39 - 11 \mathfrak{e}1 + 2 \mu_2 (5 + 3 \mathfrak{e}1)) + \\
& \quad \quad \mathfrak{e}l \mu_1^2 (130 + 3 \mathfrak{e}1^2 + 11 \mathfrak{e}2 + \mathfrak{e}1 (7 + \mathfrak{e}2)) + \\
& \quad \quad 2 \mathfrak{e}l (69 + 5 \mathfrak{e}1 - 4 \mu_2^2 (-6 + 5 \mathfrak{e}2) + \mu_2 (219 + 7 \mathfrak{e}1 + 8 \mathfrak{e}2)) + \\
& \quad \quad \mathfrak{e}l \mu_1 (268 + 9 \mathfrak{e}1^2 + \mathfrak{e}1 (41 - 5 \mathfrak{e}2) + 11 \mathfrak{e}2 + \\
& \quad \quad \mu_2 (326 + 32 \mathfrak{e}2 - 2 \mathfrak{e}1 (13 + 6 \mathfrak{e}2)))) - \\
& x^5 (-1 + \eta)^5 ((-1 + \eta) \mathfrak{e}p (112 \eta^4 (3 + 4 \mu_2 + \mathfrak{e}1 + \mu_1 (3 + \mathfrak{e}1)) + \\
& \quad 2 \times (219 + 704 \mu_2^2 + 83 \mathfrak{e}1 + \mu_1^2 (450 + 38 \mathfrak{e}1) + \\
& \quad \quad \mu_2 (833 + 145 \mathfrak{e}1) + \mu_1 (669 + \mu_2 (1169 - 41 \mathfrak{e}1) + 175 \mathfrak{e}1)) - \\
& \quad 14 \eta^3 (3 \times (-39 - 58 \mu_2 + 28 \mu_2^2 - 11 \mathfrak{e}1) - 32 \mu_1^2 (3 + \mathfrak{e}1) +
\end{aligned}$$

$$\begin{aligned}
& \mu_1 (-213 - 98 \mu_2 - 65 \mathfrak{e}_1 + 18 \mu_2 \mathfrak{e}_1) + \\
& 8 \eta t (3 + 4 \mu_2 + \mathfrak{e}_1 + \mu_1 (3 + \mathfrak{e}_1)) + \\
& \eta t (516 \mu_2^2 - 6 \times (39 + 17 \mathfrak{e}_1) - \mu_2 (113 + 35 \mathfrak{e}_1) + 4 \mu_1^2 \\
& \quad (68 + 37 \mathfrak{e}_1) + \mu_1 (38 - 218 \mathfrak{e}_1 + \mu_2 (927 + 265 \mathfrak{e}_1))) + \\
& 6 \eta^2 (693 + 1689 \mu_2 - 608 \mu_2^2 + 85 \mathfrak{e}_1 + 77 \mu_2 \mathfrak{e}_1 + 14 \mu_1^2 (75 + 17 \mathfrak{e}_1) + \\
& \quad \mu_1 (1743 + 1473 \mu_2 + 449 \mathfrak{e}_1 - 169 \mu_2 \mathfrak{e}_1) + 7 \eta t (-39 - 58 \mu_2 + \\
& \quad 28 \mu_2^2 - 11 \mathfrak{e}_1 + \mu_1 (-39 + 10 \mu_2 - 11 \mathfrak{e}_1 + 6 \mu_2 \mathfrak{e}_1))) + \\
& 2 \eta (1275 + 3770 \mu_2 + 700 \mu_2^2 + 255 \mathfrak{e}_1 + 512 \mu_2 \mathfrak{e}_1 + 48 \mu_1^2 \\
& \quad (51 + 8 \mathfrak{e}_1) + \mu_1 (3723 + 4622 \mu_2 + 963 \mathfrak{e}_1 - 346 \mu_2 \mathfrak{e}_1) + \\
& \quad 2 \eta t (-279 + 588 \mu_2^2 - 75 \mathfrak{e}_1 - 6 \mu_2 (46 + \mathfrak{e}_1) + \\
& \quad \mu_1^2 (113 + 13 \mathfrak{e}_1) + 2 \mu_1 (-83 - 49 \mathfrak{e}_1 + 6 \mu_2 (51 + 13 \mathfrak{e}_1))) - \\
& (-1 + \eta t) \mathfrak{e} l (-2 \times (84 \mu_2^2 + \mu_2 (7 - 15 \mathfrak{e}_1) - 90 \times (1 + \mathfrak{e}_1) + \\
& \quad \mu_1^2 (-80 + 84 \mathfrak{e}_1) + \mu_1 \mu_2 (-9 + 93 \mathfrak{e}_1) - 2 \mu_1 (85 + 96 \mathfrak{e}_1)) + \\
& \mathfrak{e} p (258 + 67 \mathfrak{e}_1 + 45 \mathfrak{e}_1^2 + 4 \mu_2^2 (118 + 27 \mathfrak{e}_1 - 91 \mathfrak{e}_2) - 9 \mathfrak{e}_2 - \\
& \quad 45 \mathfrak{e}_1 \mathfrak{e}_2 + \mu_2 (1146 + 237 \mathfrak{e}_1 + 45 \mathfrak{e}_1^2 + 37 \mathfrak{e}_2 - 45 \mathfrak{e}_1 \mathfrak{e}_2) + \\
& \quad \mu_1^2 (512 + 11 \mathfrak{e}_1^2 + 31 \mathfrak{e}_2 + \mathfrak{e}_1 (37 + 9 \mathfrak{e}_2)) + \\
& \quad \mu_1 (770 + 92 \mathfrak{e}_1 + 116 \mathfrak{e}_1^2 + 22 \mathfrak{e}_2 - 96 \mathfrak{e}_1 \mathfrak{e}_2 + \\
& \quad \mu_2 (1834 + 45 \mathfrak{e}_1^2 + 165 \mathfrak{e}_2 - 3 \mathfrak{e}_1 (9 + 19 \mathfrak{e}_2))) + \\
& \eta^2 (-40 \times (6 \mu_2 + \mu_1 (25 + 96 \mu_2 - 7 \mathfrak{e}_1) + \mu_1^2 (25 + 2 \mathfrak{e}_1)) + \\
& \quad 3 \mathfrak{e} p (\mu_1^2 (962 + 23 \mathfrak{e}_1^2 + 103 \mathfrak{e}_2 + \mathfrak{e}_1 (79 + 9 \mathfrak{e}_2)) + \\
& \quad \mu_1 (1976 + 65 \mathfrak{e}_1^2 + \mathfrak{e}_1 (317 - 33 \mathfrak{e}_2) + 103 \mathfrak{e}_2 + \\
& \quad 26 \mu_2 (95 + 12 \mathfrak{e}_2) - 6 \mu_2 \mathfrak{e}_1 (19 + 14 \mathfrak{e}_2)) + 2 \times (507 + \\
& \quad 35 \mathfrak{e}_1 - 4 \mu_2^2 (-38 + 35 \mathfrak{e}_2) + \mu_2 (1635 + 51 \mathfrak{e}_1 + 56 \mathfrak{e}_2))) + \\
& \eta (408 + 197 \mu_2 + 84 \mu_2^2 + 300 \mathfrak{e}_1 + 75 \mu_2 \mathfrak{e}_1 - 4 \mu_1^2 (126 + \\
& \quad 97 \mathfrak{e}_1) - \mu_1 (96 - 980 \mathfrak{e}_1 + 3 \mu_2 (889 + 95 \mathfrak{e}_1)) + \\
& \quad \mathfrak{e} p (\mu_1^2 (67 \mathfrak{e}_1^2 + 31 \mathfrak{e}_1 (3 + \mathfrak{e}_2) + 7 \times (374 + 25 \mathfrak{e}_2)) + \\
& \quad \mu_1 (4526 + 519 \mathfrak{e}_1 + 373 \mathfrak{e}_1^2 + 97 \mathfrak{e}_2 - 275 \mathfrak{e}_1 \mathfrak{e}_2 + \\
& \quad \mu_2 (7810 - 668 \mathfrak{e}_1 + 90 \mathfrak{e}_1^2 + 614 \mathfrak{e}_2 - 306 \mathfrak{e}_1 \mathfrak{e}_2)) + 2 \times \\
& \quad (954 + 105 \mathfrak{e}_1 + 45 \mathfrak{e}_1^2 + 2 \mu_2^2 (314 + 9 \mathfrak{e}_1 - 387 \mathfrak{e}_2) - 39 \mathfrak{e}_2 - 45 \\
& \quad \mathfrak{e}_1 \mathfrak{e}_2 + \mu_2 (3381 + 226 \mathfrak{e}_1 + 45 \mathfrak{e}_1^2 - 3 \mathfrak{e}_2 - 45 \mathfrak{e}_1 \mathfrak{e}_2)))) + \\
& \eta \mathfrak{e} p (2 \eta^9 (3 + 4 \mu_2 + \mathfrak{e}_1 + \mu_1 (3 + \mathfrak{e}_1)) - \eta t \mu_2 (11 + 8 \mu_2 + 5 \mathfrak{e}_1 + \\
& \quad \mu_1 (11 + 5 \mathfrak{e}_1)) - \eta \eta t (24 + 224 \mu_2^2 - 40 \mathfrak{e}_1 + 8 \mu_1^2 \mathfrak{e}_1 + \\
& \quad \mu_2 (267 + 5 \mathfrak{e}_1) + \mu_1 (24 - 44 \mathfrak{e}_1 + \mu_2 (267 + 77 \mathfrak{e}_1))) - 2 \eta^8 \\
& \quad (\eta t (3 + 4 \mu_2 + \mathfrak{e}_1 + \mu_1 (3 + \mathfrak{e}_1)) - 2 \times (18 + 27 \mu_2 - 14 \mu_2^2 + 5 \mathfrak{e}_1 + \\
& \quad 2 \mu_1^2 (3 + \mathfrak{e}_1) + \mu_1 (24 + 3 \mu_2 + 7 \mathfrak{e}_1 - 3 \mu_2 \mathfrak{e}_1))) + 2 \eta^7 \\
& \quad (135 + 269 \mu_2 - 276 \mu_2^2 + 19 \mathfrak{e}_1 + 11 \mu_2 \mathfrak{e}_1 + 6 \mu_1^2 (23 + 5 \mathfrak{e}_1) + \\
& \quad \mu_1 (273 + 133 \mu_2 + 67 \mathfrak{e}_1 - 61 \mu_2 \mathfrak{e}_1) + \\
& \quad 2 \eta t (-18 - 27 \mu_2 + 14 \mu_2^2 - 5 \mathfrak{e}_1 + \mu_1 (-18 + 5 \mu_2 - 5 \mathfrak{e}_1 + 3 \mu_2 \mathfrak{e}_1))) - \\
& \eta^4 (12 \times (24 - 4 \mu_2^2 + 5 \mathfrak{e}_1 + 6 \mu_1^2 (7 + \mathfrak{e}_1) + \mu_2 (67 + 13 \mathfrak{e}_1) + \\
& \quad \mu_1 (66 + \mu_2 (79 - 17 \mathfrak{e}_1) + 17 \mathfrak{e}_1)) - \\
& \quad \mathfrak{e} l (330 + 91 \mathfrak{e}_1 + 45 \mathfrak{e}_1^2 + 4 \mu_2^2 (134 + 45 \mathfrak{e}_1 - 73 \mathfrak{e}_2) + 15 \mathfrak{e}_2 - \\
& \quad 45 \mathfrak{e}_1 \mathfrak{e}_2 + \mu_2 (1476 + 331 \mathfrak{e}_1 + 45 \mathfrak{e}_1^2 + 133 \mathfrak{e}_2 - 45 \mathfrak{e}_1 \mathfrak{e}_2) + \\
& \quad 2 \mu_1^2 (291 + 5 \mathfrak{e}_1^2 + 33 \mathfrak{e}_2 + \mathfrak{e}_1 (35 + 4 \mathfrak{e}_2)) +
\end{aligned}$$

$$\begin{aligned}
& \mu_1 (912 + 149 \, \mathfrak{e}_1 + 115 \, \mathfrak{e}_1^2 + 81 \, \mathfrak{e}_2 - 97 \, \mathfrak{e}_1 \, \mathfrak{e}_2 + \\
& \quad \mu_2 (2172 + 131 \, \mathfrak{e}_1 + 45 \, \mathfrak{e}_1^2 + 313 \, \mathfrak{e}_2 - 57 \, \mathfrak{e}_1 \, \mathfrak{e}_2)) + \\
& \eta t (3 \times (-14 + 24 \, \mu_2^2 + 5 \, \mu_2 (-17 + \mathfrak{e}_1) - 12 \, \mu_1^2 (-11 + \mathfrak{e}_1) + \\
& \quad 30 \, \mathfrak{e}_1 + \mu_1 (118 + \mu_2 (235 - 19 \, \mathfrak{e}_1) + 54 \, \mathfrak{e}_1)) + \\
& \quad \theta l (330 + 91 \, \mathfrak{e}_1 + 45 \, \mathfrak{e}_1^2 + 4 \, \mu_2^2 (134 + 45 \, \mathfrak{e}_1 - 73 \, \mathfrak{e}_2) + 15 \, \mathfrak{e}_2 - \\
& \quad 45 \, \mathfrak{e}_1 \, \mathfrak{e}_2 + \mu_2 (1476 + 331 \, \mathfrak{e}_1 + 45 \, \mathfrak{e}_1^2 + 133 \, \mathfrak{e}_2 - 45 \, \mathfrak{e}_1 \, \mathfrak{e}_2) + \\
& \quad 2 \, \mu_1^2 (291 + 5 \, \mathfrak{e}_1^2 + 33 \, \mathfrak{e}_2 + \mathfrak{e}_1 (35 + 4 \, \mathfrak{e}_2)) + \\
& \quad \mu_1 (912 + 149 \, \mathfrak{e}_1 + 115 \, \mathfrak{e}_1^2 + 81 \, \mathfrak{e}_2 - 97 \, \mathfrak{e}_1 \, \mathfrak{e}_2 + \\
& \quad \mu_2 (2172 + 131 \, \mathfrak{e}_1 + 45 \, \mathfrak{e}_1^2 + 313 \, \mathfrak{e}_2 - 57 \, \mathfrak{e}_1 \, \mathfrak{e}_2))) + \eta^5 \\
& (2 \times (-45 + 732 \, \mu_2^2 + \mu_1^2 (42 - 26 \, \mathfrak{e}_1) + 29 \, \mathfrak{e}_1 + \mu_2 (200 + 58 \, \mathfrak{e}_1) + \\
& \quad \mu_1 (-3 + 508 \, \mu_2 + 3 \, \mathfrak{e}_1 + 64 \, \mu_2 \, \mathfrak{e}_1)) + \\
& \quad 3 \, \theta l (126 + 15 \, \mathfrak{e}_1 + 5 \, \mathfrak{e}_1^2 + 4 \, \mu_2^2 (18 + 3 \, \mathfrak{e}_1 - 19 \, \mathfrak{e}_2) - \mathfrak{e}_2 - \\
& \quad 5 \, \mathfrak{e}_1 \, \mathfrak{e}_2 + \mu_2 (464 + 39 \, \mathfrak{e}_1 + 5 \, \mathfrak{e}_1^2 + 13 \, \mathfrak{e}_2 - 5 \, \mathfrak{e}_1 \, \mathfrak{e}_2) + \\
& \quad 2 \, \mu_1^2 (83 + 2 \, \mathfrak{e}_1^2 + 10 \, \mathfrak{e}_2 + \mathfrak{e}_1 (8 + \mathfrak{e}_2)) + \mu_1 (292 + 43 \, \mathfrak{e}_1 + 21 \, \mathfrak{e}_1^2 + \\
& \quad 19 \, \mathfrak{e}_2 - 15 \, \mathfrak{e}_1 \, \mathfrak{e}_2 + \mu_2 (520 - \mathfrak{e}_1 + 5 \, \mathfrak{e}_1^2 + 73 \, \mathfrak{e}_2 - 17 \, \mathfrak{e}_1 \, \mathfrak{e}_2))) - \\
& \eta t (36 - 108 \, \mu_1 - 144 \, \mu_1^2 - 119 \, \mu_2 - 911 \, \mu_1 \, \mu_2 - 160 \, \mu_2^2 + \\
& \quad 52 \, \mathfrak{e}_1 + 156 \, \mu_1 \, \mathfrak{e}_1 - 64 \, \mu_1^2 \, \mathfrak{e}_1 + 31 \, \mu_2 \, \mathfrak{e}_1 - 161 \, \mu_1 \, \mu_2 \, \mathfrak{e}_1 + \\
& \quad 3 \, \theta l (126 + 15 \, \mathfrak{e}_1 + 5 \, \mathfrak{e}_1^2 + 4 \, \mu_2^2 (18 + 3 \, \mathfrak{e}_1 - 19 \, \mathfrak{e}_2) - \mathfrak{e}_2 - 5 \, \mathfrak{e}_1 \, \mathfrak{e}_2 + \\
& \quad \mu_2 (464 + 39 \, \mathfrak{e}_1 + 5 \, \mathfrak{e}_1^2 + 13 \, \mathfrak{e}_2 - 5 \, \mathfrak{e}_1 \, \mathfrak{e}_2) + 2 \, \mu_1^2 (83 + 2 \, \mathfrak{e}_1^2 + \\
& \quad 10 \, \mathfrak{e}_2 + \mathfrak{e}_1 (8 + \mathfrak{e}_2)) + \mu_1 (292 + 43 \, \mathfrak{e}_1 + 21 \, \mathfrak{e}_1^2 + 19 \, \mathfrak{e}_2 - \\
& \quad 15 \, \mathfrak{e}_1 \, \mathfrak{e}_2 + \mu_2 (520 - \mathfrak{e}_1 + 5 \, \mathfrak{e}_1^2 + 73 \, \mathfrak{e}_2 - 17 \, \mathfrak{e}_1 \, \mathfrak{e}_2))) - 2 \\
& \eta^6 (-2 \times (63 + 199 \, \mu_2 - 38 \, \mu_2^2 - 37 \, \mu_1 \, \mu_2 (-7 + \mathfrak{e}_1) + 15 \, \mathfrak{e}_1 + \\
& \quad 38 \, \mu_2 \, \mathfrak{e}_1 + 48 \, \mu_1 (4 + \mathfrak{e}_1) + 3 \, \mu_1^2 (43 + 5 \, \mathfrak{e}_1)) - \\
& \quad \theta l (81 + 5 \, \mathfrak{e}_1 - 4 \, \mu_2^2 (-4 + 5 \, \mathfrak{e}_2) + \mu_2 (270 + 8 \, \mathfrak{e}_1 + 8 \, \mathfrak{e}_2) + \\
& \quad \mu_1^2 (78 + 2 \, \mathfrak{e}_1^2 + 12 \, \mathfrak{e}_2 + \mathfrak{e}_1 (11 + \mathfrak{e}_2)) + \mu_1 (159 + 28 \, \mathfrak{e}_1 + \\
& \quad 5 \, \mathfrak{e}_1^2 + 12 \, \mathfrak{e}_2 - 2 \, \mathfrak{e}_1 \, \mathfrak{e}_2 + \mu_2 (210 + 4 \, \mathfrak{e}_1 + 38 \, \mathfrak{e}_2 - 6 \, \mathfrak{e}_1 \, \mathfrak{e}_2))) + \\
& \eta t (2 \times (27 - 84 \, \mu_2^2 + 7 \, \mathfrak{e}_1 - 3 \, \mu_1^2 (11 + \mathfrak{e}_1) + \mu_2 (17 + \mathfrak{e}_1) - \\
& \quad \mu_1 (6 - 10 \, \mathfrak{e}_1 + \mu_2 (147 + 23 \, \mathfrak{e}_1))) + \\
& \quad \theta l (81 + 5 \, \mathfrak{e}_1 - 4 \, \mu_2^2 (-4 + 5 \, \mathfrak{e}_2) + \mu_2 (270 + 8 \, \mathfrak{e}_1 + 8 \, \mathfrak{e}_2) + \\
& \quad \mu_1^2 (78 + 2 \, \mathfrak{e}_1^2 + 12 \, \mathfrak{e}_2 + \mathfrak{e}_1 (11 + \mathfrak{e}_2)) + \mu_1 (159 + 28 \, \mathfrak{e}_1 + 5 \, \mathfrak{e}_1^2 + \\
& \quad 12 \, \mathfrak{e}_2 - 2 \, \mathfrak{e}_1 \, \mathfrak{e}_2 + \mu_2 (210 + 4 \, \mathfrak{e}_1 + 38 \, \mathfrak{e}_2 - 6 \, \mathfrak{e}_1 \, \mathfrak{e}_2))) - \eta^3 \\
& (2 \times (93 + 344 \, \mu_2^2 + 49 \, \mathfrak{e}_1 + 4 \, \mu_1^2 (45 + \mathfrak{e}_1) + \mu_2 (441 + 61 \, \mathfrak{e}_1) + \\
& \quad \mu_1 (273 + 71 \, \mathfrak{e}_1 + \mu_2 (609 + 19 \, \mathfrak{e}_1))) - \\
& \quad 3 \, \theta l (58 + 29 \, \mathfrak{e}_1 + 15 \, \mathfrak{e}_1^2 + 4 \, \mu_2^2 (46 + 21 \, \mathfrak{e}_1 - 5 \, \mathfrak{e}_2) + 13 \, \mathfrak{e}_2 - \\
& \quad 15 \, \mathfrak{e}_1 \, \mathfrak{e}_2 + \mu_2 (312 + 125 \, \mathfrak{e}_1 + 15 \, \mathfrak{e}_1^2 + 71 \, \mathfrak{e}_2 - 15 \, \mathfrak{e}_1 \, \mathfrak{e}_2) + \\
& \quad 2 \, \mu_1^2 (49 + 8 \, \mathfrak{e}_2 + \mathfrak{e}_1 (14 + \mathfrak{e}_2)) + \mu_1 (156 + 45 \, \mathfrak{e}_1 + 27 \, \mathfrak{e}_1^2 + 29 \, \mathfrak{e}_2 - \\
& \quad 25 \, \mathfrak{e}_1 \, \mathfrak{e}_2 + \mu_2 (448 + 101 \, \mathfrak{e}_1 + 15 \, \mathfrak{e}_1^2 + 91 \, \mathfrak{e}_2 - 3 \, \mathfrak{e}_1 \, \mathfrak{e}_2))) + \\
& \eta t (4 \times (-33 - 2 \, \mu_2^2 - 8 \, \mathfrak{e}_1 - \mu_2 (64 + 9 \, \mathfrak{e}_1) + \mu_1^2 (20 + 22 \, \mathfrak{e}_1) + \\
& \quad \mu_1 (-13 - 37 \, \mathfrak{e}_1 + 2 \, \mu_2 (55 + 12 \, \mathfrak{e}_1))) + \\
& \quad 3 \, \theta l (58 + 29 \, \mathfrak{e}_1 + 15 \, \mathfrak{e}_1^2 + 4 \, \mu_2^2 (46 + 21 \, \mathfrak{e}_1 - 5 \, \mathfrak{e}_2) + 13 \, \mathfrak{e}_2 - \\
& \quad 15 \, \mathfrak{e}_1 \, \mathfrak{e}_2 + \mu_2 (312 + 125 \, \mathfrak{e}_1 + 15 \, \mathfrak{e}_1^2 + 71 \, \mathfrak{e}_2 - 15 \, \mathfrak{e}_1 \, \mathfrak{e}_2) + 2 \, \mu_1^2 \\
& \quad (49 + 8 \, \mathfrak{e}_2 + \mathfrak{e}_1 (14 + \mathfrak{e}_2)) + \mu_1 (156 + 45 \, \mathfrak{e}_1 + 27 \, \mathfrak{e}_1^2 + 29 \, \mathfrak{e}_2 -
\end{aligned}$$

$$\begin{aligned}
& 25 \, \mathfrak{e}1 \, \mathfrak{e}2 + \mu2 \left( 448 + 101 \, \mathfrak{e}1 + 15 \, \mathfrak{e}1^2 + 91 \, \mathfrak{e}2 - 3 \, \mathfrak{e}1 \, \mathfrak{e}2 \right) \Big) \Big) \Big) + \\
& \eta^2 \left( -4 \times \left( 9 + 16 \, \mu2^2 - \mu1^2 \left( -9 + \mathfrak{e}1 \right) + 5 \, \mathfrak{e}1 + \mu2 \left( 41 + 3 \, \mathfrak{e}1 \right) + \right. \right. \\
& \quad \left. \left. \mu1 \left( 18 + 4 \, \mathfrak{e}1 + \mu2 \left( 41 + 3 \, \mathfrak{e}1 \right) \right) \right) \right) + \\
& \, \mathfrak{e}l \left( 60 + 31 \, \mathfrak{e}1 + 15 \, \mathfrak{e}1^2 + 21 \, \mathfrak{e}2 - 15 \, \mathfrak{e}1 \, \mathfrak{e}2 + 4 \, \mu2^2 \left( 50 + 27 \, \mathfrak{e}1 + 11 \, \mathfrak{e}2 \right) + \right. \\
& \quad \left. \mu2 \left( 312 + 145 \, \mathfrak{e}1 + 15 \, \mathfrak{e}1^2 + 103 \, \mathfrak{e}2 - 15 \, \mathfrak{e}1 \, \mathfrak{e}2 \right) + \right. \\
& \quad \left. \mu1^2 \left( -2 \, \mathfrak{e}1^2 + 18 \times \left( 3 + \mathfrak{e}2 \right) + 2 \, \mathfrak{e}1 \left( 20 + \mathfrak{e}2 \right) \right) + \right. \\
& \quad \left. \mu1 \left( 114 + 59 \, \mathfrak{e}1 + 19 \, \mathfrak{e}1^2 + 39 \, \mathfrak{e}2 - 19 \, \mathfrak{e}1 \, \mathfrak{e}2 + \right. \right. \\
& \quad \left. \left. \mu2 \left( 312 + 161 \, \mathfrak{e}1 + 15 \, \mathfrak{e}1^2 + 103 \, \mathfrak{e}2 + 9 \, \mathfrak{e}1 \, \mathfrak{e}2 \right) \right) \right) \Big) + \\
& \, \eta t \left( -4 \times \left( 64 \, \mu2^2 - 6 \, \mu2 \left( -7 + \mathfrak{e}1 \right) + \mu1^2 \left( -50 + 4 \, \mathfrak{e}1 \right) - \right. \right. \\
& \quad \left. \left. 6 \times \left( 3 + 5 \, \mathfrak{e}1 \right) + \mu1 \left( -68 - 47 \, \mathfrak{e}1 + 12 \, \mu2 \left( 2 + 3 \, \mathfrak{e}1 \right) \right) \right) \right) + \\
& \, \mathfrak{e}l \left( -60 - 31 \, \mathfrak{e}1 - 15 \, \mathfrak{e}1^2 - 21 \, \mathfrak{e}2 + 15 \, \mathfrak{e}1 \, \mathfrak{e}2 - 4 \, \mu2^2 \right. \\
& \quad \left( 50 + 27 \, \mathfrak{e}1 + 11 \, \mathfrak{e}2 \right) - \mu2 \left( 312 + 145 \, \mathfrak{e}1 + 15 \, \mathfrak{e}1^2 + 103 \, \mathfrak{e}2 - \right. \\
& \quad \left. 15 \, \mathfrak{e}1 \, \mathfrak{e}2 \right) + 2 \, \mu1^2 \left( \mathfrak{e}1^2 - 9 \times \left( 3 + \mathfrak{e}2 \right) - \mathfrak{e}1 \left( 20 + \mathfrak{e}2 \right) \right) - \\
& \quad \left. \mu1 \left( 114 + 59 \, \mathfrak{e}1 + 19 \, \mathfrak{e}1^2 + 39 \, \mathfrak{e}2 - 19 \, \mathfrak{e}1 \, \mathfrak{e}2 + \right. \right. \\
& \quad \left. \left. \mu2 \left( 312 + 161 \, \mathfrak{e}1 + 15 \, \mathfrak{e}1^2 + 103 \, \mathfrak{e}2 + 9 \, \mathfrak{e}1 \, \mathfrak{e}2 \right) \right) \right) \Big) \Big) \Big) - \\
& \times \left( -1 + \eta \right) \times \left( 16 \, \eta^9 \, \mathfrak{e}p \left( 3 + 4 \, \mu2 + \mathfrak{e}1 + \mu1 \left( 3 + \mathfrak{e}1 \right) \right) - 2 \, \eta^8 \, \mathfrak{e}p \right. \\
& \quad \left( -249 - 374 \, \mu2 + 196 \, \mu2^2 - 69 \, \mathfrak{e}1 - 32 \, \mu1^2 \left( 3 + \mathfrak{e}1 \right) + \right. \\
& \quad \left. \mu1 \left( -345 - 58 \, \mu2 - 101 \, \mathfrak{e}1 + 42 \, \mu2 \, \mathfrak{e}1 \right) + \right. \\
& \quad \left. 8 \, \eta t \left( 3 + 4 \, \mu2 + \mathfrak{e}1 + \mu1 \left( 3 + \mathfrak{e}1 \right) \right) \right) - \eta t \, \mathfrak{e}p \\
& \quad \left( 4 + 4 \, \mu1^2 + 20 \, \mu2^2 + \mu2 \left( 27 + 5 \, \mathfrak{e}1 \right) + \mu1 \left( 8 + \mu2 \left( 27 + 5 \, \mathfrak{e}1 \right) \right) \right) \Big) + 2 \\
& \, \eta^7 \, \mathfrak{e}p \left( 840 + 1763 \, \mu2 - 1628 \, \mu2^2 + 108 \, \mathfrak{e}1 + 77 \, \mu2 \, \mathfrak{e}1 + \right. \\
& \quad \left. \mu1^2 \left( 954 + 206 \, \mathfrak{e}1 \right) + \mu1 \left( 1794 + 1015 \, \mu2 + 440 \, \mathfrak{e}1 - 367 \, \mu2 \, \mathfrak{e}1 \right) + \right. \\
& \quad \left. \eta t \left( -249 - 374 \, \mu2 + 196 \, \mu2^2 - 69 \, \mathfrak{e}1 + \right. \right. \\
& \quad \left. \left. \mu1 \left( -249 + 70 \, \mu2 - 69 \, \mathfrak{e}1 + 42 \, \mu2 \, \mathfrak{e}1 \right) \right) \right) \Big) - \eta \\
& \left( \left( -1 + \eta t \right) \, \mathfrak{e}l \left( 4 + 4 \, \mu1^2 + 5 \, \mu2 + 4 \, \mu2^2 - 5 \, \mu2 \, \mathfrak{e}1 + \mu1 \left( 8 + 5 \, \mu2 - 5 \, \mu2 \, \mathfrak{e}1 \right) \right) + \right. \\
& \quad \left. \eta t \, \mathfrak{e}p \left( 76 + 657 \, \mu2 + 540 \, \mu2^2 - 80 \, \mathfrak{e}1 + 15 \, \mu2 \, \mathfrak{e}1 + 4 \, \mu1^2 \left( 12 + 7 \, \mathfrak{e}1 \right) + \right. \right. \\
& \quad \left. \left. \mu1 \left( 124 + 665 \, \mu2 - 88 \, \mathfrak{e}1 + 159 \, \mu2 \, \mathfrak{e}1 \right) \right) \right) \Big) + \eta^6 \\
& \left( 8 \times \left( -1 + \eta t \right) \, \mathfrak{e}l \left( 2 \, \mu2 + 2 \, \mu1 \left( 7 + 26 \, \mu2 - \mathfrak{e}1 \right) + \mu1^2 \left( 14 + \mathfrak{e}1 \right) \right) + \right. \\
& \quad \mathfrak{e}p \left( 1164 + 3960 \, \mu1 + 2796 \, \mu1^2 + 4130 \, \mu2 + 6010 \, \mu1 \, \mu2 + 280 \, \mu2^2 + \right. \\
& \quad \left. 308 \, \mathfrak{e}1 + 996 \, \mu1 \, \mathfrak{e}1 + 292 \, \mu1^2 \, \mathfrak{e}1 + 886 \, \mu2 \, \mathfrak{e}1 - 674 \, \mu1 \, \mu2 \, \mathfrak{e}1 + \right. \\
& \quad \left. \mathfrak{e}l \left( \mu1^2 \left( 1066 + 27 \, \mathfrak{e}1^2 + 155 \, \mathfrak{e}2 + \mathfrak{e}1 \left( 139 + 13 \, \mathfrak{e}2 \right) \right) + 2 \times \right. \\
& \quad \left( 555 + 35 \, \mathfrak{e}1 - 20 \, \mu2^2 \left( -6 + 7 \, \mathfrak{e}2 \right) + \mu2 \left( 1839 + 55 \, \mathfrak{e}1 + 56 \, \mathfrak{e}2 \right) \right) + \\
& \quad \left. \mu1 \left( 2176 + 69 \, \mathfrak{e}1^2 - 29 \, \mathfrak{e}1 \left( -13 + \mathfrak{e}2 \right) + 155 \, \mathfrak{e}2 + \right. \right. \\
& \quad \left. \left. \mu2 \left( 2846 + \mathfrak{e}1 \left( 22 - 84 \, \mathfrak{e}2 \right) + 488 \, \mathfrak{e}2 \right) \right) \right) \Big) - \\
& \, \eta t \left( 570 + 292 \, \mu2 - 1960 \, \mu2^2 + 146 \, \mathfrak{e}1 + 24 \, \mu2 \, \mathfrak{e}1 - 4 \, \mu1^2 \right. \\
& \quad \left( 181 + 17 \, \mathfrak{e}1 \right) - 2 \, \mu1 \left( 77 - 111 \, \mathfrak{e}1 + 2 \, \mu2 \left( 817 + 135 \, \mathfrak{e}1 \right) \right) + \\
& \quad \mathfrak{e}l \, \mu1^2 \left( 1066 + 27 \, \mathfrak{e}1^2 + 155 \, \mathfrak{e}2 + \mathfrak{e}1 \left( 139 + 13 \, \mathfrak{e}2 \right) \right) + 2 \, \mathfrak{e}l \\
& \quad \left( 555 + 35 \, \mathfrak{e}1 - 20 \, \mu2^2 \left( -6 + 7 \, \mathfrak{e}2 \right) + \mu2 \left( 1839 + 55 \, \mathfrak{e}1 + 56 \, \mathfrak{e}2 \right) \right) \Big) + \\
& \quad \mathfrak{e}l \, \mu1 \left( 2176 + 69 \, \mathfrak{e}1^2 - 29 \, \mathfrak{e}1 \left( -13 + \mathfrak{e}2 \right) + 155 \, \mathfrak{e}2 + \right. \\
& \quad \left. \mu2 \left( 2846 + \mathfrak{e}1 \left( 22 - 84 \, \mathfrak{e}2 \right) + 488 \, \mathfrak{e}2 \right) \right) \Big) \Big) \Big) - \eta^4 \\
& \left( \mathfrak{e}p \left( 2 \times \left( 795 + 2467 \, \mu2 + 560 \, \mu2^2 + 203 \, \mathfrak{e}1 + 455 \, \mu2 \, \mathfrak{e}1 + 2 \, \mu1^2 \right. \right. \right. \\
& \quad \left. \left. \left( 729 + 91 \, \mathfrak{e}1 \right) + \mu1 \left( 2253 + 3091 \, \mu2 + 583 \, \mathfrak{e}1 - 439 \, \mu2 \, \mathfrak{e}1 \right) \right) \right) + \\
& \quad \left. \eta t \left( -402 - 1133 \, \mu2 + 804 \, \mu2^2 + 258 \, \mathfrak{e}1 + 25 \, \mu2 \, \mathfrak{e}1 - 4 \, \mu1^2 \right. \right.
\end{aligned}$$

$$\begin{aligned}
& (-392 + 45 \, \mathfrak{e}1) + \mu1 (1166 + 3995 \, \mu2 + 426 \, \mathfrak{e}1 + 37 \, \mu2 \, \mathfrak{e}1) \Big) \Big) + \\
& (-1 + \eta t) \, \mathfrak{el} \Big( 2 \times (-84 \, \mu2^2 + 90 \times (1 + \mathfrak{e}1) + 8 \, \mu1^2 (28 + \mathfrak{e}1) + \\
& \quad \mu2 (-7 + 15 \, \mathfrak{e}1) + \mu1 (314 + 194 \, \mathfrak{e}1 - \mu2 (115 + 93 \, \mathfrak{e}1)) \Big) + \\
& \, \mathfrak{op} \Big( 1578 + 431 \, \mathfrak{e}1 + 225 \, \mathfrak{e}1^2 + 4 \, \mu2^2 (654 + 207 \, \mathfrak{e}1 - 383 \, \mathfrak{e}2) + 51 \, \mathfrak{e}2 - \\
& \quad 225 \, \mathfrak{e}1 \, \mathfrak{e}2 + \mu2 (7050 + 1561 \, \mathfrak{e}1 + 225 \, \mathfrak{e}1^2 + 569 \, \mathfrak{e}2 - 225 \, \mathfrak{e}1 \, \mathfrak{e}2) + \\
& \quad \mu1^2 (2840 + 317 \, \mathfrak{e}1 + 51 \, \mathfrak{e}1^2 + 295 \, \mathfrak{e}2 + 41 \, \mathfrak{e}1 \, \mathfrak{e}2) + \\
& \quad \mu1 (4418 + 688 \, \mathfrak{e}1 + 576 \, \mathfrak{e}1^2 + 346 \, \mathfrak{e}2 - 484 \, \mathfrak{e}1 \, \mathfrak{e}2 + \\
& \quad \mu2 (10522 + 497 \, \mathfrak{e}1 + 225 \, \mathfrak{e}1^2 + 1417 \, \mathfrak{e}2 - 285 \, \mathfrak{e}1 \, \mathfrak{e}2) \Big) \Big) \Big) + \\
& \eta^5 \Big( \mathfrak{op} (-912 + 598 \, \mu2 + 7592 \, \mu2^2 + 200 \, \mathfrak{e}1 + 410 \, \mu2 \, \mathfrak{e}1 - 4 \, \mu1^2 \\
& \quad (99 + 97 \, \mathfrak{e}1) + 2 \, \mu1 (-654 + 1751 \, \mu2 - 148 \, \mathfrak{e}1 + 397 \, \mu2 \, \mathfrak{e}1) + \\
& \quad \eta t (-6 + 731 \, \mu2 + 372 \, \mu2^2 - 210 \, \mathfrak{e}1 - 151 \, \mu2 \, \mathfrak{e}1 + \\
& \quad 4 \, \mu1^2 (163 + 96 \, \mathfrak{e}1) + \mu1 (646 + 3595 \, \mu2 - 714 \, \mathfrak{e}1 + 701 \, \mu2 \, \mathfrak{e}1) \Big) \Big) - \\
& (-1 + \eta t) \, \mathfrak{el} \Big( 72 + \mu2 - 12 \, \mu2^2 + 60 \, \mathfrak{e}1 + 15 \, \mu2 \, \mathfrak{e}1 - 4 \, \mu1^2 \\
& \quad (26 + 5 \, \mathfrak{e}1) - \mu1 (32 - 196 \, \mathfrak{e}1 + 19 \, \mu2 (53 + 3 \, \mathfrak{e}1)) + \\
& \, \mathfrak{op} \Big( \mu1^2 (2914 + 71 \, \mathfrak{e}1^2 + 323 \, \mathfrak{e}2 + \mathfrak{e}1 (249 + 35 \, \mathfrak{e}2)) + \\
& \quad \mu1 (5110 + 723 \, \mathfrak{e}1 + 377 \, \mathfrak{e}1^2 + 293 \, \mathfrak{e}2 - 271 \, \mathfrak{e}1 \, \mathfrak{e}2 + \\
& \quad 2 \, \mu2 (4525 - 74 \, \mathfrak{e}1 + 45 \, \mathfrak{e}1^2 + 587 \, \mathfrak{e}2 - 153 \, \mathfrak{e}1 \, \mathfrak{e}2) \Big) + \\
& \quad 2 \Big( \mu2^2 (644 + 90 \, \mathfrak{e}1 - 702 \, \mathfrak{e}2) + \mu2 (4017 + 326 \, \mathfrak{e}1 + \\
& \quad 45 \, \mathfrak{e}1^2 + 93 \, \mathfrak{e}2 - 45 \, \mathfrak{e}1 \, \mathfrak{e}2) + \\
& \quad 3 \times (366 + 43 \, \mathfrak{e}1 + 15 \, \mathfrak{e}1^2 - 5 \, \mathfrak{e}2 - 15 \, \mathfrak{e}1 \, \mathfrak{e}2) \Big) \Big) \Big) - \\
& \eta^3 \Big( 2 \, \mathfrak{op} \Big( 2 \times (195 + 728 \, \mu2^2 + 103 \, \mathfrak{e}1 + \mu1^2 (369 + 7 \, \mathfrak{e}1) + 14 \, \mu2 \\
& \quad (65 + 9 \, \mathfrak{e}1) + 2 \, \mu1 (282 + 73 \, \mathfrak{e}1 + \mu2 (623 + 18 \, \mathfrak{e}1)) \Big) + \\
& \quad \eta t (168 \, \mu2^2 - 4 \times (77 + 36 \, \mathfrak{e}1) + 4 \, \mu1^2 (21 + 55 \, \mathfrak{e}1) - \\
& \quad \mu2 (369 + 79 \, \mathfrak{e}1) + \mu1 (-224 - 410 \, \mathfrak{e}1 + \mu2 (847 + 305 \, \mathfrak{e}1)) \Big) \Big) + \\
& (-1 + \eta t) \, \mathfrak{el} \Big( 2 \times (56 - 93 \, \mu2 - 148 \, \mu2^2 + 80 \, \mathfrak{e}1 + 5 \, \mu2 \, \mathfrak{e}1 + \\
& \quad 4 \, \mu1^2 (53 + 8 \, \mathfrak{e}1) + \mu1 (268 - 5 \, \mu2 + 118 \, \mathfrak{e}1 - 103 \, \mu2 \, \mathfrak{e}1) \Big) + \\
& \, \mathfrak{op} \Big( \mu1^2 (1154 + \mathfrak{e}1^2 + 181 \, \mathfrak{e}2 + \mathfrak{e}1 (327 + 25 \, \mathfrak{e}2)) + \\
& \quad \mu1 (1826 + 519 \, \mathfrak{e}1 + 325 \, \mathfrak{e}1^2 + 325 \, \mathfrak{e}2 - 299 \, \mathfrak{e}1 \, \mathfrak{e}2 + \\
& \quad 2 \, \mu2 (2627 + 575 \, \mathfrak{e}1 + 90 \, \mathfrak{e}1^2 + 520 \, \mathfrak{e}2 - 18 \, \mathfrak{e}1 \, \mathfrak{e}2) \Big) + \\
& \quad 2 \times (2 \, \mu2^2 (542 + 243 \, \mathfrak{e}1 - 69 \, \mathfrak{e}2) + \mu2 (1815 + \\
& \quad 727 \, \mathfrak{e}1 + 90 \, \mathfrak{e}1^2 + 402 \, \mathfrak{e}2 - 90 \, \mathfrak{e}1 \, \mathfrak{e}2) + \\
& \quad 6 \times (56 + 28 \, \mathfrak{e}1 + 15 \, \mathfrak{e}1^2 + 12 \, \mathfrak{e}2 - 15 \, \mathfrak{e}1 \, \mathfrak{e}2) \Big) \Big) \Big) + \\
& \eta^2 \Big( -2 \, \mathfrak{op} \Big( 6 \times (9 + 41 \, \mu2 + 16 \, \mu2^2 - \mu1^2 (-9 + \mathfrak{e}1) + 5 \, \mathfrak{e}1 + 3 \, \mu2 \\
& \quad \mathfrak{e}1 + \mu1 (18 + 41 \, \mu2 + 4 \, \mathfrak{e}1 + 3 \, \mu2 \, \mathfrak{e}1)) \Big) + \\
& \quad \eta t (-92 + 407 \, \mu2 + 512 \, \mu2^2 - 200 \, \mathfrak{e}1 - 31 \, \mu2 \, \mathfrak{e}1 + \mu1^2 \\
& \quad (-206 + 82 \, \mathfrak{e}1) + \mu1 (-298 + 311 \, \mu2 - 304 \, \mathfrak{e}1 + 257 \, \mu2 \, \mathfrak{e}1) \Big) \Big) + \\
& (-1 + \eta t) \, \mathfrak{el} \Big( -2 \times (4 - 68 \, \mu2^2 + 20 \, \mathfrak{e}1 + 2 \, \mu1^2 (13 + \mathfrak{e}1) - \\
& \quad 5 \, \mu2 (15 + \mathfrak{e}1) + \mu1 (30 + 22 \, \mathfrak{e}1 - \mu2 (71 + 41 \, \mathfrak{e}1)) \Big) + \\
& \, 3 \, \mathfrak{op} \Big( -60 - 31 \, \mathfrak{e}1 - 15 \, \mathfrak{e}1^2 - 21 \, \mathfrak{e}2 + 15 \, \mathfrak{e}1 \, \mathfrak{e}2 - 4 \, \mu2^2 \\
& \quad (50 + 27 \, \mathfrak{e}1 + 11 \, \mathfrak{e}2) - \mu2 (312 + 145 \, \mathfrak{e}1 + 15 \, \mathfrak{e}1^2 + 103 \, \mathfrak{e}2 - \\
& \quad 15 \, \mathfrak{e}1 \, \mathfrak{e}2) + 2 \, \mu1^2 (\mathfrak{e}1^2 - 9 \times (3 + \mathfrak{e}2) - \mathfrak{e}1 (20 + \mathfrak{e}2)) - \\
& \quad \mu1 (114 + 59 \, \mathfrak{e}1 + 19 \, \mathfrak{e}1^2 + 39 \, \mathfrak{e}2 - 19 \, \mathfrak{e}1 \, \mathfrak{e}2 +
\end{aligned}$$

$$\begin{aligned}
& \mu_2 (312 + 161 \mu_1 + 15 \mu_1^2 + 103 \mu_2 + 9 \mu_1 \mu_2) \Big) \Big) \Big) \Big) + \\
& x^6 (-1 + \eta)^6 \Big( 2 \times (-1 + \eta) \operatorname{Op} (195 + 603 \mu_1 + 408 \mu_1^2 + 609 \mu_2 + \\
& \quad 793 \mu_1 \mu_2 + 216 \mu_2^2 + 39 \mu_1 + 157 \mu_1 \mu_1 + 64 \mu_1^2 \mu_1 + \\
& \quad 85 \mu_2 \mu_1 - 41 \mu_1 \mu_2 \mu_1 + 28 \eta^3 (3 + 4 \mu_2 + \mu_1 + \mu_1 (3 + \mu_1)) - \\
& \quad 7 \eta^2 (-39 - 58 \mu_2 + 28 \mu_2^2 + 3 \mu_1 (-29 + 2 \mu_2 (-9 + \mu_1) - 9 \mu_1) - \\
& \quad \quad 11 \mu_1 - 16 \mu_1^2 (3 + \mu_1) + 4 \eta t (3 + 4 \mu_2 + \mu_1 + \mu_1 (3 + \mu_1))) \Big) + \\
& \quad \eta t (-93 + 196 \mu_2^2 - 25 \mu_1 + 4 \mu_1^2 (8 + \mu_1) - 2 \mu_2 (46 + \mu_1) + \\
& \quad \quad \mu_1 (-61 - 33 \mu_1 + 4 \mu_2 (46 + 13 \mu_1))) \Big) + \\
& \quad \eta (588 + 1569 \mu_2 - 304 \mu_2^2 + 60 \mu_1 + 77 \mu_2 \mu_1 + 14 \mu_1^2 (75 + 17 \mu_1) + \\
& \quad \quad \mu_1 (1638 + 1573 \mu_2 + 424 \mu_1 - 109 \mu_2 \mu_1) + 7 \eta t (-39 - 58 \mu_2 + \\
& \quad \quad \quad 28 \mu_2^2 - 11 \mu_1 + \mu_1 (-39 + 10 \mu_2 - 11 \mu_1 + 6 \mu_2 \mu_1)) \Big) - \\
& (-1 + \eta t) \operatorname{Ol} (84 - 16 \mu_1 - 332 \eta \mu_1 - 100 \mu_1^2 - 332 \eta \mu_1^2 + 49 \mu_2 - \\
& \quad 96 \eta \mu_2 - 415 \mu_1 \mu_2 - 1296 \eta \mu_1 \mu_2 + 24 \mu_2^2 + 60 \mu_1 + 196 \mu_1 \mu_1 + \\
& \quad 116 \eta \mu_1 \mu_1 - 92 \mu_1^2 \mu_1 - 28 \eta \mu_1^2 \mu_1 + 15 \mu_2 \mu_1 - 57 \mu_1 \mu_2 \mu_1 + \\
& \quad \operatorname{Op} (306 + 1074 \mu_2 + 208 \mu_2^2 + 33 \mu_1 + 67 \mu_2 \mu_1 + 15 \mu_1^2 + \\
& \quad \quad 15 \mu_2 \mu_1^2 - 15 \mu_2 - 9 \mu_2 \mu_2 - 264 \mu_2^2 \mu_2 - 15 \mu_1 \mu_2 - \\
& \quad \quad 15 \mu_2 \mu_1 \mu_2 + \mu_1^2 (424 + 11 \mu_1^2 + 23 \mu_2 + \mu_1 (9 + 5 \mu_2)) + \\
& \quad \quad \mu_1 (730 + 62 \mu_1^2 + \mu_1 (78 - 46 \mu_2) + 8 \mu_2 + \\
& \quad \quad \quad \mu_2 (1250 + 15 \mu_1^2 + 79 \mu_2 - \mu_1 (133 + 51 \mu_2))) \Big) + 2 \eta \\
& \quad (5 \times (99 + 7 \mu_1) - 20 \mu_2^2 (-8 + 7 \mu_2) + 2 \mu_2 (792 + 25 \mu_1 + 28 \mu_2) + \\
& \quad \quad \mu_1^2 (11 \mu_1^2 + 4 \mu_1 (8 + \mu_2) + 9 \times (52 + 5 \mu_2)) + \\
& \quad \quad \mu_1 (963 + 151 \mu_1 + 32 \mu_1^2 + 45 \mu_2 - 17 \mu_1 \mu_2 - \\
& \quad \quad \quad 2 \mu_2 (-594 + 37 \mu_1 - 67 \mu_2 + 21 \mu_1 \mu_2)) \Big) \Big) \Big) \Big) + \\
& x^3 (-1 + \eta)^3 \Big( -2 \times (-1 + \eta) \operatorname{Op} (18 - 4 \eta t + 36 \mu_1 + 16 \eta t \mu_1 + 18 \mu_1^2 + \\
& \quad 20 \eta t \mu_1^2 + 82 \mu_2 + 303 \eta t \mu_2 + 82 \mu_1 \mu_2 + 283 \eta t \mu_1 \mu_2 + \\
& \quad 32 \mu_2^2 + 304 \eta t \mu_2^2 + 10 \mu_1 - 80 \eta t \mu_1 + 8 \mu_1 \mu_1 - 116 \eta t \mu_1 \mu_1 - \\
& \quad 2 \mu_1^2 \mu_1 + 72 \eta t \mu_1^2 \mu_1 + 6 \mu_2 \mu_1 - 7 \eta t \mu_2 \mu_1 + 6 \mu_1 \mu_2 \mu_1 + \\
& \quad 113 \eta t \mu_1 \mu_2 \mu_1 + 56 \eta^6 (3 + 4 \mu_2 + \mu_1 + \mu_1 (3 + \mu_1)) - \\
& \quad 7 \eta^5 (5 \times (-39 - 58 \mu_2 + 28 \mu_2^2 - 11 \mu_1) - 32 \mu_1^2 (3 + \mu_1) + \\
& \quad \quad 3 \mu_1 (-97 - 26 \mu_2 - 29 \mu_1 + 10 \mu_2 \mu_1) + \\
& \quad \quad 8 \eta t (3 + 4 \mu_2 + \mu_1 + \mu_1 (3 + \mu_1))) \Big) + 5 \eta^4 \\
& \quad (903 + 1929 \mu_2 - 1216 \mu_2^2 + 135 \mu_1 + 77 \mu_2 \mu_1 + 14 \mu_1^2 (75 + 17 \mu_1) + \\
& \quad \quad \mu_1 (1953 + 1273 \mu_2 + 499 \mu_1 - 289 \mu_2 \mu_1) + 7 \eta t (-39 - 58 \mu_2 + \\
& \quad \quad \quad 28 \mu_2^2 - 11 \mu_1 + \mu_1 (-39 + 10 \mu_2 - 11 \mu_1 + 6 \mu_2 \mu_1)) \Big) + \\
& \quad 2 \eta (222 + 1007 \mu_2 + 824 \mu_2^2 + 118 \mu_1 + 137 \mu_2 \mu_1 + 4 \mu_1^2 \\
& \quad \quad (99 + \mu_1) + \mu_1 (618 + 1343 \mu_2 + 158 \mu_1 + 35 \mu_2 \mu_1) + \eta t \\
& \quad \quad (\mu_1^2 (96 + 250 \mu_1) + 2 \times (-90 + 95 \mu_2 + 240 \mu_2^2 - 96 \mu_1 - 25 \mu_2 \mu_1) + \\
& \quad \quad \quad \mu_1 (-84 + 628 \mu_2 - 377 \mu_1 + 322 \mu_2 \mu_1)) \Big) + \\
& \quad 10 \eta^3 (495 + 1334 \mu_2 - 164 \mu_2^2 + 99 \mu_1 + 172 \mu_2 \mu_1 + 16 \mu_1^2 \\
& \quad \quad (51 + 8 \mu_1) + \mu_1 (1311 + 335 \mu_1 - 2 \mu_2 (-725 + 91 \mu_1)) + \\
& \quad \quad 2 \eta t (-93 + 196 \mu_2^2 - 25 \mu_1 - 2 \mu_2 (46 + \mu_1) + \\
& \quad \quad \quad \mu_1^2 (49 + 5 \mu_1) + 4 \mu_1 (-11 - 8 \mu_1 + \mu_2 (61 + 13 \mu_1))) \Big) + \\
& \quad \eta^2 (2 \times (1167 + 2816 \mu_2^2 + 427 \mu_1 + 10 \mu_1^2 (225 + 19 \mu_1) +
\end{aligned}$$



$$\begin{aligned}
& \mu_2 (4349 + 725 \, \mathfrak{e}_1) + \mu_1 (3417 + \mu_2 (5837 - 277 \, \mathfrak{e}_1) + 887 \, \mathfrak{e}_1) \Big) + \\
& \eta t \Big( 2652 \, \mu_2^2 - 7 \, \mu_2 (67 + 25 \, \mathfrak{e}_1) - 6 \times (191 + 85 \, \mathfrak{e}_1) + 4 \, \mu_1^2 \\
& \quad (342 + 149 \, \mathfrak{e}_1) + \mu_1 (222 - 1090 \, \mathfrak{e}_1 + \mu_2 (5819 + 1325 \, \mathfrak{e}_1)) \Big) \Big) + \\
& (-1 + \eta t) \, \mathfrak{e}_l \Big( -2 \times (12 + 116 \, \mu_2^2 - 20 \, \mathfrak{e}_1 + 4 \, \mu_1^2 \, \mathfrak{e}_1 + \mu_2 (139 + 5 \, \mathfrak{e}_1) + \\
& \quad \mu_1 (12 - 22 \, \mathfrak{e}_1 + \mu_2 (139 + 41 \, \mathfrak{e}_1)) \Big) + \\
& \mathfrak{e}_p \Big( 60 + 31 \, \mathfrak{e}_1 + 15 \, \mathfrak{e}_1^2 + 21 \, \mathfrak{e}_2 - 15 \, \mathfrak{e}_1 \, \mathfrak{e}_2 + 4 \, \mu_2^2 (50 + 27 \, \mathfrak{e}_1 + 11 \, \mathfrak{e}_2) + \\
& \quad \mu_2 (312 + 145 \, \mathfrak{e}_1 + 15 \, \mathfrak{e}_1^2 + 103 \, \mathfrak{e}_2 - 15 \, \mathfrak{e}_1 \, \mathfrak{e}_2) + \\
& \quad \mu_1^2 (-2 \, \mathfrak{e}_1^2 + 18 \times (3 + \mathfrak{e}_2) + 2 \, \mathfrak{e}_1 (20 + \mathfrak{e}_2)) + \\
& \quad \mu_1 (114 + 59 \, \mathfrak{e}_1 + 19 \, \mathfrak{e}_1^2 + 39 \, \mathfrak{e}_2 - 19 \, \mathfrak{e}_1 \, \mathfrak{e}_2 + \\
& \quad \mu_2 (312 + 161 \, \mathfrak{e}_1 + 15 \, \mathfrak{e}_1^2 + 103 \, \mathfrak{e}_2 + 9 \, \mathfrak{e}_1 \, \mathfrak{e}_2)) \Big) + \\
& 2 \, \eta^2 \Big( -6 \times (84 \, \mu_2^2 + \mu_2 (7 - 15 \, \mathfrak{e}_1) + 38 \, \mu_1^2 (-4 + \mathfrak{e}_1) - \\
& \quad 90 \times (1 + \mathfrak{e}_1) + \mu_1 (-242 - 193 \, \mathfrak{e}_1 + \mu_2 (53 + 93 \, \mathfrak{e}_1)) \Big) + \\
& \mathfrak{e}_p \Big( 1434 + 383 \, \mathfrak{e}_1 + 225 \, \mathfrak{e}_1^2 + 4 \, \mu_2^2 (622 + 171 \, \mathfrak{e}_1 - 419 \, \mathfrak{e}_2) + 3 \, \mathfrak{e}_2 - \\
& \quad 225 \, \mathfrak{e}_1 \, \mathfrak{e}_2 + \mu_2 (6390 + 1373 \, \mathfrak{e}_1 + 225 \, \mathfrak{e}_1^2 + 377 \, \mathfrak{e}_2 - 225 \, \mathfrak{e}_1 \, \mathfrak{e}_2) + \\
& \quad \mu_1^2 (53 \, \mathfrak{e}_1^2 + 225 \times (12 + \mathfrak{e}_2) + \mathfrak{e}_1 (251 + 43 \, \mathfrak{e}_2)) + \\
& \quad \mu_1 (4134 + 574 \, \mathfrak{e}_1 + 578 \, \mathfrak{e}_1^2 + 228 \, \mathfrak{e}_2 - 482 \, \mathfrak{e}_1 \, \mathfrak{e}_2 + \\
& \quad \mu_2 (9846 + 181 \, \mathfrak{e}_1 + 225 \, \mathfrak{e}_1^2 + 1121 \, \mathfrak{e}_2 - 285 \, \mathfrak{e}_1 \, \mathfrak{e}_2)) \Big) \Big) + \\
& 5 \, \eta^4 \Big( -4 \times (12 \, \mu_2 + \mu_1 (67 + 252 \, \mu_2 - 13 \, \mathfrak{e}_1) + \mu_1^2 (67 + 5 \, \mathfrak{e}_1)) + \\
& \quad \mathfrak{e}_p \Big( \mu_1^2 (1014 + 109 \, \mathfrak{e}_1 + 25 \, \mathfrak{e}_1^2 + 129 \, \mathfrak{e}_2 + 11 \, \mathfrak{e}_1 \, \mathfrak{e}_2) + 2 \times (531 + \\
& \quad 35 \, \mathfrak{e}_1 - 4 \, \mu_2^2 (-34 + 35 \, \mathfrak{e}_2) + \mu_2 (1737 + 53 \, \mathfrak{e}_1 + 56 \, \mathfrak{e}_2)) + \\
& \quad \mu_1 (2076 + 347 \, \mathfrak{e}_1 + 67 \, \mathfrak{e}_1^2 + 129 \, \mathfrak{e}_2 - 31 \, \mathfrak{e}_1 \, \mathfrak{e}_2 + \\
& \quad \mu_2 (2658 - 46 \, \mathfrak{e}_1 + 400 \, \mathfrak{e}_2 - 84 \, \mathfrak{e}_1 \, \mathfrak{e}_2)) \Big) \Big) + \\
& \eta \Big( 256 - 878 \, \mu_2 - 1128 \, \mu_2^2 + \mu_1^2 (792 - 48 \, \mathfrak{e}_1) + 480 \, \mathfrak{e}_1 + \\
& \quad 30 \, \mu_2 \, \mathfrak{e}_1 + \mu_1 (1048 + 708 \, \mathfrak{e}_1 - 6 \, \mu_2 (69 + 103 \, \mathfrak{e}_1)) + \\
& \quad 3 \, \mathfrak{e}_p \Big( \mu_1^2 (370 + \mathfrak{e}_1^2 + 53 \, \mathfrak{e}_2 + \mathfrak{e}_1 (103 + 9 \, \mathfrak{e}_2)) + \\
& \quad 2 \times (104 + 52 \, \mathfrak{e}_1 + 30 \, \mathfrak{e}_1^2 + 2 \, \mu_2^2 (174 + 75 \, \mathfrak{e}_1 - 29 \, \mathfrak{e}_2) + 20 \, \mathfrak{e}_2 - \\
& \quad 30 \, \mathfrak{e}_1 \, \mathfrak{e}_2 + \mu_2 (567 + 227 \, \mathfrak{e}_1 + 30 \, \mathfrak{e}_1^2 + 118 \, \mathfrak{e}_2 - 30 \, \mathfrak{e}_1 \, \mathfrak{e}_2)) + \\
& \quad \mu_1 (578 + 159 \, \mathfrak{e}_1 + 109 \, \mathfrak{e}_1^2 + 93 \, \mathfrak{e}_2 - 99 \, \mathfrak{e}_1 \, \mathfrak{e}_2 + \\
& \quad 2 \, \mu_2 (835 + 171 \, \mathfrak{e}_1 + 30 \, \mathfrak{e}_1^2 + 156 \, \mathfrak{e}_2 - 6 \, \mathfrak{e}_1 \, \mathfrak{e}_2)) \Big) \Big) + \\
& 2 \, \eta^3 \Big( 384 + 101 \, \mu_2 + 12 \, \mu_2^2 + 300 \, \mathfrak{e}_1 + 75 \, \mu_2 \, \mathfrak{e}_1 - 4 \, \mu_1^2 \\
& \quad (128 + 61 \, \mathfrak{e}_1) - \mu_1 (128 + 3851 \, \mu_2 - 980 \, \mathfrak{e}_1 + 285 \, \mu_2 \, \mathfrak{e}_1) + \\
& \quad 5 \, \mathfrak{e}_p \Big( 4 \, \mu_2^2 (106 + 9 \, \mathfrak{e}_1 - 123 \, \mathfrak{e}_2) + 2 \, \mu_2 (1233 + 92 \, \mathfrak{e}_1 + 15 \, \mathfrak{e}_1^2 + \\
& \quad 15 \, \mathfrak{e}_2 - 15 \, \mathfrak{e}_1 \, \mathfrak{e}_2) + 6 \times (114 + 13 \, \mathfrak{e}_1 + 5 \, \mathfrak{e}_1^2 - 3 \, \mathfrak{e}_2 - 5 \, \mathfrak{e}_1 \, \mathfrak{e}_2) + \\
& \quad \mu_1^2 (922 + 23 \, \mathfrak{e}_1^2 + 83 \, \mathfrak{e}_2 + \mathfrak{e}_1 (57 + 11 \, \mathfrak{e}_2)) + \\
& \quad \mu_1 (1606 + 207 \, \mathfrak{e}_1 + 125 \, \mathfrak{e}_1^2 + 65 \, \mathfrak{e}_2 - 91 \, \mathfrak{e}_1 \, \mathfrak{e}_2 + \\
& \quad 2 \, \mu_2 (1405 + 15 \, \mathfrak{e}_1^2 + 149 \, \mathfrak{e}_2 - 17 \, \mathfrak{e}_1 (4 + 3 \, \mathfrak{e}_2)) \Big) \Big) \Big) - \\
& x^4 (-1 + \eta)^4 \Big( - \Big( (-1 + \eta) \, \mathfrak{e}_p \Big( 140 \, \eta^5 (3 + 4 \, \mu_2 + \mathfrak{e}_1 + \mu_1 (3 + \mathfrak{e}_1)) - \\
& \quad 70 \, \eta^4 (-39 - 58 \, \mu_2 + 28 \, \mu_2^2 - 11 \, \mathfrak{e}_1 - 8 \, \mu_1^2 (3 + \mathfrak{e}_1) + \\
& \quad \mu_1 (-63 - 22 \, \mu_2 - 19 \, \mathfrak{e}_1 + 6 \, \mu_2 \, \mathfrak{e}_1) + \\
& \quad 2 \, \eta t (3 + 4 \, \mu_2 + \mathfrak{e}_1 + \mu_1 (3 + \mathfrak{e}_1)) \Big) + 10 \, \eta^3 (798 + 1809 \, \mu_2 - \\
& \quad 912 \, \mu_2^2 + 110 \, \mathfrak{e}_1 + 77 \, \mu_2 \, \mathfrak{e}_1 + 14 \, \mu_1^2 (75 + 17 \, \mathfrak{e}_1) + \\
& \quad \mu_1 (1848 + 1373 \, \mu_2 + 474 \, \mathfrak{e}_1 - 229 \, \mu_2 \, \mathfrak{e}_1) + 7 \, \eta t (-39 - 58 \, \mu_2 + \\
& \quad 28 \, \mu_2^2 - 11 \, \mathfrak{e}_1 + \mu_1 (-39 + 10 \, \mu_2 - 11 \, \mathfrak{e}_1 + 6 \, \mu_2 \, \mathfrak{e}_1)) \Big) +
\end{aligned}$$

$$\begin{aligned}
& 2 \times (111 + 497 \mu_2 + 424 \mu_2^2 + 59 \mathfrak{e}_1 + 69 \mu_2 \mathfrak{e}_1 + 2 \mu_1^2 \\
& \quad (99 + \mathfrak{e}_1) + \mu_1 (309 + 665 \mu_2 + 79 \mathfrak{e}_1 + 15 \mu_2 \mathfrak{e}_1) + \\
& \quad \eta t (-90 + 95 \mu_2 + 240 \mu_2^2 - 96 \mathfrak{e}_1 - 25 \mu_2 \mathfrak{e}_1 + 4 \mu_1^2 \\
& \quad \quad (21 + 37 \mathfrak{e}_1) + \mu_1 (-6 + 283 \mu_2 - 188 \mathfrak{e}_1 + 161 \mu_2 \mathfrak{e}_1)) + \\
& \eta (2 \times (1131 + 4257 \mu_2 + 3168 \mu_2^2 + 421 \mathfrak{e}_1 + 725 \mu_2 \mathfrak{e}_1 + 10 \mu_1^2 \\
& \quad (225 + 19 \mathfrak{e}_1) + \mu_1 (3381 + 5841 \mu_2 + 881 \mathfrak{e}_1 - 241 \mu_2 \mathfrak{e}_1)) + \\
& \quad \eta t (-1158 - 517 \mu_2 + 2616 \mu_2^2 - 510 \mathfrak{e}_1 - 175 \mu_2 \mathfrak{e}_1 + 4 \mu_1^2 (341 + \\
& \quad \quad 167 \mathfrak{e}_1) + \mu_1 (206 + 5227 \mu_2 - 1090 \mathfrak{e}_1 + 1325 \mu_2 \mathfrak{e}_1)) + \\
& 10 \eta^2 (690 + 1943 \mu_2 + 52 \mu_2^2 + 138 \mathfrak{e}_1 + 257 \mu_2 \mathfrak{e}_1 + 24 \mu_1^2 \\
& \quad (51 + 8 \mathfrak{e}_1) + \mu_1 (1914 + 2243 \mu_2 + 492 \mathfrak{e}_1 - 223 \mu_2 \mathfrak{e}_1) + \\
& \quad \eta t (-279 + 588 \mu_2^2 - 75 \mathfrak{e}_1 - 6 \mu_2 (46 + \mathfrak{e}_1) + 2 \mu_1^2 (65 + 7 \mathfrak{e}_1) + \\
& \quad \quad \mu_1 (-149 - 97 \mathfrak{e}_1 + 12 \mu_2 (56 + 13 \mathfrak{e}_1))) + \\
& (-1 + \eta t) \mathfrak{e} l (2 \times (36 - 208 \mu_2^2 + \mu_1^2 (92 - 28 \mathfrak{e}_1) + 80 \mathfrak{e}_1 + \\
& \quad \mu_2 (-173 + 5 \mathfrak{e}_1) + \mu_1 (128 - 101 \mu_2 + 118 \mathfrak{e}_1 - 103 \mu_2 \mathfrak{e}_1)) + \\
& \mathfrak{e} p (8 \mu_2^2 (64 + 27 \mathfrak{e}_1 - 12 \mathfrak{e}_2) + \mu_2 (822 + 329 \mathfrak{e}_1 + 45 \mathfrak{e}_1^2 + \\
& \quad 165 \mathfrak{e}_2 - 45 \mathfrak{e}_1 \mathfrak{e}_2) + 3 \times (50 + 25 \mathfrak{e}_1 + 15 \mathfrak{e}_1^2 + 9 \mathfrak{e}_2 - 15 \mathfrak{e}_1 \mathfrak{e}_2) + \\
& \quad \mu_1^2 (272 + \mathfrak{e}_1^2 + 37 \mathfrak{e}_2 + \mathfrak{e}_1 (75 + 7 \mathfrak{e}_2)) + \mu_1 \\
& \quad (422 + 114 \mathfrak{e}_1 + 82 \mathfrak{e}_1^2 + 64 \mathfrak{e}_2 - 74 \mathfrak{e}_1 \mathfrak{e}_2 + \\
& \quad \mu_2 (1222 + 241 \mathfrak{e}_1 + 45 \mathfrak{e}_1^2 + 221 \mathfrak{e}_2 - 9 \mathfrak{e}_1 \mathfrak{e}_2))) + \\
& \eta (4 (\mu_1^2 (232 - 122 \mathfrak{e}_1) + 2 \times (-84 \mu_2^2 + 90 \times (1 + \mathfrak{e}_1) + \\
& \quad \mu_2 (-7 + 15 \mathfrak{e}_1)) + \mu_1 (412 + 385 \mathfrak{e}_1 - 2 \mu_2 (22 + 93 \mathfrak{e}_1))) + \\
& \mathfrak{e} p (1362 + 359 \mathfrak{e}_1 + 225 \mathfrak{e}_1^2 + 4 \mu_2^2 (606 + 153 \mathfrak{e}_1 - 437 \mathfrak{e}_2) - \\
& \quad 21 \mathfrak{e}_2 - 225 \mathfrak{e}_1 \mathfrak{e}_2 + \mu_2 (6060 + 1279 \mathfrak{e}_1 + 225 \mathfrak{e}_1^2 + 281 \mathfrak{e}_2 - 225 \\
& \quad \mathfrak{e}_1 \mathfrak{e}_2) + 2 \mu_1^2 (1315 + 27 \mathfrak{e}_1^2 + 95 \mathfrak{e}_2 + \mathfrak{e}_1 (109 + 22 \mathfrak{e}_2)) + \\
& \quad \mu_1 (3992 + 517 \mathfrak{e}_1 + 579 \mathfrak{e}_1^2 + 169 \mathfrak{e}_2 - 481 \mathfrak{e}_1 \mathfrak{e}_2 + \\
& \quad \mu_2 (9508 + 23 \mathfrak{e}_1 + 225 \mathfrak{e}_1^2 + 973 \mathfrak{e}_2 - 285 \mathfrak{e}_1 \mathfrak{e}_2))) + \\
& 10 \eta^3 (-4 \times (8 \mu_2 + \mu_1 (39 + 148 \mu_2 - 9 \mathfrak{e}_1) + 3 \mu_1^2 (13 + \mathfrak{e}_1)) + \\
& \quad \mathfrak{e} p (519 + 35 \mathfrak{e}_1 + 2 \mu_2 (843 + 26 \mathfrak{e}_1 + 28 \mathfrak{e}_2) - 4 \mu_2^2 (-36 + 35 \mathfrak{e}_2) + \\
& \quad \mu_1^2 (494 + 12 \mathfrak{e}_1^2 + 58 \mathfrak{e}_2 + \mathfrak{e}_1 (47 + 5 \mathfrak{e}_2)) + \\
& \quad \mu_1 (1013 + 166 \mathfrak{e}_1 + 33 \mathfrak{e}_1^2 + 58 \mathfrak{e}_2 - 16 \mathfrak{e}_1 \mathfrak{e}_2 - \\
& \quad \quad 2 \mu_2 (-641 + 20 \mathfrak{e}_1 - 89 \mathfrak{e}_2 + 21 \mathfrak{e}_1 \mathfrak{e}_2))) + \\
& \eta^2 (792 + 298 \mu_2 + 96 \mu_2^2 + 600 \mathfrak{e}_1 + 150 \mu_2 \mathfrak{e}_1 - 8 \mu_1^2 \\
& \quad (127 + 79 \mathfrak{e}_1) - 2 \mu_1 (112 - 980 \mathfrak{e}_1 + \mu_2 (3259 + 285 \mathfrak{e}_1)) + \\
& 5 \mathfrak{e} p (990 + 111 \mathfrak{e}_1 + 45 \mathfrak{e}_1^2 + 4 \mu_2^2 (158 + 9 \mathfrak{e}_1 - 189 \mathfrak{e}_2) - \\
& \quad 33 \mathfrak{e}_2 - 45 \mathfrak{e}_1 \mathfrak{e}_2 + \mu_2 (3540 + 45 \mathfrak{e}_1^2 + \mathfrak{e}_1 (251 - 45 \mathfrak{e}_2) + 21 \mathfrak{e}_2) + \\
& \quad 2 \mu_1^2 (673 + 17 \mathfrak{e}_1^2 + 53 \mathfrak{e}_2 + \mathfrak{e}_1 (33 + 8 \mathfrak{e}_2)) + \\
& \quad \mu_1 (187 \mathfrak{e}_1^2 + \mathfrak{e}_1 (285 - 137 \mathfrak{e}_2) + 73 \times (32 + \mathfrak{e}_2) + \\
& \quad \mu_2 (4060 + 45 \mathfrak{e}_1^2 + 377 \mathfrak{e}_2 - \mathfrak{e}_1 (269 + 153 \mathfrak{e}_2)))) + \\
& x^2 (-1 + \eta)^2 (-56 \eta t \mathfrak{e} p - 108 \eta t \mathfrak{e} p \mu_1 - 52 \eta t \mathfrak{e} p \mu_1^2 - 11 \mathfrak{e} l \mu_2 + \\
& 11 \eta t \mathfrak{e} l \mu_2 - 406 \eta t \mathfrak{e} p \mu_2 - 11 \mathfrak{e} l \mu_1 \mu_2 + 11 \\
& \eta t \mathfrak{e} l \mu_1 \mu_2 - 414 \eta t \mathfrak{e} p \mu_1 \mu_2 - 8 \mathfrak{e} l \mu_2^2 + 8 \\
& \eta t \mathfrak{e} l \mu_2^2 - 328 \eta t \mathfrak{e} p \mu_2^2 + 40 \eta t \mathfrak{e} p \mathfrak{e}_1 + 44 \\
& \eta t \mathfrak{e} p \mu_1 \mathfrak{e}_1 - 20 \eta t \mathfrak{e} p \mu_1^2 \mathfrak{e}_1 - 5 \mathfrak{e} l \mu_2 \mathfrak{e}_1 + 5
\end{aligned}$$

$$\begin{aligned}
& \eta t \, \theta l \, \mu_2 \, \mathfrak{e}1 - 10 \, \eta t \, \theta p \, \mu_2 \, \mathfrak{e}1 - 5 \, \theta l \, \mu_1 \, \mu_2 \\
& \mathfrak{e}1 + 5 \, \eta t \, \theta l \, \mu_1 \, \mu_2 \, \mathfrak{e}1 - 82 \, \eta t \, \theta p \, \mu_1 \, \mu_2 \, \mathfrak{e}1 + 56 \\
& \eta^8 \, \theta p \, (3 + 4 \, \mu_2 + \mathfrak{e}1 + \mu_1 \, (3 + \mathfrak{e}1)) - 14 \, \eta^7 \, \theta p \\
& (-105 - 158 \, \mu_2 + 84 \, \mu_2^2 - 29 \, \mathfrak{e}1 - 16 \, \mu_1^2 \, (3 + \mathfrak{e}1) + \\
& \mu_1 \, (-153 - 34 \, \mu_2 - 45 \, \mathfrak{e}1 + 18 \, \mu_2 \, \mathfrak{e}1) + \\
& 4 \, \eta t \, (3 + 4 \, \mu_2 + \mathfrak{e}1 + \mu_1 \, (3 + \mathfrak{e}1))) + 2 \, \eta^6 \, \theta p \\
& (14 \, \mu_1^2 \, (201 + 43 \, \mathfrak{e}1) + \mu_1 \, (5019 + 3281 \, \mu_2 + 1229 \, \mathfrak{e}1 - 921 \, \mu_2 \, \mathfrak{e}1) + \\
& 3 \times (735 + 1643 \, \mu_2 - 1324 \, \mu_2^2 + 83 \, \mathfrak{e}1 + 77 \, \mu_2 \, \mathfrak{e}1) + \\
& 7 \, \eta t \, (-105 - 158 \, \mu_2 + 84 \, \mu_2^2 - 29 \, \mathfrak{e}1 + \\
& \mu_1 \, (-105 - 29 \, \mathfrak{e}1 + 6 \, \mu_2 \, (5 + 3 \, \mathfrak{e}1))) - 2 \\
& \eta^3 \, (\theta p \, (2 \times (870 + 1264 \, \mu_2^2 + 256 \, \mathfrak{e}1 + 184 \, \mu_1^2 \, (9 + \mathfrak{e}1) + \\
& \mu_2 \, (2911 + 521 \, \mathfrak{e}1) + \mu_1 \, (2526 + \mu_2 \, (3799 - 373 \, \mathfrak{e}1) + 656 \, \mathfrak{e}1)) + \\
& \eta t \, (1248 \, \mu_2^2 + \mu_1^2 \, (1300 - 88 \, \mathfrak{e}1) + 66 \times (-9 + \mathfrak{e}1) - \\
& \mu_2 \, (991 + 25 \, \mathfrak{e}1) + \mu_1 \, (706 + 44 \, \mathfrak{e}1 + \mu_2 \, (4341 + 359 \, \mathfrak{e}1)))) + \\
& (-1 + \eta t) \, \theta l \, (360 + 1112 \, \mu_1 + 752 \, \mu_1^2 - 28 \, \mu_2 - 336 \, \mu_1 \, \mu_2 - \\
& 336 \, \mu_2^2 + 360 \, \mathfrak{e}1 + 774 \, \mu_1 \, \mathfrak{e}1 - 60 \, \mu_1^2 \, \mathfrak{e}1 + 60 \, \mu_2 \, \mathfrak{e}1 - 372 \, \mu_1 \, \mu_2 \, \mathfrak{e}1 + \\
& \theta p \, (1506 + 407 \, \mathfrak{e}1 + 225 \, \mathfrak{e}1^2 + 4 \, \mu_2^2 \, (638 + 189 \, \mathfrak{e}1 - 401 \, \mathfrak{e}2) + 27 \, \mathfrak{e}2 - \\
& 225 \, \mathfrak{e}1 \, \mathfrak{e}2 + \mu_2 \, (6720 + 1467 \, \mathfrak{e}1 + 225 \, \mathfrak{e}1^2 + 473 \, \mathfrak{e}2 - 225 \, \mathfrak{e}1 \, \mathfrak{e}2) + \\
& \mu_1^2 \, (2770 + 52 \, \mathfrak{e}1^2 + 260 \, \mathfrak{e}2 + \mathfrak{e}1 \, (284 + 42 \, \mathfrak{e}2)) + \\
& \mu_1 \, (4276 + 631 \, \mathfrak{e}1 + 577 \, \mathfrak{e}1^2 + 287 \, \mathfrak{e}2 - 483 \, \mathfrak{e}1 \, \mathfrak{e}2 + \\
& \mu_2 \, (10184 + 339 \, \mathfrak{e}1 + 225 \, \mathfrak{e}1^2 + 1269 \, \mathfrak{e}2 - 285 \, \mathfrak{e}1 \, \mathfrak{e}2)))) + \\
& \eta^4 \, (2 \, \theta p \, (-1569 - 1413 \, \mu_2 + 7648 \, \mu_2^2 + 71 \, \mathfrak{e}1 + 155 \, \mu_2 \, \mathfrak{e}1 - \\
& 20 \, \mu_1^2 \, (81 + 29 \, \mathfrak{e}1) + \mu_1 \, (-3189 + 1131 \, \mu_2 - 779 \, \mathfrak{e}1 + 989 \, \mu_2 \, \mathfrak{e}1) + \\
& \eta t \, (261 + 959 \, \mu_2 - 252 \, \mu_2^2 - 135 \, \mathfrak{e}1 - 145 \, \mu_2 \, \mathfrak{e}1 + \\
& 12 \, \mu_1^2 \, (46 + 37 \, \mathfrak{e}1) + \mu_1 \, (813 + 2451 \, \mu_2 - 615 \, \mathfrak{e}1 + 545 \, \mu_2 \, \mathfrak{e}1))) - \\
& (-1 + \eta t) \, \theta l \, (372 - 144 \, \mu_1 - 516 \, \mu_1^2 + 53 \, \mu_2 - 4443 \, \mu_1 \, \mu_2 - \\
& 24 \, \mu_2^2 + 300 \, \mathfrak{e}1 + 980 \, \mu_1 \, \mathfrak{e}1 - 172 \, \mu_1^2 \, \mathfrak{e}1 + 75 \, \mu_2 \, \mathfrak{e}1 - 285 \, \mu_1 \, \mu_2 \, \mathfrak{e}1 + \\
& 5 \, \theta p \, (8 \, \mu_2^2 \, (80 + 9 \, \mathfrak{e}1 - 90 \, \mathfrak{e}2) + \mu_2 \, (3858 + 301 \, \mathfrak{e}1 + 45 \, \mathfrak{e}1^2 + 69 \, \mathfrak{e}2 - \\
& 45 \, \mathfrak{e}1 \, \mathfrak{e}2) + 3 \times (354 + 41 \, \mathfrak{e}1 + 15 \, \mathfrak{e}1^2 - 7 \, \mathfrak{e}2 - 15 \, \mathfrak{e}1 \, \mathfrak{e}2) + \\
& \mu_1^2 \, (1420 + 35 \, \mathfrak{e}1^2 + 143 \, \mathfrak{e}2 + \mathfrak{e}1 \, (105 + 17 \, \mathfrak{e}2)) + \\
& \mu_1 \, (\mu_2 \, (4370 - 139 \, \mathfrak{e}1 + 45 \, \mathfrak{e}1^2 + 517 \, \mathfrak{e}2 - 153 \, \mathfrak{e}1 \, \mathfrak{e}2) + \\
& 2 \times (1241 + 168 \, \mathfrak{e}1 + 94 \, \mathfrak{e}1^2 + 61 \, \mathfrak{e}2 - 68 \, \mathfrak{e}1 \, \mathfrak{e}2))) - \\
& \eta^2 \, (2 \, \theta p \, (6 \times (102 + 469 \, \mu_2 + 384 \, \mu_2^2 + 54 \, \mathfrak{e}1 + 65 \, \mu_2 \, \mathfrak{e}1 + 3 \, \mu_1^2 \\
& (63 + \mathfrak{e}1) + \mu_1 \, (291 + 637 \, \mu_2 + 75 \, \mathfrak{e}1 + 17 \, \mu_2 \, \mathfrak{e}1)) + \\
& \eta t \, (-508 - 259 \, \mu_2 + 588 \, \mu_2^2 - 336 \, \mathfrak{e}1 - 129 \, \mu_2 \, \mathfrak{e}1 + 12 \, \mu_1^2 \\
& (11 + 38 \, \mathfrak{e}1) + \mu_1 \, (-376 + 1317 \, \mu_2 - 786 \, \mathfrak{e}1 + 627 \, \mu_2 \, \mathfrak{e}1))) + \\
& (-1 + \eta t) \, \theta l \, (2 \times (148 - 359 \, \mu_2 - 504 \, \mu_2^2 + 240 \, \mathfrak{e}1 + 15 \, \mu_2 \, \mathfrak{e}1 + \\
& 12 \, \mu_1^2 \, (43 + 3 \, \mathfrak{e}1) + \mu_1 \, (664 + 354 \, \mathfrak{e}1 - 3 \, \mu_2 \, (37 + 103 \, \mathfrak{e}1))) + \\
& 3 \, \theta p \, (\mu_1^2 \, (566 + \mathfrak{e}1^2 + 85 \, \mathfrak{e}2 + \mathfrak{e}1 \, (159 + 13 \, \mathfrak{e}2)) + \\
& 2 \times (162 + 81 \, \mathfrak{e}1 + 45 \, \mathfrak{e}1^2 + \mu_2^2 \, (532 + 234 \, \mathfrak{e}1 - 78 \, \mathfrak{e}2) + 33 \, \mathfrak{e}2 - \\
& 45 \, \mathfrak{e}1 \, \mathfrak{e}2 + \mu_2 \, (879 + 352 \, \mathfrak{e}1 + 45 \, \mathfrak{e}1^2 + 189 \, \mathfrak{e}2 - 45 \, \mathfrak{e}1 \, \mathfrak{e}2)) + \\
& \mu_1 \, (890 + 249 \, \mathfrak{e}1 + 163 \, \mathfrak{e}1^2 + 151 \, \mathfrak{e}2 - 149 \, \mathfrak{e}1 \, \mathfrak{e}2 + \\
& 2 \, \mu_2 \, (1283 + 272 \, \mathfrak{e}1 + 45 \, \mathfrak{e}1^2 + 247 \, \mathfrak{e}2 - 9 \, \mathfrak{e}1 \, \mathfrak{e}2)))) + \eta
\end{aligned}$$

$$\begin{aligned}
& \left( -4 \, \theta p \left( 3 \times \left( 9 + 41 \, \mu_2 + 16 \, \mu_2^2 - \mu_1^2 \left( -9 + \mathfrak{x}1 \right) + 5 \, \mathfrak{x}1 + 3 \, \mu_2 \, \mathfrak{x}1 + \right. \right. \right. \\
& \quad \left. \left. \mu_1 \left( 18 + 41 \, \mu_2 + 4 \, \mathfrak{x}1 + 3 \, \mu_2 \, \mathfrak{x}1 \right) \right) + \right. \\
& \quad \left. \eta t \left( -30 + 313 \, \mu_2 + 344 \, \mu_2^2 - 110 \, \mathfrak{x}1 - 13 \, \mu_2 \, \mathfrak{x}1 + \mu_1^2 \right. \right. \\
& \quad \left. \left. \left( -43 + 73 \, \mathfrak{x}1 \right) + \mu_1 \left( -73 + 273 \, \mu_2 - 163 \, \mathfrak{x}1 + 149 \, \mu_2 \, \mathfrak{x}1 \right) \right) \right) + \\
& \left( -1 + \eta t \right) \theta l \left( 4 \times \left( 4 + 92 \, \mu_2^2 + \mu_1^2 \left( -13 + \mathfrak{x}1 \right) - 20 \, \mathfrak{x}1 + \right. \right. \\
& \quad \left. \left. \mu_2 \left( 107 + 5 \, \mathfrak{x}1 \right) + \mu_1 \left( -9 - 22 \, \mathfrak{x}1 + \mu_2 \left( 105 + 41 \, \mathfrak{x}1 \right) \right) \right) + \right. \\
& \quad 3 \, \theta p \left( -60 - 31 \, \mathfrak{x}1 - 15 \, \mathfrak{x}1^2 - 21 \, \mathfrak{x}2 + 15 \, \mathfrak{x}1 \, \mathfrak{x}2 - 4 \, \mu_2^2 \right. \\
& \quad \left. \left( 50 + 27 \, \mathfrak{x}1 + 11 \, \mathfrak{x}2 \right) - \mu_2 \left( 312 + 145 \, \mathfrak{x}1 + 15 \, \mathfrak{x}1^2 + 103 \, \mathfrak{x}2 - \right. \right. \\
& \quad \left. \left. 15 \, \mathfrak{x}1 \, \mathfrak{x}2 \right) + 2 \, \mu_1^2 \left( \mathfrak{x}1^2 - 9 \times \left( 3 + \mathfrak{x}2 \right) - \mathfrak{x}1 \left( 20 + \mathfrak{x}2 \right) \right) - \right. \\
& \quad \left. \mu_1 \left( 114 + 59 \, \mathfrak{x}1 + 19 \, \mathfrak{x}1^2 + 39 \, \mathfrak{x}2 - 19 \, \mathfrak{x}1 \, \mathfrak{x}2 + \right. \right. \\
& \quad \left. \left. \mu_2 \left( 312 + 161 \, \mathfrak{x}1 + 15 \, \mathfrak{x}1^2 + 103 \, \mathfrak{x}2 + 9 \, \mathfrak{x}1 \, \mathfrak{x}2 \right) \right) \right) \right) - 2 \\
& \eta^5 \left( -2 \times \left( -1 + \eta t \right) \theta l \left( 24 \, \mu_2 + \mu_1 \left( 151 + 564 \, \mu_2 - 25 \, \mathfrak{x}1 \right) + \right. \right. \\
& \quad \left. \left. \mu_1^2 \left( 151 + 11 \, \mathfrak{x}1 \right) \right) + \theta p \left( -951 - 3921 \, \mu_1 - 2970 \, \mu_1^2 - \right. \right. \\
& \quad 4148 \, \mu_2 - 7016 \, \mu_1 \, \mu_2 - 1840 \, \mu_2^2 - 315 \, \mathfrak{x}1 - \\
& \quad 993 \, \mu_1 \, \mathfrak{x}1 - 246 \, \mu_1^2 \, \mathfrak{x}1 - 1064 \, \mu_2 \, \mathfrak{x}1 + 568 \, \mu_1 \, \mu_2 \, \mathfrak{x}1 - \\
& \quad 3 \, \theta l \left( 543 + 35 \, \mathfrak{x}1 + 2 \, \mu_2 \left( 894 + 27 \, \mathfrak{x}1 + 28 \, \mathfrak{x}2 \right) - 4 \, \mu_2^2 \left( -32 + 35 \, \mathfrak{x}2 \right) + \right. \\
& \quad \left. \mu_1^2 \left( 520 + 13 \, \mathfrak{x}1^2 + 71 \, \mathfrak{x}2 + \mathfrak{x}1 \left( 62 + 6 \, \mathfrak{x}2 \right) \right) + \right. \\
& \quad \left. \mu_1 \left( 1063 + 181 \, \mathfrak{x}1 + 34 \, \mathfrak{x}1^2 + 71 \, \mathfrak{x}2 - 15 \, \mathfrak{x}1 \, \mathfrak{x}2 + \right. \right. \\
& \quad \left. \left. \mu_2 \left( 1376 + 222 \, \mathfrak{x}2 - 6 \, \mathfrak{x}1 \left( 1 + 7 \, \mathfrak{x}2 \right) \right) \right) \right) + \\
& \quad \eta t \left( -2352 \, \mu_2^2 + 244 \, \mu_1 \left( -1 + \mathfrak{x}1 \right) + 144 \times \left( 4 + \mathfrak{x}1 \right) - 20 \, \mu_1^2 \right. \\
& \quad \left. \left( 41 + 4 \, \mathfrak{x}1 \right) + 6 \, \mu_2 \left( 27 + 5 \, \mathfrak{x}1 \right) - 6 \, \mu_1 \, \mu_2 \left( 625 + 109 \, \mathfrak{x}1 \right) + 3 \, \theta l \right. \\
& \quad \left. \left( 543 + 35 \, \mathfrak{x}1 + 2 \, \mu_2 \left( 894 + 27 \, \mathfrak{x}1 + 28 \, \mathfrak{x}2 \right) - 4 \, \mu_2^2 \left( -32 + 35 \, \mathfrak{x}2 \right) + \right. \right. \\
& \quad \left. \left. \mu_1^2 \left( 520 + 13 \, \mathfrak{x}1^2 + 71 \, \mathfrak{x}2 + \mathfrak{x}1 \left( 62 + 6 \, \mathfrak{x}2 \right) \right) + \right. \right. \\
& \quad \left. \left. \mu_1 \left( 1063 + 181 \, \mathfrak{x}1 + 34 \, \mathfrak{x}1^2 + 71 \, \mathfrak{x}2 - 15 \, \mathfrak{x}1 \, \mathfrak{x}2 + \right. \right. \right. \\
& \quad \left. \left. \left. \mu_2 \left( 1376 + 222 \, \mathfrak{x}2 - 6 \, \mathfrak{x}1 \left( 1 + 7 \, \mathfrak{x}2 \right) \right) \right) \right) \right) \right) \right) \Big/ \\
& \left( 96 \left( -1 + w \left( -1 + \eta \right) \right)^3 \left( x \left( -1 + \eta \right) - \eta \right)^3 \left( 1 + x + \eta - x \, \eta \right)^2 \right. \\
& \quad \left( w + \right. \\
& \quad \quad x + \\
& \quad \quad \eta - \\
& \quad \quad w \\
& \quad \quad \eta - x \\
& \quad \left. \left. \left. \eta \right)^3 \left( -1 + \eta t \right) \theta l \theta p \right) \right) \\
\beta_{\mathfrak{x}2} &= \left( \left( -1 + \eta \right) \times \right. \\
& \left( -2 \, f \left( -1 + w \left( -1 + \eta \right) \right) \left( x \left( -1 + \eta \right) - \eta \right) \left( w \left( -1 + \eta \right) + x \left( -1 + \eta \right) - \eta \right) \left( 1 + x + \eta - x \, \eta \right)^2 \right. \\
& \quad \left. \theta l \left( -2 + \mathfrak{x}2 + \mathfrak{x}2^2 \right) \left( x^2 \left( -1 + \eta \right)^2 \theta p \left( 6 - 4 \, \eta^2 - 2 \, \eta t - 6 \, \theta l + 6 \, \eta t \, \theta l + 2 \, \eta \right. \right. \right. \\
& \quad \left. \left. \left( -1 + \eta t \right) \times \left( 1 + \theta l \right) - 5 \, \theta l \, \mathfrak{x}2 + 5 \, \eta t \, \theta l \, \mathfrak{x}2 + w \left( -1 + \eta \right) \times \left( -10 + 2 \, \eta^2 - 2 \right. \right. \right. \\
& \quad \left. \left. \left. \eta \left( -4 + \eta t \right) + 2 \, \eta t + 5 \, \theta l \left( 2 + \mathfrak{x}2 \right) - 5 \, \eta t \, \theta l \left( 2 + \mathfrak{x}2 \right) \right) \right) + x \left( -1 + \eta \right) \times \right. \\
& \quad \left. \left( 2 \left( w \left( -1 + \eta \right) - 2 \, \eta \right) \left( -1 + \eta \right) \times \left( -3 - 2 \, \eta + w \left( -1 + \eta \right) \times \left( 5 + \eta - \eta t \right) + \eta t \right) \theta p - \right. \right. \\
& \quad \left. \left( -1 + \eta t \right) \theta l \left( 10 + 10 \, w^2 \left( -1 + \eta \right)^2 + \theta p \left( 4 \, \eta^2 - 5 \times \left( 2 + \mathfrak{x}2 \right) + 2 \, \eta \left( 6 + 5 \, \mathfrak{x}2 \right) \right) - w \right. \right. \\
& \quad \left. \left. \left( -1 + \eta \right) \times \left( 20 + \theta p \left( -14 + 22 \, \eta - 5 \, \mathfrak{x}2 + 10 \, \eta \, \mathfrak{x}2 \right) \right) \right) \right) + \\
& \quad \theta p \left( -4 \, \eta^4 - 2 \, w^2 \left( -1 + \eta \right)^3 \left( 5 + \eta \right) \left( \eta - \eta t \right) - 10 \, \eta t + 2 \, \eta^3 \left( -1 + \eta t \right) \times \left( 1 + \theta l \right) + \right. \\
& \quad \left. 5 \, \eta \, \theta l \left( 2 + \mathfrak{x}2 \right) - 5 \, \eta \, \eta t \left( -2 + \theta l \left( 2 + \mathfrak{x}2 \right) \right) + \right.
\end{aligned}$$

$$\begin{aligned}
& \eta^2 (6 - \theta l (6 + 5 \mathfrak{z}2) + \eta t (-2 + \theta l (6 + 5 \mathfrak{z}2))) + \\
& w (-1 + \eta) \times (2 \eta^4 - 2 \eta^3 (-6 + \eta t) + 20 \eta t + \eta^2 (-8 - (-1 + \eta t) \theta l (12 + 5 \mathfrak{z}2)) + \\
& \quad \eta (-6 - 14 \theta l - 5 \theta l \mathfrak{z}2 + \eta t (-18 + 14 \theta l + 5 \theta l \mathfrak{z}2))) + \\
& cv \, c\sigma (x (-1 + \eta) - \eta) (1 + x + \eta - x \eta)^2 ((x + \eta - x \eta)^2 (-1 + \eta t) \theta l \, \theta p \\
& \quad (1 + \mu 1) \times (-1 + \mathfrak{z}2) \times (14 x (-1 + \eta) - 14 \eta - 5 \times (2 + \mathfrak{z}1 + \mathfrak{z}2)) + \\
& w^4 (-1 + \eta)^4 (x (-1 + \eta) \times (4 \times (-1 + \eta) \, \theta p (5 - 7 \mu 1 + \eta (1 + \mu 1) \times (-1 + \mathfrak{z}2) - \\
& \quad \eta t (1 + \mu 1) \times (-1 + \mathfrak{z}2) + \mathfrak{z}2 - 5 \mu 1 \mathfrak{z}2) + (-1 + \eta t) \theta l \\
& \quad (-20 \times (1 + \mu 1) \times (-1 + \mathfrak{z}2) + \theta p (-64 + 15 \mathfrak{z}1 (-1 + \mathfrak{z}2) + 21 \mathfrak{z}2 - \\
& \quad 5 \mathfrak{z}2^2 + \mu 1 (-16 + 15 \mathfrak{z}1 (-1 + \mathfrak{z}2) + 93 \mathfrak{z}2 + 19 \mathfrak{z}2^2))) + \\
& \theta p (-4 \eta^3 (1 + \mu 1) \times (-1 + \mathfrak{z}2) - 20 \eta t (1 + \mu 1) \times (-1 + \mathfrak{z}2) + 4 \eta^2 \\
& \quad (\eta t (1 + \mu 1) \times (-1 + \mathfrak{z}2) + 6 \times (-1 + \mu 1 + \mu 1 \mathfrak{z}2)) + \eta \\
& \quad (4 \times (5 + \mathfrak{z}2 - \mu 1 (7 + 5 \mathfrak{z}2)) + \theta l (-64 + 15 \mathfrak{z}1 (-1 + \mathfrak{z}2) + 21 \mathfrak{z}2 - \\
& \quad 5 \mathfrak{z}2^2 + \mu 1 (-16 + 15 \mathfrak{z}1 (-1 + \mathfrak{z}2) + 93 \mathfrak{z}2 + 19 \mathfrak{z}2^2))) + \\
& \quad \eta t (16 \times (1 + \mu 1) \times (-1 + \mathfrak{z}2) + \theta l (64 - 15 \mathfrak{z}1 (-1 + \mathfrak{z}2) - 21 \mathfrak{z}2 + \\
& \quad 5 \mathfrak{z}2^2 + \mu 1 (16 - 15 \mathfrak{z}1 (-1 + \mathfrak{z}2) - 93 \mathfrak{z}2 - 19 \mathfrak{z}2^2)))) + \\
& w (-1 + \eta) \times (-4 x^3 (-1 + \eta)^3 \theta p (-7 + 14 \theta l + 5 \mu 1 + 2 \theta l \mu 1 + 3 \eta^2 (1 + \mu 1) \times \\
& \quad (-1 + \mathfrak{z}2) + \eta t (1 + \mu 1) \times (-1 + \mathfrak{z}2) + \mathfrak{z}2 - 8 \theta l \mathfrak{z}2 + 7 \mu 1 \mathfrak{z}2 - 14 \theta l \mu 1 \\
& \quad \mathfrak{z}2 + 2 \eta t \theta l (-7 + 4 \mathfrak{z}2 + \mu 1 (-1 + 7 \mathfrak{z}2)) + \eta (-\eta t (1 + 2 \theta l) \times (1 + \mu 1) \times \\
& \quad (-1 + \mathfrak{z}2) + 2 \times (5 - \mu 1 + \theta l (1 + \mu 1) \times (-1 + \mathfrak{z}2) - 2 \mathfrak{z}2 - 5 \mu 1 \mathfrak{z}2))) + \\
& x^2 (-1 + \eta)^2 \theta p (36 \eta^3 (1 + \mu 1) \times (-1 + \mathfrak{z}2) + (-1 + \eta t) \theta l (1 + \mu 1) \times \\
& \quad (-1 + \mathfrak{z}2) \times (58 + 15 \mathfrak{z}1 + 15 \mathfrak{z}2) - 12 \eta^2 (\eta t (1 + 2 \theta l) \times (1 + \mu 1) \times \\
& \quad (-1 + \mathfrak{z}2) + 2 \times (-5 + \mu 1 - \theta l (1 + \mu 1) \times (-1 + \mathfrak{z}2) + 2 \mathfrak{z}2 + 5 \mu 1 \mathfrak{z}2)) + \\
& 12 \eta (-7 + 5 \mu 1 + \eta t (1 + \mu 1) \times (-1 + \mathfrak{z}2) + \mathfrak{z}2 + 7 \mu 1 \mathfrak{z}2 - 2 \theta l \\
& \quad (-7 + 4 \mathfrak{z}2 + \mu 1 (-1 + 7 \mathfrak{z}2)) + 2 \eta t \theta l (-7 + 4 \mathfrak{z}2 + \mu 1 (-1 + 7 \mathfrak{z}2))) + \\
& x (-1 + \eta) \times (-12 \times (-1 + \eta) \eta^2 \theta p (7 - 5 \mu 1 + 3 \eta (1 + \mu 1) \times (-1 + \mathfrak{z}2) - \\
& \quad \eta t (1 + \mu 1) \times (-1 + \mathfrak{z}2) - \mathfrak{z}2 - 7 \mu 1 \mathfrak{z}2) + (-1 + \eta t) \theta l \\
& \quad (20 \times (1 + \mu 1) \times (-1 + \mathfrak{z}2) + \theta p (30 + 15 \mathfrak{z}1 + 24 \eta^3 (1 + \mu 1) \times (-1 + \mathfrak{z}2) - \\
& \quad 11 \mathfrak{z}2 - 15 \mathfrak{z}1 \mathfrak{z}2 + 5 \mathfrak{z}2^2 - 2 \eta (1 + \mu 1) \times (-1 + \mathfrak{z}2) \times \\
& \quad (58 + 15 \mathfrak{z}1 + 15 \mathfrak{z}2) + \mu 1 (30 - 15 \mathfrak{z}1 (-1 + \mathfrak{z}2) - 59 \mathfrak{z}2 - 19 \mathfrak{z}2^2) - \\
& \quad 24 \eta^2 (-7 + 4 \mathfrak{z}2 + \mu 1 (-1 + 7 \mathfrak{z}2)))) + \\
& \theta p (12 \eta^5 (1 + \mu 1) \times (-1 + \mathfrak{z}2) + 20 \eta t (1 + \mu 1) \times (-1 + \mathfrak{z}2) + \eta^2 \\
& \quad (-1 + \eta t) \theta l (1 + \mu 1) \times (-1 + \mathfrak{z}2) \times (58 + 15 \mathfrak{z}1 + 15 \mathfrak{z}2) - 4 \eta^4 \\
& \quad (\eta t (1 + 2 \theta l) \times (1 + \mu 1) \times (-1 + \mathfrak{z}2) + 2 \times (-5 + \mu 1 - \theta l (1 + \mu 1) \times \\
& \quad (-1 + \mathfrak{z}2) + 2 \mathfrak{z}2 + 5 \mu 1 \mathfrak{z}2)) + 4 \eta^3 (-7 + 5 \mu 1 + \eta t (1 + \mu 1) \times \\
& \quad (-1 + \mathfrak{z}2) + \mathfrak{z}2 + 7 \mu 1 \mathfrak{z}2 - 2 \theta l (-7 + 4 \mathfrak{z}2 + \mu 1 (-1 + 7 \mathfrak{z}2)) + \\
& 2 \eta t \theta l (-7 + 4 \mathfrak{z}2 + \mu 1 (-1 + 7 \mathfrak{z}2))) + \eta (\theta l (30 - 15 \mathfrak{z}1 (-1 + \mathfrak{z}2) - \\
& \quad 11 \mathfrak{z}2 + 5 \mathfrak{z}2^2 + \mu 1 (30 - 15 \mathfrak{z}1 (-1 + \mathfrak{z}2) - 59 \mathfrak{z}2 - 19 \mathfrak{z}2^2)) + \\
& \quad \eta t (-20 \times (1 + \mu 1) \times (-1 + \mathfrak{z}2) + \theta l (-30 + 15 \mathfrak{z}1 (-1 + \mathfrak{z}2) + 11 \mathfrak{z}2 - \\
& \quad 5 \mathfrak{z}2^2 + \mu 1 (-30 + 15 \mathfrak{z}1 (-1 + \mathfrak{z}2) + 59 \mathfrak{z}2 + 19 \mathfrak{z}2^2)))) + \\
& w^2 (-1 + \eta)^2 (2 x^3 (-1 + \eta)^3 \theta p (-10 + 17 \theta l + 14 \mu 1 - 7 \theta l \mu 1 + 2 \eta^2 \\
& \quad (1 + \mu 1) \times (-1 + \mathfrak{z}2) + 2 \eta t (1 + \mu 1) \times (-1 + \mathfrak{z}2) - 2 \mathfrak{z}2 - 5 \theta l \\
& \quad \mathfrak{z}2 + 10 \mu 1 \mathfrak{z}2 - 17 \theta l \mu 1 \mathfrak{z}2 + \eta t \theta l (-17 + 5 \mathfrak{z}2 + \mu 1 (7 + 17 \mathfrak{z}2)) - 2 \\
& \quad \eta (\eta t (1 + \mu 1) \times (-1 + \mathfrak{z}2) + 6 \times (-1 + \mu 1 + \mu 1 \mathfrak{z}2))) - \\
& x^2 (-1 + \eta)^2 \theta p (-56 + 142 \theta l + 40 \mu 1 + 46 \theta l \mu 1 + 15 \theta l \mathfrak{z}1 + 15 \theta l \mu 1
\end{aligned}$$

$$\begin{aligned}
& \mathfrak{z}1 + 12 \eta^3 (1 + \mu1) \times (-1 + \mathfrak{z}2) + 8 \eta t (1 + \mu1) \times (-1 + \mathfrak{z}2) + 8 \mathfrak{z}2 - 79 \mathfrak{e}l \\
& \mathfrak{z}2 + 56 \mu1 \mathfrak{z}2 - 127 \mathfrak{e}l \mu1 \mathfrak{z}2 - 15 \mathfrak{e}l \mathfrak{z}1 \mathfrak{z}2 - 15 \mathfrak{e}l \mu1 \mathfrak{z}1 \mathfrak{z}2 - 15 \mathfrak{e}l \mathfrak{z}2^2 - 15 \\
& \mathfrak{e}l \mu1 \mathfrak{z}2^2 - 12 \eta^2 (\eta t (1 + \mu1) \times (-1 + \mathfrak{z}2) + 2 \times (-1 + 2 \mu1) \times (2 + \mathfrak{z}2)) + \eta t \\
& \mathfrak{e}l (-142 + 15 \mathfrak{z}1 (-1 + \mathfrak{z}2) + 79 \mathfrak{z}2 + 15 \mathfrak{z}2^2 + \\
& \mu1 (-46 + 15 \mathfrak{z}1 (-1 + \mathfrak{z}2) + 127 \mathfrak{z}2 + 15 \mathfrak{z}2^2)) + 2 \eta \\
& (10 + 34 \mu1 + 2 \eta t (1 + \mu1) \times (-1 + \mathfrak{z}2) - 22 \mathfrak{z}2 - 10 \mu1 \mathfrak{z}2 - \mathfrak{e}l (-43 + \\
& 7 \mathfrak{z}2 + \mu1 (29 + 43 \mathfrak{z}2)) + \eta t \mathfrak{e}l (-43 + 7 \mathfrak{z}2 + \mu1 (29 + 43 \mathfrak{z}2))) + \\
& \times (-1 + \eta) \times (4 \times (-1 + \eta) \eta \mathfrak{e}p (3 \eta^2 (1 + \mu1) \times (-1 + \mathfrak{z}2) - 3 \eta \\
& (-1 + \eta t (1 + \mu1) \times (-1 + \mathfrak{z}2) - 5 \mathfrak{z}2 + \mu1 (11 + \mathfrak{z}2)) - \\
& 4 \times (-7 + \eta t (1 + \mu1) \times (-1 + \mathfrak{z}2) + \mathfrak{z}2 + \mu1 (5 + 7 \mathfrak{z}2))) + (-1 + \eta t) \mathfrak{e}l \\
& (-60 \times (1 + \mu1) \times (-1 + \mathfrak{z}2) + \mathfrak{e}p (-104 - 45 \mathfrak{z}1 + 47 \mathfrak{z}2 + 45 \mathfrak{z}1 \mathfrak{z}2 - 15 \mathfrak{z}2^2 + \\
& \mu1 (-104 + 45 \mathfrak{z}1 (-1 + \mathfrak{z}2) + 191 \mathfrak{z}2 + 57 \mathfrak{z}2^2) + \eta^2 (-2 \times (35 + \mathfrak{z}2) + \\
& \mu1 (74 + 70 \mathfrak{z}2)) + 2 \eta (-142 + 15 \mathfrak{z}1 (-1 + \mathfrak{z}2) + 79 \mathfrak{z}2 + \\
& 15 \mathfrak{z}2^2 + \mu1 (-46 + 15 \mathfrak{z}1 (-1 + \mathfrak{z}2) + 127 \mathfrak{z}2 + 15 \mathfrak{z}2^2)))) - \\
& \mathfrak{e}p (-4 \eta^4 (12 \mu1 + \eta t (1 + \mu1) \times (-1 + \mathfrak{z}2) - 6 \mathfrak{z}2) + 4 \eta^5 (1 + \mu1) \times \\
& (-1 + \mathfrak{z}2) + 60 \eta t (1 + \mu1) \times (-1 + \mathfrak{z}2) + 2 \eta^3 \\
& (-2 \eta t (1 + \mu1) \times (-1 + \mathfrak{z}2) + 6 \times (5 + \mu1 - 3 \mathfrak{z}2 - 5 \mu1 \mathfrak{z}2) + \\
& 3 \mathfrak{e}l (3 + \mathfrak{z}2 - \mu1 (5 + 3 \mathfrak{z}2)) + 3 \eta t \mathfrak{e}l (-3 - \mathfrak{z}2 + \mu1 (5 + 3 \mathfrak{z}2))) + \eta^2 \\
& (8 \times (-7 + \mathfrak{z}2 + \mu1 (5 + 7 \mathfrak{z}2)) - \mathfrak{e}l (-142 + 15 \mathfrak{z}1 (-1 + \mathfrak{z}2) + \\
& 79 \mathfrak{z}2 + 15 \mathfrak{z}2^2 + \mu1 (-46 + 15 \mathfrak{z}1 (-1 + \mathfrak{z}2) + 127 \mathfrak{z}2 + 15 \mathfrak{z}2^2))) + \\
& \eta t (8 \times (1 + \mu1) \times (-1 + \mathfrak{z}2) + \mathfrak{e}l (-142 + 15 \mathfrak{z}1 (-1 + \mathfrak{z}2) + 79 \mathfrak{z}2 + \\
& 15 \mathfrak{z}2^2 + \mu1 (-46 + 15 \mathfrak{z}1 (-1 + \mathfrak{z}2) + 127 \mathfrak{z}2 + 15 \mathfrak{z}2^2)))) + \eta \\
& (\mathfrak{e}l (104 - 45 \mathfrak{z}1 (-1 + \mathfrak{z}2) - 47 \mathfrak{z}2 + 15 \mathfrak{z}2^2 + \mu1 (104 - 45 \mathfrak{z}1 \\
& (-1 + \mathfrak{z}2) - 191 \mathfrak{z}2 - 57 \mathfrak{z}2^2)) + \eta t \\
& (-60 \times (1 + \mu1) \times (-1 + \mathfrak{z}2) + \mathfrak{e}l (-104 + 45 \mathfrak{z}1 (-1 + \mathfrak{z}2) + 47 \mathfrak{z}2 - \\
& 15 \mathfrak{z}2^2 + \mu1 (-104 + 45 \mathfrak{z}1 (-1 + \mathfrak{z}2) + 191 \mathfrak{z}2 + 57 \mathfrak{z}2^2)))) + \\
& w^3 (-1 + \eta)^3 (x^2 (-1 + \eta)^2 \mathfrak{e}p (-40 + 78 \mathfrak{e}l + 56 \mu1 - 18 \mathfrak{e}l \mu1 + 5 \mathfrak{e}l \mathfrak{z}1 + \\
& 5 \mathfrak{e}l \mu1 \mathfrak{z}1 + 8 \eta^2 (1 + \mu1) \times (-1 + \mathfrak{z}2) + 8 \eta t (1 + \mu1) \times \\
& (-1 + \mathfrak{z}2) - 8 \mathfrak{z}2 - 25 \mathfrak{e}l \mathfrak{z}2 + 40 \mu1 \mathfrak{z}2 - 73 \mathfrak{e}l \mu1 \mathfrak{z}2 - 5 \\
& \mathfrak{e}l \mathfrak{z}1 \mathfrak{z}2 - 5 \mathfrak{e}l \mu1 \mathfrak{z}1 \mathfrak{z}2 - 5 \mathfrak{e}l \mathfrak{z}2^2 - 5 \mathfrak{e}l \mu1 \mathfrak{z}2^2 - 8 \eta \\
& (\eta t (1 + \mu1) \times (-1 + \mathfrak{z}2) + 6 \times (-1 + \mu1 + \mu1 \mathfrak{z}2)) + \eta t \mathfrak{e}l (-78 + 5 \mathfrak{z}1 \\
& (-1 + \mathfrak{z}2) + 25 \mathfrak{z}2 + 5 \mathfrak{z}2^2 + \mu1 (18 + 5 \mathfrak{z}1 (-1 + \mathfrak{z}2) + 73 \mathfrak{z}2 + 5 \mathfrak{z}2^2))) - \\
& \times (-1 + \eta) \times (4 \times (-1 + \eta) \mathfrak{e}p (7 - 5 \mu1 + 4 \eta^2 (1 + \mu1) \times (-1 + \mathfrak{z}2) - \\
& \eta t (1 + \mu1) \times (-1 + \mathfrak{z}2) - \mathfrak{z}2 - 7 \mu1 \mathfrak{z}2 + \\
& \eta (17 - 31 \mu1 - 4 \eta t (1 + \mu1) \times (-1 + \mathfrak{z}2) + 7 \mathfrak{z}2 - 17 \mu1 \mathfrak{z}2)) + (-1 + \eta t) \\
& \mathfrak{e}l (-60 \times (1 + \mu1) \times (-1 + \mathfrak{z}2) + \mathfrak{e}p (-146 - 45 \mathfrak{z}1 + 65 \mathfrak{z}2 + \\
& 45 \mathfrak{z}1 \mathfrak{z}2 - 15 \mathfrak{z}2^2 + \mu1 (-98 + 45 \mathfrak{z}1 (-1 + \mathfrak{z}2) + 233 \mathfrak{z}2 + 57 \mathfrak{z}2^2) + \\
& 2 \eta (-74 + 5 \mathfrak{z}1 (-1 + \mathfrak{z}2) + 21 \mathfrak{z}2 + 5 \mathfrak{z}2^2 + \\
& \mu1 (22 + 5 \mathfrak{z}1 (-1 + \mathfrak{z}2) + 69 \mathfrak{z}2 + 5 \mathfrak{z}2^2)))) + \\
& \mathfrak{e}p (8 \eta^4 (1 + \mu1) \times (-1 + \mathfrak{z}2) + 60 \eta t (1 + \mu1) \times (-1 + \mathfrak{z}2) - 4 \eta^3 \\
& (2 \eta t (1 + \mu1) \times (-1 + \mathfrak{z}2) - 3 \times (3 + \mathfrak{z}2) + 3 \mu1 (5 + 3 \mathfrak{z}2)) + \eta^2 \\
& (48 \mu1 - 24 \mathfrak{z}2 - \mathfrak{e}l (-70 + 5 \mathfrak{z}1 (-1 + \mathfrak{z}2) + 17 \mathfrak{z}2 + \\
& 5 \mathfrak{z}2^2 + \mu1 (26 + 5 \mathfrak{z}1 (-1 + \mathfrak{z}2) + 65 \mathfrak{z}2 + 5 \mathfrak{z}2^2)) + \\
& \eta t (4 \times (1 + \mu1) \times (-1 + \mathfrak{z}2) + \mathfrak{e}l (-70 + 5 \mathfrak{z}1 (-1 + \mathfrak{z}2) + 17 \mathfrak{z}2 +
\end{aligned}$$

$$\begin{aligned}
& 5 \mathfrak{z}^2 + \mu 1 \left( 26 + 5 \mathfrak{z} 1 (-1 + \mathfrak{z} 2) + 65 \mathfrak{z} 2 + 5 \mathfrak{z}^2 \right) \Big) \Big) + \eta \\
& \left( 4 \times (-7 + \mathfrak{z} 2 + \mu 1 (5 + 7 \mathfrak{z} 2)) + \mathfrak{e} \mathfrak{l} (146 - 45 \mathfrak{z} 1 (-1 + \mathfrak{z} 2) - \right. \\
& \quad 65 \mathfrak{z} 2 + 15 \mathfrak{z}^2 + \mu 1 (98 - 45 \mathfrak{z} 1 (-1 + \mathfrak{z} 2) - 233 \mathfrak{z} 2 - 57 \mathfrak{z}^2) \Big) + \\
& \quad \eta \mathfrak{t} (-56 \times (1 + \mu 1) \times (-1 + \mathfrak{z} 2) + \mathfrak{e} \mathfrak{l} (-146 + 45 \mathfrak{z} 1 (-1 + \mathfrak{z} 2) + 65 \mathfrak{z} 2 - \\
& \quad \quad 15 \mathfrak{z}^2 + \mu 1 (-98 + 45 \mathfrak{z} 1 (-1 + \mathfrak{z} 2) + 233 \mathfrak{z} 2 + 57 \mathfrak{z}^2) \Big) \Big) \Big) \Big) + \\
& 2 \mathfrak{c} \sigma^2 (-1 + \eta) \times \left( 2 \mathfrak{x}^6 (-1 + \eta)^6 \mathfrak{e} \mathfrak{p} (-2 + 2 \mathfrak{e} \mathfrak{l} + 3 \mu 1 + 9 \mathfrak{w} \mu 1 + 4 \mathfrak{w}^2 \mu 1 + \right. \\
& \quad \mathfrak{e} \mathfrak{l} \mu 1 - \mathfrak{w} \mathfrak{e} \mathfrak{l} \mu 1 + 17 \mu 1^2 + 21 \mathfrak{w} \mu 1^2 + 4 \mathfrak{w}^2 \mu 1^2 - \\
& \quad 13 \mathfrak{e} \mathfrak{l} \mu 1^2 - 13 \mathfrak{w} \mathfrak{e} \mathfrak{l} \mu 1^2 + \mathfrak{w}^2 \eta^4 (1 + \mu 1) \times (-1 + \mathfrak{z} 2) - \\
& \quad \mathfrak{w} \eta^3 (3 + \mathfrak{w} (3 + \eta \mathfrak{t} - 4 \mu 1)) \times (1 + \mu 1) \times (-1 + \mathfrak{z} 2) + 2 \mathfrak{z} 2 - 2 \mathfrak{e} \mathfrak{l} \mathfrak{z} 2 - \\
& \quad 9 \mu 1 \mathfrak{z} 2 - 15 \mathfrak{w} \mu 1 \mathfrak{z} 2 - 4 \mathfrak{w}^2 \mu 1 \mathfrak{z} 2 + 5 \mathfrak{e} \mathfrak{l} \mu 1 \mathfrak{z} 2 + 7 \mathfrak{w} \mathfrak{e} \mathfrak{l} \mu 1 \mathfrak{z} 2 - \\
& \quad 5 \mu 1^2 \mathfrak{z} 2 - 9 \mathfrak{w} \mu 1^2 \mathfrak{z} 2 - 4 \mathfrak{w}^2 \mu 1^2 \mathfrak{z} 2 + \mathfrak{e} \mathfrak{l} \mu 1^2 \mathfrak{z} 2 + \mathfrak{w} \mathfrak{e} \mathfrak{l} \mu 1^2 \mathfrak{z} 2 + \\
& \quad \eta^2 (2 \times (1 + \mu 1) \times (-1 + \mathfrak{z} 2) + 3 \mathfrak{w}^2 (1 + \eta \mathfrak{t} - 4 \mu 1) \times (1 + \mu 1) \times (-1 + \mathfrak{z} 2) + 3 \mathfrak{w} \\
& \quad \quad (\mu 1 + \mu 1^2 (7 - 3 \mathfrak{z} 2) + 2 \times (-1 + \mathfrak{z} 2) + \eta \mathfrak{t} (1 + \mu 1) \times (-1 + \mathfrak{z} 2) - 3 \mu 1 \mathfrak{z} 2) \Big) + \\
& \quad \eta \mathfrak{t} (2 \times (1 + \mu 1) \times (-1 + \mathfrak{z} 2) + \mathfrak{w}^2 (1 + \mu 1) \times (-1 + \mathfrak{z} 2) - \mathfrak{e} \mathfrak{l} \\
& \quad \quad (2 + \mu 1 + \mu 1^2 (-13 + \mathfrak{z} 2) - 2 \mathfrak{z} 2 + 5 \mu 1 \mathfrak{z} 2) + \mathfrak{w} \\
& \quad \quad (-\mathfrak{e} \mathfrak{l} \mu 1^2 (-13 + \mathfrak{z} 2) + 3 \times (-1 + \mathfrak{z} 2) + \mu 1 (-3 + \mathfrak{e} \mathfrak{l} + 3 \mathfrak{z} 2 - 7 \mathfrak{e} \mathfrak{l} \mathfrak{z} 2) \Big) \Big) + \\
& \quad \eta (4 + 2 \eta \mathfrak{t} - \mu 1 + 2 \eta \mathfrak{t} \mu 1 - 17 \mu 1^2 - \mathfrak{w}^2 (1 + 3 \eta \mathfrak{t} - 12 \mu 1) \times (1 + \mu 1) \times \\
& \quad \quad (-1 + \mathfrak{z} 2) - 4 \mathfrak{z} 2 - 2 \eta \mathfrak{t} \mathfrak{z} 2 + 7 \mu 1 \mathfrak{z} 2 - 2 \eta \mathfrak{t} \mu 1 \mathfrak{z} 2 + 5 \mu 1^2 \mathfrak{z} 2 + \mathfrak{w} (3 - 3 \mathfrak{z} 2 + \\
& \quad \quad \mu 1 (-15 + \mathfrak{e} \mathfrak{l} + 27 \mathfrak{z} 2 - 7 \mathfrak{e} \mathfrak{l} \mathfrak{z} 2) + \mu 1^2 (-42 + 13 \mathfrak{e} \mathfrak{l} + 18 \mathfrak{z} 2 - \mathfrak{e} \mathfrak{l} \mathfrak{z} 2) + \\
& \quad \quad \eta \mathfrak{t} (6 + \mathfrak{e} \mathfrak{l} \mu 1^2 (-13 + \mathfrak{z} 2) - 6 \mathfrak{z} 2 + \mu 1 (6 - \mathfrak{e} \mathfrak{l} - 6 \mathfrak{z} 2 + 7 \mathfrak{e} \mathfrak{l} \mathfrak{z} 2) \Big) \Big) \Big) + \\
& \mathfrak{e} \mathfrak{p} (\mathfrak{w}^4 (-1 + \eta)^5 (2 \eta^5 (1 + \mu 1) \times (-1 + \mathfrak{z} 2) + 5 \eta \mathfrak{t} (1 + \mu 1) \mu 2 (-1 + \mathfrak{z} 2) + 2 \eta \eta \mathfrak{t} \\
& \quad (-1 + 5 \mu 1 (-2 + \mu 2) \times (-1 + \mathfrak{z} 2) + 5 \mu 2 (-1 + \mathfrak{z} 2) - 5 \mathfrak{z} 2 + \mu 1^2 (23 + \mathfrak{z} 2) \Big) - 2 \\
& \quad \eta^4 (-4 \mu 1^2 (-1 + \mathfrak{z} 2) + \eta \mathfrak{t} (1 + \mu 1) \times (-1 + \mathfrak{z} 2) - 2 \times (-1 + 3 \mu 2 + \mathfrak{z} 2) + \\
& \quad \quad 6 \mu 1 (1 + \mu 2 - \mathfrak{z} 2 + \mu 2 \mathfrak{z} 2) \Big) + 2 \eta^3 (13 \mu 2 + 6 \mathfrak{z} 2 + 11 \mu 2 \mathfrak{z} 2 + \\
& \quad \quad \mu 1^2 (-19 + 7 \mathfrak{z} 2) + 2 \eta \mathfrak{t} (1 + \mu 1 - 3 \mu 2 - \mathfrak{z} 2 - \mu 1 \mathfrak{z} 2 + 3 \mu 1 \mu 2 (1 + \mathfrak{z} 2) \Big) - \\
& \quad \quad \mu 1 (19 - 13 \mathfrak{z} 2 + \mu 2 (35 + 13 \mathfrak{z} 2) \Big) \Big) + \eta^2 \\
& \quad (2 + 10 \mathfrak{z} 2 - 12 \eta \mathfrak{t} \mathfrak{z} 2 + \mu 2 (-10 - 17 \eta \mathfrak{t} + 22 \mathfrak{z} 2 + 5 \eta \mathfrak{t} \mathfrak{z} 2) + \\
& \quad \quad \mu 1^2 (6 \times (-5 + \mathfrak{z} 2) + \eta \mathfrak{t} (70 + 26 \mathfrak{z} 2) + \mu 1 (2 \times (-14 - 17 \mu 2 + \\
& \quad \quad 8 \mathfrak{z} 2 + 5 \mu 2 \mathfrak{z} 2) + \eta \mathfrak{t} (-2 + 7 \mu 2 - 22 \mathfrak{z} 2 + 17 \mu 2 \mathfrak{z} 2) \Big) \Big) \Big) - \\
& \mathfrak{w}^3 (-1 + \eta)^3 (4 \eta^7 (1 + \mu 1) \times (-1 + \mathfrak{z} 2) - 15 \eta \mathfrak{t} (1 + \mu 1) \mu 2 (-1 + \mathfrak{z} 2) - \\
& \quad 2 \eta^6 (5 - 12 \mu 2 - 13 \mu 1 (-1 + \mathfrak{z} 2) - 8 \mu 1^2 (-1 + \mathfrak{z} 2) + \\
& \quad \quad 2 \eta \mathfrak{t} (1 + \mu 1) \times (-1 + \mathfrak{z} 2) - 5 \mathfrak{z} 2 + 12 \mu 1 \mu 2 (1 + \mathfrak{z} 2) \Big) - 2 \\
& \quad \eta \eta \mathfrak{t} (-4 - 17 \mu 2 - 20 \mathfrak{z} 2 + 5 \mu 2 \mathfrak{z} 2 + 4 \mu 1^2 (20 + \mathfrak{z} 2) + \\
& \quad \quad \mu 1 (40 - 34 \mathfrak{z} 2 + \mu 2 (7 + 17 \mathfrak{z} 2) \Big) \Big) + 2 \eta^5 (1 + 32 \mu 2 + 11 \mathfrak{z} 2 + 22 \mu 2 \mathfrak{z} 2 + \\
& \quad \quad 3 \mu 1^2 (-17 + 5 \mathfrak{z} 2) - 2 \mu 1 (19 + 38 \mu 2 - 16 \mathfrak{z} 2 + 16 \mu 2 \mathfrak{z} 2) + \\
& \quad \quad \eta \mathfrak{t} (5 - 12 \mu 2 - 5 \mathfrak{z} 2 + \mu 1 (5 - 5 \mathfrak{z} 2 + 12 \mu 2 (1 + \mathfrak{z} 2) \Big) \Big) \Big) + \eta^2 \\
& \quad (-8 + 12 \mu 2 + \mathfrak{e} \mathfrak{l} \mathfrak{z} 1 - 5 \mathfrak{e} \mathfrak{l} \mu 2 \mathfrak{z} 1 - 2 \mu 1^2 (12 \mathfrak{e} \mathfrak{l} (\mathfrak{z} 1 - \mathfrak{z} 2) + 5 \times (-13 + \mathfrak{z} 2) \Big) + \\
& \quad \quad \mu 1 (98 - 12 \mu 2 (-9 + \mathfrak{z} 2) + 11 \mathfrak{e} \mathfrak{l} (\mathfrak{z} 1 - \mathfrak{z} 2) (-1 + \mathfrak{z} 2) + \\
& \quad \quad 5 \mathfrak{e} \mathfrak{l} \mu 2 (\mathfrak{z} 1 - \mathfrak{z} 2) (-1 + \mathfrak{z} 2) - 62 \mathfrak{z} 2 - 40 \mathfrak{z} 2 - \mathfrak{e} \mathfrak{l} \mathfrak{z} 2 - \\
& \quad \quad 60 \mu 2 \mathfrak{z} 2 + 5 \mathfrak{e} \mathfrak{l} \mu 2 \mathfrak{z} 2 + 5 \mathfrak{e} \mathfrak{l} \mathfrak{z} 1 \mathfrak{z} 2 + 5 \mathfrak{e} \mathfrak{l} \mu 2 \mathfrak{z} 1 \mathfrak{z} 2 - 5 \mathfrak{e} \mathfrak{l} \mathfrak{z}^2 - \\
& \quad \quad 5 \mathfrak{e} \mathfrak{l} \mu 2 \mathfrak{z}^2 + \eta \mathfrak{t} (-2 - \mathfrak{e} \mathfrak{l} \mathfrak{z} 1 - 5 \mathfrak{e} \mathfrak{l} \mu 2 (\mathfrak{z} 1 - \mathfrak{z} 2) (-1 + \mathfrak{z} 2) + \\
& \quad \quad 26 \mathfrak{z} 2 + \mathfrak{e} \mathfrak{l} \mathfrak{z} 2 - 5 \mathfrak{e} \mathfrak{l} \mathfrak{z} 1 \mathfrak{z} 2 + 5 \mathfrak{e} \mathfrak{l} \mathfrak{z}^2 + 24 \mu 2 (2 + \mathfrak{z} 2) + \\
& \quad \quad \mu 1 (10 - 11 \mathfrak{e} \mathfrak{l} (\mathfrak{z} 1 - \mathfrak{z} 2) (-1 + \mathfrak{z} 2) - 5 \mathfrak{e} \mathfrak{l} \mu 2 (\mathfrak{z} 1 - \mathfrak{z} 2) (-1 + \mathfrak{z} 2) + 62 \\
& \quad \quad \mathfrak{z} 2 - 48 \mu 2 (2 + \mathfrak{z} 2) \Big) \Big) + 12 \mu 1^2 (2 \mathfrak{e} \mathfrak{l} (\mathfrak{z} 1 - \mathfrak{z} 2) - 5 \times (3 + \mathfrak{z} 2) \Big) \Big) \Big) +
\end{aligned}$$

$$\begin{aligned}
& \eta^4 \left( 18 + 4 \mu_2 + \theta_1 \mathfrak{x}_1 - 5 \theta_1 \mu_2 \mathfrak{x}_1 + 30 \mathfrak{x}_2 - \theta_1 \mathfrak{x}_2 + 68 \mu_2 \mathfrak{x}_2 + \right. \\
& \quad 5 \theta_1 \mu_2 \mathfrak{x}_2 + 5 \theta_1 \mathfrak{x}_1 \mathfrak{x}_2 + 5 \theta_1 \mu_2 \mathfrak{x}_1 \mathfrak{x}_2 - 5 \theta_1 \mathfrak{x}_2^2 - 5 \theta_1 \mu_2 \mathfrak{x}_2^2 - \\
& \quad 6 \mu_1^2 (19 + 4 \theta_1 (\mathfrak{x}_1 - \mathfrak{x}_2) + \mathfrak{x}_2) + \mu_1 (36 \times (-2 + \mathfrak{x}_2) + 11 \theta_1 (\mathfrak{x}_1 - \mathfrak{x}_2) \\
& \quad \quad (-1 + \mathfrak{x}_2) + 5 \theta_1 \mu_2 (\mathfrak{x}_1 - \mathfrak{x}_2) (-1 + \mathfrak{x}_2) - 4 \mu_2 (35 + \mathfrak{x}_2)) + \\
& \quad \eta t (-2 - \theta_1 \mathfrak{x}_1 - 5 \theta_1 \mu_2 (\mathfrak{x}_1 - \mathfrak{x}_2) (-1 + \mathfrak{x}_2) - 22 \mathfrak{x}_2 + \theta_1 \mathfrak{x}_2 - \\
& \quad \quad 5 \theta_1 \mathfrak{x}_1 \mathfrak{x}_2 + 5 \theta_1 \mathfrak{x}_2^2 - 9 \mu_2 (7 + \mathfrak{x}_2) + 4 \mu_1^2 \\
& \quad \quad (31 + 6 \theta_1 (\mathfrak{x}_1 - \mathfrak{x}_2) + 5 \mathfrak{x}_2) + \mu_1 (26 - 11 \theta_1 (\mathfrak{x}_1 - \mathfrak{x}_2) (-1 + \mathfrak{x}_2) - \\
& \quad \quad \quad 5 \theta_1 \mu_2 (\mathfrak{x}_1 - \mathfrak{x}_2) (-1 + \mathfrak{x}_2) - 50 \mathfrak{x}_2 + 9 \mu_2 (9 + 7 \mathfrak{x}_2)) \left. \right) + 2 \\
& \eta^3 \left( 1 - 52 \mu_2 + \theta_1 \mathfrak{x}_1 - 5 \theta_1 \mu_2 \mathfrak{x}_1 - 13 \mathfrak{x}_2 - \theta_1 \mathfrak{x}_2 - 26 \mu_2 \mathfrak{x}_2 + \right. \\
& \quad 5 \theta_1 \mu_2 \mathfrak{x}_2 + 5 \theta_1 \mathfrak{x}_1 \mathfrak{x}_2 + 5 \theta_1 \mu_2 \mathfrak{x}_1 \mathfrak{x}_2 - 5 \theta_1 \mathfrak{x}_2^2 - 5 \theta_1 \mu_2 \mathfrak{x}_2^2 - \\
& \quad 3 \mu_1^2 (-17 + 8 \theta_1 (\mathfrak{x}_1 - \mathfrak{x}_2) + 5 \mathfrak{x}_2) + \mu_1 (40 + 11 \theta_1 (\mathfrak{x}_1 - \mathfrak{x}_2) (-1 + \mathfrak{x}_2) + \\
& \quad \quad 5 \theta_1 \mu_2 (\mathfrak{x}_1 - \mathfrak{x}_2) (-1 + \mathfrak{x}_2) - 34 \mathfrak{x}_2 + 52 \mu_2 (2 + \mathfrak{x}_2)) + \\
& \quad \eta t (-9 - \theta_1 \mathfrak{x}_1 - 15 \mathfrak{x}_2 + \theta_1 \mathfrak{x}_2 - 5 \theta_1 \mathfrak{x}_1 \mathfrak{x}_2 + 5 \theta_1 \mathfrak{x}_2^2 + \\
& \quad \quad 12 \mu_1^2 (9 + 2 \theta_1 (\mathfrak{x}_1 - \mathfrak{x}_2) + 2 \mathfrak{x}_2) + 5 \mu_2 (-1 + \mathfrak{x}_2) \times \\
& \quad \quad (1 + \theta_1 (-\mathfrak{x}_1 + \mathfrak{x}_2)) + \mu_1 (15 - 11 \theta_1 (\mathfrak{x}_1 - \mathfrak{x}_2) (-1 + \mathfrak{x}_2) - \\
& \quad \quad \quad 33 \mathfrak{x}_2 + 5 \mu_2 (-1 + \mathfrak{x}_2) \times (1 + \theta_1 (-\mathfrak{x}_1 + \mathfrak{x}_2))) \left. \right) + \\
& w^2 (-1 + \eta)^2 \left( 2 \eta^8 (1 + \mu_1) \times (-1 + \mathfrak{x}_2) - 15 \eta t (1 + \mu_1) \mu_2 (-1 + \mathfrak{x}_2) - \right. \\
& \quad 2 \eta^7 (7 - 6 \mu_2 - 4 \mu_1^2 (-1 + \mathfrak{x}_2) + \eta t (1 + \mu_1) \times (-1 + \mathfrak{x}_2) - \\
& \quad \quad 7 \mathfrak{x}_2 + \mu_1 (11 + 6 \mu_2 - 11 \mathfrak{x}_2 + 6 \mu_2 \mathfrak{x}_2)) - 12 \eta \eta t \\
& \quad \quad (-1 - 6 \mu_2 - 5 \mathfrak{x}_2 + \mu_1^2 (17 + \mathfrak{x}_2) + \mu_1 (10 - 7 \mathfrak{x}_2 + 6 \mu_2 (1 + \mathfrak{x}_2))) \left. \right) + 2 \eta^6 \\
& \quad (-6 + 43 \mu_2 + 12 \mathfrak{x}_2 + 11 \mu_2 \mathfrak{x}_2 + 3 \mu_1^2 (-19 + 7 \mathfrak{x}_2) - \mu_1 (39 + 65 \mu_2 - 45 \mathfrak{x}_2 + \\
& \quad \quad 43 \mu_2 \mathfrak{x}_2) + \eta t (7 - 6 \mu_2 - 7 \mathfrak{x}_2 + \mu_1 (7 - 7 \mathfrak{x}_2 + 6 \mu_2 (1 + \mathfrak{x}_2))) \left. \right) + \\
& \eta^5 \left( 26 + 72 \mu_2 + 46 \mathfrak{x}_2 + 108 \mu_2 \mathfrak{x}_2 + 2 \mu_1^2 (-121 + 13 \mathfrak{x}_2) + \right. \\
& \quad \theta_1 \mu_1^2 (-52 + 3 \mathfrak{x}_1 (-5 + \mathfrak{x}_2) + 15 \mathfrak{x}_2 + \mathfrak{x}_2^2) - \\
& \quad 36 \mu_1 (4 - 3 \mathfrak{x}_2 + 2 \mu_2 (4 + \mathfrak{x}_2)) + 2 \theta_1 (1 + 5 \mathfrak{x}_2 + \mu_2 (7 + 11 \mathfrak{x}_2)) - \\
& \quad \theta_1 \mu_1 (26 + 3 \mathfrak{x}_1 - 25 \mathfrak{x}_2 - 9 \mathfrak{x}_1 \mathfrak{x}_2 + 5 \mathfrak{x}_2^2 + 2 \mu_2 (17 + 13 \mathfrak{x}_2 + 6 \mathfrak{x}_2^2)) + \\
& \quad \eta t (14 - 68 \mu_2 - 14 \mathfrak{x}_2 - 4 \mu_2 \mathfrak{x}_2 + 8 \mu_1^2 (5 + \mathfrak{x}_2) - \\
& \quad \quad \theta_1 \mu_1^2 (-52 + 3 \mathfrak{x}_1 (-5 + \mathfrak{x}_2) + 15 \mathfrak{x}_2 + \mathfrak{x}_2^2) - 2 \theta_1 (1 + 5 \mathfrak{x}_2 + \\
& \quad \quad \quad \mu_2 (7 + 11 \mathfrak{x}_2)) + 2 \mu_1 (3 - 15 \mathfrak{x}_2 + \mu_2 (38 + 34 \mathfrak{x}_2)) + \theta_1 \mu_1 \\
& \quad \quad \quad (26 + 3 \mathfrak{x}_1 - 25 \mathfrak{x}_2 - 9 \mathfrak{x}_1 \mathfrak{x}_2 + 5 \mathfrak{x}_2^2 + 2 \mu_2 (17 + 13 \mathfrak{x}_2 + 6 \mathfrak{x}_2^2))) \left. \right) + \\
& \eta^4 \left( 28 - 26 \mu_1 - 30 \mu_1^2 - 108 \mu_2 + 36 \mu_1 \mu_2 + 20 \mathfrak{x}_2 - 34 \mu_1 \mathfrak{x}_2 - \right. \\
& \quad 42 \mu_1^2 \mathfrak{x}_2 + 36 \mu_2 \mathfrak{x}_2 + 108 \mu_1 \mu_2 \mathfrak{x}_2 + \theta_1 (\mu_1^2 (-56 + 89 \mathfrak{x}_2 + 3 \mathfrak{x}_2^2 + \\
& \quad \quad \mathfrak{x}_1 (-89 + 5 \mathfrak{x}_2)) + \mu_1 (-26 - 38 \mathfrak{x}_1 + 56 \mathfrak{x}_2 + 44 \mathfrak{x}_1 \mathfrak{x}_2 - 36 \mathfrak{x}_2^2 + \\
& \quad \quad 3 \mu_2 (-2 + 5 \mathfrak{x}_1 (-1 + \mathfrak{x}_2) + 3 \mathfrak{x}_2 - 9 \mathfrak{x}_2^2)) + 3 \times (2 + \mathfrak{x}_1 + \mathfrak{x}_2 + \\
& \quad \quad 5 \mathfrak{x}_1 \mathfrak{x}_2 - 5 \mathfrak{x}_2^2 + \mu_2 (-2 + 5 \mathfrak{x}_1 (-1 + \mathfrak{x}_2) + 11 \mathfrak{x}_2 - 5 \mathfrak{x}_2^2)) \left. \right) + \\
& \quad \eta t (-22 - 97 \mu_2 - 50 \mathfrak{x}_2 - 23 \mu_2 \mathfrak{x}_2 + 4 \mu_1^2 (83 + 13 \mathfrak{x}_2) + \\
& \quad \quad \mu_1 (70 + 143 \mu_2 - 118 \mathfrak{x}_2 + 97 \mu_2 \mathfrak{x}_2) + \\
& \quad \quad \theta_1 (\mu_1^2 (56 + \mathfrak{x}_1 (89 - 5 \mathfrak{x}_2) - 89 \mathfrak{x}_2 - 3 \mathfrak{x}_2^2) + \\
& \quad \quad \quad \mu_1 (26 + 38 \mathfrak{x}_1 - 56 \mathfrak{x}_2 - 44 \mathfrak{x}_1 \mathfrak{x}_2 + 36 \mathfrak{x}_2^2 - 3 \mu_2 (-2 + 5 \mathfrak{x}_1 \\
& \quad \quad \quad (-1 + \mathfrak{x}_2) + 3 \mathfrak{x}_2 - 9 \mathfrak{x}_2^2)) - 3 \times (2 + \mathfrak{x}_1 + \mathfrak{x}_2 + 5 \mathfrak{x}_1 \mathfrak{x}_2 - \\
& \quad \quad \quad 5 \mathfrak{x}_2^2 + \mu_2 (-2 + 5 \mathfrak{x}_1 (-1 + \mathfrak{x}_2) + 11 \mathfrak{x}_2 - 5 \mathfrak{x}_2^2))) \left. \right) - \\
& \eta^3 \left( 2 \times (6 + 38 \mu_2 + 30 \mathfrak{x}_2 + 58 \mu_2 \mathfrak{x}_2 + \mu_1^2 (-125 + 17 \mathfrak{x}_2) - \right. \\
& \quad \quad \mu_1 (83 + 154 \mu_2 - 65 \mathfrak{x}_2 + 38 \mu_2 \mathfrak{x}_2)) - \\
& \quad \quad \theta_1 (\mu_1^2 (44 + \mathfrak{x}_1 (-133 + \mathfrak{x}_2) + 133 \mathfrak{x}_2 + 3 \mathfrak{x}_2^2) + 6 \times
\end{aligned}$$



$$\begin{aligned}
& \left( 1 + \mathfrak{e}1 - 4 \mathfrak{e}2 + 5 \mathfrak{e}1 \mathfrak{e}2 - 5 \mathfrak{e}2^2 + \mu 2 \left( -9 + 5 \mathfrak{e}1 (-1 + \mathfrak{e}2) - 5 \mathfrak{e}2^2 \right) \right) + \\
& \mu 1 \left( 26 - 67 \mathfrak{e}1 + 37 \mathfrak{e}2 + 61 \mathfrak{e}1 \mathfrak{e}2 - 57 \mathfrak{e}2^2 + 6 \mu 2 \right. \\
& \quad \left. \left( 15 + 5 \mathfrak{e}1 (-1 + \mathfrak{e}2) + 16 \mathfrak{e}2 - 3 \mathfrak{e}2^2 \right) \right) + \eta t \left( 4 \times (7 + \mu 2 + \right. \\
& \quad \left. \mu 1^2 (-43 + \mathfrak{e}2) + 11 \mathfrak{e}2 - \mu 2 \mathfrak{e}2 + \mu 1 (-30 + \mu 2 + 15 \mathfrak{e}2 - \mu 2 \mathfrak{e}2) \right) + \\
& \theta l \left( \mu 1^2 (44 + \mathfrak{e}1 (-133 + \mathfrak{e}2) + 133 \mathfrak{e}2 + 3 \mathfrak{e}2^2) + 6 \times (1 + \mathfrak{e}1 - \right. \\
& \quad \left. 4 \mathfrak{e}2 + 5 \mathfrak{e}1 \mathfrak{e}2 - 5 \mathfrak{e}2^2 + \mu 2 (-9 + 5 \mathfrak{e}1 (-1 + \mathfrak{e}2) - 5 \mathfrak{e}2^2) \right) + \\
& \quad \mu 1 (26 - 67 \mathfrak{e}1 + 37 \mathfrak{e}2 + 61 \mathfrak{e}1 \mathfrak{e}2 - 57 \mathfrak{e}2^2 + 6 \mu 2 \\
& \quad \left. (15 + 5 \mathfrak{e}1 (-1 + \mathfrak{e}2) + 16 \mathfrak{e}2 - 3 \mathfrak{e}2^2) \right) \left. \right) + \\
& \eta^2 \left( 2 \times (-7 + 72 \mu 1^2 + \mu 1 (53 + \mu 2 (43 - 7 \mathfrak{e}2) - 29 \mathfrak{e}2) + \mu 2 \right. \\
& \quad \left. (7 - 25 \mathfrak{e}2) - 23 \mathfrak{e}2) + \theta l (2 + 3 \mathfrak{e}1 - 17 \mathfrak{e}2 + 15 \mathfrak{e}1 \mathfrak{e}2 - \right. \\
& \quad \left. 15 \mathfrak{e}2^2 + \mu 2 (-34 + 15 \mathfrak{e}1 (-1 + \mathfrak{e}2) - 11 \mathfrak{e}2 - 15 \mathfrak{e}2^2) + \right. \\
& \quad \left. \mu 1^2 (48 + 59 \mathfrak{e}2 + \mathfrak{e}2^2 - \mathfrak{e}1 (59 + \mathfrak{e}2)) + \mu 1 (26 - 32 \mathfrak{e}1 + 6 \mathfrak{e}2 + \right. \\
& \quad \left. 26 \mathfrak{e}1 \mathfrak{e}2 - 26 \mathfrak{e}2^2 + \mu 2 (62 + 15 \mathfrak{e}1 (-1 + \mathfrak{e}2) + 61 \mathfrak{e}2 - 3 \mathfrak{e}2^2) \right) \left. \right) + \\
& \eta t \left( 8 + 94 \mu 2 + 64 \mathfrak{e}2 + 38 \mu 2 \mathfrak{e}2 - 4 \mu 1^2 (85 + 11 \mathfrak{e}2) - 2 \mu 1 (46 - \right. \\
& \quad \left. 70 \mathfrak{e}2 + \mu 2 (85 + 47 \mathfrak{e}2)) + \theta l (-2 - 3 \mathfrak{e}1 + 17 \mathfrak{e}2 - 15 \mathfrak{e}1 \mathfrak{e}2 + 15 \right. \\
& \quad \left. \mathfrak{e}2^2 + \mu 2 (34 - 15 \mathfrak{e}1 (-1 + \mathfrak{e}2) + 11 \mathfrak{e}2 + 15 \mathfrak{e}2^2) + \mu 1^2 (-48 - 59 \right. \\
& \quad \left. \mathfrak{e}2 - \mathfrak{e}2^2 + \mathfrak{e}1 (59 + \mathfrak{e}2)) - \mu 1 (26 - 32 \mathfrak{e}1 + 6 \mathfrak{e}2 + 26 \mathfrak{e}1 \mathfrak{e}2 - \right. \\
& \quad \left. 26 \mathfrak{e}2^2 + \mu 2 (62 + 15 \mathfrak{e}1 (-1 + \mathfrak{e}2) + 61 \mathfrak{e}2 - 3 \mathfrak{e}2^2) \right) \left. \right) \left. \right) - \\
& w (-1 + \eta) \times (6 \eta^8 (1 + \mu 1) \times (-1 + \mathfrak{e}2) - 5 \eta t (1 + \mu 1) \mu 2 (-1 + \mathfrak{e}2) - \\
& 2 \eta^7 (7 - 18 \mu 2 + \mu 1^2 (21 - 9 \mathfrak{e}2) + 3 \eta t (1 + \mu 1) \times (-1 + \mathfrak{e}2) - 7 \mathfrak{e}2 + \\
& 2 \mu 1 (8 - 11 \mathfrak{e}2 + 9 \mu 2 (1 + \mathfrak{e}2)) - 2 \eta \eta t (-4 - 31 \mu 2 - 20 \mathfrak{e}2 - \\
& 5 \mu 2 \mathfrak{e}2 + 4 \mu 1^2 (14 + \mathfrak{e}2) + \mu 1 (40 - 22 \mathfrak{e}2 + \mu 2 (41 + 31 \mathfrak{e}2)) + \eta^5 \\
& (34 - 20 \mu 2 + 38 \mathfrak{e}2 + 80 \mu 2 \mathfrak{e}2 + 20 \mu 1 (-5 + \mu 2 (-7 + \mathfrak{e}2) + 2 \mathfrak{e}2) - \\
& 2 \mu 1^2 (79 + 5 \mathfrak{e}2) + \theta l (6 \times (2 + 3 \mu 2 + 2 \mathfrak{e}2 + 7 \mu 2 \mathfrak{e}2) + \\
& \mu 1^2 (-106 + 31 \mathfrak{e}2 + 3 \mathfrak{e}2^2 + \mathfrak{e}1 (-31 + 7 \mathfrak{e}2)) - \\
& \mu 1 (46 + 7 \mathfrak{e}1 - 43 \mathfrak{e}2 - 19 \mathfrak{e}1 \mathfrak{e}2 + 9 \mathfrak{e}2^2 + 6 \mu 2 (9 + 7 \mathfrak{e}2 + 4 \mathfrak{e}2^2)) \left. \right) + \\
& \eta t (2 - 64 \mu 2 - 2 \mathfrak{e}2 - 8 \mu 2 \mathfrak{e}2 + 12 \mu 1^2 (7 + \mathfrak{e}2) - 6 \theta l (2 + 3 \mu 2 + \\
& 2 \mathfrak{e}2 + 7 \mu 2 \mathfrak{e}2) + \theta l \mu 1^2 (106 + \mathfrak{e}1 (31 - 7 \mathfrak{e}2) - 31 \mathfrak{e}2 - 3 \mathfrak{e}2^2) + \\
& 2 \mu 1 (-5 - 19 \mathfrak{e}2 + 8 \mu 2 (5 + 4 \mathfrak{e}2)) + \theta l \mu 1 (46 + 7 \mathfrak{e}1 - \\
& 43 \mathfrak{e}2 - 19 \mathfrak{e}1 \mathfrak{e}2 + 9 \mathfrak{e}2^2 + 6 \mu 2 (9 + 7 \mathfrak{e}2 + 4 \mathfrak{e}2^2)) \left. \right) + \eta^6 \\
& (\mu 1^2 (-154 + 34 \mathfrak{e}2 + \theta l (-28 + \mathfrak{e}1 (-1 + \mathfrak{e}2) + 3 \mathfrak{e}2 + \mathfrak{e}2^2)) + \\
& 2 \times (5 + 7 \mathfrak{e}2 + \mu 2 (38 + 22 \mathfrak{e}2 + \theta l (5 + \mathfrak{e}2))) - \mu 1 (72 - 84 \mathfrak{e}2 + 4 \mu 2 \\
& (41 + 19 \mathfrak{e}2) + \theta l (4 + \mathfrak{e}1 - 15 \mathfrak{e}2 - \mathfrak{e}1 \mathfrak{e}2 - \mathfrak{e}2^2 + 2 \mu 2 (7 + 5 \mathfrak{e}2)) \left. \right) - \\
& \eta t (\mu 1^2 (4 - 4 \mathfrak{e}2 + \theta l (-28 + \mathfrak{e}1 (-1 + \mathfrak{e}2) + 3 \mathfrak{e}2 + \mathfrak{e}2^2)) + \\
& 2 \times (7 \times (-1 + \mathfrak{e}2) + \mu 2 (12 + \theta l (5 + \mathfrak{e}2))) - \\
& \mu 1 (2 \times (5 - 5 \mathfrak{e}2 + 12 \mu 2 (1 + \mathfrak{e}2)) + \\
& \theta l (4 + \mathfrak{e}1 - 15 \mathfrak{e}2 - \mathfrak{e}1 \mathfrak{e}2 - \mathfrak{e}2^2 + 2 \mu 2 (7 + 5 \mathfrak{e}2)) \left. \right) \left. \right) + \\
& \eta^4 (2 (\mu 1^2 (55 - 19 \mathfrak{e}2) - 4 \mu 2 (16 + 5 \mathfrak{e}2) + \mu 1 (19 - 37 \mathfrak{e}2 + \\
& 8 \mu 2 (13 + 8 \mathfrak{e}2)) + \theta l (20 + 3 \mathfrak{e}1 + \mathfrak{e}2 + 15 \mathfrak{e}1 \mathfrak{e}2 - 15 \mathfrak{e}2^2 + \\
& 3 \mu 2 (-14 + 5 \mathfrak{e}1 (-1 + \mathfrak{e}2) + 15 \mathfrak{e}2 - 5 \mathfrak{e}2^2) + \mu 1^2 (-58 + \\
& 101 \mathfrak{e}2 + 5 \mathfrak{e}2^2 + 3 \mathfrak{e}1 (-35 + 3 \mathfrak{e}2)) + \mu 1 (-38 + 42 \mathfrak{e}2 - 40 \mathfrak{e}2^2 + \\
& 6 \mathfrak{e}1 (-7 + 9 \mathfrak{e}2) + 3 \mu 2 (10 + 5 \mathfrak{e}1 (-1 + \mathfrak{e}2) + 11 \mathfrak{e}2 - 13 \mathfrak{e}2^2)) \left. \right) -
\end{aligned}$$

$$\begin{aligned}
& \eta t \left( 26 - 78 \mu_1 - 296 \mu_1^2 + 53 \mu_2 - 91 \mu_1 \mu_2 + 46 \mathfrak{z}_2 + 102 \mu_1 \mathfrak{z}_2 - \right. \\
& \quad 40 \mu_1^2 \mathfrak{z}_2 + 19 \mu_2 \mathfrak{z}_2 - 53 \mu_1 \mu_2 \mathfrak{z}_2 + \theta l \left( 20 + 3 \mathfrak{z}_1 + \mathfrak{z}_2 + 15 \mathfrak{z}_1 \mathfrak{z}_2 - \right. \\
& \quad \quad 15 \mathfrak{z}_2^2 + 3 \mu_2 \left( -14 + 5 \mathfrak{z}_1 \left( -1 + \mathfrak{z}_2 \right) + 15 \mathfrak{z}_2 - 5 \mathfrak{z}_2^2 \right) + \\
& \quad \quad \mu_1^2 \left( -58 + 101 \mathfrak{z}_2 + 5 \mathfrak{z}_2^2 + 3 \mathfrak{z}_1 \left( -35 + 3 \mathfrak{z}_2 \right) \right) + \\
& \quad \quad \mu_1 \left( -38 + 42 \mathfrak{z}_2 - 40 \mathfrak{z}_2^2 + 6 \mathfrak{z}_1 \left( -7 + 9 \mathfrak{z}_2 \right) + \right. \\
& \quad \quad \quad \left. 3 \mu_2 \left( 10 + 5 \mathfrak{z}_1 \left( -1 + \mathfrak{z}_2 \right) + 11 \mathfrak{z}_2 - 13 \mathfrak{z}_2^2 \right) \right) \left. \right) \left. \right) - \\
& \eta^3 \left( 4 \times \left( 5 + 2 \mu_1^2 \left( -25 + \mathfrak{z}_2 \right) + 13 \mathfrak{z}_2 + 6 \mu_2 \left( -1 + 3 \mathfrak{z}_2 \right) + 3 \mu_1 \right. \right. \\
& \quad \left. \left. \left( -11 + 2 \mu_2 \left( -5 + \mathfrak{z}_2 \right) + 7 \mathfrak{z}_2 \right) \right) - \right. \\
& \quad \theta l \left( 4 + 6 \mathfrak{z}_1 + 30 \mu_2 \mathfrak{z}_1 \left( -1 + \mathfrak{z}_2 \right) - 34 \mathfrak{z}_2 + 30 \mathfrak{z}_1 \mathfrak{z}_2 - 30 \mathfrak{z}_2^2 + \right. \\
& \quad \quad \mu_1^2 \left( 90 + \mathfrak{z}_1 \left( -121 + \mathfrak{z}_2 \right) + 121 \mathfrak{z}_2 + 5 \mathfrak{z}_2^2 \right) - \\
& \quad \quad 2 \mu_2 \left( 49 + 14 \mathfrak{z}_2 + 15 \mathfrak{z}_2^2 \right) + \mu_1 \left( 46 - 67 \mathfrak{z}_1 + 15 \mathfrak{z}_2 + 55 \mathfrak{z}_1 \mathfrak{z}_2 - \right. \\
& \quad \quad \quad \left. 49 \mathfrak{z}_2^2 + 2 \mu_2 \left( 83 + 15 \mathfrak{z}_1 \left( -1 + \mathfrak{z}_2 \right) + 76 \mathfrak{z}_2 - 3 \mathfrak{z}_2^2 \right) \right) \left. \right) \left. \right) + \\
& \eta t \left( 2 \times \left( 8 + \mu_1 \left( -62 + \mu_2 \left( -1 + \mathfrak{z}_2 \right) - 4 \mathfrak{z}_2 \right) + \mu_2 \left( -1 + \mathfrak{z}_2 \right) + 16 \mathfrak{z}_2 + \right. \right. \\
& \quad \quad 2 \mu_1^2 \left( 7 + 11 \mathfrak{z}_2 \right) \left. \right) + \theta l \left( 4 + 6 \mathfrak{z}_1 + 30 \mu_2 \mathfrak{z}_1 \left( -1 + \mathfrak{z}_2 \right) - 34 \mathfrak{z}_2 + \right. \\
& \quad \quad 30 \mathfrak{z}_1 \mathfrak{z}_2 - 30 \mathfrak{z}_2^2 + \mu_1^2 \left( 90 + \mathfrak{z}_1 \left( -121 + \mathfrak{z}_2 \right) + 121 \mathfrak{z}_2 + 5 \mathfrak{z}_2^2 \right) - \\
& \quad \quad 2 \mu_2 \left( 49 + 14 \mathfrak{z}_2 + 15 \mathfrak{z}_2^2 \right) + \mu_1 \left( 46 - 67 \mathfrak{z}_1 + 15 \mathfrak{z}_2 + 55 \mathfrak{z}_1 \mathfrak{z}_2 - \right. \\
& \quad \quad \quad \left. 49 \mathfrak{z}_2^2 + 2 \mu_2 \left( 83 + 15 \mathfrak{z}_1 \left( -1 + \mathfrak{z}_2 \right) + 76 \mathfrak{z}_2 - 3 \mathfrak{z}_2^2 \right) \right) \left. \right) \left. \right) + \\
& \eta^2 \left( 4 \times \left( 1 + \mu_1 \right) \times \left( -1 - 3 \mu_2 \left( -1 + \mathfrak{z}_2 \right) - 5 \mathfrak{z}_2 + \mu_1 \left( 11 + \mathfrak{z}_2 \right) \right) + \right. \\
& \quad \theta l \left( \left( -4 + 3 \mathfrak{z}_1 - 3 \mathfrak{z}_2 \right) \times \left( 1 + 5 \mathfrak{z}_2 \right) + \right. \\
& \quad \quad 3 \mu_2 \left( -16 + 5 \mathfrak{z}_1 \left( -1 + \mathfrak{z}_2 \right) - 11 \mathfrak{z}_2 - 5 \mathfrak{z}_2^2 \right) + \\
& \quad \quad 2 \mu_1^2 \left( 35 + 24 \mathfrak{z}_2 + \mathfrak{z}_2^2 - \mathfrak{z}_1 \left( 23 + \mathfrak{z}_2 \right) \right) + \mu_1 \left( 42 - 31 \mathfrak{z}_1 + \mathfrak{z}_2 + \right. \\
& \quad \quad \quad \left. 19 \mathfrak{z}_1 \mathfrak{z}_2 - 19 \mathfrak{z}_2^2 + 3 \mu_2 \left( 32 + 5 \mathfrak{z}_1 \left( -1 + \mathfrak{z}_2 \right) + 29 \mathfrak{z}_2 + 3 \mathfrak{z}_2^2 \right) \right) \left. \right) \left. \right) + \\
& \eta t \left( -4 \left( \mu_1^2 \left( 59 + \mathfrak{z}_2 \right) - 3 \times \left( 1 + 5 \mathfrak{z}_2 + 2 \mu_2 \left( 3 + \mathfrak{z}_2 \right) \right) + 2 \mu_1 \left( 16 - 13 \mathfrak{z}_2 + \right. \right. \right. \\
& \quad \quad \quad \left. \left. 3 \mu_2 \left( 5 + 3 \mathfrak{z}_2 \right) \right) \right) + \theta l \left( - \left( \left( -4 + 3 \mathfrak{z}_1 - 3 \mathfrak{z}_2 \right) \times \left( 1 + 5 \mathfrak{z}_2 \right) \right) + \right. \\
& \quad \quad 3 \mu_2 \left( 16 + 5 \mathfrak{z}_1 + 11 \mathfrak{z}_2 - 5 \mathfrak{z}_1 \mathfrak{z}_2 + 5 \mathfrak{z}_2^2 \right) - 2 \mu_1^2 \left( 35 + \right. \\
& \quad \quad \quad \left. 24 \mathfrak{z}_2 + \mathfrak{z}_2^2 - \mathfrak{z}_1 \left( 23 + \mathfrak{z}_2 \right) \right) - \mu_1 \left( 42 - 31 \mathfrak{z}_1 + \mathfrak{z}_2 + 19 \mathfrak{z}_1 \mathfrak{z}_2 - \right. \\
& \quad \quad \quad \left. 19 \mathfrak{z}_2^2 + 3 \mu_2 \left( 32 + 5 \mathfrak{z}_1 \left( -1 + \mathfrak{z}_2 \right) + 29 \mathfrak{z}_2 + 3 \mathfrak{z}_2^2 \right) \right) \left. \right) \left. \right) \left. \right) + \\
& \eta \left( 4 \eta^7 \left( 1 + \mu_1 \right) \times \left( -1 + \mathfrak{z}_2 \right) - 2 \eta^6 \left( -12 \mu_2 + \mu_1^2 \left( 17 - 5 \mathfrak{z}_2 \right) + 2 \eta t \right. \right. \\
& \quad \left. \left. \left( 1 + \mu_1 \right) \times \left( -1 + \mathfrak{z}_2 \right) + \mu_1 \left( 5 - 11 \mathfrak{z}_2 + 12 \mu_2 \left( 1 + \mathfrak{z}_2 \right) \right) \right) + \eta t \left( 2 + 10 \mathfrak{z}_2 - \right. \right. \\
& \quad \quad 2 \mu_1^2 \left( 11 + \mathfrak{z}_2 \right) + \mu_2 \left( 19 + 5 \mathfrak{z}_2 \right) - \mu_1 \left( 20 - 8 \mathfrak{z}_2 + \mu_2 \left( 29 + 19 \mathfrak{z}_2 \right) \right) \left. \right) + \eta^5 \\
& \left( 4 \eta t \left( 1 - 3 \mu_2 + \mu_1^2 \left( -1 + \mathfrak{z}_2 \right) - \mathfrak{z}_2 + 3 \mu_1 \mu_2 \left( 1 + \mathfrak{z}_2 \right) \right) + 2 \times \left( 5 + 4 \mu_1^2 \right. \right. \\
& \quad \quad \left. \left. \left( -7 + \mathfrak{z}_2 \right) + \mathfrak{z}_2 + \mu_2 \left( 7 + 11 \mathfrak{z}_2 \right) - \mu_1 \left( 11 + 29 \mu_2 - 11 \mathfrak{z}_2 + 7 \mu_2 \mathfrak{z}_2 \right) \right) \right) + \\
& \quad \theta l \left( 4 - 4 \mathfrak{z}_2 + 2 \mu_2 \left( 5 + \mathfrak{z}_2 \right) + \mu_1^2 \left( -28 + \mathfrak{z}_1 \left( -1 + \mathfrak{z}_2 \right) + 3 \mathfrak{z}_2 + \mathfrak{z}_2^2 \right) + \right. \\
& \quad \quad \mu_1 \left( \mathfrak{z}_1 \left( -1 + \mathfrak{z}_2 \right) + \mathfrak{z}_2 \left( 11 + \mathfrak{z}_2 \right) - 2 \mu_2 \left( 7 + 5 \mathfrak{z}_2 \right) \right) \left. \right) - \eta t \theta l \\
& \left( 4 - 4 \mathfrak{z}_2 + 2 \mu_2 \left( 5 + \mathfrak{z}_2 \right) + \mu_1^2 \left( -28 + \mathfrak{z}_1 \left( -1 + \mathfrak{z}_2 \right) + 3 \mathfrak{z}_2 + \mathfrak{z}_2^2 \right) + \right. \\
& \quad \quad \mu_1 \left( \mathfrak{z}_1 \left( -1 + \mathfrak{z}_2 \right) + \mathfrak{z}_2 \left( 11 + \mathfrak{z}_2 \right) - 2 \mu_2 \left( 7 + 5 \mathfrak{z}_2 \right) \right) \left. \right) - \eta^3 \\
& \left( 6 - 26 \mu_1 - 56 \mu_1^2 + 30 \mu_2 - 90 \mu_1 \mu_2 + 6 \mathfrak{z}_2 + 26 \mu_1 \mathfrak{z}_2 + 8 \mu_1^2 \mathfrak{z}_2 + \right. \\
& \quad 30 \mu_2 \mathfrak{z}_2 - 30 \mu_1 \mu_2 \mathfrak{z}_2 - \theta l \left( 6 + \mathfrak{z}_1 + 5 \mathfrak{z}_2 + 5 \mathfrak{z}_1 \mathfrak{z}_2 - \right. \\
& \quad \quad 5 \mathfrak{z}_2^2 + \mu_2 \left( -36 + 5 \mathfrak{z}_1 \left( -1 + \mathfrak{z}_2 \right) + 17 \mathfrak{z}_2 - 5 \mathfrak{z}_2^2 \right) + \\
& \quad \quad 2 \mu_1^2 \left( -1 + 2 \mathfrak{z}_1 \left( -10 + \mathfrak{z}_2 \right) + 18 \mathfrak{z}_2 + \mathfrak{z}_2^2 \right) + \\
& \quad \quad \mu_1 \left( 3 \mathfrak{z}_1 \left( -5 + 7 \mathfrak{z}_2 \right) + \mu_2 \left( 36 + 5 \mathfrak{z}_1 \left( -1 + \mathfrak{z}_2 \right) + 29 \mathfrak{z}_2 - 17 \mathfrak{z}_2^2 \right) + \right. \\
& \quad \quad \quad \left. 5 \times \left( -4 + \mathfrak{z}_2 - 3 \mathfrak{z}_2^2 \right) \right) \left. \right) + \eta t \left( 8 + 7 \mu_2 + 16 \mathfrak{z}_2 + 5 \mu_2 \mathfrak{z}_2 - \right.
\end{aligned}$$

$$\begin{aligned}
& 8 \mu_1^2 (11 + \mathfrak{z}2) - \mu_1 (32 + 17 \mu_2 - 32 \mathfrak{z}2 + 7 \mu_2 \mathfrak{z}2) + \\
& \mathfrak{e}l (6 + \mathfrak{z}1 + 5 \mathfrak{z}2 + 5 \mathfrak{z}1 \mathfrak{z}2 - 5 \mathfrak{z}2^2 + \mu_2 (-36 + 5 \mathfrak{z}1 (-1 + \mathfrak{z}2) + 17 \mathfrak{z}2 - \\
& \quad 5 \mathfrak{z}2^2) + 2 \mu_1^2 (-1 + 2 \mathfrak{z}1 (-10 + \mathfrak{z}2) + 18 \mathfrak{z}2 + \mathfrak{z}2^2) + \mu_1 \\
& \quad (3 \mathfrak{z}1 (-5 + 7 \mathfrak{z}2) + \mu_2 (36 + 5 \mathfrak{z}1 (-1 + \mathfrak{z}2) + 29 \mathfrak{z}2 - 17 \mathfrak{z}2^2) + \\
& \quad 5 \times (-4 + \mathfrak{z}2 - 3 \mathfrak{z}2^2))) + \eta^2 (-2 \times (2 + 4 \mu_2 (-4 + \mathfrak{z}2) + \\
& 10 \mathfrak{z}2 - 2 \mu_1^2 (11 + \mathfrak{z}2) + 4 \mu_1 (-5 + 2 \mathfrak{z}2 + \mu_2 (2 + 4 \mathfrak{z}2)) + \\
& \mathfrak{e}l (-((-1 + \mathfrak{z}1 - \mathfrak{z}2) \times (1 + 5 \mathfrak{z}2)) + \mu_1^2 (-23 + 18 \mathfrak{z}1 - 18 \mathfrak{z}2 - \mathfrak{z}2^2) + \\
& \quad \mu_2 (22 + 5 \mathfrak{z}1 + 9 \mathfrak{z}2 - 5 \mathfrak{z}1 \mathfrak{z}2 + 5 \mathfrak{z}2^2) - \mu_1 (10 - 11 \mathfrak{z}1 + \\
& \quad 8 \mathfrak{z}1 \mathfrak{z}2 - 7 \mathfrak{z}2^2 + \mu_2 (38 + 5 \mathfrak{z}1 (-1 + \mathfrak{z}2) + 33 \mathfrak{z}2 + \mathfrak{z}2^2)))) + \\
& \eta t (-2 + \mu_2 - 10 \mathfrak{z}2 - \mu_2 \mathfrak{z}2 - 18 \mu_1^2 (3 + \mathfrak{z}2) + \mu_1 (\mu_2 - \mu_2 \mathfrak{z}2 + \\
& \quad 20 \times (2 + \mathfrak{z}2)) + 2 \mathfrak{e}l (-((-1 + \mathfrak{z}1 - \mathfrak{z}2) \times (1 + 5 \mathfrak{z}2)) + \\
& \quad \mu_1^2 (-23 + 18 \mathfrak{z}1 - 18 \mathfrak{z}2 - \mathfrak{z}2^2) + \\
& \quad \mu_2 (22 + 5 \mathfrak{z}1 + 9 \mathfrak{z}2 - 5 \mathfrak{z}1 \mathfrak{z}2 + 5 \mathfrak{z}2^2) - \mu_1 (10 - 11 \mathfrak{z}1 + 8 \mathfrak{z}1 \mathfrak{z}2 - \\
& \quad 7 \mathfrak{z}2^2 + \mu_2 (38 + 5 \mathfrak{z}1 (-1 + \mathfrak{z}2) + 33 \mathfrak{z}2 + \mathfrak{z}2^2)))) - 2 \\
& \eta^4 (-2 + 15 \mu_1 + 5 \mu_1^2 + 20 \mu_2 - 4 \mu_1 \mu_2 - 10 \mathfrak{z}2 + 3 \mu_1 \mathfrak{z}2 + \\
& \quad 7 \mu_1^2 \mathfrak{z}2 - 8 \mu_2 \mathfrak{z}2 - 20 \mu_1 \mu_2 \mathfrak{z}2 - \\
& \mathfrak{e}l (5 + \mathfrak{z}2 + 2 \mu_2 (1 + 5 \mathfrak{z}2) + \mu_1^2 (-27 + 2 \mathfrak{z}1 (-4 + \mathfrak{z}2) + 8 \mathfrak{z}2 + \mathfrak{z}2^2) - \\
& \quad \mu_1 (10 + 2 \mathfrak{z}1 - 9 \mathfrak{z}2 - 5 \mathfrak{z}1 \mathfrak{z}2 + 2 \mathfrak{z}2^2 + 2 \mu_2 (5 + 4 \mathfrak{z}2 + 3 \mathfrak{z}2^2))) + \\
& \eta t (-2 \times (-1 + \mathfrak{z}2 - \mu_2 (5 + \mathfrak{z}2) + \mu_1^2 (11 + \mathfrak{z}2) + \\
& \quad \mu_1 (-2 - 4 \mathfrak{z}2 + \mu_2 (7 + 5 \mathfrak{z}2))) + \mathfrak{e}l (5 + \mathfrak{z}2 + \\
& \quad 2 \mu_2 (1 + 5 \mathfrak{z}2) + \mu_1^2 (-27 + 2 \mathfrak{z}1 (-4 + \mathfrak{z}2) + 8 \mathfrak{z}2 + \mathfrak{z}2^2) - \mu_1 \\
& \quad (10 + 2 \mathfrak{z}1 - 9 \mathfrak{z}2 - 5 \mathfrak{z}1 \mathfrak{z}2 + 2 \mathfrak{z}2^2 + 2 \mu_2 (5 + 4 \mathfrak{z}2 + 3 \mathfrak{z}2^2)))) + \\
& \eta (\mathfrak{e}l (-\mu_1^2 (-2 + \mathfrak{z}1 - \mathfrak{z}2) \times (11 + \mathfrak{z}2) + (-2 + \mathfrak{z}1 - \mathfrak{z}2) \times (1 + 5 \mathfrak{z}2) + \\
& \quad \mu_2 (-14 + 5 \mathfrak{z}1 (-1 + \mathfrak{z}2) - 17 \mathfrak{z}2 - 5 \mathfrak{z}2^2) + \mu_1 (2 \times (-2 + \mathfrak{z}1 - \mathfrak{z}2) \times \\
& \quad (-5 + 2 \mathfrak{z}2) + \mu_2 (34 + 5 \mathfrak{z}1 (-1 + \mathfrak{z}2) + 31 \mathfrak{z}2 + 7 \mathfrak{z}2^2))) + \\
& \eta t (4 - 48 \mu_1 - 52 \mu_1^2 + 19 \mu_2 - 29 \mu_1 \mu_2 + 20 \mathfrak{z}2 + 24 \mu_1 \mathfrak{z}2 + \\
& \quad 4 \mu_1^2 \mathfrak{z}2 + 5 \mu_2 \mathfrak{z}2 - 19 \mu_1 \mu_2 \mathfrak{z}2 + \mathfrak{e}l (\mu_1^2 (-2 + \mathfrak{z}1 - \mathfrak{z}2) \times (11 + \mathfrak{z}2) - \\
& \quad (-2 + \mathfrak{z}1 - \mathfrak{z}2) \times (1 + 5 \mathfrak{z}2) + \mu_2 (14 + 5 \mathfrak{z}1 + 17 \mathfrak{z}2 - \\
& \quad 5 \mathfrak{z}1 \mathfrak{z}2 + 5 \mathfrak{z}2^2) - \mu_1 (2 \times (-2 + \mathfrak{z}1 - \mathfrak{z}2) \times (-5 + 2 \mathfrak{z}2) + \\
& \quad \mu_2 (34 + 5 \mathfrak{z}1 (-1 + \mathfrak{z}2) + 31 \mathfrak{z}2 + 7 \mathfrak{z}2^2)))) - \\
& x^3 (-1 + \eta)^3 ((-1 + \eta) \mathfrak{e}p (4 + 40 \eta + 84 \eta^2 - 80 \eta^4 - 4 \eta t + 16 \eta \eta t + 80 \\
& \quad \eta^2 \eta t + 80 \eta^3 \eta t - 40 \mu_1 - 264 \eta \mu_1 - 336 \eta^2 \mu_1 - 200 \eta^3 \mu_1 - 80 \\
& \quad \eta^4 \mu_1 - 16 \eta \eta t \mu_1 + 64 \eta^2 \eta t \mu_1 + 80 \eta^3 \eta t \mu_1 - 44 \mu_1^2 - 400 \eta \\
& \quad \mu_1^2 - 900 \eta^2 \mu_1^2 - 680 \eta^3 \mu_1^2 + 148 \eta t \mu_1^2 + 160 \eta \eta t \mu_1^2 - 16 \\
& \quad \eta^2 \eta t \mu_1^2 - 12 \mu_2 - 8 \eta \mu_2 + 116 \eta^2 \mu_2 + 240 \eta^3 \mu_2 - 39 \eta t \\
& \quad \mu_2 - 128 \eta \eta t \mu_2 - 120 \eta^2 \eta t \mu_2 - 12 \mu_1 \mu_2 - 296 \eta \mu_1 \mu_2 - 508 \\
& \quad \eta^2 \mu_1 \mu_2 - 240 \eta^3 \mu_1 \mu_2 + 57 \eta t \mu_1 \mu_2 + 160 \eta \eta t \mu_1 \mu_2 + 120 \\
& \quad \eta^2 \eta t \mu_1 \mu_2 + 20 \mathfrak{z}2 + 104 \eta \mathfrak{z}2 + 36 \eta^2 \mathfrak{z}2 + 80 \eta^4 \mathfrak{z}2 - 20 \eta t \\
& \quad \mathfrak{z}2 - 16 \eta \eta t \mathfrak{z}2 - 80 \eta^2 \eta t \mathfrak{z}2 - 80 \eta^3 \eta t \mathfrak{z}2 + 16 \mu_1 \mathfrak{z}2 + 168 \eta \\
& \quad \mu_1 \mathfrak{z}2 + 456 \eta^2 \mu_1 \mathfrak{z}2 + 440 \eta^3 \mu_1 \mathfrak{z}2 + 80 \eta^4 \mu_1 \mathfrak{z}2 - 48 \eta t \mu_1 \\
& \quad \mathfrak{z}2 - 80 \eta \eta t \mu_1 \mathfrak{z}2 - 64 \eta^2 \eta t \mu_1 \mathfrak{z}2 - 80 \eta^3 \eta t \mu_1 \mathfrak{z}2 - 4 \mu_1^2 \\
& \quad \mathfrak{z}2 + 16 \eta \mu_1^2 \mathfrak{z}2 + 180 \eta^2 \mu_1^2 \mathfrak{z}2 + 200 \eta^3 \mu_1^2 \mathfrak{z}2 + 44 \eta t \mu_1^2 \\
& \quad \mathfrak{z}2 + 32 \eta \eta t \mu_1^2 \mathfrak{z}2 + 16 \eta^2 \eta t \mu_1^2 \mathfrak{z}2 + 12 \mu_2 \mathfrak{z}2 + 152 \eta \mu_2 \\
& \quad \mathfrak{z}2 + 196 \eta^2 \mu_2 \mathfrak{z}2 - 9 \eta t \mu_2 \mathfrak{z}2 - 16 \eta \eta t \mu_2 \mathfrak{z}2 + 12 \mu_1 \mu_2 \mathfrak{z}2 + 8
\end{aligned}$$

$$\begin{aligned}
& \eta \mu_1 \mu_2 \mathfrak{z}^2 - 116 \eta^2 \mu_1 \mu_2 \mathfrak{z}^2 - 240 \eta^3 \mu_1 \mu_2 \mathfrak{z}^2 + 39 \eta \mathfrak{t} \mu_1 \mu_2 \\
& \mathfrak{z}^2 + 128 \eta \eta \mathfrak{t} \mu_1 \mu_2 \mathfrak{z}^2 + 120 \eta^2 \eta \mathfrak{t} \mu_1 \mu_2 \mathfrak{z}^2 + 2 w^4 (-1 + \eta)^4 \\
& (1 - 18 \mu_1 - 19 \mu_1^2 + 7 \mu_2 - 29 \mu_1 \mu_2 + 4 \eta^2 (1 + \mu_1) \times (-1 + \mathfrak{z}^2) + \\
& 5 \mathfrak{z}^2 + 12 \mu_1 \mathfrak{z}^2 + 7 \mu_1^2 \mathfrak{z}^2 + 11 \mu_2 \mathfrak{z}^2 - 7 \mu_1 \mu_2 \mathfrak{z}^2 + \\
& 2 \eta \mathfrak{t} (1 + \mu_1 - 3 \mu_2 - \mathfrak{z}^2 - \mu_1 \mathfrak{z}^2 + 3 \mu_1 \mu_2 (1 + \mathfrak{z}^2)) - \\
& 2 \eta (1 - 3 \mu_2 - 8 \mu_1^2 (-1 + \mathfrak{z}^2) + 2 \eta \mathfrak{t} (1 + \mu_1) \times (-1 + \mathfrak{z}^2) - \\
& \mathfrak{z}^2 + 3 \mu_1 (3 + \mu_2 - 3 \mathfrak{z}^2 + \mu_2 \mathfrak{z}^2)) - w^3 (-1 + \eta)^3 \\
& (12 + 56 \mu_2 + 40 \eta^3 (1 + \mu_1) \times (-1 + \mathfrak{z}^2) + 60 \mathfrak{z}^2 + 112 \mu_2 \mathfrak{z}^2 + \\
& 8 \mu_1^2 (-29 + 5 \mathfrak{z}^2) + 4 \eta \mathfrak{t} \mu_1^2 (37 + 11 \mathfrak{z}^2) - \\
& 4 \mu_1 (43 - 31 \mathfrak{z}^2 + 14 \mu_2 (5 + \mathfrak{z}^2)) - 3 \eta \mathfrak{t} (-4 + 12 \mathfrak{z}^2 + \mu_2 (29 + 3 \mathfrak{z}^2)) + \\
& \eta \mathfrak{t} \mu_1 (16 - 64 \mathfrak{z}^2 + 3 \mu_2 (35 + 29 \mathfrak{z}^2)) - \\
& 8 \eta^2 (7 - 12 \mu_2 - 20 \mu_1^2 (-1 + \mathfrak{z}^2) + 5 \eta \mathfrak{t} (1 + \mu_1) \times (-1 + \mathfrak{z}^2) - 7 \mathfrak{z}^2 + \\
& 3 \mu_1 (9 - 9 \mathfrak{z}^2 + 4 \mu_2 (1 + \mathfrak{z}^2)) + 4 \eta (43 \mu_2 + 24 \mathfrak{z}^2 + 44 \mu_2 \mathfrak{z}^2 + \\
& 2 \mu_1^2 (-59 + 23 \mathfrak{z}^2) - \mu_1 (94 + 131 \mu_2 - 82 \mathfrak{z}^2 + 43 \mu_2 \mathfrak{z}^2) + \\
& 2 \eta \mathfrak{t} (7 - 12 \mu_2 - 7 \mathfrak{z}^2 + \mu_1 (7 - 7 \mathfrak{z}^2 + 12 \mu_2 (1 + \mathfrak{z}^2))) - w \\
& (-1 + \eta) \times (120 \eta^4 (1 + \mu_1) \times (-1 + \mathfrak{z}^2) + 4 \times (6 + \mu_1^2 (-61 + \mathfrak{z}^2) + \\
& 18 \mathfrak{z}^2 + \mu_2 (-4 + 22 \mathfrak{z}^2) + \mu_1 (-43 + 4 \mu_2 (-10 + \mathfrak{z}^2) + 25 \mathfrak{z}^2)) - \\
& 40 \eta^3 (5 - 9 \mu_2 + \mu_1^2 (21 - 9 \mathfrak{z}^2) + 3 \eta \mathfrak{t} (1 + \mu_1) \times (-1 + \mathfrak{z}^2) - \\
& 5 \mathfrak{z}^2 + \mu_1 (14 - 20 \mathfrak{z}^2 + 9 \mu_2 (1 + \mathfrak{z}^2))) + \\
& 8 \eta^2 (4 + 62 \mu_2 + 26 \mathfrak{z}^2 + 52 \mu_2 \mathfrak{z}^2 + 5 \mu_1^2 (-49 + 13 \mathfrak{z}^2) - \\
& \mu_1 (121 + 166 \mu_2 - 151 \mathfrak{z}^2 + 62 \mu_2 \mathfrak{z}^2) + \eta \mathfrak{t} (-23 \mu_1 (-1 + \mathfrak{z}^2) + \\
& 2 \mu_1^2 (-1 + \mathfrak{z}^2) + 30 \mu_1 \mu_2 (1 + \mathfrak{z}^2) - 5 \times (-5 + 6 \mu_2 + 5 \mathfrak{z}^2))) + \\
& \eta \mathfrak{t} (-4 - 68 \mathfrak{z}^2 - 3 \mu_2 (47 + 9 \mathfrak{z}^2) + 12 \mu_1^2 (37 + 11 \mathfrak{z}^2) + \\
& \mu_1 (8 - 152 \mathfrak{z}^2 + 3 \mu_2 (65 + 47 \mathfrak{z}^2))) + 8 \eta (15 + 28 \mu_2 + 33 \mathfrak{z}^2 + \\
& 62 \mu_2 \mathfrak{z}^2 + 3 \mu_1^2 (-59 + 7 \mathfrak{z}^2) - 2 \mu_1 (51 - 42 \mathfrak{z}^2 + 2 \mu_2 (38 + 7 \mathfrak{z}^2)) + \\
& \eta \mathfrak{t} (-11 \times (-1 + \mathfrak{z}^2) + 8 \mu_1^2 (5 + \mathfrak{z}^2) - 4 \mu_2 (11 + \mathfrak{z}^2) + \\
& \mu_1 (3 - 27 \mathfrak{z}^2 + \mu_2 (52 + 44 \mathfrak{z}^2))) - w^2 (-1 + \eta)^2 \\
& (40 \eta^4 (1 + \mu_1) \times (-1 + \mathfrak{z}^2) - 40 \eta^3 (4 - 3 \mu_2 - 4 \mu_1^2 (-1 + \mathfrak{z}^2) + \\
& \eta \mathfrak{t} (1 + \mu_1) \times (-1 + \mathfrak{z}^2) - 4 \mathfrak{z}^2 + \mu_1 (8 - 8 \mathfrak{z}^2 + 3 \mu_2 (1 + \mathfrak{z}^2))) + \\
& 2 \times (15 + 51 \mathfrak{z}^2 + \mu_1^2 (-197 + 17 \mathfrak{z}^2) + \mu_2 (19 + 83 \mathfrak{z}^2) - \\
& \mu_1 (134 - 92 \mathfrak{z}^2 + \mu_2 (185 + 19 \mathfrak{z}^2))) + \\
& \eta \mathfrak{t} (8 - 80 \mathfrak{z}^2 - 3 \mu_2 (59 + 9 \mathfrak{z}^2) + 12 \mu_1^2 (37 + 11 \mathfrak{z}^2) + \\
& \mu_1 (20 - 164 \mathfrak{z}^2 + 3 \mu_2 (77 + 59 \mathfrak{z}^2))) + \\
& 4 \eta^2 (-25 + 119 \mu_2 + 55 \mathfrak{z}^2 + 55 \mu_2 \mathfrak{z}^2 + 5 \mu_1^2 (-61 + 25 \mathfrak{z}^2) - \\
& \mu_1 (210 + 229 \mu_2 - 240 \mathfrak{z}^2 + 119 \mu_2 \mathfrak{z}^2) + \\
& 10 \eta \mathfrak{t} (4 - 3 \mu_2 - 4 \mathfrak{z}^2 + \mu_1 (4 - 4 \mathfrak{z}^2 + 3 \mu_2 (1 + \mathfrak{z}^2))) + \\
& 4 \eta (13 + 98 \mu_2 + 71 \mathfrak{z}^2 + 130 \mu_2 \mathfrak{z}^2 + 4 \mu_1^2 (-91 + 19 \mathfrak{z}^2) - \\
& \mu_1 (231 - 207 \mathfrak{z}^2 + \mu_2 (358 + 98 \mathfrak{z}^2)) + \\
& \eta \mathfrak{t} (-30 \times (-1 + \mathfrak{z}^2) + 8 \mu_1^2 (5 + \mathfrak{z}^2) - 4 \mu_2 (20 + \mathfrak{z}^2) + \\
& \mu_1 (22 - 46 \mathfrak{z}^2 + \mu_2 (88 + 80 \mathfrak{z}^2)))) + \\
& (-1 + \eta \mathfrak{t}) \mathfrak{e} \mathfrak{l} (-6 - 12 \eta + 2 \mathfrak{e} \mathfrak{p} - 24 \eta \mathfrak{e} \mathfrak{p} - 100 \eta^2 \mathfrak{e} \mathfrak{p} - 80 \eta^3 \mathfrak{e} \mathfrak{p} + 56 \\
& \mu_1 + 76 \eta \mu_1 - 24 \eta^2 \mu_1 - 24 \eta^3 \mu_1 - 18 \mathfrak{e} \mathfrak{p} \mu_1 + 86 \eta \mathfrak{e} \mathfrak{p} \mu_1 + 188 \\
& \eta^2 \mathfrak{e} \mathfrak{p} \mu_1 - 20 \eta^3 \mathfrak{e} \mathfrak{p} \mu_1 + 86 \mu_1^2 + 400 \eta \mu_1^2 + 264 \eta^2 \mu_1^2 - 24 \\
& \eta^3 \mu_1^2 - 44 \mathfrak{e} \mathfrak{p} \mu_1^2 + 14 \eta \mathfrak{e} \mathfrak{p} \mu_1^2 + 528 \eta^2 \mathfrak{e} \mathfrak{p} \mu_1^2 + 540 \eta^3
\end{aligned}$$

$$\begin{aligned}
& \partial_p \mu_1^2 - 38 \mu_2 - 57 \eta \mu_2 + 34 \partial_p \mu_2 + 114 \eta \partial_p \mu_2 + 20 \eta^2 \partial_p \\
& \mu_2 - 100 \eta^3 \partial_p \mu_2 + 58 \mu_1 \mu_2 + 87 \eta \mu_1 \mu_2 - 62 \partial_p \mu_1 \mu_2 - 102 \\
& \eta \partial_p \mu_1 \mu_2 + 116 \eta^2 \partial_p \mu_1 \mu_2 + 140 \eta^3 \partial_p \mu_1 \mu_2 - 2 \partial_p \mathfrak{x}_1 - 4 \\
& \eta \partial_p \mathfrak{x}_1 + 23 \partial_p \mu_1 \mathfrak{x}_1 + 63 \eta \partial_p \mu_1 \mathfrak{x}_1 + 34 \eta^2 \partial_p \mu_1 \mathfrak{x}_1 + 10 \\
& \eta^3 \partial_p \mu_1 \mathfrak{x}_1 + 37 \partial_p \mu_1^2 \mathfrak{x}_1 + 163 \eta \partial_p \mu_1^2 \mathfrak{x}_1 + 154 \eta^2 \partial_p \\
& \mu_1^2 \mathfrak{x}_1 + 10 \eta^3 \partial_p \mu_1^2 \mathfrak{x}_1 + 10 \partial_p \mu_2 \mathfrak{x}_1 + 20 \eta \partial_p \mu_2 \mathfrak{x}_1 + 10 \\
& \partial_p \mu_1 \mu_2 \mathfrak{x}_1 + 20 \eta \partial_p \mu_1 \mu_2 \mathfrak{x}_1 - 30 \mathfrak{x}_2 - 60 \eta \mathfrak{x}_2 + 12 \partial_p \\
& \mathfrak{x}_2 - 20 \eta \partial_p \mathfrak{x}_2 - 20 \eta^2 \partial_p \mathfrak{x}_2 + 80 \eta^3 \partial_p \mathfrak{x}_2 - 32 \mu_1 \mathfrak{x}_2 - 160 \\
& \eta \mu_1 \mathfrak{x}_2 - 120 \eta^2 \mu_1 \mathfrak{x}_2 + 24 \eta^3 \mu_1 \mathfrak{x}_2 - \partial_p \mu_1 \mathfrak{x}_2 - 23 \eta \partial_p \\
& \mu_1 \mathfrak{x}_2 - 174 \eta^2 \partial_p \mu_1 \mathfrak{x}_2 - 210 \eta^3 \partial_p \mu_1 \mathfrak{x}_2 + 10 \mu_1^2 \mathfrak{x}_2 + 56 \\
& \eta \mu_1^2 \mathfrak{x}_2 + 24 \eta^2 \mu_1^2 \mathfrak{x}_2 + 24 \eta^3 \mu_1^2 \mathfrak{x}_2 - 37 \partial_p \mu_1^2 \mathfrak{x}_2 - 147 \\
& \eta \partial_p \mu_1^2 \mathfrak{x}_2 - 154 \eta^2 \partial_p \mu_1^2 \mathfrak{x}_2 - 50 \eta^3 \partial_p \mu_1^2 \mathfrak{x}_2 - 10 \mu_2 \\
& \mathfrak{x}_2 - 15 \eta \mu_2 \mathfrak{x}_2 + 16 \partial_p \mu_2 \mathfrak{x}_2 - 74 \eta \partial_p \mu_2 \mathfrak{x}_2 - 188 \eta^2 \partial_p \mu_2 \\
& \mathfrak{x}_2 - 20 \eta^3 \partial_p \mu_2 \mathfrak{x}_2 + 38 \mu_1 \mu_2 \mathfrak{x}_2 + 57 \eta \mu_1 \mu_2 \mathfrak{x}_2 - 56 \partial_p \mu_1 \\
& \mu_2 \mathfrak{x}_2 - 86 \eta \partial_p \mu_1 \mu_2 \mathfrak{x}_2 + 100 \eta^2 \partial_p \mu_1 \mu_2 \mathfrak{x}_2 + 100 \eta^3 \partial_p \\
& \mu_1 \mu_2 \mathfrak{x}_2 - 10 \partial_p \mathfrak{x}_1 \mathfrak{x}_2 - 20 \eta \partial_p \mathfrak{x}_1 \mathfrak{x}_2 - 17 \partial_p \mu_1 \mathfrak{x}_1 \mathfrak{x}_2 - 87 \\
& \eta \partial_p \mu_1 \mathfrak{x}_1 \mathfrak{x}_2 - 94 \eta^2 \partial_p \mu_1 \mathfrak{x}_1 \mathfrak{x}_2 - 10 \eta^3 \partial_p \mu_1 \mathfrak{x}_1 \mathfrak{x}_2 - \partial_p \\
& \mu_1^2 \mathfrak{x}_1 \mathfrak{x}_2 - 19 \eta \partial_p \mu_1^2 \mathfrak{x}_1 \mathfrak{x}_2 - 34 \eta^2 \partial_p \mu_1^2 \mathfrak{x}_1 \mathfrak{x}_2 - 10 \eta^3 \\
& \partial_p \mu_1^2 \mathfrak{x}_1 \mathfrak{x}_2 - 10 \partial_p \mu_2 \mathfrak{x}_1 \mathfrak{x}_2 - 20 \eta \partial_p \mu_2 \mathfrak{x}_1 \mathfrak{x}_2 - 10 \partial_p \mu_1 \\
& \mu_2 \mathfrak{x}_1 \mathfrak{x}_2 - 20 \eta \partial_p \mu_1 \mu_2 \mathfrak{x}_1 \mathfrak{x}_2 + 10 \partial_p \mathfrak{x}_2^2 + 20 \eta \partial_p \mathfrak{x}_2^2 + 13 \\
& \partial_p \mu_1 \mathfrak{x}_2^2 + 57 \eta \partial_p \mu_1 \mathfrak{x}_2^2 + 46 \eta^2 \partial_p \mu_1 \mathfrak{x}_2^2 - 10 \eta^3 \partial_p \mu_1 \\
& \mathfrak{x}_2^2 - 3 \partial_p \mu_1^2 \mathfrak{x}_2^2 - 11 \eta \partial_p \mu_1^2 \mathfrak{x}_2^2 - 14 \eta^2 \partial_p \mu_1^2 \mathfrak{x}_2^2 - 10 \\
& \eta^3 \partial_p \mu_1^2 \mathfrak{x}_2^2 + 10 \partial_p \mu_2 \mathfrak{x}_2^2 + 20 \eta \partial_p \mu_2 \mathfrak{x}_2^2 - 2 \partial_p \mu_1 \mu_2 \\
& \mathfrak{x}_2^2 + 68 \eta \partial_p \mu_1 \mu_2 \mathfrak{x}_2^2 + 120 \eta^2 \partial_p \mu_1 \mu_2 \mathfrak{x}_2^2 + w^4 (-1 + \eta)^4 \\
& (5 \mu_2 (-1 + \mathfrak{x}_2) + 5 \mu_1 \mu_2 (-1 + \mathfrak{x}_2) - 2 \times (1 + 5 \mathfrak{x}_2) - \\
& 4 \mu_1 (1 + 5 \mathfrak{x}_2) + \mu_1^2 (70 + 26 \mathfrak{x}_2)) - w^3 (-1 + \eta)^3 \\
& (-12 + 56 \mu_1 + 356 \mu_1^2 - 53 \mu_2 + 43 \mu_1 \mu_2 - 2 \partial_p \mathfrak{x}_1 + 22 \partial_p \mu_1 \mathfrak{x}_1 + \\
& 48 \partial_p \mu_1^2 \mathfrak{x}_1 + 10 \partial_p \mu_2 \mathfrak{x}_1 + 10 \partial_p \mu_1 \mu_2 \mathfrak{x}_1 - 60 \mathfrak{x}_2 + 2 \partial_p \mathfrak{x}_2 - 128 \mu_1 \mathfrak{x}_2 - \\
& 22 \partial_p \mu_1 \mathfrak{x}_2 + 76 \mu_1^2 \mathfrak{x}_2 - 48 \partial_p \mu_1^2 \mathfrak{x}_2 + 5 \mu_2 \mathfrak{x}_2 - 10 \partial_p \mu_2 \mathfrak{x}_2 + \\
& 53 \mu_1 \mu_2 \mathfrak{x}_2 - 10 \partial_p \mu_1 \mu_2 \mathfrak{x}_2 - 10 \partial_p \mathfrak{x}_1 \mathfrak{x}_2 - 22 \partial_p \mu_1 \mathfrak{x}_1 \mathfrak{x}_2 - \\
& 10 \partial_p \mu_2 \mathfrak{x}_1 \mathfrak{x}_2 - 10 \partial_p \mu_1 \mu_2 \mathfrak{x}_1 \mathfrak{x}_2 + 10 \partial_p \mathfrak{x}_2^2 + 22 \partial_p \mu_1 \mathfrak{x}_2^2 + \\
& 10 \partial_p \mu_2 \mathfrak{x}_2^2 + 10 \partial_p \mu_1 \mu_2 \mathfrak{x}_2^2 + \eta (12 \mu_1^2 (33 + 8 \partial_p (\mathfrak{x}_1 - \mathfrak{x}_2) + 5 \mathfrak{x}_2) - \\
& \mu_2 (57 + 20 \partial_p (\mathfrak{x}_1 - \mathfrak{x}_2) (-1 + \mathfrak{x}_2) + 15 \mathfrak{x}_2) + 4 \times (1 + 5 \mathfrak{x}_2) \times \\
& (-3 + \partial_p (-\mathfrak{x}_1 + \mathfrak{x}_2)) + \mu_1 (72 - 44 \partial_p (\mathfrak{x}_1 - \mathfrak{x}_2) (-1 + \mathfrak{x}_2) - \\
& 156 \mathfrak{x}_2 + \mu_2 (87 - 20 \partial_p (\mathfrak{x}_1 - \mathfrak{x}_2) (-1 + \mathfrak{x}_2) + 57 \mathfrak{x}_2))) - w^2 \\
& (-1 + \eta)^2 (24 + 129 \mu_2 + 120 \mathfrak{x}_2 + 15 \mu_2 \mathfrak{x}_2 - 84 \mu_1^2 (7 + \mathfrak{x}_2) + \\
& \partial_p \mu_1^2 (44 + \mathfrak{x}_1 (-133 + \mathfrak{x}_2) + 133 \mathfrak{x}_2 + 3 \mathfrak{x}_2^2) - \\
& 3 \mu_1 (60 - 76 \mathfrak{x}_2 + \mu_2 (53 + 43 \mathfrak{x}_2)) + \\
& 6 \partial_p (1 + \mathfrak{x}_1 - 4 \mathfrak{x}_2 + 5 \mathfrak{x}_1 \mathfrak{x}_2 - 5 \mathfrak{x}_2^2 + \mu_2 (-9 + 5 \mathfrak{x}_1 (-1 + \mathfrak{x}_2) - 5 \mathfrak{x}_2^2)) + \\
& \partial_p \mu_1 (26 - 67 \mathfrak{x}_1 + 37 \mathfrak{x}_2 + 61 \mathfrak{x}_1 \mathfrak{x}_2 - 57 \mathfrak{x}_2^2 + \\
& 6 \mu_2 (15 + 5 \mathfrak{x}_1 (-1 + \mathfrak{x}_2) + 16 \mathfrak{x}_2 - 3 \mathfrak{x}_2^2)) + \\
& \eta (-9 \times (-4 - 19 \mu_2 - 20 \mathfrak{x}_2 - 5 \mu_2 \mathfrak{x}_2 + 4 \mu_1^2 (33 + 5 \mathfrak{x}_2) + \\
& \mu_1 (24 + 29 \mu_2 - 52 \mathfrak{x}_2 + 19 \mu_2 \mathfrak{x}_2)) + \\
& 4 \partial_p (\mu_1^2 (-56 + 89 \mathfrak{x}_2 + 3 \mathfrak{x}_2^2 + \mathfrak{x}_1 (-89 + 5 \mathfrak{x}_2)) + \\
& \mu_1 (-26 - 38 \mathfrak{x}_1 + 56 \mathfrak{x}_2 + 44 \mathfrak{x}_1 \mathfrak{x}_2 - 36 \mathfrak{x}_2^2 + 3 \mu_2
\end{aligned}$$

$$\begin{aligned}
& \left( -2 + 5 \mathfrak{x}1 (-1 + \mathfrak{x}2) + 3 \mathfrak{x}2 - 9 \mathfrak{x}2^2 \right) + 3 \times \left( 2 + \mathfrak{x}1 + \mathfrak{x}2 + 5 \right. \\
& \quad \left. \mathfrak{x}1 \mathfrak{x}2 - 5 \mathfrak{x}2^2 + \mu2 \left( -2 + 5 \mathfrak{x}1 (-1 + \mathfrak{x}2) + 11 \mathfrak{x}2 - 5 \mathfrak{x}2^2 \right) \right) + \\
& 2 \eta^2 \left( -12 \mu1 (-1 - 5 \mathfrak{x}2 + \mu1 (11 + \mathfrak{x}2)) + 5 \wp \left( \mu1^2 (-52 + \right. \right. \\
& \quad \left. \left. 3 \mathfrak{x}1 (-5 + \mathfrak{x}2) + 15 \mathfrak{x}2 + \mathfrak{x}2^2 \right) + \right. \\
& \quad \left. 2 \times (1 + 5 \mathfrak{x}2 + \mu2 (7 + 11 \mathfrak{x}2)) - \mu1 (26 + 3 \mathfrak{x}1 - 25 \mathfrak{x}2 - \right. \\
& \quad \left. 9 \mathfrak{x}1 \mathfrak{x}2 + 5 \mathfrak{x}2^2 + 2 \mu2 (17 + 13 \mathfrak{x}2 + 6 \mathfrak{x}2^2) \right) \left. \right) + w \\
& (-1 + \eta) \times \left( 20 - 176 \mu1 - 388 \mu1^2 + 119 \mu2 - 169 \mu1 \mu2 + 100 \mathfrak{x}2 + \right. \\
& \quad 152 \mu1 \mathfrak{x}2 - 44 \mu1^2 \mathfrak{x}2 + 25 \mu2 \mathfrak{x}2 - 119 \mu1 \mu2 \mathfrak{x}2 + 2 \wp \left( 2 + 3 \mathfrak{x}1 - 17 \mathfrak{x}2 + \right. \\
& \quad 15 \mathfrak{x}1 \mathfrak{x}2 - 15 \mathfrak{x}2^2 + \mu2 \left( -44 + 15 \mathfrak{x}1 (-1 + \mathfrak{x}2) - 13 \mathfrak{x}2 - 15 \mathfrak{x}2^2 \right) + \\
& \quad \mu1^2 (44 + \mathfrak{x}1 (-61 + \mathfrak{x}2) + 61 \mathfrak{x}2 + 3 \mathfrak{x}2^2) + \mu1 (22 - 34 \mathfrak{x}1 + 8 \mathfrak{x}2 + \\
& \quad 28 \mathfrak{x}1 \mathfrak{x}2 - 24 \mathfrak{x}2^2 + \mu2 (76 + 15 \mathfrak{x}1 (-1 + \mathfrak{x}2) + 71 \mathfrak{x}2 - 3 \mathfrak{x}2^2) \left. \right) \left. \right) + \\
& 2 \eta^3 \left( 10 \wp \mu2 (5 + \mathfrak{x}2) + \mu1^2 \left( -12 \times (-1 + \mathfrak{x}2) + 5 \wp \right. \right. \\
& \quad \left. \left( -54 + \mathfrak{x}1 (-1 + \mathfrak{x}2) + 5 \mathfrak{x}2 + \mathfrak{x}2^2 \right) + \mu1 \left( -12 \times (-1 + \mathfrak{x}2) + \right. \right. \\
& \quad \left. \left. 5 \wp (-6 + \mathfrak{x}1 (-1 + \mathfrak{x}2) + 29 \mathfrak{x}2 + \mathfrak{x}2^2 - 2 \mu2 (7 + 5 \mathfrak{x}2)) \right) \right) + \\
& \eta \left( -8 \mu1^2 (149 + 22 \mathfrak{x}2) + 9 \times (4 + 20 \mathfrak{x}2 + \mu2 (19 + 5 \mathfrak{x}2)) - \right. \\
& \quad \mu1 (220 - 472 \mathfrak{x}2 + 9 \mu2 (29 + 19 \mathfrak{x}2)) + \\
& \quad \wp \left( 2 \mu2 (-69 + 30 \mathfrak{x}1 (-1 + \mathfrak{x}2) + 93 \mathfrak{x}2 - 30 \mathfrak{x}2^2) + \right. \\
& \quad 4 \times (20 + \mathfrak{x}2 - 15 \mathfrak{x}2^2 + 3 \mathfrak{x}1 (1 + 5 \mathfrak{x}2)) + \\
& \quad \mu1^2 (-238 + 407 \mathfrak{x}2 + 23 \mathfrak{x}2^2 + \mathfrak{x}1 (-423 + 39 \mathfrak{x}2)) + \\
& \quad \mu1 (-158 + 171 \mathfrak{x}2 - 157 \mathfrak{x}2^2 + 3 \mathfrak{x}1 (-57 + 73 \mathfrak{x}2) + \\
& \quad 6 \mu2 (13 + 10 \mathfrak{x}1 (-1 + \mathfrak{x}2) + 17 \mathfrak{x}2 - 26 \mathfrak{x}2^2) \left. \right) \left. \right) + 8 \eta^2 \left( -6 \mu1 \right. \\
& \quad \left. (-1 - 5 \mathfrak{x}2 + \mu1 (11 + \mathfrak{x}2)) + \wp \left( 3 \times (5 + 5 \mu2 + 5 \mathfrak{x}2 + 17 \mu2 \mathfrak{x}2) + \right. \right. \\
& \quad \left. \left. \mu1^2 (-131 + 38 \mathfrak{x}2 + 3 \mathfrak{x}2^2 + \mathfrak{x}1 (-38 + 8 \mathfrak{x}2)) - \mu1 (56 + 8 \mathfrak{x}1 - \right. \right. \\
& \quad \left. \left. 53 \mathfrak{x}2 - 23 \mathfrak{x}1 \mathfrak{x}2 + 12 \mathfrak{x}2^2 + \mu2 (57 + 45 \mathfrak{x}2 + 30 \mathfrak{x}2^2) \right) \right) \left. \right) \left. \right) - \\
& x^4 (-1 + \eta)^4 \left( -2 \times (-1 + \eta) \wp \left( 5 + 23 \eta + 10 \eta^2 - 30 \eta^3 + 2 \eta t + 20 \eta \eta t + \right. \right. \\
& \quad 30 \eta^2 \eta t - 33 \mu1 - 82 \eta \mu1 - 65 \eta^2 \mu1 - 30 \eta^3 \mu1 - 2 \eta t \\
& \quad \mu1 + 18 \eta \eta t \mu1 + 30 \eta^2 \eta t \mu1 - 50 \mu1^2 - 225 \eta \mu1^2 - 255 \eta^2 \\
& \quad \mu1^2 + 20 \eta t \mu1^2 - 2 \eta \eta t \mu1^2 - \mu2 + 7 \eta \mu2 + 60 \eta^2 \mu2 - 16 \\
& \quad \eta t \mu2 - 30 \eta \eta t \mu2 - 37 \mu1 \mu2 - 101 \eta \mu1 \mu2 - 60 \eta^2 \mu1 \\
& \quad \mu2 + 20 \eta t \mu1 \mu2 + 30 \eta \eta t \mu1 \mu2 + w^4 (-1 + \eta)^4 (1 + \mu1) \\
& \quad (\eta - \eta t + 4 \mu1) (-1 + \mathfrak{x}2) + 13 \mathfrak{x}2 + 7 \eta \mathfrak{x}2 - 10 \eta^2 \mathfrak{x}2 + 30 \\
& \quad \eta^3 \mathfrak{x}2 - 2 \eta t \mathfrak{x}2 - 20 \eta \eta t \mathfrak{x}2 - 30 \eta^2 \eta t \mathfrak{x}2 + 21 \mu1 \mathfrak{x}2 + 112 \\
& \quad \eta \mu1 \mathfrak{x}2 + 155 \eta^2 \mu1 \mathfrak{x}2 + 30 \eta^3 \mu1 \mathfrak{x}2 - 10 \eta t \mu1 \mathfrak{x}2 - 18 \\
& \quad \eta \eta t \mu1 \mathfrak{x}2 - 30 \eta^2 \eta t \mu1 \mathfrak{x}2 + 2 \mu1^2 \mathfrak{x}2 + 45 \eta \mu1^2 \mathfrak{x}2 + 75 \\
& \quad \eta^2 \mu1^2 \mathfrak{x}2 + 4 \eta t \mu1^2 \mathfrak{x}2 + 2 \eta \eta t \mu1^2 \mathfrak{x}2 + 19 \mu2 \mathfrak{x}2 + 47 \eta \\
& \quad \mu2 \mathfrak{x}2 - 2 \eta t \mu2 \mathfrak{x}2 + \mu1 \mu2 \mathfrak{x}2 - 7 \eta \mu1 \mu2 \mathfrak{x}2 - 60 \eta^2 \mu1 \\
& \quad \mu2 \mathfrak{x}2 + 16 \eta t \mu1 \mu2 \mathfrak{x}2 + 30 \eta \eta t \mu1 \mu2 \mathfrak{x}2 - w^3 (-1 + \eta)^3 \\
& \quad \left( 2 + 7 \eta t - 45 \mu1 + 7 \eta t \mu1 - 59 \mu1^2 + 14 \mu2 - 12 \eta t \mu2 - 58 \mu1 \mu2 + \right. \\
& \quad 12 \eta t \mu1 \mu2 + 10 \eta^2 (1 + \mu1) \times (-1 + \mathfrak{x}2) + 10 \mathfrak{x}2 - 7 \eta t \mathfrak{x}2 + \\
& \quad 39 \mu1 \mathfrak{x}2 - 7 \eta t \mu1 \mathfrak{x}2 + 23 \mu1^2 \mathfrak{x}2 + 22 \mu2 \mathfrak{x}2 - 14 \mu1 \mu2 \mathfrak{x}2 + \\
& \quad 12 \eta t \mu1 \mu2 \mathfrak{x}2 + \eta (-7 + 12 \mu2 + 47 \mu1 (-1 + \mathfrak{x}2) + 40 \mu1^2 (-1 + \mathfrak{x}2) - \\
& \quad 10 \eta t (1 + \mu1) \times (-1 + \mathfrak{x}2) + 7 \mathfrak{x}2 - 12 \mu1 \mu2 (1 + \mathfrak{x}2) \left. \right) \left. \right) + w^2 (-1 + \eta)^2 \\
& \left( 9 - 113 \mu1 - 182 \mu1^2 + 37 \mu2 - 167 \mu1 \mu2 + 15 \eta^3 (1 + \mu1) \times (-1 + \mathfrak{x}2) + \right. \\
& \quad 33 \mathfrak{x}2 + 101 \mu1 \mathfrak{x}2 + 38 \mu1^2 \mathfrak{x}2 + 65 \mu2 \mathfrak{x}2 - 37 \mu1 \mu2 \mathfrak{x}2 -
\end{aligned}$$

$$\begin{aligned}
& 5 \eta^2 (8 - 6 \mu_2 - 12 \mu_1^2 (-1 + \mathfrak{z}_2) + 3 \eta t (1 + \mu_1) \times (-1 + \mathfrak{z}_2) - \\
& \quad 8 \mathfrak{z}_2 + \mu_1 (20 + 6 \mu_2 - 20 \mathfrak{z}_2 + 6 \mu_2 \mathfrak{z}_2)) + \eta t (-15 \times (-1 + \mathfrak{z}_2) + \\
& \quad 4 \mu_1^2 (5 + \mathfrak{z}_2) - 2 \mu_2 (20 + \mathfrak{z}_2) + \mu_1 (11 - 23 \mathfrak{z}_2 + \mu_2 (44 + 40 \mathfrak{z}_2))) + \\
& \quad \eta (-10 + 77 \mu_2 + 40 \mathfrak{z}_2 + 55 \mu_2 \mathfrak{z}_2 + 5 \mu_1^2 (-61 + 25 \mathfrak{z}_2) - \\
& \quad \mu_1 (195 + 187 \mu_2 - 225 \mathfrak{z}_2 + 77 \mu_2 \mathfrak{z}_2) + \\
& \quad 10 \eta t (4 - 3 \mu_2 - 4 \mathfrak{z}_2 + \mu_1 (4 - 4 \mathfrak{z}_2 + 3 \mu_2 (1 + \mathfrak{z}_2)))) - w \\
& (-1 + \eta) \times (16 - 101 \mu_1 - 177 \mu_1^2 + 22 \mu_2 - 146 \mu_1 \mu_2 + 45 \eta^3 \\
& \quad (1 + \mu_1) \times (-1 + \mathfrak{z}_2) + 32 \mathfrak{z}_2 + 83 \mu_1 \mathfrak{z}_2 + 21 \mu_1^2 \mathfrak{z}_2 + 62 \mu_2 \mathfrak{z}_2 - \\
& \quad 22 \mu_1 \mu_2 \mathfrak{z}_2 - 5 \eta^2 (9 \eta t (1 + \mu_1) \times (-1 + \mathfrak{z}_2) - 9 \mu_1^2 (-7 + 3 \mathfrak{z}_2) - \\
& \quad 2 \times (-5 + 9 \mu_2 + 5 \mathfrak{z}_2) + \mu_1 (37 - 55 \mathfrak{z}_2 + 18 \mu_2 (1 + \mathfrak{z}_2))) + \\
& \quad \eta t (-11 \times (-1 + \mathfrak{z}_2) + 8 \mu_1^2 (5 + \mathfrak{z}_2) - 4 \mu_2 (11 + \mathfrak{z}_2) + \\
& \quad \mu_1 (3 - 27 \mathfrak{z}_2 + \mu_2 (52 + 44 \mathfrak{z}_2))) + \\
& \quad \eta (19 + 72 \mu_2 + 41 \mathfrak{z}_2 + 102 \mu_2 \mathfrak{z}_2 + 10 \mu_1^2 (-49 + 13 \mathfrak{z}_2) - \\
& \quad 3 \mu_1 (77 + 92 \mu_2 - 97 \mathfrak{z}_2 + 24 \mu_2 \mathfrak{z}_2) + 2 \eta t (\mu_1^2 (-1 + \mathfrak{z}_2) - \\
& \quad 5 \times (-5 + 6 \mu_2 + 5 \mathfrak{z}_2) + 6 \mu_1 (4 - 4 \mathfrak{z}_2 + 5 \mu_2 (1 + \mathfrak{z}_2)))) + \\
& (-1 + \eta t) \mathfrak{e} l (4 + 6 \mathfrak{e} p + 50 \eta \mathfrak{e} p + 60 \eta^2 \mathfrak{e} p - 16 \mu_1 + 16 \eta \mu_1 + 16 \eta^2 \\
& \quad \mu_1 - 22 \mathfrak{e} p \mu_1 - 92 \eta \mathfrak{e} p \mu_1 + 20 \eta^2 \mathfrak{e} p \mu_1 - 140 \mu_1^2 - 176 \eta \\
& \quad \mu_1^2 + 16 \eta^2 \mu_1^2 - 4 \mathfrak{e} p \mu_1^2 - 262 \eta \mathfrak{e} p \mu_1^2 - 400 \eta^2 \mathfrak{e} p \mu_1^2 + 19 \\
& \quad \mu_2 - 26 \mathfrak{e} p \mu_2 - 20 \eta \mathfrak{e} p \mu_2 + 50 \eta^2 \mathfrak{e} p \mu_2 - 29 \mu_1 \mu_2 + 22 \mathfrak{e} p \\
& \quad \mu_1 \mu_2 - 44 \eta \mathfrak{e} p \mu_1 \mu_2 - 70 \eta^2 \mathfrak{e} p \mu_1 \mu_2 + \mathfrak{e} p \mathfrak{z}_1 - 16 \mathfrak{e} p \mu_1 \\
& \quad \mathfrak{z}_1 - 16 \eta \mathfrak{e} p \mu_1 \mathfrak{z}_1 - 5 \eta^2 \mathfrak{e} p \mu_1 \mathfrak{z}_1 - 41 \mathfrak{e} p \mu_1^2 \mathfrak{z}_1 - 76 \eta \mathfrak{e} p \mu_1^2 \\
& \quad \mathfrak{z}_1 - 5 \eta^2 \mathfrak{e} p \mu_1^2 \mathfrak{z}_1 - 5 \mathfrak{e} p \mu_2 \mathfrak{z}_1 - 5 \mathfrak{e} p \mu_1 \mu_2 \mathfrak{z}_1 + 20 \mathfrak{z}_2 + 5 \\
& \quad \mathfrak{e} p \mathfrak{z}_2 + 10 \eta \mathfrak{e} p \mathfrak{z}_2 - 60 \eta^2 \mathfrak{e} p \mathfrak{z}_2 + 52 \mu_1 \mathfrak{z}_2 + 80 \eta \mu_1 \mathfrak{z}_2 - 16 \\
& \quad \eta^2 \mu_1 \mathfrak{z}_2 + 6 \mathfrak{e} p \mu_1 \mathfrak{z}_2 + 86 \eta \mathfrak{e} p \mu_1 \mathfrak{z}_2 + 155 \eta^2 \mathfrak{e} p \mu_1 \mathfrak{z}_2 - 28 \\
& \quad \mu_1^2 \mathfrak{z}_2 - 16 \eta \mu_1^2 \mathfrak{z}_2 - 16 \eta^2 \mu_1^2 \mathfrak{z}_2 + 37 \mathfrak{e} p \mu_1^2 \mathfrak{z}_2 + 76 \eta \mathfrak{e} p \\
& \quad \mu_1^2 \mathfrak{z}_2 + 35 \eta^2 \mathfrak{e} p \mu_1^2 \mathfrak{z}_2 + 5 \mu_2 \mathfrak{z}_2 + 19 \mathfrak{e} p \mu_2 \mathfrak{z}_2 + 92 \eta \mathfrak{e} p \\
& \quad \mu_2 \mathfrak{z}_2 + 10 \eta^2 \mathfrak{e} p \mu_2 \mathfrak{z}_2 - 19 \mu_1 \mu_2 \mathfrak{z}_2 + 19 \mathfrak{e} p \mu_1 \mu_2 \mathfrak{z}_2 - 40 \eta \\
& \quad \mathfrak{e} p \mu_1 \mu_2 \mathfrak{z}_2 - 50 \eta^2 \mathfrak{e} p \mu_1 \mu_2 \mathfrak{z}_2 + 5 \mathfrak{e} p \mathfrak{z}_1 \mathfrak{z}_2 + 22 \mathfrak{e} p \mu_1 \mathfrak{z}_1 \\
& \quad \mathfrak{z}_2 + 46 \eta \mathfrak{e} p \mu_1 \mathfrak{z}_1 \mathfrak{z}_2 + 5 \eta^2 \mathfrak{e} p \mu_1 \mathfrak{z}_1 \mathfrak{z}_2 + 5 \mathfrak{e} p \mu_1^2 \mathfrak{z}_1 \mathfrak{z}_2 + 16 \\
& \quad \eta \mathfrak{e} p \mu_1^2 \mathfrak{z}_1 \mathfrak{z}_2 + 5 \eta^2 \mathfrak{e} p \mu_1^2 \mathfrak{z}_1 \mathfrak{z}_2 + 5 \mathfrak{e} p \mu_2 \mathfrak{z}_1 \mathfrak{z}_2 + 5 \mathfrak{e} p \\
& \quad \mu_1 \mu_2 \mathfrak{z}_1 \mathfrak{z}_2 - 5 \mathfrak{e} p \mathfrak{z}_2^2 - 14 \mathfrak{e} p \mu_1 \mathfrak{z}_2^2 - 24 \eta \mathfrak{e} p \mu_1 \mathfrak{z}_2^2 + 5 \\
& \quad \eta^2 \mathfrak{e} p \mu_1 \mathfrak{z}_2^2 + 3 \mathfrak{e} p \mu_1^2 \mathfrak{z}_2^2 + 6 \eta \mathfrak{e} p \mu_1^2 \mathfrak{z}_2^2 + 5 \eta^2 \mathfrak{e} p \mu_1^2 \\
& \quad \mathfrak{z}_2^2 - 5 \mathfrak{e} p \mu_2 \mathfrak{z}_2^2 - 17 \mathfrak{e} p \mu_1 \mu_2 \mathfrak{z}_2^2 - 60 \eta \mathfrak{e} p \mu_1 \mu_2 \mathfrak{z}_2^2 + w^3 \\
& (-1 + \eta)^3 (-\mu_2 (19 + 5 \mathfrak{e} p (\mathfrak{z}_1 - \mathfrak{z}_2) (-1 + \mathfrak{z}_2) + 5 \mathfrak{z}_2) + \\
& \quad 4 \mu_1^2 (6 \mathfrak{e} p (\mathfrak{z}_1 - \mathfrak{z}_2) + 7 \times (5 + \mathfrak{z}_2)) + (1 + 5 \mathfrak{z}_2) \times (-4 + \mathfrak{e} p (-\mathfrak{z}_1 + \mathfrak{z}_2)) + \\
& \quad \mu_1 (16 - 11 \mathfrak{e} p (\mathfrak{z}_1 - \mathfrak{z}_2) (-1 + \mathfrak{z}_2) - 52 \mathfrak{z}_2 + \\
& \quad \mu_2 (29 - 5 \mathfrak{e} p (\mathfrak{z}_1 - \mathfrak{z}_2) (-1 + \mathfrak{z}_2) + 19 \mathfrak{z}_2))) + w^2 (-1 + \eta)^2 \\
& (12 - 48 \mu_1 + 16 \eta \mu_1 - 420 \mu_1^2 - 176 \eta \mu_1^2 + 57 \mu_2 - 87 \mu_1 \mu_2 + \\
& \quad 60 \mathfrak{z}_2 + 156 \mu_1 \mathfrak{z}_2 + 80 \eta \mu_1 \mathfrak{z}_2 - 84 \mu_1^2 \mathfrak{z}_2 - 16 \eta \mu_1^2 \mathfrak{z}_2 + 15 \mu_2 \mathfrak{z}_2 - \\
& \quad 57 \mu_1 \mu_2 \mathfrak{z}_2 + \mathfrak{e} p (\mu_1^2 (-56 + 89 \mathfrak{z}_2 + 3 \mathfrak{z}_2^2 + \mathfrak{z}_1 (-89 + 5 \mathfrak{z}_2)) + \\
& \quad \mu_1 (-26 - 38 \mathfrak{z}_1 + 56 \mathfrak{z}_2 + 44 \mathfrak{z}_1 \mathfrak{z}_2 - 36 \mathfrak{z}_2^2 + \\
& \quad 3 \mu_2 (-2 + 5 \mathfrak{z}_1 (-1 + \mathfrak{z}_2) + 3 \mathfrak{z}_2 - 9 \mathfrak{z}_2^2))) + 3 \times (2 + \mathfrak{z}_1 + \mathfrak{z}_2 + \\
& \quad 5 \mathfrak{z}_1 \mathfrak{z}_2 - 5 \mathfrak{z}_2^2 + \mu_2 (-2 + 5 \mathfrak{z}_1 (-1 + \mathfrak{z}_2) + 11 \mathfrak{z}_2 - 5 \mathfrak{z}_2^2)) + \\
& \quad 5 \eta (\mu_1^2 (-52 + 3 \mathfrak{z}_1 (-5 + \mathfrak{z}_2) + 15 \mathfrak{z}_2 + \mathfrak{z}_2^2) +
\end{aligned}$$

$$\begin{aligned}
& 2 \times (1 + 5 \mathfrak{z}2 + \mu2 (7 + 11 \mathfrak{z}2)) - \mu1 (26 + 3 \mathfrak{z}1 - 25 \mathfrak{z}2 - \\
& \quad 9 \mathfrak{z}1 \mathfrak{z}2 + 5 \mathfrak{z}2^2 + 2 \mu2 (17 + 13 \mathfrak{z}2 + 6 \mathfrak{z}2^2)) \Big) \Big) \Big) - w \\
& (-1 + \eta) \times (-4 \mu1^2 (4 \eta^2 (-1 + \mathfrak{z}2) + 21 \times (5 + \mathfrak{z}2) + 8 \eta (11 + \mathfrak{z}2)) + \\
& \quad 3 \times (4 + 20 \mathfrak{z}2 + \mu2 (19 + 5 \mathfrak{z}2)) + \mu1 \\
& \quad (-48 - 16 \eta^2 (-1 + \mathfrak{z}2) + 156 \mathfrak{z}2 + 32 \eta (1 + 5 \mathfrak{z}2) - 3 \mu2 (29 + 19 \mathfrak{z}2)) + \\
& \quad \text{op} (20 - 32 \mu2 + 3 \mathfrak{z}1 - 15 \mu2 \mathfrak{z}1 + \mathfrak{z}2 + 47 \mu2 \mathfrak{z}2 + 15 \mathfrak{z}1 \mathfrak{z}2 + 15 \mu2 \mathfrak{z}1 \mathfrak{z}2 - \\
& \quad 15 \mathfrak{z}2^2 - 15 \mu2 \mathfrak{z}2^2 + 2 \mu1^2 (-30 - 53 \mathfrak{z}1 + 51 \mathfrak{z}2 + 5 \mathfrak{z}1 \mathfrak{z}2 + 3 \mathfrak{z}2^2) + \\
& \quad \mu1 (-40 + \mu2 (-16 + 15 \mathfrak{z}1 - 39 \mathfrak{z}2) \times (-1 + \mathfrak{z}2) + \\
& \quad 43 \mathfrak{z}2 - 39 \mathfrak{z}2^2 + \mathfrak{z}1 (-43 + 55 \mathfrak{z}2)) + \\
& \quad 5 \eta^2 (2 \mu2 (5 + \mathfrak{z}2) + \mu1^2 (-80 + \mathfrak{z}1 (-1 + \mathfrak{z}2) + 7 \mathfrak{z}2 + \mathfrak{z}2^2) + \\
& \quad \mu1 (-8 + \mathfrak{z}1 (-1 + \mathfrak{z}2) + 43 \mathfrak{z}2 + \mathfrak{z}2^2 - 2 \mu2 (7 + 5 \mathfrak{z}2))) + \\
& \quad \eta (60 \times (1 + \mathfrak{z}2) + \mu2 (50 + 202 \mathfrak{z}2) + \mu1^2 (-522 + 151 \mathfrak{z}2 + \\
& \quad 11 \mathfrak{z}2^2 + \mathfrak{z}1 (-151 + 31 \mathfrak{z}2)) - \mu1 (222 + 31 \mathfrak{z}1 - 211 \mathfrak{z}2 - \\
& \quad 91 \mathfrak{z}1 \mathfrak{z}2 + 49 \mathfrak{z}2^2 + 2 \mu2 (107 + 85 \mathfrak{z}2 + 60 \mathfrak{z}2^2)) \Big) \Big) \Big) \Big) + \\
& x^2 (-1 + \eta)^2 ((-1 + \eta) \text{op} (12 \eta + 60 \eta^2 + 76 \eta^3 - 20 \eta^4 - 60 \eta^5 - 6 \eta t - 12 \\
& \quad \eta \eta t + 24 \eta^2 \eta t + 80 \eta^3 \eta t + 60 \eta^4 \eta t - 120 \eta \mu1 - 396 \eta^2 \\
& \quad \mu1 - 344 \eta^3 \mu1 - 170 \eta^4 \mu1 - 60 \eta^5 \mu1 + 44 \eta t \mu1 + 28 \eta \\
& \quad \eta t \mu1 - 24 \eta^2 \eta t \mu1 + 56 \eta^3 \eta t \mu1 + 60 \eta^4 \eta t \mu1 - 132 \eta \\
& \quad \mu1^2 - 600 \eta^2 \mu1^2 - 900 \eta^3 \mu1^2 - 510 \eta^4 \mu1^2 + 98 \eta t \mu1^2 + 424 \\
& \quad \eta \eta t \mu1^2 + 240 \eta^2 \eta t \mu1^2 - 24 \eta^3 \eta t \mu1^2 - 56 \eta \mu2 - 12 \eta^2 \\
& \quad \mu2 + 204 \eta^3 \mu2 + 240 \eta^4 \mu2 - 38 \eta t \mu2 - 117 \eta \eta t \mu2 - 192 \\
& \quad \eta^2 \eta t \mu2 - 120 \eta^3 \eta t \mu2 - 8 \eta \mu1 \mu2 - 444 \eta^2 \mu1 \mu2 - 612 \eta^3 \\
& \quad \mu1 \mu2 - 240 \eta^4 \mu1 \mu2 + 58 \eta t \mu1 \mu2 + 171 \eta \eta t \mu1 \mu2 + 240 \\
& \quad \eta^2 \eta t \mu1 \mu2 + 120 \eta^3 \eta t \mu1 \mu2 + 60 \eta \mathfrak{z}2 + 156 \eta^2 \mathfrak{z}2 + 44 \\
& \quad \eta^3 \mathfrak{z}2 + 20 \eta^4 \mathfrak{z}2 + 60 \eta^5 \mathfrak{z}2 - 30 \eta t \mathfrak{z}2 - 60 \eta \eta t \mathfrak{z}2 - 24 \\
& \quad \eta^2 \eta t \mathfrak{z}2 - 80 \eta^3 \eta t \mathfrak{z}2 - 60 \eta^4 \eta t \mathfrak{z}2 + 48 \eta \mu1 \mathfrak{z}2 + 252 \\
& \quad \eta^2 \mu1 \mathfrak{z}2 + 464 \eta^3 \mu1 \mathfrak{z}2 + 350 \eta^4 \mu1 \mathfrak{z}2 + 60 \eta^5 \mu1 \mathfrak{z}2 - 32 \\
& \quad \eta t \mu1 \mathfrak{z}2 - 148 \eta \eta t \mu1 \mathfrak{z}2 - 120 \eta^2 \eta t \mu1 \mathfrak{z}2 - 56 \eta^3 \eta t \\
& \quad \mu1 \mathfrak{z}2 - 60 \eta^4 \eta t \mu1 \mathfrak{z}2 - 12 \eta \mu1^2 \mathfrak{z}2 + 24 \eta^2 \mu1^2 \mathfrak{z}2 + 180 \\
& \quad \eta^3 \mu1^2 \mathfrak{z}2 + 150 \eta^4 \mu1^2 \mathfrak{z}2 + 22 \eta t \mu1^2 \mathfrak{z}2 + 104 \eta \eta t \mu1^2 \\
& \quad \mathfrak{z}2 + 48 \eta^2 \eta t \mu1^2 \mathfrak{z}2 + 24 \eta^3 \eta t \mu1^2 \mathfrak{z}2 + 32 \eta \mu2 \mathfrak{z}2 + 228 \\
& \quad \eta^2 \mu2 \mathfrak{z}2 + 204 \eta^3 \mu2 \mathfrak{z}2 - 10 \eta t \mu2 \mathfrak{z}2 - 27 \eta \eta t \mu2 \mathfrak{z}2 - 24 \\
& \quad \eta^2 \eta t \mu2 \mathfrak{z}2 + 56 \eta \mu1 \mu2 \mathfrak{z}2 + 12 \eta^2 \mu1 \mu2 \mathfrak{z}2 - 204 \eta^3 \mu1 \\
& \quad \mu2 \mathfrak{z}2 - 240 \eta^4 \mu1 \mu2 \mathfrak{z}2 + 38 \eta t \mu1 \mu2 \mathfrak{z}2 + 117 \eta \eta t \mu1 \mu2 \\
& \quad \mathfrak{z}2 + 192 \eta^2 \eta t \mu1 \mu2 \mathfrak{z}2 + 120 \eta^3 \eta t \mu1 \mu2 \mathfrak{z}2 + w^4 (-1 + \eta)^4 \\
& \quad (2 - 10 \mu2 - 17 \eta t \mu2 + 12 \eta^3 (1 + \mu1) \times (-1 + \mathfrak{z}2) + 10 \mathfrak{z}2 - 12 \eta t \mathfrak{z}2 + \\
& \quad 22 \mu2 \mathfrak{z}2 + 5 \eta t \mu2 \mathfrak{z}2 + \mu1^2 (6 \times (-5 + \mathfrak{z}2) + \eta t (82 + 38 \mathfrak{z}2)) + \mu1 \\
& \quad (-28 + 16 \mathfrak{z}2 + 2 \mu2 (-17 + 5 \mathfrak{z}2) + \eta t (-14 + 7 \mu2 - 22 \mathfrak{z}2 + 17 \mu2 \mathfrak{z}2)) - \\
& \quad 12 \eta^2 (1 - 3 \mu2 - 4 \mu1^2 (-1 + \mathfrak{z}2) + \eta t (1 + \mu1) \times (-1 + \mathfrak{z}2) - \\
& \quad \mathfrak{z}2 + \mu1 (5 - 5 \mathfrak{z}2 + 3 \mu2 (1 + \mathfrak{z}2))) + \\
& \quad 2 \eta (2 + 27 \mu2 + 16 \mathfrak{z}2 + 33 \mu2 \mathfrak{z}2 + 3 \mu1^2 (-19 + 7 \mathfrak{z}2) + \\
& \quad 6 \eta t (1 + \mu1 - 3 \mu2 - \mathfrak{z}2 - \mu1 \mathfrak{z}2 + 3 \mu1 \mu2 (1 + \mathfrak{z}2)) - \\
& \quad \mu1 (55 - 37 \mathfrak{z}2 + 3 \mu2 (31 + 9 \mathfrak{z}2))) \Big) - w^3 (-1 + \eta)^3 \\
& (40 \eta^4 (1 + \mu1) \times (-1 + \mathfrak{z}2) - 4 \eta^3 (-61 \mu1 (-1 + \mathfrak{z}2) - 40 \mu1^2 \\
& \quad (-1 + \mathfrak{z}2) + 10 \eta t (1 + \mu1) \times (-1 + \mathfrak{z}2) + 36 \mu1 \mu2 (1 + \mathfrak{z}2) -
\end{aligned}$$



$$\begin{aligned}
& 3 \times (-7 + 12 \mu_2 + 7 \mathfrak{z}_2) + 2 \times (4 + 5 \mu_1^2 (-13 + \mathfrak{z}_2) + 20 \mathfrak{z}_2 + \\
& 6 \mu_2 (-1 + 5 \mathfrak{z}_2) + \mu_1 (-49 + 6 \mu_2 (-9 + \mathfrak{z}_2) + 31 \mathfrak{z}_2)) + \\
& 3 \eta (10 + 68 \mu_2 + 62 \mathfrak{z}_2 + 112 \mu_2 \mathfrak{z}_2 + 8 \mu_1^2 (-29 + 5 \mathfrak{z}_2) + 4 \eta \mu_1^2 \\
& (35 + 9 \mathfrak{z}_2) - 3 \eta \mathfrak{t} (-4 + 12 \mathfrak{z}_2 + \mu_2 (29 + 3 \mathfrak{z}_2)) - 2 \mu_1 (87 - 63 \mathfrak{z}_2 + \\
& 2 \mu_2 (73 + 17 \mathfrak{z}_2)) + \eta \mathfrak{t} \mu_1 (24 - 64 \mathfrak{z}_2 + 3 \mu_2 (35 + 29 \mathfrak{z}_2))) + \\
& \eta \mathfrak{t} (-6 + \mu_2 (-97 + \mathfrak{z}_2) - 66 \mathfrak{z}_2 + 16 \mu_1^2 (25 + 8 \mathfrak{z}_2) + \\
& \mu_1 (10 - 130 \mathfrak{z}_2 + \mu_2 (95 + 97 \mathfrak{z}_2))) + 12 \eta^2 (-2 + 29 \mu_2 + 14 \mathfrak{z}_2 + \\
& 22 \mu_2 \mathfrak{z}_2 + \mu_1^2 (-59 + 23 \mathfrak{z}_2) - \mu_1 (49 + 73 \mu_2 - 43 \mathfrak{z}_2 + 29 \mu_2 \mathfrak{z}_2) + \\
& \eta \mathfrak{t} (7 - 12 \mu_2 - 7 \mathfrak{z}_2 + \mu_1 (7 - 7 \mathfrak{z}_2 + 12 \mu_2 (1 + \mathfrak{z}_2)))) - w \\
& (-1 + \eta) \times (90 \eta^5 (1 + \mu_1) \times (-1 + \mathfrak{z}_2) - 4 \times (1 + \mu_1) \times \\
& (-1 - 3 \mu_2 (-1 + \mathfrak{z}_2) - 5 \mathfrak{z}_2 + \mu_1 (11 + \mathfrak{z}_2)) - \\
& 10 \eta^4 (9 \eta \mathfrak{t} (1 + \mu_1) \times (-1 + \mathfrak{z}_2) - 9 \mu_1^2 (-7 + 3 \mathfrak{z}_2) - \\
& 4 \times (-5 + 9 \mu_2 + 5 \mathfrak{z}_2) + \mu_1 (47 - 65 \mathfrak{z}_2 + 36 \mu_2 (1 + \mathfrak{z}_2))) + \\
& 4 \eta^3 (-3 + 176 \mu_2 + 63 \mathfrak{z}_2 + 106 \mu_2 \mathfrak{z}_2 + 10 \mu_1^2 (-49 + 13 \mathfrak{z}_2) + \\
& \eta \mathfrak{t} (-44 \mu_1 (-1 + \mathfrak{z}_2) + 6 \mu_1^2 (-1 + \mathfrak{z}_2) + 60 \mu_1 \mu_2 (1 + \mathfrak{z}_2) - 10 \times \\
& (-5 + 6 \mu_2 + 5 \mathfrak{z}_2)) - \mu_1 (253 - 313 \mathfrak{z}_2 + 4 \mu_2 (97 + 44 \mathfrak{z}_2))) + \\
& \eta \mathfrak{t} (48 \mu_1^2 (9 + 2 \mathfrak{z}_2) - 20 \times (1 + 5 \mathfrak{z}_2) - \mu_2 (139 + 29 \mathfrak{z}_2) + \\
& \mu_1 (124 - 148 \mathfrak{z}_2 + \mu_2 (197 + 139 \mathfrak{z}_2))) + \\
& 12 \eta^2 (14 + 34 \mu_2 + 34 \mathfrak{z}_2 + 62 \mu_2 \mathfrak{z}_2 + 3 \mu_1^2 (-59 + 7 \mathfrak{z}_2) - \\
& \mu_1 (103 - 85 \mathfrak{z}_2 + 2 \mu_2 (79 + 17 \mathfrak{z}_2)) + \eta \mathfrak{t} (-11 \times (-1 + \mathfrak{z}_2) + 8 \mu_1^2 \\
& (5 + \mathfrak{z}_2) - 4 \mu_2 (11 + \mathfrak{z}_2) + \mu_1 (3 - 27 \mathfrak{z}_2 + \mu_2 (52 + 44 \mathfrak{z}_2)))) + \\
& \eta (4 \times (18 - 17 \mu_2 + 3 \mu_1^2 (-61 + \mathfrak{z}_2) + 54 \mathfrak{z}_2 + 65 \mu_2 \mathfrak{z}_2 + \\
& \mu_1 (-129 - 113 \mu_2 + 75 \mathfrak{z}_2 + 17 \mu_2 \mathfrak{z}_2)) + \\
& \eta \mathfrak{t} (16 \mu_1^2 (79 + 20 \mathfrak{z}_2) - 3 \times (4 + 68 \mathfrak{z}_2 + 3 \mu_2 (47 + 9 \mathfrak{z}_2)) + \\
& \mu_1 (100 - 460 \mathfrak{z}_2 + 9 \mu_2 (65 + 47 \mathfrak{z}_2)))) + w^2 \\
& (-1 + \eta)^2 (-2 \times (-7 + 72 \mu_1^2 + \mu_1 (53 + \mu_2 (43 - 7 \mathfrak{z}_2) - 29 \mathfrak{z}_2) + \\
& \mu_2 (7 - 25 \mathfrak{z}_2) - 23 \mathfrak{z}_2) + 30 \eta^5 (1 + \mu_1) \times (-1 + \mathfrak{z}_2) + \\
& \eta \mathfrak{t} (-\mu_2 (181 + 23 \mathfrak{z}_2) - 4 \times (5 + 31 \mathfrak{z}_2) + 4 \mu_1^2 (163 + 41 \mathfrak{z}_2) + \\
& \mu_1 (104 - 224 \mathfrak{z}_2 + \mu_2 (227 + 181 \mathfrak{z}_2))) - \\
& 10 \eta^4 (3 \eta \mathfrak{t} (1 + \mu_1) \times (-1 + \mathfrak{z}_2) - 4 \times (-4 + 3 \mu_2 + 3 \mu_1^2 \\
& (-1 + \mathfrak{z}_2) + 4 \mathfrak{z}_2 - \mu_1 (7 - 7 \mathfrak{z}_2 + 3 \mu_2 (1 + \mathfrak{z}_2)))) + \\
& 4 \eta^3 (-40 + 161 \mu_2 + 70 \mathfrak{z}_2 + 55 \mu_2 \mathfrak{z}_2 + 5 \mu_1^2 (-61 + 25 \mathfrak{z}_2) - \\
& \mu_1 (225 + 271 \mu_2 - 255 \mathfrak{z}_2 + 161 \mu_2 \mathfrak{z}_2) + \\
& 10 \eta \mathfrak{t} (4 - 3 \mu_2 - 4 \mathfrak{z}_2 + \mu_1 (4 - 4 \mathfrak{z}_2 + 3 \mu_2 (1 + \mathfrak{z}_2))) + \\
& 12 \eta^2 (4 + 61 \mu_2 + 38 \mathfrak{z}_2 + 65 \mu_2 \mathfrak{z}_2 + 2 \mu_1^2 (-91 + 19 \mathfrak{z}_2) - \\
& \mu_1 (118 - 106 \mathfrak{z}_2 + \mu_2 (191 + 61 \mathfrak{z}_2)) + \eta \mathfrak{t} (-15 \times (-1 + \mathfrak{z}_2) + 4 \mu_1^2 \\
& (5 + \mathfrak{z}_2) - 2 \mu_2 (20 + \mathfrak{z}_2) + \mu_1 (11 - 23 \mathfrak{z}_2 + \mu_2 (44 + 40 \mathfrak{z}_2)))) + \\
& \eta (86 + 310 \mathfrak{z}_2 + 6 \mu_1^2 (-197 + 17 \mathfrak{z}_2) + 6 \mu_2 (23 + 83 \mathfrak{z}_2) - \\
& 2 \mu_1 (404 - 278 \mathfrak{z}_2 + \mu_2 (567 + 69 \mathfrak{z}_2)) + \\
& 3 \eta \mathfrak{t} (8 - 80 \mathfrak{z}_2 + 12 \mu_1^2 (35 + 9 \mathfrak{z}_2) - 3 \mu_2 (59 + 9 \mathfrak{z}_2) + \\
& \mu_1 (44 - 164 \mathfrak{z}_2 + 3 \mu_2 (77 + 59 \mathfrak{z}_2)))) + \\
& (-1 + \eta \mathfrak{t}) \mathfrak{e} \mathfrak{l} (-2 - 12 \eta - 12 \eta^2 + 2 \mathfrak{e} \mathfrak{p} + 6 \eta \mathfrak{e} \mathfrak{p} - 36 \eta^2 \mathfrak{e} \mathfrak{p} - 100 \eta^3 \\
& \mathfrak{e} \mathfrak{p} - 60 \eta^4 \mathfrak{e} \mathfrak{p} + 20 \mu_1 + 136 \eta \mu_1 + 104 \eta^2 \mu_1 - 16 \eta^3 \mu_1 - 16
\end{aligned}$$

$$\begin{aligned}
& \eta^4 \mu_1 - 20 \operatorname{ep} \mu_1 - 56 \eta \operatorname{ep} \mu_1 + 126 \eta^2 \operatorname{ep} \mu_1 + 192 \eta^3 \operatorname{ep} \\
& \mu_1 - 10 \eta^4 \operatorname{ep} \mu_1 + 22 \mu_1^2 + 148 \eta \mu_1^2 + 380 \eta^2 \mu_1^2 + 176 \\
& \eta^3 \mu_1^2 - 16 \eta^4 \mu_1^2 - 22 \operatorname{ep} \mu_1^2 - 134 \eta \operatorname{ep} \mu_1^2 + 18 \eta^2 \operatorname{ep} \\
& \mu_1^2 + 532 \eta^3 \operatorname{ep} \mu_1^2 + 410 \eta^4 \operatorname{ep} \mu_1^2 - 19 \mu_2 - 76 \eta \mu_2 - 57 \\
& \eta^2 \mu_2 + 14 \operatorname{ep} \mu_2 + 112 \eta \operatorname{ep} \mu_2 + 186 \eta^2 \operatorname{ep} \mu_2 - 100 \eta^4 \operatorname{ep} \\
& \mu_2 + 29 \mu_1 \mu_2 + 116 \eta \mu_1 \mu_2 + 87 \eta^2 \mu_1 \mu_2 - 34 \operatorname{ep} \mu_1 \mu_2 - 200 \\
& \eta \operatorname{ep} \mu_1 \mu_2 - 174 \eta^2 \operatorname{ep} \mu_1 \mu_2 + 144 \eta^3 \operatorname{ep} \mu_1 \mu_2 + 140 \eta^4 \operatorname{ep} \\
& \mu_1 \mu_2 - \operatorname{ep} \mathfrak{z}_1 - 6 \eta \operatorname{ep} \mathfrak{z}_1 - 6 \eta^2 \operatorname{ep} \mathfrak{z}_1 + 10 \operatorname{ep} \mu_1 \mathfrak{z}_1 + 68 \\
& \eta \operatorname{ep} \mu_1 \mathfrak{z}_1 + 93 \eta^2 \operatorname{ep} \mu_1 \mathfrak{z}_1 + 36 \eta^3 \operatorname{ep} \mu_1 \mathfrak{z}_1 + 10 \eta^4 \operatorname{ep} \\
& \mu_1 \mathfrak{z}_1 + 11 \operatorname{ep} \mu_1^2 \mathfrak{z}_1 + 110 \eta \operatorname{ep} \mu_1^2 \mathfrak{z}_1 + 243 \eta^2 \operatorname{ep} \mu_1^2 \\
& \mathfrak{z}_1 + 156 \eta^3 \operatorname{ep} \mu_1^2 \mathfrak{z}_1 + 10 \eta^4 \operatorname{ep} \mu_1^2 \mathfrak{z}_1 + 5 \operatorname{ep} \mu_2 \mathfrak{z}_1 + 30 \eta \\
& \operatorname{ep} \mu_2 \mathfrak{z}_1 + 30 \eta^2 \operatorname{ep} \mu_2 \mathfrak{z}_1 + 5 \operatorname{ep} \mu_1 \mu_2 \mathfrak{z}_1 + 30 \eta \operatorname{ep} \mu_1 \mu_2 \\
& \mathfrak{z}_1 + 30 \eta^2 \operatorname{ep} \mu_1 \mu_2 \mathfrak{z}_1 - 10 \mathfrak{z}_2 - 60 \eta \mathfrak{z}_2 - 60 \eta^2 \mathfrak{z}_2 + 11 \operatorname{ep} \\
& \mathfrak{z}_2 + 36 \eta \operatorname{ep} \mathfrak{z}_2 - 30 \eta^2 \operatorname{ep} \mathfrak{z}_2 - 20 \eta^3 \operatorname{ep} \mathfrak{z}_2 + 60 \eta^4 \operatorname{ep} \mathfrak{z}_2 - 8 \\
& \mu_1 \mathfrak{z}_2 - 64 \eta \mu_1 \mathfrak{z}_2 - 164 \eta^2 \mu_1 \mathfrak{z}_2 - 80 \eta^3 \mu_1 \mathfrak{z}_2 + 16 \eta^4 \mu_1 \\
& \mathfrak{z}_2 - 2 \operatorname{ep} \mu_1 \mathfrak{z}_2 - 2 \eta \operatorname{ep} \mu_1 \mathfrak{z}_2 - 33 \eta^2 \operatorname{ep} \mu_1 \mathfrak{z}_2 - 176 \eta^3 \operatorname{ep} \\
& \mu_1 \mathfrak{z}_2 - 160 \eta^4 \operatorname{ep} \mu_1 \mathfrak{z}_2 + 2 \mu_1^2 \mathfrak{z}_2 - 4 \eta \mu_1^2 \mathfrak{z}_2 + 28 \eta^2 \mu_1^2 \\
& \mathfrak{z}_2 + 16 \eta^3 \mu_1^2 \mathfrak{z}_2 + 16 \eta^4 \mu_1^2 \mathfrak{z}_2 - 13 \operatorname{ep} \mu_1^2 \mathfrak{z}_2 - 110 \eta \operatorname{ep} \\
& \mu_1^2 \mathfrak{z}_2 - 219 \eta^2 \operatorname{ep} \mu_1^2 \mathfrak{z}_2 - 156 \eta^3 \operatorname{ep} \mu_1^2 \mathfrak{z}_2 - 40 \eta^4 \operatorname{ep} \mu_1^2 \\
& \mathfrak{z}_2 - 5 \mu_2 \mathfrak{z}_2 - 20 \eta \mu_2 \mathfrak{z}_2 - 15 \eta^2 \mu_2 \mathfrak{z}_2 + 17 \operatorname{ep} \mu_2 \mathfrak{z}_2 + 50 \\
& \eta \operatorname{ep} \mu_2 \mathfrak{z}_2 - 108 \eta^2 \operatorname{ep} \mu_2 \mathfrak{z}_2 - 192 \eta^3 \operatorname{ep} \mu_2 \mathfrak{z}_2 - 20 \eta^4 \operatorname{ep} \\
& \mu_2 \mathfrak{z}_2 + 19 \mu_1 \mu_2 \mathfrak{z}_2 + 76 \eta \mu_1 \mu_2 \mathfrak{z}_2 + 57 \eta^2 \mu_1 \mu_2 \mathfrak{z}_2 - 31 \\
& \operatorname{ep} \mu_1 \mu_2 \mathfrak{z}_2 - 178 \eta \operatorname{ep} \mu_1 \mu_2 \mathfrak{z}_2 - 144 \eta^2 \operatorname{ep} \mu_1 \mu_2 \mathfrak{z}_2 + 120 \\
& \eta^3 \operatorname{ep} \mu_1 \mu_2 \mathfrak{z}_2 + 100 \eta^4 \operatorname{ep} \mu_1 \mu_2 \mathfrak{z}_2 - 5 \operatorname{ep} \mathfrak{z}_1 \mathfrak{z}_2 - 30 \eta \\
& \operatorname{ep} \mathfrak{z}_1 \mathfrak{z}_2 - 30 \eta^2 \operatorname{ep} \mathfrak{z}_1 \mathfrak{z}_2 - 4 \operatorname{ep} \mu_1 \mathfrak{z}_1 \mathfrak{z}_2 - 50 \eta \operatorname{ep} \mu_1 \mathfrak{z}_1 \\
& \mathfrak{z}_2 - 129 \eta^2 \operatorname{ep} \mu_1 \mathfrak{z}_1 \mathfrak{z}_2 - 96 \eta^3 \operatorname{ep} \mu_1 \mathfrak{z}_1 \mathfrak{z}_2 - 10 \eta^4 \operatorname{ep} \\
& \mu_1 \mathfrak{z}_1 \mathfrak{z}_2 + \operatorname{ep} \mu_1^2 \mathfrak{z}_1 \mathfrak{z}_2 - 2 \eta \operatorname{ep} \mu_1^2 \mathfrak{z}_1 \mathfrak{z}_2 - 27 \eta^2 \operatorname{ep} \mu_1^2 \\
& \mathfrak{z}_1 \mathfrak{z}_2 - 36 \eta^3 \operatorname{ep} \mu_1^2 \mathfrak{z}_1 \mathfrak{z}_2 - 10 \eta^4 \operatorname{ep} \mu_1^2 \mathfrak{z}_1 \mathfrak{z}_2 - 5 \operatorname{ep} \mu_2 \\
& \mathfrak{z}_1 \mathfrak{z}_2 - 30 \eta \operatorname{ep} \mu_2 \mathfrak{z}_1 \mathfrak{z}_2 - 30 \eta^2 \operatorname{ep} \mu_2 \mathfrak{z}_1 \mathfrak{z}_2 - 5 \operatorname{ep} \mu_1 \mu_2 \\
& \mathfrak{z}_1 \mathfrak{z}_2 - 30 \eta \operatorname{ep} \mu_1 \mu_2 \mathfrak{z}_1 \mathfrak{z}_2 - 30 \eta^2 \operatorname{ep} \mu_1 \mu_2 \mathfrak{z}_1 \mathfrak{z}_2 + 5 \operatorname{ep} \\
& \mathfrak{z}_2^2 + 30 \eta \operatorname{ep} \mathfrak{z}_2^2 + 30 \eta^2 \operatorname{ep} \mathfrak{z}_2^2 + 4 \operatorname{ep} \mu_1 \mathfrak{z}_2^2 + 40 \eta \operatorname{ep} \mu_1 \\
& \mathfrak{z}_2^2 + 87 \eta^2 \operatorname{ep} \mu_1 \mathfrak{z}_2^2 + 44 \eta^3 \operatorname{ep} \mu_1 \mathfrak{z}_2^2 - 10 \eta^4 \operatorname{ep} \mu_1 \mathfrak{z}_2^2 - \operatorname{ep} \\
& \mu_1^2 \mathfrak{z}_2^2 - 8 \eta \operatorname{ep} \mu_1^2 \mathfrak{z}_2^2 - 15 \eta^2 \operatorname{ep} \mu_1^2 \mathfrak{z}_2^2 - 16 \eta^3 \operatorname{ep} \mu_1^2 \\
& \mathfrak{z}_2^2 - 10 \eta^4 \operatorname{ep} \mu_1^2 \mathfrak{z}_2^2 + 5 \operatorname{ep} \mu_2 \mathfrak{z}_2^2 + 30 \eta \operatorname{ep} \mu_2 \mathfrak{z}_2^2 + 30 \\
& \eta^2 \operatorname{ep} \mu_2 \mathfrak{z}_2^2 - 7 \operatorname{ep} \mu_1 \mu_2 \mathfrak{z}_2^2 - 6 \eta \operatorname{ep} \mu_1 \mu_2 \mathfrak{z}_2^2 + 102 \\
& \eta^2 \operatorname{ep} \mu_1 \mu_2 \mathfrak{z}_2^2 + 120 \eta^3 \operatorname{ep} \mu_1 \mu_2 \mathfrak{z}_2^2 + 2 w^4 (-1 + \eta)^4 \\
& (-1 - 5 \mu_2 + 5 \mu_1 (-2 + \mu_2) \times (-1 + \mathfrak{z}_2) - 5 \mathfrak{z}_2 + 5 \mu_2 \mathfrak{z}_2 + \\
& \mu_1^2 (23 + \mathfrak{z}_2) + \eta (-2 - 5 \mu_2 + \mu_1 (2 + 5 \mu_2 (-1 + \mathfrak{z}_2) - 20 \mathfrak{z}_2) - \\
& 10 \mathfrak{z}_2 + 5 \mu_2 \mathfrak{z}_2 + 4 \mu_1^2 (16 + 5 \mathfrak{z}_2)) - w^3 (-1 + \eta)^3 \\
& (-8 + 80 \mu_1 + 160 \mu_1^2 - 49 \mu_2 - \mu_1 \mu_2 - \operatorname{ep} \mathfrak{z}_1 + 11 \operatorname{ep} \mu_1 \mathfrak{z}_1 + \\
& 24 \operatorname{ep} \mu_1^2 \mathfrak{z}_1 + 5 \operatorname{ep} \mu_2 \mathfrak{z}_1 + 5 \operatorname{ep} \mu_1 \mu_2 \mathfrak{z}_1 - 40 \mathfrak{z}_2 + \operatorname{ep} \mathfrak{z}_2 - 68 \mu_1 \mathfrak{z}_2 - \\
& 11 \operatorname{ep} \mu_1 \mathfrak{z}_2 + 8 \mu_1^2 \mathfrak{z}_2 - 24 \operatorname{ep} \mu_1^2 \mathfrak{z}_2 + 25 \mu_2 \mathfrak{z}_2 - 5 \operatorname{ep} \mu_2 \mathfrak{z}_2 + \\
& 49 \mu_1 \mu_2 \mathfrak{z}_2 - 5 \operatorname{ep} \mu_1 \mu_2 \mathfrak{z}_2 - 5 \operatorname{ep} \mathfrak{z}_1 \mathfrak{z}_2 - 11 \operatorname{ep} \mu_1 \mathfrak{z}_1 \mathfrak{z}_2 - \\
& 5 \operatorname{ep} \mu_2 \mathfrak{z}_1 \mathfrak{z}_2 - 5 \operatorname{ep} \mu_1 \mu_2 \mathfrak{z}_1 \mathfrak{z}_2 + 5 \operatorname{ep} \mathfrak{z}_2^2 + 11 \operatorname{ep} \mu_1 \mathfrak{z}_2^2 + 5 \operatorname{ep} \mu_2 \mathfrak{z}_2^2 + \\
& 5 \operatorname{ep} \mu_1 \mu_2 \mathfrak{z}_2^2 + 3 \eta^2 (4 \mu_1^2 (31 + 12 \operatorname{ep} (\mathfrak{z}_1 - \mathfrak{z}_2) + 3 \mathfrak{z}_2) - \\
& \mu_2 (19 + 10 \operatorname{ep} (\mathfrak{z}_1 - \mathfrak{z}_2) (-1 + \mathfrak{z}_2) + 5 \mathfrak{z}_2) + 2 \times (1 + 5 \mathfrak{z}_2) \times
\end{aligned}$$

$$\begin{aligned}
& (-2 + \theta p (-\mathfrak{x}1 + \mathfrak{x}2)) + \mu1 (32 - 22 \theta p (\mathfrak{x}1 - \mathfrak{x}2) (-1 + \mathfrak{x}2) - \\
& 52 \mathfrak{x}2 + \mu2 (29 - 10 \theta p (\mathfrak{x}1 - \mathfrak{x}2) (-1 + \mathfrak{x}2) + 19 \mathfrak{x}2)) + \\
& 2 \eta (\mu2 (-53 - 15 \theta p (\mathfrak{x}1 - \mathfrak{x}2) (-1 + \mathfrak{x}2) + 5 \mathfrak{x}2) + \mu1^2 \\
& (326 + 72 \theta p (\mathfrak{x}1 - \mathfrak{x}2) + 46 \mathfrak{x}2) + 3 \times (1 + 5 \mathfrak{x}2) \times \\
& (-4 + \theta p (-\mathfrak{x}1 + \mathfrak{x}2)) + \mu1 (86 - 33 \theta p (\mathfrak{x}1 - \mathfrak{x}2) (-1 + \mathfrak{x}2) - \\
& 128 \mathfrak{x}2 + \mu2 (43 - 15 \theta p (\mathfrak{x}1 - \mathfrak{x}2) (-1 + \mathfrak{x}2) + 53 \mathfrak{x}2))) - w^2 \\
& (-1 + \eta)^2 (-3 \times (-4 - 29 \mu2 - 20 \mathfrak{x}2 + 5 \mu2 \mathfrak{x}2 + 4 \mu1^2 (17 + \mathfrak{x}2) + \\
& \mu1 (40 - 28 \mathfrak{x}2 + \mu2 (19 + 29 \mathfrak{x}2))) + \theta p (2 + 3 \mathfrak{x}1 - 17 \mathfrak{x}2 + \\
& 15 \mathfrak{x}1 \mathfrak{x}2 - 15 \mathfrak{x}2^2 + \mu2 (-34 + 15 \mathfrak{x}1 (-1 + \mathfrak{x}2) - 11 \mathfrak{x}2 - 15 \mathfrak{x}2^2) + \\
& \mu1^2 (48 + 59 \mathfrak{x}2 + \mathfrak{x}2^2 - \mathfrak{x}1 (59 + \mathfrak{x}2)) + \mu1 (26 - 32 \mathfrak{x}1 + 6 \mathfrak{x}2 + \\
& 26 \mathfrak{x}1 \mathfrak{x}2 - 26 \mathfrak{x}2^2 + \mu2 (62 + 15 \mathfrak{x}1 (-1 + \mathfrak{x}2) + 61 \mathfrak{x}2 - 3 \mathfrak{x}2^2))) + \\
& 3 \eta^2 (3 \times (4 + 19 \mu2 + 20 \mathfrak{x}2 + 5 \mu2 \mathfrak{x}2 - 4 \mu1^2 (31 + 3 \mathfrak{x}2) - \\
& \mu1 (32 + 29 \mu2 - 52 \mathfrak{x}2 + 19 \mu2 \mathfrak{x}2)) + \\
& 2 \theta p (\mu1^2 (-56 + 89 \mathfrak{x}2 + 3 \mathfrak{x}2^2 + \mathfrak{x}1 (-89 + 5 \mathfrak{x}2)) + \\
& \mu1 (-26 - 38 \mathfrak{x}1 + 56 \mathfrak{x}2 + 44 \mathfrak{x}1 \mathfrak{x}2 - 36 \mathfrak{x}2^2 + 3 \mu2 \\
& (-2 + 5 \mathfrak{x}1 (-1 + \mathfrak{x}2) + 3 \mathfrak{x}2 - 9 \mathfrak{x}2^2)) + 3 \times (2 + \mathfrak{x}1 + \mathfrak{x}2 + 5 \\
& \mathfrak{x}1 \mathfrak{x}2 - 5 \mathfrak{x}2^2 + \mu2 (-2 + 5 \mathfrak{x}1 (-1 + \mathfrak{x}2) + 11 \mathfrak{x}2 - 5 \mathfrak{x}2^2))) + \\
& 3 \eta (16 + 86 \mu2 + 80 \mathfrak{x}2 + 10 \mu2 \mathfrak{x}2 - 4 \mu1^2 (89 + 5 \mathfrak{x}2) - \\
& 2 \mu1 (78 - 76 \mathfrak{x}2 + \mu2 (53 + 43 \mathfrak{x}2)) + \\
& \theta p (\mu1^2 (44 + \mathfrak{x}1 (-133 + \mathfrak{x}2) + 133 \mathfrak{x}2 + 3 \mathfrak{x}2^2) + 6 \times (1 + \mathfrak{x}1 - \\
& 4 \mathfrak{x}2 + 5 \mathfrak{x}1 \mathfrak{x}2 - 5 \mathfrak{x}2^2 + \mu2 (-9 + 5 \mathfrak{x}1 (-1 + \mathfrak{x}2) - 5 \mathfrak{x}2^2)) + \\
& \mu1 (26 - 67 \mathfrak{x}1 + 37 \mathfrak{x}2 + 61 \mathfrak{x}1 \mathfrak{x}2 - 57 \mathfrak{x}2^2 + 6 \mu2 \\
& (15 + 5 \mathfrak{x}1 (-1 + \mathfrak{x}2) + 16 \mathfrak{x}2 - 3 \mathfrak{x}2^2)))) + 2 \eta^3 \\
& (-8 \mu1 (-1 - 5 \mathfrak{x}2 + \mu1 (11 + \mathfrak{x}2)) + 5 \theta p (\mu1^2 (-52 + 3 \mathfrak{x}1 (-5 + \mathfrak{x}2) + \\
& 15 \mathfrak{x}2 + \mathfrak{x}2^2) + 2 \times (1 + 5 \mathfrak{x}2 + \mu2 (7 + 11 \mathfrak{x}2)) - \mu1 (26 + 3 \mathfrak{x}1 - \\
& 25 \mathfrak{x}2 - 9 \mathfrak{x}1 \mathfrak{x}2 + 5 \mathfrak{x}2^2 + 2 \mu2 (17 + 13 \mathfrak{x}2 + 6 \mathfrak{x}2^2)))) + \\
& w (-1 + \eta) \times (8 - 80 \mu1 - 112 \mu1^2 + 67 \mu2 - 77 \mu1 \mu2 + 40 \mathfrak{x}2 + \\
& 44 \mu1 \mathfrak{x}2 - 8 \mu1^2 \mathfrak{x}2 + 5 \mu2 \mathfrak{x}2 - 67 \mu1 \mu2 \mathfrak{x}2 + \theta p ((-4 + 3 \mathfrak{x}1 - 3 \mathfrak{x}2) \times \\
& (1 + 5 \mathfrak{x}2) + 3 \mu2 (-16 + 5 \mathfrak{x}1 (-1 + \mathfrak{x}2) - 11 \mathfrak{x}2 - 5 \mathfrak{x}2^2) + \\
& 2 \mu1^2 (35 + 24 \mathfrak{x}2 + \mathfrak{x}2^2 - \mathfrak{x}1 (23 + \mathfrak{x}2)) + \mu1 (42 - 31 \mathfrak{x}1 + \mathfrak{x}2 + \\
& 19 \mathfrak{x}1 \mathfrak{x}2 - 19 \mathfrak{x}2^2 + 3 \mu2 (32 + 5 \mathfrak{x}1 (-1 + \mathfrak{x}2) + 29 \mathfrak{x}2 + 3 \mathfrak{x}2^2))) + \\
& 2 \eta^4 (10 \theta p \mu2 (5 + \mathfrak{x}2) + \mu1^2 (8 - 8 \mathfrak{x}2 + 5 \theta p (-41 + \mathfrak{x}1 \\
& (-1 + \mathfrak{x}2) + 4 \mathfrak{x}2 + \mathfrak{x}2^2)) + \mu1 (8 - 8 \mathfrak{x}2 + 5 \theta p \\
& (-5 + \mathfrak{x}1 (-1 + \mathfrak{x}2) + 22 \mathfrak{x}2 + \mathfrak{x}2^2 - 2 \mu2 (7 + 5 \mathfrak{x}2)))) + \\
& \eta^2 (-4 \mu1^2 (281 + 25 \mathfrak{x}2) + 9 \times (4 + 20 \mathfrak{x}2 + \mu2 (19 + 5 \mathfrak{x}2)) - \\
& \mu1 (296 - 476 \mathfrak{x}2 + 9 \mu2 (29 + 19 \mathfrak{x}2)) + 3 \theta p \\
& (\mu1^2 (-118 + 203 \mathfrak{x}2 + 11 \mathfrak{x}2^2 + \mathfrak{x}1 (-211 + 19 \mathfrak{x}2)) + \mu1 (-78 - 85 \\
& \mathfrak{x}1 + 85 \mathfrak{x}2 + 109 \mathfrak{x}1 \mathfrak{x}2 - 79 \mathfrak{x}2^2 + \mu2 (46 + 30 \mathfrak{x}1 (-1 + \mathfrak{x}2) + \\
& 56 \mathfrak{x}2 - 78 \mathfrak{x}2^2)) + 2 \times (20 + 3 \mathfrak{x}1 + \mathfrak{x}2 + 15 \mathfrak{x}1 \mathfrak{x}2 - 15 \mathfrak{x}2^2 + \\
& \mu2 (-37 + 15 \mathfrak{x}1 (-1 + \mathfrak{x}2) + 46 \mathfrak{x}2 - 15 \mathfrak{x}2^2))) + \\
& \eta (40 + 238 \mu2 + 200 \mathfrak{x}2 + 50 \mu2 \mathfrak{x}2 - 4 \mu1^2 (173 + \mathfrak{x}2) - \\
& 2 \mu1 (218 + 169 \mu2 - 152 \mathfrak{x}2 + 119 \mu2 \mathfrak{x}2) + \\
& \theta p (\mu1^2 (266 + 5 \mathfrak{x}1 (-73 + \mathfrak{x}2) + 365 \mathfrak{x}2 + 17 \mathfrak{x}2^2) +
\end{aligned}$$

$$\begin{aligned}
& 2 \times (6 + 9 \mathfrak{x}1 - 51 \mathfrak{x}2 + 45 \mathfrak{x}1 \mathfrak{x}2 - 45 \mathfrak{x}2^2 + \\
& \quad \mu2 (-137 + 45 \mathfrak{x}1 (-1 + \mathfrak{x}2) - 40 \mathfrak{x}2 - 45 \mathfrak{x}2^2)) + \\
& \quad \mu1 (134 - 203 \mathfrak{x}1 + 47 \mathfrak{x}2 + 167 \mathfrak{x}1 \mathfrak{x}2 - 145 \mathfrak{x}2^2 + \\
& \quad \quad 2 \mu2 (235 + 45 \mathfrak{x}1 (-1 + \mathfrak{x}2) + 218 \mathfrak{x}2 - 9 \mathfrak{x}2^2)) + \\
& 2 \eta^3 (-16 \mu1 (-1 - 5 \mathfrak{x}2 + \mu1 (11 + \mathfrak{x}2)) + \Theta p (60 + 70 \mu2 + 60 \mathfrak{x}2 + \\
& \quad 206 \mu2 \mathfrak{x}2 + \mu1^2 (-526 + 153 \mathfrak{x}2 + 13 \mathfrak{x}2^2 + 3 \mathfrak{x}1 (-51 + 11 \mathfrak{x}2)) - \\
& \quad \mu1 (226 + 33 \mathfrak{x}1 - 213 \mathfrak{x}2 - 93 \mathfrak{x}1 \mathfrak{x}2 + 47 \mathfrak{x}2^2 + \\
& \quad \quad 2 \mu2 (121 + 95 \mathfrak{x}2 + 60 \mathfrak{x}2^2)))))) + \\
& x^5 (-1 + \eta)^5 (-4 \times (-1 + w (-1 + \eta)) \times (-1 + \eta t) \Theta l \mu1 (1 - 11 \mu1 - \eta \\
& \quad (1 + \mu1) \times (-1 + \mathfrak{x}2) + 5 \mathfrak{x}2 - \mu1 \mathfrak{x}2 + w \\
& \quad (-1 + \eta) \times (-1 - 5 \mathfrak{x}2 + \mu1 (11 + \mathfrak{x}2))) + \\
& \Theta p (10 + 6 \eta - 40 \eta^2 + 24 \eta^3 + 8 \eta t + 16 \eta \eta t - 24 \eta^2 \eta t - 10 \Theta l - 24 \eta \\
& \quad \Theta l + 10 \eta t \Theta l + 24 \eta \eta t \Theta l - 32 \mu1 - 12 \eta \mu1 + 20 \eta^2 \mu1 + 24 \\
& \quad \eta^3 \mu1 + 8 \eta t \mu1 + 16 \eta \eta t \mu1 - 24 \eta^2 \eta t \mu1 + 18 \Theta l \mu1 - 10 \\
& \quad \eta \Theta l \mu1 - 18 \eta t \Theta l \mu1 + 10 \eta \eta t \Theta l \mu1 - 90 \mu1^2 - 114 \eta \\
& \quad \mu1^2 + 204 \eta^2 \mu1^2 + 52 \Theta l \mu1^2 + 158 \eta \Theta l \mu1^2 - 52 \eta t \Theta l \\
& \quad \mu1^2 - 158 \eta \eta t \Theta l \mu1^2 - 6 \mu2 + 30 \eta \mu2 - 24 \eta^2 \mu2 - 12 \eta t \\
& \quad \mu2 + 12 \eta \eta t \mu2 + 6 \Theta l \mu2 - 10 \eta \Theta l \mu2 - 6 \eta t \Theta l \mu2 + 10 \eta \\
& \quad \eta t \Theta l \mu2 - 30 \mu1 \mu2 + 6 \eta \mu1 \mu2 + 24 \eta^2 \mu1 \mu2 + 12 \eta t \mu1 \\
& \quad \mu2 - 12 \eta \eta t \mu1 \mu2 + 6 \Theta l \mu1 \mu2 + 14 \eta \Theta l \mu1 \mu2 - 6 \eta t \Theta l \\
& \quad \mu1 \mu2 - 14 \eta \eta t \Theta l \mu1 \mu2 + 3 \Theta l \mu1 \mathfrak{x}1 + \eta \Theta l \mu1 \mathfrak{x}1 - 3 \eta t \\
& \quad \Theta l \mu1 \mathfrak{x}1 - \eta \eta t \Theta l \mu1 \mathfrak{x}1 + 15 \Theta l \mu1^2 \mathfrak{x}1 + \eta \Theta l \mu1^2 \mathfrak{x}1 - 15 \\
& \quad \eta t \Theta l \mu1^2 \mathfrak{x}1 - \eta \eta t \Theta l \mu1^2 \mathfrak{x}1 + 4 w^3 (-1 + \eta)^4 (1 + \mu1) \\
& \quad (\eta - \eta t + 4 \mu1) (-1 + \mathfrak{x}2) + 2 \mathfrak{x}2 - 18 \eta \mathfrak{x}2 + 40 \eta^2 \mathfrak{x}2 - 24 \\
& \quad \eta^3 \mathfrak{x}2 - 8 \eta t \mathfrak{x}2 - 16 \eta \eta t \mathfrak{x}2 + 24 \eta^2 \eta t \mathfrak{x}2 - 2 \Theta l \mathfrak{x}2 + 24 \\
& \quad \eta \Theta l \mathfrak{x}2 + 2 \eta t \Theta l \mathfrak{x}2 - 24 \eta \eta t \Theta l \mathfrak{x}2 + 44 \mu1 \mathfrak{x}2 + 72 \eta \mu1 \\
& \quad \mathfrak{x}2 - 92 \eta^2 \mu1 \mathfrak{x}2 - 24 \eta^3 \mu1 \mathfrak{x}2 - 8 \eta t \mu1 \mathfrak{x}2 - 16 \eta \eta t \mu1 \\
& \quad \mathfrak{x}2 + 24 \eta^2 \eta t \mu1 \mathfrak{x}2 - 17 \Theta l \mu1 \mathfrak{x}2 - 61 \eta \Theta l \mu1 \mathfrak{x}2 + 17 \eta t \\
& \quad \Theta l \mu1 \mathfrak{x}2 + 61 \eta \eta t \Theta l \mu1 \mathfrak{x}2 + 18 \mu1^2 \mathfrak{x}2 + 42 \eta \mu1^2 \mathfrak{x}2 - 60 \\
& \quad \eta^2 \mu1^2 \mathfrak{x}2 - 15 \Theta l \mu1^2 \mathfrak{x}2 - 13 \eta \Theta l \mu1^2 \mathfrak{x}2 + 15 \eta t \Theta l \mu1^2 \\
& \quad \mathfrak{x}2 + 13 \eta \eta t \Theta l \mu1^2 \mathfrak{x}2 + 18 \mu2 \mathfrak{x}2 - 18 \eta \mu2 \mathfrak{x}2 - 18 \Theta l \mu2 \\
& \quad \mathfrak{x}2 - 2 \eta \Theta l \mu2 \mathfrak{x}2 + 18 \eta t \Theta l \mu2 \mathfrak{x}2 + 2 \eta \eta t \Theta l \mu2 \mathfrak{x}2 + 6 \mu1 \\
& \quad \mu2 \mathfrak{x}2 - 30 \eta \mu1 \mu2 \mathfrak{x}2 + 24 \eta^2 \mu1 \mu2 \mathfrak{x}2 + 12 \eta t \mu1 \mu2 \mathfrak{x}2 - 12 \\
& \quad \eta \eta t \mu1 \mu2 \mathfrak{x}2 + 6 \Theta l \mu1 \mu2 \mathfrak{x}2 + 10 \eta \Theta l \mu1 \mu2 \mathfrak{x}2 - 6 \eta t \Theta l \\
& \quad \mu1 \mu2 \mathfrak{x}2 - 10 \eta \eta t \Theta l \mu1 \mu2 \mathfrak{x}2 - 9 \Theta l \mu1 \mathfrak{x}1 \mathfrak{x}2 - \eta \Theta l \mu1 \\
& \quad \mathfrak{x}1 \mathfrak{x}2 + 9 \eta t \Theta l \mu1 \mathfrak{x}1 \mathfrak{x}2 + \eta \eta t \Theta l \mu1 \mathfrak{x}1 \mathfrak{x}2 - 3 \Theta l \mu1^2 \mathfrak{x}1 \\
& \quad \mathfrak{x}2 - \eta \Theta l \mu1^2 \mathfrak{x}1 \mathfrak{x}2 + 3 \eta t \Theta l \mu1^2 \mathfrak{x}1 \mathfrak{x}2 + \eta \eta t \Theta l \mu1^2 \mathfrak{x}1 \\
& \quad \mathfrak{x}2 + 5 \Theta l \mu1 \mathfrak{x}2^2 - \eta \Theta l \mu1 \mathfrak{x}2^2 - 5 \eta t \Theta l \mu1 \mathfrak{x}2^2 + \eta \eta t \Theta l \mu1 \\
& \quad \mathfrak{x}2^2 - \Theta l \mu1^2 \mathfrak{x}2^2 - \eta \Theta l \mu1^2 \mathfrak{x}2^2 + \eta t \Theta l \mu1^2 \mathfrak{x}2^2 + \eta \eta t \Theta l \mu1^2 \\
& \quad \mathfrak{x}2^2 + 12 \Theta l \mu1 \mu2 \mathfrak{x}2^2 - 12 \eta t \Theta l \mu1 \mu2 \mathfrak{x}2^2 - w^2 (-1 + \eta)^2 \\
& \quad (-2 + 2 \Theta l + 72 \mu1 - 26 \Theta l \mu1 + 122 \mu1^2 - 52 \Theta l \mu1^2 - 14 \mu2 + \\
& \quad 14 \Theta l \mu2 + 58 \mu1 \mu2 - 34 \Theta l \mu1 \mu2 - 3 \Theta l \mu1 \mathfrak{x}1 - 15 \Theta l \mu1^2 \mathfrak{x}1 + \\
& \quad 12 \eta^3 (1 + \mu1) \times (-1 + \mathfrak{x}2) - 10 \mathfrak{x}2 + 10 \Theta l \mathfrak{x}2 - 84 \mu1 \mathfrak{x}2 + 25 \Theta l \mu1 \mathfrak{x}2 - \\
& \quad 50 \mu1^2 \mathfrak{x}2 + 15 \Theta l \mu1^2 \mathfrak{x}2 - 22 \mu2 \mathfrak{x}2 + 22 \Theta l \mu2 \mathfrak{x}2 + 14 \mu1 \mu2 \mathfrak{x}2 - \\
& \quad 26 \Theta l \mu1 \mu2 \mathfrak{x}2 + 9 \Theta l \mu1 \mathfrak{x}1 \mathfrak{x}2 + 3 \Theta l \mu1^2 \mathfrak{x}1 \mathfrak{x}2 - 5 \Theta l \mu1 \mathfrak{x}2^2 + \\
& \quad \Theta l \mu1^2 \mathfrak{x}2^2 - 12 \Theta l \mu1 \mu2 \mathfrak{x}2^2 - 4 \eta^2 (1 - 3 \mu2 - 12 \mu1^2 (-1 + \mathfrak{x}2)) +
\end{aligned}$$

$$\begin{aligned}
& 3 \eta t (1 + \mu_1) \times (-1 + \mathfrak{z}_2) - \mathfrak{z}_2 + \mu_1 (13 + 3 \mu_2 - 13 \mathfrak{z}_2 + 3 \mu_2 \mathfrak{z}_2) + \\
& 2 \eta (9 + \mu_2 + \mu_1^2 (-37 + \mathfrak{z}_2) - 3 \mathfrak{z}_2 + 11 \mu_2 \mathfrak{z}_2 + 2 \eta t (1 + \mu_1 - 3 \mu_2 - \\
& \mathfrak{z}_2 - \mu_1 \mathfrak{z}_2 + 3 \mu_1 \mu_2 (1 + \mathfrak{z}_2)) - \mu_1 (4 - 10 \mathfrak{z}_2 + \mu_2 (23 + \mathfrak{z}_2))) - \\
& \eta t (4 \times (4 - 3 \mu_2 - 4 \mathfrak{z}_2 + \mu_1 (4 - 4 \mathfrak{z}_2 + 3 \mu_2 (1 + \mathfrak{z}_2))) + \\
& \mathfrak{el} (\mu_1^2 (-52 + 3 \mathfrak{z}_1 (-5 + \mathfrak{z}_2) + 15 \mathfrak{z}_2 + \mathfrak{z}_2^2) + \\
& 2 \times (1 + 5 \mathfrak{z}_2 + \mu_2 (7 + 11 \mathfrak{z}_2)) - \mu_1 (26 + 3 \mathfrak{z}_1 - 25 \mathfrak{z}_2 - 9 \mathfrak{z}_1 \mathfrak{z}_2 + \\
& 5 \mathfrak{z}_2^2 + 2 \mu_2 (17 + 13 \mathfrak{z}_2 + 6 \mathfrak{z}_2^2))) + w (-1 + \eta) \times \\
& (36 \eta^3 (1 + \mu_1) \times (-1 + \mathfrak{z}_2) - 4 \eta^2 (-4 - 9 \mu_2 + 9 \eta t (1 + \mu_1) \times (-1 + \\
& \mathfrak{z}_2) + 4 \mathfrak{z}_2 - 9 \mu_1^2 (-7 + 3 \mathfrak{z}_2) + \mu_1 (23 - 41 \mathfrak{z}_2 + 9 \mu_2 (1 + \mathfrak{z}_2))) + \\
& \eta (-8 \times (-4 + \mathfrak{z}_2) + 2 \mu_2 (-14 + 20 \mathfrak{z}_2 + \mathfrak{el} (5 + \mathfrak{z}_2)) + \\
& \mu_1^2 (-56 \times (-1 + \mathfrak{z}_2) + \mathfrak{el} (-158 + \mathfrak{z}_1 (-1 + \mathfrak{z}_2) + 13 \mathfrak{z}_2 + \mathfrak{z}_2^2)) + \\
& \mu_1 (40 - 52 \mu_2 - 88 \mathfrak{z}_2 + 28 \mu_2 \mathfrak{z}_2 + \mathfrak{el} (-14 + \mathfrak{z}_1 (-1 + \mathfrak{z}_2) + 85 \mathfrak{z}_2 + \\
& \mathfrak{z}_2^2 - 2 \mu_2 (7 + 5 \mathfrak{z}_2))) - \eta t (\mathfrak{el} \mu_1^2 (-158 + \mathfrak{z}_1 (-1 + \mathfrak{z}_2) + \\
& 13 \mathfrak{z}_2 + \mathfrak{z}_2^2) + 2 \times (8 - 8 \mathfrak{z}_2 + \mu_2 (12 + \mathfrak{el} (5 + \mathfrak{z}_2))) - \\
& \mu_1 (8 \times (2 \times (-1 + \mathfrak{z}_2) + 3 \mu_2 (1 + \mathfrak{z}_2)) + \mathfrak{el} \\
& (14 + \mathfrak{z}_1 - 85 \mathfrak{z}_2 - \mathfrak{z}_1 \mathfrak{z}_2 - \mathfrak{z}_2^2 + 2 \mu_2 (7 + 5 \mathfrak{z}_2)))) - \\
& 2 \times (6 - 44 \mu_1 - 98 \mu_1^2 + 4 \mu_2 - 44 \mu_1 \mu_2 + 6 \mathfrak{z}_2 + 56 \mu_1 \mathfrak{z}_2 + \\
& 26 \mu_1^2 \mathfrak{z}_2 + 20 \mu_2 \mathfrak{z}_2 - 4 \mu_1 \mu_2 \mathfrak{z}_2 - \mathfrak{el} (6 + 4 \mu_2 + 6 \mathfrak{z}_2 + \\
& 20 \mu_2 \mathfrak{z}_2 + \mu_1^2 (-52 + 3 \mathfrak{z}_1 (-5 + \mathfrak{z}_2) + 15 \mathfrak{z}_2 + \mathfrak{z}_2^2) - \mu_1 \\
& (22 + 3 \mathfrak{z}_1 - 21 \mathfrak{z}_2 - 9 \mathfrak{z}_1 \mathfrak{z}_2 + 5 \mathfrak{z}_2^2 + 4 \mu_2 (5 + 4 \mathfrak{z}_2 + 3 \mathfrak{z}_2^2))) + \\
& \eta t (2 \times (5 - 6 \mu_2 - 5 \mathfrak{z}_2 + \mu_1 (5 - 5 \mathfrak{z}_2 + 6 \mu_2 (1 + \mathfrak{z}_2))) + \\
& \mathfrak{el} (6 + 4 \mu_2 + 6 \mathfrak{z}_2 + 20 \mu_2 \mathfrak{z}_2 + \mu_1^2 (-52 + 3 \mathfrak{z}_1 (-5 + \mathfrak{z}_2) + \\
& 15 \mathfrak{z}_2 + \mathfrak{z}_2^2) - \mu_1 (22 + 3 \mathfrak{z}_1 - 21 \mathfrak{z}_2 - 9 \mathfrak{z}_1 \mathfrak{z}_2 + \\
& 5 \mathfrak{z}_2^2 + 4 \mu_2 (5 + 4 \mathfrak{z}_2 + 3 \mathfrak{z}_2^2)))))) - \\
& \times (-1 + \eta) \times (4 w^2 (3 - 5 w + 2 w^2) \eta^9 \mathfrak{op} (1 + \mu_1) \times (-1 + \mathfrak{z}_2) - 4 w \eta^8 \mathfrak{op} \\
& (9 \times (1 + \mu_1) \times (-1 + \mathfrak{z}_2) + w^3 (-7 + \mu_1 - 9 \mu_2 - 8 \mu_1^2 (-1 + \mathfrak{z}_2) + \\
& 2 \eta t (1 + \mu_1) \times (-1 + \mathfrak{z}_2) + 7 \mathfrak{z}_2 - \mu_1 \mathfrak{z}_2 + 9 \mu_1 \mu_2 (1 + \mathfrak{z}_2)) + w \\
& (11 - 15 \mu_2 - 23 \mu_1 (-1 + \mathfrak{z}_2) - 12 \mu_1^2 (-1 + \mathfrak{z}_2) + \\
& 3 \eta t (1 + \mu_1) \times (-1 + \mathfrak{z}_2) - 11 \mathfrak{z}_2 + 15 \mu_1 \mu_2 (1 + \mathfrak{z}_2)) + w^2 \\
& (6 + 24 \mu_2 + 20 \mu_1^2 (-1 + \mathfrak{z}_2) - 5 \eta t (1 + \mu_1) \times (-1 + \mathfrak{z}_2) - \\
& 6 \mathfrak{z}_2 - 2 \mu_1 (7 - 7 \mathfrak{z}_2 + 12 \mu_2 (1 + \mathfrak{z}_2)))) - \\
& (1 + w)^3 (5 w \mathfrak{el} (1 + \mu_1) \mu_2 (-1 + \mathfrak{z}_2) - 5 w \eta t \mathfrak{el} (1 + \mu_1) \mu_2 \\
& (-1 + \mathfrak{z}_2) + \eta t \mathfrak{op} (-2 - 19 \mu_2 - 10 \mathfrak{z}_2 - 5 \mu_2 \mathfrak{z}_2 + 2 \mu_1^2 (11 + \mathfrak{z}_2) + \\
& 2 w (-1 + \mu_1 (4 + 5 \mu_2 (-1 + \mathfrak{z}_2) - 10 \mathfrak{z}_2) + 5 \mu_2 (-1 + \mathfrak{z}_2) - \\
& 5 \mathfrak{z}_2 + \mu_1^2 (29 + 7 \mathfrak{z}_2)) + \mu_1 (20 - 8 \mathfrak{z}_2 + \mu_2 (29 + 19 \mathfrak{z}_2))) + \\
& 2 \eta^7 \mathfrak{op} (12 \times (1 + \mu_1) \times (-1 + \mathfrak{z}_2) + 2 w (7 - 45 \mu_2 + 9 \eta t (1 + \mu_1) \times (-1 + \mathfrak{z}_2) - \\
& 7 \mathfrak{z}_2 - 9 \mu_1^2 (-7 + 3 \mathfrak{z}_2) + \mu_1 (34 - 52 \mathfrak{z}_2 + 45 \mu_2 (1 + \mathfrak{z}_2))) + w^2 \\
& (47 + 113 \mu_2 - 17 \mathfrak{z}_2 + 55 \mu_2 \mathfrak{z}_2 + \mu_1^2 (-233 + 53 \mathfrak{z}_2) - \\
& \mu_1 (66 + 223 \mu_2 - 96 \mathfrak{z}_2 + 113 \mu_2 \mathfrak{z}_2) + \\
& \eta t (22 - 30 \mu_2 - 22 \mu_1 (-1 + \mathfrak{z}_2) - 22 \mathfrak{z}_2 + 30 \mu_1 \mu_2 (1 + \mathfrak{z}_2))) + w^4 \\
& (-9 - 57 \mu_2 + \mu_1^2 (23 - 59 \mathfrak{z}_2) + 27 \mathfrak{z}_2 + 33 \mu_2 \mathfrak{z}_2 + \\
& 2 \eta t (-7 - 9 \mu_2 + 7 \mu_1 (-1 + \mathfrak{z}_2) + 7 \mathfrak{z}_2 + 9 \mu_1 \mu_2 (1 + \mathfrak{z}_2)) +
\end{aligned}$$

$$\begin{aligned}
& \mu_1 (14 - 32 \mathfrak{z}^2 + \mu_2 (-9 + 57 \mathfrak{z}^2)) - 2 w^3 (18 - 23 \mu_2 + 6 \mathfrak{z}^2 + \\
& 44 \mu_2 \mathfrak{z}^2 - 2 \mu_1^2 (19 + 17 \mathfrak{z}^2) + \mu_1 (4 - 65 \mu_2 - 16 \mathfrak{z}^2 + 23 \mu_2 \mathfrak{z}^2) + \\
& 6 \eta t (-1 - 4 \mu_2 + \mathfrak{z}^2 + \mu_1 (-1 + \mathfrak{z}^2 + 4 \mu_2 (1 + \mathfrak{z}^2))) - \\
& \eta (\theta p (2 w^3 (\eta t (10 + \mu_2 - \mu_1 \mu_2 (-97 + \mathfrak{z}^2) + 6 \mu_1 (-8 + \mathfrak{z}^2) + 14 \mathfrak{z}^2 - \\
& 49 \mu_2 \mathfrak{z}^2 + 2 \mu_1^2 (-11 + 5 \mathfrak{z}^2)) + 2 \times (4 + 5 \mu_1^2 (-13 + \mathfrak{z}^2) + \\
& 20 \mathfrak{z}^2 + 6 \mu_2 (-1 + 5 \mathfrak{z}^2) + \mu_1 (-49 + 6 \mu_2 (-9 + \mathfrak{z}^2) + 31 \mathfrak{z}^2))) + \\
& \eta t (6 \mu_1^2 (25 + 3 \mathfrak{z}^2) - 10 \times (1 + 5 \mathfrak{z}^2) - 3 \mu_2 (19 + 5 \mathfrak{z}^2) + \\
& \mu_1 (92 - 56 \mathfrak{z}^2 + \mu_2 (87 + 57 \mathfrak{z}^2))) - \\
& 2 w^4 (\eta t (-5 - 8 \mu_2 + 4 \mu_1 (7 + 2 \mu_2 (-4 + \mathfrak{z}^2) - 7 \mathfrak{z}^2) - 13 \mathfrak{z}^2 + \\
& 20 \mu_2 \mathfrak{z}^2 + 3 \mu_1^2 (23 + \mathfrak{z}^2)) - 2 \times (1 - 5 \mu_2 + 3 \mu_1^2 (-5 + \mathfrak{z}^2) + \\
& 5 \mathfrak{z}^2 + 11 \mu_2 \mathfrak{z}^2 + \mu_1 (-14 - 17 \mu_2 + 8 \mathfrak{z}^2 + 5 \mu_2 \mathfrak{z}^2))) + \\
& w^2 (-4 \times (-7 + 72 \mu_1^2 + 7 \mu_2 - 23 \mathfrak{z}^2 - 25 \mu_2 \mathfrak{z}^2 + \mu_1 (53 + 43 \mu_2 - \\
& 29 \mathfrak{z}^2 - 7 \mu_2 \mathfrak{z}^2)) + \eta t (-4 - 101 \mu_2 - 68 \mathfrak{z}^2 - 91 \mu_2 \mathfrak{z}^2 + \\
& \mu_1^2 (476 + 76 \mathfrak{z}^2) + \mu_1 (64 + 283 \mu_2 - 196 \mathfrak{z}^2 + 101 \mu_2 \mathfrak{z}^2))) + \\
& 4 w (-2 \times (1 + \mu_1) \times (-1 + 3 \mu_2 - 5 \mathfrak{z}^2 - 3 \mu_2 \mathfrak{z}^2 + \mu_1 (11 + \mathfrak{z}^2)) + \\
& \eta t (\mu_1^2 (133 + 17 \mathfrak{z}^2) - 6 \times (1 + 5 \mathfrak{z}^2 + 2 \mu_2 (3 + \mathfrak{z}^2)) + \\
& \mu_1 (49 - 52 \mathfrak{z}^2 + 12 \mu_2 (5 + 3 \mathfrak{z}^2)))) + \\
& (-1 + \eta t) \theta l (2 - 20 \mu_1 - 22 \mu_1^2 + 19 \mu_2 - 29 \mu_1 \mu_2 + 10 \mathfrak{z}^2 + \\
& 8 \mu_1 \mathfrak{z}^2 - 2 \mu_1^2 \mathfrak{z}^2 + 5 \mu_2 \mathfrak{z}^2 - 19 \mu_1 \mu_2 \mathfrak{z}^2 + \\
& 2 w^4 (1 + \mu_1) \times (1 + 5 \mu_2 (-1 + \mathfrak{z}^2) + 5 \mathfrak{z}^2 + \mu_1 (-17 + 5 \mathfrak{z}^2)) - \\
& 2 w^3 (2 \mu_1^2 (31 + 12 \theta p (\mathfrak{z}^1 - \mathfrak{z}^2) - 7 \mathfrak{z}^2) - \\
& \mu_2 (2 + 5 \theta p (\mathfrak{z}^1 - \mathfrak{z}^2) (-1 + \mathfrak{z}^2) + 10 \mathfrak{z}^2) + \\
& \mu_1 (58 - 11 \theta p (\mathfrak{z}^1 - \mathfrak{z}^2) (-1 + \mathfrak{z}^2) - 5 \theta p \mu_2 (\mathfrak{z}^1 - \mathfrak{z}^2) (-1 + \mathfrak{z}^2) - \\
& 34 \mathfrak{z}^2 + 2 \mu_2 (11 + \mathfrak{z}^2)) + (1 + 5 \mathfrak{z}^2) \times (-4 + \theta p (-\mathfrak{z}^1 + \mathfrak{z}^2))) - \\
& 2 \theta p (\mu_1^2 (-2 + \mathfrak{z}^1 - \mathfrak{z}^2) \times (11 + \mathfrak{z}^2) - (-2 + \mathfrak{z}^1 - \mathfrak{z}^2) \times (1 + 5 \mathfrak{z}^2) + \\
& \mu_2 (14 + 5 \mathfrak{z}^1 + 17 \mathfrak{z}^2 - 5 \mathfrak{z}^1 \mathfrak{z}^2 + 5 \mathfrak{z}^2^2) - \mu_1 (2 \times (-2 + \mathfrak{z}^1 - \mathfrak{z}^2) \times \\
& (-5 + 2 \mathfrak{z}^2) + \mu_2 (34 + 5 \mathfrak{z}^1 (-1 + \mathfrak{z}^2) + 31 \mathfrak{z}^2 + 7 \mathfrak{z}^2^2))) + \\
& w^2 (3 \times (4 + 8 \mu_1^2 (-7 + \mathfrak{z}^2) + 20 \mathfrak{z}^2 + \mu_2 (19 + 5 \mathfrak{z}^2) - \mu_1 \\
& (52 - 28 \mathfrak{z}^2 + \mu_2 (29 + 19 \mathfrak{z}^2))) - 2 \theta p (-2 - 3 \mathfrak{z}^1 + 17 \mathfrak{z}^2 - \\
& 15 \mathfrak{z}^1 \mathfrak{z}^2 + 15 \mathfrak{z}^2^2 + \mu_2 (34 - 15 \mathfrak{z}^1 (-1 + \mathfrak{z}^2) + 11 \mathfrak{z}^2 + 15 \mathfrak{z}^2^2) + \\
& \mu_1^2 (-48 - 59 \mathfrak{z}^2 - \mathfrak{z}^2^2 + \mathfrak{z}^1 (59 + \mathfrak{z}^2)) - \\
& \mu_1 (26 - 32 \mathfrak{z}^1 + 6 \mathfrak{z}^2 + 26 \mathfrak{z}^1 \mathfrak{z}^2 - 26 \mathfrak{z}^2^2 + \\
& \mu_2 (62 + 15 \mathfrak{z}^1 (-1 + \mathfrak{z}^2) + 61 \mathfrak{z}^2 - 3 \mathfrak{z}^2^2))) - \\
& 2 w (-4 + 46 \mu_1 + 50 \mu_1^2 - 31 \mu_2 + 41 \mu_1 \mu_2 - 20 \mathfrak{z}^2 - 22 \mu_1 \mathfrak{z}^2 - 2 \mu_1^2 \\
& \mathfrak{z}^2 - 5 \mu_2 \mathfrak{z}^2 + 31 \mu_1 \mu_2 \mathfrak{z}^2 + \theta p (-((-4 + 3 \mathfrak{z}^1 - 3 \mathfrak{z}^2) \times (1 + 5 \mathfrak{z}^2)) + \\
& 3 \mu_2 (16 + 5 \mathfrak{z}^1 + 11 \mathfrak{z}^2 - 5 \mathfrak{z}^1 \mathfrak{z}^2 + 5 \mathfrak{z}^2^2) - 2 \mu_1^2 (35 + 24 \mathfrak{z}^2 + \\
& \mathfrak{z}^2^2 - \mathfrak{z}^1 (23 + \mathfrak{z}^2)) - \mu_1 (42 - 31 \mathfrak{z}^1 + \mathfrak{z}^2 + 19 \mathfrak{z}^1 \mathfrak{z}^2 - \\
& 19 \mathfrak{z}^2^2 + 3 \mu_2 (32 + 5 \mathfrak{z}^1 (-1 + \mathfrak{z}^2) + 29 \mathfrak{z}^2 + 3 \mathfrak{z}^2^2)))) + \\
& \eta^3 (\theta p (\eta t (-11 \mu_2 (-1 + \mathfrak{z}^2) - \mu_1 (72 + 11 \mu_2) \times (-1 + \mathfrak{z}^2) - 4 \times \\
& (7 + 11 \mathfrak{z}^2) + 4 \mu_1^2 (61 + 11 \mathfrak{z}^2)) + 4 w (8 + 28 \mathfrak{z}^2 - 30 \mu_1 (1 + \mathfrak{z}^2) - \\
& 2 \mu_2 (59 + \mathfrak{z}^2) - 2 \mu_1^2 (-5 + 17 \mathfrak{z}^2) + 2 \mu_1 \mu_2 (61 + 59 \mathfrak{z}^2) + \\
& \eta t \mu_1^2 (323 + 79 \mathfrak{z}^2) - 6 \eta t (3 + 5 \mathfrak{z}^2 + 3 \mu_2 (3 + \mathfrak{z}^2)) + \\
& \eta t \mu_1 (-1 - 104 \mathfrak{z}^2 + 18 \mu_2 (5 + 3 \mathfrak{z}^2))) -
\end{aligned}$$

$$\begin{aligned}
& 4 \times (7 + 11 \mathfrak{z}2 + \mu1^2 (-67 + 7 \mathfrak{z}2) + \mu2 (17 + 31 \mathfrak{z}2) - \\
& \quad \mu1 (36 - 30 \mathfrak{z}2 + \mu2 (79 + 17 \mathfrak{z}2))) - \\
& 4 w^3 (-8 - 203 \mu2 + \mu1^2 (188 - 44 \mathfrak{z}2) - 40 \mathfrak{z}2 - 112 \mu2 \mathfrak{z}2 + \\
& \quad \mu1 (132 - 108 \mathfrak{z}2 + 7 \mu2 (61 + 29 \mathfrak{z}2)) + \\
& \quad \eta t (5 \mu2 (-1 + \mathfrak{z}2) + 5 \mu1 \mu2 (-1 + \mathfrak{z}2) - 32 \times (1 + 2 \mathfrak{z}2) - \\
& \quad 6 \mu1 (1 + 24 \mathfrak{z}2) + 2 \mu1^2 (259 + 83 \mathfrak{z}2))) + \\
& 2 w^2 (75 - 7 \mu2 + \mu1^2 (-613 + \mathfrak{z}2) + 171 \mathfrak{z}2 + 337 \mu2 \mathfrak{z}2 + \\
& \quad \mu1 (-418 + 232 \mathfrak{z}2 + \mu2 (-667 + 7 \mathfrak{z}2)) + \\
& \quad \eta t (30 - 137 \mu2 + 42 \mathfrak{z}2 - 37 \mu2 \mathfrak{z}2 + 28 \mu1^2 (1 + 2 \mathfrak{z}2) - \\
& \quad 2 \mu1 (85 + 8 \mathfrak{z}2) + \mu1 \mu2 (211 + 137 \mathfrak{z}2))) - \\
& 2 w^4 (9 - 247 \mu2 + 21 \mathfrak{z}2 + 55 \mu2 \mathfrak{z}2 - \mu1^2 (31 + 29 \mathfrak{z}2) + \\
& \quad \mu1 (-22 + 137 \mu2 - 8 \mathfrak{z}2 + 247 \mu2 \mathfrak{z}2) + 2 \eta t (-8 - 15 \mu2 - 22 \mathfrak{z}2 + \\
& \quad 5 \mu1^2 (47 + 25 \mathfrak{z}2) + \mu1 (-73 - 47 \mathfrak{z}2 + 15 \mu2 (1 + \mathfrak{z}2)))) - \\
& (-1 + \eta t) \mathfrak{e}l (4 - 44 \mu1 - 120 \mu1^2 + 19 \mu2 - 29 \mu1 \mu2 + 20 \mathfrak{z}2 + \\
& \quad 56 \mu1 \mathfrak{z}2 + 5 \mu2 \mathfrak{z}2 - 19 \mu1 \mu2 \mathfrak{z}2 + \\
& 4 w^4 (1 - 5 \mu1 (8 + \mu2 (-1 + \mathfrak{z}2) - 2 \mathfrak{z}2) - 5 \mu2 (-1 + \mathfrak{z}2) + 5 \mathfrak{z}2 + \\
& \quad \mu1^2 (7 + 29 \mathfrak{z}2)) + 8 w^3 (-\mu2 (1 + 5 \mathfrak{e}p (\mathfrak{z}1 - \mathfrak{z}2) (-1 + \mathfrak{z}2) + 5 \mathfrak{z}2) + \\
& \quad 2 \mu1^2 (25 + 12 \mathfrak{e}p (\mathfrak{z}1 - \mathfrak{z}2) + 8 \mathfrak{z}2) + (1 + 5 \mathfrak{z}2) \times \\
& \quad (-1 + \mathfrak{e}p (-\mathfrak{z}1 + \mathfrak{z}2)) + \mu1 (-5 - 11 \mathfrak{e}p (\mathfrak{z}1 - \mathfrak{z}2) (-1 + \mathfrak{z}2) - \\
& \quad 16 \mathfrak{z}2 + \mu2 (11 - 5 \mathfrak{e}p (\mathfrak{z}1 - \mathfrak{z}2) (-1 + \mathfrak{z}2) + \mathfrak{z}2))) + \\
& \mathfrak{e}p (2 \mu2 (-67 + 10 \mathfrak{z}1 (-1 + \mathfrak{z}2) + 35 \mathfrak{z}2 - 10 \mathfrak{z}2^2) + 4 \times \\
& \quad (6 + \mathfrak{z}1 + 5 \mathfrak{z}2 + 5 \mathfrak{z}1 \mathfrak{z}2 - 5 \mathfrak{z}2^2) + \mu1^2 (-10 + 145 \mathfrak{z}2 + 9 \mathfrak{z}2^2 + \\
& \quad \mathfrak{z}1 (-161 + 17 \mathfrak{z}2)) + \mu1 (-82 - 61 \mathfrak{z}1 + 21 \mathfrak{z}2 + 85 \mathfrak{z}1 \mathfrak{z}2 - \\
& \quad 59 \mathfrak{z}2^2 + 2 \mu2 (65 + 10 \mathfrak{z}1 (-1 + \mathfrak{z}2) + 53 \mathfrak{z}2 - 34 \mathfrak{z}2^2))) + \\
& 2 w^2 (-3 \times (4 + 20 \mathfrak{z}2 + \mu2 (19 + 5 \mathfrak{z}2) + \mu1^2 (-74 + 6 \mathfrak{z}2) - \\
& \quad \mu1 (50 - 36 \mathfrak{z}2 + \mu2 (29 + 19 \mathfrak{z}2))) + \mathfrak{e}p (-4 - 9 \mathfrak{z}1 + 61 \mathfrak{z}2 - \\
& \quad 45 \mathfrak{z}1 \mathfrak{z}2 + 45 \mathfrak{z}2^2 + \mu2 (116 - 45 \mathfrak{z}1 (-1 + \mathfrak{z}2) + 55 \mathfrak{z}2 + 45 \mathfrak{z}2^2) - \\
& \quad 2 \mu1^2 (98 + 81 \mathfrak{z}2 + \mathfrak{z}2^2 - 3 \mathfrak{z}1 (27 + \mathfrak{z}2)) - \\
& \quad \mu1 (104 - 93 \mathfrak{z}1 - 7 \mathfrak{z}2 + 69 \mathfrak{z}1 \mathfrak{z}2 - 73 \mathfrak{z}2^2 + \\
& \quad \mu2 (220 + 45 \mathfrak{z}1 (-1 + \mathfrak{z}2) + 209 \mathfrak{z}2 + 3 \mathfrak{z}2^2)))) + \\
& w (-2 \times (4 + 20 \mathfrak{z}2 + 24 \mu1^2 (1 + \mathfrak{z}2) + \mu2 (31 + 5 \mathfrak{z}2) - \mu1 \\
& \quad (68 + 41 \mu2 + 4 \mathfrak{z}2 + 31 \mu2 \mathfrak{z}2)) + \mathfrak{e}p (68 - 6 \mathfrak{z}1 + 106 \mathfrak{z}2 - \\
& \quad 30 \mathfrak{z}1 \mathfrak{z}2 + 30 \mathfrak{z}2^2 - 6 \mu2 (-21 + 5 \mathfrak{z}1 (-1 + \mathfrak{z}2) - 44 \mathfrak{z}2 - 5 \mathfrak{z}2^2) + \\
& \quad \mu1^2 (-502 + 41 \mathfrak{z}2 + 5 \mathfrak{z}2^2 + \mathfrak{z}1 (-57 + 33 \mathfrak{z}2)) - \\
& \quad \mu1 (290 - 33 \mathfrak{z}1 - 123 \mathfrak{z}2 - 51 \mathfrak{z}1 \mathfrak{z}2 + 13 \mathfrak{z}2^2 + \\
& \quad 6 \mu2 (63 + 5 \mathfrak{z}1 (-1 + \mathfrak{z}2) + 54 \mathfrak{z}2 + 23 \mathfrak{z}2^2)))) + \\
& \eta^2 (\mathfrak{e}p (-12 + 76 \mu2 + 41 \eta t \mu2 - 60 \mathfrak{z}2 - 28 \mu2 \mathfrak{z}2 + 7 \eta t \mu2 \mathfrak{z}2 - \\
& \quad 4 \mu1^2 (-3 \times (11 + \mathfrak{z}2) + 2 \eta t (29 + 7 \mathfrak{z}2)) - \mu1 (4 \times (-30 + 5 \mu2 + \\
& \quad 12 \mathfrak{z}2 + 19 \mu2 \mathfrak{z}2) + \eta t (-56 + 55 \mu2 - 88 \mathfrak{z}2 + 41 \mu2 \mathfrak{z}2)) + \\
& 2 w^4 (9 - 83 \mu2 + 33 \mathfrak{z}2 + 77 \mu2 \mathfrak{z}2 + \mu1^2 (-93 + 9 \mathfrak{z}2) + \\
& \quad \mu1 (-84 - 71 \mu2 + 42 \mathfrak{z}2 + 83 \mu2 \mathfrak{z}2) + \eta t (4 - 17 \mu2 - 4 \mathfrak{z}2 - 25 \mu2 \mathfrak{z}2 + \\
& \quad 90 \mu1^2 (1 + \mathfrak{z}2) + \mu1 (-86 + 67 \mu2 - 4 \mathfrak{z}2 + 17 \mu2 \mathfrak{z}2))) - \\
& 2 w (3 \eta t (10 + 11 \mu2 + 8 \mu1^2 (-5 + \mathfrak{z}2) + 26 \mathfrak{z}2 + 5 \mu2 \mathfrak{z}2 -
\end{aligned}$$

$$\begin{aligned}
& \mu_1 (70 + 21 \mu_2 - 14 \mathfrak{z}_2 + 11 \mu_2 \mathfrak{z}_2) + \\
& 2 (\mu_1^2 (-139 + 7 \mathfrak{z}_2) + \mu_1 (-89 - 94 \mu_2 + 59 \mathfrak{z}_2 + 10 \mu_2 \mathfrak{z}_2) + \\
& 2 \times (7 - 5 \mu_2 + 17 \mathfrak{z}_2 + 26 \mu_2 \mathfrak{z}_2)) + \\
& 2 w^2 (1 - 123 \mu_2 + \mu_1^2 (159 - 51 \mathfrak{z}_2) - 19 \mathfrak{z}_2 - 99 \mu_2 \mathfrak{z}_2 + \\
& \mu_1 (88 + 321 \mu_2 - 106 \mathfrak{z}_2 + 123 \mu_2 \mathfrak{z}_2) + \\
& 3 \eta t (-18 - 49 \mu_2 - 54 \mathfrak{z}_2 - 17 \mu_2 \mathfrak{z}_2 + 4 \mu_1^2 (70 + 11 \mathfrak{z}_2) + \\
& \mu_1 (82 + 83 \mu_2 - 100 \mathfrak{z}_2 + 49 \mu_2 \mathfrak{z}_2))) + \\
& w^3 (\eta t (-36 \times (1 + 5 \mathfrak{z}_2) + 4 \mu_1^2 (347 + 109 \mathfrak{z}_2) - \mu_2 \\
& (221 + 115 \mathfrak{z}_2) + \mu_1 (-40 + 451 \mu_2 - 440 \mathfrak{z}_2 + 221 \mu_2 \mathfrak{z}_2)) + \\
& 8 \times (5 + 16 \mathfrak{z}_2 + 6 \mu_2 (-7 + 3 \mathfrak{z}_2) - \mu_1^2 (43 + 5 \mathfrak{z}_2) + \\
& 2 \mu_1 (-16 + 7 \mathfrak{z}_2 + 3 \mu_2 (1 + 7 \mathfrak{z}_2))) + (-1 + \eta t) \mathfrak{e} l \\
& (w^4 (6 + 60 \mu_1 (-2 + \mathfrak{z}_2) - 5 \mu_2 (-1 + \mathfrak{z}_2) - 5 \mu_1 \mu_2 (-1 + \mathfrak{z}_2) + \\
& 30 \mathfrak{z}_2 + 6 \mu_1^2 (-13 + 9 \mathfrak{z}_2)) + w^3 (12 + \mu_2 (49 - 25 \mathfrak{z}_2) + 60 \mathfrak{z}_2 + \\
& 4 \mu_1^2 (-19 + 25 \mathfrak{z}_2) + \mu_1 (-232 + \mu_2 + 76 \mathfrak{z}_2 - 49 \mu_2 \mathfrak{z}_2)) - \\
& 2 \times (3 + 15 \mathfrak{z}_2 + \mu_2 (19 + 5 \mathfrak{z}_2) + \mu_1^2 (-31 + 7 \mathfrak{z}_2) - \\
& \mu_1 (40 - 16 \mathfrak{z}_2 + \mu_2 (29 + 19 \mathfrak{z}_2))) - \mathfrak{e} p (6 \times (-1 + \mathfrak{z}_1 - \mathfrak{z}_2) \times \\
& (1 + 5 \mathfrak{z}_2) + 2 \mu_2 (-61 + 15 \mathfrak{z}_1 (-1 + \mathfrak{z}_2) - 26 \mathfrak{z}_2 - 15 \mathfrak{z}_2^2) + \\
& \mu_1^2 (136 + \mathfrak{z}_1 (-109 + \mathfrak{z}_2) + 109 \mathfrak{z}_2 + 7 \mathfrak{z}_2^2) + \mu_1 (58 - 67 \mathfrak{z}_1 + \mathfrak{z}_2 + 49 \\
& \mathfrak{z}_1 \mathfrak{z}_2 - 41 \mathfrak{z}_2^2 + 2 \mu_2 (107 + 15 \mathfrak{z}_1 (-1 + \mathfrak{z}_2) + 94 \mathfrak{z}_2 + 3 \mathfrak{z}_2^2))) - \\
& 4 w (3 - 42 \mu_1 - 51 \mu_1^2 + 13 \mu_2 - 23 \mu_1 \mu_2 + 15 \mathfrak{z}_2 + 27 \mu_1 \mathfrak{z}_2 + \\
& 9 \mu_1^2 \mathfrak{z}_2 + 5 \mu_2 \mathfrak{z}_2 - 13 \mu_1 \mu_2 \mathfrak{z}_2 + \mathfrak{e} p (5 + 3 \mathfrak{z}_1 - 14 \mathfrak{z}_2 + 15 \mathfrak{z}_1 \mathfrak{z}_2 - \\
& 15 \mathfrak{z}_2^2 + \mu_2 (-47 + 15 \mathfrak{z}_1 (-1 + \mathfrak{z}_2) - 4 \mathfrak{z}_2 - 15 \mathfrak{z}_2^2) + \\
& \mu_1^2 (32 + 2 \mathfrak{z}_1 (-34 + \mathfrak{z}_2) + 67 \mathfrak{z}_2 + 3 \mathfrak{z}_2^2) + \\
& \mu_1 (13 - 35 \mathfrak{z}_1 + 11 \mathfrak{z}_2 + 32 \mathfrak{z}_1 \mathfrak{z}_2 - 27 \mathfrak{z}_2^2 + \\
& \mu_2 (73 + 15 \mathfrak{z}_1 (-1 + \mathfrak{z}_2) + 68 \mathfrak{z}_2 - 9 \mathfrak{z}_2^2))) + \\
& w^2 (6 \times (-5 \mu_2 (-1 + \mathfrak{z}_2) + 4 \mu_1^2 (6 + \mathfrak{z}_2) - \mu_1 (4 + 5 \mu_2 \\
& (-1 + \mathfrak{z}_2) + 10 \mathfrak{z}_2)) + \mathfrak{e} p (-10 - 6 \mathfrak{z}_1 + 4 \mathfrak{z}_2 - 30 \mathfrak{z}_1 \mathfrak{z}_2 + \\
& 30 \mathfrak{z}_2^2 + \mu_1^2 (60 + \mathfrak{z}_1 (163 - 7 \mathfrak{z}_2) - 163 \mathfrak{z}_2 - 5 \mathfrak{z}_2^2) + \\
& \mu_2 (26 - 30 \mathfrak{z}_1 (-1 + \mathfrak{z}_2) - 44 \mathfrak{z}_2 + 30 \mathfrak{z}_2^2) + \\
& \mu_1 (26 + 73 \mathfrak{z}_1 - 87 \mathfrak{z}_2 - 79 \mathfrak{z}_1 \mathfrak{z}_2 + 67 \mathfrak{z}_2^2 + \\
& \mu_2 (-22 - 30 \mathfrak{z}_1 (-1 + \mathfrak{z}_2) - 44 \mathfrak{z}_2 + 42 \mathfrak{z}_2^2)))) + \\
& \eta^4 (6 \mathfrak{e} p - 24 \eta t \mathfrak{e} p + 50 \mathfrak{e} l \mathfrak{e} p - 50 \eta t \mathfrak{e} l \mathfrak{e} p + 4 \mathfrak{e} l \mu_1 - 4 \eta t \mathfrak{e} l \mu_1 - \\
& 88 \mathfrak{e} p \mu_1 - 40 \eta t \mathfrak{e} p \mu_1 - 98 \mathfrak{e} l \mathfrak{e} p \mu_1 + 98 \eta t \mathfrak{e} l \mathfrak{e} p \mu_1 - 44 \\
& \mathfrak{e} l \mu_1^2 + 44 \eta t \mathfrak{e} l \mu_1^2 + 50 \mathfrak{e} p \mu_1^2 + 176 \eta t \mathfrak{e} p \mu_1^2 - 268 \\
& \mathfrak{e} l \mathfrak{e} p \mu_1^2 + 268 \eta t \mathfrak{e} l \mathfrak{e} p \mu_1^2 - 154 \mathfrak{e} p \mu_2 - 68 \eta t \mathfrak{e} p \\
& \mu_2 + 10 \mathfrak{e} l \mathfrak{e} p \mu_2 - 10 \eta t \mathfrak{e} l \mathfrak{e} p \mu_2 + 62 \mathfrak{e} p \mu_1 \mu_2 + 100 \\
& \eta t \mathfrak{e} p \mu_1 \mu_2 - 86 \mathfrak{e} l \mathfrak{e} p \mu_1 \mu_2 + 86 \eta t \mathfrak{e} l \mathfrak{e} p \mu_1 \mu_2 - 19 \\
& \mathfrak{e} l \mathfrak{e} p \mu_1 \mathfrak{z}_1 + 19 \eta t \mathfrak{e} l \mathfrak{e} p \mu_1 \mathfrak{z}_1 - 79 \mathfrak{e} l \mathfrak{e} p \mu_1^2 \mathfrak{z}_1 + 79 \\
& \eta t \mathfrak{e} l \mathfrak{e} p \mu_1^2 \mathfrak{z}_1 + 78 \mathfrak{e} p \mathfrak{z}_2 + 24 \eta t \mathfrak{e} p \mathfrak{z}_2 + 10 \mathfrak{e} l \mathfrak{e} p \\
& \mathfrak{z}_2 - 10 \eta t \mathfrak{e} l \mathfrak{e} p \mathfrak{z}_2 + 20 \mathfrak{e} l \mu_1 \mathfrak{z}_2 - 20 \eta t \mathfrak{e} l \mu_1 \mathfrak{z}_2 - 68 \\
& \mathfrak{e} p \mu_1 \mathfrak{z}_2 - 56 \eta t \mathfrak{e} p \mu_1 \mathfrak{z}_2 + 89 \mathfrak{e} l \mathfrak{e} p \mu_1 \mathfrak{z}_2 - 89 \eta t \mathfrak{e} l \\
& \mathfrak{e} p \mu_1 \mathfrak{z}_2 - 4 \mathfrak{e} l \mu_1^2 \mathfrak{z}_2 + 4 \eta t \mathfrak{e} l \mu_1^2 \mathfrak{z}_2 - 74 \mathfrak{e} p \mu_1^2 \\
& \mathfrak{z}_2 + 16 \eta t \mathfrak{e} p \mu_1^2 \mathfrak{z}_2 + 79 \mathfrak{e} l \mathfrak{e} p \mu_1^2 \mathfrak{z}_2 - 79 \eta t \mathfrak{e} l \mathfrak{e} p \\
& \mu_1^2 \mathfrak{z}_2 + 46 \mathfrak{e} p \mu_2 \mathfrak{z}_2 - 16 \eta t \mathfrak{e} p \mu_2 \mathfrak{z}_2 + 98 \mathfrak{e} l \mathfrak{e} p \mu_2
\end{aligned}$$



$$\begin{aligned}
& \mathfrak{z}^2 - 98 \eta t \, \mathfrak{e} l \, \mathfrak{e} p \, \mu_2 \mathfrak{z}^2 + 154 \mathfrak{e} p \, \mu_1 \mu_2 \mathfrak{z}^2 + 68 \eta t \, \mathfrak{e} p \, \mu_1 \\
& \mu_2 \mathfrak{z}^2 - 70 \mathfrak{e} l \, \mathfrak{e} p \, \mu_1 \mu_2 \mathfrak{z}^2 + 70 \eta t \, \mathfrak{e} l \, \mathfrak{e} p \, \mu_1 \mu_2 \mathfrak{z}^2 + 49 \\
& \mathfrak{e} l \, \mathfrak{e} p \, \mu_1 \mathfrak{z}^2 - 49 \eta t \, \mathfrak{e} l \, \mathfrak{e} p \, \mu_1 \mathfrak{z}^2 + 19 \mathfrak{e} l \, \mathfrak{e} p \, \mu_1^2 \\
& \mathfrak{z}^2 - 19 \eta t \, \mathfrak{e} l \, \mathfrak{e} p \, \mu_1^2 \mathfrak{z}^2 - 21 \mathfrak{e} l \, \mathfrak{e} p \, \mu_1 \mathfrak{z}^2 + 21 \\
& \eta t \, \mathfrak{e} l \, \mathfrak{e} p \, \mu_1 \mathfrak{z}^2 + 9 \mathfrak{e} l \, \mathfrak{e} p \, \mu_1^2 \mathfrak{z}^2 - 9 \eta t \, \mathfrak{e} l \, \mathfrak{e} p \, \mu_1^2 \\
& \mathfrak{z}^2 - 60 \mathfrak{e} l \, \mathfrak{e} p \, \mu_1 \mu_2 \mathfrak{z}^2 + 60 \eta t \, \mathfrak{e} l \, \mathfrak{e} p \, \mu_1 \mu_2 \mathfrak{z}^2 + w^4 \\
& \left( (-1 + \eta t) \, \mathfrak{e} l \, (-4 + 5 \mu_2 - 20 \mathfrak{z}^2 - 5 \mu_2 \mathfrak{z}^2 + 4 \mu_1^2 (53 + 31 \mathfrak{z}^2) - \right. \\
& \quad 5 \mu_1 (\mu_2 (-1 + \mathfrak{z}^2) + 8 \times (2 + \mathfrak{z}^2))) + 2 \mathfrak{e} p (5 \eta t (-7 + 7 \mu_2 - 11 \mathfrak{z}^2 + \\
& \quad 5 \mu_2 \mathfrak{z}^2 + 3 \mu_1^2 (41 + 19 \mathfrak{z}^2) - \mu_1 (28 + 17 \mu_2 + 26 \mathfrak{z}^2 + 7 \mu_2 \mathfrak{z}^2)) - \\
& \quad 2 \times (8 + 170 \mu_2 + 22 \mathfrak{z}^2 + 55 \mu_2 \mathfrak{z}^2 + 5 \mu_1^2 (-19 + 7 \mathfrak{z}^2) - \\
& \quad \mu_1 (87 + 280 \mu_2 - 57 \mathfrak{z}^2 + 170 \mu_2 \mathfrak{z}^2))) \left. \right) + w^3 \\
& \left( (-1 + \eta t) \, \mathfrak{e} l (32 \mu_1^2 (13 + 3 \mathfrak{e} p (\mathfrak{z}^1 - \mathfrak{z}^2) + 2 \mathfrak{z}^2) + \mu_2 \right. \\
& \quad (-53 - 20 \mathfrak{e} p (\mathfrak{z}^1 - \mathfrak{z}^2) (-1 + \mathfrak{z}^2) + 5 \mathfrak{z}^2) + 4 \times (1 + 5 \mathfrak{z}^2) \times \\
& \quad (-4 + \mathfrak{e} p (-\mathfrak{z}^1 + \mathfrak{z}^2)) + \mu_1 (112 - 44 \mathfrak{e} p (\mathfrak{z}^1 - \mathfrak{z}^2) (-1 + \mathfrak{z}^2) - \\
& \quad 160 \mathfrak{z}^2 + \mu_2 (43 - 20 \mathfrak{e} p (\mathfrak{z}^1 - \mathfrak{z}^2) (-1 + \mathfrak{z}^2) + 53 \mathfrak{z}^2)) \left. \right) + \\
& \mathfrak{e} p (\eta t (-52 - 44 \mathfrak{z}^2 - 24 \mu_1 (4 + \mathfrak{z}^2) + 5 \mu_2 (91 + 29 \mathfrak{z}^2) + \\
& \quad 4 \mu_1^2 (97 + 59 \mathfrak{z}^2) - 5 \mu_1 \mu_2 (149 + 91 \mathfrak{z}^2)) + \\
& \quad 8 \times (-19 - 47 \mathfrak{z}^2 + 2 \mu_1^2 (83 + \mathfrak{z}^2) - 2 \mu_2 (29 + 52 \mathfrak{z}^2) + \\
& \quad \mu_1 (111 - 63 \mathfrak{z}^2 + \mu_2 (266 + 58 \mathfrak{z}^2))) \left. \right) + w \\
& \left( \mathfrak{e} p (4 \times (41 + 68 \mu_2 + 49 \mathfrak{z}^2 + 130 \mu_2 \mathfrak{z}^2 + 8 \mu_1^2 (-35 + 2 \mathfrak{z}^2) - \right. \\
& \quad \mu_1 (155 + 328 \mu_2 - 107 \mathfrak{z}^2 + 68 \mu_2 \mathfrak{z}^2)) + \\
& \quad \eta t (88 - 161 \mu_2 + 128 \mathfrak{z}^2 + 17 \mu_2 \mathfrak{z}^2 - 12 \mu_1^2 (45 + 11 \mathfrak{z}^2) + \\
& \quad \mu_1 (-212 + 127 \mu_2 + 116 \mathfrak{z}^2 + 161 \mu_2 \mathfrak{z}^2)) \left. \right) + \\
& (-1 + \eta t) \, \mathfrak{e} l (3 \times (4 - 88 \mu_1^2 + 20 \mathfrak{z}^2 + \mu_2 (19 + 5 \mathfrak{z}^2) - \\
& \quad \mu_1 (44 - 40 \mathfrak{z}^2 + \mu_2 (29 + 19 \mathfrak{z}^2))) + \\
& \mathfrak{e} p (20 + 60 \mu_2 \mathfrak{z}^1 (-1 + \mathfrak{z}^2) - 56 \mathfrak{z}^2 - 60 \mathfrak{z}^2 + 12 \mathfrak{z}^1 (1 + 5 \mathfrak{z}^2) + \\
& \quad \mu_1^2 (294 + 3 \mathfrak{z}^1 (-89 + \mathfrak{z}^2) + 251 \mathfrak{z}^2 + 7 \mathfrak{z}^2) - 2 \mu_2 (119 + 13 \mathfrak{z}^2 + \\
& \quad 30 \mathfrak{z}^2) + \mu_1 (74 - 45 \mathfrak{z}^2 - 113 \mathfrak{z}^2 + 3 \mathfrak{z}^1 (-45 + 41 \mathfrak{z}^2) + \\
& \quad \mu_2 (362 + 60 \mathfrak{z}^1 (-1 + \mathfrak{z}^2) + 322 \mathfrak{z}^2 - 36 \mathfrak{z}^2)) \left. \right) + \\
w^2 \left( - \left( (-1 + \eta t) \, \mathfrak{e} l (-15 \mu_2 (-1 + \mathfrak{z}^2) + 4 \mu_1^2 (43 + 11 \mathfrak{z}^2) - \right. \right. \\
& \quad \mu_1 (44 + 15 \mu_2 (-1 + \mathfrak{z}^2) + 64 \mathfrak{z}^2)) \left. \right) + \\
& \mathfrak{e} p (-2 (\mu_1^2 (250 - 178 \mathfrak{z}^2) + 4 \times (9 + 6 \mathfrak{z}^2 - \mu_2 (104 + 7 \mathfrak{z}^2)) + \\
& \quad \mu_1 (94 - 250 \mathfrak{z}^2 + 8 \mu_2 (59 + 52 \mathfrak{z}^2)) + \mathfrak{e} l (10 + 3 \mathfrak{z}^1 + 23 \mathfrak{z}^2 + 15 \\
& \quad \mathfrak{z}^1 \mathfrak{z}^2 - 15 \mathfrak{z}^2 + \mu_2 (22 + 15 \mathfrak{z}^1 (-1 + \mathfrak{z}^2) + 77 \mathfrak{z}^2 - 15 \mathfrak{z}^2) + \\
& \quad \mu_1^2 (-160 + 119 \mathfrak{z}^2 + 5 \mathfrak{z}^2 + \mathfrak{z}^1 (-119 + 11 \mathfrak{z}^2)) + \\
& \quad \mu_1 (-78 - 44 \mathfrak{z}^1 + 106 \mathfrak{z}^2 + 62 \mathfrak{z}^1 \mathfrak{z}^2 - 46 \mathfrak{z}^2 + \\
& \quad \mu_2 (-74 + 15 \mathfrak{z}^1 (-1 + \mathfrak{z}^2) - 43 \mathfrak{z}^2 - 51 \mathfrak{z}^2)) \left. \right) + \\
& \eta t (168 + 331 \mu_2 + 192 \mathfrak{z}^2 + 149 \mu_2 \mathfrak{z}^2 - 8 \mu_1^2 (236 + 55 \mathfrak{z}^2) - \\
& \quad \mu_1 (112 - 556 \mathfrak{z}^2 + \mu_2 (629 + 331 \mathfrak{z}^2)) + \\
& 2 \mathfrak{e} l (10 + 3 \mathfrak{z}^1 + 23 \mathfrak{z}^2 + 15 \mathfrak{z}^1 \mathfrak{z}^2 - 15 \mathfrak{z}^2 + \\
& \quad \mu_2 (22 + 15 \mathfrak{z}^1 (-1 + \mathfrak{z}^2) + 77 \mathfrak{z}^2 - 15 \mathfrak{z}^2) + \\
& \quad \mu_1^2 (-160 + 119 \mathfrak{z}^2 + 5 \mathfrak{z}^2 + \mathfrak{z}^1 (-119 + 11 \mathfrak{z}^2)) + \\
& \quad \mu_1 (-78 - 44 \mathfrak{z}^1 + 106 \mathfrak{z}^2 + 62 \mathfrak{z}^1 \mathfrak{z}^2 - 46 \mathfrak{z}^2 +
\end{aligned}$$

$$\begin{aligned}
& \mu^2 \left( -74 + 15 \mathfrak{e}1 (-1 + \mathfrak{e}2) - 43 \mathfrak{e}2 - 51 \mathfrak{e}2^2 \right) \Big) \Big) \Big) \Big) + \\
& \eta^6 \left( -4 \mathfrak{e}p \left( -2 - 30 \mu^2 + \mu^2 (51 - 15 \mathfrak{e}2) + 6 \eta t (1 + \mu^1) \times (-1 + \mathfrak{e}2) + \right. \right. \\
& \quad \left. \left. 2 \mathfrak{e}2 + \mu^1 (13 - 31 \mathfrak{e}2 + 30 \mu^2 (1 + \mathfrak{e}2)) \right) + w^4 \right. \\
& \quad \left( (-1 + \eta t) \mathfrak{e}l \left( \mu^1 (8 + 5 \mu^2 (-1 + \mathfrak{e}2) - 20 \mathfrak{e}2) + 5 \mu^2 (-1 + \mathfrak{e}2) - \right. \right. \\
& \quad \left. \left. 2 \times (1 + 5 \mathfrak{e}2) + 2 \mu^2 (29 + 7 \mathfrak{e}2) \right) + \right. \\
& \quad \left. 2 \mathfrak{e}p \left( -23 + 5 \mu^2 - 55 \mathfrak{e}2 - 143 \mu^2 \mathfrak{e}2 + \mu^2 (95 + 61 \mathfrak{e}2) + \right. \right. \\
& \quad \left. \left. \mu^1 (72 + 281 \mu^2 + 6 \mathfrak{e}2 - 5 \mu^2 \mathfrak{e}2) + \eta t (10 + 73 \mu^2 - 22 \mathfrak{e}2 + 5 \mu^2 \mathfrak{e}2 + \right. \right. \\
& \quad \left. \left. 4 \mu^2 (19 + 8 \mathfrak{e}2) - \mu^1 (-2 + 83 \mu^2 + 32 \mathfrak{e}2 + 73 \mu^2 \mathfrak{e}2) \right) \right) \Big) + \\
& w^3 \left( - \left( (-1 + \eta t) \mathfrak{e}l \left( 4 \mu^2 (29 + 24 \mathfrak{e}p (\mathfrak{e}1 - \mathfrak{e}2) + \mathfrak{e}2) - \mu^2 \right. \right. \right. \\
& \quad (19 + 20 \mathfrak{e}p (\mathfrak{e}1 - \mathfrak{e}2) (-1 + \mathfrak{e}2) + 5 \mathfrak{e}2) + 4 \times (1 + 5 \mathfrak{e}2) \times \\
& \quad (-1 + \mathfrak{e}p (-\mathfrak{e}1 + \mathfrak{e}2)) + \mu^1 (40 - 44 \mathfrak{e}p (\mathfrak{e}1 - \mathfrak{e}2) (-1 + \mathfrak{e}2) - \\
& \quad \left. \left. 52 \mathfrak{e}2 + \mu^2 (29 - 20 \mathfrak{e}p (\mathfrak{e}1 - \mathfrak{e}2) (-1 + \mathfrak{e}2) + 19 \mathfrak{e}2) \right) \right) \Big) + \\
& \mathfrak{e}p \left( 8 \times \left( 13 + 44 \mu^2 + 8 \mathfrak{e}2 + 46 \mu^2 \mathfrak{e}2 + \mu^2 (-89 + 17 \mathfrak{e}2) - 2 \mu^1 \right. \right. \\
& \quad \left. \left. (23 + 68 \mu^2 - 20 \mathfrak{e}2 + 22 \mu^2 \mathfrak{e}2) \right) + \eta t (68 - 123 \mu^2 + 4 \mathfrak{e}2 + 27 \mu^2 \right. \\
& \quad \left. \left. \mathfrak{e}2 - 12 \mu^2 (33 + 7 \mathfrak{e}2) + \mu^1 (8 + 69 \mu^2 + 88 \mathfrak{e}2 + 123 \mu^2 \mathfrak{e}2) \right) \right) \Big) + \\
& w \left( -4 \times (-1 + \eta t) \mathfrak{e}l \mu^1 (1 + \mu^1) \times (-1 + \mathfrak{e}2) + \mathfrak{e}p \left( -2 \times (68 - \right. \right. \\
& \quad \left. \left. 8 \mathfrak{e}2 + 5 \mathfrak{e}l \mu^2 (5 + \mathfrak{e}2) + 12 \mu^2 (4 + 9 \mathfrak{e}2)) + \right. \right. \\
& \quad \left. \left. \mu^2 (476 - 44 \mathfrak{e}2 + \mathfrak{e}l (166 + 5 \mathfrak{e}1 - 17 \mathfrak{e}2 - 5 \mathfrak{e}1 \mathfrak{e}2 - 5 \mathfrak{e}2^2)) \right) + \right. \\
& \quad \left. \mu^1 (4 \times (37 + 132 \mu^2 - 31 \mathfrak{e}2 + 24 \mu^2 \mathfrak{e}2) + \right. \\
& \quad \left. \mathfrak{e}l (22 + 70 \mu^2 + 5 \mathfrak{e}1 - 89 \mathfrak{e}2 + 50 \mu^2 \mathfrak{e}2 - 5 \mathfrak{e}1 \mathfrak{e}2 - 5 \mathfrak{e}2^2)) \right) + \\
& \quad \eta t (28 \times (-1 + \mathfrak{e}2) + 10 \mu^2 (12 + \mathfrak{e}l (5 + \mathfrak{e}2)) + \mu^2 \\
& \quad \left( -16 \times (-1 + \mathfrak{e}2) + \mathfrak{e}l (-166 + 5 \mathfrak{e}1 (-1 + \mathfrak{e}2) + 17 \mathfrak{e}2 + 5 \mathfrak{e}2^2) \right) - \\
& \quad \left. \mu^1 (12 \times (1 - \mathfrak{e}2 + 10 \mu^2 (1 + \mathfrak{e}2)) + \mathfrak{e}l (22 + 5 \mathfrak{e}1 - \right. \\
& \quad \left. \left. 89 \mathfrak{e}2 - 5 \mathfrak{e}1 \mathfrak{e}2 - 5 \mathfrak{e}2^2 + 10 \mu^2 (7 + 5 \mathfrak{e}2)) \right) \right) \Big) \Big) + \\
& w^2 \left( 4 \times (-1 + \eta t) \mathfrak{e}l \mu^1 (-1 - 5 \mathfrak{e}2 + \mu^1 (11 + \mathfrak{e}2)) + \mathfrak{e}p \right. \\
& \quad \left( 2 \times \left( 57 - 227 \mu^2 + \mu^2 (115 - 151 \mathfrak{e}2) + 21 \mathfrak{e}2 + \right. \right. \\
& \quad \left. \left. 95 \mu^2 \mathfrak{e}2 + \mu^1 (52 + 37 \mu^2 - 190 \mathfrak{e}2 + 227 \mu^2 \mathfrak{e}2) \right) + \right. \\
& \quad \left. 5 \mathfrak{e}l \left( \mu^2 (-52 + 3 \mathfrak{e}1 (-5 + \mathfrak{e}2) + 15 \mathfrak{e}2 + \mathfrak{e}2^2) + \right. \right. \\
& \quad \left. \left. 2 \times (1 + 5 \mathfrak{e}2 + \mu^2 (7 + 11 \mathfrak{e}2)) - \mu^1 (26 + 3 \mathfrak{e}1 - 25 \mathfrak{e}2 - \right. \right. \\
& \quad \left. \left. 9 \mathfrak{e}1 \mathfrak{e}2 + 5 \mathfrak{e}2^2 + 2 \mu^2 (17 + 13 \mathfrak{e}2 + 6 \mathfrak{e}2^2) \right) \right) \Big) + \\
& \quad \eta t \left( 4 \times \left( -21 - 35 \mu^2 + 21 \mathfrak{e}2 - 4 \mu^2 \mathfrak{e}2 + 8 \mu^2 (5 + \mathfrak{e}2) + \right. \right. \\
& \quad \left. \left. \mu^1 (-29 + 43 \mu^2 + 5 \mathfrak{e}2 + 35 \mu^2 \mathfrak{e}2) \right) - \right. \\
& \quad \left. 5 \mathfrak{e}l \left( \mu^2 (-52 + 3 \mathfrak{e}1 (-5 + \mathfrak{e}2) + 15 \mathfrak{e}2 + \mathfrak{e}2^2) + \right. \right. \\
& \quad \left. \left. 2 \times (1 + 5 \mathfrak{e}2 + \mu^2 (7 + 11 \mathfrak{e}2)) - \mu^1 (26 + 3 \mathfrak{e}1 - 25 \mathfrak{e}2 - \right. \right. \\
& \quad \left. \left. 9 \mathfrak{e}1 \mathfrak{e}2 + 5 \mathfrak{e}2^2 + 2 \mu^2 (17 + 13 \mathfrak{e}2 + 6 \mathfrak{e}2^2) \right) \right) \Big) \Big) \Big) + \\
& \eta^5 \left( 50 \mathfrak{e}p + 16 \eta t \mathfrak{e}p + 24 \mathfrak{e}l \mathfrak{e}p - 24 \eta t \mathfrak{e}l \mathfrak{e}p + 4 \mathfrak{e}l \mu^1 - 4 \eta t \mathfrak{e}l \mu^1 - \right. \\
& \quad 100 \mathfrak{e}p \mu^1 + 2 \mathfrak{e}l \mathfrak{e}p \mu^1 - 2 \eta t \mathfrak{e}l \mathfrak{e}p \mu^1 + 4 \mathfrak{e}l \mu^2 - 4 \\
& \quad \eta t \mathfrak{e}l \mu^2 - 246 \mathfrak{e}p \mu^2 - 16 \eta t \mathfrak{e}p \mu^2 - 166 \mathfrak{e}l \mathfrak{e}p \\
& \quad \mu^2 + 166 \eta t \mathfrak{e}l \mathfrak{e}p \mu^2 + 26 \mathfrak{e}p \mu^2 - 60 \eta t \mathfrak{e}p \mu^2 + 50 \\
& \quad \mathfrak{e}l \mathfrak{e}p \mu^2 - 50 \eta t \mathfrak{e}l \mathfrak{e}p \mu^2 - 238 \mathfrak{e}p \mu^1 \mu^2 + 60 \eta t \mathfrak{e}p \mu^1 \\
& \quad \mu^2 - 70 \mathfrak{e}l \mathfrak{e}p \mu^1 \mu^2 + 70 \eta t \mathfrak{e}l \mathfrak{e}p \mu^1 \mu^2 - 5 \mathfrak{e}l \mathfrak{e}p \mu^1 \\
& \quad \mathfrak{e}1 + 5 \eta t \mathfrak{e}l \mathfrak{e}p \mu^1 \mathfrak{e}1 - 5 \mathfrak{e}l \mathfrak{e}p \mu^2 \mathfrak{e}1 + 5 \eta t \mathfrak{e}l \mathfrak{e}p \mu^2 \\
& \quad \mathfrak{e}1 + 10 \mathfrak{e}p \mathfrak{e}2 - 16 \eta t \mathfrak{e}p \mathfrak{e}2 - 24 \mathfrak{e}l \mathfrak{e}p \mathfrak{e}2 + 24 \eta t \mathfrak{e}l
\end{aligned}$$

$$\begin{aligned}
& \epsilon p \, \mathfrak{z}^2 - 4 \, \epsilon l \, \mu_1 \, \mathfrak{z}^2 + 4 \, \eta t \, \epsilon l \, \mu_1 \, \mathfrak{z}^2 + 88 \, \epsilon p \, \mu_1 \, \mathfrak{z}^2 + 65 \\
& \epsilon l \, \epsilon p \, \mu_1 \, \mathfrak{z}^2 - 65 \, \eta t \, \epsilon l \, \epsilon p \, \mu_1 \, \mathfrak{z}^2 - 4 \, \epsilon l \, \mu_1^2 \, \mathfrak{z}^2 + 4 \, \eta t \\
& \epsilon l \, \mu_1^2 \, \mathfrak{z}^2 + 30 \, \epsilon p \, \mu_1^2 \, \mathfrak{z}^2 + 16 \, \eta t \, \epsilon p \, \mu_1^2 \, \mathfrak{z}^2 + 17 \, \epsilon l \, \epsilon p \\
& \mu_1^2 \, \mathfrak{z}^2 - 17 \, \eta t \, \epsilon l \, \epsilon p \, \mu_1^2 \, \mathfrak{z}^2 + 106 \, \epsilon p \, \mu_2 \, \mathfrak{z}^2 + 10 \, \epsilon l \\
& \epsilon p \, \mu_2 \, \mathfrak{z}^2 - 10 \, \eta t \, \epsilon l \, \epsilon p \, \mu_2 \, \mathfrak{z}^2 - 26 \, \epsilon p \, \mu_1 \, \mu_2 \, \mathfrak{z}^2 + 60 \, \eta t \\
& \epsilon p \, \mu_1 \, \mu_2 \, \mathfrak{z}^2 - 50 \, \epsilon l \, \epsilon p \, \mu_1 \, \mu_2 \, \mathfrak{z}^2 + 50 \, \eta t \, \epsilon l \, \epsilon p \, \mu_1 \, \mu_2 \\
& \mathfrak{z}^2 + 5 \, \epsilon l \, \epsilon p \, \mu_1 \, \mathfrak{z}^1 \, \mathfrak{z}^2 - 5 \, \eta t \, \epsilon l \, \epsilon p \, \mu_1 \, \mathfrak{z}^1 \, \mathfrak{z}^2 + 5 \, \epsilon l \, \epsilon p \\
& \mu_1^2 \, \mathfrak{z}^1 \, \mathfrak{z}^2 - 5 \, \eta t \, \epsilon l \, \epsilon p \, \mu_1^2 \, \mathfrak{z}^1 \, \mathfrak{z}^2 + 5 \, \epsilon l \, \epsilon p \, \mu_1 \, \mathfrak{z}^2^2 - 5 \\
& \eta t \, \epsilon l \, \epsilon p \, \mu_1 \, \mathfrak{z}^2^2 + 5 \, \epsilon l \, \epsilon p \, \mu_1^2 \, \mathfrak{z}^2^2 - 5 \, \eta t \, \epsilon l \, \epsilon p \, \mu_1^2 \\
& \mathfrak{z}^2^2 - 2 \, w^4 \left( (-1 + \eta t) \, \epsilon l \left( 5 \, \mu_1 \left( \mu_2 \left( -1 + \mathfrak{z}^2 \right) - 6 \, \mathfrak{z}^2 \right) + \right. \right. \\
& \quad \left. \left. 5 \, \mu_2 \left( -1 + \mathfrak{z}^2 \right) + 33 \, \mu_1^2 \left( 3 + \mathfrak{z}^2 \right) - 3 \times (1 + 5 \, \mathfrak{z}^2) \right) + \right. \\
& \quad \left. \epsilon p \left( \eta t \left( -19 - 35 \, \mathfrak{z}^2 + 20 \, \mu_2 \left( 5 + \mathfrak{z}^2 \right) + 9 \, \mu_1^2 \left( 39 + 17 \, \mathfrak{z}^2 \right) - 4 \, \mu_1 \right. \right. \right. \\
& \quad \left. \left. \left( 4 \times (4 + 5 \, \mathfrak{z}^2) + 5 \, \mu_2 \left( 7 + 5 \, \mathfrak{z}^2 \right) \right) \right) - 20 \times \left( 2 + \mu_1^2 \left( -13 + \mathfrak{z}^2 \right) + \right. \right. \\
& \quad \left. \left. 4 \, \mathfrak{z}^2 + \mu_2 \left( 10 + 11 \, \mathfrak{z}^2 \right) - \mu_1 \left( 11 - 5 \, \mathfrak{z}^2 + 2 \, \mu_2 \left( 16 + 5 \, \mathfrak{z}^2 \right) \right) \right) \right) \right) + \\
& 2 \, w^3 \left( -2 \times (-1 + \eta t) \, \epsilon l \left( \mu_2 + \mu_1^2 \left( -13 + \mathfrak{z}^2 \right) + 5 \, \mu_2 \, \mathfrak{z}^2 - \mu_1 \right. \right. \\
& \quad \left. \left. (1 - 7 \, \mathfrak{z}^2 + \mu_2 \left( 11 + \mathfrak{z}^2 \right)) \right) \right) + \epsilon p \left( 34 - 192 \, \mu_2 + 3 \, \epsilon l \, \mathfrak{z}^1 - \right. \\
& \quad 15 \, \epsilon l \, \mu_2 \, \mathfrak{z}^1 + 62 \, \mathfrak{z}^2 - 3 \, \epsilon l \, \mathfrak{z}^2 + 84 \, \mu_2 \, \mathfrak{z}^2 + 15 \, \epsilon l \, \mu_2 \, \mathfrak{z}^2 + \\
& \quad 15 \, \epsilon l \, \mathfrak{z}^1 \, \mathfrak{z}^2 + 15 \, \epsilon l \, \mu_2 \, \mathfrak{z}^1 \, \mathfrak{z}^2 - 15 \, \epsilon l \, \mathfrak{z}^2^2 - 15 \, \epsilon l \, \mu_2 \, \mathfrak{z}^2^2 - 6 \, \mu_1^2 \\
& \quad (1 + 12 \, \epsilon l \left( \mathfrak{z}^1 - \mathfrak{z}^2 \right) + 27 \, \mathfrak{z}^2) + \mu_1 \left( 4 + 33 \, \epsilon l \left( \mathfrak{z}^1 - \mathfrak{z}^2 \right) \left( -1 + \mathfrak{z}^2 \right) - \right. \\
& \quad \left. 112 \, \mathfrak{z}^2 + 3 \, \mu_2 \left( 8 + 5 \, \epsilon l \left( \mathfrak{z}^1 - \mathfrak{z}^2 \right) \left( -1 + \mathfrak{z}^2 \right) + 64 \, \mathfrak{z}^2 \right) \right) + \\
& \quad \eta t \left( -50 - 3 \, \epsilon l \, \mathfrak{z}^1 - 22 \, \mathfrak{z}^2 + 3 \, \epsilon l \, \mathfrak{z}^2 - 15 \, \epsilon l \, \mathfrak{z}^1 \, \mathfrak{z}^2 + 15 \, \epsilon l \, \mathfrak{z}^2^2 - \right. \\
& \quad \mu_2 \left( 137 + 15 \, \epsilon l \left( \mathfrak{z}^1 - \mathfrak{z}^2 \right) \left( -1 + \mathfrak{z}^2 \right) + 55 \, \mathfrak{z}^2 \right) + \mu_1^2 \left( 422 + 72 \, \epsilon l \right. \\
& \quad \left. \left( \mathfrak{z}^1 - \mathfrak{z}^2 \right) + 70 \, \mathfrak{z}^2 \right) + \mu_1 \left( 24 - 33 \, \epsilon l \left( \mathfrak{z}^1 - \mathfrak{z}^2 \right) \left( -1 + \mathfrak{z}^2 \right) - \right. \\
& \quad \left. 126 \, \mathfrak{z}^2 + \mu_2 \left( 247 - 15 \, \epsilon l \left( \mathfrak{z}^1 - \mathfrak{z}^2 \right) \left( -1 + \mathfrak{z}^2 \right) + 137 \, \mathfrak{z}^2 \right) \right) \right) \right) + \\
& w^2 \left( 3 \, \epsilon p \left( -4 \times \left( 17 + 9 \, \mu_1^2 \left( -13 + \mathfrak{z}^2 \right) + 19 \, \mathfrak{z}^2 + \mu_2 \left( 36 + 61 \, \mathfrak{z}^2 \right) - \right. \right. \right. \\
& \quad \left. \left. 2 \, \mu_1 \left( 32 - 23 \, \mathfrak{z}^2 + \mu_2 \left( 79 + 18 \, \mathfrak{z}^2 \right) \right) \right) \right) + \right. \\
& \quad \eta t \left( \mu_2 \left( 83 - 11 \, \mathfrak{z}^2 \right) - 36 \times (1 + \mathfrak{z}^2) + 4 \, \mu_1^2 \left( 59 + 13 \, \mathfrak{z}^2 \right) - \right. \\
& \quad \left. \mu_1 \left( 56 \times (-1 + \mathfrak{z}^2) + \mu_2 \left( 61 + 83 \, \mathfrak{z}^2 \right) \right) \right) \right) + \\
& (-1 + \eta t) \, \epsilon l \left( 4 \, \mu_1^2 \left( 65 + \mathfrak{z}^2 \right) - 3 \times (4 + 20 \, \mathfrak{z}^2 + \mu_2 \left( 19 + 5 \, \mathfrak{z}^2 \right)) + \right. \\
& \quad \mu_1 \left( 128 - 116 \, \mathfrak{z}^2 + \mu_2 \left( 87 + 57 \, \mathfrak{z}^2 \right) \right) + 2 \, \epsilon p \left( -2 - 6 \, \mathfrak{z}^1 + 44 \, \mathfrak{z}^2 - \right. \\
& \quad 30 \, \mathfrak{z}^1 \, \mathfrak{z}^2 + 30 \, \mathfrak{z}^2^2 + \mu_2 \left( 82 - 30 \, \mathfrak{z}^1 \left( -1 + \mathfrak{z}^2 \right) + 44 \, \mathfrak{z}^2 + 30 \, \mathfrak{z}^2^2 \right) - \\
& \quad \mu_1^2 \left( 148 + 103 \, \mathfrak{z}^2 + \mathfrak{z}^2^2 - \mathfrak{z}^1 \left( 103 + 5 \, \mathfrak{z}^2 \right) \right) - \\
& \quad \mu_1 \left( 78 - 61 \, \mathfrak{z}^1 - 13 \, \mathfrak{z}^2 + 43 \, \mathfrak{z}^1 \, \mathfrak{z}^2 - 47 \, \mathfrak{z}^2^2 + \right. \\
& \quad \left. 2 \, \mu_2 \left( 79 + 15 \, \mathfrak{z}^1 \left( -1 + \mathfrak{z}^2 \right) + 74 \, \mathfrak{z}^2 + 3 \, \mathfrak{z}^2^2 \right) \right) \right) \right) + w \\
& (-4 \times (-1 + \eta t) \, \epsilon l \, \mu_1 \left( -1 - 11 \, \mathfrak{z}^2 + \mu_1 \left( 23 + \mathfrak{z}^2 \right) \right) + \epsilon p \\
& \left( -60 + 412 \, \mu_2 - 84 \, \mathfrak{z}^2 - 64 \, \mu_2 \, \mathfrak{z}^2 + 4 \, \mu_1^2 \left( -73 + 61 \, \mathfrak{z}^2 \right) - \right. \\
& \quad 4 \, \mu_1 \left( 4 - 82 \, \mathfrak{z}^2 + \mu_2 \left( 71 + 103 \, \mathfrak{z}^2 \right) \right) + \\
& \quad \epsilon l \left( \mu_1^2 \left( 362 + \mathfrak{z}^1 \left( 149 - 29 \, \mathfrak{z}^2 \right) - 137 \, \mathfrak{z}^2 - 9 \, \mathfrak{z}^2^2 \right) - \right. \\
& \quad 6 \times (10 \times (1 + \mathfrak{z}^2) + \mu_2 \left( 5 + 33 \, \mathfrak{z}^2 \right)) + \mu_1 \left( 206 + 29 \, \mathfrak{z}^1 - \right. \\
& \quad \left. 125 \, \mathfrak{z}^2 - 89 \, \mathfrak{z}^1 \, \mathfrak{z}^2 + 51 \, \mathfrak{z}^2^2 + 6 \, \mu_2 \left( 31 + 25 \, \mathfrak{z}^2 + 20 \, \mathfrak{z}^2^2 \right) \right) \right) + \\
& \eta t \left( -4 \times \left( 19 \times (-1 + \mathfrak{z}^2) + 8 \, \mu_1^2 \left( 11 + \mathfrak{z}^2 \right) - 4 \, \mu_2 \left( 7 + 2 \, \mathfrak{z}^2 \right) - \right. \right. \\
& \quad \left. \left. 3 \, \mu_1 \left( 9 + 7 \, \mathfrak{z}^2 \right) + 4 \, \mu_1 \, \mu_2 \left( 11 + 7 \, \mathfrak{z}^2 \right) \right) \right) + \epsilon l \\
& \left( 60 \times (1 + \mathfrak{z}^2) + 6 \, \mu_2 \left( 5 + 33 \, \mathfrak{z}^2 \right) + \mu_1^2 \left( -362 + 137 \, \mathfrak{z}^2 + 9 \, \mathfrak{z}^2^2 + \right. \right. \\
& \quad \left. \left. \mathfrak{z}^1 \left( -149 + 29 \, \mathfrak{z}^2 \right) \right) - \mu_1 \left( 206 + 29 \, \mathfrak{z}^1 - 125 \, \mathfrak{z}^2 - 89 \, \mathfrak{z}^1 \right. \right.
\end{aligned}$$

$$\begin{aligned}
& \left( \frac{\left( 96 (-1 + w (-1 + \eta))^3 (w (-1 + \eta) + x (-1 + \eta) - \eta)^2 \right. \right. \\
& \quad (x + \\
& \quad \eta - \\
& \quad x \\
& \quad \eta)^2 (1 + x + \eta - x \\
& \quad \eta)^2 (-1 + \eta t) \theta l \theta p) \\
& \beta \mu 1 = \\
& \quad \left( f w (-1 + \eta)^2 (-1 + \mu 1 + 2 \mu 1^2) \times (14 x^2 (2 w (-1 + \eta) - 3 \eta) (-1 + \eta)^2 (-1 + \eta + \theta l - \eta t \theta l) \theta p + \right. \\
& \quad 14 x^3 (-1 + \eta)^3 (-1 + \eta + \theta l - \eta t \theta l) \theta p + \\
& \quad x (-1 + \eta) \times (14 (w (-1 + \eta) - 3 \eta) (w (-1 + \eta) - \eta) (-1 + \eta) \theta p - \\
& \quad (-1 + \eta t) \theta l (-10 + 42 \eta^2 \theta p + 5 \theta p (2 + \theta 1 + \theta 2) - 2 w (-1 + \eta) \times (-10 + 28 \eta \\
& \quad \theta p + 5 \theta p (2 + \theta 1 + \theta 2)) + w^2 (-1 + \eta)^2 (-10 + \theta p (24 + 5 \theta 1 + 5 \theta 2))) \Big) + \\
& \quad \theta p (10 \eta t + \eta (-14 \eta^3 + 14 \eta^2 (1 + (-1 + \eta t) \theta l) - 5 \theta l (2 + \theta 1 + \theta 2) + \\
& \quad 5 \eta t (-2 + \theta l (2 + \theta 1 + \theta 2))) - w^2 (-1 + \eta)^2 (-10 \eta t + \\
& \quad \eta (-14 + 14 \eta + 10 \eta t + 24 \theta l + 5 \theta l (\theta 1 + \theta 2) - \eta t \theta l (24 + 5 \theta 1 + 5 \theta 2))) + \\
& \quad 2 w (-1 + \eta) \times (-10 \eta t + \eta (14 \eta^2 - 14 \eta (1 + (-1 + \eta t) \theta l) + 5 \theta l \\
& \quad (2 + \theta 1 + \theta 2) - 5 \eta t (-2 + \theta l (2 + \theta 1 + \theta 2)))) \Big) \Big) / \\
& \quad (48 (-1 + w (-1 + \eta))^2 (x (-1 + \eta) - \eta) (w + x + \eta - (w + x) \eta)^2 (-1 + \eta t) \\
& \quad \theta p)
\end{aligned}$$

$$\begin{aligned}
\beta_{\mu 2} = & - \left( (f w (-1 + \eta))^2 (-2 x^2 (2 w (-1 + \eta) - 3 \eta) \right. \\
& (-1 + \eta)^2 (-1 + \eta + \theta l - \eta t \theta l) \theta p (-1 - \mu 1 + 2 \times (-5 + 7 \mu 1) \mu 2) - \\
& 2 x^3 (-1 + \eta)^3 (-1 + \eta + \theta l - \eta t \theta l) \theta p (-1 - \mu 1 + 2 \times (-5 + 7 \mu 1) \mu 2) - x (-1 + \eta) \times \\
& (2 (w (-1 + \eta) - 3 \eta) (w (-1 + \eta) - \eta) (-1 + \eta) \theta p (-1 - \mu 1 + 2 \times (-5 + 7 \mu 1) \mu 2) - \\
& (-1 + \eta t) \theta l (-2 \times (1 + \mu 1 - 2 \mu 2 + 10 \mu 1 \mu 2) + \eta^2 \theta p \\
& (-6 - 60 \mu 2 + \mu 1 (-6 + 84 \mu 2)) + \theta p (1 + \mu 1 - 2 \mu 2 + 10 \mu 1 \mu 2) \times (2 + \theta 1 + \theta 2) - \\
& 2 w (-1 + \eta) \times (-2 \times (1 + \mu 1 - 2 \mu 2 + 10 \mu 1 \mu 2) + \theta p (-4 \eta (1 + \mu 1) + \\
& 8 \eta (-5 + 7 \mu 1) \mu 2 + (1 + \mu 1 - 2 \mu 2 + 10 \mu 1 \mu 2) \times (2 + \theta 1 + \theta 2))) + \\
& w^2 (-1 + \eta)^2 (-2 + 4 \mu 2 + \theta p (\theta 1 + \theta 2) - 2 \theta p \mu 2 (12 + \theta 1 + \theta 2) + \\
& \mu 1 (-2 + \theta p (\theta 1 + \theta 2) + 2 \mu 2 (-10 + \theta p (24 + 5 \theta 1 + 5 \theta 2)))) \Big) + \\
& \theta p (-2 \eta t (1 + \mu 1 - 2 \mu 2 + 10 \mu 1 \mu 2) - 2 \eta^3 (1 + (-1 + \eta t) \theta l) \times \\
& (-1 - \mu 1 + 2 \times (-5 + 7 \mu 1) \mu 2) + \eta^4 (-2 \times (1 + \mu 1) + 4 \times (-5 + 7 \mu 1) \mu 2) - \\
& \eta (1 + \mu 1 - 2 \mu 2 + 10 \mu 1 \mu 2) (-\theta l (2 + \theta 1 + \theta 2) + \eta t (-2 + \theta l (2 + \theta 1 + \theta 2))) - \\
& 2 w (-1 + \eta) \times (-2 \eta t (1 + \mu 1 - 2 \mu 2 + 10 \mu 1 \mu 2) - 2 \eta^2 (1 + (-1 + \eta t) \theta l) \times \\
& (-1 - \mu 1 + 2 \times (-5 + 7 \mu 1) \mu 2) + \eta^3 (-2 \times (1 + \mu 1) + 4 \times (-5 + 7 \mu 1) \mu 2) - \\
& \eta (1 + \mu 1 - 2 \mu 2 + 10 \mu 1 \mu 2) (-\theta l (2 + \theta 1 + \theta 2) + \eta t (-2 + \theta l (2 + \theta 1 + \theta 2)))) \Big) + \\
& w^2 (-1 + \eta)^2 (-2 \eta t (1 + \mu 1 - 2 \mu 2 + 10 \mu 1 \mu 2) + \eta^2 (-2 \times (1 + \mu 1) + \\
& 4 \times (-5 + 7 \mu 1) \mu 2) + \eta (2 + 4 \times (5 - 6 \theta l) \mu 2 - \theta l (-1 + 2 \mu 2) (\theta 1 + \theta 2) + \\
& \mu 1 (2 + \theta l (\theta 1 + \theta 2) + 2 \mu 2 (-14 + \theta l (24 + 5 \theta 1 + 5 \theta 2)))) + \\
& \eta t (2 + 4 \times (-1 + 6 \theta l) \mu 2 + \theta l (-1 + 2 \mu 2) (\theta 1 + \theta 2) - \\
& \mu 1 (-2 + \theta l (\theta 1 + \theta 2) + 2 \mu 2 (-10 + \theta l (24 + 5 \theta 1 + 5 \theta 2)))) \Big) \Big) / \\
& (48 (-1 + w (-1 + \eta))^2 (x (-1 + \eta) - \eta) (w + x + \eta - (w + x) \eta)^2 \\
& (-1 + \eta t) \\
& \theta p) \Big)
\end{aligned}$$

$$\begin{aligned}
\beta_{cv} = & - \left( (-cv (1 + x + \eta - x \eta)^2 (8 \times (9 cv^2 + 40 u - 12 \epsilon) (-1 + w (-1 + \eta))^3 \right. \\
& (x + \eta - x \eta)^3 (w + x + \eta - w \eta - x \eta)^3 (-1 + \eta t) \theta p + f (-1 + \eta) \times \\
& (2 w^5 (-1 + \eta)^5 (2 \eta^2 \theta p (-30 \eta^4 + \eta^2 (77 - 25 \eta t) - 16 \eta t + 5 \eta^3 (5 + 6 \eta t) + \\
& \eta (-72 + 11 \eta t + 8 \theta l (26 + 5 \theta 1 + 5 \theta 2) - 8 \eta t \theta l (26 + 5 \theta 1 + 5 \theta 2))) + 2 \\
& x^3 (-1 + \eta)^3 ((-1 + \eta) \times (-72 + 30 \eta^2 + \eta (5 - 30 \eta t) - 5 \eta t) \theta p + \\
& 8 \times (-1 + \eta t) \theta l (-2 + \theta p (26 + 5 \theta 1 + 5 \theta 2))) - x^2 (-1 + \eta)^2 (180 \eta^4 \theta p + \\
& 29 \eta t \theta p + \eta (432 + \eta t) \theta p - 30 \eta^3 (5 + 6 \eta t) \theta p + 6 \eta^2 (-77 + 25 \eta t) \theta p + \\
& \eta (-1 + \eta t) \theta l (-67 + 48 \theta p (26 + 5 \theta 1 + 5 \theta 2))) + x (-1 + \eta) \eta \\
& (180 \eta^4 \theta p + \eta (432 - 49 \eta t) \theta p + 79 \eta t \theta p - 30 \eta^3 (5 + 6 \eta t) \theta p + 6 \eta^2 \\
& (-77 + 25 \eta t) \theta p + \eta (-1 + \eta t) \theta l (-17 + 48 \theta p (26 + 5 \theta 1 + 5 \theta 2))) \Big) + \\
& (x + \eta - x \eta)^2 (4 x^4 (-1 + \eta)^4 \theta p (48 + 90 \eta^3 - 6 \eta^2 (24 - 5 \theta l + 5 \eta t (2 + \theta l)) - \\
& 8 \theta l (17 + 3 \theta 2) + \eta t (-27 + 8 \theta l (17 + 3 \theta 2)) + \eta (6 - 27 \theta l + 6 \theta l \theta 2 + \\
& \eta t (87 + 27 \theta l - 6 \theta l \theta 2))) - 16 x^3 (-1 + \eta)^3 (3 \times (-1 + \eta) \eta \\
& (-16 + 30 \eta^2 + 9 \eta t - 2 \eta (9 + 10 \eta t)) \theta p - (-1 + \eta t) \theta l (-4 + \theta p \\
& (30 \eta^3 - 2 \times (2 + 4 \theta 1 + \theta 2) + 3 \eta^2 (-9 + 2 \theta 2) - 8 \eta (17 + 3 \theta 2))) \Big) + \\
& \eta^2 \theta p (360 \eta^5 - 70 \eta t - 24 \eta^4 (24 - 5 \theta l + 5 \eta t (2 + \theta l)) - \\
& 12 \eta^3 (-2 + 9 \theta l - 2 \theta l \theta 2 + \eta t (-29 - 9 \theta l + 2 \theta l \theta 2)) + \\
& \eta (70 \eta t - 101 \theta l \theta 1 - 29 \theta l (2 + \theta 2) + \eta t \theta l (101 \theta 1 + 29 \times (2 + \theta 2))) + \\
& 4 \eta^2 (48 - 8 \theta l (17 + 3 \theta 2) + \eta t (-27 + 8 \theta l (17 + 3 \theta 2))) \Big) - 4 x (-1 + \eta)
\end{aligned}$$

$$\begin{aligned}
& \eta \left( 360 \eta^5 \theta p - 14 \eta t \theta p - 24 \eta^4 (24 - 5 \theta l + 5 \eta t (2 + \theta l)) \theta p + \right. \\
& \quad \eta (14 \eta t \theta p + (-1 + \eta t) \theta l (28 + 87 \theta p \boxplus 1 + 27 \theta p (2 + \boxplus 2))) - \\
& \quad 12 \eta^3 \theta p (-2 + \theta l (9 - 2 \boxplus 2) + \eta t (-29 + \theta l (-9 + 2 \boxplus 2))) + \\
& \quad \left. 4 \eta^2 \theta p (48 - 8 \theta l (17 + 3 \boxplus 2) + \eta t (-27 + 8 \theta l (17 + 3 \boxplus 2))) \right) + x^2 \\
& (-1 + \eta)^2 \left( 2160 \eta^5 \theta p - 94 \eta t \theta p - 144 \eta^4 (24 - 5 \theta l + 5 \eta t (2 + \theta l)) \theta p + \right. \\
& \quad \eta (94 \eta t \theta p + (-1 + \eta t) \theta l (68 + 375 \theta p \boxplus 1 + 111 \theta p (2 + \boxplus 2))) - \\
& \quad 72 \eta^3 \theta p (-2 + \theta l (9 - 2 \boxplus 2) + \eta t (-29 + \theta l (-9 + 2 \boxplus 2))) + \\
& \quad \left. 24 \eta^2 \theta p (48 - 8 \theta l (17 + 3 \boxplus 2) + \eta t (-27 + 8 \theta l (17 + 3 \boxplus 2))) \right) + \\
w & (x (-1 + \eta) - \eta) (-1 + \eta) \times (-4 x^5 (-1 + \eta)^5 \theta p (168 + 90 \eta^3 - 15 \eta^2 \\
& \quad (5 + 6 \eta t) - 4 \theta l (86 + \boxplus 1 + 9 \boxplus 2) + \eta t (-22 + 4 \theta l (86 + \boxplus 1 + 9 \boxplus 2)) + \\
& \quad \eta (-183 + 37 \theta l + 6 \theta l \boxplus 2 + \eta t (112 - 37 \theta l - 6 \theta l \boxplus 2))) + \eta^2 \\
& \theta p (360 \eta^6 - 18 \eta t - 60 \eta^5 (-13 + 6 \eta t) - 4 \eta^4 \\
& \quad (615 - \theta l (127 + 6 \boxplus 2) + \eta t (68 + \theta l (127 + 6 \boxplus 2))) + 4 \eta^3 \\
& \quad (186 - \theta l (425 + 4 \boxplus 1 + 18 \boxplus 2) + \eta t (239 + \theta l (425 + 4 \boxplus 1 + 18 \boxplus 2))) + \\
& \quad 3 \eta^2 (192 - \theta l (602 + 101 \boxplus 1 + 125 \boxplus 2) + \eta t (-38 + \\
& \quad \theta l (602 + 101 \boxplus 1 + 125 \boxplus 2))) + \eta (-\theta l (238 + 239 \boxplus 1 + 135 \boxplus 2) + \\
& \quad \eta t (-192 + \theta l (238 + 239 \boxplus 1 + 135 \boxplus 2))) + 4 x^4 (-1 + \eta)^4 \\
& \left( (-1 + \eta) \times (450 \eta^3 + \eta^2 (345 - 450 \eta t) + 9 \times (-16 + 9 \eta t) - \right. \\
& \quad \left. 2 \eta (501 + 35 \eta t)) \theta p - (-1 + \eta t) \theta l (-48 + \theta p (-24 \times (19 + 4 \boxplus 1 + \right. \\
& \quad \left. 4 \boxplus 2) + 5 \eta^2 (55 + 6 \boxplus 2) - \eta (1801 + 20 \boxplus 1 + 162 \boxplus 2))) \right) + \\
x^2 & (-1 + \eta)^2 (3600 \eta^6 \theta p - 36 \eta t \theta p - 120 \eta^5 (-29 + 30 \eta t) \theta p - \\
& \quad 8 \eta^4 \theta p (2211 - 5 \theta l (91 + 6 \boxplus 2) + 5 \eta t (-4 + \theta l (91 + 6 \boxplus 2))) + \\
& \quad 8 \eta^3 \theta p (894 - \theta l (1963 + 20 \boxplus 1 + 126 \boxplus 2) + \eta t \\
& \quad (673 + \theta l (1963 + 20 \boxplus 1 + 126 \boxplus 2))) + 3 \eta (-138 \eta t \theta p + (-1 + \eta t) \\
& \quad \theta l (-6 + \theta p (250 + 261 \boxplus 1 + 141 \boxplus 2))) + 9 \eta^2 (2 \times (192 - 83 \eta t) \theta p + \\
& \quad (-1 + \eta t) \theta l (60 + \theta p (1234 + 241 \boxplus 1 + 265 \boxplus 2))) - x \\
& (-1 + \eta) \eta (1800 \eta^6 \theta p + 54 \eta t \theta p - 60 \eta^5 (-47 + 30 \eta t) \theta p - \\
& \quad 4 \eta^4 \theta p (2643 - 5 \theta l (109 + 6 \boxplus 2) + 5 \eta t (32 + \theta l (109 + 6 \boxplus 2))) + \\
& \quad 8 \eta^3 \theta p (456 - 2 \theta l (511 + 5 \boxplus 1 + 27 \boxplus 2) + \\
& \quad \eta t (467 + 2 \theta l (511 + 5 \boxplus 1 + 27 \boxplus 2))) + 6 \eta (-72 \eta t \theta p + (-1 + \eta t) \\
& \quad \theta l (15 + \theta p (122 + 125 \boxplus 1 + 69 \boxplus 2))) + 3 \eta^2 (6 \times (128 - 51 \eta t) \theta p + \\
& \quad (-1 + \eta t) \theta l (112 + \theta p (2450 + 449 \boxplus 1 + 521 \boxplus 2))) - x^3 \\
& (-1 + \eta)^3 (3600 \eta^5 \theta p - 120 \eta^4 (-11 + 30 \eta t) \theta p - 8 \eta^3 \theta p \\
& \quad (1779 - 5 \theta l (73 + 6 \boxplus 2) + 5 \eta t (-40 + \theta l (73 + 6 \boxplus 2))) + \\
& \quad 2 \theta p (-8 \theta l (16 + 17 \boxplus 1 + 9 \boxplus 2) + \eta t (-141 + 8 \theta l (16 + 17 \boxplus 1 + 9 \boxplus 2))) + \\
& \quad 16 \eta^2 \theta p (438 - \theta l (941 + 10 \boxplus 1 + 72 \boxplus 2) + \\
& \quad \eta t (206 + \theta l (941 + 10 \boxplus 1 + 72 \boxplus 2))) + 3 \eta ((768 - 338 \eta t) \theta p + \\
& \quad (-1 + \eta t) \theta l (132 + \theta p (2462 + 503 \boxplus 1 + 527 \boxplus 2))) + \\
w^2 & (-1 + \eta)^2 (4 x^6 (-1 + \eta)^6 \theta p (72 + 30 \eta^3 - 5 \eta^2 (5 + 6 \eta t) + \\
& \quad \eta (-77 + 25 \eta t) - 4 \theta l (40 + \boxplus 1 + 3 \boxplus 2) + \eta t (5 + 4 \theta l (40 + \boxplus 1 + 3 \boxplus 2))) - \\
12 & x^5 (-1 + \eta)^5 ((-1 + \eta) \times (-168 + 60 \eta^3 + 22 \eta t - 20 \eta^2 \\
& \quad (-5 + 3 \eta t) - \eta (129 + 100 \eta t)) \theta p + (-1 + \eta t) \theta l \\
& \quad (16 + 4 \theta p (90 + 9 \boxplus 1 + 11 \boxplus 2) + \eta \theta p (283 + 8 \boxplus 1 + 18 \boxplus 2))) + \\
& \eta^2 \theta p (120 \eta^7 + 64 \eta t - 20 \eta^6 (-49 + 6 \eta t) - 4 \eta^5 (32 + 245 \eta t) +
\end{aligned}$$

$$\begin{aligned}
& 4 \eta^4 (-909 + \eta t (161 + \theta l (-41 + 4 \mathfrak{z}1 - 6 \mathfrak{z}2)) + \theta l (41 - 4 \mathfrak{z}1 + 6 \mathfrak{z}2)) + \\
& 2 \eta (-8 \theta l (12 + 9 \mathfrak{z}1 + 7 \mathfrak{z}2) + \eta t (-59 + 8 \theta l (12 + 9 \mathfrak{z}1 + 7 \mathfrak{z}2))) + \\
& 3 \eta^3 (696 - \theta l (1542 + 117 \mathfrak{z}1 + 149 \mathfrak{z}2) + \eta t (330 + \theta l (1542 + 117 \mathfrak{z}1 + \\
& \quad 149 \mathfrak{z}2))) + 3 \eta^2 (192 - \theta l (782 + 239 \mathfrak{z}1 + 231 \mathfrak{z}2) + \\
& \quad \eta t (-160 + \theta l (782 + 239 \mathfrak{z}1 + 231 \mathfrak{z}2))) + x^2 (-1 + \eta)^2 \\
& (1800 \eta^7 \theta p + 58 \eta t \theta p - 300 \eta^6 (-31 + 6 \eta t) \theta p - 60 \eta^5 (119 + 155 \eta t) \theta p + \\
& \quad 12 \eta^4 \theta p (-2334 + 785 \eta t - 10 \theta l (25 + 2 \mathfrak{z}1) + 5 \eta t \theta l (50 + 4 \mathfrak{z}1)) + \\
& \quad 2 \eta (-2 \eta t \theta p + (-1 + \eta t) \theta l (-67 + 24 \theta p (12 + 9 \mathfrak{z}1 + 7 \mathfrak{z}2))) + \\
& \quad 12 \eta^3 ((1716 + 371 \eta t) \theta p + (-1 + \eta t) \theta l \\
& \quad \quad (73 + \theta p (3780 + 333 \mathfrak{z}1 + 413 \mathfrak{z}2))) + 9 \eta^2 (384 \theta p - 314 \eta t \theta p + \\
& \quad \quad (-1 + \eta t) \theta l (24 + \theta p (1582 + 511 \mathfrak{z}1 + 471 \mathfrak{z}2))) + 3 x^4 (-1 + \eta)^4 \\
& (600 \eta^5 \theta p - 100 \eta^4 (-13 + 6 \eta t) \theta p - 20 \eta^3 (134 + 65 \eta t) \theta p + 4 \eta^2 \theta p \\
& \quad (-699 - 5 \theta l (117 + 4 \mathfrak{z}1 + 6 \mathfrak{z}2) + 5 \eta t (105 + \theta l (117 + 4 \mathfrak{z}1 + 6 \mathfrak{z}2))) + \\
& \quad 2 \theta p (96 - 8 \theta l (50 + 17 \mathfrak{z}1 + 15 \mathfrak{z}2) + \eta t \\
& \quad \quad (-101 + 8 \theta l (50 + 17 \mathfrak{z}1 + 15 \mathfrak{z}2))) + \eta (2 \times (1692 + \eta t) \theta p + \\
& \quad \quad (-1 + \eta t) \theta l (196 + \theta p (7338 + 711 \mathfrak{z}1 + 871 \mathfrak{z}2))) - x \\
& (-1 + \eta) \eta (720 \eta^7 \theta p + 158 \eta t \theta p - 240 \eta^6 (-20 + 3 \eta t) \theta p - \\
& \quad 12 \eta^5 (169 + 400 \eta t) \theta p + 12 \eta^4 \theta p \\
& \quad \quad (-1347 + \eta t (330 + \theta l (15 + 8 \mathfrak{z}1 - 6 \mathfrak{z}2)) + \theta l (-15 - 8 \mathfrak{z}1 + 6 \mathfrak{z}2)) + \\
& \quad \eta (-50 \eta t \theta p + 2 \times (-1 + \eta t) \theta l (-17 + 24 \theta p (12 + 9 \mathfrak{z}1 + 7 \mathfrak{z}2))) + \\
& \quad 6 \eta^3 (2 \times (864 + 287 \eta t) \theta p + (-1 + \eta t) \theta l \\
& \quad \quad (56 + \theta p (3822 + 315 \mathfrak{z}1 + 395 \mathfrak{z}2))) + 3 \eta^2 (8 \times (96 - 83 \eta t) \theta p + \\
& \quad \quad (-1 + \eta t) \theta l (90 + \theta p (3146 + 989 \mathfrak{z}1 + 933 \mathfrak{z}2))) - x^3 \\
& (-1 + \eta)^3 (4 \times (-1 + \eta) \times (600 \eta^5 + \eta^3 (90 - 2800 \eta t) + 27 \eta t - \\
& \quad 200 \eta^4 (-14 + 3 \eta t) - 12 \eta^2 (474 + 5 \eta t) + \eta (-576 + 507 \eta t)) \theta p + \\
& \quad (-1 + \eta t) \theta l (40 \eta^3 \theta p (173 + 8 \mathfrak{z}1 + 6 \mathfrak{z}2) + 16 \times (-4 + \theta p \\
& \quad \quad (12 + 9 \mathfrak{z}1 + 7 \mathfrak{z}2)) + 6 \eta^2 (156 + \theta p (7458 + 693 \mathfrak{z}1 + 853 \mathfrak{z}2)) + \\
& \quad \quad 3 \eta (-18 + \theta p (3182 + 1055 \mathfrak{z}1 + 951 \mathfrak{z}2))) + w^4 (-1 + \eta)^4 \\
& (4 x^4 (-1 + \eta)^4 \theta p (216 + 90 \eta^3 - 15 \eta^2 (5 + 6 \eta t) + 3 \eta (-77 + 25 \eta t) - \\
& \quad 8 \theta l (68 + 10 \mathfrak{z}1 + 9 \mathfrak{z}2) + \eta t (15 + 8 \theta l (68 + 10 \mathfrak{z}1 + 9 \mathfrak{z}2))) + \eta^2 \\
& \theta p (360 \eta^5 + 192 \eta t - 12 \eta^3 (102 + 5 \eta t) - 60 \eta^4 (-1 + 6 \eta t) + \\
& \quad 2 \eta (336 - 16 \theta l (61 + 14 \mathfrak{z}1 + 15 \mathfrak{z}2) + \\
& \quad \quad \eta t (-149 + 16 \theta l (61 + 14 \mathfrak{z}1 + 15 \mathfrak{z}2))) + \eta^2 (132 - \theta l (2010 + \\
& \quad \quad 287 \mathfrak{z}1 + 255 \mathfrak{z}2) + \eta t (526 + \theta l (2010 + 287 \mathfrak{z}1 + 255 \mathfrak{z}2))) + 3 \\
& x^2 (-1 + \eta)^2 (720 \eta^5 \theta p + 58 \eta t \theta p + 12 \eta^3 (-179 + 20 \eta t) \theta p - \\
& \quad 240 \eta^4 (\theta p + 3 \eta t \theta p) + 2 \eta (14 \times (24 - 5 \eta t) \theta p + (-1 + \eta t) \theta l \\
& \quad \quad (-67 + 16 \theta p (61 + 14 \mathfrak{z}1 + 15 \mathfrak{z}2))) + \eta^2 (2 \times (498 + 281 \eta t) \theta p + \\
& \quad \quad (-1 + \eta t) \theta l (24 + \theta p (4186 + 607 \mathfrak{z}1 + 543 \mathfrak{z}2))) - x \\
& (-1 + \eta) \eta (1440 \eta^5 \theta p + 474 \eta t \theta p + 12 \eta^3 (-383 + 10 \eta t) \theta p - \\
& \quad 120 \eta^4 (\theta p + 12 \eta t \theta p) + 6 \eta (3 \times (112 - 39 \eta t) \theta p + (-1 + \eta t) \theta l \\
& \quad \quad (-17 + 16 \theta p (61 + 14 \mathfrak{z}1 + 15 \mathfrak{z}2))) + \eta^2 (36 \times (35 + 43 \eta t) \theta p + \\
& \quad \quad (-1 + \eta t) \theta l (90 + \theta p (8206 + 1181 \mathfrak{z}1 + 1053 \mathfrak{z}2))) - \\
& x^3 (-1 + \eta)^3 (4 \times (-1 + \eta) \times (-168 + 360 \eta^3 + 31 \eta t - 30 \eta^2 \\
& \quad (-5 + 12 \eta t) - 3 \eta (283 + 50 \eta t)) \theta p + \\
& \quad (-1 + \eta t) \theta l (32 \times (-6 + \theta p (61 + 14 \mathfrak{z}1 + 15 \mathfrak{z}2)) +
\end{aligned}$$

$$\begin{aligned}
& \eta (-18 + \text{ep} (8538 + 1247 \, \mathfrak{x}1 + 1119 \, \mathfrak{x}2))) + w^3 (-1 + \eta)^3 \\
& (4 \, x^5 (-1 + \eta)^5 (3 \times (-1 + \eta) \times (-72 + 30 \, \eta^2 + \eta (5 - 30 \, \eta t) - 5 \, \eta t) \, \text{ep} + \\
& 4 \times (-1 + \eta) \, \text{el} (4 + \text{ep} (124 + 11 \, \mathfrak{x}1 + 11 \, \mathfrak{x}2))) - x^4 (-1 + \eta)^4 \\
& (1800 \, \eta^4 \, \text{ep} + 60 \, \eta^2 (-92 + 7 \, \eta t) \, \text{ep} - 60 \, \eta^3 (7 + 30 \, \eta t) \, \text{ep} + \\
& 2 \, \eta (1062 + 869 \, \eta t) \, \text{ep} - 288 \, \text{ep} (-7 + \text{el} (17 + 3 \, \mathfrak{x}1 + 3 \, \mathfrak{x}2)) + \\
& 2 \, \eta t \, \text{ep} (-179 + 144 \, \text{el} (17 + 3 \, \mathfrak{x}1 + 3 \, \mathfrak{x}2)) + \\
& \eta (-1 + \eta t) \, \text{el} (196 + \text{ep} (9506 + 871 \, \mathfrak{x}1 + 823 \, \mathfrak{x}2))) + x (-1 + \eta) \, \eta \\
& (1800 \, \eta^6 \, \text{ep} + 474 \, \eta t \, \text{ep} - 60 \, \eta^5 (-47 + 30 \, \eta t) \, \text{ep} - 60 \, \eta^4 (119 + 47 \, \eta t) \, \text{ep} + \\
& 6 \, \eta ((96 - 115 \, \eta t) \, \text{ep} + (-1 + \eta t) \, \text{el} (-17 + 8 \, \text{ep} (70 + 27 \, \mathfrak{x}1 + 27 \, \mathfrak{x}2))) + \\
& 2 \, \eta^3 (8 \times (-387 + 322 \, \eta t) \, \text{ep} + (-1 + \eta t) \, \text{el} \\
& (56 + \text{ep} (3898 + 395 \, \mathfrak{x}1 + 299 \, \mathfrak{x}2))) + \eta^2 (4 \times (2034 - 79 \, \eta t) \, \text{ep} + \\
& 9 \times (-1 + \eta t) \, \text{el} (30 + \text{ep} (2194 + 351 \, \mathfrak{x}1 + 367 \, \mathfrak{x}2))) - x^2 \\
& (-1 + \eta)^2 (3600 \, \eta^6 \, \text{ep} + 174 \, \eta t \, \text{ep} - 120 \, \eta^4 (113 + 29 \, \eta t) \, \text{ep} - \\
& 120 \, \eta^5 (-29 + 30 \, \eta t) \, \text{ep} + 6 \, \eta ((96 - 74 \, \eta t) \, \text{ep} + \\
& (-1 + \eta t) \, \text{el} (-67 + 8 \, \text{ep} (70 + 27 \, \mathfrak{x}1 + 27 \, \mathfrak{x}2))) + \\
& 4 \, \eta^3 (3 \times (-522 + 685 \, \eta t) \, \text{ep} + (-1 + \eta t) \, \text{el} (73 + \text{ep} \\
& (4222 + 413 \, \mathfrak{x}1 + 341 \, \mathfrak{x}2))) + 3 \, \eta^2 ((4056 - 290 \, \eta t) \, \text{ep} + \\
& 3 \times (-1 + \eta t) \, \text{el} (24 + \text{ep} (3282 + 543 \, \mathfrak{x}1 + 559 \, \mathfrak{x}2))) - \eta^2 \\
& \text{ep} (360 \, \eta^6 + 192 \, \eta t - 60 \, \eta^5 (-13 + 6 \, \eta t) - 12 \, \eta^4 (122 + 65 \, \eta t) + \\
& \eta^3 (-1908 - 149 \, \text{el} \, \mathfrak{x}1 - 101 \, \text{el} (14 + \mathfrak{x}2) + \\
& \eta t (1234 + 149 \, \text{el} \, \mathfrak{x}1 + 101 \, \text{el} (14 + \mathfrak{x}2))) + 2 \, \eta (96 - \\
& 8 \, \text{el} (70 + 27 \, \mathfrak{x}1 + 27 \, \mathfrak{x}2) + \eta t (-177 + 8 \, \text{el} (70 + 27 \, \mathfrak{x}1 + 27 \, \mathfrak{x}2))) + \\
& \eta^2 (2040 - 3 \, \text{el} (1650 + 255 \, \mathfrak{x}1 + 271 \, \mathfrak{x}2) + \eta t \\
& (68 + \text{el} (4950 + 765 \, \mathfrak{x}1 + 813 \, \mathfrak{x}2))) + x^3 (-1 + \eta)^3 \\
& (4 \times (-1 + \eta) \times (900 \, \eta^4 + 6 \times (-8 + 9 \, \eta t) - 30 \, \eta^3 (-41 + 30 \, \eta t) - \\
& 30 \, \eta^2 (63 + 41 \, \eta t) + 5 \, \eta (-414 + 53 \, \eta t)) \, \text{ep} + \\
& (-1 + \eta t) \, \text{el} (16 \times (-12 + \text{ep} (70 + 27 \, \mathfrak{x}1 + 27 \, \mathfrak{x}2)) + \\
& 2 \, \eta^2 (156 + \text{ep} (9014 + 853 \, \mathfrak{x}1 + 757 \, \mathfrak{x}2)) + \\
& 3 \, \eta (-18 + \text{ep} (6546 + 1119 \, \mathfrak{x}1 + 1135 \, \mathfrak{x}2)))) + \\
& 8 \, \text{cof} (-1 + \eta)^2 (w^5 (-1 + \eta)^6 (2 \, x^5 (-1 + \eta)^5 \, \text{ep} (\eta - \eta t + 4 \, \mu1) - \\
& 2 \, x^4 (-1 + \eta)^3 ((-1 + \eta t) \, \text{el} (-4 + 4 \, \mu1 + \mu2) + (-1 + \eta) \, \text{ep} \\
& (4 + 5 \, \eta^2 + 12 \, \mu1 + \eta (2 - 5 \, \eta t + 20 \, \mu1 - 7 \, \mu2) + \eta t (-2 + 7 \, \mu2))) - \\
& 2 \, \eta \, \text{ep} (\eta^5 + \eta t \, \mu2 + 2 \, \eta \, \eta t (-2 - 2 \, \mu1 + \mu2) - \eta^4 (-2 + \eta t - 4 \, \mu1 + 7 \, \mu2) + \\
& \eta^3 (5 + 12 \, \mu1 - 13 \, \mu2 + \eta t (-2 + 7 \, \mu2)) + \eta^2 \\
& (4 + 8 \, \mu1 + 8 \, \mu2 + \eta t (-5 + 10 \, \mu1 + 8 \, \mu2))) + \\
& x (10 \, \eta^6 \, \text{ep} + \eta^3 (-2 \, \text{ep} (7 + 24 \, \mu1 - 63 \, \mu2) + \eta t \, \text{ep} (-11 + 53 \, \mu1 - 5 \, \mu2) + \\
& (-1 + \eta t) \, \text{el} (-11 + 15 \, \mu1 - \mu2)) + 2 \, \eta^5 \\
& \text{ep} (3 - 5 \, \eta t + 20 \, \mu1 - 28 \, \mu2) - \eta t \, \text{ep} (3 + 3 \, \mu1 + 5 \, \mu2) + \eta \\
& (\eta t \, \text{ep} (13 + 11 \, \mu1 - 9 \, \mu2) - (-1 + \eta t) \, \text{el} (3 + 3 \, \mu1 + \mu2)) + 2 \\
& \eta^4 \, \text{ep} (11 + 28 \, \mu1 - 11 \, \mu2 + \eta t (-3 + 28 \, \mu2)) - \eta^2 \\
& (2 \times (-1 + \eta t) \, \text{el} (7 + 8 \, \mu1 + \mu2) + \\
& 24 \, \text{ep} (1 + 2 \, \mu1 + 2 \, \mu2) + \eta t \, \text{ep} (-17 + 61 \, \mu1 + 37 \, \mu2))) - \\
& 2 \, x^2 (-1 + \eta) \times (10 \, \eta^5 \, \text{ep} + 2 \, \eta^4 \, \text{ep} (1 - 5 \, \eta t + 20 \, \mu1 - 21 \, \mu2) - \text{el} \\
& \mu2 + \eta t (\text{ep} + \text{el} \, \mu2 - 5 \, \text{ep} \, \mu2) - \eta ((-1 + \eta t) \, \text{el} (11 + 12 \, \mu1 - \mu2) +
\end{aligned}$$



$$\begin{aligned}
& 12 \, \theta p \, (1 + 2 \, \mu_1 + 2 \, \mu_2) + \eta t \, \theta p \, (-11 + 23 \, \mu_1 + 22 \, \mu_2) + \eta^3 \\
& \theta p \, (32 \, \mu_1 + 3 \times (5 + \mu_2) + \eta t \, (-2 + 42 \, \mu_2)) + \eta^2 \, ((-1 + \eta t) \, \theta l \\
& (-15 + 19 \, \mu_1) + \theta p \, (-15 - 48 \, \mu_1 + 23 \, \eta t \, \mu_1 + 63 \, \mu_2 - 15 \, \eta t \, \mu_2)) + \\
& x^3 \, (-1 + \eta)^2 \, ((-1 + \eta t) \, \theta l \, (-8 - 8 \, \mu_1 + 31 \, \eta \, \mu_1 + 3 \, \eta \, (-9 + \mu_2) + 4 \, \mu_2) + \\
& (-1 + \eta) \, \theta p \, (20 \, \eta^3 + 8 \times (1 + 2 \, \mu_1 + 2 \, \mu_2) - 4 \, \eta^2 \, (-4 + 5 \, \eta t - 20 \, \mu_1 + 14 \, \mu_2) + \\
& \eta t \, (-7 + 13 \, \mu_1 + 19 \, \mu_2) + 2 \, \eta \, (17 + 48 \, \mu_1 - 13 \, \mu_2 + 4 \, \eta t \, (-2 + 7 \, \mu_2))) + \\
& w^4 \, (-1 + \eta)^4 \, (6 \, x^6 \, (-1 + \eta)^7 \, \theta p \, (\eta - \eta t + 4 \, \mu_1) + \eta \, \theta p \, (6 \, \eta^7 + \eta^6 \\
& (16 - 6 \, \eta t + 24 \, \mu_1 - 42 \, \mu_2) + 12 \, \eta \, \eta t \, (1 + \mu_1 - 2 \, \mu_2) - 6 \\
& \eta t \, \mu_2 + 2 \, \eta^5 \, (29 + 39 \, \mu_1 - 39 \, \mu_2 + \eta t \, (-8 + 21 \, \mu_2)) + \eta^4 \\
& (50 + 42 \, \mu_1 + 130 \, \mu_2 + 3 \, \theta l \, (\mu_2 \, (6 + 3 \, \mu_1 - \mu_2) + 3 \times (6 + \mu_1 + \mu_2) + \\
& \mu_1 \, (18 + \mu_1 + 5 \, \mu_2)) - \eta t \, (4 - 110 \, \mu_1 - 46 \, \mu_2 + \\
& 3 \, \theta l \, (\mu_2 \, (6 + 3 \, \mu_1 - \mu_2) + 3 \times (6 + \mu_1 + \mu_2) + \mu_1 \, (18 + \mu_1 + 5 \, \mu_2))) - \\
& 2 \, \eta^3 \, (32 + 39 \, \mu_1 - 25 \, \mu_2 - 3 \, \theta l \, (\mu_2 \, (6 + 3 \, \mu_1 - \mu_2) + 3 \times (6 + \mu_1 + \mu_2) + \\
& \mu_1 \, (18 + \mu_1 + 5 \, \mu_2)) + \eta t \, (-2 + 20 \, \mu_1 + 9 \, \mu_2 + \\
& 3 \, \theta l \, (\mu_2 \, (6 + 3 \, \mu_1 - \mu_2) + 3 \times (6 + \mu_1 + \mu_2) + \mu_1 \, (18 + \mu_1 + 5 \, \mu_2))) - \\
& \eta^2 \, (66 + 66 \, \mu_1 + 60 \, \mu_2 - 3 \, \theta l \, (\mu_2 \, (6 + 3 \, \mu_1 - \mu_2) + 3 \times (6 + \mu_1 + \mu_2) + \\
& \mu_1 \, (18 + \mu_1 + 5 \, \mu_2)) + \eta t \, (-10 + 82 \, \mu_1 + 40 \, \mu_2 + \\
& 3 \, \theta l \, (\mu_2 \, (6 + 3 \, \mu_1 - \mu_2) + 3 \times (6 + \mu_1 + \mu_2) + \mu_1 \, (18 + \mu_1 + 5 \, \mu_2)))) - \\
& x^5 \, (-1 + \eta)^5 \, (6 \times (-1 + \eta t) \, \theta l \, (10 \, \mu_1 + 3 \, \mu_2) + \theta p \, (36 \, \eta^3 - 6 \times \\
& (9 + 17 \, \mu_1) - 2 \, \eta^2 \, (7 + 18 \, \eta t - 72 \, \mu_1 + 21 \, \mu_2) + \\
& 2 \, \eta \, (16 - 21 \, \mu_1 + 21 \, \mu_2 + 7 \, \eta t \, (1 + 3 \, \mu_2)) + 3 \, \theta l \, (\mu_2 \, (6 + 3 \, \mu_1 - \mu_2) + \\
& 3 \times (6 + \mu_1 + \mu_2) + \mu_1 \, (18 + \mu_1 + 5 \, \mu_2)) - \eta t \, (-22 + 42 \, \mu_2 + \\
& 3 \, \theta l \, (\mu_2 \, (6 + 3 \, \mu_1 - \mu_2) + 3 \times (6 + \mu_1 + \mu_2) + \mu_1 \, (18 + \mu_1 + 5 \, \mu_2)))) + \\
& x^2 \, (-1 + \eta)^2 \, (90 \, \eta^6 \, \theta p - 10 \, \eta^5 \, \theta p \, (-13 + 9 \, \eta t - 36 \, \mu_1 + 42 \, \mu_2) - 6 \\
& (\theta l \, \mu_2 - \eta t \, \theta l \, \mu_2 + \eta t \, \theta p \, (2 + 3 \, \mu_1 + 9 \, \mu_2)) + 2 \, \eta^4 \, \theta p \\
& (238 + 330 \, \mu_1 - 150 \, \mu_2 + 5 \, \eta t \, (-13 + 42 \, \mu_2)) - 3 \, \eta \\
& (2 \, \theta p \, (33 + 33 \, \mu_1 + 30 \, \mu_2 + \eta t \, (-6 + 31 \, \mu_1 + 33 \, \mu_2)) + \\
& (-1 + \eta t) \, \theta l \, (2 \times (8 + 9 \, \mu_1 - 6 \, \mu_2) + \\
& 3 \, \theta p \, (\mu_2 \, (6 + 3 \, \mu_1 - \mu_2) + 3 \times (6 + \mu_1 + \mu_2) + \mu_1 \, (18 + \mu_1 + 5 \, \mu_2))) - \\
& 2 \, \eta^3 \, (-\theta p \, (27 - 78 \, \mu_1 + 501 \, \mu_2 + \eta t \, (41 + 288 \, \mu_1 + 63 \, \mu_2)) + \\
& 3 \times (-1 + \eta t) \, \theta l \, (3 - 54 \, \mu_1 - 9 \, \mu_2 + 5 \, \theta p \\
& (\mu_2 \, (6 + 3 \, \mu_1 - \mu_2) + 3 \times (6 + \mu_1 + \mu_2) + \mu_1 \, (18 + \mu_1 + 5 \, \mu_2))) - 6 \\
& \eta^2 \, (\theta p \, (92 + 111 \, \mu_1 + 17 \, \mu_2 + \eta t \, (-19 + 62 \, \mu_1 + 49 \, \mu_2)) + \\
& (-1 + \eta t) \, \theta l \, (13 - 13 \, \mu_1 - 14 \, \mu_2 + 6 \, \theta p \\
& (\mu_2 \, (6 + 3 \, \mu_1 - \mu_2) + 3 \times (6 + \mu_1 + \mu_2) + \mu_1 \, (18 + \mu_1 + 5 \, \mu_2)))) + \\
& x^3 \, (-1 + \eta)^3 \, (-((-1 + \eta) \, \theta p \, (66 + 120 \, \eta^4 + 66 \, \mu_1 + 60 \, \mu_2 - 20 \, \eta^3 \\
& (-11 + 6 \, \eta t - 24 \, \mu_1 + 21 \, \mu_2) + \eta t \, (-1 + 67 \, \mu_1 + 91 \, \mu_2) + \\
& 4 \, \eta^2 \, (161 + 255 \, \mu_1 - 120 \, \mu_2 + 5 \, \eta t \, (-11 + 21 \, \mu_2)) + \\
& \eta \, (490 + 576 \, \mu_1 + 262 \, \mu_2 + \eta t \, (-86 + 356 \, \mu_1 + 370 \, \mu_2)))) + \\
& 3 \times (-1 + \eta t) \, \theta l \, (4 + 4 \, \mu_1 - 10 \, \mu_2 + \theta p \, (\mu_2 \, (6 + 3 \, \mu_1 - \mu_2) + \\
& 3 \times (6 + \mu_1 + \mu_2) + \mu_1 \, (18 + \mu_1 + 5 \, \mu_2)) + 2 \, \eta^2 \, (3 - 74 \, \mu_1 - 15 \, \mu_2 + \\
& 5 \, \theta p \, (\mu_2 \, (6 + 3 \, \mu_1 - \mu_2) + 3 \times (6 + \mu_1 + \mu_2) + \mu_1 \, (18 + \mu_1 + 5 \, \mu_2))) + \\
& \eta \, (19 - 25 \, \mu_1 - 35 \, \mu_2 + 8 \, \theta p \, (\mu_2 \, (6 + 3 \, \mu_1 - \mu_2) + \\
& 3 \times (6 + \mu_1 + \mu_2) + \mu_1 \, (18 + \mu_1 + 5 \, \mu_2)))) + \\
& x^4 \, (-1 + \eta)^4 \, (2 \times (-1 + \eta) \, \theta p \, (60 + 45 \, \eta^3 + 72 \, \mu_1 + 42 \, \mu_2 - 5 \, \eta^2
\end{aligned}$$

$$\begin{aligned}
& (-11 + 9 \eta t - 36 \mu_1 + 21 \mu_2) + \eta t (-10 + 41 \mu_1 + 47 \mu_2) + \\
& \eta (148 + 255 \mu_1 - 60 \mu_2 + 5 \eta t (-11 + 21 \mu_2)) - (-1 + \eta t) \theta l \\
& (6 \times (2 - 4 \mu_1 - 7 \mu_2 + \theta p (\mu_2 (6 + 3 \mu_1 - \mu_2) + 3 \times (6 + \mu_1 + \mu_2) + \\
& \mu_1 (18 + \mu_1 + 5 \mu_2))) + \eta (6 - 268 \mu_1 - 66 \mu_2 + 15 \theta p \\
& (\mu_2 (6 + 3 \mu_1 - \mu_2) + 3 \times (6 + \mu_1 + \mu_2) + \mu_1 (18 + \mu_1 + 5 \mu_2)))) - \\
& \times (-1 + \eta) \times (36 \eta^7 \theta p + 2 \eta^6 \theta p (37 - 18 \eta t + 72 \mu_1 - 105 \mu_2) - 3 \\
& \eta t \theta p (3 + 3 \mu_1 + 5 \mu_2) + \eta \\
& (3 \eta t \theta p (3 + \mu_1 - 23 \mu_2) - 3 \times (-1 + \eta t) \theta l (3 + 3 \mu_1 + \mu_2)) + 2 \\
& \eta^5 \theta p (3 \times (44 + 61 \mu_1 - 45 \mu_2) + \eta t (-37 + 105 \mu_2)) - 3 \\
& \eta^2 (\theta p (66 + 66 \mu_1 + 60 \mu_2 + \eta t (-15 + 67 \mu_1 + 49 \mu_2)) + \\
& (-1 + \eta t) \theta l (2 \times (6 + 7 \mu_1 - \mu_2) + 3 \theta p \\
& (\mu_2 (6 + 3 \mu_1 - \mu_2) + 3 \times (6 + \mu_1 + \mu_2) + \mu_1 (18 + \mu_1 + 5 \mu_2)))) - \\
& \eta^3 (\theta p (6 \times (52 + 63 \mu_1 - 11 \mu_2) + \eta t (-53 + 205 \mu_1 + 127 \mu_2)) + \\
& 3 \times (-1 + \eta t) \theta l (11 - 9 \mu_1 - 7 \mu_2 + 8 \theta p \\
& (\mu_2 (6 + 3 \mu_1 - \mu_2) + 3 \times (6 + \mu_1 + \mu_2) + \mu_1 (18 + \mu_1 + 5 \mu_2)))) + \\
& \eta^4 (2 \theta p (68 + 33 \mu_1 + 297 \mu_2 + \eta t (6 + 206 \mu_1 + 74 \mu_2)) - \\
& (-1 + \eta t) \theta l (6 - 88 \mu_1 - 12 \mu_2 + 15 \theta p \\
& (\mu_2 (6 + 3 \mu_1 - \mu_2) + 3 \times (6 + \mu_1 + \mu_2) + \mu_1 (18 + \mu_1 + 5 \mu_2)))) + \\
& w^3 (-1 + \eta)^3 (6 x^7 (-1 + \eta)^8 \theta p (\eta - \eta t + 4 \mu_1) - x^6 (-1 + \eta)^6 \\
& (6 \times (-1 + \eta) \theta p (19 + 7 \eta^2 + 27 \mu_1 + 7 \eta t (-1 + \mu_2) - 7 \eta (-1 + \eta t - 4 \mu_1 + \mu_2)) + \\
& (-1 + \eta t) \theta l (78 \mu_1 - 2 \times (3 + \mu_2) + \\
& \theta p (-108 - 12 \mu_2 - \mu_1 + \mu_1 (-96 + 9 \mu_1 - 17 \mu_2) - 5 \mu_2 + 22 \mu_2 \mu_2))) + \\
& \eta \theta p (-6 \eta^8 + 6 \eta t \mu_2 + 12 \eta \eta t (1 + \mu_1 + 5 \mu_2) + 6 \eta^7 (-6 + \eta t - 4 \mu_1 + 7 \mu_2) - \\
& 2 \eta^6 (77 + 69 \mu_1 - 81 \mu_2 + 3 \eta t (-6 + 7 \mu_2)) - \eta^5 (2 \times (76 + 88 \mu_1 + 55 \mu_2) + \\
& \theta l (122 + 4 \mu_1 + \mu_2 (14 + 3 \mu_1 - 19 \mu_2) - 2 \mu_1 (-55 + \mu_1 - 12 \mu_2) + 8 \mu_2) + \\
& \eta t (-32 + 166 \mu_1 + 88 \mu_2 - \theta l (122 + 4 \mu_1 + \mu_2 (14 + 3 \mu_1 - 19 \mu_2) - \\
& 2 \mu_1 (-55 + \mu_1 - 12 \mu_2) + 8 \mu_2))) + \eta^3 (4 \times (47 + 50 \mu_1 + 31 \mu_2) - \\
& \theta l (230 + 56 \mu_1 + \mu_2 (122 + 57 \mu_1 - 17 \mu_2) + 52 \mu_2 + 10 \mu_1 \\
& (29 + \mu_1 + 8 \mu_2))) + \eta t (-50 + 210 \mu_1 + 28 \mu_2 + \theta l (230 + 56 \mu_1 + \\
& \mu_2 (122 + 57 \mu_1 - 17 \mu_2) + 52 \mu_2 + 10 \mu_1 (29 + \mu_1 + 8 \mu_2)))) + \eta^2 \\
& (42 + 70 \mu_1 + 60 \mu_2 - \theta l (54 + 26 \mu_1 + 22 \mu_2 + \mu_2 (54 + 27 \mu_1 + \mu_2) + \\
& \mu_1 (90 + 6 \mu_1 + 28 \mu_2)) + \eta t (-12 + 38 \mu_1 + 66 \mu_2 + \theta l (54 + 26 \mu_1 + \\
& 22 \mu_2 + \mu_2 (54 + 27 \mu_1 + \mu_2) + \mu_1 (90 + 6 \mu_1 + 28 \mu_2)))) + \eta^4 \\
& (118 + 68 \mu_1 - 278 \mu_2 - \theta l (298 + 34 \mu_1 + \mu_2 (82 + 33 \mu_1 - 37 \mu_2) + \\
& 38 \mu_2 + 2 \mu_1 (155 + \mu_1 + 38 \mu_2)) + \eta t \\
& (-2 \times (12 + 47 \mu_1 + 15 \mu_2) + \theta l (298 + 34 \mu_1 + \mu_2 (82 + 33 \mu_1 - 37 \mu_2) + \\
& 38 \mu_2 + 2 \mu_1 (155 + \mu_1 + 38 \mu_2)))) + x^5 (-1 + \eta)^5 \\
& ((-1 + \eta) \theta p (126 \eta^3 + \eta (766 + 972 \mu_1 + 252 \eta t (-1 + \mu_2) - 204 \mu_2) - \\
& 126 \eta^2 (-2 + \eta t - 4 \mu_1 + 2 \mu_2) + 26 \times (11 + 13 \mu_1 + 6 \mu_2) + \\
& \eta t (-77 + 107 \mu_1 + 127 \mu_2)) + (-1 + \eta t) \theta l \\
& (-16 + 88 \mu_1 + 50 \mu_2 - \theta p (270 + 28 \mu_1 + \mu_2 (78 + 27 \mu_1 - 43 \mu_2) + 32 \mu_2 + \\
& \mu_1 (282 - 12 \mu_1 + 62 \mu_2)) + \eta (-27 + 449 \mu_1 - 7 \mu_2 - \theta p (662 + 9 \mu_1 + \\
& \mu_2 (74 + 3 \mu_1 - 129 \mu_2) + 33 \mu_2 + \mu_1 (590 - 47 \mu_1 + 109 \mu_2)))) - \\
& x^4 (-1 + \eta)^4 (2 \times (-1 + \eta) \theta p (107 + 105 \eta^4 + 135 \mu_1 + 5 \eta^2 (212 + \\
& 243 \mu_1 + 63 \eta t (-1 + \mu_2) - 102 \mu_2) + 124 \mu_2 - \\
& 105 \eta^3 (-3 + \eta t - 4 \mu_1 + 3 \mu_2) + \eta t (-19 + 87 \mu_1 + 86 \mu_2) +
\end{aligned}$$

$$\begin{aligned}
& \eta (746 + 845 \mu_1 + 265 \mu_2 + \eta t (-191 + 297 \mu_1 + 319 \mu_2)) + \\
& (-1 + \eta t) \theta l (2 - 10 \mu_1 + 112 \mu_2 - \theta p (216 + 53 \mu_1 + 2 \mu_2 \\
& (60 + 27 \mu_1 - 10 \mu_2) + 49 \mu_2 + \mu_1 (276 + 3 \mu_1 + 73 \mu_2)) + \\
& \eta^2 (8 \times (-6 + 127 \mu_1 - \mu_2) - 5 \theta p (338 + 6 \mu_1 + \mu_2 (38 + 3 \mu_1 - \\
& 63 \mu_2) + 18 \mu_2 + \mu_1 (302 - 20 \mu_1 + 58 \mu_2)) + \\
& \eta (-76 + 438 \mu_1 + 188 \mu_2 - \theta p (\mu_2 (394 + 141 \mu_1 - 209 \mu_2) + \\
& 2 \times (689 + 73 \mu_1 + 83 \mu_2) + \mu_1 (1438 - 46 \mu_1 + 324 \mu_2))) + \\
& x^3 (-1 + \eta)^3 (2 \times (-1 + \eta) \theta p (21 + 105 \eta^5 + 35 \mu_1 + 10 \eta^3 (155 + \\
& 162 \mu_1 + 42 \eta t (-1 + \mu_2) - 102 \mu_2) + 30 \mu_2 - \\
& 105 \eta^4 (-4 + \eta t - 4 \mu_1 + 4 \mu_2) + \eta t (21 + 40 \mu_1 + 87 \mu_2) + \\
& \eta (436 + 540 \mu_1 + 464 \mu_2 + \eta t (-82 + 391 \mu_1 + 338 \mu_2)) + \\
& \eta^2 (2 \times (777 + 845 \mu_1 + 140 \mu_2) + \eta t (-379 + 653 \mu_1 + 641 \mu_2)) + \\
& (-1 + \eta t) \theta l (6 \times (2 + 2 \mu_1 + 11 \mu_2) - \theta p (54 + 26 \mu_1 + 22 \mu_2 + \\
& \mu_2 (54 + 27 \mu_1 + \mu_2) + \mu_1 (90 + 6 \mu_1 + 28 \mu_2)) + \\
& 2 \eta^3 (-21 + 567 \mu_1 - \mu_2 - 5 \theta p (230 + 5 \mu_1 + \mu_2 (26 + 3 \mu_1 - 41 \mu_2) + \\
& 13 \mu_2 + \mu_1 (206 - 11 \mu_1 + 41 \mu_2))) - \\
& \eta (6 \times (6 + 10 \mu_1 - 49 \mu_2) + \theta p (878 + 215 \mu_1 + \mu_2 (482 + \\
& 219 \mu_1 - 77 \mu_2) + 199 \mu_2 + \mu_1 (1118 + 19 \mu_1 + 299 \mu_2))) + \\
& 2 \eta^2 (-66 + 393 \mu_1 + 132 \mu_2 - \theta p (\mu_2 (398 + 147 \mu_1 - 203 \mu_2) + \\
& 2 \times (703 + 76 \mu_1 + 86 \mu_2) + \mu_1 (1466 - 32 \mu_1 + 338 \mu_2))) - \\
& x^2 (-1 + \eta)^2 (126 \eta^7 \theta p - 126 \eta^6 \theta p (-4 + \eta t - 4 \mu_1 + 5 \mu_2) + 2 \eta^5 \\
& \theta p (950 + 963 \mu_1 - 705 \mu_2 + 63 \eta t (-4 + 5 \mu_2)) - 6 \\
& (\theta l \mu_2 - \eta t \theta l \mu_2 + \eta t \theta p (8 + 9 \mu_1 + 17 \mu_2)) - 3 \eta \\
& (2 \theta p (21 + 35 \mu_1 + 30 \mu_2 + \eta t (6 + 26 \mu_1 + 63 \mu_2)) + \\
& (-1 + \eta t) \theta l (4 + 6 \mu_1 - 32 \mu_2 + \theta p (54 + 26 \mu_1 + 22 \mu_2 + \\
& \mu_2 (54 + 27 \mu_1 + \mu_2) + \mu_1 (90 + 6 \mu_1 + 28 \mu_2)))) + \eta^4 \\
& (2 \theta p (351 + 475 \mu_1 + 1050 \mu_2 + \eta t (-61 + 712 \mu_1 + 329 \mu_2)) + \\
& (-1 + \eta t) \theta l (2 \times (-9 + 313 \mu_1 + \mu_2) - 5 \theta p (352 + 9 \mu_1 + \\
& \mu_2 (40 + 6 \mu_1 - 60 \mu_2) + 21 \mu_2 + \mu_1 (316 - 13 \mu_1 + 65 \mu_2)))) - 3 \\
& \eta^2 (2 \theta p (201 + 235 \mu_1 + 186 \mu_2 + 2 \eta t (-29 + 91 \mu_1 + 43 \mu_2)) + \\
& (-1 + \eta t) \theta l (26 + 30 \mu_1 - 84 \mu_2 + \theta p (446 + 109 \mu_1 + \mu_2 (242 + 111 \mu_1 - \\
& 37 \mu_2) + 101 \mu_2 + \mu_1 (566 + 13 \mu_1 + 153 \mu_2)))) + 2 \\
& \eta^3 (-\theta p (950 + 880 \mu_1 - 618 \mu_2 + \eta t (-244 + 61 \mu_1 + 146 \mu_2)) + \\
& (-1 + \eta t) \theta l (-50 + 305 \mu_1 + 82 \mu_2 - \theta p (\mu_2 (402 + 153 \mu_1 - 197 \mu_2) + \\
& 2 \times (717 + 79 \mu_1 + 89 \mu_2) + \mu_1 (1494 - 18 \mu_1 + 352 \mu_2)))) + \\
& x (-1 + \eta) \times (42 \eta^8 \theta p - 3 \eta t \theta p (3 + 3 \mu_1 + 5 \mu_2) - 42 \eta^7 \theta p (-5 + \eta t - \\
& 4 \mu_1 + 6 \mu_2) + 2 \eta^6 \theta p (421 + 402 \mu_1 - 384 \mu_2 + 21 \eta t (-5 + 6 \mu_2)) - 3 \\
& \eta ((-1 + \eta t) \theta l (3 + 3 \mu_1 + \mu_2) + \eta t \theta p (17 + 19 \mu_1 + 51 \mu_2)) - 3 \\
& \eta^2 (2 \theta p (21 + 35 \mu_1 + 30 \mu_2 + \eta t (-3 + 19 \mu_1 + 45 \mu_2)) + \\
& (-1 + \eta t) \theta l (2 \times (4 + 5 \mu_1 - 5 \mu_2) + \theta p (54 + 26 \mu_1 + 22 \mu_2 + \\
& \mu_2 (54 + 27 \mu_1 + \mu_2) + \mu_1 (90 + 6 \mu_1 + 28 \mu_2)))) + \eta^5 \\
& (\theta p (584 + 718 \mu_1 + 800 \mu_2 + \eta t (-121 + 771 \mu_1 + 395 \mu_2)) + \\
& (-1 + \eta t) \theta l (-3 + 137 \mu_1 + \mu_2 - \theta p (718 + 21 \mu_1 + \\
& \mu_2 (82 + 15 \mu_1 - 117 \mu_2) + 45 \mu_2 + \mu_1 (646 - 19 \mu_1 + 137 \mu_2)))) - \\
& \eta^3 (2 \theta p (389 + 435 \mu_1 + 310 \mu_2 + \eta t (-115 + 387 \mu_1 + 107 \mu_2)) + \\
& (-1 + \eta t) \theta l (10 \times (4 + 4 \mu_1 - 7 \mu_2) + \theta p (906 + 221 \mu_1 + \mu_2 (486 +
\end{aligned}$$

$$\begin{aligned}
& 225 \mathfrak{e}1 - 71 \mathfrak{e}2) + 205 \mathfrak{e}2 + \mu1 (1146 + 33 \mathfrak{e}1 + 313 \mathfrak{e}2) ) ) + \\
& \eta^4 (\mathfrak{e}p (-774 - 610 \mu1 + 183 \eta t \mu1 + 1020 \mu2 + 5 \eta t (37 + \mu2)) + \\
& (-1 + \eta t) \mathfrak{e}l (-28 + 174 \mu1 + 38 \mu2 - \mathfrak{e}p (\mu2 (406 + 159 \mathfrak{e}1 - 191 \mathfrak{e}2) + \\
& 2 \times (731 + 82 \mathfrak{e}1 + 92 \mathfrak{e}2) + \mu1 (1522 - 4 \mathfrak{e}1 + 366 \mathfrak{e}2) ) ) ) + \\
& w^2 (-1 + \eta)^2 (2 x^8 (-1 + \eta)^9 \mathfrak{e}p (\eta - \eta t + 4 \mu1) - x^7 (-1 + \eta)^7 \\
& (2 \times (-1 + \eta) \mathfrak{e}p (49 + 8 \eta^2 + 57 \mu1 + \eta (17 - 8 \eta t + 32 \mu1 - 7 \mu2) + \\
& \eta t (-17 + 7 \mu2)) + (-1 + \eta t) \mathfrak{e}l (4 + 44 \mu1 + \\
& \mathfrak{e}p (-102 - \mathfrak{e}1 + \mu1 (-74 + 3 \mathfrak{e}1 - 11 \mathfrak{e}2) - 7 \mathfrak{e}2 + 2 \mu2 (-6 + 5 \mathfrak{e}2) ) ) ) + \\
& x^6 (-1 + \eta)^6 (2 \times (-1 + \eta) \mathfrak{e}p (119 + 28 \eta^3 + 165 \mu1 + 54 \mu2 - \\
& 7 \eta^2 (-17 + 4 \eta t - 16 \mu1 + 7 \mu2) + \eta t (-41 + 28 \mu1 + 49 \mu2) + \\
& \eta (398 + 399 \mu1 - 76 \mu2 + 7 \eta t (-17 + 7 \mu2)) ) + (-1 + \eta t) \mathfrak{e}l \\
& (-22 + 94 \mu1 - 6 \mu2 + \mathfrak{e}p (\mu1 (-260 + 41 \mathfrak{e}1 - 37 \mathfrak{e}2) - 3 \times (72 + \mathfrak{e}1 + 5 \mathfrak{e}2) + \\
& \mu2 (-52 + 66 \mathfrak{e}2)) + \eta (24 + 324 \mu1 + \mathfrak{e}p (-738 - 80 \mu2 - \\
& 7 \mathfrak{e}1 + 2 \mu1 (-270 + 5 \mathfrak{e}1 - 44 \mathfrak{e}2) - 49 \mathfrak{e}2 + 70 \mu2 \mathfrak{e}2) ) ) + \\
& \eta \mathfrak{e}p (2 \eta^9 - 2 \eta t \mu2 - 28 \eta \eta t (1 + \mu1 + 2 \mu2) - 2 \eta^8 (-16 + \eta t - 4 \mu1 + \\
& 7 \mu2) + 2 \eta^7 (87 + 53 \mu1 - 69 \mu2 + \eta t (-16 + 7 \mu2)) + \eta^5 \\
& (-90 + 64 \mu1 + 198 \eta t \mu1 + 366 \mu2 + 40 \eta t \mu2 - 3 \times (-1 + \eta t) \mathfrak{e}l \\
& (94 + 4 \mathfrak{e}1 + \mu2 (18 + 3 \mathfrak{e}1 - 19 \mathfrak{e}2) + 8 \mathfrak{e}2 + \mu1 (108 - 3 \mathfrak{e}1 + 23 \mathfrak{e}2) ) ) - \\
& \eta^2 (4 \times (5 + 5 \mu1 + 4 \mu2) - \mathfrak{e}l (48 + 25 \mathfrak{e}1 + 19 \mathfrak{e}2 + \mu2 (50 + 27 \mathfrak{e}1 + 11 \mathfrak{e}2) + \\
& \mu1 (48 + 11 \mathfrak{e}1 + 19 \mathfrak{e}2)) + \eta t (-8 - 26 \mu1 + 64 \mu2 + \mathfrak{e}l (48 + 25 \mathfrak{e}1 + \\
& 19 \mathfrak{e}2 + \mu2 (50 + 27 \mathfrak{e}1 + 11 \mathfrak{e}2) + \mu1 (48 + 11 \mathfrak{e}1 + 19 \mathfrak{e}2) ) ) ) + \eta^3 \\
& (-2 \times (43 + 85 \mu1 + 86 \mu2) + 3 \mathfrak{e}l (42 + 20 \mathfrak{e}1 + \mu2 (46 + 21 \mathfrak{e}1 - 5 \mathfrak{e}2) + \\
& 16 \mathfrak{e}2 + \mu1 (76 - \mathfrak{e}1 + 21 \mathfrak{e}2)) + \eta t (2 \times (30 - 57 \mu1 + \mu2) - 3 \mathfrak{e}l (42 + \\
& 20 \mathfrak{e}1 + \mu2 (46 + 21 \mathfrak{e}1 - 5 \mathfrak{e}2) + 16 \mathfrak{e}2 + \mu1 (76 - \mathfrak{e}1 + 21 \mathfrak{e}2) ) ) ) + \\
& \eta^6 (156 + 216 \mu1 - 38 \mu2 + \mathfrak{e}l (126 + 8 \mu2 + \mathfrak{e}1 + 7 \mathfrak{e}2 - 10 \mu2 \mathfrak{e}2 + \\
& \mu1 (96 + 8 \mathfrak{e}1 + 22 \mathfrak{e}2)) - \eta t (48 - 116 \mu1 - 84 \mu2 + \\
& \mathfrak{e}l (126 + 8 \mu2 + \mathfrak{e}1 + 7 \mathfrak{e}2 - 10 \mu2 \mathfrak{e}2 + \mu1 (96 + 8 \mathfrak{e}1 + 22 \mathfrak{e}2) ) ) ) + \eta^4 \\
& (12 \times (-14 - 17 \mu1 + \mu2) + \mathfrak{e}l (234 + 46 \mathfrak{e}1 + \mu2 (134 + 45 \mathfrak{e}1 - 73 \mathfrak{e}2) + \\
& 46 \mathfrak{e}2 + \mu1 (408 - 31 \mathfrak{e}1 + 91 \mathfrak{e}2) ) + \\
& \eta t (-6 \times (-7 + 33 \mu1 + 3 \mu2) - \mathfrak{e}l (234 + 46 \mathfrak{e}1 + \mu2 \\
& (134 + 45 \mathfrak{e}1 - 73 \mathfrak{e}2) + 46 \mathfrak{e}2 + \mu1 (408 - 31 \mathfrak{e}1 + 91 \mathfrak{e}2) ) ) ) + \\
& x^5 (-1 + \eta)^5 (-((-1 + \eta) \mathfrak{e}p (226 + 112 \eta^4 + 394 \mu1 + 352 \mu2 - 14 \eta^3 \\
& (-51 + 8 \eta t - 32 \mu1 + 21 \mu2) + \eta t (-91 + 169 \mu1 + 129 \mu2) + \\
& 6 \eta^2 (453 + 399 \mu1 - 152 \mu2 + 7 \eta t (-17 + 7 \mu2)) + \\
& 2 \eta (777 + 990 \mu1 + 175 \mu2 + 6 \eta t (-41 + 33 \mu1 + 49 \mu2) ) ) ) + (-1 + \eta t) \\
& \mathfrak{e}l (52 + 60 \mu1 - 42 \mu2 + \mathfrak{e}p (174 + 28 \mathfrak{e}1 + \mu2 (118 + 27 \mathfrak{e}1 - 91 \mathfrak{e}2) + \\
& 28 \mathfrak{e}2 + \mu1 (346 - 62 \mathfrak{e}1 + 60 \mathfrak{e}2)) + 3 \eta^2 (-20 \times (1 + 16 \mu1) + \\
& \mathfrak{e}p (762 + 76 \mu2 + 7 \mathfrak{e}1 + 49 \mathfrak{e}2 - 70 \mu2 \mathfrak{e}2 + \mu1 (562 + \mathfrak{e}1 + 99 \mathfrak{e}2) ) + \\
& \eta (101 - 615 \mu1 + 21 \mu2 + \mathfrak{e}p (1362 + 314 \mu2 + 27 \mathfrak{e}1 + 9 \mu2 \mathfrak{e}1 + \\
& 99 \mathfrak{e}2 - 387 \mu2 \mathfrak{e}2 + \mu1 (1624 - 214 \mathfrak{e}1 + 254 \mathfrak{e}2) ) ) ) - \\
& x^4 (-1 + \eta)^4 (-2 \times (-1 + \eta) \mathfrak{e}p (53 + 70 \eta^5 + 95 \mu1 + 106 \mu2 - 35 \eta^4 \\
& (-17 + 2 \eta t - 8 \mu1 + 7 \mu2) + \eta t (-20 + 27 \mu1 + 60 \mu2) + \\
& 5 \eta^3 (508 + 399 \mu1 - 228 \mu2 + 7 \eta t (-17 + 7 \mu2)) + \\
& 5 \eta^2 (420 + 495 \mu1 + 13 \mu2 + 3 \eta t (-41 + 38 \mu1 + 49 \mu2)) + \\
& \eta (589 + 985 \mu1 + 792 \mu2 + \eta t (-223 + 495 \mu1 + 327 \mu2)) ) + (-1 + \eta t) \mathfrak{e}l
\end{aligned}$$

$$\begin{aligned}
& \left( -2 + 34 \mu_1 - 104 \mu_2 + \text{op} (108 + 51 \mathfrak{e}_1 + 2 \mu_2 (64 + 27 \mathfrak{e}_1 - 12 \mathfrak{e}_2) + \right. \\
& \quad 39 \mathfrak{e}_2 + \mu_1 (208 - 13 \mathfrak{e}_1 + 53 \mathfrak{e}_2)) + 5 \eta^3 (-8 \times (2 + 37 \mu_1) + \text{op} \\
& \quad (786 + 72 \mu_2 + 7 \mathfrak{e}_1 + 49 \mathfrak{e}_2 - 70 \mu_2 \mathfrak{e}_2 + 2 \mu_1 (292 + 6 \mathfrak{e}_1 + 55 \mathfrak{e}_2))) + \\
& \quad \eta^2 (8 \times (23 - 190 \mu_1 + 3 \mu_2) + 5 \text{op} (714 + 158 \mu_2 + 18 \mathfrak{e}_1 + \\
& \quad 9 \mu_2 \mathfrak{e}_1 + 54 \mathfrak{e}_2 - 189 \mu_2 \mathfrak{e}_2 + \mu_1 (844 - 91 \mathfrak{e}_1 + 143 \mathfrak{e}_2))) + \\
& \quad \eta (2 \times (104 + 89 \mu_1 - 84 \mu_2) + \text{op} (930 + 606 \mu_2 + 158 \mathfrak{e}_1 + 153 \\
& \quad \mu_2 \mathfrak{e}_1 + 158 \mathfrak{e}_2 - 437 \mu_2 \mathfrak{e}_2 + \mu_1 (1792 - 279 \mathfrak{e}_1 + 331 \mathfrak{e}_2))) \left. \right) + \\
& x^2 (-1 + \eta)^2 (56 \eta^8 \text{op} - 14 \eta^7 \text{op} (-47 + 4 \eta \mathfrak{t} - 16 \mu_1 + 21 \mu_2) + 2 \eta^6 \\
& \text{op} (1497 + 1085 \mu_1 - 993 \mu_2 + 7 \eta \mathfrak{t} (-47 + 21 \mu_2)) - 2 \\
& (\mathfrak{e}_1 \mu_2 - \eta \mathfrak{t} \mathfrak{e}_1 \mu_2 + \eta \mathfrak{t} \text{op} (26 + 27 \mu_1 + 41 \mu_2)) - \eta \\
& (4 \text{op} (3 \times (5 + 5 \mu_1 + 4 \mu_2) + \eta \mathfrak{t} (17 + 7 \mu_1 + 86 \mu_2)) + \\
& (-1 + \eta \mathfrak{t}) \mathfrak{e}_1 (-2 \times (16 + 15 \mu_1 + 46 \mu_2) + 3 \text{op} (48 + 25 \mathfrak{e}_1 + 19 \mathfrak{e}_2 + \\
& \mu_2 (50 + 27 \mathfrak{e}_1 + 11 \mathfrak{e}_2) + \mu_1 (48 + 11 \mathfrak{e}_1 + 19 \mathfrak{e}_2)))) + \eta^5 \\
& (2 \text{op} (561 + 1278 \mu_1 + 460 \mu_2 + 6 \eta \mathfrak{t} (-43 + 120 \mu_1 + 98 \mu_2)) - \\
& 3 \times (-1 + \eta \mathfrak{t}) \mathfrak{e}_1 (-4 \times (2 + 47 \mu_1) + \text{op} (834 + 64 \mu_2 + 7 \mathfrak{e}_1 + \\
& 49 \mathfrak{e}_2 - 70 \mu_2 \mathfrak{e}_2 + 2 \mu_1 (314 + 17 \mathfrak{e}_1 + 66 \mathfrak{e}_2)))) + \eta^2 \\
& (-2 \text{op} (36 \times (8 + 15 \mu_1 + 16 \mu_2) + \eta \mathfrak{t} (-180 + 214 \mu_1 + 147 \mu_2)) + \\
& (-1 + \eta \mathfrak{t}) \mathfrak{e}_1 (-54 - 178 \mu_1 + 252 \mu_2 - 3 \text{op} (234 + 266 \mu_2 + 111 \mathfrak{e}_1 + \\
& 117 \mu_2 \mathfrak{e}_1 + 87 \mathfrak{e}_2 - 39 \mu_2 \mathfrak{e}_2 + \mu_1 (436 - 16 \mathfrak{e}_1 + 116 \mathfrak{e}_2)))) + \eta^4 \\
& (2 \text{op} (-1141 - 505 \mu_1 + \eta \mathfrak{t} (187 + 560 \mu_1 - 63 \mu_2) + 1912 \mu_2) + \\
& (-1 + \eta \mathfrak{t}) \mathfrak{e}_1 (-74 + 1050 \mu_1 + 6 \mu_2 - 5 \text{op} (780 + 27 \mathfrak{e}_1 + \\
& 2 \mu_2 (80 + 9 \mathfrak{e}_1 - 90 \mathfrak{e}_2) + 63 \mathfrak{e}_2 + \mu_1 (908 - 59 \mathfrak{e}_1 + 175 \mathfrak{e}_2)))) + \\
& 2 \eta^3 (-\text{op} (956 + 1400 \mu_1 + 632 \mu_2 + \eta \mathfrak{t} (-308 + 1025 \mu_1 + 312 \mu_2)) + \\
& (-1 + \eta \mathfrak{t}) \mathfrak{e}_1 (-104 - 27 \mu_1 + 84 \mu_2 - \text{op} (\mu_2 (638 + 189 \mathfrak{e}_1 - 401 \mathfrak{e}_2) + \\
& 2 \times (525 + 97 \mathfrak{e}_1 + 97 \mathfrak{e}_2) + \mu_1 (1916 - 217 \mathfrak{e}_1 + 393 \mathfrak{e}_2)))) - \\
& x (-1 + \eta) \times (16 \eta^9 \text{op} + 2 \eta^8 \text{op} (111 - 8 \eta \mathfrak{t} + 32 \mu_1 - 49 \mu_2) - \eta \mathfrak{t} \text{op} \\
& (3 + 3 \mu_1 + 5 \mu_2) + 2 \eta^7 \text{op} (554 + 367 \mu_1 - 407 \mu_2 + \eta \mathfrak{t} (-111 + 49 \mu_2)) - \eta \\
& ((-1 + \eta \mathfrak{t}) \mathfrak{e}_1 (3 + 3 \mu_1 + \mu_2) + \eta \mathfrak{t} \text{op} (77 + 79 \mu_1 + 135 \mu_2)) - \eta^2 \\
& (2 \text{op} (6 \times (5 + 5 \mu_1 + 4 \mu_2) + \eta \mathfrak{t} (5 - 19 \mu_1 + 128 \mu_2)) + \\
& (-1 + \eta \mathfrak{t}) \mathfrak{e}_1 (-2 \times (2 + \mu_1 + 17 \mu_2) + 3 \text{op} (48 + 25 \mathfrak{e}_1 + 19 \mathfrak{e}_2 + \\
& \mu_2 (50 + 27 \mathfrak{e}_1 + 11 \mathfrak{e}_2) + \mu_1 (48 + 11 \mathfrak{e}_1 + 19 \mathfrak{e}_2)))) + \eta^6 \\
& (2 \text{op} (356 + 591 \mu_1 + 35 \mu_2 + \eta \mathfrak{t} (-127 + 318 \mu_1 + 245 \mu_2)) - \\
& (-1 + \eta \mathfrak{t}) \mathfrak{e}_1 (-4 \times (1 + 26 \mu_1) + \text{op} (858 + 60 \mu_2 + 7 \mathfrak{e}_1 + \\
& 49 \mathfrak{e}_2 - 70 \mu_2 \mathfrak{e}_2 + \mu_1 (650 + 45 \mathfrak{e}_1 + 143 \mathfrak{e}_2)))) + \eta^3 \\
& (-2 \text{op} (14 \times (13 + 25 \mu_1 + 26 \mu_2) + \eta \mathfrak{t} (-125 + 179 \mu_1 + 42 \mu_2)) + \\
& (-1 + \eta \mathfrak{t}) \mathfrak{e}_1 (-28 - 72 \mu_1 + 74 \mu_2 - \text{op} (486 + 542 \mu_2 + 231 \mathfrak{e}_1 + \\
& 243 \mu_2 \mathfrak{e}_1 + 183 \mathfrak{e}_2 - 69 \mu_2 \mathfrak{e}_2 + \mu_1 (892 - 22 \mathfrak{e}_1 + 242 \mathfrak{e}_2)))) + \\
& \eta^5 (\text{op} (-2 \times (368 + 5 \mu_1 - 949 \mu_2) + \eta \mathfrak{t} (73 + 789 \mu_1 + 93 \mu_2)) + \\
& (-1 + \eta \mathfrak{t}) \mathfrak{e}_1 (-13 + 239 \mu_1 + 3 \mu_2 - \text{op} (1626 + 322 \mu_2 + 63 \mathfrak{e}_1 + 45 \mu_2 \mathfrak{e}_1 + \\
& 135 \mathfrak{e}_2 - 351 \mu_2 \mathfrak{e}_2 + \mu_1 (1880 - 86 \mathfrak{e}_1 + 382 \mathfrak{e}_2)))) + \eta^4 \\
& (-\text{op} (898 + 1210 \mu_1 + 280 \mu_2 + \eta \mathfrak{t} (-259 + 1023 \mu_1 + 201 \mu_2)) + \\
& (-1 + \eta \mathfrak{t}) \mathfrak{e}_1 (2 \times (-26 + \mu_1 + 21 \mu_2) - \text{op} (1110 + 212 \mathfrak{e}_1 + \mu_2 (654 + 207 \\
& \mathfrak{e}_1 - 383 \mathfrak{e}_2) + 212 \mathfrak{e}_2 + \mu_1 (1978 - 186 \mathfrak{e}_1 + 424 \mathfrak{e}_2)))) + \\
& x^3 (-1 + \eta)^3 (-2 \times (-1 + \eta) \text{op} (56 \eta^6 + 2 \times (5 + 5 \mu_1 + 4 \mu_2) - 7 \eta^5 \\
& (-85 + 8 \eta \mathfrak{t} - 32 \mu_1 + 35 \mu_2) + \eta \mathfrak{t} (25 + 20 \mu_1 + 76 \mu_2) + \\
& 5 \eta^4 (563 + 399 \mu_1 - 304 \mu_2 + 7 \eta \mathfrak{t} (-17 + 7 \mu_2)) +
\end{aligned}$$

$$\begin{aligned}
& 10 \eta^3 (301 + 330 \mu_1 - 41 \mu_2 + \eta t (-82 + 86 \mu_1 + 98 \mu_2)) + \\
& \eta (4 \times (53 + 95 \mu_1 + 103 \mu_2) + \eta t (-80 + 139 \mu_1 + 240 \mu_2)) + \\
& \eta^2 (\eta t (-437 + 1135 \mu_1 + 663 \mu_2) + 2 \times (613 + 985 \mu_1 + 704 \mu_2)) + \\
& (-1 + \eta t) \theta l (-2 \times (14 + 14 \mu_1 + 29 \mu_2) + \theta p (48 + 25 \mathfrak{z}_1 + 19 \mathfrak{z}_2 + \\
& \mu_2 (50 + 27 \mathfrak{z}_1 + 11 \mathfrak{z}_2) + \mu_1 (48 + 11 \mathfrak{z}_1 + 19 \mathfrak{z}_2)) + \\
& \eta (24 + 140 \mu_1 - 282 \mu_2 + 3 \theta p (150 + 71 \mathfrak{z}_1 + \mu_2 (174 + 75 \mathfrak{z}_1 - \\
& 29 \mathfrak{z}_2) + 55 \mathfrak{z}_2 + \mu_1 (284 - 14 \mathfrak{z}_1 + 74 \mathfrak{z}_2))) + \\
& 2 \eta^3 (83 - 905 \mu_1 + 3 \mu_2 + 5 \theta p (498 + 15 \mathfrak{z}_1 + \mu_2 (106 + 9 \mathfrak{z}_1 - \\
& 123 \mathfrak{z}_2) + 39 \mathfrak{z}_2 + \mu_1 (584 - 50 \mathfrak{z}_1 + 106 \mathfrak{z}_2))) + \\
& 5 \eta^4 (-12 \times (1 + 21 \mu_1) + \theta p (810 + 68 \mu_2 + 7 \mathfrak{z}_1 + 49 \mathfrak{z}_2 - \\
& 70 \mu_2 \mathfrak{z}_2 + \mu_1 (606 + 23 \mathfrak{z}_1 + 121 \mathfrak{z}_2))) + \\
& \eta^2 (6 \times (52 + 29 \mu_1 - 42 \mu_2) + \theta p (2 \mu_2 (622 + 171 \mathfrak{z}_1 - 419 \mathfrak{z}_2) + \\
& 44 \times (45 + 8 \mathfrak{z}_1 + 8 \mathfrak{z}_2) + \mu_1 (3708 - 496 \mathfrak{z}_1 + 724 \mathfrak{z}_2)))) - \\
& w (x (-1 + \eta) - \eta) (-1 + \eta) \times (2 x^7 (-1 + \eta)^7 \theta p (-15 + 5 \eta^2 + 5 \eta t + 15 \\
& \theta l - 5 \eta (-2 + \eta t - 3 \mu_1) - 15 \mu_1 + 7 \theta l \mu_1 + \theta l \mathfrak{z}_2 - \eta t \theta l (15 + 7 \mu_1 + \mathfrak{z}_2)) + \\
& x^6 (-1 + \eta)^6 (-2 \times (-1 + \eta) \theta p (29 + 35 \eta^2 + 71 \mu_1 + \eta (139 - 35 \eta t + \\
& 105 \mu_1 - 21 \mu_2) + 10 \mu_2 + 2 \eta t (-11 + 7 \mu_2)) + (-1 + \eta t) \theta l \\
& (-8 - 28 \times (2 + \eta) \mu_1 + \eta \theta p (234 + 14 \mathfrak{z}_2 + 7 \mu_1 (16 + \mathfrak{z}_1 + \mathfrak{z}_2)) + \\
& 2 \theta p (33 + \mathfrak{z}_1 + 6 \mathfrak{z}_2 - 2 \mu_2 (-7 + 5 \mathfrak{z}_2) + \mu_1 (59 - 7 \mathfrak{z}_1 + 7 \mathfrak{z}_2)))) + \\
& x^5 (-1 + \eta)^5 (2 \times (-1 + \eta) \theta p (37 + 105 \eta^3 + 121 \mu_1 + 92 \mu_2 + \\
& 5 \eta t (-5 + 8 \mu_1 + 7 \mu_2) - 3 \eta^2 (-173 + 35 \eta t - 105 \mu_1 + 42 \mu_2) + \\
& \eta (227 + 426 \mu_1 - 15 \mu_2 + 2 \eta t (-66 + 7 \mu_1 + 42 \mu_2))) - \\
& (-1 + \eta t) \theta l (26 + 14 \mu_1 + 6 \mu_2 + \theta p (48 + 3 \mathfrak{z}_1 + \mu_2 (68 - 66 \mathfrak{z}_2) + \\
& 11 \mathfrak{z}_2 + \mu_1 (204 - 55 \mathfrak{z}_1 + 23 \mathfrak{z}_2)) + \\
& 2 \eta^2 (-70 \mu_1 + 3 \theta p (129 + 7 \mathfrak{z}_2 + 7 \mu_1 (9 + \mathfrak{z}_1 + \mathfrak{z}_2))) - \\
& 2 \eta (20 + 186 \mu_1 + \theta p (\mu_1 (-376 + 31 \mathfrak{z}_1 - 53 \mathfrak{z}_2) + \\
& 20 \mu_2 (-4 + 3 \mathfrak{z}_2) - 6 \times (37 + \mathfrak{z}_1 + 6 \mathfrak{z}_2)))) + \\
& \eta \theta p (-10 \eta^8 + 6 \eta t (2 + 2 \mu_1 + 3 \mu_2) + 2 \eta^7 (-44 + 5 \eta t - 15 \mu_1 + 21 \mu_2) + \\
& \eta^6 (-66 - 112 \mu_1 + 88 \mu_2 - 2 \theta l (27 + \mathfrak{z}_2) - 7 \theta l \mu_1 (4 + \mathfrak{z}_1 + \mathfrak{z}_2) + \\
& \eta t (34 - 28 \mu_1 - 28 \mu_2 + 2 \theta l (27 + \mathfrak{z}_2) + 7 \theta l \mu_1 (4 + \mathfrak{z}_1 + \mathfrak{z}_2))) + \eta \\
& (-\theta l (12 + 8 \mathfrak{z}_1 + 6 \mathfrak{z}_2 + 2 \mu_1 (6 + 4 \mathfrak{z}_1 + 3 \mathfrak{z}_2) + \mu_2 (14 + 9 \mathfrak{z}_1 + 7 \mathfrak{z}_2)) + \\
& \eta t (-4 - 10 \mu_1 + 30 \mu_2 + \theta l (12 + 8 \mathfrak{z}_1 + 6 \mathfrak{z}_2 + \\
& 2 \mu_1 (6 + 4 \mathfrak{z}_1 + 3 \mathfrak{z}_2) + \mu_2 (14 + 9 \mathfrak{z}_1 + 7 \mathfrak{z}_2)))) + \eta^2 \\
& (40 \times (1 + \mu_1 + \mu_2) - \theta l (48 + 24 \mathfrak{z}_1 + 3 \mu_2 (18 + 9 \mathfrak{z}_1 - \mathfrak{z}_2) + 14 \mathfrak{z}_2 + \\
& \mu_1 (46 - 5 \mathfrak{z}_1 + 13 \mathfrak{z}_2)) + \eta t (-2 \times (14 + 25 \mu_1 + 3 \mu_2) + \theta l (48 + \\
& 24 \mathfrak{z}_1 + 3 \mu_2 (18 + 9 \mathfrak{z}_1 - \mathfrak{z}_2) + 14 \mathfrak{z}_2 + \mu_1 (46 - 5 \mathfrak{z}_1 + 13 \mathfrak{z}_2)))) + \\
& 2 \eta^5 (21 - 50 \mu_1 - 81 \mu_2 - \theta l (57 + \mathfrak{z}_1 - 10 \mu_2 (-1 + \mathfrak{z}_2) + 6 \mathfrak{z}_2 + \\
& \mu_1 (81 + 4 \mathfrak{z}_1 + 18 \mathfrak{z}_2)) + \eta t (3 - 72 \mu_1 - 21 \mu_2 + \\
& \theta l (57 + \mathfrak{z}_1 - 10 \mu_2 (-1 + \mathfrak{z}_2) + 6 \mathfrak{z}_2 + \mu_1 (81 + 4 \mathfrak{z}_1 + 18 \mathfrak{z}_2)))) + \eta^3 \\
& (2 \times (23 + 65 \mu_1 + 74 \mu_2) - \theta l (66 + 26 \mathfrak{z}_1 + \mu_2 (86 + 27 \mathfrak{z}_1 - 47 \mathfrak{z}_2) + \\
& 18 \mathfrak{z}_2 + \mu_1 (162 - 40 \mathfrak{z}_1 + 30 \mathfrak{z}_2)) + \\
& \eta t (2 \times (-6 + 91 \mu_1 + 6 \mu_2) + \theta l (66 + 26 \mathfrak{z}_1 + \mu_2 (86 + 27 \mathfrak{z}_1 - 47 \mathfrak{z}_2) + \\
& 18 \mathfrak{z}_2 + \mu_1 (162 - 40 \mathfrak{z}_1 + 30 \mathfrak{z}_2)))) + \eta^4 \\
& (12 \times (3 + 6 \mu_1 - 13 \mu_2) - \theta l (90 + 12 \mathfrak{z}_1 + \mu_2 (66 + 9 \mathfrak{z}_1 - 57 \mathfrak{z}_2) + \\
& 20 \mathfrak{z}_2 + \mu_1 (262 - 26 \mathfrak{z}_1 + 52 \mathfrak{z}_2)) + \\
& \eta t (2 \times (-9 + 19 \mu_1 + 8 \mu_2) + \theta l (90 + 12 \mathfrak{z}_1 + \mu_2 (66 + 9 \mathfrak{z}_1 - 57 \mathfrak{z}_2) +
\end{aligned}$$

$$\begin{aligned}
& 20 \, \mathfrak{z}^2 + \mu_1 (262 - 26 \, \mathfrak{z}^1 + 52 \, \mathfrak{z}^2) \Big) \Big) + \\
& x^4 (-1 + \eta)^4 \Big( - \Big( (-1 + \eta) \, \mathfrak{e} \mathfrak{p} (86 + 350 \, \eta^4 + 170 \, \mu_1 + 228 \, \mu_2 + \eta \mathfrak{t} \\
& \quad (-41 + 49 \, \mu_1 + 45 \, \mu_2) - 10 \, \eta^3 (-207 + 35 \, \eta \mathfrak{t} - 105 \, \mu_1 + 63 \, \mu_2) + \\
& \quad 2 \, \eta (209 + 605 \, \mu_1 + 246 \, \eta \mathfrak{t} \, \mu_1 + 384 \, \mu_2 + 25 \, \eta \mathfrak{t} (-5 + 7 \, \mu_2)) + \\
& \quad 10 \, \eta^2 (140 + 213 \, \mu_1 - 45 \, \mu_2 + 2 \, \eta \mathfrak{t} (-33 + 7 \, \mu_1 + 21 \, \mu_2)) \Big) \Big) + (-1 + \eta \mathfrak{t}) \\
& \, \mathfrak{e} \mathfrak{l} (56 + 112 \, \mu_1 - 6 \, \mu_2 + \mathfrak{e} \mathfrak{p} (30 + 8 \, \mathfrak{z}^1 + \mu_2 (66 + 9 \, \mathfrak{z}^1 - 65 \, \mathfrak{z}^2) + \\
& \quad \mu_1 (122 - 60 \, \mathfrak{z}^1 + 10 \, \mathfrak{z}^2)) + \\
& \quad 5 \, \eta^3 (-56 \, \mu_1 + \mathfrak{e} \mathfrak{p} (282 + 14 \, \mathfrak{z}^2 + 7 \, \mu_1 (20 + 3 \, \mathfrak{z}^1 + 3 \, \mathfrak{z}^2))) - \\
& \quad 2 \, \eta^2 (8 \times (5 + 58 \, \mu_1) + 5 \, \mathfrak{e} \mathfrak{p} (\mu_1 (-199 + 10 \, \mathfrak{z}^1 - 32 \, \mathfrak{z}^2) - \\
& \quad 3 \times (41 + \mathfrak{z}^1 + 6 \, \mathfrak{z}^2) + \mu_2 (-38 + 30 \, \mathfrak{z}^2))) + \\
& \quad \eta (95 - 29 \, \mu_1 + 15 \, \mu_2 + \mathfrak{e} \mathfrak{p} (282 + 24 \, \mathfrak{z}^1 + \mu_2 (338 + 9 \, \mathfrak{z}^1 - 321 \, \mathfrak{z}^2) + \\
& \quad 64 \, \mathfrak{z}^2 + \mu_1 (1078 - 246 \, \mathfrak{z}^1 + 144 \, \mathfrak{z}^2))) \Big) \Big) - \\
& x^3 (-1 + \eta)^3 \Big( - \Big( (-1 + \eta) \, \mathfrak{e} \mathfrak{p} (350 \, \eta^5 + 8 \times (5 + 5 \, \mu_1 + 6 \, \mu_2) + \eta \mathfrak{t} \\
& \quad (-32 - 54 \, \mu_1 + 30 \, \mu_2) - 10 \, \eta^4 (-241 + 35 \, \eta \mathfrak{t} - 105 \, \mu_1 + 84 \, \mu_2) + \\
& \quad 4 \, \eta^2 (233 + 605 \, \mu_1 + 292 \, \eta \mathfrak{t} \, \mu_1 + 308 \, \mu_2 + 25 \, \eta \mathfrak{t} (-5 + 7 \, \mu_2)) + \\
& \quad 20 \, \eta^3 (111 + 142 \, \mu_1 - 55 \, \mu_2 + 2 \, \eta \mathfrak{t} (-22 + 7 \, \mu_1 + 14 \, \mu_2)) + \\
& \quad \eta (8 \times (43 + 85 \, \mu_1 + 109 \, \mu_2) + \eta \mathfrak{t} (-155 + 281 \, \mu_1 + 189 \, \mu_2)) \Big) \Big) + \\
& (-1 + \eta \mathfrak{t}) \, \mathfrak{e} \mathfrak{l} (2 \times (5 + 7 \, \mu_1 - 15 \, \mu_2) + \mathfrak{e} \mathfrak{p} (2 \, \mu_2 (20 + 9 \, \mathfrak{z}^1 - 6 \, \mathfrak{z}^2) + \\
& \quad 5 \times (6 + 3 \, \mathfrak{z}^1 + \mathfrak{z}^2) + \mu_1 (34 - 11 \, \mathfrak{z}^1 + 7 \, \mathfrak{z}^2)) + \\
& \quad 10 \, \eta^4 (-28 \, \mu_1 + \mathfrak{e} \mathfrak{p} (153 + 7 \, \mathfrak{z}^2 + 7 \, \mu_1 (11 + 2 \, \mathfrak{z}^1 + 2 \, \mathfrak{z}^2))) - \\
& \quad 4 \, \eta^3 (20 + 278 \, \mu_1 + 5 \, \mathfrak{e} \mathfrak{p} (3 \, \mu_1 \mathfrak{z}^1 + 4 \, \mu_2 (-6 + 5 \, \mathfrak{z}^2) - \\
& \quad 5 \, \mu_1 (28 + 5 \, \mathfrak{z}^2) - 2 \times (45 + \mathfrak{z}^1 + 6 \, \mathfrak{z}^2))) + \\
& \quad \eta (6 \times (26 + 55 \, \mu_1 - 5 \, \mu_2) + 2 \, \mathfrak{e} \mathfrak{p} (78 + 25 \, \mathfrak{z}^1 + \mu_2 (142 + 27 \, \mathfrak{z}^1 - \\
& \quad 121 \, \mathfrak{z}^2) + 9 \, \mathfrak{z}^2 + \mu_1 (264 - 110 \, \mathfrak{z}^1 + 30 \, \mathfrak{z}^2))) + \\
& \quad \eta^2 (129 - 171 \, \mu_1 + 9 \, \mu_2 + \mathfrak{e} \mathfrak{p} (648 + 66 \, \mathfrak{z}^1 + 12 \, \mu_2 (56 + 3 \, \mathfrak{z}^1 - \\
& \quad 52 \, \mathfrak{z}^2) + 146 \, \mathfrak{z}^2 + \mu_1 (2272 - 434 \, \mathfrak{z}^1 + 346 \, \mathfrak{z}^2))) \Big) \Big) + \\
& x^2 (-1 + \eta)^2 \Big( - \Big( (-1 + \eta) \, \mathfrak{e} \mathfrak{p} (210 \, \eta^6 - 6 \, \eta \, \eta \mathfrak{t} (14 + 26 \, \mu_1 - 17 \, \mu_2) + \\
& \quad 8 \, \eta (15 + 15 \, \mu_1 + 17 \, \mu_2) - 30 \, \eta^5 \\
& \quad (-55 + 7 \, \eta \mathfrak{t} - 21 \, \mu_1 + 21 \, \mu_2) + \eta \mathfrak{t} (11 + 11 \, \mu_1 + 51 \, \mu_2) + \\
& \quad 4 \, \eta^3 (257 + 605 \, \mu_1 + 338 \, \eta \mathfrak{t} \, \mu_1 + 232 \, \mu_2 + 25 \, \eta \mathfrak{t} (-5 + 7 \, \mu_2)) + \\
& \quad 10 \, \eta^4 (193 + 213 \, \mu_1 - 120 \, \mu_2 + \eta \mathfrak{t} (-66 + 28 \, \mu_1 + 42 \, \mu_2)) + \\
& \quad 3 \, \eta^2 (\eta \mathfrak{t} (-73 + 183 \, \mu_1 + 99 \, \mu_2) + 4 \times (43 + 85 \, \mu_1 + 104 \, \mu_2)) \Big) \Big) + \\
& (-1 + \eta \mathfrak{t}) \, \mathfrak{e} \mathfrak{l} (-6 \times (2 + 2 \, \mu_1 + 3 \, \mu_2) + \mathfrak{e} \mathfrak{p} (12 + 8 \, \mathfrak{z}^1 + 6 \, \mathfrak{z}^2 + \\
& \quad 2 \, \mu_1 (6 + 4 \, \mathfrak{z}^1 + 3 \, \mathfrak{z}^2) + \mu_2 (14 + 9 \, \mathfrak{z}^1 + 7 \, \mathfrak{z}^2)) + \\
& \quad \eta (23 + 37 \, \mu_1 - 57 \, \mu_2 + \mathfrak{e} \mathfrak{p} (\mu_2 (134 + 63 \, \mathfrak{z}^1 - 27 \, \mathfrak{z}^2) - \\
& \quad 3 \, \mu_1 (-38 + 9 \, \mathfrak{z}^1 - 9 \, \mathfrak{z}^2) + 6 \times (18 + 9 \, \mathfrak{z}^1 + 4 \, \mathfrak{z}^2))) + \\
& \quad \eta^5 (-140 \, \mu_1 + 3 \, \mathfrak{e} \mathfrak{p} (330 + 14 \, \mathfrak{z}^2 + 7 \, \mu_1 (24 + 5 \, \mathfrak{z}^1 + 5 \, \mathfrak{z}^2))) - \\
& \quad 6 \, \eta^2 (-24 - 54 \, \mu_1 + 7 \, \mu_2 - \mathfrak{e} \mathfrak{p} (48 + 17 \, \mathfrak{z}^1 + 2 \, \mu_2 (38 + 9 \, \mathfrak{z}^1 - 28 \, \mathfrak{z}^2) + \\
& \quad 9 \, \mathfrak{z}^2 + \mu_1 (142 - 50 \, \mathfrak{z}^1 + 20 \, \mathfrak{z}^2))) + 2 \, \eta^4 (-4 \times (5 + 81 \, \mu_1) + 5 \, \mathfrak{e} \mathfrak{p} \\
& \quad (\mu_2 (34 - 30 \, \mathfrak{z}^2) + 3 \times (49 + \mathfrak{z}^1 + 6 \, \mathfrak{z}^2) + \mu_1 (221 + \mathfrak{z}^1 + 43 \, \mathfrak{z}^2))) + \\
& \quad \eta^3 (77 - 199 \, \mu_1 - 3 \, \mu_2 + \mathfrak{e} \mathfrak{p} (732 + 84 \, \mathfrak{z}^1 + \mu_2 (668 + 54 \, \mathfrak{z}^1 - 606 \, \mathfrak{z}^2) + \\
& \quad 164 \, \mathfrak{z}^2 + \mu_1 (2388 - 376 \, \mathfrak{z}^1 + 404 \, \mathfrak{z}^2))) \Big) \Big) + \\
& x (-1 + \eta) \times (70 \, \eta^8 \, \mathfrak{e} \mathfrak{p} + 2 \, \eta^7 \, \mathfrak{e} \mathfrak{p} (274 - 35 \, \eta \mathfrak{t} + 105 \, \mu_1 - 126 \, \mu_2) - 6 \\
& \quad \eta \mathfrak{t} \, \mathfrak{e} \mathfrak{p} (3 + 3 \, \mu_1 + 4 \, \mu_2) - \eta (\eta \mathfrak{t} \, \mathfrak{e} \mathfrak{p} (1 - 5 \, \mu_1 + 75 \, \mu_2) + \\
& \quad 2 \times (-1 + \eta \mathfrak{t}) \, \mathfrak{e} \mathfrak{l} (-3 \times (1 + \mu_1 + 2 \, \mu_2) + \mathfrak{e} \mathfrak{p}
\end{aligned}$$

$$\begin{aligned}
& (12 + 8 \mathfrak{e}1 + 6 \mathfrak{e}2 + 2 \mu1 (6 + 4 \mathfrak{e}1 + 3 \mathfrak{e}2) + \mu2 (14 + 9 \mathfrak{e}1 + 7 \mathfrak{e}2))) + \\
& \eta^2 (\theta p (\eta t (91 + 163 \mu1 - 15 \mu2) - 8 \times (15 + 15 \mu1 + 16 \mu2)) + \\
& (-1 + \eta t) \theta l (-13 - 23 \mu1 + 27 \mu2 - \theta p (126 + 63 \mathfrak{e}1 + \\
& 2 \mu2 (74 + 36 \mathfrak{e}1 - 9 \mathfrak{e}2) + 33 \mathfrak{e}2 + \mu1 (126 - 21 \mathfrak{e}1 + 33 \mathfrak{e}2)))) + \\
& \eta^3 (-\theta p (8 \times (28 + 70 \mu1 + 83 \mu2) + \eta t (-65 + 601 \mu1 + 93 \mu2)) + \\
& 2 \times (-1 + \eta t) \theta l (-22 - 53 \mu1 + 9 \mu2 - \theta p (114 + 43 \mathfrak{e}1 + \\
& \mu2 (162 + 45 \mathfrak{e}1 - 103 \mathfrak{e}2) + 27 \mathfrak{e}2 + \mu1 (304 - 90 \mathfrak{e}1 + 50 \mathfrak{e}2)))) - \\
& 2 \eta^5 (-\theta p (-158 + 179 \mu1 + 471 \mu2 + \eta t (7 + 314 \mu1 + 91 \mu2)) + \\
& (-1 + \eta t) \theta l (-4 - 74 \mu1 + \theta p (\mu2 (64 - 60 \mathfrak{e}2) + \\
& 6 \times (53 + \mathfrak{e}1 + 6 \mathfrak{e}2) + \mu1 (464 + 13 \mathfrak{e}1 + 97 \mathfrak{e}2)))) + \eta^4 \\
& (-\theta p (218 + 530 \mu1 - 480 \mu2 + \eta t (-113 + 317 \mu1 + 143 \mu2)) + \\
& (-1 + \eta t) \theta l (-17 + 71 \mu1 + 3 \mu2 - \theta p (408 + 51 \mathfrak{e}1 + \mu2 (332 + 36 \mathfrak{e}1 - \\
& 294 \mathfrak{e}2) + 91 \mathfrak{e}2 + \mu1 (1252 - 159 \mathfrak{e}1 + 231 \mathfrak{e}2)))) - 2 \\
& \eta^6 (-14 \times (-1 + \eta t) \theta l \mu1 + \theta p (-130 - 321 \mu1 + 189 \mu2 - \\
& \theta l (177 + 7 \mathfrak{e}2 + 7 \mu1 (13 + 3 \mathfrak{e}1 + 3 \mathfrak{e}2)) + \eta t (97 - 70 \mu1 - \\
& 84 \mu2 + \theta l (177 + 7 \mathfrak{e}2 + 7 \mu1 (13 + 3 \mathfrak{e}1 + 3 \mathfrak{e}2)))))) - \\
& (x + \eta - x \eta)^2 (-2 x^6 (-1 + \eta)^6 \theta p (3 + 8 \eta^2 - 3 \theta l - 11 \mu1 + 7 \theta l \mu1 + \eta \\
& (-11 + 4 \theta l - 4 \eta t (1 + \theta l) + 11 \mu1) + \theta l \mathfrak{e}2 + \eta t (4 - \theta l (-3 + 7 \mu1 + \mathfrak{e}2))) + \\
& x^5 (-1 + \eta)^5 (2 \times (-1 + \eta) \theta p (-2 + 48 \eta^2 + 26 \mu1 + 10 \mu2 + \\
& \eta t (-8 + 7 \mu2) - 2 \eta (1 + 12 \eta t - 33 \mu1 + 7 \mu2)) - (-1 + \eta t) \\
& \theta l (-4 + 48 \eta^2 \theta p + 16 \theta p \mu2 + \theta p \mathfrak{e}1 + 5 \theta p \mathfrak{e}2 - 10 \theta p \mu2 \mathfrak{e}2 + \\
& \eta (-28 \mu1 + 7 \theta p \mu1 (14 + \mathfrak{e}1 + \mathfrak{e}2) + 4 \theta p (-5 + 3 \mathfrak{e}2)) + \\
& \mu1 (-12 + \theta p (44 - 11 \mathfrak{e}1 + 3 \mathfrak{e}2))) + \\
& \eta \theta p (-16 \eta^7 + 4 \eta t \mu2 + 2 \eta^6 (-5 - 4 \theta l + 4 \eta t (1 + \theta l) - 11 \mu1 + 14 \mu2) + \\
& \eta^5 (14 - 30 \mu1 - 8 \mu2 - 2 \theta l (5 + \mathfrak{e}2) - 7 \theta l \mu1 (4 + \mathfrak{e}1 + \mathfrak{e}2) + \\
& \eta t (8 - 28 \mu1 - 14 \mu2 + 2 \theta l (5 + \mathfrak{e}2) + 7 \theta l \mu1 (4 + \mathfrak{e}1 + \mathfrak{e}2))) + \eta^2 \\
& (4 \times (5 + 5 \mu1 + 6 \mu2) - \theta l (12 - 10 \mu1 (-1 + \mathfrak{e}1) + 5 \mathfrak{e}1 + \\
& 2 \mu2 (8 + 3 \mathfrak{e}1 - 4 \mathfrak{e}2) + \mathfrak{e}2) + \eta t (4 - 4 \mu2 + \\
& \theta l (12 - 10 \mu1 (-1 + \mathfrak{e}1) + 5 \mathfrak{e}1 + 2 \mu2 (8 + 3 \mathfrak{e}1 - 4 \mathfrak{e}2) + \mathfrak{e}2))) + \\
& \eta^4 (-4 \eta t (3 + 7 \mu1) + 2 \times (-5 + \mu1 - 40 \mu2) - \theta l (8 + \mathfrak{e}1 + 5 \mathfrak{e}2 - \\
& 2 \mu2 (-6 + 5 \mathfrak{e}2) + 2 \mu1 (33 + 7 \mathfrak{e}2)) + \\
& \eta t \theta l (8 + \mathfrak{e}1 + 5 \mathfrak{e}2 - 2 \mu2 (-6 + 5 \mathfrak{e}2) + 2 \mu1 (33 + 7 \mathfrak{e}2))) + \\
& \eta^3 (2 + 30 \mu1 + 70 \eta t \mu1 + 36 \mu2 + 10 \eta t \mu2 + (-1 + \eta t) \theta l \\
& (18 + 4 \mathfrak{e}1 + \mu2 (26 + 3 \mathfrak{e}1 - 19 \mathfrak{e}2) + 4 \mathfrak{e}2 + \mu1 (48 - 19 \mathfrak{e}1 + 7 \mathfrak{e}2))) + \eta \\
& (-\theta l (2 \times (1 + \mu1) \mathfrak{e}1 + \mu2 (2 + 3 \mathfrak{e}1 + \mathfrak{e}2)) + \eta t (-8 + 2 \theta l \mathfrak{e}1 + \\
& 2 \mu1 (-7 + \theta l \mathfrak{e}1) + \mu2 (4 + \theta l (2 + 3 \mathfrak{e}1 + \mathfrak{e}2)))) + \\
& x^2 (-1 + \eta)^2 (-2 \times (-1 + \eta) \theta p (120 \eta^5 + \eta t (-7 - 8 \mu1 + \mu2) - \\
& 5 \eta^4 (-23 + 12 \eta t - 33 \mu1 + 28 \mu2) + \\
& \eta (30 + 30 \mu1 + 44 \mu2 + \eta t (-9 - 20 \mu1 + 3 \mu2)) + \\
& 6 \eta^2 (11 + 25 \mu1 + 34 \mu2 + \eta t (-2 + 20 \mu1 + 7 \mu2)) + \\
& \eta^3 (4 \times (7 + 65 \mu1 - 5 \mu2) + \eta t (-80 + 84 \mu1 + 70 \mu2))) + (-1 + \eta t) \theta l \\
& (120 \eta^5 \theta p + 2 \times (3 + 3 \mu1 + \mu2) - \theta p (6 + \mathfrak{e}1 + 3 \mathfrak{e}2 + 2 \mu2 (2 + \mathfrak{e}2) + \\
& \mu1 (6 + \mathfrak{e}1 + 3 \mathfrak{e}2)) - 2 \eta^3 (8 + 72 \mu1 + \theta p (-24 - 68 \mu2 - \\
& 5 \mathfrak{e}1 + \mu1 (-286 + 22 \mathfrak{e}1 - 48 \mathfrak{e}2) - 25 \mathfrak{e}2 + 50 \mu2 \mathfrak{e}2)) + \\
& 2 \eta^4 (-56 \mu1 + 5 \theta p (7 + 3 \mathfrak{e}2 + 7 \mu1 (5 + \mathfrak{e}1 + \mathfrak{e}2))) + \\
& \eta (2 \times (17 + 23 \mu1 + \mu2) + \theta p (\mu2 (32 + 6 \mathfrak{e}1 - 36 \mathfrak{e}2) +
\end{aligned}$$



$$\begin{aligned}
& 3 \times (4 + \mathfrak{d}1 - 3 \mathfrak{d}2) - 6 \mu 1 (-3 + 6 \mathfrak{d}1 + \mathfrak{d}2)) + \\
& \eta^2 (24 + 92 \mu 1 + 3 \mathfrak{d}p (\mu 2 (54 + 3 \mathfrak{d}1 - 41 \mathfrak{d}2) + 5 \times (6 + \mathfrak{d}1 + \mathfrak{d}2) + \\
& \mu 1 (88 - 42 \mathfrak{d}1 + 10 \mathfrak{d}2))) - \\
& x^3 (-1 + \eta)^3 \left( - \left( (-1 + \eta) \mathfrak{d}p (320 \eta^4 + \eta t (-7 - 13 \mu 1 + \mu 2) - 40 \eta^3 \right. \right. \\
& (-5 + 4 \eta t - 11 \mu 1 + 7 \mu 2) + 4 \times (5 + 5 \mu 1 + 8 \mu 2) + \\
& 8 \eta (11 + 25 \mu 1 + 36 \mu 2 + \eta t (-2 + 16 \mu 1 + 7 \mu 2)) + 4 \eta^2 \\
& (2 \times (3 + 65 \mu 1 + 5 \mu 2) + \eta t (-40 + 28 \mu 1 + 35 \mu 2))) \left. \right) + (-1 + \eta t) \mathfrak{d}l \\
& (20 + 160 \eta^4 \mathfrak{d}p + 4 \mu 2 + 8 \mathfrak{d}p \mu 2 - \mathfrak{d}p \mathfrak{d}1 + \mu 1 (24 + \mathfrak{d}p (4 - 13 \mathfrak{d}1 - 3 \mathfrak{d}2)) - \\
& 5 \mathfrak{d}p \mathfrak{d}2 - 14 \mathfrak{d}p \mu 2 \mathfrak{d}2 - 2 \eta^2 (12 + 84 \mu 1 + \mathfrak{d}p (-16 - 72 \mu 2 - \\
& 5 \mathfrak{d}1 + \mu 1 (-264 + 33 \mathfrak{d}1 - 37 \mathfrak{d}2) - 25 \mathfrak{d}2 + 50 \mu 2 \mathfrak{d}2)) + \\
& 2 \eta^3 (-84 \mu 1 + 5 \mathfrak{d}p (4 \times (1 + \mathfrak{d}2) + 7 \mu 1 (6 + \mathfrak{d}1 + \mathfrak{d}2))) + \\
& \eta (27 + 91 \mu 1 + 3 \mu 2 + \mathfrak{d}p (54 + 7 \mathfrak{d}1 + \mu 2 (110 + 3 \mathfrak{d}1 - 85 \mathfrak{d}2) + \\
& 7 \mathfrak{d}2 + \mu 1 (168 - 88 \mathfrak{d}1 + 16 \mathfrak{d}2))) \left. \right) + \\
& x^4 (-1 + \eta)^4 \left( -2 \times (-1 + \eta) \mathfrak{d}p (11 + 120 \eta^3 + 25 \mu 1 + 38 \mu 2 + \eta t \right. \\
& (-2 + 12 \mu 1 + 7 \mu 2) - 5 \eta^2 (-7 + 12 \eta t - 33 \mu 1 + 14 \mu 2) + \\
& \eta (-2 + 130 \mu 1 + 30 \mu 2 + \eta t (-40 + 14 \mu 1 + 35 \mu 2)) \left. \right) + \\
& (-1 + \eta t) \mathfrak{d}l (120 \eta^3 \mathfrak{d}p + 2 \times (5 + 15 \mu 1 + \mu 2) + \mathfrak{d}p \\
& (12 + 28 \mu 2 + \mathfrak{d}1 + \mathfrak{d}2 - 22 \mu 2 \mathfrak{d}2 + \mu 1 (40 - 23 \mathfrak{d}1 + 3 \mathfrak{d}2)) + \\
& \eta^2 (-112 \mu 1 + 5 \mathfrak{d}p (-2 + 6 \mathfrak{d}2 + 7 \mu 1 (8 + \mathfrak{d}1 + \mathfrak{d}2))) + \\
& \eta (-16 \times (1 + 5 \mu 1) + \mathfrak{d}p (8 + 76 \mu 2 + 5 \mathfrak{d}1 + 25 \mathfrak{d}2 - \\
& 50 \mu 2 \mathfrak{d}2 + \mu 1 (242 - 44 \mathfrak{d}1 + 26 \mathfrak{d}2))) \left. \right) + \\
& x (-1 + \eta) \times (96 \eta^7 \mathfrak{d}p + \eta t \mathfrak{d}p (3 + 3 \mu 1 - \mu 2) - 4 \eta^6 \mathfrak{d}p (-7 - 12 \mathfrak{d}l + \\
& 12 \eta t (1 + \mathfrak{d}l) - 33 \mu 1 + 35 \mu 2) + \eta^4 \\
& (2 \mathfrak{d}p (22 - 30 \mu 1 + \eta t (32 + 40 \mu 1 - 7 \mu 2) + 158 \mu 2) + \\
& (-1 + \eta t) \mathfrak{d}l (4 + 44 \mu 1 + \mathfrak{d}p (-32 - 64 \mu 2 - 5 \mathfrak{d}1 + \\
& \mu 1 (-308 + 11 \mathfrak{d}1 - 59 \mathfrak{d}2) - 25 \mathfrak{d}2 + 50 \mu 2 \mathfrak{d}2))) + \eta^2 \\
& (\mathfrak{d}p (\eta t (-7 + 11 \mu 1 + \mu 2) - 20 \times (3 + 3 \mu 1 + 4 \mu 2)) + (-1 + \eta t) \\
& \mathfrak{d}l (2 \times (-7 - 11 \mu 1 + \mu 2) + \mathfrak{d}p (-2 \mu 2 (20 + 6 \mathfrak{d}1 - 15 \mathfrak{d}2) + \\
& 3 \times (-8 - 3 \mathfrak{d}1 + \mathfrak{d}2) + 3 \mu 1 (-8 + 11 \mathfrak{d}1 + \mathfrak{d}2))) + \eta^3 \\
& (-\mathfrak{d}p (4 \times (7 + 35 \mu 1 + 44 \mu 2) + \eta t (-1 + 233 \mu 1 + 47 \mu 2)) + \\
& (-1 + \eta t) \mathfrak{d}l (-7 - 31 \mu 1 + \mu 2 - \mathfrak{d}p (66 + 13 \mathfrak{d}1 + \mu 2 (106 + 9 \mathfrak{d}1 - 79 \mathfrak{d}2) + \\
& 13 \mathfrak{d}2 + \mu 1 (184 - 80 \mathfrak{d}1 + 24 \mathfrak{d}2))) + \eta \\
& (\eta t \mathfrak{d}p (19 + 27 \mu 1 - 9 \mu 2) - (-1 + \eta t) \mathfrak{d}l (3 + 3 \mu 1 - \mu 2 + \\
& \mathfrak{d}p (-6 + \mathfrak{d}1 + \mu 2 (-2 + 3 \mathfrak{d}1 - \mathfrak{d}2) - 3 \mathfrak{d}2 + \mu 1 (\mathfrak{d}1 - 3 \times (2 + \mathfrak{d}2)))) + \\
& \eta^5 (28 \times (-1 + \eta t) \mathfrak{d}l \mu 1 + \mathfrak{d}p (16 \times (-5 + 8 \mu 1 + 5 \mu 2) + \mathfrak{d}l \\
& (44 + 12 \mathfrak{d}2 + 7 \mu 1 (22 + 5 \mathfrak{d}1 + 5 \mathfrak{d}2)) - \eta t (32 - 112 \mu 1 - \\
& 70 \mu 2 + \mathfrak{d}l (44 + 12 \mathfrak{d}2 + 7 \mu 1 (22 + 5 \mathfrak{d}1 + 5 \mathfrak{d}2)))) \left. \right) \left. \right) \left. \right) \left. \right) / \\
& (192 (-1 + w (-1 + \eta))^3 (x (-1 + \eta) - \eta)^3 (1 + x + \eta - x \eta)^2 \\
& (w + \\
& x + \\
& \eta - \\
& w \eta - \\
& x \eta)^3 (-1 + \eta t) \mathfrak{d}p)) \\
\beta c \sigma = & - \left( (c \sigma (-8 \times (-1 + w (-1 + \eta)) (x (-1 + \eta) - \eta)^3 (w (-1 + \eta) + x (-1 + \eta) - \eta) \right. \\
& (-1 + \eta t) \mathfrak{d}p (3 (c v^2 - 4 \epsilon) (1 + w - w \eta)^2 (w + x + \eta - w \eta - x \eta)^2 +
\end{aligned}$$

$$\begin{aligned}
& 2 \, c \sigma^2 \, (-1 + \eta) \times \left( -5 \, x - 4 \, x^2 - 5 \, \eta - 3 \, x \, \eta + 8 \, x^2 \, \eta - 4 \, \eta^2 + 8 \, x \, \eta^2 - 4 \, x^2 \, \eta^2 - 4 \, x \, \mu 1 + \right. \\
& \quad 2 \, x^2 \, \mu 1 - 4 \, \eta \, \mu 1 + 8 \, x \, \eta \, \mu 1 - 3 \, x^2 \, \eta \, \mu 1 + 2 \, \eta^2 \, \mu 1 - 2 \, x \, \eta^2 \, \mu 1 + \eta^3 \, \mu 1 - 2 \, x \, \eta^3 \, \mu 1 + \\
& \quad x^2 \, \eta^3 \, \mu 1 + x \, \mu 1^2 - 3 \, x^2 \, \mu 1^2 + \eta \, \mu 1^2 - 7 \, x \, \eta \, \mu 1^2 + 7 \, x^2 \, \eta \, \mu 1^2 - 3 \, \eta^2 \, \mu 1^2 + \\
& \quad 8 \, x \, \eta^2 \, \mu 1^2 - 5 \, x^2 \, \eta^2 \, \mu 1^2 + \eta^3 \, \mu 1^2 - 2 \, x \, \eta^3 \, \mu 1^2 + x^2 \, \eta^3 \, \mu 1^2 - 2 \, x \, \mu 2 - \eta \, \mu 2 + \\
& \quad 2 \, x \, \eta \, \mu 2 - 8 \, x \, \mu 1 \, \mu 2 - 13 \, \eta \, \mu 1 \, \mu 2 + 8 \, x \, \eta \, \mu 1 \, \mu 2 + 9 \, w^3 \, (-1 + \eta)^3 \, (1 + 2 \, \mu 1 \, \mu 2) + \\
& \quad w \, (-1 + \eta) \times \left( 5 + x^2 \, (-1 + \eta)^2 \, (-2 + \mu 1)^2 + 4 \, \mu 1 - \mu 1^2 - \eta^2 \, (-4 + 6 \, \mu 1 + \mu 1^2) + \right. \\
& \quad \quad 18 \, \mu 1 \, \mu 2 + 2 \, x \, (-1 + \eta) \times \left( -9 - 2 \, \mu 1 - 2 \, \mu 1^2 + \eta \, (-4 + 5 \, \mu 1) - \right. \\
& \quad \quad \quad 2 \, \mu 2 - 8 \, \mu 1 \, \mu 2) + 2 \, \eta \, (9 + 2 \, \mu 1 + 2 \, \mu 1^2 + \mu 2 + 13 \, \mu 1 \, \mu 2) \Big) + \\
& \quad w^2 \, (-1 + \eta)^2 \, (-14 - 6 \, \mu 1 - \mu 1^2 - 36 \, \mu 1 \, \mu 2 - \eta \, (13 - 5 \, \mu 1 + \mu 2 + 13 \, \mu 1 \, \mu 2) + \\
& \quad \quad x \, (-1 + \eta) \times \left( 13 + \mu 1^2 + 2 \, \mu 2 + \mu 1 \, (-4 + 8 \, \mu 2) \right) \Big) \Big) + \\
& f \left( -16 \, w^6 \, (-1 + \eta)^6 \, (x + \eta - x \, \eta)^3 \, (-1 + \eta t) \, \theta l \, \theta p \, (-4 + \mathfrak{z}2) + \right. \\
& \quad (x + \eta - x \, \eta)^2 \, (-4 \, x^4 \, (-1 + \eta)^4 \, \theta p \, (-48 + 30 \, \eta^4 + 64 \, \theta l - \\
& \quad \quad 2 \, \eta^3 \, (39 - 5 \, \theta l + 5 \, \eta t \, (2 + \theta l)) + 4 \, \theta l \, \mathfrak{z}2 + \eta t \, (9 - 4 \, \theta l \, (16 + \mathfrak{z}2)) + \\
& \quad \quad \eta^2 \, (18 - 19 \, \theta l + 2 \, \theta l \, \mathfrak{z}2 + \eta t \, (49 + 19 \, \theta l - 2 \, \theta l \, \mathfrak{z}2)) + \\
& \quad \quad \eta \, (78 - 39 \, \theta l - 10 \, \theta l \, \mathfrak{z}2 + \eta t \, (-38 + 39 \, \theta l + 10 \, \theta l \, \mathfrak{z}2)) \Big) - x^2 \, (-1 + \eta)^2 \\
& \quad \quad \left( 720 \, \eta^6 \, \theta p - 22 \, \eta t \, \theta p - 48 \, \eta^5 \, (39 - 5 \, \theta l + 5 \, \eta t \, (2 + \theta l)) \, \theta p + \eta^2 \, (2 \times (-576 + \right. \\
& \quad \quad \quad 97 \, \eta t) \, \theta p + (-1 + \eta t) \, \theta l \, (-84 + \theta p \, (-1430 + 141 \, \mathfrak{z}1 - 43 \, \mathfrak{z}2)) \Big) - \\
& \quad \quad 24 \, \eta^4 \, \theta p \, (-18 + 19 \, \theta l - 2 \, \theta l \, \mathfrak{z}2 + \eta t \, (-49 - 19 \, \theta l + 2 \, \theta l \, \mathfrak{z}2)) + \\
& \quad \quad 24 \, \eta^3 \, \theta p \, (78 - 39 \, \theta l - 10 \, \theta l \, \mathfrak{z}2 + \eta t \, (-38 + 39 \, \theta l + 10 \, \theta l \, \mathfrak{z}2)) + \\
& \quad \quad \eta \, (44 \, \eta t \, \theta p - (-1 + \eta t) \, \theta l \, (-84 + 141 \, \theta p \, \mathfrak{z}1 + 53 \, \theta p \, (2 + \mathfrak{z}2))) \Big) + \\
& \quad 16 \, x^3 \, (-1 + \eta)^3 \, ((-1 + \eta)^2 \, \eta \, (-48 + 30 \, \eta^2 + 9 \, \eta t - 2 \, \eta \, (9 + 10 \, \eta t)) \, \theta p - \\
& \quad \quad (-1 + \eta t) \, \theta l \, (-2 + 10 \, \eta^4 \, \theta p + \theta p \, (2 + 3 \, \mathfrak{z}1 + \mathfrak{z}2) + \eta^3 \, \theta p \, (-19 + 2 \, \mathfrak{z}2) - \\
& \quad \quad \quad \eta^2 \, \theta p \, (39 + 10 \, \mathfrak{z}2) + \eta \, (2 + \theta p \, (62 - 3 \, \mathfrak{z}1 + 3 \, \mathfrak{z}2))) \Big) + \\
& \quad \eta^2 \, \theta p \, (-120 \, \eta^6 + 30 \, \eta t + 8 \, \eta^5 \, (39 - 5 \, \theta l + 5 \, \eta t \, (2 + \theta l)) + \\
& \quad \quad 3 \, \eta \, (-20 \, \eta t - 13 \, \theta l \, \mathfrak{z}1 - 5 \, \theta l \, (2 + \mathfrak{z}2) + \eta t \, \theta l \, (13 \, \mathfrak{z}1 + 5 \times (2 + \mathfrak{z}2))) + \\
& \quad \quad \eta^2 \, (192 + \theta l \, (-226 + 39 \, \mathfrak{z}1 - \mathfrak{z}2) + \eta t \, (-6 + \theta l \, (226 - 39 \, \mathfrak{z}1 + \mathfrak{z}2))) + \\
& \quad \quad 4 \, \eta^4 \, (-18 + \theta l \, (19 - 2 \, \mathfrak{z}2) + \eta t \, (-49 + \theta l \, (-19 + 2 \, \mathfrak{z}2))) - \\
& \quad \quad 4 \, \eta^3 \, (78 - \theta l \, (39 + 10 \, \mathfrak{z}2) + \eta t \, (-38 + \theta l \, (39 + 10 \, \mathfrak{z}2))) \Big) + \\
& \quad 4 \, x \, (-1 + \eta) \, \eta \, (120 \, \eta^6 \, \theta p - 22 \, \eta t \, \theta p - 8 \, \eta^5 \, (39 - 5 \, \theta l + 5 \, \eta t \, (2 + \theta l)) \, \theta p + \\
& \quad \quad \eta^2 \, (2 \times (-96 + 7 \, \eta t) \, \theta p + (-1 + \eta t) \, \theta l \, (-4 + \theta p \, (-230 + 33 \, \mathfrak{z}1 - 3 \, \mathfrak{z}2))) + \\
& \quad \quad 4 \, \eta^4 \, \theta p \, (18 + \eta t \, (49 + \theta l \, (19 - 2 \, \mathfrak{z}2)) + \theta l \, (-19 + 2 \, \mathfrak{z}2)) + \\
& \quad \quad \eta \, (44 \, \eta t \, \theta p - (-1 + \eta t) \, \theta l \, (-4 + 33 \, \theta p \, \mathfrak{z}1 + 13 \, \theta p \, (2 + \mathfrak{z}2))) + \\
& \quad \quad 4 \, \eta^3 \, \theta p \, (78 - \theta l \, (39 + 10 \, \mathfrak{z}2) + \eta t \, (-38 + \theta l \, (39 + 10 \, \mathfrak{z}2))) \Big) + \\
& w \, (x \, (-1 + \eta) - \eta) \, (-1 + \eta) \times \left( 4 \, x^4 \, (-1 + \eta)^4 \, (-(-1 + \eta)^2 \, \theta p \, (150 \, \eta^3 + \right. \\
& \quad \quad \eta^2 \, (255 - 150 \, \eta t) + 9 \times (-16 + 3 \, \eta t) - 2 \, \eta \, (437 + 35 \, \eta t - 70 \, \mu 1)) + \\
& \quad \quad (-1 + \eta t) \, \theta l \, (-24 + 24 \, \eta + 36 \, \theta p \, \mathfrak{z}1 + 4 \, \eta^2 \, \theta p \, (-258 + 35 \, \mu 1 - 16 \, \mathfrak{z}2) + \\
& \quad \quad \quad 24 \, \theta p \, (9 + \mathfrak{z}2) + 5 \, \eta^3 \, \theta p \, (37 + 2 \, \mathfrak{z}2) - \\
& \quad \quad \quad \eta \, \theta p \, (-919 + 140 \, \mu 1 + 36 \, \mathfrak{z}1 + 42 \, \mathfrak{z}2)) \Big) + 4 \, x^5 \, (-1 + \eta)^5 \\
& \quad \theta p \, (30 \, \eta^4 - 3 \, \eta^3 \, (9 + 10 \, \eta t) - 4 \times (41 - 7 \, \mu 1 + \theta l \, (-53 + 7 \, \mu 1)) + \\
& \quad \quad \eta t \, (-2 + 4 \, \theta l \, (-53 + 7 \, \mu 1)) + \eta^2 \, (-200 + 31 \, \theta l + 28 \, \mu 1 + \\
& \quad \quad \quad 2 \, \theta l \, \mathfrak{z}2 + \eta t \, (58 - \theta l \, (31 + 2 \, \mathfrak{z}2))) + \eta \, (361 - 56 \, \mu 1 + \\
& \quad \quad \quad \theta l \, (-195 + 28 \, \mu 1 - 14 \, \mathfrak{z}2) + \eta t \, (-26 + \theta l \, (195 - 28 \, \mu 1 + 14 \, \mathfrak{z}2))) \Big) - \\
& \quad \eta^2 \, \theta p \, (120 \, \eta^7 + \eta^6 \, (252 - 120 \, \eta t) + 10 \, \eta t \, (-17 + 8 \, \mu 1) - 4 \, \eta^4 \, (-415 + 56 \\
& \quad \quad \mu 1 + \eta t \, (-121 + 4 \, \theta l \, (-63 + 7 \, \mu 1 - 2 \, \mathfrak{z}2)) + \theta l \, (252 - 28 \, \mu 1 + 8 \, \mathfrak{z}2)) +
\end{aligned}$$

$$\begin{aligned}
& \eta^2 (-576 + 118 \eta t + 80 \eta t \mu_1 + 8 \theta l (86 - \mathfrak{z}1 + \mathfrak{z}2 + 5 \mu_1 (2 + \mathfrak{z}1 + \mathfrak{z}2)) - \\
& \quad 8 \eta t \theta l (86 - \mathfrak{z}1 + \mathfrak{z}2 + 5 \mu_1 (2 + \mathfrak{z}1 + \mathfrak{z}2))) - \\
& 4 \eta^5 (434 - 28 \mu_1 - \theta l (61 + 2 \mathfrak{z}2) + \eta t (2 + \theta l (61 + 2 \mathfrak{z}2))) + \\
& \eta^3 (56 \times (5 + 2 \mu_1) - \theta l (-290 + 112 \mu_1 + 117 \mathfrak{z}1 + 165 \mathfrak{z}2) + \\
& \quad \eta t (-554 + \theta l (-290 + 112 \mu_1 + 117 \mathfrak{z}1 + 165 \mathfrak{z}2))) + \\
& 5 \eta (\theta l (25 \mathfrak{z}1 + 17 \times (2 + \mathfrak{z}2) - 8 \mu_1 (2 + \mathfrak{z}1 + \mathfrak{z}2)) + \\
& \quad \eta t (50 - 32 \mu_1 + \theta l (-25 \mathfrak{z}1 - 17 \times (2 + \mathfrak{z}2) + 8 \mu_1 (2 + \mathfrak{z}1 + \mathfrak{z}2)))) + \\
& x^3 (-1 + \eta)^3 (2 (-1 + \eta)^2 \theta p (600 \eta^4 - 33 \eta t + 72 \eta (-16 + 3 \eta t) - \\
& \quad 60 \eta^3 (-23 + 10 \eta t) - 8 \eta^2 (464 + 65 \eta t - 70 \mu_1)) - (-1 + \eta t) \\
& \quad \theta l (8 \eta^3 \theta p (-1089 + 140 \mu_1 - 58 \mathfrak{z}2) + 40 \eta^4 \theta p (43 + 2 \mathfrak{z}2) + \\
& \quad \eta^2 (348 - \theta p (-6194 + 1120 \mu_1 + 567 \mathfrak{z}1 + 687 \mathfrak{z}2)) - 8 \times (26 - 10 \mu_1 + \\
& \quad \theta p (-19 \mathfrak{z}1 - 13 \times (2 + \mathfrak{z}2) + 5 \mu_1 (2 + \mathfrak{z}1 + \mathfrak{z}2))) + \eta (-20 \times (7 + \\
& \quad 4 \mu_1) + \theta p (3278 + 415 \mathfrak{z}1 + 295 \mathfrak{z}2 + 40 \mu_1 (2 + \mathfrak{z}1 + \mathfrak{z}2)))) + \\
& x (-1 + \eta) \eta (600 \eta^7 \theta p - 300 \eta^6 (-3 + 2 \eta t) \theta p + 2 \eta t \theta p (-209 + 80 \mu_1) - \\
& 4 \eta^4 \theta p (-2021 + 280 \mu_1 + \eta t (-458 + \theta l (-1203 + 140 \mu_1 - 46 \mathfrak{z}2)) + \theta l \\
& \quad (1203 - 140 \mu_1 + 46 \mathfrak{z}2)) - 4 \eta^5 \theta p (1936 - 140 \mu_1 - 5 \theta l (55 + 2 \mathfrak{z}2) + \\
& 5 \eta t (-10 + \theta l (55 + 2 \mathfrak{z}2))) + \eta^3 (2 \theta p (232 - 1109 \eta t + 280 \mu_1) + \\
& \quad (-1 + \eta t) \theta l (-48 + \theta p (-1966 + 560 \mu_1 + 513 \mathfrak{z}1 + 681 \mathfrak{z}2))) + \\
& 2 \eta (\eta t \theta p (241 - 160 \mu_1) + (-1 + \eta t) \theta l (65 - 40 \mu_1 + \\
& \quad \theta p (-201 \mathfrak{z}1 - 137 \times (2 + \mathfrak{z}2) + 60 \mu_1 (2 + \mathfrak{z}1 + \mathfrak{z}2)))) + \\
& \eta^2 (2 \theta p (-1152 + \eta t (361 + 80 \mu_1)) - (-1 + \eta t) \theta l \\
& \quad (82 - 80 \mu_1 + \theta p (2926 + 111 \mathfrak{z}1 + 119 \mathfrak{z}2 + 120 \mu_1 (2 + \mathfrak{z}1 + \mathfrak{z}2)))) - \\
& x^2 (-1 + \eta)^2 (1200 \eta^7 \theta p - 120 \eta^6 (-9 + 10 \eta t) \theta p + 4 \eta t \theta p (-53 + 20 \mu_1) - \\
& 8 \eta^4 \theta p (7 \times (-281 + 40 \mu_1) + \eta t (-311 + 2 \theta l (-573 + 70 \mu_1 - 26 \mathfrak{z}2)) + \theta l \\
& \quad (1146 - 140 \mu_1 + 52 \mathfrak{z}2)) - 8 \eta^5 \theta p (1702 - 140 \mu_1 - 5 \theta l (49 + 2 \mathfrak{z}2) + \\
& 5 \eta t (-22 + \theta l (49 + 2 \mathfrak{z}2))) + \eta^3 (-2 \theta p (472 + 1573 \eta t - 560 \mu_1) + \\
& \quad (-1 + \eta t) \theta l (-300 + \theta p (-5042 + 1120 \mu_1 + 819 \mathfrak{z}1 + 1035 \mathfrak{z}2))) - \\
& 2 \eta^2 (-4 \theta p (-432 + \eta t (137 + 10 \mu_1)) + (-1 + \eta t) \theta l \\
& \quad (37 - 80 \mu_1 + \theta p (2326 + 195 \mathfrak{z}1 + 155 \mathfrak{z}2 + 60 \mu_1 (2 + \mathfrak{z}1 + \mathfrak{z}2)))) + \\
& \eta (2 \eta t \theta p (47 - 80 \mu_1) + (-1 + \eta t) \theta l (374 - 160 \mu_1 + \\
& \quad \theta p (-429 \mathfrak{z}1 - 293 \times (2 + \mathfrak{z}2) + 120 \mu_1 (2 + \mathfrak{z}1 + \mathfrak{z}2)))) + \\
& w^2 (-1 + \eta)^2 (-4 x^6 (-1 + \eta)^6 \theta p (-76 + 10 \eta^4 - 11 \eta t - \eta^3 (9 + 10 \eta t) + \\
& 28 \mu_1 + \eta^2 (-88 + 9 \eta t + 28 \mu_1) - \\
& 4 \theta l (-31 + 7 \mu_1 + 2 \mathfrak{z}2) + 4 \eta t \theta l (-31 + 7 \mu_1 + 2 \mathfrak{z}2) + \\
& \eta (163 - 56 \mu_1 + 4 \theta l (-19 + 7 \mu_1 - \mathfrak{z}2) + 4 \eta t (3 + \theta l (19 - 7 \mu_1 + \mathfrak{z}2)))) + \\
& 12 x^5 (-1 + \eta)^5 ((-1 + \eta)^2 \theta p (20 \eta^3 + \eta^2 (52 - 20 \eta t) - \\
& 2 \times (82 + \eta t - 14 \mu_1) + \eta (-119 - 52 \eta t + 56 \mu_1)) - (-1 + \eta t) \theta l \\
& (-8 + \eta^2 \theta p (-121 + 56 \mu_1 - 6 \mathfrak{z}2) + 4 \theta p (55 - 7 \mu_1 + 3 \mathfrak{z}1 + \mathfrak{z}2) + \\
& \eta (8 - \theta p (-45 + 28 \mu_1 + 12 \mathfrak{z}1 + 34 \mathfrak{z}2))) - \\
& x^3 (-1 + \eta)^3 (-4 (-1 + \eta)^2 \theta p (200 \eta^5 + 9 \eta (-64 + \eta t) - 40 \eta^4 \\
& (-28 + 5 \eta t) - 12 \eta^2 (428 + 25 \eta t - 70 \mu_1) - \\
& 10 \eta^3 (17 + 112 \eta t - 56 \mu_1) + 3 \eta t (-53 + 20 \mu_1)) + \\
& (-1 + \eta t) \theta l (2 \eta^3 (324 + \theta p (-7718 + 560 \mu_1 - 693 \mathfrak{z}1 - 1373 \mathfrak{z}2)) + \\
& 40 \eta^4 \theta p (-47 + 56 \mu_1 - 2 \mathfrak{z}2) - 8 \times (16 - 10 \mu_1 + 5 \theta p \mu_1 (2 + \mathfrak{z}1 + \mathfrak{z}2) - \\
& 2 \theta p (8 + 5 \mathfrak{z}1 + 4 \mathfrak{z}2)) + 3 \eta^2 (366 - 240 \mu_1 +
\end{aligned}$$

$$\begin{aligned}
& \left( \text{ep} (7410 - 119 \, \mathfrak{x}1 - 383 \, \mathfrak{x}2 + 160 \, \mu1 (-5 + \mathfrak{x}1 + \mathfrak{x}2)) + \eta (-1618 + \right. \\
& \quad \left. 640 \, \mu1 + \text{ep} (5326 + 1663 \, \mathfrak{x}1 + 1319 \, \mathfrak{x}2 - 440 \, \mu1 (2 + \mathfrak{x}1 + \mathfrak{x}2))) \right) + \\
& 3 \, x^4 (-1 + \eta)^4 \left( -2 (-1 + \eta)^2 \text{ep} (-96 + 100 \, \eta^4 + \eta^3 (410 - 100 \, \eta t) + \right. \\
& \quad \left. 7 \, \eta t - 4 \, \eta (419 + 15 \, \eta t - 70 \, \mu1) - 10 \, \eta^2 (37 + 41 \, \eta t - 28 \, \mu1) \right) + \\
& (-1 + \eta t) \, \text{el} (20 \, \eta^3 \text{ep} (-43 + 28 \, \mu1 - 2 \, \mathfrak{x}2) - \\
& \quad \eta^2 (-148 + \text{ep} (1666 + 237 \, \mathfrak{x}1 + 517 \, \mathfrak{x}2)) + \\
& \quad \eta (60 - 80 \, \mu1 + \text{ep} (4046 + 85 \, \mathfrak{x}1 - 59 \, \mathfrak{x}2 + 40 \, \mu1 (-12 + \mathfrak{x}1 + \mathfrak{x}2))) - \\
& \quad \left. 8 \times (26 - 10 \, \mu1 + \text{ep} (-58 - 19 \, \mathfrak{x}1 - 15 \, \mathfrak{x}2 + 5 \, \mu1 (2 + \mathfrak{x}1 + \mathfrak{x}2))) \right) + \\
& x (-1 + \eta) \, \eta (240 \, \eta^8 \text{ep} - 48 \, \eta^7 (-33 + 5 \, \eta t) \text{ep} - 12 \, \eta^6 \text{ep} \\
& \quad (191 + 132 \, \eta t - 56 \, \mu1) + 2 \, \eta t \text{ep} (-141 + 80 \, \mu1) - \\
& 6 \, \eta^4 (-2 \text{ep} (1725 + 7 \, \eta t - 224 \, \mu1) + (-1 + \eta t) \, \text{el} \\
& \quad (8 + \text{ep} (-1688 + 168 \, \mu1 - 105 \, \mathfrak{x}1 - 197 \, \mathfrak{x}2))) - 12 \, \eta^5 \text{ep} (986 - \\
& \quad 28 \, \mu1 - \text{el} (43 + 56 \, \mu1 + 2 \, \mathfrak{x}2) + \eta t (-234 + \text{el} (43 + 56 \, \mu1 + 2 \, \mathfrak{x}2))) + \\
& 2 \, \eta (200 \, \eta t \text{ep} (-3 + \mu1) + (-1 + \eta t) \, \text{el} (51 - 40 \, \mu1 + \\
& \quad 60 \text{ep} \, \mu1 (2 + \mathfrak{x}1 + \mathfrak{x}2) - 24 \text{ep} (8 + 5 \, \mathfrak{x}1 + 4 \, \mathfrak{x}2))) + \\
& \eta^2 (-2 \text{ep} (1152 + \eta t (-1617 + 640 \, \mu1)) + (-1 + \eta t) \, \text{el} (32 \times (9 - 5 \, \mu1) + \\
& \quad 3 \text{ep} (-1614 - 447 \, \mathfrak{x}1 - 359 \, \mathfrak{x}2 + 120 \, \mu1 (2 + \mathfrak{x}1 + \mathfrak{x}2)))) - \\
& 3 \, \eta^3 (4 \text{ep} (508 + \eta t (235 - 60 \, \mu1) - 140 \, \mu1) + (-1 + \eta t) \, \text{el} (114 - \\
& \quad 80 \, \mu1 + \text{ep} (3062 - 317 \, \mathfrak{x}1 - 437 \, \mathfrak{x}2 + 80 \, \mu1 (-3 + 2 \, \mathfrak{x}1 + 2 \, \mathfrak{x}2)))) - \\
& x^2 (-1 + \eta)^2 (600 \, \eta^8 \text{ep} - 60 \, \eta^7 (-51 + 10 \, \eta t) \text{ep} - 60 \, \eta^6 \text{ep} \\
& \quad (106 + 51 \, \eta t - 28 \, \mu1) + 2 \, \eta t \text{ep} (-71 + 40 \, \mu1) - \\
& 12 \, \eta^5 \text{ep} (1653 + \text{el} (10 - 140 \, \mu1) + 10 \, \eta t (-52 + \text{el} (-1 + 14 \, \mu1))) - \\
& 12 \, \eta^4 (2 \text{ep} (-1669 + 39 \, \eta t + 210 \, \mu1) + (-1 + \eta t) \, \text{el} \\
& \quad (29 + \text{ep} (-1530 + 140 \, \mu1 - 111 \, \mathfrak{x}1 - 211 \, \mathfrak{x}2))) + \\
& 2 \, \eta (\eta t \text{ep} (-803 + 280 \, \mu1) + (-1 + \eta t) \, \text{el} (121 - 80 \, \mu1 + \\
& \quad 60 \text{ep} \, \mu1 (2 + \mathfrak{x}1 + \mathfrak{x}2) - 24 \text{ep} (8 + 5 \, \mathfrak{x}1 + 4 \, \mathfrak{x}2))) + \\
& \eta^2 (-2 \text{ep} (1728 + \eta t (-1801 + 680 \, \mu1)) + (-1 + \eta t) \, \text{el} (1270 - \\
& \quad 560 \, \mu1 + 3 \text{ep} (-2542 - 751 \, \mathfrak{x}1 - 599 \, \mathfrak{x}2 + 200 \, \mu1 (2 + \mathfrak{x}1 + \mathfrak{x}2)))) - \\
& 3 \, \eta^3 (2 \text{ep} (2344 + \eta t (583 - 120 \, \mu1) - 560 \, \mu1) + (-1 + \eta t) \, \text{el} (388 - 240 \\
& \quad \mu1 + \text{ep} (6754 - 387 \, \mathfrak{x}1 - 635 \, \mathfrak{x}2 + 80 \, \mu1 (-8 + 3 \, \mathfrak{x}1 + 3 \, \mathfrak{x}2)))) + \\
& \eta^2 \text{ep} (-40 \, \eta^8 + 4 \, \eta^7 (-81 + 10 \, \eta t) + 4 \, \eta^6 (79 + 81 \, \eta t - 28 \, \mu1) + \\
& 16 \, \eta t (8 - 5 \, \mu1) + \eta^4 (-4244 + 560 \, \mu1 + \\
& \quad \eta t (-142 + \text{el} (-2162 + 224 \, \mu1 - 117 \, \mathfrak{x}1 - 221 \, \mathfrak{x}2)) + \\
& \quad \text{el} (2162 - 224 \, \mu1 + 117 \, \mathfrak{x}1 + 221 \, \mathfrak{x}2)) + 4 \, \eta^5 (671 - 28 \, \mu1 - \\
& \quad \text{el} (47 + 28 \, \mu1 + 2 \, \mathfrak{x}2) + \eta t (-126 + \text{el} (47 + 28 \, \mu1 + 2 \, \mathfrak{x}2))) - \\
& 2 \, \eta (4 \, \text{el} (-5 \, \mu1 (2 + \mathfrak{x}1 + \mathfrak{x}2) + 2 \times (8 + 5 \, \mathfrak{x}1 + 4 \, \mathfrak{x}2)) + \\
& \quad \eta t (-127 + 40 \, \mu1 + 20 \, \text{el} \, \mu1 (2 + \mathfrak{x}1 + \mathfrak{x}2) - 8 \, \text{el} (8 + 5 \, \mathfrak{x}1 + 4 \, \mathfrak{x}2))) + \\
& \eta^2 (576 + \text{el} (-1150 - 295 \, \mathfrak{x}1 - 239 \, \mathfrak{x}2 + 80 \, \mu1 (2 + \mathfrak{x}1 + \mathfrak{x}2)) + \\
& \quad \eta t (-910 + 400 \, \mu1 + \text{el} (1150 + 295 \, \mathfrak{x}1 + 239 \, \mathfrak{x}2 - \\
& \quad 80 \, \mu1 (2 + \mathfrak{x}1 + \mathfrak{x}2)))) + 6 \, \eta^3 (172 - 56 \, \mu1 + \\
& \quad \text{el} (-276 + 43 \, \mathfrak{x}1 + 55 \, \mathfrak{x}2 - 4 \, \mu1 (-4 + 5 \, \mathfrak{x}1 + 5 \, \mathfrak{x}2)) + \eta t (135 - \\
& \quad 40 \, \mu1 + \text{el} (276 - 43 \, \mathfrak{x}1 - 55 \, \mathfrak{x}2 + 4 \, \mu1 (-4 + 5 \, \mathfrak{x}1 + 5 \, \mathfrak{x}2)))) + \\
& 2 \, w^5 (-1 + \eta)^5 (24 \, x^4 (-1 + \eta)^4 (-1 + \eta t) \, \text{el} \text{ep} (-4 + \mathfrak{x}2) + \\
& 2 \, \eta^2 \text{ep} (10 \, \eta^5 - \eta^4 (9 + 10 \, \eta t) + 4 \, \eta t (-8 + 5 \, \mu1) + \\
& \quad \eta^3 (-88 + 9 \, \eta t + 28 \, \mu1) + \eta^2 (163 + 20 \, \eta t (-1 + \mu1) - 56 \, \mu1 + \\
& \quad 2 \, \text{el} \, \mu1 (24 + 5 \, \mathfrak{x}1 + 5 \, \mathfrak{x}2) - 2 \, \eta t \, \text{el} \, \mu1 (24 + 5 \, \mathfrak{x}1 + 5 \, \mathfrak{x}2)) -
\end{aligned}$$

$$\begin{aligned}
& 4 \, \theta l \, (15 + 5 \, \mathfrak{e}1 + 8 \, \mathfrak{e}2) + 4 \, \eta t \, \theta l \, (15 + 5 \, \mathfrak{e}1 + 8 \, \mathfrak{e}2)) + \\
& \eta \, (-76 + 28 \, \mu1 + 2 \, \theta l \, (78 + 10 \, \mathfrak{e}1 + 4 \, \mathfrak{e}2 - \mu1 \, (24 + 5 \, \mathfrak{e}1 + 5 \, \mathfrak{e}2)) + \eta t \\
& \quad (53 - 40 \, \mu1 - 4 \, \theta l \, (39 + 5 \, \mathfrak{e}1 + 2 \, \mathfrak{e}2) + 2 \, \theta l \, \mu1 \, (24 + 5 \, \mathfrak{e}1 + 5 \, \mathfrak{e}2))) + \\
& 2 \, x^3 \, (-1 + \eta)^3 \, (-(-1 + \eta)^2 \, \theta p \, (-76 + 10 \, \eta^2 + \eta \, (11 - 10 \, \eta t) - \\
& \quad 11 \, \eta t + 28 \, \mu1) + 2 \times (-1 + \eta t) \, \theta l \\
& \quad (2 \times (-8 + 5 \, \mu1) + \theta p \, (78 + 10 \, \mathfrak{e}1 + 4 \, \mathfrak{e}2 - \mu1 \, (24 + 5 \, \mathfrak{e}1 + 5 \, \mathfrak{e}2)) + \\
& \quad \eta \, (16 - 10 \, \mu1 + \theta p \, (42 - 10 \, \mathfrak{e}1 - 34 \, \mathfrak{e}2 + \mu1 \, (24 + 5 \, \mathfrak{e}1 + 5 \, \mathfrak{e}2)))) - \\
& x \, (-1 + \eta) \, \eta \, (60 \, \eta^5 \, \theta p - 6 \, \eta^4 \, (9 + 10 \, \eta t) \, \theta p + 6 \, \eta^3 \, \theta p \\
& \quad (-88 + 9 \, \eta t + 28 \, \mu1) + \eta t \, \theta p \, (-141 + 80 \, \mu1) + \\
& \quad \eta \, (-8 \, \theta p \, (57 - 21 \, \mu1 + \eta t \, (-27 + 20 \, \mu1)) + (-1 + \eta t) \, \theta l \, (51 - \\
& \quad 40 \, \mu1 + 12 \, \theta p \, (-2 \times (39 + 5 \, \mathfrak{e}1 + 2 \, \mathfrak{e}2) + \mu1 \, (24 + 5 \, \mathfrak{e}1 + 5 \, \mathfrak{e}2)))) + \\
& \quad \eta^2 \, (\theta p \, (978 - 336 \, \mu1 + \eta t \, (-69 + 80 \, \mu1)) - (-1 + \eta t) \, \theta l \, (51 - \\
& \quad 40 \, \mu1 + 12 \, \theta p \, (\mu1 \, (24 + 5 \, \mathfrak{e}1 + 5 \, \mathfrak{e}2) - 2 \times (11 + 5 \, \mathfrak{e}1 + 9 \, \mathfrak{e}2)))) + \\
& x^2 \, (-1 + \eta)^2 \, (60 \, \eta^5 \, \theta p - 6 \, \eta^4 \, (9 + 10 \, \eta t) \, \theta p + 6 \, \eta^3 \, \theta p \, (-88 + \\
& \quad 9 \, \eta t + 28 \, \mu1) + \eta t \, \theta p \, (-71 + 40 \, \mu1) + \\
& \quad \eta \, (4 \, \theta p \, (-114 + 19 \, \eta t + 42 \, \mu1 - 20 \, \eta t \, \mu1) + (-1 + \eta t) \, \theta l \, (121 - \\
& \quad 80 \, \mu1 + 12 \, \theta p \, (-2 \times (39 + 5 \, \mathfrak{e}1 + 2 \, \mathfrak{e}2) + \mu1 \, (24 + 5 \, \mathfrak{e}1 + 5 \, \mathfrak{e}2)))) + \\
& \quad \eta^2 \, (\theta p \, (978 + \eta t - 336 \, \mu1 + 40 \, \eta t \, \mu1) - (-1 + \eta t) \, \theta l \, (121 - \\
& \quad 80 \, \mu1 + 12 \, \theta p \, (\mu1 \, (24 + 5 \, \mathfrak{e}1 + 5 \, \mathfrak{e}2) - 2 \times (3 + 5 \, \mathfrak{e}1 + 11 \, \mathfrak{e}2)))) - \\
& w^3 \, (-1 + \eta)^3 \, (4 \, x^5 \, (-1 + \eta)^5 \, (3 \, (-1 + \eta)^2 \, \theta p \, (-76 + 10 \, \eta^2 + \eta \, (11 - 10 \, \eta t) - \\
& \quad 11 \, \eta t + 28 \, \mu1) - 4 \times (-1 + \eta t) \, \theta l \, (-2 + \eta \, (2 + \\
& \quad \theta p \, (-35 + 21 \, \mu1 - 3 \, \mathfrak{e}1 - 10 \, \mathfrak{e}2)) + \theta p \, (95 - 21 \, \mu1 + 3 \, \mathfrak{e}1 - 5 \, \mathfrak{e}2))) - \\
& 16 \, x^6 \, (-1 + \eta)^6 \, (-1 + \eta t) \, \theta l \, \theta p \, (-4 + \mathfrak{e}2) + \eta^2 \, \theta p \, (-120 \, \eta^7 + \\
& \quad 12 \, \eta^6 \, (-21 + 10 \, \eta t) + 48 \, \eta t \, (8 - 5 \, \mu1) + 84 \, \eta^5 \, (15 + 3 \, \eta t - 4 \, \mu1) + \\
& \quad \eta^4 \, (84 \times (9 + 4 \, \mu1) + \eta t \, (-730 + \theta l \, (-466 + 336 \, \mu1 - 39 \, \mathfrak{e}1 - 55 \, \mathfrak{e}2)) + \\
& \quad \theta l \, (466 - 336 \, \mu1 + 39 \, \mathfrak{e}1 + 55 \, \mathfrak{e}2)) - \\
& \quad 2 \, \eta \, (-96 - 60 \, \theta l \, \mu1 \, (2 + \mathfrak{e}1 + \mathfrak{e}2) + 8 \, \theta l \, (40 + 15 \, \mathfrak{e}1 + 13 \, \mathfrak{e}2) + \eta t \\
& \quad (147 - 120 \, \mu1 + 60 \, \theta l \, \mu1 \, (2 + \mathfrak{e}1 + \mathfrak{e}2) - 8 \, \theta l \, (40 + 15 \, \mathfrak{e}1 + 13 \, \mathfrak{e}2))) + \\
& \quad \eta^2 \, (1656 - 336 \, \mu1 + \theta l \, (-2514 + 336 \, \mu1 - 135 \, \mathfrak{e}1 - 23 \, \mathfrak{e}2) + \\
& \quad \eta t \, (-430 + 240 \, \mu1 + \theta l \, (2514 - 336 \, \mu1 + 135 \, \mathfrak{e}1 + 23 \, \mathfrak{e}2))) + \\
& \quad 2 \, \eta^3 \, (-1746 + 168 \, \mu1 - 60 \, \theta l \, \mu1 \, (2 + \mathfrak{e}1 + \mathfrak{e}2) + 8 \, \theta l \\
& \quad (88 + 21 \, \mathfrak{e}1 + 31 \, \mathfrak{e}2) + \eta t \, (349 - 120 \, \mu1 + \\
& \quad 60 \, \theta l \, \mu1 \, (2 + \mathfrak{e}1 + \mathfrak{e}2) - 8 \, \theta l \, (88 + 21 \, \mathfrak{e}1 + 31 \, \mathfrak{e}2))) + \\
& x^4 \, (-1 + \eta)^4 \, (-2 \, (-1 + \eta)^2 \, \theta p \, (-984 + 300 \, \eta^3 + \eta^2 \, (510 - 300 \, \eta t) - \\
& \quad 23 \, \eta t - 6 \, \eta \, (347 + 85 \, \eta t - 140 \, \mu1) + 168 \, \mu1) + (-1 + \eta t) \, \theta l \\
& \quad (\eta^2 \, (148 + \theta p \, (-3398 + 1680 \, \mu1 - 237 \, \mathfrak{e}1 - 541 \, \mathfrak{e}2)) + \eta \, (476 - 240 \, \mu1 + \\
& \quad \theta p \, (4646 - 219 \, \mathfrak{e}1 - 875 \, \mathfrak{e}2 + 24 \, \mu1 \, (-46 + 5 \, \mathfrak{e}1 + 5 \, \mathfrak{e}2))) - 24 \times \\
& \quad (26 - 10 \, \mu1 + \theta p \, (-132 - 19 \, \mathfrak{e}1 - 13 \, \mathfrak{e}2 + \mu1 \, (24 + 5 \, \mathfrak{e}1 + 5 \, \mathfrak{e}2)))) + \\
& x \, (-1 + \eta) \, \eta \, (600 \, \eta^7 \, \theta p - 300 \, \eta^6 \, (-3 + 2 \, \eta t) \, \theta p - 12 \, \eta^5 \, \theta p \\
& \quad (518 + 75 \, \eta t - 140 \, \mu1) + 6 \, \eta t \, \theta p \, (-141 + 80 \, \mu1) - \\
& \quad 2 \, \eta^4 \, (2 \, \theta p \, (-779 \, \eta t + 63 \times (3 + 8 \, \mu1)) + (-1 + \eta t) \, \theta l \\
& \quad (8 + \theta p \, (-1366 + 840 \, \mu1 - 105 \, \mathfrak{e}1 - 161 \, \mathfrak{e}2))) + \\
& \quad 6 \, \eta \, (-2 \, \theta p \, (48 + \eta t \, (-3 + 20 \, \mu1)) + (-1 + \eta t) \, \theta l \, (51 - 40 \, \mu1 + \\
& \quad 60 \, \theta p \, \mu1 \, (2 + \mathfrak{e}1 + \mathfrak{e}2) - 8 \, \theta p \, (40 + 15 \, \mathfrak{e}1 + 13 \, \mathfrak{e}2))) + \\
& \quad \eta^2 \, (2 \, \theta p \, (-3468 + \eta t \, (991 - 480 \, \mu1) + 672 \, \mu1) + 3 \times (-1 + \eta t)
\end{aligned}$$

$$\begin{aligned}
& \theta l (28 + \theta p (-3570 - 287 \mu 1 - 127 \mu 2 + 8 \mu 1 (66 + 5 \mu 1 + 5 \mu 2))) + \\
& \eta^3 (4 \theta p (3246 - 252 \mu 1 + \eta t (-697 + 180 \mu 1)) - (-1 + \eta t) \\
& \theta l (374 - 240 \mu 1 + \theta p (-4138 - 1371 \mu 1 - 2123 \mu 2 + \\
& 48 \mu 1 (13 + 10 \mu 1 + 10 \mu 2))) - x^2 (-1 + \eta)^2 (1200 \eta^7 \theta p - \\
& 120 \eta^6 (-9 + 10 \eta t) \theta p - 24 \eta^5 \theta p (506 + 45 \eta t - 140 \mu 1) + \\
& 6 \eta t \theta p (-71 + 40 \mu 1) - 4 \eta^4 (-3 \theta p (352 + 429 \eta t - 392 \mu 1) + \\
& (-1 + \eta t) \theta l (29 + \theta p (-1538 + 840 \mu 1 - 111 \mu 1 - 187 \mu 2))) + \\
& 6 \eta (\theta p (-96 + 5 \eta t (-31 + 8 \mu 1)) + (-1 + \eta t) \theta l (121 - 80 \mu 1 + \\
& 60 \theta p \mu 1 (2 + \mu 1 + \mu 2) - 8 \theta p (40 + 15 \mu 1 + 13 \mu 2))) + \\
& 3 \eta^2 (2 \theta p (-1812 + \eta t (421 - 200 \mu 1) + 336 \mu 1) + (-1 + \eta t) \theta l (262 - \\
& 80 \mu 1 + \theta p (-5682 - 591 \mu 1 - 335 \mu 2 + 24 \mu 1 (38 + 5 \mu 1 + 5 \mu 2)))) + \\
& \eta^3 (6 \theta p (2848 - 112 \mu 1 + \eta t (-673 + 120 \mu 1)) - (-1 + \eta t) \\
& \theta l (1396 - 720 \mu 1 + \theta p (-2446 - 2049 \mu 1 - \\
& 3473 \mu 2 + 48 \mu 1 (2 + 15 \mu 1 + 15 \mu 2)))) + \\
& x^3 (-1 + \eta)^3 (4 (-1 + \eta)^2 \theta p (-48 + 300 \eta^4 + \eta^3 (690 - 300 \eta t) - \\
& 6 \eta^2 (309 + 115 \eta t - 140 \mu 1) + 30 \eta t (-5 + 2 \mu 1) + \\
& \eta (-1986 - 77 \eta t + 336 \mu 1)) - (-1 + \eta t) \theta l \\
& (\eta^3 (216 + \theta p (-6660 + 3360 \mu 1 - 462 \mu 1 - 878 \mu 2)) - \\
& 8 \times (48 - 30 \mu 1 + 15 \theta p \mu 1 (2 + \mu 1 + \mu 2) - 2 \theta p (40 + 15 \mu 1 + 13 \mu 2)) + \\
& \eta^2 (90 \times (17 - 8 \mu 1) + \theta p (3410 - 1281 \mu 1 - 2641 \mu 2 + \\
& 96 \mu 1 (-11 + 5 \mu 1 + 5 \mu 2))) + \eta (6 \times (-227 + 80 \mu 1) + \theta p \\
& (12018 + 1503 \mu 1 + 959 \mu 2 - 24 \mu 1 (86 + 15 \mu 1 + 15 \mu 2)))) - \\
& w^4 (-1 + \eta)^4 (-48 x^5 (-1 + \eta)^5 (-1 + \eta t) \theta l \theta p (-4 + \mu 2) + 4 x^4 (-1 + \eta)^4 \\
& (3 (-1 + \eta)^2 \theta p (-76 + 10 \eta^2 + \eta (11 - 10 \eta t) - 11 \eta t + 28 \mu 1) - 2 \times (-1 + \eta t) \\
& \theta l (-26 + 10 \mu 1 + \theta p (212 + 19 \mu 1 + \mu 2 - \mu 1 (52 + 5 \mu 1 + 5 \mu 2)) + \\
& \eta (26 - 10 \mu 1 + \theta p (-20 - 19 \mu 1 - 49 \mu 2 + \mu 1 (52 + 5 \mu 1 + 5 \mu 2)))) + \\
& 3 x^2 (-1 + \eta)^2 (240 \eta^6 \theta p - 48 \eta^5 (2 + 5 \eta t) \theta p + 2 \eta t \theta p \\
& (-71 + 40 \mu 1) + 12 \eta^4 \theta p (-185 + 8 \eta t + 56 \mu 1) + \\
& 2 \eta (\theta p (-328 + 33 \eta t + 56 \mu 1 - 40 \eta t \mu 1) + (-1 + \eta t) \theta l (121 - \\
& 80 \mu 1 - 8 \theta p (77 + 15 \mu 1 + 12 \mu 2) + 4 \theta p \mu 1 (44 + 15 \mu 1 + 15 \mu 2))) - \\
& \eta^2 (2 \theta p (190 - 224 \mu 1 + 5 \eta t (9 + 8 \mu 1)) + (-1 + \eta t) \theta l \\
& (74 - 80 \mu 1 + \theta p (2190 + 37 \mu 1 - 251 \mu 2 + 40 \mu 1 (-12 + \mu 1 + \mu 2)))) + \\
& \eta^3 (2 \theta p (1556 - 616 \mu 1 + 5 \eta t (31 + 8 \mu 1)) - (-1 + \eta t) \theta l (168 - 80 \\
& \mu 1 + \theta p (-1438 - 277 \mu 1 - 437 \mu 2 + 16 \mu 1 (52 + 5 \mu 1 + 5 \mu 2)))) + \\
& x^3 (-1 + \eta)^3 (-4 (-1 + \eta)^2 \theta p (-164 + 120 \eta^3 - 55 \eta t - 6 \eta^2 \\
& (-27 + 20 \eta t) - 3 \eta (293 + 54 \eta t - 112 \mu 1) + 28 \mu 1 + 20 \eta t \mu 1) + \\
& (-1 + \eta t) \theta l (-8 \times (48 - 30 \mu 1 - 2 \theta p (77 + 15 \mu 1 + 12 \mu 2) + \\
& \theta p \mu 1 (44 + 15 \mu 1 + 15 \mu 2)) + \eta^2 (582 - 240 \mu 1 + \\
& \theta p (-2398 - 581 \mu 1 - 1061 \mu 2 + 32 \mu 1 (52 + 5 \mu 1 + 5 \mu 2))) - \\
& \eta (198 + \theta p (-5582 - 341 \mu 1 + 235 \mu 2 + 8 \mu 1 (164 + 5 \mu 1 + 5 \mu 2)))) + \\
& \eta^2 \theta p (120 \eta^6 + \eta^5 (12 - 120 \eta t) - 12 \eta^4 (97 + \eta t - 28 \mu 1) + \\
& 48 \eta t (-8 + 5 \mu 1) + \eta^2 (28 \times (19 + 4 \mu 1) + \theta l (494 - 115 \mu 1 - \\
& 259 \mu 2 + 16 \mu 1 (-4 + 5 \mu 1 + 5 \mu 2)) + \eta t (40 \times (-7 + 2 \mu 1) + \\
& \theta l (-494 + 115 \mu 1 + 259 \mu 2 - 16 \mu 1 (-4 + 5 \mu 1 + 5 \mu 2)))) + \\
& \eta^3 (1156 - 560 \mu 1 + \theta l (-766 - 125 \mu 1 - 173 \mu 2 + 8 \mu 1
\end{aligned}$$

$$\begin{aligned}
& (52 + 5 \mu_1 + 5 \mu_2)) + \eta t (206 + 80 \mu_1 + \\
& \theta l (766 + 125 \mu_1 + 173 \mu_2 - 8 \mu_1 (52 + 5 \mu_1 + 5 \mu_2))) + \\
& 2 \eta (\eta t (295 - 200 \mu_1 - 8 \theta l (77 + 15 \mu_1 + 12 \mu_2) + 4 \theta l \mu_1 \\
& (44 + 15 \mu_1 + 15 \mu_2)) + 4 \times (-82 + 14 \mu_1 + \\
& \theta l (154 + 30 \mu_1 + 24 \mu_2 - \mu_1 (44 + 15 \mu_1 + 15 \mu_2)))) - \\
& \times (-1 + \eta) \eta (480 \eta^6 \theta p - 24 \eta^5 (3 + 20 \eta t) \theta p + 6 \eta t \theta p \\
& (-141 + 80 \mu_1) + 12 \eta^4 \theta p (-379 + 6 \eta t + 112 \mu_1) + \\
& 6 \eta (4 \theta p (-82 + \eta t (45 - 30 \mu_1) + 14 \mu_1) + (-1 + \eta t) \theta l (51 - 40 \mu_1 - \\
& 8 \theta p (77 + 15 \mu_1 + 12 \mu_2) + 4 \theta p \mu_1 (44 + 15 \mu_1 + 15 \mu_2))) + \\
& \eta^3 (12 \theta p (452 - 196 \mu_1 + \eta t (57 + 20 \mu_1)) - (-1 + \eta t) \theta l (130 - \\
& 80 \mu_1 + \theta p (-3034 - 527 \mu_1 - 767 \mu_2 + 32 \mu_1 (52 + 5 \mu_1 + 5 \mu_2)))) + \\
& \eta^2 (6 \theta p (114 - 85 \eta t + 112 \mu_1) - (-1 + \eta t) \theta l (176 - 160 \mu_1 + \\
& \theta p (3178 - 193 \mu_1 - 769 \mu_2 + 8 \mu_1 (-76 + 25 \mu_1 + 25 \mu_2)))))) / \\
& (192 (-1 + w (-1 + \eta))^3 (x (-1 + \eta) - \eta)^3 (w + x + \eta - w \eta - x \eta)^3 \\
& (-1 + \\
& \eta t) \theta p)) \\
\beta f = & \frac{1}{96} f \left( -24 c v^2 + 96 \epsilon + \frac{112 f w}{(-1 + w (-1 + \eta))^3} + \right. \\
& \frac{40 c \sigma^2}{(-1 + w (-1 + \eta)) (x (-1 + \eta) - \eta) (w (-1 + \eta) + x (-1 + \eta) - \eta)} + \\
& \frac{40 c \sigma^2 w}{(-1 + w (-1 + \eta)) (x (-1 + \eta) - \eta) (w (-1 + \eta) + x (-1 + \eta) - \eta)} + \frac{36 f \eta}{(-1 + w (-1 + \eta))^3} + \\
& \frac{672 f w \eta^2}{(-1 + w (-1 + \eta))^3} + \frac{40 c \sigma^2 \eta^2}{(-1 + w (-1 + \eta)) (x (-1 + \eta) - \eta) (w (-1 + \eta) + x (-1 + \eta) - \eta)} + \\
& \frac{120 c \sigma^2 w \eta^2}{(-1 + w (-1 + \eta)) (x (-1 + \eta) - \eta) (w (-1 + \eta) + x (-1 + \eta) - \eta)} + \frac{108 f \eta^3}{(-1 + w (-1 + \eta))^3} + \\
& \frac{112 f w \eta^4}{(-1 + w (-1 + \eta))^3} + \frac{448 f w \eta}{(1 + w - w \eta)^3} + \frac{108 f \eta^2}{(1 + w - w \eta)^3} + \frac{448 f w \eta^3}{(1 + w - w \eta)^3} + \frac{36 f \eta^4}{(1 + w - w \eta)^3} + \\
& \frac{40 f}{(1 + w - w \eta)^2} - \frac{120 f \eta}{(1 + w - w \eta)^2} - \frac{40 f w \eta}{(1 + w - w \eta)^2} + \frac{120 f \eta^2}{(1 + w - w \eta)^2} + \frac{120 f w \eta^2}{(1 + w - w \eta)^2} - \\
& \frac{40 f \eta^3}{(1 + w - w \eta)^2} - \frac{120 f w \eta^3}{(1 + w - w \eta)^2} + \frac{40 f w \eta^4}{(1 + w - w \eta)^2} - \frac{4 f}{1 + w - w \eta} + \frac{4 f \eta}{1 + w - w \eta} - \\
& \frac{32 f \eta^2}{1 + w - w \eta} + \frac{68 f \eta^3}{1 + w - w \eta} - \frac{36 f \eta^4}{1 + w - w \eta} - \frac{4 f x}{(w (-1 + \eta) + x (-1 + \eta) - \eta) (x + \eta - x \eta)^2} + \\
& \frac{12 f x \eta}{(w (-1 + \eta) + x (-1 + \eta) - \eta) (x + \eta - x \eta)^2} - \frac{12 f x \eta^2}{(w (-1 + \eta) + x (-1 + \eta) - \eta) (x + \eta - x \eta)^2} + \\
& \frac{4 f x \eta^3}{(w (-1 + \eta) + x (-1 + \eta) - \eta) (x + \eta - x \eta)^2} + \frac{6 f w^2}{(x (-1 + \eta) - \eta) (w + x + \eta - w \eta - x \eta)^3} + \\
& \frac{6 f x^2}{(x (-1 + \eta) - \eta) (w + x + \eta - w \eta - x \eta)^3} + \frac{18 f w \eta}{(x (-1 + \eta) - \eta) (w + x + \eta - w \eta - x \eta)^3} -
\end{aligned}$$

$$\begin{aligned}
& \frac{24 f w^2 \eta}{(x(-1+\eta)-\eta)(w+x+\eta-w\eta-x\eta)^3} - \frac{24 f x^2 \eta}{(x(-1+\eta)-\eta)(w+x+\eta-w\eta-x\eta)^3} - \\
& \frac{54 f w \eta^2}{(x(-1+\eta)-\eta)(w+x+\eta-w\eta-x\eta)^3} + \frac{36 f w^2 \eta^2}{(x(-1+\eta)-\eta)(w+x+\eta-w\eta-x\eta)^3} + \\
& \frac{36 f x^2 \eta^2}{(x(-1+\eta)-\eta)(w+x+\eta-w\eta-x\eta)^3} + \frac{54 f w \eta^3}{(x(-1+\eta)-\eta)(w+x+\eta-w\eta-x\eta)^3} - \\
& \frac{24 f w^2 \eta^3}{(x(-1+\eta)-\eta)(w+x+\eta-w\eta-x\eta)^3} - \frac{24 f x^2 \eta^3}{(x(-1+\eta)-\eta)(w+x+\eta-w\eta-x\eta)^3} - \\
& \frac{18 f w \eta^4}{(x(-1+\eta)-\eta)(w+x+\eta-w\eta-x\eta)^3} + \frac{6 f w^2 \eta^4}{(x(-1+\eta)-\eta)(w+x+\eta-w\eta-x\eta)^3} + \\
& \frac{6 f x^2 \eta^4}{(x(-1+\eta)-\eta)(w+x+\eta-w\eta-x\eta)^3} + \frac{72 f x}{(x+\eta-x\eta)^3(w+x+\eta-w\eta-x\eta)^3} - \\
& \frac{36 f w x}{(x+\eta-x\eta)^3(w+x+\eta-w\eta-x\eta)^3} - \frac{72 f x^2}{(x+\eta-x\eta)^3(w+x+\eta-w\eta-x\eta)^3} - \\
& \frac{12 f w^2 x^2}{(x+\eta-x\eta)^3(w+x+\eta-w\eta-x\eta)^3} - \frac{72 f w x^3}{(x+\eta-x\eta)^3(w+x+\eta-w\eta-x\eta)^3} + \\
& \frac{72 f x}{(-1+w(-1+\eta))^3(x+\eta-x\eta)^3(w+x+\eta-w\eta-x\eta)^3} + \\
& \frac{180 f w x}{(-1+w(-1+\eta))^3(x+\eta-x\eta)^3(w+x+\eta-w\eta-x\eta)^3} + \\
& \frac{108 f w^2 x}{(-1+w(-1+\eta))^3(x+\eta-x\eta)^3(w+x+\eta-w\eta-x\eta)^3} - \\
& \frac{36 f w^3 x}{(-1+w(-1+\eta))^3(x+\eta-x\eta)^3(w+x+\eta-w\eta-x\eta)^3} - \\
& \frac{36 f w^4 x}{(-1+w(-1+\eta))^3(x+\eta-x\eta)^3(w+x+\eta-w\eta-x\eta)^3} - \\
& \frac{72 f x^2}{(-1+w(-1+\eta))^3(x+\eta-x\eta)^3(w+x+\eta-w\eta-x\eta)^3} - \\
& \frac{216 f w x^2}{(-1+w(-1+\eta))^3(x+\eta-x\eta)^3(w+x+\eta-w\eta-x\eta)^3} - \\
& \frac{216 f w^2 x^2}{(-1+w(-1+\eta))^3(x+\eta-x\eta)^3(w+x+\eta-w\eta-x\eta)^3} - \\
& \frac{72 f w^3 x^2}{(-1+w(-1+\eta))^3(x+\eta-x\eta)^3(w+x+\eta-w\eta-x\eta)^3} - \\
& \frac{72 f w^4 x^3}{(-1+w(-1+\eta))^3(x+\eta-x\eta)^3(w+x+\eta-w\eta-x\eta)^3} + \\
& \frac{40 f w^5 x^3}{(-1+w(-1+\eta))^3(x+\eta-x\eta)^3(w+x+\eta-w\eta-x\eta)^3} -
\end{aligned}$$



$$\begin{aligned}
& \frac{216 f w^3 x^4}{(-1+w(-1+\eta))^3 (x+\eta-x\eta)^3 (w+x+\eta-w\eta-x\eta)^3} + \\
& \frac{120 f w^4 x^4}{(-1+w(-1+\eta))^3 (x+\eta-x\eta)^3 (w+x+\eta-w\eta-x\eta)^3} - \\
& \frac{216 f w^2 x^5}{(-1+w(-1+\eta))^3 (x+\eta-x\eta)^3 (w+x+\eta-w\eta-x\eta)^3} + \\
& \frac{120 f w^3 x^5}{(-1+w(-1+\eta))^3 (x+\eta-x\eta)^3 (w+x+\eta-w\eta-x\eta)^3} - \\
& \frac{72 f w x^6}{(-1+w(-1+\eta))^3 (x+\eta-x\eta)^3 (w+x+\eta-w\eta-x\eta)^3} + \\
& \frac{40 f w^2 x^6}{(-1+w(-1+\eta))^3 (x+\eta-x\eta)^3 (w+x+\eta-w\eta-x\eta)^3} - \\
& \frac{324 f x \eta}{(x+\eta-x\eta)^3 (w+x+\eta-w\eta-x\eta)^3} + \\
& \frac{144 f w x \eta}{(x+\eta-x\eta)^3 (w+x+\eta-w\eta-x\eta)^3} - \frac{12 f w^2 x \eta}{(x+\eta-x\eta)^3 (w+x+\eta-w\eta-x\eta)^3} + \\
& \frac{288 f x^2 \eta}{(x+\eta-x\eta)^3 (w+x+\eta-w\eta-x\eta)^3} - \frac{144 f w x^2 \eta}{(x+\eta-x\eta)^3 (w+x+\eta-w\eta-x\eta)^3} + \\
& \frac{72 f w^2 x^2 \eta}{(x+\eta-x\eta)^3 (w+x+\eta-w\eta-x\eta)^3} + \frac{432 f w x^3 \eta}{(x+\eta-x\eta)^3 (w+x+\eta-w\eta-x\eta)^3} - \\
& \frac{324 f x \eta}{(-1+w(-1+\eta))^3 (x+\eta-x\eta)^3 (w+x+\eta-w\eta-x\eta)^3} - \\
& \frac{1044 f w x \eta}{(-1+w(-1+\eta))^3 (x+\eta-x\eta)^3 (w+x+\eta-w\eta-x\eta)^3} - \\
& \frac{846 f w^2 x \eta}{(-1+w(-1+\eta))^3 (x+\eta-x\eta)^3 (w+x+\eta-w\eta-x\eta)^3} + \\
& \frac{162 f w^3 x \eta}{(-1+w(-1+\eta))^3 (x+\eta-x\eta)^3 (w+x+\eta-w\eta-x\eta)^3} + \\
& \frac{306 f w^4 x \eta}{(-1+w(-1+\eta))^3 (x+\eta-x\eta)^3 (w+x+\eta-w\eta-x\eta)^3} + \\
& \frac{18 f w^5 x \eta}{(-1+w(-1+\eta))^3 (x+\eta-x\eta)^3 (w+x+\eta-w\eta-x\eta)^3} + \\
& \frac{288 f x^2 \eta}{(-1+w(-1+\eta))^3 (x+\eta-x\eta)^3 (w+x+\eta-w\eta-x\eta)^3} + \\
& \frac{1116 f w x^2 \eta}{(-1+w(-1+\eta))^3 (x+\eta-x\eta)^3 (w+x+\eta-w\eta-x\eta)^3} + \\
& \frac{1404 f w^2 x^2 \eta}{(-1+w(-1+\eta))^3 (x+\eta-x\eta)^3 (w+x+\eta-w\eta-x\eta)^3} +
\end{aligned}$$

$$\begin{aligned}
& \frac{612 f w^3 x^2 \eta}{(-1+w(-1+\eta))^3 (x+\eta-x\eta)^3 (w+x+\eta-w\eta-x\eta)^3} - \\
& \frac{180 f w^4 x^2 \eta}{(-1+w(-1+\eta))^3 (x+\eta-x\eta)^3 (w+x+\eta-w\eta-x\eta)^3} + \\
& \frac{120 f w^5 x^2 \eta}{(-1+w(-1+\eta))^3 (x+\eta-x\eta)^3 (w+x+\eta-w\eta-x\eta)^3} + \\
& \frac{36 f x^3 \eta}{(-1+w(-1+\eta))^3 (x+\eta-x\eta)^3 (w+x+\eta-w\eta-x\eta)^3} + \\
& \frac{108 f w x^3 \eta}{(-1+w(-1+\eta))^3 (x+\eta-x\eta)^3 (w+x+\eta-w\eta-x\eta)^3} + \\
& \frac{108 f w^2 x^3 \eta}{(-1+w(-1+\eta))^3 (x+\eta-x\eta)^3 (w+x+\eta-w\eta-x\eta)^3} - \\
& \frac{828 f w^3 x^3 \eta}{(-1+w(-1+\eta))^3 (x+\eta-x\eta)^3 (w+x+\eta-w\eta-x\eta)^3} + \\
& \frac{1272 f w^4 x^3 \eta}{(-1+w(-1+\eta))^3 (x+\eta-x\eta)^3 (w+x+\eta-w\eta-x\eta)^3} - \\
& \frac{404 f w^5 x^3 \eta}{(-1+w(-1+\eta))^3 (x+\eta-x\eta)^3 (w+x+\eta-w\eta-x\eta)^3} - \\
& \frac{1080 f w^2 x^4 \eta}{(-1+w(-1+\eta))^3 (x+\eta-x\eta)^3 (w+x+\eta-w\eta-x\eta)^3} + \\
& \frac{2976 f w^3 x^4 \eta}{(-1+w(-1+\eta))^3 (x+\eta-x\eta)^3 (w+x+\eta-w\eta-x\eta)^3} - \\
& \frac{1212 f w^4 x^4 \eta}{(-1+w(-1+\eta))^3 (x+\eta-x\eta)^3 (w+x+\eta-w\eta-x\eta)^3} - \\
& \frac{432 f w x^5 \eta}{(-1+w(-1+\eta))^3 (x+\eta-x\eta)^3 (w+x+\eta-w\eta-x\eta)^3} + \\
& \frac{2616 f w^2 x^5 \eta}{(-1+w(-1+\eta))^3 (x+\eta-x\eta)^3 (w+x+\eta-w\eta-x\eta)^3} - \\
& \frac{1212 f w^3 x^5 \eta}{(-1+w(-1+\eta))^3 (x+\eta-x\eta)^3 (w+x+\eta-w\eta-x\eta)^3} + \\
& \frac{792 f w x^6 \eta}{(-1+w(-1+\eta))^3 (x+\eta-x\eta)^3 (w+x+\eta-w\eta-x\eta)^3} - \\
& \frac{404 f w^2 x^6 \eta}{(-1+w(-1+\eta))^3 (x+\eta-x\eta)^3 (w+x+\eta-w\eta-x\eta)^3} + \\
& \frac{540 f x \eta^2}{(x+\eta-x\eta)^3 (w+x+\eta-w\eta-x\eta)^3} - \\
& \frac{288 f w x \eta^2}{(x+\eta-x\eta)^3 (w+x+\eta-w\eta-x\eta)^3} + \frac{60 f w^2 x \eta^2}{(x+\eta-x\eta)^3 (w+x+\eta-w\eta-x\eta)^3} -
\end{aligned}$$

$$\begin{aligned}
& \frac{432 f x^2 \eta^2}{(x + \eta - x \eta)^3 (w + x + \eta - w \eta - x \eta)^3} + \frac{720 f w x^2 \eta^2}{(x + \eta - x \eta)^3 (w + x + \eta - w \eta - x \eta)^3} - \\
& \frac{180 f w^2 x^2 \eta^2}{(x + \eta - x \eta)^3 (w + x + \eta - w \eta - x \eta)^3} - \frac{1080 f w x^3 \eta^2}{(x + \eta - x \eta)^3 (w + x + \eta - w \eta - x \eta)^3} + \\
& \frac{540 f x \eta^2}{(-1 + w (-1 + \eta))^3 (x + \eta - x \eta)^3 (w + x + \eta - w \eta - x \eta)^3} + \\
& \frac{2412 f w x \eta^2}{(-1 + w (-1 + \eta))^3 (x + \eta - x \eta)^3 (w + x + \eta - w \eta - x \eta)^3} + \\
& \frac{2718 f w^2 x \eta^2}{(-1 + w (-1 + \eta))^3 (x + \eta - x \eta)^3 (w + x + \eta - w \eta - x \eta)^3} - \\
& \frac{108 f w^3 x \eta^2}{(-1 + w (-1 + \eta))^3 (x + \eta - x \eta)^3 (w + x + \eta - w \eta - x \eta)^3} - \\
& \frac{1314 f w^4 x \eta^2}{(-1 + w (-1 + \eta))^3 (x + \eta - x \eta)^3 (w + x + \eta - w \eta - x \eta)^3} - \\
& \frac{24 f w^5 x \eta^2}{(-1 + w (-1 + \eta))^3 (x + \eta - x \eta)^3 (w + x + \eta - w \eta - x \eta)^3} - \\
& \frac{360 f x^2 \eta^2}{(-1 + w (-1 + \eta))^3 (x + \eta - x \eta)^3 (w + x + \eta - w \eta - x \eta)^3} - \\
& \frac{2124 f w x^2 \eta^2}{(-1 + w (-1 + \eta))^3 (x + \eta - x \eta)^3 (w + x + \eta - w \eta - x \eta)^3} - \\
& \frac{3672 f w^2 x^2 \eta^2}{(-1 + w (-1 + \eta))^3 (x + \eta - x \eta)^3 (w + x + \eta - w \eta - x \eta)^3} - \\
& \frac{3492 f w^3 x^2 \eta^2}{(-1 + w (-1 + \eta))^3 (x + \eta - x \eta)^3 (w + x + \eta - w \eta - x \eta)^3} + \\
& \frac{2592 f w^4 x^2 \eta^2}{(-1 + w (-1 + \eta))^3 (x + \eta - x \eta)^3 (w + x + \eta - w \eta - x \eta)^3} - \\
& \frac{1092 f w^5 x^2 \eta^2}{(-1 + w (-1 + \eta))^3 (x + \eta - x \eta)^3 (w + x + \eta - w \eta - x \eta)^3} - \\
& \frac{180 f x^3 \eta^2}{(-1 + w (-1 + \eta))^3 (x + \eta - x \eta)^3 (w + x + \eta - w \eta - x \eta)^3} - \\
& \frac{648 f w x^3 \eta^2}{(-1 + w (-1 + \eta))^3 (x + \eta - x \eta)^3 (w + x + \eta - w \eta - x \eta)^3} - \\
& \frac{2916 f w^2 x^3 \eta^2}{(-1 + w (-1 + \eta))^3 (x + \eta - x \eta)^3 (w + x + \eta - w \eta - x \eta)^3} + \\
& \frac{9552 f w^3 x^3 \eta^2}{(-1 + w (-1 + \eta))^3 (x + \eta - x \eta)^3 (w + x + \eta - w \eta - x \eta)^3} - \\
& \frac{8328 f w^4 x^3 \eta^2}{(-1 + w (-1 + \eta))^3 (x + \eta - x \eta)^3 (w + x + \eta - w \eta - x \eta)^3} +
\end{aligned}$$

$$\begin{aligned}
& \frac{1804 f w^5 x^3 \eta^2}{(-1+w(-1+\eta))^3 (x+\eta-x\eta)^3 (w+x+\eta-w\eta-x\eta)^3} - \\
& \frac{1080 f w x^4 \eta^2}{(-1+w(-1+\eta))^3 (x+\eta-x\eta)^3 (w+x+\eta-w\eta-x\eta)^3} + \\
& \frac{11400 f w^2 x^4 \eta^2}{(-1+w(-1+\eta))^3 (x+\eta-x\eta)^3 (w+x+\eta-w\eta-x\eta)^3} - \\
& \frac{17340 f w^3 x^4 \eta^2}{(-1+w(-1+\eta))^3 (x+\eta-x\eta)^3 (w+x+\eta-w\eta-x\eta)^3} + \\
& \frac{5412 f w^4 x^4 \eta^2}{(-1+w(-1+\eta))^3 (x+\eta-x\eta)^3 (w+x+\eta-w\eta-x\eta)^3} + \\
& \frac{4320 f w x^5 \eta^2}{(-1+w(-1+\eta))^3 (x+\eta-x\eta)^3 (w+x+\eta-w\eta-x\eta)^3} - \\
& \frac{14064 f w^2 x^5 \eta^2}{(-1+w(-1+\eta))^3 (x+\eta-x\eta)^3 (w+x+\eta-w\eta-x\eta)^3} + \\
& \frac{5412 f w^3 x^5 \eta^2}{(-1+w(-1+\eta))^3 (x+\eta-x\eta)^3 (w+x+\eta-w\eta-x\eta)^3} - \\
& \frac{3960 f w x^6 \eta^2}{(-1+w(-1+\eta))^3 (x+\eta-x\eta)^3 (w+x+\eta-w\eta-x\eta)^3} + \\
& \frac{1804 f w^2 x^6 \eta^2}{(-1+w(-1+\eta))^3 (x+\eta-x\eta)^3 (w+x+\eta-w\eta-x\eta)^3} - \\
& \frac{396 f x \eta^3}{(x+\eta-x\eta)^3 (w+x+\eta-w\eta-x\eta)^3} + \\
& \frac{432 f w x \eta^3}{(x+\eta-x\eta)^3 (w+x+\eta-w\eta-x\eta)^3} - \frac{120 f w^2 x \eta^3}{(x+\eta-x\eta)^3 (w+x+\eta-w\eta-x\eta)^3} + \\
& \frac{288 f x^2 \eta^3}{(x+\eta-x\eta)^3 (w+x+\eta-w\eta-x\eta)^3} - \frac{1440 f w x^2 \eta^3}{(x+\eta-x\eta)^3 (w+x+\eta-w\eta-x\eta)^3} + \\
& \frac{240 f w^2 x^2 \eta^3}{(x+\eta-x\eta)^3 (w+x+\eta-w\eta-x\eta)^3} + \frac{1440 f w x^3 \eta^3}{(x+\eta-x\eta)^3 (w+x+\eta-w\eta-x\eta)^3} - \\
& \frac{72 f w^4 \eta^3}{(-1+w(-1+\eta))^3 (x+\eta-x\eta)^3 (w+x+\eta-w\eta-x\eta)^3} + \\
& \frac{40 f w^5 \eta^3}{(-1+w(-1+\eta))^3 (x+\eta-x\eta)^3 (w+x+\eta-w\eta-x\eta)^3} - \\
& \frac{360 f x \eta^3}{(-1+w(-1+\eta))^3 (x+\eta-x\eta)^3 (w+x+\eta-w\eta-x\eta)^3} - \\
& \frac{2700 f w x \eta^3}{(-1+w(-1+\eta))^3 (x+\eta-x\eta)^3 (w+x+\eta-w\eta-x\eta)^3} - \\
& \frac{4572 f w^2 x \eta^3}{(-1+w(-1+\eta))^3 (x+\eta-x\eta)^3 (w+x+\eta-w\eta-x\eta)^3} -
\end{aligned}$$

$$\begin{aligned}
& \frac{1566 f w^3 x \eta^3}{(-1+w(-1+\eta))^3 (x+\eta-x\eta)^3 (w+x+\eta-w\eta-x\eta)^3} + \\
& \frac{4566 f w^4 x \eta^3}{(-1+w(-1+\eta))^3 (x+\eta-x\eta)^3 (w+x+\eta-w\eta-x\eta)^3} - \\
& \frac{468 f w^5 x \eta^3}{(-1+w(-1+\eta))^3 (x+\eta-x\eta)^3 (w+x+\eta-w\eta-x\eta)^3} + \\
& \frac{1440 f w x^2 \eta^3}{(-1+w(-1+\eta))^3 (x+\eta-x\eta)^3 (w+x+\eta-w\eta-x\eta)^3} + \\
& \frac{2484 f w^2 x^2 \eta^3}{(-1+w(-1+\eta))^3 (x+\eta-x\eta)^3 (w+x+\eta-w\eta-x\eta)^3} + \\
& \frac{17148 f w^3 x^2 \eta^3}{(-1+w(-1+\eta))^3 (x+\eta-x\eta)^3 (w+x+\eta-w\eta-x\eta)^3} - \\
& \frac{14544 f w^4 x^2 \eta^3}{(-1+w(-1+\eta))^3 (x+\eta-x\eta)^3 (w+x+\eta-w\eta-x\eta)^3} + \\
& \frac{4320 f w^5 x^2 \eta^3}{(-1+w(-1+\eta))^3 (x+\eta-x\eta)^3 (w+x+\eta-w\eta-x\eta)^3} + \\
& \frac{360 f x^3 \eta^3}{(-1+w(-1+\eta))^3 (x+\eta-x\eta)^3 (w+x+\eta-w\eta-x\eta)^3} + \\
& \frac{180 f w x^3 \eta^3}{(-1+w(-1+\eta))^3 (x+\eta-x\eta)^3 (w+x+\eta-w\eta-x\eta)^3} + \\
& \frac{22508 f w^2 x^3 \eta^3}{(-1+w(-1+\eta))^3 (x+\eta-x\eta)^3 (w+x+\eta-w\eta-x\eta)^3} - \\
& \frac{47592 f w^3 x^3 \eta^3}{(-1+w(-1+\eta))^3 (x+\eta-x\eta)^3 (w+x+\eta-w\eta-x\eta)^3} + \\
& \frac{29160 f w^4 x^3 \eta^3}{(-1+w(-1+\eta))^3 (x+\eta-x\eta)^3 (w+x+\eta-w\eta-x\eta)^3} - \\
& \frac{4620 f w^5 x^3 \eta^3}{(-1+w(-1+\eta))^3 (x+\eta-x\eta)^3 (w+x+\eta-w\eta-x\eta)^3} + \\
& \frac{9720 f w x^4 \eta^3}{(-1+w(-1+\eta))^3 (x+\eta-x\eta)^3 (w+x+\eta-w\eta-x\eta)^3} - \\
& \frac{53460 f w^2 x^4 \eta^3}{(-1+w(-1+\eta))^3 (x+\eta-x\eta)^3 (w+x+\eta-w\eta-x\eta)^3} + \\
& \frac{57240 f w^3 x^4 \eta^3}{(-1+w(-1+\eta))^3 (x+\eta-x\eta)^3 (w+x+\eta-w\eta-x\eta)^3} - \\
& \frac{13860 f w^4 x^4 \eta^3}{(-1+w(-1+\eta))^3 (x+\eta-x\eta)^3 (w+x+\eta-w\eta-x\eta)^3} - \\
& \frac{19440 f w x^5 \eta^3}{(-1+w(-1+\eta))^3 (x+\eta-x\eta)^3 (w+x+\eta-w\eta-x\eta)^3} +
\end{aligned}$$

$$\begin{aligned}
& \frac{44\,280\,f\,w^2\,x^5\,\eta^3}{(-1+w(-1+\eta))^3(x+\eta-x\eta)^3(w+x+\eta-w\eta-x\eta)^3} - \\
& \frac{13\,860\,f\,w^3\,x^5\,\eta^3}{(-1+w(-1+\eta))^3(x+\eta-x\eta)^3(w+x+\eta-w\eta-x\eta)^3} + \\
& \frac{11\,880\,f\,w\,x^6\,\eta^3}{(-1+w(-1+\eta))^3(x+\eta-x\eta)^3(w+x+\eta-w\eta-x\eta)^3} - \\
& \frac{4\,620\,f\,w^2\,x^6\,\eta^3}{(-1+w(-1+\eta))^3(x+\eta-x\eta)^3(w+x+\eta-w\eta-x\eta)^3} + \\
& \frac{108\,f\,x\,\eta^4}{(x+\eta-x\eta)^3(w+x+\eta-w\eta-x\eta)^3} - \\
& \frac{468\,f\,w\,x\,\eta^4}{(x+\eta-x\eta)^3(w+x+\eta-w\eta-x\eta)^3} + \frac{120\,f\,w^2\,x\,\eta^4}{(x+\eta-x\eta)^3(w+x+\eta-w\eta-x\eta)^3} - \\
& \frac{72\,f\,x^2\,\eta^4}{(x+\eta-x\eta)^3(w+x+\eta-w\eta-x\eta)^3} + \frac{1\,440\,f\,w\,x^2\,\eta^4}{(x+\eta-x\eta)^3(w+x+\eta-w\eta-x\eta)^3} - \\
& \frac{180\,f\,w^2\,x^2\,\eta^4}{(x+\eta-x\eta)^3(w+x+\eta-w\eta-x\eta)^3} - \frac{10\,800\,f\,w\,x^3\,\eta^4}{(x+\eta-x\eta)^3(w+x+\eta-w\eta-x\eta)^3} - \\
& \frac{216\,f\,w^3\,\eta^4}{(-1+w(-1+\eta))^3(x+\eta-x\eta)^3(w+x+\eta-w\eta-x\eta)^3} + \\
& \frac{696\,f\,w^4\,\eta^4}{(-1+w(-1+\eta))^3(x+\eta-x\eta)^3(w+x+\eta-w\eta-x\eta)^3} - \\
& \frac{284\,f\,w^5\,\eta^4}{(-1+w(-1+\eta))^3(x+\eta-x\eta)^3(w+x+\eta-w\eta-x\eta)^3} + \\
& \frac{1\,260\,f\,w\,x\,\eta^4}{(-1+w(-1+\eta))^3(x+\eta-x\eta)^3(w+x+\eta-w\eta-x\eta)^3} + \\
& \frac{3\,060\,f\,w^2\,x\,\eta^4}{(-1+w(-1+\eta))^3(x+\eta-x\eta)^3(w+x+\eta-w\eta-x\eta)^3} + \\
& \frac{9\,456\,f\,w^3\,x\,\eta^4}{(-1+w(-1+\eta))^3(x+\eta-x\eta)^3(w+x+\eta-w\eta-x\eta)^3} - \\
& \frac{13\,578\,f\,w^4\,x\,\eta^4}{(-1+w(-1+\eta))^3(x+\eta-x\eta)^3(w+x+\eta-w\eta-x\eta)^3} + \\
& \frac{2\,340\,f\,w^5\,x\,\eta^4}{(-1+w(-1+\eta))^3(x+\eta-x\eta)^3(w+x+\eta-w\eta-x\eta)^3} + \\
& \frac{360\,f\,x^2\,\eta^4}{(-1+w(-1+\eta))^3(x+\eta-x\eta)^3(w+x+\eta-w\eta-x\eta)^3} - \\
& \frac{360\,f\,w\,x^2\,\eta^4}{(-1+w(-1+\eta))^3(x+\eta-x\eta)^3(w+x+\eta-w\eta-x\eta)^3} + \\
& \frac{15\,720\,f\,w^2\,x^2\,\eta^4}{(-1+w(-1+\eta))^3(x+\eta-x\eta)^3(w+x+\eta-w\eta-x\eta)^3} -
\end{aligned}$$

$$\begin{aligned}
& \frac{59\,964\,f\,w^3\,x^2\,\eta^4}{(-1+w(-1+\eta))^3(x+\eta-x\eta)^3(w+x+\eta-w\eta-x\eta)^3} + \\
& \frac{43\,992\,f\,w^4\,x^2\,\eta^4}{(-1+w(-1+\eta))^3(x+\eta-x\eta)^3(w+x+\eta-w\eta-x\eta)^3} - \\
& \frac{9540\,f\,w^5\,x^2\,\eta^4}{(-1+w(-1+\eta))^3(x+\eta-x\eta)^3(w+x+\eta-w\eta-x\eta)^3} - \\
& \frac{360\,f\,x^3\,\eta^4}{(-1+w(-1+\eta))^3(x+\eta-x\eta)^3(w+x+\eta-w\eta-x\eta)^3} + \\
& \frac{9360\,f\,w\,x^3\,\eta^4}{(-1+w(-1+\eta))^3(x+\eta-x\eta)^3(w+x+\eta-w\eta-x\eta)^3} - \\
& \frac{87\,220\,f\,w^2\,x^3\,\eta^4}{(-1+w(-1+\eta))^3(x+\eta-x\eta)^3(w+x+\eta-w\eta-x\eta)^3} + \\
& \frac{135\,144\,f\,w^3\,x^3\,\eta^4}{(-1+w(-1+\eta))^3(x+\eta-x\eta)^3(w+x+\eta-w\eta-x\eta)^3} - \\
& \frac{61\,920\,f\,w^4\,x^3\,\eta^4}{(-1+w(-1+\eta))^3(x+\eta-x\eta)^3(w+x+\eta-w\eta-x\eta)^3} + \\
& \frac{7260\,f\,w^5\,x^3\,\eta^4}{(-1+w(-1+\eta))^3(x+\eta-x\eta)^3(w+x+\eta-w\eta-x\eta)^3} - \\
& \frac{38\,880\,f\,w\,x^4\,\eta^4}{(-1+w(-1+\eta))^3(x+\eta-x\eta)^3(w+x+\eta-w\eta-x\eta)^3} + \\
& \frac{146\,340\,f\,w^2\,x^4\,\eta^4}{(-1+w(-1+\eta))^3(x+\eta-x\eta)^3(w+x+\eta-w\eta-x\eta)^3} - \\
& \frac{118\,980\,f\,w^3\,x^4\,\eta^4}{(-1+w(-1+\eta))^3(x+\eta-x\eta)^3(w+x+\eta-w\eta-x\eta)^3} + \\
& \frac{21\,780\,f\,w^4\,x^4\,\eta^4}{(-1+w(-1+\eta))^3(x+\eta-x\eta)^3(w+x+\eta-w\eta-x\eta)^3} + \\
& \frac{51\,840\,f\,w\,x^5\,\eta^4}{(-1+w(-1+\eta))^3(x+\eta-x\eta)^3(w+x+\eta-w\eta-x\eta)^3} - \\
& \frac{90\,360\,f\,w^2\,x^5\,\eta^4}{(-1+w(-1+\eta))^3(x+\eta-x\eta)^3(w+x+\eta-w\eta-x\eta)^3} + \\
& \frac{21\,780\,f\,w^3\,x^5\,\eta^4}{(-1+w(-1+\eta))^3(x+\eta-x\eta)^3(w+x+\eta-w\eta-x\eta)^3} - \\
& \frac{23\,760\,f\,w\,x^6\,\eta^4}{(-1+w(-1+\eta))^3(x+\eta-x\eta)^3(w+x+\eta-w\eta-x\eta)^3} + \\
& \frac{7260\,f\,w^2\,x^6\,\eta^4}{(-1+w(-1+\eta))^3(x+\eta-x\eta)^3(w+x+\eta-w\eta-x\eta)^3} + \\
& \frac{288\,f\,w\,x\,\eta^5}{(x+\eta-x\eta)^3(w+x+\eta-w\eta-x\eta)^3} -
\end{aligned}$$

$$\begin{aligned}
& \frac{60 f w^2 x \eta^5}{(x + \eta - x \eta)^3 (w + x + \eta - w \eta - x \eta)^3} - \frac{720 f w x^2 \eta^5}{(x + \eta - x \eta)^3 (w + x + \eta - w \eta - x \eta)^3} + \\
& \frac{72 f w^2 x^2 \eta^5}{(x + \eta - x \eta)^3 (w + x + \eta - w \eta - x \eta)^3} + \frac{432 f w x^3 \eta^5}{(x + \eta - x \eta)^3 (w + x + \eta - w \eta - x \eta)^3} - \\
& \frac{216 f w^2 \eta^5}{(-1 + w (-1 + \eta))^3 (x + \eta - x \eta)^3 (w + x + \eta - w \eta - x \eta)^3} + \\
& \frac{1632 f w^3 \eta^5}{(-1 + w (-1 + \eta))^3 (x + \eta - x \eta)^3 (w + x + \eta - w \eta - x \eta)^3} - \\
& \frac{2748 f w^4 \eta^5}{(-1 + w (-1 + \eta))^3 (x + \eta - x \eta)^3 (w + x + \eta - w \eta - x \eta)^3} + \\
& \frac{832 f w^5 \eta^5}{(-1 + w (-1 + \eta))^3 (x + \eta - x \eta)^3 (w + x + \eta - w \eta - x \eta)^3} + \\
& \frac{108 f x \eta^5}{(-1 + w (-1 + \eta))^3 (x + \eta - x \eta)^3 (w + x + \eta - w \eta - x \eta)^3} - \\
& \frac{252 f w x \eta^5}{(-1 + w (-1 + \eta))^3 (x + \eta - x \eta)^3 (w + x + \eta - w \eta - x \eta)^3} + \\
& \frac{6162 f w^2 x \eta^5}{(-1 + w (-1 + \eta))^3 (x + \eta - x \eta)^3 (w + x + \eta - w \eta - x \eta)^3} - \\
& \frac{30\,066 f w^3 x \eta^5}{(-1 + w (-1 + \eta))^3 (x + \eta - x \eta)^3 (w + x + \eta - w \eta - x \eta)^3} + \\
& \frac{29\,514 f w^4 x \eta^5}{(-1 + w (-1 + \eta))^3 (x + \eta - x \eta)^3 (w + x + \eta - w \eta - x \eta)^3} - \\
& \frac{4932 f w^5 x \eta^5}{(-1 + w (-1 + \eta))^3 (x + \eta - x \eta)^3 (w + x + \eta - w \eta - x \eta)^3} - \\
& \frac{288 f x^2 \eta^5}{(-1 + w (-1 + \eta))^3 (x + \eta - x \eta)^3 (w + x + \eta - w \eta - x \eta)^3} + \\
& \frac{5796 f w x^2 \eta^5}{(-1 + w (-1 + \eta))^3 (x + \eta - x \eta)^3 (w + x + \eta - w \eta - x \eta)^3} - \\
& \frac{65\,544 f w^2 x^2 \eta^5}{(-1 + w (-1 + \eta))^3 (x + \eta - x \eta)^3 (w + x + \eta - w \eta - x \eta)^3} + \\
& \frac{136\,596 f w^3 x^2 \eta^5}{(-1 + w (-1 + \eta))^3 (x + \eta - x \eta)^3 (w + x + \eta - w \eta - x \eta)^3} - \\
& \frac{79\,992 f w^4 x^2 \eta^5}{(-1 + w (-1 + \eta))^3 (x + \eta - x \eta)^3 (w + x + \eta - w \eta - x \eta)^3} + \\
& \frac{12\,240 f w^5 x^2 \eta^5}{(-1 + w (-1 + \eta))^3 (x + \eta - x \eta)^3 (w + x + \eta - w \eta - x \eta)^3} + \\
& \frac{180 f x^3 \eta^5}{(-1 + w (-1 + \eta))^3 (x + \eta - x \eta)^3 (w + x + \eta - w \eta - x \eta)^3} -
\end{aligned}$$



$$\begin{aligned}
& \frac{38\,700\,f\,w\,x^3\,\eta^5}{(-1+w(-1+\eta))^3(x+\eta-x\eta)^3(w+x+\eta-w\eta-x\eta)^3} + \\
& \frac{201\,860\,f\,w^2\,x^3\,\eta^5}{(-1+w(-1+\eta))^3(x+\eta-x\eta)^3(w+x+\eta-w\eta-x\eta)^3} - \\
& \frac{240\,840\,f\,w^3\,x^3\,\eta^5}{(-1+w(-1+\eta))^3(x+\eta-x\eta)^3(w+x+\eta-w\eta-x\eta)^3} + \\
& \frac{82\,224\,f\,w^4\,x^3\,\eta^5}{(-1+w(-1+\eta))^3(x+\eta-x\eta)^3(w+x+\eta-w\eta-x\eta)^3} - \\
& \frac{6600\,f\,w^5\,x^3\,\eta^5}{(-1+w(-1+\eta))^3(x+\eta-x\eta)^3(w+x+\eta-w\eta-x\eta)^3} + \\
& \frac{90\,720\,f\,w\,x^4\,\eta^5}{(-1+w(-1+\eta))^3(x+\eta-x\eta)^3(w+x+\eta-w\eta-x\eta)^3} - \\
& \frac{257\,760\,f\,w^2\,x^4\,\eta^5}{(-1+w(-1+\eta))^3(x+\eta-x\eta)^3(w+x+\eta-w\eta-x\eta)^3} + \\
& \frac{160\,992\,f\,w^3\,x^4\,\eta^5}{(-1+w(-1+\eta))^3(x+\eta-x\eta)^3(w+x+\eta-w\eta-x\eta)^3} - \\
& \frac{19\,800\,f\,w^4\,x^4\,\eta^5}{(-1+w(-1+\eta))^3(x+\eta-x\eta)^3(w+x+\eta-w\eta-x\eta)^3} - \\
& \frac{90\,720\,f\,w\,x^5\,\eta^5}{(-1+w(-1+\eta))^3(x+\eta-x\eta)^3(w+x+\eta-w\eta-x\eta)^3} + \\
& \frac{124\,272\,f\,w^2\,x^5\,\eta^5}{(-1+w(-1+\eta))^3(x+\eta-x\eta)^3(w+x+\eta-w\eta-x\eta)^3} - \\
& \frac{19\,800\,f\,w^3\,x^5\,\eta^5}{(-1+w(-1+\eta))^3(x+\eta-x\eta)^3(w+x+\eta-w\eta-x\eta)^3} + \\
& \frac{33\,264\,f\,w\,x^6\,\eta^5}{(-1+w(-1+\eta))^3(x+\eta-x\eta)^3(w+x+\eta-w\eta-x\eta)^3} - \\
& \frac{6600\,f\,w^2\,x^6\,\eta^5}{(-1+w(-1+\eta))^3(x+\eta-x\eta)^3(w+x+\eta-w\eta-x\eta)^3} - \\
& \frac{72\,f\,w\,x\,\eta^6}{(x+\eta-x\eta)^3(w+x+\eta-w\eta-x\eta)^3} + \\
& \frac{12\,f\,w^2\,x\,\eta^6}{(x+\eta-x\eta)^3(w+x+\eta-w\eta-x\eta)^3} + \frac{144\,f\,w\,x^2\,\eta^6}{(x+\eta-x\eta)^3(w+x+\eta-w\eta-x\eta)^3} - \\
& \frac{12\,f\,w^2\,x^2\,\eta^6}{(x+\eta-x\eta)^3(w+x+\eta-w\eta-x\eta)^3} - \frac{72\,f\,w\,x^3\,\eta^6}{(x+\eta-x\eta)^3(w+x+\eta-w\eta-x\eta)^3} - \\
& \frac{72\,f\,w\,\eta^6}{(-1+w(-1+\eta))^3(x+\eta-x\eta)^3(w+x+\eta-w\eta-x\eta)^3} + \\
& \frac{1336\,f\,w^2\,\eta^6}{(-1+w(-1+\eta))^3(x+\eta-x\eta)^3(w+x+\eta-w\eta-x\eta)^3} -
\end{aligned}$$

$$\begin{aligned}
& \frac{5148 f w^3 \eta^6}{(-1+w(-1+\eta))^3 (x+\eta-x\eta)^3 (w+x+\eta-w\eta-x\eta)^3} + \\
& \frac{5796 f w^4 \eta^6}{(-1+w(-1+\eta))^3 (x+\eta-x\eta)^3 (w+x+\eta-w\eta-x\eta)^3} - \\
& \frac{1232 f w^5 \eta^6}{(-1+w(-1+\eta))^3 (x+\eta-x\eta)^3 (w+x+\eta-w\eta-x\eta)^3} - \\
& \frac{36 f x \eta^6}{(-1+w(-1+\eta))^3 (x+\eta-x\eta)^3 (w+x+\eta-w\eta-x\eta)^3} + \\
& \frac{2196 f w x \eta^6}{(-1+w(-1+\eta))^3 (x+\eta-x\eta)^3 (w+x+\eta-w\eta-x\eta)^3} - \\
& \frac{24138 f w^2 x \eta^6}{(-1+w(-1+\eta))^3 (x+\eta-x\eta)^3 (w+x+\eta-w\eta-x\eta)^3} + \\
& \frac{58392 f w^3 x \eta^6}{(-1+w(-1+\eta))^3 (x+\eta-x\eta)^3 (w+x+\eta-w\eta-x\eta)^3} - \\
& \frac{42126 f w^4 x \eta^6}{(-1+w(-1+\eta))^3 (x+\eta-x\eta)^3 (w+x+\eta-w\eta-x\eta)^3} + \\
& \frac{5040 f w^5 x \eta^6}{(-1+w(-1+\eta))^3 (x+\eta-x\eta)^3 (w+x+\eta-w\eta-x\eta)^3} + \\
& \frac{72 f x^2 \eta^6}{(-1+w(-1+\eta))^3 (x+\eta-x\eta)^3 (w+x+\eta-w\eta-x\eta)^3} - \\
& \frac{21636 f w x^2 \eta^6}{(-1+w(-1+\eta))^3 (x+\eta-x\eta)^3 (w+x+\eta-w\eta-x\eta)^3} + \\
& \frac{132156 f w^2 x^2 \eta^6}{(-1+w(-1+\eta))^3 (x+\eta-x\eta)^3 (w+x+\eta-w\eta-x\eta)^3} - \\
& \frac{200508 f w^3 x^2 \eta^6}{(-1+w(-1+\eta))^3 (x+\eta-x\eta)^3 (w+x+\eta-w\eta-x\eta)^3} + \\
& \frac{88704 f w^4 x^2 \eta^6}{(-1+w(-1+\eta))^3 (x+\eta-x\eta)^3 (w+x+\eta-w\eta-x\eta)^3} - \\
& \frac{7560 f w^5 x^2 \eta^6}{(-1+w(-1+\eta))^3 (x+\eta-x\eta)^3 (w+x+\eta-w\eta-x\eta)^3} - \\
& \frac{36 f x^3 \eta^6}{(-1+w(-1+\eta))^3 (x+\eta-x\eta)^3 (w+x+\eta-w\eta-x\eta)^3} + \\
& \frac{79992 f w x^3 \eta^6}{(-1+w(-1+\eta))^3 (x+\eta-x\eta)^3 (w+x+\eta-w\eta-x\eta)^3} - \\
& \frac{299068 f w^2 x^3 \eta^6}{(-1+w(-1+\eta))^3 (x+\eta-x\eta)^3 (w+x+\eta-w\eta-x\eta)^3} + \\
& \frac{276192 f w^3 x^3 \eta^6}{(-1+w(-1+\eta))^3 (x+\eta-x\eta)^3 (w+x+\eta-w\eta-x\eta)^3} -
\end{aligned}$$

$$\begin{aligned}
& \frac{63\,504\,f\,w^4\,x^3\,\eta^6}{(-1+w(-1+\eta))^3(x+\eta-x\eta)^3(w+x+\eta-w\eta-x\eta)^3} + \\
& \frac{1848\,f\,w^5\,x^3\,\eta^6}{(-1+w(-1+\eta))^3(x+\eta-x\eta)^3(w+x+\eta-w\eta-x\eta)^3} - \\
& \frac{136\,080\,f\,w\,x^4\,\eta^6}{(-1+w(-1+\eta))^3(x+\eta-x\eta)^3(w+x+\eta-w\eta-x\eta)^3} + \\
& \frac{302\,400\,f\,w^2\,x^4\,\eta^6}{(-1+w(-1+\eta))^3(x+\eta-x\eta)^3(w+x+\eta-w\eta-x\eta)^3} - \\
& \frac{137\,592\,f\,w^3\,x^4\,\eta^6}{(-1+w(-1+\eta))^3(x+\eta-x\eta)^3(w+x+\eta-w\eta-x\eta)^3} + \\
& \frac{5544\,f\,w^4\,x^4\,\eta^6}{(-1+w(-1+\eta))^3(x+\eta-x\eta)^3(w+x+\eta-w\eta-x\eta)^3} + \\
& \frac{108\,864\,f\,w\,x^5\,\eta^6}{(-1+w(-1+\eta))^3(x+\eta-x\eta)^3(w+x+\eta-w\eta-x\eta)^3} - \\
& \frac{114\,912\,f\,w^2\,x^5\,\eta^6}{(-1+w(-1+\eta))^3(x+\eta-x\eta)^3(w+x+\eta-w\eta-x\eta)^3} + \\
& \frac{5544\,f\,w^3\,x^5\,\eta^6}{(-1+w(-1+\eta))^3(x+\eta-x\eta)^3(w+x+\eta-w\eta-x\eta)^3} - \\
& \frac{33\,264\,f\,w\,x^6\,\eta^6}{(-1+w(-1+\eta))^3(x+\eta-x\eta)^3(w+x+\eta-w\eta-x\eta)^3} + \\
& \frac{1848\,f\,w^2\,x^6\,\eta^6}{(-1+w(-1+\eta))^3(x+\eta-x\eta)^3(w+x+\eta-w\eta-x\eta)^3} + \\
& \frac{360\,f\,w\,\eta^7}{(-1+w(-1+\eta))^3(x+\eta-x\eta)^3(w+x+\eta-w\eta-x\eta)^3} - \\
& \frac{3404\,f\,w^2\,\eta^7}{(-1+w(-1+\eta))^3(x+\eta-x\eta)^3(w+x+\eta-w\eta-x\eta)^3} + \\
& \frac{8712\,f\,w^3\,\eta^7}{(-1+w(-1+\eta))^3(x+\eta-x\eta)^3(w+x+\eta-w\eta-x\eta)^3} - \\
& \frac{6972\,f\,w^4\,\eta^7}{(-1+w(-1+\eta))^3(x+\eta-x\eta)^3(w+x+\eta-w\eta-x\eta)^3} + \\
& \frac{784\,f\,w^5\,\eta^7}{(-1+w(-1+\eta))^3(x+\eta-x\eta)^3(w+x+\eta-w\eta-x\eta)^3} - \\
& \frac{6372\,f\,w\,x\,\eta^7}{(-1+w(-1+\eta))^3(x+\eta-x\eta)^3(w+x+\eta-w\eta-x\eta)^3} + \\
& \frac{40\,536\,f\,w^2\,x\,\eta^7}{(-1+w(-1+\eta))^3(x+\eta-x\eta)^3(w+x+\eta-w\eta-x\eta)^3} - \\
& \frac{70\,302\,f\,w^3\,x\,\eta^7}{(-1+w(-1+\eta))^3(x+\eta-x\eta)^3(w+x+\eta-w\eta-x\eta)^3} +
\end{aligned}$$

$$\begin{aligned}
& \frac{36\,282\,f\,w^4\,x\,\eta^7}{(-1+w(-1+\eta))^3(x+\eta-x\eta)^3(w+x+\eta-w\eta-x\eta)^3} - \\
& \frac{1008\,f\,w^5\,x\,\eta^7}{(-1+w(-1+\eta))^3(x+\eta-x\eta)^3(w+x+\eta-w\eta-x\eta)^3} + \\
& \frac{37\,584\,f\,w\,x^2\,\eta^7}{(-1+w(-1+\eta))^3(x+\eta-x\eta)^3(w+x+\eta-w\eta-x\eta)^3} - \\
& \frac{162\,048\,f\,w^2\,x^2\,\eta^7}{(-1+w(-1+\eta))^3(x+\eta-x\eta)^3(w+x+\eta-w\eta-x\eta)^3} + \\
& \frac{186\,132\,f\,w^3\,x^2\,\eta^7}{(-1+w(-1+\eta))^3(x+\eta-x\eta)^3(w+x+\eta-w\eta-x\eta)^3} - \\
& \frac{53\,424\,f\,w^4\,x^2\,\eta^7}{(-1+w(-1+\eta))^3(x+\eta-x\eta)^3(w+x+\eta-w\eta-x\eta)^3} - \\
& \frac{2016\,f\,w^5\,x^2\,\eta^7}{(-1+w(-1+\eta))^3(x+\eta-x\eta)^3(w+x+\eta-w\eta-x\eta)^3} - \\
& \frac{100\,692\,f\,w\,x^3\,\eta^7}{(-1+w(-1+\eta))^3(x+\eta-x\eta)^3(w+x+\eta-w\eta-x\eta)^3} + \\
& \frac{288\,596\,f\,w^2\,x^3\,\eta^7}{(-1+w(-1+\eta))^3(x+\eta-x\eta)^3(w+x+\eta-w\eta-x\eta)^3} - \\
& \frac{195\,552\,f\,w^3\,x^3\,\eta^7}{(-1+w(-1+\eta))^3(x+\eta-x\eta)^3(w+x+\eta-w\eta-x\eta)^3} + \\
& \frac{15\,696\,f\,w^4\,x^3\,\eta^7}{(-1+w(-1+\eta))^3(x+\eta-x\eta)^3(w+x+\eta-w\eta-x\eta)^3} + \\
& \frac{3432\,f\,w^5\,x^3\,\eta^7}{(-1+w(-1+\eta))^3(x+\eta-x\eta)^3(w+x+\eta-w\eta-x\eta)^3} + \\
& \frac{136\,080\,f\,w\,x^4\,\eta^7}{(-1+w(-1+\eta))^3(x+\eta-x\eta)^3(w+x+\eta-w\eta-x\eta)^3} - \\
& \frac{234\,360\,f\,w^2\,x^4\,\eta^7}{(-1+w(-1+\eta))^3(x+\eta-x\eta)^3(w+x+\eta-w\eta-x\eta)^3} + \\
& \frac{61\,200\,f\,w^3\,x^4\,\eta^7}{(-1+w(-1+\eta))^3(x+\eta-x\eta)^3(w+x+\eta-w\eta-x\eta)^3} + \\
& \frac{10\,296\,f\,w^4\,x^4\,\eta^7}{(-1+w(-1+\eta))^3(x+\eta-x\eta)^3(w+x+\eta-w\eta-x\eta)^3} - \\
& \frac{90\,720\,f\,w\,x^5\,\eta^7}{(-1+w(-1+\eta))^3(x+\eta-x\eta)^3(w+x+\eta-w\eta-x\eta)^3} + \\
& \frac{67\,248\,f\,w^2\,x^5\,\eta^7}{(-1+w(-1+\eta))^3(x+\eta-x\eta)^3(w+x+\eta-w\eta-x\eta)^3} + \\
& \frac{10\,296\,f\,w^3\,x^5\,\eta^7}{(-1+w(-1+\eta))^3(x+\eta-x\eta)^3(w+x+\eta-w\eta-x\eta)^3} +
\end{aligned}$$

$$\begin{aligned}
& \frac{23\,760\,f\,w\,x^6\,\eta^7}{(-1+w(-1+\eta))^3(x+\eta-x\eta)^3(w+x+\eta-w\eta-x\eta)^3} + \\
& \frac{3432\,f\,w^2\,x^6\,\eta^7}{(-1+w(-1+\eta))^3(x+\eta-x\eta)^3(w+x+\eta-w\eta-x\eta)^3} - \\
& \frac{720\,f\,w\,\eta^8}{(-1+w(-1+\eta))^3(x+\eta-x\eta)^3(w+x+\eta-w\eta-x\eta)^3} + \\
& \frac{4540\,f\,w^2\,\eta^8}{(-1+w(-1+\eta))^3(x+\eta-x\eta)^3(w+x+\eta-w\eta-x\eta)^3} - \\
& \frac{8340\,f\,w^3\,\eta^8}{(-1+w(-1+\eta))^3(x+\eta-x\eta)^3(w+x+\eta-w\eta-x\eta)^3} + \\
& \frac{4452\,f\,w^4\,\eta^8}{(-1+w(-1+\eta))^3(x+\eta-x\eta)^3(w+x+\eta-w\eta-x\eta)^3} + \\
& \frac{280\,f\,w^5\,\eta^8}{(-1+w(-1+\eta))^3(x+\eta-x\eta)^3(w+x+\eta-w\eta-x\eta)^3} + \\
& \frac{8640\,f\,w\,x\,\eta^8}{(-1+w(-1+\eta))^3(x+\eta-x\eta)^3(w+x+\eta-w\eta-x\eta)^3} - \\
& \frac{39\,468\,f\,w^2\,x\,\eta^8}{(-1+w(-1+\eta))^3(x+\eta-x\eta)^3(w+x+\eta-w\eta-x\eta)^3} + \\
& \frac{50\,376\,f\,w^3\,x\,\eta^8}{(-1+w(-1+\eta))^3(x+\eta-x\eta)^3(w+x+\eta-w\eta-x\eta)^3} - \\
& \frac{14\,586\,f\,w^4\,x\,\eta^8}{(-1+w(-1+\eta))^3(x+\eta-x\eta)^3(w+x+\eta-w\eta-x\eta)^3} - \\
& \frac{3672\,f\,w^5\,x\,\eta^8}{(-1+w(-1+\eta))^3(x+\eta-x\eta)^3(w+x+\eta-w\eta-x\eta)^3} - \\
& \frac{37\,800\,f\,w\,x^2\,\eta^8}{(-1+w(-1+\eta))^3(x+\eta-x\eta)^3(w+x+\eta-w\eta-x\eta)^3} + \\
& \frac{123\,276\,f\,w^2\,x^2\,\eta^8}{(-1+w(-1+\eta))^3(x+\eta-x\eta)^3(w+x+\eta-w\eta-x\eta)^3} - \\
& \frac{100\,068\,f\,w^3\,x^2\,\eta^8}{(-1+w(-1+\eta))^3(x+\eta-x\eta)^3(w+x+\eta-w\eta-x\eta)^3} + \\
& \frac{4464\,f\,w^4\,x^2\,\eta^8}{(-1+w(-1+\eta))^3(x+\eta-x\eta)^3(w+x+\eta-w\eta-x\eta)^3} + \\
& \frac{8280\,f\,w^5\,x^2\,\eta^8}{(-1+w(-1+\eta))^3(x+\eta-x\eta)^3(w+x+\eta-w\eta-x\eta)^3} + \\
& \frac{80\,640\,f\,w\,x^3\,\eta^8}{(-1+w(-1+\eta))^3(x+\eta-x\eta)^3(w+x+\eta-w\eta-x\eta)^3} - \\
& \frac{175\,948\,f\,w^2\,x^3\,\eta^8}{(-1+w(-1+\eta))^3(x+\eta-x\eta)^3(w+x+\eta-w\eta-x\eta)^3} +
\end{aligned}$$

$$\begin{aligned}
& \frac{68\,112\,f\,w^3\,x^3\,\eta^8}{(-1+w(-1+\eta))^3(x+\eta-x\eta)^3(w+x+\eta-w\eta-x\eta)^3} + \\
& \frac{21\,240\,f\,w^4\,x^3\,\eta^8}{(-1+w(-1+\eta))^3(x+\eta-x\eta)^3(w+x+\eta-w\eta-x\eta)^3} - \\
& \frac{5280\,f\,w^5\,x^3\,\eta^8}{(-1+w(-1+\eta))^3(x+\eta-x\eta)^3(w+x+\eta-w\eta-x\eta)^3} - \\
& \frac{90\,720\,f\,w\,x^4\,\eta^8}{(-1+w(-1+\eta))^3(x+\eta-x\eta)^3(w+x+\eta-w\eta-x\eta)^3} + \\
& \frac{111\,960\,f\,w^2\,x^4\,\eta^8}{(-1+w(-1+\eta))^3(x+\eta-x\eta)^3(w+x+\eta-w\eta-x\eta)^3} + \\
& \frac{5760\,f\,w^3\,x^4\,\eta^8}{(-1+w(-1+\eta))^3(x+\eta-x\eta)^3(w+x+\eta-w\eta-x\eta)^3} - \\
& \frac{15\,840\,f\,w^4\,x^4\,\eta^8}{(-1+w(-1+\eta))^3(x+\eta-x\eta)^3(w+x+\eta-w\eta-x\eta)^3} + \\
& \frac{51\,840\,f\,w\,x^5\,\eta^8}{(-1+w(-1+\eta))^3(x+\eta-x\eta)^3(w+x+\eta-w\eta-x\eta)^3} - \\
& \frac{19\,080\,f\,w^2\,x^5\,\eta^8}{(-1+w(-1+\eta))^3(x+\eta-x\eta)^3(w+x+\eta-w\eta-x\eta)^3} - \\
& \frac{15\,840\,f\,w^3\,x^5\,\eta^8}{(-1+w(-1+\eta))^3(x+\eta-x\eta)^3(w+x+\eta-w\eta-x\eta)^3} - \\
& \frac{11\,880\,f\,w\,x^6\,\eta^8}{(-1+w(-1+\eta))^3(x+\eta-x\eta)^3(w+x+\eta-w\eta-x\eta)^3} - \\
& \frac{5280\,f\,w^2\,x^6\,\eta^8}{(-1+w(-1+\eta))^3(x+\eta-x\eta)^3(w+x+\eta-w\eta-x\eta)^3} + \\
& \frac{720\,f\,w\,\eta^9}{(-1+w(-1+\eta))^3(x+\eta-x\eta)^3(w+x+\eta-w\eta-x\eta)^3} - \\
& \frac{3280\,f\,w^2\,\eta^9}{(-1+w(-1+\eta))^3(x+\eta-x\eta)^3(w+x+\eta-w\eta-x\eta)^3} + \\
& \frac{4176\,f\,w^3\,\eta^9}{(-1+w(-1+\eta))^3(x+\eta-x\eta)^3(w+x+\eta-w\eta-x\eta)^3} - \\
& \frac{756\,f\,w^4\,\eta^9}{(-1+w(-1+\eta))^3(x+\eta-x\eta)^3(w+x+\eta-w\eta-x\eta)^3} - \\
& \frac{896\,f\,w^5\,\eta^9}{(-1+w(-1+\eta))^3(x+\eta-x\eta)^3(w+x+\eta-w\eta-x\eta)^3} - \\
& \frac{6480\,f\,w\,x\,\eta^9}{(-1+w(-1+\eta))^3(x+\eta-x\eta)^3(w+x+\eta-w\eta-x\eta)^3} + \\
& \frac{21\,960\,f\,w^2\,x\,\eta^9}{(-1+w(-1+\eta))^3(x+\eta-x\eta)^3(w+x+\eta-w\eta-x\eta)^3} -
\end{aligned}$$

$$\begin{aligned}
& \frac{17\,856\,f\,w^3\,x\,\eta^9}{(-1+w(-1+\eta))^3(x+\eta-x\eta)^3(w+x+\eta-w\eta-x\eta)^3} - \\
& \frac{3012\,f\,w^4\,x\,\eta^9}{(-1+w(-1+\eta))^3(x+\eta-x\eta)^3(w+x+\eta-w\eta-x\eta)^3} + \\
& \frac{4770\,f\,w^5\,x\,\eta^9}{(-1+w(-1+\eta))^3(x+\eta-x\eta)^3(w+x+\eta-w\eta-x\eta)^3} + \\
& \frac{22\,680\,f\,w\,x^2\,\eta^9}{(-1+w(-1+\eta))^3(x+\eta-x\eta)^3(w+x+\eta-w\eta-x\eta)^3} - \\
& \frac{54\,180\,f\,w^2\,x^2\,\eta^9}{(-1+w(-1+\eta))^3(x+\eta-x\eta)^3(w+x+\eta-w\eta-x\eta)^3} + \\
& \frac{19\,704\,f\,w^3\,x^2\,\eta^9}{(-1+w(-1+\eta))^3(x+\eta-x\eta)^3(w+x+\eta-w\eta-x\eta)^3} + \\
& \frac{18\,828\,f\,w^4\,x^2\,\eta^9}{(-1+w(-1+\eta))^3(x+\eta-x\eta)^3(w+x+\eta-w\eta-x\eta)^3} - \\
& \frac{7560\,f\,w^5\,x^2\,\eta^9}{(-1+w(-1+\eta))^3(x+\eta-x\eta)^3(w+x+\eta-w\eta-x\eta)^3} - \\
& \frac{40\,320\,f\,w\,x^3\,\eta^9}{(-1+w(-1+\eta))^3(x+\eta-x\eta)^3(w+x+\eta-w\eta-x\eta)^3} + \\
& \frac{59\,840\,f\,w^2\,x^3\,\eta^9}{(-1+w(-1+\eta))^3(x+\eta-x\eta)^3(w+x+\eta-w\eta-x\eta)^3} + \\
& \frac{8676\,f\,w^3\,x^3\,\eta^9}{(-1+w(-1+\eta))^3(x+\eta-x\eta)^3(w+x+\eta-w\eta-x\eta)^3} - \\
& \frac{26\,280\,f\,w^4\,x^3\,\eta^9}{(-1+w(-1+\eta))^3(x+\eta-x\eta)^3(w+x+\eta-w\eta-x\eta)^3} + \\
& \frac{3740\,f\,w^5\,x^3\,\eta^9}{(-1+w(-1+\eta))^3(x+\eta-x\eta)^3(w+x+\eta-w\eta-x\eta)^3} + \\
& \frac{38\,880\,f\,w\,x^4\,\eta^9}{(-1+w(-1+\eta))^3(x+\eta-x\eta)^3(w+x+\eta-w\eta-x\eta)^3} - \\
& \frac{24\,840\,f\,w^2\,x^4\,\eta^9}{(-1+w(-1+\eta))^3(x+\eta-x\eta)^3(w+x+\eta-w\eta-x\eta)^3} - \\
& \frac{25\,920\,f\,w^3\,x^4\,\eta^9}{(-1+w(-1+\eta))^3(x+\eta-x\eta)^3(w+x+\eta-w\eta-x\eta)^3} + \\
& \frac{11\,220\,f\,w^4\,x^4\,\eta^9}{(-1+w(-1+\eta))^3(x+\eta-x\eta)^3(w+x+\eta-w\eta-x\eta)^3} - \\
& \frac{19\,440\,f\,w\,x^5\,\eta^9}{(-1+w(-1+\eta))^3(x+\eta-x\eta)^3(w+x+\eta-w\eta-x\eta)^3} - \\
& \frac{3240\,f\,w^2\,x^5\,\eta^9}{(-1+w(-1+\eta))^3(x+\eta-x\eta)^3(w+x+\eta-w\eta-x\eta)^3} +
\end{aligned}$$

$$\begin{aligned}
& \frac{11\,220\,f\,w^3\,x^5\,\eta^9}{(-1+w(-1+\eta))^3(x+\eta-x\eta)^3(w+x+\eta-w\eta-x\eta)^3} + \\
& \frac{3960\,f\,w\,x^6\,\eta^9}{(-1+w(-1+\eta))^3(x+\eta-x\eta)^3(w+x+\eta-w\eta-x\eta)^3} + \\
& \frac{3740\,f\,w^2\,x^6\,\eta^9}{(-1+w(-1+\eta))^3(x+\eta-x\eta)^3(w+x+\eta-w\eta-x\eta)^3} - \\
& \frac{360\,f\,w\,\eta^{10}}{(-1+w(-1+\eta))^3(x+\eta-x\eta)^3(w+x+\eta-w\eta-x\eta)^3} + \\
& \frac{1136\,f\,w^2\,\eta^{10}}{(-1+w(-1+\eta))^3(x+\eta-x\eta)^3(w+x+\eta-w\eta-x\eta)^3} - \\
& \frac{612\,f\,w^3\,\eta^{10}}{(-1+w(-1+\eta))^3(x+\eta-x\eta)^3(w+x+\eta-w\eta-x\eta)^3} - \\
& \frac{852\,f\,w^4\,\eta^{10}}{(-1+w(-1+\eta))^3(x+\eta-x\eta)^3(w+x+\eta-w\eta-x\eta)^3} + \\
& \frac{688\,f\,w^5\,\eta^{10}}{(-1+w(-1+\eta))^3(x+\eta-x\eta)^3(w+x+\eta-w\eta-x\eta)^3} + \\
& \frac{2592\,f\,w\,x\,\eta^{10}}{(-1+w(-1+\eta))^3(x+\eta-x\eta)^3(w+x+\eta-w\eta-x\eta)^3} - \\
& \frac{5760\,f\,w^2\,x\,\eta^{10}}{(-1+w(-1+\eta))^3(x+\eta-x\eta)^3(w+x+\eta-w\eta-x\eta)^3} - \\
& \frac{228\,f\,w^3\,x\,\eta^{10}}{(-1+w(-1+\eta))^3(x+\eta-x\eta)^3(w+x+\eta-w\eta-x\eta)^3} + \\
& \frac{6312\,f\,w^4\,x\,\eta^{10}}{(-1+w(-1+\eta))^3(x+\eta-x\eta)^3(w+x+\eta-w\eta-x\eta)^3} - \\
& \frac{2808\,f\,w^5\,x\,\eta^{10}}{(-1+w(-1+\eta))^3(x+\eta-x\eta)^3(w+x+\eta-w\eta-x\eta)^3} - \\
& \frac{7560\,f\,w\,x^2\,\eta^{10}}{(-1+w(-1+\eta))^3(x+\eta-x\eta)^3(w+x+\eta-w\eta-x\eta)^3} + \\
& \frac{10\,140\,f\,w^2\,x^2\,\eta^{10}}{(-1+w(-1+\eta))^3(x+\eta-x\eta)^3(w+x+\eta-w\eta-x\eta)^3} + \\
& \frac{8976\,f\,w^3\,x^2\,\eta^{10}}{(-1+w(-1+\eta))^3(x+\eta-x\eta)^3(w+x+\eta-w\eta-x\eta)^3} - \\
& \frac{14\,688\,f\,w^4\,x^2\,\eta^{10}}{(-1+w(-1+\eta))^3(x+\eta-x\eta)^3(w+x+\eta-w\eta-x\eta)^3} + \\
& \frac{3660\,f\,w^5\,x^2\,\eta^{10}}{(-1+w(-1+\eta))^3(x+\eta-x\eta)^3(w+x+\eta-w\eta-x\eta)^3} + \\
& \frac{11\,520\,f\,w\,x^3\,\eta^{10}}{(-1+w(-1+\eta))^3(x+\eta-x\eta)^3(w+x+\eta-w\eta-x\eta)^3} -
\end{aligned}$$



$$\begin{aligned}
& \frac{5680 f w^2 x^3 \eta^{10}}{(-1+w(-1+\eta))^3 (x+\eta-x\eta)^3 (w+x+\eta-w\eta-x\eta)^3} - \\
& \frac{19440 f w^3 x^3 \eta^{10}}{(-1+w(-1+\eta))^3 (x+\eta-x\eta)^3 (w+x+\eta-w\eta-x\eta)^3} + \\
& \frac{13848 f w^4 x^3 \eta^{10}}{(-1+w(-1+\eta))^3 (x+\eta-x\eta)^3 (w+x+\eta-w\eta-x\eta)^3} - \\
& \frac{1540 f w^5 x^3 \eta^{10}}{(-1+w(-1+\eta))^3 (x+\eta-x\eta)^3 (w+x+\eta-w\eta-x\eta)^3} - \\
& \frac{9720 f w x^4 \eta^{10}}{(-1+w(-1+\eta))^3 (x+\eta-x\eta)^3 (w+x+\eta-w\eta-x\eta)^3} - \\
& \frac{3240 f w^2 x^4 \eta^{10}}{(-1+w(-1+\eta))^3 (x+\eta-x\eta)^3 (w+x+\eta-w\eta-x\eta)^3} + \\
& \frac{15924 f w^3 x^4 \eta^{10}}{(-1+w(-1+\eta))^3 (x+\eta-x\eta)^3 (w+x+\eta-w\eta-x\eta)^3} - \\
& \frac{4620 f w^4 x^4 \eta^{10}}{(-1+w(-1+\eta))^3 (x+\eta-x\eta)^3 (w+x+\eta-w\eta-x\eta)^3} + \\
& \frac{4320 f w x^5 \eta^{10}}{(-1+w(-1+\eta))^3 (x+\eta-x\eta)^3 (w+x+\eta-w\eta-x\eta)^3} + \\
& \frac{4944 f w^2 x^5 \eta^{10}}{(-1+w(-1+\eta))^3 (x+\eta-x\eta)^3 (w+x+\eta-w\eta-x\eta)^3} - \\
& \frac{4620 f w^3 x^5 \eta^{10}}{(-1+w(-1+\eta))^3 (x+\eta-x\eta)^3 (w+x+\eta-w\eta-x\eta)^3} - \\
& \frac{792 f w x^6 \eta^{10}}{(-1+w(-1+\eta))^3 (x+\eta-x\eta)^3 (w+x+\eta-w\eta-x\eta)^3} - \\
& \frac{1540 f w^2 x^6 \eta^{10}}{(-1+w(-1+\eta))^3 (x+\eta-x\eta)^3 (w+x+\eta-w\eta-x\eta)^3} + \\
& \frac{72 f w \eta^{11}}{(-1+w(-1+\eta))^3 (x+\eta-x\eta)^3 (w+x+\eta-w\eta-x\eta)^3} - \\
& \frac{76 f w^2 \eta^{11}}{(-1+w(-1+\eta))^3 (x+\eta-x\eta)^3 (w+x+\eta-w\eta-x\eta)^3} - \\
& \frac{312 f w^3 \eta^{11}}{(-1+w(-1+\eta))^3 (x+\eta-x\eta)^3 (w+x+\eta-w\eta-x\eta)^3} + \\
& \frac{564 f w^4 \eta^{11}}{(-1+w(-1+\eta))^3 (x+\eta-x\eta)^3 (w+x+\eta-w\eta-x\eta)^3} - \\
& \frac{248 f w^5 \eta^{11}}{(-1+w(-1+\eta))^3 (x+\eta-x\eta)^3 (w+x+\eta-w\eta-x\eta)^3} - \\
& \frac{432 f w x \eta^{11}}{(-1+w(-1+\eta))^3 (x+\eta-x\eta)^3 (w+x+\eta-w\eta-x\eta)^3} +
\end{aligned}$$

$$\begin{aligned}
& \frac{24 f w^2 x \eta^{11}}{(-1+w(-1+\eta))^3 (x+\eta-x\eta)^3 (w+x+\eta-w\eta-x\eta)^3} + \\
& \frac{2316 f w^3 x \eta^{11}}{(-1+w(-1+\eta))^3 (x+\eta-x\eta)^3 (w+x+\eta-w\eta-x\eta)^3} - \\
& \frac{2760 f w^4 x \eta^{11}}{(-1+w(-1+\eta))^3 (x+\eta-x\eta)^3 (w+x+\eta-w\eta-x\eta)^3} + \\
& \frac{852 f w^5 x \eta^{11}}{(-1+w(-1+\eta))^3 (x+\eta-x\eta)^3 (w+x+\eta-w\eta-x\eta)^3} + \\
& \frac{1080 f w x^2 \eta^{11}}{(-1+w(-1+\eta))^3 (x+\eta-x\eta)^3 (w+x+\eta-w\eta-x\eta)^3} + \\
& \frac{1020 f w^2 x^2 \eta^{11}}{(-1+w(-1+\eta))^3 (x+\eta-x\eta)^3 (w+x+\eta-w\eta-x\eta)^3} - \\
& \frac{6144 f w^3 x^2 \eta^{11}}{(-1+w(-1+\eta))^3 (x+\eta-x\eta)^3 (w+x+\eta-w\eta-x\eta)^3} + \\
& \frac{4896 f w^4 x^2 \eta^{11}}{(-1+w(-1+\eta))^3 (x+\eta-x\eta)^3 (w+x+\eta-w\eta-x\eta)^3} - \\
& \frac{960 f w^5 x^2 \eta^{11}}{(-1+w(-1+\eta))^3 (x+\eta-x\eta)^3 (w+x+\eta-w\eta-x\eta)^3} - \\
& \frac{1440 f w x^3 \eta^{11}}{(-1+w(-1+\eta))^3 (x+\eta-x\eta)^3 (w+x+\eta-w\eta-x\eta)^3} - \\
& \frac{2800 f w^2 x^3 \eta^{11}}{(-1+w(-1+\eta))^3 (x+\eta-x\eta)^3 (w+x+\eta-w\eta-x\eta)^3} + \\
& \frac{7656 f w^3 x^3 \eta^{11}}{(-1+w(-1+\eta))^3 (x+\eta-x\eta)^3 (w+x+\eta-w\eta-x\eta)^3} - \\
& \frac{3768 f w^4 x^3 \eta^{11}}{(-1+w(-1+\eta))^3 (x+\eta-x\eta)^3 (w+x+\eta-w\eta-x\eta)^3} + \\
& \frac{356 f w^5 x^3 \eta^{11}}{(-1+w(-1+\eta))^3 (x+\eta-x\eta)^3 (w+x+\eta-w\eta-x\eta)^3} + \\
& \frac{1080 f w x^4 \eta^{11}}{(-1+w(-1+\eta))^3 (x+\eta-x\eta)^3 (w+x+\eta-w\eta-x\eta)^3} + \\
& \frac{3180 f w^2 x^4 \eta^{11}}{(-1+w(-1+\eta))^3 (x+\eta-x\eta)^3 (w+x+\eta-w\eta-x\eta)^3} - \\
& \frac{4584 f w^3 x^4 \eta^{11}}{(-1+w(-1+\eta))^3 (x+\eta-x\eta)^3 (w+x+\eta-w\eta-x\eta)^3} + \\
& \frac{1068 f w^4 x^4 \eta^{11}}{(-1+w(-1+\eta))^3 (x+\eta-x\eta)^3 (w+x+\eta-w\eta-x\eta)^3} - \\
& \frac{432 f w x^5 \eta^{11}}{(-1+w(-1+\eta))^3 (x+\eta-x\eta)^3 (w+x+\eta-w\eta-x\eta)^3} -
\end{aligned}$$

$$\begin{aligned}
& \frac{1704 f w^2 x^5 \eta^{11}}{(-1+w(-1+\eta))^3 (x+\eta-x\eta)^3 (w+x+\eta-w\eta-x\eta)^3} + \\
& \frac{1068 f w^3 x^5 \eta^{11}}{(-1+w(-1+\eta))^3 (x+\eta-x\eta)^3 (w+x+\eta-w\eta-x\eta)^3} + \\
& \frac{72 f w x^6 \eta^{11}}{(-1+w(-1+\eta))^3 (x+\eta-x\eta)^3 (w+x+\eta-w\eta-x\eta)^3} + \\
& \frac{356 f w^2 x^6 \eta^{11}}{(-1+w(-1+\eta))^3 (x+\eta-x\eta)^3 (w+x+\eta-w\eta-x\eta)^3} - \\
& \frac{36 f w^2 \eta^{12}}{(-1+w(-1+\eta))^3 (x+\eta-x\eta)^3 (w+x+\eta-w\eta-x\eta)^3} + \\
& \frac{108 f w^3 \eta^{12}}{(-1+w(-1+\eta))^3 (x+\eta-x\eta)^3 (w+x+\eta-w\eta-x\eta)^3} - \\
& \frac{108 f w^4 \eta^{12}}{(-1+w(-1+\eta))^3 (x+\eta-x\eta)^3 (w+x+\eta-w\eta-x\eta)^3} + \\
& \frac{36 f w^5 \eta^{12}}{(-1+w(-1+\eta))^3 (x+\eta-x\eta)^3 (w+x+\eta-w\eta-x\eta)^3} + \\
& \frac{216 f w^2 x \eta^{12}}{(-1+w(-1+\eta))^3 (x+\eta-x\eta)^3 (w+x+\eta-w\eta-x\eta)^3} - \\
& \frac{540 f w^3 x \eta^{12}}{(-1+w(-1+\eta))^3 (x+\eta-x\eta)^3 (w+x+\eta-w\eta-x\eta)^3} + \\
& \frac{432 f w^4 x \eta^{12}}{(-1+w(-1+\eta))^3 (x+\eta-x\eta)^3 (w+x+\eta-w\eta-x\eta)^3} - \\
& \frac{108 f w^5 x \eta^{12}}{(-1+w(-1+\eta))^3 (x+\eta-x\eta)^3 (w+x+\eta-w\eta-x\eta)^3} - \\
& \frac{540 f w^2 x^2 \eta^{12}}{(-1+w(-1+\eta))^3 (x+\eta-x\eta)^3 (w+x+\eta-w\eta-x\eta)^3} + \\
& \frac{1080 f w^3 x^2 \eta^{12}}{(-1+w(-1+\eta))^3 (x+\eta-x\eta)^3 (w+x+\eta-w\eta-x\eta)^3} - \\
& \frac{648 f w^4 x^2 \eta^{12}}{(-1+w(-1+\eta))^3 (x+\eta-x\eta)^3 (w+x+\eta-w\eta-x\eta)^3} + \\
& \frac{108 f w^5 x^2 \eta^{12}}{(-1+w(-1+\eta))^3 (x+\eta-x\eta)^3 (w+x+\eta-w\eta-x\eta)^3} + \\
& \frac{720 f w^2 x^3 \eta^{12}}{(-1+w(-1+\eta))^3 (x+\eta-x\eta)^3 (w+x+\eta-w\eta-x\eta)^3} - \\
& \frac{1080 f w^3 x^3 \eta^{12}}{(-1+w(-1+\eta))^3 (x+\eta-x\eta)^3 (w+x+\eta-w\eta-x\eta)^3} + \\
& \frac{432 f w^4 x^3 \eta^{12}}{(-1+w(-1+\eta))^3 (x+\eta-x\eta)^3 (w+x+\eta-w\eta-x\eta)^3} -
\end{aligned}$$

$$\begin{aligned}
& \frac{36 f w^5 x^3 \eta^{12}}{(-1+w(-1+\eta))^3 (x+\eta-x\eta)^3 (w+x+\eta-w\eta-x\eta)^3} - \\
& \frac{540 f w^2 x^4 \eta^{12}}{(-1+w(-1+\eta))^3 (x+\eta-x\eta)^3 (w+x+\eta-w\eta-x\eta)^3} + \\
& \frac{540 f w^3 x^4 \eta^{12}}{(-1+w(-1+\eta))^3 (x+\eta-x\eta)^3 (w+x+\eta-w\eta-x\eta)^3} - \\
& \frac{108 f w^4 x^4 \eta^{12}}{(-1+w(-1+\eta))^3 (x+\eta-x\eta)^3 (w+x+\eta-w\eta-x\eta)^3} + \\
& \frac{216 f w^2 x^5 \eta^{12}}{(-1+w(-1+\eta))^3 (x+\eta-x\eta)^3 (w+x+\eta-w\eta-x\eta)^3} - \\
& \frac{108 f w^3 x^5 \eta^{12}}{(-1+w(-1+\eta))^3 (x+\eta-x\eta)^3 (w+x+\eta-w\eta-x\eta)^3} - \\
& \frac{36 f w^2 x^6 \eta^{12}}{(-1+w(-1+\eta))^3 (x+\eta-x\eta)^3 (w+x+\eta-w\eta-x\eta)^3} + \\
& \frac{72 f w}{(x(-1+\eta)-\eta)(w+x+\eta-w\eta-x\eta)^2} + \frac{216 f w \eta^2}{(x(-1+\eta)-\eta)(w+x+\eta-w\eta-x\eta)^2} - \\
& \frac{80 c \sigma^2 w}{(1+w-w\eta)^2 (w+x+\eta-w\eta-x\eta)^2} - \frac{224 c \sigma^2 w^2}{(1+w-w\eta)^2 (w+x+\eta-w\eta-x\eta)^2} - \\
& \frac{144 c \sigma^2 w^3}{(1+w-w\eta)^2 (w+x+\eta-w\eta-x\eta)^2} - \frac{80 c \sigma^2 x}{(1+w-w\eta)^2 (w+x+\eta-w\eta-x\eta)^2} - \\
& \frac{288 c \sigma^2 w x}{(1+w-w\eta)^2 (w+x+\eta-w\eta-x\eta)^2} - \frac{208 c \sigma^2 w^2 x}{(1+w-w\eta)^2 (w+x+\eta-w\eta-x\eta)^2} - \\
& \frac{64 c \sigma^2 x^2}{(1+w-w\eta)^2 (w+x+\eta-w\eta-x\eta)^2} - \frac{64 c \sigma^2 w x^2}{(1+w-w\eta)^2 (w+x+\eta-w\eta-x\eta)^2} - \\
& \frac{80 c \sigma^2 \eta}{(1+w-w\eta)^2 (w+x+\eta-w\eta-x\eta)^2} - \frac{128 c \sigma^2 w \eta}{(1+w-w\eta)^2 (w+x+\eta-w\eta-x\eta)^2} + \\
& \frac{464 c \sigma^2 w^2 \eta}{(1+w-w\eta)^2 (w+x+\eta-w\eta-x\eta)^2} + \frac{576 c \sigma^2 w^3 \eta}{(1+w-w\eta)^2 (w+x+\eta-w\eta-x\eta)^2} + \\
& \frac{32 c \sigma^2 x \eta}{(1+w-w\eta)^2 (w+x+\eta-w\eta-x\eta)^2} + \frac{736 c \sigma^2 w x \eta}{(1+w-w\eta)^2 (w+x+\eta-w\eta-x\eta)^2} + \\
& \frac{832 c \sigma^2 w^2 x \eta}{(1+w-w\eta)^2 (w+x+\eta-w\eta-x\eta)^2} + \frac{192 c \sigma^2 x^2 \eta}{(1+w-w\eta)^2 (w+x+\eta-w\eta-x\eta)^2} + \\
& \frac{256 c \sigma^2 w x^2 \eta}{(1+w-w\eta)^2 (w+x+\eta-w\eta-x\eta)^2} + \frac{16 c \sigma^2 \eta^2}{(1+w-w\eta)^2 (w+x+\eta-w\eta-x\eta)^2} + \\
& \frac{432 c \sigma^2 w \eta^2}{(1+w-w\eta)^2 (w+x+\eta-w\eta-x\eta)^2} - \frac{48 c \sigma^2 w^2 \eta^2}{(1+w-w\eta)^2 (w+x+\eta-w\eta-x\eta)^2} - \\
& \frac{864 c \sigma^2 w^3 \eta^2}{(1+w-w\eta)^2 (w+x+\eta-w\eta-x\eta)^2} + \frac{176 c \sigma^2 x \eta^2}{(1+w-w\eta)^2 (w+x+\eta-w\eta-x\eta)^2} -
\end{aligned}$$

$$\begin{aligned}
& \frac{480 c \sigma^2 w x \eta^2}{(1+w-w \eta)^2 (w+x+\eta-w \eta-x \eta)^2} - \frac{1248 c \sigma^2 w^2 x \eta^2}{(1+w-w \eta)^2 (w+x+\eta-w \eta-x \eta)^2} - \\
& \frac{192 c \sigma^2 x^2 \eta^2}{(1+w-w \eta)^2 (w+x+\eta-w \eta-x \eta)^2} - \frac{384 c \sigma^2 w x^2 \eta^2}{(1+w-w \eta)^2 (w+x+\eta-w \eta-x \eta)^2} + \\
& \frac{64 c \sigma^2 \eta^3}{(1+w-w \eta)^2 (w+x+\eta-w \eta-x \eta)^2} - \frac{160 c \sigma^2 w \eta^3}{(1+w-w \eta)^2 (w+x+\eta-w \eta-x \eta)^2} - \\
& \frac{400 c \sigma^2 w^2 \eta^3}{(1+w-w \eta)^2 (w+x+\eta-w \eta-x \eta)^2} + \frac{576 c \sigma^2 w^3 \eta^3}{(1+w-w \eta)^2 (w+x+\eta-w \eta-x \eta)^2} - \\
& \frac{128 c \sigma^2 x \eta^3}{(1+w-w \eta)^2 (w+x+\eta-w \eta-x \eta)^2} - \frac{96 c \sigma^2 w x \eta^3}{(1+w-w \eta)^2 (w+x+\eta-w \eta-x \eta)^2} + \\
& \frac{832 c \sigma^2 w^2 x \eta^3}{(1+w-w \eta)^2 (w+x+\eta-w \eta-x \eta)^2} + \frac{64 c \sigma^2 x^2 \eta^3}{(1+w-w \eta)^2 (w+x+\eta-w \eta-x \eta)^2} + \\
& \frac{256 c \sigma^2 w x^2 \eta^3}{(1+w-w \eta)^2 (w+x+\eta-w \eta-x \eta)^2} - \frac{64 c \sigma^2 w \eta^4}{(1+w-w \eta)^2 (w+x+\eta-w \eta-x \eta)^2} + \\
& \frac{208 c \sigma^2 w^2 \eta^4}{(1+w-w \eta)^2 (w+x+\eta-w \eta-x \eta)^2} - \frac{144 c \sigma^2 w^3 \eta^4}{(1+w-w \eta)^2 (w+x+\eta-w \eta-x \eta)^2} + \\
& \frac{128 c \sigma^2 w x \eta^4}{(1+w-w \eta)^2 (w+x+\eta-w \eta-x \eta)^2} - \frac{208 c \sigma^2 w^2 x \eta^4}{(1+w-w \eta)^2 (w+x+\eta-w \eta-x \eta)^2} - \\
& \frac{64 c \sigma^2 w x^2 \eta^4}{(1+w-w \eta)^2 (w+x+\eta-w \eta-x \eta)^2} + \frac{12 f x^2}{(x+\eta-x \eta)^2 (w+x+\eta-w \eta-x \eta)^2} - \\
& \frac{48 f x^2 \eta}{(x+\eta-x \eta)^2 (w+x+\eta-w \eta-x \eta)^2} + \frac{72 f x^2 \eta^2}{(x+\eta-x \eta)^2 (w+x+\eta-w \eta-x \eta)^2} - \\
& \frac{48 f x^2 \eta^3}{(x+\eta-x \eta)^2 (w+x+\eta-w \eta-x \eta)^2} + \frac{12 f x^2 \eta^4}{(x+\eta-x \eta)^2 (w+x+\eta-w \eta-x \eta)^2} - \\
& \frac{4 f w}{(x+\eta-x \eta) (w+x+\eta-w \eta-x \eta)^2} + \frac{4 f x}{(x+\eta-x \eta) (w+x+\eta-w \eta-x \eta)^2} + \\
& \frac{228 f w \eta}{(x+\eta-x \eta) (w+x+\eta-w \eta-x \eta)^2} - \frac{12 f x \eta}{(x+\eta-x \eta) (w+x+\eta-w \eta-x \eta)^2} - \\
& \frac{12 f w \eta^2}{(x+\eta-x \eta) (w+x+\eta-w \eta-x \eta)^2} + \frac{12 f x \eta^2}{(x+\eta-x \eta) (w+x+\eta-w \eta-x \eta)^2} + \\
& \frac{76 f w \eta^3}{(x+\eta-x \eta) (w+x+\eta-w \eta-x \eta)^2} - \frac{4 f x \eta^3}{(x+\eta-x \eta) (w+x+\eta-w \eta-x \eta)^2} - \\
& \frac{6 f x^2}{(x+\eta-x \eta)^3 (w+x+\eta-w \eta-x \eta)} + \frac{24 f x^2 \eta}{(x+\eta-x \eta)^3 (w+x+\eta-w \eta-x \eta)} - \\
& \frac{36 f x^2 \eta^2}{(x+\eta-x \eta)^3 (w+x+\eta-w \eta-x \eta)} + \frac{24 f x^2 \eta^3}{(x+\eta-x \eta)^3 (w+x+\eta-w \eta-x \eta)} - \\
& \frac{6 f x^2 \eta^4}{(x+\eta-x \eta)^3 (w+x+\eta-w \eta-x \eta)} + \frac{42 f}{(x+\eta-x \eta) (w+x+\eta-w \eta-x \eta)} -
\end{aligned}$$

$$\begin{aligned}
& \frac{84 f \eta}{(x + \eta - x \eta) (w + x + \eta - w \eta - x \eta)} + \frac{42 f \eta^2}{(x + \eta - x \eta) (w + x + \eta - w \eta - x \eta)} + \\
& \frac{80 c \sigma^2 \eta}{(1 + w - w \eta) (x + \eta - x \eta) (w + x + \eta - w \eta - x \eta)} + \\
& \frac{120 c \sigma^2 w \eta}{(1 + w - w \eta) (x + \eta - x \eta) (w + x + \eta - w \eta - x \eta)} + \\
& \frac{40 c \sigma^2 w \eta^3}{(1 + w - w \eta) (x + \eta - x \eta) (w + x + \eta - w \eta - x \eta)} + \\
& \frac{84 f \eta}{(x + \eta - x \eta) (w + x + \eta - w \eta - x \eta) (1 - \eta t)} - \frac{4 f}{(-1 + w (-1 + \eta))^3 (-1 + \eta t)} + \\
& \frac{256 f w}{(-1 + w (-1 + \eta))^3 (-1 + \eta t)} - \frac{12 f w^2}{(-1 + w (-1 + \eta))^3 (-1 + \eta t)} + \\
& \frac{48 f}{(-1 + w (-1 + \eta)) \times (-1 + \eta t)} + \frac{42 f}{(x (-1 + \eta) - \eta) (w (-1 + \eta) + x (-1 + \eta) - \eta) (-1 + \eta t)} + \\
& \frac{40 c \sigma^2}{(-1 + w (-1 + \eta)) (x (-1 + \eta) - \eta) (w (-1 + \eta) + x (-1 + \eta) - \eta) (-1 + \eta t)} + \\
& \frac{40 c \sigma^2 w}{(-1 + w (-1 + \eta)) (x (-1 + \eta) - \eta) (w (-1 + \eta) + x (-1 + \eta) - \eta) (-1 + \eta t)} + \\
& \frac{32 c \sigma^2 w x}{(-1 + w (-1 + \eta)) (x (-1 + \eta) - \eta) (w (-1 + \eta) + x (-1 + \eta) - \eta) (-1 + \eta t)} + \\
& \frac{32 c \sigma^2 x^2}{(-1 + w (-1 + \eta)) (x (-1 + \eta) - \eta) (w (-1 + \eta) + x (-1 + \eta) - \eta) (-1 + \eta t)} + \\
& \frac{88 f \eta}{(-1 + w (-1 + \eta))^3 (-1 + \eta t)} - \frac{996 f w \eta}{(-1 + w (-1 + \eta))^3 (-1 + \eta t)} + \\
& \frac{48 f w^2 \eta}{(-1 + w (-1 + \eta))^3 (-1 + \eta t)} - \frac{96 f \eta}{(-1 + w (-1 + \eta)) \times (-1 + \eta t)} + \\
& \frac{24 f x^2 \eta}{(x (-1 + \eta) - \eta)^3 (w (-1 + \eta) + x (-1 + \eta) - \eta) (-1 + \eta t)} - \\
& \frac{80 c \sigma^2 \eta}{(-1 + w (-1 + \eta)) (x (-1 + \eta) - \eta) (w (-1 + \eta) + x (-1 + \eta) - \eta) (-1 + \eta t)} - \\
& \frac{88 c \sigma^2 w \eta}{(-1 + w (-1 + \eta)) (x (-1 + \eta) - \eta) (w (-1 + \eta) + x (-1 + \eta) - \eta) (-1 + \eta t)} + \\
& \frac{64 c \sigma^2 x \eta}{(-1 + w (-1 + \eta)) (x (-1 + \eta) - \eta) (w (-1 + \eta) + x (-1 + \eta) - \eta) (-1 + \eta t)} - \\
& \frac{128 c \sigma^2 w x \eta}{(-1 + w (-1 + \eta)) (x (-1 + \eta) - \eta) (w (-1 + \eta) + x (-1 + \eta) - \eta) (-1 + \eta t)} - \\
& \frac{128 c \sigma^2 x^2 \eta}{(-1 + w (-1 + \eta)) (x (-1 + \eta) - \eta) (w (-1 + \eta) + x (-1 + \eta) - \eta) (-1 + \eta t)} - \\
& \frac{240 f \eta^2}{(-1 + w (-1 + \eta))^3 (-1 + \eta t)} + \frac{1452 f w \eta^2}{(-1 + w (-1 + \eta))^3 (-1 + \eta t)} -
\end{aligned}$$

$$\begin{aligned}
& \frac{72 f w^2 \eta^2}{(-1+w(-1+\eta))^3 (-1+\eta t)} + \frac{44 f \eta^2}{(-1+w(-1+\eta)) \times (-1+\eta t)} + \\
& \frac{42 f \eta^2}{(x(-1+\eta) - \eta) (w(-1+\eta) + x(-1+\eta) - \eta) (-1+\eta t)} + \\
& \frac{72 c \sigma^2 \eta^2}{(-1+w(-1+\eta)) (x(-1+\eta) - \eta) (w(-1+\eta) + x(-1+\eta) - \eta) (-1+\eta t)} + \\
& \frac{24 c \sigma^2 w \eta^2}{(-1+w(-1+\eta)) (x(-1+\eta) - \eta) (w(-1+\eta) + x(-1+\eta) - \eta) (-1+\eta t)} - \\
& \frac{192 c \sigma^2 x \eta^2}{(-1+w(-1+\eta)) (x(-1+\eta) - \eta) (w(-1+\eta) + x(-1+\eta) - \eta) (-1+\eta t)} + \\
& \frac{192 c \sigma^2 w x \eta^2}{(-1+w(-1+\eta)) (x(-1+\eta) - \eta) (w(-1+\eta) + x(-1+\eta) - \eta) (-1+\eta t)} + \\
& \frac{192 c \sigma^2 x^2 \eta^2}{(-1+w(-1+\eta)) (x(-1+\eta) - \eta) (w(-1+\eta) + x(-1+\eta) - \eta) (-1+\eta t)} + \\
& \frac{232 f \eta^3}{(-1+w(-1+\eta))^3 (-1+\eta t)} - \frac{940 f w \eta^3}{(-1+w(-1+\eta))^3 (-1+\eta t)} + \\
& \frac{48 f w^2 \eta^3}{(-1+w(-1+\eta))^3 (-1+\eta t)} + \frac{8 f \eta^3}{(-1+w(-1+\eta)) \times (-1+\eta t)} + \\
& \frac{24 f x^2 \eta^3}{(x(-1+\eta) - \eta)^3 (w(-1+\eta) + x(-1+\eta) - \eta) (-1+\eta t)} - \\
& \frac{64 c \sigma^2 \eta^3}{(-1+w(-1+\eta)) (x(-1+\eta) - \eta) (w(-1+\eta) + x(-1+\eta) - \eta) (-1+\eta t)} + \\
& \frac{56 c \sigma^2 w \eta^3}{(-1+w(-1+\eta)) (x(-1+\eta) - \eta) (w(-1+\eta) + x(-1+\eta) - \eta) (-1+\eta t)} + \\
& \frac{192 c \sigma^2 x \eta^3}{(-1+w(-1+\eta)) (x(-1+\eta) - \eta) (w(-1+\eta) + x(-1+\eta) - \eta) (-1+\eta t)} - \\
& \frac{128 c \sigma^2 w x \eta^3}{(-1+w(-1+\eta)) (x(-1+\eta) - \eta) (w(-1+\eta) + x(-1+\eta) - \eta) (-1+\eta t)} - \\
& \frac{128 c \sigma^2 x^2 \eta^3}{(-1+w(-1+\eta)) (x(-1+\eta) - \eta) (w(-1+\eta) + x(-1+\eta) - \eta) (-1+\eta t)} - \\
& \frac{76 f \eta^4}{(-1+w(-1+\eta))^3 (-1+\eta t)} + \frac{228 f w \eta^4}{(-1+w(-1+\eta))^3 (-1+\eta t)} - \\
& \frac{12 f w^2 \eta^4}{(-1+w(-1+\eta))^3 (-1+\eta t)} - \frac{4 f \eta^4}{(-1+w(-1+\eta)) \times (-1+\eta t)} + \\
& \frac{32 c \sigma^2 \eta^4}{(-1+w(-1+\eta)) (x(-1+\eta) - \eta) (w(-1+\eta) + x(-1+\eta) - \eta) (-1+\eta t)} - \\
& \frac{32 c \sigma^2 w \eta^4}{(-1+w(-1+\eta)) (x(-1+\eta) - \eta) (w(-1+\eta) + x(-1+\eta) - \eta) (-1+\eta t)} -
\end{aligned}$$

$$\begin{aligned}
& \frac{64 c \sigma^2 x \eta^4}{(-1+w(-1+\eta))(x(-1+\eta)-\eta)(w(-1+\eta)+x(-1+\eta)-\eta)(-1+\eta t)} + \\
& \frac{32 c \sigma^2 w x \eta^4}{(-1+w(-1+\eta))(x(-1+\eta)-\eta)(w(-1+\eta)+x(-1+\eta)-\eta)(-1+\eta t)} + \\
& \frac{32 c \sigma^2 x^2 \eta^4}{(-1+w(-1+\eta))(x(-1+\eta)-\eta)(w(-1+\eta)+x(-1+\eta)-\eta)(-1+\eta t)} + \\
& \frac{32 f}{(1+w-w \eta)^2(-1+\eta t)} - \frac{48 f w}{(1+w-w \eta)^2(-1+\eta t)} - \frac{136 f \eta}{(1+w-w \eta)^2(-1+\eta t)} + \\
& \frac{144 f w \eta}{(1+w-w \eta)^2(-1+\eta t)} + \frac{216 f \eta^2}{(1+w-w \eta)^2(-1+\eta t)} - \frac{144 f w \eta^2}{(1+w-w \eta)^2(-1+\eta t)} - \\
& \frac{152 f \eta^3}{(1+w-w \eta)^2(-1+\eta t)} + \frac{48 f w \eta^3}{(1+w-w \eta)^2(-1+\eta t)} + \frac{40 f \eta^4}{(1+w-w \eta)^2(-1+\eta t)} - \\
& \frac{4 f x}{(w(-1+\eta)+x(-1+\eta)-\eta)(x+\eta-x \eta)^2(-1+\eta t)} + \\
& \frac{12 f x \eta}{(w(-1+\eta)+x(-1+\eta)-\eta)(x+\eta-x \eta)^2(-1+\eta t)} - \\
& \frac{12 f x \eta^2}{(w(-1+\eta)+x(-1+\eta)-\eta)(x+\eta-x \eta)^2(-1+\eta t)} + \\
& \frac{4 f x \eta^3}{(w(-1+\eta)+x(-1+\eta)-\eta)(x+\eta-x \eta)^2(-1+\eta t)} + \\
& \frac{6 f w^2}{(x(-1+\eta)-\eta)(w+x+\eta-w \eta-x \eta)^3(-1+\eta t)} + \\
& \frac{6 f x^2}{(x(-1+\eta)-\eta)(w+x+\eta-w \eta-x \eta)^3(-1+\eta t)} + \\
& \frac{18 f w \eta}{(x(-1+\eta)-\eta)(w+x+\eta-w \eta-x \eta)^3(-1+\eta t)} - \\
& \frac{24 f w^2 \eta}{(x(-1+\eta)-\eta)(w+x+\eta-w \eta-x \eta)^3(-1+\eta t)} - \\
& \frac{24 f x^2 \eta}{(x(-1+\eta)-\eta)(w+x+\eta-w \eta-x \eta)^3(-1+\eta t)} - \\
& \frac{54 f w \eta^2}{(x(-1+\eta)-\eta)(w+x+\eta-w \eta-x \eta)^3(-1+\eta t)} + \\
& \frac{36 f w^2 \eta^2}{(x(-1+\eta)-\eta)(w+x+\eta-w \eta-x \eta)^3(-1+\eta t)} + \\
& \frac{36 f x^2 \eta^2}{(x(-1+\eta)-\eta)(w+x+\eta-w \eta-x \eta)^3(-1+\eta t)} + \\
& \frac{54 f w \eta^3}{(x(-1+\eta)-\eta)(w+x+\eta-w \eta-x \eta)^3(-1+\eta t)} -
\end{aligned}$$



$$\begin{aligned}
& \frac{24 f w^2 \eta^3}{(x(-1+\eta)-\eta)(w+x+\eta-w\eta-x\eta)^3(-1+\eta t)} - \\
& \frac{24 f x^2 \eta^3}{(x(-1+\eta)-\eta)(w+x+\eta-w\eta-x\eta)^3(-1+\eta t)} - \\
& \frac{18 f w \eta^4}{(x(-1+\eta)-\eta)(w+x+\eta-w\eta-x\eta)^3(-1+\eta t)} + \\
& \frac{6 f w^2 \eta^4}{(x(-1+\eta)-\eta)(w+x+\eta-w\eta-x\eta)^3(-1+\eta t)} + \\
& \frac{6 f x^2 \eta^4}{(x(-1+\eta)-\eta)(w+x+\eta-w\eta-x\eta)^3(-1+\eta t)} + \\
& \frac{72 f x}{(x+\eta-x\eta)^3(w+x+\eta-w\eta-x\eta)^3(-1+\eta t)} - \\
& \frac{36 f w x}{(x+\eta-x\eta)^3(w+x+\eta-w\eta-x\eta)^3(-1+\eta t)} - \\
& \frac{72 f x^2}{(x+\eta-x\eta)^3(w+x+\eta-w\eta-x\eta)^3(-1+\eta t)} - \\
& \frac{12 f w^2 x^2}{(x+\eta-x\eta)^3(w+x+\eta-w\eta-x\eta)^3(-1+\eta t)} - \\
& \frac{72 f w x^3}{(x+\eta-x\eta)^3(w+x+\eta-w\eta-x\eta)^3(-1+\eta t)} + \\
& \frac{72 f x}{(-1+w(-1+\eta))^3(x+\eta-x\eta)^3(w+x+\eta-w\eta-x\eta)^3(-1+\eta t)} + \\
& \frac{180 f w x}{(-1+w(-1+\eta))^3(x+\eta-x\eta)^3(w+x+\eta-w\eta-x\eta)^3(-1+\eta t)} + \\
& \frac{108 f w^2 x}{(-1+w(-1+\eta))^3(x+\eta-x\eta)^3(w+x+\eta-w\eta-x\eta)^3(-1+\eta t)} - \\
& \frac{36 f w^3 x}{(-1+w(-1+\eta))^3(x+\eta-x\eta)^3(w+x+\eta-w\eta-x\eta)^3(-1+\eta t)} - \\
& \frac{36 f w^4 x}{(-1+w(-1+\eta))^3(x+\eta-x\eta)^3(w+x+\eta-w\eta-x\eta)^3(-1+\eta t)} - \\
& \frac{72 f x^2}{(-1+w(-1+\eta))^3(x+\eta-x\eta)^3(w+x+\eta-w\eta-x\eta)^3(-1+\eta t)} - \\
& \frac{216 f w x^2}{(-1+w(-1+\eta))^3(x+\eta-x\eta)^3(w+x+\eta-w\eta-x\eta)^3(-1+\eta t)} - \\
& \frac{216 f w^2 x^2}{(-1+w(-1+\eta))^3(x+\eta-x\eta)^3(w+x+\eta-w\eta-x\eta)^3(-1+\eta t)} - \\
& \frac{72 f w^3 x^2}{(-1+w(-1+\eta))^3(x+\eta-x\eta)^3(w+x+\eta-w\eta-x\eta)^3(-1+\eta t)} -
\end{aligned}$$

$$\begin{aligned}
& \frac{72 f w^4 x^3}{(-1+w(-1+\eta))^3 (x+\eta-x\eta)^3 (w+x+\eta-w\eta-x\eta)^3 (-1+\eta t)} + \\
& \frac{40 f w^5 x^3}{(-1+w(-1+\eta))^3 (x+\eta-x\eta)^3 (w+x+\eta-w\eta-x\eta)^3 (-1+\eta t)} - \\
& \frac{216 f w^3 x^4}{(-1+w(-1+\eta))^3 (x+\eta-x\eta)^3 (w+x+\eta-w\eta-x\eta)^3 (-1+\eta t)} + \\
& \frac{120 f w^4 x^4}{(-1+w(-1+\eta))^3 (x+\eta-x\eta)^3 (w+x+\eta-w\eta-x\eta)^3 (-1+\eta t)} - \\
& \frac{216 f w^2 x^5}{(-1+w(-1+\eta))^3 (x+\eta-x\eta)^3 (w+x+\eta-w\eta-x\eta)^3 (-1+\eta t)} + \\
& \frac{120 f w^3 x^5}{(-1+w(-1+\eta))^3 (x+\eta-x\eta)^3 (w+x+\eta-w\eta-x\eta)^3 (-1+\eta t)} - \\
& \frac{72 f w x^6}{(-1+w(-1+\eta))^3 (x+\eta-x\eta)^3 (w+x+\eta-w\eta-x\eta)^3 (-1+\eta t)} + \\
& \frac{40 f w^2 x^6}{(-1+w(-1+\eta))^3 (x+\eta-x\eta)^3 (w+x+\eta-w\eta-x\eta)^3 (-1+\eta t)} - \\
& \frac{324 f x \eta}{(x+\eta-x\eta)^3 (w+x+\eta-w\eta-x\eta)^3 (-1+\eta t)} + \\
& \frac{144 f w x \eta}{(x+\eta-x\eta)^3 (w+x+\eta-w\eta-x\eta)^3 (-1+\eta t)} - \\
& \frac{12 f w^2 x \eta}{(x+\eta-x\eta)^3 (w+x+\eta-w\eta-x\eta)^3 (-1+\eta t)} + \\
& \frac{288 f x^2 \eta}{(x+\eta-x\eta)^3 (w+x+\eta-w\eta-x\eta)^3 (-1+\eta t)} - \\
& \frac{144 f w x^2 \eta}{(x+\eta-x\eta)^3 (w+x+\eta-w\eta-x\eta)^3 (-1+\eta t)} + \\
& \frac{72 f w^2 x^2 \eta}{(x+\eta-x\eta)^3 (w+x+\eta-w\eta-x\eta)^3 (-1+\eta t)} + \\
& \frac{432 f w x^3 \eta}{(x+\eta-x\eta)^3 (w+x+\eta-w\eta-x\eta)^3 (-1+\eta t)} - \\
& \frac{324 f x \eta}{(-1+w(-1+\eta))^3 (x+\eta-x\eta)^3 (w+x+\eta-w\eta-x\eta)^3 (-1+\eta t)} - \\
& \frac{1044 f w x \eta}{(-1+w(-1+\eta))^3 (x+\eta-x\eta)^3 (w+x+\eta-w\eta-x\eta)^3 (-1+\eta t)} - \\
& \frac{846 f w^2 x \eta}{(-1+w(-1+\eta))^3 (x+\eta-x\eta)^3 (w+x+\eta-w\eta-x\eta)^3 (-1+\eta t)} + \\
& \frac{162 f w^3 x \eta}{(-1+w(-1+\eta))^3 (x+\eta-x\eta)^3 (w+x+\eta-w\eta-x\eta)^3 (-1+\eta t)} +
\end{aligned}$$

$$\begin{aligned}
& \frac{306 f w^4 x \eta}{(-1+w(-1+\eta))^3 (x+\eta-x\eta)^3 (w+x+\eta-w\eta-x\eta)^3 (-1+\eta t)} + \\
& \frac{18 f w^5 x \eta}{(-1+w(-1+\eta))^3 (x+\eta-x\eta)^3 (w+x+\eta-w\eta-x\eta)^3 (-1+\eta t)} + \\
& \frac{288 f x^2 \eta}{(-1+w(-1+\eta))^3 (x+\eta-x\eta)^3 (w+x+\eta-w\eta-x\eta)^3 (-1+\eta t)} + \\
& \frac{1116 f w x^2 \eta}{(-1+w(-1+\eta))^3 (x+\eta-x\eta)^3 (w+x+\eta-w\eta-x\eta)^3 (-1+\eta t)} + \\
& \frac{1404 f w^2 x^2 \eta}{(-1+w(-1+\eta))^3 (x+\eta-x\eta)^3 (w+x+\eta-w\eta-x\eta)^3 (-1+\eta t)} + \\
& \frac{612 f w^3 x^2 \eta}{(-1+w(-1+\eta))^3 (x+\eta-x\eta)^3 (w+x+\eta-w\eta-x\eta)^3 (-1+\eta t)} - \\
& \frac{180 f w^4 x^2 \eta}{(-1+w(-1+\eta))^3 (x+\eta-x\eta)^3 (w+x+\eta-w\eta-x\eta)^3 (-1+\eta t)} + \\
& \frac{120 f w^5 x^2 \eta}{(-1+w(-1+\eta))^3 (x+\eta-x\eta)^3 (w+x+\eta-w\eta-x\eta)^3 (-1+\eta t)} + \\
& \frac{36 f x^3 \eta}{(-1+w(-1+\eta))^3 (x+\eta-x\eta)^3 (w+x+\eta-w\eta-x\eta)^3 (-1+\eta t)} + \\
& \frac{108 f w x^3 \eta}{(-1+w(-1+\eta))^3 (x+\eta-x\eta)^3 (w+x+\eta-w\eta-x\eta)^3 (-1+\eta t)} + \\
& \frac{108 f w^2 x^3 \eta}{(-1+w(-1+\eta))^3 (x+\eta-x\eta)^3 (w+x+\eta-w\eta-x\eta)^3 (-1+\eta t)} - \\
& \frac{828 f w^3 x^3 \eta}{(-1+w(-1+\eta))^3 (x+\eta-x\eta)^3 (w+x+\eta-w\eta-x\eta)^3 (-1+\eta t)} + \\
& \frac{1272 f w^4 x^3 \eta}{(-1+w(-1+\eta))^3 (x+\eta-x\eta)^3 (w+x+\eta-w\eta-x\eta)^3 (-1+\eta t)} - \\
& \frac{404 f w^5 x^3 \eta}{(-1+w(-1+\eta))^3 (x+\eta-x\eta)^3 (w+x+\eta-w\eta-x\eta)^3 (-1+\eta t)} - \\
& \frac{1080 f w^2 x^4 \eta}{(-1+w(-1+\eta))^3 (x+\eta-x\eta)^3 (w+x+\eta-w\eta-x\eta)^3 (-1+\eta t)} + \\
& \frac{2976 f w^3 x^4 \eta}{(-1+w(-1+\eta))^3 (x+\eta-x\eta)^3 (w+x+\eta-w\eta-x\eta)^3 (-1+\eta t)} - \\
& \frac{1212 f w^4 x^4 \eta}{(-1+w(-1+\eta))^3 (x+\eta-x\eta)^3 (w+x+\eta-w\eta-x\eta)^3 (-1+\eta t)} - \\
& \frac{432 f w x^5 \eta}{(-1+w(-1+\eta))^3 (x+\eta-x\eta)^3 (w+x+\eta-w\eta-x\eta)^3 (-1+\eta t)} + \\
& \frac{2616 f w^2 x^5 \eta}{(-1+w(-1+\eta))^3 (x+\eta-x\eta)^3 (w+x+\eta-w\eta-x\eta)^3 (-1+\eta t)} - \\
& \frac{(-1+w(-1+\eta))^3 (x+\eta-x\eta)^3 (w+x+\eta-w\eta-x\eta)^3 (-1+\eta t)}{(-1+w(-1+\eta))^3 (x+\eta-x\eta)^3 (w+x+\eta-w\eta-x\eta)^3 (-1+\eta t)}
\end{aligned}$$

$$\begin{aligned}
& \frac{1212 f w^3 x^5 \eta}{(-1+w(-1+\eta))^3 (x+\eta-x\eta)^3 (w+x+\eta-w\eta-x\eta)^3 (-1+\eta t)} + \\
& \frac{792 f w x^6 \eta}{(-1+w(-1+\eta))^3 (x+\eta-x\eta)^3 (w+x+\eta-w\eta-x\eta)^3 (-1+\eta t)} - \\
& \frac{404 f w^2 x^6 \eta}{(-1+w(-1+\eta))^3 (x+\eta-x\eta)^3 (w+x+\eta-w\eta-x\eta)^3 (-1+\eta t)} + \\
& \frac{540 f x \eta^2}{(x+\eta-x\eta)^3 (w+x+\eta-w\eta-x\eta)^3 (-1+\eta t)} - \\
& \frac{288 f w x \eta^2}{(x+\eta-x\eta)^3 (w+x+\eta-w\eta-x\eta)^3 (-1+\eta t)} + \\
& \frac{60 f w^2 x \eta^2}{(x+\eta-x\eta)^3 (w+x+\eta-w\eta-x\eta)^3 (-1+\eta t)} - \\
& \frac{432 f x^2 \eta^2}{(x+\eta-x\eta)^3 (w+x+\eta-w\eta-x\eta)^3 (-1+\eta t)} + \\
& \frac{720 f w x^2 \eta^2}{(x+\eta-x\eta)^3 (w+x+\eta-w\eta-x\eta)^3 (-1+\eta t)} - \\
& \frac{180 f w^2 x^2 \eta^2}{(x+\eta-x\eta)^3 (w+x+\eta-w\eta-x\eta)^3 (-1+\eta t)} - \\
& \frac{1080 f w x^3 \eta^2}{(x+\eta-x\eta)^3 (w+x+\eta-w\eta-x\eta)^3 (-1+\eta t)} + \\
& \frac{540 f x \eta^2}{(-1+w(-1+\eta))^3 (x+\eta-x\eta)^3 (w+x+\eta-w\eta-x\eta)^3 (-1+\eta t)} + \\
& \frac{2412 f w x \eta^2}{(-1+w(-1+\eta))^3 (x+\eta-x\eta)^3 (w+x+\eta-w\eta-x\eta)^3 (-1+\eta t)} + \\
& \frac{2718 f w^2 x \eta^2}{(-1+w(-1+\eta))^3 (x+\eta-x\eta)^3 (w+x+\eta-w\eta-x\eta)^3 (-1+\eta t)} - \\
& \frac{108 f w^3 x \eta^2}{(-1+w(-1+\eta))^3 (x+\eta-x\eta)^3 (w+x+\eta-w\eta-x\eta)^3 (-1+\eta t)} - \\
& \frac{1314 f w^4 x \eta^2}{(-1+w(-1+\eta))^3 (x+\eta-x\eta)^3 (w+x+\eta-w\eta-x\eta)^3 (-1+\eta t)} - \\
& \frac{24 f w^5 x \eta^2}{(-1+w(-1+\eta))^3 (x+\eta-x\eta)^3 (w+x+\eta-w\eta-x\eta)^3 (-1+\eta t)} - \\
& \frac{360 f x^2 \eta^2}{(-1+w(-1+\eta))^3 (x+\eta-x\eta)^3 (w+x+\eta-w\eta-x\eta)^3 (-1+\eta t)} - \\
& \frac{2124 f w x^2 \eta^2}{(-1+w(-1+\eta))^3 (x+\eta-x\eta)^3 (w+x+\eta-w\eta-x\eta)^3 (-1+\eta t)} - \\
& \frac{3672 f w^2 x^2 \eta^2}{(-1+w(-1+\eta))^3 (x+\eta-x\eta)^3 (w+x+\eta-w\eta-x\eta)^3 (-1+\eta t)} -
\end{aligned}$$

$$\begin{aligned}
& \frac{3492 f w^3 x^2 \eta^2}{(-1+w(-1+\eta))^3 (x+\eta-x\eta)^3 (w+x+\eta-w\eta-x\eta)^3 (-1+\eta t)} + \\
& \frac{2592 f w^4 x^2 \eta^2}{(-1+w(-1+\eta))^3 (x+\eta-x\eta)^3 (w+x+\eta-w\eta-x\eta)^3 (-1+\eta t)} - \\
& \frac{1092 f w^5 x^2 \eta^2}{(-1+w(-1+\eta))^3 (x+\eta-x\eta)^3 (w+x+\eta-w\eta-x\eta)^3 (-1+\eta t)} - \\
& \frac{180 f x^3 \eta^2}{(-1+w(-1+\eta))^3 (x+\eta-x\eta)^3 (w+x+\eta-w\eta-x\eta)^3 (-1+\eta t)} - \\
& \frac{648 f w x^3 \eta^2}{(-1+w(-1+\eta))^3 (x+\eta-x\eta)^3 (w+x+\eta-w\eta-x\eta)^3 (-1+\eta t)} - \\
& \frac{2916 f w^2 x^3 \eta^2}{(-1+w(-1+\eta))^3 (x+\eta-x\eta)^3 (w+x+\eta-w\eta-x\eta)^3 (-1+\eta t)} + \\
& \frac{9552 f w^3 x^3 \eta^2}{(-1+w(-1+\eta))^3 (x+\eta-x\eta)^3 (w+x+\eta-w\eta-x\eta)^3 (-1+\eta t)} - \\
& \frac{8328 f w^4 x^3 \eta^2}{(-1+w(-1+\eta))^3 (x+\eta-x\eta)^3 (w+x+\eta-w\eta-x\eta)^3 (-1+\eta t)} + \\
& \frac{1804 f w^5 x^3 \eta^2}{(-1+w(-1+\eta))^3 (x+\eta-x\eta)^3 (w+x+\eta-w\eta-x\eta)^3 (-1+\eta t)} - \\
& \frac{1080 f w x^4 \eta^2}{(-1+w(-1+\eta))^3 (x+\eta-x\eta)^3 (w+x+\eta-w\eta-x\eta)^3 (-1+\eta t)} + \\
& \frac{11400 f w^2 x^4 \eta^2}{(-1+w(-1+\eta))^3 (x+\eta-x\eta)^3 (w+x+\eta-w\eta-x\eta)^3 (-1+\eta t)} - \\
& \frac{17340 f w^3 x^4 \eta^2}{(-1+w(-1+\eta))^3 (x+\eta-x\eta)^3 (w+x+\eta-w\eta-x\eta)^3 (-1+\eta t)} + \\
& \frac{5412 f w^4 x^4 \eta^2}{(-1+w(-1+\eta))^3 (x+\eta-x\eta)^3 (w+x+\eta-w\eta-x\eta)^3 (-1+\eta t)} + \\
& \frac{4320 f w x^5 \eta^2}{(-1+w(-1+\eta))^3 (x+\eta-x\eta)^3 (w+x+\eta-w\eta-x\eta)^3 (-1+\eta t)} - \\
& \frac{14064 f w^2 x^5 \eta^2}{(-1+w(-1+\eta))^3 (x+\eta-x\eta)^3 (w+x+\eta-w\eta-x\eta)^3 (-1+\eta t)} + \\
& \frac{5412 f w^3 x^5 \eta^2}{(-1+w(-1+\eta))^3 (x+\eta-x\eta)^3 (w+x+\eta-w\eta-x\eta)^3 (-1+\eta t)} - \\
& \frac{3960 f w x^6 \eta^2}{(-1+w(-1+\eta))^3 (x+\eta-x\eta)^3 (w+x+\eta-w\eta-x\eta)^3 (-1+\eta t)} + \\
& \frac{1804 f w^2 x^6 \eta^2}{(-1+w(-1+\eta))^3 (x+\eta-x\eta)^3 (w+x+\eta-w\eta-x\eta)^3 (-1+\eta t)} - \\
& \frac{396 f x \eta^3}{(x+\eta-x\eta)^3 (w+x+\eta-w\eta-x\eta)^3 (-1+\eta t)} +
\end{aligned}$$

$$\begin{aligned}
& \frac{432 f w x \eta^3}{(x + \eta - x \eta)^3 (w + x + \eta - w \eta - x \eta)^3 (-1 + \eta t)} - \\
& \frac{120 f w^2 x \eta^3}{(x + \eta - x \eta)^3 (w + x + \eta - w \eta - x \eta)^3 (-1 + \eta t)} + \\
& \frac{288 f x^2 \eta^3}{(x + \eta - x \eta)^3 (w + x + \eta - w \eta - x \eta)^3 (-1 + \eta t)} - \\
& \frac{1440 f w x^2 \eta^3}{(x + \eta - x \eta)^3 (w + x + \eta - w \eta - x \eta)^3 (-1 + \eta t)} + \\
& \frac{240 f w^2 x^2 \eta^3}{(x + \eta - x \eta)^3 (w + x + \eta - w \eta - x \eta)^3 (-1 + \eta t)} + \\
& \frac{1440 f w x^3 \eta^3}{(x + \eta - x \eta)^3 (w + x + \eta - w \eta - x \eta)^3 (-1 + \eta t)} - \\
& \frac{72 f w^4 \eta^3}{(-1 + w (-1 + \eta))^3 (x + \eta - x \eta)^3 (w + x + \eta - w \eta - x \eta)^3 (-1 + \eta t)} + \\
& \frac{40 f w^5 \eta^3}{(-1 + w (-1 + \eta))^3 (x + \eta - x \eta)^3 (w + x + \eta - w \eta - x \eta)^3 (-1 + \eta t)} - \\
& \frac{360 f x \eta^3}{(-1 + w (-1 + \eta))^3 (x + \eta - x \eta)^3 (w + x + \eta - w \eta - x \eta)^3 (-1 + \eta t)} - \\
& \frac{2700 f w x \eta^3}{(-1 + w (-1 + \eta))^3 (x + \eta - x \eta)^3 (w + x + \eta - w \eta - x \eta)^3 (-1 + \eta t)} - \\
& \frac{4572 f w^2 x \eta^3}{(-1 + w (-1 + \eta))^3 (x + \eta - x \eta)^3 (w + x + \eta - w \eta - x \eta)^3 (-1 + \eta t)} - \\
& \frac{1566 f w^3 x \eta^3}{(-1 + w (-1 + \eta))^3 (x + \eta - x \eta)^3 (w + x + \eta - w \eta - x \eta)^3 (-1 + \eta t)} + \\
& \frac{4566 f w^4 x \eta^3}{(-1 + w (-1 + \eta))^3 (x + \eta - x \eta)^3 (w + x + \eta - w \eta - x \eta)^3 (-1 + \eta t)} - \\
& \frac{468 f w^5 x \eta^3}{(-1 + w (-1 + \eta))^3 (x + \eta - x \eta)^3 (w + x + \eta - w \eta - x \eta)^3 (-1 + \eta t)} + \\
& \frac{1440 f w x^2 \eta^3}{(-1 + w (-1 + \eta))^3 (x + \eta - x \eta)^3 (w + x + \eta - w \eta - x \eta)^3 (-1 + \eta t)} + \\
& \frac{2484 f w^2 x^2 \eta^3}{(-1 + w (-1 + \eta))^3 (x + \eta - x \eta)^3 (w + x + \eta - w \eta - x \eta)^3 (-1 + \eta t)} + \\
& \frac{17148 f w^3 x^2 \eta^3}{(-1 + w (-1 + \eta))^3 (x + \eta - x \eta)^3 (w + x + \eta - w \eta - x \eta)^3 (-1 + \eta t)} - \\
& \frac{14544 f w^4 x^2 \eta^3}{(-1 + w (-1 + \eta))^3 (x + \eta - x \eta)^3 (w + x + \eta - w \eta - x \eta)^3 (-1 + \eta t)} + \\
& \frac{4320 f w^5 x^2 \eta^3}{(-1 + w (-1 + \eta))^3 (x + \eta - x \eta)^3 (w + x + \eta - w \eta - x \eta)^3 (-1 + \eta t)} +
\end{aligned}$$

$$\begin{aligned}
& \frac{360 f x^3 \eta^3}{(-1+w(-1+\eta))^3 (x+\eta-x\eta)^3 (w+x+\eta-w\eta-x\eta)^3 (-1+\eta t)} + \\
& \frac{180 f w x^3 \eta^3}{(-1+w(-1+\eta))^3 (x+\eta-x\eta)^3 (w+x+\eta-w\eta-x\eta)^3 (-1+\eta t)} + \\
& \frac{22508 f w^2 x^3 \eta^3}{(-1+w(-1+\eta))^3 (x+\eta-x\eta)^3 (w+x+\eta-w\eta-x\eta)^3 (-1+\eta t)} - \\
& \frac{47592 f w^3 x^3 \eta^3}{(-1+w(-1+\eta))^3 (x+\eta-x\eta)^3 (w+x+\eta-w\eta-x\eta)^3 (-1+\eta t)} + \\
& \frac{29160 f w^4 x^3 \eta^3}{(-1+w(-1+\eta))^3 (x+\eta-x\eta)^3 (w+x+\eta-w\eta-x\eta)^3 (-1+\eta t)} - \\
& \frac{4620 f w^5 x^3 \eta^3}{(-1+w(-1+\eta))^3 (x+\eta-x\eta)^3 (w+x+\eta-w\eta-x\eta)^3 (-1+\eta t)} + \\
& \frac{9720 f w x^4 \eta^3}{(-1+w(-1+\eta))^3 (x+\eta-x\eta)^3 (w+x+\eta-w\eta-x\eta)^3 (-1+\eta t)} - \\
& \frac{53460 f w^2 x^4 \eta^3}{(-1+w(-1+\eta))^3 (x+\eta-x\eta)^3 (w+x+\eta-w\eta-x\eta)^3 (-1+\eta t)} + \\
& \frac{57240 f w^3 x^4 \eta^3}{(-1+w(-1+\eta))^3 (x+\eta-x\eta)^3 (w+x+\eta-w\eta-x\eta)^3 (-1+\eta t)} - \\
& \frac{13860 f w^4 x^4 \eta^3}{(-1+w(-1+\eta))^3 (x+\eta-x\eta)^3 (w+x+\eta-w\eta-x\eta)^3 (-1+\eta t)} - \\
& \frac{19440 f w x^5 \eta^3}{(-1+w(-1+\eta))^3 (x+\eta-x\eta)^3 (w+x+\eta-w\eta-x\eta)^3 (-1+\eta t)} + \\
& \frac{44280 f w^2 x^5 \eta^3}{(-1+w(-1+\eta))^3 (x+\eta-x\eta)^3 (w+x+\eta-w\eta-x\eta)^3 (-1+\eta t)} - \\
& \frac{13860 f w^3 x^5 \eta^3}{(-1+w(-1+\eta))^3 (x+\eta-x\eta)^3 (w+x+\eta-w\eta-x\eta)^3 (-1+\eta t)} + \\
& \frac{11880 f w x^6 \eta^3}{(-1+w(-1+\eta))^3 (x+\eta-x\eta)^3 (w+x+\eta-w\eta-x\eta)^3 (-1+\eta t)} - \\
& \frac{4620 f w^2 x^6 \eta^3}{(-1+w(-1+\eta))^3 (x+\eta-x\eta)^3 (w+x+\eta-w\eta-x\eta)^3 (-1+\eta t)} + \\
& \frac{108 f x \eta^4}{(x+\eta-x\eta)^3 (w+x+\eta-w\eta-x\eta)^3 (-1+\eta t)} - \\
& \frac{468 f w x \eta^4}{(x+\eta-x\eta)^3 (w+x+\eta-w\eta-x\eta)^3 (-1+\eta t)} + \\
& \frac{120 f w^2 x \eta^4}{(x+\eta-x\eta)^3 (w+x+\eta-w\eta-x\eta)^3 (-1+\eta t)} - \\
& \frac{72 f x^2 \eta^4}{(x+\eta-x\eta)^3 (w+x+\eta-w\eta-x\eta)^3 (-1+\eta t)} +
\end{aligned}$$

$$\begin{aligned}
& \frac{1440 f w x^2 \eta^4}{(x + \eta - x \eta)^3 (w + x + \eta - w \eta - x \eta)^3 (-1 + \eta t)} - \\
& \frac{180 f w^2 x^2 \eta^4}{(x + \eta - x \eta)^3 (w + x + \eta - w \eta - x \eta)^3 (-1 + \eta t)} - \\
& \frac{1080 f w x^3 \eta^4}{(x + \eta - x \eta)^3 (w + x + \eta - w \eta - x \eta)^3 (-1 + \eta t)} - \\
& \frac{216 f w^3 \eta^4}{(-1 + w (-1 + \eta))^3 (x + \eta - x \eta)^3 (w + x + \eta - w \eta - x \eta)^3 (-1 + \eta t)} + \\
& \frac{696 f w^4 \eta^4}{(-1 + w (-1 + \eta))^3 (x + \eta - x \eta)^3 (w + x + \eta - w \eta - x \eta)^3 (-1 + \eta t)} - \\
& \frac{284 f w^5 \eta^4}{(-1 + w (-1 + \eta))^3 (x + \eta - x \eta)^3 (w + x + \eta - w \eta - x \eta)^3 (-1 + \eta t)} + \\
& \frac{1260 f w x \eta^4}{(-1 + w (-1 + \eta))^3 (x + \eta - x \eta)^3 (w + x + \eta - w \eta - x \eta)^3 (-1 + \eta t)} + \\
& \frac{3060 f w^2 x \eta^4}{(-1 + w (-1 + \eta))^3 (x + \eta - x \eta)^3 (w + x + \eta - w \eta - x \eta)^3 (-1 + \eta t)} + \\
& \frac{9456 f w^3 x \eta^4}{(-1 + w (-1 + \eta))^3 (x + \eta - x \eta)^3 (w + x + \eta - w \eta - x \eta)^3 (-1 + \eta t)} - \\
& \frac{13578 f w^4 x \eta^4}{(-1 + w (-1 + \eta))^3 (x + \eta - x \eta)^3 (w + x + \eta - w \eta - x \eta)^3 (-1 + \eta t)} + \\
& \frac{2340 f w^5 x \eta^4}{(-1 + w (-1 + \eta))^3 (x + \eta - x \eta)^3 (w + x + \eta - w \eta - x \eta)^3 (-1 + \eta t)} + \\
& \frac{360 f x^2 \eta^4}{(-1 + w (-1 + \eta))^3 (x + \eta - x \eta)^3 (w + x + \eta - w \eta - x \eta)^3 (-1 + \eta t)} - \\
& \frac{360 f w x^2 \eta^4}{(-1 + w (-1 + \eta))^3 (x + \eta - x \eta)^3 (w + x + \eta - w \eta - x \eta)^3 (-1 + \eta t)} + \\
& \frac{15720 f w^2 x^2 \eta^4}{(-1 + w (-1 + \eta))^3 (x + \eta - x \eta)^3 (w + x + \eta - w \eta - x \eta)^3 (-1 + \eta t)} - \\
& \frac{59964 f w^3 x^2 \eta^4}{(-1 + w (-1 + \eta))^3 (x + \eta - x \eta)^3 (w + x + \eta - w \eta - x \eta)^3 (-1 + \eta t)} + \\
& \frac{43992 f w^4 x^2 \eta^4}{(-1 + w (-1 + \eta))^3 (x + \eta - x \eta)^3 (w + x + \eta - w \eta - x \eta)^3 (-1 + \eta t)} - \\
& \frac{9540 f w^5 x^2 \eta^4}{(-1 + w (-1 + \eta))^3 (x + \eta - x \eta)^3 (w + x + \eta - w \eta - x \eta)^3 (-1 + \eta t)} - \\
& \frac{360 f x^3 \eta^4}{(-1 + w (-1 + \eta))^3 (x + \eta - x \eta)^3 (w + x + \eta - w \eta - x \eta)^3 (-1 + \eta t)} + \\
& \frac{9360 f w x^3 \eta^4}{(-1 + w (-1 + \eta))^3 (x + \eta - x \eta)^3 (w + x + \eta - w \eta - x \eta)^3 (-1 + \eta t)} -
\end{aligned}$$



$$\begin{aligned}
& \frac{87\,220\,f\,w^2\,x^3\,\eta^4}{(-1+w(-1+\eta))^3(x+\eta-x\eta)^3(w+x+\eta-w\eta-x\eta)^3(-1+\eta t)} + \\
& \frac{135\,144\,f\,w^3\,x^3\,\eta^4}{(-1+w(-1+\eta))^3(x+\eta-x\eta)^3(w+x+\eta-w\eta-x\eta)^3(-1+\eta t)} - \\
& \frac{61\,920\,f\,w^4\,x^3\,\eta^4}{(-1+w(-1+\eta))^3(x+\eta-x\eta)^3(w+x+\eta-w\eta-x\eta)^3(-1+\eta t)} + \\
& \frac{7260\,f\,w^5\,x^3\,\eta^4}{(-1+w(-1+\eta))^3(x+\eta-x\eta)^3(w+x+\eta-w\eta-x\eta)^3(-1+\eta t)} - \\
& \frac{38\,880\,f\,w\,x^4\,\eta^4}{(-1+w(-1+\eta))^3(x+\eta-x\eta)^3(w+x+\eta-w\eta-x\eta)^3(-1+\eta t)} + \\
& \frac{146\,340\,f\,w^2\,x^4\,\eta^4}{(-1+w(-1+\eta))^3(x+\eta-x\eta)^3(w+x+\eta-w\eta-x\eta)^3(-1+\eta t)} - \\
& \frac{118\,980\,f\,w^3\,x^4\,\eta^4}{(-1+w(-1+\eta))^3(x+\eta-x\eta)^3(w+x+\eta-w\eta-x\eta)^3(-1+\eta t)} + \\
& \frac{21\,780\,f\,w^4\,x^4\,\eta^4}{(-1+w(-1+\eta))^3(x+\eta-x\eta)^3(w+x+\eta-w\eta-x\eta)^3(-1+\eta t)} + \\
& \frac{51\,840\,f\,w\,x^5\,\eta^4}{(-1+w(-1+\eta))^3(x+\eta-x\eta)^3(w+x+\eta-w\eta-x\eta)^3(-1+\eta t)} - \\
& \frac{90\,360\,f\,w^2\,x^5\,\eta^4}{(-1+w(-1+\eta))^3(x+\eta-x\eta)^3(w+x+\eta-w\eta-x\eta)^3(-1+\eta t)} + \\
& \frac{21\,780\,f\,w^3\,x^5\,\eta^4}{(-1+w(-1+\eta))^3(x+\eta-x\eta)^3(w+x+\eta-w\eta-x\eta)^3(-1+\eta t)} - \\
& \frac{23\,760\,f\,w\,x^6\,\eta^4}{(-1+w(-1+\eta))^3(x+\eta-x\eta)^3(w+x+\eta-w\eta-x\eta)^3(-1+\eta t)} + \\
& \frac{7260\,f\,w^2\,x^6\,\eta^4}{(-1+w(-1+\eta))^3(x+\eta-x\eta)^3(w+x+\eta-w\eta-x\eta)^3(-1+\eta t)} + \\
& \frac{288\,f\,w\,x\,\eta^5}{(x+\eta-x\eta)^3(w+x+\eta-w\eta-x\eta)^3(-1+\eta t)} - \\
& \frac{60\,f\,w^2\,x\,\eta^5}{(x+\eta-x\eta)^3(w+x+\eta-w\eta-x\eta)^3(-1+\eta t)} - \\
& \frac{720\,f\,w\,x^2\,\eta^5}{(x+\eta-x\eta)^3(w+x+\eta-w\eta-x\eta)^3(-1+\eta t)} + \\
& \frac{72\,f\,w^2\,x^2\,\eta^5}{(x+\eta-x\eta)^3(w+x+\eta-w\eta-x\eta)^3(-1+\eta t)} + \\
& \frac{432\,f\,w\,x^3\,\eta^5}{(x+\eta-x\eta)^3(w+x+\eta-w\eta-x\eta)^3(-1+\eta t)} - \\
& \frac{216\,f\,w^2\,\eta^5}{(-1+w(-1+\eta))^3(x+\eta-x\eta)^3(w+x+\eta-w\eta-x\eta)^3(-1+\eta t)} +
\end{aligned}$$

$$\begin{aligned}
& \frac{1632 f w^3 \eta^5}{(-1+w(-1+\eta))^3 (x+\eta-x\eta)^3 (w+x+\eta-w\eta-x\eta)^3 (-1+\eta t)} - \\
& \frac{2748 f w^4 \eta^5}{(-1+w(-1+\eta))^3 (x+\eta-x\eta)^3 (w+x+\eta-w\eta-x\eta)^3 (-1+\eta t)} + \\
& \frac{832 f w^5 \eta^5}{(-1+w(-1+\eta))^3 (x+\eta-x\eta)^3 (w+x+\eta-w\eta-x\eta)^3 (-1+\eta t)} + \\
& \frac{108 f x \eta^5}{(-1+w(-1+\eta))^3 (x+\eta-x\eta)^3 (w+x+\eta-w\eta-x\eta)^3 (-1+\eta t)} - \\
& \frac{252 f w x \eta^5}{(-1+w(-1+\eta))^3 (x+\eta-x\eta)^3 (w+x+\eta-w\eta-x\eta)^3 (-1+\eta t)} + \\
& \frac{6162 f w^2 x \eta^5}{(-1+w(-1+\eta))^3 (x+\eta-x\eta)^3 (w+x+\eta-w\eta-x\eta)^3 (-1+\eta t)} - \\
& \frac{30\,066 f w^3 x \eta^5}{(-1+w(-1+\eta))^3 (x+\eta-x\eta)^3 (w+x+\eta-w\eta-x\eta)^3 (-1+\eta t)} + \\
& \frac{29\,514 f w^4 x \eta^5}{(-1+w(-1+\eta))^3 (x+\eta-x\eta)^3 (w+x+\eta-w\eta-x\eta)^3 (-1+\eta t)} - \\
& \frac{4932 f w^5 x \eta^5}{(-1+w(-1+\eta))^3 (x+\eta-x\eta)^3 (w+x+\eta-w\eta-x\eta)^3 (-1+\eta t)} - \\
& \frac{288 f x^2 \eta^5}{(-1+w(-1+\eta))^3 (x+\eta-x\eta)^3 (w+x+\eta-w\eta-x\eta)^3 (-1+\eta t)} + \\
& \frac{5796 f w x^2 \eta^5}{(-1+w(-1+\eta))^3 (x+\eta-x\eta)^3 (w+x+\eta-w\eta-x\eta)^3 (-1+\eta t)} - \\
& \frac{65\,544 f w^2 x^2 \eta^5}{(-1+w(-1+\eta))^3 (x+\eta-x\eta)^3 (w+x+\eta-w\eta-x\eta)^3 (-1+\eta t)} + \\
& \frac{136\,596 f w^3 x^2 \eta^5}{(-1+w(-1+\eta))^3 (x+\eta-x\eta)^3 (w+x+\eta-w\eta-x\eta)^3 (-1+\eta t)} - \\
& \frac{79\,992 f w^4 x^2 \eta^5}{(-1+w(-1+\eta))^3 (x+\eta-x\eta)^3 (w+x+\eta-w\eta-x\eta)^3 (-1+\eta t)} + \\
& \frac{12\,240 f w^5 x^2 \eta^5}{(-1+w(-1+\eta))^3 (x+\eta-x\eta)^3 (w+x+\eta-w\eta-x\eta)^3 (-1+\eta t)} + \\
& \frac{180 f x^3 \eta^5}{(-1+w(-1+\eta))^3 (x+\eta-x\eta)^3 (w+x+\eta-w\eta-x\eta)^3 (-1+\eta t)} - \\
& \frac{38\,700 f w x^3 \eta^5}{(-1+w(-1+\eta))^3 (x+\eta-x\eta)^3 (w+x+\eta-w\eta-x\eta)^3 (-1+\eta t)} + \\
& \frac{201\,860 f w^2 x^3 \eta^5}{(-1+w(-1+\eta))^3 (x+\eta-x\eta)^3 (w+x+\eta-w\eta-x\eta)^3 (-1+\eta t)} - \\
& \frac{240\,840 f w^3 x^3 \eta^5}{(-1+w(-1+\eta))^3 (x+\eta-x\eta)^3 (w+x+\eta-w\eta-x\eta)^3 (-1+\eta t)} +
\end{aligned}$$

$$\begin{aligned}
& \frac{82\,224\,f\,w^4\,x^3\,\eta^5}{(-1+w(-1+\eta))^3(x+\eta-x\eta)^3(w+x+\eta-w\eta-x\eta)^3(-1+\eta t)} - \\
& \frac{6600\,f\,w^5\,x^3\,\eta^5}{(-1+w(-1+\eta))^3(x+\eta-x\eta)^3(w+x+\eta-w\eta-x\eta)^3(-1+\eta t)} + \\
& \frac{90\,720\,f\,w\,x^4\,\eta^5}{(-1+w(-1+\eta))^3(x+\eta-x\eta)^3(w+x+\eta-w\eta-x\eta)^3(-1+\eta t)} - \\
& \frac{257\,760\,f\,w^2\,x^4\,\eta^5}{(-1+w(-1+\eta))^3(x+\eta-x\eta)^3(w+x+\eta-w\eta-x\eta)^3(-1+\eta t)} + \\
& \frac{160\,992\,f\,w^3\,x^4\,\eta^5}{(-1+w(-1+\eta))^3(x+\eta-x\eta)^3(w+x+\eta-w\eta-x\eta)^3(-1+\eta t)} - \\
& \frac{19\,800\,f\,w^4\,x^4\,\eta^5}{(-1+w(-1+\eta))^3(x+\eta-x\eta)^3(w+x+\eta-w\eta-x\eta)^3(-1+\eta t)} - \\
& \frac{90\,720\,f\,w\,x^5\,\eta^5}{(-1+w(-1+\eta))^3(x+\eta-x\eta)^3(w+x+\eta-w\eta-x\eta)^3(-1+\eta t)} + \\
& \frac{124\,272\,f\,w^2\,x^5\,\eta^5}{(-1+w(-1+\eta))^3(x+\eta-x\eta)^3(w+x+\eta-w\eta-x\eta)^3(-1+\eta t)} - \\
& \frac{19\,800\,f\,w^3\,x^5\,\eta^5}{(-1+w(-1+\eta))^3(x+\eta-x\eta)^3(w+x+\eta-w\eta-x\eta)^3(-1+\eta t)} + \\
& \frac{33\,264\,f\,w\,x^6\,\eta^5}{(-1+w(-1+\eta))^3(x+\eta-x\eta)^3(w+x+\eta-w\eta-x\eta)^3(-1+\eta t)} - \\
& \frac{6600\,f\,w^2\,x^6\,\eta^5}{(-1+w(-1+\eta))^3(x+\eta-x\eta)^3(w+x+\eta-w\eta-x\eta)^3(-1+\eta t)} - \\
& \frac{72\,f\,w\,x\,\eta^6}{(x+\eta-x\eta)^3(w+x+\eta-w\eta-x\eta)^3(-1+\eta t)} + \\
& \frac{12\,f\,w^2\,x\,\eta^6}{(x+\eta-x\eta)^3(w+x+\eta-w\eta-x\eta)^3(-1+\eta t)} + \\
& \frac{144\,f\,w\,x^2\,\eta^6}{(x+\eta-x\eta)^3(w+x+\eta-w\eta-x\eta)^3(-1+\eta t)} - \\
& \frac{12\,f\,w^2\,x^2\,\eta^6}{(x+\eta-x\eta)^3(w+x+\eta-w\eta-x\eta)^3(-1+\eta t)} - \\
& \frac{72\,f\,w\,x^3\,\eta^6}{(x+\eta-x\eta)^3(w+x+\eta-w\eta-x\eta)^3(-1+\eta t)} - \\
& \frac{72\,f\,w\,\eta^6}{(-1+w(-1+\eta))^3(x+\eta-x\eta)^3(w+x+\eta-w\eta-x\eta)^3(-1+\eta t)} + \\
& \frac{1336\,f\,w^2\,\eta^6}{(-1+w(-1+\eta))^3(x+\eta-x\eta)^3(w+x+\eta-w\eta-x\eta)^3(-1+\eta t)} - \\
& \frac{5148\,f\,w^3\,\eta^6}{(-1+w(-1+\eta))^3(x+\eta-x\eta)^3(w+x+\eta-w\eta-x\eta)^3(-1+\eta t)} +
\end{aligned}$$

$$\begin{aligned}
& \frac{5796 f w^4 \eta^6}{(-1+w(-1+\eta))^3 (x+\eta-x\eta)^3 (w+x+\eta-w\eta-x\eta)^3 (-1+\eta t)} - \\
& \frac{1232 f w^5 \eta^6}{(-1+w(-1+\eta))^3 (x+\eta-x\eta)^3 (w+x+\eta-w\eta-x\eta)^3 (-1+\eta t)} - \\
& \frac{36 f x \eta^6}{(-1+w(-1+\eta))^3 (x+\eta-x\eta)^3 (w+x+\eta-w\eta-x\eta)^3 (-1+\eta t)} + \\
& \frac{2196 f w x \eta^6}{(-1+w(-1+\eta))^3 (x+\eta-x\eta)^3 (w+x+\eta-w\eta-x\eta)^3 (-1+\eta t)} - \\
& \frac{24\,138 f w^2 x \eta^6}{(-1+w(-1+\eta))^3 (x+\eta-x\eta)^3 (w+x+\eta-w\eta-x\eta)^3 (-1+\eta t)} + \\
& \frac{58\,392 f w^3 x \eta^6}{(-1+w(-1+\eta))^3 (x+\eta-x\eta)^3 (w+x+\eta-w\eta-x\eta)^3 (-1+\eta t)} - \\
& \frac{42\,126 f w^4 x \eta^6}{(-1+w(-1+\eta))^3 (x+\eta-x\eta)^3 (w+x+\eta-w\eta-x\eta)^3 (-1+\eta t)} + \\
& \frac{5040 f w^5 x \eta^6}{(-1+w(-1+\eta))^3 (x+\eta-x\eta)^3 (w+x+\eta-w\eta-x\eta)^3 (-1+\eta t)} + \\
& \frac{72 f x^2 \eta^6}{(-1+w(-1+\eta))^3 (x+\eta-x\eta)^3 (w+x+\eta-w\eta-x\eta)^3 (-1+\eta t)} - \\
& \frac{21\,636 f w x^2 \eta^6}{(-1+w(-1+\eta))^3 (x+\eta-x\eta)^3 (w+x+\eta-w\eta-x\eta)^3 (-1+\eta t)} + \\
& \frac{132\,156 f w^2 x^2 \eta^6}{(-1+w(-1+\eta))^3 (x+\eta-x\eta)^3 (w+x+\eta-w\eta-x\eta)^3 (-1+\eta t)} - \\
& \frac{200\,508 f w^3 x^2 \eta^6}{(-1+w(-1+\eta))^3 (x+\eta-x\eta)^3 (w+x+\eta-w\eta-x\eta)^3 (-1+\eta t)} + \\
& \frac{88\,704 f w^4 x^2 \eta^6}{(-1+w(-1+\eta))^3 (x+\eta-x\eta)^3 (w+x+\eta-w\eta-x\eta)^3 (-1+\eta t)} - \\
& \frac{7560 f w^5 x^2 \eta^6}{(-1+w(-1+\eta))^3 (x+\eta-x\eta)^3 (w+x+\eta-w\eta-x\eta)^3 (-1+\eta t)} - \\
& \frac{36 f x^3 \eta^6}{(-1+w(-1+\eta))^3 (x+\eta-x\eta)^3 (w+x+\eta-w\eta-x\eta)^3 (-1+\eta t)} + \\
& \frac{79\,992 f w x^3 \eta^6}{(-1+w(-1+\eta))^3 (x+\eta-x\eta)^3 (w+x+\eta-w\eta-x\eta)^3 (-1+\eta t)} - \\
& \frac{299\,068 f w^2 x^3 \eta^6}{(-1+w(-1+\eta))^3 (x+\eta-x\eta)^3 (w+x+\eta-w\eta-x\eta)^3 (-1+\eta t)} + \\
& \frac{276\,192 f w^3 x^3 \eta^6}{(-1+w(-1+\eta))^3 (x+\eta-x\eta)^3 (w+x+\eta-w\eta-x\eta)^3 (-1+\eta t)} - \\
& \frac{63\,504 f w^4 x^3 \eta^6}{(-1+w(-1+\eta))^3 (x+\eta-x\eta)^3 (w+x+\eta-w\eta-x\eta)^3 (-1+\eta t)} + \\
& \frac{(-1+w(-1+\eta))^3 (x+\eta-x\eta)^3 (w+x+\eta-w\eta-x\eta)^3 (-1+\eta t)}{(-1+w(-1+\eta))^3 (x+\eta-x\eta)^3 (w+x+\eta-w\eta-x\eta)^3 (-1+\eta t)} +
\end{aligned}$$

$$\begin{aligned}
& \frac{1848 f w^5 x^3 \eta^6}{(-1+w(-1+\eta))^3 (x+\eta-x\eta)^3 (w+x+\eta-w\eta-x\eta)^3 (-1+\eta t)} - \\
& \frac{136\,080 f w x^4 \eta^6}{(-1+w(-1+\eta))^3 (x+\eta-x\eta)^3 (w+x+\eta-w\eta-x\eta)^3 (-1+\eta t)} + \\
& \frac{302\,400 f w^2 x^4 \eta^6}{(-1+w(-1+\eta))^3 (x+\eta-x\eta)^3 (w+x+\eta-w\eta-x\eta)^3 (-1+\eta t)} - \\
& \frac{137\,592 f w^3 x^4 \eta^6}{(-1+w(-1+\eta))^3 (x+\eta-x\eta)^3 (w+x+\eta-w\eta-x\eta)^3 (-1+\eta t)} + \\
& \frac{5544 f w^4 x^4 \eta^6}{(-1+w(-1+\eta))^3 (x+\eta-x\eta)^3 (w+x+\eta-w\eta-x\eta)^3 (-1+\eta t)} + \\
& \frac{108\,864 f w x^5 \eta^6}{(-1+w(-1+\eta))^3 (x+\eta-x\eta)^3 (w+x+\eta-w\eta-x\eta)^3 (-1+\eta t)} - \\
& \frac{114\,912 f w^2 x^5 \eta^6}{(-1+w(-1+\eta))^3 (x+\eta-x\eta)^3 (w+x+\eta-w\eta-x\eta)^3 (-1+\eta t)} + \\
& \frac{5544 f w^3 x^5 \eta^6}{(-1+w(-1+\eta))^3 (x+\eta-x\eta)^3 (w+x+\eta-w\eta-x\eta)^3 (-1+\eta t)} - \\
& \frac{33\,264 f w x^6 \eta^6}{(-1+w(-1+\eta))^3 (x+\eta-x\eta)^3 (w+x+\eta-w\eta-x\eta)^3 (-1+\eta t)} + \\
& \frac{1848 f w^2 x^6 \eta^6}{(-1+w(-1+\eta))^3 (x+\eta-x\eta)^3 (w+x+\eta-w\eta-x\eta)^3 (-1+\eta t)} + \\
& \frac{360 f w \eta^7}{(-1+w(-1+\eta))^3 (x+\eta-x\eta)^3 (w+x+\eta-w\eta-x\eta)^3 (-1+\eta t)} - \\
& \frac{3404 f w^2 \eta^7}{(-1+w(-1+\eta))^3 (x+\eta-x\eta)^3 (w+x+\eta-w\eta-x\eta)^3 (-1+\eta t)} + \\
& \frac{8712 f w^3 \eta^7}{(-1+w(-1+\eta))^3 (x+\eta-x\eta)^3 (w+x+\eta-w\eta-x\eta)^3 (-1+\eta t)} - \\
& \frac{6972 f w^4 \eta^7}{(-1+w(-1+\eta))^3 (x+\eta-x\eta)^3 (w+x+\eta-w\eta-x\eta)^3 (-1+\eta t)} + \\
& \frac{784 f w^5 \eta^7}{(-1+w(-1+\eta))^3 (x+\eta-x\eta)^3 (w+x+\eta-w\eta-x\eta)^3 (-1+\eta t)} - \\
& \frac{6372 f w x \eta^7}{(-1+w(-1+\eta))^3 (x+\eta-x\eta)^3 (w+x+\eta-w\eta-x\eta)^3 (-1+\eta t)} + \\
& \frac{40\,536 f w^2 x \eta^7}{(-1+w(-1+\eta))^3 (x+\eta-x\eta)^3 (w+x+\eta-w\eta-x\eta)^3 (-1+\eta t)} - \\
& \frac{70\,302 f w^3 x \eta^7}{(-1+w(-1+\eta))^3 (x+\eta-x\eta)^3 (w+x+\eta-w\eta-x\eta)^3 (-1+\eta t)} + \\
& \frac{36\,282 f w^4 x \eta^7}{(-1+w(-1+\eta))^3 (x+\eta-x\eta)^3 (w+x+\eta-w\eta-x\eta)^3 (-1+\eta t)} - \\
& \frac{(-1+w(-1+\eta))^3 (x+\eta-x\eta)^3 (w+x+\eta-w\eta-x\eta)^3 (-1+\eta t)}{(-1+w(-1+\eta))^3 (x+\eta-x\eta)^3 (w+x+\eta-w\eta-x\eta)^3 (-1+\eta t)}
\end{aligned}$$

$$\begin{aligned}
& \frac{1008 f w^5 x \eta^7}{(-1+w(-1+\eta))^3 (x+\eta-x\eta)^3 (w+x+\eta-w\eta-x\eta)^3 (-1+\eta t)} + \\
& \frac{37584 f w x^2 \eta^7}{(-1+w(-1+\eta))^3 (x+\eta-x\eta)^3 (w+x+\eta-w\eta-x\eta)^3 (-1+\eta t)} - \\
& \frac{162048 f w^2 x^2 \eta^7}{(-1+w(-1+\eta))^3 (x+\eta-x\eta)^3 (w+x+\eta-w\eta-x\eta)^3 (-1+\eta t)} + \\
& \frac{186132 f w^3 x^2 \eta^7}{(-1+w(-1+\eta))^3 (x+\eta-x\eta)^3 (w+x+\eta-w\eta-x\eta)^3 (-1+\eta t)} - \\
& \frac{53424 f w^4 x^2 \eta^7}{(-1+w(-1+\eta))^3 (x+\eta-x\eta)^3 (w+x+\eta-w\eta-x\eta)^3 (-1+\eta t)} - \\
& \frac{2016 f w^5 x^2 \eta^7}{(-1+w(-1+\eta))^3 (x+\eta-x\eta)^3 (w+x+\eta-w\eta-x\eta)^3 (-1+\eta t)} - \\
& \frac{100692 f w x^3 \eta^7}{(-1+w(-1+\eta))^3 (x+\eta-x\eta)^3 (w+x+\eta-w\eta-x\eta)^3 (-1+\eta t)} + \\
& \frac{288596 f w^2 x^3 \eta^7}{(-1+w(-1+\eta))^3 (x+\eta-x\eta)^3 (w+x+\eta-w\eta-x\eta)^3 (-1+\eta t)} - \\
& \frac{195552 f w^3 x^3 \eta^7}{(-1+w(-1+\eta))^3 (x+\eta-x\eta)^3 (w+x+\eta-w\eta-x\eta)^3 (-1+\eta t)} + \\
& \frac{15696 f w^4 x^3 \eta^7}{(-1+w(-1+\eta))^3 (x+\eta-x\eta)^3 (w+x+\eta-w\eta-x\eta)^3 (-1+\eta t)} + \\
& \frac{3432 f w^5 x^3 \eta^7}{(-1+w(-1+\eta))^3 (x+\eta-x\eta)^3 (w+x+\eta-w\eta-x\eta)^3 (-1+\eta t)} + \\
& \frac{136080 f w x^4 \eta^7}{(-1+w(-1+\eta))^3 (x+\eta-x\eta)^3 (w+x+\eta-w\eta-x\eta)^3 (-1+\eta t)} - \\
& \frac{234360 f w^2 x^4 \eta^7}{(-1+w(-1+\eta))^3 (x+\eta-x\eta)^3 (w+x+\eta-w\eta-x\eta)^3 (-1+\eta t)} + \\
& \frac{61200 f w^3 x^4 \eta^7}{(-1+w(-1+\eta))^3 (x+\eta-x\eta)^3 (w+x+\eta-w\eta-x\eta)^3 (-1+\eta t)} + \\
& \frac{10296 f w^4 x^4 \eta^7}{(-1+w(-1+\eta))^3 (x+\eta-x\eta)^3 (w+x+\eta-w\eta-x\eta)^3 (-1+\eta t)} - \\
& \frac{90720 f w x^5 \eta^7}{(-1+w(-1+\eta))^3 (x+\eta-x\eta)^3 (w+x+\eta-w\eta-x\eta)^3 (-1+\eta t)} + \\
& \frac{67248 f w^2 x^5 \eta^7}{(-1+w(-1+\eta))^3 (x+\eta-x\eta)^3 (w+x+\eta-w\eta-x\eta)^3 (-1+\eta t)} + \\
& \frac{10296 f w^3 x^5 \eta^7}{(-1+w(-1+\eta))^3 (x+\eta-x\eta)^3 (w+x+\eta-w\eta-x\eta)^3 (-1+\eta t)} + \\
& \frac{23760 f w x^6 \eta^7}{(-1+w(-1+\eta))^3 (x+\eta-x\eta)^3 (w+x+\eta-w\eta-x\eta)^3 (-1+\eta t)} +
\end{aligned}$$

$$\begin{aligned}
& \frac{3432 f w^2 x^6 \eta^7}{(-1+w(-1+\eta))^3 (x+\eta-x\eta)^3 (w+x+\eta-w\eta-x\eta)^3 (-1+\eta t)} - \\
& \frac{720 f w \eta^8}{(-1+w(-1+\eta))^3 (x+\eta-x\eta)^3 (w+x+\eta-w\eta-x\eta)^3 (-1+\eta t)} + \\
& \frac{4540 f w^2 \eta^8}{(-1+w(-1+\eta))^3 (x+\eta-x\eta)^3 (w+x+\eta-w\eta-x\eta)^3 (-1+\eta t)} - \\
& \frac{8340 f w^3 \eta^8}{(-1+w(-1+\eta))^3 (x+\eta-x\eta)^3 (w+x+\eta-w\eta-x\eta)^3 (-1+\eta t)} + \\
& \frac{4452 f w^4 \eta^8}{(-1+w(-1+\eta))^3 (x+\eta-x\eta)^3 (w+x+\eta-w\eta-x\eta)^3 (-1+\eta t)} + \\
& \frac{280 f w^5 \eta^8}{(-1+w(-1+\eta))^3 (x+\eta-x\eta)^3 (w+x+\eta-w\eta-x\eta)^3 (-1+\eta t)} + \\
& \frac{8640 f w x \eta^8}{(-1+w(-1+\eta))^3 (x+\eta-x\eta)^3 (w+x+\eta-w\eta-x\eta)^3 (-1+\eta t)} - \\
& \frac{39468 f w^2 x \eta^8}{(-1+w(-1+\eta))^3 (x+\eta-x\eta)^3 (w+x+\eta-w\eta-x\eta)^3 (-1+\eta t)} + \\
& \frac{50376 f w^3 x \eta^8}{(-1+w(-1+\eta))^3 (x+\eta-x\eta)^3 (w+x+\eta-w\eta-x\eta)^3 (-1+\eta t)} - \\
& \frac{14586 f w^4 x \eta^8}{(-1+w(-1+\eta))^3 (x+\eta-x\eta)^3 (w+x+\eta-w\eta-x\eta)^3 (-1+\eta t)} - \\
& \frac{3672 f w^5 x \eta^8}{(-1+w(-1+\eta))^3 (x+\eta-x\eta)^3 (w+x+\eta-w\eta-x\eta)^3 (-1+\eta t)} - \\
& \frac{37800 f w x^2 \eta^8}{(-1+w(-1+\eta))^3 (x+\eta-x\eta)^3 (w+x+\eta-w\eta-x\eta)^3 (-1+\eta t)} + \\
& \frac{123276 f w^2 x^2 \eta^8}{(-1+w(-1+\eta))^3 (x+\eta-x\eta)^3 (w+x+\eta-w\eta-x\eta)^3 (-1+\eta t)} - \\
& \frac{100068 f w^3 x^2 \eta^8}{(-1+w(-1+\eta))^3 (x+\eta-x\eta)^3 (w+x+\eta-w\eta-x\eta)^3 (-1+\eta t)} + \\
& \frac{4464 f w^4 x^2 \eta^8}{(-1+w(-1+\eta))^3 (x+\eta-x\eta)^3 (w+x+\eta-w\eta-x\eta)^3 (-1+\eta t)} + \\
& \frac{8280 f w^5 x^2 \eta^8}{(-1+w(-1+\eta))^3 (x+\eta-x\eta)^3 (w+x+\eta-w\eta-x\eta)^3 (-1+\eta t)} + \\
& \frac{80640 f w x^3 \eta^8}{(-1+w(-1+\eta))^3 (x+\eta-x\eta)^3 (w+x+\eta-w\eta-x\eta)^3 (-1+\eta t)} - \\
& \frac{175948 f w^2 x^3 \eta^8}{(-1+w(-1+\eta))^3 (x+\eta-x\eta)^3 (w+x+\eta-w\eta-x\eta)^3 (-1+\eta t)} + \\
& \frac{68112 f w^3 x^3 \eta^8}{(-1+w(-1+\eta))^3 (x+\eta-x\eta)^3 (w+x+\eta-w\eta-x\eta)^3 (-1+\eta t)} + \\
& \frac{(-1+w(-1+\eta))^3 (x+\eta-x\eta)^3 (w+x+\eta-w\eta-x\eta)^3 (-1+\eta t)}{(-1+w(-1+\eta))^3 (x+\eta-x\eta)^3 (w+x+\eta-w\eta-x\eta)^3 (-1+\eta t)} +
\end{aligned}$$

$$\begin{aligned}
& \frac{21\,240\,f\,w^4\,x^3\,\eta^8}{(-1+w(-1+\eta))^3(x+\eta-x\eta)^3(w+x+\eta-w\eta-x\eta)^3(-1+\eta t)} - \\
& \frac{5280\,f\,w^5\,x^3\,\eta^8}{(-1+w(-1+\eta))^3(x+\eta-x\eta)^3(w+x+\eta-w\eta-x\eta)^3(-1+\eta t)} - \\
& \frac{90\,720\,f\,w\,x^4\,\eta^8}{(-1+w(-1+\eta))^3(x+\eta-x\eta)^3(w+x+\eta-w\eta-x\eta)^3(-1+\eta t)} + \\
& \frac{111\,960\,f\,w^2\,x^4\,\eta^8}{(-1+w(-1+\eta))^3(x+\eta-x\eta)^3(w+x+\eta-w\eta-x\eta)^3(-1+\eta t)} + \\
& \frac{5760\,f\,w^3\,x^4\,\eta^8}{(-1+w(-1+\eta))^3(x+\eta-x\eta)^3(w+x+\eta-w\eta-x\eta)^3(-1+\eta t)} - \\
& \frac{15\,840\,f\,w^4\,x^4\,\eta^8}{(-1+w(-1+\eta))^3(x+\eta-x\eta)^3(w+x+\eta-w\eta-x\eta)^3(-1+\eta t)} + \\
& \frac{51\,840\,f\,w\,x^5\,\eta^8}{(-1+w(-1+\eta))^3(x+\eta-x\eta)^3(w+x+\eta-w\eta-x\eta)^3(-1+\eta t)} - \\
& \frac{19\,080\,f\,w^2\,x^5\,\eta^8}{(-1+w(-1+\eta))^3(x+\eta-x\eta)^3(w+x+\eta-w\eta-x\eta)^3(-1+\eta t)} - \\
& \frac{15\,840\,f\,w^3\,x^5\,\eta^8}{(-1+w(-1+\eta))^3(x+\eta-x\eta)^3(w+x+\eta-w\eta-x\eta)^3(-1+\eta t)} - \\
& \frac{11\,880\,f\,w\,x^6\,\eta^8}{(-1+w(-1+\eta))^3(x+\eta-x\eta)^3(w+x+\eta-w\eta-x\eta)^3(-1+\eta t)} - \\
& \frac{5280\,f\,w^2\,x^6\,\eta^8}{(-1+w(-1+\eta))^3(x+\eta-x\eta)^3(w+x+\eta-w\eta-x\eta)^3(-1+\eta t)} + \\
& \frac{720\,f\,w\,\eta^9}{(-1+w(-1+\eta))^3(x+\eta-x\eta)^3(w+x+\eta-w\eta-x\eta)^3(-1+\eta t)} - \\
& \frac{3280\,f\,w^2\,\eta^9}{(-1+w(-1+\eta))^3(x+\eta-x\eta)^3(w+x+\eta-w\eta-x\eta)^3(-1+\eta t)} + \\
& \frac{4176\,f\,w^3\,\eta^9}{(-1+w(-1+\eta))^3(x+\eta-x\eta)^3(w+x+\eta-w\eta-x\eta)^3(-1+\eta t)} - \\
& \frac{756\,f\,w^4\,\eta^9}{(-1+w(-1+\eta))^3(x+\eta-x\eta)^3(w+x+\eta-w\eta-x\eta)^3(-1+\eta t)} - \\
& \frac{896\,f\,w^5\,\eta^9}{(-1+w(-1+\eta))^3(x+\eta-x\eta)^3(w+x+\eta-w\eta-x\eta)^3(-1+\eta t)} - \\
& \frac{6480\,f\,w\,x\,\eta^9}{(-1+w(-1+\eta))^3(x+\eta-x\eta)^3(w+x+\eta-w\eta-x\eta)^3(-1+\eta t)} + \\
& \frac{21\,960\,f\,w^2\,x\,\eta^9}{(-1+w(-1+\eta))^3(x+\eta-x\eta)^3(w+x+\eta-w\eta-x\eta)^3(-1+\eta t)} - \\
& \frac{17\,856\,f\,w^3\,x\,\eta^9}{(-1+w(-1+\eta))^3(x+\eta-x\eta)^3(w+x+\eta-w\eta-x\eta)^3(-1+\eta t)} -
\end{aligned}$$



$$\begin{aligned}
& \frac{3012 f w^4 x \eta^9}{(-1+w(-1+\eta))^3 (x+\eta-x\eta)^3 (w+x+\eta-w\eta-x\eta)^3 (-1+\eta t)} + \\
& \frac{4770 f w^5 x \eta^9}{(-1+w(-1+\eta))^3 (x+\eta-x\eta)^3 (w+x+\eta-w\eta-x\eta)^3 (-1+\eta t)} + \\
& \frac{22\,680 f w x^2 \eta^9}{(-1+w(-1+\eta))^3 (x+\eta-x\eta)^3 (w+x+\eta-w\eta-x\eta)^3 (-1+\eta t)} - \\
& \frac{54\,180 f w^2 x^2 \eta^9}{(-1+w(-1+\eta))^3 (x+\eta-x\eta)^3 (w+x+\eta-w\eta-x\eta)^3 (-1+\eta t)} + \\
& \frac{19\,704 f w^3 x^2 \eta^9}{(-1+w(-1+\eta))^3 (x+\eta-x\eta)^3 (w+x+\eta-w\eta-x\eta)^3 (-1+\eta t)} + \\
& \frac{18\,828 f w^4 x^2 \eta^9}{(-1+w(-1+\eta))^3 (x+\eta-x\eta)^3 (w+x+\eta-w\eta-x\eta)^3 (-1+\eta t)} - \\
& \frac{7560 f w^5 x^2 \eta^9}{(-1+w(-1+\eta))^3 (x+\eta-x\eta)^3 (w+x+\eta-w\eta-x\eta)^3 (-1+\eta t)} - \\
& \frac{40\,320 f w x^3 \eta^9}{(-1+w(-1+\eta))^3 (x+\eta-x\eta)^3 (w+x+\eta-w\eta-x\eta)^3 (-1+\eta t)} + \\
& \frac{59\,840 f w^2 x^3 \eta^9}{(-1+w(-1+\eta))^3 (x+\eta-x\eta)^3 (w+x+\eta-w\eta-x\eta)^3 (-1+\eta t)} + \\
& \frac{8676 f w^3 x^3 \eta^9}{(-1+w(-1+\eta))^3 (x+\eta-x\eta)^3 (w+x+\eta-w\eta-x\eta)^3 (-1+\eta t)} - \\
& \frac{26\,280 f w^4 x^3 \eta^9}{(-1+w(-1+\eta))^3 (x+\eta-x\eta)^3 (w+x+\eta-w\eta-x\eta)^3 (-1+\eta t)} + \\
& \frac{3740 f w^5 x^3 \eta^9}{(-1+w(-1+\eta))^3 (x+\eta-x\eta)^3 (w+x+\eta-w\eta-x\eta)^3 (-1+\eta t)} + \\
& \frac{38\,880 f w x^4 \eta^9}{(-1+w(-1+\eta))^3 (x+\eta-x\eta)^3 (w+x+\eta-w\eta-x\eta)^3 (-1+\eta t)} - \\
& \frac{24\,840 f w^2 x^4 \eta^9}{(-1+w(-1+\eta))^3 (x+\eta-x\eta)^3 (w+x+\eta-w\eta-x\eta)^3 (-1+\eta t)} - \\
& \frac{25\,920 f w^3 x^4 \eta^9}{(-1+w(-1+\eta))^3 (x+\eta-x\eta)^3 (w+x+\eta-w\eta-x\eta)^3 (-1+\eta t)} + \\
& \frac{11\,220 f w^4 x^4 \eta^9}{(-1+w(-1+\eta))^3 (x+\eta-x\eta)^3 (w+x+\eta-w\eta-x\eta)^3 (-1+\eta t)} - \\
& \frac{19\,440 f w x^5 \eta^9}{(-1+w(-1+\eta))^3 (x+\eta-x\eta)^3 (w+x+\eta-w\eta-x\eta)^3 (-1+\eta t)} - \\
& \frac{3240 f w^2 x^5 \eta^9}{(-1+w(-1+\eta))^3 (x+\eta-x\eta)^3 (w+x+\eta-w\eta-x\eta)^3 (-1+\eta t)} + \\
& \frac{11\,220 f w^3 x^5 \eta^9}{(-1+w(-1+\eta))^3 (x+\eta-x\eta)^3 (w+x+\eta-w\eta-x\eta)^3 (-1+\eta t)} + \\
& \frac{(-1+w(-1+\eta))^3 (x+\eta-x\eta)^3 (w+x+\eta-w\eta-x\eta)^3 (-1+\eta t)}{(-1+w(-1+\eta))^3 (x+\eta-x\eta)^3 (w+x+\eta-w\eta-x\eta)^3 (-1+\eta t)} +
\end{aligned}$$

$$\begin{aligned}
& \frac{3960 f w x^6 \eta^9}{(-1+w(-1+\eta))^3 (x+\eta-x\eta)^3 (w+x+\eta-w\eta-x\eta)^3 (-1+\eta t)} + \\
& \frac{3740 f w^2 x^6 \eta^9}{(-1+w(-1+\eta))^3 (x+\eta-x\eta)^3 (w+x+\eta-w\eta-x\eta)^3 (-1+\eta t)} - \\
& \frac{360 f w \eta^{10}}{(-1+w(-1+\eta))^3 (x+\eta-x\eta)^3 (w+x+\eta-w\eta-x\eta)^3 (-1+\eta t)} + \\
& \frac{1136 f w^2 \eta^{10}}{(-1+w(-1+\eta))^3 (x+\eta-x\eta)^3 (w+x+\eta-w\eta-x\eta)^3 (-1+\eta t)} - \\
& \frac{612 f w^3 \eta^{10}}{(-1+w(-1+\eta))^3 (x+\eta-x\eta)^3 (w+x+\eta-w\eta-x\eta)^3 (-1+\eta t)} - \\
& \frac{852 f w^4 \eta^{10}}{(-1+w(-1+\eta))^3 (x+\eta-x\eta)^3 (w+x+\eta-w\eta-x\eta)^3 (-1+\eta t)} + \\
& \frac{688 f w^5 \eta^{10}}{(-1+w(-1+\eta))^3 (x+\eta-x\eta)^3 (w+x+\eta-w\eta-x\eta)^3 (-1+\eta t)} + \\
& \frac{2592 f w x \eta^{10}}{(-1+w(-1+\eta))^3 (x+\eta-x\eta)^3 (w+x+\eta-w\eta-x\eta)^3 (-1+\eta t)} - \\
& \frac{5760 f w^2 x \eta^{10}}{(-1+w(-1+\eta))^3 (x+\eta-x\eta)^3 (w+x+\eta-w\eta-x\eta)^3 (-1+\eta t)} - \\
& \frac{228 f w^3 x \eta^{10}}{(-1+w(-1+\eta))^3 (x+\eta-x\eta)^3 (w+x+\eta-w\eta-x\eta)^3 (-1+\eta t)} + \\
& \frac{6312 f w^4 x \eta^{10}}{(-1+w(-1+\eta))^3 (x+\eta-x\eta)^3 (w+x+\eta-w\eta-x\eta)^3 (-1+\eta t)} - \\
& \frac{2808 f w^5 x \eta^{10}}{(-1+w(-1+\eta))^3 (x+\eta-x\eta)^3 (w+x+\eta-w\eta-x\eta)^3 (-1+\eta t)} - \\
& \frac{7560 f w x^2 \eta^{10}}{(-1+w(-1+\eta))^3 (x+\eta-x\eta)^3 (w+x+\eta-w\eta-x\eta)^3 (-1+\eta t)} + \\
& \frac{10140 f w^2 x^2 \eta^{10}}{(-1+w(-1+\eta))^3 (x+\eta-x\eta)^3 (w+x+\eta-w\eta-x\eta)^3 (-1+\eta t)} + \\
& \frac{8976 f w^3 x^2 \eta^{10}}{(-1+w(-1+\eta))^3 (x+\eta-x\eta)^3 (w+x+\eta-w\eta-x\eta)^3 (-1+\eta t)} - \\
& \frac{14688 f w^4 x^2 \eta^{10}}{(-1+w(-1+\eta))^3 (x+\eta-x\eta)^3 (w+x+\eta-w\eta-x\eta)^3 (-1+\eta t)} + \\
& \frac{3660 f w^5 x^2 \eta^{10}}{(-1+w(-1+\eta))^3 (x+\eta-x\eta)^3 (w+x+\eta-w\eta-x\eta)^3 (-1+\eta t)} + \\
& \frac{11520 f w x^3 \eta^{10}}{(-1+w(-1+\eta))^3 (x+\eta-x\eta)^3 (w+x+\eta-w\eta-x\eta)^3 (-1+\eta t)} - \\
& \frac{5680 f w^2 x^3 \eta^{10}}{(-1+w(-1+\eta))^3 (x+\eta-x\eta)^3 (w+x+\eta-w\eta-x\eta)^3 (-1+\eta t)} - \\
& \frac{(-1+w(-1+\eta))^3 (x+\eta-x\eta)^3 (w+x+\eta-w\eta-x\eta)^3 (-1+\eta t)}{(-1+w(-1+\eta))^3 (x+\eta-x\eta)^3 (w+x+\eta-w\eta-x\eta)^3 (-1+\eta t)}
\end{aligned}$$

$$\begin{aligned}
& \frac{19\,440\,f\,w^3\,x^3\,\eta^{10}}{(-1+w(-1+\eta))^3(x+\eta-x\eta)^3(w+x+\eta-w\eta-x\eta)^3(-1+\eta t)} + \\
& \frac{13\,848\,f\,w^4\,x^3\,\eta^{10}}{(-1+w(-1+\eta))^3(x+\eta-x\eta)^3(w+x+\eta-w\eta-x\eta)^3(-1+\eta t)} - \\
& \frac{1540\,f\,w^5\,x^3\,\eta^{10}}{(-1+w(-1+\eta))^3(x+\eta-x\eta)^3(w+x+\eta-w\eta-x\eta)^3(-1+\eta t)} - \\
& \frac{9720\,f\,w\,x^4\,\eta^{10}}{(-1+w(-1+\eta))^3(x+\eta-x\eta)^3(w+x+\eta-w\eta-x\eta)^3(-1+\eta t)} - \\
& \frac{3240\,f\,w^2\,x^4\,\eta^{10}}{(-1+w(-1+\eta))^3(x+\eta-x\eta)^3(w+x+\eta-w\eta-x\eta)^3(-1+\eta t)} + \\
& \frac{15\,924\,f\,w^3\,x^4\,\eta^{10}}{(-1+w(-1+\eta))^3(x+\eta-x\eta)^3(w+x+\eta-w\eta-x\eta)^3(-1+\eta t)} - \\
& \frac{4620\,f\,w^4\,x^4\,\eta^{10}}{(-1+w(-1+\eta))^3(x+\eta-x\eta)^3(w+x+\eta-w\eta-x\eta)^3(-1+\eta t)} + \\
& \frac{4320\,f\,w\,x^5\,\eta^{10}}{(-1+w(-1+\eta))^3(x+\eta-x\eta)^3(w+x+\eta-w\eta-x\eta)^3(-1+\eta t)} + \\
& \frac{4944\,f\,w^2\,x^5\,\eta^{10}}{(-1+w(-1+\eta))^3(x+\eta-x\eta)^3(w+x+\eta-w\eta-x\eta)^3(-1+\eta t)} - \\
& \frac{4620\,f\,w^3\,x^5\,\eta^{10}}{(-1+w(-1+\eta))^3(x+\eta-x\eta)^3(w+x+\eta-w\eta-x\eta)^3(-1+\eta t)} - \\
& \frac{792\,f\,w\,x^6\,\eta^{10}}{(-1+w(-1+\eta))^3(x+\eta-x\eta)^3(w+x+\eta-w\eta-x\eta)^3(-1+\eta t)} - \\
& \frac{1540\,f\,w^2\,x^6\,\eta^{10}}{(-1+w(-1+\eta))^3(x+\eta-x\eta)^3(w+x+\eta-w\eta-x\eta)^3(-1+\eta t)} + \\
& \frac{72\,f\,w\,\eta^{11}}{(-1+w(-1+\eta))^3(x+\eta-x\eta)^3(w+x+\eta-w\eta-x\eta)^3(-1+\eta t)} - \\
& \frac{76\,f\,w^2\,\eta^{11}}{(-1+w(-1+\eta))^3(x+\eta-x\eta)^3(w+x+\eta-w\eta-x\eta)^3(-1+\eta t)} - \\
& \frac{312\,f\,w^3\,\eta^{11}}{(-1+w(-1+\eta))^3(x+\eta-x\eta)^3(w+x+\eta-w\eta-x\eta)^3(-1+\eta t)} + \\
& \frac{564\,f\,w^4\,\eta^{11}}{(-1+w(-1+\eta))^3(x+\eta-x\eta)^3(w+x+\eta-w\eta-x\eta)^3(-1+\eta t)} - \\
& \frac{248\,f\,w^5\,\eta^{11}}{(-1+w(-1+\eta))^3(x+\eta-x\eta)^3(w+x+\eta-w\eta-x\eta)^3(-1+\eta t)} - \\
& \frac{432\,f\,w\,x\,\eta^{11}}{(-1+w(-1+\eta))^3(x+\eta-x\eta)^3(w+x+\eta-w\eta-x\eta)^3(-1+\eta t)} + \\
& \frac{24\,f\,w^2\,x\,\eta^{11}}{(-1+w(-1+\eta))^3(x+\eta-x\eta)^3(w+x+\eta-w\eta-x\eta)^3(-1+\eta t)} +
\end{aligned}$$

$$\begin{aligned}
& \frac{2316 f w^3 x \eta^{11}}{(-1+w(-1+\eta))^3 (x+\eta-x\eta)^3 (w+x+\eta-w\eta-x\eta)^3 (-1+\eta t)} - \\
& \frac{2760 f w^4 x \eta^{11}}{(-1+w(-1+\eta))^3 (x+\eta-x\eta)^3 (w+x+\eta-w\eta-x\eta)^3 (-1+\eta t)} + \\
& \frac{852 f w^5 x \eta^{11}}{(-1+w(-1+\eta))^3 (x+\eta-x\eta)^3 (w+x+\eta-w\eta-x\eta)^3 (-1+\eta t)} + \\
& \frac{1080 f w x^2 \eta^{11}}{(-1+w(-1+\eta))^3 (x+\eta-x\eta)^3 (w+x+\eta-w\eta-x\eta)^3 (-1+\eta t)} + \\
& \frac{1020 f w^2 x^2 \eta^{11}}{(-1+w(-1+\eta))^3 (x+\eta-x\eta)^3 (w+x+\eta-w\eta-x\eta)^3 (-1+\eta t)} - \\
& \frac{6144 f w^3 x^2 \eta^{11}}{(-1+w(-1+\eta))^3 (x+\eta-x\eta)^3 (w+x+\eta-w\eta-x\eta)^3 (-1+\eta t)} + \\
& \frac{4896 f w^4 x^2 \eta^{11}}{(-1+w(-1+\eta))^3 (x+\eta-x\eta)^3 (w+x+\eta-w\eta-x\eta)^3 (-1+\eta t)} - \\
& \frac{960 f w^5 x^2 \eta^{11}}{(-1+w(-1+\eta))^3 (x+\eta-x\eta)^3 (w+x+\eta-w\eta-x\eta)^3 (-1+\eta t)} - \\
& \frac{1440 f w x^3 \eta^{11}}{(-1+w(-1+\eta))^3 (x+\eta-x\eta)^3 (w+x+\eta-w\eta-x\eta)^3 (-1+\eta t)} - \\
& \frac{2800 f w^2 x^3 \eta^{11}}{(-1+w(-1+\eta))^3 (x+\eta-x\eta)^3 (w+x+\eta-w\eta-x\eta)^3 (-1+\eta t)} + \\
& \frac{7656 f w^3 x^3 \eta^{11}}{(-1+w(-1+\eta))^3 (x+\eta-x\eta)^3 (w+x+\eta-w\eta-x\eta)^3 (-1+\eta t)} - \\
& \frac{3768 f w^4 x^3 \eta^{11}}{(-1+w(-1+\eta))^3 (x+\eta-x\eta)^3 (w+x+\eta-w\eta-x\eta)^3 (-1+\eta t)} + \\
& \frac{356 f w^5 x^3 \eta^{11}}{(-1+w(-1+\eta))^3 (x+\eta-x\eta)^3 (w+x+\eta-w\eta-x\eta)^3 (-1+\eta t)} + \\
& \frac{1080 f w x^4 \eta^{11}}{(-1+w(-1+\eta))^3 (x+\eta-x\eta)^3 (w+x+\eta-w\eta-x\eta)^3 (-1+\eta t)} + \\
& \frac{3180 f w^2 x^4 \eta^{11}}{(-1+w(-1+\eta))^3 (x+\eta-x\eta)^3 (w+x+\eta-w\eta-x\eta)^3 (-1+\eta t)} - \\
& \frac{4584 f w^3 x^4 \eta^{11}}{(-1+w(-1+\eta))^3 (x+\eta-x\eta)^3 (w+x+\eta-w\eta-x\eta)^3 (-1+\eta t)} + \\
& \frac{1068 f w^4 x^4 \eta^{11}}{(-1+w(-1+\eta))^3 (x+\eta-x\eta)^3 (w+x+\eta-w\eta-x\eta)^3 (-1+\eta t)} - \\
& \frac{432 f w x^5 \eta^{11}}{(-1+w(-1+\eta))^3 (x+\eta-x\eta)^3 (w+x+\eta-w\eta-x\eta)^3 (-1+\eta t)} - \\
& \frac{1704 f w^2 x^5 \eta^{11}}{(-1+w(-1+\eta))^3 (x+\eta-x\eta)^3 (w+x+\eta-w\eta-x\eta)^3 (-1+\eta t)} + \\
& \frac{(-1+w(-1+\eta))^3 (x+\eta-x\eta)^3 (w+x+\eta-w\eta-x\eta)^3 (-1+\eta t)}{(-1+w(-1+\eta))^3 (x+\eta-x\eta)^3 (w+x+\eta-w\eta-x\eta)^3 (-1+\eta t)} +
\end{aligned}$$

$$\begin{aligned}
& \frac{1068 f w^3 x^5 \eta^{11}}{(-1+w(-1+\eta))^3 (x+\eta-x\eta)^3 (w+x+\eta-w\eta-x\eta)^3 (-1+\eta t)} + \\
& \frac{72 f w x^6 \eta^{11}}{(-1+w(-1+\eta))^3 (x+\eta-x\eta)^3 (w+x+\eta-w\eta-x\eta)^3 (-1+\eta t)} + \\
& \frac{356 f w^2 x^6 \eta^{11}}{(-1+w(-1+\eta))^3 (x+\eta-x\eta)^3 (w+x+\eta-w\eta-x\eta)^3 (-1+\eta t)} - \\
& \frac{36 f w^2 \eta^{12}}{(-1+w(-1+\eta))^3 (x+\eta-x\eta)^3 (w+x+\eta-w\eta-x\eta)^3 (-1+\eta t)} + \\
& \frac{108 f w^3 \eta^{12}}{(-1+w(-1+\eta))^3 (x+\eta-x\eta)^3 (w+x+\eta-w\eta-x\eta)^3 (-1+\eta t)} - \\
& \frac{108 f w^4 \eta^{12}}{(-1+w(-1+\eta))^3 (x+\eta-x\eta)^3 (w+x+\eta-w\eta-x\eta)^3 (-1+\eta t)} + \\
& \frac{36 f w^5 \eta^{12}}{(-1+w(-1+\eta))^3 (x+\eta-x\eta)^3 (w+x+\eta-w\eta-x\eta)^3 (-1+\eta t)} + \\
& \frac{216 f w^2 x \eta^{12}}{(-1+w(-1+\eta))^3 (x+\eta-x\eta)^3 (w+x+\eta-w\eta-x\eta)^3 (-1+\eta t)} - \\
& \frac{540 f w^3 x \eta^{12}}{(-1+w(-1+\eta))^3 (x+\eta-x\eta)^3 (w+x+\eta-w\eta-x\eta)^3 (-1+\eta t)} + \\
& \frac{432 f w^4 x \eta^{12}}{(-1+w(-1+\eta))^3 (x+\eta-x\eta)^3 (w+x+\eta-w\eta-x\eta)^3 (-1+\eta t)} - \\
& \frac{108 f w^5 x \eta^{12}}{(-1+w(-1+\eta))^3 (x+\eta-x\eta)^3 (w+x+\eta-w\eta-x\eta)^3 (-1+\eta t)} - \\
& \frac{540 f w^2 x^2 \eta^{12}}{(-1+w(-1+\eta))^3 (x+\eta-x\eta)^3 (w+x+\eta-w\eta-x\eta)^3 (-1+\eta t)} + \\
& \frac{1080 f w^3 x^2 \eta^{12}}{(-1+w(-1+\eta))^3 (x+\eta-x\eta)^3 (w+x+\eta-w\eta-x\eta)^3 (-1+\eta t)} - \\
& \frac{648 f w^4 x^2 \eta^{12}}{(-1+w(-1+\eta))^3 (x+\eta-x\eta)^3 (w+x+\eta-w\eta-x\eta)^3 (-1+\eta t)} + \\
& \frac{108 f w^5 x^2 \eta^{12}}{(-1+w(-1+\eta))^3 (x+\eta-x\eta)^3 (w+x+\eta-w\eta-x\eta)^3 (-1+\eta t)} + \\
& \frac{720 f w^2 x^3 \eta^{12}}{(-1+w(-1+\eta))^3 (x+\eta-x\eta)^3 (w+x+\eta-w\eta-x\eta)^3 (-1+\eta t)} - \\
& \frac{1080 f w^3 x^3 \eta^{12}}{(-1+w(-1+\eta))^3 (x+\eta-x\eta)^3 (w+x+\eta-w\eta-x\eta)^3 (-1+\eta t)} + \\
& \frac{432 f w^4 x^3 \eta^{12}}{(-1+w(-1+\eta))^3 (x+\eta-x\eta)^3 (w+x+\eta-w\eta-x\eta)^3 (-1+\eta t)} - \\
& \frac{36 f w^5 x^3 \eta^{12}}{(-1+w(-1+\eta))^3 (x+\eta-x\eta)^3 (w+x+\eta-w\eta-x\eta)^3 (-1+\eta t)} - \\
& \frac{(-1+w(-1+\eta))^3 (x+\eta-x\eta)^3 (w+x+\eta-w\eta-x\eta)^3 (-1+\eta t)}{(-1+w(-1+\eta))^3 (x+\eta-x\eta)^3 (w+x+\eta-w\eta-x\eta)^3 (-1+\eta t)}
\end{aligned}$$

$$\begin{aligned}
& \frac{540 f w^2 x^4 \eta^{12}}{(-1+w(-1+\eta))^3 (x+\eta-x\eta)^3 (w+x+\eta-w\eta-x\eta)^3 (-1+\eta t)} + \\
& \frac{540 f w^3 x^4 \eta^{12}}{(-1+w(-1+\eta))^3 (x+\eta-x\eta)^3 (w+x+\eta-w\eta-x\eta)^3 (-1+\eta t)} - \\
& \frac{108 f w^4 x^4 \eta^{12}}{(-1+w(-1+\eta))^3 (x+\eta-x\eta)^3 (w+x+\eta-w\eta-x\eta)^3 (-1+\eta t)} + \\
& \frac{216 f w^2 x^5 \eta^{12}}{(-1+w(-1+\eta))^3 (x+\eta-x\eta)^3 (w+x+\eta-w\eta-x\eta)^3 (-1+\eta t)} - \\
& \frac{108 f w^3 x^5 \eta^{12}}{(-1+w(-1+\eta))^3 (x+\eta-x\eta)^3 (w+x+\eta-w\eta-x\eta)^3 (-1+\eta t)} - \\
& \frac{36 f w^2 x^6 \eta^{12}}{(-1+w(-1+\eta))^3 (x+\eta-x\eta)^3 (w+x+\eta-w\eta-x\eta)^3 (-1+\eta t)} + \\
& \frac{76 f w}{(x(-1+\eta)-\eta) (w+x+\eta-w\eta-x\eta)^2 (-1+\eta t)} - \\
& \frac{4 f x}{(x(-1+\eta)-\eta) (w+x+\eta-w\eta-x\eta)^2 (-1+\eta t)} - \\
& \frac{228 f w \eta}{(x(-1+\eta)-\eta) (w+x+\eta-w\eta-x\eta)^2 (-1+\eta t)} + \\
& \frac{12 f x \eta}{(x(-1+\eta)-\eta) (w+x+\eta-w\eta-x\eta)^2 (-1+\eta t)} + \\
& \frac{228 f w \eta^2}{(x(-1+\eta)-\eta) (w+x+\eta-w\eta-x\eta)^2 (-1+\eta t)} - \\
& \frac{12 f x \eta^2}{(x(-1+\eta)-\eta) (w+x+\eta-w\eta-x\eta)^2 (-1+\eta t)} - \\
& \frac{76 f w \eta^3}{(x(-1+\eta)-\eta) (w+x+\eta-w\eta-x\eta)^2 (-1+\eta t)} + \\
& \frac{4 f x \eta^3}{(x(-1+\eta)-\eta) (w+x+\eta-w\eta-x\eta)^2 (-1+\eta t)} + \\
& \frac{12 f x^2}{(x+\eta-x\eta)^2 (w+x+\eta-w\eta-x\eta)^2 (-1+\eta t)} - \\
& \frac{48 f x^2 \eta}{(x+\eta-x\eta)^2 (w+x+\eta-w\eta-x\eta)^2 (-1+\eta t)} + \\
& \frac{72 f x^2 \eta^2}{(x+\eta-x\eta)^2 (w+x+\eta-w\eta-x\eta)^2 (-1+\eta t)} - \\
& \frac{48 f x^2 \eta^3}{(x+\eta-x\eta)^2 (w+x+\eta-w\eta-x\eta)^2 (-1+\eta t)} + \\
& \frac{12 f x^2 \eta^4}{(x+\eta-x\eta)^2 (w+x+\eta-w\eta-x\eta)^2 (-1+\eta t)} -
\end{aligned}$$

$$\begin{aligned}
& \frac{6 f x^2}{(x + \eta - x \eta)^3 (w + x + \eta - w \eta - x \eta) (-1 + \eta t)} - \\
& \frac{36 f x^2 \eta^2}{(x + \eta - x \eta)^3 (w + x + \eta - w \eta - x \eta) (-1 + \eta t)} - \\
& \frac{6 f x^2 \eta^4}{(x + \eta - x \eta)^3 (w + x + \eta - w \eta - x \eta) (-1 + \eta t)} - 64 f \theta l + \frac{152 f w \theta l}{(-1 + w (-1 + \eta))^3} + \\
& \frac{48 f \eta \theta l}{(-1 + w (-1 + \eta))^3} + \frac{12 f w^2 \eta \theta l}{(-1 + w (-1 + \eta))^3} + \frac{384 f w \eta^2 \theta l}{(-1 + w (-1 + \eta))^3} + \frac{40 f \eta^3 \theta l}{(-1 + w (-1 + \eta))^3} + \\
& \frac{4 f w^2 \eta^3 \theta l}{(-1 + w (-1 + \eta))^3} + \frac{4 f \theta l}{(1 + w - w \eta)^3} + \frac{4 f w^2 \theta l}{(1 + w - w \eta)^3} + \frac{420 f w \eta \theta l}{(1 + w - w \eta)^3} + \frac{84 f \eta^2 \theta l}{(1 + w - w \eta)^3} + \\
& \frac{12 f w^2 \eta^2 \theta l}{(1 + w - w \eta)^3} + \frac{116 f w \eta^3 \theta l}{(1 + w - w \eta)^3} - \frac{8 f \theta l}{(1 + w - w \eta)^2} - \frac{40 f w \theta l}{(1 + w - w \eta)^2} + \frac{16 f \eta \theta l}{(1 + w - w \eta)^2} + \\
& \frac{80 f w \eta \theta l}{(1 + w - w \eta)^2} - \frac{8 f \eta^2 \theta l}{(1 + w - w \eta)^2} - \frac{40 f w \eta^2 \theta l}{(1 + w - w \eta)^2} - \frac{6 f w^2 \theta l}{(w + x + \eta - w \eta - x \eta)^3} + \\
& \frac{4 f w x \theta l}{(w + x + \eta - w \eta - x \eta)^3} - \frac{2 f x^2 \theta l}{(w + x + \eta - w \eta - x \eta)^3} + \frac{60 f w x^2 \theta l}{(x (-1 + \eta) - \eta) (w + x + \eta - w \eta - x \eta)^3} - \\
& \frac{18 f w \eta \theta l}{(w + x + \eta - w \eta - x \eta)^3} + \frac{18 f w^2 \eta \theta l}{(w + x + \eta - w \eta - x \eta)^3} - \frac{14 f x \eta \theta l}{(w + x + \eta - w \eta - x \eta)^3} - \\
& \frac{12 f w x \eta \theta l}{(w + x + \eta - w \eta - x \eta)^3} + \frac{6 f x^2 \eta \theta l}{(w + x + \eta - w \eta - x \eta)^3} + \frac{60 f w x \eta \theta l}{(x (-1 + \eta) - \eta) (w + x + \eta - w \eta - x \eta)^3} - \\
& \frac{240 f w x^2 \eta \theta l}{(x (-1 + \eta) - \eta) (w + x + \eta - w \eta - x \eta)^3} + \frac{36 f w \eta^2 \theta l}{(w + x + \eta - w \eta - x \eta)^3} - \frac{18 f w^2 \eta^2 \theta l}{(w + x + \eta - w \eta - x \eta)^3} + \\
& \frac{28 f x \eta^2 \theta l}{(w + x + \eta - w \eta - x \eta)^3} + \frac{12 f w x \eta^2 \theta l}{(w + x + \eta - w \eta - x \eta)^3} - \frac{6 f x^2 \eta^2 \theta l}{(w + x + \eta - w \eta - x \eta)^3} - \\
& \frac{180 f w x \eta^2 \theta l}{(x (-1 + \eta) - \eta) (w + x + \eta - w \eta - x \eta)^3} + \frac{360 f w x^2 \eta^2 \theta l}{(x (-1 + \eta) - \eta) (w + x + \eta - w \eta - x \eta)^3} - \\
& \frac{18 f w \eta^3 \theta l}{(w + x + \eta - w \eta - x \eta)^3} + \frac{6 f w^2 \eta^3 \theta l}{(w + x + \eta - w \eta - x \eta)^3} - \frac{14 f x \eta^3 \theta l}{(w + x + \eta - w \eta - x \eta)^3} - \\
& \frac{4 f w x \eta^3 \theta l}{(w + x + \eta - w \eta - x \eta)^3} + \frac{2 f x^2 \eta^3 \theta l}{(w + x + \eta - w \eta - x \eta)^3} + \frac{180 f w x \eta^3 \theta l}{(x (-1 + \eta) - \eta) (w + x + \eta - w \eta - x \eta)^3} - \\
& \frac{240 f w x^2 \eta^3 \theta l}{(x (-1 + \eta) - \eta) (w + x + \eta - w \eta - x \eta)^3} - \frac{60 f w x \eta^4 \theta l}{(x (-1 + \eta) - \eta) (w + x + \eta - w \eta - x \eta)^3} + \\
& \frac{60 f w x^2 \eta^4 \theta l}{(x (-1 + \eta) - \eta) (w + x + \eta - w \eta - x \eta)^3} - \frac{76 f w \theta l}{(w + x + \eta - w \eta - x \eta)^2} + \\
& \frac{152 f w \eta \theta l}{(w + x + \eta - w \eta - x \eta)^2} - \frac{76 f w \eta^2 \theta l}{(w + x + \eta - w \eta - x \eta)^2} - \frac{30 f \theta l}{(1 + w - w \eta) (w + x + \eta - w \eta - x \eta)} - \\
& \frac{218 f w \theta l}{(1 + w - w \eta) (w + x + \eta - w \eta - x \eta)} - \frac{188 f x \theta l}{(1 + w - w \eta) (w + x + \eta - w \eta - x \eta)} -
\end{aligned}$$

$$\begin{aligned}
& \frac{158 f \eta \theta l}{(1+w-w \eta)(w+x+\eta-w \eta-x \eta)} + \frac{436 f w \eta \theta l}{(1+w-w \eta)(w+x+\eta-w \eta-x \eta)} + \\
& \frac{376 f x \eta \theta l}{(1+w-w \eta)(w+x+\eta-w \eta-x \eta)} + \frac{188 f \eta^2 \theta l}{(1+w-w \eta)(w+x+\eta-w \eta-x \eta)} - \\
& \frac{218 f w \eta^2 \theta l}{(1+w-w \eta)(w+x+\eta-w \eta-x \eta)} - \frac{188 f x \eta^2 \theta l}{(1+w-w \eta)(w+x+\eta-w \eta-x \eta)} + \\
& 32 f \theta l^2 + \frac{80 c \sigma^2 x \eta \theta l}{(-1+w(-1+\eta))(x(-1+\eta)-\eta)(w(-1+\eta)+x(-1+\eta)-\eta) \theta p} + \\
& \frac{120 c \sigma^2 w x \eta \theta l}{(-1+w(-1+\eta))(x(-1+\eta)-\eta)(w(-1+\eta)+x(-1+\eta)-\eta) \theta p} + \\
& \frac{40 c \sigma^2 w x \eta^3 \theta l}{(-1+w(-1+\eta))(x(-1+\eta)-\eta)(w(-1+\eta)+x(-1+\eta)-\eta) \theta p} - \\
& \frac{18 f w x^3 \theta l}{(x+\eta-x \eta)^3 (w+x+\eta-w \eta-x \eta)^3 \theta p} - \frac{36 f w x^2 \eta \theta l}{(x+\eta-x \eta)^3 (w+x+\eta-w \eta-x \eta)^3 \theta p} + \\
& \frac{108 f w x^3 \eta \theta l}{(x+\eta-x \eta)^3 (w+x+\eta-w \eta-x \eta)^3 \theta p} - \frac{18 f w x \eta^2 \theta l}{(x+\eta-x \eta)^3 (w+x+\eta-w \eta-x \eta)^3 \theta p} + \\
& \frac{180 f w x^2 \eta^2 \theta l}{(x+\eta-x \eta)^3 (w+x+\eta-w \eta-x \eta)^3 \theta p} - \frac{270 f w x^3 \eta^2 \theta l}{(x+\eta-x \eta)^3 (w+x+\eta-w \eta-x \eta)^3 \theta p} + \\
& \frac{72 f w x \eta^3 \theta l}{(x+\eta-x \eta)^3 (w+x+\eta-w \eta-x \eta)^3 \theta p} - \frac{360 f w x^2 \eta^3 \theta l}{(x+\eta-x \eta)^3 (w+x+\eta-w \eta-x \eta)^3 \theta p} + \\
& \frac{360 f w x^3 \eta^3 \theta l}{(x+\eta-x \eta)^3 (w+x+\eta-w \eta-x \eta)^3 \theta p} - \frac{108 f w x \eta^4 \theta l}{(x+\eta-x \eta)^3 (w+x+\eta-w \eta-x \eta)^3 \theta p} + \\
& \frac{360 f w x^2 \eta^4 \theta l}{(x+\eta-x \eta)^3 (w+x+\eta-w \eta-x \eta)^3 \theta p} - \frac{270 f w x^3 \eta^4 \theta l}{(x+\eta-x \eta)^3 (w+x+\eta-w \eta-x \eta)^3 \theta p} + \\
& \frac{72 f w x \eta^5 \theta l}{(x+\eta-x \eta)^3 (w+x+\eta-w \eta-x \eta)^3 \theta p} - \frac{180 f w x^2 \eta^5 \theta l}{(x+\eta-x \eta)^3 (w+x+\eta-w \eta-x \eta)^3 \theta p} + \\
& \frac{108 f w x^3 \eta^5 \theta l}{(x+\eta-x \eta)^3 (w+x+\eta-w \eta-x \eta)^3 \theta p} - \frac{18 f w x \eta^6 \theta l}{(x+\eta-x \eta)^3 (w+x+\eta-w \eta-x \eta)^3 \theta p} + \\
& \frac{36 f w x^2 \eta^6 \theta l}{(x+\eta-x \eta)^3 (w+x+\eta-w \eta-x \eta)^3 \theta p} - \frac{18 f w x^3 \eta^6 \theta l}{(x+\eta-x \eta)^3 (w+x+\eta-w \eta-x \eta)^3 \theta p} + \\
& \frac{12 f w^2 x^2 \theta l}{(x+\eta-x \eta)^2 (w+x+\eta-w \eta-x \eta)^3 \theta p} + \frac{72 f w x^3 \theta l}{(x+\eta-x \eta)^2 (w+x+\eta-w \eta-x \eta)^3 \theta p} + \\
& \frac{72 f w x^2 \eta \theta l}{(x+\eta-x \eta)^2 (w+x+\eta-w \eta-x \eta)^3 \theta p} - \frac{60 f w^2 x^2 \eta \theta l}{(x+\eta-x \eta)^2 (w+x+\eta-w \eta-x \eta)^3 \theta p} - \\
& \frac{360 f w x^3 \eta \theta l}{(x+\eta-x \eta)^2 (w+x+\eta-w \eta-x \eta)^3 \theta p} - \frac{288 f w x^2 \eta^2 \theta l}{(x+\eta-x \eta)^2 (w+x+\eta-w \eta-x \eta)^3 \theta p} + \\
& \frac{120 f w^2 x^2 \eta^2 \theta l}{(x+\eta-x \eta)^2 (w+x+\eta-w \eta-x \eta)^3 \theta p} + \frac{720 f w x^3 \eta^2 \theta l}{(x+\eta-x \eta)^2 (w+x+\eta-w \eta-x \eta)^3 \theta p} +
\end{aligned}$$



$$\begin{aligned}
& \frac{432 f w x^2 \eta^3 \theta l}{(x + \eta - x \eta)^2 (w + x + \eta - w \eta - x \eta)^3 \theta p} - \frac{120 f w^2 x^2 \eta^3 \theta l}{(x + \eta - x \eta)^2 (w + x + \eta - w \eta - x \eta)^3 \theta p} - \\
& \frac{720 f w x^3 \eta^3 \theta l}{(x + \eta - x \eta)^2 (w + x + \eta - w \eta - x \eta)^3 \theta p} - \frac{288 f w x^2 \eta^4 \theta l}{(x + \eta - x \eta)^2 (w + x + \eta - w \eta - x \eta)^3 \theta p} + \\
& \frac{60 f w^2 x^2 \eta^4 \theta l}{(x + \eta - x \eta)^2 (w + x + \eta - w \eta - x \eta)^3 \theta p} + \frac{360 f w x^3 \eta^4 \theta l}{(x + \eta - x \eta)^2 (w + x + \eta - w \eta - x \eta)^3 \theta p} + \\
& \frac{72 f w x^2 \eta^5 \theta l}{(x + \eta - x \eta)^2 (w + x + \eta - w \eta - x \eta)^3 \theta p} - \frac{12 f w^2 x^2 \eta^5 \theta l}{(x + \eta - x \eta)^2 (w + x + \eta - w \eta - x \eta)^3 \theta p} - \\
& \frac{72 f w x^3 \eta^5 \theta l}{(x + \eta - x \eta)^2 (w + x + \eta - w \eta - x \eta)^3 \theta p} + \frac{18 f w x \theta l}{(x + \eta - x \eta) (w + x + \eta - w \eta - x \eta)^3 \theta p} - \\
& \frac{58 f w^2 x \theta l}{(x + \eta - x \eta) (w + x + \eta - w \eta - x \eta)^3 \theta p} - \frac{120 f w x^2 \theta l}{(x + \eta - x \eta) (w + x + \eta - w \eta - x \eta)^3 \theta p} - \\
& \frac{50 f x^3 \theta l}{(x + \eta - x \eta) (w + x + \eta - w \eta - x \eta)^3 \theta p} - \frac{174 f w x \eta \theta l}{(x + \eta - x \eta) (w + x + \eta - w \eta - x \eta)^3 \theta p} + \\
& \frac{232 f w^2 x \eta \theta l}{(x + \eta - x \eta) (w + x + \eta - w \eta - x \eta)^3 \theta p} - \frac{94 f x^2 \eta \theta l}{(x + \eta - x \eta) (w + x + \eta - w \eta - x \eta)^3 \theta p} + \\
& \frac{480 f w x^2 \eta \theta l}{(x + \eta - x \eta) (w + x + \eta - w \eta - x \eta)^3 \theta p} - \frac{200 f x^3 \eta \theta l}{(x + \eta - x \eta) (w + x + \eta - w \eta - x \eta)^3 \theta p} - \\
& \frac{56 f x \eta^2 \theta l}{(x + \eta - x \eta) (w + x + \eta - w \eta - x \eta)^3 \theta p} + \frac{414 f w x \eta^2 \theta l}{(x + \eta - x \eta) (w + x + \eta - w \eta - x \eta)^3 \theta p} - \\
& \frac{348 f w^2 x \eta^2 \theta l}{(x + \eta - x \eta) (w + x + \eta - w \eta - x \eta)^3 \theta p} + \frac{282 f x^2 \eta^2 \theta l}{(x + \eta - x \eta) (w + x + \eta - w \eta - x \eta)^3 \theta p} - \\
& \frac{720 f w x^2 \eta^2 \theta l}{(x + \eta - x \eta) (w + x + \eta - w \eta - x \eta)^3 \theta p} - \frac{300 f x^3 \eta^2 \theta l}{(x + \eta - x \eta) (w + x + \eta - w \eta - x \eta)^3 \theta p} + \\
& \frac{112 f x \eta^3 \theta l}{(x + \eta - x \eta) (w + x + \eta - w \eta - x \eta)^3 \theta p} - \frac{378 f w x \eta^3 \theta l}{(x + \eta - x \eta) (w + x + \eta - w \eta - x \eta)^3 \theta p} + \\
& \frac{232 f w^2 x \eta^3 \theta l}{(x + \eta - x \eta) (w + x + \eta - w \eta - x \eta)^3 \theta p} - \frac{282 f x^2 \eta^3 \theta l}{(x + \eta - x \eta) (w + x + \eta - w \eta - x \eta)^3 \theta p} + \\
& \frac{480 f w x^2 \eta^3 \theta l}{(x + \eta - x \eta) (w + x + \eta - w \eta - x \eta)^3 \theta p} - \frac{200 f x^3 \eta^3 \theta l}{(x + \eta - x \eta) (w + x + \eta - w \eta - x \eta)^3 \theta p} - \\
& \frac{56 f x \eta^4 \theta l}{(x + \eta - x \eta) (w + x + \eta - w \eta - x \eta)^3 \theta p} + \frac{120 f w x \eta^4 \theta l}{(x + \eta - x \eta) (w + x + \eta - w \eta - x \eta)^3 \theta p} - \\
& \frac{58 f w^2 x \eta^4 \theta l}{(x + \eta - x \eta) (w + x + \eta - w \eta - x \eta)^3 \theta p} + \frac{94 f x^2 \eta^4 \theta l}{(x + \eta - x \eta) (w + x + \eta - w \eta - x \eta)^3 \theta p} - \\
& \frac{120 f w x^2 \eta^4 \theta l}{(x + \eta - x \eta) (w + x + \eta - w \eta - x \eta)^3 \theta p} - \frac{50 f x^3 \eta^4 \theta l}{(x + \eta - x \eta) (w + x + \eta - w \eta - x \eta)^3 \theta p} - \\
& \frac{12 f x^3 \theta l}{(x + \eta - x \eta)^2 (w + x + \eta - w \eta - x \eta)^2 \theta p} + \frac{48 f x^3 \eta \theta l}{(x + \eta - x \eta)^2 (w + x + \eta - w \eta - x \eta)^2 \theta p} -
\end{aligned}$$

$$\begin{aligned}
& \frac{72 f x^3 \eta^2 \theta l}{(x + \eta - x \eta)^2 (w + x + \eta - w \eta - x \eta)^2 \theta p} + \frac{48 f x^3 \eta^3 \theta l}{(x + \eta - x \eta)^2 (w + x + \eta - w \eta - x \eta)^2 \theta p} - \\
& \frac{12 f x^3 \eta^4 \theta l}{(x + \eta - x \eta)^2 (w + x + \eta - w \eta - x \eta)^2 \theta p} + \frac{72 f w x \theta l}{(x + \eta - x \eta) (w + x + \eta - w \eta - x \eta)^2 \theta p} + \\
& \frac{8 f x^2 \theta l}{(x + \eta - x \eta) (w + x + \eta - w \eta - x \eta)^2 \theta p} - \frac{216 f w x \eta \theta l}{(x + \eta - x \eta) (w + x + \eta - w \eta - x \eta)^2 \theta p} - \\
& \frac{24 f x^2 \eta \theta l}{(x + \eta - x \eta) (w + x + \eta - w \eta - x \eta)^2 \theta p} + \frac{216 f w x \eta^2 \theta l}{(x + \eta - x \eta) (w + x + \eta - w \eta - x \eta)^2 \theta p} + \\
& \frac{24 f x^2 \eta^2 \theta l}{(x + \eta - x \eta) (w + x + \eta - w \eta - x \eta)^2 \theta p} - \frac{72 f w x \eta^3 \theta l}{(x + \eta - x \eta) (w + x + \eta - w \eta - x \eta)^2 \theta p} - \\
& \frac{8 f x^2 \eta^3 \theta l}{(x + \eta - x \eta) (w + x + \eta - w \eta - x \eta)^2 \theta p} + \frac{40 c \sigma^2 x \theta l}{(1 + w - w \eta) (x + \eta - x \eta) (w + x + \eta - w \eta - x \eta) \theta p} + \\
& \frac{40 c \sigma^2 w x \theta l}{(1 + w - w \eta) (x + \eta - x \eta) (w + x + \eta - w \eta - x \eta) \theta p} + \\
& \frac{40 c \sigma^2 x \eta^2 \theta l}{(1 + w - w \eta) (x + \eta - x \eta) (w + x + \eta - w \eta - x \eta) \theta p} + \\
& \frac{120 c \sigma^2 w x \eta^2 \theta l}{(1 + w - w \eta) (x + \eta - x \eta) (w + x + \eta - w \eta - x \eta) \theta p} + \\
& \frac{6 f x^3 \theta l}{(x + \eta - x \eta)^3 (\theta p - (-1 + w + x) \times (-1 + \eta) \theta p)} + \\
& \frac{18 f x^2 \eta \theta l}{(x + \eta - x \eta)^3 (\theta p - (-1 + w + x) \times (-1 + \eta) \theta p)} - \\
& \frac{24 f x^3 \eta \theta l}{(x + \eta - x \eta)^3 (\theta p - (-1 + w + x) \times (-1 + \eta) \theta p)} - \\
& \frac{54 f x^2 \eta^2 \theta l}{(x + \eta - x \eta)^3 (\theta p - (-1 + w + x) \times (-1 + \eta) \theta p)} + \\
& \frac{36 f x^3 \eta^2 \theta l}{(x + \eta - x \eta)^3 (\theta p - (-1 + w + x) \times (-1 + \eta) \theta p)} + \\
& \frac{54 f x^2 \eta^3 \theta l}{(x + \eta - x \eta)^3 (\theta p - (-1 + w + x) \times (-1 + \eta) \theta p)} - \\
& \frac{24 f x^3 \eta^3 \theta l}{(x + \eta - x \eta)^3 (\theta p - (-1 + w + x) \times (-1 + \eta) \theta p)} - \\
& \frac{18 f x^2 \eta^4 \theta l}{(x + \eta - x \eta)^3 (\theta p - (-1 + w + x) \times (-1 + \eta) \theta p)} + \\
& \frac{6 f x^3 \eta^4 \theta l}{(x + \eta - x \eta)^3 (\theta p - (-1 + w + x) \times (-1 + \eta) \theta p)} + \\
& \frac{8 f x^2 \theta l}{(x + \eta - x \eta)^2 (\theta p - (-1 + w + x) \times (-1 + \eta) \theta p)} -
\end{aligned}$$

$$\begin{aligned}
& \frac{24 f x^2 \eta \theta l}{(x + \eta - x \eta)^2 (\theta p - (-1 + w + x) \times (-1 + \eta) \theta p)} + \\
& \frac{24 f x^2 \eta^2 \theta l}{(x + \eta - x \eta)^2 (\theta p - (-1 + w + x) \times (-1 + \eta) \theta p)} - \\
& \frac{8 f x^2 \eta^3 \theta l}{(x + \eta - x \eta)^2 (\theta p - (-1 + w + x) \times (-1 + \eta) \theta p)} + \\
& \frac{32 c \sigma^2 \eta \mu 1}{(-1 + w (-1 + \eta)) (x (-1 + \eta) - \eta) (w (-1 + \eta) + x (-1 + \eta) - \eta)} + \\
& \frac{48 c \sigma^2 w \eta \mu 1}{(-1 + w (-1 + \eta)) (x (-1 + \eta) - \eta) (w (-1 + \eta) + x (-1 + \eta) - \eta)} + \\
& \frac{16 c \sigma^2 w \eta^3 \mu 1}{(-1 + w (-1 + \eta)) (x (-1 + \eta) - \eta) (w (-1 + \eta) + x (-1 + \eta) - \eta)} - \\
& \frac{64 c \sigma^2 w \mu 1}{(1 + w - w \eta)^2 (w + x + \eta - w \eta - x \eta)^2} - \frac{96 c \sigma^2 w^2 \mu 1}{(1 + w - w \eta)^2 (w + x + \eta - w \eta - x \eta)^2} - \\
& \frac{64 c \sigma^2 x \mu 1}{(1 + w - w \eta)^2 (w + x + \eta - w \eta - x \eta)^2} - \frac{64 c \sigma^2 w x \mu 1}{(1 + w - w \eta)^2 (w + x + \eta - w \eta - x \eta)^2} + \\
& \frac{64 c \sigma^2 w^2 x \mu 1}{(1 + w - w \eta)^2 (w + x + \eta - w \eta - x \eta)^2} + \frac{32 c \sigma^2 x^2 \mu 1}{(1 + w - w \eta)^2 (w + x + \eta - w \eta - x \eta)^2} + \\
& \frac{64 c \sigma^2 w x^2 \mu 1}{(1 + w - w \eta)^2 (w + x + \eta - w \eta - x \eta)^2} - \frac{64 c \sigma^2 \eta \mu 1}{(1 + w - w \eta)^2 (w + x + \eta - w \eta - x \eta)^2} + \\
& \frac{64 c \sigma^2 w \eta \mu 1}{(1 + w - w \eta)^2 (w + x + \eta - w \eta - x \eta)^2} + \frac{368 c \sigma^2 w^2 \eta \mu 1}{(1 + w - w \eta)^2 (w + x + \eta - w \eta - x \eta)^2} + \\
& \frac{192 c \sigma^2 x \eta \mu 1}{(1 + w - w \eta)^2 (w + x + \eta - w \eta - x \eta)^2} + \frac{352 c \sigma^2 w x \eta \mu 1}{(1 + w - w \eta)^2 (w + x + \eta - w \eta - x \eta)^2} - \\
& \frac{256 c \sigma^2 w^2 x \eta \mu 1}{(1 + w - w \eta)^2 (w + x + \eta - w \eta - x \eta)^2} - \frac{80 c \sigma^2 x^2 \eta \mu 1}{(1 + w - w \eta)^2 (w + x + \eta - w \eta - x \eta)^2} - \\
& \frac{256 c \sigma^2 w x^2 \eta \mu 1}{(1 + w - w \eta)^2 (w + x + \eta - w \eta - x \eta)^2} + \frac{96 c \sigma^2 \eta^2 \mu 1}{(1 + w - w \eta)^2 (w + x + \eta - w \eta - x \eta)^2} + \\
& \frac{160 c \sigma^2 w \eta^2 \mu 1}{(1 + w - w \eta)^2 (w + x + \eta - w \eta - x \eta)^2} - \frac{528 c \sigma^2 w^2 \eta^2 \mu 1}{(1 + w - w \eta)^2 (w + x + \eta - w \eta - x \eta)^2} - \\
& \frac{160 c \sigma^2 x \eta^2 \mu 1}{(1 + w - w \eta)^2 (w + x + \eta - w \eta - x \eta)^2} - \frac{672 c \sigma^2 w x \eta^2 \mu 1}{(1 + w - w \eta)^2 (w + x + \eta - w \eta - x \eta)^2} + \\
& \frac{384 c \sigma^2 w^2 x \eta^2 \mu 1}{(1 + w - w \eta)^2 (w + x + \eta - w \eta - x \eta)^2} + \frac{48 c \sigma^2 x^2 \eta^2 \mu 1}{(1 + w - w \eta)^2 (w + x + \eta - w \eta - x \eta)^2} + \\
& \frac{384 c \sigma^2 w x^2 \eta^2 \mu 1}{(1 + w - w \eta)^2 (w + x + \eta - w \eta - x \eta)^2} - \frac{16 c \sigma^2 \eta^3 \mu 1}{(1 + w - w \eta)^2 (w + x + \eta - w \eta - x \eta)^2} - \\
& \frac{256 c \sigma^2 w \eta^3 \mu 1}{(1 + w - w \eta)^2 (w + x + \eta - w \eta - x \eta)^2} + \frac{336 c \sigma^2 w^2 \eta^3 \mu 1}{(1 + w - w \eta)^2 (w + x + \eta - w \eta - x \eta)^2} +
\end{aligned}$$

$$\begin{aligned}
& \frac{544 c \sigma^2 w x \eta^3 \mu 1}{(1+w-w \eta)^2 (w+x+\eta-w \eta-x \eta)^2} - \frac{256 c \sigma^2 w^2 x \eta^3 \mu 1}{(1+w-w \eta)^2 (w+x+\eta-w \eta-x \eta)^2} + \\
& \frac{16 c \sigma^2 x^2 \eta^3 \mu 1}{(1+w-w \eta)^2 (w+x+\eta-w \eta-x \eta)^2} - \frac{256 c \sigma^2 w x^2 \eta^3 \mu 1}{(1+w-w \eta)^2 (w+x+\eta-w \eta-x \eta)^2} - \\
& \frac{16 c \sigma^2 \eta^4 \mu 1}{(1+w-w \eta)^2 (w+x+\eta-w \eta-x \eta)^2} + \frac{96 c \sigma^2 w \eta^4 \mu 1}{(1+w-w \eta)^2 (w+x+\eta-w \eta-x \eta)^2} - \\
& \frac{80 c \sigma^2 w^2 \eta^4 \mu 1}{(1+w-w \eta)^2 (w+x+\eta-w \eta-x \eta)^2} + \frac{32 c \sigma^2 x \eta^4 \mu 1}{(1+w-w \eta)^2 (w+x+\eta-w \eta-x \eta)^2} - \\
& \frac{160 c \sigma^2 w x \eta^4 \mu 1}{(1+w-w \eta)^2 (w+x+\eta-w \eta-x \eta)^2} + \frac{64 c \sigma^2 w^2 x \eta^4 \mu 1}{(1+w-w \eta)^2 (w+x+\eta-w \eta-x \eta)^2} - \\
& \frac{16 c \sigma^2 x^2 \eta^4 \mu 1}{(1+w-w \eta)^2 (w+x+\eta-w \eta-x \eta)^2} + \frac{64 c \sigma^2 w x^2 \eta^4 \mu 1}{(1+w-w \eta)^2 (w+x+\eta-w \eta-x \eta)^2} + \\
& \frac{16 c \sigma^2 \mu 1}{(1+w-w \eta) (x+\eta-x \eta) (w+x+\eta-w \eta-x \eta)} + \\
& \frac{16 c \sigma^2 w \mu 1}{(1+w-w \eta) (x+\eta-x \eta) (w+x+\eta-w \eta-x \eta)} + \\
& \frac{16 c \sigma^2 \eta^2 \mu 1}{(1+w-w \eta) (x+\eta-x \eta) (w+x+\eta-w \eta-x \eta)} + \\
& \frac{48 c \sigma^2 w \eta^2 \mu 1}{(1+w-w \eta) (x+\eta-x \eta) (w+x+\eta-w \eta-x \eta)} - \\
& \frac{16 c \sigma^2 \mu 1}{(-1+w(-1+\eta)) (x(-1+\eta)-\eta) (w(-1+\eta)+x(-1+\eta)-\eta) (-1+\eta \mathfrak{t})} - \\
& \frac{16 c \sigma^2 w \mu 1}{(-1+w(-1+\eta)) (x(-1+\eta)-\eta) (w(-1+\eta)+x(-1+\eta)-\eta) (-1+\eta \mathfrak{t})} + \\
& \frac{16 c \sigma^2 w x \mu 1}{(-1+w(-1+\eta)) (x(-1+\eta)-\eta) (w(-1+\eta)+x(-1+\eta)-\eta) (-1+\eta \mathfrak{t})} + \\
& \frac{16 c \sigma^2 x^2 \mu 1}{(-1+w(-1+\eta)) (x(-1+\eta)-\eta) (w(-1+\eta)+x(-1+\eta)-\eta) (-1+\eta \mathfrak{t})} + \\
& \frac{32 c \sigma^2 \eta \mu 1}{(-1+w(-1+\eta)) (x(-1+\eta)-\eta) (w(-1+\eta)+x(-1+\eta)-\eta) (-1+\eta \mathfrak{t})} + \\
& \frac{64 c \sigma^2 w \eta \mu 1}{(-1+w(-1+\eta)) (x(-1+\eta)-\eta) (w(-1+\eta)+x(-1+\eta)-\eta) (-1+\eta \mathfrak{t})} + \\
& \frac{32 c \sigma^2 x \eta \mu 1}{(-1+w(-1+\eta)) (x(-1+\eta)-\eta) (w(-1+\eta)+x(-1+\eta)-\eta) (-1+\eta \mathfrak{t})} - \\
& \frac{64 c \sigma^2 w x \eta \mu 1}{(-1+w(-1+\eta)) (x(-1+\eta)-\eta) (w(-1+\eta)+x(-1+\eta)-\eta) (-1+\eta \mathfrak{t})} - \\
& \frac{64 c \sigma^2 x^2 \eta \mu 1}{(-1+w(-1+\eta)) (x(-1+\eta)-\eta) (w(-1+\eta)+x(-1+\eta)-\eta) (-1+\eta \mathfrak{t})} -
\end{aligned}$$

$$\begin{aligned}
& \frac{96 c \sigma^2 w \eta^2 \mu 1}{(-1+w(-1+\eta))(x(-1+\eta)-\eta)(w(-1+\eta)+x(-1+\eta)-\eta)(-1+\eta t)} - \\
& \frac{96 c \sigma^2 x \eta^2 \mu 1}{(-1+w(-1+\eta))(x(-1+\eta)-\eta)(w(-1+\eta)+x(-1+\eta)-\eta)(-1+\eta t)} + \\
& \frac{96 c \sigma^2 w x \eta^2 \mu 1}{(-1+w(-1+\eta))(x(-1+\eta)-\eta)(w(-1+\eta)+x(-1+\eta)-\eta)(-1+\eta t)} + \\
& \frac{96 c \sigma^2 x^2 \eta^2 \mu 1}{(-1+w(-1+\eta))(x(-1+\eta)-\eta)(w(-1+\eta)+x(-1+\eta)-\eta)(-1+\eta t)} - \\
& \frac{32 c \sigma^2 \eta^3 \mu 1}{(-1+w(-1+\eta))(x(-1+\eta)-\eta)(w(-1+\eta)+x(-1+\eta)-\eta)(-1+\eta t)} + \\
& \frac{64 c \sigma^2 w \eta^3 \mu 1}{(-1+w(-1+\eta))(x(-1+\eta)-\eta)(w(-1+\eta)+x(-1+\eta)-\eta)(-1+\eta t)} + \\
& \frac{96 c \sigma^2 x \eta^3 \mu 1}{(-1+w(-1+\eta))(x(-1+\eta)-\eta)(w(-1+\eta)+x(-1+\eta)-\eta)(-1+\eta t)} - \\
& \frac{64 c \sigma^2 w x \eta^3 \mu 1}{(-1+w(-1+\eta))(x(-1+\eta)-\eta)(w(-1+\eta)+x(-1+\eta)-\eta)(-1+\eta t)} - \\
& \frac{64 c \sigma^2 x^2 \eta^3 \mu 1}{(-1+w(-1+\eta))(x(-1+\eta)-\eta)(w(-1+\eta)+x(-1+\eta)-\eta)(-1+\eta t)} + \\
& \frac{16 c \sigma^2 \eta^4 \mu 1}{(-1+w(-1+\eta))(x(-1+\eta)-\eta)(w(-1+\eta)+x(-1+\eta)-\eta)(-1+\eta t)} - \\
& \frac{16 c \sigma^2 w \eta^4 \mu 1}{(-1+w(-1+\eta))(x(-1+\eta)-\eta)(w(-1+\eta)+x(-1+\eta)-\eta)(-1+\eta t)} - \\
& \frac{32 c \sigma^2 x \eta^4 \mu 1}{(-1+w(-1+\eta))(x(-1+\eta)-\eta)(w(-1+\eta)+x(-1+\eta)-\eta)(-1+\eta t)} + \\
& \frac{16 c \sigma^2 w x \eta^4 \mu 1}{(-1+w(-1+\eta))(x(-1+\eta)-\eta)(w(-1+\eta)+x(-1+\eta)-\eta)(-1+\eta t)} + \\
& \frac{16 c \sigma^2 x^2 \eta^4 \mu 1}{(-1+w(-1+\eta))(x(-1+\eta)-\eta)(w(-1+\eta)+x(-1+\eta)-\eta)(-1+\eta t)} + \\
& \frac{16 c \sigma^2 x \theta l \mu 1}{(-1+w(-1+\eta))(x(-1+\eta)-\eta)(w(-1+\eta)+x(-1+\eta)-\eta) \theta p} + \\
& \frac{16 c \sigma^2 w x \theta l \mu 1}{(-1+w(-1+\eta))(x(-1+\eta)-\eta)(w(-1+\eta)+x(-1+\eta)-\eta) \theta p} + \\
& \frac{16 c \sigma^2 x \eta^2 \theta l \mu 1}{(-1+w(-1+\eta))(x(-1+\eta)-\eta)(w(-1+\eta)+x(-1+\eta)-\eta) \theta p} + \\
& \frac{48 c \sigma^2 w x \eta^2 \theta l \mu 1}{(-1+w(-1+\eta))(x(-1+\eta)-\eta)(w(-1+\eta)+x(-1+\eta)-\eta) \theta p} + \\
& \frac{32 c \sigma^2 x \eta \theta l \mu 1}{(1+w-w \eta)(x+\eta-x \eta)(w+x+\eta-w \eta-x \eta) \theta p} + \\
& \frac{48 c \sigma^2 w x \eta \theta l \mu 1}{(1+w-w \eta)(x+\eta-x \eta)(w+x+\eta-w \eta-x \eta) \theta p} +
\end{aligned}$$

$$\begin{aligned}
& \frac{16 c \sigma^2 w x \eta^3 \theta l \mu 1}{(1+w-w \eta)(x+\eta-x \eta)(w+x+\eta-w \eta-x \eta) \theta p} + \\
& \frac{88 c \sigma^2 \mu 1^2}{(-1+w(-1+\eta))(x(-1+\eta)-\eta)(w(-1+\eta)+x(-1+\eta)-\eta)} + \\
& \frac{88 c \sigma^2 w \mu 1^2}{(-1+w(-1+\eta))(x(-1+\eta)-\eta)(w(-1+\eta)+x(-1+\eta)-\eta)} + \\
& \frac{88 c \sigma^2 \eta^2 \mu 1^2}{(-1+w(-1+\eta))(x(-1+\eta)-\eta)(w(-1+\eta)+x(-1+\eta)-\eta)} + \\
& \frac{264 c \sigma^2 w \eta^2 \mu 1^2}{(-1+w(-1+\eta))(x(-1+\eta)-\eta)(w(-1+\eta)+x(-1+\eta)-\eta)} + \\
& \frac{16 c \sigma^2 w \mu 1^2}{(1+w-w \eta)^2 (w+x+\eta-w \eta-x \eta)^2} - \frac{16 c \sigma^2 w^2 \mu 1^2}{(1+w-w \eta)^2 (w+x+\eta-w \eta-x \eta)^2} + \\
& \frac{16 c \sigma^2 x \mu 1^2}{(1+w-w \eta)^2 (w+x+\eta-w \eta-x \eta)^2} - \frac{64 c \sigma^2 w x \mu 1^2}{(1+w-w \eta)^2 (w+x+\eta-w \eta-x \eta)^2} - \\
& \frac{16 c \sigma^2 w^2 x \mu 1^2}{(1+w-w \eta)^2 (w+x+\eta-w \eta-x \eta)^2} - \frac{48 c \sigma^2 x^2 \mu 1^2}{(1+w-w \eta)^2 (w+x+\eta-w \eta-x \eta)^2} - \\
& \frac{16 c \sigma^2 w x^2 \mu 1^2}{(1+w-w \eta)^2 (w+x+\eta-w \eta-x \eta)^2} + \frac{16 c \sigma^2 \eta \mu 1^2}{(1+w-w \eta)^2 (w+x+\eta-w \eta-x \eta)^2} - \\
& \frac{96 c \sigma^2 w \eta \mu 1^2}{(1+w-w \eta)^2 (w+x+\eta-w \eta-x \eta)^2} + \frac{48 c \sigma^2 w^2 \eta \mu 1^2}{(1+w-w \eta)^2 (w+x+\eta-w \eta-x \eta)^2} - \\
& \frac{128 c \sigma^2 x \eta \mu 1^2}{(1+w-w \eta)^2 (w+x+\eta-w \eta-x \eta)^2} + \frac{192 c \sigma^2 w x \eta \mu 1^2}{(1+w-w \eta)^2 (w+x+\eta-w \eta-x \eta)^2} + \\
& \frac{64 c \sigma^2 w^2 x \eta \mu 1^2}{(1+w-w \eta)^2 (w+x+\eta-w \eta-x \eta)^2} + \frac{160 c \sigma^2 x^2 \eta \mu 1^2}{(1+w-w \eta)^2 (w+x+\eta-w \eta-x \eta)^2} + \\
& \frac{64 c \sigma^2 w x^2 \eta \mu 1^2}{(1+w-w \eta)^2 (w+x+\eta-w \eta-x \eta)^2} - \frac{64 c \sigma^2 \eta^2 \mu 1^2}{(1+w-w \eta)^2 (w+x+\eta-w \eta-x \eta)^2} + \\
& \frac{160 c \sigma^2 w \eta^2 \mu 1^2}{(1+w-w \eta)^2 (w+x+\eta-w \eta-x \eta)^2} - \frac{48 c \sigma^2 w^2 \eta^2 \mu 1^2}{(1+w-w \eta)^2 (w+x+\eta-w \eta-x \eta)^2} + \\
& \frac{240 c \sigma^2 x \eta^2 \mu 1^2}{(1+w-w \eta)^2 (w+x+\eta-w \eta-x \eta)^2} - \frac{192 c \sigma^2 w x \eta^2 \mu 1^2}{(1+w-w \eta)^2 (w+x+\eta-w \eta-x \eta)^2} - \\
& \frac{96 c \sigma^2 w^2 x \eta^2 \mu 1^2}{(1+w-w \eta)^2 (w+x+\eta-w \eta-x \eta)^2} - \frac{192 c \sigma^2 x^2 \eta^2 \mu 1^2}{(1+w-w \eta)^2 (w+x+\eta-w \eta-x \eta)^2} - \\
& \frac{96 c \sigma^2 w x^2 \eta^2 \mu 1^2}{(1+w-w \eta)^2 (w+x+\eta-w \eta-x \eta)^2} + \frac{64 c \sigma^2 \eta^3 \mu 1^2}{(1+w-w \eta)^2 (w+x+\eta-w \eta-x \eta)^2} - \\
& \frac{96 c \sigma^2 w \eta^3 \mu 1^2}{(1+w-w \eta)^2 (w+x+\eta-w \eta-x \eta)^2} + \frac{16 c \sigma^2 w^2 \eta^3 \mu 1^2}{(1+w-w \eta)^2 (w+x+\eta-w \eta-x \eta)^2} - \\
& \frac{160 c \sigma^2 x \eta^3 \mu 1^2}{(1+w-w \eta)^2 (w+x+\eta-w \eta-x \eta)^2} + \frac{64 c \sigma^2 w x \eta^3 \mu 1^2}{(1+w-w \eta)^2 (w+x+\eta-w \eta-x \eta)^2} +
\end{aligned}$$

$$\begin{aligned}
& \frac{64 c \sigma^2 w^2 x \eta^3 \mu 1^2}{(1+w-w \eta)^2 (w+x+\eta-w \eta-x \eta)^2} + \frac{96 c \sigma^2 x^2 \eta^3 \mu 1^2}{(1+w-w \eta)^2 (w+x+\eta-w \eta-x \eta)^2} + \\
& \frac{64 c \sigma^2 w x^2 \eta^3 \mu 1^2}{(1+w-w \eta)^2 (w+x+\eta-w \eta-x \eta)^2} - \frac{16 c \sigma^2 \eta^4 \mu 1^2}{(1+w-w \eta)^2 (w+x+\eta-w \eta-x \eta)^2} + \\
& \frac{16 c \sigma^2 w \eta^4 \mu 1^2}{(1+w-w \eta)^2 (w+x+\eta-w \eta-x \eta)^2} + \frac{32 c \sigma^2 x \eta^4 \mu 1^2}{(1+w-w \eta)^2 (w+x+\eta-w \eta-x \eta)^2} - \\
& \frac{16 c \sigma^2 w^2 x \eta^4 \mu 1^2}{(1+w-w \eta)^2 (w+x+\eta-w \eta-x \eta)^2} - \frac{16 c \sigma^2 x^2 \eta^4 \mu 1^2}{(1+w-w \eta)^2 (w+x+\eta-w \eta-x \eta)^2} - \\
& \frac{16 c \sigma^2 w x^2 \eta^4 \mu 1^2}{(1+w-w \eta)^2 (w+x+\eta-w \eta-x \eta)^2} + \frac{176 c \sigma^2 \eta \mu 1^2}{(1+w-w \eta) (x+\eta-x \eta) (w+x+\eta-w \eta-x \eta)} + \\
& \frac{264 c \sigma^2 w \eta \mu 1^2}{(1+w-w \eta) (x+\eta-x \eta) (w+x+\eta-w \eta-x \eta)} + \\
& \frac{88 c \sigma^2 w \eta^3 \mu 1^2}{(1+w-w \eta) (x+\eta-x \eta) (w+x+\eta-w \eta-x \eta)} + \\
& \frac{88 c \sigma^2 \mu 1^2}{(-1+w(-1+\eta)) (x(-1+\eta)-\eta) (w(-1+\eta)+x(-1+\eta)-\eta) (-1+\eta \mathfrak{t})} + \\
& \frac{88 c \sigma^2 w \mu 1^2}{(-1+w(-1+\eta)) (x(-1+\eta)-\eta) (w(-1+\eta)+x(-1+\eta)-\eta) (-1+\eta \mathfrak{t})} + \\
& \frac{56 c \sigma^2 w x \mu 1^2}{(-1+w(-1+\eta)) (x(-1+\eta)-\eta) (w(-1+\eta)+x(-1+\eta)-\eta) (-1+\eta \mathfrak{t})} + \\
& \frac{56 c \sigma^2 x^2 \mu 1^2}{(-1+w(-1+\eta)) (x(-1+\eta)-\eta) (w(-1+\eta)+x(-1+\eta)-\eta) (-1+\eta \mathfrak{t})} - \\
& \frac{176 c \sigma^2 \eta \mu 1^2}{(-1+w(-1+\eta)) (x(-1+\eta)-\eta) (w(-1+\eta)+x(-1+\eta)-\eta) (-1+\eta \mathfrak{t})} - \\
& \frac{208 c \sigma^2 w \eta \mu 1^2}{(-1+w(-1+\eta)) (x(-1+\eta)-\eta) (w(-1+\eta)+x(-1+\eta)-\eta) (-1+\eta \mathfrak{t})} + \\
& \frac{112 c \sigma^2 x \eta \mu 1^2}{(-1+w(-1+\eta)) (x(-1+\eta)-\eta) (w(-1+\eta)+x(-1+\eta)-\eta) (-1+\eta \mathfrak{t})} - \\
& \frac{224 c \sigma^2 w x \eta \mu 1^2}{(-1+w(-1+\eta)) (x(-1+\eta)-\eta) (w(-1+\eta)+x(-1+\eta)-\eta) (-1+\eta \mathfrak{t})} - \\
& \frac{224 c \sigma^2 x^2 \eta \mu 1^2}{(-1+w(-1+\eta)) (x(-1+\eta)-\eta) (w(-1+\eta)+x(-1+\eta)-\eta) (-1+\eta \mathfrak{t})} + \\
& \frac{144 c \sigma^2 \eta^2 \mu 1^2}{(-1+w(-1+\eta)) (x(-1+\eta)-\eta) (w(-1+\eta)+x(-1+\eta)-\eta) (-1+\eta \mathfrak{t})} + \\
& \frac{96 c \sigma^2 w \eta^2 \mu 1^2}{(-1+w(-1+\eta)) (x(-1+\eta)-\eta) (w(-1+\eta)+x(-1+\eta)-\eta) (-1+\eta \mathfrak{t})} - \\
& \frac{336 c \sigma^2 x \eta^2 \mu 1^2}{(-1+w(-1+\eta)) (x(-1+\eta)-\eta) (w(-1+\eta)+x(-1+\eta)-\eta) (-1+\eta \mathfrak{t})} +
\end{aligned}$$

$$\begin{aligned}
& \frac{336 c \sigma^2 w x \eta^2 \mu 1^2}{(-1+w(-1+\eta))(x(-1+\eta)-\eta)(w(-1+\eta)+x(-1+\eta)-\eta)(-1+\eta t)} + \\
& \frac{336 c \sigma^2 x^2 \eta^2 \mu 1^2}{(-1+w(-1+\eta))(x(-1+\eta)-\eta)(w(-1+\eta)+x(-1+\eta)-\eta)(-1+\eta t)} - \\
& \frac{112 c \sigma^2 \eta^3 \mu 1^2}{(-1+w(-1+\eta))(x(-1+\eta)-\eta)(w(-1+\eta)+x(-1+\eta)-\eta)(-1+\eta t)} + \\
& \frac{80 c \sigma^2 w \eta^3 \mu 1^2}{(-1+w(-1+\eta))(x(-1+\eta)-\eta)(w(-1+\eta)+x(-1+\eta)-\eta)(-1+\eta t)} + \\
& \frac{336 c \sigma^2 x \eta^3 \mu 1^2}{(-1+w(-1+\eta))(x(-1+\eta)-\eta)(w(-1+\eta)+x(-1+\eta)-\eta)(-1+\eta t)} - \\
& \frac{224 c \sigma^2 w x \eta^3 \mu 1^2}{(-1+w(-1+\eta))(x(-1+\eta)-\eta)(w(-1+\eta)+x(-1+\eta)-\eta)(-1+\eta t)} - \\
& \frac{224 c \sigma^2 x^2 \eta^3 \mu 1^2}{(-1+w(-1+\eta))(x(-1+\eta)-\eta)(w(-1+\eta)+x(-1+\eta)-\eta)(-1+\eta t)} + \\
& \frac{56 c \sigma^2 \eta^4 \mu 1^2}{(-1+w(-1+\eta))(x(-1+\eta)-\eta)(w(-1+\eta)+x(-1+\eta)-\eta)(-1+\eta t)} - \\
& \frac{56 c \sigma^2 w \eta^4 \mu 1^2}{(-1+w(-1+\eta))(x(-1+\eta)-\eta)(w(-1+\eta)+x(-1+\eta)-\eta)(-1+\eta t)} - \\
& \frac{112 c \sigma^2 x \eta^4 \mu 1^2}{(-1+w(-1+\eta))(x(-1+\eta)-\eta)(w(-1+\eta)+x(-1+\eta)-\eta)(-1+\eta t)} + \\
& \frac{56 c \sigma^2 w x \eta^4 \mu 1^2}{(-1+w(-1+\eta))(x(-1+\eta)-\eta)(w(-1+\eta)+x(-1+\eta)-\eta)(-1+\eta t)} + \\
& \frac{56 c \sigma^2 x^2 \eta^4 \mu 1^2}{(-1+w(-1+\eta))(x(-1+\eta)-\eta)(w(-1+\eta)+x(-1+\eta)-\eta)(-1+\eta t)} + \\
& \frac{176 c \sigma^2 x \eta \theta l \mu 1^2}{(-1+w(-1+\eta))(x(-1+\eta)-\eta)(w(-1+\eta)+x(-1+\eta)-\eta) \theta p} + \\
& \frac{264 c \sigma^2 w x \eta \theta l \mu 1^2}{(-1+w(-1+\eta))(x(-1+\eta)-\eta)(w(-1+\eta)+x(-1+\eta)-\eta) \theta p} + \\
& \frac{88 c \sigma^2 w x \eta^3 \theta l \mu 1^2}{(-1+w(-1+\eta))(x(-1+\eta)-\eta)(w(-1+\eta)+x(-1+\eta)-\eta) \theta p} + \\
& \frac{88 c \sigma^2 x \theta l \mu 1^2}{(1+w-w \eta)(x+\eta-x \eta)(w+x+\eta-w \eta-x \eta) \theta p} + \\
& \frac{88 c \sigma^2 w x \theta l \mu 1^2}{(1+w-w \eta)(x+\eta-x \eta)(w+x+\eta-w \eta-x \eta) \theta p} + \\
& \frac{88 c \sigma^2 x \eta^2 \theta l \mu 1^2}{(1+w-w \eta)(x+\eta-x \eta)(w+x+\eta-w \eta-x \eta) \theta p} + \\
& \frac{264 c \sigma^2 w x \eta^2 \theta l \mu 1^2}{(1+w-w \eta)(x+\eta-x \eta)(w+x+\eta-w \eta-x \eta) \theta p} - \frac{32 c \sigma^2 x \mu 2}{(1+w-w \eta)^2 (w+x+\eta-w \eta-x \eta)^2} - \\
& \frac{64 c \sigma^2 w x \mu 2}{(1+w-w \eta)^2 (w+x+\eta-w \eta-x \eta)^2} - \frac{32 c \sigma^2 w^2 x \mu 2}{(1+w-w \eta)^2 (w+x+\eta-w \eta-x \eta)^2} -
\end{aligned}$$



$$\begin{aligned}
& \frac{16 c \sigma^2 \eta \mu_2}{(1+w-w \eta)^2 (w+x+\eta-w \eta-x \eta)^2} - \frac{32 c \sigma^2 w \eta \mu_2}{(1+w-w \eta)^2 (w+x+\eta-w \eta-x \eta)^2} - \\
& \frac{16 c \sigma^2 w^2 \eta \mu_2}{(1+w-w \eta)^2 (w+x+\eta-w \eta-x \eta)^2} + \frac{64 c \sigma^2 x \eta \mu_2}{(1+w-w \eta)^2 (w+x+\eta-w \eta-x \eta)^2} + \\
& \frac{192 c \sigma^2 w x \eta \mu_2}{(1+w-w \eta)^2 (w+x+\eta-w \eta-x \eta)^2} + \frac{128 c \sigma^2 w^2 x \eta \mu_2}{(1+w-w \eta)^2 (w+x+\eta-w \eta-x \eta)^2} + \\
& \frac{16 c \sigma^2 \eta^2 \mu_2}{(1+w-w \eta)^2 (w+x+\eta-w \eta-x \eta)^2} + \frac{64 c \sigma^2 w \eta^2 \mu_2}{(1+w-w \eta)^2 (w+x+\eta-w \eta-x \eta)^2} + \\
& \frac{48 c \sigma^2 w^2 \eta^2 \mu_2}{(1+w-w \eta)^2 (w+x+\eta-w \eta-x \eta)^2} - \frac{32 c \sigma^2 x \eta^2 \mu_2}{(1+w-w \eta)^2 (w+x+\eta-w \eta-x \eta)^2} - \\
& \frac{192 c \sigma^2 w x \eta^2 \mu_2}{(1+w-w \eta)^2 (w+x+\eta-w \eta-x \eta)^2} - \frac{192 c \sigma^2 w^2 x \eta^2 \mu_2}{(1+w-w \eta)^2 (w+x+\eta-w \eta-x \eta)^2} - \\
& \frac{32 c \sigma^2 w \eta^3 \mu_2}{(1+w-w \eta)^2 (w+x+\eta-w \eta-x \eta)^2} - \frac{48 c \sigma^2 w^2 \eta^3 \mu_2}{(1+w-w \eta)^2 (w+x+\eta-w \eta-x \eta)^2} + \\
& \frac{64 c \sigma^2 w x \eta^3 \mu_2}{(1+w-w \eta)^2 (w+x+\eta-w \eta-x \eta)^2} + \frac{128 c \sigma^2 w^2 x \eta^3 \mu_2}{(1+w-w \eta)^2 (w+x+\eta-w \eta-x \eta)^2} + \\
& \frac{16 c \sigma^2 w^2 \eta^4 \mu_2}{(1+w-w \eta)^2 (w+x+\eta-w \eta-x \eta)^2} - \frac{32 c \sigma^2 w^2 x \eta^4 \mu_2}{(1+w-w \eta)^2 (w+x+\eta-w \eta-x \eta)^2} - \\
& \frac{288 c \sigma^2 w \mu_1 \mu_2}{(1+w-w \eta)^2 (w+x+\eta-w \eta-x \eta)^2} - \frac{576 c \sigma^2 w^2 \mu_1 \mu_2}{(1+w-w \eta)^2 (w+x+\eta-w \eta-x \eta)^2} - \\
& \frac{288 c \sigma^2 w^3 \mu_1 \mu_2}{(1+w-w \eta)^2 (w+x+\eta-w \eta-x \eta)^2} - \frac{128 c \sigma^2 x \mu_1 \mu_2}{(1+w-w \eta)^2 (w+x+\eta-w \eta-x \eta)^2} - \\
& \frac{256 c \sigma^2 w x \mu_1 \mu_2}{(1+w-w \eta)^2 (w+x+\eta-w \eta-x \eta)^2} - \frac{128 c \sigma^2 w^2 x \mu_1 \mu_2}{(1+w-w \eta)^2 (w+x+\eta-w \eta-x \eta)^2} - \\
& \frac{208 c \sigma^2 \eta \mu_1 \mu_2}{(1+w-w \eta)^2 (w+x+\eta-w \eta-x \eta)^2} + \frac{160 c \sigma^2 w \eta \mu_1 \mu_2}{(1+w-w \eta)^2 (w+x+\eta-w \eta-x \eta)^2} + \\
& \frac{1520 c \sigma^2 w^2 \eta \mu_1 \mu_2}{(1+w-w \eta)^2 (w+x+\eta-w \eta-x \eta)^2} + \frac{1152 c \sigma^2 w^3 \eta \mu_1 \mu_2}{(1+w-w \eta)^2 (w+x+\eta-w \eta-x \eta)^2} + \\
& \frac{256 c \sigma^2 x \eta \mu_1 \mu_2}{(1+w-w \eta)^2 (w+x+\eta-w \eta-x \eta)^2} + \frac{768 c \sigma^2 w x \eta \mu_1 \mu_2}{(1+w-w \eta)^2 (w+x+\eta-w \eta-x \eta)^2} + \\
& \frac{512 c \sigma^2 w^2 x \eta \mu_1 \mu_2}{(1+w-w \eta)^2 (w+x+\eta-w \eta-x \eta)^2} + \frac{208 c \sigma^2 \eta^2 \mu_1 \mu_2}{(1+w-w \eta)^2 (w+x+\eta-w \eta-x \eta)^2} + \\
& \frac{544 c \sigma^2 w \eta^2 \mu_1 \mu_2}{(1+w-w \eta)^2 (w+x+\eta-w \eta-x \eta)^2} - \frac{1104 c \sigma^2 w^2 \eta^2 \mu_1 \mu_2}{(1+w-w \eta)^2 (w+x+\eta-w \eta-x \eta)^2} - \\
& \frac{1728 c \sigma^2 w^3 \eta^2 \mu_1 \mu_2}{(1+w-w \eta)^2 (w+x+\eta-w \eta-x \eta)^2} - \frac{128 c \sigma^2 x \eta^2 \mu_1 \mu_2}{(1+w-w \eta)^2 (w+x+\eta-w \eta-x \eta)^2} - \\
& \frac{768 c \sigma^2 w x \eta^2 \mu_1 \mu_2}{(1+w-w \eta)^2 (w+x+\eta-w \eta-x \eta)^2} - \frac{768 c \sigma^2 w^2 x \eta^2 \mu_1 \mu_2}{(1+w-w \eta)^2 (w+x+\eta-w \eta-x \eta)^2} -
\end{aligned}$$

$$\begin{aligned}
& \frac{416 c \sigma^2 w \eta^3 \mu_1 \mu_2}{(1+w-w \eta)^2 (w+x+\eta-w \eta-x \eta)^2} - \frac{48 c \sigma^2 w^2 \eta^3 \mu_1 \mu_2}{(1+w-w \eta)^2 (w+x+\eta-w \eta-x \eta)^2} + \\
& \frac{1152 c \sigma^2 w^3 \eta^3 \mu_1 \mu_2}{(1+w-w \eta)^2 (w+x+\eta-w \eta-x \eta)^2} + \frac{256 c \sigma^2 w x \eta^3 \mu_1 \mu_2}{(1+w-w \eta)^2 (w+x+\eta-w \eta-x \eta)^2} + \\
& \frac{512 c \sigma^2 w^2 x \eta^3 \mu_1 \mu_2}{(1+w-w \eta)^2 (w+x+\eta-w \eta-x \eta)^2} + \frac{208 c \sigma^2 w^2 \eta^4 \mu_1 \mu_2}{(1+w-w \eta)^2 (w+x+\eta-w \eta-x \eta)^2} - \\
& \frac{288 c \sigma^2 w^3 \eta^4 \mu_1 \mu_2}{(1+w-w \eta)^2 (w+x+\eta-w \eta-x \eta)^2} - \frac{128 c \sigma^2 w^2 x \eta^4 \mu_1 \mu_2}{(1+w-w \eta)^2 (w+x+\eta-w \eta-x \eta)^2} - \\
& \frac{36 f w^2 \vartheta l \boxplus 1}{(w+x+\eta-w \eta-x \eta)^3} - \frac{48 f x^2 \vartheta l \boxplus 1}{(w+x+\eta-w \eta-x \eta)^3} + \frac{108 f w x^2 \vartheta l \boxplus 1}{(x(-1+\eta)-\eta)(w+x+\eta-w \eta-x \eta)^3} - \\
& \frac{81 f w \eta \vartheta l \boxplus 1}{(w+x+\eta-w \eta-x \eta)^3} + \frac{108 f w^2 \eta \vartheta l \boxplus 1}{(w+x+\eta-w \eta-x \eta)^3} - \frac{93 f x \eta \vartheta l \boxplus 1}{(w+x+\eta-w \eta-x \eta)^3} + \\
& \frac{144 f x^2 \eta \vartheta l \boxplus 1}{(w+x+\eta-w \eta-x \eta)^3} + \frac{108 f w x \eta \vartheta l \boxplus 1}{(x(-1+\eta)-\eta)(w+x+\eta-w \eta-x \eta)^3} - \\
& \frac{432 f w x^2 \eta \vartheta l \boxplus 1}{(x(-1+\eta)-\eta)(w+x+\eta-w \eta-x \eta)^3} - \frac{39 f \eta^2 \vartheta l \boxplus 1}{(w+x+\eta-w \eta-x \eta)^3} + \frac{162 f w \eta^2 \vartheta l \boxplus 1}{(w+x+\eta-w \eta-x \eta)^3} - \\
& \frac{108 f w^2 \eta^2 \vartheta l \boxplus 1}{(w+x+\eta-w \eta-x \eta)^3} + \frac{186 f x \eta^2 \vartheta l \boxplus 1}{(w+x+\eta-w \eta-x \eta)^3} - \frac{144 f x^2 \eta^2 \vartheta l \boxplus 1}{(w+x+\eta-w \eta-x \eta)^3} - \\
& \frac{324 f w x \eta^2 \vartheta l \boxplus 1}{(x(-1+\eta)-\eta)(w+x+\eta-w \eta-x \eta)^3} + \frac{648 f w x^2 \eta^2 \vartheta l \boxplus 1}{(x(-1+\eta)-\eta)(w+x+\eta-w \eta-x \eta)^3} + \\
& \frac{39 f \eta^3 \vartheta l \boxplus 1}{(w+x+\eta-w \eta-x \eta)^3} - \frac{81 f w \eta^3 \vartheta l \boxplus 1}{(w+x+\eta-w \eta-x \eta)^3} + \frac{36 f w^2 \eta^3 \vartheta l \boxplus 1}{(w+x+\eta-w \eta-x \eta)^3} - \\
& \frac{93 f x \eta^3 \vartheta l \boxplus 1}{(w+x+\eta-w \eta-x \eta)^3} + \frac{48 f x^2 \eta^3 \vartheta l \boxplus 1}{(w+x+\eta-w \eta-x \eta)^3} + \frac{324 f w x \eta^3 \vartheta l \boxplus 1}{(x(-1+\eta)-\eta)(w+x+\eta-w \eta-x \eta)^3} - \\
& \frac{432 f w x^2 \eta^3 \vartheta l \boxplus 1}{(x(-1+\eta)-\eta)(w+x+\eta-w \eta-x \eta)^3} - \frac{108 f w x \eta^4 \vartheta l \boxplus 1}{(x(-1+\eta)-\eta)(w+x+\eta-w \eta-x \eta)^3} + \\
& \frac{108 f w x^2 \eta^4 \vartheta l \boxplus 1}{(x(-1+\eta)-\eta)(w+x+\eta-w \eta-x \eta)^3} - \frac{36 f w \vartheta l \boxplus 1}{(w+x+\eta-w \eta-x \eta)^2} + \\
& \frac{72 f w \eta \vartheta l \boxplus 1}{(w+x+\eta-w \eta-x \eta)^2} - \frac{36 f w \eta^2 \vartheta l \boxplus 1}{(w+x+\eta-w \eta-x \eta)^2} + 16 f \vartheta l \boxplus 2 - \frac{8 f \vartheta l \boxplus 2}{(1+w-w \eta)^2} + \\
& \frac{8 f w \vartheta l \boxplus 2}{(1+w-w \eta)^2} + \frac{16 f \eta \vartheta l \boxplus 2}{(1+w-w \eta)^2} - \frac{16 f w \eta \vartheta l \boxplus 2}{(1+w-w \eta)^2} - \frac{8 f \eta^2 \vartheta l \boxplus 2}{(1+w-w \eta)^2} + \frac{8 f w \eta^2 \vartheta l \boxplus 2}{(1+w-w \eta)^2} - \\
& \frac{3 f w^2 \vartheta l \boxplus 2}{(w+x+\eta-w \eta-x \eta)^3} + \frac{2 f w x \vartheta l \boxplus 2}{(w+x+\eta-w \eta-x \eta)^3} - \frac{f x^2 \vartheta l \boxplus 2}{(w+x+\eta-w \eta-x \eta)^3} + \\
& \frac{30 f w x^2 \vartheta l \boxplus 2}{(x(-1+\eta)-\eta)(w+x+\eta-w \eta-x \eta)^3} - \frac{9 f w \eta \vartheta l \boxplus 2}{(w+x+\eta-w \eta-x \eta)^3} + \frac{9 f w^2 \eta \vartheta l \boxplus 2}{(w+x+\eta-w \eta-x \eta)^3} - \\
& \frac{7 f x \eta \vartheta l \boxplus 2}{(w+x+\eta-w \eta-x \eta)^3} - \frac{6 f w x \eta \vartheta l \boxplus 2}{(w+x+\eta-w \eta-x \eta)^3} + \frac{3 f x^2 \eta \vartheta l \boxplus 2}{(w+x+\eta-w \eta-x \eta)^3} +
\end{aligned}$$

$$\begin{aligned}
& \frac{30 f w x \eta \vartheta \mathfrak{L} \mathfrak{L} \mathfrak{L}}{(x(-1+\eta)-\eta)(w+x+\eta-w \eta-x \eta)^3} - \frac{120 f w x^2 \eta \vartheta \mathfrak{L} \mathfrak{L} \mathfrak{L}}{(x(-1+\eta)-\eta)(w+x+\eta-w \eta-x \eta)^3} + \\
& \frac{18 f w \eta^2 \vartheta \mathfrak{L} \mathfrak{L} \mathfrak{L}}{(w+x+\eta-w \eta-x \eta)^3} - \frac{9 f w^2 \eta^2 \vartheta \mathfrak{L} \mathfrak{L} \mathfrak{L}}{(w+x+\eta-w \eta-x \eta)^3} + \frac{14 f x \eta^2 \vartheta \mathfrak{L} \mathfrak{L} \mathfrak{L}}{(w+x+\eta-w \eta-x \eta)^3} + \\
& \frac{6 f w x \eta^2 \vartheta \mathfrak{L} \mathfrak{L} \mathfrak{L}}{(w+x+\eta-w \eta-x \eta)^3} - \frac{3 f x^2 \eta^2 \vartheta \mathfrak{L} \mathfrak{L} \mathfrak{L}}{(w+x+\eta-w \eta-x \eta)^3} - \frac{90 f w x \eta^2 \vartheta \mathfrak{L} \mathfrak{L} \mathfrak{L}}{(x(-1+\eta)-\eta)(w+x+\eta-w \eta-x \eta)^3} + \\
& \frac{180 f w x^2 \eta^2 \vartheta \mathfrak{L} \mathfrak{L} \mathfrak{L}}{(x(-1+\eta)-\eta)(w+x+\eta-w \eta-x \eta)^3} - \frac{9 f w \eta^3 \vartheta \mathfrak{L} \mathfrak{L} \mathfrak{L}}{(w+x+\eta-w \eta-x \eta)^3} + \frac{3 f w^2 \eta^3 \vartheta \mathfrak{L} \mathfrak{L} \mathfrak{L}}{(w+x+\eta-w \eta-x \eta)^3} - \\
& \frac{7 f x \eta^3 \vartheta \mathfrak{L} \mathfrak{L} \mathfrak{L}}{(w+x+\eta-w \eta-x \eta)^3} - \frac{2 f w x \eta^3 \vartheta \mathfrak{L} \mathfrak{L} \mathfrak{L}}{(w+x+\eta-w \eta-x \eta)^3} + \frac{f x^2 \eta^3 \vartheta \mathfrak{L} \mathfrak{L} \mathfrak{L}}{(w+x+\eta-w \eta-x \eta)^3} + \\
& \frac{90 f w x \eta^3 \vartheta \mathfrak{L} \mathfrak{L} \mathfrak{L}}{(x(-1+\eta)-\eta)(w+x+\eta-w \eta-x \eta)^3} - \frac{120 f w x^2 \eta^3 \vartheta \mathfrak{L} \mathfrak{L} \mathfrak{L}}{(x(-1+\eta)-\eta)(w+x+\eta-w \eta-x \eta)^3} - \\
& \frac{30 f w x \eta^4 \vartheta \mathfrak{L} \mathfrak{L} \mathfrak{L}}{(x(-1+\eta)-\eta)(w+x+\eta-w \eta-x \eta)^3} + \frac{30 f w x^2 \eta^4 \vartheta \mathfrak{L} \mathfrak{L} \mathfrak{L}}{(x(-1+\eta)-\eta)(w+x+\eta-w \eta-x \eta)^3} - \\
& \frac{38 f w \vartheta \mathfrak{L} \mathfrak{L} \mathfrak{L}}{(w+x+\eta-w \eta-x \eta)^2} + \frac{76 f w \eta \vartheta \mathfrak{L} \mathfrak{L} \mathfrak{L}}{(w+x+\eta-w \eta-x \eta)^2} - \frac{38 f w \eta^2 \vartheta \mathfrak{L} \mathfrak{L} \mathfrak{L}}{(w+x+\eta-w \eta-x \eta)^2} - \\
& \frac{15 f \vartheta \mathfrak{L} \mathfrak{L} \mathfrak{L}}{(1+w-w \eta)(w+x+\eta-w \eta-x \eta)} - \frac{39 f w \vartheta \mathfrak{L} \mathfrak{L} \mathfrak{L}}{(1+w-w \eta)(w+x+\eta-w \eta-x \eta)} - \\
& \frac{24 f x \vartheta \mathfrak{L} \mathfrak{L} \mathfrak{L}}{(1+w-w \eta)(w+x+\eta-w \eta-x \eta)} - \frac{9 f \eta \vartheta \mathfrak{L} \mathfrak{L} \mathfrak{L}}{(1+w-w \eta)(w+x+\eta-w \eta-x \eta)} + \\
& \frac{78 f w \eta \vartheta \mathfrak{L} \mathfrak{L} \mathfrak{L}}{(1+w-w \eta)(w+x+\eta-w \eta-x \eta)} + \frac{48 f x \eta \vartheta \mathfrak{L} \mathfrak{L} \mathfrak{L}}{(1+w-w \eta)(w+x+\eta-w \eta-x \eta)} + \\
& \frac{24 f \eta^2 \vartheta \mathfrak{L} \mathfrak{L} \mathfrak{L}}{(1+w-w \eta)(w+x+\eta-w \eta-x \eta)} - \frac{39 f w \eta^2 \vartheta \mathfrak{L} \mathfrak{L} \mathfrak{L}}{(1+w-w \eta)(w+x+\eta-w \eta-x \eta)} - \\
& \frac{24 f x \eta^2 \vartheta \mathfrak{L} \mathfrak{L} \mathfrak{L}}{(1+w-w \eta)(w+x+\eta-w \eta-x \eta)} - 16 f \vartheta \mathfrak{L}^2 \mathfrak{L} \mathfrak{L} \mathfrak{L} + 20 f \vartheta \mathfrak{L}^2 \mathfrak{L} \mathfrak{L} \mathfrak{L} \Big)
\end{aligned}$$

$\beta u =$

$$\begin{aligned}
& - \Big( (12 c v c \sigma f w (-1+x(-1+\eta)-\eta)(-1+\eta)^3(x+\eta-x \eta)^2(4 x^5(-1+\eta)^5(-1+\eta+\vartheta \mathfrak{L}-\eta t \\
& \vartheta \mathfrak{L}) \vartheta p+x^4(-1+\eta)^4(4 \times(-1+w(-1+\eta)) \times(-1+\eta t) \vartheta \mathfrak{L} \mu_1+ \\
& \vartheta p(4+16 \eta-20 \eta^2-4 \vartheta \mathfrak{L}-20 \eta \vartheta \mathfrak{L}+4 \eta t \vartheta \mathfrak{L}+20 \eta \eta t \vartheta \mathfrak{L}-2 \vartheta \mathfrak{L} \mu_1+2 \eta t \vartheta \mathfrak{L} \mu_1- \\
& 2 \vartheta \mathfrak{L} \mu_2+2 \eta t \vartheta \mathfrak{L} \mu_2-\vartheta \mathfrak{L} \mu_1 \mathfrak{L} 1+\eta t \vartheta \mathfrak{L} \mu_1 \mathfrak{L} 1-\vartheta \mathfrak{L} \mu_1 \mathfrak{L} 2+\eta t \vartheta \mathfrak{L} \mu_1 \mathfrak{L} 2+w \\
& (-1+\eta) \times(-12+12 \eta-(-1+\eta t) \vartheta \mathfrak{L}(2 \times(6+\mu_2)+\mu_1(2+\mathfrak{L} 1+\mathfrak{L} 2)))) \Big) + \\
& \vartheta p(-3 w^2(-1+\eta)^2(1+\eta) \times(4 \eta^3-6 \eta t(1+\mu_1+\mu_2)+\eta^2 \\
& (4 \times(-1+\eta t \mu_1+\mu_2)-(-1+\eta t) \vartheta \mathfrak{L}(2 \times(2+\mu_2)+\mu_1(2+\mathfrak{L} 1+\mathfrak{L} 2)))) + \eta \\
& (-4 \mu_2+2 \eta t(3+\mu_1+3 \mu_2)+ \\
& \vartheta \mathfrak{L}(3 \times(2+\mathfrak{L} 1+\mathfrak{L} 2)+4 \mu_1(2+\mathfrak{L} 1+\mathfrak{L} 2)+\mu_2(8+3 \mathfrak{L} 1+3 \mathfrak{L} 2)) - \\
& \eta t \vartheta \mathfrak{L}(3 \times(2+\mathfrak{L} 1+\mathfrak{L} 2)+4 \mu_1(2+\mathfrak{L} 1+\mathfrak{L} 2)+\mu_2(8+3 \mathfrak{L} 1+3 \mathfrak{L} 2)))) \Big) + \\
& w^3(-1+\eta)^3(4 \eta^3-6 \eta t(1+\mu_1+\mu_2)-\eta(4+8 \eta t \mu_1+8 \mu_2+ \\
& (-1+\eta t) \vartheta \mathfrak{L}(5 \mu_1(2+\mathfrak{L} 1+\mathfrak{L} 2)+(1+\mu_2) \times(10+3 \mathfrak{L} 1+3 \mathfrak{L} 2)))) + \eta^2 \\
& (8 \mu_2+5 \vartheta \mathfrak{L} \mu_1(2+\mathfrak{L} 1+\mathfrak{L} 2)+\vartheta \mathfrak{L}(1+\mu_2) \times(10+3 \mathfrak{L} 1+3 \mathfrak{L} 2)- \\
& \eta t(-2 \times(3+7 \mu_1+3 \mu_2)+5 \vartheta \mathfrak{L} \mu_1(2+\mathfrak{L} 1+\mathfrak{L} 2)+
\end{aligned}$$

$$\begin{aligned}
& \left( \theta l (1 + \mu_2) \times (10 + 3 \mathfrak{x}1 + 3 \mathfrak{x}2) \right) + \\
& w (-1 + \eta) \times \left( 12 \eta^5 - 18 \eta t (1 + \mu_1 + \mu_2) + \eta^4 (4 (\eta t \mu_1 + \mu_2) - (-1 + \eta t) \right. \\
& \quad \left. \theta l (2 \times (6 + \mu_2) + \mu_1 (2 + \mathfrak{x}1 + \mathfrak{x}2))) + \eta^3 (12 \times (-1 + \eta t \mu_1 + \mu_2) - \right. \\
& \quad \left. (-1 + \eta t) \theta l (2 \times (6 + 5 \mu_2) + 5 \mu_1 (2 + \mathfrak{x}1 + \mathfrak{x}2))) - \eta \right. \\
& \quad \left. (4 (\eta t \mu_1 + \mu_2) + (-1 + \eta t) \theta l (9 \times (2 + \mathfrak{x}1 + \mathfrak{x}2) + 10 \mu_1 (2 + \mathfrak{x}1 + \mathfrak{x}2) + \right. \\
& \quad \left. \mu_2 (20 + 9 \mathfrak{x}1 + 9 \mathfrak{x}2))) + \eta^2 (-12 \mu_2 + 6 \eta t (3 + \mu_1 + 3 \mu_2) + \right. \\
& \quad \left. \theta l (9 \times (2 + \mathfrak{x}1 + \mathfrak{x}2) + 14 \mu_1 (2 + \mathfrak{x}1 + \mathfrak{x}2) + \mu_2 (28 + 9 \mathfrak{x}1 + 9 \mathfrak{x}2)) - \right. \\
& \quad \left. \eta t \theta l (9 \times (2 + \mathfrak{x}1 + \mathfrak{x}2) + 14 \mu_1 (2 + \mathfrak{x}1 + \mathfrak{x}2) + \mu_2 (28 + 9 \mathfrak{x}1 + 9 \mathfrak{x}2))) \right) - \\
& (1 + \eta) \times \left( 4 \eta^5 - 4 \eta^4 (1 + (-1 + \eta t) \theta l) - 6 \eta t (1 + \mu_1 + \mu_2) - 3 \eta \right. \\
& \quad \left. (1 + \mu_1 + \mu_2) (-\theta l (2 + \mathfrak{x}1 + \mathfrak{x}2) + \eta t (-2 + \theta l (2 + \mathfrak{x}1 + \mathfrak{x}2))) - \eta^2 \right. \\
& \quad \left. (4 \mu_2 - 2 \theta l \mu_2 + 2 \eta t \theta l \mu_2 - \theta l \mu_1 (2 + \mathfrak{x}1 + \mathfrak{x}2) + \right. \\
& \quad \left. \eta t \mu_1 (4 + \theta l (2 + \mathfrak{x}1 + \mathfrak{x}2))) + \eta^3 (4 \mu_2 + 2 \theta l \mu_2 + \right. \\
& \quad \left. \theta l \mu_1 (2 + \mathfrak{x}1 + \mathfrak{x}2) - \eta t (2 \theta l \mu_2 + \mu_1 (-4 + \theta l (2 + \mathfrak{x}1 + \mathfrak{x}2)))) \right) + \\
& x^3 (-1 + \eta)^3 \left( 40 \eta^3 \theta p - 8 \eta^2 (3 + 5 \times (-1 + \eta t) \theta l) \theta p - 4 \theta p (\eta t \mu_1 + \mu_2) - \right. \\
& \quad 2 \times (-1 + \eta t) \theta l (2 \theta p \mu_2 + \mu_1 (-2 + \theta p (2 + \mathfrak{x}1 + \mathfrak{x}2))) + \\
& \quad 3 w^2 (-1 + \eta)^2 (4 \times (-1 + \eta t) \theta l \mu_1 + \theta p (-4 + 4 \eta - (-1 + \eta t) \theta l \\
& \quad \quad (2 \times (2 + \mu_2) + \mu_1 (2 + \mathfrak{x}1 + \mathfrak{x}2)))) + 2 \eta (6 \times (-1 + \eta t) \theta l \mu_1 + 2 \theta p \\
& \quad \quad (-4 + \eta t \mu_1 + \mu_2 - (-1 + \eta t) \theta l (2 \times (2 + \mu_2) + \mu_1 (2 + \mathfrak{x}1 + \mathfrak{x}2)))) - \\
& \quad w (-1 + \eta) \times (4 \times (4 + 3 \eta) \times (-1 + \eta t) \theta l \mu_1 + \theta p (48 \eta^2 - 4 \times (3 + \eta t \mu_1 + \mu_2) - \\
& \quad \quad (-1 + \eta t) \theta l (2 \times (6 + 5 \mu_2) + 5 \mu_1 (2 + \mathfrak{x}1 + \mathfrak{x}2)) - \\
& \quad \quad 4 \eta (9 - \eta t \mu_1 - \mu_2 + (-1 + \eta t) \theta l (2 \times (6 + \mu_2) + \mu_1 (2 + \mathfrak{x}1 + \mathfrak{x}2)))) \right) + \\
& x^2 (-1 + \eta)^2 \left( 4 \times (-1 + \eta) \theta p (w^3 (-1 + \eta)^3 - 6 \eta^2 - 10 \eta^3 - \eta t \mu_1 - 3 \eta \eta t \right. \\
& \quad \mu_1 - \mu_2 - 3 \eta \mu_2 - 3 w^2 (-1 + \eta)^2 (1 + 3 \eta + \eta t \mu_1 + \mu_2) + w (-1 + \eta) \times \\
& \quad \left. (18 \eta^2 + 4 (\eta t \mu_1 + \mu_2) + 3 \eta (3 + \eta t \mu_1 + \mu_2))) - (-1 + \eta t) \theta l \right. \\
& \quad \left( 6 - 6 \theta p - 24 \eta^2 \theta p - 40 \eta^3 \theta p + 6 \mu_1 + 8 \eta \mu_1 + 12 \eta^2 \mu_1 - 8 \theta p \mu_1 - 12 \eta \theta p \right. \\
& \quad \mu_1 - 12 \eta^2 \theta p \mu_1 + 6 \mu_2 - 8 \theta p \mu_2 - 12 \eta \theta p \mu_2 - 12 \eta^2 \theta p \mu_2 - 3 \theta p \mathfrak{x}1 - 4 \theta p \\
& \quad \mu_1 \mathfrak{x}1 - 6 \eta \theta p \mu_1 \mathfrak{x}1 - 6 \eta^2 \theta p \mu_1 \mathfrak{x}1 - 3 \theta p \mu_2 \mathfrak{x}1 - 3 \theta p \mathfrak{x}2 - 4 \theta p \mu_1 \mathfrak{x}2 - 6 \eta \\
& \quad \theta p \mu_1 \mathfrak{x}2 - 6 \eta^2 \theta p \mu_1 \mathfrak{x}2 - 3 \theta p \mu_2 \mathfrak{x}2 + w^3 (-1 + \eta)^3 (-2 \times (3 + 7 \mu_1 + 3 \mu_2) + \\
& \quad 5 \theta p \mu_1 (2 + \mathfrak{x}1 + \mathfrak{x}2) + \theta p (1 + \mu_2) \times (10 + 3 \mathfrak{x}1 + 3 \mathfrak{x}2)) - 3 w^2 (-1 + \eta)^2 \\
& \quad (-2 \times (3 + 5 \mu_1 + 4 \eta \mu_1 + 3 \mu_2) + \theta p (6 \eta (2 + \mu_2) + 5 \mu_1 (2 + \mathfrak{x}1 + \mathfrak{x}2) + \\
& \quad 3 \eta \mu_1 (2 + \mathfrak{x}1 + \mathfrak{x}2) + (1 + \mu_2) \times (10 + 3 \mathfrak{x}1 + 3 \mathfrak{x}2))) + w (-1 + \eta) \times \\
& \quad \left. (-2 \times ((11 + 16 \eta + 6 \eta^2) \mu_1 + 9 \times (1 + \mu_2)) + \theta p (18 + 28 \mu_2 + 9 \mathfrak{x}1 + \right. \\
& \quad \quad 9 \mu_2 \mathfrak{x}1 + 9 \mathfrak{x}2 + 9 \mu_2 \mathfrak{x}2 + 14 \mu_1 (2 + \mathfrak{x}1 + \mathfrak{x}2) + 6 \eta^2 (2 \times (6 + \mu_2) + \\
& \quad \quad \mu_1 (2 + \mathfrak{x}1 + \mathfrak{x}2)) + 3 \eta (2 \times (6 + 5 \mu_2) + 5 \mu_1 (2 + \mathfrak{x}1 + \mathfrak{x}2)))) \right) - \\
& x (-1 + \eta) \times \left( 2 \times (-1 + \eta) \theta p (-8 \eta^3 - 10 \eta^4 - 3 \eta t - 3 \eta t \mu_1 - 4 \eta \eta t \mu_1 - \right. \\
& \quad 6 \eta^2 \eta t \mu_1 - 4 \eta \mu_2 - 6 \eta^2 \mu_2 - 3 \eta t \mu_2 - 3 w^2 (-1 + \eta)^2 \\
& \quad \left. (6 \eta^2 + 2 \mu_2 + 4 \eta (1 + \eta t \mu_1 + \mu_2) + \eta t (3 + 5 \mu_1 + 3 \mu_2)) + w^3 (-1 + \eta)^3 \right. \\
& \quad \left. (2 + 4 \eta + 4 \mu_2 + \eta t (3 + 7 \mu_1 + 3 \mu_2)) + w (-1 + \eta) \times (24 \eta^3 + 2 \mu_2 + \right. \\
& \quad \left. 16 \eta (\eta t \mu_1 + \mu_2) + 6 \eta^2 (3 + \eta t \mu_1 + \mu_2) + \eta t (9 + 11 \mu_1 + 9 \mu_2)) \right) - \\
& (-1 + \eta t) \theta l (6 + 6 \eta - 6 \theta p - 12 \eta \theta p - 16 \eta^3 \theta p - 20 \eta^4 \theta p + 6 \mu_1 + 6 \\
& \quad \eta \mu_1 + 4 \eta^2 \mu_1 + 4 \eta^3 \mu_1 - 6 \theta p \mu_1 - 16 \eta \theta p \mu_1 - 12 \eta^2 \theta p \mu_1 - 8 \eta^3 \theta p \\
& \quad \mu_1 + 6 \mu_2 + 6 \eta \mu_2 - 6 \theta p \mu_2 - 16 \eta \theta p \mu_2 - 12 \eta^2 \theta p \mu_2 - 8 \eta^3 \theta p \mu_2 - 3 \\
& \quad \theta p \mathfrak{x}1 - 6 \eta \theta p \mathfrak{x}1 - 3 \theta p \mu_1 \mathfrak{x}1 - 8 \eta \theta p \mu_1 \mathfrak{x}1 - 6 \eta^2 \theta p \mu_1 \mathfrak{x}1 - 4 \eta^3 \\
& \quad \theta p \mu_1 \mathfrak{x}1 - 3 \theta p \mu_2 \mathfrak{x}1 - 6 \eta \theta p \mu_2 \mathfrak{x}1 - 3 \theta p \mathfrak{x}2 - 6 \eta \theta p \mathfrak{x}2 - 3 \theta p \mu_1 \\
& \quad \mathfrak{x}2 - 8 \eta \theta p \mu_1 \mathfrak{x}2 - 6 \eta^2 \theta p \mu_1 \mathfrak{x}2 - 4 \eta^3 \theta p \mu_1 \mathfrak{x}2 - 3 \theta p \mu_2 \mathfrak{x}2 - 6 \eta
\end{aligned}$$

$$\begin{aligned}
& \epsilon p \mu_2 \mathfrak{z}_2 + w^3 (-1 + \eta)^3 (-6 \times (1 + \mu_1 + \mu_2) + 5 \epsilon p \mu_1 (2 + \mathfrak{z}_1 + \mathfrak{z}_2) + \\
& \epsilon p (1 + \mu_2) \times (10 + 3 \mathfrak{z}_1 + 3 \mathfrak{z}_2) + 2 \eta (-3 - 7 \mu_1 - 3 \mu_2 + 5 \epsilon p \mu_1 \\
& (2 + \mathfrak{z}_1 + \mathfrak{z}_2) + \epsilon p (1 + \mu_2) \times (10 + 3 \mathfrak{z}_1 + 3 \mathfrak{z}_2))) - 3 w^2 (-1 + \eta)^2 \\
& (-6 \times (1 + \mu_1 + \mu_2) + \eta^2 (-4 \mu_1 + 6 \epsilon p (2 + \mu_2) + 3 \epsilon p \mu_1 (2 + \mathfrak{z}_1 + \mathfrak{z}_2)) + \\
& \epsilon p (3 \times (2 + \mathfrak{z}_1 + \mathfrak{z}_2) + 4 \mu_1 (2 + \mathfrak{z}_1 + \mathfrak{z}_2) + \mu_2 (8 + 3 \mathfrak{z}_1 + 3 \mathfrak{z}_2)) + \\
& 2 \eta (-3 - 5 \mu_1 - 3 \mu_2 + 5 \epsilon p \mu_1 (2 + \mathfrak{z}_1 + \mathfrak{z}_2) + \\
& \epsilon p (1 + \mu_2) \times (10 + 3 \mathfrak{z}_1 + 3 \mathfrak{z}_2))) + w (-1 + \eta) \times \\
& (-18 \times (1 + \mu_1 + \mu_2) + 4 \eta^3 (-\mu_1 + 2 \epsilon p (6 + \mu_2) + \epsilon p \mu_1 (2 + \mathfrak{z}_1 + \mathfrak{z}_2)) + \\
& \eta^2 (-16 \mu_1 + 6 \epsilon p (6 + 5 \mu_2) + 15 \epsilon p \mu_1 (2 + \mathfrak{z}_1 + \mathfrak{z}_2)) + \\
& \epsilon p (9 \times (2 + \mathfrak{z}_1 + \mathfrak{z}_2) + 10 \mu_1 (2 + \mathfrak{z}_1 + \mathfrak{z}_2) + \mu_2 (20 + 9 \mathfrak{z}_1 + 9 \mathfrak{z}_2)) + \\
& 2 \eta (-9 - 11 \mu_1 - 9 \mu_2 + \epsilon p (9 \times (2 + \mathfrak{z}_1 + \mathfrak{z}_2) + \\
& 14 \mu_1 (2 + \mathfrak{z}_1 + \mathfrak{z}_2) + \mu_2 (28 + 9 \mathfrak{z}_1 + 9 \mathfrak{z}_2)))))) + \\
& (-1 + x (-1 + \eta) - \eta) \times (-48 u (17 u - 2 \epsilon) (-1 + w (-1 + \eta))^3 \\
& (-1 + x (-1 + \eta) - \eta) (x + \eta - x \eta)^3 \\
& (w + x + \eta - w \eta - x \eta)^3 (-1 + \eta t) \epsilon p - \\
& 6 c v^2 (-1 + x (-1 + \eta) - \eta) (x + \eta - x \eta)^2 \\
& (-8 u (-1 + w (-1 + \eta))^3 (x (-1 + \eta) - \eta) (w + x + \eta - w \eta - x \eta)^3 (-1 + \eta t) \epsilon p - \\
& f w^2 (-1 + \eta)^3 (-4 x^3 (3 w (-1 + \eta) - 4 \eta) (-1 + \eta)^3 (-1 + \eta + \theta l - \eta t \theta l) \\
& \epsilon p - 4 x^4 (-1 + \eta)^4 (-1 + \eta + \theta l - \eta t \theta l) \epsilon p - 12 x^2 (-1 + \eta)^2 \\
& (w^2 (-1 + \eta)^2 - 3 w (-1 + \eta) \eta + 2 \eta^2) (-1 + \eta + \theta l - \eta t \theta l) \\
& \epsilon p + \epsilon p (4 \eta^4 - 4 \eta^5 + 6 \eta t - 6 \eta \eta t - 6 \eta \theta l - 4 \eta^4 \theta l + 6 \eta \eta t \theta l + \\
& 4 \eta^4 \eta t \theta l - 3 \eta \theta l \mathfrak{z}_1 + 3 \eta \eta t \theta l \mathfrak{z}_1 - 3 \eta \theta l \mathfrak{z}_2 + 3 \eta \eta t \theta l \mathfrak{z}_2 - \\
& 3 w^2 (-1 + \eta)^2 (4 \eta^3 - 6 \eta t - 4 \eta^2 (1 + (-1 + \eta t) \theta l) + \\
& \eta (6 \eta t + 3 \theta l (2 + \mathfrak{z}_1 + \mathfrak{z}_2) - 3 \eta t \theta l (2 + \mathfrak{z}_1 + \mathfrak{z}_2))) + 3 w (-1 + \eta) \times \\
& (4 \eta^4 - 6 \eta t - 4 \eta^3 (1 + (-1 + \eta t) \theta l) + \eta (6 \eta t + 3 \theta l (2 + \mathfrak{z}_1 + \mathfrak{z}_2) - \\
& 3 \eta t \theta l (2 + \mathfrak{z}_1 + \mathfrak{z}_2))) + w^3 (-1 + \eta)^3 (4 \eta^2 - 6 \eta t + \eta (-4 + 6 \eta t + \\
& \theta l (10 + 3 \mathfrak{z}_1 + 3 \mathfrak{z}_2) - \eta t \theta l (10 + 3 \mathfrak{z}_1 + 3 \mathfrak{z}_2))) - x (-1 + \eta) \times \\
& (4 (w (-1 + \eta) - 4 \eta) (-1 + \eta) (w + \eta - w \eta)^2 \epsilon p - (-1 + \eta t) \theta l \\
& (6 - 6 \epsilon p - 16 \eta^3 \epsilon p - 3 \epsilon p \mathfrak{z}_1 - 3 \epsilon p \mathfrak{z}_2 - 3 w^2 (-1 + \eta)^2 (-6 + 8 \eta \epsilon p + 3 \\
& \epsilon p (2 + \mathfrak{z}_1 + \mathfrak{z}_2)) + 9 w (-1 + \eta) \times (-2 + \epsilon p (2 + 4 \eta^2 + \mathfrak{z}_1 + \mathfrak{z}_2))) + \\
& w^3 (-1 + \eta)^3 (-6 + \epsilon p (10 + 3 \mathfrak{z}_1 + 3 \mathfrak{z}_2)))))) - \\
& 3 f^2 (-1 + w (-1 + \eta)) (x (-1 + \eta) - \eta) (w (-1 + \eta) + x (-1 + \eta) - \eta) \\
& (-1 + \eta)^2 \theta l \\
& ((x^2 (-1 + \eta)^2 + \eta (1 + \eta) + x (1 + \eta - 2 \eta^2)) (40 x^3 (-1 + \eta)^3 (-1 + \eta + \theta l - \eta t \theta l) \\
& \epsilon p + 4 x^2 (-1 + \eta)^2 (-((-1 + \eta) \epsilon p (2 + 30 \eta + \mathfrak{z}_1 + \mathfrak{z}_2)) + \\
& 2 \times (-1 + \eta t) \theta l (-1 + \epsilon p (2 + 15 \eta + \mathfrak{z}_1 + \mathfrak{z}_2))) + \epsilon p \\
& (-40 \eta^4 + 4 \eta^3 (8 + 10 \times (-1 + \eta t) \theta l - \mathfrak{z}_1 - \mathfrak{z}_2) + 6 \eta t (2 + \mathfrak{z}_1 + \mathfrak{z}_2) + \\
& \eta (-3 \theta l (2 + \mathfrak{z}_1 + \mathfrak{z}_2)^2 + 3 \eta t \theta l (2 + \mathfrak{z}_1 + \mathfrak{z}_2)^2 - 2 \eta t (2 + 3 \mathfrak{z}_1 + 3 \mathfrak{z}_2)) + \\
& 4 \eta^2 (-((-1 + 2 \theta l) \times (2 + \mathfrak{z}_1 + \mathfrak{z}_2)) + 2 \eta t (-1 + \theta l (2 + \mathfrak{z}_1 + \mathfrak{z}_2)))) + x \\
& (-1 + \eta) \times (8 \times (-1 + \eta) \epsilon p (15 \eta^2 + \eta t + \eta (2 + \mathfrak{z}_1 + \mathfrak{z}_2)) - \\
& (-1 + \eta t) \theta l (120 \eta^2 \epsilon p + 3 \times (2 + \mathfrak{z}_1 + \mathfrak{z}_2) \times \\
& (-2 + \epsilon p (2 + \mathfrak{z}_1 + \mathfrak{z}_2)) + 8 \eta (-1 + 2 \epsilon p (2 + \mathfrak{z}_1 + \mathfrak{z}_2)))))) - \\
& w^3 (-1 + \eta)^3 (40 x^3 (-1 + \eta)^3 (-1 + \eta + \theta l - \eta t \theta l) \epsilon p + x^2 (-1 + \eta)^2 (-8 \times \\
& (-1 + \eta) \epsilon p (7 + 15 \eta + \mathfrak{z}_1 + \mathfrak{z}_2) + (-1 + \eta t) \theta l (-2 \times (14 + 3 \mathfrak{z}_1 + 3 \mathfrak{z}_2) +
\end{aligned}$$



$$\begin{aligned}
& (19 + 2 \mathfrak{z}1 + 2 \mathfrak{z}2) + \eta \eta t (28 + 6 \mathfrak{z}1 + 6 \mathfrak{z}2) + \eta t (34 + 9 \mathfrak{z}1 + 9 \mathfrak{z}2) \Big) - \\
& (-1 + \eta t) \mathfrak{el} (320 \eta^3 \mathfrak{op} + 6 \times (2 + \mathfrak{z}1 + \mathfrak{z}2) \times (-2 + \mathfrak{op} (2 + \mathfrak{z}1 + \mathfrak{z}2)) + \\
& 2 \eta (-34 - 9 \mathfrak{z}1 - 9 \mathfrak{z}2 + \mathfrak{op} (124 + 60 \mathfrak{z}1 + 9 \mathfrak{z}1^2 + 60 \mathfrak{z}2 + \\
& 18 \mathfrak{z}1 \mathfrak{z}2 + 9 \mathfrak{z}2^2)) + \eta^2 (-2 \times (14 + 3 \mathfrak{z}1 + 3 \mathfrak{z}2) + \\
& 9 \mathfrak{op} (60 + \mathfrak{z}1^2 + 12 \mathfrak{z}2 + \mathfrak{z}2^2 + 2 \mathfrak{z}1 (6 + \mathfrak{z}2))) \Big) \Big) - \\
& 2 f (-1 + x (-1 + \eta) - \eta) \times (-1 + \eta) \times (-12 u \kappa (-1 + w (-1 + \eta)))^3 \\
& (x + \eta - x \eta)^3 (w + x + \eta - w \eta - x \eta)^2 (-1 + \eta t) \mathfrak{el} \mathfrak{op} + \\
& u \Big( (x + \eta - x \eta)^2 (4 x^4 (-1 + \eta)^4 \mathfrak{op} (48 + 30 \eta^3 - 2 \eta^2 (24 - 5 \mathfrak{el} + 5 \eta t (2 + \mathfrak{el})) - \\
& 8 \mathfrak{el} (6 + \mathfrak{z}2) + \eta t (-9 + 8 \mathfrak{el} (6 + \mathfrak{z}2))) + \\
& \eta (-30 - 9 \mathfrak{el} + 2 \mathfrak{el} \mathfrak{z}2 + \eta t (29 + 9 \mathfrak{el} - 2 \mathfrak{el} \mathfrak{z}2))) \Big) + \\
& \eta^2 \mathfrak{op} (120 \eta^5 + 42 \eta t - 8 \eta^4 (24 - 5 \mathfrak{el} + 5 \eta t (2 + \mathfrak{el})) - \\
& 4 \eta^3 (30 + 9 \mathfrak{el} - 2 \mathfrak{el} \mathfrak{z}2 + \eta t (-29 - 9 \mathfrak{el} + 2 \mathfrak{el} \mathfrak{z}2)) + 3 \eta \\
& (-14 \eta t - 13 \mathfrak{el} \mathfrak{z}1 - 5 \mathfrak{el} (2 + \mathfrak{z}2) + \eta t \mathfrak{el} (13 \mathfrak{z}1 + 5 \times (2 + \mathfrak{z}2))) + \\
& 4 \eta^2 (48 - 8 \mathfrak{el} (6 + \mathfrak{z}2) + \eta t (-9 + 8 \mathfrak{el} (6 + \mathfrak{z}2))) \Big) + x^2 (-1 + \eta)^2 \\
& (720 \eta^5 \mathfrak{op} + 34 \eta t \mathfrak{op} - 48 \eta^4 (24 - 5 \mathfrak{el} + 5 \eta t (2 + \mathfrak{el})) \mathfrak{op} - \\
& 24 \eta^3 \mathfrak{op} (30 + 9 \mathfrak{el} - 2 \mathfrak{el} \mathfrak{z}2 + \eta t (-29 - 9 \mathfrak{el} + 2 \mathfrak{el} \mathfrak{z}2)) + \\
& \eta (-34 \eta t \mathfrak{op} + (-1 + \eta t) \mathfrak{el} (-108 + 141 \mathfrak{op} \mathfrak{z}1 + 53 \mathfrak{op} (2 + \mathfrak{z}2))) + \\
& 24 \eta^2 \mathfrak{op} (48 - 8 \mathfrak{el} (6 + \mathfrak{z}2) + \eta t (-9 + 8 \mathfrak{el} (6 + \mathfrak{z}2))) \Big) + \\
& 4 x^3 (-1 + \eta)^3 (-4 \times (-1 + \eta) \eta (-48 + 30 \eta^2 + 9 \eta t - 2 \eta (9 + 10 \eta t)) \\
& \mathfrak{op} + (-1 + \eta t) \mathfrak{el} (11 + 4 \mathfrak{op} (-2 + 10 \eta^3 - 3 \mathfrak{z}1 - \mathfrak{z}2 - \\
& 8 \eta (6 + \mathfrak{z}2) + \eta^2 (-9 + 2 \mathfrak{z}2))) \Big) - 4 x (-1 + \eta) \eta \\
& (120 \eta^5 \mathfrak{op} + 28 \eta t \mathfrak{op} - 8 \eta^4 (24 - 5 \mathfrak{el} + 5 \eta t (2 + \mathfrak{el})) \mathfrak{op} + \\
& \eta (-28 \eta t \mathfrak{op} + (-1 + \eta t) \mathfrak{el} (-7 + 33 \mathfrak{op} \mathfrak{z}1 + 13 \mathfrak{op} (2 + \mathfrak{z}2))) + \\
& 4 \eta^2 \mathfrak{op} (48 - 8 \mathfrak{el} (6 + \mathfrak{z}2) + \eta t (-9 + 8 \mathfrak{el} (6 + \mathfrak{z}2))) - 4 \eta^3 \mathfrak{op} \\
& (30 + \mathfrak{el} (9 - 2 \mathfrak{z}2) + \eta t (-29 + \mathfrak{el} (-9 + 2 \mathfrak{z}2))) \Big) + 2 w^5 (-1 + \eta)^5 \\
& (x^3 (-1 + \eta)^3 (2 \times (-1 + \eta) \times (10 \eta^2 + \eta (11 - 10 \eta t) - 11 \times (4 + \eta t)) \\
& \mathfrak{op} + (-1 + \eta t) \mathfrak{el} (-20 + 3 \mathfrak{op} (34 + 5 \mathfrak{z}1 + 5 \mathfrak{z}2))) - 3 x^2 (-1 + \eta)^2 \\
& (20 \eta^4 \mathfrak{op} + \eta^3 (2 - 20 \eta t) \mathfrak{op} + 9 \eta t \mathfrak{op} - 2 \eta^2 (55 + \eta t) \mathfrak{op} + \\
& \eta (88 + 13 \eta t) \mathfrak{op} + \eta (-1 + \eta t) \mathfrak{el} (-11 + 3 \mathfrak{op} (34 + 5 \mathfrak{z}1 + 5 \mathfrak{z}2))) \Big) + \\
& x (-1 + \eta) \eta (60 \eta^4 \mathfrak{op} + \eta^3 (6 - 60 \eta t) \mathfrak{op} + 53 \eta t \mathfrak{op} - 6 \eta^2 (55 + \eta t) \mathfrak{op} + \\
& \eta (264 + 13 \eta t) \mathfrak{op} + \eta (-1 + \eta t) \mathfrak{el} (-7 + 9 \mathfrak{op} (34 + 5 \mathfrak{z}1 + 5 \mathfrak{z}2))) - \\
& \eta^2 \mathfrak{op} (20 \eta^4 + \eta^3 (2 - 20 \eta t) + 20 \eta t - 2 \eta^2 (55 + \eta t) + \\
& \eta (88 - 3 \mathfrak{el} (34 + 5 \mathfrak{z}1 + 5 \mathfrak{z}2) + \eta t (2 + 3 \mathfrak{el} (34 + 5 \mathfrak{z}1 + 5 \mathfrak{z}2))) \Big) + \\
& 3 w^4 (-1 + \eta)^4 (2 x^4 (-1 + \eta)^4 (2 \times (-1 + \eta) \times (10 \eta^2 + \eta (11 - 10 \eta t) - 11 \times \\
& (4 + \eta t)) \mathfrak{op} + (-1 + \eta t) \mathfrak{el} (-22 + \mathfrak{op} (106 + 17 \mathfrak{z}1 + 17 \mathfrak{z}2))) \Big) + \\
& \eta^2 \mathfrak{op} (40 \eta^5 + \eta^4 (44 - 40 \eta t) + 40 \eta t - 4 \eta^3 (54 + 11 \eta t) + \\
& 2 \eta (88 - 3 \mathfrak{el} (34 + 5 \mathfrak{z}1 + 5 \mathfrak{z}2) + 3 \eta t (-1 + \mathfrak{el} (34 + 5 \mathfrak{z}1 + 5 \mathfrak{z}2))) + \\
& \eta^2 (-44 - \mathfrak{el} (158 + 25 \mathfrak{z}1 + 25 \mathfrak{z}2) + \\
& \eta t (50 + \mathfrak{el} (158 + 25 \mathfrak{z}1 + 25 \mathfrak{z}2))) \Big) + \\
& x^2 (-1 + \eta)^2 (240 \eta^5 \mathfrak{op} + 54 \eta t \mathfrak{op} - 48 \eta^4 (-3 + 5 \eta t) \mathfrak{op} - \\
& 12 \eta^3 (109 + 12 \eta t) \mathfrak{op} + \eta (88 \times (6 + \eta t) \mathfrak{op} + 6 \times (-1 + \eta t) \mathfrak{el} \\
& (-11 + 3 \mathfrak{op} (34 + 5 \mathfrak{z}1 + 5 \mathfrak{z}2))) + \eta^2 (22 \times (18 + 11 \eta t) \mathfrak{op} + \\
& (-1 + \eta t) \mathfrak{el} (-92 + 3 \mathfrak{op} (370 + 59 \mathfrak{z}1 + 59 \mathfrak{z}2))) \Big) -
\end{aligned}$$

$$\begin{aligned}
& \times (-1 + \eta) \eta \left( 160 \eta^5 \text{ep} + 106 \eta t \text{ep} - 8 \eta^4 (-17 + 20 \eta t) \text{ep} - \right. \\
& \quad 4 \eta^3 (217 + 34 \eta t) \text{ep} + 2 \eta (11 \times (24 + \eta t) \text{ep} + (-1 + \eta t) \text{el} \\
& \quad \quad \left. (-7 + 9 \text{ep} (34 + 5 \text{el} + 5 \text{el}2)) \right) + \eta^2 (4 \times (11 + 42 \eta t) \text{ep} + (-1 + \\
& \quad \quad \eta t) \text{el} (-18 + \text{ep} (686 + 109 \text{el} + 109 \text{el}2))) - x^3 (-1 + \eta)^3 \\
& \quad \left( 4 \times (-1 + \eta) \times (40 \eta^3 + \eta^2 (54 - 40 \eta t) - 4 \times (11 + 3 \eta t) - 3 \eta \right. \\
& \quad \quad \left. (55 + 18 \eta t)) \right) \text{ep} + (-1 + \eta t) \text{el} (-40 + 6 \text{ep} (34 + 5 \text{el} + 5 \text{el}2) + \\
& \quad \quad \eta (-118 + \text{ep} (794 + 127 \text{el} + 127 \text{el}2))) \left. \right) + w (x (-1 + \eta) - \eta) \\
& (-1 + \eta) \left( -x^3 (-1 + \eta)^3 (2 \times (-1 + \eta) \times (600 \eta^4 - 51 \eta t + 72 \eta \right. \\
& \quad \quad \left. (-16 + 3 \eta t) - 60 \eta^3 (-23 + 10 \eta t) - 8 \eta^2 (384 + 65 \eta t)) \right) \text{ep} - \\
& \quad (-1 + \eta t) \text{el} (132 + 456 \eta + 40 \eta^3 \text{ep} (43 + 2 \text{el}2) - \\
& \quad \quad 48 \eta^2 \text{ep} (119 + 8 \text{el}2) - 3 \eta \text{ep} (906 + 189 \text{el} + 197 \text{el}2) - \\
& \quad \quad 6 \text{ep} (17 \text{el} + 9 \times (2 + \text{el}2))) \left. \right) - 4 x^5 (-1 + \eta)^5 \text{ep} (30 \eta^3 + \\
& \quad \eta^2 (3 - 30 \eta t) + 2 \times (66 + \eta t - 6 \text{el} (11 + \text{el}2) + 6 \eta t \text{el} (11 + \text{el}2)) + \\
& \quad \eta (-165 + \text{el} (31 + 2 \text{el}2) + \eta t (28 - \text{el} (31 + 2 \text{el}2))) \left. \right) + 4 x^4 \\
& (-1 + \eta)^4 \left( (-1 + \eta) \times (150 \eta^3 + \eta^2 (255 - 150 \eta t) + 9 \times (-16 + 3 \eta t) - \right. \\
& \quad \quad \left. 14 \eta (51 + 5 \eta t)) \right) \text{ep} - (-1 + \eta t) \text{el} (33 + \text{ep} (5 \eta^2 (37 + 2 \text{el}2) - \\
& \quad \quad 12 \times (14 + 3 \text{el} + 3 \text{el}2) - 3 \eta (229 + 18 \text{el}2))) \left. \right) + \\
& \eta^2 \text{ep} (120 \eta^6 + \eta^5 (372 - 120 \eta t) + 94 \eta t + \eta (-5 \text{el} (15 \text{el} + \\
& \quad \quad 7 \times (2 + \text{el}2)) + \eta t (32 + 75 \text{el} \text{el} + 35 \text{el} (2 + \text{el}2))) \left. \right) + \\
& \quad 4 \eta^3 (42 - 3 \text{el} (53 + 2 \text{el}2) + \eta t (89 + 3 \text{el} (53 + 2 \text{el}2))) - 4 \eta^4 \\
& \quad (309 - \text{el} (61 + 2 \text{el}2) + \eta t (32 + \text{el} (61 + 2 \text{el}2))) + 3 \eta^2 (192 - \text{el} \\
& \quad \quad (222 + 39 \text{el} + 47 \text{el}2) + \eta t (-78 + \text{el} (222 + 39 \text{el} + 47 \text{el}2))) \left. \right) + \\
& x^2 (-1 + \eta)^2 (1200 \eta^6 \text{ep} + 136 \eta t \text{ep} - 120 \eta^5 (-19 + 10 \eta t) \text{ep} + \\
& \quad \eta (302 \eta t \text{ep} + (-1 + \eta t) \text{el} (-222 + 279 \text{ep} \text{el} + 143 \text{ep} (2 + \text{el}2))) - \\
& \quad 8 \eta^4 \text{ep} (1257 - 5 \text{el} (49 + 2 \text{el}2) + 5 \eta t (8 + \text{el} (49 + 2 \text{el}2))) + \\
& \quad 8 \eta^3 \text{ep} (390 - 3 \text{el} (247 + 14 \text{el}2) + \eta t (271 + \text{el} (741 + 42 \text{el}2))) + \\
& \quad 3 \eta^2 (2 \times (576 - 181 \eta t) \text{ep} + (-1 + \eta t) \text{el} \\
& \quad \quad (-136 + 3 \text{ep} (454 + 91 \text{el} + 99 \text{el}2))) \left. \right) - \\
& \times (-1 + \eta) \eta (600 \eta^6 \text{ep} + 266 \eta t \text{ep} - 300 \eta^5 (-5 + 2 \eta t) \text{ep} + \\
& \quad 2 \eta (98 \eta t \text{ep} + (-1 + \eta t) \text{el} (-27 + 126 \text{ep} \text{el} + 62 \text{ep} (2 + \text{el}2))) - \\
& \quad 4 \eta^4 \text{ep} (1401 - 5 \text{el} (55 + 2 \text{el}2) + 5 \eta t (20 + \text{el} (55 + 2 \text{el}2))) + \\
& \quad 8 \eta^3 \text{ep} (150 - 6 \text{el} (64 + 3 \text{el}2) + \eta t (179 + 6 \text{el} (64 + 3 \text{el}2))) + \\
& \quad 3 \eta^2 ((768 - 298 \eta t) \text{ep} + (-1 + \eta t) \text{el} \\
& \quad \quad (-28 + \text{ep} (902 + 171 \text{el} + 195 \text{el}2))) \left. \right) + w^2 (-1 + \eta)^2 \\
& (4 x^6 (-1 + \eta)^6 \text{ep} (44 + 10 \eta^3 + \eta^2 (1 - 10 \eta t) - \eta (55 + \eta t) - 44 \text{el} - \\
& \quad 4 \text{el} \text{el}2 + \eta t (11 + 4 \text{el} (11 + \text{el}2))) - 12 x^5 (-1 + \eta)^5 ((-1 + \eta) \times \\
& \quad (20 \eta^3 + \eta^2 (52 - 20 \eta t) - 2 \times (66 + \eta t) - \eta (55 + 52 \eta t)) \text{ep} + \\
& \quad (-1 + \eta t) \text{el} (-11 + 4 \text{ep} (35 + 3 \text{el} + 4 \text{el}2) + \eta \text{ep} (57 + 6 \text{el}2))) \left. \right) + \\
& 3 x^4 (-1 + \eta)^4 (2 \times (-1 + \eta) \times (-96 + 100 \eta^4 + \eta^3 (410 - 100 \eta t) + \\
& \quad \eta t - 12 \eta (113 + 5 \eta t) - 10 \eta^2 (5 + 41 \eta t)) \text{ep} + \\
& \quad (-1 + \eta t) \text{el} (-132 - 196 \eta + 20 \eta^2 \text{ep} (11 + 2 \text{el}2) + \\
& \quad \quad 2 \text{ep} (150 + 51 \text{el} + 43 \text{el}2) + \eta \text{ep} (2846 + 237 \text{el} + 317 \text{el}2))) \left. \right) + \\
& \eta^2 \text{ep} (40 \eta^7 + \eta^6 (364 - 40 \eta t) + 40 \eta t - 4 \eta^5 (-44 + 91 \eta t) + 2 \\
& \quad \eta (121 \eta t - 15 \text{el} \text{el} - 7 \text{el} (2 + \text{el}2) + \eta t \text{el} (15 \text{el} + 7 \times (2 + \text{el}2))) -
\end{aligned}$$



$$\begin{aligned}
& 4 \eta^4 (595 - \theta l (79 + 2 \mathfrak{z}2) + \eta t (-35 + \theta l (79 + 2 \mathfrak{z}2))) + \\
& 3 \eta^3 (408 - \theta l (594 + 39 \mathfrak{z}1 + 55 \mathfrak{z}2) + \\
& \quad \eta t (82 + \theta l (594 + 39 \mathfrak{z}1 + 55 \mathfrak{z}2))) + 3 \eta^2 (192 - \theta l \\
& \quad (262 + 75 \mathfrak{z}1 + 67 \mathfrak{z}2) + \eta t (-88 + \theta l (262 + 75 \mathfrak{z}1 + 67 \mathfrak{z}2))) + \\
& 3 x^2 (-1 + \eta)^2 (200 \eta^7 \theta p + 18 \eta t \theta p - 20 \eta^6 (-61 + 10 \eta t) \theta p - 20 \\
& \quad \eta^5 (13 + 61 \eta t) \theta p + 4 \eta^4 (-1718 + 215 \eta t + 150 \theta l - 150 \eta t \theta l) \theta p + \\
& \quad 2 \eta (192 \eta t \theta p + (-1 + \eta t) \theta l (-11 + 15 \theta p \mathfrak{z}1 + 7 \theta p (2 + \mathfrak{z}2))) + \\
& \quad 4 \eta^3 ((1140 + 119 \eta t) \theta p + (-1 + \eta t) \theta l (-41 + \\
& \quad \theta p (1460 + 111 \mathfrak{z}1 + 151 \mathfrak{z}2))) + 3 \eta^2 (2 \times (192 - 53 \eta t) \theta p + \\
& \quad (-1 + \eta t) \theta l (-92 + \theta p (562 + 177 \mathfrak{z}1 + 153 \mathfrak{z}2))) - \\
& x (-1 + \eta) \eta (240 \eta^7 \theta p + 12 \eta^5 (25 - 152 \eta t) \theta p + 106 \eta t \theta p - \\
& \quad 48 \eta^6 (-38 + 5 \eta t) \theta p + 2 \eta (487 \eta t \theta p + \\
& \quad (-1 + \eta t) \theta l (-7 + 45 \theta p \mathfrak{z}1 + 21 \theta p (2 + \mathfrak{z}2))) - \\
& \quad 12 \eta^4 \theta p (929 - \theta l (107 + 2 \mathfrak{z}2) + \eta t (-82 + \theta l (107 + 2 \mathfrak{z}2))) + \\
& \quad \eta^3 (12 \times (540 + 77 \eta t) \theta p + 6 \times (-1 + \eta t) \theta l \\
& \quad (-14 + \theta p (1474 + 105 \mathfrak{z}1 + 145 \mathfrak{z}2))) + 3 \eta^2 (4 \times (192 - 77 \eta t) \\
& \quad \theta p + (-1 + \eta t) \theta l (-54 + \theta p (1086 + 327 \mathfrak{z}1 + 287 \mathfrak{z}2))) - \\
& x^3 (-1 + \eta)^3 (4 \times (-1 + \eta) \times (200 \eta^5 + \eta^3 (470 - 1120 \eta t) - 102 \eta t - \\
& \quad 9 \eta (64 + 3 \eta t) - 40 \eta^4 (-28 + 5 \eta t) - 12 \eta^2 (348 + 25 \eta t)) \theta p + \\
& \quad (-1 + \eta t) \theta l (-40 + 40 \eta^3 \theta p (-17 + 2 \mathfrak{z}2) + 2 \theta p (14 + \\
& \quad 15 \mathfrak{z}1 + 7 \mathfrak{z}2) + 6 \eta^2 (-144 + \theta p (2886 + 231 \mathfrak{z}1 + 311 \mathfrak{z}2)) + \\
& \quad 3 \eta (-354 + \theta p (1162 + 381 \mathfrak{z}1 + 325 \mathfrak{z}2))) + w^3 (-1 + \eta)^3 \\
& (4 x^5 (-1 + \eta)^5 (3 \times (-1 + \eta) \times (10 \eta^2 + \eta (11 - 10 \eta t) - 11 \times (4 + \eta t)) \\
& \quad \theta p + (-1 + \eta t) \theta l (-11 + 4 \theta p (35 + 3 \mathfrak{z}1 + 4 \mathfrak{z}2))) - \\
& x^4 (-1 + \eta)^4 (2 \times (-1 + \eta) \times (-792 + 300 \eta^3 + \eta^2 (510 - 300 \eta t) - \\
& \quad 29 \eta t - 102 \eta (11 + 5 \eta t)) \theta p + (-1 + \eta t) \theta l (-396 - 196 \eta + \\
& \quad 18 \theta p (106 + 17 \mathfrak{z}1 + 17 \mathfrak{z}2) + \eta \theta p (2438 + 237 \mathfrak{z}1 + 301 \mathfrak{z}2))) - \\
& \eta^2 \theta p (120 \eta^6 + \eta^5 (372 - 120 \eta t) + 120 \eta t - 12 \eta^4 (42 + 31 \eta t) + \\
& \quad 2 \eta (96 - \theta l (138 + 45 \mathfrak{z}1 + 37 \mathfrak{z}2) + \\
& \quad \eta t (63 + \theta l (138 + 45 \mathfrak{z}1 + 37 \mathfrak{z}2))) + \eta^3 (-1644 - \\
& \quad \theta l (146 + 39 \mathfrak{z}1 + 39 \mathfrak{z}2) + \eta t (346 + \theta l (146 + 39 \mathfrak{z}1 + 39 \mathfrak{z}2))) + \\
& \quad \eta^2 (1464 - \theta l (1830 + 225 \mathfrak{z}1 + 241 \mathfrak{z}2) + \eta t \\
& \quad (-100 + \theta l (1830 + 225 \mathfrak{z}1 + 241 \mathfrak{z}2))) + \\
& x (-1 + \eta) \eta (600 \eta^6 \theta p + 318 \eta t \theta p - 300 \eta^5 (-5 + 2 \eta t) \theta p - \\
& \quad 12 \eta^4 (233 + 125 \eta t) \theta p + 6 \eta ((96 + 109 \eta t) \theta p + \\
& \quad (-1 + \eta t) \theta l (-7 + \theta p (138 + 45 \mathfrak{z}1 + 37 \mathfrak{z}2))) + \\
& \quad 2 \eta^3 (16 \times (-183 + 49 \eta t) \theta p + (-1 + \eta t) \theta l (-14 + \\
& \quad \theta p (598 + 105 \mathfrak{z}1 + 113 \mathfrak{z}2))) + \eta^2 (8 \times (747 - 55 \eta t) \theta p + \\
& \quad 3 \times (-1 + \eta t) \theta l (-54 + \theta p (2466 + 327 \mathfrak{z}1 + 343 \mathfrak{z}2))) - \\
& x^2 (-1 + \eta)^2 (1200 \eta^6 \theta p + 162 \eta t \theta p - 120 \eta^5 (-19 + 10 \eta t) \theta p - \\
& \quad 24 \eta^4 (251 + 95 \eta t) \theta p + 6 \eta (12 \times (8 + 13 \eta t) \theta p + \\
& \quad (-1 + \eta t) \theta l (-33 + \theta p (138 + 45 \mathfrak{z}1 + 37 \mathfrak{z}2))) + \\
& \quad 4 \eta^3 (3 \times (-598 + 233 \eta t) \theta p + (-1 + \eta t) \theta l (-41 + \\
& \quad \theta p (818 + 111 \mathfrak{z}1 + 127 \mathfrak{z}2))) + 3 \eta^2 (6 \times (508 - 23 \eta t) \theta p + \\
& \quad (-1 + \eta t) \theta l (-276 + \theta p (3738 + 531 \mathfrak{z}1 + 547 \mathfrak{z}2))) +
\end{aligned}$$

$$\begin{aligned}
& x^3 (-1 + \eta)^3 \left( 4 \times (-1 + \eta) \times (-48 + 300 \eta^4 + \eta^3 (690 - 300 \eta t) - \right. \\
& \quad 93 \eta t - 89 \eta (18 + \eta t) - 6 \eta^2 (149 + 115 \eta t) \left. \right) \Theta p + \\
& \quad (-1 + \eta t) \Theta l \left( -120 + \Theta p (276 + 90 \mathfrak{E}1 + 74 \mathfrak{E}2) + \right. \\
& \quad \eta^2 (-288 + \Theta p (4100 + 462 \mathfrak{E}1 + 558 \mathfrak{E}2)) + \\
& \quad \left. \eta (-1062 + \Theta p (7554 + 1143 \mathfrak{E}1 + 1159 \mathfrak{E}2)) \right) \left. \right) \left. \right) \left. \right) \left. \right) + \\
& 6 c \sigma^2 f(x (-1 + \eta) - \eta) (-1 + \eta)^3 \left( -4 x^7 (-1 + \eta)^7 (-1 + \eta + \Theta l - \eta t \Theta l) \right. \\
& \quad \Theta p + 2 \\
& \quad x^6 \\
& \quad (-1 + \eta)^6 \\
& \quad \left( -2 \times (-1 + w (-1 + \eta)) \times (-1 + \eta t) \right. \\
& \quad \quad \Theta l \mu 1 (2 + 5 \times (-1 + w (-1 + \eta)) \mu 1) + \\
& \quad \Theta p \left( -4 - 10 \eta + 14 \eta^2 + 4 \Theta l + 14 \eta \Theta l - 4 \eta t \Theta l - 14 \eta \eta t \Theta l + 2 \right. \\
& \quad \quad \Theta l \mu 1 - 2 \eta t \Theta l \mu 1 + 2 \Theta l \mu 2 - 2 \eta t \Theta l \mu 2 - 20 \mu 1 \mu 2 + 10 \\
& \quad \quad w^2 (-1 + \eta)^3 \mu 1 \mu 2 + 20 \eta \mu 1 \mu 2 + 10 \Theta l \mu 1 \mu 2 - 10 \eta t \\
& \quad \quad \Theta l \mu 1 \mu 2 + \Theta l \mu 1 \mathfrak{E}1 - \eta t \Theta l \mu 1 \mathfrak{E}1 + \Theta l \mu 1 \mathfrak{E}2 - \eta t \Theta l \mu 1 \\
& \quad \quad \mathfrak{E}2 - w (-1 + \eta) \times (-6 \times (1 + 5 \mu 1 \mu 2) + 6 \eta (1 + 5 \mu 1 \mu 2) - \\
& \quad \quad \left. \left. (-1 + \eta t) \Theta l (2 \times (3 + \mu 2) + \mu 1 (2 + 10 \mu 2 + \mathfrak{E}1 + \mathfrak{E}2)) \right) \right) \left. \right) + \\
& 2 x^5 (-1 + \eta)^5 \left( -2 \times (-1 + w (-1 + \eta)) \times (-1 + \eta t) \Theta l \mu 1 \right. \\
& \quad \left( -4 + 10 \mu 1 + 15 w^2 (-1 + \eta)^2 \mu 1 + 5 \eta (-2 + 5 \mu 1) - 2 \right. \\
& \quad \quad \mu 2 - w (-1 + \eta) \times (25 \times (1 + \eta) \mu 1 - 2 \times (3 + \mu 2)) \left. \right) \left. \right) + \\
& \Theta p \left( 2 + 22 \eta + 18 \eta^2 - 42 \eta^3 - 2 \Theta l - 24 \eta \Theta l - 42 \eta^2 \Theta l + 2 \eta t \Theta l + 24 \right. \\
& \quad \eta \eta t \Theta l + 42 \eta^2 \eta t \Theta l + 4 \eta t \mu 1 - 4 \eta \eta t \mu 1 - 6 \Theta l \mu 1 - 12 \\
& \quad \eta \Theta l \mu 1 + 6 \eta t \Theta l \mu 1 + 12 \eta \eta t \Theta l \mu 1 - 10 \eta t \mu 1^2 + 10 \eta \eta t \\
& \quad \mu 1^2 - 2 \Theta l \mu 1^2 + 2 \eta t \Theta l \mu 1^2 + 4 \mu 2 - 4 \eta \mu 2 - 6 \Theta l \mu 2 - 12 \\
& \quad \eta \Theta l \mu 2 + 6 \eta t \Theta l \mu 2 + 12 \eta \eta t \Theta l \mu 2 + 44 \mu 1 \mu 2 + 30 w^3 \\
& \quad (-1 + \eta)^4 \mu 1 \mu 2 + 76 \eta \mu 1 \mu 2 - 120 \eta^2 \mu 1 \mu 2 - 26 \Theta l \mu 1 \\
& \quad \mu 2 - 60 \eta \Theta l \mu 1 \mu 2 + 26 \eta t \Theta l \mu 1 \mu 2 + 60 \eta \eta t \Theta l \mu 1 \mu 2 + 2 \\
& \quad \mu 2^2 - 2 \eta \mu 2^2 - 2 \Theta l \mu 2^2 + 2 \eta t \Theta l \mu 2^2 - 3 \Theta l \mu 1 \mathfrak{E}1 - 6 \eta \Theta l \\
& \quad \mu 1 \mathfrak{E}1 + 3 \eta t \Theta l \mu 1 \mathfrak{E}1 + 6 \eta \eta t \Theta l \mu 1 \mathfrak{E}1 - \Theta l \mu 1^2 \mathfrak{E}1 + \eta t \Theta l \\
& \quad \mu 1^2 \mathfrak{E}1 - 2 \Theta l \mu 1 \mu 2 \mathfrak{E}1 + 2 \eta t \Theta l \mu 1 \mu 2 \mathfrak{E}1 - 3 \Theta l \mu 1 \mathfrak{E}2 - 6 \eta \\
& \quad \Theta l \mu 1 \mathfrak{E}2 + 3 \eta t \Theta l \mu 1 \mathfrak{E}2 + 6 \eta \eta t \Theta l \mu 1 \mathfrak{E}2 - \Theta l \mu 1^2 \mathfrak{E}2 + \eta t \\
& \quad \Theta l \mu 1^2 \mathfrak{E}2 - 2 \Theta l \mu 1 \mu 2 \mathfrak{E}2 + 2 \eta t \Theta l \mu 1 \mu 2 \mathfrak{E}2 - w^2 (-1 + \eta)^2 \\
& \quad \left( 60 \eta^2 \mu 1 \mu 2 + 2 \times (-3 + 5 \eta t \mu 1^2 - 52 \mu 1 \mu 2 - \mu 2^2) \right. + \\
& \quad \quad 2 \eta (3 - 5 \eta t \mu 1^2 + 22 \mu 1 \mu 2 + \mu 2^2) - (-1 + \eta t) \Theta l (2 \times (3 + 3 \mu 2 + \mu 2^2) + \\
& \quad \quad 3 \mu 1 (2 + \mathfrak{E}1 + \mathfrak{E}2) + \mu 1^2 (2 + \mathfrak{E}1 + \mathfrak{E}2) + 2 \mu 1 \mu 2 (13 + \mathfrak{E}1 + \mathfrak{E}2)) \left. \right) + 2 \\
& \quad w (-1 + \eta) \times (-6 - 2 \eta t \mu 1 + 10 \eta t \mu 1^2 - 2 \mu 2 - 59 \mu 1 \mu 2 - 2 \mu 2^2 + \\
& \quad 18 \eta^2 (1 + 5 \mu 1 \mu 2) - (-1 + \eta t) \Theta l (2 \times (3 + 3 \mu 2 + \mu 2^2) + \\
& \quad \quad 3 \mu 1 (2 + \mathfrak{E}1 + \mathfrak{E}2) + \mu 1^2 (2 + \mathfrak{E}1 + \mathfrak{E}2) + 2 \mu 1 \mu 2 (13 + \mathfrak{E}1 + \mathfrak{E}2)) \left. \right) + \\
& \quad \eta (-12 + 2 \eta t (1 - 5 \mu 1) \mu 1 + 2 \mu 2 - 31 \mu 1 \mu 2 + 2 \mu 2^2 - \\
& \quad \quad 3 \times (-1 + \eta t) \Theta l (2 \times (3 + \mu 2) + \mu 1 (2 + 10 \mu 2 + \mathfrak{E}1 + \mathfrak{E}2)) \left. \right) \left. \right) \left. \right) \left. \right) - \\
& x^4 (-1 + \eta)^4 \left( -4 \times (-1 + \eta) \Theta p (5 \eta + 30 \eta^2 + 35 \eta^3 + 4 \eta t \mu 1 + 10 \eta \eta t \right. \\
& \quad \mu 1 - 10 \eta t \mu 1^2 - 25 \eta \eta t \mu 1^2 + 4 \mu 2 + 10 \eta \mu 2 + 14 \mu 1 \\
& \quad \mu 2 + 15 w^4 (-1 + \eta)^4 \mu 1 \mu 2 + 110 \eta \mu 1 \mu 2 + 150 \eta^2 \\
& \quad \mu 1 \mu 2 + 2 \eta t \mu 1 \mu 2 + 2 \mu 2^2 + 5 \eta \mu 2^2 - w^3 (-1 + \eta)^3 \\
& \quad \left. \left( 1 - 15 \eta t \mu 1^2 + 3 \times (22 + 25 \eta) \mu 1 \mu 2 + 3 \mu 2^2 \right) + w^2 (-1 + \eta)^2 \right.
\end{aligned}$$

$$\begin{aligned}
& (6 + 6 \mu_2 + 111 \mu_1 \mu_2 + 75 \eta^2 \mu_1 \mu_2 + 8 \mu_2^2 + 2 \eta t \mu_1 (3 - 20 \mu_1 + \mu_2) + \\
& \quad 5 \eta (3 - 5 \eta t \mu_1^2 + 52 \mu_1 \mu_2 + \mu_2^2)) - w (-1 + \eta) \times \\
& (3 + 10 \mu_2 + 74 \mu_1 \mu_2 + 7 \mu_2^2 + \eta t \mu_1 (10 - 35 \mu_1 + 4 \mu_2) + 45 \eta^2 \\
& \quad (1 + 5 \mu_1 \mu_2) + 5 \eta (6 + 2 \eta t (1 - 5 \mu_1) \mu_1 + 2 \mu_2 + 59 \mu_1 \mu_2 + 2 \mu_2^2))) + \\
& (-1 + \eta t) \theta l (-6 + 6 \theta p + 20 \eta \theta p + 120 \eta^2 \theta p + 140 \eta^3 \theta p - 20 \mu_1 - 64 \\
& \quad \eta \mu_1 - 80 \eta^2 \mu_1 + 24 \theta p \mu_1 + 60 \eta \theta p \mu_1 + 60 \eta^2 \theta p \mu_1 + 14 \\
& \quad \mu_1^2 + 60 w^4 (-1 + \eta)^4 \mu_1^2 + 160 \eta \mu_1^2 + 200 \eta^2 \mu_1^2 + 14 \theta p \\
& \quad \mu_1^2 + 20 \eta \theta p \mu_1^2 - 12 \mu_2 + 24 \theta p \mu_2 + 60 \eta \theta p \mu_2 + 60 \eta^2 \\
& \quad \theta p \mu_2 - 28 \mu_1 \mu_2 - 32 \eta \mu_1 \mu_2 + 56 \theta p \mu_1 \mu_2 + 260 \eta \theta p \mu_1 \\
& \quad \mu_2 + 300 \eta^2 \theta p \mu_1 \mu_2 - 6 \mu_2^2 + 14 \theta p \mu_2^2 + 20 \eta \theta p \mu_2^2 + 3 \\
& \quad \theta p \mathfrak{z}1 + 12 \theta p \mu_1 \mathfrak{z}1 + 30 \eta \theta p \mu_1 \mathfrak{z}1 + 30 \eta^2 \theta p \mu_1 \mathfrak{z}1 + 7 \theta p \\
& \quad \mu_1^2 \mathfrak{z}1 + 10 \eta \theta p \mu_1^2 \mathfrak{z}1 + 6 \theta p \mu_2 \mathfrak{z}1 + 14 \theta p \mu_1 \mu_2 \mathfrak{z}1 + 20 \\
& \quad \eta \theta p \mu_1 \mu_2 \mathfrak{z}1 + 3 \theta p \mu_2^2 \mathfrak{z}1 + 3 \theta p \mathfrak{z}2 + 12 \theta p \mu_1 \mathfrak{z}2 + 30 \\
& \quad \eta \theta p \mu_1 \mathfrak{z}2 + 30 \eta^2 \theta p \mu_1 \mathfrak{z}2 + 7 \theta p \mu_1^2 \mathfrak{z}2 + 10 \eta \theta p \mu_1^2 \\
& \quad \mathfrak{z}2 + 6 \theta p \mu_2 \mathfrak{z}2 + 14 \theta p \mu_1 \mu_2 \mathfrak{z}2 + 20 \eta \theta p \mu_1 \mu_2 \mathfrak{z}2 + 3 \theta p \\
& \quad \mu_2^2 \mathfrak{z}2 + w^2 (-1 + \eta)^2 (2 \times ((147 + 320 \eta + 100 \eta^2) \mu_1^2 - \\
& \quad 9 (1 + \mu_2)^2 - 2 \mu_1 (21 + 13 \mu_2 + 8 \eta (3 + \mu_2))) + \\
& \quad \theta p (42 + 72 \mu_2 + 34 \mu_2^2 + 9 \mathfrak{z}1 + 18 \mu_2 \mathfrak{z}1 + 9 \mu_2^2 \mathfrak{z}1 + 9 \mathfrak{z}2 + \\
& \quad 18 \mu_2 \mathfrak{z}2 + 9 \mu_2^2 \mathfrak{z}2 + 36 \mu_1 (2 + \mathfrak{z}1 + \mathfrak{z}2) + 17 \mu_1^2 (2 + \mathfrak{z}1 + \mathfrak{z}2) + \\
& \quad 2 \mu_1 \mu_2 (92 + 17 \mathfrak{z}1 + 17 \mathfrak{z}2) + 10 \eta (2 \times (3 + 3 \mu_2 + \mu_2^2) + 3 \mu_1 \\
& \quad (2 + \mathfrak{z}1 + \mathfrak{z}2) + \mu_1^2 (2 + \mathfrak{z}1 + \mathfrak{z}2) + 2 \mu_1 \mu_2 (13 + \mathfrak{z}1 + \mathfrak{z}2))) - \\
& w (-1 + \eta) \times (2 \times ((69 + 280 \eta + 200 \eta^2) \mu_1^2 - 9 (1 + \mu_2)^2 - \\
& \quad 2 \mu_1 (19 + 20 \eta^2 + 17 \mu_2 + 8 \eta (5 + 2 \mu_2))) + \\
& \quad \theta p (30 + 76 \mu_2 + 38 \mu_2^2 + 9 \mathfrak{z}1 + 18 \mu_2 \mathfrak{z}1 + 9 \mu_2^2 \mathfrak{z}1 + 9 \mathfrak{z}2 + \\
& \quad 18 \mu_2 \mathfrak{z}2 + 9 \mu_2^2 \mathfrak{z}2 + 38 \mu_1 (2 + \mathfrak{z}1 + \mathfrak{z}2) + 19 \mu_1^2 (2 + \mathfrak{z}1 + \mathfrak{z}2) + \\
& \quad 2 \mu_1 \mu_2 (98 + 19 \mathfrak{z}1 + 19 \mathfrak{z}2) + 20 \eta (2 \times (3 + 3 \mu_2 + \mu_2^2) + \\
& \quad 3 \mu_1 (2 + \mathfrak{z}1 + \mathfrak{z}2) + \mu_1^2 (2 + \mathfrak{z}1 + \mathfrak{z}2) + 2 \mu_1 \mu_2 (13 + \mathfrak{z}1 + \mathfrak{z}2))) + \\
& \quad 30 \eta^2 (2 \times (3 + \mu_2) + \mu_1 (2 + 10 \mu_2 + \mathfrak{z}1 + \mathfrak{z}2))) - w^3 \\
& (-1 + \eta)^3 (10 \times (23 + 24 \eta) \mu_1^2 - 6 (1 + \mu_2)^2 - 4 \mu_1 (7 + 3 \mu_2) + \\
& \quad \theta p (5 \mu_1^2 (2 + \mathfrak{z}1 + \mathfrak{z}2) + (1 + \mu_2)^2 (10 + 3 \mathfrak{z}1 + 3 \mathfrak{z}2) + \\
& \quad 2 \mu_1 (5 \times (2 + \mathfrak{z}1 + \mathfrak{z}2) + \mu_2 (22 + 5 \mathfrak{z}1 + 5 \mathfrak{z}2)))) - \\
& x^2 (-1 + \eta)^2 (2 \times (-1 + \eta) \theta p (-20 \eta^3 - 60 \eta^4 - 42 \eta^5 - 6 \eta t - 9 \eta \eta t - 12 \\
& \quad \eta t \mu_1 - 30 \eta \eta t \mu_1 - 48 \eta^2 \eta t \mu_1 - 40 \eta^3 \eta t \mu_1 - 6 \eta t \\
& \quad \mu_1^2 + 21 \eta \eta t \mu_1^2 + 120 \eta^2 \eta t \mu_1^2 + 100 \eta^3 \eta t \mu_1^2 - 12 \eta \\
& \quad \mu_2 - 48 \eta^2 \mu_2 - 40 \eta^3 \mu_2 - 12 \eta t \mu_2 - 18 \eta \eta t \mu_2 - 12 \eta \mu_1 \\
& \quad \mu_2 - 168 \eta^2 \mu_1 \mu_2 - 440 \eta^3 \mu_1 \mu_2 - 300 \eta^4 \mu_1 \mu_2 - 16 \eta t \\
& \quad \mu_1 \mu_2 - 42 \eta \eta t \mu_1 \mu_2 - 24 \eta^2 \eta t \mu_1 \mu_2 - 6 \eta \mu_2^2 - 24 \eta^2 \\
& \quad \mu_2^2 - 20 \eta^3 \mu_2^2 - 6 \eta t \mu_2^2 - 9 \eta \eta t \mu_2^2 + 2 w^5 (-1 + \eta)^5 \\
& \quad (-5 \eta t \mu_1^2 + \mu_2 ((7 + 15 \eta) \mu_1 + \mu_2)) + 6 w^4 (-1 + \eta)^4 \\
& \quad (\eta t \mu_1 (3 \times (4 + 5 \eta) \mu_1 + \mu_2) - \mu_2 ((7 + 36 \eta + 30 \eta^2) \mu_1 + 3 \eta \mu_2)) + w^3 \\
& (-1 + \eta)^3 (2 + 8 \mu_2 + 56 \mu_1 \mu_2 + 300 \eta^3 \mu_1 \mu_2 - \\
& \quad 6 \mu_2^2 + 12 \eta^2 (1 - 15 \eta t \mu_1^2 + 66 \mu_1 \mu_2 + 3 \mu_2^2) + \\
& \quad 2 \eta t (-66 \mu_1^2 + 3 (1 + \mu_2)^2 + 5 \mu_1 (2 + \mu_2)) + \\
& \quad \eta (12 - 345 \eta t \mu_1^2 + 6 \times (4 + 83 \mu_1) \mu_2 + 42 \mu_2^2 + 9 \eta t (1 + \mu_2)^2 +
\end{aligned}$$

$$\begin{aligned}
& 6 \eta t \mu_1 (7 + 3 \mu_2) \Big) - w^2 (-1 + \eta)^2 (150 \eta^4 \mu_1 \mu_2 + \\
& 4 \times (3 + 8 \mu_1 - \mu_2) \mu_2 - 20 \eta^3 (-3 + 5 \eta t \mu_1^2 - 52 \mu_1 \mu_2 - \mu_2^2) + \\
& 12 \eta^2 (6 + 6 \mu_2 + 111 \mu_1 \mu_2 + 8 \mu_2^2 + 2 \eta t \mu_1 (3 - 20 \mu_1 + \mu_2) \Big) + \\
& 2 \eta t (-41 \mu_1^2 + 9 (1 + \mu_2)^2 + 3 \mu_1 (8 + 9 \mu_2) \Big) + 3 \eta (6 + 8 \times (3 + 20 \mu_1) \\
& \mu_2 + 12 \mu_2^2 + \eta t (-147 \mu_1^2 + 9 (1 + \mu_2)^2 + \mu_1 (42 + 26 \mu_2) \Big) \Big) + w \\
& (-1 + \eta) \times (4 \times (1 + \mu_1) \mu_2 + 90 \eta^4 (1 + 5 \mu_1 \mu_2) - 20 \eta^3 \\
& (-6 + 2 \eta t \mu_1 (-1 + 5 \mu_1) - 2 \mu_2 - 59 \mu_1 \mu_2 - 2 \mu_2^2) + \\
& 12 \eta^2 (3 + 10 \mu_2 + 74 \mu_1 \mu_2 + 7 \mu_2^2 + \eta t \mu_1 (10 - 35 \mu_1 + 4 \mu_2) \Big) + \eta t \\
& (-6 \mu_1^2 + 18 (1 + \mu_2)^2 + \mu_1 (40 + 54 \mu_2) \Big) + \eta (6 \mu_2 (10 + 30 \mu_1 + 3 \mu_2) + \\
& 3 \eta t (-69 \mu_1^2 + 9 (1 + \mu_2)^2 + \mu_1 (38 + 34 \mu_2) \Big) \Big) \Big) - \\
& (-1 + \eta t) \Theta_1 (6 + 24 \eta + 18 \eta^2 - 6 \Theta p - 36 \eta \Theta p - 36 \eta^2 \Theta p - 40 \eta^3 \Theta p - \\
& 120 \eta^4 \Theta p - 84 \eta^5 \Theta p + 12 \mu_1 + 48 \eta \mu_1 + 60 \eta^2 \mu_1 + 64 \eta^3 \mu_1 + 40 \\
& \eta^4 \mu_1 - 12 \Theta p \mu_1 - 84 \eta \Theta p \mu_1 - 144 \eta^2 \Theta p \mu_1 - 120 \eta^3 \Theta p \mu_1 - 60 \\
& \eta^4 \Theta p \mu_1 + 6 \mu_1^2 + 24 \eta \mu_1^2 - 42 \eta^2 \mu_1^2 - 160 \eta^3 \mu_1^2 - 100 \eta^4 \\
& \mu_1^2 - 6 \Theta p \mu_1^2 - 48 \eta \Theta p \mu_1^2 - 84 \eta^2 \Theta p \mu_1^2 - 40 \eta^3 \Theta p \mu_1^2 + 12 \\
& \mu_2 + 48 \eta \mu_2 + 36 \eta^2 \mu_2 - 12 \Theta p \mu_2 - 84 \eta \Theta p \mu_2 - 144 \eta^2 \Theta p \\
& \mu_2 - 120 \eta^3 \Theta p \mu_2 - 60 \eta^4 \Theta p \mu_2 + 12 \mu_1 \mu_2 + 64 \eta \mu_1 \mu_2 + 84 \\
& \eta^2 \mu_1 \mu_2 + 32 \eta^3 \mu_1 \mu_2 - 12 \Theta p \mu_1 \mu_2 - 108 \eta \Theta p \mu_1 \mu_2 - 336 \\
& \eta^2 \Theta p \mu_1 \mu_2 - 520 \eta^3 \Theta p \mu_1 \mu_2 - 300 \eta^4 \Theta p \mu_1 \mu_2 + 6 \mu_2^2 + 24 \\
& \eta \mu_2^2 + 18 \eta^2 \mu_2^2 - 6 \Theta p \mu_2^2 - 48 \eta \Theta p \mu_2^2 - 84 \eta^2 \Theta p \mu_2^2 - 40 \\
& \eta^3 \Theta p \mu_2^2 + 4 w^5 (-1 + \eta)^5 \mu_1 ((7 + 10 \eta) \mu_1 + \mu_2) - 12 w^4 \\
& (-1 + \eta)^4 \mu_1 ((7 + 24 \eta + 15 \eta^2) \mu_1 + 2 \eta \mu_2) - 3 \Theta p \Xi_1 - 18 \\
& \eta \Theta p \Xi_1 - 18 \eta^2 \Theta p \Xi_1 - 6 \Theta p \mu_1 \Xi_1 - 42 \eta \Theta p \mu_1 \Xi_1 - 72 \eta^2 \Theta p \\
& \mu_1 \Xi_1 - 60 \eta^3 \Theta p \mu_1 \Xi_1 - 30 \eta^4 \Theta p \mu_1 \Xi_1 - 3 \Theta p \mu_1^2 \Xi_1 - 24 \\
& \eta \Theta p \mu_1^2 \Xi_1 - 42 \eta^2 \Theta p \mu_1^2 \Xi_1 - 20 \eta^3 \Theta p \mu_1^2 \Xi_1 - 6 \Theta p \mu_2 \\
& \Xi_1 - 36 \eta \Theta p \mu_2 \Xi_1 - 36 \eta^2 \Theta p \mu_2 \Xi_1 - 6 \Theta p \mu_1 \mu_2 \Xi_1 - 48 \eta \\
& \Theta p \mu_1 \mu_2 \Xi_1 - 84 \eta^2 \Theta p \mu_1 \mu_2 \Xi_1 - 40 \eta^3 \Theta p \mu_1 \mu_2 \Xi_1 - 3 \Theta p \\
& \mu_2^2 \Xi_1 - 18 \eta \Theta p \mu_2^2 \Xi_1 - 18 \eta^2 \Theta p \mu_2^2 \Xi_1 - 3 \Theta p \Xi_2 - 18 \eta \\
& \Theta p \Xi_2 - 18 \eta^2 \Theta p \Xi_2 - 6 \Theta p \mu_1 \Xi_2 - 42 \eta \Theta p \mu_1 \Xi_2 - 72 \eta^2 \Theta p \\
& \mu_1 \Xi_2 - 60 \eta^3 \Theta p \mu_1 \Xi_2 - 30 \eta^4 \Theta p \mu_1 \Xi_2 - 3 \Theta p \mu_1^2 \Xi_2 - 24 \\
& \eta \Theta p \mu_1^2 \Xi_2 - 42 \eta^2 \Theta p \mu_1^2 \Xi_2 - 20 \eta^3 \Theta p \mu_1^2 \Xi_2 - 6 \Theta p \mu_2 \\
& \Xi_2 - 36 \eta \Theta p \mu_2 \Xi_2 - 36 \eta^2 \Theta p \mu_2 \Xi_2 - 6 \Theta p \mu_1 \mu_2 \Xi_2 - 48 \eta \\
& \Theta p \mu_1 \mu_2 \Xi_2 - 84 \eta^2 \Theta p \mu_1 \mu_2 \Xi_2 - 40 \eta^3 \Theta p \mu_1 \mu_2 \Xi_2 - 3 \Theta p \\
& \mu_2^2 \Xi_2 - 18 \eta \Theta p \mu_2^2 \Xi_2 - 18 \eta^2 \Theta p \mu_2^2 \Xi_2 - w^2 (-1 + \eta)^2 \\
& (100 \eta^4 \mu_1^2 + 8 \eta (41 \mu_1^2 - 9 (1 + \mu_2)^2 - 3 \mu_1 (8 + 9 \mu_2) \Big) + \\
& 2 \times (5 \mu_1^2 - 9 (1 + \mu_2)^2 - 2 \mu_1 (9 + 17 \mu_2) \Big) + \\
& 6 \eta \Theta p (24 + 9 \Xi_1 + 9 \Xi_2 + 27 \mu_1 (2 + \Xi_1 + \Xi_2) + 14 \mu_1^2 (2 + \Xi_1 + \Xi_2) + \\
& 18 \mu_2 (3 + \Xi_1 + \Xi_2) + \mu_2^2 (28 + 9 \Xi_1 + 9 \Xi_2) + \\
& 2 \mu_1 \mu_2 (53 + 14 \Xi_1 + 14 \Xi_2) \Big) + \Theta p (9 \times (2 + \Xi_1 + \Xi_2) + \\
& 24 \mu_1 (2 + \Xi_1 + \Xi_2) + 13 \mu_1^2 (2 + \Xi_1 + \Xi_2) + 6 \mu_2 (8 + 3 \Xi_1 + 3 \Xi_2) + \\
& \mu_2^2 (26 + 9 \Xi_1 + 9 \Xi_2) + \mu_1 \mu_2 (80 + 26 \Xi_1 + 26 \Xi_2) \Big) + \\
& 4 \eta^3 (8 \mu_1 (-3 + 20 \mu_1 - \mu_2) + 5 \Theta p (2 \times (3 + 3 \mu_2 + \mu_2^2) + \\
& 3 \mu_1 (2 + \Xi_1 + \Xi_2) + \mu_1^2 (2 + \Xi_1 + \Xi_2) + 2 \mu_1 \mu_2 (13 + \Xi_1 + \Xi_2) \Big) \Big) + \\
& 6 \eta^2 (-9 - 42 \mu_1 + 147 \mu_1^2 - 18 \mu_2 - 26 \mu_1 \mu_2 - 9 \mu_2^2 + \\
& \Theta p (42 + 9 \Xi_1 + 9 \Xi_2 + 36 \mu_1 (2 + \Xi_1 + \Xi_2) +
\end{aligned}$$

$$\begin{aligned}
& 17 \mu_1^2 (2 + \mu_1 + \mu_2) + 18 \mu_2 (4 + \mu_1 + \mu_2) + \\
& \mu_2^2 (34 + 9 \mu_1 + 9 \mu_2) + 2 \mu_1 \mu_2 (92 + 17 \mu_1 + 17 \mu_2) \Big) \Big) + w \\
& (-1 + \eta) \times \Big( -6 \times (3 \mu_1^2 + 3 (1 + \mu_2)^2 + \mu_1 (6 + 8 \mu_2)) + \\
& 8 \eta (3 \mu_1^2 - 9 (1 + \mu_2)^2 - \mu_1 (20 + 27 \mu_2)) + \\
& 10 \eta^4 (4 \mu_1 (-1 + 5 \mu_1) + 6 \theta p (3 + \mu_2) + 3 \theta p \mu_1 (2 + 10 \mu_2 + \mu_1 + \mu_2)) + \\
& 6 \eta \theta p (9 \times (2 + \mu_1 + \mu_2) + 24 \mu_1 (2 + \mu_1 + \mu_2) + \\
& 13 \mu_1^2 (2 + \mu_1 + \mu_2) + 6 \mu_2 (8 + 3 \mu_1 + 3 \mu_2) + \\
& \mu_2^2 (26 + 9 \mu_1 + 9 \mu_2) + \mu_1 \mu_2 (80 + 26 \mu_1 + 26 \mu_2) \Big) + \\
& 8 \eta^3 (2 \mu_1 (-10 + 35 \mu_1 - 4 \mu_2) + 5 \theta p (2 \times (3 + 3 \mu_2 + \mu_2^2) + \\
& 3 \mu_1 (2 + \mu_1 + \mu_2) + \mu_1^2 (2 + \mu_1 + \mu_2) + 2 \mu_1 \mu_2 (13 + \mu_1 + \mu_2)) \Big) + \\
& 6 \eta^2 (-9 - 38 \mu_1 + 69 \mu_1^2 - 18 \mu_2 - 34 \mu_1 \mu_2 - 9 \mu_2^2 + \theta p \\
& (30 + 9 \mu_1 + 9 \mu_2 + 38 \mu_1 (2 + \mu_1 + \mu_2) + 19 \mu_1^2 (2 + \mu_1 + \mu_2) + \\
& 2 \mu_2 (38 + 9 \mu_1 + 9 \mu_2) + \mu_2^2 (38 + 9 \mu_1 + 9 \mu_2) + \\
& 2 \mu_1 \mu_2 (98 + 19 \mu_1 + 19 \mu_2)) \Big) + \theta p (11 \mu_1^2 (2 + \mu_1 + \mu_2) + \\
& (1 + \mu_2) \times (9 \times (2 + \mu_1 + \mu_2) + \mu_2 (22 + 9 \mu_1 + 9 \mu_2)) + \\
& \mu_1 (20 \times (2 + \mu_1 + \mu_2) + \mu_2 (48 + 22 \mu_1 + 22 \mu_2)) \Big) \Big) + w^3 \\
& (-1 + \eta)^3 (78 \mu_1^2 + 240 \eta^3 \mu_1^2 - 6 (1 + \mu_2)^2 - 12 \mu_1 (1 + 3 \mu_2) + \\
& 8 \eta (66 \mu_1^2 - 3 (1 + \mu_2)^2 - 5 \mu_1 (2 + \mu_2)) + \\
& \theta p (5 \mu_1^2 (2 + \mu_1 + \mu_2) + (1 + \mu_2)^2 (10 + 3 \mu_1 + 3 \mu_2) + \\
& 2 \mu_1 (5 \times (2 + \mu_1 + \mu_2) + \mu_2 (22 + 5 \mu_1 + 5 \mu_2)) \Big) + \\
& 6 \eta \theta p (5 \mu_1^2 (2 + \mu_1 + \mu_2) + (1 + \mu_2)^2 (10 + 3 \mu_1 + 3 \mu_2) + \\
& 2 \mu_1 (5 \times (2 + \mu_1 + \mu_2) + \mu_2 (22 + 5 \mu_1 + 5 \mu_2)) \Big) + \\
& 6 \eta^2 (115 \mu_1^2 - 3 (1 + \mu_2)^2 - 2 \mu_1 (7 + 3 \mu_2) + \theta p \\
& (5 \mu_1^2 (2 + \mu_1 + \mu_2) + (1 + \mu_2)^2 (10 + 3 \mu_1 + 3 \mu_2) + \\
& 2 \mu_1 (5 \times (2 + \mu_1 + \mu_2) + \mu_2 (22 + 5 \mu_1 + 5 \mu_2)) \Big) \Big) \Big) \Big) + \\
& 2 x^3 (-1 + \eta)^3 \Big( (-1 + \eta) \theta p (-20 \eta^2 - 80 \eta^3 - 70 \eta^4 - 3 \eta t - 10 \eta t \mu_1 - 32 \\
& \eta \eta t \mu_1 - 40 \eta^2 \eta t \mu_1 + 7 \eta t \mu_1^2 + 80 \eta \eta t \mu_1^2 + 100 \eta^2 \eta t \mu_1^2 - 4 \\
& \mu_2 - 32 \eta \mu_2 - 40 \eta^2 \mu_2 - 6 \eta t \mu_2 - 4 \mu_1 \mu_2 + 10 w^5 (-1 + \eta)^5 \\
& \mu_1 \mu_2 - 112 \eta \mu_1 \mu_2 - 440 \eta^2 \mu_1 \mu_2 - 400 \eta^3 \mu_1 \mu_2 - 14 \eta t \mu_1 \\
& \mu_2 - 16 \eta \eta t \mu_1 \mu_2 - 2 \mu_2^2 - 16 \eta \mu_2^2 - 20 \eta^2 \mu_2^2 - 3 \eta t \mu_2^2 - 6 w^4 \\
& (-1 + \eta)^4 (-5 \eta t \mu_1^2 + \mu_2 (4 \times (3 + 5 \eta) \mu_1 + \mu_2)) \Big) + w^3 (-1 + \eta)^3 \\
& (4 - 115 \eta t \mu_1^2 + 300 \eta^2 \mu_1 \mu_2 + 2 \times (4 + 83 \mu_1) \mu_2 + 14 \mu_2^2 + 3 \eta t (1 + \mu_2)^2 + \\
& 2 \eta t \mu_1 (7 + 3 \mu_2) + 8 \eta (1 - 15 \eta t \mu_1^2 + 66 \mu_1 \mu_2 + 3 \mu_2^2)) - w^2 \\
& (-1 + \eta)^2 (6 + 200 \eta^3 \mu_1 \mu_2 + 8 \times (3 + 20 \mu_1) \mu_2 + 12 \mu_2^2 - \\
& 20 \eta^2 (-3 + 5 \eta t \mu_1^2 - 52 \mu_1 \mu_2 - \mu_2^2) + \\
& 8 \eta (6 + 6 \mu_2 + 111 \mu_1 \mu_2 + 8 \mu_2^2 + 2 \eta t \mu_1 (3 - 20 \mu_1 + \mu_2)) + \\
& \eta t (-147 \mu_1^2 + 9 (1 + \mu_2)^2 + \mu_1 (42 + 26 \mu_2)) \Big) + w \\
& (-1 + \eta) \times (2 \mu_2 (10 + 30 \mu_1 + 3 \mu_2) + 120 \eta^3 (1 + 5 \mu_1 \mu_2) - \\
& 20 \eta^2 (-6 + 2 \eta t \mu_1 (-1 + 5 \mu_1) - 2 \mu_2 - 59 \mu_1 \mu_2 - 2 \mu_2^2) + \\
& 8 \eta (3 + 10 \mu_2 + 74 \mu_1 \mu_2 + 7 \mu_2^2 + \eta t \mu_1 (10 - 35 \mu_1 + 4 \mu_2)) + \\
& \eta t (-69 \mu_1^2 + 9 (1 + \mu_2)^2 + \mu_1 (38 + 34 \mu_2)) \Big) \Big) - \\
& (-1 + \eta t) \theta l (6 + 9 \eta - 6 \theta p - 12 \eta \theta p - 20 \eta^2 \theta p - 80 \eta^3 \theta p - 70 \eta^4 \\
& \theta p + 12 \mu_1 + 30 \eta \mu_1 + 48 \eta^2 \mu_1 + 40 \eta^3 \mu_1 - 14 \theta p \mu_1 - 48 \eta
\end{aligned}$$

$$\begin{aligned}
& \Theta \mu_1 - 60 \eta^2 \Theta \mu_1 - 40 \eta^3 \Theta \mu_1 + 6 \mu_1^2 + 10 w^5 (-1 + \eta)^5 \\
& \mu_1^2 - 21 \eta \mu_1^2 - 120 \eta^2 \mu_1^2 - 100 \eta^3 \mu_1^2 - 8 \Theta \mu_1^2 - 28 \eta \\
& \Theta \mu_1^2 - 20 \eta^2 \Theta \mu_1^2 + 12 \mu_2 + 18 \eta \mu_2 - 14 \Theta \mu_2 - 48 \eta \Theta \\
& \mu_2 - 60 \eta^2 \Theta \mu_2 - 40 \eta^3 \Theta \mu_2 + 16 \mu_1 \mu_2 + 42 \eta \mu_1 \mu_2 + 24 \eta^2 \\
& \mu_1 \mu_2 - 18 \Theta \mu_1 \mu_2 - 112 \eta \Theta \mu_1 \mu_2 - 260 \eta^2 \Theta \mu_1 \mu_2 - 200 \\
& \eta^3 \Theta \mu_1 \mu_2 + 6 \mu_2^2 + 9 \eta \mu_2^2 - 8 \Theta \mu_2^2 - 28 \eta \Theta \mu_2^2 - 20 \eta^2 \Theta \\
& \mu_2^2 - 6 w^4 (-1 + \eta)^4 \mu_1 (3 \times (4 + 5 \eta) \mu_1 + \mu_2) - 3 \Theta \mu_1 - 6 \eta \\
& \Theta \mu_1 - 7 \Theta \mu_1 \mu_1 - 24 \eta \Theta \mu_1 \mu_1 - 30 \eta^2 \Theta \mu_1 \mu_1 - 20 \eta^3 \Theta \\
& \mu_1 \mu_1 - 4 \Theta \mu_1^2 \mu_1 - 14 \eta \Theta \mu_1^2 \mu_1 - 10 \eta^2 \Theta \mu_1^2 \mu_1 - 6 \Theta \\
& \mu_2 \mu_1 - 12 \eta \Theta \mu_2 \mu_1 - 8 \Theta \mu_1 \mu_2 \mu_1 - 28 \eta \Theta \mu_1 \mu_2 \mu_1 - 20 \\
& \eta^2 \Theta \mu_1 \mu_2 \mu_1 - 3 \Theta \mu_2^2 \mu_1 - 6 \eta \Theta \mu_2^2 \mu_1 - 3 \Theta \mu_2 - 6 \eta \\
& \Theta \mu_2 - 7 \Theta \mu_1 \mu_2 - 24 \eta \Theta \mu_1 \mu_2 - 30 \eta^2 \Theta \mu_1 \mu_2 - 20 \eta^3 \Theta \\
& \mu_1 \mu_2 - 4 \Theta \mu_1^2 \mu_2 - 14 \eta \Theta \mu_1^2 \mu_2 - 10 \eta^2 \Theta \mu_1^2 \mu_2 - 6 \Theta \\
& \mu_2 \mu_2 - 12 \eta \Theta \mu_2 \mu_2 - 8 \Theta \mu_1 \mu_2 \mu_2 - 28 \eta \Theta \mu_1 \mu_2 \mu_2 - 20 \\
& \eta^2 \Theta \mu_1 \mu_2 \mu_2 - 3 \Theta \mu_2^2 \mu_2 - 6 \eta \Theta \mu_2^2 \mu_2 - w^2 (-1 + \eta)^2 \\
& (82 \mu_1^2 + 100 \eta^3 \mu_1^2 - 18 (1 + \mu_2)^2 - 6 \mu_1 (8 + 9 \mu_2) + \Theta (24 + 9 \mu_1 + 9 \mu_2 + \\
& 27 \mu_1 (2 + \mu_1 + \mu_2) + 14 \mu_1^2 (2 + \mu_1 + \mu_2) + 18 \mu_2 (3 + \mu_1 + \mu_2) + \\
& \mu_2^2 (28 + 9 \mu_1 + 9 \mu_2) + 2 \mu_1 \mu_2 (53 + 14 \mu_1 + 14 \mu_2)) + \\
& 2 \eta^2 (12 \mu_1 (-3 + 20 \mu_1 - \mu_2) + 5 \Theta (2 \times (3 + 3 \mu_2 + \mu_2^2) + \\
& 3 \mu_1 (2 + \mu_1 + \mu_2) + \mu_1^2 (2 + \mu_1 + \mu_2) + 2 \mu_1 \mu_2 (13 + \mu_1 + \mu_2))) + \\
& \eta (441 \mu_1^2 - 27 (1 + \mu_2)^2 - 6 \mu_1 (21 + 13 \mu_2) + 2 \Theta (42 + 9 \mu_1 + 9 \mu_2 + \\
& 36 \mu_1 (2 + \mu_1 + \mu_2) + 17 \mu_1^2 (2 + \mu_1 + \mu_2) + 18 \mu_2 (4 + \mu_1 + \mu_2) + \\
& \mu_2^2 (34 + 9 \mu_1 + 9 \mu_2) + 2 \mu_1 \mu_2 (92 + 17 \mu_1 + 17 \mu_2))) + w \\
& (-1 + \eta) \times (6 \mu_1^2 - 18 (1 + \mu_2)^2 - 2 \mu_1 (20 + 27 \mu_2) + 20 \eta^3 \\
& (2 \mu_1 (-1 + 5 \mu_1) + 2 \Theta (3 + \mu_2) + \Theta \mu_1 (2 + 10 \mu_2 + \mu_1 + \mu_2)) + \\
& \Theta (9 \times (2 + \mu_1 + \mu_2) + 24 \mu_1 (2 + \mu_1 + \mu_2) + \\
& 13 \mu_1^2 (2 + \mu_1 + \mu_2) + 6 \mu_2 (8 + 3 \mu_1 + 3 \mu_2) + \\
& \mu_2^2 (26 + 9 \mu_1 + 9 \mu_2) + \mu_1 \mu_2 (80 + 26 \mu_1 + 26 \mu_2)) + \\
& 4 \eta^2 (3 \mu_1 (-10 + 35 \mu_1 - 4 \mu_2) + 5 \Theta (2 \times (3 + 3 \mu_2 + \mu_2^2) + \\
& 3 \mu_1 (2 + \mu_1 + \mu_2) + \mu_1^2 (2 + \mu_1 + \mu_2) + 2 \mu_1 \mu_2 (13 + \mu_1 + \mu_2))) + \\
& \eta (3 \times (69 \mu_1^2 - 9 (1 + \mu_2)^2 - 2 \mu_1 (19 + 17 \mu_2)) + 2 \Theta \\
& (30 + 9 \mu_1 + 9 \mu_2 + 38 \mu_1 (2 + \mu_1 + \mu_2) + 19 \mu_1^2 (2 + \mu_1 + \mu_2) + \\
& 2 \mu_2 (38 + 9 \mu_1 + 9 \mu_2) + \mu_2^2 (38 + 9 \mu_1 + 9 \mu_2) + \\
& 2 \mu_1 \mu_2 (98 + 19 \mu_1 + 19 \mu_2))) + w^3 \\
& (-1 + \eta)^3 (132 \mu_1^2 + 180 \eta^2 \mu_1^2 - 6 (1 + \mu_2)^2 - 10 \mu_1 (2 + \mu_2) + \\
& 5 \Theta \mu_1^2 (2 + \mu_1 + \mu_2) + \Theta (1 + \mu_2)^2 (10 + 3 \mu_1 + 3 \mu_2) + \\
& 2 \Theta \mu_1 (5 \times (2 + \mu_1 + \mu_2) + \mu_2 (22 + 5 \mu_1 + 5 \mu_2)) + \\
& \eta (345 \mu_1^2 - 9 (1 + \mu_2)^2 - 6 \mu_1 (7 + 3 \mu_2) + \\
& 2 \Theta (5 \mu_1^2 (2 + \mu_1 + \mu_2) + (1 + \mu_2)^2 (10 + 3 \mu_1 + 3 \mu_2) + \\
& 2 \mu_1 (5 \times (2 + \mu_1 + \mu_2) + \mu_2 (22 + 5 \mu_1 + 5 \mu_2)))) - \\
& \Theta (4 w^5 (-1 + \eta)^6 (-\eta \mu_1 + \eta \mu_2) (5 \eta^2 \mu_1 - \mu_2 + \eta (7 \mu_1 + \mu_2)) - \\
& 12 w^4 (-1 + \eta)^5 (1 + \eta) (-\eta \mu_1 + \eta \mu_2) \\
& (5 \eta^2 \mu_1 - \mu_2 + \eta (7 \mu_1 + \mu_2)) - \\
& \eta (1 + \eta)^2 (4 \eta^5 - 6 \eta \mu_1 (1 + \mu_1 + \mu_2)^2 + \eta^4 (-4 - 4 \times (-1 + \eta) \Theta \mu_1 + 40 \mu_1 \mu_2) + \\
& \eta (3 \Theta \mu_1 (1 + \mu_1 + \mu_2)^2 (2 + \mu_1 + \mu_2) + \eta \mu_1 (6 \mu_1^2 + 6 (1 + \mu_2)^2 +
\end{aligned}$$

$$\begin{aligned}
& 4 \mu_1 (3 + \mu_2) - 3 \theta_l (1 + \mu_1 + \mu_2)^2 (2 + \mathfrak{e}_1 + \mathfrak{e}_2) \Big) + 2 \\
& \eta^3 \Big( 2 \theta_l \mu_2 + 2 \mu_2 (2 - 8 \mu_1 + \mu_2) + \theta_l \mu_1 (2 + 10 \mu_2 + \mathfrak{e}_1 + \mathfrak{e}_2) - \\
& \eta t (10 \mu_1^2 + 2 \theta_l \mu_2 + \mu_1 (-4 + \theta_l (2 + 10 \mu_2 + \mathfrak{e}_1 + \mathfrak{e}_2))) \Big) - 2 \\
& \eta^2 \Big( 2 \mu_2 (2 + 2 \mu_1 + \mu_2) - \theta_l (2 \mu_2 (1 + \mu_2) + \mu_1^2 (2 + \mathfrak{e}_1 + \mathfrak{e}_2) + \\
& \mu_1 (2 + \mathfrak{e}_1 + \mathfrak{e}_2 + 2 \mu_2 (3 + \mathfrak{e}_1 + \mathfrak{e}_2))) \Big) + \\
& \eta t (2 \theta_l \mu_2 (1 + \mu_2) + \mu_1^2 (-10 + \theta_l (2 + \mathfrak{e}_1 + \mathfrak{e}_2)) + \\
& \mu_1 (4 - 4 \mu_2 + \theta_l (2 + \mathfrak{e}_1 + \mathfrak{e}_2 + 2 \mu_2 (3 + \mathfrak{e}_1 + \mathfrak{e}_2)))) \Big) + \\
& w^3 (-1 + \eta)^3 \Big( 60 \eta^6 \mu_1 \mu_2 - 12 \eta t \mu_1 \mu_2 + \eta^5 (4 - 60 \eta t \mu_1^2 + 204 \mu_1 \mu_2 + \\
& 12 \mu_2^2) + 6 \eta (2 \mu_2^2 + \eta t (13 \mu_1^2 - (1 + \mu_2)^2 - 2 \mu_1 (1 + 2 \mu_2))) \Big) - \eta^2 \\
& (4 + 16 \times (1 + 7 \mu_1) \mu_2 - \theta_l (5 \mu_1^2 (2 + \mathfrak{e}_1 + \mathfrak{e}_2) + (1 + \mu_2)^2 (10 + \\
& 3 \mathfrak{e}_1 + 3 \mathfrak{e}_2) + 2 \mu_1 (5 \times (2 + \mathfrak{e}_1 + \mathfrak{e}_2) + \mu_2 (22 + 5 \mathfrak{e}_1 + 5 \mathfrak{e}_2))) \Big) + \\
& \eta t (-186 \mu_1^2 + 6 (1 + \mu_2)^2 - 4 \mu_1 (-7 + 4 \mu_2) + 5 \theta_l \mu_1^2 \\
& (2 + \mathfrak{e}_1 + \mathfrak{e}_2) + \theta_l (1 + \mu_2)^2 (10 + 3 \mathfrak{e}_1 + 3 \mathfrak{e}_2) + \\
& 2 \theta_l \mu_1 (5 \times (2 + \mathfrak{e}_1 + \mathfrak{e}_2) + \mu_2 (22 + 5 \mathfrak{e}_1 + 5 \mathfrak{e}_2))) \Big) - 2 \eta^3 \\
& (2 + 110 \mu_1 \mu_2 + 20 \mu_2^2 - \theta_l (5 \mu_1^2 (2 + \mathfrak{e}_1 + \mathfrak{e}_2) + (1 + \mu_2)^2 (10 + \\
& 3 \mathfrak{e}_1 + 3 \mathfrak{e}_2) + 2 \mu_1 (5 \times (2 + \mathfrak{e}_1 + \mathfrak{e}_2) + \mu_2 (22 + 5 \mathfrak{e}_1 + 5 \mathfrak{e}_2))) \Big) + \\
& \eta t (17 \mu_1^2 - 3 (1 + \mu_2)^2 - 2 \mu_1 (3 + 2 \mu_2) + \theta_l (5 \mu_1^2 \\
& (2 + \mathfrak{e}_1 + \mathfrak{e}_2) + (1 + \mu_2)^2 (10 + 3 \mathfrak{e}_1 + 3 \mathfrak{e}_2) + \\
& 2 \mu_1 (5 \times (2 + \mathfrak{e}_1 + \mathfrak{e}_2) + \mu_2 (22 + 5 \mathfrak{e}_1 + 5 \mathfrak{e}_2)))) \Big) + \\
& \eta^4 (4 + 4 \times (4 + 17 \mu_1) \mu_2 + 16 \mu_2^2 + 5 \theta_l \mu_1^2 (2 + \mathfrak{e}_1 + \mathfrak{e}_2) + \\
& \theta_l (1 + \mu_2)^2 (10 + 3 \mathfrak{e}_1 + 3 \mathfrak{e}_2) + 2 \theta_l \mu_1 (5 \times (2 + \mathfrak{e}_1 + \mathfrak{e}_2) + \\
& \mu_2 (22 + 5 \mathfrak{e}_1 + 5 \mathfrak{e}_2)) - \eta t (170 \mu_1^2 - 6 (1 + \mu_2)^2 - 4 \mu_1 (7 + 3 \mu_2) + \\
& \theta_l (5 \mu_1^2 (2 + \mathfrak{e}_1 + \mathfrak{e}_2) + (1 + \mu_2)^2 (10 + 3 \mathfrak{e}_1 + 3 \mathfrak{e}_2) + \\
& 2 \mu_1 (5 \times (2 + \mathfrak{e}_1 + \mathfrak{e}_2) + \mu_2 (22 + 5 \mathfrak{e}_1 + 5 \mathfrak{e}_2)))) \Big) - \\
& w^2 (-1 + \eta)^2 (1 + \eta) \times (20 \eta^6 \mu_1 \mu_2 - 4 \eta t \mu_1 \mu_2 + 4 \eta^5 (3 - 5 \eta t \mu_1^2 + \\
& 42 \mu_1 \mu_2 + \mu_2^2) + 2 \eta (2 \mu_2^2 + \eta t (5 \mu_1^2 - 9 (1 + \mu_2)^2 - 6 \mu_1 (3 + 5 \mu_2))) \Big) - \\
& 2 \eta^4 (4 \eta t \mu_1 (-3 + 15 \mu_1 - \mu_2) - 2 \mu_2 (6 + 17 \mu_1 + 6 \mu_2) + \\
& (-1 + \eta t) \theta_l (2 \times (3 + 3 \mu_2 + \mu_2^2) + 3 \mu_1 (2 + \mathfrak{e}_1 + \mathfrak{e}_2) + \\
& \mu_1^2 (2 + \mathfrak{e}_1 + \mathfrak{e}_2) + 2 \mu_1 \mu_2 (13 + \mathfrak{e}_1 + \mathfrak{e}_2))) \Big) + \eta^2 \\
& (-8 \times (3 + 8 \mu_1) \mu_2 + 4 \eta t \mu_1 (-6 + 36 \mu_1 + 5 \mu_2) - (-1 + \eta t) \theta_l \\
& (9 \times (2 + \mathfrak{e}_1 + \mathfrak{e}_2) + 24 \mu_1 (2 + \mathfrak{e}_1 + \mathfrak{e}_2) + 13 \mu_1^2 (2 + \mathfrak{e}_1 + \mathfrak{e}_2) + \\
& 6 \mu_2 (8 + 3 \mathfrak{e}_1 + 3 \mathfrak{e}_2) + \mu_2^2 (26 + 9 \mathfrak{e}_1 + 9 \mathfrak{e}_2) + \\
& \mu_1 \mu_2 (80 + 26 \mathfrak{e}_1 + 26 \mathfrak{e}_2))) \Big) + \eta^3 (-4 \times (3 + 48 \mu_1 \mu_2 + 8 \mu_2^2) + \\
& 3 \theta_l (5 \mu_1^2 (2 + \mathfrak{e}_1 + \mathfrak{e}_2) + (1 + \mu_2)^2 (10 + 3 \mathfrak{e}_1 + 3 \mathfrak{e}_2) + \\
& 2 \mu_1 (5 \times (2 + \mathfrak{e}_1 + \mathfrak{e}_2) + \mu_2 (22 + 5 \mathfrak{e}_1 + 5 \mathfrak{e}_2))) \Big) - \\
& \eta t (2 \times (7 \mu_1^2 - 18 \mu_1 (1 + \mu_2) - 9 (1 + \mu_2)^2) + 3 \theta_l \\
& (5 \mu_1^2 (2 + \mathfrak{e}_1 + \mathfrak{e}_2) + (1 + \mu_2)^2 (10 + 3 \mathfrak{e}_1 + 3 \mathfrak{e}_2) + \\
& 2 \mu_1 (5 \times (2 + \mathfrak{e}_1 + \mathfrak{e}_2) + \mu_2 (22 + 5 \mathfrak{e}_1 + 5 \mathfrak{e}_2)))) \Big) + w (-1 + \eta) \\
& \eta (12 \eta^6 (1 + 5 \mu_1 \mu_2) - 6 \eta t (3 \mu_1^2 + 3 (1 + \mu_2)^2 + \mu_1 (6 + 8 \mu_2)) - \\
& 4 \eta^4 (3 - 8 \eta t \mu_1 + 25 \eta t \mu_1^2 - 8 \mu_2 - 15 \mu_1 \mu_2 - 4 \eta t \mu_1 \mu_2 - 5 \mu_2^2 + \\
& (-1 + \eta t) \theta_l (2 \times (3 + 3 \mu_2 + \mu_2^2) + 3 \mu_1 (2 + \mathfrak{e}_1 + \mathfrak{e}_2) + \\
& \mu_1^2 (2 + \mathfrak{e}_1 + \mathfrak{e}_2) + 2 \mu_1 \mu_2 (13 + \mathfrak{e}_1 + \mathfrak{e}_2))) \Big) - 2 \\
& \eta^5 (4 \eta t \mu_1 (-1 + 5 \mu_1) - 2 \times (3 + 2 \mu_2 + 44 \mu_1 \mu_2 + 2 \mu_2^2) +
\end{aligned}$$

$$\begin{aligned}
& (-1 + \eta t) \theta l (2 \times (3 + \mu_2) + \mu_1 (2 + 10 \mu_2 + \mathfrak{E}1 + \mathfrak{E}2)) + \eta^3 \\
& (-4 \times (3 + 44 \mu_1 \mu_2 + 4 \mu_2^2) + 2 \eta t (\mu_1^2 + 9 (1 + \mu_2)^2 + 2 \mu_1 (9 + 13 \mu_2)) + \\
& \theta l (30 + 9 \mathfrak{E}1 + 9 \mathfrak{E}2 + 38 \mu_1 (2 + \mathfrak{E}1 + \mathfrak{E}2) + 19 \mu_1^2 (2 + \mathfrak{E}1 + \mathfrak{E}2) + \\
& 2 \mu_2 (38 + 9 \mathfrak{E}1 + 9 \mathfrak{E}2) + \mu_2^2 (38 + 9 \mathfrak{E}1 + 9 \mathfrak{E}2) + \\
& 2 \mu_1 \mu_2 (98 + 19 \mathfrak{E}1 + 19 \mathfrak{E}2)) - \eta t \theta l (30 + 9 \mathfrak{E}1 + 9 \mathfrak{E}2 + \\
& 38 \mu_1 (2 + \mathfrak{E}1 + \mathfrak{E}2) + 19 \mu_1^2 (2 + \mathfrak{E}1 + \mathfrak{E}2) + 2 \mu_2 (38 + 9 \mathfrak{E}1 + 9 \mathfrak{E}2) + \\
& \mu_2^2 (38 + 9 \mathfrak{E}1 + 9 \mathfrak{E}2) + 2 \mu_1 \mu_2 (98 + 19 \mathfrak{E}1 + 19 \mathfrak{E}2)) - 2 \eta^2 \\
& (2 \mu_2 (8 + 28 \mu_1 + 3 \mu_2) - \theta l (9 \times (2 + \mathfrak{E}1 + \mathfrak{E}2) + 24 \mu_1 (2 + \mathfrak{E}1 + \mathfrak{E}2) + \\
& 13 \mu_1^2 (2 + \mathfrak{E}1 + \mathfrak{E}2) + 6 \mu_2 (8 + 3 \mathfrak{E}1 + 3 \mathfrak{E}2) + \mu_2^2 (26 + 9 \mathfrak{E}1 + 9 \mathfrak{E}2) + \\
& \mu_1 \mu_2 (80 + 26 \mathfrak{E}1 + 26 \mathfrak{E}2)) + \eta t (-9 - 2 \mu_1 - 63 \mu_1^2 - 18 \mu_2 - \\
& 20 \mu_1 \mu_2 - 9 \mu_2^2 + \theta l (9 \times (2 + \mathfrak{E}1 + \mathfrak{E}2) + 24 \mu_1 (2 + \mathfrak{E}1 + \mathfrak{E}2) + \\
& 13 \mu_1^2 (2 + \mathfrak{E}1 + \mathfrak{E}2) + 6 \mu_2 (8 + 3 \mathfrak{E}1 + 3 \mathfrak{E}2) + \\
& \mu_2^2 (26 + 9 \mathfrak{E}1 + 9 \mathfrak{E}2) + \mu_1 \mu_2 (80 + 26 \mathfrak{E}1 + 26 \mathfrak{E}2))) - \eta \\
& (8 \times (1 + \mu_1) \mu_2 - \theta l (11 \mu_1^2 (2 + \mathfrak{E}1 + \mathfrak{E}2) + (1 + \mu_2) \times \\
& (9 \times (2 + \mathfrak{E}1 + \mathfrak{E}2) + \mu_2 (22 + 9 \mathfrak{E}1 + 9 \mathfrak{E}2)) + \\
& \mu_1 (20 \times (2 + \mathfrak{E}1 + \mathfrak{E}2) + \mu_2 (48 + 22 \mathfrak{E}1 + 22 \mathfrak{E}2))) + \\
& \eta t (-30 \mu_1^2 + 18 (1 + \mu_2)^2 + \mu_1 (44 + 60 \mu_2) + \theta l (11 \mu_1^2 (2 + \mathfrak{E}1 + \mathfrak{E}2) + \\
& (1 + \mu_2) \times (9 \times (2 + \mathfrak{E}1 + \mathfrak{E}2) + \mu_2 (22 + 9 \mathfrak{E}1 + 9 \mathfrak{E}2)) + \\
& \mu_1 (20 \times (2 + \mathfrak{E}1 + \mathfrak{E}2) + \mu_2 (48 + 22 \mathfrak{E}1 + 22 \mathfrak{E}2)))) + \\
& 2 \times (-1 + \eta) \times (30 \times (-2 + w) (-1 + w)^2 w^2 \eta^8 \theta p \mu_1 \mu_2 - (1 + w)^3 \\
& (2 w^2 \eta t \theta l \mu_1 \mu_2 + 2 w^2 \mu_2 (-\theta l \mu_1 + \theta p \mu_2) + \eta t \theta p \\
& ((-3 + 14 w^2) \mu_1^2 - 3 (1 + \mu_2)^2 + 2 \mu_1 (-3 + (-3 - 3 w + w^2) \mu_2))) - \\
& 2 \times (-1 + w) \eta^7 (5 (-1 + w)^2 w^2 (-1 + \eta t) \theta l \mu_1^2 + \theta p \\
& (-7 + w (11 + 90 \mu_1 \mu_2) + w^2 (-4 + 25 \eta t \mu_1^2 - 80 \mu_1 \mu_2 - 5 \mu_2^2) + \\
& 2 w^4 (5 \eta t \mu_1^2 + 38 \mu_1 \mu_2 - \mu_2^2) + w^3 (-35 \eta t \mu_1^2 - 116 \mu_1 \mu_2 + 7 \mu_2^2))) - \\
& \eta^2 (\theta p (-6 \mu_2 (2 + 2 \mu_1 + \mu_2) + \eta t (33 \mu_1^2 + 3 (1 + \mu_2)^2 - 2 \mu_1 (3 + 5 \mu_2)) - \\
& 6 w^4 (5 \eta t \mu_1 (7 \mu_1 + 2 \mu_2) - \mu_2 (34 \mu_1 + 7 \mu_2)) + \\
& 6 w^5 (5 \eta t \mu_1 (3 \mu_1 + \mu_2) + \mu_2 (23 \mu_1 + 9 \mu_2)) + w^3 (4 + 40 \mu_2 - 50 \mu_1 \mu_2 - \\
& 54 \mu_2^2 + \eta t (-477 \mu_1^2 + \mu_1 (82 - 46 \mu_2) + 21 (1 + \mu_2)^2)) - \\
& 18 w^2 (1 + 16 \mu_1 \mu_2 + 3 \mu_2^2 + \eta t (2 \mu_1^2 - 3 (1 + \mu_2)^2 - 2 \mu_1 (3 + 4 \mu_2))) + \\
& 2 w (-\mu_2 (22 + 82 \mu_1 + 9 \mu_2) + \eta t (87 \mu_1^2 + 18 (1 + \mu_2)^2 + \\
& \mu_1 (14 + 45 \mu_2))) + (-1 + \eta t) \theta l (6 \mu_1^2 + 6 (1 + \mu_2)^2 + \\
& 30 w^5 \mu_1 (2 \mu_1 + \mu_2) + 4 \mu_1 (3 + 4 \mu_2) + 6 w^4 \mu_1 (16 \mu_1 + 5 \mu_2) - \\
& w^3 (15 \mu_1^2 + 3 (1 + \mu_2)^2 + \mu_1 (-2 + 26 \mu_2)) - 3 \theta p (4 \mu_1^2 (2 + \mathfrak{E}1 + \mathfrak{E}2) + \\
& (1 + \mu_2) \times (3 \times (2 + \mathfrak{E}1 + \mathfrak{E}2) + \mu_2 (8 + 3 \mathfrak{E}1 + 3 \mathfrak{E}2)) + \\
& \mu_1 (7 \times (2 + \mathfrak{E}1 + \mathfrak{E}2) + 2 \mu_2 (9 + 4 \mathfrak{E}1 + 4 \mathfrak{E}2))) - w (-9 - 22 \mu_1 + \\
& 15 \mu_1^2 - 18 \mu_2 - 30 \mu_1 \mu_2 - 9 \mu_2^2 + 2 \theta p (9 \times (2 + \mathfrak{E}1 + \mathfrak{E}2) + 26 \mu_1 \\
& (2 + \mathfrak{E}1 + \mathfrak{E}2) + 14 \mu_1^2 (2 + \mathfrak{E}1 + \mathfrak{E}2) + 4 \mu_1 \mu_2 (24 + 7 \mathfrak{E}1 + 7 \mathfrak{E}2) + \\
& 2 \mu_2 (26 + 9 \mathfrak{E}1 + 9 \mathfrak{E}2) + \mu_2^2 (28 + 9 \mathfrak{E}1 + 9 \mathfrak{E}2))) - \\
& w^2 (12 \mu_1 (-1 + 6 \mu_1 + \mu_2) + \theta p (33 \mu_1 (2 + \mathfrak{E}1 + \mathfrak{E}2) + 16 \mu_1^2 \\
& (2 + \mathfrak{E}1 + \mathfrak{E}2) + 9 \times (4 + \mathfrak{E}1 + \mathfrak{E}2) + 6 \mu_2 (11 + 3 \mathfrak{E}1 + 3 \mathfrak{E}2) + \\
& \mu_2^2 (32 + 9 \mathfrak{E}1 + 9 \mathfrak{E}2) + 2 \mu_1 \mu_2 (79 + 16 \mathfrak{E}1 + 16 \mathfrak{E}2)))) + \\
& \eta^6 (2 \theta p (-5 + 7 \times (-1 + \eta t) \theta l - 60 \mu_1 \mu_2) - 6 w^4 (\eta t \theta p \mu_1 (51 \mu_1 - 2 \mu_2) +
\end{aligned}$$



$$\begin{aligned}
& (-1 + \eta t) \theta l \mu_1 (8 \mu_1 - \mu_2) + \theta p (34 \mu_1 - 15 \mu_2) \mu_2 + 2 \\
& w^5 ((-1 + \eta t) \theta l \mu_1 (18 \mu_1 - \mu_2) + \eta t \theta p \mu_1 (53 \mu_1 - \mu_2) + \\
& \theta p (141 \mu_1 - 13 \mu_2) \mu_2) + w^2 (4 \times (-1 + \eta t) \theta l \mu_1 (-3 + 15 \mu_1 - \mu_2) + \\
& \theta p (42 - 48 \mu_2 + 492 \mu_1 \mu_2 - 34 \mu_2^2 + 2 \eta t \mu_1 (85 \mu_1 - 8 \times (3 + \mu_2))) + \\
& 5 \times (-1 + \eta t) \theta l (2 \times (3 + 3 \mu_2 + \mu_2^2) + 3 \mu_1 (2 + \mathfrak{E}1 + \mathfrak{E}2) + \\
& \mu_1^2 (2 + \mathfrak{E}1 + \mathfrak{E}2) + 2 \mu_1 \mu_2 (13 + \mathfrak{E}1 + \mathfrak{E}2))) - 2 w \\
& (2 \times (-1 + \eta t) \theta l \mu_1 (-1 + 5 \mu_1) + \theta p (6 + 10 \eta t \mu_1 (-1 + 5 \mu_1) - \\
& 10 \mu_2 - 115 \mu_1 \mu_2 - 10 \mu_2^2 + 3 \times (-1 + \eta t) \theta l (2 \times (3 + \mu_2) + \\
& \mu_1 (2 + 10 \mu_2 + \mathfrak{E}1 + \mathfrak{E}2)))) + w^3 (\theta p (-20 + (24 - 714 \mu_1) \mu_2 - \\
& 54 \mu_2^2 + 3 \eta t (45 \mu_1^2 + 3 (1 + \mu_2)^2 + 2 \mu_1 (7 + 3 \mu_2))) - \\
& (-1 + \eta t) \theta l (25 \mu_1^2 - 3 (1 + \mu_2)^2 - 2 \mu_1 (7 + 3 \mu_2) + \\
& 2 \theta p (5 \mu_1^2 (2 + \mathfrak{E}1 + \mathfrak{E}2) + (1 + \mu_2)^2 (10 + 3 \mathfrak{E}1 + 3 \mathfrak{E}2) + \\
& 2 \mu_1 (5 \times (2 + \mathfrak{E}1 + \mathfrak{E}2) + \mu_2 (22 + 5 \mathfrak{E}1 + 5 \mathfrak{E}2)))) + \\
& \eta^3 (-\theta p (-10 \mu_2 (2 + 10 \mu_1 + \mu_2) + 30 w^4 (\mu_2 (4 \mu_1 + \mu_2) + \eta t \mu_1 \\
& (19 \mu_1 + 4 \mu_2))) + 20 w^5 (\eta t \mu_1 (\mu_1 - 2 \mu_2) - \mu_2 (12 \mu_1 + 5 \mu_2)) + \\
& \eta t (59 \mu_1^2 + 9 (1 + \mu_2)^2 + \mu_1 (-2 + 26 \mu_2)) + 8 w^3 \\
& (2 + 99 \mu_1 \mu_2 + 24 \mu_2^2 + 3 \eta t (7 \mu_1^2 + \mu_1 (-2 + \mu_2) - (1 + \mu_2)^2)) - \\
& 6 w^2 (-1 - 4 \times (4 + 15 \mu_1) \mu_2 - 11 \mu_2^2 + \eta t (86 \mu_1^2 + 3 (1 + \mu_2)^2 + \\
& 2 \mu_1 (-5 + 6 \mu_2))) + w (-4 \times (6 + (-8 + 60 \mu_1) \mu_2 + 5 \mu_2^2) + \\
& 2 \eta t (-61 \mu_1^2 + 9 (1 + \mu_2)^2 + \mu_1 (34 + 32 \mu_2))) + \\
& (-1 + \eta t) \theta l (-3 - 10 \mu_1 + 7 \mu_1^2 - 6 w^4 \mu_1^2 - 6 \mu_2 - 14 \mu_1 \mu_2 - \\
& 3 \mu_2^2 + 10 w^5 \mu_1 (9 \mu_1 + 4 \mu_2) + 2 \theta p (3 \times (2 + \mathfrak{E}1 + \mathfrak{E}2) + \\
& 7 \mu_1^2 (2 + \mathfrak{E}1 + \mathfrak{E}2) + 6 \mu_2 (4 + \mathfrak{E}1 + \mathfrak{E}2) + \mu_2^2 (14 + 3 \mathfrak{E}1 + 3 \mathfrak{E}2) + \\
& 2 \mu_1 (6 \times (2 + \mathfrak{E}1 + \mathfrak{E}2) + 7 \mu_2 (4 + \mathfrak{E}1 + \mathfrak{E}2))) - \\
& w (-9 - 2 \mu_1 - 63 \mu_1^2 - 18 \mu_2 - 20 \mu_1 \mu_2 - 9 \mu_2^2 + \theta p \\
& (-6 + 9 \mathfrak{E}1 + 9 \mathfrak{E}2 + 2 \mu_1 \mu_2 (-76 + \mathfrak{E}1 + \mathfrak{E}2) - 4 \mu_1 (2 + \mathfrak{E}1 + \mathfrak{E}2) + \mu_1^2 \\
& (2 + \mathfrak{E}1 + \mathfrak{E}2) + 2 \mu_2 (-4 + 9 \mathfrak{E}1 + 9 \mathfrak{E}2) + \mu_2^2 (2 + 9 \mathfrak{E}1 + 9 \mathfrak{E}2))) - \\
& w^2 (6 \times (2 \mu_1^2 - 3 (1 + \mu_2)^2 - 2 \mu_1 (3 + 4 \mu_2)) + \theta p \\
& (66 \mu_1 (2 + \mathfrak{E}1 + \mathfrak{E}2) + 37 \mu_1^2 (2 + \mathfrak{E}1 + \mathfrak{E}2) + \\
& 3 \times (14 + 9 \mathfrak{E}1 + 9 \mathfrak{E}2) + 6 \mu_2 (22 + 9 \mathfrak{E}1 + 9 \mathfrak{E}2) + \\
& \mu_2^2 (74 + 27 \mathfrak{E}1 + 27 \mathfrak{E}2) + 2 \mu_1 \mu_2 (94 + 37 \mathfrak{E}1 + 37 \mathfrak{E}2))) - \\
& 2 w^3 (82 \mu_1^2 - 3 (1 + \mu_2)^2 + 2 \mu_1 (-7 + 6 \mu_2) + 2 \theta p \\
& (5 \mu_1^2 (2 + \mathfrak{E}1 + \mathfrak{E}2) + (1 + \mu_2)^2 (10 + 3 \mathfrak{E}1 + 3 \mathfrak{E}2) + \\
& 2 \mu_1 (5 \times (2 + \mathfrak{E}1 + \mathfrak{E}2) + \mu_2 (22 + 5 \mathfrak{E}1 + 5 \mathfrak{E}2)))) - \\
& \eta^5 (6 w^5 ((-1 + \eta t) \theta l \mu_1 (5 \mu_1 - 2 \mu_2) + 2 \eta t \theta p \mu_1 (18 \mu_1 - \mu_2) + \\
& 6 \theta p (5 \mu_1 - 2 \mu_2) \mu_2) + 6 w^4 \\
& ((-1 + \eta t) \theta l \mu_1 (11 \mu_1 + 4 \mu_2) + \eta t \theta p \mu_1 (-37 \mu_1 + 10 \mu_2) + \\
& \theta p \mu_2 (90 \mu_1 + 29 \mu_2)) - 2 ((-1 + \eta t) \theta l \mu_1 (-2 + 5 \mu_1) + \\
& \theta p (7 + 5 \eta t \mu_1 (-2 + 5 \mu_1) - 10 \mu_2 - 50 \mu_1 \mu_2 - 5 \mu_2^2 + \\
& 3 \times (-1 + \eta t) \theta l (2 \times (2 + \mu_2) + \mu_1 (2 + 10 \mu_2 + \mathfrak{E}1 + \mathfrak{E}2)))) - 3 \\
& w^2 (\theta p (6 \times (2 + (4 + 38 \mu_1) \mu_2 + 7 \mu_2^2) - \eta t (123 \mu_1^2 + \\
& 9 (1 + \mu_2)^2 + 2 \mu_1 (-3 + 5 \mu_2))) + (-1 + \eta t) \theta l \\
& (-\mu_1^2 - 6 \mu_1 (1 + \mu_2) - 3 (1 + \mu_2)^2 + 2 \theta p (4 + 3 \mathfrak{E}1 + 3 \mathfrak{E}2) +
\end{aligned}$$

$$\begin{aligned}
& 7 \mu_1 (2 + \mu_1 + \mu_2) + 4 \mu_1^2 (2 + \mu_1 + \mu_2) + 2 \mu_2 (7 + 3 \mu_1 + 3 \mu_2) + \\
& \mu_2^2 (8 + 3 \mu_1 + 3 \mu_2) + 2 \mu_1 \mu_2 (9 + 4 \mu_1 + 4 \mu_2) \Big) \Big) + 2 \\
& w \Big( (-1 + \eta t) \operatorname{el} \mu_1 (25 \mu_1 - 4 \times (2 + \mu_2)) + \operatorname{ep} (30 - 20 \eta t \mu_1 + \\
& 40 \eta t \mu_1^2 - 20 \mu_2 + 204 \mu_1 \mu_2 - 16 \eta t \mu_1 \mu_2 - 8 \mu_2^2 + \\
& (-1 + \eta t) \operatorname{el} (2 \times (6 + 12 \mu_2 + 5 \mu_2^2) + 5 \mu_1^2 (2 + \mu_1 + \mu_2) + \\
& 2 \mu_1 (6 \times (2 + \mu_1 + \mu_2) + 5 \mu_2 (10 + \mu_1 + \mu_2))) \Big) \Big) + \\
& w^3 (4 \operatorname{ep} (-1 - 4 \times (-5 + 43 \mu_1) \mu_2 + 9 \mu_2^2 + \eta t (-99 \mu_1^2 + \\
& 6 (1 + \mu_2)^2 + \mu_1 (32 + 13 \mu_2))) - \\
& (-1 + \eta t) \operatorname{el} (123 \mu_1^2 - 3 (1 + \mu_2)^2 - 2 \mu_1 (11 + 4 \mu_2) + \\
& 3 \operatorname{ep} (5 \mu_1^2 (2 + \mu_1 + \mu_2) + (1 + \mu_2)^2 (10 + 3 \mu_1 + 3 \mu_2) + \\
& 2 \mu_1 (5 \times (2 + \mu_1 + \mu_2) + \mu_2 (22 + 5 \mu_1 + 5 \mu_2))) \Big) \Big) + \\
& \eta (\operatorname{ep} (4 w^3 (1 + \eta t \mu_1 (4 - 27 \mu_1 - 13 \mu_2) + 4 \mu_2 + 28 \mu_1 \mu_2 + 3 \mu_2^2) + \\
& 4 w^5 (\eta t \mu_1 (16 \mu_1 + 3 \mu_2) + \mu_2 (7 \mu_1 + 4 \mu_2)) + \\
& 6 w^4 (\eta t \mu_1 (11 \mu_1 - 2 \mu_2) + \mu_2 (14 \mu_1 + 5 \mu_2)) + \\
& \eta t (9 \mu_1^2 + 9 (1 + \mu_2)^2 + 2 \mu_1 (9 + 13 \mu_2)) + w^2 (2 \times (12 + 32 \mu_1 - \mu_2) \mu_2 + \\
& \eta t (-149 \mu_1^2 + 9 (1 + \mu_2)^2 + 6 \mu_1 (7 + \mu_2))) + \\
& w (8 \times (1 + \mu_1) \mu_2 + \eta t (-30 \mu_1^2 + 18 (1 + \mu_2)^2 + \mu_1 (44 + 60 \mu_2))) \Big) \Big) + \\
& (-1 + \eta t) \operatorname{el} (6 w^4 \mu_1 (7 \mu_1 + 4 \mu_2) + 2 w^5 \mu_1 (7 \mu_1 + 6 \mu_2) + \\
& 3 (1 + \mu_1 + \mu_2)^2 (-1 + \operatorname{ep} (2 + \mu_1 + \mu_2)) + \\
& w^2 (-9 - 18 \mu_1 + 5 \mu_1^2 - 18 \mu_2 - 30 \mu_1 \mu_2 - 9 \mu_2^2 + \\
& \operatorname{ep} (9 \times (2 + \mu_1 + \mu_2) + 24 \mu_1 (2 + \mu_1 + \mu_2) + 13 \mu_1^2 (2 + \mu_1 + \mu_2) + \\
& 6 \mu_2 (8 + 3 \mu_1 + 3 \mu_2) + \mu_2^2 (26 + 9 \mu_1 + 9 \mu_2) + \mu_1 \mu_2 \\
& (80 + 26 \mu_1 + 26 \mu_2))) + w^3 (-6 \mu_1 + 39 \mu_1^2 - 3 (1 + \mu_2)^2 + \\
& \operatorname{ep} (5 \mu_1^2 (2 + \mu_1 + \mu_2) + (1 + \mu_2)^2 (10 + 3 \mu_1 + 3 \mu_2) + \\
& 2 \mu_1 (5 \times (2 + \mu_1 + \mu_2) + \mu_2 (22 + 5 \mu_1 + 5 \mu_2))) \Big) \Big) + \\
& w (-3 \times (3 \mu_1^2 + 3 (1 + \mu_2)^2 + \mu_1 (6 + 8 \mu_2)) + \operatorname{ep} (11 \mu_1^2 (2 + \mu_1 + \mu_2) + \\
& (1 + \mu_2) \times (9 \times (2 + \mu_1 + \mu_2) + \mu_2 (22 + 9 \mu_1 + 9 \mu_2)) + \\
& \mu_1 (20 \times (2 + \mu_1 + \mu_2) + \mu_2 (48 + 22 \mu_1 + 22 \mu_2))) \Big) \Big) + \\
& \eta^4 (10 \operatorname{ep} - 10 \operatorname{el} \operatorname{ep} + 10 \eta t \operatorname{el} \operatorname{ep} + 8 \operatorname{el} \mu_1 - 8 \eta t \operatorname{el} \mu_1 - 12 \eta t \operatorname{ep} \\
& \mu_1 - 30 \operatorname{el} \operatorname{ep} \mu_1 + 30 \eta t \operatorname{el} \operatorname{ep} \mu_1 - 20 \operatorname{el} \mu_1^2 + 20 \eta t \operatorname{el} \\
& \mu_1^2 + 30 \eta t \operatorname{ep} \mu_1^2 - 10 \operatorname{el} \operatorname{ep} \mu_1^2 + 10 \eta t \operatorname{el} \operatorname{ep} \mu_1^2 - 12 \operatorname{ep} \\
& \mu_2 - 30 \operatorname{el} \operatorname{ep} \mu_2 + 30 \eta t \operatorname{el} \operatorname{ep} \mu_2 + 4 \operatorname{el} \mu_1 \mu_2 - 4 \eta t \operatorname{el} \mu_1 \\
& \mu_2 + 108 \operatorname{ep} \mu_1 \mu_2 - 16 \eta t \operatorname{ep} \mu_1 \mu_2 - 130 \operatorname{el} \operatorname{ep} \mu_1 \mu_2 + 130 \\
& \eta t \operatorname{el} \operatorname{ep} \mu_1 \mu_2 - 6 \operatorname{ep} \mu_2^2 - 10 \operatorname{el} \operatorname{ep} \mu_2^2 + 10 \eta t \operatorname{el} \operatorname{ep} \\
& \mu_2^2 - 10 w^5 (11 \operatorname{ep} \mu_2 (\mu_1 + \mu_2) + \eta t \operatorname{ep} \mu_1 (-19 \mu_1 + 3 \mu_2) + \\
& (-1 + \eta t) \operatorname{el} \mu_1 (4 \mu_1 + 3 \mu_2)) + 6 w^4 ((-1 + \eta t) \operatorname{el} \mu_1 (24 \mu_1 + 5 \mu_2) + \\
& 5 \operatorname{ep} (\eta t \mu_1 (11 \mu_1 + 4 \mu_2) + \mu_2 (24 \mu_1 + 5 \mu_2))) - 15 \\
& \operatorname{el} \operatorname{ep} \mu_1 \mu_1 + 15 \eta t \operatorname{el} \operatorname{ep} \mu_1 \mu_1 - 5 \operatorname{el} \operatorname{ep} \mu_1^2 \mu_1 + 5 \eta t \operatorname{el} \\
& \operatorname{ep} \mu_1^2 \mu_1 - 10 \operatorname{el} \operatorname{ep} \mu_1 \mu_2 \mu_1 + 10 \eta t \operatorname{el} \operatorname{ep} \mu_1 \mu_2 \\
& \mu_1 - 15 \operatorname{el} \operatorname{ep} \mu_1 \mu_2 + 15 \eta t \operatorname{el} \operatorname{ep} \mu_1 \mu_2 - 5 \operatorname{el} \operatorname{ep} \mu_1^2 \\
& \mu_2 + 5 \eta t \operatorname{el} \operatorname{ep} \mu_1^2 \mu_2 - 10 \operatorname{el} \operatorname{ep} \mu_1 \mu_2 \mu_2 + 10 \eta t \operatorname{el} \\
& \operatorname{ep} \mu_1 \mu_2 \mu_2 + w^3 (\operatorname{ep} (24 + (80 + 578 \mu_1) \mu_2 + 198 \mu_2^2 + \\
& \eta t (-573 \mu_1^2 + 9 (1 + \mu_2)^2 + \mu_1 (98 + 46 \mu_2))) + \\
& 2 \times (-1 + \eta t) \operatorname{el} (21 \mu_1^2 + 3 \mu_1 (-2 + \mu_2) - 3 (1 + \mu_2)^2 +
\end{aligned}$$

$$\begin{aligned}
& 5 \operatorname{erf} \mu_1^2 (2 + \mathfrak{x}_1 + \mathfrak{x}_2) + \operatorname{erf} (1 + \mu_2)^2 (10 + 3 \mathfrak{x}_1 + 3 \mathfrak{x}_2) + \\
& 2 \operatorname{erf} \mu_1 (5 \times (2 + \mathfrak{x}_1 + \mathfrak{x}_2) + \mu_2 (22 + 5 \mathfrak{x}_1 + 5 \mathfrak{x}_2)) \Big) + w \\
& \Big( \operatorname{erf} (12 + 253 \eta t \mu_1^2 - 2 \times (40 + 207 \mu_1) \mu_2 - 74 \mu_2^2 + 27 \eta t (1 + \mu_2)^2 + \\
& \eta t \mu_1 (-26 + 38 \mu_2)) - (-1 + \eta t) \operatorname{erf} (-9 + 18 \operatorname{erf} (\mathfrak{x}_1 + \mathfrak{x}_2) + \\
& \mu_1^2 (-1 + 28 \operatorname{erf} (2 + \mathfrak{x}_1 + \mathfrak{x}_2)) + 2 \mu_2 (-9 + 2 \operatorname{erf} (23 + 9 \mathfrak{x}_1 + 9 \mathfrak{x}_2)) + \\
& \mu_2^2 (-9 + 2 \operatorname{erf} (28 + 9 \mathfrak{x}_1 + 9 \mathfrak{x}_2)) + 2 \mu_1 \\
& (-9 - 13 \mu_2 + 23 \operatorname{erf} (2 + \mathfrak{x}_1 + \mathfrak{x}_2) + \operatorname{erf} \mu_2 (66 + 28 \mathfrak{x}_1 + 28 \mathfrak{x}_2)) \Big) - \\
& 3 w^2 \Big( 2 \times (-1 + \eta t) \operatorname{erf} \mu_1 (-4 + 22 \mu_1 + \mu_2) + \operatorname{erf} (20 - 16 \mu_2 + \\
& 256 \mu_1 \mu_2 + 22 \mu_2^2 - \operatorname{erf} (22 + 3 \mathfrak{x}_1 + 3 \mathfrak{x}_2 + 7 \mu_1^2 (2 + \mathfrak{x}_1 + \mathfrak{x}_2) + \\
& \mu_2^2 (14 + 3 \mathfrak{x}_1 + 3 \mathfrak{x}_2) + \mu_2 (32 + 6 \mathfrak{x}_1 + 6 \mathfrak{x}_2) + \\
& 2 \mu_1 (8 \times (2 + \mathfrak{x}_1 + \mathfrak{x}_2) + \mu_2 (48 + 7 \mathfrak{x}_1 + 7 \mathfrak{x}_2)) \Big) + \eta t (83 \mu_1^2 - \\
& 15 (1 + \mu_2)^2 - 2 \mu_1 (23 + 13 \mu_2) + \operatorname{erf} (22 + 3 \mathfrak{x}_1 + 3 \mathfrak{x}_2 + 7 \mu_1^2 (2 + \\
& \mathfrak{x}_1 + \mathfrak{x}_2) + \mu_2^2 (14 + 3 \mathfrak{x}_1 + 3 \mathfrak{x}_2) + \mu_2 (32 + 6 \mathfrak{x}_1 + 6 \mathfrak{x}_2) + \\
& 2 \mu_1 (8 \times (2 + \mathfrak{x}_1 + \mathfrak{x}_2) + \mu_2 (48 + 7 \mathfrak{x}_1 + 7 \mathfrak{x}_2)) \Big) \Big) \Big) \Big) \Big) \Big) / \\
& (96 (-1 + w (-1 + \eta))^3 (x (-1 + \eta) - \eta)^3 (1 + x + \eta - x \eta)^2 \\
& (w + \\
& \quad x + \\
& \quad \eta - \\
& \quad w \eta - \\
& \quad x \eta)^3 (-1 + \eta t) \operatorname{erf} \Big)
\end{aligned}$$

$\beta_{ux} =$

$$\begin{aligned}
& - \Big( \Big( u x \Big( c v c \sigma (w (-1 + \eta) + x (-1 + \eta) - \eta) (-1 + \eta) (x^2 (-1 + \eta)^2 + \eta (1 + \eta) + x (1 + \eta - 2 \eta^2)) \Big)^2 \\
& \Big( (x + \eta - x \eta)^2 (-1 + \eta t) \operatorname{erf} \operatorname{erf} (1 + \mu_1) \times (14 x (-1 + \eta) - 14 \eta - 5 \times (2 + \mathfrak{x}_1 + \mathfrak{x}_2)) + \\
& w (-1 + \eta) \times (-4 x^3 (-1 + \eta)^3 \operatorname{erf} (1 - 8 \operatorname{erf} + 7 \mu_1 - 14 \operatorname{erf} \mu_1 + 3 \eta^2 (1 + \mu_1) - \\
& \eta \eta t (1 + 2 \operatorname{erf}) \times (1 + \mu_1) + 2 \eta (-2 + \operatorname{erf} - 5 \mu_1 + \operatorname{erf} \mu_1) + \\
& \eta t (1 + 8 \operatorname{erf} + \mu_1 + 14 \operatorname{erf} \mu_1) \Big) + x^2 (-1 + \eta)^2 \operatorname{erf} (36 \eta^3 (1 + \mu_1) - \\
& 12 \eta^2 (\eta t (1 + 2 \operatorname{erf}) \times (1 + \mu_1) - 2 \times (-2 + \operatorname{erf} - 5 \mu_1 + \operatorname{erf} \mu_1)) + \\
& 12 \eta (1 + 7 \mu_1 - 2 \operatorname{erf} (4 + 7 \mu_1) + \eta t (1 + \mu_1 + 2 \operatorname{erf} (4 + 7 \mu_1))) + \\
& (-1 + \eta t) \operatorname{erf} (1 + \mu_1) \times (58 + 15 \mathfrak{x}_1 + 15 \mathfrak{x}_2) \Big) - \\
& x (-1 + \eta) \times (12 \times (-1 + \eta) \eta^2 \operatorname{erf} (-1 - 7 \mu_1 + 3 \eta (1 + \mu_1) - \eta t (1 + \mu_1)) - \\
& (-1 + \eta t) \operatorname{erf} (20 \times (1 + \mu_1) + \operatorname{erf} (24 \eta^3 (1 + \mu_1) - 24 \eta^2 (4 + 7 \mu_1) + \\
& 5 \times (-6 - 3 \mathfrak{x}_1 + \mathfrak{x}_2) - 2 \eta (1 + \mu_1) \times (58 + 15 \mathfrak{x}_1 + 15 \mathfrak{x}_2) - \\
& \mu_1 (30 + 15 \mathfrak{x}_1 + 19 \mathfrak{x}_2)) \Big) + \operatorname{erf} (12 \eta^5 (1 + \mu_1) + 20 \eta t (1 + \mu_1) - \\
& 4 \eta^4 (\eta t (1 + 2 \operatorname{erf}) \times (1 + \mu_1) - 2 \times (-2 + \operatorname{erf} - 5 \mu_1 + \operatorname{erf} \mu_1)) + \\
& 4 \eta^3 (1 + 7 \mu_1 - 2 \operatorname{erf} (4 + 7 \mu_1) + \eta t (1 + \mu_1 + 2 \operatorname{erf} (4 + 7 \mu_1))) + \\
& \eta^2 (-1 + \eta t) \operatorname{erf} (1 + \mu_1) \times (58 + 15 \mathfrak{x}_1 + 15 \mathfrak{x}_2) + \\
& \eta (-20 \eta t (1 + \mu_1) - 5 \operatorname{erf} (6 + 3 \mathfrak{x}_1 - \mathfrak{x}_2) - \operatorname{erf} \mu_1 (30 + 15 \mathfrak{x}_1 + 19 \mathfrak{x}_2) + \\
& \eta t \operatorname{erf} (5 \times (6 + 3 \mathfrak{x}_1 - \mathfrak{x}_2) + \mu_1 (30 + 15 \mathfrak{x}_1 + 19 \mathfrak{x}_2))) \Big) + w^4 (-1 + \eta)^4 \\
& \Big( x (-1 + \eta) \times (4 \times (-1 + \eta) \operatorname{erf} (1 - 5 \mu_1 + \eta (1 + \mu_1) - \eta t (1 + \mu_1)) + (-1 + \eta t) \\
& \operatorname{erf} (-20 \times (1 + \mu_1) + 5 \operatorname{erf} (8 + 3 \mathfrak{x}_1 - \mathfrak{x}_2) + \operatorname{erf} \mu_1 (64 + 15 \mathfrak{x}_1 + 19 \mathfrak{x}_2))) + \\
& \operatorname{erf} (-4 \eta^3 (1 + \mu_1) - 20 \eta t (1 + \mu_1) + 4 \eta^2 (\eta t + 6 \mu_1 + \eta t \mu_1) + \eta (4 - 20 \mu_1 + \\
& 16 \eta t (1 + \mu_1) + \operatorname{erf} (40 + 64 \mu_1 + 15 \mathfrak{x}_1 + 15 \mu_1 \mathfrak{x}_1 - 5 \mathfrak{x}_2 + 19 \mu_1 \mathfrak{x}_2) - \\
& \eta t \operatorname{erf} (5 \times (8 + 3 \mathfrak{x}_1 - \mathfrak{x}_2) + \mu_1 (64 + 15 \mathfrak{x}_1 + 19 \mathfrak{x}_2))) \Big) + \\
& w^2 (-1 + \eta)^2 \Big( 2 x^3 (-1 + \eta)^3 \operatorname{erf} (-2 - 5 \operatorname{erf} + 10 \mu_1 - 17 \operatorname{erf} \mu_1 + 2 \eta^2
\end{aligned}$$

$$\begin{aligned}
& (1 + \mu_1) - 2 \eta (\eta t + 6 \mu_1 + \eta t \mu_1) + \eta t (2 + 5 \theta l + 2 \mu_1 + 17 \theta l \mu_1) \Big) - \\
& x^2 (-1 + \eta)^2 \theta p \Big( 8 - 94 \theta l + 56 \mu_1 - 142 \theta l \mu_1 + 12 \eta^3 (1 + \mu_1) + \\
& 8 \eta t (1 + \mu_1) - 12 \eta^2 (-2 + \eta t + 4 \mu_1 + \eta t \mu_1) + \\
& 2 \eta (-22 - 7 \theta l - 10 \mu_1 - 43 \theta l \mu_1 + \eta t (2 + 7 \theta l + 2 \mu_1 + 43 \theta l \mu_1)) - \\
& 15 \theta l \mathfrak{x}1 - 15 \theta l \mu_1 \mathfrak{x}1 - 15 \theta l \mathfrak{x}2 - 15 \theta l \mu_1 \mathfrak{x}2 + \\
& \eta t \theta l (94 + 15 \mathfrak{x}1 + 15 \mathfrak{x}2 + \mu_1 (142 + 15 \mathfrak{x}1 + 15 \mathfrak{x}2)) \Big) + \\
& \times (-1 + \eta) \times \Big( 4 \times (-1 + \eta) \eta \theta p \Big( 3 \eta^2 (1 + \mu_1) - 3 \eta (-5 + \eta t + \mu_1 + \eta t \mu_1) - \\
& 4 \times (1 + \eta t + 7 \mu_1 + \eta t \mu_1) \Big) + (-1 + \eta t) \theta l \Big( -60 \times (1 + \mu_1) + \\
& \theta p \Big( 104 + \eta^2 (-2 + 70 \mu_1) + 45 \mathfrak{x}1 - 15 \mathfrak{x}2 + \mu_1 (104 + 45 \mathfrak{x}1 + 57 \mathfrak{x}2) + \\
& 2 \eta (94 + 15 \mathfrak{x}1 + 15 \mathfrak{x}2 + \mu_1 (142 + 15 \mathfrak{x}1 + 15 \mathfrak{x}2)) \Big) \Big) \Big) + \\
& \theta p \Big( -4 \eta^5 (1 + \mu_1) - 60 \eta t (1 + \mu_1) + 4 \eta^4 (-6 + \eta t + \eta t \mu_1) + \\
& \eta^3 (36 + 60 \mu_1 + 6 \theta l (-1 + 3 \mu_1) + \eta t (4 + 6 \theta l + 4 \mu_1 - 18 \theta l \mu_1)) + \\
& \eta (60 \eta t (1 + \mu_1) + \theta l (104 + 45 \mathfrak{x}1 - 15 \mathfrak{x}2 + \mu_1 (104 + 45 \mathfrak{x}1 + 57 \mathfrak{x}2)) - \\
& \eta t \theta l (104 + 45 \mathfrak{x}1 - 15 \mathfrak{x}2 + \mu_1 (104 + 45 \mathfrak{x}1 + 57 \mathfrak{x}2))) - \eta^2 (8 + \\
& 56 \mu_1 - \theta l (94 + 15 \mathfrak{x}1 + 15 \mathfrak{x}2 + \mu_1 (142 + 15 \mathfrak{x}1 + 15 \mathfrak{x}2)) + \eta t (8 \times (1 + \\
& \mu_1) + \theta l (94 + 15 \mathfrak{x}1 + 15 \mathfrak{x}2 + \mu_1 (142 + 15 \mathfrak{x}1 + 15 \mathfrak{x}2)))) \Big) \Big) + \\
& w^3 (-1 + \eta)^3 \Big( x^2 (-1 + \eta)^2 \theta p \Big( -8 - 30 \theta l + 40 \mu_1 - 78 \theta l \mu_1 + 8 \eta^2 (1 + \mu_1) - \\
& 8 \eta (\eta t + 6 \mu_1 + \eta t \mu_1) - 5 \theta l \mathfrak{x}1 - 5 \theta l \mu_1 \mathfrak{x}1 - 5 \theta l \mathfrak{x}2 - 5 \theta l \mu_1 \mathfrak{x}2 + \\
& \eta t (8 \times (1 + \mu_1) + 5 \theta l (6 + \mathfrak{x}1 + \mathfrak{x}2) + \theta l \mu_1 (78 + 5 \mathfrak{x}1 + 5 \mathfrak{x}2)) \Big) - \\
& \times (-1 + \eta) \times \Big( 4 \times (-1 + \eta) \theta p \Big( -1 - 7 \mu_1 + 4 \eta^2 (1 + \mu_1) - \eta t (1 + \mu_1) - \\
& \eta (-7 + 17 \mu_1 + 4 \eta t (1 + \mu_1)) \Big) + (-1 + \eta t) \theta l \\
& \Big( -60 \times (1 + \mu_1) + \theta p (122 + 45 \mathfrak{x}1 - 15 \mathfrak{x}2 + \mu_1 (146 + 45 \mathfrak{x}1 + 57 \mathfrak{x}2) + \\
& 2 \eta (26 + 5 \mathfrak{x}1 + 5 \mathfrak{x}2 + \mu_1 (74 + 5 \mathfrak{x}1 + 5 \mathfrak{x}2))) \Big) \Big) + \\
& \theta p \Big( 8 \eta^4 (1 + \mu_1) + 60 \eta t (1 + \mu_1) - 4 \eta^3 (-3 + 9 \mu_1 + 2 \eta t (1 + \mu_1)) + \\
& \eta^2 (-24 - \theta l (22 + 5 \mathfrak{x}1 + 5 \mathfrak{x}2 + 5 \mu_1 (14 + \mathfrak{x}1 + \mathfrak{x}2)) + \\
& \eta t (4 \times (1 + \mu_1) + \theta l (22 + 5 \mathfrak{x}1 + 5 \mathfrak{x}2 + 5 \mu_1 (14 + \mathfrak{x}1 + \mathfrak{x}2))) \Big) + \\
& \eta (4 + 28 \mu_1 - \theta l (122 + 45 \mathfrak{x}1 - 15 \mathfrak{x}2 + \mu_1 (146 + 45 \mathfrak{x}1 + 57 \mathfrak{x}2)) + \\
& \eta t (-56 \times (1 + \mu_1) + \theta l (122 + 45 \mathfrak{x}1 - 15 \mathfrak{x}2 + \\
& \mu_1 (146 + 45 \mathfrak{x}1 + 57 \mathfrak{x}2)))) \Big) \Big) - \\
& (1 + x + \eta - x \eta)^2 \theta l \Big( 24 (c v^2 + 34 u - 4 \epsilon) (-1 + w (-1 + \eta))^3 (x + \eta - x \eta)^3 \\
& (w + x + \eta - w \eta - x \eta)^3 (-1 + \eta t) \theta p + \\
& f (-1 + \eta) \times \Big( 2 w^5 (-1 + \eta)^5 \Big( 2 x^3 (-1 + \eta)^3 \\
& \Big( (-1 + \eta) \theta p \Big( -118 + 10 \eta^2 + 5 \mathfrak{x}2 - \eta t (7 + \mathfrak{x}2) + \eta (7 - 10 \eta t + \mathfrak{x}2) \Big) + \\
& (-1 + \eta t) \theta l \Big( -5 \times (10 + \mathfrak{x}2) + 6 \theta p (28 + 5 \mathfrak{x}1 + 5 \mathfrak{x}2) \Big) \Big) - \\
& 2 \eta^2 \theta p \Big( 10 \eta^4 + 5 \eta t (10 + \mathfrak{x}2) + \eta^3 (-3 - 10 \eta t + \mathfrak{x}2) + \eta^2 (-125 - \\
& \eta t (-3 + \mathfrak{x}2) + 4 \mathfrak{x}2) + \eta (118 - 5 \mathfrak{x}2 - 6 \theta l (28 + 5 \mathfrak{x}1 + 5 \mathfrak{x}2) + \\
& \eta t (-43 - 4 \mathfrak{x}2 + 6 \theta l (28 + 5 \mathfrak{x}1 + 5 \mathfrak{x}2))) \Big) - x^2 (-1 + \eta)^2 \\
& \Big( 60 \eta^4 \theta p - 6 \eta^2 \theta p (125 + \eta t (-3 + \mathfrak{x}2) - 4 \mathfrak{x}2) - 6 \eta^3 \theta p (3 + 10 \eta t - \mathfrak{x}2) + \\
& \eta t \theta p (107 + 10 \mathfrak{x}2) + \eta (-\theta p (-708 + 30 \mathfrak{x}2 + \eta t (65 + 4 \mathfrak{x}2)) + \\
& (-1 + \eta t) \theta l (-193 - 20 \mathfrak{x}2 + 36 \theta p (28 + 5 \mathfrak{x}1 + 5 \mathfrak{x}2))) \Big) + \\
& \times (-1 + \eta) \eta \Big( 60 \eta^4 \theta p - 6 \eta^2 \theta p (125 + \eta t (-3 + \mathfrak{x}2) - 4 \mathfrak{x}2) - \\
& 6 \eta^3 \theta p (3 + 10 \eta t - \mathfrak{x}2) + \eta t \theta p (213 + 20 \mathfrak{x}2) + \\
& \eta ((-1 + \eta t) \theta l (-87 - 10 \mathfrak{x}2 + 36 \theta p (28 + 5 \mathfrak{x}1 + 5 \mathfrak{x}2)) - \\
& \theta p (-708 + 30 \mathfrak{x}2 + \eta t (171 + 14 \mathfrak{x}2))) \Big) \Big) +
\end{aligned}$$

$$\begin{aligned}
& w^3 (-1 + \eta)^3 (4 x^5 (-1 + \eta)^5 (3 \times (-1 + \eta) \operatorname{erf}(-118 + 10 \eta^2 + 5 \eta^2 - \\
& \quad \eta t (7 + \eta^2) + \eta (7 - 10 \eta t + \eta^2)) + (-1 + \eta t) \operatorname{erf} \\
& \quad (-5 \times (6 + \eta^2) + \operatorname{erf}(384 + 24 \eta^1 + 20 \eta^2 - 5 \eta^2))) + \\
& x^3 (-1 + \eta)^3 (4 \times (-1 + \eta) \operatorname{erf}(-78 + 300 \eta^4 - 266 \eta t + 3 \eta^2 - 31 \eta t \eta^2 + \\
& \quad 30 \eta^3 (19 - 10 \eta t + \eta^2) - 6 \eta^2 (543 - 31 \eta^2 + 5 \eta t (19 + \eta^2)) - \\
& \quad \eta (2858 - 98 \eta^2 + \eta t (69 + 44 \eta^2))) + (-1 + \eta t) \operatorname{erf} \\
& \quad (-60 \times (10 + \eta^2) + 4 \operatorname{erf}(228 + 90 \eta^1 + 96 \eta^2 + 5 \eta^2)) + \\
& \quad \eta (-18 \times (177 + 20 \eta^2) + \operatorname{erf}(15682 + 2799 \eta^1 + 2907 \eta^2)) + 2 \eta^2 \\
& \quad (-12 \times (31 + 5 \eta^2) + \operatorname{erf}(7026 + 471 \eta^1 + 335 \eta^2 - 100 \eta^2))) - \\
& x^4 (-1 + \eta)^4 (2 \times (-1 + \eta) \operatorname{erf}(-1416 + 300 \eta^3 - 19 \eta t + 48 \eta^2 - 22 \eta t \eta^2 + \\
& \quad 30 \eta^2 (13 - 10 \eta t + \eta^2) - 6 \eta (569 - 28 \eta^2 + 5 \eta t (13 + \eta^2))) + \\
& \quad (-1 + \eta t) \operatorname{erf}(24 \times (-46 - 5 \eta^2 + \operatorname{erf}(164 + 30 \eta^1 + 31 \eta^2)) + \\
& \quad \eta (-20 \times (25 + 4 \eta^2) + \operatorname{erf}(7366 + 477 \eta^1 + 369 \eta^2 - 100 \eta^2))) - \\
& \eta^2 \operatorname{erf}(120 \eta^6 + 60 \eta t (10 + \eta^2) + 12 \eta^5 (27 - 10 \eta t + \eta^2) - 12 \eta^4 \\
& \quad (124 - 7 \eta^2 + \eta t (27 + \eta^2)) + \eta^2 (2624 - 92 \eta^2 - \operatorname{erf}(3874 + 639 \eta^1 + \\
& \quad 675 \eta^2) + \eta t (-812 - 80 \eta^2 + \operatorname{erf}(3874 + 639 \eta^1 + 675 \eta^2))) + \\
& \eta^3 (-1892 + 8 \eta^2 - \operatorname{erf}(1170 + 87 \eta^1 + 43 \eta^2 - 20 \eta^2)) + \\
& \quad \eta t (318 - 32 \eta^2 + \operatorname{erf}(1170 + 87 \eta^1 + 43 \eta^2 - 20 \eta^2))) + \\
& 2 \eta (-2 \times (3 \times (-26 + \eta^2) + \operatorname{erf}(228 + 90 \eta^1 + 96 \eta^2 + 5 \eta^2))) + \\
& \quad \eta t (169 + 32 \eta^2 + 2 \operatorname{erf}(228 + 90 \eta^1 + 96 \eta^2 + 5 \eta^2))) - \\
& x^2 (-1 + \eta)^2 (1200 \eta^6 \operatorname{erf} - 120 \eta^5 \operatorname{erf}(-15 + 10 \eta t - \eta^2) + \\
& 6 \eta t \operatorname{erf}(107 + 10 \eta^2) - 24 \eta^4 \operatorname{erf}(637 - 29 \eta^2 + 5 \eta t (15 + \eta^2)) + \\
& 3 \eta^2 (-2 \operatorname{erf}(-2728 + 94 \eta^2 + 3 \eta t (145 + 6 \eta^2)) + (-1 + \eta t) \operatorname{erf} \\
& \quad (-24 \times (41 + 5 \eta^2) + \operatorname{erf}(7810 + 1359 \eta^1 + 1419 \eta^2))) + \\
& 4 \eta^3 (-3 \operatorname{erf}(418 + 18 \eta^2 + \eta t (-203 + 12 \eta^2)) + (-1 + \eta t) \\
& \quad \operatorname{erf}(-117 - 20 \eta^2 + \operatorname{erf}(3330 + 231 \eta^1 + 149 \eta^2 - 50 \eta^2))) + \\
& 6 \eta (2 \operatorname{erf}(78 - 3 \eta^2 + \eta t (211 + 26 \eta^2)) + (-1 + \eta t) \operatorname{erf} \\
& \quad (-193 - 20 \eta^2 + 2 \operatorname{erf}(228 + 90 \eta^1 + 96 \eta^2 + 5 \eta^2))) + \\
& x (-1 + \eta) \eta (600 \eta^6 \operatorname{erf} - 60 \eta^5 \operatorname{erf}(-21 + 10 \eta t - \eta^2) + 6 \eta t \\
& \quad \operatorname{erf}(213 + 20 \eta^2) - 12 \eta^4 \operatorname{erf}(631 - 32 \eta^2 + 5 \eta t (21 + \eta^2)) + \\
& \eta^2 (-4 \operatorname{erf}(-2676 + 93 \eta^2 + \eta t (649 + 49 \eta^2)) + 3 \times (-1 + \eta t) \\
& \quad \operatorname{erf}(-10 \times (29 + 4 \eta^2) + \operatorname{erf}(5186 + 879 \eta^1 + 923 \eta^2))) + \\
& 2 \eta^3 (-2 \operatorname{erf}(1482 + 9 \eta^2 + \eta t (-352 + 29 \eta^2)) + (-1 + \eta t) \\
& \quad \operatorname{erf}(-2 \times (26 + 5 \eta^2) + \operatorname{erf}(3134 + 225 \eta^1 + 129 \eta^2 - 50 \eta^2))) + \\
& 6 \eta (\operatorname{erf}(156 + 295 \eta t - 6 \eta^2 + 42 \eta t \eta^2) + (-1 + \eta t) \operatorname{erf} \\
& \quad (-87 - 10 \eta^2 + 2 \operatorname{erf}(228 + 90 \eta^1 + 96 \eta^2 + 5 \eta^2))) + \\
& w^4 (-1 + \eta)^4 (2 x^4 (-1 + \eta)^4 (6 \times (-1 + \eta) \operatorname{erf}(-118 + 10 \eta^2 + 5 \eta^2 - \\
& \quad \eta t (7 + \eta^2) + \eta (7 - 10 \eta t + \eta^2)) + (-1 + \eta t) \operatorname{erf} \\
& \quad (-4 \times (46 + 5 \eta^2) + \operatorname{erf}(892 + 120 \eta^1 + 112 \eta^2 - 5 \eta^2))) + \\
& \eta^2 \operatorname{erf}(120 \eta^5 + 60 \eta t (10 + \eta^2) + 12 \eta^4 (7 - 10 \eta t + \eta^2) - \\
& 12 \eta^3 (128 - 5 \eta^2 + \eta t (7 + \eta^2)) + \eta^2 (388 - 40 \eta^2 - \\
& 6 \eta t (17 + 6 \eta^2) - \operatorname{erf}(1638 + 213 \eta^1 + 193 \eta^2 - 10 \eta^2)) + \\
& \eta t \operatorname{erf}(1638 + 213 \eta^1 + 193 \eta^2 - 10 \eta^2)) + 2 \eta
\end{aligned}$$

$$\begin{aligned}
& (472 - 16 \, \mathfrak{z}2 - 3 \, \eta \mathfrak{t} (49 + 2 \, \mathfrak{z}2) - \mathfrak{el} (772 + 180 \, \mathfrak{z}1 + 192 \, \mathfrak{z}2 + 5 \, \mathfrak{z}2^2) + \\
& \quad \eta \mathfrak{t} \mathfrak{el} (772 + 180 \, \mathfrak{z}1 + 192 \, \mathfrak{z}2 + 5 \, \mathfrak{z}2^2)) - x^3 (-1 + \eta)^3 ((-1 + \eta \mathfrak{t}) \\
& \quad \mathfrak{el} (-60 \times (10 + \mathfrak{z}2) - 6 \, \eta (177 + 20 \, \mathfrak{z}2) + \eta \mathfrak{op} (6990 + 933 \, \mathfrak{z}1 + \\
& \quad \quad 865 \, \mathfrak{z}2 - 40 \, \mathfrak{z}2^2) + 2 \mathfrak{op} (772 + 180 \, \mathfrak{z}1 + 192 \, \mathfrak{z}2 + 5 \, \mathfrak{z}2^2)) + \\
& \quad 4 \times (-1 + \eta) \mathfrak{op} (-236 + 120 \, \eta^3 - 6 \, \eta^2 (-19 + 20 \, \eta \mathfrak{t} - 2 \, \mathfrak{z}2) + \\
& \quad \quad 8 \, \mathfrak{z}2 - 3 \, \eta \mathfrak{t} (29 + 4 \, \mathfrak{z}2) - 3 \, \eta (465 - 21 \, \mathfrak{z}2 + \eta \mathfrak{t} (38 + 4 \, \mathfrak{z}2))) + \\
& \quad 3 x^2 (-1 + \eta)^2 (240 \, \eta^5 \mathfrak{op} + 24 \, \eta^4 \mathfrak{op} (2 - 10 \, \eta \mathfrak{t} + \mathfrak{z}2) + 2 \, \eta \mathfrak{t} \mathfrak{op} \\
& \quad \quad (107 + 10 \, \mathfrak{z}2) - 12 \, \eta^3 \mathfrak{op} (253 - 9 \, \mathfrak{z}2 + 2 \, \eta \mathfrak{t} (2 + \mathfrak{z}2)) + \\
& \quad \quad \eta^2 (-2 \mathfrak{op} (-902 + 50 \, \mathfrak{z}2 + \eta \mathfrak{t} (29 + 12 \, \mathfrak{z}2)) + (-1 + \eta \mathfrak{t}) \mathfrak{el} \\
& \quad \quad \quad (-8 \times (41 + 5 \, \mathfrak{z}2) + \mathfrak{op} (3422 + 453 \, \mathfrak{z}1 + 417 \, \mathfrak{z}2 - 20 \, \mathfrak{z}2^2))) + \\
& \quad \quad 2 \, \eta (2 \mathfrak{op} (236 - 8 \, \mathfrak{z}2 + \eta \mathfrak{t} (33 + 7 \, \mathfrak{z}2)) + (-1 + \eta \mathfrak{t}) \mathfrak{el} \\
& \quad \quad \quad (-193 - 20 \, \mathfrak{z}2 + \mathfrak{op} (772 + 180 \, \mathfrak{z}1 + 192 \, \mathfrak{z}2 + 5 \, \mathfrak{z}2^2))) - \\
& \quad x (-1 + \eta) \, \eta (480 \, \eta^5 \mathfrak{op} - 24 \, \eta^4 \mathfrak{op} (-9 + 20 \, \eta \mathfrak{t} - 2 \, \mathfrak{z}2) + \\
& \quad \quad 6 \, \eta \mathfrak{t} \mathfrak{op} (213 + 20 \, \mathfrak{z}2) - 12 \, \eta^3 \mathfrak{op} (509 - 19 \, \mathfrak{z}2 + 2 \, \eta \mathfrak{t} (9 + 2 \, \mathfrak{z}2)) + \\
& \quad \quad \eta^2 (-12 \mathfrak{op} (-215 + 25 \, \eta \mathfrak{t} + 15 \, \mathfrak{z}2 + 8 \, \eta \mathfrak{t} \mathfrak{z}2) + (-1 + \eta \mathfrak{t}) \mathfrak{el} \\
& \quad \quad \quad (-10 \times (29 + 4 \, \mathfrak{z}2) + \mathfrak{op} (6698 + 879 \, \mathfrak{z}1 + 803 \, \mathfrak{z}2 - 40 \, \mathfrak{z}2^2))) + \\
& \quad \quad 6 \, \eta (\mathfrak{op} (472 - 16 \, \mathfrak{z}2 + \eta \mathfrak{t} (-47 + 4 \, \mathfrak{z}2)) + (-1 + \eta \mathfrak{t}) \mathfrak{el} \\
& \quad \quad \quad (-87 - 10 \, \mathfrak{z}2 + \mathfrak{op} (772 + 180 \, \mathfrak{z}1 + 192 \, \mathfrak{z}2 + 5 \, \mathfrak{z}2^2)))) + \\
& \quad (x + \eta - x \, \eta)^2 (2 x^4 (-1 + \eta)^4 \mathfrak{op} (156 + 60 \, \eta^3 - 156 \mathfrak{el} - 4 \, \eta^2 \\
& \quad \quad (28 - 5 \mathfrak{el} + 5 \, \eta \mathfrak{t} (2 + \mathfrak{el}) - \mathfrak{z}2) - 6 \, \mathfrak{z}2 - 12 \mathfrak{el} \mathfrak{z}2 + \\
& \quad \quad 5 \mathfrak{el} \mathfrak{z}2^2 + \eta \mathfrak{t} (-26 + 156 \mathfrak{el} + 2 \, \mathfrak{z}2 + 12 \mathfrak{el} \mathfrak{z}2 - 5 \mathfrak{el} \mathfrak{z}2^2) - \\
& \quad \quad 2 \, \eta (52 + 13 \mathfrak{el} - \mathfrak{z}2 - 3 \mathfrak{el} \mathfrak{z}2 + \eta \mathfrak{t} (-33 - 13 \mathfrak{el} + \mathfrak{z}2 + 3 \mathfrak{el} \mathfrak{z}2))) + \\
& \quad 2 x^3 (-1 + \eta)^3 (-8 \times (-1 + \eta) \, \eta \mathfrak{op} (-78 + 30 \, \eta^2 + 13 \, \eta \mathfrak{t} + 3 \, \mathfrak{z}2 - \\
& \quad \quad \eta \mathfrak{t} \mathfrak{z}2 + \eta (-26 - 20 \, \eta \mathfrak{t} + 2 \, \mathfrak{z}2)) + (-1 + \eta \mathfrak{t}) \mathfrak{el} \\
& \quad \quad (10 \times (6 + \mathfrak{z}2) + \mathfrak{op} (80 \, \eta^3 - 48 \, \mathfrak{z}1 + 8 \, \eta^2 (-13 + 3 \, \mathfrak{z}2) - \\
& \quad \quad \quad 5 \times (12 + 8 \, \mathfrak{z}2 + \mathfrak{z}2^2) + 4 \, \eta (-156 - 12 \, \mathfrak{z}2 + 5 \, \mathfrak{z}2^2)))) + \eta^2 \mathfrak{op} \\
& \quad (120 \, \eta^5 - 8 \, \eta^4 (28 - 5 \mathfrak{el} + 5 \, \eta \mathfrak{t} (2 + \mathfrak{el}) - \mathfrak{z}2) + 2 \, \eta \mathfrak{t} (59 + 10 \, \mathfrak{z}2) + \\
& \quad \quad \eta (-2 \, \eta \mathfrak{t} (59 + 10 \, \mathfrak{z}2) - \mathfrak{el} (118 + 87 \, \mathfrak{z}1 + 79 \, \mathfrak{z}2 + 10 \, \mathfrak{z}2^2) + \\
& \quad \quad \quad \eta \mathfrak{t} \mathfrak{el} (118 + 87 \, \mathfrak{z}1 + 79 \, \mathfrak{z}2 + 10 \, \mathfrak{z}2^2)) - 4 \, \eta^3 \\
& \quad \quad (52 + \mathfrak{el} (13 - 3 \, \mathfrak{z}2) - \mathfrak{z}2 + \eta \mathfrak{t} (-33 + \mathfrak{z}2 + \mathfrak{el} (-13 + 3 \, \mathfrak{z}2))) - \\
& \quad \quad 2 \, \eta^2 (6 \times (-26 + \mathfrak{z}2) + \mathfrak{el} (156 + 12 \, \mathfrak{z}2 - 5 \, \mathfrak{z}2^2) + \eta \mathfrak{t} (26 - 2 \, \mathfrak{z}2 + \\
& \quad \quad \quad \mathfrak{el} (-156 - 12 \, \mathfrak{z}2 + 5 \, \mathfrak{z}2^2)))) + x^2 (-1 + \eta)^2 (720 \, \eta^5 \mathfrak{op} - \\
& \quad \quad 48 \, \eta^4 \mathfrak{op} (28 - 5 \mathfrak{el} + 5 \, \eta \mathfrak{t} (2 + \mathfrak{el}) - \mathfrak{z}2) + 10 \, \eta \mathfrak{t} \mathfrak{op} (11 + 2 \, \mathfrak{z}2) - \\
& \quad \quad 24 \, \eta^3 \mathfrak{op} (52 + \mathfrak{el} (13 - 3 \, \mathfrak{z}2) - \mathfrak{z}2 + \eta \mathfrak{t} (-33 + \mathfrak{z}2 + \mathfrak{el} (-13 + 3 \, \mathfrak{z}2))) - \\
& \quad \quad 12 \, \eta^2 \mathfrak{op} (6 \times (-26 + \mathfrak{z}2) + \mathfrak{el} (156 + 12 \, \mathfrak{z}2 - 5 \, \mathfrak{z}2^2) + \\
& \quad \quad \quad \eta \mathfrak{t} (26 - 2 \, \mathfrak{z}2 + \mathfrak{el} (-156 - 12 \, \mathfrak{z}2 + 5 \, \mathfrak{z}2^2)))) + \\
& \quad 5 \, \eta (-2 \, \eta \mathfrak{t} \mathfrak{op} (11 + 2 \, \mathfrak{z}2) + (-1 + \eta \mathfrak{t}) \mathfrak{el} (-52 - 8 \, \mathfrak{z}2 + \\
& \quad \quad \quad \mathfrak{op} (74 + 57 \, \mathfrak{z}1 + 49 \, \mathfrak{z}2 + 6 \, \mathfrak{z}2^2))) - 2 x (-1 + \eta) \, \eta (240 \, \eta^5 \mathfrak{op} - \\
& \quad \quad 16 \, \eta^4 \mathfrak{op} (28 - 5 \mathfrak{el} + 5 \, \eta \mathfrak{t} (2 + \mathfrak{el}) - \mathfrak{z}2) + 4 \, \eta \mathfrak{t} \mathfrak{op} (33 + 5 \, \mathfrak{z}2) - \\
& \quad \quad 8 \, \eta^3 \mathfrak{op} (52 + \mathfrak{el} (13 - 3 \, \mathfrak{z}2) - \mathfrak{z}2 + \eta \mathfrak{t} (-33 + \mathfrak{z}2 + \mathfrak{el} (-13 + 3 \, \mathfrak{z}2))) - \\
& \quad \quad 4 \, \eta^2 \mathfrak{op} (6 \times (-26 + \mathfrak{z}2) + \mathfrak{el} (156 + 12 \, \mathfrak{z}2 - 5 \, \mathfrak{z}2^2) + \\
& \quad \quad \quad \eta \mathfrak{t} (26 - 2 \, \mathfrak{z}2 + \mathfrak{el} (-156 - 12 \, \mathfrak{z}2 + 5 \, \mathfrak{z}2^2)))) + \\
& \quad \eta (-4 \, \eta \mathfrak{t} \mathfrak{op} (33 + 5 \, \mathfrak{z}2) + (-1 + \eta \mathfrak{t}) \mathfrak{el} (-2 \times (26 + 5 \, \mathfrak{z}2) +
\end{aligned}$$



$$\begin{aligned}
& x^3 (-1 + \eta)^3 \left( -4 \times (-1 + \eta) \operatorname{ep} \left( 200 \eta^5 - 20 \eta^4 (-52 + 10 \eta t - \mathfrak{z}2) - \right. \right. \\
& \quad 3 \eta t (93 + 10 \mathfrak{z}2) - 9 \eta (104 + 23 \eta t - 4 \mathfrak{z}2 + 8 \eta t \mathfrak{z}2) - \\
& \quad 12 \eta^2 (-22 \times (-28 + \mathfrak{z}2) + 5 \eta t (1 + \mathfrak{z}2)) - 10 \eta^3 \\
& \quad \left. (137 - 19 \mathfrak{z}2 + 2 \eta t (52 + \mathfrak{z}2)) \right) + (-1 + \eta t) \operatorname{el} \left( 20 \times (10 + \mathfrak{z}2) - \right. \\
& \quad 10 \operatorname{ep} \left( 20 + 12 \mathfrak{z}1 + 12 \mathfrak{z}2 + \mathfrak{z}2^2 \right) + 40 \eta^3 \operatorname{ep} \left( -143 + 9 \mathfrak{z}2 + 5 \mathfrak{z}2^2 \right) + \\
& \quad 6 \eta^2 \left( 372 + 60 \mathfrak{z}2 - \operatorname{ep} \left( 5438 + 471 \mathfrak{z}1 + 503 \mathfrak{z}2 - 50 \mathfrak{z}2^2 \right) \right) - 3 \eta \\
& \quad \left. \left( -6 \times (177 + 20 \mathfrak{z}2) + \operatorname{ep} \left( 2682 + 933 \mathfrak{z}1 + 973 \mathfrak{z}2 + 40 \mathfrak{z}2^2 \right) \right) \right) + \\
& w \left( x (-1 + \eta) - \eta \right) (-1 + \eta) \times \left( -4 x^5 (-1 + \eta)^5 \operatorname{ep} \left( 236 + 30 \eta^3 - \right. \right. \\
& \quad 236 \operatorname{el} - 8 \mathfrak{z}2 - 6 \operatorname{el} \mathfrak{z}2 + 5 \operatorname{el} \mathfrak{z}2^2 + \eta^2 (-9 - 30 \eta t + 3 \mathfrak{z}2) + \\
& \quad \eta (-257 - 2 \eta t (-18 + \mathfrak{z}2) + 5 \mathfrak{z}2 + 3 \operatorname{el} (9 + \mathfrak{z}2) - 3 \eta t \operatorname{el} (9 + \mathfrak{z}2)) + \\
& \quad \eta t \left( 2 \times (-3 + \mathfrak{z}2) + \operatorname{el} \left( 236 + 6 \mathfrak{z}2 - 5 \mathfrak{z}2^2 \right) \right) - x^3 (-1 + \eta)^3 \\
& \quad \left. \left( -((-1 + \eta t) \operatorname{el} \left( 120 \eta^3 \operatorname{ep} (13 + \mathfrak{z}2) + 60 \eta (19 + 3 \mathfrak{z}2) + \right. \right. \right. \\
& \quad \quad 8 \times (46 + 5 \mathfrak{z}2) - 3 \eta \operatorname{ep} (1738 + 381 \mathfrak{z}1 + 421 \mathfrak{z}2) - 4 \operatorname{ep} (92 + 60 \\
& \quad \quad \mathfrak{z}1 + 56 \mathfrak{z}2 + 5 \mathfrak{z}2^2) + 8 \eta^2 \operatorname{ep} (-1258 - 12 \mathfrak{z}2 + 25 \mathfrak{z}2^2) \left. \right) \right) + \\
& \quad 2 \times (-1 + \eta) \operatorname{ep} \left( 600 \eta^4 - 24 \eta (78 + \eta t (-13 + \mathfrak{z}2) - 3 \mathfrak{z}2) - \right. \\
& \quad 60 \eta^3 (-19 + 10 \eta t - \mathfrak{z}2) - 15 \eta t (11 + 2 \mathfrak{z}2) - \\
& \quad \left. 8 \eta^2 (668 - 26 \mathfrak{z}2 + 5 \eta t (9 + \mathfrak{z}2)) \right) + \\
& \eta^2 \operatorname{ep} \left( 120 \eta^6 + 12 \eta^5 (27 - 10 \eta t + \mathfrak{z}2) + 10 \eta t (33 + 4 \mathfrak{z}2) - 4 \eta^4 \right. \\
& \quad (425 - 11 \mathfrak{z}2 + 2 \eta t (12 + \mathfrak{z}2) - 3 \operatorname{el} (19 + \mathfrak{z}2) + 3 \eta t \operatorname{el} (19 + \mathfrak{z}2)) + \\
& \quad 3 \eta^2 (-12 \times (-26 + \mathfrak{z}2) - 2 \eta t (85 + 8 \mathfrak{z}2) - \\
& \quad \operatorname{el} (430 + 87 \mathfrak{z}1 + 103 \mathfrak{z}2) + \eta t \operatorname{el} (430 + 87 \mathfrak{z}1 + 103 \mathfrak{z}2)) + \\
& \quad \eta (-213 \operatorname{el} \mathfrak{z}1 + 4 \eta t (6 + 5 \mathfrak{z}2) - 5 \operatorname{el} (66 + 41 \mathfrak{z}2 + 4 \mathfrak{z}2^2) + \\
& \quad \left. \eta t \operatorname{el} (213 \mathfrak{z}1 + 5 \times (66 + 41 \mathfrak{z}2 + 4 \mathfrak{z}2^2)) \right) - \\
& \quad 4 \eta^3 \left( 5 \times (-16 + \mathfrak{z}2) + \operatorname{el} (275 - 3 \mathfrak{z}2 - 5 \mathfrak{z}2^2) + \right. \\
& \quad \left. \eta t (-93 + \mathfrak{z}2 + \operatorname{el} (-275 + 3 \mathfrak{z}2 + 5 \mathfrak{z}2^2)) \right) + 4 x^4 (-1 + \eta)^4 \\
& \quad \left( (-1 + \eta) \operatorname{ep} \left( 150 \eta^3 + 9 \times (-26 + \mathfrak{z}2) - 3 \eta t (-13 + \mathfrak{z}2) + \right. \right. \\
& \quad \quad 15 \eta^2 (13 - 10 \eta t + \mathfrak{z}2) - 2 \eta (629 - 23 \mathfrak{z}2 + 5 \eta t (3 + \mathfrak{z}2)) \left. \right) - \\
& \quad (-1 + \eta t) \operatorname{el} \left( 15 \times (6 + \mathfrak{z}2) + \operatorname{ep} \left( 15 \eta^2 (11 + \mathfrak{z}2) - 6 \times (54 + 12 \mathfrak{z}1 + \right. \right. \\
& \quad \quad 13 \mathfrak{z}2) + \eta (-1219 - 21 \mathfrak{z}2 + 25 \mathfrak{z}2^2) \left. \right) \left. \right) - x (-1 + \eta) \eta \\
& \quad \left( 600 \eta^6 \operatorname{ep} - 60 \eta^5 \operatorname{ep} (-21 + 10 \eta t - \mathfrak{z}2) + 2 \eta t \operatorname{ep} (369 + 40 \mathfrak{z}2) - \right. \\
& \quad 4 \eta^3 \operatorname{ep} (-556 + 2 \eta t (-183 + \mathfrak{z}2) + 28 \mathfrak{z}2 + \operatorname{el} (1336 - 6 \mathfrak{z}2 - 25 \mathfrak{z}2^2) + \\
& \quad \left. \eta t \operatorname{el} (-1336 + 6 \mathfrak{z}2 + 25 \mathfrak{z}2^2) \right) - 4 \eta^4 \operatorname{ep} (1957 - 49 \mathfrak{z}2 - \\
& \quad 15 \operatorname{el} (17 + \mathfrak{z}2) + 5 \eta t (2 \times (6 + \mathfrak{z}2) + 3 \operatorname{el} (17 + \mathfrak{z}2))) + \\
& \quad 3 \eta^2 (-2 \operatorname{ep} (24 \times (-26 + \mathfrak{z}2) + \eta t (295 + 22 \mathfrak{z}2)) + \\
& \quad (-1 + \eta t) \operatorname{el} (-4 \times (26 + 5 \mathfrak{z}2) + \operatorname{ep} (1734 + 363 \mathfrak{z}1 + 419 \mathfrak{z}2))) + \\
& \quad 2 \eta \left( 2 \eta t \operatorname{ep} (102 + 25 \mathfrak{z}2) + (-1 + \eta t) \operatorname{el} (-5 \times (29 + 4 \mathfrak{z}2) + \right. \\
& \quad \left. \operatorname{ep} (514 + 333 \mathfrak{z}1 + 317 \mathfrak{z}2 + 30 \mathfrak{z}2^2)) \right) + x^2 (-1 + \eta)^2 \\
& \quad \left( 1200 \eta^6 \operatorname{ep} - 120 \eta^5 \operatorname{ep} (-15 + 10 \eta t - \mathfrak{z}2) + 4 \eta t \operatorname{ep} (93 + 10 \mathfrak{z}2) - \right. \\
& \quad 8 \eta^4 \operatorname{ep} (1789 + (-43 + 10 \eta t) \mathfrak{z}2 + 15 \times (-1 + \eta t) \operatorname{el} (15 + \mathfrak{z}2)) + \\
& \quad 3 \eta^2 (-2 \operatorname{ep} (36 \times (-26 + \mathfrak{z}2) + \eta t (343 + 18 \mathfrak{z}2)) + \\
& \quad (-1 + \eta t) \operatorname{el} (-4 \times (91 + 15 \mathfrak{z}2) + 3 \operatorname{ep} (870 + 187 \mathfrak{z}1 + 211 \mathfrak{z}2))) - \\
& \quad 8 \eta^3 \operatorname{ep} (-712 + 31 \mathfrak{z}2 + \operatorname{el} (1297 + 3 \mathfrak{z}2 - 25 \mathfrak{z}2^2) + \\
& \quad \left. \eta t (-267 - \mathfrak{z}2 + \operatorname{el} (-1297 - 3 \mathfrak{z}2 + 25 \mathfrak{z}2^2)) \right) + \\
& \quad \eta (10 \eta t \operatorname{ep} (75 + 14 \mathfrak{z}2) + (-1 + \eta t) \operatorname{el} (-694 - 80 \mathfrak{z}2 +
\end{aligned}$$





$$\begin{aligned}
& (3 + 2 \, \mathfrak{e}1 + \mathfrak{e}2) + \mu1 (10 - 2 \, \mu2 + 5 \, \mathfrak{e}1 - 2 \, \mathfrak{e}2 - 6 \, \mu2 \, \mathfrak{e}2) \Big) + \\
& \eta t \Big( -2 \times \Big( 1 + \mu1^2 - \mu2 + \mu1 (-4 + 5 \, \mu2) \Big) + \theta l \Big( 1 + 4 \, \mu2 + \\
& \quad \mu1^2 (3 + 2 \, \mathfrak{e}1 + \mathfrak{e}2) + \mu1 (10 - 2 \, \mu2 + 5 \, \mathfrak{e}1 - 2 \, \mathfrak{e}2 - 6 \, \mu2 \, \mathfrak{e}2) \Big) \Big) \Big) + \\
& \eta \Big( \theta l \Big( 5 \times (1 + \mu2) \times (-2 + \mathfrak{e}1 - \mathfrak{e}2) + \mu1^2 (2 - \mathfrak{e}1 + \mathfrak{e}2) + \\
& \quad \mu1 (5 \, \mu2 \, \mathfrak{e}1 + 4 \times (-2 + \mathfrak{e}1 - \mathfrak{e}2) + 7 \, \mu2 (2 + \mathfrak{e}2)) \Big) \Big) + \\
& \eta t \Big( 20 + 24 \, \mu1 + 4 \, \mu1^2 + 5 \, \mu2 - 19 \, \mu1 \, \mu2 + \theta l \\
& \quad \Big( \mu1^2 (-2 + \mathfrak{e}1 - \mathfrak{e}2) - 5 \times (1 + \mu2) \times (-2 + \mathfrak{e}1 - \mathfrak{e}2) - \\
& \quad \mu1 (5 \, \mu2 \, \mathfrak{e}1 + 4 \times (-2 + \mathfrak{e}1 - \mathfrak{e}2) + 7 \, \mu2 (2 + \mathfrak{e}2)) \Big) \Big) \Big) - \\
& \eta^2 \Big( -2 \times \Big( 2 \times \Big( -5 + \mu1^2 - 2 \, \mu2 - 4 \, \mu1 (1 + 2 \, \mu2) \Big) + \theta l \Big( -5 - \\
& \quad 8 \, \mu2 + 5 \, \mathfrak{e}1 + 5 \, \mu2 \, \mathfrak{e}1 - 5 \, \mathfrak{e}2 - 5 \, \mu2 \, \mathfrak{e}2 + \mu1^2 (1 + \mathfrak{e}2) + \\
& \quad \mu1 (-10 + 8 \, \mathfrak{e}1 - 7 \, \mathfrak{e}2 + \mu2 (22 + 5 \, \mathfrak{e}1 + \mathfrak{e}2)) \Big) \Big) \Big) + \\
& \eta t \Big( 10 + 18 \, \mu1^2 + \mu1 (-20 + \mu2) + \mu2 + 2 \, \theta l \Big( -5 - 8 \, \mu2 + \\
& \quad 5 \, \mathfrak{e}1 + 5 \, \mu2 \, \mathfrak{e}1 - 5 \, \mathfrak{e}2 - 5 \, \mu2 \, \mathfrak{e}2 + \mu1^2 (1 + \mathfrak{e}2) + \\
& \quad \mu1 (-10 + 8 \, \mathfrak{e}1 - 7 \, \mathfrak{e}2 + \mu2 (22 + 5 \, \mathfrak{e}1 + \mathfrak{e}2)) \Big) \Big) \Big) \Big) - w (-1 + \eta) \times \\
& (6 \, \eta^8 (1 + \mu1) + 2 \, \eta^7 (7 + 9 \, \mu1^2 - 3 \, \eta t (1 + \mu1) + \mu1 (22 - 18 \, \mu2)) - \\
& 5 \, \eta t (1 + \mu1) \, \mu2 + 2 \, \eta \, \eta t (-4 \, \mu1^2 + \mu1 (22 - 31 \, \mu2) + 5 \times (4 + \mu2)) + \\
& \eta^6 (2 \times (7 + (22 + \theta l) \, \mu2) + \mu1^2 (34 + \theta l (4 + \mathfrak{e}1 + \mathfrak{e}2)) + \\
& \quad \mu1 (84 - 76 \, \mu2 + \theta l (16 - 10 \, \mu2 + \mathfrak{e}1 + \mathfrak{e}2)) - \\
& \quad \eta t (2 \times (7 + \theta l \, \mu2) + \mu1^2 (-4 + \theta l (4 + \mathfrak{e}1 + \mathfrak{e}2)) + \\
& \quad \mu1 (10 - 24 \, \mu2 + \theta l (16 - 10 \, \mu2 + \mathfrak{e}1 + \mathfrak{e}2)) \Big) \Big) - \\
& \eta^3 (52 + 84 \, \mu1 + 8 \, \mu1^2 + 72 \, \mu2 + 24 \, \mu1 \, \mu2 - \theta l (-28 + 30 \, \mathfrak{e}1 + \\
& \quad \mu1 (-46 + 55 \, \mathfrak{e}1 + \mu2 (98 + 30 \, \mathfrak{e}1 - 6 \, \mathfrak{e}2) - 49 \, \mathfrak{e}2) + \\
& \quad \mu2 (-34 + 30 \, \mathfrak{e}1 - 30 \, \mathfrak{e}2) - 30 \, \mathfrak{e}2 + \mu1^2 (6 + \mathfrak{e}1 + 5 \, \mathfrak{e}2)) \Big) + \\
& \eta t (2 \times (16 + 22 \, \mu1^2 + \mu1 (-4 + \mu2) + \mu2) + \theta l (-28 + 30 \, \mathfrak{e}1 + \\
& \quad \mu1 (-46 + 55 \, \mathfrak{e}1 + \mu2 (98 + 30 \, \mathfrak{e}1 - 6 \, \mathfrak{e}2) - 49 \, \mathfrak{e}2) + \\
& \quad \mu2 (-34 + 30 \, \mathfrak{e}1 - 30 \, \mathfrak{e}2) - 30 \, \mathfrak{e}2 + \mu1^2 (6 + \mathfrak{e}1 + 5 \, \mathfrak{e}2)) \Big) \Big) - \\
& \eta^4 (74 \, \mu1 + 38 \, \mu1^2 + 40 \, \mu2 - 128 \, \mu1 \, \mu2 - \theta l (4 + 15 \, \mathfrak{e}1 + \mu1 \\
& \quad (14 + 54 \, \mathfrak{e}1 + 3 \, \mu2 (14 + 5 \, \mathfrak{e}1 - 13 \, \mathfrak{e}2) - 40 \, \mathfrak{e}2) + \\
& \quad 3 \, \mu2 (2 + 5 \, \mathfrak{e}1 - 5 \, \mathfrak{e}2) - 15 \, \mathfrak{e}2 + \mu1^2 (9 \, \mathfrak{e}1 + 5 \times (2 + \mathfrak{e}2)) \Big) \Big) + \\
& \eta t (46 + 102 \, \mu1 - 40 \, \mu1^2 + 19 \, \mu2 - 53 \, \mu1 \, \mu2 + \theta l \\
& \quad (4 + 15 \, \mathfrak{e}1 + \mu1 (14 + 54 \, \mathfrak{e}1 + 3 \, \mu2 (14 + 5 \, \mathfrak{e}1 - 13 \, \mathfrak{e}2) - 40 \, \mathfrak{e}2) + \\
& \quad 3 \, \mu2 (2 + 5 \, \mathfrak{e}1 - 5 \, \mathfrak{e}2) - 15 \, \mathfrak{e}2 + \mu1^2 (9 \, \mathfrak{e}1 + 5 \times (2 + \mathfrak{e}2)) \Big) \Big) \Big) + \\
& \eta^2 (4 \times (1 + \mu1) \times (-5 + \mu1 - 3 \, \mu2) + \theta l (3 \, \mu2 (-8 + 5 \, \mathfrak{e}1 - 5 \, \mathfrak{e}2) + \\
& \quad 5 \times (-4 + 3 \, \mathfrak{e}1 - 3 \, \mathfrak{e}2) + \mu1^2 (2 - 2 \, \mathfrak{e}1 + 2 \, \mathfrak{e}2) + \\
& \quad \mu1 (-30 + 19 \, \mathfrak{e}1 - 19 \, \mathfrak{e}2 + 3 \, \mu2 (16 + 5 \, \mathfrak{e}1 + 3 \, \mathfrak{e}2)) \Big) \Big) + \\
& \eta t (-4 \times (-15 - 26 \, \mu1 + \mu1^2 - 6 \, \mu2 + 18 \, \mu1 \, \mu2) + \theta l (-3 \, \mu2 (-8 + \\
& \quad 5 \, \mathfrak{e}1 - 5 \, \mathfrak{e}2) + 2 \, \mu1^2 (-1 + \mathfrak{e}1 - \mathfrak{e}2) + 5 \times (4 - 3 \, \mathfrak{e}1 + 3 \, \mathfrak{e}2) - \\
& \quad \mu1 (-30 + 19 \, \mathfrak{e}1 - 19 \, \mathfrak{e}2 + 3 \, \mu2 (16 + 5 \, \mathfrak{e}1 + 3 \, \mathfrak{e}2)) \Big) \Big) \Big) + \\
& \eta^5 (38 + 40 \, \mu1 - 10 \, \mu1^2 + 80 \, \mu2 + 20 \, \mu1 \, \mu2 + \theta l (6 \times (2 + 3 \, \mu2) + \\
& \quad \mu1^2 (10 + 7 \, \mathfrak{e}1 + 3 \, \mathfrak{e}2) + \mu1 (46 + 19 \, \mathfrak{e}1 - 9 \, \mathfrak{e}2 - 6 \, \mu2 (3 + 4 \, \mathfrak{e}2)) \Big) - \\
& \eta t (2 + 38 \, \mu1 - 12 \, \mu1^2 + 8 \, \mu2 - 64 \, \mu1 \, \mu2 + \theta l \\
& \quad (6 \times (2 + 3 \, \mu2) + \mu1^2 (10 + 7 \, \mathfrak{e}1 + 3 \, \mathfrak{e}2) + \\
& \quad \mu1 (46 + 19 \, \mathfrak{e}1 - 9 \, \mathfrak{e}2 - 6 \, \mu2 (3 + 4 \, \mathfrak{e}2)) \Big) \Big) \Big) \Big) +
\end{aligned}$$

$$\begin{aligned}
& w^2 (-1 + \eta)^2 \left( 2 \eta^8 (1 + \mu_1) - 15 \eta t (1 + \mu_1) \mu_2 - 2 \eta^7 (-7 + \eta t - \right. \\
& \quad 11 \mu_1 + \eta t \mu_1 - 4 \mu_1^2 + 6 \mu_1 \mu_2) - 12 \eta \eta t (-5 + \mu_1^2 + \mu_1 (-7 + 6 \mu_2)) + \\
& \quad 2 \eta^6 (12 + 21 \mu_1^2 + \mu_1 (45 - 43 \mu_2) + 11 \mu_2 + \eta t (-7 + \mu_1 (-7 + 6 \mu_2))) - \\
& \quad \eta^3 (2 \times (30 + 17 \mu_1^2 + \mu_1 (65 - 38 \mu_2) + 58 \mu_2) - \\
& \quad \theta l (\mu_1 (-26 + 61 \mu_1 + 6 \mu_2 (9 + 5 \mu_1 - 3 \mu_2) - 57 \mu_2) + \\
& \quad 6 \times (1 + \mu_2) \times (-3 + 5 \mu_1 - 5 \mu_2) + \mu_1^2 (4 + \mu_1 + 3 \mu_2)) + \\
& \quad \eta t (44 + 4 \mu_1^2 - 4 \mu_1 (-15 + \mu_2) - 4 \mu_2 + \theta l \mu_1 \\
& \quad (-26 + 61 \mu_1 + 6 \mu_2 (9 + 5 \mu_1 - 3 \mu_2) - 57 \mu_2) + \\
& \quad 6 \theta l (1 + \mu_2) \times (-3 + 5 \mu_1 - 5 \mu_2) + \theta l \mu_1^2 (4 + \mu_1 + 3 \mu_2)) \Big) + \\
& \quad \eta^2 (-2 \times (23 + 25 \mu_2 + \mu_1 (29 + 7 \mu_2)) - \theta l (-((1 + \mu_2) \times \\
& \quad (-14 + 15 \mu_1 - 15 \mu_2)) + \mu_1^2 (\mu_1 - \mu_2) + \\
& \quad 26 \mu_1 (1 - \mu_1 + \mu_2) + \mu_1 \mu_2 (-34 - 15 \mu_1 + 3 \mu_2)) + \\
& \quad \eta t (64 + 140 \mu_1 - 44 \mu_1^2 + 38 \mu_2 - 94 \mu_1 \mu_2 + \theta l \\
& \quad (-((1 + \mu_2) \times (-14 + 15 \mu_1 - 15 \mu_2)) + \mu_1^2 (\mu_1 - \mu_2) + \\
& \quad 26 \mu_1 (1 - \mu_1 + \mu_2) + \mu_1 \mu_2 (-34 - 15 \mu_1 + 3 \mu_2))) \Big) + \\
& \quad \eta^4 (20 - 34 \mu_1 - 42 \mu_1^2 + 36 \mu_2 + 108 \mu_1 \mu_2 + \theta l (\mu_1 (26 + \\
& \quad 44 \mu_1 + 3 \mu_2 (2 + 5 \mu_1 - 9 \mu_2) - 36 \mu_2) + \\
& \quad 3 \times (1 + \mu_2) \times (2 + 5 \mu_1 - 5 \mu_2) + \mu_1^2 (8 + 5 \mu_1 + 3 \mu_2)) - \\
& \quad \eta t (50 + 118 \mu_1 - 52 \mu_1^2 + 23 \mu_2 - 97 \mu_1 \mu_2 + \theta l \\
& \quad (\mu_1 (26 + 44 \mu_1 + 3 \mu_2 (2 + 5 \mu_1 - 9 \mu_2) - 36 \mu_2) + \\
& \quad 3 \times (1 + \mu_2) \times (2 + 5 \mu_1 - 5 \mu_2) + \mu_1^2 (8 + 5 \mu_1 + 3 \mu_2))) \Big) + \\
& \quad \eta^5 (46 + 26 \mu_1^2 + 108 \mu_2 + 10 \theta l (1 + \mu_2) - 36 \mu_1 (-3 + 2 \mu_2) + \\
& \quad \theta l \mu_1^2 (4 + 3 \mu_1 + \mu_2) + \theta l \mu_1 (26 + 9 \mu_1 - 5 \mu_2 - 2 \mu_2 (7 + 6 \mu_2)) - \\
& \quad \eta t (14 + 30 \mu_1 - 8 \mu_1^2 + 4 \mu_2 - 68 \mu_1 \mu_2 + \theta l (10 \times (1 + \mu_2) + \mu_1^2 (4 + \\
& \quad 3 \mu_1 + \mu_2) + \mu_1 (26 + 9 \mu_1 - 5 \mu_2 - 2 \mu_2 (7 + 6 \mu_2)))) \Big) - \\
& x^3 (-1 + \eta)^3 ((-1 + \eta) \theta p (20 + 104 \eta + 36 \eta^2 + 80 \eta^4 - 20 \eta t - 16 \eta \eta t - \\
& \quad 80 \eta^2 \eta t - 80 \eta^3 \eta t + 16 \mu_1 + 168 \eta \mu_1 + 456 \eta^2 \mu_1 + 440 \eta^3 \mu_1 + \\
& \quad 80 \eta^4 \mu_1 - 48 \eta t \mu_1 - 80 \eta \eta t \mu_1 - 64 \eta^2 \eta t \mu_1 - 80 \eta^3 \eta t \mu_1 - \\
& \quad 4 \mu_1^2 + 16 \eta \mu_1^2 + 180 \eta^2 \mu_1^2 + 200 \eta^3 \mu_1^2 + 44 \eta t \mu_1^2 + \\
& \quad 32 \eta \eta t \mu_1^2 + 16 \eta^2 \eta t \mu_1^2 + 12 \mu_2 + 152 \eta \mu_2 + 196 \eta^2 \mu_2 - \\
& \quad 9 \eta t \mu_2 - 16 \eta \eta t \mu_2 + 12 \mu_1 \mu_2 + 8 \eta \mu_1 \mu_2 - 116 \eta^2 \mu_1 \mu_2 - \\
& \quad 240 \eta^3 \mu_1 \mu_2 + 39 \eta t \mu_1 \mu_2 + 128 \eta \eta t \mu_1 \mu_2 + 120 \eta^2 \eta t \mu_1 \mu_2 + \\
& \quad 2 w^4 (-1 + \eta)^4 (5 + 12 \mu_1 + 7 \mu_1^2 + 4 \eta^2 (1 + \mu_1) + 11 \mu_2 - \\
& \quad 7 \mu_1 \mu_2 + 2 \eta (1 + 9 \mu_1 + 8 \mu_1^2 - 2 \eta t (1 + \mu_1) - 3 \mu_1 \mu_2) + \\
& \quad \eta t (-2 - 2 \mu_1 + 6 \mu_1 \mu_2)) - w^3 (-1 + \eta)^3 \\
& \quad (60 + 40 \mu_1^2 + 44 \eta t \mu_1^2 + 40 \eta^3 (1 + \mu_1) + 4 \mu_1 (31 - 14 \mu_2) + \\
& \quad 112 \mu_2 - 9 \eta t (4 + \mu_2) + \eta t \mu_1 (-64 + 87 \mu_2) + \\
& \quad 8 \eta^2 (7 + 27 \mu_1 + 20 \mu_1^2 - 5 \eta t (1 + \mu_1) - 12 \mu_1 \mu_2) + 4 \eta (24 + 82 \mu_1 + \\
& \quad 46 \mu_1^2 + 44 \mu_2 - 43 \mu_1 \mu_2 + 2 \eta t (-7 - 7 \mu_1 + 12 \mu_1 \mu_2))) + \\
& w^2 (-1 + \eta)^2 (40 \eta^4 (1 + \mu_1) + 2 \times (51 + 92 \mu_1 + 17 \mu_1^2 + 83 \mu_2 - \\
& \quad 19 \mu_1 \mu_2) - 40 \eta^3 (-4 + \eta t - 8 \mu_1 + \eta t \mu_1 - 4 \mu_1^2 + 3 \mu_1 \mu_2) + \\
& \quad \eta t (-80 - 164 \mu_1 + 132 \mu_1^2 - 27 \mu_2 + 177 \mu_1 \mu_2) + \\
& \quad 4 \eta^2 (55 + 240 \mu_1 + 125 \mu_1^2 + 55 \mu_2 - 119 \mu_1 \mu_2 +
\end{aligned}$$

$$\begin{aligned}
& 10 \eta t (-4 - 4 \mu_1 + 3 \mu_1 \mu_2) + 4 \eta (71 + 207 \mu_1 + 76 \mu_1^2 + \\
& 130 \mu_2 - 98 \mu_1 \mu_2 + \eta t (-30 - 46 \mu_1 + 8 \mu_1^2 - 4 \mu_2 + 80 \mu_1 \mu_2)) - \\
& w (-1 + \eta) \times (120 \eta^4 (1 + \mu_1) + 40 \eta^3 (5 + 9 \mu_1^2 - 3 \eta t (1 + \mu_1) + \\
& \mu_1 (20 - 9 \mu_2)) + 4 \times (18 + \mu_1^2 + 22 \mu_2 + \mu_1 (25 + 4 \mu_2)) + \\
& \eta t (-68 + 132 \mu_1^2 - 27 \mu_2 + \mu_1 (-152 + 141 \mu_2)) + \\
& 8 \eta^2 (26 + 65 \mu_1^2 + \mu_1 (151 - 62 \mu_2) + 52 \mu_2 + \eta t (-25 + 2 \mu_1^2 + \\
& \mu_1 (-23 + 30 \mu_2))) + 8 \eta (33 + 21 \mu_1^2 - 28 \mu_1 (-3 + \mu_2) + \\
& 62 \mu_2 + \eta t (-11 + 8 \mu_1^2 - 4 \mu_2 + \mu_1 (-27 + 44 \mu_2))) + \\
& (-1 + \eta t) \theta l (-30 - 60 \eta + 10 \theta p - 24 \eta \theta p - 20 \eta^2 \theta p + 80 \eta^3 \theta p - \\
& 32 \mu_1 - 160 \eta \mu_1 - 120 \eta^2 \mu_1 + 24 \eta^3 \mu_1 + 18 \theta p \mu_1 + 10 \eta \theta p \mu_1 - \\
& 188 \eta^2 \theta p \mu_1 - 220 \eta^3 \theta p \mu_1 + 10 \mu_1^2 + 56 \eta \mu_1^2 + 24 \eta^2 \mu_1^2 + \\
& 24 \eta^3 \mu_1^2 - 4 \theta p \mu_1^2 - 14 \eta \theta p \mu_1^2 - 48 \eta^2 \theta p \mu_1^2 - 60 \eta^3 \theta p \mu_1^2 + \\
& w^4 (-1 + \eta)^4 (26 \mu_1^2 + 5 \mu_1 (-4 + \mu_2) + 5 \times (-2 + \mu_2)) - \\
& 10 \mu_2 - 15 \eta \mu_2 + 14 \theta p \mu_2 - 6 \eta \theta p \mu_2 - 68 \eta^2 \theta p \mu_2 - \\
& 20 \eta^3 \theta p \mu_2 + 38 \mu_1 \mu_2 + 57 \eta \mu_1 \mu_2 - 34 \theta p \mu_1 \mu_2 - \\
& 114 \eta \theta p \mu_1 \mu_2 - 20 \eta^2 \theta p \mu_1 \mu_2 + 100 \eta^3 \theta p \mu_1 \mu_2 - \\
& 10 \theta p \mathfrak{z}1 - 20 \eta \theta p \mathfrak{z}1 - 17 \theta p \mu_1 \mathfrak{z}1 - 87 \eta \theta p \mu_1 \mathfrak{z}1 - \\
& 94 \eta^2 \theta p \mu_1 \mathfrak{z}1 - 10 \eta^3 \theta p \mu_1 \mathfrak{z}1 - \theta p \mu_1^2 \mathfrak{z}1 - 19 \eta \theta p \mu_1^2 \mathfrak{z}1 - \\
& 34 \eta^2 \theta p \mu_1^2 \mathfrak{z}1 - 10 \eta^3 \theta p \mu_1^2 \mathfrak{z}1 - 10 \theta p \mu_2 \mathfrak{z}1 - 20 \eta \theta p \mu_2 \mathfrak{z}1 - \\
& 10 \theta p \mu_1 \mu_2 \mathfrak{z}1 - 20 \eta \theta p \mu_1 \mu_2 \mathfrak{z}1 - w^3 (-1 + \eta)^3 (76 \mu_1^2 + \\
& \eta (60 \mu_1^2 + \mu_1 (-156 + \mu_2 (57 - 20 \theta p (\mathfrak{z}1 - \mathfrak{z}2)) - 44 \theta p (\mathfrak{z}1 - \mathfrak{z}2)) - \\
& 5 \times (12 + 3 \mu_2 + 4 \theta p (\mathfrak{z}1 - \mathfrak{z}2) + 4 \theta p \mu_2 (\mathfrak{z}1 - \mathfrak{z}2))) + \\
& \mu_1 (-128 + \mu_2 (53 - 10 \theta p (\mathfrak{z}1 - \mathfrak{z}2)) - 22 \theta p (\mathfrak{z}1 - \mathfrak{z}2)) - \\
& 5 \times (12 - \mu_2 + 2 \theta p (\mathfrak{z}1 - \mathfrak{z}2) + 2 \theta p \mu_2 (\mathfrak{z}1 - \mathfrak{z}2))) + 10 \theta p \mathfrak{z}2 + \\
& 20 \eta \theta p \mathfrak{z}2 + 13 \theta p \mu_1 \mathfrak{z}2 + 57 \eta \theta p \mu_1 \mathfrak{z}2 + 46 \eta^2 \theta p \mu_1 \mathfrak{z}2 - \\
& 10 \eta^3 \theta p \mu_1 \mathfrak{z}2 - 3 \theta p \mu_1^2 \mathfrak{z}2 - 11 \eta \theta p \mu_1^2 \mathfrak{z}2 - 14 \eta^2 \theta p \mu_1^2 \mathfrak{z}2 - \\
& 10 \eta^3 \theta p \mu_1^2 \mathfrak{z}2 + 10 \theta p \mu_2 \mathfrak{z}2 + 20 \eta \theta p \mu_2 \mathfrak{z}2 - \\
& 2 \theta p \mu_1 \mu_2 \mathfrak{z}2 + 68 \eta \theta p \mu_1 \mu_2 \mathfrak{z}2 + 120 \eta^2 \theta p \mu_1 \mu_2 \mathfrak{z}2 + \\
& w (-1 + \eta) \times (100 + 152 \mu_1 - 44 \mu_1^2 + 25 \mu_2 - 119 \mu_1 \mu_2 + \\
& 2 \theta p (-14 + 15 \mathfrak{z}1 + \mu_1 (-22 + 28 \mathfrak{z}1 + \mu_2 (44 + 15 \mathfrak{z}1 - 3 \mathfrak{z}2) - 24 \mathfrak{z}2) + \\
& \mu_2 (-16 + 15 \mathfrak{z}1 - 15 \mathfrak{z}2) - 15 \mathfrak{z}2 + \mu_1^2 (4 + \mathfrak{z}1 + 3 \mathfrak{z}2)) + \\
& 2 \eta^3 (10 \theta p \mu_2 + \mu_1^2 (-12 + 5 \theta p (6 + \mathfrak{z}1 + \mathfrak{z}2)) + \\
& \mu_1 (-12 + 5 \theta p (30 - 10 \mu_2 + \mathfrak{z}1 + \mathfrak{z}2))) + \\
& \eta (180 + 472 \mu_1 - 176 \mu_1^2 + 45 \mu_2 - 171 \mu_1 \mu_2 + \theta p (16 + 60 \mathfrak{z}1 + \\
& \mu_1 (62 + 219 \mathfrak{z}1 + 6 \mu_2 (23 + 10 \mathfrak{z}1 - 26 \mathfrak{z}2) - 157 \mathfrak{z}2) + 30 \mu_2 \\
& (1 + 2 \mathfrak{z}1 - 2 \mathfrak{z}2) - 60 \mathfrak{z}2 + \mu_1^2 (39 \mathfrak{z}1 + 23 \times (2 + \mathfrak{z}2)))) + \\
& 8 \eta^2 (-6 \times (-5 + \mu_1) \mu_1 + \theta p (3 \times (5 + 7 \mu_2) + \mu_1^2 (11 + 8 \mathfrak{z}1 + \\
& 3 \mathfrak{z}2) + \mu_1 (56 + 23 \mathfrak{z}1 - 12 \mathfrak{z}2 - 15 \mu_2 (1 + 2 \mathfrak{z}2)))) - \\
& w^2 (-1 + \eta)^2 (-84 \mu_1^2 + 3 \mu_1 (76 - 43 \mu_2) + 15 \times (8 + \mu_2) + \\
& \theta p \mu_1 (-26 + 61 \mathfrak{z}1 + 6 \mu_2 (9 + 5 \mathfrak{z}1 - 3 \mathfrak{z}2) - 57 \mathfrak{z}2) + \\
& 6 \theta p (1 + \mu_2) \times (-3 + 5 \mathfrak{z}1 - 5 \mathfrak{z}2) + \theta p \mu_1^2 (4 + \mathfrak{z}1 + 3 \mathfrak{z}2) + \\
& \eta (-9 \times (20 \mu_1^2 - 5 \times (4 + \mu_2) + \mu_1 (-52 + 19 \mu_2)) + \\
& 4 \theta p (\mu_1 (26 + 44 \mathfrak{z}1 + 3 \mu_2 (2 + 5 \mathfrak{z}1 - 9 \mathfrak{z}2) - 36 \mathfrak{z}2) + \\
& 3 \times (1 + \mu_2) \times (2 + 5 \mathfrak{z}1 - 5 \mathfrak{z}2) + \mu_1^2 (8 + 5 \mathfrak{z}1 + 3 \mathfrak{z}2))) +
\end{aligned}$$

$$\begin{aligned}
& 2 \eta^2 \left( -12 \times (-5 + \mu_1) \mu_1 + 5 \theta p \left( 10 \times (1 + \mu_2) + \mu_1^2 (4 + \right. \right. \\
& \quad \left. \left. 3 \mathfrak{E}1 + \mathfrak{E}2) + \mu_1 (26 + 9 \mathfrak{E}1 - 5 \mathfrak{E}2 - 2 \mu_2 (7 + 6 \mathfrak{E}2)) \right) \right) + \\
& x^4 (-1 + \eta)^4 \left( 2 \times (-1 + \eta) \theta p \left( 13 + 7 \eta - 10 \eta^2 + 30 \eta^3 - 2 \eta t - 20 \eta \eta t - \right. \right. \\
& \quad 30 \eta^2 \eta t + 21 \mu_1 + 112 \eta \mu_1 + 155 \eta^2 \mu_1 + 30 \eta^3 \mu_1 - 10 \eta t \mu_1 - \\
& \quad 18 \eta \eta t \mu_1 - 30 \eta^2 \eta t \mu_1 + 2 \mu_1^2 + 45 \eta \mu_1^2 + 75 \eta^2 \mu_1^2 + \\
& \quad 4 \eta t \mu_1^2 + 2 \eta \eta t \mu_1^2 + w^4 (-1 + \eta)^4 (1 + \mu_1) (\eta - \eta t + 4 \mu_1) + \\
& \quad 19 \mu_2 + 47 \eta \mu_2 - 2 \eta t \mu_2 + \mu_1 \mu_2 - 7 \eta \mu_1 \mu_2 - \\
& \quad 60 \eta^2 \mu_1 \mu_2 + 16 \eta t \mu_1 \mu_2 + 30 \eta \eta t \mu_1 \mu_2 - \\
& \quad w^3 (-1 + \eta)^3 \left( 10 + 39 \mu_1 + 23 \mu_1^2 + 10 \eta^2 (1 + \mu_1) + 22 \mu_2 - \right. \\
& \quad \left. 14 \mu_1 \mu_2 + \eta (7 + 47 \mu_1 + 40 \mu_1^2 - 10 \eta t (1 + \mu_1) - 12 \mu_1 \mu_2) + \right. \\
& \quad \left. \eta t (-7 - 7 \mu_1 + 12 \mu_1 \mu_2) \right) + w^2 (-1 + \eta)^2 \\
& \quad \left( 33 + 101 \mu_1 + 38 \mu_1^2 + 15 \eta^3 (1 + \mu_1) + 65 \mu_2 - 37 \mu_1 \mu_2 + \right. \\
& \quad \left. \eta t (-15 - 23 \mu_1 + 4 \mu_1^2 - 2 \mu_2 + 40 \mu_1 \mu_2) - 5 \eta^2 \right. \\
& \quad \left. (3 \eta t (1 + \mu_1) - 2 \times (4 + 10 \mu_1 + 6 \mu_1^2 - 3 \mu_1 \mu_2)) + \eta (40 + 225 \mu_1 + \right. \\
& \quad \left. 125 \mu_1^2 + 55 \mu_2 - 77 \mu_1 \mu_2 + 10 \eta t (-4 - 4 \mu_1 + 3 \mu_1 \mu_2)) \right) - \\
& w (-1 + \eta) \times \left( 32 + 83 \mu_1 + 21 \mu_1^2 + 45 \eta^3 (1 + \mu_1) + 62 \mu_2 - \right. \\
& \quad 22 \mu_1 \mu_2 + 5 \eta^2 (10 + 55 \mu_1 + 27 \mu_1^2 - 9 \eta t (1 + \mu_1) - 18 \mu_1 \mu_2) + \\
& \quad \left. \eta t (-11 - 27 \mu_1 + 8 \mu_1^2 - 4 \mu_2 + 44 \mu_1 \mu_2) + \eta (41 + 291 \mu_1 + 130 \mu_1^2 + \right. \\
& \quad \left. 102 \mu_2 - 72 \mu_1 \mu_2 + 2 \eta t (-25 + \mu_1^2 + 6 \mu_1 (-4 + 5 \mu_2)) \right) + \\
& (-1 + \eta t) \theta l \left( -20 - 6 \theta p - 10 \eta \theta p + 60 \eta^2 \theta p - 52 \mu_1 - 80 \eta \mu_1 + \right. \\
& \quad 16 \eta^2 \mu_1 + 2 \theta p \mu_1 - 92 \eta \theta p \mu_1 - 160 \eta^2 \theta p \mu_1 + \\
& \quad 28 \mu_1^2 + 16 \eta \mu_1^2 + 16 \eta^2 \mu_1^2 - 4 \theta p \mu_1^2 - 22 \eta \theta p \mu_1^2 - \\
& \quad 40 \eta^2 \theta p \mu_1^2 - 5 \mu_2 - 2 \theta p \mu_2 - 32 \eta \theta p \mu_2 - 10 \eta^2 \theta p \mu_2 + \\
& \quad 19 \mu_1 \mu_2 - 26 \theta p \mu_1 \mu_2 - 20 \eta \theta p \mu_1 \mu_2 + 50 \eta^2 \theta p \mu_1 \mu_2 - \\
& \quad 5 \theta p \mathfrak{E}1 - 22 \theta p \mu_1 \mathfrak{E}1 - 46 \eta \theta p \mu_1 \mathfrak{E}1 - 5 \eta^2 \theta p \mu_1 \mathfrak{E}1 - \\
& \quad 5 \theta p \mu_1^2 \mathfrak{E}1 - 16 \eta \theta p \mu_1^2 \mathfrak{E}1 - 5 \eta^2 \theta p \mu_1^2 \mathfrak{E}1 - 5 \theta p \mu_2 \mathfrak{E}1 - \\
& \quad 5 \theta p \mu_1 \mu_2 \mathfrak{E}1 + 5 \theta p \mathfrak{E}2 + 14 \theta p \mu_1 \mathfrak{E}2 + 24 \eta \theta p \mu_1 \mathfrak{E}2 - \\
& \quad 5 \eta^2 \theta p \mu_1 \mathfrak{E}2 - 3 \theta p \mu_1^2 \mathfrak{E}2 - 6 \eta \theta p \mu_1^2 \mathfrak{E}2 - 5 \eta^2 \theta p \mu_1^2 \mathfrak{E}2 + \\
& \quad 5 \theta p \mu_2 \mathfrak{E}2 + 17 \theta p \mu_1 \mu_2 \mathfrak{E}2 + 60 \eta \theta p \mu_1 \mu_2 \mathfrak{E}2 - \\
& \quad w^3 (-1 + \eta)^3 \left( 28 \mu_1^2 - 5 \times (4 + \mu_2 + \theta p (\mathfrak{E}1 - \mathfrak{E}2) + \theta p \mu_2 (\mathfrak{E}1 - \mathfrak{E}2)) + \right. \\
& \quad \left. \mu_1 (-52 - 11 \theta p (\mathfrak{E}1 - \mathfrak{E}2) + \mu_2 (19 - 5 \theta p \mathfrak{E}1 + 5 \theta p \mathfrak{E}2)) \right) - \\
& \quad w^2 (-1 + \eta)^2 \left( 60 + 156 \mu_1 + 80 \eta \mu_1 - 84 \mu_1^2 - 16 \eta \mu_1^2 + 15 \mu_2 - 57 \mu_1 \mu_2 + \right. \\
& \quad \left. \theta p (\mu_1 (26 + 44 \mathfrak{E}1 + 3 \mu_2 (2 + 5 \mathfrak{E}1 - 9 \mathfrak{E}2) - 36 \mathfrak{E}2) + 3 \times (1 + \mu_2) \times \right. \\
& \quad \left. (2 + 5 \mathfrak{E}1 - 5 \mathfrak{E}2) + \mu_1^2 (8 + 5 \mathfrak{E}1 + 3 \mathfrak{E}2) + 5 \eta (10 \times (1 + \mu_2) + \mu_1^2 \right. \\
& \quad \left. (4 + 3 \mathfrak{E}1 + \mathfrak{E}2) + \mu_1 (26 + 9 \mathfrak{E}1 - 5 \mathfrak{E}2 - 2 \mu_2 (7 + 6 \mathfrak{E}2)) \right) \right) + \\
& w (-1 + \eta) \times \left( 60 + 156 \mu_1 + 160 \eta \mu_1 - 16 \eta^2 \mu_1 - 84 \mu_1^2 - \right. \\
& \quad 32 \eta \mu_1^2 - 16 \eta^2 \mu_1^2 + 15 \mu_2 - 57 \mu_1 \mu_2 + \theta p (4 + 8 \mu_2 + 15 \mathfrak{E}1 + \\
& \quad 15 \mu_2 \mathfrak{E}1 + \mu_1 (16 + 55 \mathfrak{E}1 + \mu_2 (32 + 15 \mathfrak{E}1 - 39 \mathfrak{E}2) - 39 \mathfrak{E}2) - \\
& \quad 15 \mathfrak{E}2 - 15 \mu_2 \mathfrak{E}2 + 2 \mu_1^2 (6 + 5 \mathfrak{E}1 + 3 \mathfrak{E}2) + \\
& \quad 5 \eta^2 (2 \mu_2 + \mu_1^2 (8 + \mathfrak{E}1 + \mathfrak{E}2) + \mu_1 (44 - 10 \mu_2 + \mathfrak{E}1 + \mathfrak{E}2)) + \\
& \quad \left. \eta (60 + 82 \mu_2 + \mu_1^2 (42 + 31 \mathfrak{E}1 + 11 \mathfrak{E}2) + \right. \\
& \quad \left. \mu_1 (222 + 91 \mathfrak{E}1 - 49 \mathfrak{E}2 - 10 \mu_2 (5 + 12 \mathfrak{E}2)) \right) \right) + \\
& x^2 (-1 + \eta)^2 \left( (-1 + \eta) \theta p (60 \eta + 156 \eta^2 + 44 \eta^3 + 20 \eta^4 + 60 \eta^5 - 30 \eta t - \right. \\
& \quad \left. 60 \eta \eta t - 24 \eta^2 \eta t - 80 \eta^3 \eta t - 60 \eta^4 \eta t + 48 \eta \mu_1 + \right.
\end{aligned}$$

$$\begin{aligned}
& 252 \eta^2 \mu_1 + 464 \eta^3 \mu_1 + 350 \eta^4 \mu_1 + 60 \eta^5 \mu_1 - 32 \eta t \mu_1 - \\
& 148 \eta \eta t \mu_1 - 120 \eta^2 \eta t \mu_1 - 56 \eta^3 \eta t \mu_1 - 60 \eta^4 \eta t \mu_1 - \\
& 12 \eta \mu_1^2 + 24 \eta^2 \mu_1^2 + 180 \eta^3 \mu_1^2 + 150 \eta^4 \mu_1^2 + \\
& 22 \eta t \mu_1^2 + 104 \eta \eta t \mu_1^2 + 48 \eta^2 \eta t \mu_1^2 + 24 \eta^3 \eta t \mu_1^2 + \\
& 32 \eta \mu_2 + 228 \eta^2 \mu_2 + 204 \eta^3 \mu_2 - 10 \eta t \mu_2 - 27 \eta \eta t \mu_2 - \\
& 24 \eta^2 \eta t \mu_2 + 56 \eta \mu_1 \mu_2 + 12 \eta^2 \mu_1 \mu_2 - 204 \eta^3 \mu_1 \mu_2 - \\
& 240 \eta^4 \mu_1 \mu_2 + 38 \eta t \mu_1 \mu_2 + 117 \eta \eta t \mu_1 \mu_2 + \\
& 192 \eta^2 \eta t \mu_1 \mu_2 + 120 \eta^3 \eta t \mu_1 \mu_2 + w^4 (-1 + \eta)^4 \\
& \left( (12 \eta^3 (1 + \mu_1) - 12 \eta^2 (-1 + \eta t - 5 \mu_1 + \eta t \mu_1 - 4 \mu_1^2 + 3 \mu_1 \mu_2) + \right. \\
& \quad 2 \times (5 + 8 \mu_1 + 3 \mu_1^2 + 11 \mu_2 + 5 \mu_1 \mu_2) + \\
& \quad \eta t (-12 - 22 \mu_1 + 38 \mu_1^2 + 5 \mu_2 + 17 \mu_1 \mu_2) + 2 \eta \\
& \quad \left. (16 + 37 \mu_1 + 21 \mu_1^2 + 33 \mu_2 - 27 \mu_1 \mu_2 + 6 \eta t (-1 - \mu_1 + 3 \mu_1 \mu_2)) \right) - \\
& w^3 (-1 + \eta)^3 (40 \eta^4 (1 + \mu_1) + 2 \times (20 + 31 \mu_1 + 5 \mu_1^2 + 30 \mu_2 + 6 \mu_1 \mu_2) - \\
& \quad 4 \eta^3 (-21 - 61 \mu_1 - 40 \mu_1^2 + 10 \eta t (1 + \mu_1) + 36 \mu_1 \mu_2) + \\
& \quad \eta t (-66 - 130 \mu_1 + 128 \mu_1^2 + \mu_2 + 97 \mu_1 \mu_2) + \\
& \quad 3 \eta (62 + 40 \mu_1^2 + 36 \eta t \mu_1^2 + 2 \mu_1 (63 - 34 \mu_2) + 112 \mu_2 - \\
& \quad \quad 9 \eta t (4 + \mu_2) + \eta t \mu_1 (-64 + 87 \mu_2)) + 12 \eta^2 (14 + 43 \mu_1 + \\
& \quad \quad 23 \mu_1^2 + 22 \mu_2 - 29 \mu_1 \mu_2 + \eta t (-7 - 7 \mu_1 + 12 \mu_1 \mu_2)) \Big) + \\
& w^2 (-1 + \eta)^2 (46 + 58 \mu_1 + 30 \eta^5 (1 + \mu_1) + 50 \mu_2 + 14 \mu_1 \mu_2 + \\
& \quad \eta t (-124 - 224 \mu_1 + 164 \mu_1^2 - 23 \mu_2 + 181 \mu_1 \mu_2) - \\
& \quad 10 \eta^4 (3 \eta t (1 + \mu_1) - 4 \times (4 + 7 \mu_1 + 3 \mu_1^2 - 3 \mu_1 \mu_2)) + \\
& \quad 4 \eta^3 (70 + 255 \mu_1 + 125 \mu_1^2 + 55 \mu_2 - 161 \mu_1 \mu_2 + \\
& \quad \quad 10 \eta t (-4 - 4 \mu_1 + 3 \mu_1 \mu_2)) + 12 \eta^2 (38 + 106 \mu_1 + 38 \mu_1^2 + \\
& \quad \quad 65 \mu_2 - 61 \mu_1 \mu_2 + \eta t (-15 - 23 \mu_1 + 4 \mu_1^2 - 2 \mu_2 + 40 \mu_1 \mu_2)) \Big) + \\
& \quad \eta (2 \times (155 + 278 \mu_1 + 51 \mu_1^2 + 249 \mu_2 - 69 \mu_1 \mu_2) + \\
& \quad \quad 3 \eta t (-80 - 164 \mu_1 + 108 \mu_1^2 - 27 \mu_2 + 177 \mu_1 \mu_2)) \Big) - \\
& w (-1 + \eta) \times (90 \eta^5 (1 + \mu_1) - 4 \times (1 + \mu_1) \times (-5 + \mu_1 - 3 \mu_2) + \\
& \quad 10 \eta^4 (20 + 65 \mu_1 + 27 \mu_1^2 - 9 \eta t (1 + \mu_1) - 36 \mu_1 \mu_2) + \\
& \quad \eta t (-100 - 148 \mu_1 + 96 \mu_1^2 - 29 \mu_2 + 139 \mu_1 \mu_2) + \\
& \quad 12 \eta^2 (34 + 85 \mu_1 + 21 \mu_1^2 + 62 \mu_2 - 34 \mu_1 \mu_2 + \eta t \\
& \quad \quad (-11 - 27 \mu_1 + 8 \mu_1^2 - 4 \mu_2 + 44 \mu_1 \mu_2)) + 4 \eta^3 (63 + 313 \mu_1 + 130 \\
& \quad \quad \mu_1^2 + 106 \mu_2 - 176 \mu_1 \mu_2 + \eta t (-50 - 44 \mu_1 + 6 \mu_1^2 + 60 \mu_1 \mu_2)) \Big) + \\
& \quad \eta (4 \times (54 + 75 \mu_1 + 3 \mu_1^2 + 65 \mu_2 + 17 \mu_1 \mu_2) + \eta t \\
& \quad \quad (-204 - 460 \mu_1 + 320 \mu_1^2 - 81 \mu_2 + 423 \mu_1 \mu_2)) \Big) \Big) + \\
& (-1 + \eta t) \theta l (-10 - 60 \eta - 60 \eta^2 + 10 \theta p + 30 \eta \theta p - 36 \eta^2 \theta p - \\
& \quad 20 \eta^3 \theta p + 60 \eta^4 \theta p - 8 \mu_1 - 64 \eta \mu_1 - 164 \eta^2 \mu_1 - 80 \eta^3 \mu_1 + \\
& \quad 16 \eta^4 \mu_1 + 8 \theta p \mu_1 + 56 \eta \theta p \mu_1 + 18 \eta^2 \theta p \mu_1 - 192 \eta^3 \theta p \mu_1 - \\
& \quad 170 \eta^4 \theta p \mu_1 + 2 \mu_1^2 - 4 \eta \mu_1^2 + 28 \eta^2 \mu_1^2 + 16 \eta^3 \mu_1^2 + \\
& \quad 16 \eta^4 \mu_1^2 - 2 \theta p \mu_1^2 - 10 \eta \theta p \mu_1^2 - 18 \eta^2 \theta p \mu_1^2 - \\
& \quad 52 \eta^3 \theta p \mu_1^2 - 50 \eta^4 \theta p \mu_1^2 - 5 \mu_2 - 20 \eta \mu_2 - 15 \eta^2 \mu_2 + \\
& \quad 10 \theta p \mu_2 + 44 \eta \theta p \mu_2 - 6 \eta^2 \theta p \mu_2 - 72 \eta^3 \theta p \mu_2 - 20 \eta^4 \theta p \mu_2 + \\
& \quad 19 \mu_1 \mu_2 + 76 \eta \mu_1 \mu_2 + 57 \eta^2 \mu_1 \mu_2 - 14 \theta p \mu_1 \mu_2 - \\
& \quad 112 \eta \theta p \mu_1 \mu_2 - 186 \eta^2 \theta p \mu_1 \mu_2 + 100 \eta^4 \theta p \mu_1 \mu_2 + \\
& \quad 2 w^4 (-1 + \eta)^4 (\mu_1^2 + 5 \mu_1 (-2 + \mu_2) + 5 \times (-1 + \mu_2) +
\end{aligned}$$

$$\begin{aligned}
& 5 \eta \left( -2 + 4 \mu_1^2 + \mu_1 (-4 + \mu_2) + \mu_2 \right) - 5 \operatorname{er} \mathfrak{s}1 - 30 \eta \operatorname{er} \mathfrak{s}1 - \\
& 30 \eta^2 \operatorname{er} \mathfrak{s}1 - 4 \operatorname{er} \mu_1 \mathfrak{s}1 - 50 \eta \operatorname{er} \mu_1 \mathfrak{s}1 - 129 \eta^2 \operatorname{er} \mu_1 \mathfrak{s}1 - \\
& 96 \eta^3 \operatorname{er} \mu_1 \mathfrak{s}1 - 10 \eta^4 \operatorname{er} \mu_1 \mathfrak{s}1 + \operatorname{er} \mu_1^2 \mathfrak{s}1 - 2 \eta \operatorname{er} \mu_1^2 \mathfrak{s}1 - \\
& 27 \eta^2 \operatorname{er} \mu_1^2 \mathfrak{s}1 - 36 \eta^3 \operatorname{er} \mu_1^2 \mathfrak{s}1 - 10 \eta^4 \operatorname{er} \mu_1^2 \mathfrak{s}1 - \\
& 5 \operatorname{er} \mu_2 \mathfrak{s}1 - 30 \eta \operatorname{er} \mu_2 \mathfrak{s}1 - 30 \eta^2 \operatorname{er} \mu_2 \mathfrak{s}1 - 5 \operatorname{er} \mu_1 \mu_2 \mathfrak{s}1 - \\
& 30 \eta \operatorname{er} \mu_1 \mu_2 \mathfrak{s}1 - 30 \eta^2 \operatorname{er} \mu_1 \mu_2 \mathfrak{s}1 + 5 \operatorname{er} \mathfrak{s}2 + 30 \eta \operatorname{er} \mathfrak{s}2 + \\
& 30 \eta^2 \operatorname{er} \mathfrak{s}2 + 4 \operatorname{er} \mu_1 \mathfrak{s}2 + 40 \eta \operatorname{er} \mu_1 \mathfrak{s}2 + 87 \eta^2 \operatorname{er} \mu_1 \mathfrak{s}2 + \\
& 44 \eta^3 \operatorname{er} \mu_1 \mathfrak{s}2 - 10 \eta^4 \operatorname{er} \mu_1 \mathfrak{s}2 - \operatorname{er} \mu_1^2 \mathfrak{s}2 - 8 \eta \operatorname{er} \mu_1^2 \mathfrak{s}2 - \\
& 15 \eta^2 \operatorname{er} \mu_1^2 \mathfrak{s}2 - 16 \eta^3 \operatorname{er} \mu_1^2 \mathfrak{s}2 - 10 \eta^4 \operatorname{er} \mu_1^2 \mathfrak{s}2 + 5 \operatorname{er} \mu_2 \mathfrak{s}2 + \\
& 30 \eta \operatorname{er} \mu_2 \mathfrak{s}2 + 30 \eta^2 \operatorname{er} \mu_2 \mathfrak{s}2 - 7 \operatorname{er} \mu_1 \mu_2 \mathfrak{s}2 - 6 \eta \operatorname{er} \mu_1 \mu_2 \mathfrak{s}2 + \\
& 102 \eta^2 \operatorname{er} \mu_1 \mu_2 \mathfrak{s}2 + 120 \eta^3 \operatorname{er} \mu_1 \mu_2 \mathfrak{s}2 - w^3 (-1 + \eta)^3 (8 \mu_1^2 + \\
& 3 \eta^2 (12 \mu_1^2 + \mu_1 (-52 + \mu_2 (19 - 10 \operatorname{er} (\mathfrak{s}1 - \mathfrak{s}2)) - 22 \operatorname{er} (\mathfrak{s}1 - \mathfrak{s}2)) - \\
& 5 \times (4 + \mu_2 + 2 \operatorname{er} (\mathfrak{s}1 - \mathfrak{s}2) + 2 \operatorname{er} \mu_2 (\mathfrak{s}1 - \mathfrak{s}2))) + 2 \eta \\
& (46 \mu_1^2 + \mu_1 (-128 + \mu_2 (53 - 15 \operatorname{er} (\mathfrak{s}1 - \mathfrak{s}2)) - 33 \operatorname{er} (\mathfrak{s}1 - \mathfrak{s}2)) - \\
& 5 \times (12 - \mu_2 + 3 \operatorname{er} (\mathfrak{s}1 - \mathfrak{s}2) + 3 \operatorname{er} \mu_2 (\mathfrak{s}1 - \mathfrak{s}2))) - \\
& 5 \times (8 + \mu_2 (-5 + \operatorname{er} (\mathfrak{s}1 - \mathfrak{s}2)) + \operatorname{er} (\mathfrak{s}1 - \mathfrak{s}2)) + \\
& \mu_1 (-68 - 11 \operatorname{er} (\mathfrak{s}1 - \mathfrak{s}2) + \mu_2 (49 - 5 \operatorname{er} \mathfrak{s}1 + 5 \operatorname{er} \mathfrak{s}2))) - \\
& w^2 (-1 + \eta)^2 (-3 \times (4 \mu_1^2 + 5 \times (-4 + \mu_2) + \mu_1 (-28 + 29 \mu_2)) - \\
& \operatorname{er} (-((1 + \mu_2) \times (-14 + 15 \mathfrak{s}1 - 15 \mathfrak{s}2)) + \mu_1^2 (\mathfrak{s}1 - \mathfrak{s}2) + \\
& 26 \mu_1 (1 - \mathfrak{s}1 + \mathfrak{s}2) + \mu_1 \mu_2 (-34 - 15 \mathfrak{s}1 + 3 \mathfrak{s}2))) + \\
& 3 \eta (80 + 152 \mu_1 - 20 \mu_1^2 + 10 \mu_2 - 86 \mu_1 \mu_2 + \operatorname{er} \\
& (\mu_1 (-26 + 61 \mathfrak{s}1 + 6 \mu_2 (9 + 5 \mathfrak{s}1 - 3 \mathfrak{s}2) - 57 \mathfrak{s}2) + \\
& 6 \times (1 + \mu_2) \times (-3 + 5 \mathfrak{s}1 - 5 \mathfrak{s}2) + \mu_1^2 (4 + \mathfrak{s}1 + 3 \mathfrak{s}2))) + \\
& 3 \eta^2 (60 + 156 \mu_1 - 36 \mu_1^2 + 15 \mu_2 - 57 \mu_1 \mu_2 + 2 \operatorname{er} \\
& (\mu_1 (26 + 44 \mathfrak{s}1 + 3 \mu_2 (2 + 5 \mathfrak{s}1 - 9 \mathfrak{s}2) - 36 \mathfrak{s}2) + \\
& 3 \times (1 + \mu_2) \times (2 + 5 \mathfrak{s}1 - 5 \mathfrak{s}2) + \mu_1^2 (8 + 5 \mathfrak{s}1 + 3 \mathfrak{s}2))) + \\
& 2 \eta^3 (-8 \times (-5 + \mu_1) \mu_1 + 5 \operatorname{er} (10 \times (1 + \mu_2) + \mu_1^2 \\
& (4 + 3 \mathfrak{s}1 + \mathfrak{s}2) + \mu_1 (26 + 9 \mathfrak{s}1 - 5 \mathfrak{s}2 - 2 \mu_2 (7 + 6 \mathfrak{s}2)))) + \\
& w (-1 + \eta) \times (40 + 44 \mu_1 - 8 \mu_1^2 + 5 \mu_2 - 67 \mu_1 \mu_2 + 2 \eta^4 \\
& (10 \operatorname{er} \mu_2 + \mu_1^2 (-8 + 5 \operatorname{er} (5 + \mathfrak{s}1 + \mathfrak{s}2)) + \\
& \mu_1 (-8 + 5 \operatorname{er} (23 - 10 \mu_2 + \mathfrak{s}1 + \mathfrak{s}2))) + \operatorname{er} (3 \mu_2 \\
& (-8 + 5 \mathfrak{s}1 - 5 \mathfrak{s}2) + 5 \times (-4 + 3 \mathfrak{s}1 - 3 \mathfrak{s}2) + \mu_1^2 (2 - 2 \mathfrak{s}1 + 2 \mathfrak{s}2) + \\
& \mu_1 (-30 + 19 \mathfrak{s}1 - 19 \mathfrak{s}2 + 3 \mu_2 (16 + 5 \mathfrak{s}1 + 3 \mathfrak{s}2))) + \\
& \eta (-4 \mu_1^2 + \mu_1 (304 - 238 \mu_2) + 50 \times (4 + \mu_2) + \operatorname{er} (-84 + 90 \mathfrak{s}1 + \\
& \mu_1 (-134 + 167 \mathfrak{s}1 + 2 \mu_2 (137 + 45 \mathfrak{s}1 - 9 \mathfrak{s}2) - 145 \mathfrak{s}2) + \\
& \mu_2 (-98 + 90 \mathfrak{s}1 - 90 \mathfrak{s}2) - 90 \mathfrak{s}2 + \mu_1^2 (22 + 5 \mathfrak{s}1 + 17 \mathfrak{s}2))) + \\
& \eta^2 (-100 \mu_1^2 + \mu_1 (476 - 171 \mu_2) + 45 \times (4 + \mu_2) + 3 \operatorname{er} (8 + 30 \\
& \mathfrak{s}1 + \mu_1 (30 + 109 \mathfrak{s}1 + \mu_2 (74 + 30 \mathfrak{s}1 - 78 \mathfrak{s}2) - 79 \mathfrak{s}2) + 2 \mu_2 \\
& (7 + 15 \mathfrak{s}1 - 15 \mathfrak{s}2) - 30 \mathfrak{s}2 + \mu_1^2 (19 \mathfrak{s}1 + 11 \times (2 + \mathfrak{s}2)))) + \\
& 2 \eta^3 (-16 \times (-5 + \mu_1) \mu_1 + \operatorname{er} (60 + 86 \mu_2 + \mu_1^2 (46 + 33 \mathfrak{s}1 + 13 \mathfrak{s}2) + \\
& \mu_1 (226 + 93 \mathfrak{s}1 - 47 \mathfrak{s}2 - 10 \mu_2 (7 + 12 \mathfrak{s}2)))) + \\
& x^5 (-1 + \eta)^5 (-4 \times (-1 + w (-1 + \eta)) \times (-1 + \eta t) \operatorname{er} \mu_1 (5 + w (-1 + \eta) \times \\
& (-5 + \mu_1) - \mu_1 - \eta (1 + \mu_1)) + \\
& \operatorname{er} (2 - 18 \eta + 40 \eta^2 - 24 \eta^3 - 8 \eta t - 16 \eta \eta t + 24 \eta^2 \eta t - 2 \operatorname{er} l +
\end{aligned}$$

$$\begin{aligned}
& 24 \eta \theta l + 2 \eta t \theta l - 24 \eta \eta t \theta l + 44 \mu_1 + 72 \eta \mu_1 - 92 \eta^2 \mu_1 - \\
& 24 \eta^3 \mu_1 - 8 \eta t \mu_1 - 16 \eta \eta t \mu_1 + 24 \eta^2 \eta t \mu_1 - 18 \theta l \mu_1 - \\
& 62 \eta \theta l \mu_1 + 18 \eta t \theta l \mu_1 + 62 \eta \eta t \theta l \mu_1 + 18 \mu_1^2 + \\
& 42 \eta \mu_1^2 - 60 \eta^2 \mu_1^2 - 4 \theta l \mu_1^2 - 14 \eta \theta l \mu_1^2 + 4 \eta t \theta l \mu_1^2 + \\
& 14 \eta \eta t \theta l \mu_1^2 + 4 w^3 (-1 + \eta)^4 (1 + \mu_1) (\eta - \eta t + 4 \mu_1) + \\
& 18 \mu_2 - 18 \eta \mu_2 - 6 \theta l \mu_2 - 2 \eta \theta l \mu_2 + 6 \eta t \theta l \mu_2 + \\
& 2 \eta \eta t \theta l \mu_2 + 6 \mu_1 \mu_2 - 30 \eta \mu_1 \mu_2 + 24 \eta^2 \mu_1 \mu_2 + 12 \eta t \mu_1 \mu_2 - \\
& 12 \eta \eta t \mu_1 \mu_2 - 6 \theta l \mu_1 \mu_2 + 10 \eta \theta l \mu_1 \mu_2 + 6 \eta t \theta l \mu_1 \mu_2 - \\
& 10 \eta \eta t \theta l \mu_1 \mu_2 - 9 \theta l \mu_1 \mathfrak{z}1 - \eta \theta l \mu_1 \mathfrak{z}1 + 9 \eta t \theta l \mu_1 \mathfrak{z}1 + \\
& \eta \eta t \theta l \mu_1 \mathfrak{z}1 - 3 \theta l \mu_1^2 \mathfrak{z}1 - \eta \theta l \mu_1^2 \mathfrak{z}1 + 3 \eta t \theta l \mu_1^2 \mathfrak{z}1 + \\
& \eta \eta t \theta l \mu_1^2 \mathfrak{z}1 + 5 \theta l \mu_1 \mathfrak{z}2 - \eta \theta l \mu_1 \mathfrak{z}2 - 5 \eta t \theta l \mu_1 \mathfrak{z}2 + \\
& \eta \eta t \theta l \mu_1 \mathfrak{z}2 - \theta l \mu_1^2 \mathfrak{z}2 - \eta \theta l \mu_1^2 \mathfrak{z}2 + \eta t \theta l \mu_1^2 \mathfrak{z}2 + \\
& \eta \eta t \theta l \mu_1^2 \mathfrak{z}2 + 12 \theta l \mu_1 \mu_2 \mathfrak{z}2 - 12 \eta t \theta l \mu_1 \mu_2 \mathfrak{z}2 - \\
& w^2 (-1 + \eta)^2 (-10 + 10 \theta l - 84 \mu_1 + 26 \theta l \mu_1 - 50 \mu_1^2 + 4 \theta l \mu_1^2 + \\
& 12 \eta^3 (1 + \mu_1) - 22 \mu_2 + 10 \theta l \mu_2 + 14 \mu_1 \mu_2 - 14 \theta l \mu_1 \mu_2 + \\
& 4 \eta^2 (1 + 13 \mu_1 + 12 \mu_1^2 - 3 \eta t (1 + \mu_1) - 3 \mu_1 \mu_2) + \\
& 2 \eta (-3 + 10 \mu_1 + \mu_1^2 + 11 \mu_2 - \mu_1 \mu_2 + \eta t (-2 - 2 \mu_1 + 6 \mu_1 \mu_2)) + \\
& 9 \theta l \mu_1 \mathfrak{z}1 + 3 \theta l \mu_1^2 \mathfrak{z}1 - 5 \theta l \mu_1 \mathfrak{z}2 + \theta l \mu_1^2 \mathfrak{z}2 - 12 \theta l \mu_1 \mu_2 \mathfrak{z}2 - \\
& \eta t (-16 + 10 \theta l (1 + \mu_2) + 4 \mu_1 (-4 + 3 \mu_2) + \theta l \mu_1^2 (4 + 3 \mathfrak{z}1 + \mathfrak{z}2) + \\
& \theta l \mu_1 (26 + 9 \mathfrak{z}1 - 5 \mathfrak{z}2 - 2 \mu_2 (7 + 6 \mathfrak{z}2))) + w (-1 + \eta) \times \\
& (36 \eta^3 (1 + \mu_1) - 4 \eta^2 (4 - 27 \mu_1^2 + 9 \eta t (1 + \mu_1) + \mu_1 (-41 + 9 \mu_2)) + \\
& \eta (-8 + 40 \mu_2 + 2 \theta l \mu_2 + \mu_1^2 (-56 + \theta l (14 + \mathfrak{z}1 + \mathfrak{z}2)) + \\
& \mu_1 (-88 + 28 \mu_2 + \theta l (86 - 10 \mu_2 + \mathfrak{z}1 + \mathfrak{z}2)) - \\
& \eta t (-8 \mu_1 (2 + 3 \mu_2) + 2 \times (-8 + \theta l \mu_2) + \\
& \theta l \mu_1^2 (14 + \mathfrak{z}1 + \mathfrak{z}2) + \theta l \mu_1 (86 - 10 \mu_2 + \mathfrak{z}1 + \mathfrak{z}2))) - \\
& 2 \times (6 + 56 \mu_1 + 26 \mu_1^2 + 20 \mu_2 - 4 \mu_1 \mu_2 - \theta l (6 + 8 \mu_2 + \\
& \mu_1^2 (4 + 3 \mathfrak{z}1 + \mathfrak{z}2) + \mu_1 (22 + 9 \mathfrak{z}1 - 5 \mathfrak{z}2 - 4 \mu_2 (1 + 3 \mathfrak{z}2))) + \\
& \eta t (2 \times (-5 + \mu_1 (-5 + 6 \mu_2)) + \theta l (6 + 8 \mu_2 + \mu_1^2 (4 + 3 \mathfrak{z}1 + \mathfrak{z}2) + \\
& \mu_1 (22 + 9 \mathfrak{z}1 - 5 \mathfrak{z}2 - 4 \mu_2 (1 + 3 \mathfrak{z}2)))))) - \\
& \times (-1 + \eta) \times (4 w^2 (3 - 5 w + 2 w^2) \eta^9 \theta p (1 + \mu_1) - 4 w \eta^8 \theta p (9 \times (1 + \mu_1) + \\
& w^3 (7 - \mu_1 - 8 \mu_1^2 + 2 \eta t (1 + \mu_1) + 9 \mu_1 \mu_2) + \\
& w (-11 - 23 \mu_1 - 12 \mu_1^2 + 3 \eta t (1 + \mu_1) + 15 \mu_1 \mu_2) - \\
& w^2 (6 - 14 \mu_1 - 20 \mu_1^2 + 5 \eta t (1 + \mu_1) + 24 \mu_1 \mu_2)) - \\
& (1 + w)^3 (5 w \theta l (1 + \mu_1) \mu_2 - 5 w \eta t \theta l (1 + \mu_1) \mu_2 + \\
& \eta t \theta p (2 \mu_1^2 + 2 w (7 \mu_1^2 + 5 \mu_1 (-2 + \mu_2) + 5 \times (-1 + \mu_2)) - \\
& 5 \times (2 + \mu_2) + \mu_1 (-8 + 19 \mu_2))) + 2 \eta^7 \theta p \\
& (12 \times (1 + \mu_1) + 2 w (-7 - 52 \mu_1 - 27 \mu_1^2 + 9 \eta t (1 + \mu_1) + 45 \mu_1 \mu_2) - \\
& 2 w^3 (6 - 16 \mu_1 - 34 \mu_1^2 + 44 \mu_2 + 23 \mu_1 \mu_2 + 6 \eta t (1 + \mu_1 + 4 \mu_1 \mu_2)) + \\
& w^4 (27 - 32 \mu_1 - 59 \mu_1^2 + 33 \mu_2 + 57 \mu_1 \mu_2 + 2 \eta t (7 + 7 \mu_1 + 9 \mu_1 \mu_2)) + \\
& w^2 (-17 + 96 \mu_1 + 53 \mu_1^2 + 55 \mu_2 - 113 \mu_1 \mu_2 + \\
& \eta t (-22 - 22 \mu_1 + 30 \mu_1 \mu_2))) + \\
& \eta^2 (\theta p (-60 + (12 - 56 \eta t) \mu_1^2 - 28 \mu_2 + 7 \eta t \mu_2 - \mu_1 (48 - 88 \eta t + 76 \mu_2 + \\
& 41 \eta t \mu_2) - 2 w (3 \eta t (26 + 14 \mu_1 + 8 \mu_1^2 + 5 \mu_2 - 11 \mu_1 \mu_2) + \\
& 2 \times (34 + 59 \mu_1 + 7 \mu_1^2 + 52 \mu_2 + 10 \mu_1 \mu_2))) +
\end{aligned}$$



$$\begin{aligned}
& 2 w^4 (33 + 42 \mu_1 + 9 \mu_1^2 + 77 \mu_2 + 83 \mu_1 \mu_2 + \eta t \\
& \quad (-4 - 4 \mu_1 + 90 \mu_1^2 - 25 \mu_2 + 17 \mu_1 \mu_2)) + \\
& 2 w^2 (-19 - 106 \mu_1 - 51 \mu_1^2 - 99 \mu_2 + 123 \mu_1 \mu_2 + 3 \eta t \\
& \quad (-54 - 100 \mu_1 + 44 \mu_1^2 - 17 \mu_2 + 49 \mu_1 \mu_2)) + \\
& w^3 (8 \times (16 + 14 \mu_1 - 5 \mu_1^2 + 18 \mu_2 + 42 \mu_1 \mu_2) + \eta t \\
& \quad (-180 - 440 \mu_1 + 436 \mu_1^2 - 115 \mu_2 + 221 \mu_1 \mu_2)) + \\
& (-1 + \eta t) \, \text{el} (w^3 (60 + 100 \mu_1^2 + \mu_1 (76 - 49 \mu_2) - 25 \mu_2) + \\
& \quad w^4 (30 + 60 \mu_1 + 54 \mu_1^2 - 5 \mu_2 - 5 \mu_1 \mu_2) - \\
& \quad 2 \times (7 \mu_1^2 + \mu_1 (16 - 19 \mu_2) + 5 \times (3 + \mu_2)) - \\
& \quad 4 w (15 + 27 \mu_1 + 9 \mu_1^2 + 5 \mu_2 - 13 \mu_1 \mu_2 + \text{ep} \\
& \quad (-11 + 15 \, \text{el} + \mu_1 (-19 + 32 \, \text{el} + \mu_2 (47 + 15 \, \text{el} - 9 \, \text{el}2) - 27 \, \text{el}2) + \\
& \quad \mu_2 (-13 + 15 \, \text{el} - 15 \, \text{el}2) - 15 \, \text{el}2 + \mu_1^2 (4 + 2 \, \text{el} + 3 \, \text{el}2))) - \\
& \text{ep} (\mu_2 (-46 + 30 \, \text{el} - 30 \, \text{el}2) + 30 \times (-1 + \, \text{el} - \, \text{el}2) + \\
& \quad \mu_1^2 (8 + \, \text{el} + 7 \, \text{el}2) + \mu_1 (-58 + 49 \, \text{el} - 41 \, \text{el}2 + 2 \mu_2 (61 + 15 \, \text{el} + \\
& \quad 3 \, \text{el}2))) - w^2 (6 \times (-4 \mu_1^2 + 5 \mu_2 + 5 \mu_1 (2 + \mu_2)) + \\
& \quad \text{ep} (\mu_1 (26 + 79 \, \text{el} + \mu_2 (26 + 30 \, \text{el} - 42 \, \text{el}2) - 67 \, \text{el}2) + \\
& \quad 2 \times (1 + \mu_2) \times (1 + 15 \, \text{el} - 15 \, \text{el}2) + \mu_1^2 (12 + 7 \, \text{el} + 5 \, \text{el}2)))) - \\
& \eta (\text{ep} (\eta t (-50 - 56 \mu_1 + 18 \mu_1^2 - 15 \mu_2 + 57 \mu_1 \mu_2) + 2 w^3 \\
& \quad (\eta t (14 + 6 \mu_1 + 10 \mu_1^2 - 49 \mu_2 - \mu_1 \mu_2) + \\
& \quad 2 \times (20 + 31 \mu_1 + 5 \mu_1^2 + 30 \mu_2 + 6 \mu_1 \mu_2)) + \\
& \quad w^4 (4 \times (5 + 8 \mu_1 + 3 \mu_1^2 + 11 \mu_2 + 5 \mu_1 \mu_2) - 2 \eta t \\
& \quad (-13 - 28 \mu_1 + 3 \mu_1^2 + 20 \mu_2 + 8 \mu_1 \mu_2)) + 4 w (-2 \times (1 + \mu_1) \times \\
& \quad (-5 + \mu_1 - 3 \mu_2) + \eta t (-30 - 52 \mu_1 + 17 \mu_1^2 - 12 \mu_2 + 36 \mu_1 \mu_2)) + \\
& \quad w^2 (4 \times (23 + 29 \mu_1 + 25 \mu_2 + 7 \mu_1 \mu_2) + \eta t (-68 - 196 \mu_1 + \\
& \quad 76 \mu_1^2 - 91 \mu_2 + 101 \mu_1 \mu_2))) + (-1 + \eta t) \, \text{el} \\
& (10 + 8 \mu_1 - 2 \mu_1^2 + 5 \mu_2 - 19 \mu_1 \mu_2 + 10 w^4 (1 + \mu_1) \times (1 + \mu_1 + \mu_2) + \\
& \quad 2 w^3 (14 \mu_1^2 + 5 \times (4 + \mu_2 (2 + \text{ep} (\, \text{el} - \, \text{el}2)) + \text{ep} (\, \text{el} - \, \text{el}2)) + \\
& \quad \mu_1 (34 + \mu_2 (-2 + 5 \text{ep} (\, \text{el} - \, \text{el}2)) + 11 \text{ep} (\, \text{el} - \, \text{el}2))) - \\
& \quad 2 \text{ep} \mu_1^2 (-2 + \, \text{el} - \, \text{el}2) + 10 \text{ep} (1 + \mu_2) \times (-2 + \, \text{el} - \, \text{el}2) + \\
& \quad 2 \text{ep} \mu_1 (5 \mu_2 \, \text{el} + 4 \times (-2 + \, \text{el} - \, \text{el}2) + 7 \mu_2 (2 + \, \text{el}2) + \\
& \quad w^2 (3 \times (8 \mu_1^2 + \mu_1 (28 - 19 \mu_2) + 5 \times (4 + \mu_2)) - \\
& \quad 2 \text{ep} (-((1 + \mu_2) \times (-14 + 15 \, \text{el} - 15 \, \text{el}2)) + \mu_1^2 (\, \text{el} - \, \text{el}2) + \\
& \quad 26 \mu_1 (1 - \, \text{el} + \, \text{el}2) + \mu_1 \mu_2 (-34 - 15 \, \text{el} + 3 \, \text{el}2))) + \\
& \quad w (40 + 44 \mu_1 + 4 \mu_1^2 + 10 \mu_2 - 62 \mu_1 \mu_2 + \text{ep} (6 \mu_2 (-8 + 5 \, \text{el} - \\
& \quad 5 \, \text{el}2) + 10 \times (-4 + 3 \, \text{el} - 3 \, \text{el}2) + \mu_1^2 (4 - 4 \, \text{el} + 4 \, \text{el}2) + \\
& \quad 2 \mu_1 (-30 + 19 \, \text{el} - 19 \, \text{el}2 + 3 \mu_2 (16 + 5 \, \text{el} + 3 \, \text{el}2)))) + \\
& \eta^4 (78 \text{ep} + 24 \eta t \text{ep} + 10 \, \text{el} \text{ep} - 10 \eta t \, \text{el} \text{ep} + 20 \, \text{el} \mu_1 - 20 \eta t \, \text{el} \mu_1 - \\
& \quad 68 \text{ep} \mu_1 - 56 \eta t \text{ep} \mu_1 + 98 \, \text{el} \text{ep} \mu_1 - 98 \eta t \, \text{el} \text{ep} \mu_1 - \\
& \quad 4 \, \text{el} \mu_1^2 + 4 \eta t \, \text{el} \mu_1^2 - 74 \text{ep} \mu_1^2 + 16 \eta t \text{ep} \mu_1^2 + \\
& \quad 28 \, \text{el} \text{ep} \mu_1^2 - 28 \eta t \, \text{el} \text{ep} \mu_1^2 + 46 \text{ep} \mu_2 - 16 \eta t \text{ep} \mu_2 + \\
& \quad 38 \, \text{el} \text{ep} \mu_2 - 38 \eta t \, \text{el} \text{ep} \mu_2 + 154 \text{ep} \mu_1 \mu_2 + \\
& \quad 68 \eta t \text{ep} \mu_1 \mu_2 - 10 \, \text{el} \text{ep} \mu_1 \mu_2 + 10 \eta t \, \text{el} \text{ep} \mu_1 \mu_2 + \\
& \quad w^4 ((-1 + \eta t) \, \text{el} (124 \mu_1^2 - 5 \times (4 + \mu_2) - 5 \mu_1 (8 + \mu_2)) +
\end{aligned}$$

$$\begin{aligned}
& 2 \, \theta p \left( -2 \times \left( 22 + 57 \, \mu_1 + 35 \, \mu_1^2 + 55 \, \mu_2 - 170 \, \mu_1 \mu_2 \right) + \right. \\
& \quad \left. 5 \, \eta t \left( -11 - 26 \, \mu_1 + 57 \, \mu_1^2 + 5 \, \mu_2 - 7 \, \mu_1 \mu_2 \right) \right) + 49 \, \theta l \, \theta p \, \mu_1 \, \mathfrak{x}1 - \\
& 49 \, \eta t \, \theta l \, \theta p \, \mu_1 \, \mathfrak{x}1 + 19 \, \theta l \, \theta p \, \mu_1^2 \, \mathfrak{x}1 - 19 \, \eta t \, \theta l \, \theta p \, \mu_1^2 \, \mathfrak{x}1 - \\
& w^3 \left( \theta p \left( 8 \times \left( 47 - 2 \, \mu_1^2 + \mu_1 \left( 63 - 58 \, \mu_2 \right) + 104 \, \mu_2 \right) + \right. \right. \\
& \quad \left. \left. \eta t \left( 44 - 236 \, \mu_1^2 - 145 \, \mu_2 + \mu_1 \left( 24 + 455 \, \mu_2 \right) \right) \right) - (-1 + \eta t) \, \theta l \right. \\
& \quad \left( 64 \, \mu_1^2 + \mu_1 \left( -160 + \mu_2 \left( 53 - 20 \, \theta p \left( \mathfrak{x}1 - \mathfrak{x}2 \right) \right) - 44 \, \theta p \left( \mathfrak{x}1 - \mathfrak{x}2 \right) \right) - \right. \\
& \quad \left. 5 \times \left( 16 - \mu_2 + 4 \, \theta p \left( \mathfrak{x}1 - \mathfrak{x}2 \right) + 4 \, \theta p \, \mu_2 \left( \mathfrak{x}1 - \mathfrak{x}2 \right) \right) \right) - \\
& 21 \, \theta l \, \theta p \, \mu_1 \, \mathfrak{x}2 + 21 \, \eta t \, \theta l \, \theta p \, \mu_1 \, \mathfrak{x}2 + 9 \, \theta l \, \theta p \, \mu_1^2 \, \mathfrak{x}2 - 9 \, \eta t \, \theta l \\
& \quad \theta p \, \mu_1^2 \, \mathfrak{x}2 - 60 \, \theta l \, \theta p \, \mu_1 \, \mu_2 \, \mathfrak{x}2 + 60 \, \eta t \, \theta l \, \theta p \, \mu_1 \, \mu_2 \, \mathfrak{x}2 + \\
& w \left( \theta p \left( 4 \times \left( 49 + 16 \, \mu_1^2 + \mu_1 \left( 107 - 68 \, \mu_2 \right) + 130 \, \mu_2 \right) + \right. \right. \\
& \quad \left. \left. \eta t \left( 128 - 132 \, \mu_1^2 + 17 \, \mu_2 + \mu_1 \left( 116 + 161 \, \mu_2 \right) \right) \right) + \right. \\
& \quad \left( -1 + \eta t \right) \, \theta l \left( 60 + 120 \, \mu_1 + 15 \, \mu_2 - 57 \, \mu_1 \, \mu_2 + \theta p \left( -44 + 60 \, \mathfrak{x}1 + \right. \right. \\
& \quad \left. \left. \mu_1 \left( -170 + 123 \, \mathfrak{x}1 + \mu_2 \left( 238 + 60 \, \mathfrak{x}1 - 36 \, \mathfrak{x}2 \right) - 113 \, \mathfrak{x}2 \right) + \right. \right. \\
& \quad \left. \left. \mu_2 \left( -62 + 60 \, \mathfrak{x}1 - 60 \, \mathfrak{x}2 \right) - 60 \, \mathfrak{x}2 + \mu_1^2 \left( -6 + 3 \, \mathfrak{x}1 + 7 \, \mathfrak{x}2 \right) \right) \right) \right) + \\
& w^2 \left( - \left( (-1 + \eta t) \, \theta l \left( 44 \, \mu_1^2 - 15 \, \mu_2 - \mu_1 \left( 64 + 15 \, \mu_2 \right) \right) \right) + \right. \\
& \quad \left. \theta p \left( -48 + 500 \, \mu_1 + 356 \, \mu_1^2 + 56 \, \mu_2 - 832 \, \mu_1 \, \mu_2 - \right. \right. \\
& \quad \left. \left. 2 \, \theta l \left( \mu_1 \left( 78 + 62 \, \mathfrak{x}1 + \mu_2 \left( -22 + 15 \, \mathfrak{x}1 - 51 \, \mathfrak{x}2 \right) - 46 \, \mathfrak{x}2 \right) + \right. \right. \right. \\
& \quad \left. \left. \left( 1 + \mu_2 \right) \times \left( 26 + 15 \, \mathfrak{x}1 - 15 \, \mathfrak{x}2 \right) + \mu_1^2 \left( 16 + 11 \, \mathfrak{x}1 + 5 \, \mathfrak{x}2 \right) \right) + \right. \\
& \quad \left. \left. \eta t \left( 192 + 556 \, \mu_1 - 440 \, \mu_1^2 + 149 \, \mu_2 - 331 \, \mu_1 \, \mu_2 + 2 \, \theta l \left( \mu_1 \left( 78 + \right. \right. \right. \right. \right. \\
& \quad \left. \left. \left. 62 \, \mathfrak{x}1 + \mu_2 \left( -22 + 15 \, \mathfrak{x}1 - 51 \, \mathfrak{x}2 \right) - 46 \, \mathfrak{x}2 \right) + \left( 1 + \mu_2 \right) \times \right. \right. \right. \\
& \quad \left. \left. \left. \left( 26 + 15 \, \mathfrak{x}1 - 15 \, \mathfrak{x}2 \right) + \mu_1^2 \left( 16 + 11 \, \mathfrak{x}1 + 5 \, \mathfrak{x}2 \right) \right) \right) \right) \right) \right) + \\
& \eta^3 \left( \theta p \left( -4 \times \left( 11 + 7 \, \mu_1^2 + \mu_1 \left( 30 - 17 \, \mu_2 \right) + 31 \, \mu_2 \right) + \eta t \left( 44 \, \mu_1^2 - \right. \right. \right. \\
& \quad \left. \left. 11 \times \left( 4 + \mu_2 \right) - \mu_1 \left( 72 + 11 \, \mu_2 \right) \right) - \right. \\
& 4 \, w^3 \left( -40 - 108 \, \mu_1 - 44 \, \mu_1^2 - 112 \, \mu_2 + 203 \, \mu_1 \, \mu_2 + \right. \\
& \quad \left. \eta t \left( -64 - 144 \, \mu_1 + 166 \, \mu_1^2 + 5 \, \mu_2 + 5 \, \mu_1 \, \mu_2 \right) \right) - 2 \, w^4 \left( 21 - 8 \, \mu_1 - 29 \right. \\
& \quad \left. \mu_1^2 + 55 \, \mu_2 + 247 \, \mu_1 \, \mu_2 + \eta t \left( -44 - 94 \, \mu_1 + 250 \, \mu_1^2 + 30 \, \mu_1 \, \mu_2 \right) \right) + \\
& 4 \, w \left( -2 \times \left( -14 + 15 \, \mu_1 + 17 \, \mu_1^2 + \mu_2 - 59 \, \mu_1 \, \mu_2 \right) + \right. \\
& \quad \left. \eta t \left( -30 - 104 \, \mu_1 + 79 \, \mu_1^2 - 18 \, \mu_2 + 54 \, \mu_1 \, \mu_2 \right) \right) + \\
& 2 \, w^2 \left( 171 + 232 \, \mu_1 + \mu_1^2 + 337 \, \mu_2 + 7 \, \mu_1 \, \mu_2 + \eta t \right. \\
& \quad \left. \left( 42 - 16 \, \mu_1 + 56 \, \mu_1^2 - 37 \, \mu_2 + 137 \, \mu_1 \, \mu_2 \right) \right) - (-1 + \eta t) \, \theta l \\
& \left( 20 + 56 \, \mu_1 + 4 \, w^4 \left( 5 + 29 \, \mu_1^2 - 5 \, \mu_1 \left( -2 + \mu_2 \right) - 5 \, \mu_2 \right) + 5 \, \mu_2 - \right. \\
& 19 \, \mu_1 \, \mu_2 + \theta p \left( \mu_1 \left( -14 + 85 \, \mathfrak{x}1 + 2 \, \mu_2 \left( 67 + 10 \, \mathfrak{x}1 - 34 \, \mathfrak{x}2 \right) - 59 \, \mathfrak{x}2 \right) + \right. \\
& \quad \left. \mu_1^2 \left( 10 + 17 \, \mathfrak{x}1 + 9 \, \mathfrak{x}2 \right) + 2 \times \left( 12 + \mu_2 + 10 \, \mathfrak{x}1 + 10 \, \mu_2 \, \mathfrak{x}1 - 10 \, \mathfrak{x}2 - \right. \right. \\
& \quad \left. \left. 10 \, \mu_2 \, \mathfrak{x}2 \right) + 8 \, w^3 \left( 16 \, \mu_1^2 - 5 \times \left( 1 + \mu_2 \right) \times \left( 1 + \theta p \left( \mathfrak{x}1 - \mathfrak{x}2 \right) \right) + \right. \right. \\
& \quad \left. \left. \mu_1 \left( -16 + \mu_2 - 11 \, \theta p \, \mathfrak{x}1 - 5 \, \theta p \, \mu_2 \, \mathfrak{x}1 + 11 \, \theta p \, \mathfrak{x}2 + 5 \, \theta p \, \mu_2 \, \mathfrak{x}2 \right) \right) + \right. \\
& 2 \, w^2 \left( -3 \times \left( 6 \, \mu_1^2 + \mu_1 \left( 36 - 19 \, \mu_2 \right) + 5 \times \left( 4 + \mu_2 \right) \right) + \right. \\
& \quad \left. \theta p \left( - \left( \left( 1 + \mu_2 \right) \times \left( -52 + 45 \, \mathfrak{x}1 - 45 \, \mathfrak{x}2 \right) \right) + \mu_1^2 \left( 4 + 6 \, \mathfrak{x}1 - 2 \, \mathfrak{x}2 \right) - \right. \right. \\
& \quad \left. \left. \mu_1 \left( -104 + 69 \, \mathfrak{x}1 - 73 \, \mathfrak{x}2 + \mu_2 \left( 116 + 45 \, \mathfrak{x}1 + 3 \, \mathfrak{x}2 \right) \right) \right) \right) + \\
& w \left( -48 \, \mu_1^2 - 10 \times \left( 4 + \mu_2 \right) + \mu_1 \left( 8 + 62 \, \mu_2 \right) + \theta p \left( 100 - 30 \, \mathfrak{x}1 - \right. \right. \\
& \quad \left. \left. 6 \, \mu_2 \left( -21 + 5 \, \mathfrak{x}1 - 5 \, \mathfrak{x}2 \right) + 30 \, \mathfrak{x}2 + \mu_1^2 \left( 22 + 33 \, \mathfrak{x}1 + 5 \, \mathfrak{x}2 \right) - \right. \right. \\
& \quad \left. \left. \mu_1 \left( -194 - 51 \, \mathfrak{x}1 + 13 \, \mathfrak{x}2 + 6 \, \mu_2 \left( 21 + 5 \, \mathfrak{x}1 + 23 \, \mathfrak{x}2 \right) \right) \right) \right) \right) + \\
& \eta^5 \left( 4 \times \left( -1 + \eta t \right) \, \theta l \, \mu_1 \left( 1 + \mu_1 \right) - 2 \, w^4 \left( \left( -1 + \eta t \right) \, \theta l \left( 33 \, \mu_1^2 + \right. \right. \right. \\
& \quad \left. \left. 5 \, \mu_1 \left( -6 + \mu_2 \right) + 5 \times \left( -3 + \mu_2 \right) \right) + \right.
\end{aligned}$$

$$\begin{aligned} & \Theta p \left( -20 \times (4 + \mu_1^2 + \mu_1 (5 - 10 \mu_2) + 11 \mu_2) + \eta t \right. \\ & \quad \left. (153 \mu_1^2 + 5 \times (-7 + 4 \mu_2) - 20 \mu_1 (4 + 5 \mu_2)) \right) + \\ & \Theta p \left( 2 \times (5 + 15 \mu_1^2 + \mu_1 (44 - 13 \mu_2) + 53 \mu_2) + 4 \eta t (-4 + 4 \mu_1^2 + \right. \\ & \quad 15 \mu_1 \mu_2) + \Theta l (-24 + 10 \mu_2 + 5 \mu_1 (14 - 10 \mu_2 + \Xi_1 + \Xi_2) + \\ & \quad \mu_1^2 (22 + 5 \Xi_1 + 5 \Xi_2)) - \eta t \Theta l (-24 + 10 \mu_2 + \\ & \quad 5 \mu_1 (14 - 10 \mu_2 + \Xi_1 + \Xi_2) + \mu_1^2 (22 + 5 \Xi_1 + 5 \Xi_2)) \Big) - \\ & 2 w^3 \left( 2 \times (-1 + \eta t) \Theta l (\mu_1^2 - \mu_1 (-7 + \mu_2) + 5 \mu_2) + \Theta p \right. \\ & \quad (-62 + 162 \mu_1^2 - 84 \mu_2 - 15 \Theta l \Xi_1 - 15 \Theta l \mu_2 \Xi_1 + \\ & \quad \mu_1 (112 - 3 \mu_2 (64 + 5 \Theta l (\Xi_1 - \Xi_2)) - 33 \Theta l (\Xi_1 - \Xi_2)) + \\ & \quad 15 \Theta l \Xi_2 + 15 \Theta l \mu_2 \Xi_2 + \eta t (22 - 70 \mu_1^2 + 15 \Theta l \Xi_1 + \\ & \quad 5 \mu_2 (11 + 3 \Theta l (\Xi_1 - \Xi_2)) + \mu_1 (126 + \mu_2 (-137 + \\ & \quad 15 \Theta l (\Xi_1 - \Xi_2)) + 33 \Theta l (\Xi_1 - \Xi_2)) - 15 \Theta l \Xi_2) \Big) \Big) + \\ & w^2 \left( 3 \Theta p (-4 \times (19 + 9 \mu_1^2 + \mu_1 (46 - 36 \mu_2) + 61 \mu_2) + \eta t \right. \\ & \quad (-36 + 52 \mu_1^2 - 11 \mu_2 - \mu_1 (56 + 83 \mu_2)) \Big) + \\ & \quad (-1 + \eta t) \Theta l (4 \mu_1^2 - 15 \times (4 + \mu_2) + \mu_1 (-116 + 57 \mu_2) + \\ & \quad 2 \Theta p (-2 \times (1 + \mu_2) \times (-19 + 15 \Xi_1 - 15 \Xi_2) + \mu_1^2 (4 + 5 \Xi_1 - \Xi_2) - \\ & \quad \mu_1 (-78 + 43 \Xi_1 - 47 \Xi_2 + \mu_2 (82 + 30 \Xi_1 + 6 \Xi_2))) \Big) \Big) + \\ & w \left( -4 \times (-1 + \eta t) \Theta l (-11 + \mu_1) \mu_1 + \Theta p (4 \times (-21 + 61 \mu_1^2 + \right. \\ & \quad \mu_1 (82 - 103 \mu_2) - 16 \mu_2) - \Theta l (60 + 78 \mu_2 + \mu_1^2 (26 + 29 \Xi_1 + \\ & \quad 9 \Xi_2) + \mu_1 (134 + 89 \Xi_1 - 51 \Xi_2 - 30 \mu_2 (1 + 4 \Xi_2))) \Big) + \\ & \quad \eta t (-4 \times (19 + 8 \mu_1^2 - 8 \mu_2 + 7 \mu_1 (-3 + 4 \mu_2)) + \\ & \quad \Theta l (60 + 78 \mu_2 + \mu_1^2 (26 + 29 \Xi_1 + 9 \Xi_2) + \\ & \quad \mu_1 (134 + 89 \Xi_1 - 51 \Xi_2 - 30 \mu_2 (1 + 4 \Xi_2)))) \Big) \Big) + \\ & \eta^6 \left( -4 \Theta p (2 - 15 \mu_1^2 + 6 \eta t (1 + \mu_1) + \mu_1 (-31 + 30 \mu_2)) + \right. \\ & \quad w^4 ((-1 + \eta t) \Theta l (14 \mu_1^2 + 5 \mu_1 (-4 + \mu_2) + 5 \times (-2 + \mu_2)) + \\ & \quad 2 \Theta p (-55 + 6 \mu_1 + 61 \mu_1^2 - 143 \mu_2 - 5 \mu_1 \mu_2 + \\ & \quad \eta t (-22 - 32 \mu_1 + 32 \mu_1^2 + 5 \mu_2 - 73 \mu_1 \mu_2)) \Big) + \\ & \quad w^3 (\Theta p (8 \times (8 + 17 \mu_1^2 + \mu_1 (40 - 44 \mu_2) + 46 \mu_2) + \eta t \\ & \quad (4 - 84 \mu_1^2 + 27 \mu_2 + \mu_1 (88 + 123 \mu_2))) - (-1 + \eta t) \Theta l \\ & \quad (4 \mu_1^2 + \mu_1 (-52 + \mu_2 (19 - 20 \Theta p (\Xi_1 - \Xi_2)) - 44 \Theta p (\Xi_1 - \Xi_2)) - \\ & \quad 5 \times (4 + \mu_2 + 4 \Theta p (\Xi_1 - \Xi_2) + 4 \Theta p \mu_2 (\Xi_1 - \Xi_2))) \Big) + \\ & \quad w (-4 \times (-1 + \eta t) \Theta l \mu_1 (1 + \mu_1) + \Theta p (16 - 2 \times (108 + 5 \Theta l) \mu_2 + \\ & \quad \mu_1 (-124 + 96 \mu_2 + \Theta l (-94 + 50 \mu_2 - 5 \Xi_1 - 5 \Xi_2)) - \\ & \quad \mu_1^2 (44 + \Theta l (22 + 5 \Xi_1 + 5 \Xi_2)) + \\ & \quad \eta t (28 + 10 \Theta l \mu_2 + \mu_1^2 (-16 + \Theta l (22 + 5 \Xi_1 + 5 \Xi_2)) + \\ & \quad \mu_1 (12 - 120 \mu_2 + \Theta l (94 - 50 \mu_2 + 5 \Xi_1 + 5 \Xi_2))) \Big) \Big) + \\ & \quad w^2 (4 \times (-1 + \eta t) \Theta l (-5 + \mu_1) \mu_1 + \Theta p (42 - 380 \mu_1 - 302 \mu_1^2 + \\ & \quad 190 \mu_2 + 454 \mu_1 \mu_2 + 5 \Theta l (10 \times (1 + \mu_2) + \mu_1^2 (4 + 3 \Xi_1 + \Xi_2) + \\ & \quad \mu_1 (26 + 9 \Xi_1 - 5 \Xi_2 - 2 \mu_2 (7 + 6 \Xi_2))) \Big) + \\ & \quad \eta t (4 \times (21 + 8 \mu_1^2 - 4 \mu_2 + 5 \mu_1 (1 + 7 \mu_2)) - \\ & \quad 5 \Theta l (10 \times (1 + \mu_2) + \mu_1^2 (4 + 3 \Xi_1 + \Xi_2) + \\ & \quad \mu_1 (26 + 9 \Xi_1 - 5 \Xi_2 - 2 \mu_2 (7 + 6 \Xi_2)))))) \Big) \Big) / \end{aligned}$$

$$\begin{aligned} & (96 (-1+w (-1+\eta))^3 (x (-1+\eta) - \eta)^3 (1+x+\eta-x\eta)^2 \\ & (w + \\ & x + \\ & \eta - \\ & w \\ & \eta - x \\ & \eta)^3 (-1+\eta t) \theta l \theta p) \end{aligned}$$

$$\beta \eta =$$

$$\begin{aligned} & ((-1+\eta) \eta (c\sigma^2 (-1+\eta) \times (-5x-4x^2-5\eta-3x\eta+8x^2\eta-4\eta^2+8x\eta^2-4x^2\eta^2-4x\mu_1+2 \\ & x^2\mu_1-4\eta\mu_1+8x\eta\mu_1-3x^2\eta\mu_1+2\eta^2\mu_1-2x\eta^2\mu_1+\eta^3\mu_1-2x\eta^3\mu_1+ \\ & x^2\eta^3\mu_1+x\mu_1^2-3x^2\mu_1^2+\eta\mu_1^2-7x\eta\mu_1^2+7x^2\eta\mu_1^2-3\eta^2\mu_1^2+ \\ & 8x\eta^2\mu_1^2-5x^2\eta^2\mu_1^2+\eta^3\mu_1^2-2x\eta^3\mu_1^2+x^2\eta^3\mu_1^2-2x\mu_2-\eta\mu_2+ \\ & 2x\eta\mu_2-8x\mu_1\mu_2-13\eta\mu_1\mu_2+8x\eta\mu_1\mu_2+9w^3(-1+\eta)^3(1+2\mu_1\mu_2)+ \\ & w(-1+\eta) \times (5+x^2(-1+\eta)^2(-2+\mu_1)^2+4\mu_1-\mu_1^2-\eta^2(-4+6\mu_1+\mu_1^2)+ \\ & 18\mu_1\mu_2+2x(-1+\eta) \times (-9-2\mu_1-2\mu_1^2+\eta(-4+5\mu_1)-2\mu_2-8\mu_1\mu_2)+ \\ & 2\eta(9+2\mu_1+2\mu_1^2+\mu_2+13\mu_1\mu_2)) + w^2(-1+\eta)^2(-14-6\mu_1-\mu_1^2-36\mu_1\mu_2- \\ & \eta(13-5\mu_1+\mu_2+13\mu_1\mu_2)+x(-1+\eta) \times (13+\mu_1^2+2\mu_2+\mu_1(-4+8\mu_2))) - \\ & (-1+w(-1+\eta))^2(w+x+\eta-w\eta-x\eta)^2(24+f\theta l(-4+\mathfrak{E}2))) / \\ & (12(-1+w(-1+\eta))^2(w(-1+\eta)+x(-1+\eta)-\eta)^2) \end{aligned}$$

$$\beta \eta t =$$

$$\begin{aligned} & \frac{1}{24} \eta t \left( (2c\sigma^2(-1+\eta)^2(x(w(-1+\eta)-2\eta)(-1+\eta)\theta p(4+2\mu_1+7\mu_1^2)+x^2(-1+\eta)^2\theta p \right. \\ & (4+2\mu_1+7\mu_1^2)+\eta^2\theta p(4+2\mu_1+7\mu_1^2)+ \\ & x(-1+w(-1+\eta)) \times (-1+\eta t) \theta l(5-2\mu_1+11\mu_1^2)+\eta t \theta p(5-2\mu_1+11\mu_1^2)- \\ & w(-1+\eta) \theta p(\eta(4+2\mu_1+7\mu_1^2)+\eta t(5-2\mu_1+11\mu_1^2))) / \\ & ((-1+w(-1+\eta))(x(-1+\eta)-\eta)(w(-1+\eta)+x(-1+\eta)-\eta)\theta p) + \\ & (-1+\eta t) \times (-48+f\theta l^2(8-4\mathfrak{E}2+5\mathfrak{E}2^2))) \end{aligned}$$

$$\beta r = \frac{9u}{2} - \frac{1}{4} r (-8+cv^2+18u) +$$

$$\begin{aligned} & (f(-1+\eta) \times (36(1+w-w\eta)^2(x+\eta-x\eta)^2(w+x+\eta-w\eta-x\eta)^2 \\ & (-4x^2(-1+\eta)^2(-1+\eta+\theta l-\eta t \theta l) \theta p + \theta p(-4\eta^3+2\eta t+4\eta^2(1+(-1+\eta t) \theta l) + \\ & \eta(-\theta l(2+\mathfrak{E}1+\mathfrak{E}2)+\eta t(-2+\theta l(2+\mathfrak{E}1+\mathfrak{E}2))) + w(-1+\eta) \times \\ & (4\eta^2-2\eta t+\eta(-4+2\eta t+\theta l(6+\mathfrak{E}1+\mathfrak{E}2)-\eta t \theta l(6+\mathfrak{E}1+\mathfrak{E}2)))) + \\ & x(-1+\eta) \times (-4(w(-1+\eta)-2\eta)(-1+\eta) \theta p + (-1+\eta t) \theta l \\ & (2-\theta p(2+8\eta+\mathfrak{E}1+\mathfrak{E}2)+w(-1+\eta) \times (-2+\theta p(6+\mathfrak{E}1+\mathfrak{E}2)))) + \\ & r(2w^5(-1+\eta)^5(2x^3(-1+\eta)^3((-1+\eta) \times (28+10\eta^2+\eta(11-10\eta t)-11\eta t) \\ & \theta p - (-1+\eta t) \theta l(-26+9\theta p(6+\mathfrak{E}1+\mathfrak{E}2))) - \\ & 3x^2(-1+\eta)^2(20\eta^4\theta p + \eta^3(2-20\eta t) \theta p - 2\eta^2(-17+\eta t) \theta p - 15\eta t \theta p + \\ & \eta(-56+37\eta t) \theta p - \eta(-1+\eta t) \theta l(-37+18\theta p(6+\mathfrak{E}1+\mathfrak{E}2))) + \\ & x(-1+\eta) \eta(60\eta^4\theta p + \eta^3(6-60\eta t) \theta p - 6\eta^2(-17+\eta t) \theta p - 91\eta t \theta p + \\ & \eta(-168+157\eta t) \theta p - \eta(-1+\eta t) \theta l(-65+54\theta p(6+\mathfrak{E}1+\mathfrak{E}2))) - \\ & 2\eta^2\theta p(10\eta^4+\eta^3(1-10\eta t)-\eta^2(-17+\eta t)-26\eta t+ \\ & \eta(-28+9\theta l(6+\mathfrak{E}1+\mathfrak{E}2)+\eta t(37-9\theta l(6+\mathfrak{E}1+\mathfrak{E}2)))) + \end{aligned}$$

$$\begin{aligned}
& (x + \eta - x \eta)^2 \left( 4 x^4 (-1 + \eta)^4 \operatorname{ep} \left( 12 + 30 \eta^3 - 2 \eta^2 (24 - 5 \operatorname{el} + 5 \eta t (2 + \operatorname{el})) - \right. \right. \\
& \quad 4 \operatorname{el} (3 + 2 \operatorname{el} 2) + \eta (6 + \eta t (29 + \operatorname{el} (9 - 2 \operatorname{el} 2)) + \operatorname{el} (-9 + 2 \operatorname{el} 2)) + \\
& \quad \left. \left. \eta t (-9 + 4 \operatorname{el} (3 + 2 \operatorname{el} 2)) \right) - 4 x^3 (-1 + \eta)^3 \right. \\
& \quad \left( 4 \times (-1 + \eta) \eta (-12 + 30 \eta^2 + 9 \eta t - 2 \eta (9 + 10 \eta t)) \operatorname{ep} - (-1 + \eta t) \operatorname{el} \right. \\
& \quad \left. \left( -10 + \operatorname{ep} (10 + 40 \eta^3 - 3 \operatorname{el} 1 + 5 \operatorname{el} 2 + 4 \eta^2 (-9 + 2 \operatorname{el} 2) - 16 \eta (3 + 2 \operatorname{el} 2)) \right) \right) + \\
& \quad \eta^2 \operatorname{ep} (120 \eta^5 - 42 \eta t - 8 \eta^4 (24 - 5 \operatorname{el} + 5 \eta t (2 + \operatorname{el})) + \\
& \quad 3 \eta (14 \eta t - \operatorname{el} \operatorname{el} 1 + 7 \operatorname{el} (2 + \operatorname{el} 2) + \eta t \operatorname{el} (\operatorname{el} 1 - 7 \times (2 + \operatorname{el} 2))) - \\
& \quad 4 \eta^3 (-6 + \operatorname{el} (9 - 2 \operatorname{el} 2) + \eta t (-29 + \operatorname{el} (-9 + 2 \operatorname{el} 2))) + \\
& \quad \left. 4 \eta^2 (12 - 4 \operatorname{el} (3 + 2 \operatorname{el} 2) + \eta t (-9 + 4 \operatorname{el} (3 + 2 \operatorname{el} 2))) \right) - \\
& \quad 8 x (-1 + \eta) \eta (60 \eta^5 \operatorname{ep} - 7 \eta t \operatorname{ep} - 4 \eta^4 (24 - 5 \operatorname{el} + 5 \eta t (2 + \operatorname{el})) \operatorname{ep} + \\
& \quad 2 \eta^3 \operatorname{ep} (6 + \eta t (29 + \operatorname{el} (9 - 2 \operatorname{el} 2)) + \operatorname{el} (-9 + 2 \operatorname{el} 2)) + \\
& \quad \eta (7 \eta t \operatorname{ep} + (-1 + \eta t) \operatorname{el} (7 + 3 \operatorname{ep} \operatorname{el} 1 - 7 \operatorname{ep} (2 + \operatorname{el} 2))) + \\
& \quad \left. 2 \eta^2 \operatorname{ep} (12 - 4 \operatorname{el} (3 + 2 \operatorname{el} 2) + \eta t (-9 + 4 \operatorname{el} (3 + 2 \operatorname{el} 2))) \right) + \\
& \quad x^2 (-1 + \eta)^2 (720 \eta^5 \operatorname{ep} - 50 \eta t \operatorname{ep} - 48 \eta^4 (24 - 5 \operatorname{el} + 5 \eta t (2 + \operatorname{el})) \operatorname{ep} + \\
& \quad \eta (50 \eta t \operatorname{ep} + (-1 + \eta t) \operatorname{el} (60 + 33 \operatorname{ep} \operatorname{el} 1 - 55 \operatorname{ep} (2 + \operatorname{el} 2))) - \\
& \quad 24 \eta^3 \operatorname{ep} (-6 + \operatorname{el} (9 - 2 \operatorname{el} 2) + \eta t (-29 + \operatorname{el} (-9 + 2 \operatorname{el} 2))) + \\
& \quad \left. 24 \eta^2 \operatorname{ep} (12 - 4 \operatorname{el} (3 + 2 \operatorname{el} 2) + \eta t (-9 + 4 \operatorname{el} (3 + 2 \operatorname{el} 2))) \right) + \\
& \quad 3 w^4 (-1 + \eta)^4 \left( 4 x^4 (-1 + \eta)^4 \left( (-1 + \eta) \times (28 + 10 \eta^2 + \eta (11 - 10 \eta t) - 11 \eta t) \right. \right. \\
& \quad \left. \left. \operatorname{ep} - 4 \times (-1 + \eta t) \operatorname{el} (-2 + 9 \operatorname{ep}) \right) + x^3 (-1 + \eta)^3 \right. \\
& \quad \left( -4 \times (-1 + \eta) \times (-8 + 40 \eta^3 + \eta (123 - 54 \eta t) + \eta^2 (54 - 40 \eta t) + 7 \eta t) \operatorname{ep} + \right. \\
& \quad \left. (-1 + \eta t) \operatorname{el} (-104 - 110 \eta + 36 \operatorname{ep} (2 + \operatorname{el} 1 + \operatorname{el} 2) + 9 \eta \operatorname{ep} (70 + \operatorname{el} 1 + \operatorname{el} 2)) \right) + \\
& \quad \eta^2 \operatorname{ep} (40 \eta^5 + \eta^3 (72 - 44 \eta t) + \eta^4 (44 - 40 \eta t) - 104 \eta t + \\
& \quad \eta (32 + 62 \eta t + 36 \operatorname{el} (2 + \operatorname{el} 1 + \operatorname{el} 2) - 36 \eta t \operatorname{el} (2 + \operatorname{el} 1 + \operatorname{el} 2)) + \\
& \quad \left. \eta^2 (-188 + 9 \operatorname{el} (22 + \operatorname{el} 1 + \operatorname{el} 2) - 9 \eta t (-14 + \operatorname{el} (22 + \operatorname{el} 1 + \operatorname{el} 2))) \right) + \\
& \quad x^2 (-1 + \eta)^2 (240 \eta^5 \operatorname{ep} + 12 \eta^3 (35 - 12 \eta t) \operatorname{ep} - 90 \eta t \operatorname{ep} + 4 \eta (24 + \eta t) \operatorname{ep} - \\
& \quad 48 \eta^4 (-3 + 5 \eta t) \operatorname{ep} - 6 \eta (-1 + \eta t) \operatorname{el} (-37 + 18 \operatorname{ep} (2 + \operatorname{el} 1 + \operatorname{el} 2)) + \\
& \quad \left. \eta^2 (10 \times (-90 + 47 \eta t) \operatorname{ep} - (-1 + \eta t) \operatorname{el} (-136 + 27 \operatorname{ep} (38 + \operatorname{el} 1 + \operatorname{el} 2))) \right) - \\
& \quad x (-1 + \eta) \eta (160 \eta^5 \operatorname{ep} - 182 \eta t \operatorname{ep} - 8 \eta^4 (-17 + 20 \eta t) \operatorname{ep} - 4 \eta^3 (-71 + 34 \eta t) \\
& \quad \operatorname{ep} + 2 \eta (48 + 41 \eta t) \operatorname{ep} - 2 \eta (-1 + \eta t) \operatorname{el} (-65 + 54 \operatorname{ep} (2 + \operatorname{el} 1 + \operatorname{el} 2)) + \eta^2 \\
& \quad \left. (4 \times (-169 + 99 \eta t) \operatorname{ep} - (-1 + \eta t) \operatorname{el} (-58 + 9 \operatorname{ep} (82 + 3 \operatorname{el} 1 + 3 \operatorname{el} 2))) \right) + \\
& \quad w (x (-1 + \eta) - \eta) (-1 + \eta) \times (-4 x^5 (-1 + \eta)^5 \operatorname{ep} (30 \eta^3 + \eta^2 (3 - 30 \eta t) + \\
& \quad 2 \times (12 + \eta t - 6 \operatorname{el} (2 + \operatorname{el} 2) + 6 \eta t \operatorname{el} (2 + \operatorname{el} 2)) + \\
& \quad \eta (-57 + \operatorname{el} (31 + 2 \operatorname{el} 2) + \eta t (28 - \operatorname{el} (31 + 2 \operatorname{el} 2)))) + \\
& \quad \eta^2 \operatorname{ep} (120 \eta^6 + \eta^5 (372 - 120 \eta t) - 134 \eta t + \eta (8 \eta t + 27 \operatorname{el} \operatorname{el} 1 - \\
& \quad 27 \eta t \operatorname{el} \operatorname{el} 1 + 67 \operatorname{el} (2 + \operatorname{el} 2) - 67 \eta t \operatorname{el} (2 + \operatorname{el} 2)) - \\
& \quad 4 \eta^4 (201 - \operatorname{el} (61 + 2 \operatorname{el} 2) + \eta t (32 + \operatorname{el} (61 + 2 \operatorname{el} 2))) + \\
& \quad 4 \eta^3 (42 - 3 \operatorname{el} (17 + 2 \operatorname{el} 2) + \eta t (89 + \operatorname{el} (51 + 6 \operatorname{el} 2))) + \\
& \quad \left. 3 \eta^2 (48 - \operatorname{el} (6 + 3 \operatorname{el} 1 + 11 \operatorname{el} 2) + \eta t (6 + \operatorname{el} (6 + 3 \operatorname{el} 1 + 11 \operatorname{el} 2))) \right) + \\
& \quad 4 x^4 (-1 + \eta)^4 \left( (-1 + \eta) \times (150 \eta^3 + \eta^2 (255 - 150 \eta t) + \right. \\
& \quad 9 \times (-4 + 3 \eta t) - 2 \eta (87 + 35 \eta t)) \operatorname{ep} - (-1 + \eta t) \operatorname{el} \\
& \quad \left. \left( -30 + \operatorname{ep} (5 \eta^2 (37 + 2 \operatorname{el} 2) - 3 \times (2 + 3 \operatorname{el} 1 + 3 \operatorname{el} 2) - 3 \eta (49 + 18 \operatorname{el} 2)) \right) \right) - \\
& \quad x (-1 + \eta) \eta (600 \eta^6 \operatorname{ep} - 190 \eta t \operatorname{ep} - 300 \eta^5 (-5 + 2 \eta t) \operatorname{ep} - \\
& \quad 2 \eta (52 \eta t \operatorname{ep} + (-1 + \eta t) \operatorname{el} (-87 + 27 \operatorname{ep} \operatorname{el} 1 + 91 \operatorname{ep} (2 + \operatorname{el} 2))) - \\
& \quad \left. 4 \eta^4 \operatorname{ep} (861 - 5 \operatorname{el} (55 + 2 \operatorname{el} 2) + 5 \eta t (20 + \operatorname{el} (55 + 2 \operatorname{el} 2))) \right) +
\end{aligned}$$

$$\begin{aligned}
& 8 \eta^3 \theta p (96 - 6 \theta l (19 + 3 \mathfrak{z}2) + \eta t (179 + 6 \theta l (19 + 3 \mathfrak{z}2))) + \\
& 3 \eta^2 (2 \times (96 - 23 \eta t) \theta p + (-1 + \eta t) \theta l (56 + \theta p (38 + 27 \mathfrak{z}1 + 51 \mathfrak{z}2))) - \\
& x^3 (-1 + \eta)^3 (2 \times (-1 + \eta) \times (600 \eta^4 + 75 \eta t + 72 \eta (-4 + 3 \eta t) - \\
& 60 \eta^3 (-23 + 10 \eta t) - 8 \eta^2 (114 + 65 \eta t)) \theta p - \\
& (-1 + \eta t) \theta l (40 \eta^3 \theta p (43 + 2 \mathfrak{z}2) - 48 \eta^2 \theta p (29 + 8 \mathfrak{z}2) + \\
& 48 \times (-2 + \theta p (2 + \mathfrak{z}2)) - 3 \eta (100 + \theta p (42 + 45 \mathfrak{z}1 + 53 \mathfrak{z}2))) + \\
& x^2 (-1 + \eta)^2 (1200 \eta^6 \theta p - 92 \eta t \theta p - 120 \eta^5 (-19 + 10 \eta t) \theta p + \\
& \eta (-226 \eta t \theta p - (-1 + \eta t) \theta l (-234 + 27 \theta p \mathfrak{z}1 + 163 \theta p (2 + \mathfrak{z}2))) - \\
& 8 \eta^4 \theta p (717 - 5 \theta l (49 + 2 \mathfrak{z}2) + 5 \eta t (8 + \theta l (49 + 2 \mathfrak{z}2))) + \\
& 8 \eta^3 \theta p (174 - 3 \theta l (67 + 14 \mathfrak{z}2) + \eta t (271 + 3 \theta l (67 + 14 \mathfrak{z}2))) + 3 \eta^2 \\
& (2 \times (144 - 55 \eta t) \theta p + (-1 + \eta t) \theta l (116 + \theta p (66 + 57 \mathfrak{z}1 + 81 \mathfrak{z}2)))) + \\
& w^3 (-1 + \eta)^3 (4 x^5 (-1 + \eta)^5 (3 \times (-1 + \eta) \times (28 + 10 \eta^2 + \eta (11 - 10 \eta t) - 11 \eta t) \\
& \theta p + (-1 + \eta t) \theta l (10 + \theta p (-94 + 3 \mathfrak{z}1 + 7 \mathfrak{z}2))) - \\
& \eta^2 \theta p (120 \eta^6 + \eta^4 (360 - 372 \eta t) + \eta^5 (372 - 120 \eta t) - 312 \eta t - \\
& 2 \eta (-24 + 63 \eta t - 2 \theta l (66 + 27 \mathfrak{z}1 + 31 \mathfrak{z}2) + 2 \eta t \theta l (66 + 27 \mathfrak{z}1 + 31 \mathfrak{z}2)) + \\
& \eta^2 (312 + 500 \eta t + \theta l (78 + 81 \mathfrak{z}1 + 65 \mathfrak{z}2) - \eta t \theta l (78 + 81 \mathfrak{z}1 + 65 \mathfrak{z}2)) + \\
& \eta^3 (-1212 + \theta l (790 - 3 \mathfrak{z}1 - 3 \mathfrak{z}2) + \eta t (430 + \theta l (-790 + 3 \mathfrak{z}1 + 3 \mathfrak{z}2)))) - \\
& x^2 (-1 + \eta)^2 (1200 \eta^6 \theta p - 270 \eta t \theta p - 120 \eta^5 (-19 + 10 \eta t) \theta p - \\
& 24 \eta^4 (-109 + 95 \eta t) \theta p - 6 \eta (6 \times (-4 + 19 \eta t) \theta p + (-1 + \eta t) \theta l \\
& (-111 + 2 \theta p (66 + 27 \mathfrak{z}1 + 31 \mathfrak{z}2))) + 4 \eta^3 (15 \times (-134 + 55 \eta t) \theta p + \\
& (-1 + \eta t) \theta l (43 + \theta p (-1522 + 21 \mathfrak{z}1 + 37 \mathfrak{z}2))) - 3 \eta^2 (-6 \times \\
& (100 + 63 \eta t) \theta p + (-1 + \eta t) \theta l (-408 + \theta p (78 + 81 \mathfrak{z}1 + 65 \mathfrak{z}2)))) + \\
& x (-1 + \eta) \eta (600 \eta^6 \theta p + 12 \eta^4 (127 - 125 \eta t) \theta p - 546 \eta t \theta p - \\
& 300 \eta^5 (-5 + 2 \eta t) \theta p + 2 \eta^3 (8 \times (-312 + 119 \eta t) \theta p + (-1 + \eta t) \theta l \\
& (28 + \theta p (-1742 + 15 \mathfrak{z}1 + 23 \mathfrak{z}2))) - 6 \eta ((-24 + 89 \eta t) \theta p + \\
& (-1 + \eta t) \theta l (-65 + 2 \theta p (66 + 27 \mathfrak{z}1 + 31 \mathfrak{z}2))) + \eta^2 (4 \times (306 + \\
& 319 \eta t) \theta p - 3 \times (-1 + \eta t) \theta l (-174 + \theta p (78 + 81 \mathfrak{z}1 + 65 \mathfrak{z}2)))) + \\
& x^3 (-1 + \eta)^3 (4 \times (-1 + \eta) \times (-12 + 300 \eta^4 + \eta^2 (1266 - 690 \eta t) + \\
& \eta^3 (690 - 300 \eta t) + 78 \eta t - \eta (306 + 5 \eta t)) \theta p + (-1 + \eta t) \theta l \\
& (312 - 4 \theta p (66 + 27 \mathfrak{z}1 + 31 \mathfrak{z}2) - \eta (-990 + \theta p (78 + 81 \mathfrak{z}1 + 65 \mathfrak{z}2)) + \\
& 2 \eta^2 (108 + \theta p (-2630 + 51 \mathfrak{z}1 + 99 \mathfrak{z}2))) - x^4 (-1 + \eta)^4 (2 \times (-1 + \eta) \times \\
& (-144 + 300 \eta^3 + \eta^2 (510 - 300 \eta t) + 13 \eta t - 6 \eta (-173 + 85 \eta t)) \theta p + \\
& (-1 + \eta t) \theta l (288 + \eta (140 + \theta p (-2242 + 57 \mathfrak{z}1 + 121 \mathfrak{z}2)))) + \\
& w^2 (-1 + \eta)^2 (4 x^6 (-1 + \eta)^6 \theta p (10 \eta^3 + \eta^2 (1 - 10 \eta t) - \eta (-17 + \eta t) - \\
& 4 \times (7 + \theta l (-7 + \mathfrak{z}2)) + \eta t (11 + 4 \theta l (-7 + \mathfrak{z}2))) - 12 x^5 (-1 + \eta)^5 \\
& ((-1 + \eta) \times (20 \eta^3 + \eta (89 - 52 \eta t) + \eta^2 (52 - 20 \eta t) - 2 \times (12 + \eta t)) \theta p + \\
& (-1 + \eta t) \theta l (10 + \theta p (14 - 87 \eta + 3 \mathfrak{z}1 + 7 \mathfrak{z}2 + 6 \eta \mathfrak{z}2))) + \\
& \eta^2 \theta p (40 \eta^7 + \eta^5 (464 - 364 \eta t) + \eta^6 (364 - 40 \eta t) - 104 \eta t + \\
& 4 \eta \theta l (9 \mathfrak{z}1 + 13 \times (2 + \mathfrak{z}2)) - 2 \eta \eta t (149 + 18 \theta l \mathfrak{z}1 + 26 \theta l (2 + \mathfrak{z}2)) - \\
& 4 \eta^4 (343 - \theta l (151 + 2 \mathfrak{z}2) + \eta t (-35 + \theta l (151 + 2 \mathfrak{z}2))) + \\
& 3 \eta^3 (120 - \theta l (90 + 3 \mathfrak{z}1 + 19 \mathfrak{z}2) + \eta t (166 + \theta l (90 + 3 \mathfrak{z}1 + 19 \mathfrak{z}2))) - \\
& 3 \eta^2 (-48 - \theta l (86 + 27 \mathfrak{z}1 + 35 \mathfrak{z}2) + \eta t (-56 + \theta l (86 + 27 \mathfrak{z}1 + 35 \mathfrak{z}2)))) + \\
& 3 x^2 (-1 + \eta)^2 (200 \eta^7 \theta p - 30 \eta t \theta p - 20 \eta^6 (-61 + 10 \eta t) \theta p - \\
& 20 \eta^5 (-59 + 61 \eta t) \theta p - 4 \eta^4 (998 - 510 \theta l + 5 \eta t (-43 + 102 \theta l)) \theta p -
\end{aligned}$$

$$\begin{aligned}
& 2 \eta (126 \eta t \theta p + (-1 + \eta t) \theta l (-37 + 18 \theta p \mathfrak{x}1 + 26 \theta p (2 + \mathfrak{x}2))) - 3 \eta^2 \\
& (2 \times (-48 + 23 \eta t) \theta p + (-1 + \eta t) \theta l (-136 + \theta p (134 + 27 \mathfrak{x}1 + 51 \mathfrak{x}2))) + \\
& 4 \eta^3 ((276 + 245 \eta t) \theta p + (-1 + \eta t) \theta l (43 + \theta p (200 + 21 \mathfrak{x}1 + 61 \mathfrak{x}2))) - \\
& \times (-1 + \eta) \eta (240 \eta^7 \theta p + 12 \eta^5 (169 - 152 \eta t) \theta p - 182 \eta t \theta p - \\
& 48 \eta^6 (-38 + 5 \eta t) \theta p - 2 \eta (395 \eta t \theta p + (-1 + \eta t) \theta l \\
& (-65 + 54 \theta p \mathfrak{x}1 + 78 \theta p (2 + \mathfrak{x}2))) - 12 \eta^4 \theta p (533 - \theta l (251 + 2 \mathfrak{x}2) + \\
& \eta t (-82 + \theta l (251 + 2 \mathfrak{x}2))) + 6 \eta^3 (2 \times (144 + 161 \eta t) \theta p + \\
& (-1 + \eta t) \theta l (28 + \theta p (214 + 15 \mathfrak{x}1 + 55 \mathfrak{x}2))) + 3 \eta^2 \\
& (8 \times (24 + 5 \eta t) \theta p - (-1 + \eta t) \theta l (-174 + \theta p (306 + 81 \mathfrak{x}1 + 121 \mathfrak{x}2))) - \\
& \mathfrak{x}^3 (-1 + \eta)^3 (4 \times (-1 + \eta) \times (200 \eta^5 + \eta^3 (1910 - 1120 \eta t) + 69 \eta t - \\
& 40 \eta^4 (-28 + 5 \eta t) + 9 \eta (-16 + 25 \eta t) - 12 \eta^2 (78 + 25 \eta t)) \theta p + \\
& (-1 + \eta t) \theta l (104 + 40 \eta^3 \theta p (-161 + 2 \mathfrak{x}2) - 4 \theta p (26 + 9 \mathfrak{x}1 + 13 \mathfrak{x}2) - \\
& 3 \eta (-330 + \theta p (230 + 27 \mathfrak{x}1 + 83 \mathfrak{x}2)) + \\
& 6 \eta^2 (108 + \theta p (366 + 51 \mathfrak{x}1 + 131 \mathfrak{x}2))) + 3 \mathfrak{x}^4 (-1 + \eta)^4 \\
& (2 \times (-1 + \eta) \times (-24 + 100 \eta^4 + \eta^2 (670 - 410 \eta t) + \eta^3 (410 - 100 \eta t) + \\
& 43 \eta t - 12 \eta (23 + 5 \eta t)) \theta p + (-1 + \eta t) \theta l (96 - 16 \theta p (3 + \mathfrak{x}2) + \\
& 20 \eta^2 \theta p (-61 + 2 \mathfrak{x}2) + \eta (140 + \theta p (326 + 57 \mathfrak{x}1 + 137 \mathfrak{x}2)))))) / \\
& (96 (-1 + w (-1 + \eta))^3 (\mathfrak{x} (-1 + \eta) - \eta)^3 (w + \mathfrak{x} + \eta - w \eta - \mathfrak{x} \eta)^3 \\
& (-1 + \\
& \eta t) \theta p)
\end{aligned}$$

## Perturbative corrections

The following notation has been used in the following definitions :

$$\delta \Gamma \quad ( \delta \Gamma )$$

$$\delta \lambda^\perp \quad ( \delta \lambda p )$$

$$\delta \lambda'' \quad ( \delta \lambda l )$$

$$\delta \tilde{\Gamma} \quad ( \delta \Gamma t )$$

$$\delta \tilde{\lambda}^\perp \quad ( \delta \lambda p t )$$

$$\delta \tilde{\lambda}'' \quad ( \delta \lambda l t )$$

$$\delta \Omega \quad ( \delta \Omega )$$

$$\delta m \quad ( \delta m )$$

$$\delta g_\psi \quad ( \delta g \psi )$$

$$\delta g_s \quad ( \delta g s )$$

$$\delta g_{s1} \quad ( \delta g s1 )$$

$$\delta g_{s2} \quad ( \delta g s2 )$$

$$\delta \gamma_\psi \quad ( \delta \gamma \psi )$$

$$\delta \gamma_s \quad ( \delta \gamma s )$$

$$\delta \gamma_{s1} \quad ( \delta \gamma s1 )$$

$$\delta \gamma_{s2} \quad ( \delta \gamma s2 )$$

$$\delta J \quad ( \delta J )$$

$$\delta K \quad ( \delta K )$$

$$ln[ \circ ] := \delta \Gamma = \frac{c v^2}{4} -$$

$$\begin{aligned} & w \left( x \left( -1 + \eta \right) - \eta \right) \left( -1 + \eta \right) \times \left( -4 x^5 \left( -1 + \eta \right)^5 \operatorname{erf} \left( 30 \eta^3 + \eta^2 \left( 3 - 30 \eta t \right) + \right. \right. \\ & \quad \left. \left. 2 \times \left( 30 + \eta t - 6 \operatorname{erf} \left( 11 + 2 \right) + 6 \eta t \operatorname{erf} \left( 11 + 2 \right) \right) + \right. \right. \\ & \quad \left. \left. \eta \left( -93 + \operatorname{erf} \left( 31 + 2 \right) \right) + \eta t \left( 28 - \operatorname{erf} \left( 31 + 2 \right) \right) \right) \right) + 4 x^4 \left( -1 + \eta \right)^4 \\ & \quad \left( \left( -1 + \eta \right) \times \left( 150 \eta^3 + \eta^2 \left( 255 - 150 \eta t \right) + 9 \times \left( -4 + 3 \eta t \right) - 2 \eta \left( 177 + 35 \eta t \right) \right) \operatorname{erf} - \right. \\ & \quad \left. \left( -1 + \eta t \right) \operatorname{erf} \left( -30 + \operatorname{erf} \left( 5 \eta^2 \left( 37 + 2 \right) - 12 \times \left( 14 + 3 \right) + 3 \right) - \right. \right. \end{aligned}$$



$$\begin{aligned}
& 3 \eta (229 + 18 \mathfrak{z}2) \Big) \Big) + \eta^2 \mathfrak{e}p \Big( 120 \eta^6 + \eta^5 (372 - 120 \eta t) - 62 \eta t + \\
& \eta (-64 \eta t - 81 \mathfrak{e}l \mathfrak{z}1 - 41 \mathfrak{e}l (2 + \mathfrak{z}2) + \eta t \mathfrak{e}l (81 \mathfrak{z}1 + 41 \times (2 + \mathfrak{z}2)) \Big) + \\
& 4 \eta^3 (78 - 3 \mathfrak{e}l (53 + 2 \mathfrak{z}2) + \eta t (89 + 3 \mathfrak{e}l (53 + 2 \mathfrak{z}2)) \Big) - \\
& 4 \eta^4 (237 - \mathfrak{e}l (61 + 2 \mathfrak{z}2) + \eta t (32 + \mathfrak{e}l (61 + 2 \mathfrak{z}2)) \Big) + \\
& 3 \eta^2 (48 - \mathfrak{e}l (222 + 39 \mathfrak{z}1 + 47 \mathfrak{z}2) + \eta t (6 + \mathfrak{e}l (222 + 39 \mathfrak{z}1 + 47 \mathfrak{z}2)) \Big) \Big) + \\
& x^2 (-1 + \eta)^2 \Big( 1200 \eta^6 \mathfrak{e}p - 20 \eta t \mathfrak{e}p - 120 \eta^5 (-19 + 10 \eta t) \mathfrak{e}p + \\
& \eta (-298 \eta t \mathfrak{e}p + (-1 + \eta t) \mathfrak{e}l (90 + 297 \mathfrak{e}p \mathfrak{z}1 + 161 \mathfrak{e}p (2 + \mathfrak{z}2)) \Big) - \\
& 8 \eta^4 \mathfrak{e}p (897 - 5 \mathfrak{e}l (49 + 2 \mathfrak{z}2) + 5 \eta t (8 + \mathfrak{e}l (49 + 2 \mathfrak{z}2)) \Big) + \\
& 8 \eta^3 \mathfrak{e}p (354 - 3 \mathfrak{e}l (247 + 14 \mathfrak{z}2) + \eta t (271 + \mathfrak{e}l (741 + 42 \mathfrak{z}2)) \Big) + \eta^2 \\
& (6 \times (144 - 55 \eta t) \mathfrak{e}p + 3 \times (-1 + \eta t) \mathfrak{e}l (116 + 3 \mathfrak{e}p (454 + 91 \mathfrak{z}1 + 99 \mathfrak{z}2)) \Big) \Big) - \\
& x (-1 + \eta) \eta \Big( 600 \eta^6 \mathfrak{e}p - 46 \eta t \mathfrak{e}p - 300 \eta^5 (-5 + 2 \eta t) \mathfrak{e}p + \\
& 2 \eta (-124 \eta t \mathfrak{e}p + (-1 + \eta t) \mathfrak{e}l (51 + 135 \mathfrak{e}p \mathfrak{z}1 + 71 \mathfrak{e}p (2 + \mathfrak{z}2)) \Big) - \\
& 4 \eta^4 \mathfrak{e}p (1041 - 5 \mathfrak{e}l (55 + 2 \mathfrak{z}2) + 5 \eta t (20 + \mathfrak{e}l (55 + 2 \mathfrak{z}2)) \Big) + \\
& 8 \eta^3 \mathfrak{e}p (186 - 6 \mathfrak{e}l (64 + 3 \mathfrak{z}2) + \eta t (179 + 6 \mathfrak{e}l (64 + 3 \mathfrak{z}2)) \Big) + \\
& 3 \eta^2 (2 \times (96 - 23 \eta t) \mathfrak{e}p + (-1 + \eta t) \mathfrak{e}l (56 + \mathfrak{e}p (902 + 171 \mathfrak{z}1 + 195 \mathfrak{z}2)) \Big) \Big) - \\
& x^3 (-1 + \eta)^3 \Big( 2 \times (-1 + \eta) \times \Big( 600 \eta^4 + 75 \eta t + 72 \eta (-4 + 3 \eta t) - \\
& 60 \eta^3 (-23 + 10 \eta t) - 8 \eta^2 (204 + 65 \eta t) \Big) \mathfrak{e}p - \\
& (-1 + \eta t) \mathfrak{e}l \Big( 40 \eta^3 \mathfrak{e}p (43 + 2 \mathfrak{z}2) - 48 \eta^2 \mathfrak{e}p (119 + 8 \mathfrak{z}2) - 12 \times \\
& (2 + 9 \mathfrak{e}p \mathfrak{z}1 + 5 \mathfrak{e}p (2 + \mathfrak{z}2)) - 3 \eta (100 + \mathfrak{e}p (906 + 189 \mathfrak{z}1 + 197 \mathfrak{z}2)) \Big) \Big) \Big) + \\
& w^2 (-1 + \eta)^2 \Big( 4 x^6 (-1 + \eta)^6 \mathfrak{e}p \Big( 8 + 10 \eta^3 + \eta^2 (1 - 10 \eta t) - \eta (19 + \eta t) - \\
& 44 \mathfrak{e}l - 4 \mathfrak{e}l \mathfrak{z}2 + \eta t (11 + 4 \mathfrak{e}l (11 + \mathfrak{z}2)) \Big) - 12 x^5 (-1 + \eta)^5 \\
& \Big( (-1 + \eta) \times \Big( 20 \eta^3 + \eta (17 - 52 \eta t) + \eta^2 (52 - 20 \eta t) - 2 \times (30 + \eta t) \Big) \mathfrak{e}p + \\
& (-1 + \eta t) \mathfrak{e}l (10 + 4 \mathfrak{e}p (35 + 3 \mathfrak{z}1 + 4 \mathfrak{z}2) + \eta \mathfrak{e}p (57 + 6 \mathfrak{z}2)) \Big) + 3 x^4 (-1 + \eta)^4 \\
& \Big( 2 \times (-1 + \eta) \times \Big( -24 + 100 \eta^4 + \eta^2 (310 - 410 \eta t) + \eta^3 (410 - 100 \eta t) + 43 \eta t - \\
& 12 \eta (53 + 5 \eta t) \Big) \mathfrak{e}p + (-1 + \eta t) \mathfrak{e}l \Big( 24 + 140 \eta + 20 \eta^2 \mathfrak{e}p (11 + 2 \mathfrak{z}2) + \\
& 4 \mathfrak{e}p (78 + 27 \mathfrak{z}1 + 23 \mathfrak{z}2) + \eta \mathfrak{e}p (2846 + 237 \mathfrak{z}1 + 317 \mathfrak{z}2) \Big) \Big) + \\
& \eta^2 \mathfrak{e}p \Big( 40 \eta^7 + \eta^6 (364 - 40 \eta t) - 32 \eta t - 4 \eta^5 (-80 + 91 \eta t) - \\
& 4 \eta^4 (415 - \mathfrak{e}l (79 + 2 \mathfrak{z}2) + \eta t (-35 + \mathfrak{e}l (79 + 2 \mathfrak{z}2)) \Big) + \\
& 2 \eta (-2 \mathfrak{e}l (9 \mathfrak{z}1 + 5 \times (2 + \mathfrak{z}2)) + \eta t (-77 + 2 \mathfrak{e}l (10 + 9 \mathfrak{z}1 + 5 \mathfrak{z}2)) \Big) + \\
& 3 \eta^3 (264 - \mathfrak{e}l (594 + 39 \mathfrak{z}1 + 55 \mathfrak{z}2) + \eta t (166 + \mathfrak{e}l (594 + 39 \mathfrak{z}1 + 55 \mathfrak{z}2)) \Big) + \\
& 3 \eta^2 (48 - \mathfrak{e}l (274 + 81 \mathfrak{z}1 + 73 \mathfrak{z}2) + \eta t (-16 + \mathfrak{e}l (274 + 81 \mathfrak{z}1 + 73 \mathfrak{z}2)) \Big) \Big) + \\
& 3 x^2 (-1 + \eta)^2 \Big( 200 \eta^7 \mathfrak{e}p - 6 \eta t \mathfrak{e}p - 20 \eta^6 (-61 + 10 \eta t) \mathfrak{e}p - \\
& 20 \eta^5 (-23 + 61 \eta t) \mathfrak{e}p + 4 \eta^4 (-1178 + 215 \eta t + 150 \mathfrak{e}l - 150 \eta t \mathfrak{e}l) \mathfrak{e}p + \\
& \eta (-60 \eta t \mathfrak{e}p + 2 \times (-1 + \eta t) \mathfrak{e}l (13 + 2 \mathfrak{e}p (10 + 9 \mathfrak{z}1 + 5 \mathfrak{z}2)) \Big) + \\
& 4 \eta^3 ((636 + 245 \eta t) \mathfrak{e}p + (-1 + \eta t) \mathfrak{e}l (43 + \mathfrak{e}p (1460 + 111 \mathfrak{z}1 + 151 \mathfrak{z}2)) \Big) + \\
& 3 \eta^2 (2 \times (48 - 59 \eta t) \mathfrak{e}p + (-1 + \eta t) \mathfrak{e}l (64 + \mathfrak{e}p (586 + 189 \mathfrak{z}1 + 165 \mathfrak{z}2)) \Big) \Big) - \\
& x (-1 + \eta) \eta \Big( 240 \eta^7 \mathfrak{e}p - 38 \eta t \mathfrak{e}p - 48 \eta^6 (-38 + 5 \eta t) \mathfrak{e}p - 12 \eta^5 (-97 + 152 \eta t) \\
& \mathfrak{e}p - 12 \eta^4 \mathfrak{e}p (641 - 107 \mathfrak{e}l - 2 \mathfrak{e}l \mathfrak{z}2 + \eta t (-82 + 107 \mathfrak{e}l + 2 \mathfrak{e}l \mathfrak{z}2)) \Big) + \\
& 2 \eta (-143 \eta t \mathfrak{e}p + (-1 + \eta t) \mathfrak{e}l (29 + 6 \mathfrak{e}p (10 + 9 \mathfrak{z}1 + 5 \mathfrak{z}2)) \Big) + 6 \eta^3 (2 \times (324 + \\
& 161 \eta t) \mathfrak{e}p + (-1 + \eta t) \mathfrak{e}l (28 + \mathfrak{e}p (1474 + 105 \mathfrak{z}1 + 145 \mathfrak{z}2)) \Big) + 3 \eta^2 \\
& (16 \times (12 - 11 \eta t) \mathfrak{e}p + (-1 + \eta t) \mathfrak{e}l (102 + \mathfrak{e}p (1134 + 351 \mathfrak{z}1 + 311 \mathfrak{z}2)) \Big) \Big) - \\
& x^3 (-1 + \eta)^3 \Big( 4 \times (-1 + \eta) \times \Big( 200 \eta^5 + 15 \eta t - 40 \eta^4 (-28 + 5 \eta t) - \\
& 70 \eta^3 (-17 + 16 \eta t) + 9 \eta (-16 + 25 \eta t) - 12 \eta^2 (168 + 25 \eta t) \Big) \mathfrak{e}p + \\
& (-1 + \eta t) \mathfrak{e}l \Big( 40 \eta^3 \mathfrak{e}p (-17 + 2 \mathfrak{z}2) + 4 \times (8 + 9 \mathfrak{e}p \mathfrak{z}1 + 5 \mathfrak{e}p (2 + \mathfrak{z}2)) \Big) +
\end{aligned}$$

$$\begin{aligned}
& 6 \eta^2 (108 + \theta p (2886 + 231 \mathfrak{e}1 + 311 \mathfrak{e}2)) + \\
& 3 \eta (114 + \theta p (1210 + 405 \mathfrak{e}1 + 349 \mathfrak{e}2)) \Big) \Big) + \\
& w^3 (-1 + \eta)^3 \Big( 4 x^5 (-1 + \eta)^5 \Big( 3 \times (-1 + \eta) \times (-8 + 10 \eta^2 + \eta (11 - 10 \eta t) - 11 \eta t) \theta p + \\
& 2 \times (-1 + \eta t) \mathfrak{e}l (5 + \theta p (70 + 6 \mathfrak{e}1 + 8 \mathfrak{e}2)) \Big) - x^4 (-1 + \eta)^4 \Big( 2 \times (-1 + \eta) \times \\
& (-360 + 300 \eta^3 + \eta^2 (510 - 300 \eta t) + 13 \eta t - 6 \eta (7 + 85 \eta t)) \theta p + (-1 + \eta t) \\
& \mathfrak{e}l (72 + 140 \eta + 324 \theta p (6 + \mathfrak{e}1 + \mathfrak{e}2) + \eta \theta p (2438 + 237 \mathfrak{e}1 + 301 \mathfrak{e}2)) \Big) + \\
& \eta^2 \theta p (-120 \eta^6 + 96 \eta t + 12 \eta^5 (-31 + 10 \eta t) + 12 \eta^4 (6 + 31 \eta t) - \\
& 2 \eta (24 - 2 \mathfrak{e}l (78 + 27 \mathfrak{e}1 + 23 \mathfrak{e}2) + \eta t (-63 + 2 \mathfrak{e}l (78 + 27 \mathfrak{e}1 + 23 \mathfrak{e}2))) + \\
& \eta^3 (1212 + \mathfrak{e}l (146 + 39 \mathfrak{e}1 + 39 \mathfrak{e}2) - \eta t (430 + \mathfrak{e}l (146 + 39 \mathfrak{e}1 + 39 \mathfrak{e}2))) - \\
& \eta^2 (744 - \mathfrak{e}l (1866 + 243 \mathfrak{e}1 + 259 \mathfrak{e}2) + \\
& \eta t (284 + \mathfrak{e}l (1866 + 243 \mathfrak{e}1 + 259 \mathfrak{e}2))) \Big) + x (-1 + \eta) \eta \\
& (600 \eta^6 \theta p - 114 \eta t \theta p - 300 \eta^5 (-5 + 2 \eta t) \theta p - 12 \eta^4 (53 + 125 \eta t) \theta p + \\
& 6 \eta ((24 - 53 \eta t) \theta p + (-1 + \eta t) \mathfrak{e}l (29 + 2 \theta p (78 + 27 \mathfrak{e}1 + 23 \mathfrak{e}2))) + 2 \eta^3 \\
& (8 \times (-285 + 119 \eta t) \theta p + (-1 + \eta t) \mathfrak{e}l (28 + \theta p (598 + 105 \mathfrak{e}1 + 113 \mathfrak{e}2))) + \\
& \eta^2 (4 \times (738 + 157 \eta t) \theta p + 3 \times (-1 + \eta t) \mathfrak{e}l \\
& (102 + \theta p (2514 + 351 \mathfrak{e}1 + 367 \mathfrak{e}2))) \Big) - x^2 (-1 + \eta)^2 \\
& (1200 \eta^6 \theta p - 54 \eta t \theta p - 120 \eta^5 (-19 + 10 \eta t) \theta p - 24 \eta^4 (71 + 95 \eta t) \theta p + \\
& 6 \eta (6 \times (4 - 7 \eta t) \theta p + (-1 + \eta t) \mathfrak{e}l (39 + 2 \theta p (78 + 27 \mathfrak{e}1 + 23 \mathfrak{e}2))) + \\
& 4 \eta^3 (3 \times (-526 + 275 \eta t) \theta p + \\
& (-1 + \eta t) \mathfrak{e}l (43 + \theta p (818 + 111 \mathfrak{e}1 + 127 \mathfrak{e}2))) + 3 \eta^2 \\
& (6 \times (244 + 27 \eta t) \theta p + (-1 + \eta t) \mathfrak{e}l (192 + \theta p (3810 + 567 \mathfrak{e}1 + 583 \mathfrak{e}2))) \Big) + \\
& x^3 (-1 + \eta)^3 \Big( 4 \times (-1 + \eta) \times (-12 + 300 \eta^4 + \eta^2 (186 - 690 \eta t) + \\
& \eta^3 (690 - 300 \eta t) + 24 \eta t - \eta (738 + 5 \eta t)) \theta p + (-1 + \eta t) \mathfrak{e}l \\
& (96 + 4 \theta p (78 + 27 \mathfrak{e}1 + 23 \mathfrak{e}2) + \eta^2 (216 + \theta p (4100 + 462 \mathfrak{e}1 + 558 \mathfrak{e}2)) + \\
& \eta (342 + \theta p (7698 + 1215 \mathfrak{e}1 + 1231 \mathfrak{e}2))) \Big) \Big) \Big) \Big) / \\
& (96 (-1 + w (-1 + \eta))^3 (x (-1 + \eta) - \eta)^3 (w + x + \eta - w \eta - x \eta)^3 \\
& (-1 + \\
& \eta t) \theta p)
\end{aligned}$$

$$Out[4]= \frac{cv^2}{4} -$$

$$\begin{aligned}
& (f (-1 + \eta) \times (2 w^5 (-1 + \eta)^5 (2 x^3 (-1 + \eta)^3 ((-1 + \eta) \times (-8 + 10 \eta^2 + \eta (11 - 10 \eta t) - 11 \eta t) \\
& \theta p + (-1 + \eta t) \mathfrak{e}l (8 + 9 \theta p (6 + \mathfrak{e}1 + \mathfrak{e}2))) - \\
& 3 x^2 (-1 + \eta)^2 (20 \eta^4 \theta p + \eta^3 (2 - 20 \eta t) \theta p - 3 \eta t \theta p - 2 \eta^2 (19 + \eta t) \theta p + \\
& \eta (16 + 25 \eta t) \theta p + \eta (-1 + \eta t) \mathfrak{e}l (13 + 18 \theta p (6 + \mathfrak{e}1 + \mathfrak{e}2))) + \\
& x (-1 + \eta) \eta (60 \eta^4 \theta p + \eta^3 (6 - 60 \eta t) \theta p - 19 \eta t \theta p - 6 \eta^2 (19 + \eta t) \theta p + \\
& \eta (48 + 85 \eta t) \theta p + \eta (-1 + \eta t) \mathfrak{e}l (29 + 54 \theta p (6 + \mathfrak{e}1 + \mathfrak{e}2))) - \\
& 2 \eta^2 \theta p (10 \eta^4 + \eta^3 (1 - 10 \eta t) - 8 \eta t - \eta^2 (19 + \eta t) + \\
& \eta (8 - 9 \mathfrak{e}l (6 + \mathfrak{e}1 + \mathfrak{e}2) + \eta t (19 + 9 \mathfrak{e}l (6 + \mathfrak{e}1 + \mathfrak{e}2)))) + \\
& 3 w^4 (-1 + \eta)^4 (4 x^4 (-1 + \eta)^4 ((-1 + \eta) \times (-8 + 10 \eta^2 + \eta (11 - 10 \eta t) - 11 \eta t) \theta p + \\
& (-1 + \eta t) \mathfrak{e}l (2 + 9 \theta p (6 + \mathfrak{e}1 + \mathfrak{e}2))) - \\
& x^3 (-1 + \eta)^3 (4 \times (-1 + \eta) \times (-20 + 40 \eta^3 + \eta^2 (54 - 40 \eta t) + \eta t - 3 \eta (7 + 18 \eta t)) \theta p + \\
& (-1 + \eta t) \mathfrak{e}l (32 + 38 \eta + 36 \theta p (6 + \mathfrak{e}1 + \mathfrak{e}2) + 135 \eta \theta p (6 + \mathfrak{e}1 + \mathfrak{e}2))) + \\
& \eta^2 \theta p (40 \eta^5 + \eta^4 (44 - 40 \eta t) - 32 \eta t - 4 \eta^3 (18 + 11 \eta t) +
\end{aligned}$$

$$\begin{aligned}
& \eta^2 (-92 - 27 \theta l (6 + \Phi 1 + \Phi 2) + 3 \eta t (34 + 9 \theta l (6 + \Phi 1 + \Phi 2))) + \\
& 2 \eta (40 - 18 \theta l (6 + \Phi 1 + \Phi 2) + \eta t (7 + 18 \theta l (6 + \Phi 1 + \Phi 2))) - \\
& x (-1 + \eta) \eta (160 \eta^5 \theta p - 38 \eta t \theta p - 8 \eta^4 (-17 + 20 \eta t) \theta p - 4 \eta^3 (73 + 34 \eta t) \theta p + \\
& 2 \eta (5 \times (24 + \eta t) \theta p + (-1 + \eta t) \theta l (29 + 54 \theta p (6 + \Phi 1 + \Phi 2))) + \\
& \eta^2 (4 \times (-61 + 81 \eta t) \theta p + (-1 + \eta t) \theta l (34 + 117 \theta p (6 + \Phi 1 + \Phi 2))) + \\
& x^2 (-1 + \eta)^2 (240 \eta^5 \theta p - 18 \eta t \theta p + 4 \eta (60 + \eta t) \theta p - 48 \eta^4 (-3 + 5 \eta t) \theta p - \\
& 12 \eta^3 (37 + 12 \eta t) \theta p + 6 \eta (-1 + \eta t) \theta l (13 + 18 \theta p (6 + \Phi 1 + \Phi 2)) + \\
& \eta^2 (2 \times (-90 + 199 \eta t) \theta p + (-1 + \eta t) \theta l (64 + 189 \theta p (6 + \Phi 1 + \Phi 2)))) + \\
& (x + \eta - x \eta)^2 (4 x^4 (-1 + \eta)^4 \theta p (12 + 30 \eta^3 - 48 \theta l - 2 \eta^2 (24 - 5 \theta l + 5 \eta t (2 + \theta l))) - \\
& 8 \theta l \Phi 2 + \eta t (-9 + 8 \theta l (6 + \Phi 2)) + \\
& \eta (6 - 9 \theta l + 2 \theta l \Phi 2 + \eta t (29 + 9 \theta l - 2 \theta l \Phi 2))) - \\
& 8 x^3 (-1 + \eta)^3 (2 \times (-1 + \eta) \eta (-12 + 30 \eta^2 + 9 \eta t - 2 \eta (9 + 10 \eta t)) \theta p - (-1 + \eta t) \\
& \theta l (-5 + 2 \theta p (-2 + 10 \eta^3 - 3 \Phi 1 - \Phi 2 - 8 \eta (6 + \Phi 2) + \eta^2 (-9 + 2 \Phi 2)))) + \\
& \eta^2 \theta p (120 \eta^5 - 42 \eta t - 8 \eta^4 (24 - 5 \theta l + 5 \eta t (2 + \theta l)) + \\
& 3 \eta (14 \eta t - 13 \theta l \Phi 1 - 5 \theta l (2 + \Phi 2) + \eta t \theta l (13 \Phi 1 + 5 \times (2 + \Phi 2))) + \\
& 4 \eta^2 (12 - 8 \theta l (6 + \Phi 2) + \eta t (-9 + 8 \theta l (6 + \Phi 2))) - \\
& 4 \eta^3 (-6 + \theta l (9 - 2 \Phi 2) + \eta t (-29 + \theta l (-9 + 2 \Phi 2)))) + \\
& x^2 (-1 + \eta)^2 (720 \eta^5 \theta p - 50 \eta t \theta p - 48 \eta^4 (24 - 5 \theta l + 5 \eta t (2 + \theta l)) \theta p + \\
& \eta (50 \eta t \theta p + (-1 + \eta t) \theta l (60 + 141 \theta p \Phi 1 + 53 \theta p (2 + \Phi 2))) + \\
& 24 \eta^2 \theta p (12 - 8 \theta l (6 + \Phi 2) + \eta t (-9 + 8 \theta l (6 + \Phi 2))) - \\
& 24 \eta^3 \theta p (-6 + \theta l (9 - 2 \Phi 2) + \eta t (-29 + \theta l (-9 + 2 \Phi 2)))) - \\
& 4 x (-1 + \eta) \eta (120 \eta^5 \theta p - 14 \eta t \theta p - 8 \eta^4 (24 - 5 \theta l + 5 \eta t (2 + \theta l)) \theta p + \\
& \eta (14 \eta t \theta p + (-1 + \eta t) \theta l (14 + 33 \theta p \Phi 1 + 13 \theta p (2 + \Phi 2))) + \\
& 4 \eta^2 \theta p (12 - 8 \theta l (6 + \Phi 2) + \eta t (-9 + 8 \theta l (6 + \Phi 2))) - \\
& 4 \eta^3 \theta p (-6 + \theta l (9 - 2 \Phi 2) + \eta t (-29 + \theta l (-9 + 2 \Phi 2)))) + \\
& w (x (-1 + \eta) - \eta) (-1 + \eta) \times (-4 x^5 (-1 + \eta)^5 \theta p (30 \eta^3 + \eta^2 (3 - 30 \eta t) + \\
& 2 \times (30 + \eta t - 6 \theta l (11 + \Phi 2) + 6 \eta t \theta l (11 + \Phi 2)) + \\
& \eta (-93 + \theta l (31 + 2 \Phi 2) + \eta t (28 - \theta l (31 + 2 \Phi 2)))) + 4 x^4 (-1 + \eta)^4 \\
& ((-1 + \eta) \times (150 \eta^3 + \eta^2 (255 - 150 \eta t) + 9 \times (-4 + 3 \eta t) - 2 \eta (177 + 35 \eta t)) \theta p - \\
& (-1 + \eta t) \theta l (-30 + \theta p (5 \eta^2 (37 + 2 \Phi 2) - 12 \times (14 + 3 \Phi 1 + 3 \Phi 2) - \\
& 3 \eta (229 + 18 \Phi 2)))) + \eta^2 \theta p (120 \eta^6 + \eta^5 (372 - 120 \eta t) - 62 \eta t + \\
& \eta (-64 \eta t - 81 \theta l \Phi 1 - 41 \theta l (2 + \Phi 2) + \eta t \theta l (81 \Phi 1 + 41 \times (2 + \Phi 2))) + \\
& 4 \eta^3 (78 - 3 \theta l (53 + 2 \Phi 2) + \eta t (89 + 3 \theta l (53 + 2 \Phi 2))) - \\
& 4 \eta^4 (237 - \theta l (61 + 2 \Phi 2) + \eta t (32 + \theta l (61 + 2 \Phi 2))) + \\
& 3 \eta^2 (48 - \theta l (222 + 39 \Phi 1 + 47 \Phi 2) + \eta t (6 + \theta l (222 + 39 \Phi 1 + 47 \Phi 2)))) + \\
& x^2 (-1 + \eta)^2 (1200 \eta^6 \theta p - 20 \eta t \theta p - 120 \eta^5 (-19 + 10 \eta t) \theta p + \\
& \eta (-298 \eta t \theta p + (-1 + \eta t) \theta l (90 + 297 \theta p \Phi 1 + 161 \theta p (2 + \Phi 2))) - \\
& 8 \eta^4 \theta p (897 - 5 \theta l (49 + 2 \Phi 2) + 5 \eta t (8 + \theta l (49 + 2 \Phi 2))) + \\
& 8 \eta^3 \theta p (354 - 3 \theta l (247 + 14 \Phi 2) + \eta t (271 + \theta l (741 + 42 \Phi 2))) + \\
& \eta^2 (6 \times (144 - 55 \eta t) \theta p + 3 \times (-1 + \eta t) \theta l (116 + 3 \theta p (454 + 91 \Phi 1 + 99 \Phi 2)))) - \\
& x (-1 + \eta) \eta (600 \eta^6 \theta p - 46 \eta t \theta p - 300 \eta^5 (-5 + 2 \eta t) \theta p + \\
& 2 \eta (-124 \eta t \theta p + (-1 + \eta t) \theta l (51 + 135 \theta p \Phi 1 + 71 \theta p (2 + \Phi 2))) - \\
& 4 \eta^4 \theta p (1041 - 5 \theta l (55 + 2 \Phi 2) + 5 \eta t (20 + \theta l (55 + 2 \Phi 2))) + \\
& 8 \eta^3 \theta p (186 - 6 \theta l (64 + 3 \Phi 2) + \eta t (179 + 6 \theta l (64 + 3 \Phi 2))) +
\end{aligned}$$

$$\begin{aligned}
& 3 \eta^2 (2 \times (96 - 23 \eta t) \Theta p + (-1 + \eta t) \Theta l (56 + \Theta p (902 + 171 \oplus 1 + 195 \oplus 2))) - \\
& x^3 (-1 + \eta)^3 (2 \times (-1 + \eta) \times (600 \eta^4 + 75 \eta t + 72 \eta (-4 + 3 \eta t) - 60 \\
& \eta^3 (-23 + 10 \eta t) - 8 \eta^2 (204 + 65 \eta t)) \Theta p - \\
& (-1 + \eta t) \Theta l (40 \eta^3 \Theta p (43 + 2 \oplus 2) - 48 \eta^2 \Theta p (119 + 8 \oplus 2) - 12 \times \\
& (2 + 9 \Theta p \oplus 1 + 5 \Theta p (2 + \oplus 2)) - 3 \eta (100 + \Theta p (906 + 189 \oplus 1 + 197 \oplus 2))) + \\
& w^2 (-1 + \eta)^2 (4 x^6 (-1 + \eta)^6 \Theta p (8 + 10 \eta^3 + \eta^2 (1 - 10 \eta t) - \eta (19 + \eta t) - \\
& 44 \Theta l - 4 \Theta l \oplus 2 + \eta t (11 + 4 \Theta l (11 + \oplus 2))) - 12 x^5 (-1 + \eta)^5 \\
& ((-1 + \eta) \times (20 \eta^3 + \eta (17 - 52 \eta t) + \eta^2 (52 - 20 \eta t) - 2 \times (30 + \eta t)) \Theta p + \\
& (-1 + \eta t) \Theta l (10 + 4 \Theta p (35 + 3 \oplus 1 + 4 \oplus 2) + \eta \Theta p (57 + 6 \oplus 2))) + \\
& 3 x^4 (-1 + \eta)^4 (2 \times (-1 + \eta) \times (-24 + 100 \eta^4 + \eta^2 (310 - 410 \eta t) + \eta^3 (410 - 100 \eta t) + \\
& 43 \eta t - 12 \eta (53 + 5 \eta t)) \Theta p + (-1 + \eta t) \Theta l (24 + 140 \eta + 20 \eta^2 \Theta p \\
& (11 + 2 \oplus 2) + 4 \Theta p (78 + 27 \oplus 1 + 23 \oplus 2) + \eta \Theta p (2846 + 237 \oplus 1 + 317 \oplus 2))) + \\
& \eta^2 \Theta p (40 \eta^7 + \eta^6 (364 - 40 \eta t) - 32 \eta t - 4 \eta^5 (-80 + 91 \eta t) - \\
& 4 \eta^4 (415 - \Theta l (79 + 2 \oplus 2) + \eta t (-35 + \Theta l (79 + 2 \oplus 2))) + \\
& 2 \eta (-2 \Theta l (9 \oplus 1 + 5 \times (2 + \oplus 2)) + \eta t (-77 + 2 \Theta l (10 + 9 \oplus 1 + 5 \oplus 2))) + \\
& 3 \eta^3 (264 - \Theta l (594 + 39 \oplus 1 + 55 \oplus 2) + \eta t (166 + \Theta l (594 + 39 \oplus 1 + 55 \oplus 2))) + \\
& 3 \eta^2 (48 - \Theta l (274 + 81 \oplus 1 + 73 \oplus 2) + \eta t (-16 + \Theta l (274 + 81 \oplus 1 + 73 \oplus 2))) + \\
& 3 x^2 (-1 + \eta)^2 (200 \eta^7 \Theta p - 6 \eta t \Theta p - 20 \eta^6 (-61 + 10 \eta t) \Theta p - \\
& 20 \eta^5 (-23 + 61 \eta t) \Theta p + 4 \eta^4 (-1178 + 215 \eta t + 150 \Theta l - 150 \eta t \Theta l) \Theta p + \\
& \eta (-60 \eta t \Theta p + 2 \times (-1 + \eta t) \Theta l (13 + 2 \Theta p (10 + 9 \oplus 1 + 5 \oplus 2))) + \\
& 4 \eta^3 ((636 + 245 \eta t) \Theta p + (-1 + \eta t) \Theta l (43 + \Theta p (1460 + 111 \oplus 1 + 151 \oplus 2))) + \\
& 3 \eta^2 (2 \times (48 - 59 \eta t) \Theta p + (-1 + \eta t) \Theta l (64 + \Theta p (586 + 189 \oplus 1 + 165 \oplus 2))) - \\
& x (-1 + \eta) \eta (240 \eta^7 \Theta p - 38 \eta t \Theta p - 48 \eta^6 (-38 + 5 \eta t) \Theta p - 12 \eta^5 (-97 + 152 \eta t) \Theta p - \\
& 12 \eta^4 \Theta p (641 - 107 \Theta l - 2 \Theta l \oplus 2 + \eta t (-82 + 107 \Theta l + 2 \Theta l \oplus 2)) + \\
& 2 \eta (-143 \eta t \Theta p + (-1 + \eta t) \Theta l (29 + 6 \Theta p (10 + 9 \oplus 1 + 5 \oplus 2))) + \\
& 6 \eta^3 (2 \times (324 + 161 \eta t) \Theta p + (-1 + \eta t) \Theta l (28 + \Theta p (1474 + 105 \oplus 1 + 145 \oplus 2))) + \\
& 3 \eta^2 (16 \times (12 - 11 \eta t) \Theta p + (-1 + \eta t) \Theta l (102 + \Theta p (1134 + 351 \oplus 1 + 311 \oplus 2))) - \\
& x^3 (-1 + \eta)^3 (4 \times (-1 + \eta) \times (200 \eta^5 + 15 \eta t - 40 \eta^4 (-28 + 5 \eta t) - 70 \eta^3 \\
& (-17 + 16 \eta t) + 9 \eta (-16 + 25 \eta t) - 12 \eta^2 (168 + 25 \eta t)) \Theta p + \\
& (-1 + \eta t) \Theta l (40 \eta^3 \Theta p (-17 + 2 \oplus 2) + 4 \times (8 + 9 \Theta p \oplus 1 + 5 \Theta p (2 + \oplus 2)) + \\
& 6 \eta^2 (108 + \Theta p (2886 + 231 \oplus 1 + 311 \oplus 2)) + 3 \\
& \eta (114 + \Theta p (1210 + 405 \oplus 1 + 349 \oplus 2))) + \\
& w^3 (-1 + \eta)^3 (4 x^5 (-1 + \eta)^5 (3 \times (-1 + \eta) \times (-8 + 10 \eta^2 + \eta (11 - 10 \eta t) - 11 \eta t) \Theta p + \\
& 2 \times (-1 + \eta t) \Theta l (5 + \Theta p (70 + 6 \oplus 1 + 8 \oplus 2))) - x^4 (-1 + \eta)^4 (2 \times (-1 + \eta) \times \\
& (-360 + 300 \eta^3 + \eta^2 (510 - 300 \eta t) + 13 \eta t - 6 \eta (7 + 85 \eta t)) \Theta p + (-1 + \eta t) \\
& \Theta l (72 + 140 \eta + 324 \Theta p (6 + \oplus 1 + \oplus 2) + \eta \Theta p (2438 + 237 \oplus 1 + 301 \oplus 2))) + \\
& \eta^2 \Theta p (-120 \eta^6 + 96 \eta t + 12 \eta^5 (-31 + 10 \eta t) + 12 \eta^4 (6 + 31 \eta t) - \\
& 2 \eta (24 - 2 \Theta l (78 + 27 \oplus 1 + 23 \oplus 2) + \eta t (-63 + 2 \Theta l (78 + 27 \oplus 1 + 23 \oplus 2))) + \\
& \eta^3 (1212 + \Theta l (146 + 39 \oplus 1 + 39 \oplus 2) - \eta t (430 + \Theta l (146 + 39 \oplus 1 + 39 \oplus 2))) - \\
& \eta^2 (744 - \Theta l (1866 + 243 \oplus 1 + 259 \oplus 2) + \eta t \\
& (284 + \Theta l (1866 + 243 \oplus 1 + 259 \oplus 2))) + x (-1 + \eta) \eta \\
& (600 \eta^6 \Theta p - 114 \eta t \Theta p - 300 \eta^5 (-5 + 2 \eta t) \Theta p - 12 \eta^4 (53 + 125 \eta t) \Theta p + \\
& 6 \eta ((24 - 53 \eta t) \Theta p + (-1 + \eta t) \Theta l (29 + 2 \Theta p (78 + 27 \oplus 1 + 23 \oplus 2))) + \\
& 2 \eta^3 (8 \times (-285 + 119 \eta t) \Theta p + (-1 + \eta t) \Theta l (28 + \Theta p (598 + 105 \oplus 1 + 113 \oplus 2))) +
\end{aligned}$$

$$\begin{aligned}
& \eta^2 (4 \times (738 + 157 \eta t) \ominus p + 3 \times (-1 + \eta t) \ominus l \\
& \quad (102 + \ominus p (2514 + 351 \oplus 1 + 367 \oplus 2))) - x^2 (-1 + \eta)^2 \\
& (1200 \eta^6 \ominus p - 54 \eta t \ominus p - 120 \eta^5 (-19 + 10 \eta t) \ominus p - 24 \eta^4 (71 + 95 \eta t) \ominus p + \\
& \quad 6 \eta (6 \times (4 - 7 \eta t) \ominus p + (-1 + \eta t) \ominus l (39 + 2 \ominus p (78 + 27 \oplus 1 + 23 \oplus 2))) + \\
& \quad 4 \eta^3 (3 \times (-526 + 275 \eta t) \ominus p + (-1 + \eta t) \ominus l (43 + \ominus p (818 + 111 \oplus 1 + 127 \oplus 2))) + \\
& \quad 3 \eta^2 (6 \times (244 + 27 \eta t) \ominus p + (-1 + \eta t) \ominus l (192 + \ominus p (3810 + 567 \oplus 1 + 583 \oplus 2))) + \\
& \quad x^3 (-1 + \eta)^3 (4 \times (-1 + \eta) \times (-12 + 300 \eta^4 + \eta^2 (186 - 690 \eta t) + \eta^3 \\
& \quad (690 - 300 \eta t) + 24 \eta t - \eta (738 + 5 \eta t)) \ominus p + (-1 + \eta t) \ominus l \\
& \quad (96 + 4 \ominus p (78 + 27 \oplus 1 + 23 \oplus 2) + \eta^2 (216 + \ominus p (4100 + 462 \oplus 1 + 558 \oplus 2)) + \\
& \quad \eta (342 + \ominus p (7698 + 1215 \oplus 1 + 1231 \oplus 2)))) / \\
& (96 (-1 + w (-1 + \eta))^3 (x (-1 + \eta) - \eta)^3 (w + x + \eta - w \eta - x \eta)^3 \\
& \quad (-1 + \\
& \quad \eta t) \ominus p)
\end{aligned}$$

$\delta \lambda p =$

$$\begin{aligned}
& (c \sigma^2 (-1 + \eta) \times (-4 x - 5 x^2 - 4 \eta - 6 x \eta + 10 x^2 \eta - 5 \eta^2 + 10 x \eta^2 - 5 x^2 \eta^2 - 8 x \mu_1 - 8 x^2 \mu_1 - 8 \eta \\
& \quad \mu_1 - 8 x \eta \mu_1 + 15 x^2 \eta \mu_1 - 8 \eta^2 \mu_1 + 14 x \eta^2 \mu_1 - 6 x^2 \eta^2 \mu_1 - \eta^3 \mu_1 + 2 x \eta^3 \mu_1 - \\
& \quad x^2 \eta^3 \mu_1 - 4 x \mu_1^2 - 3 x^2 \mu_1^2 - 4 \eta \mu_1^2 - 2 x \eta \mu_1^2 + 5 x^2 \eta \mu_1^2 - 3 \eta^2 \mu_1^2 + \\
& \quad 4 x \eta^2 \mu_1^2 - x^2 \eta^2 \mu_1^2 - \eta^3 \mu_1^2 + 2 x \eta^3 \mu_1^2 - x^2 \eta^3 \mu_1^2 - 10 x \mu_2 - 6 x^2 \mu_2 - \\
& \quad 11 \eta \mu_2 - 2 x \eta \mu_2 + 12 x^2 \eta \mu_2 - 6 \eta^2 \mu_2 + 12 x \eta^2 \mu_2 - 6 x^2 \eta^2 \mu_2 - 10 x \mu_1 \mu_2 - \\
& \quad 12 x^2 \mu_1 \mu_2 - 11 \eta \mu_1 \mu_2 - 14 x \eta \mu_1 \mu_2 + 18 x^2 \eta \mu_1 \mu_2 - 12 \eta^2 \mu_1 \mu_2 + 12 x \eta^2 \mu_1 \mu_2 - \\
& \quad 6 \eta^3 \mu_1 \mu_2 + 12 x \eta^3 \mu_1 \mu_2 - 6 x^2 \eta^3 \mu_1 \mu_2 - 9 x \mu_2^2 - 9 \eta \mu_2^2 + 9 x \eta \mu_2^2 + \\
& \quad 9 w^3 (-1 + \eta)^3 (\mu_1^2 + (1 + \mu_2)^2 + \mu_1 (2 + 4 \mu_2)) + w^2 (-1 + \eta)^2 (-13 - 24 \mu_1 - 11 \mu_1^2 - \\
& \quad 30 \mu_2 - 36 \mu_1 \mu_2 - 18 \mu_2^2 - \eta (14 + 29 \mu_1 + 15 \mu_1^2 + 23 \mu_2 + 65 \mu_1 \mu_2 + 9 \mu_2^2) + \\
& \quad x (-1 + \eta) \times (14 + 14 \mu_1^2 + 22 \mu_2 + 9 \mu_2^2 + \mu_1 (28 + 58 \mu_2))) + \\
& \quad w (-1 + \eta) ((2 + 2 \mu_1 + 3 \mu_2)^2 + \eta^2 (5 + 7 \mu_1^2 + 6 \mu_2 + 12 \mu_1 (1 + 3 \mu_2)) + \\
& \quad x^2 (-1 + \eta)^2 (5 + 5 \mu_1^2 + 6 \mu_2 + 2 \mu_1 (5 + 12 \mu_2)) + \\
& \quad 2 \eta (9 + 7 \mu_1^2 + 17 \mu_2 + 9 \mu_2^2 + \mu_1 (16 + 23 \mu_2)) - 2 x (-1 + \eta) \times (9 + 7 \mu_1^2 + \\
& \quad 16 \mu_2 + 9 \mu_2^2 + 2 \mu_1 (8 + 11 \mu_2) + \eta (5 + 6 \mu_1^2 + 6 \mu_2 + \mu_1 (11 + 30 \mu_2)))) + \\
& \quad f (-1 + w (-1 + \eta))^2 (w + x + \eta - w \eta - x \eta)^2 \ominus l (2 + \oplus 2)) / (12 x \\
& \quad (-1 + w (-1 + \eta))^2 \\
& \quad (w (-1 + \eta) + x (-1 + \eta) - \eta)^2)
\end{aligned}$$

$\delta \lambda l =$

$$\begin{aligned}
& (c \sigma^2 (-1 + \eta) \times (-5 x - 4 x^2 - 5 \eta - 3 x \eta + 8 x^2 \eta - 4 \eta^2 + 8 x \eta^2 - 4 x^2 \eta^2 - 4 x \mu_1 + 2 x^2 \mu_1 - 4 \eta \\
& \quad \mu_1 + 8 x \eta \mu_1 - 3 x^2 \eta \mu_1 + 2 \eta^2 \mu_1 - 2 x \eta^2 \mu_1 + \eta^3 \mu_1 - 2 x \eta^3 \mu_1 + x^2 \eta^3 \mu_1 + \\
& \quad x \mu_1^2 - 3 x^2 \mu_1^2 + \eta \mu_1^2 - 7 x \eta \mu_1^2 + 7 x^2 \eta \mu_1^2 - 3 \eta^2 \mu_1^2 + 8 x \eta^2 \mu_1^2 - \\
& \quad 5 x^2 \eta^2 \mu_1^2 + \eta^3 \mu_1^2 - 2 x \eta^3 \mu_1^2 + x^2 \eta^3 \mu_1^2 - 2 x \mu_2 - \eta \mu_2 + 2 x \eta \mu_2 - \\
& \quad 8 x \mu_1 \mu_2 - 13 \eta \mu_1 \mu_2 + 8 x \eta \mu_1 \mu_2 + 9 w^3 (-1 + \eta)^3 (1 + 2 \mu_1 \mu_2) + \\
& \quad w (-1 + \eta) \times (5 + x^2 (-1 + \eta)^2 (-2 + \mu_1)^2 + 4 \mu_1 - \mu_1^2 - \eta^2 (-4 + 6 \mu_1 + \mu_1^2) + \\
& \quad 18 \mu_1 \mu_2 + 2 x (-1 + \eta) \times (-9 - 2 \mu_1 - 2 \mu_1^2 + \eta (-4 + 5 \mu_1) - 2 \mu_2 - 8 \mu_1 \mu_2) + \\
& \quad 2 \eta (9 + 2 \mu_1 + 2 \mu_1^2 + \mu_2 + 13 \mu_1 \mu_2)) + w^2 (-1 + \eta)^2 (-14 - 6 \mu_1 - \mu_1^2 - 36 \mu_1 \mu_2 - \\
& \quad \eta (13 - 5 \mu_1 + \mu_2 + 13 \mu_1 \mu_2) + x (-1 + \eta) \times (13 + \mu_1^2 + 2 \mu_2 + \mu_1 (-4 + 8 \mu_2)))) - \\
& \quad f (-1 + w (-1 + \eta))^2 (w + x + \eta - w \eta - x \eta)^2 \ominus l (-4 + \oplus 2)) / \\
& (12 (-1 + w (-1 + \eta))^2 (w (-1 + \eta) + x (-1 + \eta) - \eta)^2)
\end{aligned}$$

$$\delta\Gamma t = \left( 3 f (-1+\eta)^2 \left( 2 x^2 (-1+\eta)^2 \Theta p + (2 \eta^2 + \eta t - w (-1+\eta) \times (2 \eta + \eta t)) \Theta p + \right. \right. \\ \left. \left. x ((-1+w (-1+\eta)) \times (-1+\eta t) \Theta l + 2 (w (-1+\eta) - 2 \eta) (-1+\eta) \Theta p) \right) \right) / \\ (4 \times (-1+w (-1+\eta)) (x (-1+\eta) - \eta) (w (-1+\eta) + x (-1+\eta) - \eta) (-1+\eta t) \Theta p)$$

$$\delta\lambda p t =$$

$$\frac{1}{24 x \Theta l} \left( (2 c \sigma^2 (-1+\eta)^2 \left( x^2 (-1+\eta)^2 \Theta p (5 + 5 \mu 1^2 + 12 \mu 2 + 18 \mu 2^2 + 2 \mu 1 (5 + 6 \mu 2)) + x \right. \right. \\ \left. \left( (w (-1+\eta) - 2 \eta) (-1+\eta) \Theta p (5 + 5 \mu 1^2 + 12 \mu 2 + 18 \mu 2^2 + 2 \mu 1 (5 + 6 \mu 2)) + \right. \right. \\ \left. \left. (-1+w (-1+\eta)) \times (-1+\eta t) \Theta l (4 + 4 \mu 1^2 + 6 \mu 2 + 9 \mu 2^2 + \mu 1 (8 + 6 \mu 2)) \right) + \right. \\ \left. \Theta p (\eta^2 (5 + 5 \mu 1^2 + 12 \mu 2 + 18 \mu 2^2 + 2 \mu 1 (5 + 6 \mu 2)) + \eta t (4 + 4 \mu 1^2 + 6 \mu 2 + 9 \mu 2^2 + \right. \\ \left. \mu 1 (8 + 6 \mu 2)) - w (-1+\eta) (\eta (5 + 5 \mu 1^2 + 12 \mu 2 + 18 \mu 2^2 + 2 \mu 1 (5 + 6 \mu 2)) + \right. \\ \left. \eta t (4 + 4 \mu 1^2 + 6 \mu 2 + 9 \mu 2^2 + \mu 1 (8 + 6 \mu 2))) \right) \right) / \\ ((-1+w (-1+\eta)) (x (-1+\eta) - \eta) (w (-1+\eta) + x (-1+\eta) - \eta) (-1+\eta t) \Theta p) + f \\ \Theta l^2 \Theta p (2 + 5 \mu 2)^2)$$

$$\delta\lambda l t =$$

$$\frac{1}{24} \times \left( (2 c \sigma^2 (-1+\eta)^2 \left( x (w (-1+\eta) - 2 \eta) (-1+\eta) \Theta p (4 + 2 \mu 1 + 7 \mu 1^2) + x^2 (-1+\eta)^2 \Theta p \right. \right. \\ \left. \left. (4 + 2 \mu 1 + 7 \mu 1^2) + \eta^2 \Theta p (4 + 2 \mu 1 + 7 \mu 1^2) + \right. \right. \\ \left. x (-1+w (-1+\eta)) \times (-1+\eta t) \Theta l (5 - 2 \mu 1 + 11 \mu 1^2) + \eta t \Theta p (5 - 2 \mu 1 + 11 \mu 1^2) - \right. \\ \left. w (-1+\eta) \Theta p (\eta (4 + 2 \mu 1 + 7 \mu 1^2) + \eta t (5 - 2 \mu 1 + 11 \mu 1^2)) \right) \right) / \\ ((-1+w (-1+\eta)) (x (-1+\eta) - \eta) (w (-1+\eta) + x (-1+\eta) - \eta) (-1+\eta t) \Theta p) + f \\ \Theta l^2 (8 - 4 \mu 2 + 5 \mu 2^2))$$

$$\delta\Omega =$$

$$(3 f w (-2 x (-1+w (-1+\eta)))^2 \Theta l + 6 x (-1+w (-1+\eta))^2 \eta \Theta l - 6 x (-1+w (-1+\eta))^2 \eta^2 \Theta l + \\ 2 x (-1+w (-1+\eta))^2 \eta^3 \Theta l + 2 x (-1+w (-1+\eta))^2 \eta t \Theta l - \\ 6 x (-1+w (-1+\eta))^2 \eta \eta t \Theta l + 6 x (-1+w (-1+\eta))^2 \eta^2 \eta t \Theta l - \\ 2 x (-1+w (-1+\eta))^2 \eta^3 \eta t \Theta l - 4 (x + \eta - x \eta) (w + x + \eta - w \eta - x \eta)^2 \Theta p + \\ 12 \eta (x + \eta - x \eta) (w + x + \eta - w \eta - x \eta)^2 \Theta p + 4 \eta^3 (x + \eta - x \eta) (w + x + \eta - w \eta - x \eta)^2 \Theta p - \\ 12 (x + \eta - x \eta) (\eta - (-1+w + x) \times (-1+\eta) \eta)^2 \Theta p - 2 (-1+w (-1+\eta))^2 \eta t \Theta p + \\ 6 (-1+w (-1+\eta))^2 \eta \eta t \Theta p - 6 (-1+w (-1+\eta))^2 \eta^2 \eta t \Theta p + \\ 2 (-1+w (-1+\eta))^2 \eta^3 \eta t \Theta p + 4 (x + \eta - x \eta) (w + x + \eta - w \eta - x \eta)^2 (1 - \eta t) \Theta l \Theta p - \\ 8 \eta (x + \eta - x \eta) (w + x + \eta - w \eta - x \eta)^2 (1 - \eta t) \Theta l \Theta p + \\ 4 (x + \eta - x \eta) (\eta - (-1+w + x) \times (-1+\eta) \eta)^2 (1 - \eta t) \Theta l \Theta p + \\ 2 (-1+w (-1+\eta))^2 (x (-1+\eta) - \eta) (-1+\eta t) \Theta l \Theta p - \\ 4 (-1+w (-1+\eta))^2 (x (-1+\eta) - \eta) \eta (-1+\eta t) \Theta l \Theta p + \\ 2 (-1+w (-1+\eta))^2 (x (-1+\eta) - \eta) \eta^2 (-1+\eta t) \Theta l \Theta p + \\ (-1+w (-1+\eta))^2 (x (-1+\eta) - \eta) (-1+\eta t) \Theta l \Theta p \mu 1 - \\ 2 (-1+w (-1+\eta))^2 (x (-1+\eta) - \eta) \eta (-1+\eta t) \Theta l \Theta p \mu 1 + \\ (-1+w (-1+\eta))^2 (x (-1+\eta) - \eta) \eta^2 (-1+\eta t) \Theta l \Theta p \mu 1 + \\ (-1+w (-1+\eta))^2 (x (-1+\eta) - \eta) (-1+\eta t) \Theta l \Theta p \mu 2 - \\ 2 (-1+w (-1+\eta))^2 (x (-1+\eta) - \eta) \eta (-1+\eta t) \Theta l \Theta p \mu 2 + \\ (-1+w (-1+\eta))^2 (x (-1+\eta) - \eta) \eta^2 (-1+\eta t) \Theta l \Theta p \mu 2) \right) / \\ (8 (x (-1+\eta) - \eta) (1+w - w \eta)^2 (w + x + \eta - w \eta - x \eta)^2 (-1+\eta t) \Theta p)$$

$$\begin{aligned}
\ln[\#] := \delta m = & \frac{1}{8 r (w (-1 + \eta) + x (-1 + \eta) - \eta)^2} 3 \times \\
& \left( -12 \times (-1 + r) u (w + x + \eta - w \eta - x \eta)^2 - \frac{1}{(-1 + w (-1 + \eta))^2 (x (-1 + \eta) - \eta) (-1 + \eta t) \theta p} \right. \\
& f (-1 + \eta) \left( (x (-1 + \eta) - \eta) \left( 4 x^2 (-1 + \eta)^2 (-1 + \eta + (-1 + r) \times (-1 + \eta t) \theta l \right) \theta p - x (-1 + \right. \\
& \eta) \times (8 \times (-1 + \eta) \eta \theta p + (-1 + \eta t) \theta l (2 + (-1 + r) \theta p (2 + 8 \eta + \mathfrak{x}1 + \mathfrak{x}2))) + \\
& \theta p (4 \eta^3 - 2 \eta t + 4 \eta^2 (-1 + (-1 + r) \times (-1 + \eta t) \theta l) + \\
& \eta (-((-1 + r) \theta l (2 + \mathfrak{x}1 + \mathfrak{x}2)) + \eta t (2 + (-1 + r) \theta l (2 + \mathfrak{x}1 + \mathfrak{x}2))) \left. \right) + \\
& w^2 (-1 + \eta)^2 \left( x^2 (-1 + \eta)^2 (8 \times (-1 + r) \times (-1 + \eta) \theta p - (-1 + \eta t) \theta l \right. \\
& (2 + \theta p (-10 - \mathfrak{x}1 - \mathfrak{x}2 + r (18 + \mathfrak{x}1 + \mathfrak{x}2))) - 2 x (-1 + \eta) ((-1 + \eta) \times \\
& (-2 + 8 \times (-1 + r) \eta - \eta t) \theta p - (-1 + \eta t) \theta l (2 + \eta - 4 \theta p - \theta p \mathfrak{x}1 - \theta p \mathfrak{x}2 - \\
& \eta \theta p (10 + \mathfrak{x}1 + \mathfrak{x}2) + r (-2 + 2 \theta p (3 + \mathfrak{x}1 + \mathfrak{x}2) + \eta \theta p (18 + \mathfrak{x}1 + \mathfrak{x}2))) + \\
& \theta p (8 \times (-1 + r) \eta^3 - 4 \times (-1 + r) \eta t + \eta^2 (4 - 10 \theta l - \theta l \mathfrak{x}1 - \theta l \mathfrak{x}2 + \\
& \eta t (-2 + \theta l (10 + \mathfrak{x}1 + \mathfrak{x}2)) + r (-8 - (-1 + \eta t) \theta l (18 + \mathfrak{x}1 + \mathfrak{x}2))) - \\
& 2 \eta (-2 + \theta l (4 + \mathfrak{x}1 + \mathfrak{x}2 - 2 r (3 + \mathfrak{x}1 + \mathfrak{x}2)) + \eta t \\
& (1 - \theta l (4 + \mathfrak{x}1 + \mathfrak{x}2) + 2 r (-1 + \theta l (3 + \mathfrak{x}1 + \mathfrak{x}2)))) \left. \right) + \\
& w (-1 + \eta) \times \left( 4 x^3 (-1 + \eta)^3 (1 - \eta - \theta l + \eta t \theta l + r (-1 + \eta + 2 \theta l - 2 \eta t \theta l)) \theta p - \right. \\
& 2 x^2 (-1 + \eta)^2 (2 \times (-1 + \eta) \times (-2 + 3 \times (-1 + r) \eta) \theta p - \\
& (-1 + \eta t) \theta l (2 + \theta p (-6 - 6 \eta - \mathfrak{x}1 - \mathfrak{x}2 + r (6 + 12 \eta + \mathfrak{x}1 + \mathfrak{x}2)))) + \theta p \\
& (-4 \times (-1 + r) \eta^4 + 2 \times (-1 + r) \eta t + 4 \eta^3 (1 + r + \theta l + 2 r (-1 + \eta t) \theta l - \eta t \theta l) + \\
& 2 \eta^2 (-4 - (-1 + r) \theta l (6 + \mathfrak{x}1 + \mathfrak{x}2) + \eta t (2 + (-1 + r) \theta l (6 + \mathfrak{x}1 + \mathfrak{x}2))) + \\
& \eta (-((-1 + 2 r) \theta l (2 + \mathfrak{x}1 + \mathfrak{x}2)) + \\
& \eta t (-2 - \theta l (2 + \mathfrak{x}1 + \mathfrak{x}2) + 2 r (-1 + \theta l (2 + \mathfrak{x}1 + \mathfrak{x}2)))) \left. \right) + \\
& x (-1 + \eta) \times \left( 4 \times (-1 + \eta) \times (-4 \eta + 3 \times (-1 + r) \eta^2 - \eta t) \theta p - \right. \\
& (-1 + \eta t) \theta l (2 + 4 \eta - 2 \theta p - 12 \eta^2 \theta p - \theta p \mathfrak{x}1 - \theta p \mathfrak{x}2 - 4 \eta \theta p (6 + \mathfrak{x}1 + \mathfrak{x}2) + \\
& 2 r (-1 + \theta p (2 + 12 \eta^2 + \mathfrak{x}1 + \mathfrak{x}2 + 2 \eta (6 + \mathfrak{x}1 + \mathfrak{x}2)))) \left. \right) + \\
& w^3 (-1 + \eta)^3 \left( x (-1 + \eta) \times (4 \times (-1 + r) \times (-1 + \eta) \theta p - (-1 + \eta t) \theta l \right. \\
& (2 - \theta p (6 + \mathfrak{x}1 + \mathfrak{x}2) + 2 r (-1 + \theta p (6 + \mathfrak{x}1 + \mathfrak{x}2))) + \theta p (-4 \times (-1 + r) \eta^2 + \\
& 2 \times (-1 + r) \eta t + \eta (-4 + 2 \eta t + 6 \theta l + \theta l \mathfrak{x}1 + \theta l \mathfrak{x}2 - \eta t \theta l (6 + \mathfrak{x}1 + \mathfrak{x}2) + \\
& 2 r (2 - \theta l (6 + \mathfrak{x}1 + \mathfrak{x}2) + \eta t (-1 + \theta l (6 + \mathfrak{x}1 + \mathfrak{x}2)))) \left. \right) \left. \right)
\end{aligned}$$

$$\begin{aligned}
& \text{Out}[*]= \frac{1}{8 r (w (-1+\eta) + x (-1+\eta) - \eta)^2} \\
& 3 \times \left( -12 \times (-1+r) u (w+x+\eta-w\eta-x\eta)^2 - \frac{1}{(-1+w(-1+\eta))^2 (x(-1+\eta)-\eta) (-1+\eta t) \theta p} \right. \\
& \quad f(-1+\eta) \left( (x(-1+\eta)-\eta) \left( 4x^2(-1+\eta)^2 (-1+\eta+(-1+r) \times (-1+\eta t) \theta l) \theta p - x(-1+\eta) \right. \right. \\
& \quad \quad \eta) \times (8 \times (-1+\eta) \eta \theta p + (-1+\eta t) \theta l (2+(-1+r) \theta p (2+8\eta+\mathfrak{E}1+\mathfrak{E}2))) + \\
& \quad \quad \theta p (4\eta^3-2\eta t+4\eta^2(-1+(-1+r) \times (-1+\eta t) \theta l) + \\
& \quad \quad \quad \eta(-((-1+r) \theta l (2+\mathfrak{E}1+\mathfrak{E}2)) + \eta t (2+(-1+r) \theta l (2+\mathfrak{E}1+\mathfrak{E}2))) \left. \right) \left. \right) + \\
& \quad w^2 (-1+\eta)^2 \left( x^2 (-1+\eta)^2 (8 \times (-1+r) \times (-1+\eta) \theta p - (-1+\eta t) \theta l \right. \\
& \quad \quad (2+\theta p (-10-\mathfrak{E}1-\mathfrak{E}2+r (18+\mathfrak{E}1+\mathfrak{E}2))) - 2x(-1+\eta) ((-1+\eta) \times \\
& \quad \quad (-2+8 \times (-1+r) \eta - \eta t) \theta p - (-1+\eta t) \theta l (2+\eta-4\theta p-\theta p \mathfrak{E}1-\theta p \mathfrak{E}2- \\
& \quad \quad \eta \theta p (10+\mathfrak{E}1+\mathfrak{E}2) + r (-2+2\theta p (3+\mathfrak{E}1+\mathfrak{E}2) + \eta \theta p (18+\mathfrak{E}1+\mathfrak{E}2))) + \\
& \quad \quad \theta p (8 \times (-1+r) \eta^3-4 \times (-1+r) \eta t + \eta^2 (4-10\theta l-\theta l \mathfrak{E}1-\theta l \mathfrak{E}2+ \\
& \quad \quad \eta t (-2+\theta l (10+\mathfrak{E}1+\mathfrak{E}2)) + r (-8-(-1+\eta t) \theta l (18+\mathfrak{E}1+\mathfrak{E}2))) - \\
& \quad \quad 2\eta (-2+\theta l (4+\mathfrak{E}1+\mathfrak{E}2-2r (3+\mathfrak{E}1+\mathfrak{E}2))) + \\
& \quad \quad \left. \eta t (1-\theta l (4+\mathfrak{E}1+\mathfrak{E}2) + 2r (-1+\theta l (3+\mathfrak{E}1+\mathfrak{E}2))) \right) \left. \right) + \\
& \quad w(-1+\eta) \times \left( 4x^3(-1+\eta)^3 (1-\eta-\theta l+\eta t \theta l+r(-1+\eta+2\theta l-2\eta t \theta l)) \theta p - \right. \\
& \quad 2x^2(-1+\eta)^2 (2 \times (-1+\eta) \times (-2+3 \times (-1+r) \eta) \theta p - \\
& \quad \quad (-1+\eta t) \theta l (2+\theta p (-6-6\eta-\mathfrak{E}1-\mathfrak{E}2+r (6+12\eta+\mathfrak{E}1+\mathfrak{E}2)))) + \theta p \\
& \quad \quad (-4 \times (-1+r) \eta^4+2 \times (-1+r) \eta t+4\eta^3 (1+r+\theta l+2r(-1+\eta t) \theta l-\eta t \theta l) + \\
& \quad \quad 2\eta^2 (-4-(-1+r) \theta l (6+\mathfrak{E}1+\mathfrak{E}2) + \eta t (2+(-1+r) \theta l (6+\mathfrak{E}1+\mathfrak{E}2))) + \\
& \quad \quad \eta(-((-1+2r) \theta l (2+\mathfrak{E}1+\mathfrak{E}2)) + \\
& \quad \quad \left. \eta t (-2-\theta l (2+\mathfrak{E}1+\mathfrak{E}2) + 2r (-1+\theta l (2+\mathfrak{E}1+\mathfrak{E}2))) \right) \left. \right) + \\
& \quad x(-1+\eta) \times \left( 4 \times (-1+\eta) \times (-4\eta+3 \times (-1+r) \eta^2-\eta t) \theta p - \right. \\
& \quad \quad (-1+\eta t) \theta l (2+4\eta-2\theta p-12\eta^2\theta p-\theta p \mathfrak{E}1-\theta p \mathfrak{E}2-4\eta \theta p (6+\mathfrak{E}1+\mathfrak{E}2) + \\
& \quad \quad 2r (-1+\theta p (2+12\eta^2+\mathfrak{E}1+\mathfrak{E}2+2\eta (6+\mathfrak{E}1+\mathfrak{E}2)))) \left. \right) \left. \right) + \\
& \quad w^3 (-1+\eta)^3 \left( x(-1+\eta) \times (4 \times (-1+r) \times (-1+\eta) \theta p - (-1+\eta t) \theta l \right. \\
& \quad \quad (2-\theta p (6+\mathfrak{E}1+\mathfrak{E}2) + 2r (-1+\theta p (6+\mathfrak{E}1+\mathfrak{E}2))) + \theta p (-4 \times (-1+r) \eta^2 + \\
& \quad \quad 2 \times (-1+r) \eta t + \eta (-4+2\eta t+6\theta l+\theta l \mathfrak{E}1+\theta l \mathfrak{E}2-\eta t \theta l (6+\mathfrak{E}1+\mathfrak{E}2) + \\
& \quad \quad \left. 2r (2-\theta l (6+\mathfrak{E}1+\mathfrak{E}2) + \eta t (-1+\theta l (6+\mathfrak{E}1+\mathfrak{E}2)))) \right) \left. \right) \left. \right) \left. \right) \left. \right)
\end{aligned}$$

$$\delta g\psi = - \frac{f w (-1+\eta)^2 (-1+\eta+\theta l-\eta t \theta l)}{2 (-1+w(-1+\eta))^2 (-1+\eta t)}$$

$$\begin{aligned}
\delta g_s = - & \left( (-1+\eta) \times \right. \\
& (-2 f (-1+w(-1+\eta)) (x(-1+\eta)-\eta) (w(-1+\eta)+x(-1+\eta)-\eta) (1+x+\eta-x\eta)^2 \\
& \quad \theta l (x^2 (-1+\eta)^2 \theta p (12+8\eta t-12\theta l+12\eta t \theta l+2\eta (-14-\theta l (-4+\mathfrak{E}2) + \\
& \quad \quad \eta t (1+\theta l) \times (-4+\mathfrak{E}2)-\mathfrak{E}2)-4\eta^2 (-4+\mathfrak{E}2)+6\mathfrak{E}2- \\
& \quad \quad 2\eta t \mathfrak{E}2-4\theta l \mathfrak{E}2+4\eta t \theta l \mathfrak{E}2-5\theta l \mathfrak{E}2^2+5\eta t \theta l \mathfrak{E}2^2+ \\
& \quad \quad w(-1+\eta) \times (2\eta^2 (-4+\mathfrak{E}2) + \eta (4-2\eta t (-4+\mathfrak{E}2) + 8\mathfrak{E}2) + (-2+5\mathfrak{E}2) \times \\
& \quad \quad (-2+\theta l (2+\mathfrak{E}2)) + \eta t (2 \times (-4+\mathfrak{E}2) + \theta l (4-8\mathfrak{E}2-5\mathfrak{E}2^2)))) \left. \right) \left. \right) + \\
& \theta p (12\eta^2-28\eta^3+16\eta^4+4\eta t-4\eta \eta t+8\eta^2 \eta t-8\eta^3 \eta t-4\eta \theta l- \\
& \quad 12\eta^2 \theta l+8\eta^3 \theta l+4\eta \eta t \theta l+12\eta^2 \eta t \theta l-8\eta^3 \eta t \theta l+6\eta^2 \mathfrak{E}2- \\
& \quad 2\eta^3 \mathfrak{E}2-4\eta^4 \mathfrak{E}2-10\eta t \mathfrak{E}2+10\eta \eta t \mathfrak{E}2-2\eta^2 \eta t \mathfrak{E}2+2\eta^3 \eta t \mathfrak{E}2+
\end{aligned}$$



$$\begin{aligned}
& 8 \eta \theta l \mathfrak{z} 2 - 4 \eta^2 \theta l \mathfrak{z} 2 - 2 \eta^3 \theta l \mathfrak{z} 2 - 8 \eta \eta t \theta l \mathfrak{z} 2 + 4 \eta^2 \eta t \theta l \mathfrak{z} 2 + \\
& 2 \eta^3 \eta t \theta l \mathfrak{z} 2 + 5 \eta \theta l \mathfrak{z} 2^2 - 5 \eta^2 \theta l \mathfrak{z} 2^2 - 5 \eta \eta t \theta l \mathfrak{z} 2^2 + \\
& 5 \eta^2 \eta t \theta l \mathfrak{z} 2^2 - 2 w^2 (-1 + \eta)^3 (\eta - \eta t) (-2 + \eta (-4 + \mathfrak{z} 2) + 5 \mathfrak{z} 2) + \\
& w (-1 + \eta) \times (-2 \eta^3 (6 + \eta t (-4 + \mathfrak{z} 2) - 6 \mathfrak{z} 2) + 2 \eta^4 (-4 + \mathfrak{z} 2) + 4 \eta t \\
& \quad (-2 + 5 \mathfrak{z} 2) + \eta^2 (-8 \times (-4 + \mathfrak{z} 2) - (-1 + \eta t) \theta l (-12 + 10 \mathfrak{z} 2 + 5 \mathfrak{z} 2^2))) + \\
& \quad \eta (-6 \times (2 + \mathfrak{z} 2 + 3 \eta t \mathfrak{z} 2) + (-1 + \eta t) \theta l (-20 + 12 \mathfrak{z} 2 + 5 \mathfrak{z} 2^2))) - \\
& \times (-1 + \eta) \times (-2 (w (-1 + \eta) - 2 \eta) (-1 + \eta) \theta p (-6 - 4 \eta t - 2 \eta (-4 + \mathfrak{z} 2) - \\
& \quad 3 \mathfrak{z} 2 + \eta t \mathfrak{z} 2 + w (-1 + \eta) \times (-2 + 4 \eta t + \eta (-4 + \mathfrak{z} 2) + 5 \mathfrak{z} 2 - \eta t \mathfrak{z} 2)) + \\
& \quad (-1 + \eta t) \theta l (-4 + 10 \mathfrak{z} 2 + 2 w^2 (-1 + \eta)^2 (-2 + 5 \mathfrak{z} 2) + \\
& \quad \theta p (4 + 4 \eta^2 (-4 + \mathfrak{z} 2) - 8 \mathfrak{z} 2 - 5 \mathfrak{z} 2^2 + 2 \eta (12 + 4 \mathfrak{z} 2 + 5 \mathfrak{z} 2^2))) - w (-1 + \eta) \times \\
& \quad (-8 + 20 \mathfrak{z} 2 + \theta p (20 - 12 \mathfrak{z} 2 - 5 \mathfrak{z} 2^2 + 2 \eta (-8 + 9 \mathfrak{z} 2 + 5 \mathfrak{z} 2^2)))) + \\
& cv \, c\sigma (x (-1 + \eta) - \eta) (1 + x + \eta - x \eta)^2 ((x + \eta - x \eta)^2 (-1 + \eta t) \theta l \theta p \\
& \quad (1 + \mu 1) \times (14 x (-1 + \eta) - 14 \eta - 5 \times (2 + \mathfrak{z} 1 + \mathfrak{z} 2)) + \\
& w (-1 + \eta) \times (-4 x^3 (-1 + \eta)^3 \theta p (1 - 8 \theta l + 7 \mu 1 - 14 \theta l \mu 1 + 3 \eta^2 (1 + \mu 1) - \\
& \quad \eta \eta t (1 + 2 \theta l) \times (1 + \mu 1) + 2 \eta (-2 + \theta l - 5 \mu 1 + \theta l \mu 1) + \\
& \quad \eta t (1 + 8 \theta l + \mu 1 + 14 \theta l \mu 1)) + x^2 (-1 + \eta)^2 \theta p (36 \eta^3 (1 + \mu 1) - \\
& \quad 12 \eta^2 (\eta t (1 + 2 \theta l) \times (1 + \mu 1) - 2 \times (-2 + \theta l - 5 \mu 1 + \theta l \mu 1)) + \\
& \quad 12 \eta (1 + 7 \mu 1 - 2 \theta l (4 + 7 \mu 1) + \eta t (1 + \mu 1 + 2 \theta l (4 + 7 \mu 1))) + \\
& \quad (-1 + \eta t) \theta l (1 + \mu 1) \times (58 + 15 \mathfrak{z} 1 + 15 \mathfrak{z} 2)) - \\
& \times (-1 + \eta) \times (12 \times (-1 + \eta) \eta^2 \theta p (-1 - 7 \mu 1 + 3 \eta (1 + \mu 1) - \eta t (1 + \mu 1)) - \\
& \quad (-1 + \eta t) \theta l (20 \times (1 + \mu 1) + \theta p (24 \eta^3 (1 + \mu 1) - 24 \eta^2 (4 + 7 \mu 1) + \\
& \quad 5 \times (-6 - 3 \mathfrak{z} 1 + \mathfrak{z} 2) - 2 \eta (1 + \mu 1) \times (58 + 15 \mathfrak{z} 1 + 15 \mathfrak{z} 2) - \\
& \quad \mu 1 (30 + 15 \mathfrak{z} 1 + 19 \mathfrak{z} 2)))) + \theta p (12 \eta^5 (1 + \mu 1) + 20 \eta t (1 + \mu 1) - \\
& \quad 4 \eta^4 (\eta t (1 + 2 \theta l) \times (1 + \mu 1) - 2 \times (-2 + \theta l - 5 \mu 1 + \theta l \mu 1)) + \\
& \quad 4 \eta^3 (1 + 7 \mu 1 - 2 \theta l (4 + 7 \mu 1) + \eta t (1 + \mu 1 + 2 \theta l (4 + 7 \mu 1))) + \\
& \quad \eta^2 (-1 + \eta t) \theta l (1 + \mu 1) \times (58 + 15 \mathfrak{z} 1 + 15 \mathfrak{z} 2) + \\
& \quad \eta (-20 \eta t (1 + \mu 1) - 5 \theta l (6 + 3 \mathfrak{z} 1 - \mathfrak{z} 2) - \theta l \mu 1 (30 + 15 \mathfrak{z} 1 + 19 \mathfrak{z} 2) + \\
& \quad \eta t \theta l (5 \times (6 + 3 \mathfrak{z} 1 - \mathfrak{z} 2) + \mu 1 (30 + 15 \mathfrak{z} 1 + 19 \mathfrak{z} 2)))) + w^4 (-1 + \eta)^4 \\
& (x (-1 + \eta) \times (4 \times (-1 + \eta) \theta p (1 - 5 \mu 1 + \eta (1 + \mu 1) - \eta t (1 + \mu 1)) + (-1 + \eta t) \\
& \quad \theta l (-20 \times (1 + \mu 1) + 5 \theta p (8 + 3 \mathfrak{z} 1 - \mathfrak{z} 2) + \theta p \mu 1 (64 + 15 \mathfrak{z} 1 + 19 \mathfrak{z} 2))) + \\
& \theta p (-4 \eta^3 (1 + \mu 1) - 20 \eta t (1 + \mu 1) + 4 \eta^2 (\eta t + 6 \mu 1 + \eta t \mu 1) + \eta (4 - 20 \mu 1 + \\
& \quad 16 \eta t (1 + \mu 1) + \theta l (40 + 64 \mu 1 + 15 \mathfrak{z} 1 + 15 \mu 1 \mathfrak{z} 1 - 5 \mathfrak{z} 2 + 19 \mu 1 \mathfrak{z} 2) - \\
& \quad \eta t \theta l (5 \times (8 + 3 \mathfrak{z} 1 - \mathfrak{z} 2) + \mu 1 (64 + 15 \mathfrak{z} 1 + 19 \mathfrak{z} 2)))) + \\
& w^2 (-1 + \eta)^2 (2 x^3 (-1 + \eta)^3 \theta p (-2 - 5 \theta l + 10 \mu 1 - 17 \theta l \mu 1 + 2 \eta^2 \\
& \quad (1 + \mu 1) - 2 \eta (\eta t + 6 \mu 1 + \eta t \mu 1) + \eta t (2 + 5 \theta l + 2 \mu 1 + 17 \theta l \mu 1)) - \\
& x^2 (-1 + \eta)^2 \theta p (8 - 94 \theta l + 56 \mu 1 - 142 \theta l \mu 1 + 12 \eta^3 (1 + \mu 1) + \\
& \quad 8 \eta t (1 + \mu 1) - 12 \eta^2 (-2 + \eta t + 4 \mu 1 + \eta t \mu 1) + \\
& \quad 2 \eta (-22 - 7 \theta l - 10 \mu 1 - 43 \theta l \mu 1 + \eta t (2 + 7 \theta l + 2 \mu 1 + 43 \theta l \mu 1)) - \\
& \quad 15 \theta l \mathfrak{z} 1 - 15 \theta l \mu 1 \mathfrak{z} 1 - 15 \theta l \mathfrak{z} 2 - 15 \theta l \mu 1 \mathfrak{z} 2 + \\
& \quad \eta t \theta l (94 + 15 \mathfrak{z} 1 + 15 \mathfrak{z} 2 + \mu 1 (142 + 15 \mathfrak{z} 1 + 15 \mathfrak{z} 2))) + \\
& \times (-1 + \eta) \times (4 \times (-1 + \eta) \eta \theta p (3 \eta^2 (1 + \mu 1) - 3 \eta (-5 + \eta t + \mu 1 + \eta t \mu 1) - \\
& \quad 4 \times (1 + \eta t + 7 \mu 1 + \eta t \mu 1)) + (-1 + \eta t) \theta l (-60 \times (1 + \mu 1) + \\
& \quad \theta p (104 + \eta^2 (-2 + 70 \mu 1) + 45 \mathfrak{z} 1 - 15 \mathfrak{z} 2 + \mu 1 (104 + 45 \mathfrak{z} 1 + 57 \mathfrak{z} 2) + \\
& \quad 2 \eta (94 + 15 \mathfrak{z} 1 + 15 \mathfrak{z} 2 + \mu 1 (142 + 15 \mathfrak{z} 1 + 15 \mathfrak{z} 2)))) +
\end{aligned}$$

$$\begin{aligned}
& \theta p \left( -4 \eta^5 (1 + \mu_1) - 60 \eta t (1 + \mu_1) + 4 \eta^4 (-6 + \eta t + \eta t \mu_1) + \right. \\
& \quad \eta^3 (36 + 60 \mu_1 + 6 \theta l (-1 + 3 \mu_1) + \eta t (4 + 6 \theta l + 4 \mu_1 - 18 \theta l \mu_1)) + \\
& \quad \eta (60 \eta t (1 + \mu_1) + \theta l (104 + 45 \mathfrak{z}_1 - 15 \mathfrak{z}_2 + \mu_1 (104 + 45 \mathfrak{z}_1 + 57 \mathfrak{z}_2)) - \\
& \quad \quad \eta t \theta l (104 + 45 \mathfrak{z}_1 - 15 \mathfrak{z}_2 + \mu_1 (104 + 45 \mathfrak{z}_1 + 57 \mathfrak{z}_2))) - \eta^2 (8 + \\
& \quad \quad 56 \mu_1 - \theta l (94 + 15 \mathfrak{z}_1 + 15 \mathfrak{z}_2 + \mu_1 (142 + 15 \mathfrak{z}_1 + 15 \mathfrak{z}_2)) + \eta t (8 \times (1 + \\
& \quad \quad \mu_1) + \theta l (94 + 15 \mathfrak{z}_1 + 15 \mathfrak{z}_2 + \mu_1 (142 + 15 \mathfrak{z}_1 + 15 \mathfrak{z}_2)))) \Big) + \\
& w^3 (-1 + \eta)^3 \left( x^2 (-1 + \eta)^2 \theta p \left( -8 - 30 \theta l + 40 \mu_1 - 78 \theta l \mu_1 + 8 \eta^2 (1 + \mu_1) - \right. \right. \\
& \quad 8 \eta (\eta t + 6 \mu_1 + \eta t \mu_1) - 5 \theta l \mathfrak{z}_1 - 5 \theta l \mu_1 \mathfrak{z}_1 - 5 \theta l \mathfrak{z}_2 - 5 \theta l \mu_1 \mathfrak{z}_2 + \\
& \quad \eta t (8 \times (1 + \mu_1) + 5 \theta l (6 + \mathfrak{z}_1 + \mathfrak{z}_2) + \theta l \mu_1 (78 + 5 \mathfrak{z}_1 + 5 \mathfrak{z}_2))) - \\
& \quad \times (-1 + \eta) \times \left( 4 \times (-1 + \eta) \theta p \left( -1 - 7 \mu_1 + 4 \eta^2 (1 + \mu_1) - \eta t (1 + \mu_1) - \right. \right. \\
& \quad \quad \eta (-7 + 17 \mu_1 + 4 \eta t (1 + \mu_1))) + (-1 + \eta t) \theta l \\
& \quad \quad (-60 \times (1 + \mu_1) + \theta p (122 + 45 \mathfrak{z}_1 - 15 \mathfrak{z}_2 + \mu_1 (146 + 45 \mathfrak{z}_1 + 57 \mathfrak{z}_2) + \\
& \quad \quad 2 \eta (26 + 5 \mathfrak{z}_1 + 5 \mathfrak{z}_2 + \mu_1 (74 + 5 \mathfrak{z}_1 + 5 \mathfrak{z}_2)))) \Big) + \\
& \theta p \left( 8 \eta^4 (1 + \mu_1) + 60 \eta t (1 + \mu_1) - 4 \eta^3 (-3 + 9 \mu_1 + 2 \eta t (1 + \mu_1)) + \right. \\
& \quad \eta^2 (-24 - \theta l (22 + 5 \mathfrak{z}_1 + 5 \mathfrak{z}_2 + 5 \mu_1 (14 + \mathfrak{z}_1 + \mathfrak{z}_2)) + \\
& \quad \quad \eta t (4 \times (1 + \mu_1) + \theta l (22 + 5 \mathfrak{z}_1 + 5 \mathfrak{z}_2 + 5 \mu_1 (14 + \mathfrak{z}_1 + \mathfrak{z}_2)))) + \\
& \quad \eta (4 + 28 \mu_1 - \theta l (122 + 45 \mathfrak{z}_1 - 15 \mathfrak{z}_2 + \mu_1 (146 + 45 \mathfrak{z}_1 + 57 \mathfrak{z}_2)) + \\
& \quad \quad \eta t (-56 \times (1 + \mu_1) + \theta l (122 + 45 \mathfrak{z}_1 - 15 \mathfrak{z}_2 + \\
& \quad \quad \mu_1 (146 + 45 \mathfrak{z}_1 + 57 \mathfrak{z}_2)))) \Big) + \\
& 2 c \sigma^2 (-1 + \eta) \times \left( 2 x^6 (-1 + \eta)^6 \theta p \left( 2 - 2 \theta l - 9 \mu_1 - 15 w \mu_1 - 4 w^2 \mu_1 + \right. \right. \\
& \quad 5 \theta l \mu_1 + 7 w \theta l \mu_1 - 5 \mu_1^2 - 9 w \mu_1^2 - 4 w^2 \mu_1^2 + \theta l \mu_1^2 + \\
& \quad w \theta l \mu_1^2 + w^2 \eta^4 (1 + \mu_1) - w \eta^3 (3 + w (3 + \eta t - 4 \mu_1)) \times (1 + \mu_1) + \\
& \quad \eta^2 (2 \times (1 + \mu_1) + 3 w^2 (1 + \eta t - 4 \mu_1) \times (1 + \mu_1) + \\
& \quad \quad 3 w (2 + \eta t - 3 \mu_1 + \eta t \mu_1 - 3 \mu_1^2)) + \eta t (2 \times (1 + \mu_1) + w^2 (1 + \mu_1) - \\
& \quad \quad \theta l (-2 + 5 \mu_1 + \mu_1^2) + w (3 + (3 - 7 \theta l) \mu_1 - \theta l \mu_1^2)) - \\
& \quad \eta (4 + 2 \eta t - 7 \mu_1 + 2 \eta t \mu_1 - 5 \mu_1^2 + w^2 (1 + 3 \eta t - 12 \mu_1) \times (1 + \mu_1) + w (3 + \\
& \quad \quad (-27 + 7 \theta l) \mu_1 + (-18 + \theta l) \mu_1^2 + \eta t (6 + (6 - 7 \theta l) \mu_1 - \theta l \mu_1^2))) \Big) + \\
& \theta p \left( w^4 (-1 + \eta)^5 \left( 2 \eta^5 (1 + \mu_1) + 2 \eta \eta t (\mu_1^2 + 5 \mu_1 (-2 + \mu_2) + 5 \times (-1 + \mu_2)) - \right. \right. \\
& \quad 2 \eta^4 (-2 - 4 \mu_1^2 + \eta t (1 + \mu_1) + 6 \mu_1 (-1 + \mu_2)) + 5 \eta t (1 + \mu_1) \mu_2 + \\
& \quad 2 \eta^3 (6 + 7 \mu_1^2 - 13 \mu_1 (-1 + \mu_2) + 11 \mu_2 + \eta t (-2 + \mu_1 (-2 + 6 \mu_2))) + \\
& \quad \eta^2 (2 \times (5 + 3 \mu_1^2 + 11 \mu_2 + \mu_1 (8 + 5 \mu_2)) + \\
& \quad \quad \eta t (-12 + 26 \mu_1^2 + 5 \mu_2 + \mu_1 (-22 + 17 \mu_2))) \Big) - w^3 (-1 + \eta)^3 \\
& \quad \left( 4 \eta^7 (1 + \mu_1) + 2 \eta^6 (5 + 8 \mu_1^2 - 2 \eta t (1 + \mu_1) + \mu_1 (13 - 12 \mu_2)) - \right. \\
& \quad 2 \eta \eta t (4 \mu_1^2 + 5 \times (-4 + \mu_2) + 17 \mu_1 (-2 + \mu_2)) - 15 \eta t (1 + \mu_1) \mu_2 + \\
& \quad 2 \eta^5 (11 + 15 \mu_1^2 - 32 \mu_1 (-1 + \mu_2) + 22 \mu_2 + \eta t (-5 + \mu_1 (-5 + 12 \mu_2))) - \\
& \quad \eta^2 (10 \mu_1^2 + \eta t (-26 + 60 \mu_1^2 + 5 \theta l \mathfrak{z}_1 + \mu_2 (-24 + 5 \theta l (\mathfrak{z}_1 - \mathfrak{z}_2)) + \\
& \quad \quad \mu_1 (-62 + \mu_2 (48 + 5 \theta l (\mathfrak{z}_1 - \mathfrak{z}_2)) + 11 \theta l (\mathfrak{z}_1 - \mathfrak{z}_2)) - 5 \theta l \mathfrak{z}_2) + \\
& \quad \quad \mu_1 (62 - 11 \theta l (\mathfrak{z}_1 - \mathfrak{z}_2) + \mu_2 (12 - 5 \theta l \mathfrak{z}_1 + 5 \theta l \mathfrak{z}_2)) + \\
& \quad \quad 5 \times (8 + \theta l (-\mathfrak{z}_1 + \mathfrak{z}_2) + \mu_2 (12 + \theta l (-\mathfrak{z}_1 + \mathfrak{z}_2))) \Big) + \\
& \quad 2 \eta^3 (-13 - 15 \mu_1^2 - 26 \mu_2 + 5 \theta l \mathfrak{z}_1 + 5 \theta l \mu_2 \mathfrak{z}_1 + \mu_1 (-34 + \\
& \quad \quad \mu_2 (52 + 5 \theta l (\mathfrak{z}_1 - \mathfrak{z}_2)) + 11 \theta l (\mathfrak{z}_1 - \mathfrak{z}_2)) - 5 \theta l \mathfrak{z}_2 - 5 \theta l \mu_2 \mathfrak{z}_2 + \\
& \quad \eta t (24 \mu_1^2 - 11 \mu_1 (3 + \theta l (\mathfrak{z}_1 - \mathfrak{z}_2)) + \mu_1 \mu_2 (5 - 5 \theta l \mathfrak{z}_1 + 5 \theta l \mathfrak{z}_2) + \\
& \quad \quad 5 \times (-3 + \mu_2 + \theta l (-\mathfrak{z}_1 + \mathfrak{z}_2) + \theta l \mu_2 (-\mathfrak{z}_1 + \mathfrak{z}_2))) \Big) + \\
& \quad \eta^4 (30 - 6 \mu_1^2 + 68 \mu_2 + 5 \theta l \mathfrak{z}_1 + 5 \theta l \mu_2 \mathfrak{z}_1 + \mu_1 (36 + \mu_2
\end{aligned}$$

$$\begin{aligned}
& (-4 + 5 \, \theta l \, (\mathfrak{h}1 - \mathfrak{h}2)) + 11 \, \theta l \, (\mathfrak{h}1 - \mathfrak{h}2)) - 5 \, \theta l \, \mathfrak{h}2 - 5 \, \theta l \, \mu 2 \, \mathfrak{h}2 + \\
& \eta t \, (-22 + 20 \, \mu 1^2 - 5 \, \theta l \, \mathfrak{h}1 + 5 \, \theta l \, \mathfrak{h}2 + \mu 2 \, (-9 - 5 \, \theta l \, \mathfrak{h}1 + 5 \, \theta l \, \mathfrak{h}2) + \\
& \mu 1 \, (-50 - 11 \, \theta l \, \mathfrak{h}1 + 11 \, \theta l \, \mathfrak{h}2 + \mu 2 \, (63 - 5 \, \theta l \, \mathfrak{h}1 + 5 \, \theta l \, \mathfrak{h}2))) + \\
& \eta \, (4 \, \eta^7 \, (1 + \mu 1) + \eta t \, (-2 \, \mu 1^2 + \mu 1 \, (8 - 19 \, \mu 2) + 5 \times (2 + \mu 2)) - \\
& 2 \, \eta^6 \, (2 \, \eta t \, (1 + \mu 1) + \mu 1 \, (-11 - 5 \, \mu 1 + 12 \, \mu 2)) + \\
& \eta^5 \, (2 + 22 \, \mu 1 + 8 \, \mu 1^2 + 22 \, \mu 2 - 14 \, \mu 1 \, \mu 2 + 4 \, \eta t \, (-1 + \mu 1^2 + 3 \, \mu 1 \, \mu 2) + \\
& \theta l \, (2 \times (-2 + \mu 2) + \mu 1^2 \, (4 + \mathfrak{h}1 + \mathfrak{h}2) + \mu 1 \, (12 - 10 \, \mu 2 + \mathfrak{h}1 + \mathfrak{h}2)) - \\
& \eta t \, \theta l \, (2 \times (-2 + \mu 2) + \mu 1^2 \, (4 + \mathfrak{h}1 + \mathfrak{h}2) + \mu 1 \, (12 - 10 \, \mu 2 + \mathfrak{h}1 + \mathfrak{h}2))) - \\
& \eta^3 \, (6 + 26 \, \mu 1 + 8 \, \mu 1^2 + 30 \, \mu 2 - 30 \, \mu 1 \, \mu 2 - \theta l \, (6 + 5 \times (1 + \mu 2) \, \mathfrak{h}1 + \\
& \mu 1 \, (-4 + 21 \, \mathfrak{h}1 + \mu 2 \, (36 + 5 \, \mathfrak{h}1 - 17 \, \mathfrak{h}2) - 15 \, \mathfrak{h}2) - 5 \, \mathfrak{h}2 - 5 \, \mu 2 \, \mathfrak{h}2 + \\
& 2 \, \mu 1^2 \, (1 + 2 \, \mathfrak{h}1 + \mathfrak{h}2)) + \eta t \, (16 + 32 \, \mu 1 - 8 \, \mu 1^2 + 5 \, \mu 2 - 7 \, \mu 1 \, \mu 2 + \\
& \theta l \, (6 + 5 \times (1 + \mu 2) \, \mathfrak{h}1 + \mu 1 \, (-4 + 21 \, \mathfrak{h}1 + \mu 2 \, (36 + 5 \, \mathfrak{h}1 - 17 \, \mathfrak{h}2) - \\
& 15 \, \mathfrak{h}2) - 5 \, \mathfrak{h}2 - 5 \, \mu 2 \, \mathfrak{h}2 + 2 \, \mu 1^2 \, (1 + 2 \, \mathfrak{h}1 + \mathfrak{h}2))) - \\
& 2 \, \eta^4 \, (-10 + 3 \, \mu 1 + 7 \, \mu 1^2 - 8 \, \mu 2 - 20 \, \mu 1 \, \mu 2 - \theta l \, (1 + 4 \, \mu 2 + \mu 1^2 \\
& (3 + 2 \, \mathfrak{h}1 + \mathfrak{h}2) + \mu 1 \, (10 - 2 \, \mu 2 + 5 \, \mathfrak{h}1 - 2 \, \mathfrak{h}2 - 6 \, \mu 2 \, \mathfrak{h}2)) + \\
& \eta t \, (-2 \times (1 + \mu 1^2 - \mu 2 + \mu 1 \, (-4 + 5 \, \mu 2)) + \theta l \, (1 + 4 \, \mu 2 + \\
& \mu 1^2 \, (3 + 2 \, \mathfrak{h}1 + \mathfrak{h}2) + \mu 1 \, (10 - 2 \, \mu 2 + 5 \, \mathfrak{h}1 - 2 \, \mathfrak{h}2 - 6 \, \mu 2 \, \mathfrak{h}2))) + \\
& \eta \, (\theta l \, (5 \times (1 + \mu 2) \times (-2 + \mathfrak{h}1 - \mathfrak{h}2) + \mu 1^2 \, (2 - \mathfrak{h}1 + \mathfrak{h}2) + \\
& \mu 1 \, (5 \, \mu 2 \, \mathfrak{h}1 + 4 \times (-2 + \mathfrak{h}1 - \mathfrak{h}2) + 7 \, \mu 2 \, (2 + \mathfrak{h}2))) + \\
& \eta t \, (20 + 24 \, \mu 1 + 4 \, \mu 1^2 + 5 \, \mu 2 - 19 \, \mu 1 \, \mu 2 + \theta l \, \\
& (\mu 1^2 \, (-2 + \mathfrak{h}1 - \mathfrak{h}2) - 5 \times (1 + \mu 2) \times (-2 + \mathfrak{h}1 - \mathfrak{h}2) - \\
& \mu 1 \, (5 \, \mu 2 \, \mathfrak{h}1 + 4 \times (-2 + \mathfrak{h}1 - \mathfrak{h}2) + 7 \, \mu 2 \, (2 + \mathfrak{h}2)))) - \\
& \eta^2 \, (-2 \times (2 \times (-5 + \mu 1^2 - 2 \, \mu 2 - 4 \, \mu 1 \, (1 + 2 \, \mu 2)) + \theta l \, (-5 - \\
& 8 \, \mu 2 + 5 \, \mathfrak{h}1 + 5 \, \mu 2 \, \mathfrak{h}1 - 5 \, \mathfrak{h}2 - 5 \, \mu 2 \, \mathfrak{h}2 + \mu 1^2 \, (1 + \mathfrak{h}2) + \\
& \mu 1 \, (-10 + 8 \, \mathfrak{h}1 - 7 \, \mathfrak{h}2 + \mu 2 \, (22 + 5 \, \mathfrak{h}1 + \mathfrak{h}2)))) + \\
& \eta t \, (10 + 18 \, \mu 1^2 + \mu 1 \, (-20 + \mu 2) + \mu 2 + 2 \, \theta l \, (-5 - 8 \, \mu 2 + \\
& 5 \, \mathfrak{h}1 + 5 \, \mu 2 \, \mathfrak{h}1 - 5 \, \mathfrak{h}2 - 5 \, \mu 2 \, \mathfrak{h}2 + \mu 1^2 \, (1 + \mathfrak{h}2) + \\
& \mu 1 \, (-10 + 8 \, \mathfrak{h}1 - 7 \, \mathfrak{h}2 + \mu 2 \, (22 + 5 \, \mathfrak{h}1 + \mathfrak{h}2)))) - w \, (-1 + \eta) \times \\
& (6 \, \eta^8 \, (1 + \mu 1) + 2 \, \eta^7 \, (7 + 9 \, \mu 1^2 - 3 \, \eta t \, (1 + \mu 1) + \mu 1 \, (22 - 18 \, \mu 2)) - \\
& 5 \, \eta t \, (1 + \mu 1) \, \mu 2 + 2 \, \eta \, \eta t \, (-4 \, \mu 1^2 + \mu 1 \, (22 - 31 \, \mu 2) + 5 \times (4 + \mu 2)) + \\
& \eta^6 \, (2 \times (7 + (22 + \theta l) \, \mu 2) + \mu 1^2 \, (34 + \theta l \, (4 + \mathfrak{h}1 + \mathfrak{h}2)) + \\
& \mu 1 \, (84 - 76 \, \mu 2 + \theta l \, (16 - 10 \, \mu 2 + \mathfrak{h}1 + \mathfrak{h}2)) - \\
& \eta t \, (2 \times (7 + \theta l \, \mu 2) + \mu 1^2 \, (-4 + \theta l \, (4 + \mathfrak{h}1 + \mathfrak{h}2)) + \\
& \mu 1 \, (10 - 24 \, \mu 2 + \theta l \, (16 - 10 \, \mu 2 + \mathfrak{h}1 + \mathfrak{h}2)))) - \\
& \eta^3 \, (52 + 84 \, \mu 1 + 8 \, \mu 1^2 + 72 \, \mu 2 + 24 \, \mu 1 \, \mu 2 - \theta l \, (-28 + 30 \, \mathfrak{h}1 + \\
& \mu 1 \, (-46 + 55 \, \mathfrak{h}1 + \mu 2 \, (98 + 30 \, \mathfrak{h}1 - 6 \, \mathfrak{h}2) - 49 \, \mathfrak{h}2) + \\
& \mu 2 \, (-34 + 30 \, \mathfrak{h}1 - 30 \, \mathfrak{h}2) - 30 \, \mathfrak{h}2 + \mu 1^2 \, (6 + \mathfrak{h}1 + 5 \, \mathfrak{h}2)) + \\
& \eta t \, (2 \times (16 + 22 \, \mu 1^2 + \mu 1 \, (-4 + \mu 2) + \mu 2) + \theta l \, (-28 + 30 \, \mathfrak{h}1 + \\
& \mu 1 \, (-46 + 55 \, \mathfrak{h}1 + \mu 2 \, (98 + 30 \, \mathfrak{h}1 - 6 \, \mathfrak{h}2) - 49 \, \mathfrak{h}2) + \\
& \mu 2 \, (-34 + 30 \, \mathfrak{h}1 - 30 \, \mathfrak{h}2) - 30 \, \mathfrak{h}2 + \mu 1^2 \, (6 + \mathfrak{h}1 + 5 \, \mathfrak{h}2)))) - \\
& \eta^4 \, (74 \, \mu 1 + 38 \, \mu 1^2 + 40 \, \mu 2 - 128 \, \mu 1 \, \mu 2 - \theta l \, (4 + 15 \, \mathfrak{h}1 + \mu 1 \\
& (14 + 54 \, \mathfrak{h}1 + 3 \, \mu 2 \, (14 + 5 \, \mathfrak{h}1 - 13 \, \mathfrak{h}2) - 40 \, \mathfrak{h}2) + \\
& 3 \, \mu 2 \, (2 + 5 \, \mathfrak{h}1 - 5 \, \mathfrak{h}2) - 15 \, \mathfrak{h}2 + \mu 1^2 \, (9 \, \mathfrak{h}1 + 5 \times (2 + \mathfrak{h}2))) +
\end{aligned}$$

$$\begin{aligned}
& \eta t \left( 46 + 102 \mu_1 - 40 \mu_1^2 + 19 \mu_2 - 53 \mu_1 \mu_2 + \theta l \right. \\
& \quad \left( 4 + 15 \mathfrak{z}_1 + \mu_1 (14 + 54 \mathfrak{z}_1 + 3 \mu_2 (14 + 5 \mathfrak{z}_1 - 13 \mathfrak{z}_2) - 40 \mathfrak{z}_2) + \right. \\
& \quad \left. 3 \mu_2 (2 + 5 \mathfrak{z}_1 - 5 \mathfrak{z}_2) - 15 \mathfrak{z}_2 + \mu_1^2 (9 \mathfrak{z}_1 + 5 \times (2 + \mathfrak{z}_2)) \right) \left. \right) + \\
& \eta^2 \left( 4 \times (1 + \mu_1) \times (-5 + \mu_1 - 3 \mu_2) + \theta l \left( 3 \mu_2 (-8 + 5 \mathfrak{z}_1 - 5 \mathfrak{z}_2) + \right. \right. \\
& \quad \left. 5 \times (-4 + 3 \mathfrak{z}_1 - 3 \mathfrak{z}_2) + \mu_1^2 (2 - 2 \mathfrak{z}_1 + 2 \mathfrak{z}_2) + \right. \\
& \quad \left. \mu_1 (-30 + 19 \mathfrak{z}_1 - 19 \mathfrak{z}_2 + 3 \mu_2 (16 + 5 \mathfrak{z}_1 + 3 \mathfrak{z}_2)) \right) \left. \right) + \\
& \eta t \left( -4 \times (-15 - 26 \mu_1 + \mu_1^2 - 6 \mu_2 + 18 \mu_1 \mu_2) + \theta l \left( -3 \mu_2 (-8 + \right. \right. \\
& \quad \left. 5 \mathfrak{z}_1 - 5 \mathfrak{z}_2) + 2 \mu_1^2 (-1 + \mathfrak{z}_1 - \mathfrak{z}_2) + 5 \times (4 - 3 \mathfrak{z}_1 + 3 \mathfrak{z}_2) - \right. \\
& \quad \left. \mu_1 (-30 + 19 \mathfrak{z}_1 - 19 \mathfrak{z}_2 + 3 \mu_2 (16 + 5 \mathfrak{z}_1 + 3 \mathfrak{z}_2)) \right) \left. \right) + \\
& \eta^5 \left( 38 + 40 \mu_1 - 10 \mu_1^2 + 80 \mu_2 + 20 \mu_1 \mu_2 + \theta l \left( 6 \times (2 + 3 \mu_2) + \mu_1^2 \right. \right. \\
& \quad \left. (10 + 7 \mathfrak{z}_1 + 3 \mathfrak{z}_2) + \mu_1 (46 + 19 \mathfrak{z}_1 - 9 \mathfrak{z}_2 - 6 \mu_2 (3 + 4 \mathfrak{z}_2)) \right) - \eta t \\
& \quad \left( 2 + 38 \mu_1 - 12 \mu_1^2 + 8 \mu_2 - 64 \mu_1 \mu_2 + \theta l \left( 6 \times (2 + 3 \mu_2) + \mu_1^2 (10 + 7 \right. \right. \\
& \quad \left. \mathfrak{z}_1 + 3 \mathfrak{z}_2) + \mu_1 (46 + 19 \mathfrak{z}_1 - 9 \mathfrak{z}_2 - 6 \mu_2 (3 + 4 \mathfrak{z}_2)) \right) \left. \right) \left. \right) + \\
& w^2 (-1 + \eta)^2 \left( 2 \eta^8 (1 + \mu_1) - 15 \eta t (1 + \mu_1) \mu_2 - 2 \eta^7 (-7 + \eta t - \right. \\
& \quad \left. 11 \mu_1 + \eta t \mu_1 - 4 \mu_1^2 + 6 \mu_1 \mu_2) - 12 \eta \eta t (-5 + \mu_1^2 + \mu_1 (-7 + 6 \mu_2)) + \right. \\
& \quad \left. 2 \eta^6 (12 + 21 \mu_1^2 + \mu_1 (45 - 43 \mu_2) + 11 \mu_2 + \eta t (-7 + \mu_1 (-7 + 6 \mu_2))) - \right. \\
& \quad \left. \eta^3 (2 \times (30 + 17 \mu_1^2 + \mu_1 (65 - 38 \mu_2) + 58 \mu_2) - \right. \\
& \quad \left. \theta l (\mu_1 (-26 + 61 \mathfrak{z}_1 + 6 \mu_2 (9 + 5 \mathfrak{z}_1 - 3 \mathfrak{z}_2) - 57 \mathfrak{z}_2) + \right. \\
& \quad \left. 6 \times (1 + \mu_2) \times (-3 + 5 \mathfrak{z}_1 - 5 \mathfrak{z}_2) + \mu_1^2 (4 + \mathfrak{z}_1 + 3 \mathfrak{z}_2)) \right) + \\
& \eta t \left( 44 + 4 \mu_1^2 - 4 \mu_1 (-15 + \mu_2) - 4 \mu_2 + \theta l \mu_1 \right. \\
& \quad \left. (-26 + 61 \mathfrak{z}_1 + 6 \mu_2 (9 + 5 \mathfrak{z}_1 - 3 \mathfrak{z}_2) - 57 \mathfrak{z}_2) + \right. \\
& \quad \left. 6 \theta l (1 + \mu_2) \times (-3 + 5 \mathfrak{z}_1 - 5 \mathfrak{z}_2) + \theta l \mu_1^2 (4 + \mathfrak{z}_1 + 3 \mathfrak{z}_2) \right) \left. \right) + \\
& \eta^2 \left( -2 \times (23 + 25 \mu_2 + \mu_1 (29 + 7 \mu_2)) - \theta l \left( -((1 + \mu_2) \times \right. \right. \\
& \quad \left. (-14 + 15 \mathfrak{z}_1 - 15 \mathfrak{z}_2)) + \mu_1^2 (\mathfrak{z}_1 - \mathfrak{z}_2) + 26 \mu_1 (1 - \mathfrak{z}_1 + \mathfrak{z}_2) + \right. \\
& \quad \left. \mu_1 \mu_2 (-34 - 15 \mathfrak{z}_1 + 3 \mathfrak{z}_2) \right) + \eta t \left( 64 + 140 \mu_1 - 44 \mu_1^2 + 38 \mu_2 - 94 \right. \\
& \quad \left. \mu_1 \mu_2 + \theta l \left( -((1 + \mu_2) \times (-14 + 15 \mathfrak{z}_1 - 15 \mathfrak{z}_2)) + \mu_1^2 (\mathfrak{z}_1 - \mathfrak{z}_2) + \right. \right. \\
& \quad \left. 26 \mu_1 (1 - \mathfrak{z}_1 + \mathfrak{z}_2) + \mu_1 \mu_2 (-34 - 15 \mathfrak{z}_1 + 3 \mathfrak{z}_2) \right) \left. \right) \left. \right) + \\
& \eta^4 \left( 20 - 34 \mu_1 - 42 \mu_1^2 + 36 \mu_2 + 108 \mu_1 \mu_2 + \theta l \left( \mu_1 (26 + 44 \mathfrak{z}_1 + 3 \mu_2 \right. \right. \\
& \quad \left. (2 + 5 \mathfrak{z}_1 - 9 \mathfrak{z}_2) - 36 \mathfrak{z}_2) + 3 \times (1 + \mu_2) \times (2 + 5 \mathfrak{z}_1 - 5 \mathfrak{z}_2) + \right. \\
& \quad \left. \mu_1^2 (8 + 5 \mathfrak{z}_1 + 3 \mathfrak{z}_2) \right) - \eta t \left( 50 + 118 \mu_1 - 52 \mu_1^2 + 23 \mu_2 - \right. \\
& \quad \left. 97 \mu_1 \mu_2 + \theta l \left( \mu_1 (26 + 44 \mathfrak{z}_1 + 3 \mu_2 (2 + 5 \mathfrak{z}_1 - 9 \mathfrak{z}_2) - 36 \mathfrak{z}_2) + \right. \right. \\
& \quad \left. 3 \times (1 + \mu_2) \times (2 + 5 \mathfrak{z}_1 - 5 \mathfrak{z}_2) + \mu_1^2 (8 + 5 \mathfrak{z}_1 + 3 \mathfrak{z}_2) \right) \left. \right) \left. \right) + \\
& \eta^5 \left( 46 + 26 \mu_1^2 + 108 \mu_2 + 10 \theta l (1 + \mu_2) - 36 \mu_1 (-3 + 2 \mu_2) + \right. \\
& \quad \left. \theta l \mu_1^2 (4 + 3 \mathfrak{z}_1 + \mathfrak{z}_2) + \theta l \mu_1 (26 + 9 \mathfrak{z}_1 - 5 \mathfrak{z}_2 - 2 \mu_2 (7 + 6 \mathfrak{z}_2)) - \right. \\
& \quad \left. \eta t \left( 14 + 30 \mu_1 - 8 \mu_1^2 + 4 \mu_2 - 68 \mu_1 \mu_2 + \theta l \left( 10 \times (1 + \mu_2) + \mu_1^2 (4 + \right. \right. \right. \\
& \quad \left. \left. 3 \mathfrak{z}_1 + \mathfrak{z}_2) + \mu_1 (26 + 9 \mathfrak{z}_1 - 5 \mathfrak{z}_2 - 2 \mu_2 (7 + 6 \mathfrak{z}_2)) \right) \right) \left. \right) \left. \right) - \\
& x^3 (-1 + \eta)^3 \left( (-1 + \eta) \theta p \left( 20 + 104 \eta + 36 \eta^2 + 80 \eta^4 - 20 \eta t - 16 \eta \eta t - \right. \right. \\
& \quad \left. 80 \eta^2 \eta t - 80 \eta^3 \eta t + 16 \mu_1 + 168 \eta \mu_1 + 456 \eta^2 \mu_1 + 440 \eta^3 \mu_1 + \right. \\
& \quad \left. 80 \eta^4 \mu_1 - 48 \eta t \mu_1 - 80 \eta \eta t \mu_1 - 64 \eta^2 \eta t \mu_1 - 80 \eta^3 \eta t \mu_1 - \right. \\
& \quad \left. 4 \mu_1^2 + 16 \eta \mu_1^2 + 180 \eta^2 \mu_1^2 + 200 \eta^3 \mu_1^2 + 44 \eta t \mu_1^2 + \right. \\
& \quad \left. 32 \eta \eta t \mu_1^2 + 16 \eta^2 \eta t \mu_1^2 + 12 \mu_2 + 152 \eta \mu_2 + 196 \eta^2 \mu_2 - \right. \\
& \quad \left. 9 \eta t \mu_2 - 16 \eta \eta t \mu_2 + 12 \mu_1 \mu_2 + 8 \eta \mu_1 \mu_2 - 116 \eta^2 \mu_1 \mu_2 - \right. \\
& \quad \left. 240 \eta^3 \mu_1 \mu_2 + 39 \eta t \mu_1 \mu_2 + 128 \eta \eta t \mu_1 \mu_2 + 120 \eta^2 \eta t \mu_1 \mu_2 + \right.
\end{aligned}$$

$$\begin{aligned}
& 2 w^4 (-1 + \eta)^4 (5 + 12 \mu_1 + 7 \mu_1^2 + 4 \eta^2 (1 + \mu_1) + 11 \mu_2 - 7 \mu_1 \mu_2 + 2 \eta (1 + \\
& \quad 9 \mu_1 + 8 \mu_1^2 - 2 \eta t (1 + \mu_1) - 3 \mu_1 \mu_2) + \eta t (-2 - 2 \mu_1 + 6 \mu_1 \mu_2)) - \\
& w^3 (-1 + \eta)^3 (60 + 40 \mu_1^2 + 44 \eta t \mu_1^2 + 40 \eta^3 (1 + \mu_1) + \\
& \quad 4 \mu_1 (31 - 14 \mu_2) + 112 \mu_2 - 9 \eta t (4 + \mu_2) + \eta t \mu_1 (-64 + 87 \mu_2) + \\
& \quad 8 \eta^2 (7 + 27 \mu_1 + 20 \mu_1^2 - 5 \eta t (1 + \mu_1) - 12 \mu_1 \mu_2) + 4 \eta (24 + 82 \mu_1 + \\
& \quad 46 \mu_1^2 + 44 \mu_2 - 43 \mu_1 \mu_2 + 2 \eta t (-7 - 7 \mu_1 + 12 \mu_1 \mu_2))) + \\
& w^2 (-1 + \eta)^2 (40 \eta^4 (1 + \mu_1) + 2 \times (51 + 92 \mu_1 + 17 \mu_1^2 + 83 \mu_2 - \\
& \quad 19 \mu_1 \mu_2) - 40 \eta^3 (-4 + \eta t - 8 \mu_1 + \eta t \mu_1 - 4 \mu_1^2 + 3 \mu_1 \mu_2) + \\
& \quad \eta t (-80 - 164 \mu_1 + 132 \mu_1^2 - 27 \mu_2 + 177 \mu_1 \mu_2) + \\
& \quad 4 \eta^2 (55 + 240 \mu_1 + 125 \mu_1^2 + 55 \mu_2 - 119 \mu_1 \mu_2 + \\
& \quad 10 \eta t (-4 - 4 \mu_1 + 3 \mu_1 \mu_2)) + 4 \eta (71 + 207 \mu_1 + 76 \mu_1^2 + \\
& \quad 130 \mu_2 - 98 \mu_1 \mu_2 + \eta t (-30 - 46 \mu_1 + 8 \mu_1^2 - 4 \mu_2 + 80 \mu_1 \mu_2))) - \\
& w (-1 + \eta) \times (120 \eta^4 (1 + \mu_1) + 40 \eta^3 (5 + 9 \mu_1^2 - 3 \eta t (1 + \mu_1) + \\
& \quad \mu_1 (20 - 9 \mu_2)) + 4 \times (18 + \mu_1^2 + 22 \mu_2 + \mu_1 (25 + 4 \mu_2)) + \\
& \quad \eta t (-68 + 132 \mu_1^2 - 27 \mu_2 + \mu_1 (-152 + 141 \mu_2)) + \\
& \quad 8 \eta^2 (26 + 65 \mu_1^2 + \mu_1 (151 - 62 \mu_2) + 52 \mu_2 + \eta t (-25 + 2 \mu_1^2 + \\
& \quad \mu_1 (-23 + 30 \mu_2))) + 8 \eta (33 + 21 \mu_1^2 - 28 \mu_1 (-3 + \mu_2) + \\
& \quad 62 \mu_2 + \eta t (-11 + 8 \mu_1^2 - 4 \mu_2 + \mu_1 (-27 + 44 \mu_2)))) + \\
& (-1 + \eta t) \text{el} (-30 - 60 \eta + 10 \text{ep} - 24 \eta \text{ep} - 20 \eta^2 \text{ep} + 80 \eta^3 \text{ep} - \\
& \quad 32 \mu_1 - 160 \eta \mu_1 - 120 \eta^2 \mu_1 + 24 \eta^3 \mu_1 + 18 \text{ep} \mu_1 + 10 \eta \text{ep} \mu_1 - \\
& \quad 188 \eta^2 \text{ep} \mu_1 - 220 \eta^3 \text{ep} \mu_1 + 10 \mu_1^2 + 56 \eta \mu_1^2 + 24 \eta^2 \mu_1^2 + \\
& \quad 24 \eta^3 \mu_1^2 - 4 \text{ep} \mu_1^2 - 14 \eta \text{ep} \mu_1^2 - 48 \eta^2 \text{ep} \mu_1^2 - 60 \eta^3 \text{ep} \mu_1^2 + \\
& w^4 (-1 + \eta)^4 (26 \mu_1^2 + 5 \mu_1 (-4 + \mu_2) + 5 \times (-2 + \mu_2)) - 10 \mu_2 - \\
& \quad 15 \eta \mu_2 + 14 \text{ep} \mu_2 - 6 \eta \text{ep} \mu_2 - 68 \eta^2 \text{ep} \mu_2 - 20 \eta^3 \text{ep} \mu_2 + 38 \mu_1 \mu_2 + \\
& \quad 57 \eta \mu_1 \mu_2 - 34 \text{ep} \mu_1 \mu_2 - 114 \eta \text{ep} \mu_1 \mu_2 - 20 \eta^2 \text{ep} \mu_1 \mu_2 + \\
& \quad 100 \eta^3 \text{ep} \mu_1 \mu_2 - 10 \text{ep} \text{e1} - 20 \eta \text{ep} \text{e1} - 17 \text{ep} \mu_1 \text{e1} - 87 \eta \text{ep} \mu_1 \text{e1} - \\
& \quad 94 \eta^2 \text{ep} \mu_1 \text{e1} - 10 \eta^3 \text{ep} \mu_1 \text{e1} - \text{ep} \mu_1^2 \text{e1} - 19 \eta \text{ep} \mu_1^2 \text{e1} - \\
& \quad 34 \eta^2 \text{ep} \mu_1^2 \text{e1} - 10 \eta^3 \text{ep} \mu_1^2 \text{e1} - 10 \text{ep} \mu_2 \text{e1} - 20 \eta \text{ep} \mu_2 \text{e1} - \\
& \quad 10 \text{ep} \mu_1 \mu_2 \text{e1} - 20 \eta \text{ep} \mu_1 \mu_2 \text{e1} - w^3 (-1 + \eta)^3 (76 \mu_1^2 + \\
& \quad \eta (60 \mu_1^2 + \mu_1 (-156 + \mu_2 (57 - 20 \text{ep} (\text{e1} - \text{e2})) - 44 \text{ep} (\text{e1} - \text{e2})) - \\
& \quad 5 \times (12 + 3 \mu_2 + 4 \text{ep} (\text{e1} - \text{e2}) + 4 \text{ep} \mu_2 (\text{e1} - \text{e2}))) + \\
& \quad \mu_1 (-128 + \mu_2 (53 - 10 \text{ep} (\text{e1} - \text{e2})) - 22 \text{ep} (\text{e1} - \text{e2})) - \\
& \quad 5 \times (12 - \mu_2 + 2 \text{ep} (\text{e1} - \text{e2}) + 2 \text{ep} \mu_2 (\text{e1} - \text{e2}))) + 10 \text{ep} \text{e2} + \\
& \quad 20 \eta \text{ep} \text{e2} + 13 \text{ep} \mu_1 \text{e2} + 57 \eta \text{ep} \mu_1 \text{e2} + 46 \eta^2 \text{ep} \mu_1 \text{e2} - \\
& \quad 10 \eta^3 \text{ep} \mu_1 \text{e2} - 3 \text{ep} \mu_1^2 \text{e2} - 11 \eta \text{ep} \mu_1^2 \text{e2} - 14 \eta^2 \text{ep} \mu_1^2 \text{e2} - \\
& \quad 10 \eta^3 \text{ep} \mu_1^2 \text{e2} + 10 \text{ep} \mu_2 \text{e2} + 20 \eta \text{ep} \mu_2 \text{e2} - \\
& \quad 2 \text{ep} \mu_1 \mu_2 \text{e2} + 68 \eta \text{ep} \mu_1 \mu_2 \text{e2} + 120 \eta^2 \text{ep} \mu_1 \mu_2 \text{e2} + \\
& w (-1 + \eta) \times (100 + 152 \mu_1 - 44 \mu_1^2 + 25 \mu_2 - 119 \mu_1 \mu_2 + \\
& \quad 2 \text{ep} (-14 + 15 \text{e1} + \mu_1 (-22 + 28 \text{e1} + \mu_2 (44 + 15 \text{e1} - 3 \text{e2}) - 24 \text{e2}) + \\
& \quad \mu_2 (-16 + 15 \text{e1} - 15 \text{e2}) - 15 \text{e2} + \mu_1^2 (4 + \text{e1} + 3 \text{e2})) + \\
& \quad 2 \eta^3 (10 \text{ep} \mu_2 + \mu_1^2 (-12 + 5 \text{ep} (6 + \text{e1} + \text{e2})) + \\
& \quad \mu_1 (-12 + 5 \text{ep} (30 - 10 \mu_2 + \text{e1} + \text{e2}))) + \\
& \quad \eta (180 + 472 \mu_1 - 176 \mu_1^2 + 45 \mu_2 - 171 \mu_1 \mu_2 + \text{ep} (16 + 60 \text{e1} + \\
& \quad \mu_1 (62 + 219 \text{e1} + 6 \mu_2 (23 + 10 \text{e1} - 26 \text{e2}) - 157 \text{e2}) + 30 \mu_2
\end{aligned}$$

$$\begin{aligned}
& \left( (1 + 2 \mathfrak{x}1 - 2 \mathfrak{x}2) - 60 \mathfrak{x}2 + \mu1^2 (39 \mathfrak{x}1 + 23 \times (2 + \mathfrak{x}2)) \right) \Big) + \\
& 8 \eta^2 \left( -6 \times (-5 + \mu1) \mu1 + \mathfrak{op} \left( 3 \times (5 + 7 \mu2) + \mu1^2 (11 + 8 \mathfrak{x}1 + \right. \right. \\
& \quad \left. \left. 3 \mathfrak{x}2) + \mu1 (56 + 23 \mathfrak{x}1 - 12 \mathfrak{x}2 - 15 \mu2 (1 + 2 \mathfrak{x}2)) \right) \right) \Big) - \\
& w^2 (-1 + \eta)^2 \left( -84 \mu1^2 + 3 \mu1 (76 - 43 \mu2) + 15 \times (8 + \mu2) + \right. \\
& \quad \mathfrak{op} \mu1 (-26 + 61 \mathfrak{x}1 + 6 \mu2 (9 + 5 \mathfrak{x}1 - 3 \mathfrak{x}2) - 57 \mathfrak{x}2) + \\
& \quad 6 \mathfrak{op} (1 + \mu2) \times (-3 + 5 \mathfrak{x}1 - 5 \mathfrak{x}2) + \mathfrak{op} \mu1^2 (4 + \mathfrak{x}1 + 3 \mathfrak{x}2) + \\
& \quad \eta (-9 \times (20 \mu1^2 - 5 \times (4 + \mu2) + \mu1 (-52 + 19 \mu2)) + \\
& \quad 4 \mathfrak{op} (\mu1 (26 + 44 \mathfrak{x}1 + 3 \mu2 (2 + 5 \mathfrak{x}1 - 9 \mathfrak{x}2) - 36 \mathfrak{x}2) + \\
& \quad 3 \times (1 + \mu2) \times (2 + 5 \mathfrak{x}1 - 5 \mathfrak{x}2) + \mu1^2 (8 + 5 \mathfrak{x}1 + 3 \mathfrak{x}2)) \Big) + \\
& 2 \eta^2 \left( -12 \times (-5 + \mu1) \mu1 + 5 \mathfrak{op} (10 \times (1 + \mu2) + \mu1^2 (4 + \right. \\
& \quad \left. 3 \mathfrak{x}1 + \mathfrak{x}2) + \mu1 (26 + 9 \mathfrak{x}1 - 5 \mathfrak{x}2 - 2 \mu2 (7 + 6 \mathfrak{x}2)) \right) \Big) \Big) + \\
& x^4 (-1 + \eta)^4 \left( 2 \times (-1 + \eta) \mathfrak{op} (13 + 7 \eta - 10 \eta^2 + 30 \eta^3 - 2 \eta t - 20 \eta \eta t - \right. \\
& \quad 30 \eta^2 \eta t + 21 \mu1 + 112 \eta \mu1 + 155 \eta^2 \mu1 + 30 \eta^3 \mu1 - 10 \eta t \mu1 - \\
& \quad 18 \eta \eta t \mu1 - 30 \eta^2 \eta t \mu1 + 2 \mu1^2 + 45 \eta \mu1^2 + 75 \eta^2 \mu1^2 + \\
& \quad 4 \eta t \mu1^2 + 2 \eta \eta t \mu1^2 + w^4 (-1 + \eta)^4 (1 + \mu1) (\eta - \eta t + 4 \mu1) + \\
& \quad 19 \mu2 + 47 \eta \mu2 - 2 \eta t \mu2 + \mu1 \mu2 - 7 \eta \mu1 \mu2 - \\
& \quad 60 \eta^2 \mu1 \mu2 + 16 \eta t \mu1 \mu2 + 30 \eta \eta t \mu1 \mu2 - w^3 (-1 + \eta)^3 \\
& \quad \left( 10 + 39 \mu1 + 23 \mu1^2 + 10 \eta^2 (1 + \mu1) + 22 \mu2 - 14 \mu1 \mu2 + \eta (7 + 47 \mu1 + \right. \\
& \quad \left. 40 \mu1^2 - 10 \eta t (1 + \mu1) - 12 \mu1 \mu2) + \eta t (-7 - 7 \mu1 + 12 \mu1 \mu2) \right) + \\
& w^2 (-1 + \eta)^2 \left( 33 + 101 \mu1 + 38 \mu1^2 + 15 \eta^3 (1 + \mu1) + 65 \mu2 - \right. \\
& \quad 37 \mu1 \mu2 + \eta t (-15 - 23 \mu1 + 4 \mu1^2 - 2 \mu2 + 40 \mu1 \mu2) - 5 \eta^2 \\
& \quad \left( 3 \eta t (1 + \mu1) - 2 \times (4 + 10 \mu1 + 6 \mu1^2 - 3 \mu1 \mu2) \right) + \eta (40 + 225 \mu1 + \\
& \quad 125 \mu1^2 + 55 \mu2 - 77 \mu1 \mu2 + 10 \eta t (-4 - 4 \mu1 + 3 \mu1 \mu2)) \Big) - \\
& w (-1 + \eta) \times \left( 32 + 83 \mu1 + 21 \mu1^2 + 45 \eta^3 (1 + \mu1) + 62 \mu2 - \right. \\
& \quad 22 \mu1 \mu2 + 5 \eta^2 (10 + 55 \mu1 + 27 \mu1^2 - 9 \eta t (1 + \mu1) - 18 \mu1 \mu2) + \\
& \quad \eta t (-11 - 27 \mu1 + 8 \mu1^2 - 4 \mu2 + 44 \mu1 \mu2) + \eta (41 + 291 \mu1 + 130 \mu1^2 + \\
& \quad 102 \mu2 - 72 \mu1 \mu2 + 2 \eta t (-25 + \mu1^2 + 6 \mu1 (-4 + 5 \mu2)) \Big) \Big) + \\
& (-1 + \eta t) \mathfrak{el} \left( -20 - 6 \mathfrak{op} - 10 \eta \mathfrak{op} + 60 \eta^2 \mathfrak{op} - 52 \mu1 - 80 \eta \mu1 + \right. \\
& \quad 16 \eta^2 \mu1 + 2 \mathfrak{op} \mu1 - 92 \eta \mathfrak{op} \mu1 - 160 \eta^2 \mathfrak{op} \mu1 + 28 \mu1^2 + 16 \eta \mu1^2 + \\
& \quad 16 \eta^2 \mu1^2 - 4 \mathfrak{op} \mu1^2 - 22 \eta \mathfrak{op} \mu1^2 - 40 \eta^2 \mathfrak{op} \mu1^2 - 5 \mu2 - \\
& \quad 2 \mathfrak{op} \mu2 - 32 \eta \mathfrak{op} \mu2 - 10 \eta^2 \mathfrak{op} \mu2 + 19 \mu1 \mu2 - 26 \mathfrak{op} \mu1 \mu2 - \\
& \quad 20 \eta \mathfrak{op} \mu1 \mu2 + 50 \eta^2 \mathfrak{op} \mu1 \mu2 - 5 \mathfrak{op} \mathfrak{x}1 - 22 \mathfrak{op} \mu1 \mathfrak{x}1 - \\
& \quad 46 \eta \mathfrak{op} \mu1 \mathfrak{x}1 - 5 \eta^2 \mathfrak{op} \mu1 \mathfrak{x}1 - 5 \mathfrak{op} \mu1^2 \mathfrak{x}1 - 16 \eta \mathfrak{op} \mu1^2 \mathfrak{x}1 - \\
& \quad 5 \eta^2 \mathfrak{op} \mu1^2 \mathfrak{x}1 - 5 \mathfrak{op} \mu2 \mathfrak{x}1 - 5 \mathfrak{op} \mu1 \mu2 \mathfrak{x}1 + 5 \mathfrak{op} \mathfrak{x}2 + 14 \mathfrak{op} \mu1 \mathfrak{x}2 + \\
& \quad 24 \eta \mathfrak{op} \mu1 \mathfrak{x}2 - 5 \eta^2 \mathfrak{op} \mu1 \mathfrak{x}2 - 3 \mathfrak{op} \mu1^2 \mathfrak{x}2 - 6 \eta \mathfrak{op} \mu1^2 \mathfrak{x}2 - \\
& \quad 5 \eta^2 \mathfrak{op} \mu1^2 \mathfrak{x}2 + 5 \mathfrak{op} \mu2 \mathfrak{x}2 + 17 \mathfrak{op} \mu1 \mu2 \mathfrak{x}2 + 60 \eta \mathfrak{op} \mu1 \mu2 \mathfrak{x}2 - \\
& w^3 (-1 + \eta)^3 \left( 28 \mu1^2 - 5 \times (4 + \mu2 + \mathfrak{op} (\mathfrak{x}1 - \mathfrak{x}2) + \mathfrak{op} \mu2 (\mathfrak{x}1 - \mathfrak{x}2)) + \right. \\
& \quad \left. \mu1 (-52 - 11 \mathfrak{op} (\mathfrak{x}1 - \mathfrak{x}2) + \mu2 (19 - 5 \mathfrak{op} \mathfrak{x}1 + 5 \mathfrak{op} \mathfrak{x}2)) \right) - \\
& w^2 (-1 + \eta)^2 \left( 60 + 156 \mu1 + 80 \eta \mu1 - 84 \mu1^2 - 16 \eta \mu1^2 + 15 \mu2 - 57 \mu1 \mu2 + \right. \\
& \quad \mathfrak{op} (\mu1 (26 + 44 \mathfrak{x}1 + 3 \mu2 (2 + 5 \mathfrak{x}1 - 9 \mathfrak{x}2) - 36 \mathfrak{x}2) + 3 \times (1 + \mu2) \times \\
& \quad \left. (2 + 5 \mathfrak{x}1 - 5 \mathfrak{x}2) + \mu1^2 (8 + 5 \mathfrak{x}1 + 3 \mathfrak{x}2) + 5 \eta (10 \times (1 + \mu2) + \mu1^2 \right. \\
& \quad \left. (4 + 3 \mathfrak{x}1 + \mathfrak{x}2) + \mu1 (26 + 9 \mathfrak{x}1 - 5 \mathfrak{x}2 - 2 \mu2 (7 + 6 \mathfrak{x}2)) \right) \Big) \Big) + \\
& w (-1 + \eta) \times \left( 60 + 156 \mu1 + 160 \eta \mu1 - 16 \eta^2 \mu1 - 84 \mu1^2 - \right. \\
& \quad 32 \eta \mu1^2 - 16 \eta^2 \mu1^2 + 15 \mu2 - 57 \mu1 \mu2 + \mathfrak{op} (4 + 8 \mu2 + 15 \mathfrak{x}1 +
\end{aligned}$$

$$\begin{aligned}
& 15 \mu_2 \mathfrak{e}_1 + \mu_1 (16 + 55 \mathfrak{e}_1 + \mu_2 (32 + 15 \mathfrak{e}_1 - 39 \mathfrak{e}_2) - 39 \mathfrak{e}_2) - \\
& 15 \mathfrak{e}_2 - 15 \mu_2 \mathfrak{e}_2 + 2 \mu_1^2 (6 + 5 \mathfrak{e}_1 + 3 \mathfrak{e}_2) + \\
& 5 \eta^2 (2 \mu_2 + \mu_1^2 (8 + \mathfrak{e}_1 + \mathfrak{e}_2) + \mu_1 (44 - 10 \mu_2 + \mathfrak{e}_1 + \mathfrak{e}_2)) + \\
& \eta (60 + 82 \mu_2 + \mu_1^2 (42 + 31 \mathfrak{e}_1 + 11 \mathfrak{e}_2) + \\
& \quad \mu_1 (222 + 91 \mathfrak{e}_1 - 49 \mathfrak{e}_2 - 10 \mu_2 (5 + 12 \mathfrak{e}_2))) + \\
& x^2 (-1 + \eta)^2 ((-1 + \eta) \Theta p (60 \eta + 156 \eta^2 + 44 \eta^3 + 20 \eta^4 + 60 \eta^5 - 30 \eta t - \\
& 60 \eta \eta t - 24 \eta^2 \eta t - 80 \eta^3 \eta t - 60 \eta^4 \eta t + 48 \eta \mu_1 + \\
& 252 \eta^2 \mu_1 + 464 \eta^3 \mu_1 + 350 \eta^4 \mu_1 + 60 \eta^5 \mu_1 - 32 \eta t \mu_1 - \\
& 148 \eta \eta t \mu_1 - 120 \eta^2 \eta t \mu_1 - 56 \eta^3 \eta t \mu_1 - 60 \eta^4 \eta t \mu_1 - \\
& 12 \eta \mu_1^2 + 24 \eta^2 \mu_1^2 + 180 \eta^3 \mu_1^2 + 150 \eta^4 \mu_1^2 + 22 \eta t \mu_1^2 + \\
& 104 \eta \eta t \mu_1^2 + 48 \eta^2 \eta t \mu_1^2 + 24 \eta^3 \eta t \mu_1^2 + 32 \eta \mu_2 + 228 \eta^2 \mu_2 + \\
& 204 \eta^3 \mu_2 - 10 \eta t \mu_2 - 27 \eta \eta t \mu_2 - 24 \eta^2 \eta t \mu_2 + 56 \eta \mu_1 \mu_2 + \\
& 12 \eta^2 \mu_1 \mu_2 - 204 \eta^3 \mu_1 \mu_2 - 240 \eta^4 \mu_1 \mu_2 + 38 \eta t \mu_1 \mu_2 + \\
& 117 \eta \eta t \mu_1 \mu_2 + 192 \eta^2 \eta t \mu_1 \mu_2 + 120 \eta^3 \eta t \mu_1 \mu_2 + w^4 (-1 + \eta)^4 \\
& (12 \eta^3 (1 + \mu_1) - 12 \eta^2 (-1 + \eta t - 5 \mu_1 + \eta t \mu_1 - 4 \mu_1^2 + 3 \mu_1 \mu_2) + \\
& 2 \times (5 + 8 \mu_1 + 3 \mu_1^2 + 11 \mu_2 + 5 \mu_1 \mu_2) + \\
& \eta t (-12 - 22 \mu_1 + 38 \mu_1^2 + 5 \mu_2 + 17 \mu_1 \mu_2) + 2 \eta \\
& (16 + 37 \mu_1 + 21 \mu_1^2 + 33 \mu_2 - 27 \mu_1 \mu_2 + 6 \eta t (-1 - \mu_1 + 3 \mu_1 \mu_2))) - \\
& w^3 (-1 + \eta)^3 (40 \eta^4 (1 + \mu_1) + 2 \times (20 + 31 \mu_1 + 5 \mu_1^2 + 30 \mu_2 + 6 \mu_1 \mu_2) - \\
& 4 \eta^3 (-21 - 61 \mu_1 - 40 \mu_1^2 + 10 \eta t (1 + \mu_1) + 36 \mu_1 \mu_2) + \\
& \eta t (-66 - 130 \mu_1 + 128 \mu_1^2 + \mu_2 + 97 \mu_1 \mu_2) + \\
& 3 \eta (62 + 40 \mu_1^2 + 36 \eta t \mu_1^2 + 2 \mu_1 (63 - 34 \mu_2) + 112 \mu_2 - \\
& 9 \eta t (4 + \mu_2) + \eta t \mu_1 (-64 + 87 \mu_2)) + 12 \eta^2 (14 + 43 \mu_1 + \\
& 23 \mu_1^2 + 22 \mu_2 - 29 \mu_1 \mu_2 + \eta t (-7 - 7 \mu_1 + 12 \mu_1 \mu_2))) + \\
& w^2 (-1 + \eta)^2 (46 + 58 \mu_1 + 30 \eta^5 (1 + \mu_1) + 50 \mu_2 + 14 \mu_1 \mu_2 + \\
& \eta t (-124 - 224 \mu_1 + 164 \mu_1^2 - 23 \mu_2 + 181 \mu_1 \mu_2) - \\
& 10 \eta^4 (3 \eta t (1 + \mu_1) - 4 \times (4 + 7 \mu_1 + 3 \mu_1^2 - 3 \mu_1 \mu_2)) + \\
& 4 \eta^3 (70 + 255 \mu_1 + 125 \mu_1^2 + 55 \mu_2 - 161 \mu_1 \mu_2 + \\
& 10 \eta t (-4 - 4 \mu_1 + 3 \mu_1 \mu_2)) + 12 \eta^2 (38 + 106 \mu_1 + 38 \mu_1^2 + \\
& 65 \mu_2 - 61 \mu_1 \mu_2 + \eta t (-15 - 23 \mu_1 + 4 \mu_1^2 - 2 \mu_2 + 40 \mu_1 \mu_2)) + \\
& \eta (2 \times (155 + 278 \mu_1 + 51 \mu_1^2 + 249 \mu_2 - 69 \mu_1 \mu_2) + \\
& 3 \eta t (-80 - 164 \mu_1 + 108 \mu_1^2 - 27 \mu_2 + 177 \mu_1 \mu_2))) - \\
& w (-1 + \eta) \times (90 \eta^5 (1 + \mu_1) - 4 \times (1 + \mu_1) \times (-5 + \mu_1 - 3 \mu_2) + \\
& 10 \eta^4 (20 + 65 \mu_1 + 27 \mu_1^2 - 9 \eta t (1 + \mu_1) - 36 \mu_1 \mu_2) + \\
& \eta t (-100 - 148 \mu_1 + 96 \mu_1^2 - 29 \mu_2 + 139 \mu_1 \mu_2) + \\
& 12 \eta^2 (34 + 85 \mu_1 + 21 \mu_1^2 + 62 \mu_2 - 34 \mu_1 \mu_2 + \eta t \\
& (-11 - 27 \mu_1 + 8 \mu_1^2 - 4 \mu_2 + 44 \mu_1 \mu_2)) + 4 \eta^3 (63 + 313 \mu_1 + 130 \\
& \mu_1^2 + 106 \mu_2 - 176 \mu_1 \mu_2 + \eta t (-50 - 44 \mu_1 + 6 \mu_1^2 + 60 \mu_1 \mu_2)) + \\
& \eta (4 \times (54 + 75 \mu_1 + 3 \mu_1^2 + 65 \mu_2 + 17 \mu_1 \mu_2) + \eta t \\
& (-204 - 460 \mu_1 + 320 \mu_1^2 - 81 \mu_2 + 423 \mu_1 \mu_2))) + \\
& (-1 + \eta t) \Theta l (-10 - 60 \eta - 60 \eta^2 + 10 \Theta p + 30 \eta \Theta p - 36 \eta^2 \Theta p - \\
& 20 \eta^3 \Theta p + 60 \eta^4 \Theta p - 8 \mu_1 - 64 \eta \mu_1 - 164 \eta^2 \mu_1 - 80 \eta^3 \mu_1 + \\
& 16 \eta^4 \mu_1 + 8 \Theta p \mu_1 + 56 \eta \Theta p \mu_1 + 18 \eta^2 \Theta p \mu_1 - 192 \eta^3 \Theta p \mu_1 - \\
& 170 \eta^4 \Theta p \mu_1 + 2 \mu_1^2 - 4 \eta \mu_1^2 + 28 \eta^2 \mu_1^2 + 16 \eta^3 \mu_1^2 +
\end{aligned}$$

$$\begin{aligned}
& 16 \eta^4 \mu_1^2 - 2 \operatorname{ep} \mu_1^2 - 10 \eta \operatorname{ep} \mu_1^2 - 18 \eta^2 \operatorname{ep} \mu_1^2 - 52 \eta^3 \operatorname{ep} \mu_1^2 - \\
& 50 \eta^4 \operatorname{ep} \mu_1^2 - 5 \mu_2 - 20 \eta \mu_2 - 15 \eta^2 \mu_2 + 10 \operatorname{ep} \mu_2 + 44 \eta \operatorname{ep} \mu_2 - \\
& 6 \eta^2 \operatorname{ep} \mu_2 - 72 \eta^3 \operatorname{ep} \mu_2 - 20 \eta^4 \operatorname{ep} \mu_2 + 19 \mu_1 \mu_2 + 76 \eta \mu_1 \mu_2 + \\
& 57 \eta^2 \mu_1 \mu_2 - 14 \operatorname{ep} \mu_1 \mu_2 - 112 \eta \operatorname{ep} \mu_1 \mu_2 - 186 \eta^2 \operatorname{ep} \mu_1 \mu_2 + \\
& 100 \eta^4 \operatorname{ep} \mu_1 \mu_2 + 2 w^4 (-1 + \eta)^4 (\mu_1^2 + 5 \mu_1 (-2 + \mu_2) + \\
& \quad 5 \times (-1 + \mu_2) + 5 \eta (-2 + 4 \mu_1^2 + \mu_1 (-4 + \mu_2) + \mu_2)) - \\
& 5 \operatorname{ep} \mathfrak{x}1 - 30 \eta \operatorname{ep} \mathfrak{x}1 - 30 \eta^2 \operatorname{ep} \mathfrak{x}1 - 4 \operatorname{ep} \mu_1 \mathfrak{x}1 - 50 \eta \operatorname{ep} \mu_1 \mathfrak{x}1 - \\
& 129 \eta^2 \operatorname{ep} \mu_1 \mathfrak{x}1 - 96 \eta^3 \operatorname{ep} \mu_1 \mathfrak{x}1 - 10 \eta^4 \operatorname{ep} \mu_1 \mathfrak{x}1 + \operatorname{ep} \mu_1^2 \mathfrak{x}1 - \\
& 2 \eta \operatorname{ep} \mu_1^2 \mathfrak{x}1 - 27 \eta^2 \operatorname{ep} \mu_1^2 \mathfrak{x}1 - 36 \eta^3 \operatorname{ep} \mu_1^2 \mathfrak{x}1 - 10 \eta^4 \operatorname{ep} \mu_1^2 \mathfrak{x}1 - \\
& 5 \operatorname{ep} \mu_2 \mathfrak{x}1 - 30 \eta \operatorname{ep} \mu_2 \mathfrak{x}1 - 30 \eta^2 \operatorname{ep} \mu_2 \mathfrak{x}1 - 5 \operatorname{ep} \mu_1 \mu_2 \mathfrak{x}1 - \\
& 30 \eta \operatorname{ep} \mu_1 \mu_2 \mathfrak{x}1 - 30 \eta^2 \operatorname{ep} \mu_1 \mu_2 \mathfrak{x}1 + 5 \operatorname{ep} \mathfrak{x}2 + 30 \eta \operatorname{ep} \mathfrak{x}2 + \\
& 30 \eta^2 \operatorname{ep} \mathfrak{x}2 + 4 \operatorname{ep} \mu_1 \mathfrak{x}2 + 40 \eta \operatorname{ep} \mu_1 \mathfrak{x}2 + 87 \eta^2 \operatorname{ep} \mu_1 \mathfrak{x}2 + \\
& 44 \eta^3 \operatorname{ep} \mu_1 \mathfrak{x}2 - 10 \eta^4 \operatorname{ep} \mu_1 \mathfrak{x}2 - \operatorname{ep} \mu_1^2 \mathfrak{x}2 - 8 \eta \operatorname{ep} \mu_1^2 \mathfrak{x}2 - \\
& 15 \eta^2 \operatorname{ep} \mu_1^2 \mathfrak{x}2 - 16 \eta^3 \operatorname{ep} \mu_1^2 \mathfrak{x}2 - 10 \eta^4 \operatorname{ep} \mu_1^2 \mathfrak{x}2 + 5 \operatorname{ep} \mu_2 \mathfrak{x}2 + \\
& 30 \eta \operatorname{ep} \mu_2 \mathfrak{x}2 + 30 \eta^2 \operatorname{ep} \mu_2 \mathfrak{x}2 - 7 \operatorname{ep} \mu_1 \mu_2 \mathfrak{x}2 - 6 \eta \operatorname{ep} \mu_1 \mu_2 \mathfrak{x}2 + \\
& 102 \eta^2 \operatorname{ep} \mu_1 \mu_2 \mathfrak{x}2 + 120 \eta^3 \operatorname{ep} \mu_1 \mu_2 \mathfrak{x}2 - w^3 (-1 + \eta)^3 (8 \mu_1^2 + \\
& \quad 3 \eta^2 (12 \mu_1^2 + \mu_1 (-52 + \mu_2 (19 - 10 \operatorname{ep} (\mathfrak{x}1 - \mathfrak{x}2)) - 22 \operatorname{ep} (\mathfrak{x}1 - \mathfrak{x}2)) - \\
& \quad 5 \times (4 + \mu_2 + 2 \operatorname{ep} (\mathfrak{x}1 - \mathfrak{x}2) + 2 \operatorname{ep} \mu_2 (\mathfrak{x}1 - \mathfrak{x}2))) + 2 \eta \\
& \quad (46 \mu_1^2 + \mu_1 (-128 + \mu_2 (53 - 15 \operatorname{ep} (\mathfrak{x}1 - \mathfrak{x}2)) - 33 \operatorname{ep} (\mathfrak{x}1 - \mathfrak{x}2)) - \\
& \quad 5 \times (12 - \mu_2 + 3 \operatorname{ep} (\mathfrak{x}1 - \mathfrak{x}2) + 3 \operatorname{ep} \mu_2 (\mathfrak{x}1 - \mathfrak{x}2))) - \\
& \quad 5 \times (8 + \mu_2 (-5 + \operatorname{ep} (\mathfrak{x}1 - \mathfrak{x}2)) + \operatorname{ep} (\mathfrak{x}1 - \mathfrak{x}2)) + \\
& \quad \mu_1 (-68 - 11 \operatorname{ep} (\mathfrak{x}1 - \mathfrak{x}2) + \mu_2 (49 - 5 \operatorname{ep} \mathfrak{x}1 + 5 \operatorname{ep} \mathfrak{x}2))) - \\
& w^2 (-1 + \eta)^2 (-3 \times (4 \mu_1^2 + 5 \times (-4 + \mu_2) + \mu_1 (-28 + 29 \mu_2)) - \\
& \quad \operatorname{ep} (-((1 + \mu_2) \times (-14 + 15 \mathfrak{x}1 - 15 \mathfrak{x}2)) + \mu_1^2 (\mathfrak{x}1 - \mathfrak{x}2) + \\
& \quad 26 \mu_1 (1 - \mathfrak{x}1 + \mathfrak{x}2) + \mu_1 \mu_2 (-34 - 15 \mathfrak{x}1 + 3 \mathfrak{x}2)) + \\
& \quad 3 \eta (80 + 152 \mu_1 - 20 \mu_1^2 + 10 \mu_2 - 86 \mu_1 \mu_2 + \operatorname{ep} \\
& \quad (\mu_1 (-26 + 61 \mathfrak{x}1 + 6 \mu_2 (9 + 5 \mathfrak{x}1 - 3 \mathfrak{x}2)) - 57 \mathfrak{x}2) + \\
& \quad 6 \times (1 + \mu_2) \times (-3 + 5 \mathfrak{x}1 - 5 \mathfrak{x}2) + \mu_1^2 (4 + \mathfrak{x}1 + 3 \mathfrak{x}2))) + \\
& \quad 3 \eta^2 (60 + 156 \mu_1 - 36 \mu_1^2 + 15 \mu_2 - 57 \mu_1 \mu_2 + 2 \operatorname{ep} \\
& \quad (\mu_1 (26 + 44 \mathfrak{x}1 + 3 \mu_2 (2 + 5 \mathfrak{x}1 - 9 \mathfrak{x}2)) - 36 \mathfrak{x}2) + \\
& \quad 3 \times (1 + \mu_2) \times (2 + 5 \mathfrak{x}1 - 5 \mathfrak{x}2) + \mu_1^2 (8 + 5 \mathfrak{x}1 + 3 \mathfrak{x}2))) + \\
& \quad 2 \eta^3 (-8 \times (-5 + \mu_1) \mu_1 + 5 \operatorname{ep} (10 \times (1 + \mu_2) + \mu_1^2 \\
& \quad (4 + 3 \mathfrak{x}1 + \mathfrak{x}2) + \mu_1 (26 + 9 \mathfrak{x}1 - 5 \mathfrak{x}2 - 2 \mu_2 (7 + 6 \mathfrak{x}2)))) + \\
& w (-1 + \eta) \times (40 + 44 \mu_1 - 8 \mu_1^2 + 5 \mu_2 - 67 \mu_1 \mu_2 + 2 \eta^4 \\
& \quad (10 \operatorname{ep} \mu_2 + \mu_1^2 (-8 + 5 \operatorname{ep} (5 + \mathfrak{x}1 + \mathfrak{x}2)) + \\
& \quad \mu_1 (-8 + 5 \operatorname{ep} (23 - 10 \mu_2 + \mathfrak{x}1 + \mathfrak{x}2))) + \operatorname{ep} (3 \mu_2 \\
& \quad (-8 + 5 \mathfrak{x}1 - 5 \mathfrak{x}2) + 5 \times (-4 + 3 \mathfrak{x}1 - 3 \mathfrak{x}2) + \mu_1^2 (2 - 2 \mathfrak{x}1 + 2 \mathfrak{x}2) + \\
& \quad \mu_1 (-30 + 19 \mathfrak{x}1 - 19 \mathfrak{x}2 + 3 \mu_2 (16 + 5 \mathfrak{x}1 + 3 \mathfrak{x}2))) + \\
& \quad \eta (-4 \mu_1^2 + \mu_1 (304 - 238 \mu_2) + 50 \times (4 + \mu_2) + \operatorname{ep} (-84 + 90 \mathfrak{x}1 + \\
& \quad \mu_1 (-134 + 167 \mathfrak{x}1 + 2 \mu_2 (137 + 45 \mathfrak{x}1 - 9 \mathfrak{x}2)) - 145 \mathfrak{x}2) + \\
& \quad \mu_2 (-98 + 90 \mathfrak{x}1 - 90 \mathfrak{x}2) - 90 \mathfrak{x}2 + \mu_1^2 (22 + 5 \mathfrak{x}1 + 17 \mathfrak{x}2))) + \\
& \quad \eta^2 (-100 \mu_1^2 + \mu_1 (476 - 171 \mu_2) + 45 \times (4 + \mu_2) + 3 \operatorname{ep} (8 + 30 \\
& \quad \mathfrak{x}1 + \mu_1 (30 + 109 \mathfrak{x}1 + \mu_2 (74 + 30 \mathfrak{x}1 - 78 \mathfrak{x}2)) - 79 \mathfrak{x}2) + 2 \mu_2 \\
& \quad (7 + 15 \mathfrak{x}1 - 15 \mathfrak{x}2) - 30 \mathfrak{x}2 + \mu_1^2 (19 \mathfrak{x}1 + 11 \times (2 + \mathfrak{x}2)))) +
\end{aligned}$$



$$\begin{aligned}
& 2 \eta^3 \left( -16 \times (-5 + \mu_1) \mu_1 + \text{op} \left( 60 + 86 \mu_2 + \mu_1^2 (46 + 33 \mathfrak{z}_1 + 13 \mathfrak{z}_2) + \right. \right. \\
& \quad \left. \left. \mu_1 (226 + 93 \mathfrak{z}_1 - 47 \mathfrak{z}_2 - 10 \mu_2 (7 + 12 \mathfrak{z}_2)) \right) \right) + \\
& x^5 (-1 + \eta)^5 \left( -4 \times (-1 + w (-1 + \eta)) \times (-1 + \eta t) \text{el} \mu_1 (5 + w (-1 + \eta) \times \right. \\
& \quad \left. (-5 + \mu_1) - \mu_1 - \eta (1 + \mu_1)) + \right. \\
& \text{op} \left( 2 - 18 \eta + 40 \eta^2 - 24 \eta^3 - 8 \eta t - 16 \eta \eta t + 24 \eta^2 \eta t - 2 \text{el} + \right. \\
& \quad 24 \eta \text{el} + 2 \eta t \text{el} - 24 \eta \eta t \text{el} + 44 \mu_1 + 72 \eta \mu_1 - 92 \eta^2 \mu_1 - \\
& \quad 24 \eta^3 \mu_1 - 8 \eta t \mu_1 - 16 \eta \eta t \mu_1 + 24 \eta^2 \eta t \mu_1 - 18 \text{el} \mu_1 - \\
& \quad 62 \eta \text{el} \mu_1 + 18 \eta t \text{el} \mu_1 + 62 \eta \eta t \text{el} \mu_1 + 18 \mu_1^2 + \\
& \quad 42 \eta \mu_1^2 - 60 \eta^2 \mu_1^2 - 4 \text{el} \mu_1^2 - 14 \eta \text{el} \mu_1^2 + 4 \eta t \text{el} \mu_1^2 + \\
& \quad 14 \eta \eta t \text{el} \mu_1^2 + 4 w^3 (-1 + \eta)^4 (1 + \mu_1) (\eta - \eta t + 4 \mu_1) + \\
& \quad 18 \mu_2 - 18 \eta \mu_2 - 6 \text{el} \mu_2 - 2 \eta \text{el} \mu_2 + 6 \eta t \text{el} \mu_2 + \\
& \quad 2 \eta \eta t \text{el} \mu_2 + 6 \mu_1 \mu_2 - 30 \eta \mu_1 \mu_2 + 24 \eta^2 \mu_1 \mu_2 + 12 \eta t \mu_1 \mu_2 - \\
& \quad 12 \eta \eta t \mu_1 \mu_2 - 6 \text{el} \mu_1 \mu_2 + 10 \eta \text{el} \mu_1 \mu_2 + 6 \eta t \text{el} \mu_1 \mu_2 - \\
& \quad 10 \eta \eta t \text{el} \mu_1 \mu_2 - 9 \text{el} \mu_1 \mathfrak{z}_1 - \eta \text{el} \mu_1 \mathfrak{z}_1 + 9 \eta t \text{el} \mu_1 \mathfrak{z}_1 + \\
& \quad \eta \eta t \text{el} \mu_1 \mathfrak{z}_1 - 3 \text{el} \mu_1^2 \mathfrak{z}_1 - \eta \text{el} \mu_1^2 \mathfrak{z}_1 + 3 \eta t \text{el} \mu_1^2 \mathfrak{z}_1 + \\
& \quad \eta \eta t \text{el} \mu_1^2 \mathfrak{z}_1 + 5 \text{el} \mu_1 \mathfrak{z}_2 - \eta \text{el} \mu_1 \mathfrak{z}_2 - 5 \eta t \text{el} \mu_1 \mathfrak{z}_2 + \\
& \quad \eta \eta t \text{el} \mu_1 \mathfrak{z}_2 - \text{el} \mu_1^2 \mathfrak{z}_2 - \eta \text{el} \mu_1^2 \mathfrak{z}_2 + \eta t \text{el} \mu_1^2 \mathfrak{z}_2 + \\
& \quad \eta \eta t \text{el} \mu_1^2 \mathfrak{z}_2 + 12 \text{el} \mu_1 \mu_2 \mathfrak{z}_2 - 12 \eta t \text{el} \mu_1 \mu_2 \mathfrak{z}_2 - \\
& \quad w^2 (-1 + \eta)^2 \left( -10 + 10 \text{el} - 84 \mu_1 + 26 \text{el} \mu_1 - 50 \mu_1^2 + 4 \text{el} \mu_1^2 + \right. \\
& \quad 12 \eta^3 (1 + \mu_1) - 22 \mu_2 + 10 \text{el} \mu_2 + 14 \mu_1 \mu_2 - 14 \text{el} \mu_1 \mu_2 + \\
& \quad 4 \eta^2 (1 + 13 \mu_1 + 12 \mu_1^2 - 3 \eta t (1 + \mu_1) - 3 \mu_1 \mu_2) + \\
& \quad 2 \eta (-3 + 10 \mu_1 + \mu_1^2 + 11 \mu_2 - \mu_1 \mu_2 + \eta t (-2 - 2 \mu_1 + 6 \mu_1 \mu_2)) + \\
& \quad 9 \text{el} \mu_1 \mathfrak{z}_1 + 3 \text{el} \mu_1^2 \mathfrak{z}_1 - 5 \text{el} \mu_1 \mathfrak{z}_2 + \text{el} \mu_1^2 \mathfrak{z}_2 - 12 \text{el} \mu_1 \mu_2 \mathfrak{z}_2 - \\
& \quad \eta t (-16 + 10 \text{el} (1 + \mu_2) + 4 \mu_1 (-4 + 3 \mu_2) + \text{el} \mu_1^2 (4 + 3 \mathfrak{z}_1 + \mathfrak{z}_2) + \\
& \quad \text{el} \mu_1 (26 + 9 \mathfrak{z}_1 - 5 \mathfrak{z}_2 - 2 \mu_2 (7 + 6 \mathfrak{z}_2))) + w (-1 + \eta) \times \\
& \quad (36 \eta^3 (1 + \mu_1) - 4 \eta^2 (4 - 27 \mu_1^2 + 9 \eta t (1 + \mu_1) + \mu_1 (-41 + 9 \mu_2)) + \\
& \quad \eta (-8 + 40 \mu_2 + 2 \text{el} \mu_2 + \mu_1^2 (-56 + \text{el} (14 + \mathfrak{z}_1 + \mathfrak{z}_2)) + \\
& \quad \mu_1 (-88 + 28 \mu_2 + \text{el} (86 - 10 \mu_2 + \mathfrak{z}_1 + \mathfrak{z}_2)) - \\
& \quad \eta t (-8 \mu_1 (2 + 3 \mu_2) + 2 \times (-8 + \text{el} \mu_2) + \\
& \quad \text{el} \mu_1^2 (14 + \mathfrak{z}_1 + \mathfrak{z}_2) + \text{el} \mu_1 (86 - 10 \mu_2 + \mathfrak{z}_1 + \mathfrak{z}_2))) - \\
& \quad 2 \times (6 + 56 \mu_1 + 26 \mu_1^2 + 20 \mu_2 - 4 \mu_1 \mu_2 - \text{el} (6 + 8 \mu_2 + \\
& \quad \mu_1^2 (4 + 3 \mathfrak{z}_1 + \mathfrak{z}_2) + \mu_1 (22 + 9 \mathfrak{z}_1 - 5 \mathfrak{z}_2 - 4 \mu_2 (1 + 3 \mathfrak{z}_2))) + \\
& \quad \eta t (2 \times (-5 + \mu_1 (-5 + 6 \mu_2)) + \text{el} (6 + 8 \mu_2 + \mu_1^2 (4 + 3 \mathfrak{z}_1 + \mathfrak{z}_2) + \\
& \quad \mu_1 (22 + 9 \mathfrak{z}_1 - 5 \mathfrak{z}_2 - 4 \mu_2 (1 + 3 \mathfrak{z}_2)))))) - \\
& x (-1 + \eta) \times (4 w^2 (3 - 5 w + 2 w^2) \eta^9 \text{op} (1 + \mu_1) - 4 w \eta^8 \text{op} (9 \times (1 + \mu_1) + \\
& \quad w^3 (7 - \mu_1 - 8 \mu_1^2 + 2 \eta t (1 + \mu_1) + 9 \mu_1 \mu_2) + \\
& \quad w (-11 - 23 \mu_1 - 12 \mu_1^2 + 3 \eta t (1 + \mu_1) + 15 \mu_1 \mu_2) - \\
& \quad w^2 (6 - 14 \mu_1 - 20 \mu_1^2 + 5 \eta t (1 + \mu_1) + 24 \mu_1 \mu_2)) - \\
& (1 + w)^3 (5 w \text{el} (1 + \mu_1) \mu_2 - 5 w \eta t \text{el} (1 + \mu_1) \mu_2 + \\
& \quad \eta t \text{op} (2 \mu_1^2 + 2 w (7 \mu_1^2 + 5 \mu_1 (-2 + \mu_2) + 5 \times (-1 + \mu_2)) - \\
& \quad 5 \times (2 + \mu_2) + \mu_1 (-8 + 19 \mu_2))) + 2 \eta^7 \text{op} \\
& (12 \times (1 + \mu_1) + 2 w (-7 - 52 \mu_1 - 27 \mu_1^2 + 9 \eta t (1 + \mu_1) + 45 \mu_1 \mu_2) - \\
& \quad 2 w^3 (6 - 16 \mu_1 - 34 \mu_1^2 + 44 \mu_2 + 23 \mu_1 \mu_2 + 6 \eta t (1 + \mu_1 + 4 \mu_1 \mu_2)) + \\
& \quad w^4 (27 - 32 \mu_1 - 59 \mu_1^2 + 33 \mu_2 + 57 \mu_1 \mu_2 + 2 \eta t (7 + 7 \mu_1 + 9 \mu_1 \mu_2)) +
\end{aligned}$$

$$\begin{aligned}
& w^2 \left( -17 + 96 \mu_1 + 53 \mu_1^2 + 55 \mu_2 - 113 \mu_1 \mu_2 + \right. \\
& \quad \left. \eta t \left( -22 - 22 \mu_1 + 30 \mu_1 \mu_2 \right) \right) + \eta^2 \left( \theta p \left( -60 + (12 - 56 \eta t) \mu_1^2 - \right. \right. \\
& \quad \left. \left. 28 \mu_2 + 7 \eta t \mu_2 - \mu_1 (48 - 88 \eta t + 76 \mu_2 + 41 \eta t \mu_2) - \right. \right. \\
& \quad \left. \left. 2 w \left( 3 \eta t \left( 26 + 14 \mu_1 + 8 \mu_1^2 + 5 \mu_2 - 11 \mu_1 \mu_2 \right) + 2 \times (34 + 59 \mu_1 + \right. \right. \right. \\
& \quad \left. \left. \left. 7 \mu_1^2 + 52 \mu_2 + 10 \mu_1 \mu_2 \right) \right) + 2 w^4 \left( 33 + 42 \mu_1 + 9 \mu_1^2 + 77 \mu_2 + \right. \right. \\
& \quad \left. \left. 83 \mu_1 \mu_2 + \eta t \left( -4 - 4 \mu_1 + 90 \mu_1^2 - 25 \mu_2 + 17 \mu_1 \mu_2 \right) \right) \right) + \\
& \quad 2 w^2 \left( -19 - 106 \mu_1 - 51 \mu_1^2 - 99 \mu_2 + 123 \mu_1 \mu_2 + \right. \\
& \quad \left. 3 \eta t \left( -54 - 100 \mu_1 + 44 \mu_1^2 - 17 \mu_2 + 49 \mu_1 \mu_2 \right) \right) + \\
& \quad w^3 \left( 8 \times (16 + 14 \mu_1 - 5 \mu_1^2 + 18 \mu_2 + 42 \mu_1 \mu_2) + \right. \\
& \quad \left. \eta t \left( -180 - 440 \mu_1 + 436 \mu_1^2 - 115 \mu_2 + 221 \mu_1 \mu_2 \right) \right) + \\
& \quad (-1 + \eta t) \theta l \left( w^3 \left( 60 + 100 \mu_1^2 + \mu_1 (76 - 49 \mu_2) - 25 \mu_2 \right) + \right. \\
& \quad \left. w^4 \left( 30 + 60 \mu_1 + 54 \mu_1^2 - 5 \mu_2 - 5 \mu_1 \mu_2 \right) - 2 \times (7 \mu_1^2 + \mu_1 (16 - 19 \mu_2) + \right. \\
& \quad \left. 5 \times (3 + \mu_2)) - 4 w \left( 15 + 27 \mu_1 + 9 \mu_1^2 + 5 \mu_2 - 13 \mu_1 \mu_2 + \theta p \right. \right. \\
& \quad \left. \left( -11 + 15 \mathfrak{e}1 + \mu_1 (-19 + 32 \mathfrak{e}1 + \mu_2 (47 + 15 \mathfrak{e}1 - 9 \mathfrak{e}2) - 27 \mathfrak{e}2) + \right. \right. \\
& \quad \left. \left. \mu_2 (-13 + 15 \mathfrak{e}1 - 15 \mathfrak{e}2) - 15 \mathfrak{e}2 + \mu_1^2 (4 + 2 \mathfrak{e}1 + 3 \mathfrak{e}2) \right) \right) - \\
& \quad \theta p \left( \mu_2 (-46 + 30 \mathfrak{e}1 - 30 \mathfrak{e}2) + 30 \times (-1 + \mathfrak{e}1 - \mathfrak{e}2) + \right. \\
& \quad \left. \mu_1^2 (8 + \mathfrak{e}1 + 7 \mathfrak{e}2) + \mu_1 (-58 + 49 \mathfrak{e}1 - 41 \mathfrak{e}2 + 2 \mu_2 (61 + 15 \mathfrak{e}1 + \right. \\
& \quad \left. 3 \mathfrak{e}2)) \right) - w^2 \left( 6 \times (-4 \mu_1^2 + 5 \mu_2 + 5 \mu_1 (2 + \mu_2)) + \right. \\
& \quad \left. \theta p \left( \mu_1 (26 + 79 \mathfrak{e}1 + \mu_2 (26 + 30 \mathfrak{e}1 - 42 \mathfrak{e}2) - 67 \mathfrak{e}2) + \right. \right. \\
& \quad \left. \left. 2 \times (1 + \mu_2) \times (1 + 15 \mathfrak{e}1 - 15 \mathfrak{e}2) + \mu_1^2 (12 + 7 \mathfrak{e}1 + 5 \mathfrak{e}2) \right) \right) \Big) - \\
& \quad \eta \left( \theta p \left( \eta t \left( -50 - 56 \mu_1 + 18 \mu_1^2 - 15 \mu_2 + 57 \mu_1 \mu_2 \right) + 2 w^3 \right. \right. \\
& \quad \left. \left( \eta t \left( 14 + 6 \mu_1 + 10 \mu_1^2 - 49 \mu_2 - \mu_1 \mu_2 \right) + 2 \times (20 + 31 \mu_1 + 5 \mu_1^2 + \right. \right. \\
& \quad \left. \left. 30 \mu_2 + 6 \mu_1 \mu_2) \right) + w^4 \left( 4 \times (5 + 8 \mu_1 + 3 \mu_1^2 + 11 \mu_2 + 5 \mu_1 \mu_2) - \right. \right. \\
& \quad \left. \left. 2 \eta t \left( -13 - 28 \mu_1 + 3 \mu_1^2 + 20 \mu_2 + 8 \mu_1 \mu_2 \right) \right) + \right. \\
& \quad \left. 4 w \left( -2 \times (1 + \mu_1) \times (-5 + \mu_1 - 3 \mu_2) + \eta t \left( -30 - 52 \mu_1 + 17 \mu_1^2 - \right. \right. \right. \\
& \quad \left. \left. 12 \mu_2 + 36 \mu_1 \mu_2) \right) + w^2 \left( 4 \times (23 + 29 \mu_1 + 25 \mu_2 + 7 \mu_1 \mu_2) + \right. \right. \\
& \quad \left. \left. \eta t \left( -68 - 196 \mu_1 + 76 \mu_1^2 - 91 \mu_2 + 101 \mu_1 \mu_2 \right) \right) \right) + (-1 + \eta t) \\
& \quad \theta l \left( 10 + 8 \mu_1 - 2 \mu_1^2 + 5 \mu_2 - 19 \mu_1 \mu_2 + 10 w^4 (1 + \mu_1) \times (1 + \mu_1 + \mu_2) + \right. \\
& \quad \left. 2 w^3 \left( 14 \mu_1^2 + 5 \times (4 + \mu_2 (2 + \theta p (\mathfrak{e}1 - \mathfrak{e}2)) + \theta p (\mathfrak{e}1 - \mathfrak{e}2)) + \right. \right. \\
& \quad \left. \left. \mu_1 (34 + \mu_2 (-2 + 5 \theta p (\mathfrak{e}1 - \mathfrak{e}2)) + 11 \theta p (\mathfrak{e}1 - \mathfrak{e}2)) \right) - \right. \\
& \quad \left. 2 \theta p \mu_1^2 (-2 + \mathfrak{e}1 - \mathfrak{e}2) + 10 \theta p (1 + \mu_2) \times (-2 + \mathfrak{e}1 - \mathfrak{e}2) + \right. \\
& \quad \left. 2 \theta p \mu_1 (5 \mu_2 \mathfrak{e}1 + 4 \times (-2 + \mathfrak{e}1 - \mathfrak{e}2) + 7 \mu_2 (2 + \mathfrak{e}2)) + \right. \\
& \quad \left. w^2 \left( 3 \times (8 \mu_1^2 + \mu_1 (28 - 19 \mu_2) + 5 \times (4 + \mu_2)) - \right. \right. \\
& \quad \left. \left. 2 \theta p \left( -((1 + \mu_2) \times (-14 + 15 \mathfrak{e}1 - 15 \mathfrak{e}2)) + \mu_1^2 (\mathfrak{e}1 - \mathfrak{e}2) + \right. \right. \right. \\
& \quad \left. \left. 26 \mu_1 (1 - \mathfrak{e}1 + \mathfrak{e}2) + \mu_1 \mu_2 (-34 - 15 \mathfrak{e}1 + 3 \mathfrak{e}2) \right) \right) + \\
& \quad \left. w \left( 40 + 44 \mu_1 + 4 \mu_1^2 + 10 \mu_2 - 62 \mu_1 \mu_2 + \theta p \left( 6 \mu_2 (-8 + 5 \mathfrak{e}1 - \right. \right. \right. \\
& \quad \left. \left. 5 \mathfrak{e}2) + 10 \times (-4 + 3 \mathfrak{e}1 - 3 \mathfrak{e}2) + \mu_1^2 (4 - 4 \mathfrak{e}1 + 4 \mathfrak{e}2) + \right. \right. \\
& \quad \left. \left. 2 \mu_1 (-30 + 19 \mathfrak{e}1 - 19 \mathfrak{e}2 + 3 \mu_2 (16 + 5 \mathfrak{e}1 + 3 \mathfrak{e}2)) \right) \right) \Big) + \\
& \quad \eta^4 \left( 78 \theta p + 24 \eta t \theta p + 10 \theta l \theta p - 10 \eta t \theta l \theta p + 20 \theta l \mu_1 - 20 \eta t \theta l \mu_1 - \right. \\
& \quad \left. 68 \theta p \mu_1 - 56 \eta t \theta p \mu_1 + 98 \theta l \theta p \mu_1 - 98 \eta t \theta l \theta p \mu_1 - \right. \\
& \quad \left. 4 \theta l \mu_1^2 + 4 \eta t \theta l \mu_1^2 - 74 \theta p \mu_1^2 + 16 \eta t \theta p \mu_1^2 + \right. \\
& \quad \left. 28 \theta l \theta p \mu_1^2 - 28 \eta t \theta l \theta p \mu_1^2 + 46 \theta p \mu_2 - 16 \eta t \theta p \mu_2 + \right. \\
& \quad \left. 38 \theta l \theta p \mu_2 - 38 \eta t \theta l \theta p \mu_2 + 154 \theta p \mu_1 \mu_2 + \right.
\end{aligned}$$

$$\begin{aligned}
& 68 \eta t \partial p \mu_1 \mu_2 - 10 \partial l \partial p \mu_1 \mu_2 + 10 \eta t \partial l \partial p \mu_1 \mu_2 + \\
& w^4 \left( (-1 + \eta t) \partial l \left( 124 \mu_1^2 - 5 \times (4 + \mu_2) - 5 \mu_1 (8 + \mu_2) \right) + \right. \\
& \quad 2 \partial p \left( -2 \times \left( 22 + 57 \mu_1 + 35 \mu_1^2 + 55 \mu_2 - 170 \mu_1 \mu_2 \right) + \right. \\
& \quad \quad \left. 5 \eta t \left( -11 - 26 \mu_1 + 57 \mu_1^2 + 5 \mu_2 - 7 \mu_1 \mu_2 \right) \right) \left. \right) + 49 \partial l \partial p \mu_1 \mathfrak{x}_1 - \\
& 49 \eta t \partial l \partial p \mu_1 \mathfrak{x}_1 + 19 \partial l \partial p \mu_1^2 \mathfrak{x}_1 - 19 \eta t \partial l \partial p \mu_1^2 \mathfrak{x}_1 - \\
& w^3 \left( \partial p \left( 8 \times \left( 47 - 2 \mu_1^2 + \mu_1 (63 - 58 \mu_2) + 104 \mu_2 \right) + \right. \right. \\
& \quad \eta t \left( 44 - 236 \mu_1^2 - 145 \mu_2 + \mu_1 (24 + 455 \mu_2) \right) \left. \right) - (-1 + \eta t) \partial l \\
& \quad \left( 64 \mu_1^2 + \mu_1 (-160 + \mu_2 (53 - 20 \partial p (\mathfrak{x}_1 - \mathfrak{x}_2)) - 44 \partial p (\mathfrak{x}_1 - \mathfrak{x}_2)) - \right. \\
& \quad \quad \left. 5 \times (16 - \mu_2 + 4 \partial p (\mathfrak{x}_1 - \mathfrak{x}_2) + 4 \partial p \mu_2 (\mathfrak{x}_1 - \mathfrak{x}_2)) \right) \left. \right) - \\
& 21 \partial l \partial p \mu_1 \mathfrak{x}_2 + 21 \eta t \partial l \partial p \mu_1 \mathfrak{x}_2 + 9 \partial l \partial p \mu_1^2 \mathfrak{x}_2 - 9 \eta t \partial l \\
& \quad \partial p \mu_1^2 \mathfrak{x}_2 - 60 \partial l \partial p \mu_1 \mu_2 \mathfrak{x}_2 + 60 \eta t \partial l \partial p \mu_1 \mu_2 \mathfrak{x}_2 + \\
& w \left( \partial p \left( 4 \times \left( 49 + 16 \mu_1^2 + \mu_1 (107 - 68 \mu_2) + 130 \mu_2 \right) + \right. \right. \\
& \quad \eta t \left( 128 - 132 \mu_1^2 + 17 \mu_2 + \mu_1 (116 + 161 \mu_2) \right) \left. \right) + \\
& \quad (-1 + \eta t) \partial l \left( 60 + 120 \mu_1 + 15 \mu_2 - 57 \mu_1 \mu_2 + \partial p \left( -44 + 60 \mathfrak{x}_1 + \right. \right. \\
& \quad \quad \mu_1 (-170 + 123 \mathfrak{x}_1 + \mu_2 (238 + 60 \mathfrak{x}_1 - 36 \mathfrak{x}_2) - 113 \mathfrak{x}_2) + \\
& \quad \quad \left. \mu_2 (-62 + 60 \mathfrak{x}_1 - 60 \mathfrak{x}_2) - 60 \mathfrak{x}_2 + \mu_1^2 (-6 + 3 \mathfrak{x}_1 + 7 \mathfrak{x}_2) \right) \left. \right) \left. \right) + \\
& w^2 \left( - \left( (-1 + \eta t) \partial l \left( 44 \mu_1^2 - 15 \mu_2 - \mu_1 (64 + 15 \mu_2) \right) \right) + \right. \\
& \quad \partial p \left( -48 + 500 \mu_1 + 356 \mu_1^2 + 56 \mu_2 - 832 \mu_1 \mu_2 - \right. \\
& \quad \quad 2 \partial l \left( \mu_1 (78 + 62 \mathfrak{x}_1 + \mu_2 (-22 + 15 \mathfrak{x}_1 - 51 \mathfrak{x}_2) - 46 \mathfrak{x}_2) + \right. \\
& \quad \quad \quad (1 + \mu_2) \times (26 + 15 \mathfrak{x}_1 - 15 \mathfrak{x}_2) + \mu_1^2 (16 + 11 \mathfrak{x}_1 + 5 \mathfrak{x}_2) \left. \right) + \\
& \quad \quad \eta t \left( 192 + 556 \mu_1 - 440 \mu_1^2 + 149 \mu_2 - 331 \mu_1 \mu_2 + 2 \partial l \left( \mu_1 (78 + \right. \right. \\
& \quad \quad \quad 62 \mathfrak{x}_1 + \mu_2 (-22 + 15 \mathfrak{x}_1 - 51 \mathfrak{x}_2) - 46 \mathfrak{x}_2) + (1 + \mu_2) \times \\
& \quad \quad \quad \left. \left. (26 + 15 \mathfrak{x}_1 - 15 \mathfrak{x}_2) + \mu_1^2 (16 + 11 \mathfrak{x}_1 + 5 \mathfrak{x}_2) \right) \right) \left. \right) \left. \right) + \\
& \eta^3 \left( \partial p \left( -4 \times \left( 11 + 7 \mu_1^2 + \mu_1 (30 - 17 \mu_2) + 31 \mu_2 \right) + \eta t \left( 44 \mu_1^2 - \right. \right. \right. \\
& \quad \quad 11 \times (4 + \mu_2) - \mu_1 (72 + 11 \mu_2) \left. \right) - \\
& \quad 4 w^3 \left( -40 - 108 \mu_1 - 44 \mu_1^2 - 112 \mu_2 + 203 \mu_1 \mu_2 + \right. \\
& \quad \quad \eta t \left( -64 - 144 \mu_1 + 166 \mu_1^2 + 5 \mu_2 + 5 \mu_1 \mu_2 \right) \left. \right) - 2 w^4 \left( 21 - 8 \mu_1 - 29 \right. \\
& \quad \quad \mu_1^2 + 55 \mu_2 + 247 \mu_1 \mu_2 + \eta t \left( -44 - 94 \mu_1 + 250 \mu_1^2 + 30 \mu_1 \mu_2 \right) \left. \right) + \\
& \quad 4 w \left( -2 \times \left( -14 + 15 \mu_1 + 17 \mu_1^2 + \mu_2 - 59 \mu_1 \mu_2 \right) + \right. \\
& \quad \quad \eta t \left( -30 - 104 \mu_1 + 79 \mu_1^2 - 18 \mu_2 + 54 \mu_1 \mu_2 \right) \left. \right) + \\
& \quad 2 w^2 \left( 171 + 232 \mu_1 + \mu_1^2 + 337 \mu_2 + 7 \mu_1 \mu_2 + \eta t \right. \\
& \quad \quad \left. \left( 42 - 16 \mu_1 + 56 \mu_1^2 - 37 \mu_2 + 137 \mu_1 \mu_2 \right) \right) \left. \right) - (-1 + \eta t) \partial l \\
& \left( 20 + 56 \mu_1 + 4 w^4 \left( 5 + 29 \mu_1^2 - 5 \mu_1 (-2 + \mu_2) - 5 \mu_2 \right) + 5 \mu_2 - \right. \\
& \quad 19 \mu_1 \mu_2 + \partial p \left( \mu_1 (-14 + 85 \mathfrak{x}_1 + 2 \mu_2 (67 + 10 \mathfrak{x}_1 - 34 \mathfrak{x}_2) - 59 \mathfrak{x}_2) + \right. \\
& \quad \quad \mu_1^2 (10 + 17 \mathfrak{x}_1 + 9 \mathfrak{x}_2) + 2 \times (12 + \mu_2 + 10 \mathfrak{x}_1 + 10 \mu_2 \mathfrak{x}_1 - 10 \mathfrak{x}_2 - \\
& \quad \quad \quad 10 \mu_2 \mathfrak{x}_2) \left. \right) + 8 w^3 \left( 16 \mu_1^2 - 5 \times (1 + \mu_2) \times (1 + \partial p (\mathfrak{x}_1 - \mathfrak{x}_2)) + \right. \\
& \quad \quad \mu_1 (-16 + \mu_2 - 11 \partial p \mathfrak{x}_1 - 5 \partial p \mu_2 \mathfrak{x}_1 + 11 \partial p \mathfrak{x}_2 + 5 \partial p \mu_2 \mathfrak{x}_2) \left. \right) + \\
& \quad 2 w^2 \left( -3 \times \left( 6 \mu_1^2 + \mu_1 (36 - 19 \mu_2) + 5 \times (4 + \mu_2) \right) + \right. \\
& \quad \quad \partial p \left( - \left( (1 + \mu_2) \times (-52 + 45 \mathfrak{x}_1 - 45 \mathfrak{x}_2) \right) + \mu_1^2 (4 + 6 \mathfrak{x}_1 - 2 \mathfrak{x}_2) - \right. \\
& \quad \quad \quad \mu_1 (-104 + 69 \mathfrak{x}_1 - 73 \mathfrak{x}_2 + \mu_2 (116 + 45 \mathfrak{x}_1 + 3 \mathfrak{x}_2)) \left. \right) \left. \right) + \\
& \quad w \left( -48 \mu_1^2 - 10 \times (4 + \mu_2) + \mu_1 (8 + 62 \mu_2) + \partial p \left( 100 - 30 \mathfrak{x}_1 - \right. \right. \\
& \quad \quad 6 \mu_2 (-21 + 5 \mathfrak{x}_1 - 5 \mathfrak{x}_2) + 30 \mathfrak{x}_2 + \mu_1^2 (22 + 33 \mathfrak{x}_1 + 5 \mathfrak{x}_2) - \\
& \quad \quad \left. \mu_1 (-194 - 51 \mathfrak{x}_1 + 13 \mathfrak{x}_2 + 6 \mu_2 (21 + 5 \mathfrak{x}_1 + 23 \mathfrak{x}_2)) \right) \left. \right) \left. \right) +
\end{aligned}$$

$$\begin{aligned}
& \eta^5 \left( 4 \times (-1 + \eta t) \, \text{el} \, \mu_1 (1 + \mu_1) - 2 w^4 \left( (-1 + \eta t) \, \text{el} \left( 33 \mu_1^2 + 5 \mu_1 \right. \right. \right. \\
& \quad \left. \left. (-6 + \mu_2) + 5 \times (-3 + \mu_2) \right) + \text{ep} \left( -20 \times (4 + \mu_1^2 + \mu_1 (5 - 10 \mu_2) + \right. \right. \\
& \quad \left. \left. 11 \mu_2) + \eta t (153 \mu_1^2 + 5 \times (-7 + 4 \mu_2) - 20 \mu_1 (4 + 5 \mu_2)) \right) \right) + \\
& \text{ep} \left( 2 \times (5 + 15 \mu_1^2 + \mu_1 (44 - 13 \mu_2) + 53 \mu_2) + 4 \eta t (-4 + 4 \mu_1^2 + \right. \\
& \quad \left. 15 \mu_1 \mu_2) + \text{el} (-24 + 10 \mu_2 + 5 \mu_1 (14 - 10 \mu_2 + \mathfrak{e}_1 + \mathfrak{e}_2) + \right. \\
& \quad \left. \mu_1^2 (22 + 5 \mathfrak{e}_1 + 5 \mathfrak{e}_2)) - \eta t \, \text{el} (-24 + 10 \mu_2 + \right. \\
& \quad \left. 5 \mu_1 (14 - 10 \mu_2 + \mathfrak{e}_1 + \mathfrak{e}_2) + \mu_1^2 (22 + 5 \mathfrak{e}_1 + 5 \mathfrak{e}_2)) \right) - \\
& 2 w^3 \left( 2 \times (-1 + \eta t) \, \text{el} (\mu_1^2 - \mu_1 (-7 + \mu_2) + 5 \mu_2) + \text{ep} \right. \\
& \quad \left( -62 + 162 \mu_1^2 - 84 \mu_2 - 15 \, \text{el} \, \mathfrak{e}_1 - 15 \, \text{el} \, \mu_2 \mathfrak{e}_1 + \right. \\
& \quad \mu_1 (112 - 3 \mu_2 (64 + 5 \, \text{el} (\mathfrak{e}_1 - \mathfrak{e}_2)) - 33 \, \text{el} (\mathfrak{e}_1 - \mathfrak{e}_2)) + \\
& \quad 15 \, \text{el} \, \mathfrak{e}_2 + 15 \, \text{el} \, \mu_2 \mathfrak{e}_2 + \eta t (22 - 70 \mu_1^2 + 15 \, \text{el} \, \mathfrak{e}_1 + \\
& \quad 5 \mu_2 (11 + 3 \, \text{el} (\mathfrak{e}_1 - \mathfrak{e}_2)) + \mu_1 (126 + \mu_2 (-137 + \\
& \quad 15 \, \text{el} (\mathfrak{e}_1 - \mathfrak{e}_2)) + 33 \, \text{el} (\mathfrak{e}_1 - \mathfrak{e}_2)) - 15 \, \text{el} \, \mathfrak{e}_2) \left. \right) \left. \right) + \\
& w^2 \left( 3 \, \text{ep} (-4 \times (19 + 9 \mu_1^2 + \mu_1 (46 - 36 \mu_2) + 61 \mu_2) + \eta t \right. \\
& \quad \left. (-36 + 52 \mu_1^2 - 11 \mu_2 - \mu_1 (56 + 83 \mu_2)) \right) + \\
& (-1 + \eta t) \, \text{el} (4 \mu_1^2 - 15 \times (4 + \mu_2) + \mu_1 (-116 + 57 \mu_2) + \\
& \quad 2 \, \text{ep} (-2 \times (1 + \mu_2) \times (-19 + 15 \mathfrak{e}_1 - 15 \mathfrak{e}_2) + \mu_1^2 (4 + 5 \mathfrak{e}_1 - \mathfrak{e}_2) - \\
& \quad \mu_1 (-78 + 43 \mathfrak{e}_1 - 47 \mathfrak{e}_2 + \mu_2 (82 + 30 \mathfrak{e}_1 + 6 \mathfrak{e}_2)) \left. \right) \left. \right) + \\
& w (-4 \times (-1 + \eta t) \, \text{el} (-11 + \mu_1) \mu_1 + \text{ep} (4 \times (-21 + 61 \mu_1^2 + \\
& \quad \mu_1 (82 - 103 \mu_2) - 16 \mu_2) - \text{el} (60 + 78 \mu_2 + \mu_1^2 (26 + 29 \mathfrak{e}_1 + \\
& \quad 9 \mathfrak{e}_2) + \mu_1 (134 + 89 \mathfrak{e}_1 - 51 \mathfrak{e}_2 - 30 \mu_2 (1 + 4 \mathfrak{e}_2)) \left. \right) + \\
& \eta t (-4 \times (19 + 8 \mu_1^2 - 8 \mu_2 + 7 \mu_1 (-3 + 4 \mu_2)) + \\
& \quad \text{el} (60 + 78 \mu_2 + \mu_1^2 (26 + 29 \mathfrak{e}_1 + 9 \mathfrak{e}_2) + \\
& \quad \mu_1 (134 + 89 \mathfrak{e}_1 - 51 \mathfrak{e}_2 - 30 \mu_2 (1 + 4 \mathfrak{e}_2)) \left. \right) \left. \right) \left. \right) \left. \right) + \\
& \eta^6 (-4 \, \text{ep} (2 - 15 \mu_1^2 + 6 \eta t (1 + \mu_1) + \mu_1 (-31 + 30 \mu_2)) + \\
& w^4 ((-1 + \eta t) \, \text{el} (14 \mu_1^2 + 5 \mu_1 (-4 + \mu_2) + 5 \times (-2 + \mu_2)) + \\
& \quad 2 \, \text{ep} (-55 + 6 \mu_1 + 61 \mu_1^2 - 143 \mu_2 - 5 \mu_1 \mu_2 + \\
& \quad \eta t (-22 - 32 \mu_1 + 32 \mu_1^2 + 5 \mu_2 - 73 \mu_1 \mu_2)) \left. \right) + \\
& w^3 (\text{ep} (8 \times (8 + 17 \mu_1^2 + \mu_1 (40 - 44 \mu_2) + 46 \mu_2) + \eta t \\
& \quad (4 - 84 \mu_1^2 + 27 \mu_2 + \mu_1 (88 + 123 \mu_2)) \left. \right) - (-1 + \eta t) \, \text{el} \\
& \quad (4 \mu_1^2 + \mu_1 (-52 + \mu_2 (19 - 20 \, \text{ep} (\mathfrak{e}_1 - \mathfrak{e}_2)) - 44 \, \text{ep} (\mathfrak{e}_1 - \mathfrak{e}_2)) - \\
& \quad 5 \times (4 + \mu_2 + 4 \, \text{ep} (\mathfrak{e}_1 - \mathfrak{e}_2) + 4 \, \text{ep} \mu_2 (\mathfrak{e}_1 - \mathfrak{e}_2)) \left. \right) \left. \right) + \\
& w (-4 \times (-1 + \eta t) \, \text{el} \mu_1 (1 + \mu_1) + \text{ep} (16 - 2 \times (108 + 5 \, \text{el} \mu_2 + \\
& \quad \mu_1 (-124 + 96 \mu_2 + \text{el} (-94 + 50 \mu_2 - 5 \mathfrak{e}_1 - 5 \mathfrak{e}_2)) - \\
& \quad \mu_1^2 (44 + \text{el} (22 + 5 \mathfrak{e}_1 + 5 \mathfrak{e}_2)) + \\
& \quad \eta t (28 + 10 \, \text{el} \mu_2 + \mu_1^2 (-16 + \text{el} (22 + 5 \mathfrak{e}_1 + 5 \mathfrak{e}_2)) + \\
& \quad \mu_1 (12 - 120 \mu_2 + \text{el} (94 - 50 \mu_2 + 5 \mathfrak{e}_1 + 5 \mathfrak{e}_2)) \left. \right) \left. \right) \left. \right) + \\
& w^2 (4 \times (-1 + \eta t) \, \text{el} (-5 + \mu_1) \mu_1 + \text{ep} (42 - 380 \mu_1 - 302 \mu_1^2 + \\
& \quad 190 \mu_2 + 454 \mu_1 \mu_2 + 5 \, \text{el} (10 \times (1 + \mu_2) + \mu_1^2 (4 + 3 \mathfrak{e}_1 + \mathfrak{e}_2) + \\
& \quad \mu_1 (26 + 9 \mathfrak{e}_1 - 5 \mathfrak{e}_2 - 2 \mu_2 (7 + 6 \mathfrak{e}_2)) \left. \right) + \\
& \eta t (4 \times (21 + 8 \mu_1^2 - 4 \mu_2 + 5 \mu_1 (1 + 7 \mu_2)) - \\
& \quad 5 \, \text{el} (10 \times (1 + \mu_2) + \mu_1^2 (4 + 3 \mathfrak{e}_1 + \mathfrak{e}_2) + \\
& \quad \mu_1 (26 + 9 \mathfrak{e}_1 - 5 \mathfrak{e}_2 - 2 \mu_2 (7 + 6 \mathfrak{e}_2)) \left. \right) \left. \right) \left. \right) \left. \right) \left. \right) \left. \right) /
\end{aligned}$$

$$\begin{aligned}
& (96 (-1 + w (-1 + \eta))^3 (w (-1 + \eta) + x (-1 + \eta) - \eta)^2 (x + \eta - x \eta)^2 (1 + \\
& \quad x + \\
& \quad \eta - \\
& \quad x \\
& \quad \eta)^2 (-1 + \eta t) \operatorname{erf}(\eta p)) \\
\delta_{gs1} = & - \left( \left( c v c \sigma (x (-1 + \eta) - \eta) (-1 + \eta) (1 + x + \eta - x \eta)^2 \right. \right. \\
& \left( (x + \eta - x \eta)^4 (-1 + \eta t) \operatorname{erf}(\eta p) (2 x (-1 + \eta) \times (1 + \mu_1 - 32 \mu_2) - \right. \\
& \quad 2 \eta (1 + \mu_1 - 32 \mu_2) - (11 + 11 \mu_1 + 8 \mu_2) \times (2 + \mathfrak{e}_1 + \mathfrak{e}_2)) + \\
& w^5 (-1 + \eta)^5 (x^2 (-1 + \eta)^2 (4 \times (-1 + \eta) \operatorname{erf}(-7 \times (1 + \mu_1) + \eta (9 + 9 \mu_1 + 28 \mu_2) - \\
& \quad \eta t (9 + 9 \mu_1 + 28 \mu_2)) + (-1 + \eta t) \operatorname{erf}(-4 \times (3 + 3 \mu_1 - 8 \mu_2) + \operatorname{erf} \\
& \quad (64 + 17 \mathfrak{e}_1 + \mu_1 (64 + 17 \mathfrak{e}_1 - 3 \mathfrak{e}_2) - 3 \mathfrak{e}_2 - 8 \mu_2 (10 + 3 \mathfrak{e}_1 + 3 \mathfrak{e}_2))) + \\
& \eta \operatorname{erf} (4 \eta t (3 + 3 \mu_1 - 8 \mu_2) + 4 \eta^3 (9 + 9 \mu_1 + 28 \mu_2) - 4 \eta^2 \\
& \quad (4 \times (4 + 4 \mu_1 + 7 \mu_2) + \eta t (9 + 9 \mu_1 + 28 \mu_2)) + \eta \\
& \quad (28 \times (1 + \mu_1) + \operatorname{erf}(-64 - 17 \mathfrak{e}_1 + 3 \mathfrak{e}_2 + \mu_1 (-64 - 17 \mathfrak{e}_1 + 3 \mathfrak{e}_2) + \\
& \quad 8 \mu_2 (10 + 3 \mathfrak{e}_1 + 3 \mathfrak{e}_2)) + \eta t (24 \times (1 + \mu_1 + 6 \mu_2) + \operatorname{erf}(64 + 17 \mathfrak{e}_1 + \\
& \quad \mu_1 (64 + 17 \mathfrak{e}_1 - 3 \mathfrak{e}_2) - 3 \mathfrak{e}_2 - 8 \mu_2 (10 + 3 \mathfrak{e}_1 + 3 \mathfrak{e}_2))) \left. \right) - \\
& 2 x (-1 + \eta) \times (2 \eta t \operatorname{erf}(7 + 7 \mu_1 + 4 \mu_2) + 4 \eta^3 \operatorname{erf}(9 + 9 \mu_1 + 28 \mu_2) - \\
& 4 \eta^2 \operatorname{erf}(4 \times (4 + 4 \mu_1 + 7 \mu_2) + \eta t (9 + 9 \mu_1 + 28 \mu_2)) + \eta \\
& \quad (2 \operatorname{erf}(14 \times (1 + \mu_1) + \eta t (11 + 11 \mu_1 + 52 \mu_2)) + \\
& \quad (-1 + \eta t) \operatorname{erf}(2 \times (1 + \mu_1 + 20 \mu_2) + \operatorname{erf}(64 + 17 \mathfrak{e}_1 + \\
& \quad \mu_1 (64 + 17 \mathfrak{e}_1 - 3 \mathfrak{e}_2) - 3 \mathfrak{e}_2 - 8 \mu_2 (10 + 3 \mathfrak{e}_1 + 3 \mathfrak{e}_2)))) \left. \right) - \\
& w (x (-1 + \eta) - \eta) (-1 + \eta) \times (4 x^4 (-1 + \eta)^4 \operatorname{erf}(29 - 30 \operatorname{erf} + 29 \mu_1 - 30 \\
& \quad \operatorname{erf} \mu_1 + 72 \mu_2 - 40 \operatorname{erf} \mu_2 + 3 \eta^2 (9 + 9 \mu_1 + 28 \mu_2) - \eta (56 + 56 \mu_1 + 156 \mu_2 - \\
& \quad 2 \operatorname{erf}(9 + 9 \mu_1 + 28 \mu_2) + \eta t (1 + 2 \operatorname{erf}) \times (9 + 9 \mu_1 + 28 \mu_2)) + 4 \operatorname{erf} \\
& \quad \mu_2 \mathfrak{e}_1 + \eta t (9 + 9 \mu_1 + 28 \mu_2 + \operatorname{erf}(30 + 30 \mu_1 + 40 \mu_2 - 4 \mu_2 \mathfrak{e}_1))) \left. \right) - \\
& x^3 (-1 + \eta)^3 \operatorname{erf}(48 \eta^3 (9 + 9 \mu_1 + 28 \mu_2) - 16 \eta^2 (56 + 56 \mu_1 + 156 \mu_2 - \\
& \quad 2 \operatorname{erf}(9 + 9 \mu_1 + 28 \mu_2) + \eta t (1 + 2 \operatorname{erf}) \times (9 + 9 \mu_1 + 28 \mu_2)) + 16 \\
& \eta (29 + 29 \mu_1 + 72 \mu_2 - 2 \operatorname{erf}(15 + 15 \mu_1 + 20 \mu_2 - 2 \mu_2 \mathfrak{e}_1) + \\
& \quad \eta t (9 + 9 \mu_1 + 28 \mu_2 + \operatorname{erf}(30 + 30 \mu_1 + 40 \mu_2 - 4 \mu_2 \mathfrak{e}_1))) + 3 \times (-1 + \eta t) \\
& \quad \operatorname{erf}(24 + 11 \mathfrak{e}_1 + 11 \mathfrak{e}_2 + 8 \mu_2 (-6 + \mathfrak{e}_1 + \mathfrak{e}_2) + \mu_1 (24 + 11 \mathfrak{e}_1 + 11 \mathfrak{e}_2))) + \\
& \eta \operatorname{erf}(4 \eta t (7 + 7 \mu_1 + 4 \mu_2) + 12 \eta^5 (9 + 9 \mu_1 + 28 \mu_2) - 4 \eta^4 (56 + 56 \mu_1 + \\
& \quad 156 \mu_2 - 2 \operatorname{erf}(9 + 9 \mu_1 + 28 \mu_2) + \eta t (1 + 2 \operatorname{erf}) \times (9 + 9 \mu_1 + 28 \mu_2)) + 4 \\
& \eta^3 (29 + 29 \mu_1 + 72 \mu_2 - 2 \operatorname{erf}(15 + 15 \mu_1 + 20 \mu_2 - 2 \mu_2 \mathfrak{e}_1) + \\
& \quad \eta t (9 + 9 \mu_1 + 28 \mu_2 + \operatorname{erf}(30 + 30 \mu_1 + 40 \mu_2 - 4 \mu_2 \mathfrak{e}_1))) + 3 \eta^2 (-1 + \eta t) \\
& \quad \operatorname{erf}(24 + 11 \mathfrak{e}_1 + 11 \mathfrak{e}_2 + 8 \mu_2 (-6 + \mathfrak{e}_1 + \mathfrak{e}_2) + \mu_1 (24 + 11 \mathfrak{e}_1 + 11 \mathfrak{e}_2)) + 4 \\
& \eta (-\operatorname{erf}(18 + 9 \mathfrak{e}_1 + 4 \mathfrak{e}_2 + 2 \mu_2 (6 + 3 \mathfrak{e}_1 + \mathfrak{e}_2) + \mu_1 (18 + 9 \mathfrak{e}_1 + 4 \mathfrak{e}_2)) + \\
& \quad \eta t (-7 - 7 \mu_1 - 4 \mu_2 + \operatorname{erf}(18 + 9 \mathfrak{e}_1 + 4 \mathfrak{e}_2 + \\
& \quad 2 \mu_2 (6 + 3 \mathfrak{e}_1 + \mathfrak{e}_2) + \mu_1 (18 + 9 \mathfrak{e}_1 + 4 \mathfrak{e}_2)))) \left. \right) - \\
& x (-1 + \eta) \times (48 \eta^5 \operatorname{erf}(9 + 9 \mu_1 + 28 \mu_2) + 4 \eta t \operatorname{erf}(19 + 19 \mu_1 + 40 \mu_2) - \\
& 16 \eta^4 \operatorname{erf}(56 + 56 \mu_1 + 156 \mu_2 - 2 \operatorname{erf}(9 + 9 \mu_1 + 28 \mu_2) + \\
& \quad \eta t (1 + 2 \operatorname{erf}) \times (9 + 9 \mu_1 + 28 \mu_2)) + 16 \eta^3 \operatorname{erf} \\
& \quad (29 + 29 \mu_1 + 72 \mu_2 - 2 \operatorname{erf}(15 + 15 \mu_1 + 20 \mu_2 - 2 \mu_2 \mathfrak{e}_1) + \\
& \quad \eta t (9 + 9 \mu_1 + 28 \mu_2 + \operatorname{erf}(30 + 30 \mu_1 + 40 \mu_2 - 4 \mu_2 \mathfrak{e}_1))) + 9 \\
& \eta^2 (-1 + \eta t) \operatorname{erf}(\operatorname{erf}(24 + 11 \mathfrak{e}_1 + 11 \mathfrak{e}_2 + 8 \mu_2 (-6 + \mathfrak{e}_1 + \mathfrak{e}_2) + \\
& \quad \mu_1 (24 + 11 \mathfrak{e}_1 + 11 \mathfrak{e}_2)) + 4 \eta (-\eta t \operatorname{erf}(19 + 19 \mu_1 + 40 \mu_2) +
\end{aligned}$$

$$\begin{aligned}
& (-1 + \eta t) \, \theta l \, (-3 - 3 \mu 1 + 8 \mu 2 + 2 \, \theta p \, (22 + 11 \, \theta 1 + 6 \, \theta 2 + \\
& \quad 4 \mu 2 \, (6 + 3 \, \theta 1 + 2 \, \theta 2) + \mu 1 \, (22 + 11 \, \theta 1 + 6 \, \theta 2))) + \\
& x^2 \, (-1 + \eta)^2 \, (24 \times (-1 + \eta) \, \eta^2 \, \theta p \, (-29 - 29 \mu 1 - 72 \mu 2 + 3 \, \eta \\
& \quad (9 + 9 \mu 1 + 28 \mu 2) - \eta t \, (9 + 9 \mu 1 + 28 \mu 2)) - (-1 + \eta t) \\
& \quad \theta l \, (60 + 60 \mu 1 + 112 \mu 2 + \theta p \, (48 \eta^3 \, (9 + 9 \mu 1 + 28 \mu 2) - \\
& \quad 48 \eta^2 \, (15 + 15 \mu 1 - 2 \mu 2 \, (-10 + \theta 1)) - 4 \times (26 + 13 \, \theta 1 + 8 \, \theta 2 + \\
& \quad 2 \mu 2 \, (18 + 9 \, \theta 1 + 7 \, \theta 2) + \mu 1 \, (26 + 13 \, \theta 1 + 8 \, \theta 2)) - 9 \, \eta \, (24 + 11 \\
& \quad \theta 1 + 11 \, \theta 2 + 8 \mu 2 \, (-6 + \theta 1 + \theta 2) + \mu 1 \, (24 + 11 \, \theta 1 + 11 \, \theta 2))) + \\
& w^2 \, (-1 + \eta)^2 \, (2 \, x^5 \, (-1 + \eta)^5 \, \theta p \, (14 - 15 \, \theta l + 14 \mu 1 - 15 \, \theta l \, \mu 1 + 32 \, \theta l \, \mu 2 + \\
& \quad 2 \eta^2 \, (9 + 9 \mu 1 + 28 \mu 2) + 2 \, \eta t \, (9 + 9 \mu 1 + 28 \mu 2) - 2 \, \eta \, (4 \times (4 + 4 \mu 1 + 7 \mu 2) + \\
& \quad \eta t \, (9 + 9 \mu 1 + 28 \mu 2)) + 8 \, \theta l \, \mu 2 \, \theta 1 + \eta t \, \theta l \, (15 + 15 \mu 1 - 8 \mu 2 \, (4 + \theta 1))) - \\
& x^4 \, (-1 + \eta)^4 \, \theta p \, (20 \eta^3 \, (9 + 9 \mu 1 + 28 \mu 2) - 4 \eta^2 \, (-1 - \mu 1 - 112 \mu 2 + \\
& \quad 5 \, \eta t \, (9 + 9 \mu 1 + 28 \mu 2)) + \eta \, (8 \, \eta t \, (9 + 9 \mu 1 + 28 \mu 2) - \\
& \quad 4 \times (133 + 133 \mu 1 + 468 \mu 2) - 2 \, \eta t \, \theta l \, (33 + 33 \mu 1 + 8 \mu 2 \, (62 + 5 \, \theta 1)) + \\
& \quad \theta l \, (66 + 66 \mu 1 + 16 \mu 2 \, (62 + 5 \, \theta 1))) + 3 \times (4 \times (29 + 29 \mu 1 + 72 \mu 2) - \theta l \\
& \quad (142 + 11 \, \theta 1 - 8 \mu 2 \, (-22 + \theta 1 - \theta 2) + 11 \, \theta 2 + \mu 1 \, (142 + 11 \, \theta 1 + 11 \, \theta 2)) + \\
& \quad \eta t \, (4 \times (9 + 9 \mu 1 + 28 \mu 2) + \theta l \, (142 + 11 \, \theta 1 - 8 \mu 2 \, (-22 + \theta 1 - \theta 2) + \\
& \quad 11 \, \theta 2 + \mu 1 \, (142 + 11 \, \theta 1 + 11 \, \theta 2)))) - \\
& \eta \, \theta p \, (4 \, \eta t \, (3 + 3 \mu 1 - 8 \mu 2) + 4 \eta^6 \, (9 + 9 \mu 1 + 28 \mu 2) - 4 \eta^5 \\
& \quad (-65 - 65 \mu 1 - 224 \mu 2 + \eta t \, (9 + 9 \mu 1 + 28 \mu 2)) - 2 \\
& \quad \eta^4 \, (322 + 322 \mu 1 + 936 \mu 2 + 4 \, \eta t \, (9 + 9 \mu 1 + 28 \mu 2) - \\
& \quad \theta l \, (93 + 93 \mu 1 + 8 \mu 2 \, (46 + \theta 1)) + \eta t \, \theta l \, (93 + 93 \mu 1 + 8 \mu 2 \, (46 + \theta 1))) + \\
& \eta \, (\theta l \, (-34 - 17 \, \theta 1 + 3 \, \theta 2 + \mu 1 \, (-34 - 17 \, \theta 1 + 3 \, \theta 2) + 8 \mu 2 \, (2 + \theta 1 + 3 \, \theta 2)) + \\
& \quad \eta t \, (8 \times (9 + 9 \mu 1 + 10 \mu 2) + \theta l \, (34 + 17 \, \theta 1 + \mu 1 \, (34 + 17 \, \theta 1 - 3 \, \theta 2) - \\
& \quad 3 \, \theta 2 - 8 \mu 2 \, (2 + \theta 1 + 3 \, \theta 2)))) + 6 \eta^2 \\
& \quad (-\theta l \, (37 + 18 \, \theta 1 + 8 \, \theta 2 + 4 \mu 2 \, (-2 + 3 \, \theta 1 + \theta 2) + \mu 1 \, (37 + 18 \, \theta 1 + 8 \, \theta 2)) + \\
& \quad \eta t \, (-2 \times (7 + 7 \mu 1 + 4 \mu 2) + \theta l \, (37 + 18 \, \theta 1 + 8 \, \theta 2 + 4 \mu 2 \, (-2 + 3 \, \theta 1 + \theta 2) + \\
& \quad \mu 1 \, (37 + 18 \, \theta 1 + 8 \, \theta 2)))) + 3 \eta^3 \, (4 \times (29 + 29 \mu 1 + 72 \mu 2) - \theta l \\
& \quad (142 + 11 \, \theta 1 - 8 \mu 2 \, (-22 + \theta 1 - \theta 2) + 11 \, \theta 2 + \mu 1 \, (142 + 11 \, \theta 1 + 11 \, \theta 2)) + \\
& \quad \eta t \, (4 \times (9 + 9 \mu 1 + 28 \mu 2) + \theta l \, (142 + 11 \, \theta 1 - 8 \mu 2 \, (-22 + \theta 1 - \theta 2) + \\
& \quad 11 \, \theta 2 + \mu 1 \, (142 + 11 \, \theta 1 + 11 \, \theta 2)))) + \\
& 2 \, x^3 \, (-1 + \eta)^3 \, (4 \times (-1 + \eta) \, \eta \, \theta p \, (5 \eta^2 \, (9 + 9 \mu 1 + 28 \mu 2) + \eta \\
& \quad (127 + 127 \mu 1 + 504 \mu 2 - 5 \, \eta t \, (9 + 9 \mu 1 + 28 \mu 2)) - \\
& \quad 6 \times (29 + 29 \mu 1 + 72 \mu 2 + \eta t \, (9 + 9 \mu 1 + 28 \mu 2))) - (-1 + \eta t) \, \theta l \\
& \quad (90 + 90 \mu 1 + 168 \mu 2 + \theta p \, (2 \eta^2 \, (141 + 141 \mu 1 + 8 \mu 2 \, (104 + 5 \, \theta 1)) - \\
& \quad 6 \, \eta \, (142 + 11 \, \theta 1 - 8 \mu 2 \, (-22 + \theta 1 - \theta 2) + 11 \, \theta 2 + \\
& \quad \mu 1 \, (142 + 11 \, \theta 1 + 11 \, \theta 2)) - 3 \times (53 + 26 \, \theta 1 + 16 \, \theta 2 + \\
& \quad 4 \mu 2 \, (10 + 9 \, \theta 1 + 7 \, \theta 2) + \mu 1 \, (53 + 26 \, \theta 1 + 16 \, \theta 2))) + \\
& 2 \times (-1 + \eta) \times (2 \, \eta t \, \theta p \, (7 + 7 \mu 1 + 4 \mu 2) + 10 \eta^6 \, \theta p \, (9 + 9 \mu 1 + 28 \mu 2) + \\
& 2 \eta^5 \, \theta p \, (-5 \, \eta t \, (9 + 9 \mu 1 + 28 \mu 2) + 4 \times (61 + 61 \mu 1 + 217 \mu 2)) - \eta^4 \\
& \quad \theta p \, (14 \, \eta t \, (9 + 9 \mu 1 + 28 \mu 2) + 26 \times (49 + 49 \mu 1 + 144 \mu 2) - \\
& \quad \theta l \, (357 + 357 \mu 1 + 8 \mu 2 \, (188 + 5 \, \theta 1)) + \eta t \, \theta l \\
& \quad (357 + 357 \mu 1 + 8 \mu 2 \, (188 + 5 \, \theta 1))) + \eta \, (2 \, \eta t \, \theta p \, (71 + 71 \mu 1 + 128 \mu 2) + \\
& \quad (-1 + \eta t) \, \theta l \, (2 \times (1 + \mu 1 + 20 \mu 2) + \theta p \, (34 + 17 \, \theta 1 + \\
& \quad \mu 1 \, (34 + 17 \, \theta 1 - 3 \, \theta 2) - 3 \, \theta 2 - 8 \mu 2 \, (2 + \theta 1 + 3 \, \theta 2)))) + 6 \eta^3 \, \theta p
\end{aligned}$$

$$\begin{aligned}
& (4 \times (29 + 29 \mu_1 + 72 \mu_2) - \theta l (142 + 11 \mathfrak{z}_1 - 8 \mu_2 (-22 + \mathfrak{z}_1 - \mathfrak{z}_2) + \\
& \quad 11 \mathfrak{z}_2 + \mu_1 (142 + 11 \mathfrak{z}_1 + 11 \mathfrak{z}_2)) + \eta t (4 \times (9 + 9 \mu_1 + 28 \mu_2) + \\
& \quad \theta l (142 + 11 \mathfrak{z}_1 - 8 \mu_2 (-22 + \mathfrak{z}_1 - \mathfrak{z}_2) + 11 \mathfrak{z}_2 + \mu_1 \\
& \quad (142 + 11 \mathfrak{z}_1 + 11 \mathfrak{z}_2))) + 3 \eta^2 (-4 \eta t \theta p (13 + 13 \mu_1 + 22 \mu_2) + \\
& \quad (-1 + \eta t) \theta l (-6 - 6 \mu_1 + 16 \mu_2 + \theta p (127 + 62 \mathfrak{z}_1 + 32 \mathfrak{z}_2 + \\
& \quad 12 \mu_2 (2 + 5 \mathfrak{z}_1 + 3 \mathfrak{z}_2) + \mu_1 (127 + 62 \mathfrak{z}_1 + 32 \mathfrak{z}_2)))) - \\
& x^2 (-1 + \eta)^2 (4 \times (-1 + \eta) \theta p (10 \eta^4 (9 + 9 \mu_1 + 28 \mu_2) - 3 \eta t (19 + \\
& \quad 19 \mu_1 + 40 \mu_2) - 18 \eta^2 (29 + 29 \mu_1 + 72 \mu_2 + \eta t (9 + 9 \mu_1 + 28 \mu_2)) + \\
& \quad \eta^3 (-10 \eta t (9 + 9 \mu_1 + 28 \mu_2) + 8 \times (52 + 52 \mu_1 + 189 \mu_2))) - (-1 + \eta t) \\
& \quad \theta l (4 \times (3 + 3 \mu_1 - 8 \mu_2) + 4 \eta^3 \theta p (249 + 249 \mu_1 + 8 \mu_2 (146 + 5 \mathfrak{z}_1)) + \\
& \quad \theta p (-34 - 17 \mathfrak{z}_1 + 3 \mathfrak{z}_2 + \mu_1 (-34 - 17 \mathfrak{z}_1 + 3 \mathfrak{z}_2) + 8 \mu_2 (2 + \mathfrak{z}_1 + 3 \mathfrak{z}_2)) - \\
& \quad 18 \eta^2 \theta p (142 + 11 \mathfrak{z}_1 - 8 \mu_2 (-22 + \mathfrak{z}_1 - \mathfrak{z}_2) + 11 \mathfrak{z}_2 + \mu_1 (142 + 11 \mathfrak{z}_1 + \\
& \quad 11 \mathfrak{z}_2)) - 6 \eta (-4 \times (9 + 9 \mu_1 + 10 \mu_2) + \theta p (143 + 70 \mathfrak{z}_1 + 40 \mathfrak{z}_2 + \\
& \quad 12 \mu_2 (6 + 7 \mathfrak{z}_1 + 5 \mathfrak{z}_2) + \mu_1 (143 + 70 \mathfrak{z}_1 + 40 \mathfrak{z}_2)))) + \\
& w^4 (-1 + \eta)^4 (2 x^3 (-1 + \eta)^3 (6 \times (-1 + \eta) \theta p (-7 \times (1 + \mu_1) + \eta \\
& \quad (9 + 9 \mu_1 + 28 \mu_2) - \eta t (9 + 9 \mu_1 + 28 \mu_2)) + (-1 + \eta t) \\
& \quad \theta l (-2 \times (15 + 15 \mu_1 + 28 \mu_2) + \theta p (97 + 26 \mathfrak{z}_1 + 16 \mathfrak{z}_2 + \\
& \quad 4 \mu_2 (-6 + 3 \mathfrak{z}_1 + 7 \mathfrak{z}_2) + \mu_1 (97 + 26 \mathfrak{z}_1 + 16 \mathfrak{z}_2)))) - \\
& \eta \theta p (12 \eta t (3 + 3 \mu_1 - 8 \mu_2) + 12 \eta^4 (9 + 9 \mu_1 + 28 \mu_2) - 12 \eta^3 \\
& \quad (7 \times (1 + \mu_1) + \eta t (9 + 9 \mu_1 + 28 \mu_2)) + 2 \eta^2 (-2 \times (35 + 35 \mu_1 + 156 \mu_2) - \\
& \quad \theta l (45 + 18 \mathfrak{z}_1 - 4 \mu_2 (46 + 3 \mathfrak{z}_1 - \mathfrak{z}_2) + 8 \mathfrak{z}_2 + \mu_1 (45 + 18 \mathfrak{z}_1 + 8 \mathfrak{z}_2)) + \\
& \quad \eta t (22 + 22 \mu_1 + 104 \mu_2 + \theta l (45 + 18 \mathfrak{z}_1 - 4 \mu_2 (46 + 3 \mathfrak{z}_1 - \mathfrak{z}_2) + 8 \mathfrak{z}_2 + \\
& \quad \mu_1 (45 + 18 \mathfrak{z}_1 + 8 \mathfrak{z}_2)))) + \eta (4 \times (29 + 29 \mu_1 + 72 \mu_2) + \\
& \quad \theta l (-222 - 51 \mathfrak{z}_1 - 3 \mu_1 (74 + 17 \mathfrak{z}_1 - 3 \mathfrak{z}_2) + 9 \mathfrak{z}_2 + 8 \mu_2 \\
& \quad (-14 + 5 \mathfrak{z}_1 + 9 \mathfrak{z}_2)) + \eta t (28 \times (1 + \mu_1 + 8 \mu_2) + \theta l (222 + 51 \mathfrak{z}_1 + \\
& \quad 3 \mu_1 (74 + 17 \mathfrak{z}_1 - 3 \mathfrak{z}_2) - 9 \mathfrak{z}_2 - 8 \mu_2 (-14 + 5 \mathfrak{z}_1 + 9 \mathfrak{z}_2)))) + \\
& 2 \times (-1 + \eta) \times (6 \eta t \theta p (7 + 7 \mu_1 + 4 \mu_2) + 18 \eta^4 \theta p (9 + 9 \mu_1 + 28 \mu_2) - \\
& \quad 6 \eta^3 \theta p (30 + 30 \mu_1 + 28 \mu_2 + 3 \eta t (9 + 9 \mu_1 + 28 \mu_2)) + \eta \\
& \quad (2 \theta p (58 + 58 \mu_1 + 144 \mu_2 + \eta t (23 + 23 \mu_1 + 88 \mu_2)) + \\
& \quad (-1 + \eta t) \theta l (6 \times (1 + \mu_1 + 20 \mu_2) + \theta p (222 + 51 \mathfrak{z}_1 + \\
& \quad 3 \mu_1 (74 + 17 \mathfrak{z}_1 - 3 \mathfrak{z}_2) - 9 \mathfrak{z}_2 - 8 \mu_2 (-14 + 5 \mathfrak{z}_1 + 9 \mathfrak{z}_2)))) + \\
& \eta^2 (2 \theta p (-49 - 49 \mu_1 - 312 \mu_2 + \eta t (37 + 37 \mu_1 + 152 \mu_2)) + \\
& \quad (-1 + \eta t) \theta l (-6 - 6 \mu_1 + 16 \mu_2 + \theta p (187 + 62 \mathfrak{z}_1 - \\
& \quad 4 \mu_2 (98 + 3 \mathfrak{z}_1 - 9 \mathfrak{z}_2) + 32 \mathfrak{z}_2 + \mu_1 (187 + 62 \mathfrak{z}_1 + 32 \mathfrak{z}_2)))) - \\
& x^2 (-1 + \eta)^2 (4 \times (-1 + \eta) \theta p (-29 - 29 \mu_1 - 72 \mu_2 - 4 \eta t (7 + 7 \mu_1 + \\
& \quad 17 \mu_2) + 9 \eta^2 (9 + 9 \mu_1 + 28 \mu_2) - \\
& \quad 3 \eta (4 \times (3 + 3 \mu_1 - 7 \mu_2) + 3 \eta t (9 + 9 \mu_1 + 28 \mu_2))) + \\
& \quad (-1 + \eta t) \theta l (-12 \times (3 + 3 \mu_1 - 8 \mu_2) + \theta p (222 + 51 \mathfrak{z}_1 + \\
& \quad 3 \mu_1 (74 + 17 \mathfrak{z}_1 - 3 \mathfrak{z}_2) - 9 \mathfrak{z}_2 - 8 \mu_2 (-14 + 5 \mathfrak{z}_1 + 9 \mathfrak{z}_2)) + \\
& \quad 2 \eta (-4 \times (9 + 9 \mu_1 + 10 \mu_2) + \theta p (239 + 70 \mathfrak{z}_1 + 40 \mathfrak{z}_2 + \\
& \quad 4 \mu_2 (-58 + 3 \mathfrak{z}_1 + 15 \mathfrak{z}_2) + \mu_1 (239 + 70 \mathfrak{z}_1 + 40 \mathfrak{z}_2)))) + \\
& w^3 (-1 + \eta)^3 (x^4 (-1 + \eta)^4 \theta p (84 - 112 \theta l + 84 \mu_1 - 112 \theta l \mu_1 + 176 \theta l \\
& \quad \mu_2 + 12 \eta^2 (9 + 9 \mu_1 + 28 \mu_2) + 12 \eta t (9 + 9 \mu_1 + 28 \mu_2) - 12 \eta \\
& \quad (4 \times (4 + 4 \mu_1 + 7 \mu_2) + \eta t (9 + 9 \mu_1 + 28 \mu_2)) - 11 \theta l \mathfrak{z}_1 - 11 \theta l \\
& \quad \mu_1 \mathfrak{z}_1 + 40 \theta l \mu_2 \mathfrak{z}_1 - 11 \theta l \mathfrak{z}_2 - 11 \theta l \mu_1 \mathfrak{z}_2 - 8 \theta l \mu_2 \mathfrak{z}_2 + \eta t \theta l
\end{aligned}$$

$$\begin{aligned}
& \left( (112 + 11 \, \mathfrak{e}1 - 8 \, \mu2 \, (22 + 5 \, \mathfrak{e}1 - \mathfrak{e}2) + 11 \, \mathfrak{e}2 + \mu1 \, (112 + 11 \, \mathfrak{e}1 + 11 \, \mathfrak{e}2)) \right) - \\
& 4 \, x^3 \, (-1 + \eta)^3 \left( 3 \times (-1 + \eta) \, \text{op} \left( -29 - 29 \, \mu1 - 72 \, \mu2 + 4 \, \eta^2 \, (9 + 9 \, \mu1 + 28 \, \mu2) - \right. \right. \\
& \quad \left. \left. \eta \mathfrak{t} \, (9 + 9 \, \mu1 + 28 \, \mu2) - \eta \, (1 + \mu1 - 84 \, \mu2 + 4 \, \eta \mathfrak{t} \, (9 + 9 \, \mu1 + 28 \, \mu2)) \right) + \right. \\
& \quad \left. (-1 + \eta \mathfrak{t}) \, \text{el} \left( -3 \times (15 + 15 \, \mu1 + 28 \, \mu2) + 3 \, \text{op} \, (56 + 13 \, \mathfrak{e}1 + \right. \right. \\
& \quad \left. \left. 13 \, \mu1 \, \mathfrak{e}1 + 8 \, \mathfrak{e}2 + 8 \, \mu1 \, (7 + \mathfrak{e}2) + 2 \, \mu2 \, (38 + 7 \, \mathfrak{e}1 + 7 \, \mathfrak{e}2)) + \eta \, \text{op} \right. \right. \\
& \quad \left. \left. (58 + 11 \, \mathfrak{e}1 - 8 \, \mu2 \, (43 + 5 \, \mathfrak{e}1 - \mathfrak{e}2) + 11 \, \mathfrak{e}2 + \mu1 \, (58 + 11 \, \mathfrak{e}1 + 11 \, \mathfrak{e}2)) \right) \right) + \\
& \eta \, \text{op} \left( 12 \, \eta \mathfrak{t} \, (3 + 3 \, \mu1 - 8 \, \mu2) + 12 \, \eta^5 \, (9 + 9 \, \mu1 + 28 \, \mu2) - 12 \, \eta^4 \right. \\
& \quad \left. (-11 - 11 \, \mu1 - 56 \, \mu2 + \eta \mathfrak{t} \, (9 + 9 \, \mu1 + 28 \, \mu2)) + \eta^3 \right. \\
& \quad \left. (-12 \times (49 + 49 \, \mu1 + 156 \, \mu2) + (-1 + \eta \mathfrak{t}) \, \text{el} \, (-104 + 11 \, \mathfrak{e}1 - \right. \\
& \quad \left. 8 \, \mu2 \, (106 + 5 \, \mathfrak{e}1 - \mathfrak{e}2) + 11 \, \mathfrak{e}2 + \mu1 \, (-104 + 11 \, \mathfrak{e}1 + 11 \, \mathfrak{e}2)) \right) + 12 \, \eta^2 \\
& \quad \left. (29 + 29 \, \mu1 + 72 \, \mu2 - \text{el} \, (48 + 9 \, \mathfrak{e}1 + 4 \, \mathfrak{e}2 + 2 \, \mu2 \, (26 + \mathfrak{e}1 + \mathfrak{e}2) + \right. \\
& \quad \left. \mu1 \, (48 + 9 \, \mathfrak{e}1 + 4 \, \mathfrak{e}2)) + \eta \mathfrak{t} \, (2 \times (1 + \mu1 + 12 \, \mu2) + \right. \\
& \quad \left. \text{el} \, (48 + 9 \, \mathfrak{e}1 + 4 \, \mathfrak{e}2 + 2 \, \mu2 \, (26 + \mathfrak{e}1 + \mathfrak{e}2) + \mu1 \, (48 + 9 \, \mathfrak{e}1 + 4 \, \mathfrak{e}2))) \right) + \\
& \eta \, (\text{el} \, (-104 - 51 \, \mathfrak{e}1 + 9 \, \mathfrak{e}2 + \mu1 \, (-104 - 51 \, \mathfrak{e}1 + 9 \, \mathfrak{e}2) + 8 \, \mu2 \\
& \quad (14 + 3 \, \mathfrak{e}1 + 9 \, \mathfrak{e}2)) + \eta \mathfrak{t} \, (48 \times (1 + \mu1 + 3 \, \mu2) + \text{el} \, (104 + 51 \, \mathfrak{e}1 + \\
& \quad \mu1 \, (104 + 51 \, \mathfrak{e}1 - 9 \, \mathfrak{e}2) - 9 \, \mathfrak{e}2 - 8 \, \mu2 \, (14 + 3 \, \mathfrak{e}1 + 9 \, \mathfrak{e}2))) \right) - \\
& 2 \times (-1 + \eta) \times \left( 6 \, \eta \mathfrak{t} \, \text{op} \, (7 + 7 \, \mu1 + 4 \, \mu2) + 24 \, \eta^5 \, \text{op} \, (9 + 9 \, \mu1 + 28 \, \mu2) - \right. \\
& \quad 6 \, \eta^4 \, \text{op} \, (-17 - 17 \, \mu1 - 140 \, \mu2 + 4 \, \eta \mathfrak{t} \, (9 + 9 \, \mu1 + 28 \, \mu2)) + \eta \\
& \quad \left. (6 \, \eta \mathfrak{t} \, \text{op} \, (19 + 19 \, \mu1 + 40 \, \mu2) + (-1 + \eta \mathfrak{t}) \, \text{el} \, (6 \times (1 + \mu1 + 20 \, \mu2) + \right. \\
& \quad \left. \text{op} \, (104 + 51 \, \mathfrak{e}1 + \mu1 \, (104 + 51 \, \mathfrak{e}1 - 9 \, \mathfrak{e}2) - 9 \, \mathfrak{e}2 - 8 \, \mu2 \right. \\
& \quad \left. (14 + 3 \, \mathfrak{e}1 + 9 \, \mathfrak{e}2))) \right) + 2 \, \eta^3 \, \text{op} \, (-12 \times (35 + 35 \, \mu1 + 117 \, \mu2) + \\
& \quad \text{el} \, (50 - 11 \, \mathfrak{e}1 + \mu1 \, (50 - 11 \, \mathfrak{e}1 - 11 \, \mathfrak{e}2) + 8 \, \mu2 \, (85 + 5 \, \mathfrak{e}1 - \mathfrak{e}2) - \\
& \quad 11 \, \mathfrak{e}2) + \eta \mathfrak{t} \, (3 \times (9 + 9 \, \mu1 + 28 \, \mu2) + \text{el} \, (-50 + 11 \, \mathfrak{e}1 - \\
& \quad 8 \, \mu2 \, (85 + 5 \, \mathfrak{e}1 - \mathfrak{e}2) + 11 \, \mathfrak{e}2 + \mu1 \, (-50 + 11 \, \mathfrak{e}1 + 11 \, \mathfrak{e}2))) \right) + 6 \\
& \quad \eta^2 \, (\text{op} \, (87 + 87 \, \mu1 + 216 \, \mu2 + \eta \mathfrak{t} \, (1 + \mu1 + 40 \, \mu2)) + (-1 + \eta \mathfrak{t}) \\
& \quad \left. \text{el} \, (-3 - 3 \, \mu1 + 8 \, \mu2 + \text{op} \, (152 + 31 \, \mathfrak{e}1 + 16 \, \mathfrak{e}2 + 18 \, \mu2 \, (10 + \mathfrak{e}1 + \mathfrak{e}2) + \right. \\
& \quad \left. \mu1 \, (152 + 31 \, \mathfrak{e}1 + 16 \, \mathfrak{e}2))) \right) + x^2 \, (-1 + \eta)^2 \\
& \left( 12 \times (-1 + \eta) \, \text{op} \left( 6 \, \eta^3 \, (9 + 9 \, \mu1 + 28 \, \mu2) - \eta \mathfrak{t} \, (19 + 19 \, \mu1 + 40 \, \mu2) - \right. \right. \\
& \quad \left. \left. 3 \, \eta \, (29 + 29 \, \mu1 + 72 \, \mu2 + \eta \mathfrak{t} \, (9 + 9 \, \mu1 + 28 \, \mu2)) - \right. \right. \\
& \quad \left. \left. 3 \, \eta^2 \, (-13 - 13 \, \mu1 - 84 \, \mu2 + 2 \, \eta \mathfrak{t} \, (9 + 9 \, \mu1 + 28 \, \mu2)) \right) + \right. \\
& \quad \left. (-1 + \eta \mathfrak{t}) \, \text{el} \left( -12 \times (3 + 3 \, \mu1 - 8 \, \mu2) + \text{op} \, (104 + 51 \, \mathfrak{e}1 + \right. \right. \\
& \quad \left. \left. \mu1 \, (104 + 51 \, \mathfrak{e}1 - 9 \, \mathfrak{e}2) - 9 \, \mathfrak{e}2 - 8 \, \mu2 \, (14 + 3 \, \mathfrak{e}1 + 9 \, \mathfrak{e}2)) + 6 \, \eta^2 \, \text{op} \right. \right. \\
& \quad \left. \left. (4 + 11 \, \mathfrak{e}1 - 8 \, \mu2 \, (64 + 5 \, \mathfrak{e}1 - \mathfrak{e}2) + 11 \, \mathfrak{e}2 + \mu1 \, (4 + 11 \, \mathfrak{e}1 + 11 \, \mathfrak{e}2)) + \right. \right. \\
& \quad \left. \left. 12 \, \eta \, (-2 \times (9 + 9 \, \mu1 + 10 \, \mu2) + \text{op} \, (5 \times (32 + 7 \, \mathfrak{e}1 + 4 \, \mathfrak{e}2) + \right. \right. \\
& \quad \left. \left. 6 \, \mu2 \, (34 + 5 \, \mathfrak{e}1 + 5 \, \mathfrak{e}2) + 5 \, \mu1 \, (7 \, \mathfrak{e}1 + 4 \times (8 + \mathfrak{e}2))) \right) \right) \right) + \\
& 2 \times (-1 + w \, (-1 + \eta)) \, (w + x + \eta - w \, \eta - x \, \eta)^2 \left( x^2 \, (-1 + \eta)^2 + \eta \, (1 + \eta) + \right. \\
& \quad \left. x \, (1 + \eta - 2 \, \eta^2) \right)^2 \\
& \text{el} \left( -8 \, (x \, (-1 + \eta) - \eta) \, (w \, (-1 + \eta) + x \, (-1 + \eta) - \eta) \right. \\
& \quad \left. (1 + w - w \, \eta)^2 \right. \\
& \quad \left. (-1 + \eta \mathfrak{t}) \, \text{op} \right. \\
& \quad \left. (-6 \, ux + u \, (6 + 7 \, \mathfrak{e}1 + 3 \, \mathfrak{e}2)) + f \right. \\
& \quad \left. (-1 + \eta) \right. \\
& \quad \left. (x^2 \, (-1 + \eta)^2 \, \text{op} \left( -20 + 28 \, \eta - 8 \, \eta^2 - 4 \, \eta \mathfrak{t} + 4 \, \eta \, \eta \mathfrak{t} + 20 \, \text{el} - 4 \, \eta \right. \right. \\
& \quad \left. \left. \text{el} - 20 \, \eta \mathfrak{t} \, \text{el} + 4 \, \eta \, \eta \mathfrak{t} \, \text{el} - 24 \, \mathfrak{e}1 + 24 \, \eta \, \mathfrak{e}1 + 24 \, \text{el} \, \mathfrak{e}1 - 24 \, \eta \mathfrak{t} \right. \right. \\
& \quad \left. \left. \text{el} \, \mathfrak{e}1 - 10 \, \mathfrak{e}2 + 14 \, \eta \, \mathfrak{e}2 - 4 \, \eta^2 \, \mathfrak{e}2 - 2 \, \eta \mathfrak{t} \, \mathfrak{e}2 + 2 \, \eta \, \eta \mathfrak{t} \, \mathfrak{e}2 + 16 \right. \right.
\end{aligned}$$



$$\begin{aligned}
& \theta l \, \mathfrak{x}2 - 2 \, \eta \, \theta l \, \mathfrak{x}2 - 16 \, \eta t \, \theta l \, \mathfrak{x}2 + 2 \, \eta \, \eta t \, \theta l \, \mathfrak{x}2 + 3 \, \theta l \, \mathfrak{x}2^2 - 3 \\
& \eta t \, \theta l \, \mathfrak{x}2^2 + w \, (-1 + \eta) \times (2 \, \eta^2 \, (2 + \mathfrak{x}2) + 6 \times (2 + 4 \, \mathfrak{x}1 + \mathfrak{x}2) - \\
& 3 \, \theta l \, (8 \, \mathfrak{x}1 + (2 + \mathfrak{x}2)^2) - 2 \, \eta \, (\eta t \, (2 + \mathfrak{x}2) + 4 \times (2 + 3 \, \mathfrak{x}1 + \mathfrak{x}2)) + \\
& \eta t \, (2 \times (2 + \mathfrak{x}2) + 3 \, \theta l \, (8 \, \mathfrak{x}1 + (2 + \mathfrak{x}2)^2))) + x \, (-1 + \eta) \times \\
& (2 \, (w \, (-1 + \eta) - 2 \, \eta) \, (-1 + \eta) \, \theta p \, (10 - 4 \, \eta + 2 \, \eta t + 12 \, \mathfrak{x}1 + 5 \, \mathfrak{x}2 - 2 \, \eta \, \mathfrak{x}2 + \\
& \eta t \, \mathfrak{x}2 + w \, (-1 + \eta) \, (\eta \, (2 + \mathfrak{x}2) - \eta t \, (2 + \mathfrak{x}2) - 3 \times (2 + 4 \, \mathfrak{x}1 + \mathfrak{x}2))) + \\
& (-1 + \eta t) \, \theta l \, (-12 + 12 \, \theta p + 40 \, \eta \, \theta p - 8 \, \eta^2 \, \theta p - 4 \, \mathfrak{x}1 + 8 \, \theta p \, \mathfrak{x}1 + \\
& 48 \, \eta \, \theta p \, \mathfrak{x}1 + 2 \, \theta p \, \mathfrak{x}1^2 - 6 \, \mathfrak{x}2 + 12 \, \theta p \, \mathfrak{x}2 + 32 \, \eta \, \theta p \, \mathfrak{x}2 - \\
& 4 \, \eta^2 \, \theta p \, \mathfrak{x}2 + 4 \, \theta p \, \mathfrak{x}1 \, \mathfrak{x}2 + 3 \, \theta p \, \mathfrak{x}2^2 + 6 \, \eta \, \theta p \, \mathfrak{x}2^2 + 2 \, w^2 \, (-1 + \eta)^2 \\
& (-2 \, \mathfrak{x}1 - 3 \times (2 + \mathfrak{x}2) + \theta p \, (\mathfrak{x}1^2 + 3 \, (2 + \mathfrak{x}2)^2 + 2 \, \mathfrak{x}1 \, (8 + \mathfrak{x}2))) - \\
& w \, (-1 + \eta) \times (-4 \times (6 + 2 \, \mathfrak{x}1 + 3 \, \mathfrak{x}2) + \theta p \, (44 + 4 \, \mathfrak{x}1^2 + 40 \, \mathfrak{x}2 + \\
& 9 \, \mathfrak{x}2^2 + 8 \, \mathfrak{x}1 \, (5 + \mathfrak{x}2) + \eta \, (20 + 48 \, \mathfrak{x}1 + 22 \, \mathfrak{x}2 + 6 \, \mathfrak{x}2^2)))) - \\
& \theta p \, (20 \, \eta^2 - 28 \, \eta^3 + 8 \, \eta^4 + 12 \, \eta t - 12 \, \eta \, \eta t + 4 \, \eta^2 \, \eta t - 4 \, \eta^3 \, \eta t - 12 \, \eta \\
& \theta l - 20 \, \eta^2 \, \theta l + 4 \, \eta^3 \, \theta l + 12 \, \eta \, \eta t \, \theta l + 20 \, \eta^2 \, \eta t \, \theta l - 4 \, \eta^3 \, \eta t \, \theta l + 24 \\
& \eta^2 \, \mathfrak{x}1 - 24 \, \eta^3 \, \mathfrak{x}1 + 4 \, \eta t \, \mathfrak{x}1 - 4 \, \eta \, \eta t \, \mathfrak{x}1 - 8 \, \eta \, \theta l \, \mathfrak{x}1 - 24 \, \eta^2 \, \theta l \, \mathfrak{x}1 + 8 \, \eta \\
& \eta t \, \theta l \, \mathfrak{x}1 + 24 \, \eta^2 \, \eta t \, \theta l \, \mathfrak{x}1 - 2 \, \eta \, \theta l \, \mathfrak{x}1^2 + 2 \, \eta \, \eta t \, \theta l \, \mathfrak{x}1^2 + 10 \, \eta^2 \, \mathfrak{x}2 - 14 \\
& \eta^3 \, \mathfrak{x}2 + 4 \, \eta^4 \, \mathfrak{x}2 + 6 \, \eta t \, \mathfrak{x}2 - 6 \, \eta \, \eta t \, \mathfrak{x}2 + 2 \, \eta^2 \, \eta t \, \mathfrak{x}2 - 2 \, \eta^3 \, \eta t \, \mathfrak{x}2 - 12 \, \eta \\
& \theta l \, \mathfrak{x}2 - 16 \, \eta^2 \, \theta l \, \mathfrak{x}2 + 2 \, \eta^3 \, \theta l \, \mathfrak{x}2 + 12 \, \eta \, \eta t \, \theta l \, \mathfrak{x}2 + 16 \, \eta^2 \, \eta t \, \theta l \, \mathfrak{x}2 - 2 \\
& \eta^3 \, \eta t \, \theta l \, \mathfrak{x}2 - 4 \, \eta \, \theta l \, \mathfrak{x}1 \, \mathfrak{x}2 + 4 \, \eta \, \eta t \, \theta l \, \mathfrak{x}1 \, \mathfrak{x}2 - 3 \, \eta \, \theta l \, \mathfrak{x}2^2 - 3 \, \eta^2 \, \theta l \\
& \mathfrak{x}2^2 + 3 \, \eta \, \eta t \, \theta l \, \mathfrak{x}2^2 + 3 \, \eta^2 \, \eta t \, \theta l \, \mathfrak{x}2^2 - w \, (-1 + \eta) \times (2 \, \eta^4 \, (2 + \mathfrak{x}2) + \\
& 4 \, \eta t \, (6 + 2 \, \mathfrak{x}1 + 3 \, \mathfrak{x}2) - 2 \, \eta^3 \, (\eta t \, (2 + \mathfrak{x}2) + 2 \times (2 + 6 \, \mathfrak{x}1 + \mathfrak{x}2)) + \\
& \eta^2 \, (-8 \times (2 + \mathfrak{x}2) + (-1 + \eta t) \, \theta l \, (8 + 24 \, \mathfrak{x}1 + 10 \, \mathfrak{x}2 + 3 \, \mathfrak{x}2^2)) + \\
& \eta \, (20 + 24 \, \mathfrak{x}1 + 10 \, \mathfrak{x}2 - \theta l \, (44 + 4 \, \mathfrak{x}1^2 + 40 \, \mathfrak{x}2 + 9 \, \mathfrak{x}2^2 + 8 \, \mathfrak{x}1 \, (5 + \mathfrak{x}2)) + \\
& \eta t \, (-2 \times (4 \, \mathfrak{x}1 + 5 \times (2 + \mathfrak{x}2)) + \theta l \, (44 + 4 \, \mathfrak{x}1^2 + 40 \, \mathfrak{x}2 + 9 \, \mathfrak{x}2^2 + \\
& 8 \, \mathfrak{x}1 \, (5 + \mathfrak{x}2)))) + 2 \, w^2 \, (-1 + \eta)^2 \, (\eta^3 \, (2 + \mathfrak{x}2) + \\
& \eta t \, (6 + 2 \, \mathfrak{x}1 + 3 \, \mathfrak{x}2) - \eta^2 \, (\eta t \, (2 + \mathfrak{x}2) + 4 \times (2 + 3 \, \mathfrak{x}1 + \mathfrak{x}2)) + \\
& \eta \, (3 \times (2 + 4 \, \mathfrak{x}1 + \mathfrak{x}2) - \theta l \, (\mathfrak{x}1^2 + 3 \, (2 + \mathfrak{x}2)^2 + 2 \, \mathfrak{x}1 \, (8 + \mathfrak{x}2)) + \eta t \\
& (-2 \times (2 + \mathfrak{x}1 + \mathfrak{x}2) + \theta l \, (\mathfrak{x}1^2 + 3 \, (2 + \mathfrak{x}2)^2 + 2 \, \mathfrak{x}1 \, (8 + \mathfrak{x}2)))))) + \\
& 2 \, c \sigma^2 \, (-1 + \eta)^2 \, (w^5 \, (-1 + \eta)^6 \, (2 \, x^5 \, (-1 + \eta)^5 \, \theta p \, (\eta - \eta t + 4 \, \mu 1) \, (3 + 3 \, \mu 1 + 4 \, \mu 2) - \\
& \eta \, \theta p \, (\eta^5 \, (6 + 6 \, \mu 1 + 8 \, \mu 2) + \eta t \, \mu 2 \, (11 + 11 \, \mu 1 + 8 \, \mu 2) - 2 \, \eta \, \eta t \\
& (9 + 21 \, \mu 1^2 + 5 \, \mu 2 - 8 \, \mu 2^2 + 5 \, \mu 1 \, (6 + \mu 2)) + 2 \, \eta^3 \, (12 + 45 \, \mu 1 + 33 \, \mu 1^2 + \\
& 21 \, \mu 2 + 49 \, \mu 1 \, \mu 2 - 52 \, \mu 2^2 + 2 \, \eta t \, (-3 - 3 \, \mu 1 + \mu 2 + 5 \, \mu 1 \, \mu 2 + 14 \, \mu 2^2)) + \\
& \eta^2 \, (-\eta t \, (24 + 26 \, \mu 1 + 2 \, \mu 1^2 + 9 \, \mu 2 - 111 \, \mu 1 \, \mu 2 - 64 \, \mu 2^2) + \\
& 2 \times (9 + 30 \, \mu 1 + 21 \, \mu 1^2 + 47 \, \mu 2 + 63 \, \mu 1 \, \mu 2 + 32 \, \mu 2^2)) - 2 \, \eta^4 \\
& (\eta t \, (3 + 3 \, \mu 1 + 4 \, \mu 2) + 2 \times (-3 - 6 \, \mu 1^2 + \mu 2 + 14 \, \mu 2^2 - 3 \, \mu 1 \, (3 + \mu 2)))) + \\
& x^4 \, (-1 + \eta)^3 \, ((-1 + \eta t) \, \theta l \, (18 + 2 \, \mu 1^2 + \mu 1 \, (20 - 43 \, \mu 2) + 21 \, \mu 2 - 8 \, \mu 2^2) - \\
& 2 \times (-1 + \eta) \, \theta p \, (9 + 42 \, \mu 1 + 33 \, \mu 1^2 + 27 \, \mu 2 + 59 \, \mu 1 \, \mu 2 + 5 \, \eta^2 \, (3 + 3 \, \mu 1 + 4 \, \mu 2) + \\
& 2 \, \eta t \, (-3 - 3 \, \mu 1 + \mu 2 + 5 \, \mu 1 \, \mu 2 + 14 \, \mu 2^2) + \eta \, (6 + 66 \, \mu 1 + 60 \, \mu 1^2 - \\
& 2 \, \mu 2 + 70 \, \mu 1 \, \mu 2 - 28 \, \mu 2^2 - 5 \, \eta t \, (3 + 3 \, \mu 1 + 4 \, \mu 2)))) + \\
& x \, (10 \, \eta^6 \, \theta p \, (3 + 3 \, \mu 1 + 4 \, \mu 2) - 2 \, \eta^5 \, \theta p \, (-9 - 69 \, \mu 1 - 60 \, \mu 1^2 + 28 \, \mu 2 - \\
& 40 \, \mu 1 \, \mu 2 + 112 \, \mu 2^2 + 5 \, \eta t \, (3 + 3 \, \mu 1 + 4 \, \mu 2)) - \eta t \\
& \theta p \, (4 + 4 \, \mu 1^2 + 27 \, \mu 2 + 20 \, \mu 2^2 + \mu 1 \, (8 + 27 \, \mu 2)) + \eta \\
& (\eta t \, \theta p \, (32 + 92 \, \mu 1 + 60 \, \mu 1^2 + 15 \, \mu 2 + 7 \, \mu 1 \, \mu 2 - 36 \, \mu 2^2) -
\end{aligned}$$

$$\begin{aligned}
& (-1 + \eta t) \, \text{el} \left( 4 + 8 \mu_1 + 4 \mu_1^2 + 5 \mu_2 + 5 \mu_1 \mu_2 + 4 \mu_2^2 \right) + 2 \\
& \eta^4 \, \text{ep} \left( 21 + 93 \mu_1 + 72 \mu_1^2 + 98 \mu_2 + 166 \mu_1 \mu_2 - 44 \mu_2^2 + \right. \\
& \quad \left. \eta t \left( -9 - 9 \mu_1 + 28 \mu_2 + 40 \mu_1 \mu_2 + 112 \mu_2^2 \right) \right) - \eta^3 \\
& \left( (-1 + \eta t) \, \text{el} \left( 22 + 26 \mu_1^2 + \mu_1 (48 - 67 \mu_2) + 37 \mu_2 + 4 \mu_2^2 \right) + \right. \\
& \quad \text{ep} \left( 2 \times (18 + 87 \mu_1 + 69 \mu_1^2 - 51 \mu_2 + 17 \mu_1 \mu_2 - 252 \mu_2^2) + \right. \\
& \quad \quad \left. \eta t (20 + 2 \mu_1 - 18 \mu_1^2 + 27 \mu_2 - 229 \mu_1 \mu_2 + 20 \mu_2^2) \right) \left. \right) - \eta^2 \\
& \left( 2 \times (-1 + \eta t) \, \text{el} \left( 13 + 35 \mu_1^2 + 21 \mu_2 + 4 \mu_2^2 + \mu_1 (48 + 25 \mu_2) \right) + \right. \\
& \quad \text{ep} \left( 6 \times (9 + 30 \mu_1 + 21 \mu_1^2 + 47 \mu_2 + 63 \mu_1 \mu_2 + 32 \mu_2^2) + \right. \\
& \quad \quad \left. \eta t (-40 + 34 \mu_1 + 74 \mu_1^2 - 23 \mu_2 + 289 \mu_1 \mu_2 + 148 \mu_2^2) \right) \left. \right) - \\
& x^2 (-1 + \eta) \times (20 \eta^5 \, \text{ep} (3 + 3 \mu_1 + 4 \mu_2) - \text{el} \mu_2 (11 + 11 \mu_1 + 8 \mu_2) + \\
& \quad \eta t \, \text{el} \mu_2 (11 + 11 \mu_1 + 8 \mu_2) + 2 \eta t \, \text{ep} \\
& \quad (5 + 7 \mu_1^2 - 11 \mu_2 - 20 \mu_2^2 - 3 \mu_1 (-4 + 5 \mu_2)) - 4 \eta^4 \, \text{ep} \\
& \quad (-3 - 60 \mu_1^2 + 26 \mu_2 + 84 \mu_2^2 + 5 \eta t (3 + 3 \mu_1 + 4 \mu_2) - \mu_1 (63 + 50 \mu_2)) + 2 \\
& \eta^3 \, \text{ep} (78 \mu_1^2 + 7 \mu_1 (15 + 32 \mu_2) + 3 \times (9 + 52 \mu_2 + 4 \mu_2^2) + \\
& \quad 2 \eta t (-3 + 26 \mu_2 + 84 \mu_2^2 + \mu_1 (-3 + 30 \mu_2)) \left. \right) - \eta^2 \\
& \left( (-1 + \eta t) \, \text{el} (62 + 54 \mu_1^2 + \mu_1 (116 - 177 \mu_2) + 95 \mu_2) + \right. \\
& \quad \text{ep} (-\eta t (8 + 50 \mu_1 + 42 \mu_1^2 - 19 \mu_2 + 165 \mu_1 \mu_2 - 120 \mu_2^2) + \\
& \quad \quad \left. 6 \times (12 + 57 \mu_1 + 45 \mu_1^2 + \mu_2 + 45 \mu_1 \mu_2 - 84 \mu_2^2) \right) \left. \right) - \eta \\
& \left( 4 \times (-1 + \eta t) \, \text{el} (11 + 28 \mu_1^2 + 13 \mu_2 - 2 \mu_2^2 + 3 \mu_1 (13 + 5 \mu_2)) + \right. \\
& \quad \text{ep} (6 \times (9 + 30 \mu_1 + 21 \mu_1^2 + 47 \mu_2 + 63 \mu_1 \mu_2 + 32 \mu_2^2) + \eta t (-54 + \\
& \quad \quad \left. 2 \mu_1 + 56 \mu_1^2 - 17 \mu_2 + 255 \mu_1 \mu_2 + 176 \mu_2^2) \right) \left. \right) + x^3 (-1 + \eta)^2 \\
& \left( - \left( (-1 + \eta t) \, \text{el} (\eta (58 + 30 \mu_1^2 + \mu_1 (88 - 153 \mu_2) + 79 \mu_2 - 12 \mu_2^2) + \right. \right. \\
& \quad \left. \left. 2 \times (9 + 21 \mu_1^2 + 5 \mu_2 - 8 \mu_2^2 + 5 \mu_1 (6 + \mu_2)) \right) \right) + (-1 + \eta) \, \text{ep} \\
& \left( 20 \eta^3 (3 + 3 \mu_1 + 4 \mu_2) + 2 \times (9 + 30 \mu_1 + 21 \mu_1^2 + 47 \mu_2 + 63 \mu_1 \mu_2 + \right. \\
& \quad \left. 32 \mu_2^2) + \eta t (-20 + 2 \mu_1 + 22 \mu_1^2 + 7 \mu_2 + 87 \mu_1 \mu_2 + 76 \mu_2^2) + \right. \\
& \quad 2 \eta (39 + 171 \mu_1 + 132 \mu_1^2 + 102 \mu_2 + 226 \mu_1 \mu_2 - 52 \mu_2^2 + 8 \eta t \\
& \quad \quad \left. (-3 - 3 \mu_1 + \mu_2 + 5 \mu_1 \mu_2 + 14 \mu_2^2) \right) - 4 \eta^2 (5 \eta t (3 + 3 \mu_1 + 4 \mu_2) + \\
& \quad \quad \left. 4 \times (-3 - 15 \mu_1^2 + \mu_2 + 14 \mu_2^2 - 3 \mu_1 (6 + 5 \mu_2)) \right) \left. \right) + \\
& w^4 (-1 + \eta)^4 (6 x^6 (-1 + \eta)^7 \, \text{ep} (\eta - \eta t + 4 \mu_1) (3 + 3 \mu_1 + 4 \mu_2) + \\
& \quad x^5 (-1 + \eta)^5 (-2 \times (-1 + \eta) \, \text{ep} (47 + 185 \mu_1 + 138 \mu_1^2 + 141 \mu_2 + 237 \mu_1 \mu_2 + \\
& \quad \quad 18 \eta^2 (3 + 3 \mu_1 + 4 \mu_2) + \eta t (-29 - 29 \mu_1 - 14 \mu_2 + 30 \mu_1 \mu_2 + 84 \mu_2^2) + \\
& \quad \quad \eta (29 + 245 \mu_1 + 216 \mu_1^2 + 14 \mu_2 + 258 \mu_1 \mu_2 - \\
& \quad \quad \quad 84 \mu_2^2 - 18 \eta t (3 + 3 \mu_1 + 4 \mu_2)) \left. \right) + (-1 + \eta t) \\
& \quad \text{el} (-2 \times (-11 + 29 \mu_1^2 + 24 \mu_2 + 36 \mu_2^2 + 18 \mu_1 (1 + 8 \mu_2)) + \\
& \quad \quad \text{ep} (72 + 17 \mu_1 + 12 \mu_2^2 (6 + 3 \mu_1 - \mu_2) + 7 \mu_2 + \\
& \quad \quad \quad 12 \mu_1^2 (6 + \mu_1 + \mu_2) + \mu_2 (288 + 59 \mu_1 + 37 \mu_2) + \\
& \quad \quad \quad \mu_1 (144 + 29 \mu_1 + 19 \mu_2 + \mu_2 (288 + 35 \mu_1 + 61 \mu_2)) \left. \right) \left. \right) + \\
& \eta \, \text{ep} (6 \eta^7 (3 + 3 \mu_1 + 4 \mu_2) - 3 \eta t \mu_2 (11 + 11 \mu_1 + 8 \mu_2) + \eta \eta t \\
& \quad (40 + 112 \mu_1^2 + \mu_1 (152 - 33 \mu_2) - 33 \mu_2 - 96 \mu_2^2) + 2 \eta^5 \\
& \quad (49 + 102 \mu_1^2 + 119 \mu_2 - 156 \mu_2^2 + \mu_1 (151 + 159 \mu_2) + \\
& \quad \quad \eta t (-20 - 2 \mu_2 + 84 \mu_2^2 + 10 \mu_1 (-2 + 3 \mu_2)) \left. \right) - 2 \eta^6 \\
& \quad (3 \eta t (3 + 3 \mu_1 + 4 \mu_2) - 2 \times (10 + 18 \mu_1^2 + \mu_2 - 42 \mu_2^2 + \mu_1 (28 + 9 \mu_2)) \left. \right) -
\end{aligned}$$

$$\begin{aligned}
& \eta^3 \left( 116 + 320 \mu_1 + 144 \eta t \mu_1 + 204 \mu_1^2 + 144 \eta t \mu_1^2 + 294 \mu_2 - \right. \\
& \quad 37 \eta t \mu_2 + 350 \mu_1 \mu_2 + 139 \eta t \mu_1 \mu_2 - 200 \mu_2^2 + 72 \eta t \mu_2^2 + \\
& \quad 2 \times (-1 + \eta t) \theta l \left( 72 + 17 \mathfrak{e}1 + 12 \mu_2^2 (6 + 3 \mathfrak{e}1 - \mathfrak{e}2) + \right. \\
& \quad \quad 7 \mathfrak{e}2 + 12 \mu_1^2 (6 + \mathfrak{e}1 + \mathfrak{e}2) + \mu_2 (288 + 59 \mathfrak{e}1 + 37 \mathfrak{e}2) + \\
& \quad \quad \left. \mu_1 (144 + 29 \mathfrak{e}1 + 19 \mathfrak{e}2 + \mu_2 (288 + 35 \mathfrak{e}1 + 61 \mathfrak{e}2)) \right) \left. \right) + \\
& \eta^4 \left( 72 + 150 \mu_1 + 78 \mu_1^2 + 520 \mu_2 + 488 \mu_1 \mu_2 + 520 \mu_2^2 + \right. \\
& \quad 2 \eta t (-13 + 37 \mu_1^2 + 38 \mu_2 + 92 \mu_2^2 + \mu_1 (24 + 266 \mu_2)) + \\
& \quad \theta l \left( 72 + 17 \mathfrak{e}1 + 12 \mu_2^2 (6 + 3 \mathfrak{e}1 - \mathfrak{e}2) + 7 \mathfrak{e}2 + \right. \\
& \quad \quad 12 \mu_1^2 (6 + \mathfrak{e}1 + \mathfrak{e}2) + \mu_2 (288 + 59 \mathfrak{e}1 + 37 \mathfrak{e}2) + \\
& \quad \quad \left. \mu_1 (144 + 29 \mathfrak{e}1 + 19 \mathfrak{e}2 + \mu_2 (288 + 35 \mathfrak{e}1 + 61 \mathfrak{e}2)) \right) - \\
& \quad \eta t \theta l \left( 72 + 17 \mathfrak{e}1 + 12 \mu_2^2 (6 + 3 \mathfrak{e}1 - \mathfrak{e}2) + 7 \mathfrak{e}2 + \right. \\
& \quad \quad 12 \mu_1^2 (6 + \mathfrak{e}1 + \mathfrak{e}2) + \mu_2 (288 + 59 \mathfrak{e}1 + 37 \mathfrak{e}2) + \\
& \quad \quad \left. \mu_1 (144 + 29 \mathfrak{e}1 + 19 \mathfrak{e}2 + \mu_2 (288 + 35 \mathfrak{e}1 + 61 \mathfrak{e}2)) \right) \left. \right) - \eta^2 \\
& \quad \left( 2 \times (56 + 75 \mu_1^2 + 246 \mu_2 + 120 \mu_2^2 + \mu_1 (131 + 246 \mu_2)) - \right. \\
& \quad \theta l \left( 72 + 17 \mathfrak{e}1 + 12 \mu_2^2 (6 + 3 \mathfrak{e}1 - \mathfrak{e}2) + 7 \mathfrak{e}2 + 12 \mu_1^2 (6 + \mathfrak{e}1 + \mathfrak{e}2) + \right. \\
& \quad \quad \mu_2 (288 + 59 \mathfrak{e}1 + 37 \mathfrak{e}2) + \mu_1 (144 + 29 \mathfrak{e}1 + 19 \mathfrak{e}2 + \\
& \quad \quad \quad \left. \mu_2 (288 + 35 \mathfrak{e}1 + 61 \mathfrak{e}2)) \right) + \eta t (-44 - 2 \mu_1 + 42 \mu_1^2 + 19 \mu_2 + \\
& \quad \quad 387 \mu_1 \mu_2 + 160 \mu_2^2 + \theta l \left( 72 + 17 \mathfrak{e}1 + 12 \mu_2^2 (6 + 3 \mathfrak{e}1 - \mathfrak{e}2) + \right. \\
& \quad \quad \quad 7 \mathfrak{e}2 + 12 \mu_1^2 (6 + \mathfrak{e}1 + \mathfrak{e}2) + \mu_2 (288 + 59 \mathfrak{e}1 + 37 \mathfrak{e}2) + \\
& \quad \quad \quad \left. \mu_1 (144 + 29 \mathfrak{e}1 + 19 \mathfrak{e}2 + \mu_2 (288 + 35 \mathfrak{e}1 + 61 \mathfrak{e}2)) \right) \left. \right) \left. \right) + \\
& x^4 (-1 + \eta)^4 \left( 2 \times (-1 + \eta) \theta p \left( 103 + 280 \mu_1 + 177 \mu_1^2 + 395 \mu_2 + \right. \right. \\
& \quad 443 \mu_1 \mu_2 + 168 \mu_2^2 + 45 \eta^3 (3 + 3 \mu_1 + 4 \mu_2) + \\
& \quad \eta t (-38 + 25 \mu_1 + 63 \mu_1^2 + 40 \mu_2 + 244 \mu_1 \mu_2 + 188 \mu_2^2) - \\
& \quad 5 \eta^2 (-29 - 137 \mu_1 - 108 \mu_1^2 - 14 \mu_2 - 114 \mu_1 \mu_2 + 84 \mu_2^2 + \\
& \quad \quad 9 \eta t (3 + 3 \mu_1 + 4 \mu_2)) + \eta (266 + 956 \mu_1 + 690 \mu_1^2 + 697 \mu_2 + 1125 \\
& \quad \quad \mu_1 \mu_2 - 240 \mu_2^2 + 5 \eta t (-29 - 29 \mu_1 - 14 \mu_2 + 30 \mu_1 \mu_2 + 84 \mu_2^2)) \left. \right) - \\
& \quad (-1 + \eta t) \theta l \left( 62 + 132 \mu_1 + 70 \mu_1^2 - 81 \mu_2 - 225 \mu_1 \mu_2 - 168 \mu_2^2 + \right. \\
& \quad 2 \theta p \left( 72 + 17 \mathfrak{e}1 + 12 \mu_2^2 (6 + 3 \mathfrak{e}1 - \mathfrak{e}2) + 7 \mathfrak{e}2 + \right. \\
& \quad \quad 12 \mu_1^2 (6 + \mathfrak{e}1 + \mathfrak{e}2) + \mu_2 (288 + 59 \mathfrak{e}1 + 37 \mathfrak{e}2) + \\
& \quad \quad \left. \mu_1 (144 + 29 \mathfrak{e}1 + 19 \mathfrak{e}2 + \mu_2 (288 + 35 \mathfrak{e}1 + 61 \mathfrak{e}2)) \right) + \\
& \quad \eta (-4 \times (-24 + 45 \mu_1^2 + 40 \mu_2 + 66 \mu_2^2 + \mu_1 (21 + 314 \mu_2)) + \\
& \quad 5 \theta p \left( 72 + 17 \mathfrak{e}1 + 12 \mu_2^2 (6 + 3 \mathfrak{e}1 - \mathfrak{e}2) + 7 \mathfrak{e}2 + \right. \\
& \quad \quad 12 \mu_1^2 (6 + \mathfrak{e}1 + \mathfrak{e}2) + \mu_2 (288 + 59 \mathfrak{e}1 + 37 \mathfrak{e}2) + \\
& \quad \quad \left. \mu_1 (144 + 29 \mathfrak{e}1 + 19 \mathfrak{e}2 + \mu_2 (288 + 35 \mathfrak{e}1 + 61 \mathfrak{e}2)) \right) \left. \right) \left. \right) + \\
& x^3 (-1 + \eta)^3 \left( - \left( (-1 + \eta) \theta p \left( 120 \eta^4 (3 + 3 \mu_1 + 4 \mu_2) + 2 \times (56 + \right. \right. \right. \\
& \quad 131 \mu_1 + 75 \mu_1^2 + 246 \mu_2 + 246 \mu_1 \mu_2 + 120 \mu_2^2) + \eta t (-56 + 22 \mu_1 + \\
& \quad 78 \mu_1^2 + 197 \mu_2 + 469 \mu_1 \mu_2 + 364 \mu_2^2) - 20 \eta^3 (-29 - 101 \mu_1 - \\
& \quad 72 \mu_1^2 - 14 \mu_2 - 66 \mu_1 \mu_2 + 84 \mu_2^2 + 6 \eta t (3 + 3 \mu_1 + 4 \mu_2)) + \\
& \quad 4 \eta^2 (297 + 987 \mu_1 + 690 \mu_1^2 + 689 \mu_2 + 1065 \mu_1 \mu_2 - 480 \mu_2^2 + \\
& \quad \quad 5 \eta t (-29 - 29 \mu_1 - 14 \mu_2 + 30 \mu_1 \mu_2 + 84 \mu_2^2)) + \\
& \quad 2 \eta (423 + 1131 \mu_1 + 708 \mu_1^2 + 1578 \mu_2 + 1750 \mu_1 \mu_2 + 524 \mu_2^2 + \\
& \quad \quad 2 \eta t (-78 + 35 \mu_1 + 113 \mu_1^2 + 72 \mu_2 + 514 \mu_1 \mu_2 + 370 \mu_2^2)) \left. \right) + \\
& \quad (-1 + \eta t) \theta l \left( 2 \times (20 + 56 \mu_1^2 + \mu_1 (76 - 33 \mu_2) - 33 \mu_2 - 60 \mu_2^2) + \right.
\end{aligned}$$

$$\begin{aligned}
& \left( \begin{aligned}
& \text{ep} \left( 72 + 17 \, \mathfrak{e}1 + 12 \, \mu^2 (6 + 3 \, \mathfrak{e}1 - \mathfrak{e}2) + 7 \, \mathfrak{e}2 + \right. \\
& \quad 12 \, \mu^2 (6 + \mathfrak{e}1 + \mathfrak{e}2) + \mu^2 (288 + 59 \, \mathfrak{e}1 + 37 \, \mathfrak{e}2) + \\
& \quad \left. \mu^1 (144 + 29 \, \mathfrak{e}1 + 19 \, \mathfrak{e}2 + \mu^2 (288 + 35 \, \mathfrak{e}1 + 61 \, \mathfrak{e}2)) \right) + \\
& 2 \, \eta^2 \left( -6 \times \left( -13 + 16 \, \mu^2 + 16 \, \mu^2 + 30 \, \mu^2 + \mu^1 (3 + 170 \, \mu^2) \right) + \right. \\
& \quad \left. 5 \, \text{ep} \left( 72 + 17 \, \mathfrak{e}1 + 12 \, \mu^2 (6 + 3 \, \mathfrak{e}1 - \mathfrak{e}2) + 7 \, \mathfrak{e}2 + \right. \right. \\
& \quad \quad 12 \, \mu^2 (6 + \mathfrak{e}1 + \mathfrak{e}2) + \mu^2 (288 + 59 \, \mathfrak{e}1 + 37 \, \mathfrak{e}2) + \\
& \quad \quad \left. \mu^1 (144 + 29 \, \mathfrak{e}1 + 19 \, \mathfrak{e}2 + \mu^2 (288 + 35 \, \mathfrak{e}1 + 61 \, \mathfrak{e}2)) \right) \right) + \\
& \eta \left( 214 + 572 \, \mu^1 + 358 \, \mu^2 - 131 \, \mu^2 - 659 \, \mu^1 \mu^2 - 420 \, \mu^2 + \right. \\
& \quad \left. 8 \, \text{ep} \left( 72 + 17 \, \mathfrak{e}1 + 12 \, \mu^2 (6 + 3 \, \mathfrak{e}1 - \mathfrak{e}2) + 7 \, \mathfrak{e}2 + \right. \right. \\
& \quad \quad 12 \, \mu^2 (6 + \mathfrak{e}1 + \mathfrak{e}2) + \mu^2 (288 + 59 \, \mathfrak{e}1 + 37 \, \mathfrak{e}2) + \\
& \quad \quad \left. \mu^1 (144 + 29 \, \mathfrak{e}1 + 19 \, \mathfrak{e}2 + \mu^2 (288 + 35 \, \mathfrak{e}1 + 61 \, \mathfrak{e}2)) \right) \right) \Big) - \\
& \times (-1 + \eta) \times \left( 36 \, \eta^7 \, \text{ep} (3 + 3 \, \mu^1 + 4 \, \mu^2) - 3 \, \eta \mathfrak{t} \, \text{ep} (4 + 4 \, \mu^2 + 27 \, \mu^2 + \right. \\
& \quad 20 \, \mu^2 + \mu^1 (8 + 27 \, \mu^2)) - 2 \, \eta^6 \, \text{ep} (-91 - 216 \, \mu^2 + 2 \, \mu^2 + \\
& \quad 420 \, \mu^2 + 18 \, \eta \mathfrak{t} (3 + 3 \, \mu^1 + 4 \, \mu^2) - \mu^1 (307 + 138 \, \mu^2)) + \eta \\
& \quad \left( \eta \mathfrak{t} \, \text{ep} (60 + 144 \, \mu^2 + \mu^1 (204 - 203 \, \mu^2) - 179 \, \mu^2 - 276 \, \mu^2) - \right. \\
& \quad \left. 3 \times (-1 + \eta \mathfrak{t}) \, \mathfrak{el} (4 + 4 \, \mu^2 + 5 \, \mu^2 + 4 \, \mu^2 + \mu^1 (8 + 5 \, \mu^2)) \right) + 2 \\
& \eta^5 \, \text{ep} (214 + 474 \, \mu^2 + 603 \, \mu^2 - 540 \, \mu^2 + \mu^1 (688 + 807 \, \mu^2) + \\
& \quad \eta \mathfrak{t} (-91 + 2 \, \mu^2 + 420 \, \mu^2 + \mu^1 (-91 + 150 \, \mu^2)) \Big) - \eta^2 \\
& \left( \text{ep} (6 \times (56 + 75 \, \mu^2 + 246 \, \mu^2 + 120 \, \mu^2 + \mu^1 (131 + 246 \, \mu^2)) + \right. \\
& \quad \eta \mathfrak{t} (-176 + 70 \, \mu^2 + 107 \, \mu^2 + 588 \, \mu^2 + \mu^1 (-106 + 1091 \, \mu^2)) \Big) + \\
& \quad (-1 + \eta \mathfrak{t}) \, \mathfrak{el} (72 + 276 \, \mu^1 + 204 \, \mu^2 + 62 \, \mu^2 + 86 \, \mu^1 \mu^2 - \\
& \quad 24 \, \mu^2 + 3 \, \text{ep} (72 + 17 \, \mathfrak{e}1 + 12 \, \mu^2 (6 + 3 \, \mathfrak{e}1 - \mathfrak{e}2) + 7 \, \mathfrak{e}2 + \\
& \quad \quad 12 \, \mu^2 (6 + \mathfrak{e}1 + \mathfrak{e}2) + \mu^2 (288 + 59 \, \mathfrak{e}1 + 37 \, \mathfrak{e}2) + \\
& \quad \quad \left. \mu^1 (144 + 29 \, \mathfrak{e}1 + 19 \, \mathfrak{e}2 + \mu^2 (288 + 35 \, \mathfrak{e}1 + 61 \, \mathfrak{e}2)) \right) \Big) + \\
& \eta^4 \left( 2 \, \text{ep} (86 + 18 \, \mu^2 + 901 \, \mu^2 + 1188 \, \mu^2 + \mu^1 (104 + 761 \, \mu^2) + \right. \\
& \quad \eta \mathfrak{t} (-19 + 174 \, \mu^2 + 182 \, \mu^2 + 296 \, \mu^2 + \mu^1 (155 + 982 \, \mu^2)) \Big) - \\
& \quad (-1 + \eta \mathfrak{t}) \, \mathfrak{el} (-2 \times (-15 + 3 \, \mu^2 + 8 \, \mu^2 + 24 \, \mu^2 + 4 \, \mu^1 (-3 + 49 \, \mu^2)) + \\
& \quad 5 \, \text{ep} (72 + 17 \, \mathfrak{e}1 + 12 \, \mu^2 (6 + 3 \, \mathfrak{e}1 - \mathfrak{e}2) + 7 \, \mathfrak{e}2 + \\
& \quad \quad 12 \, \mu^2 (6 + \mathfrak{e}1 + \mathfrak{e}2) + \mu^2 (288 + 59 \, \mathfrak{e}1 + 37 \, \mathfrak{e}2) + \\
& \quad \quad \left. \mu^1 (144 + 29 \, \mathfrak{e}1 + 19 \, \mathfrak{e}2 + \mu^2 (288 + 35 \, \mathfrak{e}1 + 61 \, \mathfrak{e}2)) \right) \Big) - \eta^3 \\
& \left( \text{ep} (2 \times (277 + 483 \, \mu^2 + 836 \, \mu^2 - 132 \, \mu^2 + 8 \, \mu^1 (95 + 121 \, \mu^2)) + \right. \\
& \quad \eta \mathfrak{t} (-104 + 410 \, \mu^2 - 143 \, \mu^2 + 508 \, \mu^2 + \mu^1 (306 + 889 \, \mu^2)) \Big) + \\
& \quad (-1 + \eta \mathfrak{t}) \, \mathfrak{el} (90 + 308 \, \mu^1 + 218 \, \mu^2 + 31 \, \mu^2 - 209 \, \mu^1 \mu^2 - \\
& \quad 84 \, \mu^2 + 8 \, \text{ep} (72 + 17 \, \mathfrak{e}1 + 12 \, \mu^2 (6 + 3 \, \mathfrak{e}1 - \mathfrak{e}2) + 7 \, \mathfrak{e}2 + \\
& \quad \quad 12 \, \mu^2 (6 + \mathfrak{e}1 + \mathfrak{e}2) + \mu^2 (288 + 59 \, \mathfrak{e}1 + 37 \, \mathfrak{e}2) + \\
& \quad \quad \left. \mu^1 (144 + 29 \, \mathfrak{e}1 + 19 \, \mathfrak{e}2 + \mu^2 (288 + 35 \, \mathfrak{e}1 + 61 \, \mathfrak{e}2)) \right) \Big) \Big) + \\
& x^2 (-1 + \eta)^2 \left( 8 \, \eta \mathfrak{t} \, \text{ep} + 28 \, \eta \mathfrak{t} \, \text{ep} \, \mu^1 + 20 \, \eta \mathfrak{t} \, \text{ep} \, \mu^2 - 33 \, \mathfrak{el} \, \mu^2 + 33 \right. \\
& \quad \eta \mathfrak{t} \, \mathfrak{el} \, \mu^2 - 194 \, \eta \mathfrak{t} \, \text{ep} \, \mu^2 - 33 \, \mathfrak{el} \, \mu^1 \mu^2 + 33 \, \eta \mathfrak{t} \, \mathfrak{el} \, \mu^1 \\
& \quad \mu^2 - 218 \, \eta \mathfrak{t} \, \text{ep} \, \mu^1 \mu^2 - 24 \, \mathfrak{el} \, \mu^2 + 24 \, \eta \mathfrak{t} \, \mathfrak{el} \, \mu^2 - 216 \\
& \quad \eta \mathfrak{t} \, \text{ep} \, \mu^2 + 90 \, \eta^6 \, \text{ep} (3 + 3 \, \mu^1 + 4 \, \mu^2) - 10 \, \eta^5 \, \text{ep} \\
& \quad \left( -31 - 108 \, \mu^2 + 8 \, \mu^2 + 168 \, \mu^2 + 9 \, \eta \mathfrak{t} (3 + 3 \, \mu^1 + 4 \, \mu^2) - \mu^1 (139 + 84 \, \mu^2) \right) + \\
& 2 \, \eta^4 \, \text{ep} (5 \, \eta \mathfrak{t} (-31 + 8 \, \mu^2 + 168 \, \mu^2 + \mu^1 (-31 + 60 \, \mu^2)) + \\
& \quad 2 \times (183 + 420 \, \mu^2 + 611 \, \mu^2 - 300 \, \mu^2 + \mu^1 (603 + 795 \, \mu^2)) \Big) - \eta
\end{aligned}$$

$$\begin{aligned}
& \left( \theta p \left( 6 \times (56 + 75 \mu_1^2 + 246 \mu_2 + 120 \mu_2^2 + \mu_1 (131 + 246 \mu_2)) + \right. \right. \\
& \quad \left. \eta t (-188 + 106 \mu_1^2 + 285 \mu_2 + 792 \mu_2^2 + \mu_1 (-82 + 1173 \mu_2)) \right) + \\
& \quad (-1 + \eta t) \theta l \left( 4 \times (28 + 79 \mu_1^2 - \mu_2 - 36 \mu_2^2 + \mu_1 (107 + 5 \mu_2)) + \right. \\
& \quad \left. 3 \theta p (72 + 17 \mathfrak{e}1 + 12 \mu_2^2 (6 + 3 \mathfrak{e}1 - \mathfrak{e}2) + 7 \mathfrak{e}2 + \right. \\
& \quad \left. 12 \mu_1^2 (6 + \mathfrak{e}1 + \mathfrak{e}2) + \mu_2 (288 + 59 \mathfrak{e}1 + 37 \mathfrak{e}2) + \right. \\
& \quad \left. \mu_1 (144 + 29 \mathfrak{e}1 + 19 \mathfrak{e}2 + \mu_2 (288 + 35 \mathfrak{e}1 + 61 \mathfrak{e}2)) \right) \left. \right) - 2 \eta^3 \\
& \left( -\theta p (-5 - 318 \mu_1^2 + 1002 \mu_2 + 2004 \mu_2^2 + \mu_1 (-323 + 582 \mu_2) + \right. \\
& \quad \left. 2 \eta t (25 + 150 \mu_1^2 + 166 \mu_2 + 126 \mu_2^2 + 5 \mu_1 (35 + 132 \mu_2)) \right) + \\
& \quad (-1 + \eta t) \theta l (-2 \times (-28 + 19 \mu_1^2 + 24 \mu_2 + 54 \mu_2^2 + \mu_1 (-9 + 366 \mu_2)) + \\
& \quad \left. 5 \theta p (72 + 17 \mathfrak{e}1 + 12 \mu_2^2 (6 + 3 \mathfrak{e}1 - \mathfrak{e}2) + 7 \mathfrak{e}2 + \right. \\
& \quad \left. 12 \mu_1^2 (6 + \mathfrak{e}1 + \mathfrak{e}2) + \mu_2 (288 + 59 \mathfrak{e}1 + 37 \mathfrak{e}2) + \right. \\
& \quad \left. \mu_1 (144 + 29 \mathfrak{e}1 + 19 \mathfrak{e}2 + \mu_2 (288 + 35 \mathfrak{e}1 + 61 \mathfrak{e}2)) \right) \left. \right) - \eta^2 \\
& \left( \theta p \left( 6 \times (161 + 279 \mu_1^2 + 542 \mu_2 + 68 \mu_2^2 + \mu_1 (440 + 618 \mu_2)) + \right. \right. \\
& \quad \left. \eta t (-284 + 514 \mu_1^2 - 95 \mu_2 + 1176 \mu_2^2 + \mu_1 (230 + 1849 \mu_2)) \right) + \\
& \quad (-1 + \eta t) \theta l (242 + 748 \mu_1 + 506 \mu_1^2 - 19 \mu_2 - 643 \mu_1 \mu_2 - \\
& \quad \left. 336 \mu_2^2 + 12 \theta p (72 + 17 \mathfrak{e}1 + 12 \mu_2^2 (6 + 3 \mathfrak{e}1 - \mathfrak{e}2) + \right. \\
& \quad \left. 7 \mathfrak{e}2 + 12 \mu_1^2 (6 + \mathfrak{e}1 + \mathfrak{e}2) + \mu_2 (288 + 59 \mathfrak{e}1 + 37 \mathfrak{e}2) + \right. \\
& \quad \left. \mu_1 (144 + 29 \mathfrak{e}1 + 19 \mathfrak{e}2 + \mu_2 (288 + 35 \mathfrak{e}1 + 61 \mathfrak{e}2)) \right) \left. \right) \left. \right) - \\
& (x + \eta - x \eta)^2 (-2 x^6 (-1 + \eta)^6 \theta p (2 - 2 \theta l - 25 \mu_1 + 13 \theta l \mu_1 - 27 \mu_1^2 + \\
& \quad 15 \theta l \mu_1^2 + 12 \mu_2 - 12 \theta l \mu_2 - 44 \mu_1 \mu_2 + 28 \theta l \mu_1 \\
& \quad \mu_2 + 8 \eta t (1 + \mu_1 + 2 \mu_2) + 4 \eta^2 (3 + 3 \mu_1 + 8 \mu_2) - \eta \\
& \quad (14 - 13 \mu_1 - 27 \mu_1^2 + 44 \mu_2 - 44 \mu_1 \mu_2 - 4 \theta l (1 + \mu_1 + 4 \mu_2) + \\
& \quad 4 \eta t (2 + \theta l + 2 \mu_1 + \theta l \mu_1 + 4 \mu_2 + 4 \theta l \mu_2)) - \eta t \theta l \\
& \quad (-2 + 15 \mu_1^2 + \mu_1 (13 + 28 \mu_2) + 4 \mu_2 (-3 + \mathfrak{e}2)) + 4 \theta l \mu_2 \mathfrak{e}2) - \\
& \eta \theta p (8 \eta^7 (3 + 3 \mu_1 + 8 \mu_2) + \eta t (2 + 2 \mu_1^2 + \mu_1 (4 - 21 \mu_2) - 21 \mu_2 - 16 \mu_2^2) - \\
& \quad 2 \eta^6 (-10 - 37 \mu_1 - 27 \mu_1^2 - 24 \mu_1 \mu_2 + 56 \mu_2^2 - 4 \theta l (1 + \mu_1 + 4 \mu_2) + \\
& \quad 4 \eta t (2 + \theta l + 2 \mu_1 + \theta l \mu_1 + 4 \mu_2 + 4 \theta l \mu_2)) - \eta^2 \\
& \quad (4 \times (9 + 9 \mu_1^2 + 38 \mu_2 + 24 \mu_2^2 + 2 \mu_1 (9 + 19 \mu_2)) - 2 \theta l (7 + 9 \mathfrak{e}1 + \\
& \quad 4 \mu_2^2 (8 + 3 \mathfrak{e}1 - 4 \mathfrak{e}2) + \mu_1^2 (5 + 3 \mathfrak{e}1 - 2 \mathfrak{e}2) + 3 \mu_1 (4 + 4 \mathfrak{e}1 - \mathfrak{e}2) - \\
& \quad \mathfrak{e}2 - \mu_1 \mu_2 (-48 + 5 \mathfrak{e}1 + \mathfrak{e}2) + \mu_2 (52 + 25 \mathfrak{e}1 + \mathfrak{e}2)) + \\
& \quad \eta t (2 - 2 \mu_1^2 - \mu_2 - 17 \mu_1 \mu_2 - 16 \mu_2^2 + 2 \theta l (7 + 9 \mathfrak{e}1 + 4 \mu_2^2 \\
& \quad (8 + 3 \mathfrak{e}1 - 4 \mathfrak{e}2) + \mu_1^2 (5 + 3 \mathfrak{e}1 - 2 \mathfrak{e}2) + 3 \mu_1 (4 + 4 \mathfrak{e}1 - \mathfrak{e}2) - \\
& \quad \mathfrak{e}2 - \mu_1 \mu_2 (-48 + 5 \mathfrak{e}1 + \mathfrak{e}2) + \mu_2 (52 + 25 \mathfrak{e}1 + \mathfrak{e}2)) \left. \right) \left. \right) + \\
& \eta^3 (-2 \times (7 + 36 \mu_1^2 + 35 \mu_2 + 72 \mu_2^2 + \mu_1 (43 + 91 \mu_2)) + \\
& \quad \eta t (-4 - 108 \mu_1 - 104 \mu_1^2 + \mu_2 - 279 \mu_1 \mu_2 - 40 \mu_2^2 + \\
& \quad \theta l (-30 - 9 \mathfrak{e}1 - 4 \mu_2^2 (26 + 3 \mathfrak{e}1 - 19 \mathfrak{e}2) + \mu_1^2 (-74 + 6 \mathfrak{e}1 - 4 \mathfrak{e}2) + \\
& \quad \mu_1 (-104 - 3 \mathfrak{e}1 + \mu_2 (-272 + 61 \mathfrak{e}1 - 9 \mathfrak{e}2) - 3 \mathfrak{e}2) + \mathfrak{e}2 + \\
& \quad \mu_2 (-152 - 31 \mathfrak{e}1 + 3 \mathfrak{e}2)) \left. \right) + \theta l (30 + 9 \mathfrak{e}1 + 4 \mu_2^2 (26 + 3 \mathfrak{e}1 - \\
& \quad 19 \mathfrak{e}2) + \mu_2 (152 + 31 \mathfrak{e}1 - 3 \mathfrak{e}2) - \mathfrak{e}2 + \mu_1^2 (74 - 6 \mathfrak{e}1 + 4 \mathfrak{e}2) + \\
& \quad \mu_1 (104 + 3 \mathfrak{e}1 + 3 \mathfrak{e}2 + \mu_2 (272 - 61 \mathfrak{e}1 + 9 \mathfrak{e}2)) \left. \right) \left. \right) + \eta^5 \\
& (4 \eta t (-4 + 9 \mu_1^2 - 3 \mu_2 + 14 \mu_2^2 + \mu_1 (5 + 33 \mu_2)) + \\
& \quad 2 \times (-5 + 36 \mu_1^2 - 13 \mu_2 + 16 \mu_2^2 + \mu_1 (31 + 75 \mu_2)) + \\
& \quad \theta l (12 + 38 \mu_2 + 8 \mu_2 \mathfrak{e}2 + \mu_1^2 (48 + 9 \mathfrak{e}1 + 9 \mathfrak{e}2) +
\end{aligned}$$

$$\begin{aligned}
& \mu_1 (60 + 9 \mathfrak{E}_1 + 9 \mathfrak{E}_2 + 2 \mu_2 (55 + 14 \mathfrak{E}_1 + 14 \mathfrak{E}_2)) - \\
& \eta \mathfrak{t} \mathfrak{e} \mathfrak{l} (12 + 38 \mu_2 + 8 \mu_2 \mathfrak{E}_2 + \mu_1^2 (48 + 9 \mathfrak{E}_1 + 9 \mathfrak{E}_2) + \\
& \mu_1 (60 + 9 \mathfrak{E}_1 + 9 \mathfrak{E}_2 + 2 \mu_2 (55 + 14 \mathfrak{E}_1 + 14 \mathfrak{E}_2))) + \eta \\
& (\mathfrak{e} \mathfrak{l} (-2 + 9 \mathfrak{E}_1 + \mu_1^2 (-2 + 9 \mathfrak{E}_1 - \mathfrak{E}_2) - \mathfrak{E}_2 + 4 \mu_2^2 (2 + 3 \mathfrak{E}_1 + \mathfrak{E}_2) + \\
& \mu_2 (23 \mathfrak{E}_1 + 5 \times (2 + \mathfrak{E}_2)) + \mu_1 (18 \mathfrak{E}_1 + 23 \mu_2 \mathfrak{E}_1 - 2 \times (2 + \mathfrak{E}_2) + \\
& 5 \mu_2 (2 + \mathfrak{E}_2))) + \eta \mathfrak{t} (20 + 56 \mu_1 + 36 \mu_1^2 + 11 \mu_2 + \\
& 35 \mu_1 \mu_2 - 16 \mu_2^2 - \mathfrak{e} \mathfrak{l} (-2 + 9 \mathfrak{E}_1 + \mu_1^2 (-2 + 9 \mathfrak{E}_1 - \mathfrak{E}_2) - \\
& \mathfrak{E}_2 + 4 \mu_2^2 (2 + 3 \mathfrak{E}_1 + \mathfrak{E}_2) + \mu_2 (23 \mathfrak{E}_1 + 5 \times (2 + \mathfrak{E}_2)) + \\
& \mu_1 (18 \mathfrak{E}_1 + 23 \mu_2 \mathfrak{E}_1 - 2 \times (2 + \mathfrak{E}_2) + 5 \mu_2 (2 + \mathfrak{E}_2))) - 2 \\
& \eta^4 (-8 + \mu_1 + 9 \mu_1^2 - 92 \mu_2 - 68 \mu_1 \mu_2 - 160 \mu_2^2 - \mathfrak{e} \mathfrak{l} \\
& (9 + 2 \mu_2 (16 + \mathfrak{E}_1 + 2 \mathfrak{E}_2) - 4 \mu_2^2 (-6 + 5 \mathfrak{E}_2) + \\
& \mu_1^2 (55 + 3 \mathfrak{E}_1 + 8 \mathfrak{E}_2) + \mu_1 (64 + 3 \mathfrak{E}_1 + 8 \mathfrak{E}_2 + 2 \mu_2 (74 + 11 \mathfrak{E}_2))) + \\
& \eta \mathfrak{t} (-2 \times (4 + 7 \mu_1^2 + 13 \mu_2 + \mu_1 (11 + 29 \mu_2)) + \mathfrak{e} \mathfrak{l} (9 + \\
& 2 \mu_2 (16 + \mathfrak{E}_1 + 2 \mathfrak{E}_2) - 4 \mu_2^2 (-6 + 5 \mathfrak{E}_2) + \mu_1^2 (55 + 3 \mathfrak{E}_1 + 8 \mathfrak{E}_2) + \\
& \mu_1 (64 + 3 \mathfrak{E}_1 + 8 \mathfrak{E}_2 + 2 \mu_2 (74 + 11 \mathfrak{E}_2)))) - \\
& x^3 (-1 + \eta)^3 (-((-1 + \eta) \mathfrak{e} \mathfrak{p} (160 \eta^4 (3 + 3 \mu_1 + 8 \mu_2) + \eta \mathfrak{t} (-24 - \\
& 8 \mu_1 + 16 \mu_1^2 - 7 \mu_2 - 31 \mu_1 \mu_2 + 4 \mu_2^2) + \\
& 4 \times (9 + 18 \mu_1 + 9 \mu_1^2 + 33 \mu_2 + 33 \mu_1 \mu_2 + 32 \mu_2^2) - 40 \eta^3 (-10 - \\
& 37 \mu_1 - 27 \mu_1^2 - 10 \mu_2 - 34 \mu_1 \mu_2 + 28 \mu_2^2 + 8 \eta \mathfrak{t} (1 + \mu_1 + 2 \mu_2)) + \\
& 8 \eta (25 + 79 \mu_1 + 54 \mu_1^2 + 99 \mu_2 + 155 \mu_1 \mu_2 + 144 \mu_2^2 + \\
& 4 \eta \mathfrak{t} (-2 + 3 \mu_1 + 5 \mu_1^2 + \mu_2 + 19 \mu_1 \mu_2 + 7 \mu_2^2)) + \\
& 4 \eta^2 (49 + 364 \mu_1 + 315 \mu_1^2 + 65 \mu_2 + 561 \mu_1 \mu_2 + 40 \mu_2^2 + 2 \eta \mathfrak{t} \\
& (-40 - 22 \mu_1 + 18 \mu_1^2 - 55 \mu_2 + 81 \mu_1 \mu_2 + 70 \mu_2^2)))) + (-1 + \eta \mathfrak{t}) \\
& \mathfrak{e} \mathfrak{l} (38 + 72 \mu_1 + 34 \mu_1^2 + 54 \mu_2 + 70 \mu_1 \mu_2 + 16 \mu_2^2 + 160 \eta^4 \mathfrak{e} \mathfrak{p} \\
& (1 + \mu_1 + 4 \mu_2) + \mathfrak{e} \mathfrak{p} (\mu_1 (2 + 13 \mathfrak{E}_1 + \mu_2 (46 - 30 \mathfrak{E}_1 - 22 \mathfrak{E}_2) - 17 \mathfrak{E}_2) + \\
& \mu_1^2 (4 + 3 \mathfrak{E}_1 - 7 \mathfrak{E}_2) + 2 \times (-1 + 5 \mathfrak{E}_1 + 3 \mu_2 (5 + 3 \mathfrak{E}_1 - 5 \mathfrak{E}_2) - \\
& 5 \mathfrak{E}_2 - 4 \mu_2^2 (-4 + 7 \mathfrak{E}_2))) - 2 \eta^2 (12 \times (7 \mu_1^2 + 4 \mu_2 + \\
& 7 \mu_1 (1 + 4 \mu_2)) + \mathfrak{e} \mathfrak{p} (-66 + \mu_1^2 (-472 + 9 \mathfrak{E}_1 - 41 \mathfrak{E}_2) + \\
& \mu_1 (-538 + 9 \mathfrak{E}_1 + 2 \mu_2 (-599 + 66 \mathfrak{E}_1 - 44 \mathfrak{E}_2) - 41 \mathfrak{E}_2) - \\
& 2 \mu_2 (103 + 10 \mathfrak{E}_1 + 20 \mathfrak{E}_2) + 8 \mu_2^2 (-36 + 25 \mathfrak{E}_2))) + 2 \eta^3 \\
& (-12 \mu_1 (9 + 9 \mu_1 + 28 \mu_2) + 5 \mathfrak{e} \mathfrak{p} (8 + 2 \mu_2 (7 + 8 \mathfrak{E}_2) + \mu_1^2 (78 + 9 \mathfrak{E}_1 + \\
& 9 \mathfrak{E}_2) + \mu_1 (86 + 9 \mathfrak{E}_1 + 9 \mathfrak{E}_2 + 2 \mu_2 (83 + 14 \mathfrak{E}_1 + 14 \mathfrak{E}_2))) + \\
& \eta (80 + 140 \mu_1^2 + 65 \mu_2 + 12 \mu_2^2 + \mu_1 (220 + 321 \mu_2) + \\
& \mathfrak{e} \mathfrak{p} (2 \times (48 + 12 \mathfrak{E}_1 + 2 \mu_2^2 (110 + 3 \mathfrak{E}_1 - 85 \mathfrak{E}_2) + \\
& \mu_2 (229 + 38 \mathfrak{E}_1 - 30 \mathfrak{E}_2) - 8 \mathfrak{E}_2) + \mu_1^2 (278 - 33 \mathfrak{E}_1 + 7 \mathfrak{E}_2) - \\
& \mu_1 (-374 + 9 \mathfrak{E}_1 + 9 \mathfrak{E}_2 + \mu_2 (-914 + 304 \mathfrak{E}_1 + 24 \mathfrak{E}_2)))) + \\
& x^4 (-1 + \eta)^4 (-2 \times (-1 + \eta) \mathfrak{e} \mathfrak{p} (25 + 79 \mu_1 + 54 \mu_1^2 + 95 \mu_2 + 151 \\
& \mu_1 \mu_2 + 152 \mu_2^2 + 60 \eta^3 (3 + 3 \mu_1 + 8 \mu_2) + \\
& 4 \eta \mathfrak{t} (-2 + 2 \mu_1 + 4 \mu_1^2 + \mu_2 + 15 \mu_1 \mu_2 + 7 \mu_2^2) - 5 \eta^2 (-18 - \\
& 99 \mu_1 - 81 \mu_1^2 - 8 \mu_2 - 112 \mu_1 \mu_2 + 56 \mu_2^2 + 24 \eta \mathfrak{t} (1 + \mu_1 + 2 \mu_2)) + \\
& \eta (37 + 352 \mu_1 + 315 \mu_1^2 + 55 \mu_2 + 583 \mu_1 \mu_2 + 120 \mu_2^2 + \\
& 2 \eta \mathfrak{t} (-40 - 31 \mu_1 + 9 \mu_1^2 - 55 \mu_2 + 53 \mu_1 \mu_2 + 70 \mu_2^2))) + \\
& (-1 + \eta \mathfrak{t}) \mathfrak{e} \mathfrak{l} (28 - 4 \times (-7 + 20 \eta + 36 \eta^2) \mu_1^2 + 27 \mu_2 - 64 \eta \mu_2 +
\end{aligned}$$

$$\begin{aligned}
& 8 \mu^2 - \mu_1 \left( -56 - 107 \mu_2 + 80 \eta (1 + 4 \mu_2) + 16 \eta^2 (9 + 28 \mu_2) \right) + \theta p \\
& \left( 22 + 102 \mu_2 + 112 \mu_2^2 + 120 \eta^3 (1 + \mu_1 + 4 \mu_2) + 5 \mathfrak{z}_1 + 15 \mu_2 \mathfrak{z}_1 - 5 \mathfrak{z}_2 - \right. \\
& 19 \mu_2 \mathfrak{z}_2 - 88 \mu_2^2 \mathfrak{z}_2 + \mu_1^2 (68 - 9 \mathfrak{z}_1 + \mathfrak{z}_2) - \mu_1 (-90 + 4 \mathfrak{z}_1 + 4 \mathfrak{z}_2 + \\
& \mu_2 (-214 + 81 \mathfrak{z}_1 + 11 \mathfrak{z}_2)) + 2 \eta (29 + 2 \mu_2 (42 + 5 \mathfrak{z}_1 + 10 \mathfrak{z}_2) + \\
& \mu_1^2 (223 - 11 \mathfrak{z}_1 + 14 \mathfrak{z}_2) - 4 \mu_2^2 (-38 + 25 \mathfrak{z}_2) + \\
& \mu_1 (252 - 11 \mathfrak{z}_1 + 14 \mathfrak{z}_2 + \mu_2 (552 - 88 \mathfrak{z}_1 + 22 \mathfrak{z}_2)) \left. \right) + \\
& 5 \eta^2 (4 + 9 \mu_1^2 (12 + \mathfrak{z}_1 + \mathfrak{z}_2) + 2 \mu_2 (-5 + 12 \mathfrak{z}_2) + \mu_1 (112 + \\
& 9 \mathfrak{z}_1 + 9 \mathfrak{z}_2 + \mu_2 (222 + 28 \mathfrak{z}_1 + 28 \mathfrak{z}_2))) \left. \right) + x^5 (-1 + \eta)^5 \\
& (4 \times (-1 + \eta t) \theta l \left( (3 + 9 \eta) \mu_1^2 + 4 \mu_2 + \mu_1 (3 + 12 \mu_2 + \eta (9 + 28 \mu_2)) \right) + \\
& \theta p \left( -10 + 10 \theta l - 136 \mu_1 + 94 \theta l \mu_1 - 126 \mu_1^2 + 84 \theta l \mu_1^2 - 18 \mu_2 + \right. \\
& 26 \theta l \mu_2 - 242 \mu_1 \mu_2 + 202 \theta l \mu_1 \mu_2 - 80 \mu_2^2 + 64 \theta l \mu_2^2 + \\
& 48 \eta^3 (3 + 3 \mu_1 + 8 \mu_2) + 4 \eta t (8 + \mu_1 (8 - 5 \mu_2) + 11 \mu_2 - 14 \mu_2^2) - \\
& 4 \eta^2 (30 - 51 \mu_1 - 81 \mu_1^2 + 110 \mu_2 - 122 \mu_1 \mu_2 + 28 \mu_2^2 - \\
& 12 \theta l (1 + \mu_1 + 4 \mu_2) + 12 \eta t (2 + \theta l + 2 \mu_1 + \theta l \mu_1 + 4 \mu_2 + 4 \theta l \mu_2) \left. \right) - \\
& 7 \theta l \mu_1 \mathfrak{z}_1 - 7 \theta l \mu_1^2 \mathfrak{z}_1 + 4 \theta l \mu_2 \mathfrak{z}_1 - 44 \theta l \mu_1 \mu_2 \mathfrak{z}_1 + \\
& 3 \theta l \mu_1 \mathfrak{z}_2 + 3 \theta l \mu_1^2 \mathfrak{z}_2 + 8 \theta l \mu_2 \mathfrak{z}_2 - 40 \theta l \mu_2^2 \mathfrak{z}_2 + \\
& \eta t \theta l \left( -10 + \mu_1 (-94 + 7 \mathfrak{z}_1 + \mu_2 (-202 + 44 \mathfrak{z}_1) - 3 \mathfrak{z}_2) - 2 \mu_2 \right. \\
& (13 + 2 \mathfrak{z}_1 + 4 \mathfrak{z}_2) + 8 \mu_2^2 (-8 + 5 \mathfrak{z}_2) + \mu_1^2 (7 \mathfrak{z}_1 - 3 \times (28 + \mathfrak{z}_2)) \left. \right) + \\
& \eta (4 \eta t (16 + 37 \mu_2 + 14 \mu_2^2 + \mu_1 (16 + 5 \mu_2)) - 2 \times \\
& (7 + 99 \mu_1^2 - 37 \mu_2 - 96 \mu_2^2 + \mu_1 (106 + 123 \mu_2)) + \\
& \theta l (-8 - 82 \mu_2 + 48 \mu_2 \mathfrak{z}_2 + 9 \mu_1^2 (22 + \mathfrak{z}_1 + \mathfrak{z}_2) + \\
& \mu_1 (190 + 9 \mathfrak{z}_1 + 9 \mathfrak{z}_2 + \mu_2 (390 + 28 \mathfrak{z}_1 + 28 \mathfrak{z}_2))) - \\
& \eta t \theta l (-8 - 82 \mu_2 + 48 \mu_2 \mathfrak{z}_2 + 9 \mu_1^2 (22 + \mathfrak{z}_1 + \mathfrak{z}_2) + \\
& \mu_1 (190 + 9 \mathfrak{z}_1 + 9 \mathfrak{z}_2 + \mu_2 (390 + 28 \mathfrak{z}_1 + 28 \mathfrak{z}_2))) \left. \right) - \\
& x^2 (-1 + \eta)^2 \left( (-1 + \eta) \theta p (120 \eta^5 (3 + 3 \mu_1 + 8 \mu_2) - 10 \eta^4 (-42 - \right. \\
& 123 \mu_1 - 81 \mu_1^2 - 52 \mu_2 - 92 \mu_1 \mu_2 + 112 \mu_2^2 + 24 \eta t (1 + \mu_1 + 2 \mu_2)) - \\
& 2 \eta t (15 + 3 \mu_1^2 + 11 \mu_2 - 4 \mu_2^2 + 3 \mu_1 (6 + 5 \mu_2)) + \\
& 12 \eta^2 (25 + 79 \mu_1 + 54 \mu_1^2 + 103 \mu_2 + 159 \mu_1 \mu_2 + 136 \mu_2^2 + \\
& 4 \eta t (-2 + 4 \mu_1 + 6 \mu_1^2 + \mu_2 + 23 \mu_1 \mu_2 + 7 \mu_2^2)) + \\
& 4 \eta^3 (61 + 376 \mu_1 + 315 \mu_1^2 + 75 \mu_2 + 539 \mu_1 \mu_2 - 40 \mu_2^2 + \\
& 2 \eta t (-40 - 13 \mu_1 + 27 \mu_1^2 - 55 \mu_2 + 109 \mu_1 \mu_2 + 70 \mu_2^2)) + \\
& \eta (-\eta t (68 + 76 \mu_1 + 8 \mu_1^2 + 5 \mu_2 + 93 \mu_1 \mu_2 - 24 \mu_2^2) + \\
& 4 \times (27 + 54 \mu_1 + 27 \mu_1^2 + 104 \mu_2 + 104 \mu_1 \mu_2 + 88 \mu_2^2)) \left. \right) - \\
& (-1 + \eta t) \theta l (10 + 20 \mu_1 + 10 \mu_1^2 + 11 \mu_2 + 11 \mu_1 \mu_2 + 8 \mu_2^2 + \\
& 120 \eta^5 \theta p (1 + \mu_1 + 4 \mu_2) + 2 \eta (34 + 84 \mu_1 + 50 \mu_1^2 + 38 \mu_2 + \\
& 62 \mu_1 \mu_2 + 4 \mu_2^2 + \theta p (5 + 19 \mathfrak{z}_1 + \mu_2 (82 + 43 \mathfrak{z}_1 - 29 \mathfrak{z}_2) + \\
& \mu_1 (14 + 25 \mathfrak{z}_1 + \mu_2 (94 - 35 \mathfrak{z}_1 - 23 \mathfrak{z}_2) - 20 \mathfrak{z}_2) + \\
& 4 \mu_2^2 (16 + 3 \mathfrak{z}_1 - 18 \mathfrak{z}_2) + \mu_1^2 (9 + 6 \mathfrak{z}_1 - 9 \mathfrak{z}_2) - 11 \mathfrak{z}_2)) + \\
& \theta p (7 \mu_2 \mathfrak{z}_1 + 5 \times (-2 + \mathfrak{z}_1 - \mathfrak{z}_2) + 5 \mu_1^2 (-2 + \mathfrak{z}_1 - \mathfrak{z}_2) - 11 \mu_2 (2 + \mathfrak{z}_2) - \\
& 8 \mu_2^2 (2 + \mathfrak{z}_2) + \mu_1 (7 \mu_2 \mathfrak{z}_1 + 10 \times (-2 + \mathfrak{z}_1 - \mathfrak{z}_2) - 11 \mu_2 (2 + \mathfrak{z}_2))) + \\
& \eta^2 (76 + 196 \mu_1^2 + 49 \mu_2 + \mu_1 (272 + 321 \mu_2) - 3 \theta p \\
& (\mu_1^2 (-142 + 15 \mathfrak{z}_1 - 5 \mathfrak{z}_2) - 2 \times (26 + 7 \mathfrak{z}_1 + 2 \mu_2^2 \\
& (54 + 3 \mathfrak{z}_1 - 41 \mathfrak{z}_2) + \mu_2 (127 + 23 \mathfrak{z}_1 - 11 \mathfrak{z}_2) - 3 \mathfrak{z}_2) +
\end{aligned}$$

$$\begin{aligned}
& \mu_1 (-194 + \mathfrak{x}1 + \mathfrak{x}2 + 2 \mu_2 (-243 + 71 \mathfrak{x}1 + \mathfrak{x}2)) \Big) + \\
& 2 \eta^4 \Big( -8 \mu_1 (9 + 9 \mu_1 + 28 \mu_2) + 5 \wp \Big( 9 \mu_1^2 (7 + \mathfrak{x}1 + \mathfrak{x}2) + \\
& \quad 2 \times (5 + \mu_2 (13 + 6 \mathfrak{x}2)) + \\
& \quad \mu_1 (73 + 9 \mathfrak{x}1 + 9 \mathfrak{x}2 + 2 \mu_2 (69 + 14 \mathfrak{x}1 + 14 \mathfrak{x}2)) \Big) \Big) + \\
& 4 \eta^3 \Big( -4 \times \Big( 9 \mu_1^2 + 4 \mu_2 + 9 \mu_1 (1 + 4 \mu_2) \Big) + \wp \Big( 37 + 2 \mu_2 (61 + 5 \mathfrak{x}1 + \\
& \quad 10 \mathfrak{x}2) - 4 \mu_2^2 (-34 + 25 \mathfrak{x}2) + \mu_1^2 (249 + 2 \mathfrak{x}1 + 27 \mathfrak{x}2) + \\
& \quad \mu_1 (286 + 2 \mathfrak{x}1 + 27 \mathfrak{x}2 + \mu_2 (646 - 44 \mathfrak{x}1 + 66 \mathfrak{x}2)) \Big) \Big) \Big) + \\
& \times (-1 + \eta) \times \Big( 48 \eta^7 \wp (3 + 3 \mu_1 + 8 \mu_2) + \eta \mathfrak{t} \wp (6 + 6 \mu_1^2 + \mu_1 (12 - 5 \mu_2) - \\
& \quad 5 \mu_2 - 4 \mu_2^2) - 4 \eta^6 \wp (-18 - 99 \mu_1 - 81 \mu_1^2 + 22 \mu_2 - 82 \mu_1 \mu_2 + 140 \mu_2^2 - \\
& \quad 12 \wp (1 + \mu_1 + 4 \mu_2) + 12 \eta \mathfrak{t} (2 + \wp (1 + 2 \mu_1 + \wp (1 + 4 \mu_2 + 4 \wp (1 + 4 \mu_2)) - \\
& \quad \eta^2 (\wp (-\eta \mathfrak{t} (12 + 20 \mu_1^2 - 23 \mu_2 + 4 \mu_2^2 + \mu_1 (32 + 49 \mu_2)) + \\
& \quad 4 \times (27 + 27 \mu_1^2 + 109 \mu_2 + 80 \mu_2^2 + \mu_1 (54 + 109 \mu_2)) \Big) + \\
& \quad (-1 + \eta \mathfrak{t}) \wp (30 + 66 \mu_1^2 + 22 \mu_2 - 8 \mu_2^2 + 6 \mu_1 (16 + 9 \mu_2) + \\
& \quad \wp (\mu_1 (50 + 61 \mathfrak{x}1 + \mu_2 (238 - 50 \mathfrak{x}1 - 26 \mathfrak{x}2) - 29 \mathfrak{x}2) + \\
& \quad 2 \times (13 + 23 \mathfrak{x}1 + 4 \mu_2^2 (20 + 6 \mathfrak{x}1 - 15 \mathfrak{x}2) + \\
& \quad \mu_2 (119 + 59 \mathfrak{x}1 - 13 \mathfrak{x}2) - 7 \mathfrak{x}2) + 3 \mu_1^2 (8 + 5 \mathfrak{x}1 - 5 \mathfrak{x}2)) \Big) \Big) + \\
& \eta^3 \Big( -\wp (92 + 36 \times (9 + 8 \eta \mathfrak{t}) \mu_1^2 + 21 \times (20 + \eta \mathfrak{t}) \mu_2 + 4 \times \\
& \quad (176 + 47 \eta \mathfrak{t}) \mu_2^2 + \mu_1 (416 + 868 \mu_2 + 3 \eta \mathfrak{t} (96 + 319 \mu_2)) \Big) + \\
& \quad (-1 + \eta \mathfrak{t}) \wp (-24 - 84 \mu_1^2 - 11 \mu_2 + 4 \mu_2^2 - \mu_1 (108 + 107 \mu_2) + \\
& \quad \wp (\mu_1^2 (-290 + 27 \mathfrak{x}1 - 13 \mathfrak{x}2) + \mu_1 (-402 - 5 \mathfrak{x}1 + \\
& \quad 2 \mu_2 (-515 + 132 \mathfrak{x}1 - 8 \mathfrak{x}2) - 5 \mathfrak{x}2) - 2 \times (56 + 16 \mathfrak{x}1 + 2 \mu_2^2 \\
& \quad (106 + 9 \mathfrak{x}1 - 79 \mathfrak{x}2) + \mu_2 (279 + 54 \mathfrak{x}1 - 14 \mathfrak{x}2) - 4 \mathfrak{x}2) \Big) \Big) \Big) + \\
& \eta^4 \Big( 4 \times (-1 + \eta \mathfrak{t}) \wp (11 \mu_1^2 + 4 \mu_2 + 11 \mu_1 (1 + 4 \mu_2)) + \wp \\
& \quad \Big( 2 \times (27 - 99 \mu_1^2 + 343 \mu_2 + 632 \mu_2^2 + 9 \mu_1 (-8 + 15 \mu_2)) + \\
& \quad 4 \eta \mathfrak{t} (24 + 20 \mu_1^2 + 63 \mu_2 - 14 \mu_2^2 + \mu_1 (44 + 79 \mu_2)) + \\
& \quad \wp (82 - 8 \mu_2^2 (-32 + 25 \mathfrak{x}2) + \mu_2 (282 + 20 \mathfrak{x}1 + 40 \mathfrak{x}2) + \\
& \quad \mu_1^2 (524 + 17 \mathfrak{x}1 + 67 \mathfrak{x}2) + \mu_1 (606 + 17 \mathfrak{x}1 - 22 \mu_2 (-63 + 2 \mathfrak{x}1 - \\
& \quad 8 \mathfrak{x}2) + 67 \mathfrak{x}2) \Big) - \eta \mathfrak{t} \wp (82 - 8 \mu_2^2 (-32 + 25 \mathfrak{x}2) + \\
& \quad \mu_2 (282 + 20 \mathfrak{x}1 + 40 \mathfrak{x}2) + \mu_1^2 (524 + 17 \mathfrak{x}1 + 67 \mathfrak{x}2) + \\
& \quad \mu_1 (606 + 17 \mathfrak{x}1 - 22 \mu_2 (-63 + 2 \mathfrak{x}1 - 8 \mathfrak{x}2) + 67 \mathfrak{x}2) \Big) \Big) \Big) + \eta \\
& \quad (\eta \mathfrak{t} \wp (46 + 38 \mu_1^2 + 17 \mu_2 - 36 \mu_2^2 + 7 \mu_1 (12 + 7 \mu_2)) - \\
& \quad (-1 + \eta \mathfrak{t}) \wp (6 + 12 \mu_1 + 6 \mu_1^2 - 5 \mu_2 - 5 \mu_1 \mu_2 - 4 \mu_2^2 + \\
& \quad 2 \wp (-6 + 7 \mathfrak{x}1 + 3 \mu_2 (-2 + 5 \mathfrak{x}1 - \mathfrak{x}2) - 3 \mathfrak{x}2 + \\
& \quad \mu_1 (14 \mathfrak{x}1 + 3 \mu_2 (-2 + 5 \mathfrak{x}1 - \mathfrak{x}2) - 6 \times (2 + \mathfrak{x}2)) + \\
& \quad \mu_1^2 (7 \mathfrak{x}1 - 3 \times (2 + \mathfrak{x}2)) + \mu_2^2 (6 \mathfrak{x}1 - 2 \times (2 + \mathfrak{x}2)) \Big) \Big) \Big) + \\
& \eta^5 \Big( 4 \times (-1 + \eta \mathfrak{t}) \wp \mu_1 (9 + 9 \mu_1 + 28 \mu_2) + \wp (-70 + 236 \mu_1 + \\
& \quad 306 \mu_1^2 - 126 \mu_2 + 706 \mu_1 \mu_2 + 320 \mu_2^2 + \\
& \quad 4 \eta \mathfrak{t} (-16 + 36 \mu_1^2 - 7 \mu_2 + 70 \mu_2^2 + \mu_1 (20 + 137 \mu_2)) + \\
& \quad \wp (56 + 166 \mu_2 + 48 \mu_2 \mathfrak{x}2 + 45 \mu_1^2 (6 + \mathfrak{x}1 + \mathfrak{x}2) + \\
& \quad \mu_1 (326 + 45 \mathfrak{x}1 + 45 \mathfrak{x}2 + 2 \mu_2 (303 + 70 \mathfrak{x}1 + 70 \mathfrak{x}2)) \Big) - \\
& \quad \eta \mathfrak{t} \wp (56 + 166 \mu_2 + 48 \mu_2 \mathfrak{x}2 + 45 \mu_1^2 (6 + \mathfrak{x}1 + \mathfrak{x}2) + \\
& \quad \mu_1 (326 + 45 \mathfrak{x}1 + 45 \mathfrak{x}2 + 2 \mu_2 (303 + 70 \mathfrak{x}1 + 70 \mathfrak{x}2)) \Big) \Big) \Big) \Big) + \\
& w^3 (-1 + \eta)^3 \Big( 6 x^7 (-1 + \eta)^8 \wp (\eta - \eta \mathfrak{t} + 4 \mu_1) (3 + 3 \mu_1 + 4 \mu_2) -
\end{aligned}$$



$$\begin{aligned}
& x^6 (-1 + \eta)^6 \left( 6 \times (-1 + \eta) \operatorname{erf} \left( 29 + 101 \mu_1 + 72 \mu_1^2 + 87 \mu_2 + 119 \mu_1 \mu_2 + \right. \right. \\
& \quad \left. \left. 7 \eta^2 (3 + 3 \mu_1 + 4 \mu_2) + \eta t (-17 - 17 \mu_1 - 18 \mu_2 + 10 \mu_1 \mu_2 + 28 \mu_2^2) + \right. \right. \\
& \quad \left. \left. \eta (17 + 101 \mu_1 + 84 \mu_1^2 + 18 \mu_2 + 102 \mu_1 \mu_2 - \right. \right. \\
& \quad \left. \left. 28 \mu_2^2 - 7 \eta t (3 + 3 \mu_1 + 4 \mu_2) \right) \right) - (-1 + \eta t) \operatorname{erf} \\
& \quad \left( 28 - 52 \mu_1 - 80 \mu_1^2 + 11 \mu_2 - 325 \mu_1 \mu_2 + 8 \mu_2^2 + \operatorname{erf} \left( 146 + 5 \mu_1 + \right. \right. \\
& \quad \left. \left. \mu_2^2 (48 - 88 \mu_2) + 3 \mu_2 (170 + 5 \mu_1 - \mu_2) - 5 \mu_2 + 6 \mu_1 (49 + \mu_1 + \mu_2) + \right. \right. \\
& \quad \left. \left. \mu_1^2 (148 + \mu_1 + 11 \mu_2) + \mu_1 \mu_2 (462 - 25 \mu_1 + 45 \mu_2) \right) \right) + \\
& \eta \operatorname{erf} \left( -6 \eta^8 (3 + 3 \mu_1 + 4 \mu_2) + 3 \eta t \mu_2 (11 + 11 \mu_1 + 8 \mu_2) - 3 \eta \eta t \right. \\
& \quad \left( 4 + 28 \mu_1^2 + \mu_1 (32 - 75 \mu_2) - 75 \mu_2 - 80 \mu_2^2 \right) - 2 \eta^6 \\
& \quad \left( 123 + 180 \mu_1^2 + 251 \mu_2 - 324 \mu_2^2 + 3 \mu_1 (101 + 73 \mu_2) + \right. \\
& \quad \left. 6 \eta t (-7 - 7 \mu_2 + 14 \mu_2^2 + \mu_1 (-7 + 5 \mu_2)) \right) + 6 \eta^7 \\
& \quad \left( \eta t (3 + 3 \mu_1 + 4 \mu_2) - 2 \times (6 \mu_1^2 + \mu_1 (13 + 3 \mu_2) + 7 \times (1 + \mu_2 - 2 \mu_2^2)) \right) + \\
& \eta^5 \left( -4 \times (59 + 99 \mu_1^2 + 267 \mu_2 + 110 \mu_2^2 + \mu_1 (158 + 291 \mu_2)) - \right. \\
& \quad \operatorname{erf} \left( 162 + 9 \mu_1 + 4 \mu_2^2 (14 + 3 \mu_1 - 19 \mu_2) - \mu_2 + 2 \mu_1 (163 + 9 \mu_1 + 9 \mu_2) + \right. \\
& \quad \left. \mu_2 (582 + 31 \mu_1 + 13 \mu_2) + \mu_1^2 (164 + 9 \mu_1 + 19 \mu_2) + \right. \\
& \quad \left. \mu_1 \mu_2 (534 + 7 \mu_1 + 77 \mu_2) \right) + \eta t \left( 84 - 72 \mu_1 - 156 \mu_1^2 - 21 \mu_2 - \right. \\
& \quad \left. 813 \mu_1 \mu_2 - 352 \mu_2^2 + \operatorname{erf} \left( 162 + 9 \mu_1 + 4 \mu_2^2 (14 + 3 \mu_1 - 19 \mu_2) - \right. \right. \\
& \quad \left. \left. \mu_2 + 2 \mu_1 (163 + 9 \mu_1 + 9 \mu_2) + \mu_2 (582 + 31 \mu_1 + 13 \mu_2) + \right. \right. \\
& \quad \left. \left. \mu_1^2 (164 + 9 \mu_1 + 19 \mu_2) + \mu_1 \mu_2 (534 + 7 \mu_1 + 77 \mu_2) \right) \right) + \eta^4 \\
& \quad \left( 178 + 394 \mu_1 + 52 \eta t \mu_1 + 216 \mu_1^2 + 52 \eta t \mu_1^2 + 28 \mu_2 - 229 \eta t \mu_2 - \right. \\
& \quad \left. 172 \mu_1 \mu_2 - 509 \eta t \mu_1 \mu_2 - 1112 \mu_2^2 - 120 \eta t \mu_2^2 + \right. \\
& \quad \left. (-1 + \eta t) \operatorname{erf} \left( 398 + 69 \mu_1 + 4 \mu_2^2 (82 + 33 \mu_1 - 37 \mu_2) + 19 \mu_2 + \right. \right. \\
& \quad \left. \left. \mu_1^2 (440 + 51 \mu_1 + 61 \mu_2) + \mu_2 (1546 + 235 \mu_1 + 129 \mu_2) + \right. \right. \\
& \quad \left. \left. \mu_1 (838 + 120 \mu_1 + 80 \mu_2 + \mu_2 (1594 + 107 \mu_1 + 281 \mu_2)) \right) \right) + \eta^3 \\
& \quad \left( 4 \times (80 + 197 \mu_1 + 117 \mu_1^2 + 308 \mu_2 + 320 \mu_1 \mu_2 + 124 \mu_2^2) - \right. \\
& \quad \operatorname{erf} \left( 310 + 111 \mu_1 + 4 \mu_2^2 (122 + 57 \mu_1 - 17 \mu_2) + 41 \mu_2 + \right. \\
& \quad \left. 2 \mu_1 (349 + 93 \mu_1 + 53 \mu_2) + \mu_1^2 (388 + 75 \mu_1 + 65 \mu_2) + \right. \\
& \quad \left. \mu_2 (1346 + 377 \mu_1 + 219 \mu_2) + \mu_1 \mu_2 (1586 + 193 \mu_1 + 331 \mu_2) \right) + \\
& \eta t \left( -90 + 230 \mu_1 + 320 \mu_1^2 - 228 \mu_2 + 812 \mu_1 \mu_2 + 112 \mu_2^2 + \right. \\
& \quad \operatorname{erf} \left( 310 + 111 \mu_1 + 4 \mu_2^2 (122 + 57 \mu_1 - 17 \mu_2) + 41 \mu_2 + \right. \\
& \quad \left. 2 \mu_1 (349 + 93 \mu_1 + 53 \mu_2) + \mu_1^2 (388 + 75 \mu_1 + 65 \mu_2) + \mu_2 \right. \\
& \quad \left. (1346 + 377 \mu_1 + 219 \mu_2) + \mu_1 \mu_2 (1586 + 193 \mu_1 + 331 \mu_2) \right) + \eta^2 \\
& \quad \left( 86 + 230 \mu_1 + 144 \mu_1^2 + 418 \mu_2 + 530 \mu_1 \mu_2 + 240 \mu_2^2 - \right. \\
& \quad \operatorname{erf} \left( 74 + 51 \mu_1 + 21 \mu_2 + 4 \mu_2^2 (54 + 27 \mu_1 + \mu_2) + \right. \\
& \quad \left. \mu_1^2 (112 + 33 \mu_1 + 23 \mu_2) + \mu_2 (382 + 173 \mu_1 + 103 \mu_2) + \right. \\
& \quad \left. \mu_1 (186 + 84 \mu_1 + 44 \mu_2 + \mu_2 (526 + 93 \mu_1 + 127 \mu_2)) \right) + \\
& \eta t \left( -4 \times (21 + 33 \mu_1^2 + \mu_1 (54 - 78 \mu_2) - 28 \mu_2 - 66 \mu_2^2) + \right. \\
& \quad \operatorname{erf} \left( 74 + 51 \mu_1 + 21 \mu_2 + 4 \mu_2^2 (54 + 27 \mu_1 + \mu_2) + \right. \\
& \quad \left. \mu_1^2 (112 + 33 \mu_1 + 23 \mu_2) + \mu_2 (382 + 173 \mu_1 + 103 \mu_2) + \right. \\
& \quad \left. \mu_1 (186 + 84 \mu_1 + 44 \mu_2 + \mu_2 (526 + 93 \mu_1 + 127 \mu_2)) \right) + \eta^4 + \\
& x^5 (-1 + \eta)^5 \left( (-1 + \eta) \operatorname{erf} \left( 126 \eta^3 (3 + 3 \mu_1 + 4 \mu_2) + \eta t (-190 + \right. \right. \\
& \quad \left. \left. 144 \mu_1^2 - 103 \mu_2 + 508 \mu_2^2 + \mu_1 (-46 + 633 \mu_2)) + \right. \right. \\
& \quad \left. \left. 2 \times (235 + 414 \mu_1^2 + 801 \mu_2 + 312 \mu_2^2 + \mu_1 (649 + 905 \mu_2)) + \right. \right.
\end{aligned}$$

$$\begin{aligned}
& 2 \eta \left( 609 + 1296 \mu_1^2 + 1610 \mu_2 - 408 \mu_2^2 + 3 \mu_1 (635 + 674 \mu_2) + \right. \\
& \quad \left. 18 \eta t (-17 - 18 \mu_2 + 28 \mu_2^2 + \mu_1 (-17 + 10 \mu_2)) \right) - \\
& 18 \eta^2 \left( 7 \eta t (3 + 3 \mu_1 + 4 \mu_2) - 2 \times (17 + 42 \mu_1^2 + 18 \mu_2 - \right. \\
& \quad \left. 28 \mu_2^2 + \mu_1 (59 + 46 \mu_2)) \right) - (-1 + \eta t) \theta l \\
& (-2 \times (-52 + 20 \mu_1^2 + 53 \mu_2 + 100 \mu_2^2 + \mu_1 (-32 + 261 \mu_2)) + \\
& \quad \text{op} (366 + 61 \mu_1 + 4 \mu_2^2 (78 + 27 \mu_1 - 43 \mu_2) + 11 \mu_2 + \\
& \quad \mu_1^2 (408 + 35 \mu_1 + 45 \mu_2) + \mu_2 (1402 + 203 \mu_1 + 97 \mu_2) + \\
& \quad \mu_1 (774 + 96 \mu_1 + 56 \mu_2 + \mu_2 (1450 + 43 \mu_1 + 217 \mu_2))) + \\
& \quad \eta (136 - 276 \mu_1 - 412 \mu_1^2 + 39 \mu_2 - 1865 \mu_1 \mu_2 + 28 \mu_2^2 + \\
& \quad 2 \text{op} (446 + 17 \mu_1 + 2 \mu_2^2 (74 + 3 \mu_1 - 129 \mu_2) + \\
& \quad \mu_2 (1566 + 53 \mu_1 - \mu_2) - 13 \mu_2 + \mu_1^2 (452 + 7 \mu_1 + 37 \mu_2) + \\
& \quad \mu_1 (898 + 24 \mu_1 + 24 \mu_2 + \mu_2 (1422 - 59 \mu_1 + 151 \mu_2))) + \\
& x^4 (-1 + \eta)^4 \left( - \left( (-1 + \eta) \text{op} (210 \eta^4 (3 + 3 \mu_1 + 4 \mu_2) - 30 \eta^3 (-51 - 135 \right. \right. \\
& \quad \left. \mu_1 - 84 \mu_1^2 - 54 \mu_2 - 82 \mu_1 \mu_2 + 84 \mu_2^2 + 7 \eta t (3 + 3 \mu_1 + 4 \mu_2)) + \right. \\
& \quad 10 \eta^2 (348 + 996 \mu_1 + 648 \mu_1^2 + 827 \mu_2 + 951 \mu_1 \mu_2 - 408 \mu_2^2 + \\
& \quad 9 \eta t (-17 - 17 \mu_1 - 18 \mu_2 + 10 \mu_1 \mu_2 + 28 \mu_2^2)) + \\
& \quad 2 \times (191 + 497 \mu_1 + 306 \mu_1^2 + 789 \mu_2 + 901 \mu_1 \mu_2 + 496 \mu_2^2 + \\
& \quad \eta t (-85 + 61 \mu_1 + 146 \mu_1^2 + 103 \mu_2 + 527 \mu_1 \mu_2 + 344 \mu_2^2)) + \\
& \quad \eta (2464 + 6604 \mu_1 + 4140 \mu_1^2 + 8086 \mu_2 + 8878 \mu_1 \mu_2 + 2120 \mu_2^2 + \eta t \\
& \quad \left. (-946 - 214 \mu_1 + 732 \mu_1^2 - 499 \mu_2 + 3405 \mu_1 \mu_2 + 2552 \mu_2^2)) \right) + \\
& (-1 + \eta t) \theta l (88 + 292 \mu_1 + 204 \mu_1^2 - 342 \mu_2 - 294 \mu_1 \mu_2 - 448 \mu_2^2 + \\
& \quad \text{op} (294 + 107 \mu_1 + 8 \mu_2^2 (60 + 27 \mu_1 - 10 \mu_2) + 37 \mu_2 + \\
& \quad \mu_1^2 (372 + 67 \mu_1 + 57 \mu_2) + \mu_2 (1274 + 361 \mu_1 + 203 \mu_2) + \\
& \quad \mu_1 (666 + 174 \mu_1 + 94 \mu_2 + \mu_2 (1514 + 161 \mu_1 + 299 \mu_2))) + \\
& \quad \eta^2 (264 - 584 \mu_1 - 848 \mu_1^2 + 46 \mu_2 - 4210 \mu_1 \mu_2 + 32 \mu_2^2 + \\
& \quad 5 \text{op} (454 + 19 \mu_1 + 4 \mu_2^2 (38 + 3 \mu_1 - 63 \mu_2) - 11 \mu_2 + \\
& \quad \mu_2 (1602 + 61 \mu_1 + 7 \mu_2) + \mu_1^2 (460 + 11 \mu_1 + 41 \mu_2) + \\
& \quad \mu_1 (914 + 30 \mu_1 + 30 \mu_2 + \mu_2 (1458 - 43 \mu_1 + 167 \mu_2))) + \\
& \quad \eta (4 \times (108 + 115 \mu_1 + 7 \mu_1^2 - 90 \mu_2 - 604 \mu_1 \mu_2 - 188 \mu_2^2) + \\
& \quad \text{op} (1862 + 313 \mu_1 + 4 \mu_2^2 (394 + 141 \mu_1 - 209 \mu_2) + 63 \mu_2 + \\
& \quad \mu_1^2 (2072 + 191 \mu_1 + 241 \mu_2) + \mu_2 (7154 + 1047 \mu_1 + 517 \mu_2) + \mu_1 \\
& \quad (3934 + 504 \mu_1 + 304 \mu_2 + \mu_2 (7394 + 279 \mu_1 + 1149 \mu_2))) + \\
& x^3 (-1 + \eta)^3 \left( -2 \times (-1 + \eta) \text{op} (43 + 115 \mu_1 + 72 \mu_1^2 + 209 \mu_2 + \right. \\
& \quad 265 \mu_1 \mu_2 + 120 \mu_2^2 + 105 \eta^5 (3 + 3 \mu_1 + 4 \mu_2) + \\
& \quad \eta t (-20 + 40 \mu_1^2 + 297 \mu_2 + 348 \mu_2^2 + \mu_1 (20 + 373 \mu_2)) - \\
& \quad 15 \eta^4 (7 \eta t (3 + 3 \mu_1 + 4 \mu_2) - \\
& \quad 4 \times (17 + 21 \mu_1^2 + 18 \mu_2 - 28 \mu_2^2 + 2 \mu_1 (19 + 9 \mu_2))) + \\
& \quad 10 \eta^3 (261 + 432 \mu_1^2 + 566 \mu_2 - 408 \mu_2^2 + 99 \mu_1 (7 + 6 \mu_2) + \\
& \quad 6 \eta t (-17 - 18 \mu_2 + 28 \mu_2^2 + \mu_1 (-17 + 10 \mu_2))) + \\
& \quad \eta^2 (2578 + 4140 \mu_1^2 + 8162 \mu_2 + 1120 \mu_2^2 + \mu_1 (6718 + 8706 \mu_2) + \\
& \quad \eta t (-942 + 744 \mu_1^2 - 483 \mu_2 + 2564 \mu_2^2 + 9 \mu_1 (-22 + 405 \mu_2))) + \\
& \quad 2 \eta (4 \times (97 + 153 \mu_1^2 + 399 \mu_2 + 232 \mu_2^2 + \mu_1 (250 + 451 \mu_2)) + \\
& \quad \eta t (245 \mu_1^2 + 71 \mu_1 (1 + 16 \mu_2) + 2 \times (-87 + 95 \mu_2 + 338 \mu_2^2))) +
\end{aligned}$$

$$\begin{aligned}
& (-1 + \eta t) \, \text{el} \left( 6 \times (2 + 14 \mu_1^2 + \mu_1 (16 - 43 \mu_2) - 43 \mu_2 - 44 \mu_2^2) + \right. \\
& 2 \eta^3 (128 - 308 \mu_1 - 436 \mu_1^2 + 7 \mu_2 - 2345 \mu_1 \mu_2 + 4 \mu_2^2 + \\
& 10 \, \text{op} (154 + 7 \, \text{el} + \mu_2^2 (52 + 6 \, \text{el} - 82 \, \text{el}_2) - 3 \, \text{el}_2 + \\
& \mu_2 (546 + 23 \, \text{el} + 5 \, \text{el}_2) + 2 \mu_1 (155 + 6 \, \text{el} + 6 \, \text{el}_2) + \\
& \mu_1^2 (156 + 5 \, \text{el} + 15 \, \text{el}_2) + \mu_1 \mu_2 (498 - 9 \, \text{el} + 61 \, \text{el}_2) \left. \right) + \\
& \text{op} (74 + 51 \, \text{el} + 21 \, \text{el}_2 + 4 \mu_2^2 (54 + 27 \, \text{el} + \, \text{el}_2) + \mu_1^2 \\
& (112 + 33 \, \text{el} + 23 \, \text{el}_2) + \mu_2 (382 + 173 \, \text{el} + 103 \, \text{el}_2) + \\
& \mu_1 (186 + 84 \, \text{el} + 44 \, \text{el}_2 + \mu_2 (526 + 93 \, \text{el} + 127 \, \text{el}_2) \left. \right) + \\
& 2 \eta (160 + 614 \mu_1 + 454 \mu_1^2 - 401 \mu_2 - 353 \mu_1 \mu_2 - 588 \mu_2^2 + \\
& 2 \, \text{op} (298 + 108 \, \text{el} + \mu_2^2 (482 + 219 \, \text{el} - 77 \, \text{el}_2) + 38 \, \text{el}_2 + \\
& \mu_1^2 (376 + 69 \, \text{el} + 59 \, \text{el}_2) + \mu_2 (1292 + 365 \, \text{el} + 207 \, \text{el}_2) + \\
& \mu_1 (674 + 177 \, \text{el} + 97 \, \text{el}_2 + \mu_2 (1532 + 169 \, \text{el} + 307 \, \text{el}_2) \left. \right) \left. \right) + \\
& 2 \eta^2 (6 \times (56 + 27 \mu_1^2 + \mu_1 (83 - 343 \mu_2) - 37 \mu_2 - 88 \mu_2^2) + \\
& \text{op} (1894 + 321 \, \text{el} + 4 \mu_2^2 (398 + 147 \, \text{el} - 203 \, \text{el}_2) + 71 \, \text{el}_2 + \\
& \mu_1^2 (2104 + 207 \, \text{el} + 257 \, \text{el}_2) + \mu_2 (7298 + 1079 \, \text{el} + 549 \, \text{el}_2) + \mu_1 \\
& (3998 + 528 \, \text{el} + 328 \, \text{el}_2 + \mu_2 (7538 + 343 \, \text{el} + 1213 \, \text{el}_2) \left. \right) \left. \right) \left. \right) - \\
& x^2 (-1 + \eta)^2 (126 \eta^7 \, \text{op} (3 + 3 \mu_1 + 4 \mu_2) - 3 \, \text{el} \mu_2 (11 + 11 \mu_1 + 8 \mu_2) + \\
& 3 \eta t \, \text{el} \mu_2 (11 + 11 \mu_1 + 8 \mu_2) - 6 \eta t \, \text{op} \\
& (6 + 4 \mu_1^2 + 75 \mu_2 + 68 \mu_2^2 + \mu_1 (10 + 79 \mu_2) \left. \right) + 2 \eta^5 \, \text{op} \\
& (2484 \mu_1^2 + 33 \mu_1 (118 + 109 \mu_2) + 5 \times (282 + 709 \mu_2 - 564 \mu_2^2) + \\
& 18 \eta t (-32 - 31 \mu_2 + 70 \mu_2^2 + \mu_1 (-32 + 25 \mu_2) \left. \right) - 18 \eta^6 \, \text{op} (7 \eta t \\
& (3 + 3 \mu_1 + 4 \mu_2) - 2 \times (32 + 42 \mu_1^2 + 31 \mu_2 - 70 \mu_2^2 + \mu_1 (74 + 31 \mu_2) \left. \right) \left. \right) - \\
& 2 \eta^2 (\text{op} (3 \times (351 + 540 \mu_1^2 + 1405 \mu_2 + 744 \mu_2^2 + \mu_1 (891 + 1541 \mu_2) \left. \right) + \\
& \eta t (-446 + 622 \mu_1^2 - 257 \mu_2 + 1032 \mu_2^2 + \mu_1 (176 + 2623 \mu_2) \left. \right) \left. \right) + \\
& (-1 + \eta t) \, \text{el} (188 + 790 \mu_1 + 602 \mu_1^2 - 289 \mu_2 - 265 \mu_1 \mu_2 - \\
& 504 \mu_2^2 + 3 \, \text{op} (302 + 109 \, \text{el} + \mu_2^2 (484 + 222 \, \text{el} - 74 \, \text{el}_2) + 39 \, \text{el}_2 + \\
& 2 \mu_1 (341 + 90 \, \text{el} + 50 \, \text{el}_2) + \mu_1^2 (380 + 71 \, \text{el} + 61 \, \text{el}_2) + \mu_2 \\
& (1310 + 369 \, \text{el} + 211 \, \text{el}_2) + \mu_1 \mu_2 (1550 + 177 \, \text{el} + 315 \, \text{el}_2) \left. \right) \left. \right) - \\
& \eta (-4 \eta t \, \text{op} (53 + 20 \mu_1^2 + \mu_1 (73 - 397 \mu_2) - 277 \mu_2 - 378 \mu_2^2) + \\
& 6 \, \text{op} (43 + 72 \mu_1^2 + 209 \mu_2 + 120 \mu_2^2 + 5 \mu_1 (23 + 53 \mu_2) \left. \right) + \\
& 3 \times (-1 + \eta t) \, \text{el} (4 \times (6 + 23 \mu_1^2 + \mu_1 (29 - 25 \mu_2) - 27 \mu_2 - 32 \mu_2^2) + \\
& \text{op} (74 + 51 \, \text{el} + 21 \, \text{el}_2 + 4 \mu_2^2 (54 + 27 \, \text{el} + \, \text{el}_2) + \\
& \mu_1^2 (112 + 33 \, \text{el} + 23 \, \text{el}_2) + \mu_2 (382 + 173 \, \text{el} + 103 \, \text{el}_2) + \\
& \mu_1 (186 + 84 \, \text{el} + 44 \, \text{el}_2 + \mu_2 (526 + 93 \, \text{el} + 127 \, \text{el}_2) \left. \right) \left. \right) + \eta^4 \\
& (2 \, \text{op} (517 + 900 \mu_1^2 + 3883 \mu_2 + 4200 \mu_2^2 + \mu_1 (1417 + 4379 \mu_2) + \\
& \eta t (-173 + 756 \mu_1^2 + 343 \mu_2 + 1316 \mu_2^2 + \mu_1 (583 + 3435 \mu_2) \left. \right) \left. \right) - \\
& (-1 + \eta t) \, \text{el} (124 - 324 \mu_1 - 448 \mu_1^2 - 9 \mu_2 - 2585 \mu_1 \mu_2 - \\
& 8 \mu_2^2 + 5 \, \text{op} (470 + 23 \, \text{el} + 8 \mu_2^2 (20 + 3 \, \text{el} - 30 \, \text{el}_2) - 7 \, \text{el}_2 + \\
& \mu_2 (1674 + 77 \, \text{el} + 23 \, \text{el}_2) + \mu_1^2 (476 + 19 \, \text{el} + 49 \, \text{el}_2) + \\
& \mu_1 (946 + 42 \, \text{el} + 42 \, \text{el}_2 + \mu_2 (1530 - 11 \, \text{el} + 199 \, \text{el}_2) \left. \right) \left. \right) \left. \right) - 2 \eta^3 \\
& (\text{op} (1510 + 2304 \mu_1^2 + 3396 \mu_2 - 2472 \mu_2^2 + \mu_1 (3814 + 3116 \mu_2) + \\
& \eta t (-404 + 162 \mu_1^2 - 989 \mu_2 + 584 \mu_2^2 + 11 \mu_1 (-22 + 21 \mu_2) \left. \right) \left. \right) + \\
& (-1 + \eta t) \, \text{el} (2 \times (116 + 217 \mu_1 + 101 \mu_1^2 - 58 \mu_2 - 768 \mu_1 \mu_2 - 164 \mu_2^2) +
\end{aligned}$$

$$\begin{aligned}
& \left( \begin{aligned} & \text{op} \left( 1926 + 329 \, \mathfrak{x}1 + 4 \, \mu2^2 \left( 402 + 153 \, \mathfrak{x}1 - 197 \, \mathfrak{x}2 \right) + 79 \, \mathfrak{x}2 + \right. \\ & \quad \mu1^2 \left( 2136 + 223 \, \mathfrak{x}1 + 273 \, \mathfrak{x}2 \right) + \mu2 \left( 7442 + 1111 \, \mathfrak{x}1 + 581 \, \mathfrak{x}2 \right) + \mu1 \\ & \quad \left. \left( 4062 + 552 \, \mathfrak{x}1 + 352 \, \mathfrak{x}2 + \mu2 \left( 7682 + 407 \, \mathfrak{x}1 + 1277 \, \mathfrak{x}2 \right) \right) \right) \right) + \\ & \times (-1 + \eta) \times \left( \begin{aligned} & 42 \, \eta^8 \text{op} \left( 3 + 3 \, \mu1 + 4 \, \mu2 \right) - 3 \, \eta \mathfrak{t} \text{op} \left( 4 + 4 \, \mu1^2 + 27 \, \mu2 + \right. \\ & \quad 20 \, \mu2^2 + \mu1 \left( 8 + 27 \, \mu2 \right) \right) - 6 \, \eta^7 \text{op} \left( -81 - 84 \, \mu1^2 - 80 \, \mu2 + \right. \\ & \quad \left. 168 \, \mu2^2 + 7 \, \eta \mathfrak{t} \left( 3 + 3 \, \mu1 + 4 \, \mu2 \right) - \mu1 \left( 165 + 52 \, \mu2 \right) \right) + 2 \, \eta^6 \text{op} \\ & \left( 651 + 1044 \, \mu1^2 + 1462 \, \mu2 - 1536 \, \mu2^2 + 3 \, \mu1 \left( 565 + 462 \, \mu2 \right) + \right. \\ & \quad \left. 3 \, \eta \mathfrak{t} \left( -81 - 80 \, \mu2 + 168 \, \mu2^2 + \mu1 \left( -81 + 60 \, \mu2 \right) \right) \right) - 3 \\ & \eta \left( (-1 + \eta \mathfrak{t}) \, \mathfrak{el} \left( 4 + 4 \, \mu1^2 + 5 \, \mu2 + 4 \, \mu2^2 + \mu1 \left( 8 + 5 \, \mu2 \right) \right) + \right. \\ & \quad \left. \eta \mathfrak{t} \text{op} \left( 4 - 24 \, \mu1^2 + 209 \, \mu2 + 204 \, \mu2^2 + \mu1 \left( -20 + 217 \, \mu2 \right) \right) \right) - \eta^2 \\ & \left( 2 \text{op} \left( 3 \times \left( 43 + 72 \, \mu1^2 + 209 \, \mu2 + 120 \, \mu2^2 + 5 \, \mu1 \left( 23 + 53 \, \mu2 \right) \right) + \right. \right. \\ & \quad \left. \left. \eta \mathfrak{t} \left( -128 - 146 \, \mu1^2 + 313 \, \mu2 + 540 \, \mu2^2 + \mu1 \left( -274 + 577 \, \mu2 \right) \right) \right) \right) + \\ & 3 \times (-1 + \eta \mathfrak{t}) \, \mathfrak{el} \left( 20 + 84 \, \mu1 + 64 \, \mu1^2 - 22 \, \mu2 - 14 \, \mu1 \, \mu2 - \right. \\ & \quad \left. 40 \, \mu2^2 + \text{op} \left( 74 + 51 \, \mathfrak{x}1 + 21 \, \mathfrak{x}2 + 4 \, \mu2^2 \left( 54 + 27 \, \mathfrak{x}1 + \mathfrak{x}2 \right) + \right. \right. \\ & \quad \left. \left. \mu1^2 \left( 112 + 33 \, \mathfrak{x}1 + 23 \, \mathfrak{x}2 \right) + \mu2 \left( 382 + 173 \, \mathfrak{x}1 + 103 \, \mathfrak{x}2 \right) + \right. \right. \\ & \quad \left. \left. \mu1 \left( 186 + 84 \, \mathfrak{x}1 + 44 \, \mathfrak{x}2 + \mu2 \left( 526 + 93 \, \mathfrak{x}1 + 127 \, \mathfrak{x}2 \right) \right) \right) \right) \right) + \eta^5 \\ & \left( \text{op} \left( 892 + 1548 \, \mu1^2 + 4742 \, \mu2 + 3200 \, \mu2^2 + \mu1 \left( 2440 + 5278 \, \mu2 \right) + \right. \right. \\ & \quad \left. \left. \eta \mathfrak{t} \left( -322 + 768 \, \mu1^2 + 197 \, \mu2 + 1580 \, \mu2^2 + \mu1 \left( 446 + 3765 \, \mu2 \right) \right) \right) \right) - \\ & (-1 + \eta \mathfrak{t}) \, \mathfrak{el} \left( 24 - 68 \, \mu1 - 92 \, \mu1^2 - 5 \, \mu2 - 565 \, \mu1 \, \mu2 - 4 \, \mu2^2 + \right. \\ & \quad \left. 2 \text{op} \left( 478 + 25 \, \mathfrak{x}1 + 2 \, \mu2^2 \left( 82 + 15 \, \mathfrak{x}1 - 117 \, \mathfrak{x}2 \right) - 5 \, \mathfrak{x}2 + \right. \right. \\ & \quad \left. \left. \mu2 \left( 1710 + 85 \, \mathfrak{x}1 + 31 \, \mathfrak{x}2 \right) + \mu1^2 \left( 484 + 23 \, \mathfrak{x}1 + 53 \, \mathfrak{x}2 \right) + \right. \right. \\ & \quad \left. \left. \mu1 \left( 962 + 48 \, \mathfrak{x}1 + 48 \, \mathfrak{x}2 + \mu2 \left( 1566 + 5 \, \mathfrak{x}1 + 215 \, \mathfrak{x}2 \right) \right) \right) \right) \right) - 2 \, \eta^3 \\ & \left( \text{op} \left( 671 + 1008 \, \mu1^2 + 2637 \, \mu2 + 1240 \, \mu2^2 + \mu1 \left( 1679 + 2821 \, \mu2 \right) + \right. \right. \\ & \quad \left. \left. \eta \mathfrak{t} \left( -248 + 478 \, \mu1^2 - 351 \, \mu2 + 428 \, \mu2^2 + \mu1 \left( 230 + 1657 \, \mu2 \right) \right) \right) \right) + \\ & (-1 + \eta \mathfrak{t}) \, \mathfrak{el} \left( 72 + 322 \, \mu1 + 250 \, \mu1^2 - 59 \, \mu2 - 59 \, \mu1 \, \mu2 - 140 \, \mu2^2 + \right. \\ & \quad \left. 2 \text{op} \left( 306 + 110 \, \mathfrak{x}1 + \mu2^2 \left( 486 + 225 \, \mathfrak{x}1 - 71 \, \mathfrak{x}2 \right) + 40 \, \mathfrak{x}2 + \right. \right. \\ & \quad \left. \left. \mu1^2 \left( 384 + 73 \, \mathfrak{x}1 + 63 \, \mathfrak{x}2 \right) + \mu2 \left( 1328 + 373 \, \mathfrak{x}1 + 215 \, \mathfrak{x}2 \right) + \right. \right. \\ & \quad \left. \left. \mu1 \left( 690 + 183 \, \mathfrak{x}1 + 103 \, \mathfrak{x}2 + \mu2 \left( 1568 + 185 \, \mathfrak{x}1 + 323 \, \mathfrak{x}2 \right) \right) \right) \right) \right) + \eta^4 \\ & \left( \text{op} \left( -2 \times \left( 603 + 846 \, \mu1^2 + 893 \, \mu2 - 2040 \, \mu2^2 + \mu1 \left( 1449 + 565 \, \mu2 \right) \right) + \right. \right. \\ & \quad \left. \left. \eta \mathfrak{t} \left( 206 - 164 \, \mu1^2 + 1083 \, \mu2 + 20 \, \mu2^2 + \mu1 \left( 42 + 1075 \, \mu2 \right) \right) \right) \right) - \\ & (-1 + \eta \mathfrak{t}) \, \mathfrak{el} \left( 2 \times \left( 60 + 74 \, \mu1^2 + \mu1 \left( 134 - 425 \, \mu2 \right) - 21 \, \mu2 - 76 \, \mu2^2 \right) + \right. \\ & \quad \left. \text{op} \left( 1958 + 337 \, \mathfrak{x}1 + 4 \, \mu2^2 \left( 406 + 159 \, \mathfrak{x}1 - 191 \, \mathfrak{x}2 \right) + 87 \, \mathfrak{x}2 + \right. \right. \\ & \quad \left. \left. \mu1^2 \left( 2168 + 239 \, \mathfrak{x}1 + 289 \, \mathfrak{x}2 \right) + \mu2 \left( 7586 + 1143 \, \mathfrak{x}1 + 613 \, \mathfrak{x}2 \right) + \mu1 \right. \right. \\ & \quad \left. \left. \left( 4126 + 576 \, \mathfrak{x}1 + 376 \, \mathfrak{x}2 + \mu2 \left( 7826 + 471 \, \mathfrak{x}1 + 1341 \, \mathfrak{x}2 \right) \right) \right) \right) \right) + \\ & w^2 (-1 + \eta)^2 \left( 2 \, x^8 (-1 + \eta)^9 \text{op} \left( \eta - \eta \mathfrak{t} + 4 \, \mu1 \right) \left( 3 + 3 \, \mu1 + 4 \, \mu2 \right) - \right. \\ & \quad x^7 (-1 + \eta)^7 \left( 4 \times (-1 + \eta \mathfrak{t}) \, \mathfrak{el} \left( 11 \, \mu1^2 + 4 \, \mu2 + 11 \, \mu1 \left( 1 + 4 \, \mu2 \right) \right) + \text{op} \right. \\ & \quad \left( -138 + 138 \, \mathfrak{el} - 438 \, \mu1 + 268 \, \mathfrak{el} \, \mu1 - 300 \, \mu1^2 + 130 \, \mathfrak{el} \, \mu1^2 - \right. \\ & \quad \left. 414 \, \mu2 + 438 \, \mathfrak{el} \, \mu2 - 478 \, \mu1 \, \mu2 + 326 \, \mathfrak{el} \, \mu1 \, \mu2 + 48 \, \mathfrak{el} \, \mu2^2 + \right. \\ & \quad \left. 16 \, \eta^3 \left( 3 + 3 \, \mu1 + 4 \, \mu2 \right) + \eta^2 \left( 30 + 192 \, \mu1^2 + 52 \, \mu2 - \right. \right. \\ & \quad \left. \left. 56 \, \mu2^2 - 16 \, \eta \mathfrak{t} \left( 3 + 3 \, \mu1 + 4 \, \mu2 \right) + \mu1 \left( 222 + 236 \, \mu2 \right) \right) + \right. \\ & \quad \left. 2 \, \eta \left( 30 + 54 \, \mu1^2 + 149 \, \mu2 + 28 \, \mu2^2 + \mu1 \left( 84 + 121 \, \mu2 \right) + \right. \right. \\ & \quad \left. \left. \eta \mathfrak{t} \left( -15 - 26 \, \mu2 + 28 \, \mu2^2 + 5 \, \mu1 \left( -3 + 2 \, \mu2 \right) \right) \right) + \mathfrak{el} \, \mu1 \, \mathfrak{x}1 + \right. \\ & \quad \left. \mathfrak{el} \, \mu1^2 \, \mathfrak{x}1 + 4 \, \mathfrak{el} \, \mu2 \, \mathfrak{x}1 - 12 \, \mathfrak{el} \, \mu1 \, \mu2 \, \mathfrak{x}1 + 11 \, \mathfrak{el} \, \mu1 \, \mathfrak{x}2 + \right. \end{aligned}
\end{aligned}$$

$$\begin{aligned}
& 11 \, \theta \, \mu_1^2 \, \mu_2 + 16 \, \theta \, \mu_2 \, \mu_2 + 32 \, \theta \, \mu_1 \, \mu_2 \, \mu_2 - 40 \, \theta \, \mu_2^2 \, \mu_2 - \\
& \eta t \left( -78 - 78 \, \mu_1 - 116 \, \mu_2 + 20 \, \mu_1 \, \mu_2 + 56 \, \mu_2^2 + \theta \left( 138 - 8 \, \mu_2^2 \right. \right. \\
& \quad \left. \left. (-6 + 5 \, \mu_2) + 2 \, \mu_2 (219 + 2 \, \mu_1 + 8 \, \mu_2) + \mu_1^2 (130 + \mu_1 + 11 \, \mu_2) + \right. \right. \\
& \quad \left. \left. \mu_1 (268 + \mu_1 + 11 \, \mu_2 + \mu_2 (326 - 12 \, \mu_1 + 32 \, \mu_2)) \right) \right) + \\
& x^6 (-1 + \eta)^6 \left( 2 \times (-1 + \eta) \, \theta p \left( 195 + 603 \, \mu_1 + 408 \, \mu_1^2 + 609 \, \mu_2 + \right. \right. \\
& \quad 793 \, \mu_1 \, \mu_2 + 216 \, \mu_2^2 + 28 \, \eta^3 (3 + 3 \, \mu_1 + 4 \, \mu_2) + \\
& \quad \eta t \left( -93 - 61 \, \mu_1 + 32 \, \mu_1^2 - 92 \, \mu_2 + 184 \, \mu_1 \, \mu_2 + 196 \, \mu_2^2 \right) - 7 \, \eta^2 \left( -39 - \right. \\
& \quad \left. 87 \, \mu_1 - 48 \, \mu_1^2 - 58 \, \mu_2 - 54 \, \mu_1 \, \mu_2 + 28 \, \mu_2^2 + 4 \, \eta t (3 + 3 \, \mu_1 + 4 \, \mu_2) \right) + \\
& \quad \eta \left( 588 + 1638 \, \mu_1 + 1050 \, \mu_1^2 + 1569 \, \mu_2 + 1573 \, \mu_1 \, \mu_2 - 304 \, \mu_2^2 + \right. \\
& \quad \left. 7 \, \eta t \left( -39 - 39 \, \mu_1 - 58 \, \mu_2 + 10 \, \mu_1 \, \mu_2 + 28 \, \mu_2^2 \right) \right) - \\
& (-1 + \eta t) \, \theta \left( 84 - 16 \, \mu_1 - 332 \, \eta \, \mu_1 - 100 \, \mu_1^2 - 332 \, \eta \, \mu_1^2 + \right. \\
& \quad 49 \, \mu_2 - 96 \, \eta \, \mu_2 - 415 \, \mu_1 \, \mu_2 - 1296 \, \eta \, \mu_1 \, \mu_2 + 24 \, \mu_2^2 + \\
& \quad \theta p \left( 306 + 1074 \, \mu_2 + 208 \, \mu_2^2 + 15 \, \mu_1 + 45 \, \mu_2 \, \mu_1 - 15 \, \mu_2 - 9 \, \mu_2 \, \mu_2 - \right. \\
& \quad 264 \, \mu_2^2 \, \mu_2 + \mu_1^2 (424 - 7 \, \mu_1 + 23 \, \mu_2) + \mu_1 (730 + 8 \, \mu_1 + 8 \, \mu_2 + \\
& \quad \mu_2 (1250 - 131 \, \mu_1 + 79 \, \mu_2)) + 2 \, \eta \left( 495 - 20 \, \mu_2^2 (-8 + 7 \, \mu_2) + \right. \\
& \quad 2 \, \mu_2 (792 + 7 \, \mu_1 + 28 \, \mu_2) + \mu_1^2 (468 + 10 \, \mu_1 + 45 \, \mu_2) + \\
& \quad \left. \left. \mu_1 (963 + 10 \, \mu_1 + 45 \, \mu_2 + \mu_2 (1188 - 20 \, \mu_1 + 134 \, \mu_2)) \right) \right) \right) + \\
& \eta \, \theta p \left( \eta^9 (6 + 6 \, \mu_1 + 8 \, \mu_2) - \eta t \, \mu_2 (11 + 11 \, \mu_1 + 8 \, \mu_2) - \eta \, \eta t \right. \\
& \quad \left. (24 + 267 \, \mu_2 + 224 \, \mu_2^2 + 3 \, \mu_1 (8 + 89 \, \mu_2)) + \eta^8 \right. \\
& \quad \left. (-2 \, \eta t (3 + 3 \, \mu_1 + 4 \, \mu_2) + 4 \times (18 + 6 \, \mu_1^2 + 27 \, \mu_2 - 14 \, \mu_2^2 + 3 \, \mu_1 (8 + \mu_2)) \right) + \\
& 2 \, \eta^7 (135 + 138 \, \mu_1^2 + 269 \, \mu_2 - 276 \, \mu_2^2 + 7 \, \mu_1 (39 + 19 \, \mu_2) + \\
& \quad 2 \, \eta t (-18 - 27 \, \mu_2 + 14 \, \mu_2^2 + \mu_1 (-18 + 5 \, \mu_2)) - 2 \, \eta^6 \\
& \quad (-2 \times (63 + 129 \, \mu_1^2 + 199 \, \mu_2 - 38 \, \mu_2^2 + \mu_1 (192 + 259 \, \mu_2)) - \\
& \quad \theta \left( 81 + 2 \, \mu_2 (135 + \mu_1 + 4 \, \mu_2) - 4 \, \mu_2^2 (-4 + 5 \, \mu_2) + \mu_1^2 (78 + 7 \, \mu_1 + \right. \\
& \quad \left. 12 \, \mu_2) + \mu_1 (159 + 7 \, \mu_1 + 12 \, \mu_2 + 2 \, \mu_2 (105 + 8 \, \mu_1 + 19 \, \mu_2)) \right) + \\
& \quad \eta t (54 - 66 \, \mu_1^2 + 34 \, \mu_2 - 168 \, \mu_2^2 - 6 \, \mu_1 (2 + 49 \, \mu_2) + \theta \left( 81 + 2 \, \mu_2 \right. \\
& \quad \left. (135 + \mu_1 + 4 \, \mu_2) - 4 \, \mu_2^2 (-4 + 5 \, \mu_2) + \mu_1^2 (78 + 7 \, \mu_1 + 12 \, \mu_2) + \right. \\
& \quad \left. \left. \mu_1 (159 + 7 \, \mu_1 + 12 \, \mu_2 + 2 \, \mu_2 (105 + 8 \, \mu_1 + 19 \, \mu_2)) \right) \right) \right) + \\
& \eta^5 \left( 2 \times (-45 + 42 \, \mu_1^2 + 200 \, \mu_2 + 732 \, \mu_2^2 + \mu_1 (-3 + 508 \, \mu_2)) + \right. \\
& \quad 3 \, \theta \left( 126 + 9 \, \mu_1 + 4 \, \mu_2^2 (18 + 3 \, \mu_1 - 19 \, \mu_2) - \mu_2 + \right. \\
& \quad 2 \, \mu_1^2 (83 + 5 \, \mu_1 + 10 \, \mu_2) + \mu_2 (464 + 31 \, \mu_1 + 13 \, \mu_2) + \\
& \quad \left. \mu_1 (292 + 19 \, \mu_1 + 19 \, \mu_2 + \mu_2 (520 + 3 \, \mu_1 + 73 \, \mu_2)) \right) - \\
& \quad \eta t (36 - 108 \, \mu_1 - 144 \, \mu_1^2 - 119 \, \mu_2 - 911 \, \mu_1 \, \mu_2 - 160 \, \mu_2^2 + \\
& \quad 3 \, \theta \left( 126 + 9 \, \mu_1 + 4 \, \mu_2^2 (18 + 3 \, \mu_1 - 19 \, \mu_2) - \mu_2 + \right. \\
& \quad 2 \, \mu_1^2 (83 + 5 \, \mu_1 + 10 \, \mu_2) + \mu_2 (464 + 31 \, \mu_1 + 13 \, \mu_2) + \\
& \quad \left. \mu_1 (292 + 19 \, \mu_1 + 19 \, \mu_2 + \mu_2 (520 + 3 \, \mu_1 + 73 \, \mu_2)) \right) \right) - \\
& \eta^3 (186 + 360 \, \mu_1^2 + 882 \, \mu_2 + 688 \, \mu_2^2 + 42 \, \mu_1 (13 + 29 \, \mu_2) - \\
& \quad 3 \, \theta \left( 58 + 43 \, \mu_1 + 4 \, \mu_2^2 (46 + 21 \, \mu_1 - 5 \, \mu_2) + 13 \, \mu_2 + \right. \\
& \quad 2 \, \mu_1^2 (49 + 13 \, \mu_1 + 8 \, \mu_2) + \mu_2 (312 + 141 \, \mu_1 + 71 \, \mu_2) + \\
& \quad \left. \mu_1 (156 + 69 \, \mu_1 + 29 \, \mu_2 + \mu_2 (448 + 57 \, \mu_1 + 91 \, \mu_2)) \right) + \\
& \quad \eta t (4 \times (-33 + 20 \, \mu_1^2 - 64 \, \mu_2 - 2 \, \mu_2^2 + \mu_1 (-13 + 110 \, \mu_2)) + \\
& \quad 3 \, \theta \left( 58 + 43 \, \mu_1 + 4 \, \mu_2^2 (46 + 21 \, \mu_1 - 5 \, \mu_2) + 13 \, \mu_2 + \right. \\
& \quad \left. 2 \, \mu_1^2 (49 + 13 \, \mu_1 + 8 \, \mu_2) + \mu_2 (312 + 141 \, \mu_1 + 71 \, \mu_2) + \right.
\end{aligned}$$

$$\begin{aligned}
& \mu_1 (156 + 69 \mathfrak{e}_1 + 29 \mathfrak{e}_2 + \mu_2 (448 + 57 \mathfrak{e}_1 + 91 \mathfrak{e}_2)) \Big) \Big) - \\
& \eta^2 \Big( 4 \times (9 + 9 \mu_1^2 + 41 \mu_2 + 16 \mu_2^2 + \mu_1 (18 + 41 \mu_2)) - \mathfrak{e}_1 \\
& \quad (60 + 51 \mathfrak{e}_1 + 21 \mathfrak{e}_2 + 4 \mu_2^2 (50 + 27 \mathfrak{e}_1 + 11 \mathfrak{e}_2) + \\
& \quad \mu_2 (312 + 169 \mathfrak{e}_1 + 103 \mathfrak{e}_2) + 2 \mu_1^2 (19 \mathfrak{e}_1 + 9 \times (3 + \mathfrak{e}_2)) + \\
& \quad \mu_1 (114 + 89 \mathfrak{e}_1 + 39 \mathfrak{e}_2 + \mu_2 (312 + 113 \mathfrak{e}_1 + 103 \mathfrak{e}_2)) \Big) + \\
& \eta \mathfrak{t} (-8 \times (9 + 25 \mu_1^2 + \mu_1 (34 - 12 \mu_2) - 21 \mu_2 - 32 \mu_2^2) + \\
& \quad \mathfrak{e}_1 (60 + 51 \mathfrak{e}_1 + 21 \mathfrak{e}_2 + 4 \mu_2^2 (50 + 27 \mathfrak{e}_1 + 11 \mathfrak{e}_2) + \\
& \quad \mu_2 (312 + 169 \mathfrak{e}_1 + 103 \mathfrak{e}_2) + 2 \mu_1^2 (19 \mathfrak{e}_1 + 9 \times (3 + \mathfrak{e}_2)) + \\
& \quad \mu_1 (114 + 89 \mathfrak{e}_1 + 39 \mathfrak{e}_2 + \mu_2 (312 + 113 \mathfrak{e}_1 + 103 \mathfrak{e}_2)) \Big) \Big) - \\
& \eta^4 \Big( 12 \times (24 + 42 \mu_1^2 + 67 \mu_2 - 4 \mu_2^2 + \mu_1 (66 + 79 \mu_2)) - \\
& \quad \mathfrak{e}_1 (4 \mu_2^2 (134 + 45 \mathfrak{e}_1 - 73 \mathfrak{e}_2) + 15 \times (22 + 7 \mathfrak{e}_1 + \mathfrak{e}_2) + \\
& \quad \mu_1^2 (582 + 56 \mathfrak{e}_1 + 66 \mathfrak{e}_2) + \mu_2 (1476 + 343 \mathfrak{e}_1 + 133 \mathfrak{e}_2) + \\
& \quad \mu_1 (912 + 161 \mathfrak{e}_1 + 81 \mathfrak{e}_2 + \mu_2 (2172 + 35 \mathfrak{e}_1 + 313 \mathfrak{e}_2)) \Big) + \\
& \eta \mathfrak{t} (-42 + 354 \mu_1 + 396 \mu_1^2 - 255 \mu_2 + 705 \mu_1 \mu_2 + 72 \mu_2^2 + \\
& \quad \mathfrak{e}_1 (4 \mu_2^2 (134 + 45 \mathfrak{e}_1 - 73 \mathfrak{e}_2) + 15 \times (22 + 7 \mathfrak{e}_1 + \mathfrak{e}_2) + \\
& \quad \mu_1^2 (582 + 56 \mathfrak{e}_1 + 66 \mathfrak{e}_2) + \mu_2 (1476 + 343 \mathfrak{e}_1 + 133 \mathfrak{e}_2) + \\
& \quad \mu_1 (912 + 161 \mathfrak{e}_1 + 81 \mathfrak{e}_2 + \mu_2 (2172 + 35 \mathfrak{e}_1 + 313 \mathfrak{e}_2)) \Big) \Big) \Big) + \\
& x^5 (-1 + \eta)^5 \Big( - \Big( (-1 + \eta) \mathfrak{e}_p \Big( 112 \eta^4 (3 + 3 \mu_1 + 4 \mu_2) - 14 \eta^3 (-117 - 213 \\
& \quad \mu_1 - 96 \mu_1^2 - 174 \mu_2 - 98 \mu_1 \mu_2 + 84 \mu_2^2 + 8 \eta \mathfrak{t} (3 + 3 \mu_1 + 4 \mu_2)) \Big) + \\
& \eta \mathfrak{t} (-234 + 272 \mu_1^2 - 113 \mu_2 + 516 \mu_2^2 + \mu_1 (38 + 927 \mu_2)) \Big) + \\
& 2 \times (219 + 450 \mu_1^2 + 833 \mu_2 + 704 \mu_2^2 + \mu_1 (669 + 1169 \mu_2)) \Big) + \\
& 2 \eta (1275 + 3723 \mu_1 + 2448 \mu_1^2 + 3770 \mu_2 + 4622 \mu_1 \mu_2 + 700 \mu_2^2 + \\
& \quad 2 \eta \mathfrak{t} (-279 - 166 \mu_1 + 113 \mu_1^2 - 276 \mu_2 + 612 \mu_1 \mu_2 + 588 \mu_2^2)) \Big) + \\
& 6 \eta^2 (693 + 1050 \mu_1^2 + 1689 \mu_2 - 608 \mu_2^2 + 3 \mu_1 (581 + 491 \mu_2) + \\
& \quad 7 \eta \mathfrak{t} (-39 - 58 \mu_2 + 28 \mu_2^2 + \mu_1 (-39 + 10 \mu_2)) \Big) \Big) \Big) + \\
& (-1 + \eta \mathfrak{t}) \mathfrak{e}_1 \Big( 2 \times (90 + 80 \mu_1^2 - 7 \mu_2 - 84 \mu_2^2 + \mu_1 (170 + 9 \mu_2)) \Big) + \\
& \mathfrak{e}_p (258 + 81 \mathfrak{e}_1 + 4 \mu_2^2 (118 + 27 \mathfrak{e}_1 - 91 \mathfrak{e}_2) - 9 \mathfrak{e}_2 + \\
& \quad \mu_1^2 (512 + 21 \mathfrak{e}_1 + 31 \mathfrak{e}_2) + \mu_2 (1146 + 247 \mathfrak{e}_1 + 37 \mathfrak{e}_2) + \\
& \quad \mu_1 (770 + 102 \mathfrak{e}_1 + 22 \mathfrak{e}_2 + \mu_2 (1834 - 113 \mathfrak{e}_1 + 165 \mathfrak{e}_2)) \Big) + \\
& \eta^2 (-40 \times (25 \mu_1^2 + 6 \mu_2 + \mu_1 (25 + 96 \mu_2)) + 3 \mathfrak{e}_p \\
& \quad (1014 - 8 \mu_2^2 (-38 + 35 \mathfrak{e}_2) + 2 \mu_2 (1635 + 14 \mathfrak{e}_1 + 56 \mathfrak{e}_2) + \\
& \quad \mu_1^2 (962 + 33 \mathfrak{e}_1 + 103 \mathfrak{e}_2) + \\
& \quad \mu_1 (1976 + 33 \mathfrak{e}_1 + 103 \mathfrak{e}_2 + \mu_2 (2470 + 4 \mathfrak{e}_1 + 312 \mathfrak{e}_2)) \Big) \Big) + \\
& \eta (408 - 504 \mu_1^2 + 197 \mu_2 + 84 \mu_2^2 - 3 \mu_1 (32 + 889 \mu_2) + \\
& \quad \mathfrak{e}_p (2 \times (954 + 51 \mathfrak{e}_1 + 2 \mu_2^2 (314 + 9 \mathfrak{e}_1 - 387 \mathfrak{e}_2) + 3 \mu_2 \\
& \quad (1127 + 53 \mathfrak{e}_1 - \mathfrak{e}_2) - 39 \mathfrak{e}_2) + \mu_1^2 (2618 - 5 \mathfrak{e}_1 + 175 \mathfrak{e}_2) + \\
& \quad \mu_1 (4526 + 97 \mathfrak{e}_1 + 97 \mathfrak{e}_2 + \mu_2 (7810 - 646 \mathfrak{e}_1 + 614 \mathfrak{e}_2)) \Big) \Big) \Big) - \\
& x^4 (-1 + \eta)^4 \Big( - \Big( (-1 + \eta) \mathfrak{e}_p \Big( 140 \eta^5 (3 + 3 \mu_1 + 4 \mu_2) + 70 \eta^4 (39 + \\
& \quad 63 \mu_1 + 24 \mu_1^2 + 58 \mu_2 + 22 \mu_1 \mu_2 - 28 \mu_2^2 - 2 \eta \mathfrak{t} (3 + 3 \mu_1 + 4 \mu_2)) \Big) + \\
& 10 \eta^3 (798 + 1848 \mu_1 + 1050 \mu_1^2 + 1809 \mu_2 + 1373 \mu_1 \mu_2 - \\
& \quad 912 \mu_2^2 + 7 \eta \mathfrak{t} (-39 - 39 \mu_1 - 58 \mu_2 + 10 \mu_1 \mu_2 + 28 \mu_2^2)) \Big) + \\
& 2 \times (111 + 309 \mu_1 + 198 \mu_1^2 + 497 \mu_2 + 665 \mu_1 \mu_2 + 424 \mu_2^2 + \\
& \quad \eta \mathfrak{t} (-90 - 6 \mu_1 + 84 \mu_1^2 + 95 \mu_2 + 283 \mu_1 \mu_2 + 240 \mu_2^2)) \Big) +
\end{aligned}$$

$$\begin{aligned}
& 10 \eta^2 \left( 690 + 1914 \mu_1 + 1224 \mu_1^2 + 1943 \mu_2 + 2243 \mu_1 \mu_2 + 52 \mu_2^2 + \right. \\
& \quad \left. \eta t \left( -279 - 149 \mu_1 + 130 \mu_1^2 - 276 \mu_2 + 672 \mu_1 \mu_2 + 588 \mu_2^2 \right) \right) + \\
& \quad \eta \left( 6 \times \left( 377 + 1127 \mu_1 + 750 \mu_1^2 + 1419 \mu_2 + 1947 \mu_1 \mu_2 + \right. \right. \\
& \quad \quad \left. 1056 \mu_2^2 \right) + \eta t \left( -1158 + 206 \mu_1 + 1364 \mu_1^2 - \right. \\
& \quad \quad \left. 517 \mu_2 + 5227 \mu_1 \mu_2 + 2616 \mu_2^2 \right) \left. \right) \left. \right) + (-1 + \eta t) \\
& \quad \Theta l \left( 72 + 256 \mu_1 + 184 \mu_1^2 - 346 \mu_2 - 202 \mu_1 \mu_2 - 416 \mu_2^2 + \right. \\
& \quad \Theta p \left( 8 \mu_2^2 (64 + 27 \Xi_1 - 12 \Xi_2) + 3 \times (50 + 39 \Xi_1 + 9 \Xi_2) + \right. \\
& \quad \quad \mu_1^2 (272 + 67 \Xi_1 + 37 \Xi_2) + 3 \mu_2 (274 + 125 \Xi_1 + 55 \Xi_2) + \\
& \quad \quad \mu_1 (422 + 184 \Xi_1 + 64 \Xi_2 + \mu_2 (1222 + 119 \Xi_1 + 221 \Xi_2)) \left. \right) + \\
& \quad \eta^2 \left( 792 - 224 \mu_1 - 1016 \mu_1^2 + 298 \mu_2 - 6518 \mu_1 \mu_2 + 96 \mu_2^2 + \right. \\
& \quad 5 \Theta p \left( 990 + 57 \Xi_1 + 4 \mu_2^2 (158 + 9 \Xi_1 - 189 \Xi_2) - 33 \Xi_2 + \right. \\
& \quad \quad 73 \mu_1 (32 + \Xi_1 + \Xi_2) + 3 \mu_2 (1180 + 61 \Xi_1 + 7 \Xi_2) + \\
& \quad \quad 2 \mu_1^2 (673 + 8 \Xi_1 + 53 \Xi_2) + \mu_1 \mu_2 (4060 - 253 \Xi_1 + 377 \Xi_2) \left. \right) \left. \right) + \\
& \quad 10 \eta^3 \left( -4 \times \left( 39 \mu_1^2 + 8 \mu_2 + \mu_1 (39 + 148 \mu_2) \right) + \Theta p \right. \\
& \quad \quad \left( 519 + 2 \mu_2 (843 + 7 \Xi_1 + 28 \Xi_2) - \right. \\
& \quad \quad 4 \mu_2^2 (-36 + 35 \Xi_2) + \mu_1^2 (494 + 23 \Xi_1 + 58 \Xi_2) + \\
& \quad \quad \mu_1 (1013 + 23 \Xi_1 + 58 \Xi_2 + 2 \mu_2 (641 + 12 \Xi_1 + 89 \Xi_2)) \left. \right) \left. \right) + \\
& \quad \eta \left( 8 \times \left( 90 + 116 \mu_1^2 + \mu_1 (206 - 22 \mu_2) - 7 \mu_2 - 84 \mu_2^2 \right) + \right. \\
& \quad \Theta p \left( 4 \mu_2^2 (606 + 153 \Xi_1 - 437 \Xi_2) + 3 \times (454 + 143 \Xi_1 - 7 \Xi_2) + \right. \\
& \quad \quad 10 \mu_1^2 (263 + 14 \Xi_1 + 19 \Xi_2) + \mu_2 (6060 + 1331 \Xi_1 + 281 \Xi_2) + \\
& \quad \quad \mu_1 (3992 + 569 \Xi_1 + 169 \Xi_2 + \mu_2 (9508 - 417 \Xi_1 + 973 \Xi_2)) \left. \right) \left. \right) \left. \right) + \\
& \quad x^3 (-1 + \eta)^3 \left( -2 \times (-1 + \eta) \Theta p \left( 56 \eta^6 (3 + 3 \mu_1 + 4 \mu_2) + 2 \times \right. \right. \\
& \quad \quad \left( 9 + 9 \mu_1^2 + 41 \mu_2 + 16 \mu_2^2 + \mu_1 (18 + 41 \mu_2) \right) + \\
& \quad \quad \eta t \left( -4 + 20 \mu_1^2 + 303 \mu_2 + 304 \mu_2^2 + \mu_1 (16 + 283 \mu_2) \right) - \\
& \quad \quad 7 \eta^5 \left( -96 \mu_1^2 + 8 \eta t (3 + 3 \mu_1 + 4 \mu_2) - \right. \\
& \quad \quad 3 \mu_1 (97 + 26 \mu_2) + 5 \times (-39 - 58 \mu_2 + 28 \mu_2^2) \left. \right) + \\
& \quad 5 \eta^4 \left( 903 + 1050 \mu_1^2 + 1929 \mu_2 - 1216 \mu_2^2 + \mu_1 (1953 + 1273 \mu_2) + \right. \\
& \quad \quad 7 \eta t \left( -39 - 58 \mu_2 + 28 \mu_2^2 + \mu_1 (-39 + 10 \mu_2) \right) \left. \right) + \\
& \quad 10 \eta^3 \left( 495 + 816 \mu_1^2 + 1334 \mu_2 - 164 \mu_2^2 + \mu_1 (1311 + 1450 \mu_2) + \right. \\
& \quad \quad 2 \eta t \left( -93 + 49 \mu_1^2 - 92 \mu_2 + 196 \mu_2^2 + 4 \mu_1 (-11 + 61 \mu_2) \right) \left. \right) + \\
& \quad 2 \eta \left( 222 + 396 \mu_1^2 + 1007 \mu_2 + 824 \mu_2^2 + \mu_1 (618 + 1343 \mu_2) + \right. \\
& \quad \quad 2 \eta t \left( -90 + 48 \mu_1^2 + 95 \mu_2 + 240 \mu_2^2 + \mu_1 (-42 + 314 \mu_2) \right) \left. \right) + \\
& \quad \eta^2 \left( 2334 + 4500 \mu_1^2 + 8698 \mu_2 + 5632 \mu_2^2 + 2 \mu_1 (3417 + 5837 \mu_2) + \right. \\
& \quad \quad \eta t \left( -1146 + 1368 \mu_1^2 - 469 \mu_2 + 2652 \mu_2^2 + \mu_1 (222 + 5819 \mu_2) \right) \left. \right) \left. \right) + \\
& \quad (-1 + \eta t) \Theta l \left( -2 \times \left( 12 + 139 \mu_2 + 116 \mu_2^2 + \mu_1 (12 + 139 \mu_2) \right) + \right. \\
& \quad \Theta p \left( 60 + 51 \Xi_1 + 21 \Xi_2 + 4 \mu_2^2 (50 + 27 \Xi_1 + 11 \Xi_2) + \right. \\
& \quad \quad \mu_2 (312 + 169 \Xi_1 + 103 \Xi_2) + 2 \mu_1^2 (19 \Xi_1 + 9 \times (3 + \Xi_2)) + \\
& \quad \quad \mu_1 (114 + 89 \Xi_1 + 39 \Xi_2 + \mu_2 (312 + 113 \Xi_1 + 103 \Xi_2)) \left. \right) + \\
& \quad \eta \left( 2 \times \left( 128 + 396 \mu_1^2 + \mu_1 (524 - 207 \mu_2) - 439 \mu_2 - 564 \mu_2^2 \right) + \right. \\
& \quad \quad 3 \Theta p \left( 4 \mu_2^2 (75 \Xi_1 - 29 \times (-6 + \Xi_2)) + 8 \times (26 + 20 \Xi_1 + 5 \Xi_2) + \right. \\
& \quad \quad \mu_1^2 (370 + 93 \Xi_1 + 53 \Xi_2) + 2 \mu_2 (567 + 258 \Xi_1 + 118 \Xi_2) + \\
& \quad \quad \mu_1 (578 + 253 \Xi_1 + 93 \Xi_2 + 2 \mu_2 (835 + 88 \Xi_1 + 156 \Xi_2)) \left. \right) \left. \right) + \\
& \quad 2 \eta^3 \left( 384 - 512 \mu_1^2 + 101 \mu_2 + 12 \mu_2^2 - \mu_1 (128 + 3851 \mu_2) + \right.
\end{aligned}$$

$$\begin{aligned}
& 5 \, \text{op} \left( 684 + 42 \, \mathfrak{x}1 + 4 \, \mu^2 \left( 106 + 9 \, \mathfrak{x}1 - 123 \, \mathfrak{x}2 \right) - 18 \, \mathfrak{x}2 + \right. \\
& \quad 6 \, \mu^2 \left( 411 + 23 \, \mathfrak{x}1 + 5 \, \mathfrak{x}2 \right) + \mu^2 \left( 922 + 23 \, \mathfrak{x}1 + 83 \, \mathfrak{x}2 \right) + \\
& \quad \left. \mu^1 \left( 1606 + 65 \, \mathfrak{x}1 + 65 \, \mathfrak{x}2 + \mu^2 \left( 2810 - 122 \, \mathfrak{x}1 + 298 \, \mathfrak{x}2 \right) \right) \right) + \\
& 5 \, \eta^4 \left( -4 \times \left( 67 \, \mu^2 + 12 \, \mu^2 + \mu^1 \left( 67 + 252 \, \mu^2 \right) \right) + \text{op} \right. \\
& \quad \left( 1062 - 8 \, \mu^2 \left( -34 + 35 \, \mathfrak{x}2 \right) + 2 \, \mu^2 \left( 1737 + 14 \, \mathfrak{x}1 + 56 \, \mathfrak{x}2 \right) + \right. \\
& \quad \mu^2 \left( 1014 + 59 \, \mathfrak{x}1 + 129 \, \mathfrak{x}2 \right) + \\
& \quad \left. \mu^1 \left( 2076 + 59 \, \mathfrak{x}1 + 129 \, \mathfrak{x}2 + \mu^2 \left( 2658 + 92 \, \mathfrak{x}1 + 400 \, \mathfrak{x}2 \right) \right) \right) + \\
& 2 \, \eta^2 \left( 6 \times \left( 90 + 152 \, \mu^2 + \mu^1 \left( 242 - 53 \, \mu^2 \right) - 7 \, \mu^2 - 84 \, \mu^2 \right) + \right. \\
& \quad \text{op} \left( 4 \, \mu^2 \left( 622 + 171 \, \mathfrak{x}1 - 419 \, \mathfrak{x}2 \right) + 3 \times \left( 478 + 151 \, \mathfrak{x}1 + \mathfrak{x}2 \right) + \right. \\
& \quad \mu^2 \left( 6390 + 1427 \, \mathfrak{x}1 + 377 \, \mathfrak{x}2 \right) + 25 \, \mu^2 \left( 7 \, \mathfrak{x}1 + 9 \times \left( 12 + \mathfrak{x}2 \right) \right) + \mu^1 \\
& \quad \left. \left( 4134 + 628 \, \mathfrak{x}1 + 228 \, \mathfrak{x}2 + \mu^2 \left( 9846 - 269 \, \mathfrak{x}1 + 1121 \, \mathfrak{x}2 \right) \right) \right) \right) + \\
& x^2 \left( -1 + \eta \right)^2 \left( -56 \, \eta \, \text{t} \, \text{op} - 108 \, \eta \, \text{t} \, \text{op} \, \mu^1 - 52 \, \eta \, \text{t} \, \text{op} \, \mu^2 - 11 \, \text{el} \, \mu^2 + 11 \right. \\
& \quad \eta \, \text{t} \, \text{el} \, \mu^2 - 406 \, \eta \, \text{t} \, \text{op} \, \mu^2 - 11 \, \text{el} \, \mu^1 \, \mu^2 + 11 \, \eta \, \text{t} \, \text{el} \, \mu^1 \, \mu^2 - 414 \\
& \quad \eta \, \text{t} \, \text{op} \, \mu^1 \, \mu^2 - 8 \, \text{el} \, \mu^2 + 8 \, \eta \, \text{t} \, \text{el} \, \mu^2 - 328 \, \eta \, \text{t} \, \text{op} \, \mu^2 + 56 \\
& \quad \eta^8 \, \text{op} \left( 3 + 3 \, \mu^1 + 4 \, \mu^2 \right) - 14 \, \eta^7 \, \text{op} \left( -105 - 48 \, \mu^2 - 158 \, \mu^2 + \right. \\
& \quad \left. 84 \, \mu^2 - 17 \, \mu^1 \left( 9 + 2 \, \mu^2 \right) + 4 \, \eta \, \text{t} \left( 3 + 3 \, \mu^1 + 4 \, \mu^2 \right) \right) + 2 \, \eta^6 \, \text{op} \\
& \quad \left( 2205 + 2814 \, \mu^2 + 4929 \, \mu^2 - 3972 \, \mu^2 + \mu^1 \left( 5019 + 3281 \, \mu^2 \right) + \right. \\
& \quad \left. 7 \, \eta \, \text{t} \left( -105 - 158 \, \mu^2 + 84 \, \mu^2 + 15 \, \mu^1 \left( -7 + 2 \, \mu^2 \right) \right) \right) + 4 \, \eta \\
& \quad \text{op} \left( \eta \, \text{t} \left( 30 + 43 \, \mu^2 + \mu^1 \left( 73 - 273 \, \mu^2 \right) - 313 \, \mu^2 - 344 \, \mu^2 \right) - \right. \\
& \quad \left. 3 \times \left( 9 + 9 \, \mu^2 + 41 \, \mu^2 + 16 \, \mu^2 + \mu^1 \left( 18 + 41 \, \mu^2 \right) \right) \right) - \eta \left( -1 + \eta \, \text{t} \right) \\
& \quad \text{el} \left( 4 \times \left( -4 + 13 \, \mu^2 + \mu^1 \left( 9 - 105 \, \mu^2 \right) - 107 \, \mu^2 - 92 \, \mu^2 \right) + \right. \\
& \quad \left. 3 \, \text{op} \left( 60 + 51 \, \mathfrak{x}1 + 21 \, \mathfrak{x}2 + 4 \, \mu^2 \left( 50 + 27 \, \mathfrak{x}1 + 11 \, \mathfrak{x}2 \right) + \right. \right. \\
& \quad \mu^2 \left( 312 + 169 \, \mathfrak{x}1 + 103 \, \mathfrak{x}2 \right) + 2 \, \mu^2 \left( 19 \, \mathfrak{x}1 + 9 \times \left( 3 + \mathfrak{x}2 \right) \right) + \\
& \quad \left. \mu^1 \left( 114 + 89 \, \mathfrak{x}1 + 39 \, \mathfrak{x}2 + \mu^2 \left( 312 + 113 \, \mathfrak{x}1 + 103 \, \mathfrak{x}2 \right) \right) \right) \right) + \eta^4 \\
& \quad \left( 2 \, \text{op} \left( -1569 - 1620 \, \mu^2 - 1413 \, \mu^2 + 7648 \, \mu^2 + 3 \, \mu^1 \left( -1063 + 377 \, \mu^2 \right) + \right. \right. \\
& \quad \left. \eta \, \text{t} \left( 261 + 552 \, \mu^2 + 959 \, \mu^2 - 252 \, \mu^2 + 3 \, \mu^1 \left( 271 + 817 \, \mu^2 \right) \right) \right) - \\
& \quad \left( -1 + \eta \, \text{t} \right) \, \text{el} \left( 372 - 144 \, \mu^1 - 516 \, \mu^2 + 53 \, \mu^2 - 4443 \, \mu^1 \, \mu^2 - \right. \\
& \quad \left. 24 \, \mu^2 + 5 \, \text{op} \left( 8 \, \mu^2 \left( 80 + 9 \, \mathfrak{x}1 - 90 \, \mathfrak{x}2 \right) + 3 \times \left( 354 + 23 \, \mathfrak{x}1 - 7 \, \mathfrak{x}2 \right) + \right. \right. \\
& \quad \left. 3 \, \mu^2 \left( 1286 + 77 \, \mathfrak{x}1 + 23 \, \mathfrak{x}2 \right) + 2 \, \mu^1 \left( 1241 + 61 \, \mathfrak{x}1 + 61 \, \mathfrak{x}2 \right) + \mu^2 \right. \\
& \quad \left. \left( 1420 + 53 \, \mathfrak{x}1 + 143 \, \mathfrak{x}2 \right) + \mu^1 \, \mu^2 \left( 4370 - 113 \, \mathfrak{x}1 + 517 \, \mathfrak{x}2 \right) \right) \right) \right) + \\
& 2 \, \eta^5 \left( 2 \times \left( -1 + \eta \, \text{t} \right) \, \text{el} \left( 151 \, \mu^2 + 24 \, \mu^2 + \mu^1 \left( 151 + 564 \, \mu^2 \right) \right) + \right. \\
& \quad \text{op} \left( 951 + 3921 \, \mu^1 + 2970 \, \mu^2 + 4148 \, \mu^2 + 7016 \, \mu^1 \, \mu^2 + 1840 \, \mu^2 + \right. \\
& \quad \left. 2 \, \eta \, \text{t} \left( -288 + 122 \, \mu^1 + 410 \, \mu^2 - 81 \, \mu^2 + 1875 \, \mu^1 \, \mu^2 + 1176 \, \mu^2 \right) + \right. \\
& \quad \left. 3 \, \text{el} \left( 543 + 2 \, \mu^2 \left( 894 + 7 \, \mathfrak{x}1 + 28 \, \mathfrak{x}2 \right) - \right. \right. \\
& \quad \left. 4 \, \mu^2 \left( -32 + 35 \, \mathfrak{x}2 \right) + \mu^2 \left( 520 + 36 \, \mathfrak{x}1 + 71 \, \mathfrak{x}2 \right) + \right. \\
& \quad \left. \mu^1 \left( 1063 + 36 \, \mathfrak{x}1 + 71 \, \mathfrak{x}2 + 2 \, \mu^2 \left( 688 + 34 \, \mathfrak{x}1 + 111 \, \mathfrak{x}2 \right) \right) \right) - \\
& \quad \left. 3 \, \eta \, \text{t} \, \text{el} \left( 543 + 2 \, \mu^2 \left( 894 + 7 \, \mathfrak{x}1 + 28 \, \mathfrak{x}2 \right) - 4 \, \mu^2 \right. \right. \\
& \quad \left. \left( -32 + 35 \, \mathfrak{x}2 \right) + \mu^2 \left( 520 + 36 \, \mathfrak{x}1 + 71 \, \mathfrak{x}2 \right) + \mu^1 \right. \\
& \quad \left. \left( 1063 + 36 \, \mathfrak{x}1 + 71 \, \mathfrak{x}2 + 2 \, \mu^2 \left( 688 + 34 \, \mathfrak{x}1 + 111 \, \mathfrak{x}2 \right) \right) \right) \right) \right) - \eta^2 \\
& \quad \left( 2 \, \text{op} \left( 6 \times \left( 102 + 189 \, \mu^2 + 469 \, \mu^2 + 384 \, \mu^2 + \mu^1 \left( 291 + 637 \, \mu^2 \right) \right) + \eta \, \text{t} \right. \right. \\
& \quad \left. \left( -508 + 132 \, \mu^2 - 259 \, \mu^2 + 588 \, \mu^2 + \mu^1 \left( -376 + 1317 \, \mu^2 \right) \right) \right) + \left( -1 + \right. \\
& \quad \left. \eta \, \text{t} \right) \, \text{el} \left( 2 \times \left( 148 + 516 \, \mu^2 + \mu^1 \left( 664 - 111 \, \mu^2 \right) - 359 \, \mu^2 - 504 \, \mu^2 \right) + \right. \\
& \quad \left. 3 \, \text{op} \left( 4 \, \mu^2 \left( 266 + 117 \, \mathfrak{x}1 - 39 \, \mathfrak{x}2 \right) + 6 \times \left( 54 + 41 \, \mathfrak{x}1 + 11 \, \mathfrak{x}2 \right) + \right. \right.
\end{aligned}$$



$$\begin{aligned}
& 6 \mu_2 (293 + 133 \mathfrak{e}_1 + 63 \mathfrak{e}_2) + \mu_1^2 (566 + 145 \mathfrak{e}_1 + 85 \mathfrak{e}_2) + \\
& \mu_1 (890 + 391 \mathfrak{e}_1 + 151 \mathfrak{e}_2 + \mu_2 (2566 + 290 \mathfrak{e}_1 + 494 \mathfrak{e}_2)) \Big) \Big) - 2 \\
& \eta^3 \Big( \mathfrak{e}_p \Big( 1740 + 3312 \mu_1^2 + 5822 \mu_2 + 2528 \mu_2^2 + \mu_1 (5052 + 7598 \mu_2) + \\
& \eta t \Big( -594 + 1300 \mu_1^2 - 991 \mu_2 + 1248 \mu_2^2 + \mu_1 (706 + 4341 \mu_2) \Big) \Big) + \\
& (-1 + \eta t) \mathfrak{e}_l \Big( 4 \times \Big( 90 + 188 \mu_1^2 + \mu_1 (278 - 84 \mu_2) - 7 \mu_2 - 84 \mu_2^2 \Big) + \\
& \mathfrak{e}_p \Big( 4 \mu_2^2 (638 + 189 \mathfrak{e}_1 - 401 \mathfrak{e}_2) + \\
& 3 \times (502 + 159 \mathfrak{e}_1 + 9 \mathfrak{e}_2) + 10 \mu_1^2 (277 + 21 \mathfrak{e}_1 + 26 \mathfrak{e}_2) + \\
& \mu_2 (6720 + 1523 \mathfrak{e}_1 + 473 \mathfrak{e}_2) + \mu_1 (4276 + 687 \mathfrak{e}_1 + \\
& 287 \mathfrak{e}_2 + \mu_2 (10184 - 121 \mathfrak{e}_1 + 1269 \mathfrak{e}_2)) \Big) \Big) \Big) - \\
& \times (-1 + \eta) \times \Big( 16 \eta^9 \mathfrak{e}_p (3 + 3 \mu_1 + 4 \mu_2) - \eta t \mathfrak{e}_p (4 + 4 \mu_1^2 + 27 \mu_2 + \\
& 20 \mu_2^2 + \mu_1 (8 + 27 \mu_2)) + 2 \eta^8 \mathfrak{e}_p (249 + 96 \mu_1^2 + 374 \mu_2 - \\
& 196 \mu_2^2 - 8 \eta t (3 + 3 \mu_1 + 4 \mu_2) + \mu_1 (345 + 58 \mu_2)) + 2 \eta^7 \\
& \mathfrak{e}_p (840 + 954 \mu_1^2 + 1763 \mu_2 - 1628 \mu_2^2 + \mu_1 (1794 + 1015 \mu_2) + \\
& \eta t (-249 - 374 \mu_2 + 196 \mu_2^2 + \mu_1 (-249 + 70 \mu_2)) \Big) - \eta \\
& ((-1 + \eta t) \mathfrak{e}_l (4 + 4 \mu_1^2 + 5 \mu_2 + 4 \mu_2^2 + \mu_1 (8 + 5 \mu_2)) + \\
& \eta t \mathfrak{e}_p (76 + 48 \mu_1^2 + 657 \mu_2 + 540 \mu_2^2 + \mu_1 (124 + 665 \mu_2)) \Big) - \eta^2 \\
& (2 \mathfrak{e}_p (6 \times (9 + 9 \mu_1^2 + 41 \mu_2 + 16 \mu_2^2 + \mu_1 (18 + 41 \mu_2)) + \\
& \eta t (-92 - 206 \mu_1^2 + 407 \mu_2 + 512 \mu_2^2 + \mu_1 (-298 + 311 \mu_2)) \Big) + \\
& (-1 + \eta t) \mathfrak{e}_l (2 \times (4 + 26 \mu_1^2 + \mu_1 (30 - 71 \mu_2) - 75 \mu_2 - 68 \mu_2^2) + \\
& 3 \mathfrak{e}_p (60 + 51 \mathfrak{e}_1 + 21 \mathfrak{e}_2 + 4 \mu_2^2 (50 + 27 \mathfrak{e}_1 + 11 \mathfrak{e}_2) + \\
& \mu_2 (312 + 169 \mathfrak{e}_1 + 103 \mathfrak{e}_2) + 2 \mu_1^2 (19 \mathfrak{e}_1 + 9 \times (3 + \mathfrak{e}_2)) + \\
& \mu_1 (114 + 89 \mathfrak{e}_1 + 39 \mathfrak{e}_2 + \mu_2 (312 + 113 \mathfrak{e}_1 + 103 \mathfrak{e}_2)) \Big) \Big) \Big) + \\
& \eta^6 \Big( 16 \times (-1 + \eta t) \mathfrak{e}_l (7 \mu_1^2 + \mu_2 + \mu_1 (7 + 26 \mu_2)) + \mathfrak{e}_p \\
& (1164 + 3960 \mu_1 + 2796 \mu_1^2 + 4130 \mu_2 + 6010 \mu_1 \mu_2 + 280 \mu_2^2 + \\
& 2 \eta t (-285 + 362 \mu_1^2 - 146 \mu_2 + 980 \mu_2^2 + \mu_1 (77 + 1634 \mu_2)) + \\
& \mathfrak{e}_l (1110 - 40 \mu_2^2 (-6 + 7 \mathfrak{e}_2) + 2 \mu_2 (1839 + 14 \mathfrak{e}_1 + 56 \mathfrak{e}_2) + \\
& \mu_1^2 (1066 + 85 \mathfrak{e}_1 + 155 \mathfrak{e}_2) + \\
& \mu_1 (2176 + 85 \mathfrak{e}_1 + 155 \mathfrak{e}_2 + 2 \mu_2 (1423 + 90 \mathfrak{e}_1 + 244 \mathfrak{e}_2)) \Big) - \\
& \eta t \mathfrak{e}_l (1110 - 40 \mu_2^2 (-6 + 7 \mathfrak{e}_2) + 2 \mu_2 (1839 + 14 \mathfrak{e}_1 + 56 \mathfrak{e}_2) + \\
& \mu_1^2 (1066 + 85 \mathfrak{e}_1 + 155 \mathfrak{e}_2) + \mu_1 (2176 + 85 \mathfrak{e}_1 + \\
& 155 \mathfrak{e}_2 + 2 \mu_2 (1423 + 90 \mathfrak{e}_1 + 244 \mathfrak{e}_2)) \Big) \Big) \Big) - \eta^3 \\
& (2 \mathfrak{e}_p (2 \times (195 + 564 \mu_1 + 369 \mu_1^2 + 910 \mu_2 + 1246 \mu_1 \mu_2 + 728 \mu_2^2) + \\
& \eta t (-308 + 84 \mu_1^2 - 369 \mu_2 + 168 \mu_2^2 + 7 \mu_1 (-32 + 121 \mu_2)) \Big) + \\
& (-1 + \eta t) \mathfrak{e}_l (2 \times (56 + 212 \mu_1^2 + \mu_1 (268 - 5 \mu_2) - 93 \mu_2 - 148 \mu_2^2) + \\
& \mathfrak{e}_p (4 \mu_2^2 (542 + 243 \mathfrak{e}_1 - 69 \mathfrak{e}_2) + 24 \times (28 + 21 \mathfrak{e}_1 + 6 \mathfrak{e}_2) + \\
& 6 \mu_2 (605 + 274 \mathfrak{e}_1 + 134 \mathfrak{e}_2) + \mu_1^2 (1154 + 301 \mathfrak{e}_1 + 181 \mathfrak{e}_2) + \\
& \mu_1 (1826 + 805 \mathfrak{e}_1 + 325 \mathfrak{e}_2 + 2 \mu_2 (2627 + 316 \mathfrak{e}_1 + 520 \mathfrak{e}_2)) \Big) \Big) \Big) + \\
& \eta^5 \Big( \mathfrak{e}_p (-912 - 396 \mu_1^2 + 598 \mu_2 + 7592 \mu_2^2 + 2 \mu_1 (-654 + 1751 \mu_2) + \\
& \eta t (-6 + 652 \mu_1^2 + 731 \mu_2 + 372 \mu_2^2 + \mu_1 (646 + 3595 \mu_2)) \Big) - \\
& (-1 + \eta t) \mathfrak{e}_l (72 - 104 \mu_1^2 + \mu_2 - 12 \mu_2^2 - \mu_1 (32 + 1007 \mu_2) + \\
& \mathfrak{e}_p (4 \mu_2^2 (322 + 45 \mathfrak{e}_1 - 351 \mathfrak{e}_2) + 6 \times (366 + 25 \mathfrak{e}_1 - 5 \mathfrak{e}_2) + \\
& 6 \mu_2 (1339 + 85 \mathfrak{e}_1 + 31 \mathfrak{e}_2) + \mu_1^2 (2914 + 143 \mathfrak{e}_1 + 323 \mathfrak{e}_2) + \\
& \mu_1 (5110 + 293 \mathfrak{e}_1 + 293 \mathfrak{e}_2 + \mu_2 (9050 - 86 \mathfrak{e}_1 + 1174 \mathfrak{e}_2)) \Big) \Big) \Big) -
\end{aligned}$$

$$\begin{aligned}
& \eta^4 \left( \theta p \left( 2 \times \left( 795 + 1458 \mu_1^2 + 2467 \mu_2 + 560 \mu_2^2 + \mu_1 (2253 + 3091 \mu_2) \right) + \right. \right. \\
& \quad \left. \eta t \left( -402 + 1568 \mu_1^2 - 1133 \mu_2 + 804 \mu_2^2 + \mu_1 (1166 + 3995 \mu_2) \right) \right) + \\
& \quad \left( -1 + \eta t \right) \theta l \left( 2 \times \left( 90 + 224 \mu_1^2 + \mu_1 (314 - 115 \mu_2) - 7 \mu_2 - 84 \mu_2^2 \right) + \right. \\
& \quad \left. \theta p \left( 1578 + 501 \mathfrak{z}_1 + 4 \mu_2^2 (654 + 207 \mathfrak{z}_1 - 383 \mathfrak{z}_2) + \right. \right. \\
& \quad \quad 51 \mathfrak{z}_2 + 5 \mu_1^2 (568 + 49 \mathfrak{z}_1 + 59 \mathfrak{z}_2) + \\
& \quad \quad \mu_2 (7050 + 1619 \mathfrak{z}_1 + 569 \mathfrak{z}_2) + \mu_1 (4418 + 746 \mathfrak{z}_1 + \\
& \quad \quad \quad 346 \mathfrak{z}_2 + \mu_2 (10522 + 27 \mathfrak{z}_1 + 1417 \mathfrak{z}_2)) \left. \right) \left. \right) \left. \right) - \\
& w \left( x \left( -1 + \eta \right) - \eta \right) \left( -1 + \eta \right) \times \left( 2 x^7 \left( -1 + \eta \right)^7 \theta p \left( -20 + 11 \eta t + 20 \theta l - 59 \right. \right. \\
& \quad \mu_1 + 11 \eta t \mu_1 + 35 \theta l \mu_1 - 39 \mu_1^2 + 15 \theta l \mu_1^2 - 60 \mu_2 + 20 \eta t \\
& \quad \mu_2 + 60 \theta l \mu_2 - 60 \mu_1 \mu_2 + 28 \theta l \mu_1 \mu_2 + \eta^2 (11 + 11 \mu_1 + 20 \mu_2) + \eta \\
& \quad (9 + 39 \mu_1^2 + 40 \mu_2 + 12 \mu_1 (4 + 5 \mu_2) - \eta t (11 + 11 \mu_1 + 20 \mu_2)) + 4 \\
& \quad \left. \theta l \mu_2 \mathfrak{z}_2 - \eta t \theta l (20 + 15 \mu_1^2 + 7 \mu_1 (5 + 4 \mu_2) + 4 \mu_2 (15 + \mathfrak{z}_2)) \right) + \\
& x^5 \left( -1 + \eta \right)^5 \left( 2 \times \left( -1 + \eta \right) \theta p \left( 89 + 371 \mu_1 + 282 \mu_1^2 + 299 \mu_2 + \right. \right. \\
& \quad 635 \mu_1 \mu_2 + 368 \mu_2^2 + 21 \eta^3 (11 + 11 \mu_1 + 20 \mu_2) + \\
& \quad \eta t (-59 - 11 \mu_1 + 48 \mu_1^2 - 46 \mu_2 + 214 \mu_1 \mu_2 + 140 \mu_2^2) + \\
& \quad 3 \eta^2 (256 + 529 \mu_1 + 273 \mu_1^2 + 632 \mu_2 + 360 \mu_1 \mu_2 - \\
& \quad \quad 168 \mu_2^2 - 7 \eta t (11 + 11 \mu_1 + 20 \mu_2)) + \\
& \quad \eta (395 + 1457 \mu_1 + 1062 \mu_1^2 + 984 \mu_2 + 1780 \mu_1 \mu_2 - 60 \mu_2^2 + \\
& \quad \quad 2 \eta t (-138 - 129 \mu_1 + 9 \mu_1^2 - 204 \mu_2 + 88 \mu_1 \mu_2 + 168 \mu_2^2)) \left. \right) - \\
& \left( -1 + \eta t \right) \theta l \left( 84 + 92 \mu_1 - 380 \eta \mu_1 - 180 \eta^2 \mu_1 + 8 \mu_1^2 - 380 \eta \mu_1^2 - \right. \\
& \quad 180 \eta^2 \mu_1^2 + 65 \mu_2 - 160 \eta \mu_2 + 17 \mu_1 \mu_2 - 1488 \eta \mu_1 \mu_2 - 560 \eta^2 \mu_1 \mu_2 + \\
& \quad 24 \mu_2^2 + \theta p \left( 94 + 378 \mu_2 + 272 \mu_2^2 + 15 \mathfrak{z}_1 + 45 \mu_2 \mathfrak{z}_1 - 15 \mathfrak{z}_2 - 25 \mu_2 \mathfrak{z}_2 - \right. \\
& \quad \quad 264 \mu_2^2 \mathfrak{z}_2 - 2 \mu_1 (-219 + \mathfrak{z}_1 + \mathfrak{z}_2) + \mu_1^2 (344 - 17 \mathfrak{z}_1 + 13 \mathfrak{z}_2) + \\
& \quad \quad \mu_1 \mu_2 (1002 - 187 \mathfrak{z}_1 + 23 \mathfrak{z}_2) + 2 \eta (336 - 80 \mu_2^2 (-4 + 3 \mathfrak{z}_2) + \\
& \quad \quad 6 \mu_2 (177 + 4 \mathfrak{z}_1 + 12 \mathfrak{z}_2) + \mu_1^2 (668 - 5 \mathfrak{z}_1 + 55 \mathfrak{z}_2) + \\
& \quad \quad \mu_1 (1004 - 5 \mathfrak{z}_1 - 2 \mu_2 (-839 + 62 \mathfrak{z}_1 - 70 \mathfrak{z}_2) + 55 \mathfrak{z}_2)) \left. \right) + \\
& \quad 6 \eta^2 (164 + 3 \mu_1^2 (41 + 3 \mathfrak{z}_1 + 3 \mathfrak{z}_2) + \mu_2 (514 + 28 \mathfrak{z}_2) + \\
& \quad \quad \mu_1 (287 + 9 \mathfrak{z}_1 + 9 \mathfrak{z}_2 + \mu_2 (250 + 28 \mathfrak{z}_1 + 28 \mathfrak{z}_2)) \left. \right) \left. \right) - \\
& x^6 \left( -1 + \eta \right)^6 \left( 4 \times \left( -1 + \eta t \right) \theta l \left( (14 + 9 \eta) \mu_1^2 + 8 \mu_2 + \mu_1 (14 + \right. \right. \\
& \quad \quad 56 \mu_2 + \eta (9 + 28 \mu_2)) \left. \right) + \theta p \\
& \quad \left( 14 \eta^3 (11 + 11 \mu_1 + 20 \mu_2) + 2 \eta^2 (121 + 273 \mu_1^2 + 386 \mu_2 - \right. \\
& \quad \quad 84 \mu_2^2 - 7 \eta t (11 + 11 \mu_1 + 20 \mu_2) + \mu_1 (394 + 390 \mu_2)) + \\
& \quad 2 \times \left( -52 - 229 \mu_1 - 177 \mu_1^2 - 144 \mu_2 - 312 \mu_1 \mu_2 - 40 \mu_2^2 + \right. \\
& \quad \quad \theta l \left( 52 + 4 \mu_2 (40 + \mathfrak{z}_1 + 3 \mathfrak{z}_2) - 8 \mu_2^2 (-7 + 5 \mathfrak{z}_2) + \mu_1^2 (107 - 3 \mathfrak{z}_1 + \right. \\
& \quad \quad \quad 7 \mathfrak{z}_2) + \mu_1 (159 - 3 \mathfrak{z}_1 - 4 \mu_2 (-66 + 7 \mathfrak{z}_1 - 4 \mathfrak{z}_2) + 7 \mathfrak{z}_2) \left. \right) + \\
& \quad \quad \eta t \left( 46 + 46 \mu_1 + 68 \mu_2 - 20 \mu_1 \mu_2 - 56 \mu_2^2 + \theta l \left( -52 + \mu_1^2 (-107 + \right. \right. \\
& \quad \quad \quad 3 \mathfrak{z}_1 - 7 \mathfrak{z}_2) + \mu_1 (-159 + 3 \mathfrak{z}_1 + 4 \mu_2 (-66 + 7 \mathfrak{z}_1 - 4 \mathfrak{z}_2) - \\
& \quad \quad \quad 7 \mathfrak{z}_2) - 4 \mu_2 (40 + \mathfrak{z}_1 + 3 \mathfrak{z}_2) + 8 \mu_2^2 (-7 + 5 \mathfrak{z}_2)) \left. \right) \left. \right) + \\
& \quad \eta \left( 2 \eta t \left( 31 + 72 \mu_2 + 56 \mu_2^2 + \mu_1 (31 + 20 \mu_2) \right) - 4 \times \left( 73 + \right. \right. \\
& \quad \quad 48 \mu_1^2 + 191 \mu_2 - 62 \mu_2^2 + \mu_1 (121 + 39 \mu_2)) + \\
& \quad \quad \theta l \left( 304 + 934 \mu_2 + 56 \mu_2 \mathfrak{z}_2 + 3 \mu_1^2 (76 + 3 \mathfrak{z}_1 + 3 \mathfrak{z}_2) + \right. \\
& \quad \quad \quad \mu_1 (532 + 9 \mathfrak{z}_1 + 9 \mathfrak{z}_2 + \mu_2 (446 + 28 \mathfrak{z}_1 + 28 \mathfrak{z}_2)) \left. \right) - \\
& \quad \quad \eta t \theta l \left( 304 + 934 \mu_2 + 56 \mu_2 \mathfrak{z}_2 + 3 \mu_1^2 (76 + 3 \mathfrak{z}_1 + 3 \mathfrak{z}_2) + \right.
\end{aligned}$$

$$\begin{aligned}
& \mu_1 (532 + 9 \mu_1 + 9 \mu_2 + \mu_2 (446 + 28 \mu_1 + 28 \mu_2)) \Big) \Big) \Big) + \\
& x^2 (-1 + \eta)^2 \Big( - \Big( (-1 + \eta) \Theta p \Big( 42 \eta^6 (11 + 11 \mu_1 + 20 \mu_2) + \eta t \\
& \quad (-10 + 10 \mu_1^2 + 207 \mu_2 + 207 \mu_1 \mu_2 + 204 \mu_2^2) - \\
& \quad 2 \eta \eta t (148 + 98 \mu_1^2 - 89 \mu_2 - 204 \mu_2^2 + \mu_1 (246 + 55 \mu_2)) + \\
& \quad 4 \eta (54 + 54 \mu_1^2 + 227 \mu_2 + 136 \mu_2^2 + \mu_1 (108 + 227 \mu_2)) + \\
& \quad 6 \eta^5 (430 + 273 \mu_1^2 + 950 \mu_2 - 420 \mu_2^2 - \\
& \quad 7 \eta t (11 + 11 \mu_1 + 20 \mu_2) + \mu_1 (703 + 270 \mu_2)) + \\
& \quad 4 \eta^3 (553 + 1410 \mu_1^2 + 1693 \mu_2 + 928 \mu_2^2 + \mu_1 (1963 + 3085 \mu_2) + \\
& \quad \eta t (-295 + 95 \mu_1 + 390 \mu_1^2 - 230 \mu_2 + 1622 \mu_1 \mu_2 + 700 \mu_2^2) \Big) + \\
& \quad 10 \eta^4 (322 + 531 \mu_1^2 + 672 \mu_2 - 480 \mu_2^2 + \mu_1 (853 + 752 \mu_2) + \\
& \quad 2 \eta t (-69 + 18 \mu_1^2 - 102 \mu_2 + 84 \mu_2^2 + \mu_1 (-51 + 86 \mu_2)) \Big) + \\
& \quad 6 \eta^2 (186 + 360 \mu_1^2 + 808 \mu_2 + 832 \mu_2^2 + 26 \mu_1 (21 + 44 \mu_2) + \\
& \quad \eta t (-114 + 112 \mu_1^2 - 13 \mu_2 + 198 \mu_2^2 + \mu_1 (-2 + 499 \mu_2)) \Big) \Big) \Big) + \\
& (-1 + \eta t) \Theta l \Big( -2 \times (7 + 7 \mu_1^2 + 48 \mu_2 + 36 \mu_2^2 + 2 \mu_1 (7 + 24 \mu_2)) + \\
& \Theta p \Big( 14 + 17 \mu_1 + 7 \mu_2 + 4 \mu_2^2 (9 \mu_1 + 7 \times (2 + \mu_2)) + \\
& \quad \mu_1^2 (17 \mu_1 + 7 \times (2 + \mu_2)) + \mu_2 (55 \mu_1 + 37 \times (2 + \mu_2)) + \\
& \quad \mu_1 (34 \mu_1 + 55 \mu_2 \mu_1 + 14 \times (2 + \mu_2) + 37 \mu_2 (2 + \mu_2)) \Big) + \\
& \eta^5 \Big( -20 \mu_1 (9 + 9 \mu_1 + 28 \mu_2) + 3 \Theta p \Big( 400 + 1310 \mu_2 + 56 \mu_2 \mu_2 + \\
& \quad 15 \mu_1^2 (20 + 3 \mu_1 + 3 \mu_2) + 5 \mu_1 (140 + 9 \mu_1 + 9 \mu_2) + \\
& \quad 2 \mu_1 \mu_2 (331 + 70 \mu_1 + 70 \mu_2) \Big) \Big) + \\
& 2 \eta^3 \Big( 2 \times (75 + 56 \mu_1^2 + \mu_1 (131 - 247 \mu_2) + 29 \mu_2 - 3 \mu_2^2) + \\
& \Theta p \Big( 614 + 111 \mu_1 + 4 \mu_2^2 (334 + 27 \mu_1 - 303 \mu_2) - 39 \mu_2 + \\
& \quad \mu_2 (2586 + 369 \mu_1 + 19 \mu_2) + 2 \mu_1 (1263 + 61 \mu_1 + 61 \mu_2) + \\
& \quad \mu_1^2 (1912 + 11 \mu_1 + 161 \mu_2) + \mu_1 \mu_2 (5898 - 551 \mu_1 + 499 \mu_2) \Big) \Big) + \\
& 2 \eta^4 \Big( -4 \times (85 \mu_1^2 + 20 \mu_2 + \mu_1 (85 + 324 \mu_2)) + 5 \Theta p \Big( \mu_1^2 (373 + 17 \mu_1 + \\
& \quad 47 \mu_2) + 4 \times (51 + \mu_2^2 (34 - 30 \mu_2) + 3 \mu_2 (57 + \mu_1 + 3 \mu_2)) + \\
& \quad \mu_1 (577 + 17 \mu_1 + 47 \mu_2 + 4 \mu_2 (245 + \mu_1 + 34 \mu_2)) \Big) \Big) + \\
& 2 \eta^2 \Big( 188 + 636 \mu_1 + 448 \mu_1^2 + 83 \mu_2 + 443 \mu_1 \mu_2 - 84 \mu_2^2 + \\
& 3 \Theta p \Big( 74 + 59 \mu_1 + 8 \mu_2^2 (38 + 9 \mu_1 - 28 \mu_2) + \\
& \quad \mu_2 (464 + 169 \mu_1 - 5 \mu_2) - 11 \mu_2 + 2 \mu_1^2 (101 + 6 \mu_1 + \mu_2) + \\
& \quad \mu_1 (276 + 71 \mu_1 - 9 \mu_2 + \mu_2 (840 - 99 \mu_1 + 39 \mu_2)) \Big) \Big) + \\
& \eta \Big( 2 \times (40 + 90 \mu_1^2 + \mu_1 (130 - 59 \mu_2) - 87 \mu_2 - 114 \mu_2^2) + \\
& \Theta p \Big( 4 \mu_2^2 (134 + 63 \mu_1 - 27 \mu_2) + 2 \mu_1^2 (58 + 47 \mu_1 + 2 \mu_2) + \\
& \quad 3 \times (42 + 53 \mu_1 + 3 \mu_2) + \mu_2 (844 + 465 \mu_1 + 123 \mu_2) + \\
& \quad \mu_1 (242 + 253 \mu_1 + 13 \mu_2 + \mu_2 (868 + 141 \mu_1 + 135 \mu_2)) \Big) \Big) \Big) + \\
& \eta \Theta p \Big( -2 \eta^8 (11 + 11 \mu_1 + 20 \mu_2) + 2 \eta^7 (-67 - 39 \mu_1^2 - 146 \mu_2 + \\
& \quad 84 \mu_2^2 - 2 \mu_1 (53 + 15 \mu_2) + \eta t (11 + 11 \mu_1 + 20 \mu_2)) + 2 \\
& \eta t (7 + 7 \mu_1^2 + 48 \mu_2 + 36 \mu_2^2 + 2 \mu_1 (7 + 24 \mu_2)) + \eta \\
& \Big( -\Theta l \Big( 14 + 17 \mu_1 + 7 \mu_2 + 4 \mu_2^2 (9 \mu_1 + 7 \times (2 + \mu_2)) + \\
& \quad \mu_1^2 (17 \mu_1 + 7 \times (2 + \mu_2)) + \mu_2 (55 \mu_1 + 37 \times (2 + \mu_2)) + \\
& \quad \mu_1 (34 \mu_1 + 55 \mu_2 \mu_1 + 14 \times (2 + \mu_2) + 37 \mu_2 (2 + \mu_2)) \Big) + \\
& \eta t (-28 - 96 \mu_1 - 68 \mu_1^2 + 95 \mu_2 + 71 \mu_1 \mu_2 + 120 \mu_2^2 + \\
& \Theta l \Big( 14 + 17 \mu_1 + 7 \mu_2 + 4 \mu_2^2 (9 \mu_1 + 7 \times (2 + \mu_2)) +
\end{aligned}$$

$$\begin{aligned}
& \mu_1^2 (17 \mathfrak{e}_1 + 7 \times (2 + \mathfrak{e}_2)) + \mu_2 (55 \mathfrak{e}_1 + 37 \times (2 + \mathfrak{e}_2)) + \\
& \mu_1 (34 \mathfrak{e}_1 + 55 \mu_2 \mathfrak{e}_1 + 14 \times (2 + \mathfrak{e}_2) + 37 \mu_2 (2 + \mathfrak{e}_2)) \Big) \Big) + \\
& \eta^6 \Big( -2 \times (57 + 138 \mu_1^2 + 98 \mu_2 - 176 \mu_2^2 + 5 \mu_1 (39 + 38 \mu_2)) - \\
& \mathfrak{e}_l (64 + 214 \mu_2 + 8 \mu_2 \mathfrak{e}_2 + \mu_1^2 (48 + 9 \mathfrak{e}_1 + 9 \mathfrak{e}_2) + \\
& \mu_1 (112 + 9 \mathfrak{e}_1 + 9 \mathfrak{e}_2 + 2 \mu_2 (55 + 14 \mathfrak{e}_1 + 14 \mathfrak{e}_2)) \Big) + \\
& \eta t (70 + 34 \mu_1 - 36 \mu_1^2 + 96 \mu_2 - 152 \mu_1 \mu_2 - 112 \mu_2^2 + \\
& \mathfrak{e}_l (64 + 214 \mu_2 + 8 \mu_2 \mathfrak{e}_2 + \mu_1^2 (48 + 9 \mathfrak{e}_1 + 9 \mathfrak{e}_2) + \\
& \mu_1 (112 + 9 \mathfrak{e}_1 + 9 \mathfrak{e}_2 + 2 \mu_2 (55 + 14 \mathfrak{e}_1 + 14 \mathfrak{e}_2)) \Big) \Big) \Big) + 2 \\
& \eta^5 (10 - 95 \mu_1 - 105 \mu_1^2 - 101 \mu_2 - 385 \mu_1 \mu_2 - 324 \mu_2^2 - \\
& \mathfrak{e}_l (76 - 40 \mu_2^2 (-1 + \mathfrak{e}_2) + 2 \mu_2 (131 + 2 \mathfrak{e}_1 + 6 \mathfrak{e}_2) + \\
& \mu_1^2 (133 + 10 \mathfrak{e}_1 + 20 \mathfrak{e}_2) + \mu_1 (209 + 10 \mathfrak{e}_1 + 20 \mathfrak{e}_2 + \\
& 2 \mu_2 (179 + 8 \mathfrak{e}_1 + 30 \mathfrak{e}_2)) \Big) + \eta t (13 - 67 \mu_1 - 80 \mu_1^2 - \\
& 22 \mu_2 - 322 \mu_1 \mu_2 - 84 \mu_2^2 + \mathfrak{e}_l (76 - 40 \mu_2^2 (-1 + \mathfrak{e}_2) + \\
& 2 \mu_2 (131 + 2 \mathfrak{e}_1 + 6 \mathfrak{e}_2) + \mu_1^2 (133 + 10 \mathfrak{e}_1 + 20 \mathfrak{e}_2) + \\
& \mu_1 (209 + 10 \mathfrak{e}_1 + 20 \mathfrak{e}_2 + 2 \mu_2 (179 + 8 \mathfrak{e}_1 + 30 \mathfrak{e}_2)) \Big) \Big) \Big) + \\
& \eta^2 (4 \times (18 + 18 \mu_1^2 + 79 \mu_2 + 40 \mu_2^2 + \mu_1 (36 + 79 \mu_2)) - \\
& \mathfrak{e}_l (58 + 61 \mathfrak{e}_1 + 12 \mu_2^2 (18 + 9 \mathfrak{e}_1 - \mathfrak{e}_2) + 11 \mathfrak{e}_2 + \\
& 6 \mu_1^2 (8 + 6 \mathfrak{e}_1 + \mathfrak{e}_2) + \mu_2 (352 + 187 \mathfrak{e}_1 + 73 \mathfrak{e}_2) + \\
& \mu_1 (106 + 97 \mathfrak{e}_1 + 17 \mathfrak{e}_2 + \mu_2 (344 + 71 \mathfrak{e}_1 + 69 \mathfrak{e}_2)) \Big) + \\
& \eta t (-74 - 208 \mu_1 - 134 \mu_1^2 - 89 \mu_2 - 177 \mu_1 \mu_2 - 24 \mu_2^2 + \\
& \mathfrak{e}_l (58 + 61 \mathfrak{e}_1 + 12 \mu_2^2 (18 + 9 \mathfrak{e}_1 - \mathfrak{e}_2) + 11 \mathfrak{e}_2 + \\
& 6 \mu_1^2 (8 + 6 \mathfrak{e}_1 + \mathfrak{e}_2) + \mu_2 (352 + 187 \mathfrak{e}_1 + 73 \mathfrak{e}_2) + \\
& \mu_1 (106 + 97 \mathfrak{e}_1 + 17 \mathfrak{e}_2 + \mu_2 (344 + 71 \mathfrak{e}_1 + 69 \mathfrak{e}_2)) \Big) \Big) \Big) + \\
& \eta^3 (114 + 402 \mu_1 + 288 \mu_1^2 + 534 \mu_2 + 870 \mu_1 \mu_2 + 592 \mu_2^2 - \\
& \mathfrak{e}_l (98 + 71 \mathfrak{e}_1 + 4 \mu_2^2 (86 + 27 \mathfrak{e}_1 - 47 \mathfrak{e}_2) + \mathfrak{e}_2 + \\
& \mu_1^2 (224 + 23 \mathfrak{e}_1 + 13 \mathfrak{e}_2) + \mu_2 (578 + 217 \mathfrak{e}_1 + 43 \mathfrak{e}_2) + \\
& \mu_1 (322 + 94 \mathfrak{e}_1 + 14 \mathfrak{e}_2 + \mu_2 (962 - 47 \mathfrak{e}_1 + 91 \mathfrak{e}_2)) \Big) + \\
& \eta t (-20 + 248 \mu_1 + 268 \mu_1^2 - 91 \mu_2 + 685 \mu_1 \mu_2 + 48 \mu_2^2 + \\
& \mathfrak{e}_l (98 + 71 \mathfrak{e}_1 + 4 \mu_2^2 (86 + 27 \mathfrak{e}_1 - 47 \mathfrak{e}_2) + \mathfrak{e}_2 + \\
& \mu_1^2 (224 + 23 \mathfrak{e}_1 + 13 \mathfrak{e}_2) + \mu_2 (578 + 217 \mathfrak{e}_1 + 43 \mathfrak{e}_2) + \\
& \mu_1 (322 + 94 \mathfrak{e}_1 + 14 \mathfrak{e}_2 + \mu_2 (962 - 47 \mathfrak{e}_1 + 91 \mathfrak{e}_2)) \Big) \Big) \Big) + \\
& \eta^4 (4 \times (16 + 67 \mu_1 + 51 \mu_1^2 - 30 \mu_2 + 6 \mu_1 \mu_2 - 156 \mu_2^2) - \\
& \mathfrak{e}_l (142 + 27 \mathfrak{e}_1 + 12 \mu_2^2 (22 + 3 \mathfrak{e}_1 - 19 \mathfrak{e}_2) - 3 \mathfrak{e}_2 + \\
& 3 \mu_1^2 (136 + 5 \mathfrak{e}_1 + 15 \mathfrak{e}_2) + \mu_2 (610 + 93 \mathfrak{e}_1 + 23 \mathfrak{e}_2) + \\
& \mu_1 (550 + 42 \mathfrak{e}_1 + 42 \mathfrak{e}_2 + \mu_2 (1298 - 59 \mathfrak{e}_1 + 151 \mathfrak{e}_2)) \Big) + \\
& \eta t (-10 + 106 \mu_1 + 116 \mu_1^2 - 103 \mu_2 + 121 \mu_1 \mu_2 + 64 \mu_2^2 + \\
& \mathfrak{e}_l (142 + 27 \mathfrak{e}_1 + 12 \mu_2^2 (22 + 3 \mathfrak{e}_1 - 19 \mathfrak{e}_2) - 3 \mathfrak{e}_2 + \\
& 3 \mu_1^2 (136 + 5 \mathfrak{e}_1 + 15 \mathfrak{e}_2) + \mu_2 (610 + 93 \mathfrak{e}_1 + 23 \mathfrak{e}_2) + \\
& \mu_1 (550 + 42 \mathfrak{e}_1 + 42 \mathfrak{e}_2 + \mu_2 (1298 - 59 \mathfrak{e}_1 + 151 \mathfrak{e}_2)) \Big) \Big) \Big) \Big) + \\
& x^4 (-1 + \eta)^4 \Big( - \Big( (-1 + \eta) \mathfrak{e}_p (70 \eta^4 (11 + 11 \mu_1 + 20 \mu_2) + \eta t \\
& (-120 + 24 \mu_1 + 144 \mu_1^2 - 37 \mu_2 + 323 \mu_1 \mu_2 + 180 \mu_2^2) + \\
& 2 \times (93 + 273 \mu_1 + 180 \mu_1^2 + 383 \mu_2 + 551 \mu_1 \mu_2 + 456 \mu_2^2) + \\
& 10 \eta^3 (314 + 587 \mu_1 + 273 \mu_1^2 + 738 \mu_2 + 330 \mu_1 \mu_2 -
\end{aligned}$$

$$\begin{aligned}
& 252 \mu_2^2 - 7 \eta t (11 + 11 \mu_1 + 20 \mu_2) + \\
& 10 \eta^2 (239 + 770 \mu_1 + 531 \mu_1^2 + 552 \mu_2 + 844 \mu_1 \mu_2 - 180 \mu_2^2 + \\
& 2 \eta t (-69 - 60 \mu_1 + 9 \mu_1^2 - 102 \mu_2 + 58 \mu_1 \mu_2 + 84 \mu_2^2)) + \\
& 2 \eta (481 + 1891 \mu_1 + 1410 \mu_1^2 + 1561 \mu_2 + 3145 \mu_1 \mu_2 + 1536 \mu_2^2 + \\
& \eta t (-295 - 5 \mu_1 + 290 \mu_1^2 - 230 \mu_2 + 1254 \mu_1 \mu_2 + 700 \mu_2^2))) + \\
& (-1 + \eta t) \theta l (2 \times (68 + 88 \mu_1^2 + 49 \mu_2 - 12 \mu_2^2 + \mu_1 (156 + 161 \mu_2)) + \\
& \theta p (50 + 47 \mu_1 + 4 \mu_2^2 (66 + 9 \mu_1 - 65 \mu_2) + \mu_2 (350 + 121 \mu_1 - 53 \mu_2) + \\
& \mu_1 (230 + 48 \mu_1 + \mu_2 (718 - 151 \mu_1 - 13 \mu_2) - 32 \mu_2) + \\
& \mu_1^2 (180 + \mu_1 - 9 \mu_2) - 23 \mu_2) + 5 \eta^3 (-8 \mu_1 (9 + 9 \mu_1 + 28 \mu_2) + \\
& \theta p (352 + 1122 \mu_2 + 56 \mu_2 \mu_2 + 3 \mu_1^2 (88 + 9 \mu_1 + 9 \mu_2) + \\
& \mu_1 (616 + 27 \mu_1 + 27 \mu_2 + \mu_2 (554 + 84 \mu_1 + 84 \mu_2))) + 2 \eta^2 \\
& (-32 \times (15 \mu_1^2 + 5 \mu_2 + \mu_1 (15 + 58 \mu_2)) + 5 \theta p (\mu_1^2 (347 + 4 \mu_1 + 34 \\
& \mu_2) + 2 \times (90 + \mu_2^2 (76 - 60 \mu_2) + 3 \mu_2 (97 + 2 \mu_1 + 6 \mu_2)) + \\
& \mu_1 (527 + 4 \mu_1 + 34 \mu_2 + \mu_2 (886 - 40 \mu_1 + 92 \mu_2))) + \\
& \eta (4 \times (81 + 24 \mu_1^2 + \mu_1 (105 - 71 \mu_2) + 53 \mu_2 + 15 \mu_2^2) + \\
& \theta p (518 + 87 \mu_1 + 4 \mu_2^2 (338 + 9 \mu_1 - 321 \mu_2) + \\
& \mu_2 (2122 + 273 \mu_1 - 77 \mu_2) - 63 \mu_2 + \mu_1^2 (1784 - 53 \mu_1 + 97 \mu_2) + \\
& \mu_1 (2302 + 34 \mu_1 + 34 \mu_2 + \mu_2 (5306 - 807 \mu_1 + 243 \mu_2)))) - \\
& x^3 (-1 + \eta)^3 (-2 \times (-1 + \eta) \theta p (35 \eta^5 (11 + 11 \mu_1 + 20 \mu_2) - \eta t \\
& (52 + 54 \mu_1 + 2 \mu_1^2 - 19 \mu_2 + 25 \mu_1 \mu_2 - 60 \mu_2^2) + \\
& 4 \times (9 + 18 \mu_1 + 9 \mu_1^2 + 37 \mu_2 + 37 \mu_1 \mu_2 + 24 \mu_2^2) + \\
& 5 \eta^4 (372 + 645 \mu_1 + 273 \mu_1^2 + 844 \mu_2 + 300 \mu_1 \mu_2 - \\
& 336 \mu_2^2 - 7 \eta t (11 + 11 \mu_1 + 20 \mu_2)) + \\
& 10 \eta^3 (187 + 541 \mu_1 + 354 \mu_1^2 + 408 \mu_2 + 532 \mu_1 \mu_2 - 220 \mu_2^2 + \\
& 2 \eta t (-46 - 37 \mu_1 + 9 \mu_1^2 - 68 \mu_2 + 48 \mu_1 \mu_2 + 56 \mu_2^2)) + \\
& 2 \eta (186 + 546 \mu_1 + 360 \mu_1^2 + 787 \mu_2 + 1123 \mu_1 \mu_2 + 872 \mu_2^2 + \\
& \eta t (-117 + 11 \mu_1 + 128 \mu_1^2 - 25 \mu_2 + 411 \mu_1 \mu_2 + 189 \mu_2^2)) + \\
& 2 \eta^2 (517 + 1927 \mu_1 + 1410 \mu_1^2 + 1627 \mu_2 + 3115 \mu_1 \mu_2 + 1232 \mu_2^2 + \\
& \eta t (-295 + 45 \mu_1 + 340 \mu_1^2 - 230 \mu_2 + 1438 \mu_1 \mu_2 + 700 \mu_2^2))) + \\
& (-1 + \eta t) \theta l (38 + 96 \mu_1 + 58 \mu_1^2 - 95 \mu_2 - 79 \mu_1 \mu_2 - 120 \mu_2^2 + \\
& \theta p (34 + 49 \mu_1 + 8 \mu_2^2 (20 + 9 \mu_1 - 6 \mu_2) + \mu_1^2 (34 + 29 \mu_1 - \mu_2) - \\
& \mu_2 + \mu_2 (246 + 139 \mu_1 + 25 \mu_2) + \mu_1 (68 + 78 \mu_1 - 2 \mu_2 + \\
& \mu_2 (262 + 35 \mu_1 + 33 \mu_2))) + 10 \eta^4 (-4 \mu_1 (9 + 9 \mu_1 + 28 \mu_2) + \\
& \theta p (3 \mu_1^2 (47 + 6 \mu_1 + 6 \mu_2) + 4 \times (47 + \mu_2 (152 + 7 \mu_2)) + \\
& \mu_1 (329 + 18 \mu_1 + 18 \mu_2 + 8 \mu_2 (38 + 7 \mu_1 + 7 \mu_2))) + \\
& 2 \eta (196 + 356 \mu_1^2 + 115 \mu_2 - 60 \mu_2^2 + \mu_1 (552 + 463 \mu_2) + \\
& \theta p (2 \times (62 + 53 \mu_1 + \mu_2^2 (284 + 54 \mu_1 - 242 \mu_2) + \mu_2 \\
& (407 + 145 \mu_1 - 29 \mu_2) - 17 \mu_2) + \mu_1^2 (382 + 13 \mu_1 - 7 \mu_2) + \\
& \mu_1 (506 + 119 \mu_1 - 41 \mu_2 + \mu_2 (1558 - 250 \mu_1 + 26 \mu_2))) + \\
& 4 \eta^3 (-2 \times (145 \mu_1^2 + 40 \mu_2 + \mu_1 (145 + 556 \mu_2)) + 5 \theta p (128 + \\
& \mu_2^2 (96 - 80 \mu_2) + \mu_2 (422 + 8 \mu_1 + 24 \mu_2) + \mu_1^2 (240 + 7 \mu_1 + 27 \\
& \mu_2) + \mu_1 (368 + 7 \mu_1 + 27 \mu_2 + \mu_2 (622 - 12 \mu_1 + 76 \mu_2))) + \\
& \eta^2 (6 \times (78 + 40 \mu_1^2 + \mu_1 (118 - 159 \mu_2) + 41 \mu_2 + 6 \mu_2^2) +
\end{aligned}$$

$$\begin{aligned}
& 2 \, \text{op} \left( 566 + 99 \, \mathfrak{e}1 + 24 \, \mu^2 \left( 56 + 3 \, \mathfrak{e}1 - 52 \, \mathfrak{e}2 \right) - \right. \\
& \quad \left. 3 \, \mu^2 \left( -616 + 7 \, \mathfrak{e}1 - 43 \, \mathfrak{e}2 \right) + \mu^2 \left( 2354 + 321 \, \mathfrak{e}1 - 29 \, \mathfrak{e}2 \right) - 51 \, \mathfrak{e}2 + \right. \\
& \quad \left. \mu^1 \left( 2414 + 78 \, \mathfrak{e}1 + 78 \, \mathfrak{e}2 + \mu^2 \left( 5602 - 679 \, \mathfrak{e}1 + 371 \, \mathfrak{e}2 \right) \right) \right) + \\
& \times (-1 + \eta) \times \left( 14 \, \eta^8 \, \text{op} \left( 11 + 11 \, \mu^1 + 20 \, \mu^2 \right) + 2 \, \eta^7 \, \text{op} \left( 411 + 273 \, \mu^1 + \right. \right. \\
& \quad \left. \left. 916 \, \mu^2 - 504 \, \mu^2 + 12 \, \mu^1 \left( 57 + 20 \, \mu^2 \right) - 7 \, \eta \mathfrak{t} \left( 11 + 11 \, \mu^1 + 20 \, \mu^2 \right) \right) - 2 \right. \\
& \quad \left. \eta \mathfrak{t} \, \text{op} \left( 11 + 11 \, \mu^1 + 64 \, \mu^2 + 48 \, \mu^2 + \mu^1 \left( 22 + 64 \, \mu^2 \right) \right) - \eta^2 \right. \\
& \quad \left( 4 \, \text{op} \left( 54 + 54 \, \mu^1 + 232 \, \mu^2 + 128 \, \mu^2 + 4 \, \mu^1 \left( 27 + 58 \, \mu^2 \right) - \right. \right. \\
& \quad \left. \left. \eta \mathfrak{t} \left( 64 + 84 \, \mu^1 + 39 \, \mu^2 - 15 \, \mu^2 + 37 \, \mu^1 \left( 4 + 3 \, \mu^2 \right) \right) \right) + \right. \\
& \quad \left( -1 + \eta \mathfrak{t} \right) \, \text{el} \left( 42 + 164 \, \mu^1 + 122 \, \mu^1 - 79 \, \mu^2 - 39 \, \mu^1 \, \mu^2 - 108 \, \mu^2 + \right. \\
& \quad \left. \text{op} \left( 8 \, \mu^2 \left( 74 + 36 \, \mathfrak{e}1 - 9 \, \mathfrak{e}2 \right) + 8 \, \mu^1 \left( 35 + 34 \, \mathfrak{e}1 + 4 \, \mathfrak{e}2 \right) + \right. \right. \\
& \quad \left. \left. 3 \times \left( 50 + 57 \, \mathfrak{e}1 + 7 \, \mathfrak{e}2 \right) + 19 \, \mu^2 \left( 50 + 27 \, \mathfrak{e}1 + 9 \, \mathfrak{e}2 \right) + \right. \right. \\
& \quad \left. \left. \mu^1 \left( 130 + 101 \, \mathfrak{e}1 + 11 \, \mathfrak{e}2 \right) + \mu^1 \, \mu^2 \left( 950 + 177 \, \mathfrak{e}1 + 171 \, \mathfrak{e}2 \right) \right) \right) - \\
& \eta^4 \left( 2 \, \text{op} \left( 217 + 690 \, \mu^1 + 101 \, \mu^2 - 960 \, \mu^2 + \mu^1 \left( 907 + 725 \, \mu^2 \right) + \right. \right. \\
& \quad \left. \left. \eta \mathfrak{t} \left( -73 + 248 \, \mu^1 - 228 \, \mu^2 + 286 \, \mu^2 + \mu^1 \left( 175 + 632 \, \mu^2 \right) \right) \right) + \right. \\
& \quad \left( -1 + \eta \mathfrak{t} \right) \, \text{el} \left( 72 + 144 \, \mu^1 + 72 \, \mu^1 + 17 \, \mu^2 - 335 \, \mu^1 \, \mu^2 - 12 \, \mu^2 + \right. \\
& \quad \left. \text{op} \left( 662 + 123 \, \mathfrak{e}1 + 8 \, \mu^2 \left( 166 + 18 \, \mathfrak{e}1 - 147 \, \mathfrak{e}2 \right) - 27 \, \mathfrak{e}2 + \right. \right. \\
& \quad \left. \left. \mu^2 \left( 2818 + 417 \, \mathfrak{e}1 + 67 \, \mathfrak{e}2 \right) + 2 \, \mu^1 \left( 1319 + 83 \, \mathfrak{e}1 + 83 \, \mathfrak{e}2 \right) + \mu^1 \right. \right. \\
& \quad \left. \left. \left( 1976 + 43 \, \mathfrak{e}1 + 193 \, \mathfrak{e}2 \right) + \mu^1 \, \mu^2 \left( 6194 - 423 \, \mathfrak{e}1 + 627 \, \mathfrak{e}2 \right) \right) \right) - \\
& 2 \, \eta \left( \eta \mathfrak{t} \, \text{op} \left( -23 - 33 \, \mu^1 + 135 \, \mu^2 + 150 \, \mu^2 + \mu^1 \left( -56 + 123 \, \mu^2 \right) \right) + \right. \\
& \quad \left( -1 + \eta \mathfrak{t} \right) \, \text{el} \left( -3 - 6 \, \mu^1 - 3 \, \mu^1 - 32 \, \mu^2 - 32 \, \mu^1 \, \mu^2 - 24 \, \mu^2 + \right. \\
& \quad \left. \text{op} \left( 14 + 17 \, \mathfrak{e}1 + 7 \, \mathfrak{e}2 + 4 \, \mu^2 \left( 9 \, \mathfrak{e}1 + 7 \times \left( 2 + \mathfrak{e}2 \right) \right) + \right. \right. \\
& \quad \left. \left. \mu^1 \left( 17 \, \mathfrak{e}1 + 7 \times \left( 2 + \mathfrak{e}2 \right) \right) + \mu^2 \left( 55 \, \mathfrak{e}1 + 37 \times \left( 2 + \mathfrak{e}2 \right) \right) + \right. \right. \\
& \quad \left. \left. \mu^1 \left( 34 \, \mathfrak{e}1 + 55 \, \mu^2 \, \mathfrak{e}1 + 14 \times \left( 2 + \mathfrak{e}2 \right) + 37 \, \mu^2 \left( 2 + \mathfrak{e}2 \right) \right) \right) \right) - 2 \, \eta^3 \\
& \left( \text{op} \left( \eta \mathfrak{t} \left( -82 + 382 \, \mu^1 - 123 \, \mu^2 + 186 \, \mu^2 + 3 \, \mu^1 \left( 100 + 403 \, \mu^2 \right) \right) + \right. \right. \\
& \quad \left. \left. 2 \times \left( 132 + 306 \, \mu^1 + 597 \, \mu^2 + 664 \, \mu^2 + \mu^1 \left( 438 + 933 \, \mu^2 \right) \right) \right) + \right. \\
& \quad \left( -1 + \eta \mathfrak{t} \right) \, \text{el} \left( 60 + 180 \, \mu^1 + 17 \, \mu^2 - 36 \, \mu^2 + 3 \, \mu^1 \left( 80 + 47 \, \mu^2 \right) + \right. \\
& \quad \left. \text{op} \left( \mu^1 \left( 598 + 165 \, \mathfrak{e}1 - 2 \, \mu^2 \left( -901 + 73 \, \mathfrak{e}1 - 65 \, \mathfrak{e}2 \right) + 5 \, \mathfrak{e}2 \right) + \right. \right. \\
& \quad \left. \left. \mu^1 \left( 426 + 35 \, \mathfrak{e}1 + 15 \, \mathfrak{e}2 \right) + 2 \times \left( 86 + 65 \, \mathfrak{e}1 + \mu^2 \left( 324 + 90 \, \mathfrak{e}1 - \right. \right. \right. \\
& \quad \left. \left. \left. 206 \, \mathfrak{e}2 \right) - 5 \, \mathfrak{e}2 + \mu^2 \left( 521 + 193 \, \mathfrak{e}1 + 19 \, \mathfrak{e}2 \right) \right) \right) \right) - 2 \, \eta^6 \\
& \left( -2 \times \left( -1 + \eta \mathfrak{t} \right) \, \text{el} \, \mu^1 \left( 9 + 9 \, \mu^1 + 28 \, \mu^2 \right) + \text{op} \left( -239 - 1028 \, \mu^1 - \right. \right. \\
& \quad \left. \left. 789 \, \mu^1 - 408 \, \mu^2 - 1172 \, \mu^1 \, \mu^2 + 756 \, \mu^2 - \right. \right. \\
& \quad \left. \left. \text{el} \left( 212 + 702 \, \mu^2 + 28 \, \mu^2 \, \mathfrak{e}2 + 3 \, \mu^1 \left( 53 + 9 \, \mathfrak{e}1 + 9 \, \mathfrak{e}2 \right) + \right. \right. \right. \\
& \quad \left. \left. \left. \mu^1 \left( 371 + 27 \, \mathfrak{e}1 + 27 \, \mathfrak{e}2 + \mu^2 \left( 358 + 84 \, \mathfrak{e}1 + 84 \, \mathfrak{e}2 \right) \right) \right) \right) + \right. \\
& \quad \left. \eta \mathfrak{t} \left( 199 + 109 \, \mu^1 - 90 \, \mu^1 + 268 \, \mu^2 - 400 \, \mu^1 \, \mu^2 - 336 \, \mu^2 + \right. \right. \\
& \quad \left. \left. \text{el} \left( 212 + 702 \, \mu^2 + 28 \, \mu^2 \, \mathfrak{e}2 + 3 \, \mu^1 \left( 53 + 9 \, \mathfrak{e}1 + 9 \, \mathfrak{e}2 \right) + \right. \right. \right. \\
& \quad \left. \left. \left. \mu^1 \left( 371 + 27 \, \mathfrak{e}1 + 27 \, \mathfrak{e}2 + \mu^2 \left( 358 + 84 \, \mathfrak{e}1 + 84 \, \mathfrak{e}2 \right) \right) \right) \right) \right) - \\
& 2 \, \eta^5 \left( -2 \times \left( -1 + \eta \mathfrak{t} \right) \, \text{el} \left( 39 \, \mu^1 + 8 \, \mu^2 + \mu^1 \left( 39 + 148 \, \mu^2 \right) \right) + \right. \\
& \quad \left. \text{op} \left( 138 - 210 \, \mu^1 - 348 \, \mu^1 - 295 \, \mu^2 - 1643 \, \mu^1 \, \mu^2 - \right. \right. \\
& \quad \left. \left. 1884 \, \mu^2 - \text{el} \left( 432 + \mu^2 \left( 256 - 240 \, \mathfrak{e}2 \right) + \right. \right. \right. \\
& \quad \left. \left. \left. 6 \, \mu^2 \left( 245 + 4 \, \mathfrak{e}1 + 12 \, \mathfrak{e}2 \right) + \mu^1 \left( 772 + 47 \, \mathfrak{e}1 + 107 \, \mathfrak{e}2 \right) + \right. \right. \right. \\
& \quad \left. \left. \left. \mu^1 \left( 1204 + 47 \, \mathfrak{e}1 + 107 \, \mathfrak{e}2 + \mu^2 \left( 2054 + 52 \, \mathfrak{e}1 + 316 \, \mathfrak{e}2 \right) \right) \right) \right) + \right. \\
& \quad \left. \eta \mathfrak{t} \left( 19 - 331 \, \mu^1 - 350 \, \mu^1 - 178 \, \mu^2 - 1406 \, \mu^1 \, \mu^2 - 364 \, \mu^2 + \right. \right. \\
& \quad \left. \left. \text{el} \left( 432 + \mu^2 \left( 256 - 240 \, \mathfrak{e}2 \right) + 6 \, \mu^2 \left( 245 + 4 \, \mathfrak{e}1 + 12 \, \mathfrak{e}2 \right) + \right. \right. \right.
\end{aligned}$$

$$\begin{aligned}
& \left( \mu_1^2 (772 + 47 \mathfrak{x}1 + 107 \mathfrak{x}2) + \mu_1 (1204 + 47 \mathfrak{x}1 + 107 \mathfrak{x}2 + \mu_2 (2054 + 52 \mathfrak{x}1 + 316 \mathfrak{x}2)) \right) / \\
& (96 (-1 + w (-1 + \eta))^3 (x (-1 + \eta) - \eta)^3 (1 + x + \eta - x \eta)^2 \\
& (w + \\
& \quad x + \\
& \quad \eta - \\
& \quad w \\
& \quad \eta - x \\
& \quad \eta)^3 (-1 + \eta t) \theta l \theta p \mathfrak{x}1) \Big) \\
\delta_{gs2} = & - \left( \left( (-1 + \eta) \times (-2 f (-1 + w (-1 + \eta)) (x (-1 + \eta) - \eta) (w (-1 + \eta) + x (-1 + \eta) - \eta) (1 + x + \eta - x \eta)^2 \theta l (-x^2 (-1 + \eta)^2 \theta p (-12 + 4 \eta t + 12 \theta l - 12 \eta t \theta l + \eta^2 (8 - 20 \mathfrak{x}2) - 6 \mathfrak{x}2 - 10 \eta t \mathfrak{x}2 + 16 \theta l \mathfrak{x}2 - 16 \eta t \theta l \mathfrak{x}2 - 7 \theta l \mathfrak{x}2^2 + 7 \eta t \theta l \mathfrak{x}2^2 + 2 \eta (2 + \theta l (2 - 5 \mathfrak{x}2) + 13 \mathfrak{x}2 + \eta t (1 + \theta l) \times (-2 + 5 \mathfrak{x}2)) + w (-1 + \eta) \times (2 \eta^2 (-2 + 5 \mathfrak{x}2) + (-10 + 7 \mathfrak{x}2) \times (-2 + \theta l (2 + \mathfrak{x}2)) - 2 \eta (8 - 2 \mathfrak{x}2 + \eta t (-2 + 5 \mathfrak{x}2)) + \eta t (-4 + 10 \mathfrak{x}2 + \theta l (20 - 4 \mathfrak{x}2 - 7 \mathfrak{x}2^2))) \right) + \theta p (4 \eta^4 (-2 + 5 \mathfrak{x}2) + 2 \eta t (-10 + 7 \mathfrak{x}2) + 2 w^2 (-1 + \eta)^3 (\eta - \eta t) (-10 + 7 \mathfrak{x}2 + \eta (-2 + 5 \mathfrak{x}2)) - 2 \eta^3 (2 + \theta l (2 - 5 \mathfrak{x}2) + 13 \mathfrak{x}2 + \eta t (1 + \theta l) \times (-2 + 5 \mathfrak{x}2)) + \eta (-10 + 7 \mathfrak{x}2) (-\theta l (2 + \mathfrak{x}2) + \eta t (-2 + \theta l (2 + \mathfrak{x}2))) + \eta^2 (6 \times (2 + \mathfrak{x}2) + \theta l (-12 - 16 \mathfrak{x}2 + 7 \mathfrak{x}2^2) + \eta t (-4 + 10 \mathfrak{x}2 + \theta l (12 + 16 \mathfrak{x}2 - 7 \mathfrak{x}2^2))) \right) - w (-1 + \eta) (\eta^3 (\eta t (4 - 10 \mathfrak{x}2) + 24 \times (-1 + \mathfrak{x}2)) + 2 \eta^4 (-2 + 5 \mathfrak{x}2) + 4 \eta t (-10 + 7 \mathfrak{x}2) + \eta^2 (16 - 40 \mathfrak{x}2 - (-1 + \eta t) \theta l (-24 + 14 \mathfrak{x}2 + 7 \mathfrak{x}2^2)) + \eta (-18 \eta t (-2 + \mathfrak{x}2) + 6 \times (2 + \mathfrak{x}2) + \theta l (28 - 24 \mathfrak{x}2 - 7 \mathfrak{x}2^2) + \eta t \theta l (-28 + 24 \mathfrak{x}2 + 7 \mathfrak{x}2^2))) \right) + x (-1 + \eta) \times (-2 (w (-1 + \eta) - 2 \eta) (-1 + \eta) \theta p (6 - 2 \eta t + \eta (4 - 10 \mathfrak{x}2) + 3 \mathfrak{x}2 + 5 \eta t \mathfrak{x}2 + w (-1 + \eta) \times (-10 + 2 \eta t + 7 \mathfrak{x}2 - 5 \eta t \mathfrak{x}2 + \eta (-2 + 5 \mathfrak{x}2))) + (-1 + \eta t) \theta l (-20 + 14 \mathfrak{x}2 + 2 w^2 (-1 + \eta)^2 (-10 + 7 \mathfrak{x}2) + \theta p (20 - 4 \mathfrak{x}2 - 7 \mathfrak{x}2^2 + 4 \eta^2 (-2 + 5 \mathfrak{x}2) + 2 \eta (-12 - 16 \mathfrak{x}2 + 7 \mathfrak{x}2^2)) - w (-1 + \eta) \times (-40 + 28 \mathfrak{x}2 + \theta p (28 - 24 \mathfrak{x}2 - 7 \mathfrak{x}2^2 + 2 \eta (-22 + 9 \mathfrak{x}2 + 7 \mathfrak{x}2^2))) \right) + cv c\sigma (x (-1 + \eta) - \eta) (1 + x + \eta - x \eta)^2 ((x + \eta - x \eta)^2 (-1 + \eta t) \theta l \theta p (1 + \mu_1) \times (14 x (-1 + \eta) - 14 \eta - 5 \times (2 + \mathfrak{x}1 + \mathfrak{x}2)) + w^4 (-1 + \eta)^4 (\theta p (-4 \eta^3 (1 + \mu_1) - 20 \eta t (1 + \mu_1) + 4 \eta^2 (6 + \eta t - 6 \mu_1 + \eta t \mu_1) + \eta (16 \eta t (1 + \mu_1) + 4 \times (-5 + 7 \mu_1) + \theta l (64 + 15 \mathfrak{x}1 + \mu_1 (16 + 15 \mathfrak{x}1 - 29 \mathfrak{x}2) + 19 \mathfrak{x}2) - \eta t \theta l (64 + 15 \mathfrak{x}1 + \mu_1 (16 + 15 \mathfrak{x}1 - 29 \mathfrak{x}2) + 19 \mathfrak{x}2))) + x (-1 + \eta) \times (4 \times (-1 + \eta) \theta p (-5 + 7 \mu_1 + \eta (1 + \mu_1) - \eta t (1 + \mu_1)) + (-1 + \eta t) \theta l (-20 \times (1 + \mu_1) + \theta p (64 + 15 \mathfrak{x}1 + \mu_1 (16 + 15 \mathfrak{x}1 - 29 \mathfrak{x}2) + 19 \mathfrak{x}2))) \Big) + w (-1 + \eta) \times (-4 x^3 (-1 + \eta)^3 \theta p (7 - 14 \theta l - 5 \mu_1 - 2 \theta l \mu_1 + 3 \eta^2 (1 + \mu_1) - \eta \eta t (1 + 2 \theta l) \times (1 + \mu_1) + 2 \eta (-5 + \theta l + \mu_1 + \theta l \mu_1) + \eta t (1 + \mu_1 + 2 \theta l (7 + \mu_1))) + x^2 (-1 + \eta)^2 \theta p (36 \eta^3 (1 + \mu_1) - 12 \eta^2 (\eta t (1 + 2 \theta l) \times (1 + \mu_1) - 2 \times (-5 + \theta l + \mu_1 + \theta l \mu_1)) + 12 \eta (7 - 5 \mu_1 - 2 \theta l (7 + \mu_1) + \eta t (1 + \mu_1 + 2 \theta l (7 + \mu_1))) +
\end{aligned}$$

$$\begin{aligned}
& (-1 + \eta t) \, \theta l \, (1 + \mu 1) \times (58 + 15 \, \mathfrak{e} 1 + 15 \, \mathfrak{e} 2) + \theta p \, (12 \, \eta^5 (1 + \mu 1) + 20 \, \eta t \\
& \quad (1 + \mu 1) - 4 \, \eta^4 (\eta t (1 + 2 \, \theta l) \times (1 + \mu 1) - 2 \times (-5 + \theta l + \mu 1 + \theta l \, \mu 1)) + \\
& \quad 4 \, \eta^3 (7 - 5 \, \mu 1 - 2 \, \theta l (7 + \mu 1) + \eta t (1 + \mu 1 + 2 \, \theta l (7 + \mu 1))) + \\
& \quad \eta^2 (-1 + \eta t) \, \theta l \, (1 + \mu 1) \times (58 + 15 \, \mathfrak{e} 1 + 15 \, \mathfrak{e} 2) + \\
& \quad \eta (-\theta l (30 + 15 \, \mathfrak{e} 1 + \mu 1 (30 + 15 \, \mathfrak{e} 1 - 29 \, \mathfrak{e} 2) + 19 \, \mathfrak{e} 2) + \eta t (-20 \times \\
& \quad \quad (1 + \mu 1) + \theta l (30 + 15 \, \mathfrak{e} 1 + \mu 1 (30 + 15 \, \mathfrak{e} 1 - 29 \, \mathfrak{e} 2) + 19 \, \mathfrak{e} 2))) - \\
& \quad \times (-1 + \eta) \times (12 \times (-1 + \eta) \, \eta^2 \, \theta p (-7 + 5 \, \mu 1 + 3 \, \eta (1 + \mu 1) - \eta t (1 + \mu 1)) - \\
& \quad (-1 + \eta t) \, \theta l (20 \times (1 + \mu 1) + \theta p (-30 + 24 \, \eta^3 (1 + \mu 1) - \\
& \quad \quad 24 \, \eta^2 (7 + \mu 1) - 15 \, \mathfrak{e} 1 - 19 \, \mathfrak{e} 2 - 2 \, \eta (1 + \mu 1) \times \\
& \quad \quad (58 + 15 \, \mathfrak{e} 1 + 15 \, \mathfrak{e} 2) + \mu 1 (-30 - 15 \, \mathfrak{e} 1 + 29 \, \mathfrak{e} 2)))) + \\
& w^3 (-1 + \eta)^3 (x^2 (-1 + \eta)^2 \, \theta p (40 - 78 \, \theta l - 56 \, \mu 1 + 18 \, \theta l \, \mu 1 + 8 \, \eta^2 (1 + \mu 1) + \\
& \quad 8 \, \eta t (1 + \mu 1) - 8 \, \eta (6 + \eta t - 6 \, \mu 1 + \eta t \, \mu 1) - 5 \, \theta l \, \mathfrak{e} 1 - 5 \, \theta l \, \mu 1 \, \mathfrak{e} 1 - \\
& \quad 5 \, \theta l \, \mathfrak{e} 2 - 5 \, \theta l \, \mu 1 \, \mathfrak{e} 2 + \eta t \, \theta l (78 + 5 \, \mathfrak{e} 1 + 5 \, \mathfrak{e} 2 + \mu 1 (-18 + 5 \, \mathfrak{e} 1 + 5 \, \mathfrak{e} 2))) + \\
& \quad \theta p (8 \, \eta^4 (1 + \mu 1) + 60 \, \eta t (1 + \mu 1) - 4 \, \eta^3 (9 - 15 \, \mu 1 + 2 \, \eta t (1 + \mu 1)) + \\
& \quad \eta^2 (-48 \, \mu 1 - \theta l (5 \times (14 + \mathfrak{e} 1 + \mathfrak{e} 2) + \mu 1 (-26 + 5 \, \mathfrak{e} 1 + 5 \, \mathfrak{e} 2)) + \\
& \quad \eta t (4 \times (1 + \mu 1) + 5 \, \theta l (14 + \mathfrak{e} 1 + \mathfrak{e} 2) + \theta l \, \mu 1 (-26 + 5 \, \mathfrak{e} 1 + 5 \, \mathfrak{e} 2))) + \\
& \quad \eta (28 - 20 \, \mu 1 - \theta l (146 + 45 \, \mathfrak{e} 1 + \mu 1 (98 + 45 \, \mathfrak{e} 1 - 87 \, \mathfrak{e} 2) + 57 \, \mathfrak{e} 2) + \\
& \quad \eta t (-56 \times (1 + \mu 1) + \theta l (146 + 45 \, \mathfrak{e} 1 + \mu 1 (98 + 45 \, \mathfrak{e} 1 - 87 \, \mathfrak{e} 2) + \\
& \quad \quad 57 \, \mathfrak{e} 2))) - \times (-1 + \eta) \times (4 \times (-1 + \eta) \, \theta p (-7 + 5 \, \mu 1 + \\
& \quad 4 \, \eta^2 (1 + \mu 1) - \eta t (1 + \mu 1) - \eta (17 - 31 \, \mu 1 + 4 \, \eta t (1 + \mu 1))) + \\
& \quad (-1 + \eta t) \, \theta l (-60 \times (1 + \mu 1) + \theta p (146 + 45 \, \mathfrak{e} 1 + \mu 1 (98 + 45 \, \mathfrak{e} 1 - 87 \, \mathfrak{e} 2) + \\
& \quad \quad 57 \, \mathfrak{e} 2 + 2 \, \eta (74 + 5 \, \mathfrak{e} 1 + 5 \, \mathfrak{e} 2 + \mu 1 (-22 + 5 \, \mathfrak{e} 1 + 5 \, \mathfrak{e} 2)))) + \\
& w^2 (-1 + \eta)^2 (2 \, x^3 (-1 + \eta)^3 \, \theta p (10 - 17 \, \theta l - 14 \, \mu 1 + 7 \, \theta l \, \mu 1 + 2 \, \eta^2 \\
& \quad (1 + \mu 1) - 2 \, \eta (6 + \eta t - 6 \, \mu 1 + \eta t \, \mu 1) + \eta t (2 + 17 \, \theta l + 2 \, \mu 1 - 7 \, \theta l \, \mu 1)) - \\
& \quad x^2 (-1 + \eta)^2 \, \theta p (56 - 142 \, \theta l - 40 \, \mu 1 - 46 \, \theta l \, \mu 1 + 12 \, \eta^3 (1 + \mu 1) + \\
& \quad 8 \, \eta t (1 + \mu 1) - 12 \, \eta^2 (4 + \eta t - 8 \, \mu 1 + \eta t \, \mu 1) + \\
& \quad \eta (-20 - 86 \, \theta l - 68 \, \mu 1 + 58 \, \theta l \, \mu 1 + \eta t (4 + 86 \, \theta l + 4 \, \mu 1 - 58 \, \theta l \, \mu 1)) - \\
& \quad 15 \, \theta l \, \mathfrak{e} 1 - 15 \, \theta l \, \mu 1 \, \mathfrak{e} 1 - 15 \, \theta l \, \mathfrak{e} 2 - 15 \, \theta l \, \mu 1 \, \mathfrak{e} 2 + \\
& \quad \eta t \, \theta l (142 + 15 \, \mathfrak{e} 1 + 15 \, \mathfrak{e} 2 + \mu 1 (46 + 15 \, \mathfrak{e} 1 + 15 \, \mathfrak{e} 2))) + \\
& \quad \times (-1 + \eta) \times (4 \times (-1 + \eta) \, \eta \, \theta p (3 \, \eta^2 (1 + \mu 1) - 3 \, \eta (1 + \eta t - 11 \, \mu 1 + \eta t \, \mu 1) - \\
& \quad 4 \times (7 + \eta t - 5 \, \mu 1 + \eta t \, \mu 1)) - (-1 + \eta t) \, \theta l (60 \times (1 + \mu 1) + \theta p (-104 + \\
& \quad \eta^2 (-70 + 74 \, \mu 1) - 45 \, \mathfrak{e} 1 - 57 \, \mathfrak{e} 2 + \mu 1 (-104 - 45 \, \mathfrak{e} 1 + 87 \, \mathfrak{e} 2) - \\
& \quad 2 \, \eta (142 + 15 \, \mathfrak{e} 1 + 15 \, \mathfrak{e} 2 + \mu 1 (46 + 15 \, \mathfrak{e} 1 + 15 \, \mathfrak{e} 2)))) + \\
& \quad \theta p (-4 \, \eta^5 (1 + \mu 1) - 60 \, \eta t (1 + \mu 1) + 4 \, \eta^4 (\eta t - 12 \, \mu 1 + \eta t \, \mu 1) + \\
& \quad 2 \, \eta^3 (\theta l (9 - 15 \, \mu 1) + 6 \times (5 + \mu 1) + \eta t (2 - 9 \, \theta l + 2 \, \mu 1 + 15 \, \theta l \, \mu 1)) + \\
& \quad \eta (60 \, \eta t (1 + \mu 1) + \theta l (104 + 45 \, \mathfrak{e} 1 + \mu 1 (104 + 45 \, \mathfrak{e} 1 - 87 \, \mathfrak{e} 2) + 57 \, \mathfrak{e} 2) - \\
& \quad \eta t \, \theta l (104 + 45 \, \mathfrak{e} 1 + \mu 1 (104 + 45 \, \mathfrak{e} 1 - 87 \, \mathfrak{e} 2) + 57 \, \mathfrak{e} 2)) - \\
& \quad \eta^2 (56 - 40 \, \mu 1 - \theta l (142 + 15 \, \mathfrak{e} 1 + 15 \, \mathfrak{e} 2 + \mu 1 (46 + 15 \, \mathfrak{e} 1 + 15 \, \mathfrak{e} 2)) + \\
& \quad \eta t (8 \times (1 + \mu 1) + \theta l (142 + 15 \, \mathfrak{e} 1 + 15 \, \mathfrak{e} 2 + \\
& \quad \quad \mu 1 (46 + 15 \, \mathfrak{e} 1 + 15 \, \mathfrak{e} 2)))) + \\
& 2 \, \text{co}^2 (-1 + \eta) \times (2 \, x^6 (-1 + \eta)^6 \, \theta p (2 - 2 \, \theta l - 3 \, \mu 1 - 9 \, w \, \mu 1 - 4 \, w^2 \, \mu 1 - \\
& \quad \theta l \, \mu 1 + w \, \theta l \, \mu 1 - 17 \, \mu 1^2 - 21 \, w \, \mu 1^2 - 4 \, w^2 \, \mu 1^2 + 13 \, \theta l \, \mu 1^2 + \\
& \quad 13 \, w \, \theta l \, \mu 1^2 + w^2 \, \eta^4 (1 + \mu 1) - w \, \eta^3 (3 + w (3 + \eta t - 4 \, \mu 1)) \times (1 + \mu 1) + \\
& \quad \eta^2 (2 \times (1 + \mu 1) + 3 \, w^2 (1 + \eta t - 4 \, \mu 1) \times (1 + \mu 1) +
\end{aligned}$$



$$\begin{aligned}
& 3w(2 + \eta t - \mu_1 + \eta t \mu_1 - 7\mu_1^2) + \eta t(2 \times (1 + \mu_1) + w^2(1 + \mu_1) + \\
& \theta l(2 + \mu_1 - 13\mu_1^2) + w(3 - (-3 + \theta l)\mu_1 - 13\theta l\mu_1^2)) - \eta(4 + 2\eta t - \mu_1 + \\
& 2\eta t \mu_1 - 17\mu_1^2 + w^2(1 + 3\eta t - 12\mu_1) \times (1 + \mu_1) + w(3 + (-15 + \theta l)\mu_1 + \\
& (-42 + 13\theta l)\mu_1^2 + \eta t(6 - (-6 + \theta l)\mu_1 - 13\theta l\mu_1^2))) + \\
& x^4(-1 + \eta)^4(2 \times (-1 + \eta)\theta p(-5 - 23\eta - 10\eta^2 + 30\eta^3 - 2\eta t - 20\eta\eta t - \\
& 30\eta^2\eta t + 33\mu_1 + 82\eta\mu_1 + 65\eta^2\mu_1 + 30\eta^3\mu_1 + 2\eta t\mu_1 - 18\eta\eta t\mu_1 - \\
& 30\eta^2\eta t\mu_1 + 50\mu_1^2 + 225\eta\mu_1^2 + 255\eta^2\mu_1^2 - 20\eta t\mu_1^2 + 2\eta\eta t\mu_1^2 + \\
& w^4(-1 + \eta)^4(1 + \mu_1)(\eta - \eta t + 4\mu_1) + \mu_2 - 7\eta\mu_2 - 60\eta^2\mu_2 + \\
& 16\eta t\mu_2 + 30\eta\eta t\mu_2 + 37\mu_1\mu_2 + 101\eta\mu_1\mu_2 + 60\eta^2\mu_1\mu_2 - \\
& 20\eta t\mu_1\mu_2 - 30\eta\eta t\mu_1\mu_2 - w^3(-1 + \eta)^3(-2 + 45\mu_1 + 59\mu_1^2 + \\
& 10\eta^2(1 + \mu_1) - 14\mu_2 + 58\mu_1\mu_2 - \eta t(7 + 7\mu_1 - 12\mu_2 + 12\mu_1\mu_2) + \\
& \eta(7 + 47\mu_1 + 40\mu_1^2 - 10\eta t(1 + \mu_1) - 12\mu_2 + 12\mu_1\mu_2)) + \\
& w^2(-1 + \eta)^2(-9 + 113\mu_1 + 182\mu_1^2 + 15\eta^3(1 + \mu_1) - 37\mu_2 + 167 \\
& \mu_1\mu_2 - \eta t(15 + 11\mu_1 + 20\mu_1^2 - 40\mu_2 + 44\mu_1\mu_2) + \eta(10 + 195\mu_1 + \\
& 305\mu_1^2 - 77\mu_2 + 187\mu_1\mu_2 - 10\eta t(4 + 4\mu_1 - 3\mu_2 + 3\mu_1\mu_2)) - \\
& 5\eta^2(3\eta t(1 + \mu_1) - 2 \times (4 + 10\mu_1 + 6\mu_1^2 - 3\mu_2 + 3\mu_1\mu_2))) - \\
& w(-1 + \eta) \times (-16 + 101\mu_1 + 177\mu_1^2 + 45\eta^3(1 + \mu_1) - 22\mu_2 + 146\mu_1\mu_2 + \\
& 5\eta^2(10 + 63\mu_1^2 - 9\eta t(1 + \mu_1) - 18\mu_2 + \mu_1(37 + 18\mu_2)) - \eta t(11 + \\
& 40\mu_1^2 - 44\mu_2 + \mu_1(3 + 52\mu_2)) + \eta(-19 + 490\mu_1^2 - 72\mu_2 + 3\mu_1 \\
& (77 + 92\mu_2) + 2\eta t(\mu_1^2 - 6\mu_1(4 + 5\mu_2) + 5 \times (-5 + 6\mu_2)))) + \\
& (-1 + \eta t)\theta l(4 + 6\theta p + 50\eta\theta p + 60\eta^2\theta p - 16\mu_1 + 16\eta\mu_1 + \\
& 16\eta^2\mu_1 - 22\theta p\mu_1 - 92\eta\theta p\mu_1 + 20\eta^2\theta p\mu_1 - 140\mu_1^2 - 176\eta\mu_1^2 + \\
& 16\eta^2\mu_1^2 - 4\theta p\mu_1^2 - 262\eta\theta p\mu_1^2 - 400\eta^2\theta p\mu_1^2 + 19\mu_2 - 26\theta p\mu_2 - \\
& 20\eta\theta p\mu_2 + 50\eta^2\theta p\mu_2 - 29\mu_1\mu_2 + 22\theta p\mu_1\mu_2 - 44\eta\theta p\mu_1\mu_2 - \\
& 70\eta^2\theta p\mu_1\mu_2 + \theta p\mathfrak{z}1 - 16\theta p\mu_1\mathfrak{z}1 - 16\eta\theta p\mu_1\mathfrak{z}1 - 5\eta^2\theta p\mu_1\mathfrak{z}1 - \\
& 41\theta p\mu_1^2\mathfrak{z}1 - 76\eta\theta p\mu_1^2\mathfrak{z}1 - 5\eta^2\theta p\mu_1^2\mathfrak{z}1 - 5\theta p\mu_2\mathfrak{z}1 - \\
& 5\theta p\mu_1\mu_2\mathfrak{z}1 - \theta p\mathfrak{z}2 + 8\theta p\mu_1\mathfrak{z}2 - 6\eta\theta p\mu_1\mathfrak{z}2 - 5\eta^2\theta p\mu_1\mathfrak{z}2 + \\
& 33\theta p\mu_1^2\mathfrak{z}2 + 54\eta\theta p\mu_1^2\mathfrak{z}2 - 5\eta^2\theta p\mu_1^2\mathfrak{z}2 + 17\theta p\mu_2\mathfrak{z}2 + \\
& 60\eta\theta p\mu_2\mathfrak{z}2 - 7\theta p\mu_1\mu_2\mathfrak{z}2 - 60\eta\theta p\mu_1\mu_2\mathfrak{z}2 + w^3(-1 + \eta)^3 \\
& (-4 - \theta p\mathfrak{z}1 + \mu_2(-19 + 5\theta p(\mathfrak{z}1 - \mathfrak{z}2)) + 4\mu_1^2(35 + 6\theta p(\mathfrak{z}1 - \mathfrak{z}2)) + \\
& \mu_1(16 + \mu_2(29 + 5\theta p(\mathfrak{z}1 - \mathfrak{z}2)) + 11\theta p(\mathfrak{z}1 - \mathfrak{z}2)) + \theta p\mathfrak{z}2) - w^2 \\
& (-1 + \eta)^2(-12 + 48\mu_1 - 16\eta\mu_1 + 420\mu_1^2 + 176\eta\mu_1^2 - 57\mu_2 + 87\mu_1\mu_2 + \\
& \theta p(\mu_1^2(56 + 89\mathfrak{z}1 - 81\mathfrak{z}2) + \mu_1(26 + 38\mathfrak{z}1 + 3\mu_2(2 + 5\mathfrak{z}1 - \mathfrak{z}2) - \\
& 30\mathfrak{z}2) + 3 \times (-2 - \mathfrak{z}1 + \mu_2(2 + 5\mathfrak{z}1 - 9\mathfrak{z}2) + \mathfrak{z}2) + \\
& 5\eta(\mu_1^2(52 + 15\mathfrak{z}1 - 11\mathfrak{z}2) - 2 \times (1 + 7\mu_2 + 6\mu_2\mathfrak{z}2) + \\
& \mu_1(26 + 34\mu_2 + 3\mathfrak{z}1 + \mathfrak{z}2 + 12\mu_2\mathfrak{z}2)))) + \\
& w(-1 + \eta) \times (-12 + 48\mu_1 - 32\eta\mu_1 - 16\eta^2\mu_1 + 420\mu_1^2 + \\
& 352\eta\mu_1^2 - 16\eta^2\mu_1^2 - 57\mu_2 + 87\mu_1\mu_2 + \theta p(-20 + 32\mu_2 - 3\mathfrak{z}1 + \\
& 15\mu_2\mathfrak{z}1 + 2\mu_1^2(30 + 53\mathfrak{z}1 - 45\mathfrak{z}2) + 3\mathfrak{z}2 - 39\mu_2\mathfrak{z}2 + \\
& 5\eta^2(-10\mu_2 + \mu_1^2(80 + \mathfrak{z}1 + \mathfrak{z}2) + \mu_1(8 + 14\mu_2 + \mathfrak{z}1 + \mathfrak{z}2)) + \\
& \mu_1(40 + 43\mathfrak{z}1 - 27\mathfrak{z}2 + \mu_2(-16 + 15\mathfrak{z}1 + 9\mathfrak{z}2)) + \\
& \eta(\mu_1^2(522 + 151\mathfrak{z}1 - 109\mathfrak{z}2) - 10 \times (6 + 5\mu_2 + 12\mu_2\mathfrak{z}2) + \\
& \mu_1(222 + 214\mu_2 + 31\mathfrak{z}1 + 11\mathfrak{z}2 + 120\mu_2\mathfrak{z}2)))) + \\
& x^3(-1 + \eta)^3(-((-1 + \eta)\theta p(-4 - 40\eta - 84\eta^2 + 80\eta^4 + 4\eta t - 16\eta\eta t -
\end{aligned}$$

$$\begin{aligned}
& 80 \eta^2 \eta t - 80 \eta^3 \eta t + 40 \mu_1 + 264 \eta \mu_1 + 336 \eta^2 \mu_1 + 200 \eta^3 \mu_1 + 80 \eta^4 \mu_1 + \\
& 16 \eta \eta t \mu_1 - 64 \eta^2 \eta t \mu_1 - 80 \eta^3 \eta t \mu_1 + 44 \mu_1^2 + 400 \eta \mu_1^2 + 900 \eta^2 \mu_1^2 + \\
& 680 \eta^3 \mu_1^2 - 148 \eta t \mu_1^2 - 160 \eta \eta t \mu_1^2 + 16 \eta^2 \eta t \mu_1^2 + 12 \mu_2 + 8 \eta \mu_2 - \\
& 116 \eta^2 \mu_2 - 240 \eta^3 \mu_2 + 39 \eta t \mu_2 + 128 \eta \eta t \mu_2 + 120 \eta^2 \eta t \mu_2 + \\
& 12 \mu_1 \mu_2 + 296 \eta \mu_1 \mu_2 + 508 \eta^2 \mu_1 \mu_2 + 240 \eta^3 \mu_1 \mu_2 - 57 \eta t \mu_1 \mu_2 - \\
& 160 \eta \eta t \mu_1 \mu_2 - 120 \eta^2 \eta t \mu_1 \mu_2 + 2 w^4 (-1 + \eta)^4 (-1 + 18 \mu_1 + 19 \mu_1^2 + \\
& 4 \eta^2 (1 + \mu_1) - 7 \mu_2 + 29 \mu_1 \mu_2 - 2 \eta t (1 + \mu_1 - 3 \mu_2 + 3 \mu_1 \mu_2) + \\
& 2 \eta (1 + 8 \mu_1^2 - 2 \eta t (1 + \mu_1) - 3 \mu_2 + 3 \mu_1 (3 + \mu_2))) + \\
& w^2 (-1 + \eta)^2 (-30 + 268 \mu_1 + 394 \mu_1^2 + 40 \eta^4 (1 + \mu_1) - 38 \mu_2 + \\
& 370 \mu_1 \mu_2 - 40 \eta^3 (-4 + \eta t - 8 \mu_1 + \eta t \mu_1 - 4 \mu_1^2 + 3 \mu_2 - 3 \mu_1 \mu_2) - \\
& \eta t (8 + 20 \mu_1 + 444 \mu_1^2 - 177 \mu_2 + 231 \mu_1 \mu_2) - \\
& 4 \eta^2 (-25 - 210 \mu_1 - 305 \mu_1^2 + 119 \mu_2 - 229 \mu_1 \mu_2 + 10 \eta t \\
& (4 + 4 \mu_1 - 3 \mu_2 + 3 \mu_1 \mu_2)) - 4 \eta (13 - 231 \mu_1 - 364 \mu_1^2 + 98 \\
& \mu_2 - 358 \mu_1 \mu_2 + \eta t (30 + 22 \mu_1 + 40 \mu_1^2 - 80 \mu_2 + 88 \mu_1 \mu_2))) - \\
& w^3 (-1 + \eta)^3 (40 \eta^3 (1 + \mu_1) + 8 \eta^2 (7 + 20 \mu_1^2 - 5 \eta t (1 + \mu_1) - 12 \mu_2 + \\
& 3 \mu_1 (9 + 4 \mu_2)) + 4 \times (-3 + 58 \mu_1^2 - 14 \mu_2 + \mu_1 (43 + 70 \mu_2)) - \\
& \eta t (12 + 148 \mu_1^2 - 87 \mu_2 + \mu_1 (16 + 105 \mu_2)) - 4 \eta (-118 \mu_1^2 + \\
& 43 \mu_2 - \mu_1 (94 + 131 \mu_2) + 2 \eta t (7 - 12 \mu_2 + \mu_1 (7 + 12 \mu_2))) - \\
& w (-1 + \eta) \times (120 \eta^4 (1 + \mu_1) + 40 \eta^3 (5 + 21 \mu_1^2 - 3 \eta t (1 + \mu_1) - 9 \mu_2 + \\
& \mu_1 (14 + 9 \mu_2)) + 4 \times (-6 + 61 \mu_1^2 + 4 \mu_2 + \mu_1 (43 + 40 \mu_2)) + \\
& \eta t (4 - 444 \mu_1^2 + 141 \mu_2 - \mu_1 (8 + 195 \mu_2)) + 8 \eta^2 \\
& (-4 + 245 \mu_1^2 - 62 \mu_2 + \mu_1 (121 + 166 \mu_2) + \eta t (-25 - 23 \mu_1 + \\
& 2 \mu_1^2 + 30 \mu_2 - 30 \mu_1 \mu_2)) - 8 \eta (15 - 177 \mu_1^2 + 28 \mu_2 - 2 \mu_1 \\
& (51 + 76 \mu_2) + \eta t (11 + 40 \mu_1^2 - 44 \mu_2 + \mu_1 (3 + 52 \mu_2)))) + \\
& (-1 + \eta t) \otimes (-6 - 12 \eta + 2 \otimes p - 24 \eta \otimes p - 100 \eta^2 \otimes p - 80 \eta^3 \otimes p + \\
& 56 \mu_1 + 76 \eta \mu_1 - 24 \eta^2 \mu_1 - 24 \eta^3 \mu_1 - 18 \otimes p \mu_1 + 86 \eta \otimes p \mu_1 + 188 \eta^2 \otimes p \mu_1 - \\
& 20 \eta^3 \otimes p \mu_1 + 86 \mu_1^2 + 400 \eta \mu_1^2 + 264 \eta^2 \mu_1^2 - 24 \eta^3 \mu_1^2 - 44 \otimes p \mu_1^2 + \\
& 14 \eta \otimes p \mu_1^2 + 528 \eta^2 \otimes p \mu_1^2 + 540 \eta^3 \otimes p \mu_1^2 - 38 \mu_2 - 57 \eta \mu_2 + 34 \otimes p \mu_2 + \\
& 114 \eta \otimes p \mu_2 + 20 \eta^2 \otimes p \mu_2 - 100 \eta^3 \otimes p \mu_2 + 58 \mu_1 \mu_2 + 87 \eta \mu_1 \mu_2 - \\
& 62 \otimes p \mu_1 \mu_2 - 102 \eta \otimes p \mu_1 \mu_2 + 116 \eta^2 \otimes p \mu_1 \mu_2 + 140 \eta^3 \otimes p \mu_1 \mu_2 + \\
& w^4 (-1 + \eta)^4 (-2 + 70 \mu_1^2 - 5 \mu_2 - \mu_1 (4 + 5 \mu_2)) - 2 \otimes p \otimes 1 - 4 \eta \otimes p \otimes 1 + \\
& 23 \otimes p \mu_1 \otimes 1 + 63 \eta \otimes p \mu_1 \otimes 1 + 34 \eta^2 \otimes p \mu_1 \otimes 1 + 10 \eta^3 \otimes p \mu_1 \otimes 1 + \\
& 37 \otimes p \mu_1^2 \otimes 1 + 163 \eta \otimes p \mu_1^2 \otimes 1 + 154 \eta^2 \otimes p \mu_1^2 \otimes 1 + 10 \eta^3 \otimes p \mu_1^2 \otimes 1 + \\
& 10 \otimes p \mu_2 \otimes 1 + 20 \eta \otimes p \mu_2 \otimes 1 + 10 \otimes p \mu_1 \mu_2 \otimes 1 + 20 \eta \otimes p \mu_1 \mu_2 \otimes 1 + \\
& 2 \otimes p \otimes 2 + 4 \eta \otimes p \otimes 2 - 19 \otimes p \mu_1 \otimes 2 - 33 \eta \otimes p \mu_1 \otimes 2 + 14 \eta^2 \otimes p \mu_1 \otimes 2 + \\
& 10 \eta^3 \otimes p \mu_1 \otimes 2 - 33 \otimes p \mu_1^2 \otimes 2 - 133 \eta \otimes p \mu_1^2 \otimes 2 - 106 \eta^2 \otimes p \mu_1^2 \otimes 2 + \\
& 10 \eta^3 \otimes p \mu_1^2 \otimes 2 + 2 \otimes p \mu_2 \otimes 2 - 68 \eta \otimes p \mu_2 \otimes 2 - 120 \eta^2 \otimes p \mu_2 \otimes 2 - \\
& 22 \otimes p \mu_1 \mu_2 \otimes 2 + 28 \eta \otimes p \mu_1 \mu_2 \otimes 2 + 120 \eta^2 \otimes p \mu_1 \mu_2 \otimes 2 - w^3 (-1 + \eta)^3 \\
& (-12 - 53 \mu_2 - 2 \otimes p \otimes 1 + 10 \otimes p \mu_2 \otimes 1 + 4 \mu_1^2 (89 + 12 \otimes p (\otimes 1 - \otimes 2)) + \\
& \mu_1 (56 + \mu_2 (43 + 10 \otimes p (\otimes 1 - \otimes 2)) + 22 \otimes p (\otimes 1 - \otimes 2)) + \\
& 2 \otimes p \otimes 2 - 10 \otimes p \mu_2 \otimes 2 + \eta (-12 - 57 \mu_2 - 4 \otimes p \otimes 1 + 20 \otimes p \mu_2 \otimes 1 + \\
& 12 \mu_1^2 (33 + 8 \otimes p (\otimes 1 - \otimes 2)) + \mu_1 (72 + \mu_2 (87 + 20 \otimes p (\otimes 1 - \otimes 2)) + \\
& 44 \otimes p (\otimes 1 - \otimes 2)) + 4 \otimes p \otimes 2 - 20 \otimes p \mu_2 \otimes 2)) + \\
& w^2 (-1 + \eta)^2 (3 \times (-8 + 196 \mu_1^2 - 43 \mu_2 + \mu_1 (60 + 53 \mu_2)) +
\end{aligned}$$

$$\begin{aligned}
& \theta p \left( \mu^2 (-44 + 133 \mathfrak{x}1 - 129 \mathfrak{x}2) + \mu1 (-26 + 67 \mathfrak{x}1 + 6 \mu2 (-15 + 5 \mathfrak{x}1 - 7 \mathfrak{x}2) - 63 \mathfrak{x}2) + 6 \times (-1 - \mathfrak{x}1 + \mu2 (9 + 5 \mathfrak{x}1 - 3 \mathfrak{x}2) + \mathfrak{x}2) \right) + \\
& \eta \left( 9 \times (-4 + 132 \mu^2 - 19 \mu2 + \mu1 (24 + 29 \mu2)) + 4 \theta p \right. \\
& \quad \left( \mu^2 (56 + 89 \mathfrak{x}1 - 81 \mathfrak{x}2) + \mu1 (26 + 38 \mathfrak{x}1 + 3 \mu2 (2 + 5 \mathfrak{x}1 - \mathfrak{x}2) - 30 \mathfrak{x}2) + 3 \times (-2 - \mathfrak{x}1 + \mu2 (2 + 5 \mathfrak{x}1 - 9 \mathfrak{x}2) + \mathfrak{x}2) \right) \Big) + 2 \eta^2 \\
& \quad \left( 12 \mu1 (-1 + 11 \mu1) + 5 \theta p \left( \mu^2 (52 + 15 \mathfrak{x}1 - 11 \mathfrak{x}2) - 2 \times (1 + 7 \mu2 + 6 \mu2 \mathfrak{x}2) + \mu1 (26 + 34 \mu2 + 3 \mathfrak{x}1 + \mathfrak{x}2 + 12 \mu2 \mathfrak{x}2) \right) \right) \Big) - \\
& w (-1 + \eta) \times (-20 + 176 \mu1 + 388 \mu^2 - 119 \mu2 + 169 \mu1 \mu2 + \\
& \quad 2 \theta p (-2 - 3 \mathfrak{x}1 + \mu^2 (-44 + 61 \mathfrak{x}1 - 57 \mathfrak{x}2) + \mu1 (-22 + 34 \mathfrak{x}1 + \mu2 (-76 + 15 \mathfrak{x}1 - 27 \mathfrak{x}2) - 30 \mathfrak{x}2) + \mu2 (44 + 15 \mathfrak{x}1 - 3 \mathfrak{x}2) + \\
& \quad 3 \mathfrak{x}2) + 2 \eta^3 (-50 \theta p \mu2 + \mu^2 (-12 + 5 \theta p (54 + \mathfrak{x}1 + \mathfrak{x}2)) + \mu1 (-12 + 5 \theta p (6 + 14 \mu2 + \mathfrak{x}1 + \mathfrak{x}2))) + 8 \eta^2 (6 \mu1 (-1 + 11 \mu1) + \\
& \quad \theta p (\mu^2 (131 + 38 \mathfrak{x}1 - 27 \mathfrak{x}2) - 15 \times (1 + \mu2 + 2 \mu2 \mathfrak{x}2) + \mu1 (56 + 57 \mu2 + 8 \mathfrak{x}1 + 3 \mathfrak{x}2 + 30 \mu2 \mathfrak{x}2))) + \\
& \quad \eta (1192 \mu^2 - 9 \times (4 + 19 \mu2) + \mu1 (220 + 261 \mu2) + \theta p (\mu^2 (238 + 423 \mathfrak{x}1 - 361 \mathfrak{x}2) + \\
& \quad 2 \times (-40 - 6 \mathfrak{x}1 + \mu2 (69 + 30 \mathfrak{x}1 - 78 \mathfrak{x}2) + 6 \mathfrak{x}2) + \mu1 (158 + 171 \mathfrak{x}1 - 109 \mathfrak{x}2 + 6 \mu2 (-13 + 10 \mathfrak{x}1 + 6 \mathfrak{x}2))) \Big) \Big) + \\
& \theta p (w^4 (-1 + \eta)^5 (2 \eta^5 (1 + \mu1) + 5 \eta t (1 + \mu1) \mu2 + 2 \eta \eta t (1 - 23 \mu^2 + 5 \mu1 (-2 + \mu2) + 5 \mu2) - 2 \eta^4 (-2 - 4 \mu^2 + \eta t (1 + \mu1) + 6 \mu2 - 6 \mu1 (1 + \mu2)) + \eta^2 (-2 + (30 - 70 \eta t) \mu^2 + (10 + 17 \eta t) \mu2 + \mu1 (28 + \eta t (2 - 7 \mu2) + 34 \mu2)) - \\
& \quad 2 \eta^3 (-19 \mu^2 + 13 \mu2 - \mu1 (19 + 35 \mu2) + 2 \eta t (1 + \mu1 - 3 \mu2 + 3 \mu1 \mu2))) - \\
& w^3 (-1 + \eta)^3 (4 \eta^7 (1 + \mu1) - 15 \eta t (1 + \mu1) \mu2 + 2 \eta \eta t (-4 + 80 \mu^2 - 17 \mu2 + \mu1 (40 + 7 \mu2)) + \\
& \quad 2 \eta^6 (5 + 8 \mu^2 - 2 \eta t (1 + \mu1) - 12 \mu2 + \mu1 (13 + 12 \mu2)) - 2 \eta^5 (1 - 51 \mu^2 + 32 \mu2 - 38 \mu1 (1 + 2 \mu2) + \eta t (5 - 12 \mu2 + \mu1 (5 + 12 \mu2))) + \\
& \quad \eta^4 (-18 - 4 \mu2 - \theta l \mathfrak{x}1 + 5 \theta l \mu2 \mathfrak{x}1 + 6 \mu^2 (19 + 4 \theta l (\mathfrak{x}1 - \mathfrak{x}2)) + \mu1 (72 + 5 \mu2 (28 + \theta l (\mathfrak{x}1 - \mathfrak{x}2)) + 11 \theta l (\mathfrak{x}1 - \mathfrak{x}2)) + \theta l \mathfrak{x}2 - 5 \theta l \mu2 \mathfrak{x}2 + \eta t (2 + \theta l \mathfrak{x}1 - 4 \mu^2 (31 + 6 \theta l (\mathfrak{x}1 - \mathfrak{x}2)) - \mu1 (26 + \mu2 (81 + 5 \theta l (\mathfrak{x}1 - \mathfrak{x}2)) + 11 \theta l (\mathfrak{x}1 - \mathfrak{x}2)) - \theta l \mathfrak{x}2 + \mu2 (63 - 5 \theta l \mathfrak{x}1 + 5 \theta l \mathfrak{x}2))) - 2 \eta^3 (1 - 52 \mu2 + \theta l \mathfrak{x}1 - 5 \theta l \mu2 \mathfrak{x}1 + \mu^2 (51 - 24 \theta l (\mathfrak{x}1 - \mathfrak{x}2)) - \theta l \mathfrak{x}2 + 5 \theta l \mu2 \mathfrak{x}2 + \eta t (-9 - \theta l \mathfrak{x}1 + 5 \mu2 (-1 + \theta l (\mathfrak{x}1 - \mathfrak{x}2)) + 12 \mu^2 (9 + 2 \theta l (\mathfrak{x}1 - \mathfrak{x}2)) + \mu1 (15 + 5 \mu2 (-1 + \theta l (\mathfrak{x}1 - \mathfrak{x}2)) + 11 \theta l (\mathfrak{x}1 - \mathfrak{x}2)) + \theta l \mathfrak{x}2) + \mu1 (40 - 11 \theta l (\mathfrak{x}1 - \mathfrak{x}2) + \mu2 (104 - 5 \theta l \mathfrak{x}1 + 5 \theta l \mathfrak{x}2))) - \eta^2 (-8 + 12 \mu2 + \theta l \mathfrak{x}1 - 5 \theta l \mu2 \mathfrak{x}1 + \mu^2 (130 - 24 \theta l (\mathfrak{x}1 - \mathfrak{x}2)) - \theta l \mathfrak{x}2 + 5 \theta l \mu2 \mathfrak{x}2 + \eta t (-2 - \theta l \mathfrak{x}1 + 12 \mu^2 (-15 + 2 \theta l (\mathfrak{x}1 - \mathfrak{x}2)) + \mu2 (48 + 5 \theta l (\mathfrak{x}1 - \mathfrak{x}2)) + \mu1 (10 + \mu2 (-96 + 5 \theta l (\mathfrak{x}1 - \mathfrak{x}2)) + 11 \theta l (\mathfrak{x}1 - \mathfrak{x}2)) + \theta l \mathfrak{x}2) + \mu1 (98 - 11 \theta l (\mathfrak{x}1 - \mathfrak{x}2) + \mu2 (108 - 5 \theta l \mathfrak{x}1 + 5 \theta l \mathfrak{x}2))) \Big) + \\
& w^2 (-1 + \eta)^2 (2 \eta^8 (1 + \mu1) - 15 \eta t (1 + \mu1) \mu2 - 2 \eta^7 (-7 + \eta t - 11 \mu1 + \eta t \mu1 - 4 \mu^2 + 6 \mu2 - 6 \mu1 \mu2) +
\end{aligned}$$

$$\begin{aligned}
& 12 \eta \eta t \left( -1 + 17 \mu_1^2 - 6 \mu_2 + 2 \mu_1 (5 + 3 \mu_2) \right) + \\
& 2 \eta^6 \left( 6 + 57 \mu_1^2 - 43 \mu_2 + 13 \mu_1 (3 + 5 \mu_2) - \eta t (7 - 6 \mu_2 + \mu_1 (7 + 6 \mu_2)) \right) + \\
& \eta^4 \left( -28 + 26 \mu_1 + 30 \mu_1^2 + 108 \mu_2 - 36 \mu_1 \mu_2 + \right. \\
& \quad \left. \theta l \left( \mu_1^2 (56 + 89 \mathfrak{e}_1 - 81 \mathfrak{e}_2) + \mu_1 (26 + 38 \mathfrak{e}_1 + 3 \mu_2 (2 + 5 \mathfrak{e}_1 - \mathfrak{e}_2) - \right. \right. \\
& \quad \left. \left. 30 \mathfrak{e}_2) + 3 \times (-2 - \mathfrak{e}_1 + \mu_2 (2 + 5 \mathfrak{e}_1 - 9 \mathfrak{e}_2) + \mathfrak{e}_2) \right) - \right. \\
& \quad \left. \eta t (-22 + 70 \mu_1 + 332 \mu_1^2 - 97 \mu_2 + 143 \mu_1 \mu_2 + \theta l \right. \\
& \quad \left. (\mu_1^2 (56 + 89 \mathfrak{e}_1 - 81 \mathfrak{e}_2) + \mu_1 (26 + 38 \mathfrak{e}_1 + 3 \mu_2 (2 + 5 \mathfrak{e}_1 - \mathfrak{e}_2) - \right. \\
& \quad \left. 30 \mathfrak{e}_2) + 3 \times (-2 - \mathfrak{e}_1 + \mu_2 (2 + 5 \mathfrak{e}_1 - 9 \mathfrak{e}_2) + \mathfrak{e}_2) \right) \left. \right) - \\
& \eta^2 \left( 2 \times (-7 + 53 \mu_1 + 72 \mu_1^2 + 7 \mu_2 + 43 \mu_1 \mu_2) + \eta t (8 - 340 \mu_1^2 + \right. \\
& \quad 94 \mu_2 - 2 \mu_1 (46 + 85 \mu_2) + \theta l (-2 - 3 \mathfrak{e}_1 + \mu_1^2 (-48 + 59 \mathfrak{e}_1 - \\
& \quad 59 \mathfrak{e}_2) + \mu_1 (-26 + 32 \mathfrak{e}_1 + \mu_2 (-62 + 15 \mathfrak{e}_1 - 27 \mathfrak{e}_2) - \\
& \quad 32 \mathfrak{e}_2) + \mu_2 (34 + 15 \mathfrak{e}_1 - 3 \mathfrak{e}_2) + 3 \mathfrak{e}_2) \left. \right) + \theta l (2 + 3 \mathfrak{e}_1 - \\
& \quad 3 \mathfrak{e}_2 + \mu_2 (-34 - 15 \mathfrak{e}_1 + 3 \mathfrak{e}_2) + \mu_1^2 (48 - 59 \mathfrak{e}_1 + 59 \mathfrak{e}_2) + \\
& \quad \mu_1 (26 - 32 \mathfrak{e}_1 + 32 \mathfrak{e}_2 + \mu_2 (62 - 15 \mathfrak{e}_1 + 27 \mathfrak{e}_2)) \left. \right) + \\
& \eta^3 (12 - 250 \mu_1^2 + 76 \mu_2 + 4 \eta t (7 - 43 \mu_1^2 + \mu_1 (-30 + \mu_2) + \mu_2) - \\
& \quad 2 \mu_1 (83 + 154 \mu_2) + \theta l \mu_1^2 (-44 + 133 \mathfrak{e}_1 - 129 \mathfrak{e}_2) + \\
& \quad \theta l \mu_1 (-26 + 67 \mathfrak{e}_1 + 6 \mu_2 (-15 + 5 \mathfrak{e}_1 - 7 \mathfrak{e}_2) - 63 \mathfrak{e}_2) + \\
& \quad 6 \theta l (-1 - \mathfrak{e}_1 + \mu_2 (9 + 5 \mathfrak{e}_1 - 3 \mathfrak{e}_2) + \mathfrak{e}_2) + \\
& \quad \eta t \theta l (-6 \times (-1 - \mathfrak{e}_1 + \mu_2 (9 + 5 \mathfrak{e}_1 - 3 \mathfrak{e}_2) + \mathfrak{e}_2) + \mu_1^2 (44 - 133 \mathfrak{e}_1 + \\
& \quad 129 \mathfrak{e}_2) + \mu_1 (26 - 67 \mathfrak{e}_1 + 63 \mathfrak{e}_2 + \mu_2 (90 - 30 \mathfrak{e}_1 + 42 \mathfrak{e}_2)) \left. \right) - \\
& \eta^5 (26 - 144 \mu_1 - 242 \mu_1^2 + 72 \mu_2 - 288 \mu_1 \mu_2 - \theta l (\mu_1^2 \\
& \quad (52 + 15 \mathfrak{e}_1 - 11 \mathfrak{e}_2) - 2 \times (1 + 7 \mu_2 + 6 \mu_2 \mathfrak{e}_2) + \\
& \quad \mu_1 (26 + 34 \mu_2 + 3 \mathfrak{e}_1 + \mathfrak{e}_2 + 12 \mu_2 \mathfrak{e}_2) \left. \right) + \eta t (14 + 6 \mu_1 + 40 \mu_1^2 - \\
& \quad 68 \mu_2 + 76 \mu_1 \mu_2 + \theta l (\mu_1^2 (52 + 15 \mathfrak{e}_1 - 11 \mathfrak{e}_2) - 2 \times (1 + 7 \mu_2 + \\
& \quad 6 \mu_2 \mathfrak{e}_2) + \mu_1 (26 + 34 \mu_2 + 3 \mathfrak{e}_1 + \mathfrak{e}_2 + 12 \mu_2 \mathfrak{e}_2)) \left. \right) \left. \right) - \\
& w (-1 + \eta) \times (6 \eta^8 (1 + \mu_1) - 5 \eta t (1 + \mu_1) \mu_2 + \eta^7 (14 + 42 \mu_1^2 - \\
& \quad 6 \eta t (1 + \mu_1) - 36 \mu_2 + 4 \mu_1 (8 + 9 \mu_2)) + \\
& 2 \eta \eta t (-4 + 56 \mu_1^2 - 31 \mu_2 + \mu_1 (40 + 41 \mu_2)) + \\
& \eta^6 (-2 \times (5 + (38 + 5 \theta l) \mu_2) + \mu_1^2 (154 + \theta l (28 + \mathfrak{e}_1 + \mathfrak{e}_2)) + \\
& \quad \mu_1 (72 + 164 \mu_2 + \theta l (4 + 14 \mu_2 + \mathfrak{e}_1 + \mathfrak{e}_2)) - \\
& \quad \eta t (14 - 2 \times (12 + 5 \theta l) \mu_2 + \mu_1^2 (-4 + \theta l (28 + \mathfrak{e}_1 + \mathfrak{e}_2)) + \\
& \quad \mu_1 (10 + 24 \mu_2 + \theta l (4 + 14 \mu_2 + \mathfrak{e}_1 + \mathfrak{e}_2)) \left. \right) - \\
& \eta^2 (4 \times (1 + \mu_1) \times (-1 + 11 \mu_1 + 3 \mu_2) + \eta t (-4 \times (-3 + 32 \mu_1 + 59 \mu_1^2 - \\
& \quad 18 \mu_2 + 30 \mu_1 \mu_2) + \theta l (4 - 3 \mathfrak{e}_1 + \mu_1^2 (-70 + 46 \mathfrak{e}_1 - 46 \mathfrak{e}_2) + \\
& \quad \mu_1 (-42 + 31 \mathfrak{e}_1 + 3 \mu_2 (-32 + 5 \mathfrak{e}_1 - 13 \mathfrak{e}_2) - 31 \mathfrak{e}_2) + \\
& \quad 3 \mathfrak{e}_2 + 3 \mu_2 (16 + 5 \mathfrak{e}_1 + 3 \mathfrak{e}_2)) \left. \right) + \theta l (-4 + 3 \mathfrak{e}_1 - 3 \mathfrak{e}_2 - \\
& \quad 3 \mu_2 (16 + 5 \mathfrak{e}_1 + 3 \mathfrak{e}_2) + \mu_1^2 (70 - 46 \mathfrak{e}_1 + 46 \mathfrak{e}_2) + \\
& \quad \mu_1 (42 - 31 \mathfrak{e}_1 + 31 \mathfrak{e}_2 + \mu_2 (96 - 15 \mathfrak{e}_1 + 39 \mathfrak{e}_2)) \left. \right) - \\
& \eta^3 (4 \times (-5 + 50 \mu_1^2 + 6 \mu_2 + \mu_1 (33 + 30 \mu_2)) + \eta t (2 \times (-8 - 14 \mu_1^2 + \mu_2 + \\
& \quad \mu_1 (62 + \mu_2)) + \theta l (-4 - 6 \mathfrak{e}_1 + \mu_1^2 (-90 + 121 \mathfrak{e}_1 - 115 \mathfrak{e}_2) + \\
& \quad \mu_1 (-46 + 67 \mathfrak{e}_1 + 2 \mu_2 (-83 + 15 \mathfrak{e}_1 - 27 \mathfrak{e}_2) - 61 \mathfrak{e}_2) + \\
& \quad \mu_2 (98 + 30 \mathfrak{e}_1 - 6 \mathfrak{e}_2) + 6 \mathfrak{e}_2) \left. \right) + \theta l (4 + 6 \mathfrak{e}_1 - 6 \mathfrak{e}_2 + \\
& \quad \mu_2 (-98 - 30 \mathfrak{e}_1 + 6 \mathfrak{e}_2) + \mu_1^2 (90 - 121 \mathfrak{e}_1 + 115 \mathfrak{e}_2) +
\end{aligned}$$

$$\begin{aligned}
& \mu_1 (46 - 67 \mathfrak{e}_1 + 61 \mathfrak{e}_2 + \mu_2 (166 - 30 \mathfrak{e}_1 + 54 \mathfrak{e}_2)) \Big) - \\
& \eta^4 \Big( 2 \times (55 \mu_1^2 - 64 \mu_2 + \mu_1 (19 + 104 \mu_2)) - \mathfrak{e}_1 (-20 - 3 \mathfrak{e}_1 + \\
& \mu_1^2 (58 + 105 \mathfrak{e}_1 - 91 \mathfrak{e}_2) + 3 \mu_2 (14 + 5 \mathfrak{e}_1 - 13 \mathfrak{e}_2) + \\
& 3 \mathfrak{e}_2 + \mu_1 (38 + 42 \mathfrak{e}_1 - 28 \mathfrak{e}_2 + 3 \mu_2 (-10 + 5 \mathfrak{e}_1 + 3 \mathfrak{e}_2)) \Big) + \\
& \eta \mathfrak{t} (-26 + 78 \mu_1 + 296 \mu_1^2 - 53 \mu_2 + 91 \mu_1 \mu_2 + \mathfrak{e}_1 (-20 - \\
& 3 \mathfrak{e}_1 + \mu_1^2 (58 + 105 \mathfrak{e}_1 - 91 \mathfrak{e}_2) + 3 \mu_2 (14 + 5 \mathfrak{e}_1 - 13 \mathfrak{e}_2) + \\
& 3 \mathfrak{e}_2 + \mu_1 (38 + 42 \mathfrak{e}_1 - 28 \mathfrak{e}_2 + 3 \mu_2 (-10 + 5 \mathfrak{e}_1 + 3 \mathfrak{e}_2)) \Big) \Big) + \\
& \eta^5 (-34 + 158 \mu_1^2 + 20 \mu_2 + 20 \mu_1 (5 + 7 \mu_2) + \mathfrak{e}_1 (\mu_1^2 (106 + \\
& 31 \mathfrak{e}_1 - 21 \mathfrak{e}_2) - 6 \times (2 + \mu_2 (3 + 4 \mathfrak{e}_2)) + \mu_1 (46 + 7 \mathfrak{e}_1 + 3 \mathfrak{e}_2 + \\
& 6 \mu_2 (9 + 4 \mathfrak{e}_2)) \Big) - \eta \mathfrak{t} (2 - 10 \mu_1 + 84 \mu_1^2 - 64 \mu_2 + 80 \mu_1 \mu_2 + \\
& \mathfrak{e}_1 (\mu_1^2 (106 + 31 \mathfrak{e}_1 - 21 \mathfrak{e}_2) - 6 \times (2 + \mu_2 (3 + 4 \mathfrak{e}_2)) + \\
& \mu_1 (46 + 7 \mathfrak{e}_1 + 3 \mathfrak{e}_2 + 6 \mu_2 (9 + 4 \mathfrak{e}_2)) \Big) \Big) + \\
& \eta (4 \eta^7 (1 + \mu_1) + \eta^6 (34 \mu_1^2 - 4 \eta \mathfrak{t} (1 + \mu_1) - 24 \mu_2 + 2 \mu_1 (5 + 12 \mu_2)) + \\
& \eta \mathfrak{t} (-2 + 22 \mu_1^2 - 19 \mu_2 + \mu_1 (20 + 29 \mu_2)) + \eta^5 (4 \eta \mathfrak{t} (-1 + \mu_1) \times \\
& (1 + \mu_1 - 3 \mu_2) + 2 \times (-5 + 28 \mu_1^2 - 7 \mu_2 + \mu_1 (11 + 29 \mu_2)) + \\
& \mathfrak{e}_1 (-2 \times (2 + 5 \mu_2) + \mu_1^2 (28 + \mathfrak{e}_1 + \mathfrak{e}_2) + \mu_1 (14 \mu_2 + \mathfrak{e}_1 + \mathfrak{e}_2)) - \\
& \eta \mathfrak{t} \mathfrak{e}_1 (-2 \times (2 + 5 \mu_2) + \mu_1^2 (28 + \mathfrak{e}_1 + \mathfrak{e}_2) + \mu_1 (14 \mu_2 + \mathfrak{e}_1 + \mathfrak{e}_2)) \Big) + \\
& \eta (\mathfrak{e}_1 (2 - \mathfrak{e}_1 + 11 \mu_1^2 (-2 + \mathfrak{e}_1 - \mathfrak{e}_2) + \mathfrak{e}_2 + \mu_2 (14 + 5 \mathfrak{e}_1 + 7 \mathfrak{e}_2) + \\
& \mu_1 (5 \mu_2 \mathfrak{e}_1 + 10 \times (-2 + \mathfrak{e}_1 - \mathfrak{e}_2) - 17 \mu_2 (2 + \mathfrak{e}_2)) \Big) + \\
& \eta \mathfrak{t} (-4 + 48 \mu_1 + 52 \mu_1^2 - 19 \mu_2 + 29 \mu_1 \mu_2 + \mathfrak{e}_1 (-2 + \mathfrak{e}_1 - \\
& 5 \mu_2 \mathfrak{e}_1 - 5 \mu_1 \mu_2 \mathfrak{e}_1 - 11 \mu_1^2 (-2 + \mathfrak{e}_1 - \mathfrak{e}_2) - \mathfrak{e}_2 - \\
& 7 \mu_2 (2 + \mathfrak{e}_2) + 17 \mu_1 \mu_2 (2 + \mathfrak{e}_2) + 10 \mu_1 (2 - \mathfrak{e}_1 + \mathfrak{e}_2)) \Big) \Big) - \\
& 2 \eta^4 (2 - 15 \mu_1 - 5 \mu_1^2 - 20 \mu_2 + 4 \mu_1 \mu_2 - \mathfrak{e}_1 (-5 - 2 \mu_2 + \mu_1^2 (27 + \\
& 8 \mathfrak{e}_1 - 5 \mathfrak{e}_2) - 6 \mu_2 \mathfrak{e}_2 + \mu_1 (10 + 10 \mu_2 + 2 \mathfrak{e}_1 + \mathfrak{e}_2 + 6 \mu_2 \mathfrak{e}_2)) \Big) + \\
& \eta \mathfrak{t} (2 \times (-1 + 11 \mu_1^2 - 5 \mu_2 + \mu_1 (-2 + 7 \mu_2)) + \mathfrak{e}_1 \\
& (-5 - 2 \mu_2 + \mu_1^2 (27 + 8 \mathfrak{e}_1 - 5 \mathfrak{e}_2) - 6 \mu_2 \mathfrak{e}_2 + \\
& \mu_1 (10 + 10 \mu_2 + 2 \mathfrak{e}_1 + \mathfrak{e}_2 + 6 \mu_2 \mathfrak{e}_2)) \Big) \Big) - \\
& \eta^2 (-4 + 40 \mu_1 + 44 \mu_1^2 + 32 \mu_2 - 16 \mu_1 \mu_2 - 2 \mathfrak{e}_1 (1 - \mathfrak{e}_1 + \\
& \mu_1^2 (-23 + 18 \mathfrak{e}_1 - 17 \mathfrak{e}_2) + \mathfrak{e}_2 + \mu_2 (22 + 5 \mathfrak{e}_1 + \mathfrak{e}_2) + \\
& \mu_1 (11 \mathfrak{e}_1 + \mu_2 (-38 + 5 \mathfrak{e}_1 - 11 \mathfrak{e}_2) - 10 \times (1 + \mathfrak{e}_2)) \Big) + \\
& \eta \mathfrak{t} (-2 + 40 \mu_1 - 54 \mu_1^2 + \mu_2 + \mu_1 \mu_2 + 2 \mathfrak{e}_1 (1 - \mathfrak{e}_1 + \\
& \mu_1^2 (-23 + 18 \mathfrak{e}_1 - 17 \mathfrak{e}_2) + \mathfrak{e}_2 + \mu_2 (22 + 5 \mathfrak{e}_1 + \mathfrak{e}_2) + \\
& \mu_1 (11 \mathfrak{e}_1 + \mu_2 (-38 + 5 \mathfrak{e}_1 - 11 \mathfrak{e}_2) - 10 \times (1 + \mathfrak{e}_2)) \Big) \Big) - \\
& \eta^3 (-6 + 26 \mu_1 + 56 \mu_1^2 - 30 \mu_2 + 90 \mu_1 \mu_2 - \mathfrak{e}_1 (-6 - \mathfrak{e}_1 + \\
& \mu_1^2 (2 + 40 \mathfrak{e}_1 - 34 \mathfrak{e}_2) + \mu_2 (36 + 5 \mathfrak{e}_1 - 17 \mathfrak{e}_2) + \mathfrak{e}_2 + \\
& \mu_1 (20 + 15 \mathfrak{e}_1 - 9 \mathfrak{e}_2 + \mu_2 (-36 + 5 \mathfrak{e}_1 + 7 \mathfrak{e}_2)) \Big) + \\
& \eta \mathfrak{t} (-8 + 32 \mu_1 + 88 \mu_1^2 - 7 \mu_2 + 17 \mu_1 \mu_2 + \mathfrak{e}_1 (-6 - \mathfrak{e}_1 + \\
& \mu_1^2 (2 + 40 \mathfrak{e}_1 - 34 \mathfrak{e}_2) + \mu_2 (36 + 5 \mathfrak{e}_1 - 17 \mathfrak{e}_2) + \mathfrak{e}_2 + \\
& \mu_1 (20 + 15 \mathfrak{e}_1 - 9 \mathfrak{e}_2 + \mu_2 (-36 + 5 \mathfrak{e}_1 + 7 \mathfrak{e}_2)) \Big) \Big) \Big) - \\
& x^2 (-1 + \eta)^2 \Big( - \Big( (-1 + \eta) \mathfrak{e}_p (-12 \eta - 60 \eta^2 - 76 \eta^3 + 20 \eta^4 + 60 \eta^5 + \\
& 6 \eta \mathfrak{t} + 12 \eta \eta \mathfrak{t} - 24 \eta^2 \eta \mathfrak{t} - 80 \eta^3 \eta \mathfrak{t} - 60 \eta^4 \eta \mathfrak{t} + 120 \eta \mu_1 + \\
& 396 \eta^2 \mu_1 + 344 \eta^3 \mu_1 + 170 \eta^4 \mu_1 + 60 \eta^5 \mu_1 - 44 \eta \mathfrak{t} \mu_1 - \\
& 28 \eta \eta \mathfrak{t} \mu_1 + 24 \eta^2 \eta \mathfrak{t} \mu_1 - 56 \eta^3 \eta \mathfrak{t} \mu_1 - 60 \eta^4 \eta \mathfrak{t} \mu_1 + 132 \eta \mu_1^2 +
\end{aligned}$$

$$\begin{aligned}
& 600 \eta^2 \mu_1^2 + 900 \eta^3 \mu_1^2 + 510 \eta^4 \mu_1^2 - 98 \eta t \mu_1^2 - 424 \eta \eta t \mu_1^2 - \\
& 240 \eta^2 \eta t \mu_1^2 + 24 \eta^3 \eta t \mu_1^2 + 56 \eta \mu_2 + 12 \eta^2 \mu_2 - 204 \eta^3 \mu_2 - \\
& 240 \eta^4 \mu_2 + 38 \eta t \mu_2 + 117 \eta \eta t \mu_2 + 192 \eta^2 \eta t \mu_2 + 120 \eta^3 \eta t \mu_2 + \\
& 8 \eta \mu_1 \mu_2 + 444 \eta^2 \mu_1 \mu_2 + 612 \eta^3 \mu_1 \mu_2 + 240 \eta^4 \mu_1 \mu_2 - \\
& 58 \eta t \mu_1 \mu_2 - 171 \eta \eta t \mu_1 \mu_2 - 240 \eta^2 \eta t \mu_1 \mu_2 - 120 \eta^3 \eta t \mu_1 \mu_2 + \\
& w^4 (-1 + \eta)^4 (-2 + (30 - 82 \eta t) \mu_1^2 + 12 \eta^3 (1 + \mu_1) + 10 \mu_2 + \\
& \quad 17 \eta t \mu_2 + \mu_1 (28 - 7 \eta t (-2 + \mu_2) + 34 \mu_2) - 12 \eta^2 \\
& \quad (-1 + \eta t - 5 \mu_1 + \eta t \mu_1 - 4 \mu_1^2 + 3 \mu_2 - 3 \mu_1 \mu_2) - 2 \eta (2 - 55 \mu_1 - \\
& \quad 57 \mu_1^2 + 27 \mu_2 - 93 \mu_1 \mu_2 + 6 \eta t (1 + \mu_1 - 3 \mu_2 + 3 \mu_1 \mu_2)) + \\
& w^2 (-1 + \eta)^2 (30 \eta^5 (1 + \mu_1) + \eta t (20 - 104 \mu_1 - 652 \mu_1^2 + 181 \\
& \quad \mu_2 - 227 \mu_1 \mu_2) + 2 \times (-7 + 53 \mu_1 + 72 \mu_1^2 + 7 \mu_2 + 43 \mu_1 \mu_2) - \\
& \quad 3 \eta \eta t (8 + 420 \mu_1^2 - 177 \mu_2 + 11 \mu_1 (4 + 21 \mu_2)) + \\
& \quad 2 \eta (-43 + 591 \mu_1^2 - 69 \mu_2 + \mu_1 (404 + 567 \mu_2)) - \\
& \quad 4 \eta^3 (-40 - 225 \mu_1 - 305 \mu_1^2 + 161 \mu_2 - 271 \mu_1 \mu_2 + \\
& \quad 10 \eta t (4 + 4 \mu_1 - 3 \mu_2 + 3 \mu_1 \mu_2)) - 10 \eta^4 \\
& \quad (3 \eta t (1 + \mu_1) - 4 \times (4 + 7 \mu_1 + 3 \mu_1^2 - 3 \mu_2 + 3 \mu_1 \mu_2)) - \\
& \quad 12 \eta^2 (4 - 118 \mu_1 - 182 \mu_1^2 + 61 \mu_2 - 191 \mu_1 \mu_2 + \\
& \quad \eta t (15 + 11 \mu_1 + 20 \mu_1^2 - 40 \mu_2 + 44 \mu_1 \mu_2)) - w^3 (-1 + \eta)^3 \\
& (40 \eta^4 (1 + \mu_1) + 4 \eta^3 (21 + 61 \mu_1 + 40 \mu_1^2 - 10 \eta t (1 + \mu_1) - \\
& \quad 36 \mu_2 + 36 \mu_1 \mu_2) + \eta t (6 - 400 \mu_1^2 + 97 \mu_2 - 5 \mu_1 (2 + 19 \mu_2)) + \\
& \quad 2 \times (-4 + 65 \mu_1^2 + 6 \mu_2 + \mu_1 (49 + 54 \mu_2)) + 12 \eta^2 (2 + 49 \mu_1 + \\
& \quad 59 \mu_1^2 - 29 \mu_2 + 73 \mu_1 \mu_2 - \eta t (7 + 7 \mu_1 - 12 \mu_2 + 12 \mu_1 \mu_2)) - \\
& \quad 3 \eta (10 - 232 \mu_1^2 + 68 \mu_2 - 2 \mu_1 (87 + 146 \mu_2) + \\
& \quad \eta t (12 + 140 \mu_1^2 - 87 \mu_2 + 3 \mu_1 (8 + 35 \mu_2))) - \\
& w (-1 + \eta) \times (90 \eta^5 (1 + \mu_1) + 4 \times (1 + \mu_1) \times (-1 + 11 \mu_1 + 3 \mu_2) + \\
& \quad \eta t (20 - 124 \mu_1 - 432 \mu_1^2 + 139 \mu_2 - 197 \mu_1 \mu_2) + \\
& \quad 10 \eta^4 (20 + 47 \mu_1 + 63 \mu_1^2 - 9 \eta t (1 + \mu_1) - 36 \mu_2 + 36 \mu_1 \mu_2) + \\
& \quad 4 \eta^3 (3 + 253 \mu_1 + 490 \mu_1^2 - 176 \mu_2 + 388 \mu_1 \mu_2 + \\
& \quad \eta t (-50 - 44 \mu_1 + 6 \mu_1^2 + 60 \mu_2 - 60 \mu_1 \mu_2)) - \\
& \quad 12 \eta^2 (14 - 103 \mu_1 - 177 \mu_1^2 + 34 \mu_2 - 158 \mu_1 \mu_2 + \\
& \quad \eta t (11 + 3 \mu_1 + 40 \mu_1^2 - 44 \mu_2 + 52 \mu_1 \mu_2)) + \\
& \quad \eta (-72 + 516 \mu_1 + 732 \mu_1^2 + 68 \mu_2 + 452 \mu_1 \mu_2 + \\
& \quad \eta t (12 - 1264 \mu_1^2 + 423 \mu_2 - 5 \mu_1 (20 + 117 \mu_2)))) + \\
& (-1 + \eta t) \theta l (-2 - 12 \eta - 12 \eta^2 + 2 \theta p + 6 \eta \theta p - 36 \eta^2 \theta p - 100 \eta^3 \theta p - \\
& \quad 60 \eta^4 \theta p + 20 \mu_1 + 136 \eta \mu_1 + 104 \eta^2 \mu_1 - 16 \eta^3 \mu_1 - 16 \eta^4 \mu_1 - \\
& \quad 20 \theta p \mu_1 - 56 \eta \theta p \mu_1 + 126 \eta^2 \theta p \mu_1 + 192 \eta^3 \theta p \mu_1 - 10 \eta^4 \theta p \mu_1 + \\
& \quad 22 \mu_1^2 + 148 \eta \mu_1^2 + 380 \eta^2 \mu_1^2 + 176 \eta^3 \mu_1^2 - 16 \eta^4 \mu_1^2 - 22 \theta p \mu_1^2 - \\
& \quad 134 \eta \theta p \mu_1^2 + 18 \eta^2 \theta p \mu_1^2 + 532 \eta^3 \theta p \mu_1^2 + 410 \eta^4 \theta p \mu_1^2 + \\
& \quad 2 w^4 (-1 + \eta)^4 (-1 + 23 \mu_1^2 + \eta (-2 + 64 \mu_1^2 + \mu_1 (2 - 5 \mu_2) - 5 \mu_2) - \\
& \quad 5 \mu_1 (-2 + \mu_2) - 5 \mu_2) - 19 \mu_2 - 76 \eta \mu_2 - 57 \eta^2 \mu_2 + \\
& \quad 14 \theta p \mu_2 + 112 \eta \theta p \mu_2 + 186 \eta^2 \theta p \mu_2 - 100 \eta^4 \theta p \mu_2 + 29 \mu_1 \mu_2 + \\
& \quad 116 \eta \mu_1 \mu_2 + 87 \eta^2 \mu_1 \mu_2 - 34 \theta p \mu_1 \mu_2 - 200 \eta \theta p \mu_1 \mu_2 - \\
& \quad 174 \eta^2 \theta p \mu_1 \mu_2 + 144 \eta^3 \theta p \mu_1 \mu_2 + 140 \eta^4 \theta p \mu_1 \mu_2 - \\
& \quad \theta p \mathfrak{s} 1 - 6 \eta \theta p \mathfrak{s} 1 - 6 \eta^2 \theta p \mathfrak{s} 1 + 10 \theta p \mu_1 \mathfrak{s} 1 + 68 \eta \theta p \mu_1 \mathfrak{s} 1 +
\end{aligned}$$

$$\begin{aligned}
& 93 \eta^2 \operatorname{er} \mu_1 \mathfrak{x}_1 + 36 \eta^3 \operatorname{er} \mu_1 \mathfrak{x}_1 + 10 \eta^4 \operatorname{er} \mu_1 \mathfrak{x}_1 + 11 \operatorname{er} \mu_1^2 \mathfrak{x}_1 + \\
& 110 \eta \operatorname{er} \mu_1^2 \mathfrak{x}_1 + 243 \eta^2 \operatorname{er} \mu_1^2 \mathfrak{x}_1 + 156 \eta^3 \operatorname{er} \mu_1^2 \mathfrak{x}_1 + \\
& 10 \eta^4 \operatorname{er} \mu_1^2 \mathfrak{x}_1 + 5 \operatorname{er} \mu_2 \mathfrak{x}_1 + 30 \eta \operatorname{er} \mu_2 \mathfrak{x}_1 + 30 \eta^2 \operatorname{er} \mu_2 \mathfrak{x}_1 + \\
& 5 \operatorname{er} \mu_1 \mu_2 \mathfrak{x}_1 + 30 \eta \operatorname{er} \mu_1 \mu_2 \mathfrak{x}_1 + 30 \eta^2 \operatorname{er} \mu_1 \mu_2 \mathfrak{x}_1 + \\
& \operatorname{er} \mathfrak{x}_2 + 6 \eta \operatorname{er} \mathfrak{x}_2 + 6 \eta^2 \operatorname{er} \mathfrak{x}_2 - 10 \operatorname{er} \mu_1 \mathfrak{x}_2 - 58 \eta \operatorname{er} \mu_1 \mathfrak{x}_2 - \\
& 51 \eta^2 \operatorname{er} \mu_1 \mathfrak{x}_2 + 16 \eta^3 \operatorname{er} \mu_1 \mathfrak{x}_2 + 10 \eta^4 \operatorname{er} \mu_1 \mathfrak{x}_2 - \\
& 11 \operatorname{er} \mu_1^2 \mathfrak{x}_2 - 100 \eta \operatorname{er} \mu_1^2 \mathfrak{x}_2 - 201 \eta^2 \operatorname{er} \mu_1^2 \mathfrak{x}_2 - \\
& 104 \eta^3 \operatorname{er} \mu_1^2 \mathfrak{x}_2 + 10 \eta^4 \operatorname{er} \mu_1^2 \mathfrak{x}_2 + 7 \operatorname{er} \mu_2 \mathfrak{x}_2 + 6 \eta \operatorname{er} \mu_2 \mathfrak{x}_2 - \\
& 102 \eta^2 \operatorname{er} \mu_2 \mathfrak{x}_2 - 120 \eta^3 \operatorname{er} \mu_2 \mathfrak{x}_2 - 17 \operatorname{er} \mu_1 \mu_2 \mathfrak{x}_2 - \\
& 66 \eta \operatorname{er} \mu_1 \mu_2 \mathfrak{x}_2 + 42 \eta^2 \operatorname{er} \mu_1 \mu_2 \mathfrak{x}_2 + 120 \eta^3 \operatorname{er} \mu_1 \mu_2 \mathfrak{x}_2 - \\
& w^3 (-1 + \eta)^3 (-8 - 49 \mu_2 - \operatorname{er} \mathfrak{x}_1 + 5 \operatorname{er} \mu_2 \mathfrak{x}_1 + 8 \mu_1^2 (20 + 3 \operatorname{er} (\mathfrak{x}_1 - \mathfrak{x}_2)) + \\
& \quad \mu_1 (80 + \mu_2 (-1 + 5 \operatorname{er} (\mathfrak{x}_1 - \mathfrak{x}_2)) + 11 \operatorname{er} (\mathfrak{x}_1 - \mathfrak{x}_2)) + \\
& \quad \operatorname{er} \mathfrak{x}_2 - 5 \operatorname{er} \mu_2 \mathfrak{x}_2 + 3 \eta^2 (-4 - 2 \operatorname{er} \mathfrak{x}_1 + \\
& \quad \mu_2 (-19 + 10 \operatorname{er} (\mathfrak{x}_1 - \mathfrak{x}_2)) + 4 \mu_1^2 (31 + 12 \operatorname{er} (\mathfrak{x}_1 - \mathfrak{x}_2)) + \\
& \quad \mu_1 (32 + \mu_2 (29 + 10 \operatorname{er} (\mathfrak{x}_1 - \mathfrak{x}_2)) + 22 \operatorname{er} (\mathfrak{x}_1 - \mathfrak{x}_2)) + \\
& \quad 2 \operatorname{er} \mathfrak{x}_2) + 2 \eta (-12 - 53 \mu_2 - 3 \operatorname{er} \mathfrak{x}_1 + 15 \operatorname{er} \mu_2 \mathfrak{x}_1 + \\
& \quad \mu_1 (86 + \mu_2 (43 + 15 \operatorname{er} (\mathfrak{x}_1 - \mathfrak{x}_2)) + 33 \operatorname{er} (\mathfrak{x}_1 - \mathfrak{x}_2)) + \\
& \quad \mu_1^2 (326 + 72 \operatorname{er} (\mathfrak{x}_1 - \mathfrak{x}_2)) + 3 \operatorname{er} \mathfrak{x}_2 - 15 \operatorname{er} \mu_2 \mathfrak{x}_2) + \\
& w^2 (-1 + \eta)^2 (3 \times (-4 + 68 \mu_1^2 - 29 \mu_2 + \mu_1 (40 + 19 \mu_2)) + \\
& \quad \operatorname{er} (-2 - 3 \mathfrak{x}_1 + \mu_1^2 (-48 + 59 \mathfrak{x}_1 - 59 \mathfrak{x}_2) + \\
& \quad \mu_1 (-26 + 32 \mathfrak{x}_1 + \mu_2 (-62 + 15 \mathfrak{x}_1 - 27 \mathfrak{x}_2) - 32 \mathfrak{x}_2) + \\
& \quad \mu_2 (34 + 15 \mathfrak{x}_1 - 3 \mathfrak{x}_2) + 3 \mathfrak{x}_2) + 3 \eta (-16 + 356 \mu_1^2 - 86 \mu_2 + \\
& \quad 2 \mu_1 (78 + 53 \mu_2) + \operatorname{er} \mu_1^2 (-44 + 133 \mathfrak{x}_1 - 129 \mathfrak{x}_2) + \\
& \quad \operatorname{er} \mu_1 (-26 + 67 \mathfrak{x}_1 + 6 \mu_2 (-15 + 5 \mathfrak{x}_1 - 7 \mathfrak{x}_2) - 63 \mathfrak{x}_2) + \\
& \quad 6 \operatorname{er} (-1 - \mathfrak{x}_1 + \mu_2 (9 + 5 \mathfrak{x}_1 - 3 \mathfrak{x}_2) + \mathfrak{x}_2)) + \\
& 3 \eta^2 (-12 + 96 \mu_1 + 372 \mu_1^2 - 57 \mu_2 + 87 \mu_1 \mu_2 + 2 \operatorname{er} \\
& \quad (\mu_1^2 (56 + 89 \mathfrak{x}_1 - 81 \mathfrak{x}_2) + \mu_1 (26 + 38 \mathfrak{x}_1 + 3 \mu_2 (2 + 5 \mathfrak{x}_1 - \mathfrak{x}_2) - \\
& \quad 30 \mathfrak{x}_2) + 3 \times (-2 - \mathfrak{x}_1 + \mu_2 (2 + 5 \mathfrak{x}_1 - 9 \mathfrak{x}_2) + \mathfrak{x}_2))) + 2 \eta^3 \\
& \quad (8 \mu_1 (-1 + 11 \mu_1) + 5 \operatorname{er} (\mu_1^2 (52 + 15 \mathfrak{x}_1 - 11 \mathfrak{x}_2) - 2 \times (1 + 7 \\
& \quad \mu_2 + 6 \mu_2 \mathfrak{x}_2) + \mu_1 (26 + 34 \mu_2 + 3 \mathfrak{x}_1 + \mathfrak{x}_2 + 12 \mu_2 \mathfrak{x}_2))) - \\
& w (-1 + \eta) \times (-8 + 80 \mu_1 + 112 \mu_1^2 - 67 \mu_2 + 77 \mu_1 \mu_2 + \operatorname{er} \\
& \quad (4 - 3 \mathfrak{x}_1 + \mu_1^2 (-70 + 46 \mathfrak{x}_1 - 46 \mathfrak{x}_2) + \mu_1 (-42 + 31 \mathfrak{x}_1 + 3 \mu_2 (-32 + \\
& \quad 5 \mathfrak{x}_1 - 13 \mathfrak{x}_2) - 31 \mathfrak{x}_2) + 3 \mathfrak{x}_2 + 3 \mu_2 (16 + 5 \mathfrak{x}_1 + 3 \mathfrak{x}_2)) + \\
& 2 \eta^4 (-50 \operatorname{er} \mu_2 + \mu_1^2 (-8 + 5 \operatorname{er} (41 + \mathfrak{x}_1 + \mathfrak{x}_2)) + \mu_1 \\
& \quad (-8 + 5 \operatorname{er} (5 + 14 \mu_2 + \mathfrak{x}_1 + \mathfrak{x}_2))) + 2 \eta^3 (16 \mu_1 (-1 + 11 \mu_1) + \\
& \quad \operatorname{er} (\mu_1^2 (526 + 153 \mathfrak{x}_1 - 107 \mathfrak{x}_2) - 10 \times (6 + 7 \mu_2 + 12 \mu_2 \mathfrak{x}_2) + \\
& \quad \mu_1 (226 + 242 \mu_2 + 33 \mathfrak{x}_1 + 13 \mathfrak{x}_2 + 120 \mu_2 \mathfrak{x}_2))) + \\
& \eta^2 (-36 + 296 \mu_1 + 1124 \mu_1^2 - 171 \mu_2 + 261 \mu_1 \mu_2 + 3 \operatorname{er} (-40 - \\
& \quad 6 \mathfrak{x}_1 + \mu_1^2 (118 + 211 \mathfrak{x}_1 - 181 \mathfrak{x}_2) + \mu_2 (74 + 30 \mathfrak{x}_1 - 78 \mathfrak{x}_2) + \\
& \quad 6 \mathfrak{x}_2 + \mu_1 (78 + 85 \mathfrak{x}_1 - 55 \mathfrak{x}_2 + 2 \mu_2 (-23 + 15 \mathfrak{x}_1 + 9 \mathfrak{x}_2))) + \\
& \eta (-40 + 692 \mu_1^2 - 238 \mu_2 + \mu_1 (436 + 338 \mu_2) + \operatorname{er} \\
& \quad (\mu_1 (-134 + 203 \mathfrak{x}_1 + 2 \mu_2 (-235 + 45 \mathfrak{x}_1 - 81 \mathfrak{x}_2) - 181 \mathfrak{x}_2) + \\
& \quad 2 \times (-6 - 9 \mathfrak{x}_1 + \mu_2 (137 + 45 \mathfrak{x}_1 - 9 \mathfrak{x}_2) + 9 \mathfrak{x}_2) + \\
& \quad \mu_1^2 (365 \mathfrak{x}_1 - 7 \times (38 + 49 \mathfrak{x}_2)))) +
\end{aligned}$$

$$\begin{aligned}
& x^5 (-1 + \eta)^5 \left( 4 \times (-1 + w (-1 + \eta)) \times (-1 + \eta t) \, \text{el} \, \mu_1 (1 + \eta - 11 \mu_1 + \right. \\
& \quad \left. \eta \mu_1 + w (-1 + \eta) \times (-1 + 11 \mu_1)) + \right. \\
& \quad \text{op} \left( -10 - 6 \eta + 40 \eta^2 - 24 \eta^3 - 8 \eta t - 16 \eta \eta t + 24 \eta^2 \eta t + 10 \, \text{el} + \right. \\
& \quad 24 \eta \, \text{el} - 10 \eta t \, \text{el} - 24 \eta \eta t \, \text{el} + 32 \mu_1 + 12 \eta \mu_1 - 20 \eta^2 \mu_1 - \\
& \quad 24 \eta^3 \mu_1 - 8 \eta t \mu_1 - 16 \eta \eta t \mu_1 + 24 \eta^2 \eta t \mu_1 - 18 \, \text{el} \mu_1 + \\
& \quad 10 \eta \, \text{el} \mu_1 + 18 \eta t \, \text{el} \mu_1 - 10 \eta \eta t \, \text{el} \mu_1 + 90 \mu_1^2 + 114 \eta \mu_1^2 - \\
& \quad 204 \eta^2 \mu_1^2 - 52 \, \text{el} \mu_1^2 - 158 \eta \, \text{el} \mu_1^2 + 52 \eta t \, \text{el} \mu_1^2 + \\
& \quad 158 \eta \eta t \, \text{el} \mu_1^2 + 4 w^3 (-1 + \eta)^4 (1 + \mu_1) (\eta - \eta t + 4 \mu_1) + \\
& \quad 6 \mu_2 - 30 \eta \mu_2 + 24 \eta^2 \mu_2 + 12 \eta t \mu_2 - 12 \eta \eta t \mu_2 - 6 \, \text{el} \mu_2 + \\
& \quad 10 \eta \, \text{el} \mu_2 + 6 \eta t \, \text{el} \mu_2 - 10 \eta \eta t \, \text{el} \mu_2 + 30 \mu_1 \mu_2 - 6 \eta \mu_1 \mu_2 - \\
& \quad 24 \eta^2 \mu_1 \mu_2 - 12 \eta t \mu_1 \mu_2 + 12 \eta \eta t \mu_1 \mu_2 - 6 \, \text{el} \mu_1 \mu_2 - \\
& \quad 14 \eta \, \text{el} \mu_1 \mu_2 + 6 \eta t \, \text{el} \mu_1 \mu_2 + 14 \eta \eta t \, \text{el} \mu_1 \mu_2 - 3 \, \text{el} \mu_1 \, \text{el} \mu_1 - \\
& \quad \eta \, \text{el} \mu_1 \, \text{el} \mu_1 + 3 \eta t \, \text{el} \mu_1 \, \text{el} \mu_1 + \eta \eta t \, \text{el} \mu_1 \, \text{el} \mu_1 - 15 \, \text{el} \mu_1^2 \, \text{el} \mu_1 - \\
& \quad \eta \, \text{el} \mu_1^2 \, \text{el} \mu_1 + 15 \eta t \, \text{el} \mu_1^2 \, \text{el} \mu_1 + \eta \eta t \, \text{el} \mu_1^2 \, \text{el} \mu_1 - \, \text{el} \mu_1 \, \text{el} \mu_2 - \\
& \quad \eta \, \text{el} \mu_1 \, \text{el} \mu_2 + \eta t \, \text{el} \mu_1 \, \text{el} \mu_2 + \eta \eta t \, \text{el} \mu_1 \, \text{el} \mu_2 + 11 \, \text{el} \mu_1^2 \, \text{el} \mu_2 - \\
& \quad \eta \, \text{el} \mu_1^2 \, \text{el} \mu_2 - 11 \eta t \, \text{el} \mu_1^2 \, \text{el} \mu_2 + \eta \eta t \, \text{el} \mu_1^2 \, \text{el} \mu_2 + 12 \, \text{el} \mu_2 \, \text{el} \mu_2 - \\
& \quad 12 \eta t \, \text{el} \mu_2 \, \text{el} \mu_2 - 12 \, \text{el} \mu_1 \mu_2 \, \text{el} \mu_2 + 12 \eta t \, \text{el} \mu_1 \mu_2 \, \text{el} \mu_2 - \\
& \quad w^2 (-1 + \eta)^2 (2 - 2 \, \text{el} - 72 \mu_1 + 26 \, \text{el} \mu_1 - 122 \mu_1^2 + 52 \, \text{el} \mu_1^2 + \\
& \quad 12 \eta^3 (1 + \mu_1) + 14 \mu_2 - 14 \, \text{el} \mu_2 - 58 \mu_1 \mu_2 + 34 \, \text{el} \mu_1 \mu_2 + \\
& \quad 4 \eta^2 (1 + 13 \mu_1 + 12 \mu_1^2 - 3 \eta t (1 + \mu_1) - 3 \mu_2 + 3 \mu_1 \mu_2) + \\
& \quad 4 \eta t (4 - 3 \mu_2 + \mu_1 (4 + 3 \mu_2)) - 2 \eta (9 - 4 \mu_1 - 37 \mu_1^2 + \mu_2 - 23 \mu_1 \mu_2 + \\
& \quad 2 \eta t (1 + \mu_1 - 3 \mu_2 + 3 \mu_1 \mu_2)) + 3 \, \text{el} \mu_1 \, \text{el} \mu_1 + 15 \, \text{el} \mu_1^2 \, \text{el} \mu_1 + \\
& \quad \text{el} \mu_1 \, \text{el} \mu_2 - 11 \, \text{el} \mu_1^2 \, \text{el} \mu_2 - 12 \, \text{el} \mu_2 \, \text{el} \mu_2 + 12 \, \text{el} \mu_1 \mu_2 \, \text{el} \mu_2 - \\
& \quad \eta t \, \text{el} (\mu_1^2 (52 + 15 \, \text{el} - 11 \, \text{el} \mu_2) - 2 \times (1 + 7 \mu_2 + 6 \mu_2 \, \text{el} \mu_2) + \\
& \quad \mu_1 (26 + 34 \mu_2 + 3 \, \text{el} \mu_1 + \, \text{el} \mu_2 + 12 \mu_2 \, \text{el} \mu_2)) + w (-1 + \eta) \times \\
& \quad (36 \eta^3 (1 + \mu_1) - 4 \eta^2 (4 - 63 \mu_1^2 + 9 \eta t (1 + \mu_1) + 9 \mu_2 - \mu_1 (23 + 9 \mu_2)) + \\
& \quad \eta (-32 + 28 \mu_2 - 10 \, \text{el} \mu_2 + \mu_1^2 (-56 + \, \text{el} (158 + \, \text{el} \mu_1 + \, \text{el} \mu_2)) + \\
& \quad \mu_1 (-40 + 52 \mu_2 + \, \text{el} (14 + 14 \mu_2 + \, \text{el} \mu_1 + \, \text{el} \mu_2)) - \\
& \quad \eta t (-16 - 2 \times (12 + 5 \, \text{el} \mu_2) + 8 \mu_1 (-2 + 3 \mu_2) + \\
& \quad \, \text{el} \mu_1^2 (158 + \, \text{el} \mu_1 + \, \text{el} \mu_2) + \, \text{el} \mu_1 (14 + 14 \mu_2 + \, \text{el} \mu_1 + \, \text{el} \mu_2))) - \\
& \quad 2 \times (-6 + 44 \mu_1 + 98 \mu_1^2 - 4 \mu_2 + 44 \mu_1 \mu_2 - \, \text{el} \\
& \quad (\mu_1^2 (52 + 15 \, \text{el} - 11 \, \text{el} \mu_2) + \mu_1 (22 + 3 \, \text{el} \mu_1 + \, \text{el} \mu_2 + 4 \mu_2 (5 + 3 \, \text{el} \mu_2)) - \\
& \quad 2 \times (3 + \mu_2 (2 + 6 \, \text{el} \mu_2))) + \eta t (-2 \times (5 - 6 \mu_2 + \mu_1 (5 + 6 \mu_2)) + \\
& \quad \, \text{el} (\mu_1^2 (52 + 15 \, \text{el} - 11 \, \text{el} \mu_2) + \mu_1 (22 + 3 \, \text{el} \mu_1 + \, \text{el} \mu_2 + \\
& \quad 4 \mu_2 (5 + 3 \, \text{el} \mu_2)) - 2 \times (3 + \mu_2 (2 + 6 \, \text{el} \mu_2)))))) - \\
& \quad \times (-1 + \eta) \times (4 w^2 (3 - 5 w + 2 w^2) \eta^9 \, \text{op} (1 + \mu_1) - 4 w \eta^8 \, \text{op} (9 \times (1 + \mu_1) + \\
& \quad w (-11 - 23 \mu_1 - 12 \mu_1^2 + 3 \eta t (1 + \mu_1) + 15 \mu_2 - 15 \mu_1 \mu_2) + \\
& \quad w^3 (7 - \mu_1 - 8 \mu_1^2 + 2 \eta t (1 + \mu_1) + 9 \mu_2 - 9 \mu_1 \mu_2) + \\
& \quad w^2 (-6 + 14 \mu_1 + 20 \mu_1^2 - 5 \eta t (1 + \mu_1) - 24 \mu_2 + 24 \mu_1 \mu_2)) + \\
& \quad (1 + w)^3 (-5 w \, \text{el} (1 + \mu_1) \mu_2 + 5 w \eta t \, \text{el} (1 + \mu_1) \mu_2 + \\
& \quad \eta t \, \text{op} (-2 + 22 \mu_1^2 + 2 w (-1 + 29 \mu_1^2 + \mu_1 (4 - 5 \mu_2) - 5 \mu_2) - \\
& \quad 19 \mu_2 + \mu_1 (20 + 29 \mu_2))) - 2 \eta^7 \, \text{op} (-12 \times (1 + \mu_1) + \\
& \quad 2 w (7 + 34 \mu_1 + 63 \mu_1^2 - 9 \eta t (1 + \mu_1) - 45 \mu_2 + 45 \mu_1 \mu_2) + 2 w^3 \\
& \quad (-18 - 4 \mu_1 + 38 \mu_1^2 + 23 \mu_2 + 65 \mu_1 \mu_2 + 6 \eta t (1 + \mu_1 + 4 \mu_2 - 4 \mu_1 \mu_2)) +
\end{aligned}$$



$$\begin{aligned}
& w^4 \left( -9 + 14 \mu_1 + 23 \mu_1^2 - 57 \mu_2 - 9 \mu_1 \mu_2 + 2 \eta t \right. \\
& \quad \left. (-7 - 7 \mu_1 - 9 \mu_2 + 9 \mu_1 \mu_2) \right) + w^2 \left( 47 - 66 \mu_1 - 233 \mu_1^2 + \right. \\
& \quad \left. 113 \mu_2 - 223 \mu_1 \mu_2 + \eta t (22 + 22 \mu_1 - 30 \mu_2 + 30 \mu_1 \mu_2) \right) - \\
& \eta \left( \theta p \left( 8 w (1 + \mu_1) \times (-1 + 11 \mu_1 + 3 \mu_2) - 4 w \eta t (-6 + 49 \mu_1 + \right. \right. \\
& \quad \left. 133 \mu_1^2 - 36 \mu_2 + 60 \mu_1 \mu_2) + \eta t (10 - 150 \mu_1^2 + 57 \mu_2 - \right. \\
& \quad \left. \mu_1 (92 + 87 \mu_2)) + 2 w^4 (-2 + 28 \mu_1 + 30 \mu_1^2 + 10 \mu_2 + \right. \\
& \quad \left. 34 \mu_1 \mu_2 + \eta t (-5 + 28 \mu_1 + 69 \mu_1^2 - 8 \mu_2 - 32 \mu_1 \mu_2) \right) + \\
& w^2 \left( \eta t (4 - 64 \mu_1 - 476 \mu_1^2 + 101 \mu_2 - 283 \mu_1 \mu_2) + \right. \\
& \quad \left. 4 \times (-7 + 53 \mu_1 + 72 \mu_1^2 + 7 \mu_2 + 43 \mu_1 \mu_2) \right) + \\
& 2 w^3 \left( \eta t (-10 + 48 \mu_1 + 22 \mu_1^2 - \mu_2 - 97 \mu_1 \mu_2) + \right. \\
& \quad \left. 2 \times (-4 + 49 \mu_1 + 65 \mu_1^2 + 6 \mu_2 + 54 \mu_1 \mu_2) \right) + \\
& (-1 + \eta t) \theta l \left( -2 + 20 \mu_1 + 22 \mu_1^2 - 19 \mu_2 + 29 \mu_1 \mu_2 + 2 w^4 (1 + \mu_1) \times \right. \\
& \quad \left. (-1 + 17 \mu_1 + 5 \mu_2) + 2 w^3 (-4 - \theta p \mathfrak{x}1 + \mu_2 (-2 + 5 \theta p (\mathfrak{x}1 - \mathfrak{x}2)) + \right. \\
& \quad \left. \mu_1 (58 + \mu_2 (22 + 5 \theta p (\mathfrak{x}1 - \mathfrak{x}2)) + 11 \theta p (\mathfrak{x}1 - \mathfrak{x}2)) + \right. \\
& \quad \left. \mu_1^2 (62 + 24 \theta p (\mathfrak{x}1 - \mathfrak{x}2)) + \theta p \mathfrak{x}2) \right) + \\
& w^2 \left( 3 \times (-4 + 56 \mu_1^2 - 19 \mu_2 + \mu_1 (52 + 29 \mu_2)) + \right. \\
& \quad \left. 2 \theta p (-2 - 3 \mathfrak{x}1 + \mu_1^2 (-48 + 59 \mathfrak{x}1 - 59 \mathfrak{x}2) + \right. \\
& \quad \left. \mu_1 (-26 + 32 \mathfrak{x}1 + \mu_2 (-62 + 15 \mathfrak{x}1 - 27 \mathfrak{x}2) - 32 \mathfrak{x}2) + \right. \\
& \quad \left. \mu_2 (34 + 15 \mathfrak{x}1 - 3 \mathfrak{x}2) + 3 \mathfrak{x}2) \right) + 2 \theta p \\
& \left( 2 - \mathfrak{x}1 + 11 \mu_1^2 (-2 + \mathfrak{x}1 - \mathfrak{x}2) + \mathfrak{x}2 + \mu_2 (14 + 5 \mathfrak{x}1 + 7 \mathfrak{x}2) + \right. \\
& \quad \left. \mu_1 (5 \mu_2 \mathfrak{x}1 + 10 \times (-2 + \mathfrak{x}1 - \mathfrak{x}2) - 17 \mu_2 (2 + \mathfrak{x}2)) \right) + \\
& 2 w \left( -4 + 46 \mu_1 + 50 \mu_1^2 - 31 \mu_2 + 41 \mu_1 \mu_2 + \theta p (4 - 3 \mathfrak{x}1 + \mu_1^2 \right. \\
& \quad \left. (-70 + 46 \mathfrak{x}1 - 46 \mathfrak{x}2) + \mu_1 (-42 + 31 \mathfrak{x}1 + 3 \mu_2 (-32 + 5 \mathfrak{x}1 - \right. \\
& \quad \left. 13 \mathfrak{x}2) - 31 \mathfrak{x}2) + 3 \mathfrak{x}2 + 3 \mu_2 (16 + 5 \mathfrak{x}1 + 3 \mathfrak{x}2) \right) \left. \right) + \\
& \eta^3 \left( \theta p (-\eta t (-28 + 72 \mu_1 + 244 \mu_1^2 + 11 \mu_2 + 11 \mu_1 \mu_2) - 4 \times (-7 + \right. \\
& \quad \left. 36 \mu_1 + 67 \mu_1^2 - 17 \mu_2 + 79 \mu_1 \mu_2) + 4 w^3 (-8 + 132 \mu_1 + 188 \mu_1^2 - \right. \\
& \quad \left. 203 \mu_2 + 427 \mu_1 \mu_2 + \eta t (-32 - 6 \mu_1 + 518 \mu_1^2 - 5 \mu_2 - 5 \mu_1 \mu_2) \right) + \\
& 2 w^4 \left( 9 - 22 \mu_1 - 31 \mu_1^2 - 247 \mu_2 + 137 \mu_1 \mu_2 + 2 \eta t \right. \\
& \quad \left. (-8 - 73 \mu_1 + 235 \mu_1^2 - 15 \mu_2 + 15 \mu_1 \mu_2) \right) - \\
& 4 w \left( 2 \times (4 - 15 \mu_1 + 5 \mu_1^2 - 59 \mu_2 + 61 \mu_1 \mu_2) + \eta t \right. \\
& \quad \left. (-18 - \mu_1 + 323 \mu_1^2 - 54 \mu_2 + 90 \mu_1 \mu_2) \right) - \\
& 2 w^2 \left( 75 - 418 \mu_1 - 613 \mu_1^2 - 7 \mu_2 - 667 \mu_1 \mu_2 + \eta t \right. \\
& \quad \left. (30 - 170 \mu_1 + 28 \mu_1^2 - 137 \mu_2 + 211 \mu_1 \mu_2) \right) + \\
& (-1 + \eta t) \theta l \left( 4 - 44 \mu_1 - 120 \mu_1^2 + 19 \mu_2 - 29 \mu_1 \mu_2 + 4 w^4 \right. \\
& \quad \left. (1 + 7 \mu_1^2 + 5 \mu_1 (-8 + \mu_2) + 5 \mu_2) + 8 w^3 (-1 - \theta p \mathfrak{x}1 + \right. \\
& \quad \left. \mu_2 (-1 + 5 \theta p (\mathfrak{x}1 - \mathfrak{x}2)) + \mu_1 (-5 + \mu_2 (11 + 5 \theta p (\mathfrak{x}1 - \mathfrak{x}2)) + \right. \\
& \quad \left. 11 \theta p (\mathfrak{x}1 - \mathfrak{x}2)) + \mu_1^2 (50 + 24 \theta p (\mathfrak{x}1 - \mathfrak{x}2)) + \theta p \mathfrak{x}2) \right) + \\
& 2 w^2 \left( 3 \times (-4 + 74 \mu_1^2 - 19 \mu_2 + \mu_1 (50 + 29 \mu_2)) + \theta p (-4 - 9 \mathfrak{x}1 + \right. \\
& \quad \left. \mu_1 (-104 + 93 \mathfrak{x}1 + \mu_2 (-220 + 45 \mathfrak{x}1 - 93 \mathfrak{x}2) - 97 \mathfrak{x}2) + 2 \mu_1^2 \right. \\
& \quad \left. (-98 + 81 \mathfrak{x}1 - 83 \mathfrak{x}2) + 9 \mathfrak{x}2 + \mu_2 (116 + 45 \mathfrak{x}1 + 3 \mathfrak{x}2) \right) \left. \right) - \\
& \theta p \left( \mu_1^2 (10 + 161 \mathfrak{x}1 - 135 \mathfrak{x}2) + 2 \mu_2 (67 + 10 \mathfrak{x}1 - 34 \mathfrak{x}2) - \right. \\
& \quad \left. 4 \times (6 + \mathfrak{x}1 - \mathfrak{x}2) + \mu_1 (82 + 61 \mathfrak{x}1 - \right. \\
& \quad \left. 35 \mathfrak{x}2 + 2 \mu_2 (-65 + 10 \mathfrak{x}1 + 14 \mathfrak{x}2)) \right) +
\end{aligned}$$

$$\begin{aligned}
& w \left( -8 - 48 \mu_1^2 - 62 \mu_2 + 2 \mu_1 (68 + 41 \mu_2) + \text{op} \left( 68 - 6 \mathfrak{e}1 + \right. \right. \\
& \quad \left. \mu_1 (-290 + 33 \mathfrak{e}1 + 6 \mu_2 (-63 + 5 \mathfrak{e}1 - 33 \mathfrak{e}2) - 71 \mathfrak{e}2) + 6 \mathfrak{e}2 + \right. \\
& \quad \left. \mu_1^2 (-502 - 57 \mathfrak{e}1 + 19 \mathfrak{e}2) + 6 \mu_2 (21 + 5 \mathfrak{e}1 + 23 \mathfrak{e}2) \right) \left. \right) \left. \right) + \\
& \eta^2 \left( -\text{op} \left( -12 - 4 \times (-33 + 58 \eta t) \mu_1^2 + 76 \mu_2 + 41 \eta t \mu_2 + \mu_1 \right. \right. \\
& \quad \left. (120 + 56 \eta t - 20 \mu_2 - 55 \eta t \mu_2) + \right. \\
& \quad 4 w \left( -14 + 89 \mu_1 + 139 \mu_1^2 + 10 \mu_2 + 94 \mu_1 \mu_2 \right) + 6 w \eta t \\
& \quad \left( -10 + 40 \mu_1^2 - 11 \mu_2 + 7 \mu_1 (10 + 3 \mu_2) \right) + 2 w^4 \left( 9 - 84 \mu_1 - 93 \mu_1^2 - \right. \\
& \quad \left. 83 \mu_2 - 71 \mu_1 \mu_2 + \eta t \left( 4 - 86 \mu_1 + 90 \mu_1^2 - 17 \mu_2 + 67 \mu_1 \mu_2 \right) \right) + \\
& \quad 2 w^2 \left( 1 + 88 \mu_1 + 159 \mu_1^2 - 123 \mu_2 + 321 \mu_1 \mu_2 + 3 \eta t \right. \\
& \quad \left. \left( -18 + 82 \mu_1 + 280 \mu_1^2 - 49 \mu_2 + 83 \mu_1 \mu_2 \right) \right) + \\
& \quad w^3 \left( -8 \times \left( -5 + 32 \mu_1 + 43 \mu_1^2 + 42 \mu_2 - 6 \mu_1 \mu_2 \right) + \eta t \right. \\
& \quad \left. \left( -36 - 40 \mu_1 + 1388 \mu_1^2 - 221 \mu_2 + 451 \mu_1 \mu_2 \right) \right) \left. \right) + (-1 + \eta t) \text{el} \\
& \left( 6 - 80 \mu_1 - 62 \mu_1^2 + w^3 \left( -12 + 76 \mu_1^2 - \mu_1 (-232 + \mu_2) - 49 \mu_2 \right) + \right. \\
& \quad w^4 \left( -6 + 78 \mu_1^2 - 5 \mu_1 (-24 + \mu_2) - 5 \mu_2 \right) + 38 \mu_2 - \\
& \quad 58 \mu_1 \mu_2 - 4 w \left( -3 + 42 \mu_1 + 51 \mu_1^2 - 13 \mu_2 + 23 \mu_1 \mu_2 + \right. \\
& \quad \text{op} \left( -5 - 3 \mathfrak{e}1 + \mu_1^2 (-32 + 68 \mathfrak{e}1 - 63 \mathfrak{e}2) + \right. \\
& \quad \mu_1 (-13 + 35 \mathfrak{e}1 + \mu_2 (-73 + 15 \mathfrak{e}1 - 21 \mathfrak{e}2) - 30 \mathfrak{e}2) + \\
& \quad \mu_2 (47 + 15 \mathfrak{e}1 - 9 \mathfrak{e}2) + 3 \mathfrak{e}2) \left. \right) - w^2 \left( 6 \times \left( 24 \mu_1^2 + 5 \mu_2 + \right. \right. \\
& \quad \mu_1 (-4 + 5 \mu_2) \left. \right) + \text{op} \left( -10 - 6 \mathfrak{e}1 + \mu_1^2 (60 + 163 \mathfrak{e}1 - 151 \mathfrak{e}2) + \right. \\
& \quad \mu_1 (26 + 73 \mathfrak{e}1 + 2 \mu_2 (-11 + 15 \mathfrak{e}1 - 9 \mathfrak{e}2) - 61 \mathfrak{e}2) + \\
& \quad \mu_2 (26 + 30 \mathfrak{e}1 - 42 \mathfrak{e}2) + 6 \mathfrak{e}2) \left. \right) + \text{op} \left( \mu_1^2 (136 - 109 \mathfrak{e}1 + \right. \\
& \quad 101 \mathfrak{e}2) - 2 \times (3 - 3 \mathfrak{e}1 + 3 \mathfrak{e}2 + \mu_2 (61 + 15 \mathfrak{e}1 + 3 \mathfrak{e}2)) \left. \right) + \\
& \quad \mu_1 (58 - 67 \mathfrak{e}1 + 59 \mathfrak{e}2 + \mu_2 (214 - 30 \mathfrak{e}1 + 66 \mathfrak{e}2)) \left. \right) \left. \right) + \\
& \eta^5 \left( 4 \times (-1 + \eta t) \text{el} \mu_1 (1 + \mu_1) + 2 w^4 \left( (-1 + \eta t) \text{el} \left( -3 + 99 \mu_1^2 - \right. \right. \right. \\
& \quad \left. 5 \mu_2 - 5 \mu_1 \mu_2 \right) + 20 \text{op} \left( -2 + 11 \mu_1 + 13 \mu_1^2 - 10 \mu_2 + 32 \mu_1 \mu_2 \right) + \\
& \quad \eta t \text{op} \left( -19 + 351 \mu_1^2 + 100 \mu_2 - 4 \mu_1 (16 + 35 \mu_2) \right) \left. \right) + \\
& \text{op} \left( -50 + 100 \mu_1 + 246 \mu_1^2 + 4 \eta t (-1 + \mu_1) \times (4 + 4 \mu_1 - 15 \mu_2) - \right. \\
& \quad 26 \mu_2 + 238 \mu_1 \mu_2 + \text{el} \left( -24 - 50 \mu_2 + \mu_1^2 (166 + 5 \mathfrak{e}1 + 5 \mathfrak{e}2) + \right. \\
& \quad \mu_1 (-2 + 70 \mu_2 + 5 \mathfrak{e}1 + 5 \mathfrak{e}2) \left. \right) - \eta t \text{el} \left( -24 - 50 \mu_2 + \right. \\
& \quad \mu_1^2 (166 + 5 \mathfrak{e}1 + 5 \mathfrak{e}2) + \mu_1 (-2 + 70 \mu_2 + 5 \mathfrak{e}1 + 5 \mathfrak{e}2) \left. \right) \left. \right) - \\
& 2 w^3 \left( 2 \times (-1 + \eta t) \text{el} \left( \mu_1 + 13 \mu_1^2 - \mu_2 + 11 \mu_1 \mu_2 \right) + \right. \\
& \quad \text{op} \left( 34 - 192 \mu_2 + 3 \text{el} \mathfrak{e}1 - 15 \text{el} \mu_2 \mathfrak{e}1 + \mu_1^2 (-6 - 72 \text{el} (\mathfrak{e}1 - \mathfrak{e}2)) + \right. \\
& \quad \mu_1 (4 - 3 \mu_2 (-8 + 5 \text{el} (\mathfrak{e}1 - \mathfrak{e}2)) - 33 \text{el} (\mathfrak{e}1 - \mathfrak{e}2)) - 3 \text{el} \mathfrak{e}2 + \\
& \quad 15 \text{el} \mu_2 \mathfrak{e}2 + \eta t \left( -50 - 3 \text{el} \mathfrak{e}1 + \mu_2 (-137 + 15 \text{el} (\mathfrak{e}1 - \mathfrak{e}2)) + \right. \\
& \quad \mu_1 (24 + \mu_2 (247 + 15 \text{el} (\mathfrak{e}1 - \mathfrak{e}2)) + 33 \text{el} (\mathfrak{e}1 - \mathfrak{e}2)) + \\
& \quad \mu_1^2 (422 + 72 \text{el} (\mathfrak{e}1 - \mathfrak{e}2)) + 3 \text{el} \mathfrak{e}2) \left. \right) \left. \right) - \\
& w^2 \left( 3 \text{op} \left( -68 + 468 \mu_1^2 - 144 \mu_2 + 8 \mu_1 (32 + 79 \mu_2) + \eta t \right. \right. \\
& \quad \left. \left( -36 + 236 \mu_1^2 + \mu_1 (56 - 61 \mu_2) + 83 \mu_2 \right) \right) + \\
& \quad (-1 + \eta t) \text{el} \left( -12 + 128 \mu_1 + 260 \mu_1^2 - 57 \mu_2 + 87 \mu_1 \mu_2 + \right. \\
& \quad 2 \text{op} \left( -2 - 6 \mathfrak{e}1 + \mu_1^2 (-148 + 103 \mathfrak{e}1 - 107 \mathfrak{e}2) + \right. \\
& \quad \mu_1 (-78 + 61 \mathfrak{e}1 + 2 \mu_2 (-79 + 15 \mathfrak{e}1 - 33 \mathfrak{e}2) - 65 \mathfrak{e}2) + \\
& \quad \left. 6 \mathfrak{e}2 + \mu_2 (82 + 30 \mathfrak{e}1 + 6 \mathfrak{e}2) \right) \left. \right) \left. \right) + \\
& w \left( 4 \times (-1 + \eta t) \text{el} \mu_1 (-1 + 23 \mu_1) + \text{op} \left( 60 + 292 \mu_1^2 - 412 \mu_2 + \right. \right.
\end{aligned}$$

$$\begin{aligned}
& 4 \mu_1 (4 + 71 \mu_2) + 4 \eta t (-19 + 88 \mu_1^2 - 28 \mu_2 + \mu_1 (-27 + 44 \mu_2)) - \\
& \theta l \mu_1^2 (362 + 149 \mu_1 - 111 \mu_2) + 30 \theta l (2 + \mu_2 + 4 \mu_2 \mu_2) - \\
& \theta l \mu_1 (206 + 29 \mu_1 + 9 \mu_2 + 6 \mu_2 (31 + 20 \mu_2)) + \\
& \eta t \theta l (\mu_1^2 (362 + 149 \mu_1 - 111 \mu_2) - 30 \times (2 + \mu_2 + 4 \mu_2 \mu_2) + \\
& \quad \mu_1 (206 + 29 \mu_1 + 9 \mu_2 + 6 \mu_2 (31 + 20 \mu_2))) - \\
& \eta^6 (4 \theta p (2 - 51 \mu_1^2 + 6 \eta t (1 + \mu_1) + 30 \mu_2 - \mu_1 (13 + 30 \mu_2)) + \\
& \quad w^4 ((-1 + \eta t) \theta l (-2 + 58 \mu_1^2 + \mu_1 (8 - 5 \mu_2) - 5 \mu_2) + \\
& \quad 2 \theta p (-23 + 72 \mu_1 + 95 \mu_1^2 + 5 \mu_2 + 281 \mu_1 \mu_2 + \\
& \quad \eta t (10 + 2 \mu_1 + 76 \mu_1^2 + 73 \mu_2 - 83 \mu_1 \mu_2))) + \\
& w^3 (\theta p (-8 \times (-13 + 89 \mu_1^2 - 44 \mu_2 + 2 \mu_1 (23 + 68 \mu_2)) + \\
& \quad \eta t (68 - 396 \mu_1^2 - 123 \mu_2 + \mu_1 (8 + 69 \mu_2))) - \\
& \quad (-1 + \eta t) \theta l (-4 - 4 \theta p \mu_1 + \mu_2 (-19 + 20 \theta p (\mu_1 - \mu_2)) + \\
& \quad 4 \mu_1^2 (29 + 24 \theta p (\mu_1 - \mu_2)) + \\
& \quad \mu_1 (40 + \mu_2 (29 + 20 \theta p (\mu_1 - \mu_2)) + 44 \theta p (\mu_1 - \mu_2)) + 4 \theta p \mu_2)) + \\
& w (4 \times (-1 + \eta t) \theta l \mu_1 (1 + \mu_1) + \theta p (-2 \times (68 + (48 + 25 \theta l) \mu_2) + \\
& \quad \mu_1^2 (476 + \theta l (166 + 5 \mu_1 + 5 \mu_2)) + \\
& \quad \mu_1 (148 + 528 \mu_2 + \theta l (22 + 70 \mu_2 + 5 \mu_1 + 5 \mu_2)) - \\
& \quad \eta t (28 - 10 \times (12 + 5 \theta l) \mu_2 + \mu_1^2 (-16 + \theta l (166 + 5 \mu_1 + 5 \mu_2)) + \\
& \quad \mu_1 (12 + 120 \mu_2 + \theta l (22 + 70 \mu_2 + 5 \mu_1 + 5 \mu_2)))) + \\
& w^2 (4 \times (-1 + \eta t) \theta l \mu_1 (-1 + 11 \mu_1) + \theta p (2 \times (57 + 115 \mu_1^2 - \\
& \quad 227 \mu_2 + \mu_1 (52 + 37 \mu_2)) - 5 \theta l (\mu_1^2 (52 + 15 \mu_1 - 11 \mu_2) - 2 \times \\
& \quad (1 + 7 \mu_2 + 6 \mu_2 \mu_2) + \mu_1 (26 + 34 \mu_2 + 3 \mu_1 + \mu_2 + 12 \mu_2 \mu_2)) + \\
& \quad \eta t (4 \times (40 \mu_1^2 - 7 \times (3 + 5 \mu_2) + \mu_1 (-29 + 43 \mu_2)) + \\
& \quad 5 \theta l (\mu_1^2 (52 + 15 \mu_1 - 11 \mu_2) - 2 \times (1 + 7 \mu_2 + 6 \mu_2 \mu_2) + \\
& \quad \mu_1 (26 + 34 \mu_2 + 3 \mu_1 + \mu_2 + 12 \mu_2 \mu_2)))) + \\
& \eta^4 (-4 \times (-1 + \eta t) \theta l \mu_1 (-1 + 11 \mu_1) + w^4 (-((-1 + \eta t) \theta l \\
& \quad (-4 + 212 \mu_1^2 + 5 \mu_1 (-16 + \mu_2) + 5 \mu_2)) + \\
& \quad 2 \theta p (-5 \eta t (-7 - 28 \mu_1 + 123 \mu_1^2 + 7 \mu_2 - 17 \mu_1 \mu_2) - \\
& \quad 2 \times (-8 + 87 \mu_1 + 95 \mu_1^2 - 170 \mu_2 + 280 \mu_1 \mu_2))) + \\
& w^3 (\theta p (-8 \times (-19 + 166 \mu_1^2 - 58 \mu_2 + \mu_1 (111 + 266 \mu_2)) + \\
& \quad \eta t (52 - 388 \mu_1^2 - 455 \mu_2 + \mu_1 (96 + 745 \mu_2))) - \\
& \quad (-1 + \eta t) \theta l (-16 - 53 \mu_2 - 4 \theta p \mu_1 + 20 \theta p \mu_2 \mu_1 + 32 \mu_1^2 \\
& \quad (13 + 3 \theta p (\mu_1 - \mu_2)) + \mu_1 (112 + \mu_2 (43 + 20 \theta p (\mu_1 - \mu_2)) + \\
& \quad 44 \theta p (\mu_1 - \mu_2)) + 4 \theta p \mu_2 - 20 \theta p \mu_2 \mu_2)) + \\
& w (\theta p (\eta t (-88 + 540 \mu_1^2 + \mu_1 (212 - 127 \mu_2) + 161 \mu_2) + \\
& \quad 4 \times (-41 + 280 \mu_1^2 - 68 \mu_2 + \mu_1 (155 + 328 \mu_2))) + \\
& \quad (-1 + \eta t) \theta l (3 \times (-4 + 88 \mu_1^2 - 19 \mu_2 + \mu_1 (44 + 29 \mu_2)) + \\
& \quad \theta p (\mu_1^2 (-294 + 267 \mu_1 - 257 \mu_2) + \\
& \quad \mu_1 (-74 + 135 \mu_1 + \mu_2 (-362 + 60 \mu_1 - 84 \mu_2) - 125 \mu_2) + \\
& \quad 2 \times (-10 - 6 \mu_1 + \mu_2 (119 + 30 \mu_1 - 18 \mu_2) + 6 \mu_2))) + \\
& \theta p (-6 + 88 \mu_1 - 50 \mu_1^2 + 154 \mu_2 - 62 \mu_1 \mu_2 + \theta l (\mu_1^2 (268 + \\
& \quad 79 \mu_1 - 51 \mu_2) - 10 \times (5 + \mu_2 + 6 \mu_2 \mu_2) + \\
& \quad \mu_1 (98 + 86 \mu_2 + 19 \mu_1 + 9 \mu_2 + 60 \mu_2 \mu_2)) -
\end{aligned}$$

$$\begin{aligned}
& \eta t \left( 4 \times \left( -6 + 44 \mu_1^2 - 17 \mu_2 + 5 \mu_1 (-2 + 5 \mu_2) \right) + \right. \\
& \quad \left. \theta l \left( \mu_1^2 (268 + 79 \mu_1 - 51 \mu_2) - 10 \times (5 + \mu_2 + 6 \mu_2 \mu_2) + \right. \right. \\
& \quad \quad \left. \left. \mu_1 (98 + 86 \mu_2 + 19 \mu_1 + 9 \mu_2 + 60 \mu_2 \mu_2) \right) \right) + \\
& w^2 \left( (-1 + \eta t) \theta l \left( 172 \mu_1^2 + 15 \mu_2 + \mu_1 (-44 + 15 \mu_2) \right) + \right. \\
& \quad \left. \theta p \left( 72 + 500 \mu_1^2 - 832 \mu_2 + 4 \mu_1 (47 + 236 \mu_2) - 2 \theta l \left( -10 - 3 \mu_1 + \right. \right. \right. \\
& \quad \quad \left. \mu_1^2 (160 + 119 \mu_1 - 103 \mu_2) + \mu_2 (-22 + 15 \mu_1 - 51 \mu_2) + \right. \\
& \quad \quad \left. 3 \mu_2 + \mu_1 (78 + 44 \mu_1 - 28 \mu_2 + \mu_2 (74 + 15 \mu_1 + 21 \mu_2)) \right) \right) + \\
& \quad \eta t \left( -168 + 112 \mu_1 + 1888 \mu_1^2 - 331 \mu_2 + 629 \mu_1 \mu_2 + \right. \\
& \quad \quad 2 \theta l \left( -10 - 3 \mu_1 + \mu_1^2 (160 + 119 \mu_1 - 103 \mu_2) + \right. \\
& \quad \quad \quad \left. \mu_2 (-22 + 15 \mu_1 - 51 \mu_2) + 3 \mu_2 + \mu_1 (78 + 44 \mu_1 - \right. \\
& \quad \quad \quad \left. 28 \mu_2 + \mu_2 (74 + 15 \mu_1 + 21 \mu_2)) \right) \left. \right) \left. \right) \left. \right) \left. \right) \left. \right) \left. \right) / \\
& (96 (-1 + w (-1 + \eta))^3 (w (-1 + \eta) + x (-1 + \eta) - \eta)^2 (x + \eta - x \eta)^2 \\
& (1 + \\
& \quad x + \\
& \quad \eta - \\
& \quad x \\
& \quad \eta)^2 (-1 + \eta t) \theta l \theta p \mu_2) \\
\delta \chi \psi = & - \left( (c v (x (-1 + \eta) - \eta) (1 + x + \eta - x \eta))^2 \right. \\
& (40 u (-1 + w (-1 + \eta))^3 (x + \eta - x \eta)^2 (w + x + \eta - w \eta - x \eta)^3 (-1 + \eta t) \theta p - \\
& f (-1 + \eta) \times (-2 w^5 (-1 + \eta)^5 (\eta \theta p (7 \eta^3 - \eta t - \eta^2 (13 + 7 \eta t) + \\
& \quad \eta (6 + 8 \eta t + \theta l (-2 + \mu_1 + \mu_2) - \eta t \theta l (-2 + \mu_1 + \mu_2))) - 2 x \\
& (-1 + \eta) \times (7 \eta^3 \theta p + \eta t \theta p + 6 \eta (1 + \eta t) \theta p - \eta^2 (13 + 7 \eta t) \theta p - \\
& \quad \eta (-1 + \eta t) \theta l (-2 + \theta p (-2 + \mu_1 + \mu_2))) + x^2 (-1 + \eta)^2 \\
& ((-1 + \eta) \times (-6 + 7 \eta - 7 \eta t) \theta p - (-1 + \eta t) \theta l (-1 + \theta p (-2 + \mu_1 + \mu_2))) \left. \right) - \\
& 2 (x + \eta - x \eta)^3 (2 x^2 (-1 + \eta)^2 (-3 + 3 \eta + \theta l - \eta t \theta l) \theta p + \theta p \\
& (6 \eta^3 - \eta t - 2 \eta^2 (3 + (-1 + \eta t) \theta l) + \\
& \quad \eta (\eta t + \theta l (2 + \mu_1 + \mu_2) - \eta t \theta l (2 + \mu_1 + \mu_2))) + x (-1 + \eta) \times \\
& (-12 \times (-1 + \eta) \eta \theta p + (-1 + \eta t) \theta l (-1 + \theta p (2 + 4 \eta + \mu_1 + \mu_2))) \left. \right) + \\
& w (x (-1 + \eta) - \eta) (-1 + \eta) \times (2 x^4 (-1 + \eta)^4 \theta p (30 + 21 \eta^2 - 22 \theta l - \\
& \quad \eta (51 - 14 \theta l + 7 \eta t (1 + 2 \theta l)) + \theta l \mu_1 + \eta t (7 + 22 \theta l - \theta l \mu_1)) - 2 \\
& x^3 (-1 + \eta)^3 (2 \times (-1 + \eta) \times (-9 + 42 \eta^2 - 2 \eta (30 + 7 \eta t)) \theta p - \\
& (-1 + \eta t) \theta l (3 + \theta p (56 \eta^2 + 4 \eta (-22 + \mu_1) - 3 \times (4 + \mu_1 + \mu_2))) \left. \right) + \eta \\
& \theta p (42 \eta^5 + 6 \eta t - 2 \eta^4 (51 - 14 \theta l + 7 \eta t (1 + 2 \theta l)) + \\
& \quad \eta^3 (24 + \eta t (14 - 2 \theta l (-22 + \mu_1)) + 2 \theta l (-22 + \mu_1)) + \\
& \quad \eta (-1 + \eta t) \theta l (10 + 5 \mu_1 + 3 \mu_2) + \\
& \quad 6 \eta^2 (6 - \theta l (4 + \mu_1 + \mu_2) + \eta t (-1 + \theta l (4 + \mu_1 + \mu_2))) \left. \right) + x^2 \\
& (-1 + \eta)^2 (6 \times (-1 + \eta) \times (-18 \eta + 42 \eta^3 - \eta t - 2 \eta^2 (30 + 7 \eta t)) \theta p - \\
& (-1 + \eta t) \theta l (18 + 168 \eta^3 \theta p + 12 \eta^2 \theta p (-22 + \mu_1) - \theta p \\
& \quad (22 + 11 \mu_1 + 9 \mu_2) - 6 \eta (-2 + 3 \theta p (4 + \mu_1 + \mu_2))) \left. \right) - 2 x (-1 + \eta) \times \\
& (84 \eta^5 \theta p + 12 \eta t \theta p - 4 \eta^4 (51 - 14 \theta l + 7 \eta t (1 + 2 \theta l)) \theta p + \\
& \quad 2 \eta^3 \theta p (33 + \eta t (14 - 2 \theta l (-22 + \mu_1)) + 2 \theta l (-22 + \mu_1)) + \\
& \quad 3 \eta^2 (-2 \times (-9 + \eta t) \theta p + (-1 + \eta t) \theta l (-1 + 3 \theta p (4 + \mu_1 + \mu_2))) + \\
& \quad 2 \eta \theta p (-\theta l (8 + 4 \mu_1 + 3 \mu_2) + \eta t (-3 + \theta l (8 + 4 \mu_1 + 3 \mu_2))) \left. \right) -
\end{aligned}$$

$$\begin{aligned}
& w^3 (-1 + \eta)^3 (2 x^4 (-1 + \eta)^4 (3 \times (-1 + \eta) \times (-6 + 7 \eta - 7 \eta t) \text{ep} - \\
& \quad (-1 + \eta t) \text{el} (1 + \text{ep} (-8 + 2 \mathfrak{x}1 - \mathfrak{x}2))) + x^3 (-1 + \eta)^3 \\
& \quad (-2 \times (-1 + \eta) \times (-90 + 84 \eta^2 - 22 \eta t - 3 \eta (3 + 28 \eta t)) \text{ep} + (-1 + \eta t) \\
& \quad \text{el} (54 + 6 \eta + 4 \eta \text{ep} (5 + 4 \mathfrak{x}1 - 2 \mathfrak{x}2) - 9 \text{ep} (22 + 3 \mathfrak{x}1 + 3 \mathfrak{x}2))) + \eta \\
& \quad \text{ep} (42 \eta^5 - 6 \eta t - 6 \eta^4 (-8 + 7 \eta t) - 2 \eta^3 (135 + \eta t + \\
& \quad \eta t \text{el} (34 + 2 \mathfrak{x}1 - \mathfrak{x}2) + \text{el} (-34 - 2 \mathfrak{x}1 + \mathfrak{x}2))) + \\
& \quad \eta (12 + \eta t (24 + \text{el} (4 - 6 \mathfrak{x}2))) + \text{el} (-4 + 6 \mathfrak{x}2)) + \\
& \quad \eta^2 (168 - 9 \text{el} (18 + \mathfrak{x}1 + \mathfrak{x}2) + \eta t (26 + 9 \text{el} (18 + \mathfrak{x}1 + \mathfrak{x}2)))) - x \\
& \quad (-1 + \eta) \times (168 \eta^5 \text{ep} + 6 \eta^4 (11 - 28 \eta t) \text{ep} + 12 \eta t \text{ep} - \\
& \quad 2 \eta^3 (9 \times (43 - 2 \eta t) \text{ep} + (-1 + \eta t) \text{el} (1 + \text{ep} (94 + 8 \mathfrak{x}1 - 4 \mathfrak{x}2))) + \\
& \quad \eta (6 \times (4 + 13 \eta t) \text{ep} - 4 \times (-1 + \eta t) \text{el} (-6 + \text{ep} (-2 + 3 \mathfrak{x}2))) + 3 \eta^2 \text{ep} \\
& \quad (172 - 3 \text{el} (58 + 5 \mathfrak{x}1 + 5 \mathfrak{x}2) + \eta t (14 + 3 \text{el} (58 + 5 \mathfrak{x}1 + 5 \mathfrak{x}2)))) + x^2 \\
& \quad (-1 + \eta)^2 (6 \times (-1 + \eta) \times (42 \eta^3 + \eta^2 (27 - 42 \eta t) - 2 \times (1 + 6 \eta t) - 2 \eta (45 + \\
& \quad 11 \eta t)) \text{ep} - (-1 + \eta t) \text{el} (-6 + 6 \eta^2 (1 + \text{ep} (26 + 4 \mathfrak{x}1 - 2 \mathfrak{x}2)) + \\
& \quad \text{ep} (-4 + 6 \mathfrak{x}2) - 9 \eta (-6 + \text{ep} (62 + 7 \mathfrak{x}1 + 7 \mathfrak{x}2)))) + \\
& w^2 (-1 + \eta)^2 (-2 x^5 (-1 + \eta)^5 \text{ep} (6 + 7 \eta^2 - \eta (13 + 7 \eta t) - 2 \text{el} + \\
& \quad \text{el} \mathfrak{x}1 + \eta t (7 + 2 \text{el} - \text{el} \mathfrak{x}1)) + 2 x^4 (-1 + \eta)^4 \\
& \quad ((-1 + \eta) \times (-90 + 33 \eta + 35 \eta^2 - 21 \eta t - 35 \eta \eta t) \text{ep} - \\
& \quad (-1 + \eta t) \text{el} (3 + \eta \text{ep} (32 + 5 \mathfrak{x}1) - 3 \text{ep} (24 + \mathfrak{x}2))) - x^3 (-1 + \eta)^3 \\
& \quad (2 \times (-1 + \eta) \times (70 \eta^3 + \eta^2 (192 - 70 \eta t) - 3 \times (6 + \eta t) - 12 \eta (30 + 7 \eta t)) \\
& \quad \text{ep} - (-1 + \eta t) \text{el} (54 + 4 \eta^2 \text{ep} (74 + 5 \mathfrak{x}1) - \\
& \quad 3 \text{ep} (26 + 11 \mathfrak{x}1 + 9 \mathfrak{x}2) - 6 \eta (-3 + 4 \text{ep} (24 + \mathfrak{x}2)))) + \eta \\
& \quad \text{ep} (14 \eta^6 - 2 \eta t - 2 \eta^5 (-50 + 7 \eta t) - 2 \eta^4 (147 - \text{el} (40 + \mathfrak{x}1) + \\
& \quad \eta t (14 + \text{el} (40 + \mathfrak{x}1))) + \eta (2 \text{el} \mathfrak{x}2 + \eta t (20 - 2 \text{el} \mathfrak{x}2)) + \\
& \quad 6 \eta^3 (24 - \text{el} (24 + \mathfrak{x}2) + \eta t (6 + \text{el} (24 + \mathfrak{x}2))) + 3 \eta^2 \\
& \quad (12 - \text{el} (14 + 5 \mathfrak{x}1 + 3 \mathfrak{x}2) + \eta t (-4 + \text{el} (14 + 5 \mathfrak{x}1 + 3 \mathfrak{x}2)))) - x \\
& \quad (-1 + \eta) \times (70 \eta^6 \text{ep} + \eta^5 (374 - 70 \eta t) \text{ep} + 4 \eta t \text{ep} - \\
& \quad 2 \eta^4 \text{ep} (582 - \text{el} (158 + 5 \mathfrak{x}1) + \eta t (49 + \text{el} (158 + 5 \mathfrak{x}1))) + \\
& \quad \eta (86 \eta t \text{ep} - 4 \times (-1 + \eta t) \text{el} (-2 + \text{ep} \mathfrak{x}2)) + \\
& \quad 6 \eta^3 ((102 + 25 \eta t) \text{ep} + (-1 + \eta t) \text{el} (-1 + 4 \text{ep} (24 + \mathfrak{x}2))) + \\
& \quad 9 \eta^2 \text{ep} (12 - \text{el} (18 + 7 \mathfrak{x}1 + 5 \mathfrak{x}2) + \eta t (-8 + \text{el} (18 + 7 \mathfrak{x}1 + 5 \mathfrak{x}2)))) + \\
& x^2 (-1 + \eta)^2 (2 \times (-1 + \eta) \times (70 \eta^4 + \eta^3 (318 - 70 \eta t) - 36 \eta t - \\
& \quad 9 \eta (6 + \eta t) - 18 \eta^2 (30 + 7 \eta t)) \text{ep} - (-1 + \eta t) \text{el} \\
& \quad (-2 + 4 \eta^3 \text{ep} (116 + 5 \mathfrak{x}1) + 2 \text{ep} \mathfrak{x}2 - 18 \eta^2 (-1 + 2 \text{ep} (24 + \mathfrak{x}2)) - \\
& \quad 9 \eta (-6 + \text{ep} (22 + 9 \mathfrak{x}1 + 7 \mathfrak{x}2)))) - w^4 (-1 + \eta)^4 \\
& (x^3 (-1 + \eta)^3 (6 \times (-1 + \eta) \times (-6 + 7 \eta - 7 \eta t) \text{ep} + (-1 + \eta t) \text{el} \\
& \quad (-18 + \text{ep} (34 + 5 \mathfrak{x}1 + 9 \mathfrak{x}2))) + \eta \text{ep} (-42 \eta^4 + 6 \eta t + 6 \eta^3 (6 + 7 \eta t) + \\
& \quad \eta^2 (66 + \eta t (-22 + \text{el} (6 + \mathfrak{x}1 - 3 \mathfrak{x}2)) - \text{el} (6 + \mathfrak{x}1 - 3 \mathfrak{x}2)) + \\
& \quad 2 \eta (-30 - \text{el} (-22 + \mathfrak{x}1 + 3 \mathfrak{x}2) + \eta t (-13 + \text{el} (-22 + \mathfrak{x}1 + 3 \mathfrak{x}2)))) + x \\
& \quad (-1 + \eta) \times (126 \eta^4 \text{ep} + 12 \eta t \text{ep} - 6 \eta^3 (25 + 21 \eta t) \text{ep} + \\
& \quad 2 \eta ((60 + 23 \eta t) \text{ep} - 2 \times (-1 + \eta t) \text{el} (-6 + \text{ep} (-22 + \mathfrak{x}1 + 3 \mathfrak{x}2))) + \\
& \quad \eta^2 \text{ep} (-96 - \text{el} (22 + 3 \mathfrak{x}1 + 15 \mathfrak{x}2) + \eta t (68 + \text{el} (22 + 3 \mathfrak{x}1 + 15 \mathfrak{x}2)))) - \\
& x^2 (-1 + \eta)^2 (2 \times (-1 + \eta) \times (-30 + 63 \eta^2 - 19 \eta t - 3 \eta (11 + 21 \eta t)) \\
& \quad \text{ep} + (-1 + \eta t) \text{el} (6 - 2 \text{ep} (-22 + \mathfrak{x}1 + 3 \mathfrak{x}2)) +
\end{aligned}$$

$$\begin{aligned}
& \eta (-18 + \operatorname{erf} (62 + 9 \sqrt{1} + 21 \sqrt{2})) \Big) \Big) \Big) + \\
& \operatorname{erf} (-1 + \eta)^2 \Big( w^5 (-1 + \eta)^6 \Big( 2 x^5 (-1 + \eta)^5 \operatorname{erf} (\eta - \eta t + 4 \mu_1) - \\
& 2 x^4 (-1 + \eta)^3 \Big( (-1 + \eta t) \operatorname{erf} (-4 + 4 \mu_1 + \mu_2) + (-1 + \eta) \operatorname{erf} \\
& (4 + 5 \eta^2 + 12 \mu_1 + \eta (2 - 5 \eta t + 20 \mu_1 - 7 \mu_2) + \eta t (-2 + 7 \mu_2)) \Big) - \\
& 2 \eta \operatorname{erf} (\eta^5 + \eta t \mu_2 + 2 \eta \eta t (-2 - 2 \mu_1 + \mu_2) - \eta^4 (-2 + \eta t - 4 \mu_1 + 7 \mu_2) + \\
& \eta^3 (5 + 12 \mu_1 - 13 \mu_2 + \eta t (-2 + 7 \mu_2)) + \eta^2 \\
& (4 + 8 \mu_1 + 8 \mu_2 + \eta t (-5 + 10 \mu_1 + 8 \mu_2)) \Big) + \\
& x \Big( 10 \eta^6 \operatorname{erf} + \eta^3 (-2 \operatorname{erf} (7 + 24 \mu_1 - 63 \mu_2) + \eta t \operatorname{erf} (-11 + 53 \mu_1 - 5 \mu_2) + \\
& (-1 + \eta t) \operatorname{erf} (-11 + 15 \mu_1 - \mu_2)) + 2 \eta^5 \\
& \operatorname{erf} (3 - 5 \eta t + 20 \mu_1 - 28 \mu_2) - \eta t \operatorname{erf} (3 + 3 \mu_1 + 5 \mu_2) + \eta \\
& (\eta t \operatorname{erf} (13 + 11 \mu_1 - 9 \mu_2) - (-1 + \eta t) \operatorname{erf} (3 + 3 \mu_1 + \mu_2)) + 2 \eta^4 \operatorname{erf} (11 + \\
& 28 \mu_1 - 11 \mu_2 + \eta t (-3 + 28 \mu_2)) - \eta^2 (2 \times (-1 + \eta t) \operatorname{erf} (7 + 8 \mu_1 + \mu_2) + \\
& 24 \operatorname{erf} (1 + 2 \mu_1 + 2 \mu_2) + \eta t \operatorname{erf} (-17 + 61 \mu_1 + 37 \mu_2)) \Big) - \\
& 2 x^2 (-1 + \eta) \times \Big( 10 \eta^5 \operatorname{erf} + 2 \eta^4 \operatorname{erf} (1 - 5 \eta t + 20 \mu_1 - 21 \mu_2) - \operatorname{erf} \\
& \mu_2 + \eta t (\operatorname{erf} + \operatorname{erf} \mu_2 - 5 \operatorname{erf} \mu_2) - \eta ((-1 + \eta t) \operatorname{erf} (11 + 12 \mu_1 - \mu_2) + \\
& 12 \operatorname{erf} (1 + 2 \mu_1 + 2 \mu_2) + \eta t \operatorname{erf} (-11 + 23 \mu_1 + 22 \mu_2)) + \eta^3 \\
& \operatorname{erf} (32 \mu_1 + 3 \times (5 + \mu_2) + \eta t (-2 + 42 \mu_2)) + \eta^2 ((-1 + \eta t) \operatorname{erf} \\
& (-15 + 19 \mu_1) + \operatorname{erf} (-15 - 48 \mu_1 + 23 \eta t \mu_1 + 63 \mu_2 - 15 \eta t \mu_2)) \Big) + \\
& x^3 (-1 + \eta)^2 \Big( (-1 + \eta t) \operatorname{erf} (-8 - 8 \mu_1 + 31 \eta \mu_1 + 3 \eta (-9 + \mu_2) + 4 \mu_2) + \\
& (-1 + \eta) \operatorname{erf} (20 \eta^3 + 8 \times (1 + 2 \mu_1 + 2 \mu_2) - 4 \eta^2 (-4 + 5 \eta t - 20 \mu_1 + 14 \mu_2) + \\
& \eta t (-7 + 13 \mu_1 + 19 \mu_2) + 2 \eta (17 + 48 \mu_1 - 13 \mu_2 + 4 \eta t (-2 + 7 \mu_2)) \Big) \Big) + \\
& w^4 (-1 + \eta)^4 \Big( 6 x^6 (-1 + \eta)^7 \operatorname{erf} (\eta - \eta t + 4 \mu_1) + \eta \operatorname{erf} (6 \eta^7 + \eta^6 \\
& (16 - 6 \eta t + 24 \mu_1 - 42 \mu_2) + 12 \eta \eta t (1 + \mu_1 - 2 \mu_2) - 6 \\
& \eta t \mu_2 + 2 \eta^5 (29 + 39 \mu_1 - 39 \mu_2 + \eta t (-8 + 21 \mu_2)) + \eta^4 \\
& (50 + 42 \mu_1 + 130 \mu_2 + 3 \operatorname{erf} (\mu_2 (6 + 3 \sqrt{1} - \sqrt{2}) + 3 \times (6 + \sqrt{1} + \sqrt{2}) + \\
& \mu_1 (18 + \sqrt{1} + 5 \sqrt{2})) - \eta t (4 - 110 \mu_1 - 46 \mu_2 + \\
& 3 \operatorname{erf} (\mu_2 (6 + 3 \sqrt{1} - \sqrt{2}) + 3 \times (6 + \sqrt{1} + \sqrt{2}) + \mu_1 (18 + \sqrt{1} + 5 \sqrt{2}))) \Big) - \\
& 2 \eta^3 (32 + 39 \mu_1 - 25 \mu_2 - 3 \operatorname{erf} (\mu_2 (6 + 3 \sqrt{1} - \sqrt{2}) + 3 \times (6 + \sqrt{1} + \sqrt{2}) + \\
& \mu_1 (18 + \sqrt{1} + 5 \sqrt{2})) + \eta t (-2 + 20 \mu_1 + 9 \mu_2 + \\
& 3 \operatorname{erf} (\mu_2 (6 + 3 \sqrt{1} - \sqrt{2}) + 3 \times (6 + \sqrt{1} + \sqrt{2}) + \mu_1 (18 + \sqrt{1} + 5 \sqrt{2}))) \Big) - \\
& \eta^2 (66 + 66 \mu_1 + 60 \mu_2 - 3 \operatorname{erf} (\mu_2 (6 + 3 \sqrt{1} - \sqrt{2}) + 3 \times (6 + \sqrt{1} + \sqrt{2}) + \\
& \mu_1 (18 + \sqrt{1} + 5 \sqrt{2})) + \eta t (-10 + 82 \mu_1 + 40 \mu_2 + \\
& 3 \operatorname{erf} (\mu_2 (6 + 3 \sqrt{1} - \sqrt{2}) + 3 \times (6 + \sqrt{1} + \sqrt{2}) + \mu_1 (18 + \sqrt{1} + 5 \sqrt{2}))) \Big) \Big) - \\
& x^5 (-1 + \eta)^5 \Big( 6 \times (-1 + \eta t) \operatorname{erf} (10 \mu_1 + 3 \mu_2) + \operatorname{erf} (36 \eta^3 - 6 \times \\
& (9 + 17 \mu_1) - 2 \eta^2 (7 + 18 \eta t - 72 \mu_1 + 21 \mu_2) + \\
& 2 \eta (16 - 21 \mu_1 + 21 \mu_2 + 7 \eta t (1 + 3 \mu_2)) + 3 \operatorname{erf} (\mu_2 (6 + 3 \sqrt{1} - \sqrt{2}) + \\
& 3 \times (6 + \sqrt{1} + \sqrt{2}) + \mu_1 (18 + \sqrt{1} + 5 \sqrt{2})) - \eta t (-22 + 42 \mu_2 + \\
& 3 \operatorname{erf} (\mu_2 (6 + 3 \sqrt{1} - \sqrt{2}) + 3 \times (6 + \sqrt{1} + \sqrt{2}) + \mu_1 (18 + \sqrt{1} + 5 \sqrt{2}))) \Big) \Big) + \\
& x^2 (-1 + \eta)^2 \Big( 90 \eta^6 \operatorname{erf} - 10 \eta^5 \operatorname{erf} (-13 + 9 \eta t - 36 \mu_1 + 42 \mu_2) - 6 \\
& (\operatorname{erf} \mu_2 - \eta t \operatorname{erf} \mu_2 + \eta t \operatorname{erf} (2 + 3 \mu_1 + 9 \mu_2)) + 2 \eta^4 \operatorname{erf} \\
& (238 + 330 \mu_1 - 150 \mu_2 + 5 \eta t (-13 + 42 \mu_2)) - 3 \eta \\
& (2 \operatorname{erf} (33 + 33 \mu_1 + 30 \mu_2 + \eta t (-6 + 31 \mu_1 + 33 \mu_2)) + \\
& (-1 + \eta t) \operatorname{erf} (2 \times (8 + 9 \mu_1 - 6 \mu_2) + \\
& 3 \operatorname{erf} (\mu_2 (6 + 3 \sqrt{1} - \sqrt{2}) + 3 \times (6 + \sqrt{1} + \sqrt{2}) + \mu_1 (18 + \sqrt{1} + 5 \sqrt{2}))) \Big) - \\
& 2 \eta^3 (-\operatorname{erf} (27 - 78 \mu_1 + 501 \mu_2 + \eta t (41 + 288 \mu_1 + 63 \mu_2)) +
\end{aligned}$$

$$\begin{aligned}
& 3 \times (-1 + \eta t) \, \text{el} \, (3 - 54 \mu_1 - 9 \mu_2 + 5 \, \text{ep} \\
& \quad (\mu_2 (6 + 3 \, \text{el} - \text{el}_2) + 3 \times (6 + \, \text{el}_1 + \text{el}_2) + \mu_1 (18 + \, \text{el}_1 + 5 \, \text{el}_2))) - 6 \\
& \eta^2 (\text{ep} (92 + 111 \mu_1 + 17 \mu_2 + \eta t (-19 + 62 \mu_1 + 49 \mu_2)) + \\
& \quad (-1 + \eta t) \, \text{el} \, (13 - 13 \mu_1 - 14 \mu_2 + 6 \, \text{ep} \\
& \quad (\mu_2 (6 + 3 \, \text{el} - \text{el}_2) + 3 \times (6 + \, \text{el}_1 + \text{el}_2) + \mu_1 (18 + \, \text{el}_1 + 5 \, \text{el}_2)))) + \\
& x^3 (-1 + \eta)^3 \left( - \left( (-1 + \eta) \, \text{ep} (66 + 120 \eta^4 + 66 \mu_1 + 60 \mu_2 - 20 \eta^3 \right. \right. \\
& \quad (-11 + 6 \eta t - 24 \mu_1 + 21 \mu_2) + \eta t (-1 + 67 \mu_1 + 91 \mu_2) + \\
& \quad 4 \eta^2 (161 + 255 \mu_1 - 120 \mu_2 + 5 \eta t (-11 + 21 \mu_2)) + \\
& \quad \left. \left. \eta (490 + 576 \mu_1 + 262 \mu_2 + \eta t (-86 + 356 \mu_1 + 370 \mu_2)) \right) \right) + \\
& 3 \times (-1 + \eta t) \, \text{el} \, (4 + 4 \mu_1 - 10 \mu_2 + \text{ep} (\mu_2 (6 + 3 \, \text{el} - \text{el}_2) + \\
& \quad 3 \times (6 + \, \text{el}_1 + \text{el}_2) + \mu_1 (18 + \, \text{el}_1 + 5 \, \text{el}_2)) + 2 \eta^2 (3 - 74 \mu_1 - 15 \mu_2 + \\
& \quad 5 \, \text{ep} (\mu_2 (6 + 3 \, \text{el} - \text{el}_2) + 3 \times (6 + \, \text{el}_1 + \text{el}_2) + \mu_1 (18 + \, \text{el}_1 + 5 \, \text{el}_2))) + \\
& \quad \eta (19 - 25 \mu_1 - 35 \mu_2 + 8 \, \text{ep} (\mu_2 (6 + 3 \, \text{el} - \text{el}_2) + \\
& \quad 3 \times (6 + \, \text{el}_1 + \text{el}_2) + \mu_1 (18 + \, \text{el}_1 + 5 \, \text{el}_2)))) + \\
& x^4 (-1 + \eta)^4 \left( 2 \times (-1 + \eta) \, \text{ep} (60 + 45 \eta^3 + 72 \mu_1 + 42 \mu_2 - 5 \eta^2 \right. \\
& \quad (-11 + 9 \eta t - 36 \mu_1 + 21 \mu_2) + \eta t (-10 + 41 \mu_1 + 47 \mu_2) + \\
& \quad \left. \eta (148 + 255 \mu_1 - 60 \mu_2 + 5 \eta t (-11 + 21 \mu_2)) \right) - (-1 + \eta t) \, \text{el} \\
& \quad (6 \times (2 - 4 \mu_1 - 7 \mu_2 + \text{ep} (\mu_2 (6 + 3 \, \text{el} - \text{el}_2) + 3 \times (6 + \, \text{el}_1 + \text{el}_2) + \\
& \quad \mu_1 (18 + \, \text{el}_1 + 5 \, \text{el}_2))) + \eta (6 - 268 \mu_1 - 66 \mu_2 + 15 \, \text{ep} \\
& \quad (\mu_2 (6 + 3 \, \text{el} - \text{el}_2) + 3 \times (6 + \, \text{el}_1 + \text{el}_2) + \mu_1 (18 + \, \text{el}_1 + 5 \, \text{el}_2)))) - \\
& x (-1 + \eta) \times (36 \eta^7 \, \text{ep} + 2 \eta^6 \, \text{ep} (37 - 18 \eta t + 72 \mu_1 - 105 \mu_2) - 3 \\
& \quad \eta t \, \text{ep} (3 + 3 \mu_1 + 5 \mu_2) + \eta \\
& \quad (3 \eta t \, \text{ep} (3 + \mu_1 - 23 \mu_2) - 3 \times (-1 + \eta t) \, \text{el} (3 + 3 \mu_1 + \mu_2)) + 2 \\
& \quad \eta^5 \, \text{ep} (3 \times (44 + 61 \mu_1 - 45 \mu_2) + \eta t (-37 + 105 \mu_2)) - 3 \\
& \quad \eta^2 (\text{ep} (66 + 66 \mu_1 + 60 \mu_2 + \eta t (-15 + 67 \mu_1 + 49 \mu_2)) + \\
& \quad (-1 + \eta t) \, \text{el} (2 \times (6 + 7 \mu_1 - \mu_2) + 3 \, \text{ep} \\
& \quad (\mu_2 (6 + 3 \, \text{el} - \text{el}_2) + 3 \times (6 + \, \text{el}_1 + \text{el}_2) + \mu_1 (18 + \, \text{el}_1 + 5 \, \text{el}_2)))) - \\
& \eta^3 (\text{ep} (6 \times (52 + 63 \mu_1 - 11 \mu_2) + \eta t (-53 + 205 \mu_1 + 127 \mu_2)) + \\
& \quad 3 \times (-1 + \eta t) \, \text{el} (11 - 9 \mu_1 - 7 \mu_2 + 8 \, \text{ep} \\
& \quad (\mu_2 (6 + 3 \, \text{el} - \text{el}_2) + 3 \times (6 + \, \text{el}_1 + \text{el}_2) + \mu_1 (18 + \, \text{el}_1 + 5 \, \text{el}_2)))) + \\
& \eta^4 (2 \, \text{ep} (68 + 33 \mu_1 + 297 \mu_2 + \eta t (6 + 206 \mu_1 + 74 \mu_2)) - \\
& \quad (-1 + \eta t) \, \text{el} (6 - 88 \mu_1 - 12 \mu_2 + 15 \, \text{ep} \\
& \quad (\mu_2 (6 + 3 \, \text{el} - \text{el}_2) + 3 \times (6 + \, \text{el}_1 + \text{el}_2) + \mu_1 (18 + \, \text{el}_1 + 5 \, \text{el}_2)))) + \\
& w^3 (-1 + \eta)^3 \left( 6 x^7 (-1 + \eta)^8 \, \text{ep} (\eta - \eta t + 4 \mu_1) - x^6 (-1 + \eta)^6 \right. \\
& \quad (6 \times (-1 + \eta) \, \text{ep} (19 + 7 \eta^2 + 27 \mu_1 + 7 \eta t (-1 + \mu_2) - 7 \eta (-1 + \eta t - 4 \mu_1 + \mu_2)) + \\
& \quad (-1 + \eta t) \, \text{el} (78 \mu_1 - 2 \times (3 + \mu_2) + \\
& \quad \text{ep} (-108 - 12 \mu_2 - \, \text{el}_1 + \mu_1 (-96 + 9 \, \text{el}_1 - 17 \, \text{el}_2) - 5 \, \text{el}_2 + 22 \mu_2 \, \text{el}_2))) + \\
& \eta \, \text{ep} (-6 \eta^8 + 6 \eta t \mu_2 + 12 \eta \eta t (1 + \mu_1 + 5 \mu_2) + 6 \eta^7 (-6 + \eta t - 4 \mu_1 + 7 \mu_2) - \\
& \quad 2 \eta^6 (77 + 69 \mu_1 - 81 \mu_2 + 3 \eta t (-6 + 7 \mu_2)) - \eta^5 (2 \times (76 + 88 \mu_1 + 55 \mu_2) + \\
& \quad \text{el} (122 + 4 \, \text{el}_1 + \mu_2 (14 + 3 \, \text{el}_1 - 19 \, \text{el}_2) - 2 \mu_1 (-55 + \, \text{el}_1 - 12 \, \text{el}_2) + 8 \, \text{el}_2) + \\
& \quad \eta t (-32 + 166 \mu_1 + 88 \mu_2 - \text{el} (122 + 4 \, \text{el}_1 + \mu_2 (14 + 3 \, \text{el}_1 - 19 \, \text{el}_2) - \\
& \quad 2 \mu_1 (-55 + \, \text{el}_1 - 12 \, \text{el}_2) + 8 \, \text{el}_2))) + \eta^3 (4 \times (47 + 50 \mu_1 + 31 \mu_2) - \\
& \quad \text{el} (230 + 56 \, \text{el}_1 + \mu_2 (122 + 57 \, \text{el}_1 - 17 \, \text{el}_2) + 52 \, \text{el}_2 + 10 \mu_1 \\
& \quad (29 + \, \text{el}_1 + 8 \, \text{el}_2))) + \eta t (-50 + 210 \mu_1 + 28 \mu_2 + \text{el} (230 + 56 \, \text{el}_1 + \\
& \quad \mu_2 (122 + 57 \, \text{el}_1 - 17 \, \text{el}_2) + 52 \, \text{el}_2 + 10 \mu_1 (29 + \, \text{el}_1 + 8 \, \text{el}_2)))) + \eta^2
\end{aligned}$$

$$\begin{aligned}
& (42 + 70 \mu_1 + 60 \mu_2 - \theta l (54 + 26 \mathfrak{z}_1 + 22 \mathfrak{z}_2 + \mu_2 (54 + 27 \mathfrak{z}_1 + \mathfrak{z}_2) + \\
& \quad \mu_1 (90 + 6 \mathfrak{z}_1 + 28 \mathfrak{z}_2)) + \eta t (-12 + 38 \mu_1 + 66 \mu_2 + \theta l (54 + 26 \mathfrak{z}_1 + \\
& \quad 22 \mathfrak{z}_2 + \mu_2 (54 + 27 \mathfrak{z}_1 + \mathfrak{z}_2) + \mu_1 (90 + 6 \mathfrak{z}_1 + 28 \mathfrak{z}_2))) + \eta^4 \\
& (118 + 68 \mu_1 - 278 \mu_2 - \theta l (298 + 34 \mathfrak{z}_1 + \mu_2 (82 + 33 \mathfrak{z}_1 - 37 \mathfrak{z}_2) + \\
& \quad 38 \mathfrak{z}_2 + 2 \mu_1 (155 + \mathfrak{z}_1 + 38 \mathfrak{z}_2)) + \eta t \\
& \quad (-2 \times (12 + 47 \mu_1 + 15 \mu_2) + \theta l (298 + 34 \mathfrak{z}_1 + \mu_2 (82 + 33 \mathfrak{z}_1 - 37 \mathfrak{z}_2) + \\
& \quad 38 \mathfrak{z}_2 + 2 \mu_1 (155 + \mathfrak{z}_1 + 38 \mathfrak{z}_2)))) + x^5 (-1 + \eta)^5 \\
& ((-1 + \eta) \theta p (126 \eta^3 + \eta (766 + 972 \mu_1 + 252 \eta t (-1 + \mu_2) - 204 \mu_2) - \\
& \quad 126 \eta^2 (-2 + \eta t - 4 \mu_1 + 2 \mu_2) + 26 \times (11 + 13 \mu_1 + 6 \mu_2) + \\
& \quad \eta t (-77 + 107 \mu_1 + 127 \mu_2)) + (-1 + \eta t) \theta l \\
& (-16 + 88 \mu_1 + 50 \mu_2 - \theta p (270 + 28 \mathfrak{z}_1 + \mu_2 (78 + 27 \mathfrak{z}_1 - 43 \mathfrak{z}_2) + 32 \mathfrak{z}_2 + \\
& \quad \mu_1 (282 - 12 \mathfrak{z}_1 + 62 \mathfrak{z}_2)) + \eta (-27 + 449 \mu_1 - 7 \mu_2 - \theta p (662 + 9 \mathfrak{z}_1 + \\
& \quad \mu_2 (74 + 3 \mathfrak{z}_1 - 129 \mathfrak{z}_2) + 33 \mathfrak{z}_2 + \mu_1 (590 - 47 \mathfrak{z}_1 + 109 \mathfrak{z}_2)))) - \\
& x^4 (-1 + \eta)^4 (2 \times (-1 + \eta) \theta p (107 + 105 \eta^4 + 135 \mu_1 + 5 \eta^2 (212 + \\
& \quad 243 \mu_1 + 63 \eta t (-1 + \mu_2) - 102 \mu_2) + 124 \mu_2 - \\
& \quad 105 \eta^3 (-3 + \eta t - 4 \mu_1 + 3 \mu_2) + \eta t (-19 + 87 \mu_1 + 86 \mu_2) + \\
& \quad \eta (746 + 845 \mu_1 + 265 \mu_2 + \eta t (-191 + 297 \mu_1 + 319 \mu_2))) + \\
& (-1 + \eta t) \theta l (2 - 10 \mu_1 + 112 \mu_2 - \theta p (216 + 53 \mathfrak{z}_1 + 2 \mu_2 \\
& \quad (60 + 27 \mathfrak{z}_1 - 10 \mathfrak{z}_2) + 49 \mathfrak{z}_2 + \mu_1 (276 + 3 \mathfrak{z}_1 + 73 \mathfrak{z}_2)) + \\
& \quad \eta^2 (8 \times (-6 + 127 \mu_1 - \mu_2) - 5 \theta p (338 + 6 \mathfrak{z}_1 + \mu_2 (38 + 3 \mathfrak{z}_1 - \\
& \quad 63 \mathfrak{z}_2) + 18 \mathfrak{z}_2 + \mu_1 (302 - 20 \mathfrak{z}_1 + 58 \mathfrak{z}_2))) + \\
& \quad \eta (-76 + 438 \mu_1 + 188 \mu_2 - \theta p (\mu_2 (394 + 141 \mathfrak{z}_1 - 209 \mathfrak{z}_2) + \\
& \quad 2 \times (689 + 73 \mathfrak{z}_1 + 83 \mathfrak{z}_2) + \mu_1 (1438 - 46 \mathfrak{z}_1 + 324 \mathfrak{z}_2)))) + \\
& x^3 (-1 + \eta)^3 (2 \times (-1 + \eta) \theta p (21 + 105 \eta^5 + 35 \mu_1 + 10 \eta^3 (155 + \\
& \quad 162 \mu_1 + 42 \eta t (-1 + \mu_2) - 102 \mu_2) + 30 \mu_2 - \\
& \quad 105 \eta^4 (-4 + \eta t - 4 \mu_1 + 4 \mu_2) + \eta t (21 + 40 \mu_1 + 87 \mu_2) + \\
& \quad \eta (436 + 540 \mu_1 + 464 \mu_2 + \eta t (-82 + 391 \mu_1 + 338 \mu_2)) + \\
& \quad \eta^2 (2 \times (777 + 845 \mu_1 + 140 \mu_2) + \eta t (-379 + 653 \mu_1 + 641 \mu_2))) + \\
& (-1 + \eta t) \theta l (6 \times (2 + 2 \mu_1 + 11 \mu_2) - \theta p (54 + 26 \mathfrak{z}_1 + 22 \mathfrak{z}_2 + \\
& \quad \mu_2 (54 + 27 \mathfrak{z}_1 + \mathfrak{z}_2) + \mu_1 (90 + 6 \mathfrak{z}_1 + 28 \mathfrak{z}_2)) + \\
& \quad 2 \eta^3 (-21 + 567 \mu_1 - \mu_2 - 5 \theta p (230 + 5 \mathfrak{z}_1 + \mu_2 (26 + 3 \mathfrak{z}_1 - 41 \mathfrak{z}_2) + \\
& \quad 13 \mathfrak{z}_2 + \mu_1 (206 - 11 \mathfrak{z}_1 + 41 \mathfrak{z}_2))) - \\
& \quad \eta (6 \times (6 + 10 \mu_1 - 49 \mu_2) + \theta p (878 + 215 \mathfrak{z}_1 + \mu_2 (482 + \\
& \quad 219 \mathfrak{z}_1 - 77 \mathfrak{z}_2) + 199 \mathfrak{z}_2 + \mu_1 (1118 + 19 \mathfrak{z}_1 + 299 \mathfrak{z}_2))) + \\
& \quad 2 \eta^2 (-66 + 393 \mu_1 + 132 \mu_2 - \theta p (\mu_2 (398 + 147 \mathfrak{z}_1 - 203 \mathfrak{z}_2) + \\
& \quad 2 \times (703 + 76 \mathfrak{z}_1 + 86 \mathfrak{z}_2) + \mu_1 (1466 - 32 \mathfrak{z}_1 + 338 \mathfrak{z}_2)))) - \\
& x^2 (-1 + \eta)^2 (126 \eta^7 \theta p - 126 \eta^6 \theta p (-4 + \eta t - 4 \mu_1 + 5 \mu_2) + 2 \eta^5 \\
& \quad \theta p (950 + 963 \mu_1 - 705 \mu_2 + 63 \eta t (-4 + 5 \mu_2)) - 6 \\
& \quad (\theta l \mu_2 - \eta t \theta l \mu_2 + \eta t \theta p (8 + 9 \mu_1 + 17 \mu_2)) - 3 \eta \\
& \quad (2 \theta p (21 + 35 \mu_1 + 30 \mu_2 + \eta t (6 + 26 \mu_1 + 63 \mu_2)) + \\
& \quad (-1 + \eta t) \theta l (4 + 6 \mu_1 - 32 \mu_2 + \theta p (54 + 26 \mathfrak{z}_1 + 22 \mathfrak{z}_2 + \\
& \quad \mu_2 (54 + 27 \mathfrak{z}_1 + \mathfrak{z}_2) + \mu_1 (90 + 6 \mathfrak{z}_1 + 28 \mathfrak{z}_2)))) + \eta^4 \\
& \quad (2 \theta p (351 + 475 \mu_1 + 1050 \mu_2 + \eta t (-61 + 712 \mu_1 + 329 \mu_2)) + \\
& \quad (-1 + \eta t) \theta l (2 \times (-9 + 313 \mu_1 + \mu_2) - 5 \theta p (352 + 9 \mathfrak{z}_1 + \\
& \quad \mu_2 (40 + 6 \mathfrak{z}_1 - 60 \mathfrak{z}_2) + 21 \mathfrak{z}_2 + \mu_1 (316 - 13 \mathfrak{z}_1 + 65 \mathfrak{z}_2)))) - 3 \\
& \quad \eta^2 (2 \theta p (201 + 235 \mu_1 + 186 \mu_2 + 2 \eta t (-29 + 91 \mu_1 + 43 \mu_2)) +
\end{aligned}$$



$$\begin{aligned}
& (-1 + \eta t) \, \theta l \, (26 + 30 \mu_1 - 84 \mu_2 + \theta p \, (446 + 109 \, \mathfrak{z}1 + \mu_2 \, (242 + 111 \, \mathfrak{z}1 - \\
& \quad 37 \, \mathfrak{z}2) + 101 \, \mathfrak{z}2 + \mu_1 \, (566 + 13 \, \mathfrak{z}1 + 153 \, \mathfrak{z}2))) + 2 \\
& \eta^3 \, (-\theta p \, (950 + 880 \mu_1 - 618 \mu_2 + \eta t \, (-244 + 61 \mu_1 + 146 \mu_2)) + \\
& \quad (-1 + \eta t) \, \theta l \, (-50 + 305 \mu_1 + 82 \mu_2 - \theta p \, (\mu_2 \, (402 + 153 \, \mathfrak{z}1 - 197 \, \mathfrak{z}2) + \\
& \quad 2 \times (717 + 79 \, \mathfrak{z}1 + 89 \, \mathfrak{z}2) + \mu_1 \, (1494 - 18 \, \mathfrak{z}1 + 352 \, \mathfrak{z}2)))) + \\
& \times (-1 + \eta) \times (42 \eta^8 \theta p - 3 \eta t \theta p \, (3 + 3 \mu_1 + 5 \mu_2) - 42 \eta^7 \theta p \, (-5 + \eta t - \\
& \quad 4 \mu_1 + 6 \mu_2) + 2 \eta^6 \theta p \, (421 + 402 \mu_1 - 384 \mu_2 + 21 \eta t \, (-5 + 6 \mu_2)) - 3 \\
& \quad \eta \, ((-1 + \eta t) \, \theta l \, (3 + 3 \mu_1 + \mu_2) + \eta t \theta p \, (17 + 19 \mu_1 + 51 \mu_2)) - 3 \\
& \quad \eta^2 \, (2 \theta p \, (21 + 35 \mu_1 + 30 \mu_2 + \eta t \, (-3 + 19 \mu_1 + 45 \mu_2)) + \\
& \quad (-1 + \eta t) \, \theta l \, (2 \times (4 + 5 \mu_1 - 5 \mu_2) + \theta p \, (54 + 26 \, \mathfrak{z}1 + 22 \, \mathfrak{z}2 + \\
& \quad \mu_2 \, (54 + 27 \, \mathfrak{z}1 + \mathfrak{z}2) + \mu_1 \, (90 + 6 \, \mathfrak{z}1 + 28 \, \mathfrak{z}2)))) + \eta^5 \\
& \quad (\theta p \, (584 + 718 \mu_1 + 800 \mu_2 + \eta t \, (-121 + 771 \mu_1 + 395 \mu_2)) + \\
& \quad (-1 + \eta t) \, \theta l \, (-3 + 137 \mu_1 + \mu_2 - \theta p \, (718 + 21 \, \mathfrak{z}1 + \\
& \quad \mu_2 \, (82 + 15 \, \mathfrak{z}1 - 117 \, \mathfrak{z}2) + 45 \, \mathfrak{z}2 + \mu_1 \, (646 - 19 \, \mathfrak{z}1 + 137 \, \mathfrak{z}2)))) - \\
& \quad \eta^3 \, (2 \theta p \, (389 + 435 \mu_1 + 310 \mu_2 + \eta t \, (-115 + 387 \mu_1 + 107 \mu_2)) + \\
& \quad (-1 + \eta t) \, \theta l \, (10 \times (4 + 4 \mu_1 - 7 \mu_2) + \theta p \, (906 + 221 \, \mathfrak{z}1 + \mu_2 \, (486 + \\
& \quad 225 \, \mathfrak{z}1 - 71 \, \mathfrak{z}2) + 205 \, \mathfrak{z}2 + \mu_1 \, (1146 + 33 \, \mathfrak{z}1 + 313 \, \mathfrak{z}2)))) + \\
& \quad \eta^4 \, (\theta p \, (-774 - 610 \mu_1 + 183 \eta t \mu_1 + 1020 \mu_2 + 5 \eta t \, (37 + \mu_2)) + \\
& \quad (-1 + \eta t) \, \theta l \, (-28 + 174 \mu_1 + 38 \mu_2 - \theta p \, (\mu_2 \, (406 + 159 \, \mathfrak{z}1 - 191 \, \mathfrak{z}2) + \\
& \quad 2 \times (731 + 82 \, \mathfrak{z}1 + 92 \, \mathfrak{z}2) + \mu_1 \, (1522 - 4 \, \mathfrak{z}1 + 366 \, \mathfrak{z}2)))) + \\
& w^2 \, (-1 + \eta)^2 \, (2 x^8 \, (-1 + \eta)^9 \theta p \, (\eta - \eta t + 4 \mu_1) - x^7 \, (-1 + \eta)^7 \\
& \quad (2 \times (-1 + \eta) \theta p \, (49 + 8 \eta^2 + 57 \mu_1 + \eta \, (17 - 8 \eta t + 32 \mu_1 - 7 \mu_2) + \\
& \quad \eta t \, (-17 + 7 \mu_2)) + (-1 + \eta t) \, \theta l \, (4 + 44 \mu_1 + \\
& \quad \theta p \, (-102 - \mathfrak{z}1 + \mu_1 \, (-74 + 3 \, \mathfrak{z}1 - 11 \, \mathfrak{z}2) - 7 \, \mathfrak{z}2 + 2 \mu_2 \, (-6 + 5 \, \mathfrak{z}2)))) + \\
& x^6 \, (-1 + \eta)^6 \, (2 \times (-1 + \eta) \theta p \, (119 + 28 \eta^3 + 165 \mu_1 + 54 \mu_2 - \\
& \quad 7 \eta^2 \, (-17 + 4 \eta t - 16 \mu_1 + 7 \mu_2) + \eta t \, (-41 + 28 \mu_1 + 49 \mu_2) + \\
& \quad \eta \, (398 + 399 \mu_1 - 76 \mu_2 + 7 \eta t \, (-17 + 7 \mu_2))) + (-1 + \eta t) \, \theta l \\
& \quad (-22 + 94 \mu_1 - 6 \mu_2 + \theta p \, (\mu_1 \, (-260 + 41 \, \mathfrak{z}1 - 37 \, \mathfrak{z}2) - 3 \times (72 + \mathfrak{z}1 + 5 \, \mathfrak{z}2) + \\
& \quad \mu_2 \, (-52 + 66 \, \mathfrak{z}2)) + \eta \, (24 + 324 \mu_1 + \theta p \, (-738 - 80 \mu_2 - \\
& \quad 7 \, \mathfrak{z}1 + 2 \mu_1 \, (-270 + 5 \, \mathfrak{z}1 - 44 \, \mathfrak{z}2) - 49 \, \mathfrak{z}2 + 70 \mu_2 \, \mathfrak{z}2))) + \\
& \eta \theta p \, (2 \eta^9 - 2 \eta t \mu_2 - 28 \eta \eta t \, (1 + \mu_1 + 2 \mu_2) - 2 \eta^8 \, (-16 + \eta t - 4 \mu_1 + \\
& \quad 7 \mu_2) + 2 \eta^7 \, (87 + 53 \mu_1 - 69 \mu_2 + \eta t \, (-16 + 7 \mu_2)) + \eta^5 \\
& \quad (-90 + 64 \mu_1 + 198 \eta t \mu_1 + 366 \mu_2 + 40 \eta t \mu_2 - 3 \times (-1 + \eta t) \, \theta l \\
& \quad (94 + 4 \, \mathfrak{z}1 + \mu_2 \, (18 + 3 \, \mathfrak{z}1 - 19 \, \mathfrak{z}2) + 8 \, \mathfrak{z}2 + \mu_1 \, (108 - 3 \, \mathfrak{z}1 + 23 \, \mathfrak{z}2))) - \\
& \quad \eta^2 \, (4 \times (5 + 5 \mu_1 + 4 \mu_2) - \theta l \, (48 + 25 \, \mathfrak{z}1 + 19 \, \mathfrak{z}2 + \mu_2 \, (50 + 27 \, \mathfrak{z}1 + 11 \, \mathfrak{z}2) + \\
& \quad \mu_1 \, (48 + 11 \, \mathfrak{z}1 + 19 \, \mathfrak{z}2)) + \eta t \, (-8 - 26 \mu_1 + 64 \mu_2 + \theta l \, (48 + 25 \, \mathfrak{z}1 + \\
& \quad 19 \, \mathfrak{z}2 + \mu_2 \, (50 + 27 \, \mathfrak{z}1 + 11 \, \mathfrak{z}2) + \mu_1 \, (48 + 11 \, \mathfrak{z}1 + 19 \, \mathfrak{z}2)))) + \eta^3 \\
& \quad (-2 \times (43 + 85 \mu_1 + 86 \mu_2) + 3 \theta l \, (42 + 20 \, \mathfrak{z}1 + \mu_2 \, (46 + 21 \, \mathfrak{z}1 - 5 \, \mathfrak{z}2) + \\
& \quad 16 \, \mathfrak{z}2 + \mu_1 \, (76 - \mathfrak{z}1 + 21 \, \mathfrak{z}2)) + \eta t \, (2 \times (30 - 57 \mu_1 + \mu_2) - 3 \theta l \, (42 + \\
& \quad 20 \, \mathfrak{z}1 + \mu_2 \, (46 + 21 \, \mathfrak{z}1 - 5 \, \mathfrak{z}2) + 16 \, \mathfrak{z}2 + \mu_1 \, (76 - \mathfrak{z}1 + 21 \, \mathfrak{z}2)))) + \\
& \eta^6 \, (156 + 216 \mu_1 - 38 \mu_2 + \theta l \, (126 + 8 \mu_2 + \mathfrak{z}1 + 7 \, \mathfrak{z}2 - 10 \mu_2 \, \mathfrak{z}2 + \\
& \quad \mu_1 \, (96 + 8 \, \mathfrak{z}1 + 22 \, \mathfrak{z}2)) - \eta t \, (48 - 116 \mu_1 - 84 \mu_2 + \\
& \quad \theta l \, (126 + 8 \mu_2 + \mathfrak{z}1 + 7 \, \mathfrak{z}2 - 10 \mu_2 \, \mathfrak{z}2 + \mu_1 \, (96 + 8 \, \mathfrak{z}1 + 22 \, \mathfrak{z}2)))) + \eta^4 \\
& \quad (12 \times (-14 - 17 \mu_1 + \mu_2) + \theta l \, (234 + 46 \, \mathfrak{z}1 + \mu_2 \, (134 + 45 \, \mathfrak{z}1 - 73 \, \mathfrak{z}2) + \\
& \quad 46 \, \mathfrak{z}2 + \mu_1 \, (408 - 31 \, \mathfrak{z}1 + 91 \, \mathfrak{z}2)) + \\
& \quad \eta t \, (-6 \times (-7 + 33 \mu_1 + 3 \mu_2) - \theta l \, (234 + 46 \, \mathfrak{z}1 + \mu_2
\end{aligned}$$

$$\begin{aligned}
& (134 + 45 \, \mathfrak{e}1 - 73 \, \mathfrak{e}2) + 46 \, \mathfrak{e}2 + \mu1 (408 - 31 \, \mathfrak{e}1 + 91 \, \mathfrak{e}2) \Big) \Big) + \\
& x^5 (-1 + \eta)^5 \Big( - \Big( (-1 + \eta) \, \mathfrak{e}p \Big( 226 + 112 \, \eta^4 + 394 \, \mu1 + 352 \, \mu2 - 14 \, \eta^3 \\
& \quad (-51 + 8 \, \eta t - 32 \, \mu1 + 21 \, \mu2) + \eta t (-91 + 169 \, \mu1 + 129 \, \mu2) + \\
& \quad 6 \, \eta^2 (453 + 399 \, \mu1 - 152 \, \mu2 + 7 \, \eta t (-17 + 7 \, \mu2)) + \\
& \quad 2 \, \eta (777 + 990 \, \mu1 + 175 \, \mu2 + 6 \, \eta t (-41 + 33 \, \mu1 + 49 \, \mu2)) \Big) \Big) + (-1 + \eta t) \\
& \, \mathfrak{e}l \Big( 52 + 60 \, \mu1 - 42 \, \mu2 + \mathfrak{e}p (174 + 28 \, \mathfrak{e}1 + \mu2 (118 + 27 \, \mathfrak{e}1 - 91 \, \mathfrak{e}2) + \\
& \quad 28 \, \mathfrak{e}2 + \mu1 (346 - 62 \, \mathfrak{e}1 + 60 \, \mathfrak{e}2)) + 3 \, \eta^2 (-20 \times (1 + 16 \, \mu1) + \\
& \quad \mathfrak{e}p (762 + 76 \, \mu2 + 7 \, \mathfrak{e}1 + 49 \, \mathfrak{e}2 - 70 \, \mu2 \, \mathfrak{e}2 + \mu1 (562 + \mathfrak{e}1 + 99 \, \mathfrak{e}2)) + \\
& \quad \eta (101 - 615 \, \mu1 + 21 \, \mu2 + \mathfrak{e}p (1362 + 314 \, \mu2 + 27 \, \mathfrak{e}1 + 9 \, \mu2 \, \mathfrak{e}1 + \\
& \quad 99 \, \mathfrak{e}2 - 387 \, \mu2 \, \mathfrak{e}2 + \mu1 (1624 - 214 \, \mathfrak{e}1 + 254 \, \mathfrak{e}2)) \Big) \Big) - \\
& x^4 (-1 + \eta)^4 \Big( -2 \times (-1 + \eta) \, \mathfrak{e}p \Big( 53 + 70 \, \eta^5 + 95 \, \mu1 + 106 \, \mu2 - 35 \, \eta^4 \\
& \quad (-17 + 2 \, \eta t - 8 \, \mu1 + 7 \, \mu2) + \eta t (-20 + 27 \, \mu1 + 60 \, \mu2) + \\
& \quad 5 \, \eta^3 (508 + 399 \, \mu1 - 228 \, \mu2 + 7 \, \eta t (-17 + 7 \, \mu2)) + \\
& \quad 5 \, \eta^2 (420 + 495 \, \mu1 + 13 \, \mu2 + 3 \, \eta t (-41 + 38 \, \mu1 + 49 \, \mu2)) + \\
& \quad \eta (589 + 985 \, \mu1 + 792 \, \mu2 + \eta t (-223 + 495 \, \mu1 + 327 \, \mu2)) \Big) + (-1 + \eta t) \, \mathfrak{e}l \\
& \Big( -2 + 34 \, \mu1 - 104 \, \mu2 + \mathfrak{e}p (108 + 51 \, \mathfrak{e}1 + 2 \, \mu2 (64 + 27 \, \mathfrak{e}1 - 12 \, \mathfrak{e}2) + \\
& \quad 39 \, \mathfrak{e}2 + \mu1 (208 - 13 \, \mathfrak{e}1 + 53 \, \mathfrak{e}2)) + 5 \, \eta^3 (-8 \times (2 + 37 \, \mu1) + \mathfrak{e}p \\
& \quad (786 + 72 \, \mu2 + 7 \, \mathfrak{e}1 + 49 \, \mathfrak{e}2 - 70 \, \mu2 \, \mathfrak{e}2 + 2 \, \mu1 (292 + 6 \, \mathfrak{e}1 + 55 \, \mathfrak{e}2)) \Big) + \\
& \quad \eta^2 (8 \times (23 - 190 \, \mu1 + 3 \, \mu2) + 5 \, \mathfrak{e}p (714 + 158 \, \mu2 + 18 \, \mathfrak{e}1 + \\
& \quad 9 \, \mu2 \, \mathfrak{e}1 + 54 \, \mathfrak{e}2 - 189 \, \mu2 \, \mathfrak{e}2 + \mu1 (844 - 91 \, \mathfrak{e}1 + 143 \, \mathfrak{e}2)) \Big) + \\
& \quad \eta (2 \times (104 + 89 \, \mu1 - 84 \, \mu2) + \mathfrak{e}p (930 + 606 \, \mu2 + 158 \, \mathfrak{e}1 + 153 \\
& \quad \mu2 \, \mathfrak{e}1 + 158 \, \mathfrak{e}2 - 437 \, \mu2 \, \mathfrak{e}2 + \mu1 (1792 - 279 \, \mathfrak{e}1 + 331 \, \mathfrak{e}2)) \Big) \Big) + \\
& x^2 (-1 + \eta)^2 \Big( 56 \, \eta^8 \, \mathfrak{e}p - 14 \, \eta^7 \, \mathfrak{e}p (-47 + 4 \, \eta t - 16 \, \mu1 + 21 \, \mu2) + 2 \, \eta^6 \\
& \, \mathfrak{e}p (1497 + 1085 \, \mu1 - 993 \, \mu2 + 7 \, \eta t (-47 + 21 \, \mu2)) - 2 \\
& \, (\mathfrak{e}l \, \mu2 - \eta t \, \mathfrak{e}l \, \mu2 + \eta t \, \mathfrak{e}p (26 + 27 \, \mu1 + 41 \, \mu2)) - \eta \\
& (4 \, \mathfrak{e}p (3 \times (5 + 5 \, \mu1 + 4 \, \mu2) + \eta t (17 + 7 \, \mu1 + 86 \, \mu2)) + \\
& \quad (-1 + \eta t) \, \mathfrak{e}l (-2 \times (16 + 15 \, \mu1 + 46 \, \mu2) + 3 \, \mathfrak{e}p (48 + 25 \, \mathfrak{e}1 + 19 \, \mathfrak{e}2 + \\
& \quad \mu2 (50 + 27 \, \mathfrak{e}1 + 11 \, \mathfrak{e}2) + \mu1 (48 + 11 \, \mathfrak{e}1 + 19 \, \mathfrak{e}2))) \Big) + \eta^5 \\
& (2 \, \mathfrak{e}p (561 + 1278 \, \mu1 + 460 \, \mu2 + 6 \, \eta t (-43 + 120 \, \mu1 + 98 \, \mu2)) - \\
& \quad 3 \times (-1 + \eta t) \, \mathfrak{e}l (-4 \times (2 + 47 \, \mu1) + \mathfrak{e}p (834 + 64 \, \mu2 + 7 \, \mathfrak{e}1 + \\
& \quad 49 \, \mathfrak{e}2 - 70 \, \mu2 \, \mathfrak{e}2 + 2 \, \mu1 (314 + 17 \, \mathfrak{e}1 + 66 \, \mathfrak{e}2))) \Big) + \eta^2 \\
& (-2 \, \mathfrak{e}p (36 \times (8 + 15 \, \mu1 + 16 \, \mu2) + \eta t (-180 + 214 \, \mu1 + 147 \, \mu2)) + \\
& \quad (-1 + \eta t) \, \mathfrak{e}l (-54 - 178 \, \mu1 + 252 \, \mu2 - 3 \, \mathfrak{e}p (234 + 266 \, \mu2 + 111 \, \mathfrak{e}1 + \\
& \quad 117 \, \mu2 \, \mathfrak{e}1 + 87 \, \mathfrak{e}2 - 39 \, \mu2 \, \mathfrak{e}2 + \mu1 (436 - 16 \, \mathfrak{e}1 + 116 \, \mathfrak{e}2))) \Big) + \eta^4 \\
& (2 \, \mathfrak{e}p (-1141 - 505 \, \mu1 + \eta t (187 + 560 \, \mu1 - 63 \, \mu2) + 1912 \, \mu2) + \\
& \quad (-1 + \eta t) \, \mathfrak{e}l (-74 + 1050 \, \mu1 + 6 \, \mu2 - 5 \, \mathfrak{e}p (780 + 27 \, \mathfrak{e}1 + \\
& \quad 2 \, \mu2 (80 + 9 \, \mathfrak{e}1 - 90 \, \mathfrak{e}2) + 63 \, \mathfrak{e}2 + \mu1 (908 - 59 \, \mathfrak{e}1 + 175 \, \mathfrak{e}2))) \Big) + \\
& 2 \, \eta^3 (-\mathfrak{e}p (956 + 1400 \, \mu1 + 632 \, \mu2 + \eta t (-308 + 1025 \, \mu1 + 312 \, \mu2)) + \\
& \quad (-1 + \eta t) \, \mathfrak{e}l (-104 - 27 \, \mu1 + 84 \, \mu2 - \mathfrak{e}p (\mu2 (638 + 189 \, \mathfrak{e}1 - 401 \, \mathfrak{e}2) + \\
& \quad 2 \times (525 + 97 \, \mathfrak{e}1 + 97 \, \mathfrak{e}2) + \mu1 (1916 - 217 \, \mathfrak{e}1 + 393 \, \mathfrak{e}2))) \Big) - \\
& x (-1 + \eta) \times \Big( 16 \, \eta^9 \, \mathfrak{e}p + 2 \, \eta^8 \, \mathfrak{e}p (111 - 8 \, \eta t + 32 \, \mu1 - 49 \, \mu2) - \eta t \, \mathfrak{e}p \\
& \quad (3 + 3 \, \mu1 + 5 \, \mu2) + 2 \, \eta^7 \, \mathfrak{e}p (554 + 367 \, \mu1 - 407 \, \mu2 + \eta t (-111 + 49 \, \mu2)) - \eta \\
& \quad ((-1 + \eta t) \, \mathfrak{e}l (3 + 3 \, \mu1 + \mu2) + \eta t \, \mathfrak{e}p (77 + 79 \, \mu1 + 135 \, \mu2)) - \eta^2 \\
& \quad (2 \, \mathfrak{e}p (6 \times (5 + 5 \, \mu1 + 4 \, \mu2) + \eta t (5 - 19 \, \mu1 + 128 \, \mu2)) + \\
& \quad (-1 + \eta t) \, \mathfrak{e}l (-2 \times (2 + \mu1 + 17 \, \mu2) + 3 \, \mathfrak{e}p (48 + 25 \, \mathfrak{e}1 + 19 \, \mathfrak{e}2 + \\
& \quad \mu2 (50 + 27 \, \mathfrak{e}1 + 11 \, \mathfrak{e}2) + \mu1 (48 + 11 \, \mathfrak{e}1 + 19 \, \mathfrak{e}2))) \Big) + \eta^6
\end{aligned}$$

$$\begin{aligned}
& (2 \, \theta p \, (356 + 591 \, \mu_1 + 35 \, \mu_2 + \eta t \, (-127 + 318 \, \mu_1 + 245 \, \mu_2)) - \\
& \quad (-1 + \eta t) \, \theta l \, (-4 \times (1 + 26 \, \mu_1) + \theta p \, (858 + 60 \, \mu_2 + 7 \, \mu_1 + \\
& \quad \quad 49 \, \mu_2 - 70 \, \mu_2 \, \mu_2 + \mu_1 \, (650 + 45 \, \mu_1 + 143 \, \mu_2))) + \eta^3 \\
& \quad (-2 \, \theta p \, (14 \times (13 + 25 \, \mu_1 + 26 \, \mu_2) + \eta t \, (-125 + 179 \, \mu_1 + 42 \, \mu_2)) + \\
& \quad \quad (-1 + \eta t) \, \theta l \, (-28 - 72 \, \mu_1 + 74 \, \mu_2 - \theta p \, (486 + 542 \, \mu_2 + 231 \, \mu_1 + \\
& \quad \quad \quad 243 \, \mu_2 \, \mu_1 + 183 \, \mu_2 - 69 \, \mu_2 \, \mu_2 + \mu_1 \, (892 - 22 \, \mu_1 + 242 \, \mu_2))) + \\
& \quad \eta^5 \, (\theta p \, (-2 \times (368 + 5 \, \mu_1 - 949 \, \mu_2) + \eta t \, (73 + 789 \, \mu_1 + 93 \, \mu_2)) + \\
& \quad \quad (-1 + \eta t) \, \theta l \, (-13 + 239 \, \mu_1 + 3 \, \mu_2 - \theta p \, (1626 + 322 \, \mu_2 + 63 \, \mu_1 + 45 \, \mu_2 \, \mu_1 + \\
& \quad \quad \quad 135 \, \mu_2 - 351 \, \mu_2 \, \mu_2 + \mu_1 \, (1880 - 86 \, \mu_1 + 382 \, \mu_2))) + \eta^4 \\
& \quad (-\theta p \, (898 + 1210 \, \mu_1 + 280 \, \mu_2 + \eta t \, (-259 + 1023 \, \mu_1 + 201 \, \mu_2)) + \\
& \quad \quad (-1 + \eta t) \, \theta l \, (2 \times (-26 + \mu_1 + 21 \, \mu_2) - \theta p \, (1110 + 212 \, \mu_1 + \mu_2 \, (654 + 207 \\
& \quad \quad \quad \mu_1 - 383 \, \mu_2) + 212 \, \mu_2 + \mu_1 \, (1978 - 186 \, \mu_1 + 424 \, \mu_2)))) + \\
& \quad x^3 \, (-1 + \eta)^3 \, (-2 \times (-1 + \eta) \, \theta p \, (56 \, \eta^6 + 2 \times (5 + 5 \, \mu_1 + 4 \, \mu_2) - 7 \, \eta^5 \\
& \quad \quad (-85 + 8 \, \eta t - 32 \, \mu_1 + 35 \, \mu_2) + \eta t \, (25 + 20 \, \mu_1 + 76 \, \mu_2) + \\
& \quad \quad 5 \, \eta^4 \, (563 + 399 \, \mu_1 - 304 \, \mu_2 + 7 \, \eta t \, (-17 + 7 \, \mu_2)) + \\
& \quad \quad 10 \, \eta^3 \, (301 + 330 \, \mu_1 - 41 \, \mu_2 + \eta t \, (-82 + 86 \, \mu_1 + 98 \, \mu_2)) + \\
& \quad \quad \eta \, (4 \times (53 + 95 \, \mu_1 + 103 \, \mu_2) + \eta t \, (-80 + 139 \, \mu_1 + 240 \, \mu_2)) + \\
& \quad \quad \eta^2 \, (\eta t \, (-437 + 1135 \, \mu_1 + 663 \, \mu_2) + 2 \times (613 + 985 \, \mu_1 + 704 \, \mu_2))) + \\
& \quad \quad (-1 + \eta t) \, \theta l \, (-2 \times (14 + 14 \, \mu_1 + 29 \, \mu_2) + \theta p \, (48 + 25 \, \mu_1 + 19 \, \mu_2 + \\
& \quad \quad \quad \mu_2 \, (50 + 27 \, \mu_1 + 11 \, \mu_2) + \mu_1 \, (48 + 11 \, \mu_1 + 19 \, \mu_2)) + \\
& \quad \quad \eta \, (24 + 140 \, \mu_1 - 282 \, \mu_2 + 3 \, \theta p \, (150 + 71 \, \mu_1 + \mu_2 \, (174 + 75 \, \mu_1 - 29 \, \mu_2) + \\
& \quad \quad \quad 55 \, \mu_2 + \mu_1 \, (284 - 14 \, \mu_1 + 74 \, \mu_2))) + 2 \, \eta^3 \, (83 - 905 \, \mu_1 + \\
& \quad \quad 3 \, \mu_2 + 5 \, \theta p \, (498 + 15 \, \mu_1 + \mu_2 \, (106 + 9 \, \mu_1 - 123 \, \mu_2) + 39 \, \mu_2 + \\
& \quad \quad \quad \mu_1 \, (584 - 50 \, \mu_1 + 106 \, \mu_2))) + 5 \, \eta^4 \, (-12 \times (1 + 21 \, \mu_1) + \theta p \, (810 + \\
& \quad \quad 68 \, \mu_2 + 7 \, \mu_1 + 49 \, \mu_2 - 70 \, \mu_2 \, \mu_2 + \mu_1 \, (606 + 23 \, \mu_1 + 121 \, \mu_2))) + \\
& \quad \quad \eta^2 \, (6 \times (52 + 29 \, \mu_1 - 42 \, \mu_2) + \theta p \, (2 \, \mu_2 \, (622 + 171 \, \mu_1 - 419 \, \mu_2) + \\
& \quad \quad \quad 44 \times (45 + 8 \, \mu_1 + 8 \, \mu_2) + \mu_1 \, (3708 - 496 \, \mu_1 + 724 \, \mu_2)))) - \\
& \quad w \, (x \, (-1 + \eta) - \eta) \, (-1 + \eta) \times (2 \, x^7 \, (-1 + \eta)^7 \, \theta p \, (-15 + 5 \, \eta^2 + 5 \, \eta t + 15 \\
& \quad \quad \theta l - 5 \, \eta \, (-2 + \eta t - 3 \, \mu_1) - 15 \, \mu_1 + 7 \, \theta l \, \mu_1 + \theta l \, \mu_2 - \eta t \, \theta l \, (15 + 7 \, \mu_1 + \mu_2)) + \\
& \quad \quad x^6 \, (-1 + \eta)^6 \, (-2 \times (-1 + \eta) \, \theta p \, (29 + 35 \, \eta^2 + 71 \, \mu_1 + \eta \, (139 - 35 \, \eta t + \\
& \quad \quad \quad 105 \, \mu_1 - 21 \, \mu_2) + 10 \, \mu_2 + 2 \, \eta t \, (-11 + 7 \, \mu_2)) + (-1 + \eta t) \, \theta l \\
& \quad \quad (-8 - 28 \times (2 + \eta) \, \mu_1 + \eta \, \theta p \, (234 + 14 \, \mu_2 + 7 \, \mu_1 \, (16 + \mu_1 + \mu_2)) + \\
& \quad \quad 2 \, \theta p \, (33 + \mu_1 + 6 \, \mu_2 - 2 \, \mu_2 \, (-7 + 5 \, \mu_2) + \mu_1 \, (59 - 7 \, \mu_1 + 7 \, \mu_2))) + \\
& \quad \quad x^5 \, (-1 + \eta)^5 \, (2 \times (-1 + \eta) \, \theta p \, (37 + 105 \, \eta^3 + 121 \, \mu_1 + 92 \, \mu_2 + \\
& \quad \quad 5 \, \eta t \, (-5 + 8 \, \mu_1 + 7 \, \mu_2) - 3 \, \eta^2 \, (-173 + 35 \, \eta t - 105 \, \mu_1 + 42 \, \mu_2) + \\
& \quad \quad \eta \, (227 + 426 \, \mu_1 - 15 \, \mu_2 + 2 \, \eta t \, (-66 + 7 \, \mu_1 + 42 \, \mu_2))) - \\
& \quad \quad (-1 + \eta t) \, \theta l \, (26 + 14 \, \mu_1 + 6 \, \mu_2 + \theta p \, (48 + 3 \, \mu_1 + \mu_2 \, (68 - 66 \, \mu_2) + \\
& \quad \quad \quad 11 \, \mu_2 + \mu_1 \, (204 - 55 \, \mu_1 + 23 \, \mu_2)) + \\
& \quad \quad 2 \, \eta^2 \, (-70 \, \mu_1 + 3 \, \theta p \, (129 + 7 \, \mu_2 + 7 \, \mu_1 \, (9 + \mu_1 + \mu_2))) - \\
& \quad \quad 2 \, \eta \, (20 + 186 \, \mu_1 + \theta p \, (\mu_1 \, (-376 + 31 \, \mu_1 - 53 \, \mu_2) + \\
& \quad \quad \quad 20 \, \mu_2 \, (-4 + 3 \, \mu_2) - 6 \times (37 + \mu_1 + 6 \, \mu_2)))) + \\
& \quad \eta \, \theta p \, (-10 \, \eta^8 + 6 \, \eta t \, (2 + 2 \, \mu_1 + 3 \, \mu_2) + 2 \, \eta^7 \, (-44 + 5 \, \eta t - 15 \, \mu_1 + 21 \, \mu_2) + \\
& \quad \eta^6 \, (-66 - 112 \, \mu_1 + 88 \, \mu_2 - 2 \, \theta l \, (27 + \mu_2) - 7 \, \theta l \, \mu_1 \, (4 + \mu_1 + \mu_2) + \\
& \quad \eta t \, (34 - 28 \, \mu_1 - 28 \, \mu_2 + 2 \, \theta l \, (27 + \mu_2) + 7 \, \theta l \, \mu_1 \, (4 + \mu_1 + \mu_2))) + \eta \\
& \quad (-\theta l \, (12 + 8 \, \mu_1 + 6 \, \mu_2 + 2 \, \mu_1 \, (6 + 4 \, \mu_1 + 3 \, \mu_2) + \mu_2 \, (14 + 9 \, \mu_1 + 7 \, \mu_2)) +
\end{aligned}$$

$$\begin{aligned}
& \eta t (-4 - 10 \mu_1 + 30 \mu_2 + \theta l (12 + 8 \mathfrak{z}_1 + 6 \mathfrak{z}_2 + \\
& \quad 2 \mu_1 (6 + 4 \mathfrak{z}_1 + 3 \mathfrak{z}_2) + \mu_2 (14 + 9 \mathfrak{z}_1 + 7 \mathfrak{z}_2))) + \eta^2 \\
& (40 \times (1 + \mu_1 + \mu_2) - \theta l (48 + 24 \mathfrak{z}_1 + 3 \mu_2 (18 + 9 \mathfrak{z}_1 - \mathfrak{z}_2) + 14 \mathfrak{z}_2 + \\
& \quad \mu_1 (46 - 5 \mathfrak{z}_1 + 13 \mathfrak{z}_2)) + \eta t (-2 \times (14 + 25 \mu_1 + 3 \mu_2) + \theta l (48 + \\
& \quad 24 \mathfrak{z}_1 + 3 \mu_2 (18 + 9 \mathfrak{z}_1 - \mathfrak{z}_2) + 14 \mathfrak{z}_2 + \mu_1 (46 - 5 \mathfrak{z}_1 + 13 \mathfrak{z}_2)))) + \\
& 2 \eta^5 (21 - 50 \mu_1 - 81 \mu_2 - \theta l (57 + \mathfrak{z}_1 - 10 \mu_2 (-1 + \mathfrak{z}_2) + 6 \mathfrak{z}_2 + \\
& \quad \mu_1 (81 + 4 \mathfrak{z}_1 + 18 \mathfrak{z}_2)) + \eta t (3 - 72 \mu_1 - 21 \mu_2 + \\
& \quad \theta l (57 + \mathfrak{z}_1 - 10 \mu_2 (-1 + \mathfrak{z}_2) + 6 \mathfrak{z}_2 + \mu_1 (81 + 4 \mathfrak{z}_1 + 18 \mathfrak{z}_2)))) + \eta^3 \\
& (2 \times (23 + 65 \mu_1 + 74 \mu_2) - \theta l (66 + 26 \mathfrak{z}_1 + \mu_2 (86 + 27 \mathfrak{z}_1 - 47 \mathfrak{z}_2) + \\
& \quad 18 \mathfrak{z}_2 + \mu_1 (162 - 40 \mathfrak{z}_1 + 30 \mathfrak{z}_2)) + \\
& \quad \eta t (2 \times (-6 + 91 \mu_1 + 6 \mu_2) + \theta l (66 + 26 \mathfrak{z}_1 + \mu_2 (86 + 27 \mathfrak{z}_1 - 47 \mathfrak{z}_2) + \\
& \quad 18 \mathfrak{z}_2 + \mu_1 (162 - 40 \mathfrak{z}_1 + 30 \mathfrak{z}_2)))) + \eta^4 \\
& (12 \times (3 + 6 \mu_1 - 13 \mu_2) - \theta l (90 + 12 \mathfrak{z}_1 + \mu_2 (66 + 9 \mathfrak{z}_1 - 57 \mathfrak{z}_2) + \\
& \quad 20 \mathfrak{z}_2 + \mu_1 (262 - 26 \mathfrak{z}_1 + 52 \mathfrak{z}_2)) + \\
& \quad \eta t (2 \times (-9 + 19 \mu_1 + 8 \mu_2) + \theta l (90 + 12 \mathfrak{z}_1 + \mu_2 (66 + 9 \mathfrak{z}_1 - 57 \mathfrak{z}_2) + \\
& \quad 20 \mathfrak{z}_2 + \mu_1 (262 - 26 \mathfrak{z}_1 + 52 \mathfrak{z}_2)))) + \\
& x^4 (-1 + \eta)^4 \left( - \left( (-1 + \eta) \theta p (86 + 350 \eta^4 + 170 \mu_1 + 228 \mu_2 + \eta t \right. \right. \\
& \quad (-41 + 49 \mu_1 + 45 \mu_2) - 10 \eta^3 (-207 + 35 \eta t - 105 \mu_1 + 63 \mu_2) + \\
& \quad 2 \eta (209 + 605 \mu_1 + 246 \eta t \mu_1 + 384 \mu_2 + 25 \eta t (-5 + 7 \mu_2)) + \\
& \quad \left. \left. 10 \eta^2 (140 + 213 \mu_1 - 45 \mu_2 + 2 \eta t (-33 + 7 \mu_1 + 21 \mu_2)) \right) \right) + (-1 + \eta t) \\
& \quad \theta l (56 + 112 \mu_1 - 6 \mu_2 + \theta p (30 + 8 \mathfrak{z}_1 + \mu_2 (66 + 9 \mathfrak{z}_1 - 65 \mathfrak{z}_2) + \\
& \quad \mu_1 (122 - 60 \mathfrak{z}_1 + 10 \mathfrak{z}_2)) + \\
& \quad 5 \eta^3 (-56 \mu_1 + \theta p (282 + 14 \mathfrak{z}_2 + 7 \mu_1 (20 + 3 \mathfrak{z}_1 + 3 \mathfrak{z}_2))) - \\
& \quad 2 \eta^2 (8 \times (5 + 58 \mu_1) + 5 \theta p (\mu_1 (-199 + 10 \mathfrak{z}_1 - 32 \mathfrak{z}_2) - \\
& \quad 3 \times (41 + \mathfrak{z}_1 + 6 \mathfrak{z}_2) + \mu_2 (-38 + 30 \mathfrak{z}_2))) + \\
& \quad \eta (95 - 29 \mu_1 + 15 \mu_2 + \theta p (282 + 24 \mathfrak{z}_1 + \mu_2 (338 + 9 \mathfrak{z}_1 - 321 \mathfrak{z}_2) + \\
& \quad 64 \mathfrak{z}_2 + \mu_1 (1078 - 246 \mathfrak{z}_1 + 144 \mathfrak{z}_2)))) - \\
& x^3 (-1 + \eta)^3 \left( - \left( (-1 + \eta) \theta p (350 \eta^5 + 8 \times (5 + 5 \mu_1 + 6 \mu_2) + \eta t \right. \right. \\
& \quad (-32 - 54 \mu_1 + 30 \mu_2) - 10 \eta^4 (-241 + 35 \eta t - 105 \mu_1 + 84 \mu_2) + \\
& \quad 4 \eta^2 (233 + 605 \mu_1 + 292 \eta t \mu_1 + 308 \mu_2 + 25 \eta t (-5 + 7 \mu_2)) + \\
& \quad 20 \eta^3 (111 + 142 \mu_1 - 55 \mu_2 + 2 \eta t (-22 + 7 \mu_1 + 14 \mu_2)) + \\
& \quad \left. \left. \eta (8 \times (43 + 85 \mu_1 + 109 \mu_2) + \eta t (-155 + 281 \mu_1 + 189 \mu_2)) \right) \right) + \\
& (-1 + \eta t) \theta l (2 \times (5 + 7 \mu_1 - 15 \mu_2) + \theta p (2 \mu_2 (20 + 9 \mathfrak{z}_1 - 6 \mathfrak{z}_2) + \\
& \quad 5 \times (6 + 3 \mathfrak{z}_1 + \mathfrak{z}_2) + \mu_1 (34 - 11 \mathfrak{z}_1 + 7 \mathfrak{z}_2)) + \\
& \quad 10 \eta^4 (-28 \mu_1 + \theta p (153 + 7 \mathfrak{z}_2 + 7 \mu_1 (11 + 2 \mathfrak{z}_1 + 2 \mathfrak{z}_2))) - \\
& \quad 4 \eta^3 (20 + 278 \mu_1 + 5 \theta p (3 \mu_1 \mathfrak{z}_1 + 4 \mu_2 (-6 + 5 \mathfrak{z}_2) - \\
& \quad 5 \mu_1 (28 + 5 \mathfrak{z}_2) - 2 \times (45 + \mathfrak{z}_1 + 6 \mathfrak{z}_2))) + \\
& \quad \eta (6 \times (26 + 55 \mu_1 - 5 \mu_2) + 2 \theta p (78 + 25 \mathfrak{z}_1 + \mu_2 (142 + 27 \mathfrak{z}_1 - \\
& \quad 121 \mathfrak{z}_2) + 9 \mathfrak{z}_2 + \mu_1 (264 - 110 \mathfrak{z}_1 + 30 \mathfrak{z}_2))) + \\
& \quad \eta^2 (129 - 171 \mu_1 + 9 \mu_2 + \theta p (648 + 66 \mathfrak{z}_1 + 12 \mu_2 (56 + 3 \mathfrak{z}_1 - \\
& \quad 52 \mathfrak{z}_2) + 146 \mathfrak{z}_2 + \mu_1 (2272 - 434 \mathfrak{z}_1 + 346 \mathfrak{z}_2)))) + \\
& x^2 (-1 + \eta)^2 \left( - \left( (-1 + \eta) \theta p (210 \eta^6 - 6 \eta \eta t (14 + 26 \mu_1 - 17 \mu_2) + \right. \right. \\
& \quad 8 \eta (15 + 15 \mu_1 + 17 \mu_2) - 30 \eta^5 \\
& \quad (-55 + 7 \eta t - 21 \mu_1 + 21 \mu_2) + \eta t (11 + 11 \mu_1 + 51 \mu_2) + \\
& \quad 4 \eta^3 (257 + 605 \mu_1 + 338 \eta t \mu_1 + 232 \mu_2 + 25 \eta t (-5 + 7 \mu_2)) + \\
& \quad \left. \left. 10 \eta^4 (193 + 213 \mu_1 - 120 \mu_2 + \eta t (-66 + 28 \mu_1 + 42 \mu_2)) \right) \right) +
\end{aligned}$$

$$\begin{aligned}
& 3 \eta^2 (\eta t (-73 + 183 \mu_1 + 99 \mu_2) + 4 \times (43 + 85 \mu_1 + 104 \mu_2)) + \\
& (-1 + \eta t) \theta l (-6 \times (2 + 2 \mu_1 + 3 \mu_2) + \theta p (12 + 8 \mu_1 + 6 \mu_2 + \\
& 2 \mu_1 (6 + 4 \mu_1 + 3 \mu_2) + \mu_2 (14 + 9 \mu_1 + 7 \mu_2)) + \\
& \eta (23 + 37 \mu_1 - 57 \mu_2 + \theta p (\mu_2 (134 + 63 \mu_1 - 27 \mu_2) - \\
& 3 \mu_1 (-38 + 9 \mu_1 - 9 \mu_2) + 6 \times (18 + 9 \mu_1 + 4 \mu_2))) + \\
& \eta^5 (-140 \mu_1 + 3 \theta p (330 + 14 \mu_2 + 7 \mu_1 (24 + 5 \mu_1 + 5 \mu_2))) - \\
& 6 \eta^2 (-24 - 54 \mu_1 + 7 \mu_2 - \theta p (48 + 17 \mu_1 + 2 \mu_2 (38 + 9 \mu_1 - 28 \mu_2) + \\
& 9 \mu_2 + \mu_1 (142 - 50 \mu_1 + 20 \mu_2))) + 2 \eta^4 (-4 \times (5 + 81 \mu_1) + 5 \theta p \\
& (\mu_2 (34 - 30 \mu_2) + 3 \times (49 + \mu_1 + 6 \mu_2) + \mu_1 (221 + \mu_1 + 43 \mu_2))) + \\
& \eta^3 (77 - 199 \mu_1 - 3 \mu_2 + \theta p (732 + 84 \mu_1 + \mu_2 (668 + 54 \mu_1 - 606 \mu_2) + \\
& 164 \mu_2 + \mu_1 (2388 - 376 \mu_1 + 404 \mu_2))) + \\
& \times (-1 + \eta) \times (70 \eta^8 \theta p + 2 \eta^7 \theta p (274 - 35 \eta t + 105 \mu_1 - 126 \mu_2) - 6 \\
& \eta t \theta p (3 + 3 \mu_1 + 4 \mu_2) - \eta (\eta t \theta p (1 - 5 \mu_1 + 75 \mu_2) + \\
& 2 \times (-1 + \eta t) \theta l (-3 \times (1 + \mu_1 + 2 \mu_2) + \theta p \\
& (12 + 8 \mu_1 + 6 \mu_2 + 2 \mu_1 (6 + 4 \mu_1 + 3 \mu_2) + \mu_2 (14 + 9 \mu_1 + 7 \mu_2)))) + \\
& \eta^2 (\theta p (\eta t (91 + 163 \mu_1 - 15 \mu_2) - 8 \times (15 + 15 \mu_1 + 16 \mu_2)) + \\
& (-1 + \eta t) \theta l (-13 - 23 \mu_1 + 27 \mu_2 - \theta p (126 + 63 \mu_1 + \\
& 2 \mu_2 (74 + 36 \mu_1 - 9 \mu_2) + 33 \mu_2 + \mu_1 (126 - 21 \mu_1 + 33 \mu_2)))) + \\
& \eta^3 (-\theta p (8 \times (28 + 70 \mu_1 + 83 \mu_2) + \eta t (-65 + 601 \mu_1 + 93 \mu_2)) + \\
& 2 \times (-1 + \eta t) \theta l (-22 - 53 \mu_1 + 9 \mu_2 - \theta p (114 + 43 \mu_1 + \\
& \mu_2 (162 + 45 \mu_1 - 103 \mu_2) + 27 \mu_2 + \mu_1 (304 - 90 \mu_1 + 50 \mu_2)))) - \\
& 2 \eta^5 (-\theta p (-158 + 179 \mu_1 + 471 \mu_2 + \eta t (7 + 314 \mu_1 + 91 \mu_2)) + \\
& (-1 + \eta t) \theta l (-4 - 74 \mu_1 + \theta p (\mu_2 (64 - 60 \mu_2) + \\
& 6 \times (53 + \mu_1 + 6 \mu_2) + \mu_1 (464 + 13 \mu_1 + 97 \mu_2)))) + \eta^4 \\
& (-\theta p (218 + 530 \mu_1 - 480 \mu_2 + \eta t (-113 + 317 \mu_1 + 143 \mu_2)) + \\
& (-1 + \eta t) \theta l (-17 + 71 \mu_1 + 3 \mu_2 - \theta p (408 + 51 \mu_1 + \mu_2 (332 + 36 \mu_1 - \\
& 294 \mu_2) + 91 \mu_2 + \mu_1 (1252 - 159 \mu_1 + 231 \mu_2)))) - 2 \\
& \eta^6 (-14 \times (-1 + \eta t) \theta l \mu_1 + \theta p (-130 - 321 \mu_1 + 189 \mu_2 - \\
& \theta l (177 + 7 \mu_2 + 7 \mu_1 (13 + 3 \mu_1 + 3 \mu_2)) + \eta t (97 - 70 \mu_1 - \\
& 84 \mu_2 + \theta l (177 + 7 \mu_2 + 7 \mu_1 (13 + 3 \mu_1 + 3 \mu_2)))) - \\
& (x + \eta - x \eta)^2 (-2 x^6 (-1 + \eta)^6 \theta p (3 + 8 \eta^2 - 3 \theta l - 11 \mu_1 + 7 \theta l \mu_1 + \eta \\
& (-11 + 4 \theta l - 4 \eta t (1 + \theta l) + 11 \mu_1) + \theta l \mu_2 + \eta t (4 - \theta l (-3 + 7 \mu_1 + \mu_2))) + \\
& x^5 (-1 + \eta)^5 (2 \times (-1 + \eta) \theta p (-2 + 48 \eta^2 + 26 \mu_1 + 10 \mu_2 + \\
& \eta t (-8 + 7 \mu_2) - 2 \eta (1 + 12 \eta t - 33 \mu_1 + 7 \mu_2)) - (-1 + \eta t) \\
& \theta l (-4 + 48 \eta^2 \theta p + 16 \theta p \mu_2 + \theta p \mu_1 + 5 \theta p \mu_2 - 10 \theta p \mu_2 \mu_2 + \\
& \eta (-28 \mu_1 + 7 \theta p \mu_1 (14 + \mu_1 + \mu_2) + 4 \theta p (-5 + 3 \mu_2)) + \\
& \mu_1 (-12 + \theta p (44 - 11 \mu_1 + 3 \mu_2))) + \\
& \eta \theta p (-16 \eta^7 + 4 \eta t \mu_2 + 2 \eta^6 (-5 - 4 \theta l + 4 \eta t (1 + \theta l) - 11 \mu_1 + 14 \mu_2) + \\
& \eta^5 (14 - 30 \mu_1 - 8 \mu_2 - 2 \theta l (5 + \mu_2) - 7 \theta l \mu_1 (4 + \mu_1 + \mu_2) + \\
& \eta t (8 - 28 \mu_1 - 14 \mu_2 + 2 \theta l (5 + \mu_2) + 7 \theta l \mu_1 (4 + \mu_1 + \mu_2))) + \eta^2 \\
& (4 \times (5 + 5 \mu_1 + 6 \mu_2) - \theta l (12 - 10 \mu_1 (-1 + \mu_1) + 5 \mu_1 + \\
& 2 \mu_2 (8 + 3 \mu_1 - 4 \mu_2) + \mu_2) + \eta t (4 - 4 \mu_2 + \\
& \theta l (12 - 10 \mu_1 (-1 + \mu_1) + 5 \mu_1 + 2 \mu_2 (8 + 3 \mu_1 - 4 \mu_2) + \mu_2))) + \\
& \eta^4 (-4 \eta t (3 + 7 \mu_1) + 2 \times (-5 + \mu_1 - 40 \mu_2) - \theta l (8 + \mu_1 + 5 \mu_2 - \\
& 2 \mu_2 (-6 + 5 \mu_2) + 2 \mu_1 (33 + 7 \mu_2)) + \\
& \eta t \theta l (8 + \mu_1 + 5 \mu_2 - 2 \mu_2 (-6 + 5 \mu_2) + 2 \mu_1 (33 + 7 \mu_2))) +
\end{aligned}$$

$$\begin{aligned}
& \eta^3 (2 + 30 \mu_1 + 70 \eta t \mu_1 + 36 \mu_2 + 10 \eta t \mu_2 + (-1 + \eta t) \theta l \\
& \quad (18 + 4 \mathfrak{e}1 + \mu_2 (26 + 3 \mathfrak{e}1 - 19 \mathfrak{e}2) + 4 \mathfrak{e}2 + \mu_1 (48 - 19 \mathfrak{e}1 + 7 \mathfrak{e}2))) + \eta \\
& \quad (-\theta l (2 \times (1 + \mu_1) \mathfrak{e}1 + \mu_2 (2 + 3 \mathfrak{e}1 + \mathfrak{e}2)) + \eta t (-8 + 2 \theta l \mathfrak{e}1 + \\
& \quad 2 \mu_1 (-7 + \theta l \mathfrak{e}1) + \mu_2 (4 + \theta l (2 + 3 \mathfrak{e}1 + \mathfrak{e}2)))) + \\
& x^2 (-1 + \eta)^2 (-2 \times (-1 + \eta) \theta p (120 \eta^5 + \eta t (-7 - 8 \mu_1 + \mu_2) - \\
& \quad 5 \eta^4 (-23 + 12 \eta t - 33 \mu_1 + 28 \mu_2) + \\
& \quad \eta (30 + 30 \mu_1 + 44 \mu_2 + \eta t (-9 - 20 \mu_1 + 3 \mu_2)) + \\
& \quad 6 \eta^2 (11 + 25 \mu_1 + 34 \mu_2 + \eta t (-2 + 20 \mu_1 + 7 \mu_2)) + \\
& \quad \eta^3 (4 \times (7 + 65 \mu_1 - 5 \mu_2) + \eta t (-80 + 84 \mu_1 + 70 \mu_2))) + (-1 + \eta t) \theta l \\
& \quad (120 \eta^5 \theta p + 2 \times (3 + 3 \mu_1 + \mu_2) - \theta p (6 + \mathfrak{e}1 + 3 \mathfrak{e}2 + 2 \mu_2 (2 + \mathfrak{e}2) + \\
& \quad \mu_1 (6 + \mathfrak{e}1 + 3 \mathfrak{e}2)) - 2 \eta^3 (8 + 72 \mu_1 + \theta p (-24 - 68 \mu_2 - \\
& \quad 5 \mathfrak{e}1 + \mu_1 (-286 + 22 \mathfrak{e}1 - 48 \mathfrak{e}2) - 25 \mathfrak{e}2 + 50 \mu_2 \mathfrak{e}2)) + \\
& \quad 2 \eta^4 (-56 \mu_1 + 5 \theta p (7 + 3 \mathfrak{e}2 + 7 \mu_1 (5 + \mathfrak{e}1 + \mathfrak{e}2))) + \\
& \quad \eta (2 \times (17 + 23 \mu_1 + \mu_2) + \theta p (\mu_2 (32 + 6 \mathfrak{e}1 - 36 \mathfrak{e}2) + 3 \times (4 + \mathfrak{e}1 - 3 \mathfrak{e}2) - \\
& \quad 6 \mu_1 (-3 + 6 \mathfrak{e}1 + \mathfrak{e}2))) + \eta^2 (24 + 92 \mu_1 + 3 \theta p (\mu_2 (54 + 3 \mathfrak{e}1 - \\
& \quad 41 \mathfrak{e}2) + 5 \times (6 + \mathfrak{e}1 + \mathfrak{e}2) + \mu_1 (88 - 42 \mathfrak{e}1 + 10 \mathfrak{e}2)))) - \\
& x^3 (-1 + \eta)^3 (-((-1 + \eta) \theta p (320 \eta^4 + \eta t (-7 - 13 \mu_1 + \mu_2) - 40 \eta^3 \\
& \quad (-5 + 4 \eta t - 11 \mu_1 + 7 \mu_2) + 4 \times (5 + 5 \mu_1 + 8 \mu_2) + \\
& \quad 8 \eta (11 + 25 \mu_1 + 36 \mu_2 + \eta t (-2 + 16 \mu_1 + 7 \mu_2)) + 4 \eta^2 \\
& \quad (2 \times (3 + 65 \mu_1 + 5 \mu_2) + \eta t (-40 + 28 \mu_1 + 35 \mu_2)))) + (-1 + \eta t) \theta l \\
& \quad (20 + 160 \eta^4 \theta p + 4 \mu_2 + 8 \theta p \mu_2 - \theta p \mathfrak{e}1 + \mu_1 (24 + \theta p (4 - 13 \mathfrak{e}1 - 3 \mathfrak{e}2)) - \\
& \quad 5 \theta p \mathfrak{e}2 - 14 \theta p \mu_2 \mathfrak{e}2 - 2 \eta^2 (12 + 84 \mu_1 + \theta p (-16 - 72 \mu_2 - \\
& \quad 5 \mathfrak{e}1 + \mu_1 (-264 + 33 \mathfrak{e}1 - 37 \mathfrak{e}2) - 25 \mathfrak{e}2 + 50 \mu_2 \mathfrak{e}2)) + \\
& \quad 2 \eta^3 (-84 \mu_1 + 5 \theta p (4 \times (1 + \mathfrak{e}2) + 7 \mu_1 (6 + \mathfrak{e}1 + \mathfrak{e}2))) + \\
& \quad \eta (27 + 91 \mu_1 + 3 \mu_2 + \theta p (54 + 7 \mathfrak{e}1 + \mu_2 (110 + 3 \mathfrak{e}1 - 85 \mathfrak{e}2) + \\
& \quad 7 \mathfrak{e}2 + \mu_1 (168 - 88 \mathfrak{e}1 + 16 \mathfrak{e}2)))) + \\
& x^4 (-1 + \eta)^4 (-2 \times (-1 + \eta) \theta p (11 + 120 \eta^3 + 25 \mu_1 + 38 \mu_2 + \eta t \\
& \quad (-2 + 12 \mu_1 + 7 \mu_2) - 5 \eta^2 (-7 + 12 \eta t - 33 \mu_1 + 14 \mu_2) + \\
& \quad \eta (-2 + 130 \mu_1 + 30 \mu_2 + \eta t (-40 + 14 \mu_1 + 35 \mu_2))) + \\
& \quad (-1 + \eta t) \theta l (120 \eta^3 \theta p + 2 \times (5 + 15 \mu_1 + \mu_2) + \theta p \\
& \quad (12 + 28 \mu_2 + \mathfrak{e}1 + \mathfrak{e}2 - 22 \mu_2 \mathfrak{e}2 + \mu_1 (40 - 23 \mathfrak{e}1 + 3 \mathfrak{e}2)) + \\
& \quad \eta^2 (-112 \mu_1 + 5 \theta p (-2 + 6 \mathfrak{e}2 + 7 \mu_1 (8 + \mathfrak{e}1 + \mathfrak{e}2))) + \\
& \quad \eta (-16 \times (1 + 5 \mu_1) + \theta p (8 + 76 \mu_2 + 5 \mathfrak{e}1 + 25 \mathfrak{e}2 - \\
& \quad 50 \mu_2 \mathfrak{e}2 + \mu_1 (242 - 44 \mathfrak{e}1 + 26 \mathfrak{e}2)))) + \\
& x (-1 + \eta) \times (96 \eta^7 \theta p + \eta t \theta p (3 + 3 \mu_1 - \mu_2) - 4 \eta^6 \theta p (-7 - 12 \theta l + \\
& \quad 12 \eta t (1 + \theta l) - 33 \mu_1 + 35 \mu_2) + \eta^4 \\
& \quad (2 \theta p (22 - 30 \mu_1 + \eta t (32 + 40 \mu_1 - 7 \mu_2) + 158 \mu_2) + \\
& \quad (-1 + \eta t) \theta l (4 + 44 \mu_1 + \theta p (-32 - 64 \mu_2 - 5 \mathfrak{e}1 + \\
& \quad \mu_1 (-308 + 11 \mathfrak{e}1 - 59 \mathfrak{e}2) - 25 \mathfrak{e}2 + 50 \mu_2 \mathfrak{e}2))) + \eta^2 \\
& \quad (\theta p (\eta t (-7 + 11 \mu_1 + \mu_2) - 20 \times (3 + 3 \mu_1 + 4 \mu_2)) + (-1 + \eta t) \\
& \quad \theta l (2 \times (-7 - 11 \mu_1 + \mu_2) + \theta p (-2 \mu_2 (20 + 6 \mathfrak{e}1 - 15 \mathfrak{e}2) + \\
& \quad 3 \times (-8 - 3 \mathfrak{e}1 + \mathfrak{e}2) + 3 \mu_1 (-8 + 11 \mathfrak{e}1 + \mathfrak{e}2)))) + \eta^3 \\
& \quad (-\theta p (4 \times (7 + 35 \mu_1 + 44 \mu_2) + \eta t (-1 + 233 \mu_1 + 47 \mu_2)) + \\
& \quad (-1 + \eta t) \theta l (-7 - 31 \mu_1 + \mu_2 - \theta p (66 + 13 \mathfrak{e}1 + \mu_2 (106 + 9 \mathfrak{e}1 - 79 \mathfrak{e}2) + \\
& \quad 13 \mathfrak{e}2 + \mu_1 (184 - 80 \mathfrak{e}1 + 24 \mathfrak{e}2)))) + \eta
\end{aligned}$$

$$\begin{aligned}
& \left( \eta t \, \theta p \, (19 + 27 \mu 1 - 9 \mu 2) - (-1 + \eta t) \, \theta l \, (3 + 3 \mu 1 - \mu 2 + \right. \\
& \quad \left. \theta p \, (-6 + \mathfrak{x} 1 + \mu 2 \, (-2 + 3 \mathfrak{x} 1 - \mathfrak{x} 2) - 3 \mathfrak{x} 2 + \mu 1 \, (\mathfrak{x} 1 - 3 \times (2 + \mathfrak{x} 2)))) + \right. \\
& \quad \left. \eta^5 \, (28 \times (-1 + \eta t) \, \theta l \, \mu 1 + \theta p \, (16 \times (-5 + 8 \mu 1 + 5 \mu 2) + \theta l \, \right. \\
& \quad \left. (44 + 12 \mathfrak{x} 2 + 7 \mu 1 \, (22 + 5 \mathfrak{x} 1 + 5 \mathfrak{x} 2)) - \eta t \, (32 - 112 \mu 1 - \right. \\
& \quad \left. 70 \mu 2 + \theta l \, (44 + 12 \mathfrak{x} 2 + 7 \mu 1 \, (22 + 5 \mathfrak{x} 1 + 5 \mathfrak{x} 2)))))) \right) / \\
& \left( 24 \, c v \, (-1 + w \, (-1 + \eta))^3 \, (x \, (-1 + \eta) - \eta)^3 \, (1 + x + \eta - x \eta)^2 \right. \\
& \quad (w + \\
& \quad x + \\
& \quad \eta - \\
& \quad w \eta - \\
& \quad \left. x \eta)^3 \, (-1 + \eta t) \, \theta p) \right) \\
\delta \chi_s = & \\
& - \left( (f \, w \, (-1 + \eta)^2 \, (2 \, x^2 \, (2 \, w \, (-1 + \eta) - 3 \eta) \, (-1 + \eta)^2 \, (-1 + \eta + \theta l - \eta t \, \theta l) \, \theta p \, (1 + 7 \mu 1) + 2 \, x^3 \right. \\
& \quad \left. (-1 + \eta)^3 \, (-1 + \eta + \theta l - \eta t \, \theta l) \, \theta p \, (1 + 7 \mu 1) + \right. \\
& \quad x \, (-1 + \eta) \times (2 \times (-1 + \eta) \, (w^2 \, (-1 + \eta)^2 - 4 \, w \, (-1 + \eta) \, \eta + 3 \eta^2) \, \theta p \, (1 + 7 \mu 1) - \\
& \quad \left. (-1 + \eta t) \, \theta l \, (2 - 2 \, \theta p + 6 \eta^2 \, \theta p - 10 \mu 1 + 10 \, \theta p \, \mu 1 + \right. \\
& \quad \left. 42 \eta^2 \, \theta p \, \mu 1 - \theta p \, \mathfrak{x} 1 + 5 \, \theta p \, \mu 1 \, \mathfrak{x} 1 - \theta p \, \mathfrak{x} 2 + 5 \, \theta p \, \mu 1 \, \mathfrak{x} 2 - \right. \\
& \quad \left. 2 \, w \, (-1 + \eta) \times (2 - 10 \mu 1 + 4 \eta \, \theta p \, (1 + 7 \mu 1) + \theta p \, (-1 + 5 \mu 1) \times (2 + \mathfrak{x} 1 + \mathfrak{x} 2)) + \right. \\
& \quad \left. w^2 \, (-1 + \eta)^2 \, (2 - \theta p \, (\mathfrak{x} 1 + \mathfrak{x} 2) + \mu 1 \, (-10 + \theta p \, (24 + 5 \mathfrak{x} 1 + 5 \mathfrak{x} 2)))) \right) + \\
& \theta p \, (2 \eta^3 - 2 \eta^4 - 2 \eta t + 2 \eta \eta t + 2 \eta \theta l - 2 \eta^3 \theta l - 2 \eta \eta t \theta l + 2 \eta^3 \eta t \theta l + \\
& \quad 14 \eta^3 \mu 1 - 14 \eta^4 \mu 1 + 10 \eta t \mu 1 - 10 \eta \eta t \mu 1 - 10 \eta \theta l \mu 1 - 14 \eta^3 \theta l \mu 1 + \\
& \quad 10 \eta \eta t \theta l \mu 1 + 14 \eta^3 \eta t \theta l \mu 1 + \eta \theta l \mathfrak{x} 1 - \eta \eta t \theta l \mathfrak{x} 1 - 5 \eta \theta l \mu 1 \mathfrak{x} 1 + \\
& \quad 5 \eta \eta t \theta l \mu 1 \mathfrak{x} 1 + \eta \theta l \mathfrak{x} 2 - \eta \eta t \theta l \mathfrak{x} 2 - 5 \eta \theta l \mu 1 \mathfrak{x} 2 + 5 \eta \eta t \theta l \mu 1 \mathfrak{x} 2 + \\
& \quad 2 \, w \, (-1 + \eta) \times (2 \eta t \, (1 - 5 \mu 1) + 2 \eta^3 \, (1 + 7 \mu 1) - 2 \eta^2 \, (1 + (-1 + \eta t) \, \theta l) \times \\
& \quad \left. (1 + 7 \mu 1) - \eta \, (-1 + 5 \mu 1) \, (-\theta l \, (2 + \mathfrak{x} 1 + \mathfrak{x} 2) + \eta t \, (-2 + \theta l \, (2 + \mathfrak{x} 1 + \mathfrak{x} 2)))) \right) - \\
& \quad w^2 \, (-1 + \eta)^2 \, (2 \eta t \, (1 - 5 \mu 1) + 2 \eta^2 \, (1 + 7 \mu 1) - \eta \, (2 + 14 \mu 1 + \\
& \quad \theta l \mathfrak{x} 1 + \theta l \mathfrak{x} 2 - \theta l \mu 1 \, (24 + 5 \mathfrak{x} 1 + 5 \mathfrak{x} 2) + \\
& \quad \eta t \, (2 - \theta l \, (\mathfrak{x} 1 + \mathfrak{x} 2) + \mu 1 \, (-10 + \theta l \, (24 + 5 \mathfrak{x} 1 + 5 \mathfrak{x} 2)))))) / \\
& \left( 24 \, (-1 + w \, (-1 + \eta))^2 \, (x \, (-1 + \eta) - \eta) \, (w \, (-1 + \eta) + x \, (-1 + \eta) - \eta)^2 \right. \\
& \quad (-1 + \eta t) \\
& \quad \left. \theta p) \right)
\end{aligned}$$

$$\begin{aligned}
\delta\gamma_{S1} = & \left( f w (-1 + \eta)^2 \left( 2 x^2 (2 w (-1 + \eta) - 3 \eta) (-1 + \eta)^2 (-1 + \eta + \theta l - \eta t \theta l) \theta p (-7 + 5 \mu 1) + \right. \right. \\
& 2 x^3 (-1 + \eta)^3 (-1 + \eta + \theta l - \eta t \theta l) \theta p (-7 + 5 \mu 1) + \\
& x (-1 + \eta) \times \left( 2 \times (-1 + \eta) \left( w^2 (-1 + \eta)^2 - 4 w (-1 + \eta) \eta + 3 \eta^2 \right) \theta p (-7 + 5 \mu 1) - \right. \\
& (-1 + \eta t) \theta l \left( 10 - 10 \theta p - 42 \eta^2 \theta p - 14 \mu 1 + 14 \theta p \mu 1 + \right. \\
& 30 \eta^2 \theta p \mu 1 - 5 \theta p \mathfrak{x} 1 + 7 \theta p \mu 1 \mathfrak{x} 1 - 5 \theta p \mathfrak{x} 2 + 7 \theta p \mu 1 \mathfrak{x} 2 - \\
& 2 w (-1 + \eta) \times (10 - 14 \mu 1 + 4 \eta \theta p (-7 + 5 \mu 1) + \theta p (-5 + 7 \mu 1) \times (2 + \mathfrak{x} 1 + \mathfrak{x} 2)) + \\
& w^2 (-1 + \eta)^2 (10 - 14 \mu 1 + \theta p (-24 - 5 \mathfrak{x} 1 - 5 \mathfrak{x} 2 + \mu 1 (24 + 7 \mathfrak{x} 1 + 7 \mathfrak{x} 2))) \left. \right) \left. \right) + \\
& \theta p \left( -14 \eta^3 + 14 \eta^4 - 10 \eta t + 10 \eta \eta t + 10 \eta \theta l + 14 \eta^3 \theta l - 10 \eta \eta t \theta l - 14 \eta^3 \eta t \theta l + \right. \\
& 10 \eta^3 \mu 1 - 10 \eta^4 \mu 1 + 14 \eta t \mu 1 - 14 \eta \eta t \mu 1 - 14 \eta \theta l \mu 1 - 10 \eta^3 \theta l \mu 1 + \\
& 14 \eta \eta t \theta l \mu 1 + 10 \eta^3 \eta t \theta l \mu 1 + 5 \eta \theta l \mathfrak{x} 1 - 5 \eta \eta t \theta l \mathfrak{x} 1 - 7 \eta \theta l \mu 1 \mathfrak{x} 1 + \\
& 7 \eta \eta t \theta l \mu 1 \mathfrak{x} 1 + 5 \eta \theta l \mathfrak{x} 2 - 5 \eta \eta t \theta l \mathfrak{x} 2 - 7 \eta \theta l \mu 1 \mathfrak{x} 2 + 7 \eta \eta t \theta l \mu 1 \mathfrak{x} 2 + \\
& 2 w (-1 + \eta) \times \left( 2 \eta t (5 - 7 \mu 1) + 2 \eta^3 (-7 + 5 \mu 1) - 2 \eta^2 (1 + (-1 + \eta t) \theta l) \times \right. \\
& (-7 + 5 \mu 1) - \eta (-5 + 7 \mu 1) (-\theta l (2 + \mathfrak{x} 1 + \mathfrak{x} 2) + \eta t (-2 + \theta l (2 + \mathfrak{x} 1 + \mathfrak{x} 2))) \left. \right) \times \\
& w^2 (-1 + \eta)^2 \left( 2 \eta t (5 - 7 \mu 1) + 2 \eta^2 (-7 + 5 \mu 1) + \right. \\
& \eta (14 - 10 \mu 1 + \theta l (-24 - 5 \mathfrak{x} 1 - 5 \mathfrak{x} 2 + \mu 1 (24 + 7 \mathfrak{x} 1 + 7 \mathfrak{x} 2)) + \eta t \\
& (2 \times (-5 + 7 \mu 1) + \theta l (24 + 5 \mathfrak{x} 1 + 5 \mathfrak{x} 2 - \mu 1 (24 + 7 \mathfrak{x} 1 + 7 \mathfrak{x} 2)))) \left. \right) \left. \right) \left. \right) / \\
& (48 (-1 + w (-1 + \eta))^2 (x (-1 + \eta) - \eta) (w (-1 + \eta) + x (-1 + \eta) - \eta)^2 \\
& (-1 + \eta t) \\
& \theta p \\
& \mu 1)
\end{aligned}$$

$\delta\gamma_{S2} -$

$$\begin{aligned}
& \left( (f w (-1 + \eta)^2 \left( 2 x^2 (2 w (-1 + \eta) - 3 \eta) (-1 + \eta)^2 (-1 + \eta + \theta l - \eta t \theta l) \theta p (1 + \mu 1 + 12 \mu 2) + \right. \right. \\
& 2 x^3 (-1 + \eta)^3 (-1 + \eta + \theta l - \eta t \theta l) \theta p (1 + \mu 1 + 12 \mu 2) + \\
& x (-1 + \eta) \times \left( 2 \times (-1 + \eta) \left( w^2 (-1 + \eta)^2 - 4 w (-1 + \eta) \eta + 3 \eta^2 \right) \theta p (1 + \mu 1 + 12 \mu 2) + \right. \\
& (-1 + \eta t) \theta l \left( -2 + 2 \theta p - 6 \eta^2 \theta p - 2 \mu 1 + 2 \theta p \mu 1 - 6 \eta^2 \theta p \mu 1 - \right. \\
& 72 \eta^2 \theta p \mu 2 + \theta p \mathfrak{x} 1 + \theta p \mu 1 \mathfrak{x} 1 + \theta p \mathfrak{x} 2 + \theta p \mu 1 \mathfrak{x} 2 + 2 w (-1 + \eta) \times \\
& (2 \times (1 + \mu 1) + 4 \eta \theta p (1 + \mu 1 + 12 \mu 2) - \theta p (1 + \mu 1) \times (2 + \mathfrak{x} 1 + \mathfrak{x} 2)) + \\
& w^2 (-1 + \eta)^2 (-2 + \theta p (-24 \mu 2 + \mathfrak{x} 1 + \mathfrak{x} 2) + \mu 1 (-2 + \theta p (\mathfrak{x} 1 + \mathfrak{x} 2))) \left. \right) \left. \right) + \\
& \theta p \left( 2 \eta^3 - 2 \eta^4 - 2 \eta t + 2 \eta \eta t + 2 \eta \theta l - 2 \eta^3 \theta l - 2 \eta \eta t \theta l + 2 \eta^3 \eta t \theta l + 2 \eta^3 \mu 1 - \right. \\
& 2 \eta^4 \mu 1 - 2 \eta t \mu 1 + 2 \eta \eta t \mu 1 + 2 \eta \theta l \mu 1 - 2 \eta^3 \theta l \mu 1 - 2 \eta \eta t \theta l \mu 1 + 2 \eta^3 \eta t \theta l \mu 1 + \\
& 24 \eta^3 \mu 2 - 24 \eta^4 \mu 2 - 24 \eta^3 \theta l \mu 2 + 24 \eta^3 \eta t \theta l \mu 2 + \eta \theta l \mathfrak{x} 1 - \eta \eta t \theta l \mathfrak{x} 1 + \eta \theta l \mu 1 \mathfrak{x} 1 - \\
& \eta \eta t \theta l \mu 1 \mathfrak{x} 1 + \eta \theta l \mathfrak{x} 2 - \eta \eta t \theta l \mathfrak{x} 2 + \eta \theta l \mu 1 \mathfrak{x} 2 - \eta \eta t \theta l \mu 1 \mathfrak{x} 2 + 2 w (-1 + \eta) \times \\
& (2 \eta t (1 + \mu 1) + 2 \eta^3 (1 + \mu 1 + 12 \mu 2) - 2 \eta^2 (1 + (-1 + \eta t) \theta l) \times (1 + \mu 1 + 12 \mu 2) + \\
& \eta (1 + \mu 1) (-\theta l (2 + \mathfrak{x} 1 + \mathfrak{x} 2) + \eta t (-2 + \theta l (2 + \mathfrak{x} 1 + \mathfrak{x} 2))) \left. \right) - \\
& w^2 (-1 + \eta)^2 \left( 2 \eta t (1 + \mu 1) + 2 \eta^2 (1 + \mu 1 + 12 \mu 2) + \right. \\
& \eta (-2 - 24 \mu 2 + 24 \theta l \mu 2 - \theta l \mathfrak{x} 1 - \theta l \mathfrak{x} 2 - \mu 1 (2 + \theta l (\mathfrak{x} 1 + \mathfrak{x} 2)) + \\
& \eta t (-2 + \theta l (-24 \mu 2 + \mathfrak{x} 1 + \mathfrak{x} 2) + \mu 1 (-2 + \theta l (\mathfrak{x} 1 + \mathfrak{x} 2)))) \left. \right) \left. \right) \left. \right) / \\
& (48 (-1 + w (-1 + \eta))^2 (x (-1 + \eta) - \eta) (w (-1 + \eta) + x (-1 + \eta) - \eta)^2 \\
& (-1 + \eta t) \\
& \theta p \\
& \mu 2)
\end{aligned}$$

$\delta J =$

$$- \left( (4 c v c \sigma f w (-1 + \eta)^3 \left( x^2 (-1 + \eta)^2 + \eta (1 + \eta) + x (1 + \eta - 2 \eta^2) \right) \left( 4 x^5 (-1 + \eta)^5 (-1 + \eta + \right. \right.$$



$$\begin{aligned}
& \theta l - \eta t \theta l) \theta p + x^4 (-1 + \eta)^4 (4 \times (-1 + w (-1 + \eta)) \times (-1 + \eta t) \theta l \mu 1 + \\
& \theta p (4 + 16 \eta - 20 \eta^2 - 4 \theta l - 20 \eta \theta l + 4 \eta t \theta l + 20 \eta \eta t \theta l - 2 \theta l \mu 1 + 2 \eta t \theta l \mu 1 - \\
& 2 \theta l \mu 2 + 2 \eta t \theta l \mu 2 - \theta l \mu 1 \mathfrak{x} 1 + \eta t \theta l \mu 1 \mathfrak{x} 1 - \theta l \mu 1 \mathfrak{x} 2 + \eta t \theta l \mu 1 \mathfrak{x} 2 + w \\
& (-1 + \eta) \times (-12 + 12 \eta - (-1 + \eta t) \theta l (2 \times (6 + \mu 2) + \mu 1 (2 + \mathfrak{x} 1 + \mathfrak{x} 2)))))) + \\
& \theta p (-3 w^2 (-1 + \eta)^2 (1 + \eta) \times (4 \eta^3 - 6 \eta t (1 + \mu 1 + \mu 2) + \eta^2 \\
& (4 \times (-1 + \eta t \mu 1 + \mu 2) - (-1 + \eta t) \theta l (2 \times (2 + \mu 2) + \mu 1 (2 + \mathfrak{x} 1 + \mathfrak{x} 2))) + \eta \\
& (-4 \mu 2 + 2 \eta t (3 + \mu 1 + 3 \mu 2) + \\
& \theta l (3 \times (2 + \mathfrak{x} 1 + \mathfrak{x} 2) + 4 \mu 1 (2 + \mathfrak{x} 1 + \mathfrak{x} 2) + \mu 2 (8 + 3 \mathfrak{x} 1 + 3 \mathfrak{x} 2)) - \\
& \eta t \theta l (3 \times (2 + \mathfrak{x} 1 + \mathfrak{x} 2) + 4 \mu 1 (2 + \mathfrak{x} 1 + \mathfrak{x} 2) + \mu 2 (8 + 3 \mathfrak{x} 1 + 3 \mathfrak{x} 2)))) + \\
& w^3 (-1 + \eta)^3 (4 \eta^3 - 6 \eta t (1 + \mu 1 + \mu 2) - \eta (4 + 8 \eta t \mu 1 + 8 \mu 2 + \\
& (-1 + \eta t) \theta l (5 \mu 1 (2 + \mathfrak{x} 1 + \mathfrak{x} 2) + (1 + \mu 2) \times (10 + 3 \mathfrak{x} 1 + 3 \mathfrak{x} 2))) + \eta^2 \\
& (8 \mu 2 + 5 \theta l \mu 1 (2 + \mathfrak{x} 1 + \mathfrak{x} 2) + \theta l (1 + \mu 2) \times (10 + 3 \mathfrak{x} 1 + 3 \mathfrak{x} 2) - \\
& \eta t (-2 \times (3 + 7 \mu 1 + 3 \mu 2) + 5 \theta l \mu 1 (2 + \mathfrak{x} 1 + \mathfrak{x} 2) + \\
& \theta l (1 + \mu 2) \times (10 + 3 \mathfrak{x} 1 + 3 \mathfrak{x} 2)))) + \\
& w (-1 + \eta) \times (12 \eta^5 - 18 \eta t (1 + \mu 1 + \mu 2) + \eta^4 (4 (\eta t \mu 1 + \mu 2) - (-1 + \eta t) \\
& \theta l (2 \times (6 + \mu 2) + \mu 1 (2 + \mathfrak{x} 1 + \mathfrak{x} 2))) + \eta^3 (12 \times (-1 + \eta t \mu 1 + \mu 2) - \\
& (-1 + \eta t) \theta l (2 \times (6 + 5 \mu 2) + 5 \mu 1 (2 + \mathfrak{x} 1 + \mathfrak{x} 2))) - \eta \\
& (4 (\eta t \mu 1 + \mu 2) + (-1 + \eta t) \theta l (9 \times (2 + \mathfrak{x} 1 + \mathfrak{x} 2) + 10 \mu 1 (2 + \mathfrak{x} 1 + \mathfrak{x} 2) + \\
& \mu 2 (20 + 9 \mathfrak{x} 1 + 9 \mathfrak{x} 2))) + \eta^2 (-12 \mu 2 + 6 \eta t (3 + \mu 1 + 3 \mu 2) + \\
& \theta l (9 \times (2 + \mathfrak{x} 1 + \mathfrak{x} 2) + 14 \mu 1 (2 + \mathfrak{x} 1 + \mathfrak{x} 2) + \mu 2 (28 + 9 \mathfrak{x} 1 + 9 \mathfrak{x} 2)) - \\
& \eta t \theta l (9 \times (2 + \mathfrak{x} 1 + \mathfrak{x} 2) + 14 \mu 1 (2 + \mathfrak{x} 1 + \mathfrak{x} 2) + \mu 2 (28 + 9 \mathfrak{x} 1 + 9 \mathfrak{x} 2)))) - \\
& (1 + \eta) \times (4 \eta^5 - 4 \eta^4 (1 + (-1 + \eta t) \theta l) - 6 \eta t (1 + \mu 1 + \mu 2) - 3 \eta \\
& (1 + \mu 1 + \mu 2) (-\theta l (2 + \mathfrak{x} 1 + \mathfrak{x} 2) + \eta t (-2 + \theta l (2 + \mathfrak{x} 1 + \mathfrak{x} 2)))) - \eta^2 \\
& (4 \mu 2 - 2 \theta l \mu 2 + 2 \eta t \theta l \mu 2 - \theta l \mu 1 (2 + \mathfrak{x} 1 + \mathfrak{x} 2) + \\
& \eta t \mu 1 (4 + \theta l (2 + \mathfrak{x} 1 + \mathfrak{x} 2))) + \eta^3 (4 \mu 2 + 2 \theta l \mu 2 + \\
& \theta l \mu 1 (2 + \mathfrak{x} 1 + \mathfrak{x} 2) - \eta t (2 \theta l \mu 2 + \mu 1 (-4 + \theta l (2 + \mathfrak{x} 1 + \mathfrak{x} 2)))))) + \\
& x^3 (-1 + \eta)^3 (40 \eta^3 \theta p - 8 \eta^2 (3 + 5 \times (-1 + \eta t) \theta l) \theta p - 4 \theta p (\eta t \mu 1 + \mu 2) - \\
& 2 \times (-1 + \eta t) \theta l (2 \theta p \mu 2 + \mu 1 (-2 + \theta p (2 + \mathfrak{x} 1 + \mathfrak{x} 2))) + \\
& 3 w^2 (-1 + \eta)^2 (4 \times (-1 + \eta t) \theta l \mu 1 + \theta p (-4 + 4 \eta - (-1 + \eta t) \theta l \\
& (2 \times (2 + \mu 2) + \mu 1 (2 + \mathfrak{x} 1 + \mathfrak{x} 2)))) + 2 \eta (6 \times (-1 + \eta t) \theta l \mu 1 + 2 \theta p \\
& (-4 + \eta t \mu 1 + \mu 2 - (-1 + \eta t) \theta l (2 \times (2 + \mu 2) + \mu 1 (2 + \mathfrak{x} 1 + \mathfrak{x} 2)))) - \\
& w (-1 + \eta) \times (4 \times (4 + 3 \eta) \times (-1 + \eta t) \theta l \mu 1 + \theta p (48 \eta^2 - 4 \times (3 + \eta t \mu 1 + \mu 2) - \\
& (-1 + \eta t) \theta l (2 \times (6 + 5 \mu 2) + 5 \mu 1 (2 + \mathfrak{x} 1 + \mathfrak{x} 2))) - \\
& 4 \eta (9 - \eta t \mu 1 - \mu 2 + (-1 + \eta t) \theta l (2 \times (6 + \mu 2) + \mu 1 (2 + \mathfrak{x} 1 + \mathfrak{x} 2)))))) + \\
& x^2 (-1 + \eta)^2 (4 \times (-1 + \eta) \theta p (w^3 (-1 + \eta)^3 - 6 \eta^2 - 10 \eta^3 - \eta t \mu 1 - 3 \eta \eta t \\
& \mu 1 - \mu 2 - 3 \eta \mu 2 - 3 w^2 (-1 + \eta)^2 (1 + 3 \eta + \eta t \mu 1 + \mu 2) + w (-1 + \eta) \times \\
& (18 \eta^2 + 4 (\eta t \mu 1 + \mu 2) + 3 \eta (3 + \eta t \mu 1 + \mu 2))) - (-1 + \eta t) \theta l \\
& (6 - 6 \theta p - 24 \eta^2 \theta p - 40 \eta^3 \theta p + 6 \mu 1 + 8 \eta \mu 1 + 12 \eta^2 \mu 1 - 8 \theta p \mu 1 - 12 \eta \theta p \\
& \mu 1 - 12 \eta^2 \theta p \mu 1 + 6 \mu 2 - 8 \theta p \mu 2 - 12 \eta \theta p \mu 2 - 12 \eta^2 \theta p \mu 2 - 3 \theta p \mathfrak{x} 1 - 4 \theta p \\
& \mu 1 \mathfrak{x} 1 - 6 \eta \theta p \mu 1 \mathfrak{x} 1 - 6 \eta^2 \theta p \mu 1 \mathfrak{x} 1 - 3 \theta p \mu 2 \mathfrak{x} 1 - 3 \theta p \mathfrak{x} 2 - 4 \theta p \mu 1 \mathfrak{x} 2 - 6 \eta \\
& \theta p \mu 1 \mathfrak{x} 2 - 6 \eta^2 \theta p \mu 1 \mathfrak{x} 2 - 3 \theta p \mu 2 \mathfrak{x} 2 + w^3 (-1 + \eta)^3 (-2 \times (3 + 7 \mu 1 + 3 \mu 2) + \\
& 5 \theta p \mu 1 (2 + \mathfrak{x} 1 + \mathfrak{x} 2) + \theta p (1 + \mu 2) \times (10 + 3 \mathfrak{x} 1 + 3 \mathfrak{x} 2)) - 3 w^2 (-1 + \eta)^2 \\
& (-2 \times (3 + 5 \mu 1 + 4 \eta \mu 1 + 3 \mu 2) + \theta p (6 \eta (2 + \mu 2) + 5 \mu 1 (2 + \mathfrak{x} 1 + \mathfrak{x} 2) + \\
& 3 \eta \mu 1 (2 + \mathfrak{x} 1 + \mathfrak{x} 2) + (1 + \mu 2) \times (10 + 3 \mathfrak{x} 1 + 3 \mathfrak{x} 2))) + w (-1 + \eta) \times \\
& (-2 \times ((11 + 16 \eta + 6 \eta^2) \mu 1 + 9 \times (1 + \mu 2)) + \theta p (18 + 28 \mu 2 + 9 \mathfrak{x} 1 +
\end{aligned}$$

$$\begin{aligned}
& 9 \mu_2 \mathfrak{e}_1 + 9 \mathfrak{e}_2 + 9 \mu_2 \mathfrak{e}_2 + 14 \mu_1 (2 + \mathfrak{e}_1 + \mathfrak{e}_2) + 6 \eta^2 (2 \times (6 + \mu_2) + \\
& \mu_1 (2 + \mathfrak{e}_1 + \mathfrak{e}_2)) + 3 \eta (2 \times (6 + 5 \mu_2) + 5 \mu_1 (2 + \mathfrak{e}_1 + \mathfrak{e}_2))) \Big) \Big) - \\
& \times (-1 + \eta) \times \Big( 2 \times (-1 + \eta) \Theta p \Big( -8 \eta^3 - 10 \eta^4 - 3 \eta t - 3 \eta t \mu_1 - 4 \eta \eta t \mu_1 - \\
& 6 \eta^2 \eta t \mu_1 - 4 \eta \mu_2 - 6 \eta^2 \mu_2 - 3 \eta t \mu_2 - 3 w^2 (-1 + \eta)^2 \\
& \Big( 6 \eta^2 + 2 \mu_2 + 4 \eta (1 + \eta t \mu_1 + \mu_2) + \eta t (3 + 5 \mu_1 + 3 \mu_2) \Big) + w^3 (-1 + \eta)^3 \\
& (2 + 4 \eta + 4 \mu_2 + \eta t (3 + 7 \mu_1 + 3 \mu_2)) + w (-1 + \eta) \times \Big( 24 \eta^3 + 2 \mu_2 + \\
& 16 \eta (\eta t \mu_1 + \mu_2) + 6 \eta^2 (3 + \eta t \mu_1 + \mu_2) + \eta t (9 + 11 \mu_1 + 9 \mu_2) \Big) \Big) - \\
& (-1 + \eta t) \Theta l \Big( 6 + 6 \eta - 6 \Theta p - 12 \eta \Theta p - 16 \eta^3 \Theta p - 20 \eta^4 \Theta p + 6 \mu_1 + 6 \\
& \eta \mu_1 + 4 \eta^2 \mu_1 + 4 \eta^3 \mu_1 - 6 \Theta p \mu_1 - 16 \eta \Theta p \mu_1 - 12 \eta^2 \Theta p \mu_1 - 8 \eta^3 \Theta p \\
& \mu_1 + 6 \mu_2 + 6 \eta \mu_2 - 6 \Theta p \mu_2 - 16 \eta \Theta p \mu_2 - 12 \eta^2 \Theta p \mu_2 - 8 \eta^3 \Theta p \mu_2 - 3 \\
& \Theta p \mathfrak{e}_1 - 6 \eta \Theta p \mathfrak{e}_1 - 3 \Theta p \mu_1 \mathfrak{e}_1 - 8 \eta \Theta p \mu_1 \mathfrak{e}_1 - 6 \eta^2 \Theta p \mu_1 \mathfrak{e}_1 - 4 \eta^3 \\
& \Theta p \mu_1 \mathfrak{e}_1 - 3 \Theta p \mu_2 \mathfrak{e}_1 - 6 \eta \Theta p \mu_2 \mathfrak{e}_1 - 3 \Theta p \mathfrak{e}_2 - 6 \eta \Theta p \mathfrak{e}_2 - 3 \Theta p \mu_1 \\
& \mathfrak{e}_2 - 8 \eta \Theta p \mu_1 \mathfrak{e}_2 - 6 \eta^2 \Theta p \mu_1 \mathfrak{e}_2 - 4 \eta^3 \Theta p \mu_1 \mathfrak{e}_2 - 3 \Theta p \mu_2 \mathfrak{e}_2 - 6 \eta \\
& \Theta p \mu_2 \mathfrak{e}_2 + w^3 (-1 + \eta)^3 (-6 \times (1 + \mu_1 + \mu_2) + 5 \Theta p \mu_1 (2 + \mathfrak{e}_1 + \mathfrak{e}_2) + \\
& \Theta p (1 + \mu_2) \times (10 + 3 \mathfrak{e}_1 + 3 \mathfrak{e}_2) + 2 \eta (-3 - 7 \mu_1 - 3 \mu_2 + 5 \Theta p \mu_1 \\
& (2 + \mathfrak{e}_1 + \mathfrak{e}_2) + \Theta p (1 + \mu_2) \times (10 + 3 \mathfrak{e}_1 + 3 \mathfrak{e}_2)) \Big) - 3 w^2 (-1 + \eta)^2 \\
& \Big( -6 \times (1 + \mu_1 + \mu_2) + \eta^2 (-4 \mu_1 + 6 \Theta p (2 + \mu_2) + 3 \Theta p \mu_1 (2 + \mathfrak{e}_1 + \mathfrak{e}_2)) + \\
& \Theta p (3 \times (2 + \mathfrak{e}_1 + \mathfrak{e}_2) + 4 \mu_1 (2 + \mathfrak{e}_1 + \mathfrak{e}_2) + \mu_2 (8 + 3 \mathfrak{e}_1 + 3 \mathfrak{e}_2)) + \\
& 2 \eta (-3 - 5 \mu_1 - 3 \mu_2 + 5 \Theta p \mu_1 (2 + \mathfrak{e}_1 + \mathfrak{e}_2) + \\
& \Theta p (1 + \mu_2) \times (10 + 3 \mathfrak{e}_1 + 3 \mathfrak{e}_2)) \Big) + w (-1 + \eta) \times \\
& \Big( -18 \times (1 + \mu_1 + \mu_2) + 4 \eta^3 (-\mu_1 + 2 \Theta p (6 + \mu_2) + \Theta p \mu_1 (2 + \mathfrak{e}_1 + \mathfrak{e}_2)) + \\
& \eta^2 (-16 \mu_1 + 6 \Theta p (6 + 5 \mu_2) + 15 \Theta p \mu_1 (2 + \mathfrak{e}_1 + \mathfrak{e}_2)) + \\
& \Theta p (9 \times (2 + \mathfrak{e}_1 + \mathfrak{e}_2) + 10 \mu_1 (2 + \mathfrak{e}_1 + \mathfrak{e}_2) + \mu_2 (20 + 9 \mathfrak{e}_1 + 9 \mathfrak{e}_2)) + \\
& 2 \eta (-9 - 11 \mu_1 - 9 \mu_2 + \Theta p (9 \times (2 + \mathfrak{e}_1 + \mathfrak{e}_2) + \\
& 14 \mu_1 (2 + \mathfrak{e}_1 + \mathfrak{e}_2) + \mu_2 (28 + 9 \mathfrak{e}_1 + 9 \mathfrak{e}_2))) \Big) \Big) \Big) + \\
& (-1 + \times (-1 + \eta) - \eta) \times \Big( 2 \text{cv}^2 f w^2 (-1 + \eta)^3 \Big( x^2 (-1 + \eta)^2 + \eta (1 + \eta) + \\
& \times (1 + \eta - 2 \eta^2) \Big) \\
& (-4 x^3 (3 w (-1 + \eta) - 4 \eta) (-1 + \eta)^3 (-1 + \eta + \Theta l - \eta t \Theta l) \Theta p - \\
& 4 x^4 (-1 + \eta)^4 (-1 + \eta + \Theta l - \eta t \Theta l) \Theta p - \\
& 12 x^2 (-1 + \eta)^2 \Big( w^2 (-1 + \eta)^2 - 3 w (-1 + \eta) \eta + 2 \eta^2 \Big) (-1 + \eta + \Theta l - \eta t \Theta l) \Theta p + \\
& \Theta p \Big( 4 \eta^4 - 4 \eta^5 + 6 \eta t - 6 \eta \eta t - 6 \eta \Theta l - 4 \eta^4 \Theta l + 6 \eta \eta t \Theta l + 4 \\
& \eta^4 \eta t \Theta l - 3 \eta \Theta l \mathfrak{e}_1 + 3 \eta \eta t \Theta l \mathfrak{e}_1 - 3 \eta \Theta l \mathfrak{e}_2 + 3 \eta \eta t \Theta l \\
& \mathfrak{e}_2 - 3 w^2 (-1 + \eta)^2 \Big( 4 \eta^3 - 6 \eta t - 4 \eta^2 (1 + (-1 + \eta t) \Theta l) + \\
& \eta (6 \eta t + 3 \Theta l (2 + \mathfrak{e}_1 + \mathfrak{e}_2) - 3 \eta t \Theta l (2 + \mathfrak{e}_1 + \mathfrak{e}_2)) \Big) + 3 \\
& w (-1 + \eta) \times \Big( 4 \eta^4 - 6 \eta t - 4 \eta^3 (1 + (-1 + \eta t) \Theta l) + \eta \\
& (6 \eta t + 3 \Theta l (2 + \mathfrak{e}_1 + \mathfrak{e}_2) - 3 \eta t \Theta l (2 + \mathfrak{e}_1 + \mathfrak{e}_2)) \Big) + w^3 (-1 + \eta)^3 \Big( 4 \eta^2 - \\
& 6 \eta t + \eta (-4 + 6 \eta t + \Theta l (10 + 3 \mathfrak{e}_1 + 3 \mathfrak{e}_2) - \eta t \Theta l (10 + 3 \mathfrak{e}_1 + 3 \mathfrak{e}_2)) \Big) \Big) - \\
& \times (-1 + \eta) \times \Big( 4 (w (-1 + \eta) - 4 \eta) (-1 + \eta) (w + \eta - w \eta)^2 \Theta p - (-1 + \eta t) \\
& \Theta l \Big( 6 - 6 \Theta p - 16 \eta^3 \Theta p - 3 \Theta p \mathfrak{e}_1 - 3 \Theta p \mathfrak{e}_2 - 3 w^2 (-1 + \eta)^2 (-6 + 8 \eta \Theta p + \\
& 3 \Theta p (2 + \mathfrak{e}_1 + \mathfrak{e}_2)) + 9 w (-1 + \eta) \times \Big( -2 + \Theta p (2 + 4 \eta^2 + \mathfrak{e}_1 + \mathfrak{e}_2) \Big) + \\
& w^3 (-1 + \eta)^3 (-6 + \Theta p (10 + 3 \mathfrak{e}_1 + 3 \mathfrak{e}_2)) \Big) \Big) \Big) - \\
& (-1 + w (-1 + \eta)) (w (-1 + \eta) + \times (-1 + \eta) - \eta) \Big( 272 u^2 (-1 + \times (-1 + \eta) - \eta) \\
& (1 + w - w \eta)^2 (\times + \eta - \times \eta)^2 (w + \times + \eta - w \eta - \times \eta)^2 (-1 + \eta t) \Theta p - \\
& 8 f (-1 + \times (-1 + \eta) - \eta) \times (-1 + \eta) (\times + \eta - \times \eta)^2
\end{aligned}$$

$$\begin{aligned}
& (-ux(w(-1+\eta)+x(-1+\eta)-\eta)(1+w-w\eta)^2(-1+\eta t)\theta l \\
& \quad \theta p+2u(-1+\eta)\times(3x^2(-1+\eta)^2(-1+w(-1+\eta t)\theta l)\theta p+ \\
& \quad 2\times(-3(w(-1+\eta)-\eta)(-1+\eta)\theta p+(-1+\eta t)\theta l \\
& \quad \quad (1+w^2(-1+\eta)^2(1+3\theta p)-w(-1+\eta)\times(2+3\eta\theta p))) + \\
& \quad \theta p(-3\eta^2-2\eta t+w^3(-1+\eta)^2(-1+\eta t)\theta l(5+\mathfrak{x}1+\mathfrak{x}2)+ \\
& \quad w(\eta(-6+4\eta t)+3\eta^2(2+(-1+\eta t)\theta l)- \\
& \quad \quad \theta l(2+\mathfrak{x}1+\mathfrak{x}2)+\eta t(-4+\theta l(2+\mathfrak{x}1+\mathfrak{x}2))) - \\
& \quad w^2(-1+\eta)\times(-3-4\theta l+\eta(3-6\theta l+\eta t(2+6\theta l))- \\
& \quad \quad 2\theta l\mathfrak{x}1-2\theta l\mathfrak{x}2+2\eta t(-1+\theta l(2+\mathfrak{x}1+\mathfrak{x}2)))) + \\
& f^2(-1+\eta)^2\theta l((x^2(-1+\eta)^2+\eta(1+\eta)+x(1+\eta-2\eta^2)) \\
& \quad (40x^3(-1+\eta)^3(-1+\eta+\theta l-\eta t\theta l)\theta p+4x^2(-1+\eta)^2 \\
& \quad (-((-1+\eta)\theta p(2+30\eta+\mathfrak{x}1+\mathfrak{x}2))+2\times(-1+\eta t)\theta l(-1+ \\
& \quad \quad \theta p(2+15\eta+\mathfrak{x}1+\mathfrak{x}2))) + \theta p(-40\eta^4+4\eta^3(8+10\times(-1+\eta t) \\
& \quad \quad \theta l-\mathfrak{x}1-\mathfrak{x}2)+6\eta t(2+\mathfrak{x}1+\mathfrak{x}2)+\eta(-3\theta l(2+\mathfrak{x}1+\mathfrak{x}2)^2+ \\
& \quad \quad 3\eta t\theta l(2+\mathfrak{x}1+\mathfrak{x}2)^2-2\eta t(2+3\mathfrak{x}1+3\mathfrak{x}2)))+4\eta^2 \\
& \quad (-((-1+2\theta l)\times(2+\mathfrak{x}1+\mathfrak{x}2))+2\eta t(-1+\theta l(2+\mathfrak{x}1+\mathfrak{x}2)))) + \\
& \quad \times(-1+\eta)\times(8\times(-1+\eta)\theta p(15\eta^2+\eta t+\eta(2+\mathfrak{x}1+\mathfrak{x}2))- \\
& \quad (-1+\eta t)\theta l(120\eta^2\theta p+3\times(2+\mathfrak{x}1+\mathfrak{x}2)\times(-2+\theta p(2+\mathfrak{x}1+\mathfrak{x}2))+ \\
& \quad \quad 8\eta(-1+2\theta p(2+\mathfrak{x}1+\mathfrak{x}2)))) - w^3(-1+\eta)^3 \\
& \quad (40x^3(-1+\eta)^3(-1+\eta+\theta l-\eta t\theta l)\theta p+x^2(-1+\eta)^2(-8\times(-1+\eta) \\
& \quad \quad \theta p(7+15\eta+\mathfrak{x}1+\mathfrak{x}2)+(-1+\eta t)\theta l(-2\times(14+3\mathfrak{x}1+3\mathfrak{x}2)+ \\
& \quad \quad \theta p(84+120\eta+28\mathfrak{x}1+3\mathfrak{x}1^2+28\mathfrak{x}2+6\mathfrak{x}1\mathfrak{x}2+3\mathfrak{x}2^2))) + \\
& \quad \theta p(-40\eta^4+8\eta^3(-2+5\times(-1+\eta t)\theta l-\mathfrak{x}1-\mathfrak{x}2)+6\eta t(2+\mathfrak{x}1+\mathfrak{x}2)+ \\
& \quad \eta(-3\theta l(2+\mathfrak{x}1+\mathfrak{x}2)^2+\eta t(16+3\theta l(2+\mathfrak{x}1+\mathfrak{x}2)^2)) + \\
& \quad \eta^2(8\times(7+\mathfrak{x}1+\mathfrak{x}2)-2\eta t(14+3\mathfrak{x}1+3\mathfrak{x}2)- \\
& \quad \quad \theta l(84+3\mathfrak{x}1^2+28\mathfrak{x}2+3\mathfrak{x}2^2+\mathfrak{x}1(28+6\mathfrak{x}2)) + \\
& \quad \quad \eta t\theta l(84+3\mathfrak{x}1^2+28\mathfrak{x}2+3\mathfrak{x}2^2+\mathfrak{x}1(28+6\mathfrak{x}2)))) + \\
& \quad \times(-1+\eta)\times(2\times(-1+\eta)\theta p(60\eta^2+8\eta(7+\mathfrak{x}1+\mathfrak{x}2)+ \\
& \quad \eta t(14+3\mathfrak{x}1+3\mathfrak{x}2))-(-1+\eta t)\theta l(120\eta^2\theta p+ \\
& \quad \quad 3\times(2+\mathfrak{x}1+\mathfrak{x}2)\times(-2+\theta p(2+\mathfrak{x}1+\mathfrak{x}2))+2\eta(-14-3\mathfrak{x}1- \\
& \quad \quad 3\mathfrak{x}2+\theta p(84+28\mathfrak{x}1+3\mathfrak{x}1^2+28\mathfrak{x}2+6\mathfrak{x}1\mathfrak{x}2+3\mathfrak{x}2^2)))) + \\
& w(-1+x(-1+\eta)-\eta)\times(-1+\eta)\times(-40x^4(-1+\eta)^4(-1+\eta+ \\
& \quad \theta l-\eta t\theta l)\theta p+4x^3(-1+\eta)^3(2\times(-1+\eta)\theta p(12+20\eta+\mathfrak{x}1+\mathfrak{x}2)- \\
& \quad (-1+\eta t)\theta l(-2+\theta p(26+40\eta+3\mathfrak{x}1+3\mathfrak{x}2)))+2x^2(-1+\eta)^2 \\
& \quad (-2\times(-1+\eta)\theta p(2+60\eta^2+2\eta t+\mathfrak{x}1+\mathfrak{x}2+6\eta(12+\mathfrak{x}1+\mathfrak{x}2))+(-1+ \\
& \quad \eta t)\theta l(120\eta^2\theta p-2\times(10+3\mathfrak{x}1+3\mathfrak{x}2)+3\theta p(8+\mathfrak{x}1^2+6\mathfrak{x}2+ \\
& \quad \quad \mathfrak{x}2^2+2\mathfrak{x}1(3+\mathfrak{x}2))+2\eta(-4+\theta p(78+9\mathfrak{x}1+9\mathfrak{x}2)))) + \\
& \quad \theta p(-40\eta^5+8\eta^4(-7+5\times(-1+\eta t)\theta l-\mathfrak{x}1-\mathfrak{x}2)+6\eta t \\
& \quad \quad (2+\mathfrak{x}1+\mathfrak{x}2)+\eta(-3\theta l(2+\mathfrak{x}1+\mathfrak{x}2)^2+ \\
& \quad \quad \eta t(28+6\mathfrak{x}1+6\mathfrak{x}2+3\theta l(2+\mathfrak{x}1+\mathfrak{x}2)^2))+4\eta^3(22+\mathfrak{x}1+\mathfrak{x}2- \\
& \quad \quad \theta l(26+3\mathfrak{x}1+3\mathfrak{x}2)+\eta t(-2+\theta l(26+3\mathfrak{x}1+3\mathfrak{x}2)))+2\eta^2 \\
& \quad \quad (-((2+\mathfrak{x}1+\mathfrak{x}2)\times(-2+3\theta l(4+\mathfrak{x}1+\mathfrak{x}2)))+\eta t(-2\times(8+3\mathfrak{x}1+ \\
& \quad \quad 3\mathfrak{x}2)+3\theta l(8+\mathfrak{x}1^2+6\mathfrak{x}2+\mathfrak{x}2^2+2\mathfrak{x}1(3+\mathfrak{x}2)))) +
\end{aligned}$$

$$\begin{aligned}
& \times (-1 + \eta) \times (4 \times (-1 + \eta) \operatorname{ep} (40 \eta^3 + 6 \eta^2 (12 + \mathfrak{x}1 + \mathfrak{x}2) + \\
& \quad 2 \eta (2 + 2 \eta \mathfrak{t} + \mathfrak{x}1 + \mathfrak{x}2) + \eta \mathfrak{t} (10 + 3 \mathfrak{x}1 + 3 \mathfrak{x}2)) - (-1 + \eta \mathfrak{t}) \mathfrak{el} \\
& \quad (160 \eta^3 \operatorname{ep} + 3 \times (2 + \mathfrak{x}1 + \mathfrak{x}2) \times (-2 + \operatorname{ep} (2 + \mathfrak{x}1 + \mathfrak{x}2)) + \\
& \quad 4 \eta^2 (-2 + \operatorname{ep} (78 + 9 \mathfrak{x}1 + 9 \mathfrak{x}2)) + 4 \eta (-10 - 3 \mathfrak{x}1 - 3 \mathfrak{x}2 + \\
& \quad 3 \operatorname{ep} (8 + \mathfrak{x}1^2 + 6 \mathfrak{x}2 + \mathfrak{x}2^2 + 2 \mathfrak{x}1 (3 + \mathfrak{x}2))) + \\
& w^2 (-1 + \eta)^2 (-80 \mathfrak{x}^4 (-1 + \eta)^4 (-1 + \eta + \mathfrak{el} - \eta \mathfrak{t} \mathfrak{el}) \operatorname{ep} + \\
& \quad \mathfrak{x}^3 (-1 + \eta)^3 (8 \times (-1 + \eta) \operatorname{ep} (19 + 40 \eta + 2 \mathfrak{x}1 + 2 \mathfrak{x}2) - \\
& \quad (-1 + \eta \mathfrak{t}) \mathfrak{el} (320 \eta \operatorname{ep} - 2 \times (14 + 3 \mathfrak{x}1 + 3 \mathfrak{x}2) + \\
& \quad 3 \operatorname{ep} (60 + \mathfrak{x}1^2 + 12 \mathfrak{x}2 + \mathfrak{x}2^2 + 2 \mathfrak{x}1 (6 + \mathfrak{x}2))) + \\
& \quad \mathfrak{x}^2 (-1 + \eta)^2 (-2 \times (-1 + \eta) \operatorname{ep} (240 \eta^2 + 4 \times (7 + \mathfrak{x}1 + \mathfrak{x}2) + \\
& \quad 12 \eta (19 + 2 \mathfrak{x}1 + 2 \mathfrak{x}2) + \eta \mathfrak{t} (14 + 3 \mathfrak{x}1 + 3 \mathfrak{x}2)) + (-1 + \eta \mathfrak{t}) \mathfrak{el} \\
& \quad (480 \eta^2 \operatorname{ep} - 4 \eta (14 + 3 \mathfrak{x}1 + 3 \mathfrak{x}2) - 2 \times (34 + 9 \mathfrak{x}1 + 9 \mathfrak{x}2) + \\
& \quad 9 \eta \operatorname{ep} (60 + \mathfrak{x}1^2 + 12 \mathfrak{x}2 + \mathfrak{x}2^2 + 2 \mathfrak{x}1 (6 + \mathfrak{x}2)) + \operatorname{ep} \\
& \quad (124 + 9 \mathfrak{x}1^2 + 60 \mathfrak{x}2 + 9 \mathfrak{x}2^2 + 6 \mathfrak{x}1 (10 + 3 \mathfrak{x}2))) + \operatorname{ep} (-80 \eta^5 + \\
& \quad 8 \eta^4 (-9 + 10 \times (-1 + \eta \mathfrak{t}) \mathfrak{el} - 2 \mathfrak{x}1 - 2 \mathfrak{x}2) + 12 \eta \mathfrak{t} (2 + \mathfrak{x}1 + \mathfrak{x}2) + 2 \eta \\
& \quad (-3 \mathfrak{el} (2 + \mathfrak{x}1 + \mathfrak{x}2)^2 + \eta \mathfrak{t} (22 + 3 \mathfrak{x}1 + 3 \mathfrak{x}2 + 3 \mathfrak{el} (2 + \mathfrak{x}1 + \mathfrak{x}2)^2)) + \\
& \quad \eta^2 (8 \times (7 + \mathfrak{x}1 + \mathfrak{x}2) - 4 \eta \mathfrak{t} (10 + 3 \mathfrak{x}1 + 3 \mathfrak{x}2) - \\
& \quad \mathfrak{el} (124 + 9 \mathfrak{x}1^2 + 60 \mathfrak{x}2 + 9 \mathfrak{x}2^2 + 6 \mathfrak{x}1 (10 + 3 \mathfrak{x}2)) + \\
& \quad \eta \mathfrak{t} \mathfrak{el} (124 + 9 \mathfrak{x}1^2 + 60 \mathfrak{x}2 + 9 \mathfrak{x}2^2 + 6 \mathfrak{x}1 (10 + 3 \mathfrak{x}2))) + \\
& \quad \eta^3 (8 \times (12 + \mathfrak{x}1 + \mathfrak{x}2) - 3 \mathfrak{el} (60 + \mathfrak{x}1^2 + 12 \mathfrak{x}2 + \mathfrak{x}2^2 + \\
& \quad 2 \mathfrak{x}1 (6 + \mathfrak{x}2)) + \eta \mathfrak{t} (-2 \times (14 + 3 \mathfrak{x}1 + 3 \mathfrak{x}2) + \\
& \quad 3 \mathfrak{el} (60 + \mathfrak{x}1^2 + 12 \mathfrak{x}2 + \mathfrak{x}2^2 + 2 \mathfrak{x}1 (6 + \mathfrak{x}2))) + \mathfrak{x} (-1 + \eta) \times \\
& \quad (2 \times (-1 + \eta) \operatorname{ep} (160 \eta^3 + 8 \eta (7 + \mathfrak{x}1 + \mathfrak{x}2) + 12 \eta^2 (19 + 2 \mathfrak{x}1 + 2 \mathfrak{x}2) + \\
& \quad \eta \eta \mathfrak{t} (28 + 6 \mathfrak{x}1 + 6 \mathfrak{x}2) + \eta \mathfrak{t} (34 + 9 \mathfrak{x}1 + 9 \mathfrak{x}2)) - (-1 + \eta \mathfrak{t}) \mathfrak{el} \\
& \quad (320 \eta^3 \operatorname{ep} + 6 \times (2 + \mathfrak{x}1 + \mathfrak{x}2) \times (-2 + \operatorname{ep} (2 + \mathfrak{x}1 + \mathfrak{x}2)) + \\
& \quad 2 \eta (-34 - 9 \mathfrak{x}1 - 9 \mathfrak{x}2 + \operatorname{ep} (124 + 60 \mathfrak{x}1 + 9 \mathfrak{x}1^2 + 60 \mathfrak{x}2 + \\
& \quad 18 \mathfrak{x}1 \mathfrak{x}2 + 9 \mathfrak{x}2^2)) + \eta^2 (-2 \times (14 + 3 \mathfrak{x}1 + 3 \mathfrak{x}2) + \\
& \quad 9 \operatorname{ep} (60 + \mathfrak{x}1^2 + 12 \mathfrak{x}2 + \mathfrak{x}2^2 + 2 \mathfrak{x}1 (6 + \mathfrak{x}2)))) + \\
& 2 \operatorname{co}^2 f (-1 + \eta)^3 (-4 \mathfrak{x}^7 (-1 + \eta)^7 (-1 + \eta + \mathfrak{el} - \eta \mathfrak{t} \mathfrak{el}) \operatorname{ep} + 2 \mathfrak{x}^6 (-1 + \eta)^6 \\
& \quad (-2 \times (-1 + w (-1 + \eta)) \times (-1 + \eta \mathfrak{t}) \mathfrak{el} \mu1 (2 + 5 \times (-1 + w (-1 + \eta)) \mu1) + \\
& \quad \operatorname{ep} (-4 - 10 \eta + 14 \eta^2 + 4 \mathfrak{el} + 14 \eta \mathfrak{el} - 4 \eta \mathfrak{t} \mathfrak{el} - 14 \eta \eta \mathfrak{t} \mathfrak{el} + 2 \mathfrak{el} \mu1 - 2 \eta \mathfrak{t} \\
& \quad \mathfrak{el} \mu1 + 2 \mathfrak{el} \mu2 - 2 \eta \mathfrak{t} \mathfrak{el} \mu2 - 20 \mu1 \mu2 + 10 w^2 (-1 + \eta)^3 \mu1 \mu2 + 20 \eta \\
& \quad \mu1 \mu2 + 10 \mathfrak{el} \mu1 \mu2 - 10 \eta \mathfrak{t} \mathfrak{el} \mu1 \mu2 + \mathfrak{el} \mu1 \mathfrak{x}1 - \eta \mathfrak{t} \mathfrak{el} \mu1 \mathfrak{x}1 + \mathfrak{el} \mu1 \\
& \quad \mathfrak{x}2 - \eta \mathfrak{t} \mathfrak{el} \mu1 \mathfrak{x}2 - w (-1 + \eta) \times (-6 \times (1 + 5 \mu1 \mu2) + 6 \eta (1 + 5 \mu1 \mu2) - \\
& \quad (-1 + \eta \mathfrak{t}) \mathfrak{el} (2 \times (3 + \mu2) + \mu1 (2 + 10 \mu2 + \mathfrak{x}1 + \mathfrak{x}2)))) + \\
& 2 \mathfrak{x}^5 (-1 + \eta)^5 (-2 \times (-1 + w (-1 + \eta)) \times (-1 + \eta \mathfrak{t}) \mathfrak{el} \mu1 \\
& \quad (-4 + 10 \mu1 + 15 w^2 (-1 + \eta)^2 \mu1 + 5 \eta (-2 + 5 \mu1) - 2 \\
& \quad \mu2 - w (-1 + \eta) \times (25 \times (1 + \eta) \mu1 - 2 \times (3 + \mu2))) + \\
& \operatorname{ep} (2 + 22 \eta + 18 \eta^2 - 42 \eta^3 - 2 \mathfrak{el} - 24 \eta \mathfrak{el} - 42 \eta^2 \mathfrak{el} + 2 \eta \mathfrak{t} \mathfrak{el} + 24 \\
& \quad \eta \eta \mathfrak{t} \mathfrak{el} + 42 \eta^2 \eta \mathfrak{t} \mathfrak{el} + 4 \eta \mathfrak{t} \mu1 - 4 \eta \eta \mathfrak{t} \mu1 - 6 \mathfrak{el} \mu1 - 12 \eta \mathfrak{el} \\
& \quad \mu1 + 6 \eta \mathfrak{t} \mathfrak{el} \mu1 + 12 \eta \eta \mathfrak{t} \mathfrak{el} \mu1 - 10 \eta \mathfrak{t} \mu1^2 + 10 \eta \eta \mathfrak{t} \mu1^2 - 2 \mathfrak{el} \\
& \quad \mu1^2 + 2 \eta \mathfrak{t} \mathfrak{el} \mu1^2 + 4 \mu2 - 4 \eta \mu2 - 6 \mathfrak{el} \mu2 - 12 \eta \mathfrak{el} \mu2 + 6 \eta \mathfrak{t} \mathfrak{el} \\
& \quad \mu2 + 12 \eta \eta \mathfrak{t} \mathfrak{el} \mu2 + 44 \mu1 \mu2 + 30 w^3 (-1 + \eta)^4 \mu1 \mu2 + 76 \eta \mu1
\end{aligned}$$

$$\begin{aligned}
& \mu_2 - 120 \eta^2 \mu_1 \mu_2 - 26 \theta_l \mu_1 \mu_2 - 60 \eta \theta_l \mu_1 \mu_2 + 26 \eta t \theta_l \mu_1 \\
& \mu_2 + 60 \eta \eta t \theta_l \mu_1 \mu_2 + 2 \mu_2^2 - 2 \eta \mu_2^2 - 2 \theta_l \mu_2^2 + 2 \eta t \theta_l \mu_2^2 - 3 \\
& \theta_l \mu_1 \boxplus 1 - 6 \eta \theta_l \mu_1 \boxplus 1 + 3 \eta t \theta_l \mu_1 \boxplus 1 + 6 \eta \eta t \theta_l \mu_1 \boxplus 1 - \theta_l \\
& \mu_1^2 \boxplus 1 + \eta t \theta_l \mu_1^2 \boxplus 1 - 2 \theta_l \mu_1 \mu_2 \boxplus 1 + 2 \eta t \theta_l \mu_1 \mu_2 \boxplus 1 - 3 \\
& \theta_l \mu_1 \boxplus 2 - 6 \eta \theta_l \mu_1 \boxplus 2 + 3 \eta t \theta_l \mu_1 \boxplus 2 + 6 \eta \eta t \theta_l \mu_1 \boxplus 2 - \theta_l \\
& \mu_1^2 \boxplus 2 + \eta t \theta_l \mu_1^2 \boxplus 2 - 2 \theta_l \mu_1 \mu_2 \boxplus 2 + 2 \eta t \theta_l \mu_1 \mu_2 \boxplus 2 - w^2 \\
& (-1 + \eta)^2 (60 \eta^2 \mu_1 \mu_2 + 2 \times (-3 + 5 \eta t \mu_1^2 - 52 \mu_1 \mu_2 - \mu_2^2) + \\
& 2 \eta (3 - 5 \eta t \mu_1^2 + 22 \mu_1 \mu_2 + \mu_2^2) - (-1 + \eta t) \theta_l (2 \times (3 + 3 \mu_2 + \mu_2^2) + \\
& 3 \mu_1 (2 + \boxplus 1 + \boxplus 2) + \mu_1^2 (2 + \boxplus 1 + \boxplus 2) + 2 \mu_1 \mu_2 (13 + \boxplus 1 + \boxplus 2))) + 2 \\
& w (-1 + \eta) \times (-6 - 2 \eta t \mu_1 + 10 \eta t \mu_1^2 - 2 \mu_2 - 59 \mu_1 \mu_2 - 2 \mu_2^2 + \\
& 18 \eta^2 (1 + 5 \mu_1 \mu_2) - (-1 + \eta t) \theta_l (2 \times (3 + 3 \mu_2 + \mu_2^2) + \\
& 3 \mu_1 (2 + \boxplus 1 + \boxplus 2) + \mu_1^2 (2 + \boxplus 1 + \boxplus 2) + 2 \mu_1 \mu_2 (13 + \boxplus 1 + \boxplus 2)) + \\
& \eta (-12 + 2 \eta t (1 - 5 \mu_1) \mu_1 + 2 \mu_2 - 31 \mu_1 \mu_2 + 2 \mu_2^2 - \\
& 3 \times (-1 + \eta t) \theta_l (2 \times (3 + \mu_2) + \mu_1 (2 + 10 \mu_2 + \boxplus 1 + \boxplus 2)))) - \\
& x^4 (-1 + \eta)^4 (-4 \times (-1 + \eta) \theta_p (5 \eta + 30 \eta^2 + 35 \eta^3 + 4 \eta t \mu_1 + 10 \eta \eta t \mu_1 - \\
& 10 \eta t \mu_1^2 - 25 \eta \eta t \mu_1^2 + 4 \mu_2 + 10 \eta \mu_2 + 14 \mu_1 \mu_2 + 15 w^4 (-1 + \eta)^4 \\
& \mu_1 \mu_2 + 110 \eta \mu_1 \mu_2 + 150 \eta^2 \mu_1 \mu_2 + 2 \eta t \mu_1 \mu_2 + 2 \mu_2^2 + 5 \eta \mu_2^2 - w^3 \\
& (-1 + \eta)^3 (1 - 15 \eta t \mu_1^2 + 3 \times (22 + 25 \eta) \mu_1 \mu_2 + 3 \mu_2^2) + w^2 (-1 + \eta)^2 \\
& (6 + 6 \mu_2 + 111 \mu_1 \mu_2 + 75 \eta^2 \mu_1 \mu_2 + 8 \mu_2^2 + 2 \eta t \mu_1 (3 - 20 \mu_1 + \mu_2) + \\
& 5 \eta (3 - 5 \eta t \mu_1^2 + 52 \mu_1 \mu_2 + \mu_2^2)) - w (-1 + \eta) \times \\
& (3 + 10 \mu_2 + 74 \mu_1 \mu_2 + 7 \mu_2^2 + \eta t \mu_1 (10 - 35 \mu_1 + 4 \mu_2) + 45 \eta^2 \\
& (1 + 5 \mu_1 \mu_2) + 5 \eta (6 + 2 \eta t (1 - 5 \mu_1) \mu_1 + 2 \mu_2 + 59 \mu_1 \mu_2 + 2 \mu_2^2))) + \\
& (-1 + \eta t) \theta_l (-6 + 6 \theta_p + 20 \eta \theta_p + 120 \eta^2 \theta_p + 140 \eta^3 \theta_p - 20 \mu_1 - 64 \\
& \eta \mu_1 - 80 \eta^2 \mu_1 + 24 \theta_p \mu_1 + 60 \eta \theta_p \mu_1 + 60 \eta^2 \theta_p \mu_1 + 14 \mu_1^2 + 60 \\
& w^4 (-1 + \eta)^4 \mu_1^2 + 160 \eta \mu_1^2 + 200 \eta^2 \mu_1^2 + 14 \theta_p \mu_1^2 + 20 \eta \\
& \theta_p \mu_1^2 - 12 \mu_2 + 24 \theta_p \mu_2 + 60 \eta \theta_p \mu_2 + 60 \eta^2 \theta_p \mu_2 - 28 \mu_1 \\
& \mu_2 - 32 \eta \mu_1 \mu_2 + 56 \theta_p \mu_1 \mu_2 + 260 \eta \theta_p \mu_1 \mu_2 + 300 \eta^2 \theta_p \mu_1 \\
& \mu_2 - 6 \mu_2^2 + 14 \theta_p \mu_2^2 + 20 \eta \theta_p \mu_2^2 + 3 \theta_p \boxplus 1 + 12 \theta_p \mu_1 \boxplus 1 + 30 \\
& \eta \theta_p \mu_1 \boxplus 1 + 30 \eta^2 \theta_p \mu_1 \boxplus 1 + 7 \theta_p \mu_1^2 \boxplus 1 + 10 \eta \theta_p \mu_1^2 \boxplus 1 + 6 \\
& \theta_p \mu_2 \boxplus 1 + 14 \theta_p \mu_1 \mu_2 \boxplus 1 + 20 \eta \theta_p \mu_1 \mu_2 \boxplus 1 + 3 \theta_p \mu_2^2 \boxplus 1 + 3 \\
& \theta_p \boxplus 2 + 12 \theta_p \mu_1 \boxplus 2 + 30 \eta \theta_p \mu_1 \boxplus 2 + 30 \eta^2 \theta_p \mu_1 \boxplus 2 + 7 \theta_p \mu_1^2 \\
& \boxplus 2 + 10 \eta \theta_p \mu_1^2 \boxplus 2 + 6 \theta_p \mu_2 \boxplus 2 + 14 \theta_p \mu_1 \mu_2 \boxplus 2 + 20 \eta \theta_p \mu_1 \mu_2 \\
& \boxplus 2 + 3 \theta_p \mu_2^2 \boxplus 2 + w^2 (-1 + \eta)^2 (2 \times ((147 + 320 \eta + 100 \eta^2) \mu_1^2 - \\
& 9 (1 + \mu_2)^2 - 2 \mu_1 (21 + 13 \mu_2 + 8 \eta (3 + \mu_2))) + \\
& \theta_p (42 + 72 \mu_2 + 34 \mu_2^2 + 9 \boxplus 1 + 18 \mu_2 \boxplus 1 + 9 \mu_2^2 \boxplus 1 + 9 \boxplus 2 + \\
& 18 \mu_2 \boxplus 2 + 9 \mu_2^2 \boxplus 2 + 36 \mu_1 (2 + \boxplus 1 + \boxplus 2) + 17 \mu_1^2 (2 + \boxplus 1 + \boxplus 2) + \\
& 2 \mu_1 \mu_2 (92 + 17 \boxplus 1 + 17 \boxplus 2) + 10 \eta (2 \times (3 + 3 \mu_2 + \mu_2^2) + 3 \mu_1 \\
& (2 + \boxplus 1 + \boxplus 2) + \mu_1^2 (2 + \boxplus 1 + \boxplus 2) + 2 \mu_1 \mu_2 (13 + \boxplus 1 + \boxplus 2)))) - \\
& w (-1 + \eta) \times (2 \times ((69 + 280 \eta + 200 \eta^2) \mu_1^2 - 9 (1 + \mu_2)^2 - \\
& 2 \mu_1 (19 + 20 \eta^2 + 17 \mu_2 + 8 \eta (5 + 2 \mu_2))) + \\
& \theta_p (30 + 76 \mu_2 + 38 \mu_2^2 + 9 \boxplus 1 + 18 \mu_2 \boxplus 1 + 9 \mu_2^2 \boxplus 1 + 9 \boxplus 2 + \\
& 18 \mu_2 \boxplus 2 + 9 \mu_2^2 \boxplus 2 + 38 \mu_1 (2 + \boxplus 1 + \boxplus 2) + 19 \mu_1^2 (2 + \boxplus 1 + \boxplus 2) + \\
& 2 \mu_1 \mu_2 (98 + 19 \boxplus 1 + 19 \boxplus 2) + 20 \eta (2 \times (3 + 3 \mu_2 + \mu_2^2) + \\
& 3 \mu_1 (2 + \boxplus 1 + \boxplus 2) + \mu_1^2 (2 + \boxplus 1 + \boxplus 2) + 2 \mu_1 \mu_2 (13 + \boxplus 1 + \boxplus 2))) +
\end{aligned}$$

$$\begin{aligned}
& 30 \eta^2 (2 \times (3 + \mu_2) + \mu_1 (2 + 10 \mu_2 + \mathfrak{E}_1 + \mathfrak{E}_2)) - w^3 \\
& (-1 + \eta)^3 (10 \times (23 + 24 \eta) \mu_1^2 - 6 (1 + \mu_2)^2 - 4 \mu_1 (7 + 3 \mu_2) + \\
& \quad \text{ep} (5 \mu_1^2 (2 + \mathfrak{E}_1 + \mathfrak{E}_2) + (1 + \mu_2)^2 (10 + 3 \mathfrak{E}_1 + 3 \mathfrak{E}_2) + \\
& \quad 2 \mu_1 (5 \times (2 + \mathfrak{E}_1 + \mathfrak{E}_2) + \mu_2 (22 + 5 \mathfrak{E}_1 + 5 \mathfrak{E}_2))) - \\
& x^2 (-1 + \eta)^2 (2 \times (-1 + \eta) \text{ep} (-20 \eta^3 - 60 \eta^4 - 42 \eta^5 - 6 \eta t - 9 \eta \eta t - 12 \\
& \quad \eta t \mu_1 - 30 \eta \eta t \mu_1 - 48 \eta^2 \eta t \mu_1 - 40 \eta^3 \eta t \mu_1 - 6 \eta t \mu_1^2 + 21 \eta \\
& \quad \eta t \mu_1^2 + 120 \eta^2 \eta t \mu_1^2 + 100 \eta^3 \eta t \mu_1^2 - 12 \eta \mu_2 - 48 \eta^2 \mu_2 - 40 \\
& \quad \eta^3 \mu_2 - 12 \eta t \mu_2 - 18 \eta \eta t \mu_2 - 12 \eta \mu_1 \mu_2 - 168 \eta^2 \mu_1 \mu_2 - 440 \eta^3 \\
& \quad \mu_1 \mu_2 - 300 \eta^4 \mu_1 \mu_2 - 16 \eta t \mu_1 \mu_2 - 42 \eta \eta t \mu_1 \mu_2 - 24 \eta^2 \eta t \mu_1 \\
& \quad \mu_2 - 6 \eta \mu_2^2 - 24 \eta^2 \mu_2^2 - 20 \eta^3 \mu_2^2 - 6 \eta t \mu_2^2 - 9 \eta \eta t \mu_2^2 + 2 w^5 \\
& \quad (-1 + \eta)^5 (-5 \eta t \mu_1^2 + \mu_2 ((7 + 15 \eta) \mu_1 + \mu_2)) + 6 w^4 (-1 + \eta)^4 \\
& \quad (\eta t \mu_1 (3 \times (4 + 5 \eta) \mu_1 + \mu_2) - \mu_2 ((7 + 36 \eta + 30 \eta^2) \mu_1 + 3 \eta \mu_2)) + w^3 \\
& \quad (-1 + \eta)^3 (2 + 8 \mu_2 + 56 \mu_1 \mu_2 + 300 \eta^3 \mu_1 \mu_2 - 6 \mu_2^2 + 12 \eta^2 (1 - 15 \eta t \mu_1^2 + \\
& \quad 66 \mu_1 \mu_2 + 3 \mu_2^2) + 2 \eta t (-66 \mu_1^2 + 3 (1 + \mu_2)^2 + 5 \mu_1 (2 + \mu_2)) + \\
& \quad \eta (12 - 345 \eta t \mu_1^2 + 6 \times (4 + 83 \mu_1) \mu_2 + 42 \mu_2^2 + 9 \eta t (1 + \mu_2)^2 + \\
& \quad 6 \eta t \mu_1 (7 + 3 \mu_2))) - w^2 (-1 + \eta)^2 (150 \eta^4 \mu_1 \mu_2 + \\
& \quad 4 \times (3 + 8 \mu_1 - \mu_2) \mu_2 - 20 \eta^3 (-3 + 5 \eta t \mu_1^2 - 52 \mu_1 \mu_2 - \mu_2^2) + \\
& \quad 12 \eta^2 (6 + 6 \mu_2 + 111 \mu_1 \mu_2 + 8 \mu_2^2 + 2 \eta t \mu_1 (3 - 20 \mu_1 + \mu_2)) + \\
& \quad 2 \eta t (-41 \mu_1^2 + 9 (1 + \mu_2)^2 + 3 \mu_1 (8 + 9 \mu_2)) + 3 \eta (6 + 8 \times (3 + 20 \mu_1) \\
& \quad \mu_2 + 12 \mu_2^2 + \eta t (-147 \mu_1^2 + 9 (1 + \mu_2)^2 + \mu_1 (42 + 26 \mu_2))) + w \\
& \quad (-1 + \eta) \times (4 \times (1 + \mu_1) \mu_2 + 90 \eta^4 (1 + 5 \mu_1 \mu_2) - 20 \eta^3 \\
& \quad (-6 + 2 \eta t \mu_1 (-1 + 5 \mu_1) - 2 \mu_2 - 59 \mu_1 \mu_2 - 2 \mu_2^2) + \\
& \quad 12 \eta^2 (3 + 10 \mu_2 + 74 \mu_1 \mu_2 + 7 \mu_2^2 + \eta t \mu_1 (10 - 35 \mu_1 + 4 \mu_2)) + \eta t \\
& \quad (-6 \mu_1^2 + 18 (1 + \mu_2)^2 + \mu_1 (40 + 54 \mu_2)) + \eta (6 \mu_2 (10 + 30 \mu_1 + 3 \mu_2) + \\
& \quad 3 \eta t (-69 \mu_1^2 + 9 (1 + \mu_2)^2 + \mu_1 (38 + 34 \mu_2)))) - \\
& (-1 + \eta t) \text{el} (6 + 24 \eta + 18 \eta^2 - 6 \text{ep} - 36 \eta \text{ep} - 36 \eta^2 \text{ep} - 40 \eta^3 \text{ep} - \\
& 120 \eta^4 \text{ep} - 84 \eta^5 \text{ep} + 12 \mu_1 + 48 \eta \mu_1 + 60 \eta^2 \mu_1 + 64 \eta^3 \mu_1 + 40 \\
& \eta^4 \mu_1 - 12 \text{ep} \mu_1 - 84 \eta \text{ep} \mu_1 - 144 \eta^2 \text{ep} \mu_1 - 120 \eta^3 \text{ep} \mu_1 - 60 \\
& \eta^4 \text{ep} \mu_1 + 6 \mu_1^2 + 24 \eta \mu_1^2 - 42 \eta^2 \mu_1^2 - 160 \eta^3 \mu_1^2 - 100 \eta^4 \\
& \mu_1^2 - 6 \text{ep} \mu_1^2 - 48 \eta \text{ep} \mu_1^2 - 84 \eta^2 \text{ep} \mu_1^2 - 40 \eta^3 \text{ep} \mu_1^2 + 12 \\
& \mu_2 + 48 \eta \mu_2 + 36 \eta^2 \mu_2 - 12 \text{ep} \mu_2 - 84 \eta \text{ep} \mu_2 - 144 \eta^2 \text{ep} \\
& \mu_2 - 120 \eta^3 \text{ep} \mu_2 - 60 \eta^4 \text{ep} \mu_2 + 12 \mu_1 \mu_2 + 64 \eta \mu_1 \mu_2 + 84 \\
& \eta^2 \mu_1 \mu_2 + 32 \eta^3 \mu_1 \mu_2 - 12 \text{ep} \mu_1 \mu_2 - 108 \eta \text{ep} \mu_1 \mu_2 - 336 \\
& \eta^2 \text{ep} \mu_1 \mu_2 - 520 \eta^3 \text{ep} \mu_1 \mu_2 - 300 \eta^4 \text{ep} \mu_1 \mu_2 + 6 \mu_2^2 + 24 \eta \\
& \mu_2^2 + 18 \eta^2 \mu_2^2 - 6 \text{ep} \mu_2^2 - 48 \eta \text{ep} \mu_2^2 - 84 \eta^2 \text{ep} \mu_2^2 - 40 \eta^3 \text{ep} \\
& \mu_2^2 + 4 w^5 (-1 + \eta)^5 \mu_1 ((7 + 10 \eta) \mu_1 + \mu_2) - 12 w^4 (-1 + \eta)^4 \\
& \mu_1 ((7 + 24 \eta + 15 \eta^2) \mu_1 + 2 \eta \mu_2) - 3 \text{ep} \mathfrak{E}_1 - 18 \eta \text{ep} \mathfrak{E}_1 - 18 \\
& \eta^2 \text{ep} \mathfrak{E}_1 - 6 \text{ep} \mu_1 \mathfrak{E}_1 - 42 \eta \text{ep} \mu_1 \mathfrak{E}_1 - 72 \eta^2 \text{ep} \mu_1 \mathfrak{E}_1 - 60 \eta^3 \\
& \text{ep} \mu_1 \mathfrak{E}_1 - 30 \eta^4 \text{ep} \mu_1 \mathfrak{E}_1 - 3 \text{ep} \mu_1^2 \mathfrak{E}_1 - 24 \eta \text{ep} \mu_1^2 \mathfrak{E}_1 - 42 \\
& \eta^2 \text{ep} \mu_1^2 \mathfrak{E}_1 - 20 \eta^3 \text{ep} \mu_1^2 \mathfrak{E}_1 - 6 \text{ep} \mu_2 \mathfrak{E}_1 - 36 \eta \text{ep} \mu_2 \mathfrak{E}_1 - 36 \\
& \eta^2 \text{ep} \mu_2 \mathfrak{E}_1 - 6 \text{ep} \mu_1 \mu_2 \mathfrak{E}_1 - 48 \eta \text{ep} \mu_1 \mu_2 \mathfrak{E}_1 - 84 \eta^2 \text{ep} \mu_1 \mu_2 \\
& \mathfrak{E}_1 - 40 \eta^3 \text{ep} \mu_1 \mu_2 \mathfrak{E}_1 - 3 \text{ep} \mu_2^2 \mathfrak{E}_1 - 18 \eta \text{ep} \mu_2^2 \mathfrak{E}_1 - 18 \eta^2 \text{ep} \\
& \mu_2^2 \mathfrak{E}_1 - 3 \text{ep} \mathfrak{E}_2 - 18 \eta \text{ep} \mathfrak{E}_2 - 18 \eta^2 \text{ep} \mathfrak{E}_2 - 6 \text{ep} \mu_1 \mathfrak{E}_2 - 42 \eta \\
& \text{ep} \mu_1 \mathfrak{E}_2 - 72 \eta^2 \text{ep} \mu_1 \mathfrak{E}_2 - 60 \eta^3 \text{ep} \mu_1 \mathfrak{E}_2 - 30 \eta^4 \text{ep} \mu_1 \mathfrak{E}_2 - 3 \\
& \text{ep} \mu_1^2 \mathfrak{E}_2 - 24 \eta \text{ep} \mu_1^2 \mathfrak{E}_2 - 42 \eta^2 \text{ep} \mu_1^2 \mathfrak{E}_2 - 20 \eta^3 \text{ep} \mu_1^2
\end{aligned}$$

$$\begin{aligned}
& \mathfrak{z}^2 - 6 \, \Theta \rho \, \mu^2 \mathfrak{z}^2 - 36 \, \eta \, \Theta \rho \, \mu^2 \mathfrak{z}^2 - 36 \, \eta^2 \, \Theta \rho \, \mu^2 \mathfrak{z}^2 - 6 \, \Theta \rho \, \mu^1 \mu^2 \\
& \mathfrak{z}^2 - 48 \, \eta \, \Theta \rho \, \mu^1 \mu^2 \mathfrak{z}^2 - 84 \, \eta^2 \, \Theta \rho \, \mu^1 \mu^2 \mathfrak{z}^2 - 40 \, \eta^3 \, \Theta \rho \, \mu^1 \mu^2 \mathfrak{z}^2 - 3 \\
& \Theta \rho \, \mu^2{}^2 \mathfrak{z}^2 - 18 \, \eta \, \Theta \rho \, \mu^2{}^2 \mathfrak{z}^2 - 18 \, \eta^2 \, \Theta \rho \, \mu^2{}^2 \mathfrak{z}^2 - w^2 \, (-1 + \eta)^2 \\
& (100 \, \eta^4 \, \mu^1{}^2 + 8 \, \eta \, (41 \, \mu^1{}^2 - 9 \, (1 + \mu^2)^2 - 3 \, \mu^1 \, (8 + 9 \, \mu^2)) + \\
& 2 \times (5 \, \mu^1{}^2 - 9 \, (1 + \mu^2)^2 - 2 \, \mu^1 \, (9 + 17 \, \mu^2)) + 6 \, \eta \, \Theta \rho \, (24 + 9 \, \mathfrak{z}^1 + 9 \, \mathfrak{z}^2 + \\
& 27 \, \mu^1 \, (2 + \mathfrak{z}^1 + \mathfrak{z}^2) + 14 \, \mu^1{}^2 \, (2 + \mathfrak{z}^1 + \mathfrak{z}^2) + 18 \, \mu^2 \, (3 + \mathfrak{z}^1 + \mathfrak{z}^2) + \\
& \mu^2{}^2 \, (28 + 9 \, \mathfrak{z}^1 + 9 \, \mathfrak{z}^2) + 2 \, \mu^1 \, \mu^2 \, (53 + 14 \, \mathfrak{z}^1 + 14 \, \mathfrak{z}^2)) + \\
& \Theta \rho \, (9 \times (2 + \mathfrak{z}^1 + \mathfrak{z}^2) + 24 \, \mu^1 \, (2 + \mathfrak{z}^1 + \mathfrak{z}^2) + 13 \, \mu^1{}^2 \, (2 + \mathfrak{z}^1 + \mathfrak{z}^2) + \\
& 6 \, \mu^2 \, (8 + 3 \, \mathfrak{z}^1 + 3 \, \mathfrak{z}^2) + \mu^2{}^2 \, (26 + 9 \, \mathfrak{z}^1 + 9 \, \mathfrak{z}^2) + \\
& \mu^1 \, \mu^2 \, (80 + 26 \, \mathfrak{z}^1 + 26 \, \mathfrak{z}^2)) + 4 \, \eta^3 \, (8 \, \mu^1 \, (-3 + 20 \, \mu^1 - \mu^2) + \\
& 5 \, \Theta \rho \, (2 \times (3 + 3 \, \mu^2 + \mu^2{}^2) + 3 \, \mu^1 \, (2 + \mathfrak{z}^1 + \mathfrak{z}^2) + \mu^1{}^2 \, (2 + \mathfrak{z}^1 + \mathfrak{z}^2) + \\
& 2 \, \mu^1 \, \mu^2 \, (13 + \mathfrak{z}^1 + \mathfrak{z}^2))) + 6 \, \eta^2 \, (-9 - 42 \, \mu^1 + \\
& 147 \, \mu^1{}^2 - 18 \, \mu^2 - 26 \, \mu^1 \, \mu^2 - 9 \, \mu^2{}^2 + \Theta \rho \, (42 + 9 \, \mathfrak{z}^1 + 9 \, \mathfrak{z}^2 + \\
& 36 \, \mu^1 \, (2 + \mathfrak{z}^1 + \mathfrak{z}^2) + 17 \, \mu^1{}^2 \, (2 + \mathfrak{z}^1 + \mathfrak{z}^2) + 18 \, \mu^2 \, (4 + \mathfrak{z}^1 + \mathfrak{z}^2) + \\
& \mu^2{}^2 \, (34 + 9 \, \mathfrak{z}^1 + 9 \, \mathfrak{z}^2) + 2 \, \mu^1 \, \mu^2 \, (92 + 17 \, \mathfrak{z}^1 + 17 \, \mathfrak{z}^2))) + w \\
& (-1 + \eta) \times (-6 \times (3 \, \mu^1{}^2 + 3 \, (1 + \mu^2)^2 + \mu^1 \, (6 + 8 \, \mu^2)) + \\
& 8 \, \eta \, (3 \, \mu^1{}^2 - 9 \, (1 + \mu^2)^2 - \mu^1 \, (20 + 27 \, \mu^2)) + \\
& 10 \, \eta^4 \, (4 \, \mu^1 \, (-1 + 5 \, \mu^1) + 6 \, \Theta \rho \, (3 + \mu^2) + 3 \, \Theta \rho \, \mu^1 \, (2 + 10 \, \mu^2 + \mathfrak{z}^1 + \mathfrak{z}^2)) + \\
& 6 \, \eta \, \Theta \rho \, (9 \times (2 + \mathfrak{z}^1 + \mathfrak{z}^2) + 24 \, \mu^1 \, (2 + \mathfrak{z}^1 + \mathfrak{z}^2) + \\
& 13 \, \mu^1{}^2 \, (2 + \mathfrak{z}^1 + \mathfrak{z}^2) + 6 \, \mu^2 \, (8 + 3 \, \mathfrak{z}^1 + 3 \, \mathfrak{z}^2) + \\
& \mu^2{}^2 \, (26 + 9 \, \mathfrak{z}^1 + 9 \, \mathfrak{z}^2) + \mu^1 \, \mu^2 \, (80 + 26 \, \mathfrak{z}^1 + 26 \, \mathfrak{z}^2)) + \\
& 8 \, \eta^3 \, (2 \, \mu^1 \, (-10 + 35 \, \mu^1 - 4 \, \mu^2) + 5 \, \Theta \rho \, (2 \times (3 + 3 \, \mu^2 + \mu^2{}^2) + \\
& 3 \, \mu^1 \, (2 + \mathfrak{z}^1 + \mathfrak{z}^2) + \mu^1{}^2 \, (2 + \mathfrak{z}^1 + \mathfrak{z}^2) + 2 \, \mu^1 \, \mu^2 \, (13 + \mathfrak{z}^1 + \mathfrak{z}^2))) + \\
& 6 \, \eta^2 \, (-9 - 38 \, \mu^1 + 69 \, \mu^1{}^2 - 18 \, \mu^2 - 34 \, \mu^1 \, \mu^2 - 9 \, \mu^2{}^2 + \Theta \rho \, \\
& (30 + 9 \, \mathfrak{z}^1 + 9 \, \mathfrak{z}^2 + 38 \, \mu^1 \, (2 + \mathfrak{z}^1 + \mathfrak{z}^2) + 19 \, \mu^1{}^2 \, (2 + \mathfrak{z}^1 + \mathfrak{z}^2) + \\
& 2 \, \mu^2 \, (38 + 9 \, \mathfrak{z}^1 + 9 \, \mathfrak{z}^2) + \mu^2{}^2 \, (38 + 9 \, \mathfrak{z}^1 + 9 \, \mathfrak{z}^2) + \\
& 2 \, \mu^1 \, \mu^2 \, (98 + 19 \, \mathfrak{z}^1 + 19 \, \mathfrak{z}^2))) + \Theta \rho \, (11 \, \mu^1{}^2 \, (2 + \mathfrak{z}^1 + \mathfrak{z}^2) + \\
& (1 + \mu^2) \times (9 \times (2 + \mathfrak{z}^1 + \mathfrak{z}^2) + \mu^2 \, (22 + 9 \, \mathfrak{z}^1 + 9 \, \mathfrak{z}^2)) + \\
& \mu^1 \, (20 \times (2 + \mathfrak{z}^1 + \mathfrak{z}^2) + \mu^2 \, (48 + 22 \, \mathfrak{z}^1 + 22 \, \mathfrak{z}^2)))) + w^3 \\
& (-1 + \eta)^3 \, (78 \, \mu^1{}^2 + 240 \, \eta^3 \, \mu^1{}^2 - 6 \, (1 + \mu^2)^2 - 12 \, \mu^1 \, (1 + 3 \, \mu^2) + \\
& 8 \, \eta \, (66 \, \mu^1{}^2 - 3 \, (1 + \mu^2)^2 - 5 \, \mu^1 \, (2 + \mu^2)) + \\
& \Theta \rho \, (5 \, \mu^1{}^2 \, (2 + \mathfrak{z}^1 + \mathfrak{z}^2) + (1 + \mu^2)^2 \, (10 + 3 \, \mathfrak{z}^1 + 3 \, \mathfrak{z}^2) + \\
& 2 \, \mu^1 \, (5 \times (2 + \mathfrak{z}^1 + \mathfrak{z}^2) + \mu^2 \, (22 + 5 \, \mathfrak{z}^1 + 5 \, \mathfrak{z}^2))) + \\
& 6 \, \eta \, \Theta \rho \, (5 \, \mu^1{}^2 \, (2 + \mathfrak{z}^1 + \mathfrak{z}^2) + (1 + \mu^2)^2 \, (10 + 3 \, \mathfrak{z}^1 + 3 \, \mathfrak{z}^2) + \\
& 2 \, \mu^1 \, (5 \times (2 + \mathfrak{z}^1 + \mathfrak{z}^2) + \mu^2 \, (22 + 5 \, \mathfrak{z}^1 + 5 \, \mathfrak{z}^2))) + \\
& 6 \, \eta^2 \, (115 \, \mu^1{}^2 - 3 \, (1 + \mu^2)^2 - 2 \, \mu^1 \, (7 + 3 \, \mu^2) + \Theta \rho \, \\
& (5 \, \mu^1{}^2 \, (2 + \mathfrak{z}^1 + \mathfrak{z}^2) + (1 + \mu^2)^2 \, (10 + 3 \, \mathfrak{z}^1 + 3 \, \mathfrak{z}^2) + \\
& 2 \, \mu^1 \, (5 \times (2 + \mathfrak{z}^1 + \mathfrak{z}^2) + \mu^2 \, (22 + 5 \, \mathfrak{z}^1 + 5 \, \mathfrak{z}^2)))))) + \\
& 2 \, x^3 \, (-1 + \eta)^3 \, ((-1 + \eta) \, \Theta \rho \, (-20 \, \eta^2 - 80 \, \eta^3 - 70 \, \eta^4 - 3 \, \eta \mathfrak{t} - 10 \, \eta \mathfrak{t} \, \mu^1 - 32 \\
& \eta \, \eta \mathfrak{t} \, \mu^1 - 40 \, \eta^2 \, \eta \mathfrak{t} \, \mu^1 + 7 \, \eta \mathfrak{t} \, \mu^1{}^2 + 80 \, \eta \, \eta \mathfrak{t} \, \mu^1{}^2 + 100 \, \eta^2 \, \eta \mathfrak{t} \, \mu^1{}^2 - 4 \\
& \mu^2 - 32 \, \eta \, \mu^2 - 40 \, \eta^2 \, \mu^2 - 6 \, \eta \mathfrak{t} \, \mu^2 - 4 \, \mu^1 \, \mu^2 + 10 \, w^5 \, (-1 + \eta)^5 \\
& \mu^1 \, \mu^2 - 112 \, \eta \, \mu^1 \, \mu^2 - 440 \, \eta^2 \, \mu^1 \, \mu^2 - 400 \, \eta^3 \, \mu^1 \, \mu^2 - 14 \, \eta \mathfrak{t} \, \mu^1 \\
& \mu^2 - 16 \, \eta \, \eta \mathfrak{t} \, \mu^1 \, \mu^2 - 2 \, \mu^2{}^2 - 16 \, \eta \, \mu^2{}^2 - 20 \, \eta^2 \, \mu^2{}^2 - 3 \, \eta \mathfrak{t} \, \mu^2{}^2 - 6 \, w^4 \\
& (-1 + \eta)^4 \, (-5 \, \eta \mathfrak{t} \, \mu^1{}^2 + \mu^2 \, (4 \times (3 + 5 \, \eta) \, \mu^1 + \mu^2)) + w^3 \, (-1 + \eta)^3
\end{aligned}$$

$$\begin{aligned}
& \left( 4 - 115 \eta t \mu_1^2 + 300 \eta^2 \mu_1 \mu_2 + 2 \times (4 + 83 \mu_1) \mu_2 + 14 \mu_2^2 + 3 \eta t (1 + \mu_2)^2 + \right. \\
& \quad \left. 2 \eta t \mu_1 (7 + 3 \mu_2) + 8 \eta (1 - 15 \eta t \mu_1^2 + 66 \mu_1 \mu_2 + 3 \mu_2^2) \right) - w^2 \\
& (-1 + \eta)^2 (6 + 200 \eta^3 \mu_1 \mu_2 + 8 \times (3 + 20 \mu_1) \mu_2 + 12 \mu_2^2 - \\
& \quad 20 \eta^2 (-3 + 5 \eta t \mu_1^2 - 52 \mu_1 \mu_2 - \mu_2^2) + \\
& \quad 8 \eta (6 + 6 \mu_2 + 111 \mu_1 \mu_2 + 8 \mu_2^2 + 2 \eta t \mu_1 (3 - 20 \mu_1 + \mu_2)) + \\
& \quad \eta t (-147 \mu_1^2 + 9 (1 + \mu_2)^2 + \mu_1 (42 + 26 \mu_2))) + w \\
& (-1 + \eta) \times (2 \mu_2 (10 + 30 \mu_1 + 3 \mu_2) + 120 \eta^3 (1 + 5 \mu_1 \mu_2) - \\
& \quad 20 \eta^2 (-6 + 2 \eta t \mu_1 (-1 + 5 \mu_1) - 2 \mu_2 - 59 \mu_1 \mu_2 - 2 \mu_2^2) + \\
& \quad 8 \eta (3 + 10 \mu_2 + 74 \mu_1 \mu_2 + 7 \mu_2^2 + \eta t \mu_1 (10 - 35 \mu_1 + 4 \mu_2)) + \\
& \quad \eta t (-69 \mu_1^2 + 9 (1 + \mu_2)^2 + \mu_1 (38 + 34 \mu_2))) - \\
& (-1 + \eta t) \Theta (6 + 9 \eta - 6 \Theta p - 12 \eta \Theta p - 20 \eta^2 \Theta p - 80 \eta^3 \Theta p - 70 \eta^4 \\
& \quad \Theta p + 12 \mu_1 + 30 \eta \mu_1 + 48 \eta^2 \mu_1 + 40 \eta^3 \mu_1 - 14 \Theta p \mu_1 - 48 \eta \\
& \quad \Theta p \mu_1 - 60 \eta^2 \Theta p \mu_1 - 40 \eta^3 \Theta p \mu_1 + 6 \mu_1^2 + 10 w^5 (-1 + \eta)^5 \\
& \quad \mu_1^2 - 21 \eta \mu_1^2 - 120 \eta^2 \mu_1^2 - 100 \eta^3 \mu_1^2 - 8 \Theta p \mu_1^2 - 28 \eta \\
& \quad \Theta p \mu_1^2 - 20 \eta^2 \Theta p \mu_1^2 + 12 \mu_2 + 18 \eta \mu_2 - 14 \Theta p \mu_2 - 48 \eta \Theta p \\
& \quad \mu_2 - 60 \eta^2 \Theta p \mu_2 - 40 \eta^3 \Theta p \mu_2 + 16 \mu_1 \mu_2 + 42 \eta \mu_1 \mu_2 + 24 \eta^2 \\
& \quad \mu_1 \mu_2 - 18 \Theta p \mu_1 \mu_2 - 112 \eta \Theta p \mu_1 \mu_2 - 260 \eta^2 \Theta p \mu_1 \mu_2 - 200 \\
& \quad \eta^3 \Theta p \mu_1 \mu_2 + 6 \mu_2^2 + 9 \eta \mu_2^2 - 8 \Theta p \mu_2^2 - 28 \eta \Theta p \mu_2^2 - 20 \eta^2 \Theta p \\
& \quad \mu_2^2 - 6 w^4 (-1 + \eta)^4 \mu_1 (3 \times (4 + 5 \eta) \mu_1 + \mu_2) - 3 \Theta p \mathfrak{E}1 - 6 \eta \\
& \quad \Theta p \mathfrak{E}1 - 7 \Theta p \mu_1 \mathfrak{E}1 - 24 \eta \Theta p \mu_1 \mathfrak{E}1 - 30 \eta^2 \Theta p \mu_1 \mathfrak{E}1 - 20 \eta^3 \Theta p \\
& \quad \mu_1 \mathfrak{E}1 - 4 \Theta p \mu_1^2 \mathfrak{E}1 - 14 \eta \Theta p \mu_1^2 \mathfrak{E}1 - 10 \eta^2 \Theta p \mu_1^2 \mathfrak{E}1 - 6 \Theta p \\
& \quad \mu_2 \mathfrak{E}1 - 12 \eta \Theta p \mu_2 \mathfrak{E}1 - 8 \Theta p \mu_1 \mu_2 \mathfrak{E}1 - 28 \eta \Theta p \mu_1 \mu_2 \mathfrak{E}1 - 20 \\
& \quad \eta^2 \Theta p \mu_1 \mu_2 \mathfrak{E}1 - 3 \Theta p \mu_2^2 \mathfrak{E}1 - 6 \eta \Theta p \mu_2^2 \mathfrak{E}1 - 3 \Theta p \mathfrak{E}2 - 6 \eta \\
& \quad \Theta p \mathfrak{E}2 - 7 \Theta p \mu_1 \mathfrak{E}2 - 24 \eta \Theta p \mu_1 \mathfrak{E}2 - 30 \eta^2 \Theta p \mu_1 \mathfrak{E}2 - 20 \eta^3 \Theta p \\
& \quad \mu_1 \mathfrak{E}2 - 4 \Theta p \mu_1^2 \mathfrak{E}2 - 14 \eta \Theta p \mu_1^2 \mathfrak{E}2 - 10 \eta^2 \Theta p \mu_1^2 \mathfrak{E}2 - 6 \Theta p \\
& \quad \mu_2 \mathfrak{E}2 - 12 \eta \Theta p \mu_2 \mathfrak{E}2 - 8 \Theta p \mu_1 \mu_2 \mathfrak{E}2 - 28 \eta \Theta p \mu_1 \mu_2 \mathfrak{E}2 - 20 \\
& \quad \eta^2 \Theta p \mu_1 \mu_2 \mathfrak{E}2 - 3 \Theta p \mu_2^2 \mathfrak{E}2 - 6 \eta \Theta p \mu_2^2 \mathfrak{E}2 - w^2 (-1 + \eta)^2 \\
& \quad (82 \mu_1^2 + 100 \eta^3 \mu_1^2 - 18 (1 + \mu_2)^2 - 6 \mu_1 (8 + 9 \mu_2) + \Theta p (24 + 9 \mathfrak{E}1 + 9 \mathfrak{E}2 + \\
& \quad 27 \mu_1 (2 + \mathfrak{E}1 + \mathfrak{E}2) + 14 \mu_1^2 (2 + \mathfrak{E}1 + \mathfrak{E}2) + 18 \mu_2 (3 + \mathfrak{E}1 + \mathfrak{E}2) + \\
& \quad \mu_2^2 (28 + 9 \mathfrak{E}1 + 9 \mathfrak{E}2) + 2 \mu_1 \mu_2 (53 + 14 \mathfrak{E}1 + 14 \mathfrak{E}2)) + \\
& \quad 2 \eta^2 (12 \mu_1 (-3 + 20 \mu_1 - \mu_2) + 5 \Theta p (2 \times (3 + 3 \mu_2 + \mu_2^2) + \\
& \quad 3 \mu_1 (2 + \mathfrak{E}1 + \mathfrak{E}2) + \mu_1^2 (2 + \mathfrak{E}1 + \mathfrak{E}2) + 2 \mu_1 \mu_2 (13 + \mathfrak{E}1 + \mathfrak{E}2))) + \\
& \quad \eta (441 \mu_1^2 - 27 (1 + \mu_2)^2 - 6 \mu_1 (21 + 13 \mu_2) + 2 \Theta p (42 + 9 \mathfrak{E}1 + 9 \mathfrak{E}2 + \\
& \quad 36 \mu_1 (2 + \mathfrak{E}1 + \mathfrak{E}2) + 17 \mu_1^2 (2 + \mathfrak{E}1 + \mathfrak{E}2) + 18 \mu_2 (4 + \mathfrak{E}1 + \mathfrak{E}2) + \\
& \quad \mu_2^2 (34 + 9 \mathfrak{E}1 + 9 \mathfrak{E}2) + 2 \mu_1 \mu_2 (92 + 17 \mathfrak{E}1 + 17 \mathfrak{E}2))) + w \\
& (-1 + \eta) \times (6 \mu_1^2 - 18 (1 + \mu_2)^2 - 2 \mu_1 (20 + 27 \mu_2) + 20 \eta^3 \\
& \quad (2 \mu_1 (-1 + 5 \mu_1) + 2 \Theta p (3 + \mu_2) + \Theta p \mu_1 (2 + 10 \mu_2 + \mathfrak{E}1 + \mathfrak{E}2)) + \\
& \quad \Theta p (9 \times (2 + \mathfrak{E}1 + \mathfrak{E}2) + 24 \mu_1 (2 + \mathfrak{E}1 + \mathfrak{E}2) + \\
& \quad 13 \mu_1^2 (2 + \mathfrak{E}1 + \mathfrak{E}2) + 6 \mu_2 (8 + 3 \mathfrak{E}1 + 3 \mathfrak{E}2) + \\
& \quad \mu_2^2 (26 + 9 \mathfrak{E}1 + 9 \mathfrak{E}2) + \mu_1 \mu_2 (80 + 26 \mathfrak{E}1 + 26 \mathfrak{E}2)) + \\
& \quad 4 \eta^2 (3 \mu_1 (-10 + 35 \mu_1 - 4 \mu_2) + 5 \Theta p (2 \times (3 + 3 \mu_2 + \mu_2^2) + \\
& \quad 3 \mu_1 (2 + \mathfrak{E}1 + \mathfrak{E}2) + \mu_1^2 (2 + \mathfrak{E}1 + \mathfrak{E}2) + 2 \mu_1 \mu_2 (13 + \mathfrak{E}1 + \mathfrak{E}2))) + \\
& \quad \eta (3 \times (69 \mu_1^2 - 9 (1 + \mu_2)^2 - 2 \mu_1 (19 + 17 \mu_2)) + 2 \Theta p \\
& \quad (30 + 9 \mathfrak{E}1 + 9 \mathfrak{E}2 + 38 \mu_1 (2 + \mathfrak{E}1 + \mathfrak{E}2) + 19 \mu_1^2 (2 + \mathfrak{E}1 + \mathfrak{E}2) +
\end{aligned}$$



$$\begin{aligned}
& 2 \mu_2 (38 + 9 \mathfrak{e}_1 + 9 \mathfrak{e}_2) + \mu_2^2 (38 + 9 \mathfrak{e}_1 + 9 \mathfrak{e}_2) + \\
& 2 \mu_1 \mu_2 (98 + 19 \mathfrak{e}_1 + 19 \mathfrak{e}_2) \Big) \Big) + w^3 \\
& (-1 + \eta)^3 \Big( 132 \mu_1^2 + 180 \eta^2 \mu_1^2 - 6 (1 + \mu_2)^2 - 10 \mu_1 (2 + \mu_2) + \\
& 5 \theta p \mu_1^2 (2 + \mathfrak{e}_1 + \mathfrak{e}_2) + \theta p (1 + \mu_2)^2 (10 + 3 \mathfrak{e}_1 + 3 \mathfrak{e}_2) + \\
& 2 \theta p \mu_1 (5 \times (2 + \mathfrak{e}_1 + \mathfrak{e}_2) + \mu_2 (22 + 5 \mathfrak{e}_1 + 5 \mathfrak{e}_2)) + \\
& \eta (345 \mu_1^2 - 9 (1 + \mu_2)^2 - 6 \mu_1 (7 + 3 \mu_2) + \\
& 2 \theta p (5 \mu_1^2 (2 + \mathfrak{e}_1 + \mathfrak{e}_2) + (1 + \mu_2)^2 (10 + 3 \mathfrak{e}_1 + 3 \mathfrak{e}_2) + \\
& 2 \mu_1 (5 \times (2 + \mathfrak{e}_1 + \mathfrak{e}_2) + \mu_2 (22 + 5 \mathfrak{e}_1 + 5 \mathfrak{e}_2))) \Big) \Big) \Big) - \\
& \theta p (4 w^5 (-1 + \eta)^6 (-\eta t \mu_1 + \eta \mu_2) (5 \eta^2 \mu_1 - \mu_2 + \eta (7 \mu_1 + \mu_2)) - \\
& 12 w^4 (-1 + \eta)^5 (1 + \eta) (-\eta t \mu_1 + \eta \mu_2) (5 \eta^2 \mu_1 - \mu_2 + \eta (7 \mu_1 + \mu_2)) - \\
& \eta (1 + \eta)^2 (4 \eta^5 - 6 \eta t (1 + \mu_1 + \mu_2)^2 + \eta^4 (-4 - 4 \times (-1 + \eta t) \theta l + 40 \mu_1 \mu_2) + \eta \\
& (3 \theta l (1 + \mu_1 + \mu_2)^2 (2 + \mathfrak{e}_1 + \mathfrak{e}_2) + \eta t (6 \mu_1^2 + 6 (1 + \mu_2)^2 + \\
& 4 \mu_1 (3 + \mu_2) - 3 \theta l (1 + \mu_1 + \mu_2)^2 (2 + \mathfrak{e}_1 + \mathfrak{e}_2))) + 2 \\
& \eta^3 (2 \theta l \mu_2 + 2 \mu_2 (2 - 8 \mu_1 + \mu_2) + \theta l \mu_1 (2 + 10 \mu_2 + \mathfrak{e}_1 + \mathfrak{e}_2) - \\
& \eta t (10 \mu_1^2 + 2 \theta l \mu_2 + \mu_1 (-4 + \theta l (2 + 10 \mu_2 + \mathfrak{e}_1 + \mathfrak{e}_2))) - 2 \\
& \eta^2 (2 \mu_2 (2 + 2 \mu_1 + \mu_2) - \theta l (2 \mu_2 (1 + \mu_2) + \mu_1^2 (2 + \mathfrak{e}_1 + \mathfrak{e}_2) + \\
& \mu_1 (2 + \mathfrak{e}_1 + \mathfrak{e}_2 + 2 \mu_2 (3 + \mathfrak{e}_1 + \mathfrak{e}_2))) + \\
& \eta t (2 \theta l \mu_2 (1 + \mu_2) + \mu_1^2 (-10 + \theta l (2 + \mathfrak{e}_1 + \mathfrak{e}_2)) + \\
& \mu_1 (4 - 4 \mu_2 + \theta l (2 + \mathfrak{e}_1 + \mathfrak{e}_2 + 2 \mu_2 (3 + \mathfrak{e}_1 + \mathfrak{e}_2)))) \Big) \Big) + \\
& w^3 (-1 + \eta)^3 (60 \eta^6 \mu_1 \mu_2 - 12 \eta t \mu_1 \mu_2 + \eta^5 (4 - 60 \eta t \mu_1^2 + 204 \mu_1 \mu_2 + \\
& 12 \mu_2^2) + 6 \eta (2 \mu_2^2 + \eta t (13 \mu_1^2 - (1 + \mu_2)^2 - 2 \mu_1 (1 + 2 \mu_2))) - \eta^2 \\
& (4 + 16 \times (1 + 7 \mu_1) \mu_2 - \theta l (5 \mu_1^2 (2 + \mathfrak{e}_1 + \mathfrak{e}_2) + (1 + \mu_2)^2 (10 + \\
& 3 \mathfrak{e}_1 + 3 \mathfrak{e}_2) + 2 \mu_1 (5 \times (2 + \mathfrak{e}_1 + \mathfrak{e}_2) + \mu_2 (22 + 5 \mathfrak{e}_1 + 5 \mathfrak{e}_2))) + \\
& \eta t (-186 \mu_1^2 + 6 (1 + \mu_2)^2 - 4 \mu_1 (-7 + 4 \mu_2) + 5 \theta l \mu_1^2 \\
& (2 + \mathfrak{e}_1 + \mathfrak{e}_2) + \theta l (1 + \mu_2)^2 (10 + 3 \mathfrak{e}_1 + 3 \mathfrak{e}_2) + \\
& 2 \theta l \mu_1 (5 \times (2 + \mathfrak{e}_1 + \mathfrak{e}_2) + \mu_2 (22 + 5 \mathfrak{e}_1 + 5 \mathfrak{e}_2))) \Big) - 2 \eta^3 \\
& (2 + 110 \mu_1 \mu_2 + 20 \mu_2^2 - \theta l (5 \mu_1^2 (2 + \mathfrak{e}_1 + \mathfrak{e}_2) + (1 + \mu_2)^2 (10 + \\
& 3 \mathfrak{e}_1 + 3 \mathfrak{e}_2) + 2 \mu_1 (5 \times (2 + \mathfrak{e}_1 + \mathfrak{e}_2) + \mu_2 (22 + 5 \mathfrak{e}_1 + 5 \mathfrak{e}_2))) + \\
& \eta t (17 \mu_1^2 - 3 (1 + \mu_2)^2 - 2 \mu_1 (3 + 2 \mu_2) + \theta l (5 \mu_1^2 \\
& (2 + \mathfrak{e}_1 + \mathfrak{e}_2) + (1 + \mu_2)^2 (10 + 3 \mathfrak{e}_1 + 3 \mathfrak{e}_2) + \\
& 2 \mu_1 (5 \times (2 + \mathfrak{e}_1 + \mathfrak{e}_2) + \mu_2 (22 + 5 \mathfrak{e}_1 + 5 \mathfrak{e}_2))) \Big) \Big) + \\
& \eta^4 (4 + 4 \times (4 + 17 \mu_1) \mu_2 + 16 \mu_2^2 + 5 \theta l \mu_1^2 (2 + \mathfrak{e}_1 + \mathfrak{e}_2) + \\
& \theta l (1 + \mu_2)^2 (10 + 3 \mathfrak{e}_1 + 3 \mathfrak{e}_2) + 2 \theta l \mu_1 (5 \times (2 + \mathfrak{e}_1 + \mathfrak{e}_2) + \\
& \mu_2 (22 + 5 \mathfrak{e}_1 + 5 \mathfrak{e}_2)) - \eta t (170 \mu_1^2 - 6 (1 + \mu_2)^2 - 4 \mu_1 (7 + 3 \mu_2) + \\
& \theta l (5 \mu_1^2 (2 + \mathfrak{e}_1 + \mathfrak{e}_2) + (1 + \mu_2)^2 (10 + 3 \mathfrak{e}_1 + 3 \mathfrak{e}_2) + \\
& 2 \mu_1 (5 \times (2 + \mathfrak{e}_1 + \mathfrak{e}_2) + \mu_2 (22 + 5 \mathfrak{e}_1 + 5 \mathfrak{e}_2))) \Big) \Big) \Big) - \\
& w^2 (-1 + \eta)^2 (1 + \eta) \times (20 \eta^6 \mu_1 \mu_2 - 4 \eta t \mu_1 \mu_2 + 4 \eta^5 (3 - 5 \eta t \mu_1^2 + \\
& 42 \mu_1 \mu_2 + \mu_2^2) + 2 \eta (2 \mu_2^2 + \eta t (5 \mu_1^2 - 9 (1 + \mu_2)^2 - 6 \mu_1 (3 + 5 \mu_2))) - \\
& 2 \eta^4 (4 \eta t \mu_1 (-3 + 15 \mu_1 - \mu_2) - 2 \mu_2 (6 + 17 \mu_1 + 6 \mu_2) + \\
& (-1 + \eta t) \theta l (2 \times (3 + 3 \mu_2 + \mu_2^2) + 3 \mu_1 (2 + \mathfrak{e}_1 + \mathfrak{e}_2) + \\
& \mu_1^2 (2 + \mathfrak{e}_1 + \mathfrak{e}_2) + 2 \mu_1 \mu_2 (13 + \mathfrak{e}_1 + \mathfrak{e}_2))) + \eta^2 \\
& (-8 \times (3 + 8 \mu_1) \mu_2 + 4 \eta t \mu_1 (-6 + 36 \mu_1 + 5 \mu_2) - (-1 + \eta t) \theta l \\
& (9 \times (2 + \mathfrak{e}_1 + \mathfrak{e}_2) + 24 \mu_1 (2 + \mathfrak{e}_1 + \mathfrak{e}_2) + 13 \mu_1^2 (2 + \mathfrak{e}_1 + \mathfrak{e}_2) +
\end{aligned}$$

$$\begin{aligned}
& 6 \mu_2 (8 + 3 \mu_1 + 3 \mu_2) + \mu_2^2 (26 + 9 \mu_1 + 9 \mu_2) + \\
& \mu_1 \mu_2 (80 + 26 \mu_1 + 26 \mu_2) \Big) + \eta^3 \Big( -4 \times (3 + 48 \mu_1 \mu_2 + 8 \mu_2^2) + \\
& 3 \theta_l (5 \mu_1^2 (2 + \mu_1 + \mu_2) + (1 + \mu_2)^2 (10 + 3 \mu_1 + 3 \mu_2) + \\
& 2 \mu_1 (5 \times (2 + \mu_1 + \mu_2) + \mu_2 (22 + 5 \mu_1 + 5 \mu_2)) \Big) - \\
& \eta t \Big( 2 \times (7 \mu_1^2 - 18 \mu_1 (1 + \mu_2) - 9 (1 + \mu_2)^2) + 3 \theta_l \\
& (5 \mu_1^2 (2 + \mu_1 + \mu_2) + (1 + \mu_2)^2 (10 + 3 \mu_1 + 3 \mu_2) + \\
& 2 \mu_1 (5 \times (2 + \mu_1 + \mu_2) + \mu_2 (22 + 5 \mu_1 + 5 \mu_2)) \Big) \Big) + w (-1 + \eta) \\
& \eta (12 \eta^6 (1 + 5 \mu_1 \mu_2) - 6 \eta t (3 \mu_1^2 + 3 (1 + \mu_2)^2 + \mu_1 (6 + 8 \mu_2)) - \\
& 4 \eta^4 (3 - 8 \eta t \mu_1 + 25 \eta t \mu_1^2 - 8 \mu_2 - 15 \mu_1 \mu_2 - 4 \eta t \mu_1 \mu_2 - 5 \mu_2^2 + \\
& (-1 + \eta t) \theta_l (2 \times (3 + 3 \mu_2 + \mu_2^2) + 3 \mu_1 (2 + \mu_1 + \mu_2) + \\
& \mu_1^2 (2 + \mu_1 + \mu_2) + 2 \mu_1 \mu_2 (13 + \mu_1 + \mu_2)) \Big) - 2 \\
& \eta^5 (4 \eta t \mu_1 (-1 + 5 \mu_1) - 2 \times (3 + 2 \mu_2 + 44 \mu_1 \mu_2 + 2 \mu_2^2) + \\
& (-1 + \eta t) \theta_l (2 \times (3 + \mu_2) + \mu_1 (2 + 10 \mu_2 + \mu_1 + \mu_2)) \Big) + \eta^3 \\
& (-4 \times (3 + 44 \mu_1 \mu_2 + 4 \mu_2^2) + 2 \eta t (\mu_1^2 + 9 (1 + \mu_2)^2 + 2 \mu_1 (9 + 13 \mu_2)) + \\
& \theta_l (30 + 9 \mu_1 + 9 \mu_2 + 38 \mu_1 (2 + \mu_1 + \mu_2) + 19 \mu_1^2 (2 + \mu_1 + \mu_2) + \\
& 2 \mu_2 (38 + 9 \mu_1 + 9 \mu_2) + \mu_2^2 (38 + 9 \mu_1 + 9 \mu_2) + \\
& 2 \mu_1 \mu_2 (98 + 19 \mu_1 + 19 \mu_2) \Big) - \eta t \theta_l (30 + 9 \mu_1 + 9 \mu_2 + \\
& 38 \mu_1 (2 + \mu_1 + \mu_2) + 19 \mu_1^2 (2 + \mu_1 + \mu_2) + 2 \mu_2 (38 + 9 \mu_1 + 9 \mu_2) + \\
& \mu_2^2 (38 + 9 \mu_1 + 9 \mu_2) + 2 \mu_1 \mu_2 (98 + 19 \mu_1 + 19 \mu_2) \Big) \Big) - 2 \eta^2 \\
& (2 \mu_2 (8 + 28 \mu_1 + 3 \mu_2) - \theta_l (9 \times (2 + \mu_1 + \mu_2) + 24 \mu_1 (2 + \mu_1 + \mu_2) + \\
& 13 \mu_1^2 (2 + \mu_1 + \mu_2) + 6 \mu_2 (8 + 3 \mu_1 + 3 \mu_2) + \mu_2^2 (26 + 9 \mu_1 + 9 \mu_2) + \\
& \mu_1 \mu_2 (80 + 26 \mu_1 + 26 \mu_2) \Big) + \eta t (-9 - 2 \mu_1 - 63 \mu_1^2 - 18 \mu_2 - \\
& 20 \mu_1 \mu_2 - 9 \mu_2^2 + \theta_l (9 \times (2 + \mu_1 + \mu_2) + 24 \mu_1 (2 + \mu_1 + \mu_2) + \\
& 13 \mu_1^2 (2 + \mu_1 + \mu_2) + 6 \mu_2 (8 + 3 \mu_1 + 3 \mu_2) + \\
& \mu_2^2 (26 + 9 \mu_1 + 9 \mu_2) + \mu_1 \mu_2 (80 + 26 \mu_1 + 26 \mu_2) \Big) \Big) \Big) - \eta \\
& (8 \times (1 + \mu_1) \mu_2 - \theta_l (11 \mu_1^2 (2 + \mu_1 + \mu_2) + (1 + \mu_2) \times \\
& (9 \times (2 + \mu_1 + \mu_2) + \mu_2 (22 + 9 \mu_1 + 9 \mu_2)) + \\
& \mu_1 (20 \times (2 + \mu_1 + \mu_2) + \mu_2 (48 + 22 \mu_1 + 22 \mu_2)) \Big) + \\
& \eta t (-30 \mu_1^2 + 18 (1 + \mu_2)^2 + \mu_1 (44 + 60 \mu_2) + \theta_l (11 \mu_1^2 (2 + \mu_1 + \mu_2) + \\
& (1 + \mu_2) \times (9 \times (2 + \mu_1 + \mu_2) + \mu_2 (22 + 9 \mu_1 + 9 \mu_2)) + \\
& \mu_1 (20 \times (2 + \mu_1 + \mu_2) + \mu_2 (48 + 22 \mu_1 + 22 \mu_2)) \Big) \Big) \Big) \Big) + \\
& 2 \times (-1 + \eta) \times (30 \times (-2 + w) (-1 + w)^2 w^2 \eta^8 \theta_p \mu_1 \mu_2 - (1 + w)^3 \\
& (2 w^2 \eta t \theta_l \mu_1 \mu_2 + 2 w^2 \mu_2 (-\theta_l \mu_1 + \theta_p \mu_2) + \eta t \theta_p \\
& ((-3 + 14 w^2) \mu_1^2 - 3 (1 + \mu_2)^2 + 2 \mu_1 (-3 + (-3 - 3 w + w^2) \mu_2)) \Big) - \\
& 2 \times (-1 + w) \eta^7 (5 (-1 + w)^2 w^2 (-1 + \eta t) \theta_l \mu_1^2 + \theta_p \\
& (-7 + w (11 + 90 \mu_1 \mu_2) + w^2 (-4 + 25 \eta t \mu_1^2 - 80 \mu_1 \mu_2 - 5 \mu_2^2) + \\
& 2 w^4 (5 \eta t \mu_1^2 + 38 \mu_1 \mu_2 - \mu_2^2) + w^3 (-35 \eta t \mu_1^2 - 116 \mu_1 \mu_2 + 7 \mu_2^2) \Big) \Big) - \\
& \eta^2 (\theta_p (-6 \mu_2 (2 + 2 \mu_1 + \mu_2) + \eta t (33 \mu_1^2 + 3 (1 + \mu_2)^2 - 2 \mu_1 (3 + 5 \mu_2)) - \\
& 6 w^4 (5 \eta t \mu_1 (7 \mu_1 + 2 \mu_2) - \mu_2 (34 \mu_1 + 7 \mu_2)) + \\
& 6 w^5 (5 \eta t \mu_1 (3 \mu_1 + \mu_2) + \mu_2 (23 \mu_1 + 9 \mu_2)) + w^3 (4 + 40 \mu_2 - 50 \mu_1 \mu_2 - \\
& 54 \mu_2^2 + \eta t (-477 \mu_1^2 + \mu_1 (82 - 46 \mu_2) + 21 (1 + \mu_2)^2) \Big) - \\
& 18 w^2 (1 + 16 \mu_1 \mu_2 + 3 \mu_2^2 + \eta t (2 \mu_1^2 - 3 (1 + \mu_2)^2 - 2 \mu_1 (3 + 4 \mu_2)) \Big) + \\
& 2 w (-\mu_2 (22 + 82 \mu_1 + 9 \mu_2) + \eta t (87 \mu_1^2 + 18 (1 + \mu_2)^2 +
\end{aligned}$$

$$\begin{aligned}
& \mu_1 (14 + 45 \mu_2) \Big) \Big) + (-1 + \eta t) \operatorname{el} \left( 6 \mu_1^2 + 6 (1 + \mu_2)^2 + \right. \\
& 30 w^5 \mu_1 (2 \mu_1 + \mu_2) + 4 \mu_1 (3 + 4 \mu_2) + 6 w^4 \mu_1 (16 \mu_1 + 5 \mu_2) - \\
& w^3 \left( 15 \mu_1^2 + 3 (1 + \mu_2)^2 + \mu_1 (-2 + 26 \mu_2) \right) - 3 \operatorname{ep} \left( 4 \mu_1^2 (2 + \mathfrak{e}1 + \mathfrak{e}2) + \right. \\
& (1 + \mu_2) \times (3 \times (2 + \mathfrak{e}1 + \mathfrak{e}2) + \mu_2 (8 + 3 \mathfrak{e}1 + 3 \mathfrak{e}2)) + \\
& \mu_1 (7 \times (2 + \mathfrak{e}1 + \mathfrak{e}2) + 2 \mu_2 (9 + 4 \mathfrak{e}1 + 4 \mathfrak{e}2)) \Big) - w \left( -9 - 22 \mu_1 + \right. \\
& 15 \mu_1^2 - 18 \mu_2 - 30 \mu_1 \mu_2 - 9 \mu_2^2 + 2 \operatorname{ep} \left( 9 \times (2 + \mathfrak{e}1 + \mathfrak{e}2) + 26 \mu_1 \right. \\
& (2 + \mathfrak{e}1 + \mathfrak{e}2) + 14 \mu_1^2 (2 + \mathfrak{e}1 + \mathfrak{e}2) + 4 \mu_1 \mu_2 (24 + 7 \mathfrak{e}1 + 7 \mathfrak{e}2) + \\
& 2 \mu_2 (26 + 9 \mathfrak{e}1 + 9 \mathfrak{e}2) + \mu_2^2 (28 + 9 \mathfrak{e}1 + 9 \mathfrak{e}2) \Big) \Big) - \\
& w^2 \left( 12 \mu_1 (-1 + 6 \mu_1 + \mu_2) + \operatorname{ep} \left( 33 \mu_1 (2 + \mathfrak{e}1 + \mathfrak{e}2) + 16 \mu_1^2 \right. \right. \\
& (2 + \mathfrak{e}1 + \mathfrak{e}2) + 9 \times (4 + \mathfrak{e}1 + \mathfrak{e}2) + 6 \mu_2 (11 + 3 \mathfrak{e}1 + 3 \mathfrak{e}2) + \\
& \mu_2^2 (32 + 9 \mathfrak{e}1 + 9 \mathfrak{e}2) + 2 \mu_1 \mu_2 (79 + 16 \mathfrak{e}1 + 16 \mathfrak{e}2) \Big) \Big) \Big) + \\
& \eta^6 \left( 2 \operatorname{ep} (-5 + 7 \times (-1 + \eta t) \operatorname{el} - 60 \mu_1 \mu_2) - 6 w^4 (\eta t \operatorname{ep} \mu_1 (51 \mu_1 - 2 \mu_2) + \right. \\
& (-1 + \eta t) \operatorname{el} \mu_1 (8 \mu_1 - \mu_2) + \operatorname{ep} (34 \mu_1 - 15 \mu_2) \mu_2) + 2 \\
& w^5 ((-1 + \eta t) \operatorname{el} \mu_1 (18 \mu_1 - \mu_2) + \eta t \operatorname{ep} \mu_1 (53 \mu_1 - \mu_2) + \\
& \operatorname{ep} (141 \mu_1 - 13 \mu_2) \mu_2) + w^2 (4 \times (-1 + \eta t) \operatorname{el} \mu_1 (-3 + 15 \mu_1 - \mu_2) + \\
& \operatorname{ep} (42 - 48 \mu_2 + 492 \mu_1 \mu_2 - 34 \mu_2^2 + 2 \eta t \mu_1 (85 \mu_1 - 8 \times (3 + \mu_2)) + \\
& 5 \times (-1 + \eta t) \operatorname{el} (2 \times (3 + 3 \mu_2 + \mu_2^2) + 3 \mu_1 (2 + \mathfrak{e}1 + \mathfrak{e}2) + \\
& \mu_1^2 (2 + \mathfrak{e}1 + \mathfrak{e}2) + 2 \mu_1 \mu_2 (13 + \mathfrak{e}1 + \mathfrak{e}2) \Big) \Big) \Big) - 2 w \\
& (2 \times (-1 + \eta t) \operatorname{el} \mu_1 (-1 + 5 \mu_1) + \operatorname{ep} (6 + 10 \eta t \mu_1 (-1 + 5 \mu_1) - \\
& 10 \mu_2 - 115 \mu_1 \mu_2 - 10 \mu_2^2 + 3 \times (-1 + \eta t) \operatorname{el} (2 \times (3 + \mu_2) + \\
& \mu_1 (2 + 10 \mu_2 + \mathfrak{e}1 + \mathfrak{e}2)) \Big) \Big) + w^3 (\operatorname{ep} (-20 + (24 - 714 \mu_1) \mu_2 - \\
& 54 \mu_2^2 + 3 \eta t (45 \mu_1^2 + 3 (1 + \mu_2)^2 + 2 \mu_1 (7 + 3 \mu_2)) \Big) - \\
& (-1 + \eta t) \operatorname{el} (25 \mu_1^2 - 3 (1 + \mu_2)^2 - 2 \mu_1 (7 + 3 \mu_2) + \\
& 2 \operatorname{ep} (5 \mu_1^2 (2 + \mathfrak{e}1 + \mathfrak{e}2) + (1 + \mu_2)^2 (10 + 3 \mathfrak{e}1 + 3 \mathfrak{e}2) + \\
& 2 \mu_1 (5 \times (2 + \mathfrak{e}1 + \mathfrak{e}2) + \mu_2 (22 + 5 \mathfrak{e}1 + 5 \mathfrak{e}2)) \Big) \Big) \Big) + \\
& \eta^3 (-\operatorname{ep} (-10 \mu_2 (2 + 10 \mu_1 + \mu_2) + 30 w^4 (\mu_2 (4 \mu_1 + \mu_2) + \eta t \mu_1 \\
& (19 \mu_1 + 4 \mu_2)) + 20 w^5 (\eta t \mu_1 (\mu_1 - 2 \mu_2) - \mu_2 (12 \mu_1 + 5 \mu_2)) + \\
& \eta t (59 \mu_1^2 + 9 (1 + \mu_2)^2 + \mu_1 (-2 + 26 \mu_2)) + 8 w^3 \\
& (2 + 99 \mu_1 \mu_2 + 24 \mu_2^2 + 3 \eta t (7 \mu_1^2 + \mu_1 (-2 + \mu_2) - (1 + \mu_2)^2)) - \\
& 6 w^2 (-1 - 4 \times (4 + 15 \mu_1) \mu_2 - 11 \mu_2^2 + \eta t (86 \mu_1^2 + 3 (1 + \mu_2)^2 + \\
& 2 \mu_1 (-5 + 6 \mu_2)) \Big) \Big) + w (-4 \times (6 + (-8 + 60 \mu_1) \mu_2 + 5 \mu_2^2) + \\
& 2 \eta t (-61 \mu_1^2 + 9 (1 + \mu_2)^2 + \mu_1 (34 + 32 \mu_2)) \Big) \Big) + \\
& (-1 + \eta t) \operatorname{el} (-3 - 10 \mu_1 + 7 \mu_1^2 - 6 w^4 \mu_1^2 - 6 \mu_2 - 14 \mu_1 \mu_2 - \\
& 3 \mu_2^2 + 10 w^5 \mu_1 (9 \mu_1 + 4 \mu_2) + 2 \operatorname{ep} (3 \times (2 + \mathfrak{e}1 + \mathfrak{e}2) + \\
& 7 \mu_1^2 (2 + \mathfrak{e}1 + \mathfrak{e}2) + 6 \mu_2 (4 + \mathfrak{e}1 + \mathfrak{e}2) + \mu_2^2 (14 + 3 \mathfrak{e}1 + 3 \mathfrak{e}2) + \\
& 2 \mu_1 (6 \times (2 + \mathfrak{e}1 + \mathfrak{e}2) + 7 \mu_2 (4 + \mathfrak{e}1 + \mathfrak{e}2)) \Big) - \\
& w (-9 - 2 \mu_1 - 63 \mu_1^2 - 18 \mu_2 - 20 \mu_1 \mu_2 - 9 \mu_2^2 + \operatorname{ep} \\
& (-6 + 9 \mathfrak{e}1 + 9 \mathfrak{e}2 + 2 \mu_1 \mu_2 (-76 + \mathfrak{e}1 + \mathfrak{e}2) - 4 \mu_1 (2 + \mathfrak{e}1 + \mathfrak{e}2) + \mu_1^2 \\
& (2 + \mathfrak{e}1 + \mathfrak{e}2) + 2 \mu_2 (-4 + 9 \mathfrak{e}1 + 9 \mathfrak{e}2) + \mu_2^2 (2 + 9 \mathfrak{e}1 + 9 \mathfrak{e}2)) \Big) - \\
& w^2 (6 \times (2 \mu_1^2 - 3 (1 + \mu_2)^2 - 2 \mu_1 (3 + 4 \mu_2)) + \operatorname{ep} \\
& (66 \mu_1 (2 + \mathfrak{e}1 + \mathfrak{e}2) + 37 \mu_1^2 (2 + \mathfrak{e}1 + \mathfrak{e}2) + \\
& 3 \times (14 + 9 \mathfrak{e}1 + 9 \mathfrak{e}2) + 6 \mu_2 (22 + 9 \mathfrak{e}1 + 9 \mathfrak{e}2) + \\
& \mu_2^2 (74 + 27 \mathfrak{e}1 + 27 \mathfrak{e}2) + 2 \mu_1 \mu_2 (94 + 37 \mathfrak{e}1 + 37 \mathfrak{e}2)) \Big) -
\end{aligned}$$

$$\begin{aligned}
& 2 w^3 \left( 82 \mu_1^2 - 3 (1 + \mu_2)^2 + 2 \mu_1 (-7 + 6 \mu_2) + 2 \theta p \right. \\
& \quad \left. (5 \mu_1^2 (2 + \mathfrak{E}1 + \mathfrak{E}2) + (1 + \mu_2)^2 (10 + 3 \mathfrak{E}1 + 3 \mathfrak{E}2) + \right. \\
& \quad \left. 2 \mu_1 (5 \times (2 + \mathfrak{E}1 + \mathfrak{E}2) + \mu_2 (22 + 5 \mathfrak{E}1 + 5 \mathfrak{E}2)) \right) \Big) - \\
& \eta^5 \left( 6 w^5 \left( (-1 + \eta t) \theta l \mu_1 (5 \mu_1 - 2 \mu_2) + 2 \eta t \theta p \mu_1 (18 \mu_1 - \mu_2) + \right. \right. \\
& \quad \left. 6 \theta p (5 \mu_1 - 2 \mu_2) \mu_2 \right) + 6 w^4 \\
& \quad \left( (-1 + \eta t) \theta l \mu_1 (11 \mu_1 + 4 \mu_2) + \eta t \theta p \mu_1 (-37 \mu_1 + 10 \mu_2) + \right. \\
& \quad \left. \theta p \mu_2 (90 \mu_1 + 29 \mu_2) \right) - 2 \left( (-1 + \eta t) \theta l \mu_1 (-2 + 5 \mu_1) + \right. \\
& \quad \left. \theta p (7 + 5 \eta t \mu_1 (-2 + 5 \mu_1) - 10 \mu_2 - 50 \mu_1 \mu_2 - 5 \mu_2^2 + \right. \\
& \quad \left. 3 \times (-1 + \eta t) \theta l (2 \times (2 + \mu_2) + \mu_1 (2 + 10 \mu_2 + \mathfrak{E}1 + \mathfrak{E}2)) \right) \Big) - 3 \\
& w^2 \left( \theta p \left( 6 \times (2 + (4 + 38 \mu_1) \mu_2 + 7 \mu_2^2) - \eta t (123 \mu_1^2 + \right. \right. \\
& \quad \left. 9 (1 + \mu_2)^2 + 2 \mu_1 (-3 + 5 \mu_2)) \right) + (-1 + \eta t) \theta l \\
& \quad \left( -\mu_1^2 - 6 \mu_1 (1 + \mu_2) - 3 (1 + \mu_2)^2 + 2 \theta p (4 + 3 \mathfrak{E}1 + 3 \mathfrak{E}2 + \right. \\
& \quad \left. 7 \mu_1 (2 + \mathfrak{E}1 + \mathfrak{E}2) + 4 \mu_1^2 (2 + \mathfrak{E}1 + \mathfrak{E}2) + 2 \mu_2 (7 + 3 \mathfrak{E}1 + 3 \mathfrak{E}2) + \right. \\
& \quad \left. \mu_2^2 (8 + 3 \mathfrak{E}1 + 3 \mathfrak{E}2) + 2 \mu_1 \mu_2 (9 + 4 \mathfrak{E}1 + 4 \mathfrak{E}2)) \right) \Big) + 2 \\
& w \left( (-1 + \eta t) \theta l \mu_1 (25 \mu_1 - 4 \times (2 + \mu_2)) + \theta p (30 - 20 \eta t \mu_1 + \right. \\
& \quad \left. 40 \eta t \mu_1^2 - 20 \mu_2 + 204 \mu_1 \mu_2 - 16 \eta t \mu_1 \mu_2 - 8 \mu_2^2 + \right. \\
& \quad \left. (-1 + \eta t) \theta l (2 \times (6 + 12 \mu_2 + 5 \mu_2^2) + 5 \mu_1^2 (2 + \mathfrak{E}1 + \mathfrak{E}2) + \right. \\
& \quad \left. 2 \mu_1 (6 \times (2 + \mathfrak{E}1 + \mathfrak{E}2) + 5 \mu_2 (10 + \mathfrak{E}1 + \mathfrak{E}2)) \right) \Big) + \\
& w^3 \left( 4 \theta p (-1 - 4 \times (-5 + 43 \mu_1) \mu_2 + 9 \mu_2^2 + \eta t (-99 \mu_1^2 + \right. \\
& \quad \left. 6 (1 + \mu_2)^2 + \mu_1 (32 + 13 \mu_2)) \right) - \\
& \quad (-1 + \eta t) \theta l (123 \mu_1^2 - 3 (1 + \mu_2)^2 - 2 \mu_1 (11 + 4 \mu_2) + \\
& \quad 3 \theta p (5 \mu_1^2 (2 + \mathfrak{E}1 + \mathfrak{E}2) + (1 + \mu_2)^2 (10 + 3 \mathfrak{E}1 + 3 \mathfrak{E}2) + \\
& \quad 2 \mu_1 (5 \times (2 + \mathfrak{E}1 + \mathfrak{E}2) + \mu_2 (22 + 5 \mathfrak{E}1 + 5 \mathfrak{E}2)) \Big) \Big) + \\
& \eta \left( \theta p (4 w^3 (1 + \eta t \mu_1 (4 - 27 \mu_1 - 13 \mu_2) + 4 \mu_2 + 28 \mu_1 \mu_2 + 3 \mu_2^2) + \right. \\
& \quad 4 w^5 (\eta t \mu_1 (16 \mu_1 + 3 \mu_2) + \mu_2 (7 \mu_1 + 4 \mu_2)) + \\
& \quad 6 w^4 (\eta t \mu_1 (11 \mu_1 - 2 \mu_2) + \mu_2 (14 \mu_1 + 5 \mu_2)) + \\
& \quad \eta t (9 \mu_1^2 + 9 (1 + \mu_2)^2 + 2 \mu_1 (9 + 13 \mu_2)) + w^2 (2 \times (12 + 32 \mu_1 - \mu_2) \mu_2 + \\
& \quad \eta t (-149 \mu_1^2 + 9 (1 + \mu_2)^2 + 6 \mu_1 (7 + \mu_2)) \Big) + \\
& \quad w (8 \times (1 + \mu_1) \mu_2 + \eta t (-30 \mu_1^2 + 18 (1 + \mu_2)^2 + \mu_1 (44 + 60 \mu_2)) \Big) \Big) + \\
& (-1 + \eta t) \theta l (6 w^4 \mu_1 (7 \mu_1 + 4 \mu_2) + 2 w^5 \mu_1 (7 \mu_1 + 6 \mu_2) + \\
& \quad 3 (1 + \mu_1 + \mu_2)^2 (-1 + \theta p (2 + \mathfrak{E}1 + \mathfrak{E}2)) + w^2 (-9 - 18 \mu_1 + 5 \mu_1^2 - 18 \mu_2 - \\
& \quad 30 \mu_1 \mu_2 - 9 \mu_2^2 + \theta p (9 \times (2 + \mathfrak{E}1 + \mathfrak{E}2) + 24 \mu_1 (2 + \mathfrak{E}1 + \mathfrak{E}2) + 13 \mu_1^2 \\
& \quad (2 + \mathfrak{E}1 + \mathfrak{E}2) + 6 \mu_2 (8 + 3 \mathfrak{E}1 + 3 \mathfrak{E}2) + \mu_2^2 (26 + 9 \mathfrak{E}1 + 9 \mathfrak{E}2) + \\
& \quad \mu_1 \mu_2 (80 + 26 \mathfrak{E}1 + 26 \mathfrak{E}2)) \Big) + w^3 (-6 \mu_1 + 39 \mu_1^2 - 3 (1 + \mu_2)^2 + \\
& \quad \theta p (5 \mu_1^2 (2 + \mathfrak{E}1 + \mathfrak{E}2) + (1 + \mu_2)^2 (10 + 3 \mathfrak{E}1 + 3 \mathfrak{E}2) + \\
& \quad 2 \mu_1 (5 \times (2 + \mathfrak{E}1 + \mathfrak{E}2) + \mu_2 (22 + 5 \mathfrak{E}1 + 5 \mathfrak{E}2)) \Big) \Big) + \\
& w (-3 \times (3 \mu_1^2 + 3 (1 + \mu_2)^2 + \mu_1 (6 + 8 \mu_2)) + \theta p (11 \mu_1^2 (2 + \mathfrak{E}1 + \mathfrak{E}2) + \\
& \quad (1 + \mu_2) \times (9 \times (2 + \mathfrak{E}1 + \mathfrak{E}2) + \mu_2 (22 + 9 \mathfrak{E}1 + 9 \mathfrak{E}2)) + \\
& \quad \mu_1 (20 \times (2 + \mathfrak{E}1 + \mathfrak{E}2) + \mu_2 (48 + 22 \mathfrak{E}1 + 22 \mathfrak{E}2)) \Big) \Big) \Big) + \\
& \eta^4 (10 \theta p - 10 \theta l \theta p + 10 \eta t \theta l \theta p + 8 \theta l \mu_1 - 8 \eta t \theta l \mu_1 - 12 \eta t \theta p \\
& \quad \mu_1 - 30 \theta l \theta p \mu_1 + 30 \eta t \theta l \theta p \mu_1 - 20 \theta l \mu_1^2 + 20 \eta t \theta l \\
& \quad \mu_1^2 + 30 \eta t \theta p \mu_1^2 - 10 \theta l \theta p \mu_1^2 + 10 \eta t \theta l \theta p \mu_1^2 - 12 \theta p \\
& \quad \mu_2 - 30 \theta l \theta p \mu_2 + 30 \eta t \theta l \theta p \mu_2 + 4 \theta l \mu_1 \mu_2 - 4 \eta t \theta l \mu_1
\end{aligned}$$

$$\begin{aligned}
& \mu^2 + 108 \operatorname{ep} \mu_1 \mu_2 - 16 \eta t \operatorname{ep} \mu_1 \mu_2 - 130 \operatorname{el} \operatorname{ep} \mu_1 \mu_2 + 130 \\
& \eta t \operatorname{el} \operatorname{ep} \mu_1 \mu_2 - 6 \operatorname{ep} \mu_2^2 - 10 \operatorname{el} \operatorname{ep} \mu_2^2 + 10 \eta t \operatorname{el} \operatorname{ep} \\
& \mu_2^2 - 10 w^5 (11 \operatorname{ep} \mu_2 (\mu_1 + \mu_2) + \eta t \operatorname{ep} \mu_1 (-19 \mu_1 + 3 \mu_2) + \\
& (-1 + \eta t) \operatorname{el} \mu_1 (4 \mu_1 + 3 \mu_2)) + 6 w^4 ((-1 + \eta t) \operatorname{el} \mu_1 (24 \mu_1 + 5 \mu_2) + \\
& 5 \operatorname{ep} (\eta t \mu_1 (11 \mu_1 + 4 \mu_2) + \mu_2 (24 \mu_1 + 5 \mu_2))) - 15 \\
& \operatorname{el} \operatorname{ep} \mu_1 \mathfrak{x}_1 + 15 \eta t \operatorname{el} \operatorname{ep} \mu_1 \mathfrak{x}_1 - 5 \operatorname{el} \operatorname{ep} \mu_1^2 \mathfrak{x}_1 + 5 \eta t \operatorname{el} \\
& \operatorname{ep} \mu_1^2 \mathfrak{x}_1 - 10 \operatorname{el} \operatorname{ep} \mu_1 \mu_2 \mathfrak{x}_1 + 10 \eta t \operatorname{el} \operatorname{ep} \mu_1 \mu_2 \\
& \mathfrak{x}_1 - 15 \operatorname{el} \operatorname{ep} \mu_1 \mathfrak{x}_2 + 15 \eta t \operatorname{el} \operatorname{ep} \mu_1 \mathfrak{x}_2 - 5 \operatorname{el} \operatorname{ep} \mu_1^2 \\
& \mathfrak{x}_2 + 5 \eta t \operatorname{el} \operatorname{ep} \mu_1^2 \mathfrak{x}_2 - 10 \operatorname{el} \operatorname{ep} \mu_1 \mu_2 \mathfrak{x}_2 + 10 \eta t \operatorname{el} \\
& \operatorname{ep} \mu_1 \mu_2 \mathfrak{x}_2 + w^3 (\operatorname{ep} (24 + (80 + 578 \mu_1) \mu_2 + 198 \mu_2^2 + \\
& \eta t (-573 \mu_1^2 + 9 (1 + \mu_2)^2 + \mu_1 (98 + 46 \mu_2))) + \\
& 2 \times (-1 + \eta t) \operatorname{el} (21 \mu_1^2 + 3 \mu_1 (-2 + \mu_2) - 3 (1 + \mu_2)^2 + \\
& 5 \operatorname{ep} \mu_1^2 (2 + \mathfrak{x}_1 + \mathfrak{x}_2) + \operatorname{ep} (1 + \mu_2)^2 (10 + 3 \mathfrak{x}_1 + 3 \mathfrak{x}_2) + \\
& 2 \operatorname{ep} \mu_1 (5 \times (2 + \mathfrak{x}_1 + \mathfrak{x}_2) + \mu_2 (22 + 5 \mathfrak{x}_1 + 5 \mathfrak{x}_2))) + w \\
& (\operatorname{ep} (12 + 253 \eta t \mu_1^2 - 2 \times (40 + 207 \mu_1) \mu_2 - 74 \mu_2^2 + 27 \eta t (1 + \mu_2)^2 + \\
& \eta t \mu_1 (-26 + 38 \mu_2)) - (-1 + \eta t) \operatorname{el} (-9 + 18 \operatorname{ep} (\mathfrak{x}_1 + \mathfrak{x}_2) + \\
& \mu_1^2 (-1 + 28 \operatorname{ep} (2 + \mathfrak{x}_1 + \mathfrak{x}_2)) + 2 \mu_2 (-9 + 2 \operatorname{ep} (23 + 9 \mathfrak{x}_1 + 9 \mathfrak{x}_2)) + \\
& \mu_2^2 (-9 + 2 \operatorname{ep} (28 + 9 \mathfrak{x}_1 + 9 \mathfrak{x}_2)) + 2 \mu_1 \\
& (-9 - 13 \mu_2 + 23 \operatorname{ep} (2 + \mathfrak{x}_1 + \mathfrak{x}_2) + \operatorname{ep} \mu_2 (66 + 28 \mathfrak{x}_1 + 28 \mathfrak{x}_2))) - \\
& 3 w^2 (2 \times (-1 + \eta t) \operatorname{el} \mu_1 (-4 + 22 \mu_1 + \mu_2) + \operatorname{ep} (20 - 16 \mu_2 + \\
& 256 \mu_1 \mu_2 + 22 \mu_2^2 - \operatorname{el} (22 + 3 \mathfrak{x}_1 + 3 \mathfrak{x}_2 + 7 \mu_1^2 (2 + \mathfrak{x}_1 + \mathfrak{x}_2) + \\
& \mu_2^2 (14 + 3 \mathfrak{x}_1 + 3 \mathfrak{x}_2) + \mu_2 (32 + 6 \mathfrak{x}_1 + 6 \mathfrak{x}_2) + \\
& 2 \mu_1 (8 \times (2 + \mathfrak{x}_1 + \mathfrak{x}_2) + \mu_2 (48 + 7 \mathfrak{x}_1 + 7 \mathfrak{x}_2))) + \eta t (83 \mu_1^2 - \\
& 15 (1 + \mu_2)^2 - 2 \mu_1 (23 + 13 \mu_2) + \operatorname{el} (22 + 3 \mathfrak{x}_1 + 3 \mathfrak{x}_2 + 7 \mu_1^2 (2 + \\
& \mathfrak{x}_1 + \mathfrak{x}_2) + \mu_2^2 (14 + 3 \mathfrak{x}_1 + 3 \mathfrak{x}_2) + \mu_2 (32 + 6 \mathfrak{x}_1 + 6 \mathfrak{x}_2) + \\
& 2 \mu_1 (8 \times (2 + \mathfrak{x}_1 + \mathfrak{x}_2) + \mu_2 (48 + 7 \mathfrak{x}_1 + 7 \mathfrak{x}_2)))))) / \\
& (32 u (-1 + w (-1 + \eta))^3 (x + \eta - x \eta)^2 (1 + x + \eta - x \eta)^2 \\
& (w + \\
& x + \\
& \eta - \\
& w \eta - \\
& x \eta)^3 (-1 + \eta t) \operatorname{ep})) \\
\delta K = & -\frac{17 u}{2} - (f (-1 + \eta) \times \\
& (-3 x^2 (-1 + \eta)^2 (-1 + \eta + \operatorname{el} - \eta t \operatorname{el}) \operatorname{ep} + \operatorname{ep} (-3 \eta^3 + 2 \eta t + 3 \eta^2 (1 + (-1 + \eta t) \operatorname{el}) + \\
& \eta (-\operatorname{el} (2 + \mathfrak{x}_1 + \mathfrak{x}_2) + \eta t (-2 + \operatorname{el} (2 + \mathfrak{x}_1 + \mathfrak{x}_2))) + w (-1 + \eta) \times \\
& (3 \eta^2 - 2 \eta t + \eta (-3 + 2 \eta t + \operatorname{el} (5 + \mathfrak{x}_1 + \mathfrak{x}_2) - \eta t \operatorname{el} (5 + \mathfrak{x}_1 + \mathfrak{x}_2)))) + \\
& x (-1 + \eta) \times (-3 (w (-1 + \eta) - 2 \eta) (-1 + \eta) \operatorname{ep} + (-1 + \eta t) \operatorname{el} \\
& (2 - \operatorname{ep} (2 + 6 \eta + \mathfrak{x}_1 + \mathfrak{x}_2) + w (-1 + \eta) \times (-2 + \operatorname{ep} (5 + \mathfrak{x}_1 + \mathfrak{x}_2)))))) / \\
& (2 \times (-1 + w (-1 + \eta)) (x (-1 + \eta) - \eta) (w (-1 + \eta) + x (-1 + \eta) - \eta) (-1 + \eta t) \operatorname{ep})
\end{aligned}$$
